# Supplementary material for: A mathematical model for universal semantics
Source: arXiv:1907.12293 ancillary file (2020-07-12)
Supplement: Supplementary file 1 [file SoftwareManualPartA.pdf]

# *Software Manual*

## A mathematical model for universal semantics

Weinan E<sup>1,2\*</sup>, Yajun Zhou<sup>2\*</sup>

<sup>1</sup>Department of Mathematics & Program in Applied and Computational Mathematics,  
Princeton University, Princeton, NJ 08544, USA

<sup>2</sup>Beijing Institute of Big Data Research, Beijing 100871, P. R. China

\*Corresponding authors. E-mail: weinan@math.princeton.edu (W.E), yajun.zhou.1982@pku.edu.cn (Y.Z.)

March 2020

## Contents

|            |                                                                     |           |
|------------|---------------------------------------------------------------------|-----------|
| <b>I</b>   | <b>Scope and Limitations</b>                                        | <b>1</b>  |
| 1          | What our software does                                              |           |
| 1.1        | Markov analysis of word patterns and topic extraction . . . . .     | 1         |
| 1.2        | Semantic fingerprints from invariant Markov spectra . . . . .       | 2         |
| 1.3        | Automated word translation based on semantic fingerprints . . . . . | 5         |
| 1.4        | Automated question answering based on Markov semantics . . . . .    | 11        |
| 2          | What our software does not                                          |           |
| 2.1        | Non-universal statistics on short time scales . . . . .             | 11        |
| 2.2        | Word disambiguation and stylistic adaptability . . . . .            | 12        |
| 2.3        | Causal inference and deductive reasoning . . . . .                  | 14        |
| <b>II</b>  | <b>Protocols for text cleansing</b>                                 | <b>15</b> |
| 3          | String manipulations and text normalizations                        |           |
| 3.1        | Notational conventions . . . . .                                    | 16        |
| 3.2        | Normalizations of Wikipedia pages and WikiQA dataset . . . . .      | 18        |
| 3.3        | Normalizations of ebooks for text mining . . . . .                  | 22        |
| <b>III</b> | <b>Protocols for word clustering</b>                                | <b>24</b> |
| 4          | Approximate word clustering in English                              |           |
| 4.1        | Capitalization and stop words . . . . .                             | 24        |
| 4.2        | Modified Porter stemming algorithm for English . . . . .            | 25        |
| 4.2.1      | Effective spelling and essential root . . . . .                     | 26        |
| 4.2.2      | Admissible mutation and approximate clustering . . . . .            | 30        |
| 5          | Approximate word clustering in selected Germanic languages          |           |
| 5.1        | Modified Porter stemming algorithm for Danish . . . . .             | 60        |
| 5.1.1      | Effective spelling and essential root . . . . .                     | 61        |
| 5.1.2      | Admissible mutation and approximate clustering . . . . .            | 62        |
| 5.1.3      | Heuristic detection of compounds . . . . .                          | 66        |

|       |                                                                          |     |
|-------|--------------------------------------------------------------------------|-----|
| 5.2   | Modified Porter stemming algorithm for German . . . . .                  | 70  |
| 5.2.1 | Effective spelling and essential root . . . . .                          | 71  |
| 5.2.2 | Admissible mutation and approximate clustering . . . . .                 | 73  |
| 5.2.3 | Heuristic detection of compounds . . . . .                               | 77  |
| 5.3   | Modified Porter stemming algorithm for Dutch . . . . .                   | 81  |
| 5.3.1 | Effective spelling and essential root . . . . .                          | 81  |
| 5.3.2 | Admissible mutation and approximate clustering . . . . .                 | 83  |
| 5.3.3 | Heuristic detection of compounds . . . . .                               | 86  |
| 6     | Approximate word clustering in selected Romance languages . . . . .      |     |
| 6.1   | Modified Porter stemming algorithm for Spanish . . . . .                 | 89  |
| 6.1.1 | Effective spelling and essential root . . . . .                          | 90  |
| 6.1.2 | Admissible mutation and approximate clustering . . . . .                 | 92  |
| 6.2   | Modified Porter stemming algorithm for French . . . . .                  | 103 |
| 6.2.1 | Effective spelling and essential root . . . . .                          | 104 |
| 6.2.2 | Admissible mutation and approximate clustering . . . . .                 | 106 |
| 6.3   | Modified Porter stemming algorithm for Latin . . . . .                   | 120 |
| 6.3.1 | Effective spelling and essential root . . . . .                          | 122 |
| 6.3.2 | Admissible mutation and approximate clustering . . . . .                 | 125 |
| 7     | Approximate word clustering in selected Slavic languages . . . . .       |     |
| 7.1   | Modified Porter stemming algorithm for Polish . . . . .                  | 148 |
| 7.1.1 | Effective spelling and essential root . . . . .                          | 149 |
| 7.1.2 | Admissible mutation and approximate clustering . . . . .                 | 152 |
| 7.2   | Modified Porter stemming algorithm for Russian . . . . .                 | 164 |
| 7.2.1 | Effective spelling and essential root . . . . .                          | 166 |
| 7.2.2 | Admissible mutation and approximate clustering . . . . .                 | 169 |
| 8     | Approximate word clustering in selected Uralic languages . . . . .       |     |
| 8.1   | Modified Porter stemming algorithm for Finnish . . . . .                 | 187 |
| 8.1.1 | Effective spelling and essential root . . . . .                          | 190 |
| 8.1.2 | Admissible mutation and approximate clustering . . . . .                 | 194 |
| 8.1.3 | Heuristic detection of compounds . . . . .                               | 210 |
| 8.2   | Modified Porter stemming algorithm for Hungarian . . . . .               | 216 |
| 8.2.1 | Effective spelling and essential root . . . . .                          | 218 |
| 8.2.2 | Admissible mutation and approximate clustering . . . . .                 | 221 |
| 8.2.3 | Heuristic detection of compounds . . . . .                               | 227 |
| 9     | Approximate word clustering in various agglutinative languages . . . . . |     |
| 9.1   | Modified Porter stemming algorithm for Basque . . . . .                  | 231 |
| 9.1.1 | Effective spelling and essential root . . . . .                          | 234 |
| 9.1.2 | Approximate clustering . . . . .                                         | 235 |
| 9.2   | Modified Porter stemming algorithm for Korean . . . . .                  | 241 |
| 9.2.1 | Stop words and transliterations . . . . .                                | 242 |
| 9.2.2 | Effective spelling and essential root . . . . .                          | 245 |
| 9.2.3 | Approximate clustering . . . . .                                         | 250 |
| 9.3   | Modified Porter stemming algorithm for Turkish . . . . .                 | 255 |
| 9.3.1 | Effective spelling and essential root . . . . .                          | 256 |
| 9.3.2 | Approximate clustering . . . . .                                         | 257 |

This Software Manual accompanies our article entitled “A mathematical model for universal semantics” [1], supplying linguistic and algorithmic details. Mathematical proofs behind our model are elaborated in [1, Appendices A and B], so they will not be repeated here.

In Part I, we describe the scope and limitations of our current computational methods for automated word translation and text comprehension. Numerical tests on corpora are also briefly summarized in tables and figures.

In Part II, we define some terminologies and notations in linguistics, in the context of our current software implementation. We also list all the procedures required to cleanse our text corpora.

In Part III, we present detailed algorithms for treating 14 languages out of 5 representative language families, including 12 European languages (Danish, German, Dutch, Spanish, French, Latin, Polish and Russian from the Indo–European language family; Finnish and Hungarian from the Uralic language family; Basque from the Vasconic language family) and 2 Asian languages (Korean from the Koreanic language family; Turkish from the Turkic language family). We illustrate these algorithms with automated word translations from English masterpieces to other languages, and with question answering on the WikiQA dataset.

## Part I

# Scope and Limitations

## 1 What our software does

### 1.1 Markov analysis of word patterns and topic extraction

As in [1, §1], we are interested in word patterns, each of which is a collection of morphologically related content words. We refer our readers to Part III for the working definition of content words (which varies from language to language), and how we recognize and group content words that have related morphologies.

In our numerical studies of text documents, we count waiting times between two word patterns  $W_i$  and  $W_j$  by the *effective fragment length*  $L_{ij}$  (defined in [1, Fig. 1]). As we have mentioned in the caption to [1, Fig. 1], a text fragment qualifies as an *long-range transition* from  $W_i$  and  $W_j$ , if

- it is flanked by a word in  $W_i$  to the left and a word in  $W_j$  to the right;
- it does not mention any word in the set  $W_i$ ;
- it is longer than the longest word in the set  $W_i \cup W_j$ .

We always ignore close encounters of words (that is, those failing the last of the three criteria above), while collecting data for effective fragment lengths over long-range transitions.

With  $n_{ij}$  samples of effective fragment lengths  $L_{ij}$  in long-range transitions from  $W_i$  to  $W_j$ ,<sup>1</sup> we model a text by a Markov matrix  $\mathbf{P} = (p_{ij})_{1 \leq i, j \leq N}$ , whose entries are given by [1, (5)]

$$p_{ij} := \frac{n_{ij} e^{-\langle \log L_{ij} \rangle}}{\sum_{k=1}^N n_{ik} e^{-\langle \log L_{ik} \rangle}}. \quad (1.1)$$

Numerical evidence suggests that this empirical Markov matrix  $\mathbf{P} = (p_{ij})_{1 \leq i, j \leq N}$  is a fair approximation to an *ergodic* matrix  $\mathbf{P}^* = (p_{ij}^*)_{1 \leq i, j \leq N}$ , whose equilibrium state  $\boldsymbol{\pi}^* = (\pi_1^*, \dots, \pi_N^*)$  matches word count statistics [1, Fig. 4a], and honors the *detailed balance* condition  $\pi_i^* p_{ij}^* = \pi_j^* p_{ji}^*$  [1, Fig. 4b].

For an ergodic Markov chain satisfying the detailed balance condition, one can show that the probability distribution of recurrence times  $\tau = L_{ii}$  goes like [1, Appendix B.3]

$$\mathbb{P}(\tau > t) \sim \sum_m c_m e^{-k_m t}, \quad \left( \text{where } c_m, k_m > 0, \text{ and } \sum_m c_m = 1 \right), \quad (1.2)$$

a functional form that frequently crops up in dynamic studies of biological macromolecules [7]. This weighted mixture of multiple exponential decay laws imposes an inequality constraint on the recurrence time  $\tau$  [1, (3)]:

$$\langle \log \tau \rangle - \log \langle \tau \rangle + \gamma_0 = \sum_m c_m \log \frac{1}{k_m} - \log \sum_m \frac{c_m}{k_m} \leq 0, \quad (1.3)$$

<sup>1</sup>It is worth noting that we construct an empirical Markov matrix by an *in situ* analysis of a text, without digesting a document (or small parts of it) as a scrambled bag of words, a procedure implemented in conventional algorithms [2, 3, 4, 5, 6]. The notation  $p_{ij}$  in the semantic model of Turney–Pantel [4] is unrelated to ours.

where  $\gamma_0 := \lim_{n \rightarrow \infty} (-\log n + \sum_{m=1}^n \frac{1}{m})$  is the Euler–Mascheroni constant. This inequality explains the systematic data trend in [1, Fig. 2e], where most data points reside on one side of the line of Poissonian banality  $(\log \tau) - \log \langle \tau \rangle + \gamma_0 = 0$  (blue line in [1, Fig. 2e]).

In [1, Appendix A], we have shown that the statistic

$$\delta_i := \log \langle L_{ii} \rangle - \langle \log L_{ii} \rangle - \gamma_0 + \frac{1}{2n_{ii}} \quad (1.4)$$

satisfies

$$|\delta_i| < \frac{2}{\sqrt{n_{ii}}} \sqrt{\frac{\pi^2}{6} - 1 - \frac{1}{2n_{ii}}} \quad (1.5)$$

with probability 95%, when there are  $n_{ii}$  independent samples of exponentially distributed (hence banal)  $L_{ii}$ . In our current work, we automatically extract topics (Figs. S3–S16 in Part III), by identifying all the word patterns that violate the inequality above. Being consistent with the weighted exponential mixture model in (1.2), almost all of our automatically identified topics in Figs. S3–S16 satisfy

$$\delta_i \geq \frac{2}{\sqrt{n_{ii}}} \sqrt{\frac{\pi^2}{6} - 1 - \frac{1}{2n_{ii}}} > 0. \quad (1.6)$$

If a concept (representable by a word pattern) qualifies as a topical (resp. non-topical) pattern in a certain document, according to the algorithm above, then this concept usually remains topical (resp. non-topical) if we examine the long-range statistic  $\delta_i$  in a parallel document written in a different language [1, Fig. 3b,b’]. In other words, topicality/non-topicality is an invariant (*i.e.* a language-independent property) under translations.

Generalizing this further, we hypothesize that temporal structures are nearly universal across different languages, on all the scales longer than next-to-nearest neighboring words. In fact, later in §1.2, we will demonstrate that the statistics of effective fragment lengths  $L_{ij}$  almost represent a complete set of semantic invariants, quantifying the semantic similarity between  $W_i$  and  $W_j$  in a language-independent way.

## 1.2 Semantic fingerprints from invariant Markov spectra

What gives meanings to things? If we threw this ontological question to paleolithic cavemen or preschool children, we would probably expect tangible answers that define objects by physical and physiological stimuli. Putatively speaking, cavemen would conceptualize “fire” by associating it to “brightness” (visual impression), “warmth” (feeling at a distance) and “pain” (reaction upon touch); children would recognize an “apple” as something that is “round” (in shape), “red” (in color) and “sweet” (in taste). While this reductionist view of semantics does not generalize well to abstract concepts (“love”, “pride”, ...), fictional characters (“Elizabeth Bennet”, “Harry Potter”, ...) or non-existent places (“Meryton”, “Hogwarts”, ...), we still find it an attractive idea to generate semantic tags by association—perhaps a universal way to clarify the meaning of a word is to link it to a small set of other words (even if they do not represent bodily stimuli).<sup>2</sup>

Such an ontological picture motivates us to define the meaning of words in terms of a language-independent numerical fingerprint, using Markov matrices that characterize association and connectivity. As we will soon see, certain invariance properties of Markov matrices account for the translatability of concepts across a wide variety of languages. Put differently, in our Markov language model, the semantic context of an individual word pattern is (up to numerical errors) independent of the language in which it is expressed—the mental states underlying a text thus remain (approximately) invariant under translation.

Through numerical experiments ([1, Fig. 2e] and Fig. S1a,a’,a’’), we find that the spectrum of a Markov matrix (collection of eigenvalues, counting multiplicity) is language-independent.

In [1, §2.2.3], we have designed a thought experiment (estimation of brainstorming rates from words in language A to words in language B) involving two monolingual human subjects, which has led us to an equation [1, (6)]

$$\mathbf{P}_A \mathbf{T}_{A \rightarrow B} = \mathbf{T}_{A \rightarrow B} \mathbf{P}_B. \quad (1.7)$$

Here,  $\mathbf{P}_A$  and  $\mathbf{P}_B$  are, respectively, the Markov matrices characterizing the mental language of Alice (knowing only language A) and Bob (knowing only language B), while  $\mathbf{T}_{A \rightarrow B}$  is the common dictionary matrix shared by both people. If we have an invertible Markov matrix  $\mathbf{T}_{A \rightarrow B}$  (when translations are lossless), then  $\mathbf{P}_A$  and  $\mathbf{P}_B$  share the same characteristic polynomial  $\det(\lambda \mathbf{I} - \mathbf{P}_A) = \det(\lambda \mathbf{I} - \mathbf{P}_B)$ , hence the same spectrum. We note that the dictionary matrix  $\mathbf{T}_{A \rightarrow B}$  here does not need to be

<sup>2</sup>It is worth mentioning that Jane Austen has written several novels, besides *Pride and Prejudice*, with themes of love and marriage, despite her very lack of personal experience in these matters—she was able to create vivid characters out of her pure imagination, while tagging them with appropriate contexts.

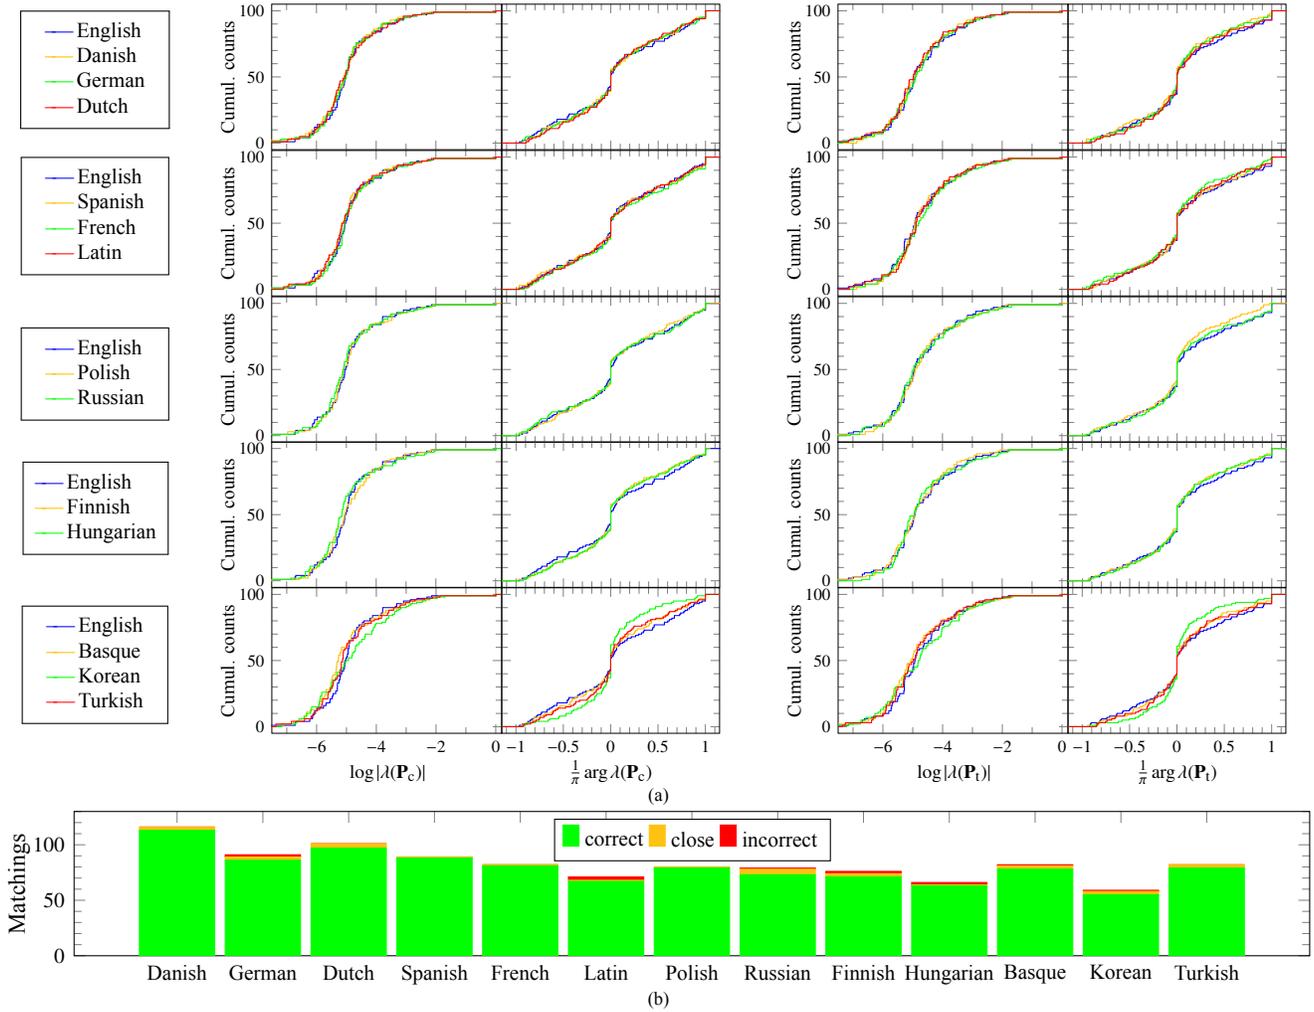

Fig. S1. Language-independence of Markov spectra. (a) Approximate spectral invariance in the Markov matrices  $\mathbf{P}_c$  (resp.  $\mathbf{P}_t$ ) for top 100 content (resp. topic) word clusters from the English original and 13 different translations of *Pride and Prejudice*. (See §9.2 for difficulties in analyzing Korean texts.) (b) Evaluations of automated semantic alignments ([1, Fig. 6] and Figs. S4–S7, S9–S16) between topics in the English version of *Pride and Prejudice* and those in the 13 different translations.

a permutation matrix<sup>3</sup> to qualify for spectral invariance. An invertible  $\mathbf{T}_{A \rightarrow B}$  may assume non-permutation forms (which partially accommodates to polysemy of words in realistic languages), such as  $\begin{pmatrix} \frac{1}{2} & \frac{1}{2} \\ 0 & 1 \end{pmatrix}$ . Furthermore, the inverse matrix  $\mathbf{T}_{A \rightarrow B}^{-1}$  does not necessarily coincide with the dictionary matrix  $\mathbf{T}_{B \rightarrow A}$ . This is because  $\mathbf{P}_A(\mathbf{A}\mathbf{T}_{A \rightarrow B}) = (\mathbf{A}\mathbf{T}_{A \rightarrow B})\mathbf{P}_B$  and  $\mathbf{P}_A(\mathbf{T}_{A \rightarrow B}\mathbf{B}) = (\mathbf{T}_{A \rightarrow B}\mathbf{B})\mathbf{P}_B$  hold for any matrices  $\mathbf{A}$  and  $\mathbf{B}$  satisfying  $\mathbf{A}\mathbf{P}_A = \mathbf{P}_A\mathbf{A}$  and  $\mathbf{B}\mathbf{P}_B = \mathbf{P}_B\mathbf{B}$ .

In [1, Fig. 4c], we have demonstrated approximate spectral invariance, by localizing Markov matrices on the top 100 content word patterns, in the English, French, Russian and Finnish versions of *Pride and Prejudice*. Such invariance properties remain unscathed when we consider translations of the same novel into other languages, and when we localize on the top 100 topical patterns instead (Fig. S1a). The numerical agreement is understandable from the language-independence of semantic content. In fact, we have pushed this spectral invariance down to an even more local scale in [1, Fig. 5b]: after translations, there are only small perturbations in the dominant eigenvalues for Markov matrices localized on *semantic cliques* surrounding specific concepts.

Here, to define a semantic clique  $\mathcal{S}_i$  surrounding a specific word pattern  $W_i$ , we need to specify numerical semantic fields through an affinity score  $\alpha_{ij}(\ell)$ . If we have a Markov process on a semantic web that honors detailed balance, then for each fixed word pattern  $W_i$ , we can determine [8] the distribution of hitting times  $L_{ij}$ ,  $1 \leq j \leq N$  from that of the return times  $L_{ii}$ . Further assuming that the distribution of  $\langle \log L_{ij} \rangle$  is nearly Gaussian, we can use the following approximation [1, (7)]:

$$\mathbb{P}(\langle \log L_{ij} \rangle > \ell) \approx \alpha_{ij}(\ell) := \sqrt{\frac{n_{ij}}{2\pi\beta_i}} \int_{\ell}^{\infty} e^{-\frac{n_{ij}(x-\ell_i)^2}{2\beta_i}} dx, \quad (1.8)$$

<sup>3</sup>A permutation matrix is a Markov matrix whose entries are either 0 or 1. When the dictionary matrix  $\mathbf{T}_{A \rightarrow B}$  is a permutation matrix, translation becomes a bijection of words between two languages. This picture, of course, is much too restrictive.

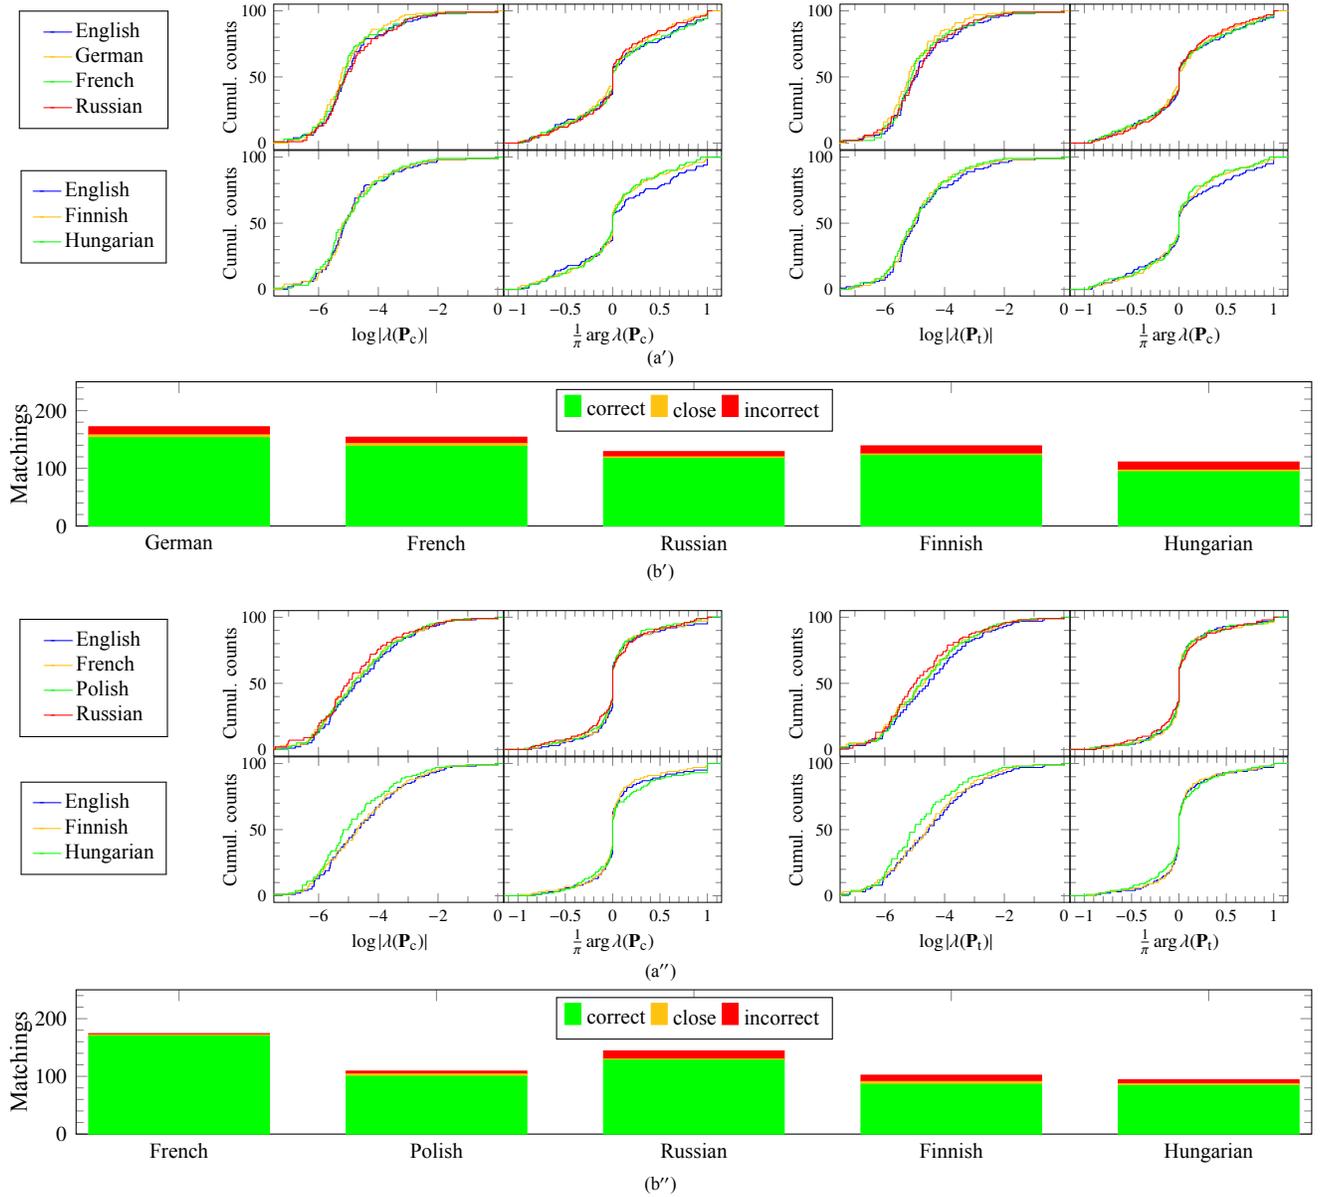

Fig. S1. Language-independence of Markov spectra. (*Continued*) Similar service on multiple versions of (a')–(b') *Jane Eyre* and (a'')–(b'') *Origin of Species*.

where [1, (8) and Theorem 4 in Appendix B.4]

$$\ell_i := \frac{\langle L_{ii} \log L_{ii} \rangle}{\langle L_{ii} \rangle} - 1, \quad \beta_i := \frac{\langle L_{ii} (\ell_i - \log L_{ii})^2 \rangle}{\langle L_{ii} \rangle}. \quad (1.9)$$

Our semantic clique  $\mathcal{S}_i$  [1, Fig. 5a,b] admits  $W_j$  as its member if and only if

$$\min\{\alpha_{ij}(\langle \log L_{ij} \rangle), \alpha_{ji}(\langle \log L_{ji} \rangle)\} > \frac{1}{\sqrt{2\pi}} \int_{-\infty}^1 e^{-\frac{x^2}{2}} dx. \quad (1.10)$$

Here, we give some caveats on the spectral invariance for localized Markov models of semantic cliques, and further clarify the meaning of “dominant eigenvalues”. The criterion (1.10) for membership in semantic cliques and the 95% confidence interval for topicality [see (1.5)] both involve arbitrary cut-offs. Whenever there are close calls, our algorithm may include certain topics in a particular semantic clique  $\mathcal{S}_i^A$  in language A, but exclude them from a parallel clique  $\mathcal{S}_i^B$  in language B. Thus, the size of semantic cliques might not be stable across languages (see dashed lines in [1, Fig. 5b]), due to the presence of marginal topics. To combat this instability, we have proposed to use the entropy production rate<sup>4</sup> to compress dimensions (see

<sup>4</sup>Heuristically speaking, the entropy production rate  $\eta(\mathbf{P}) = -\sum_{i,j} \pi_i p_{ij} \log p_{ij}$  [9, (4.27)] of a Markov matrix  $\mathbf{P}$  represents the weighted average (assigning

solid lines in [1, Fig. 5b]). For an  $N \times N$  Markov matrix  $\mathbf{P}$  with strictly positive entries, the entropy production rate  $\eta(\mathbf{P})$  satisfies a sharp inequality<sup>5</sup>  $\eta(\mathbf{P}) \leq \log N$  [10, Theorem 14.1], so  $\lfloor e^{\eta(\mathbf{P})} \rfloor$  represents the effective dimension of our localized Markov matrix  $\mathbf{P}$  for a semantic clique. This effective dimension is less susceptible to marginal topics than the number of members in a numerically constructed semantic clique (= the size of matrix  $\mathbf{P}$ ), hence we use it to decide how many dominant eigenvalues to keep before vectorizing a topic from the recurrence eigenvalues [1, Fig. 5b] in its surrounding semantic clique. The vector that arranges these recurrence eigenvalues (corresponding to decay modes in (1.2)) in descending order is a *language-independent semantic fingerprint* for a topic.

### 1.3 Automated word translation based on semantic fingerprints

Our machine translation experiments solve bipartite matching problems involving the Ružička similarities [11, 12]

$$s_R(\mathbf{a}, \mathbf{b}) := \frac{\|\mathbf{a} \wedge \mathbf{b}\|_1}{\|\mathbf{a} \vee \mathbf{b}\|_1} \equiv \frac{\sum_i \min(a_i, b_i)}{\sum_i \max(a_i, b_i)} \quad (1.11)$$

between vectorized topics.<sup>6</sup> The Ružička dissimilarity function  $d_R(\mathbf{a}, \mathbf{b}) = 1 - s_R(\mathbf{a}, \mathbf{b})$  measures the distance between two non-zero vectors with non-negative components, and satisfies the three axioms for a distance metric:

1. (Discernibility)  $d_R(\mathbf{a}, \mathbf{b}) = 0 \iff \mathbf{a} = \mathbf{b}$ ;
2. (Symmetry)  $d_R(\mathbf{a}, \mathbf{b}) = d_R(\mathbf{b}, \mathbf{a})$ ;
3. (Subadditivity)  $d_R(\mathbf{a}, \mathbf{c}) \leq d_R(\mathbf{a}, \mathbf{b}) + d_R(\mathbf{b}, \mathbf{c})$ .

To verify subadditivity, one can use Gilbert’s bounds [13]

$$1 - \frac{\|\mathbf{v}_1 \wedge \mathbf{v}_2 \wedge \mathbf{v}_3\|_1}{\|\mathbf{v}_1 \vee \mathbf{v}_2 \vee \mathbf{v}_3\|_1} \geq d_R(\mathbf{v}_i, \mathbf{v}_j) = 1 - \frac{\|\mathbf{v}_i \wedge \mathbf{v}_j\|_1}{\|\mathbf{v}_i \vee \mathbf{v}_j\|_1} \geq \frac{\|\mathbf{v}_i \vee \mathbf{v}_j\|_1 - \|\mathbf{v}_i \wedge \mathbf{v}_j\|_1}{\|\mathbf{v}_1 \vee \mathbf{v}_2 \vee \mathbf{v}_3\|_1} \quad (1.12)$$

for  $i, j \in \{1, 2, 3\}$ , together with the fact that  $\|\mathbf{a} \vee \mathbf{b} \vee \mathbf{c}\|_1 - \|\mathbf{a} \wedge \mathbf{b} \wedge \mathbf{c}\|_1 \leq (\|\mathbf{a} \vee \mathbf{b}\|_1 - \|\mathbf{a} \wedge \mathbf{b}\|_1) + (\|\mathbf{b} \vee \mathbf{c}\|_1 - \|\mathbf{b} \wedge \mathbf{c}\|_1)$ . Since the Ružička dissimilarity satisfies the axioms for a distance metric, our bipartite matching model for machine translation is a discrete version of the optimal transport in variational calculus.

During the ballpark screening stage of our machine translation algorithm, we divide our target document into  $K$  chapters and vectorize each topic pattern  $W_i$  by its chapter-wise counts  $\mathbf{b}_i \in \mathbb{R}^K$ . To pass a ballpark screening test, a pair of topics  $W_i^A$  and  $W_j^B$  from parallel versions (in languages A and B) of the same document have to satisfy

$$d_R(\mathbf{b}_i^A, \mathbf{b}_j^B) \leq \varepsilon \sqrt{K} \quad \text{and} \quad d_R(\mathbf{b}_i^A, \mathbf{b}_j^B) \leq \sqrt{\frac{\|\mathbf{b}_i^A \wedge \mathbf{b}_j^B\|_0}{\|\mathbf{b}_i^A \vee \mathbf{b}_j^B\|_1}}. \quad (1.13)$$

Here, the coefficient  $\varepsilon = 0.07$  in the first inequality above is chosen empirically (see control experiments in Figs. S5, S8, S10, S11, S12, S13), so that the right-hand side extrapolates to a reasonable error margin<sup>7</sup> for total word counts (when  $K = 1$ ). The second inequality in (1.13) draws upon a Poisson approximation to word count fluctuations, with  $\|\mathbf{b}_i^A \wedge \mathbf{b}_j^B\|_0$  being the number of corresponding chapters that contain both  $W_i^A$  and  $W_j^B$ . Through numerical experiments, we find that the screening criteria in (1.13) lead to acceptable recall and precision of machine translation later afterwards.

The vector  $\mathbf{b}_i \in \mathbb{R}^K$  captures only the temporal behavior of  $W_i$  on the chapter scale. To paint a fuller kinetic picture of  $W_i$  above the discourse level, we vectorize it by  $\mathbf{v}_i$ , the list of dominant recurrence eigenvalues in its semantic clique, and use  $s_R(\mathbf{v}_i^A, \mathbf{v}_j^B)$  in our final similarity score for bipartite matching (see Fig. S1b, b', b'', Tables S2–S5 for summaries of performance; see [1, Fig. 6] and Figs. S4–S16 for detailed bipartite matching of semantic fingerprints  $\mathbf{v}_i$ ). In the current work, we do impose an additional censorship  $s_R(\mathbf{v}_i^A, \mathbf{v}_j^B) \geq 0.7$  before throwing similarity scores to the Hungarian algorithm for bipartite matching. This threshold value 0.7 is somewhat arbitrary. Relaxing this arbitrary censorship (*i.e.* reducing the threshold to 0) seems to have minimal consequences for translations between English and its close relative (see a control experiment for English–French in Table S6 and Fig. S8c), but seems to boost the recall rate significantly for translations between English and a non-Indo-European language (see a control experiment for English–Korean in Table S6 and Fig. S15c). Perhaps more work is needed to understand whether/how the threshold here adapts to the specific language pairs.

probability mass  $\pi_i$  to the  $i$ th Markov state) of Boltzmann’s partition entropies  $-\sum_j p_{ij} \log p_{ij}$  [10, §8.2]. For a formal discussion of entropy production and information compressibility in Markov chains, see [9, Chaps. 4–5] and [10, Chaps. 3, 8 and 14].

<sup>5</sup>The equality is attained when  $\mathbf{P} = (p_{ij} = \frac{1}{N})_{1 \leq i, j \leq N}$ . This is the case of the least compressible Markov chain, whose maximal effective dimension is equal to  $N$ .

<sup>6</sup>Here as in [1, (4)],  $\mathbf{a} \wedge \mathbf{b} = (\min\{a_1, b_1\}, \dots, \min\{a_N, b_N\})$  and  $\mathbf{a} \vee \mathbf{b} = (\max\{a_1, b_1\}, \dots, \max\{a_N, b_N\})$  for  $\mathbf{a} = (a_1, \dots, a_N)$ ,  $\mathbf{b} = (b_1, \dots, b_N)$ ;  $\|\mathbf{u}\|_1 = \sum_{i=1}^N |u_i|$  for  $\mathbf{u} = (u_1, \dots, u_N)$ .

<sup>7</sup>Possible error sources are imperfections in translation and word clustering. See discussions below.

In Figs. S3–S16, we run our experiments on multilingual corpora (Table S1) involving 9 members (Danish, Dutch, English, French, German, Latin, Polish, Russian and Spanish) in the Indo-European language family, 2 members (Finnish and Hungarian) in the Uralic language family, and 3 more agglutinative languages (Basque, Korean, Turkish) that are neither Indo-European nor Uralic, which exhibit diverse word orders<sup>8</sup> for subject (S), verb (V) and object (O):

- SVO: Danish, English, French, Spanish,<sup>9</sup>  
 SV<sub>1</sub>O(V<sub>2</sub>): Dutch, German,<sup>10</sup>  
 SOV: Basque, Latin, Korean, Turkish,<sup>11</sup>  
 Free word order: Finnish, Hungarian, Polish, Russian.<sup>12</sup>

The partial success of these experiments demonstrates that our Markov model (of topics on the long-range length scale) is translatable, regardless of a language’s genealogical affiliation and syntactical structure.

Table S1. Provenances of multilingual texts used in our experiments and discussions

| Language             | Author/Adaptor                                                    | Title                                                  | Publisher                                                                                                                        | Electronic availability                                                                                                                                                                                                                                                                                                             |
|----------------------|-------------------------------------------------------------------|--------------------------------------------------------|----------------------------------------------------------------------------------------------------------------------------------|-------------------------------------------------------------------------------------------------------------------------------------------------------------------------------------------------------------------------------------------------------------------------------------------------------------------------------------|
| <i>Indo-European</i> |                                                                   |                                                        |                                                                                                                                  |                                                                                                                                                                                                                                                                                                                                     |
| English              | Jane Austen                                                       | <i>Pride and Prejudice</i>                             | T. Egerton (Whitehall, UK, 1813)                                                                                                 | ExampleData in <i>Mathematica</i> (essentially identical to the 1813 version, with modernized spellings)                                                                                                                                                                                                                            |
|                      | Deborah Moggach                                                   | <i>Pride and Prejudice</i>                             | Internet Movie Scripts Database (2005)                                                                                           | * <a href="https://www.imdb.com/scripts/Pride-and-Prejudice.html">https://www.imdb.com/scripts/Pride-and-Prejudice.html</a>                                                                                                                                                                                                         |
| Danish               | Vibeke Houstrup                                                   | <i>Stolthed og fordom</i>                              | Lindhardt og Ringhof Forlag (Copenhagen, Denmark, 2015)                                                                          | <a href="https://play.google.com/store/books/details?id=dd0-CgAAQBAJ&amp;rdid=book-dd0-CgAAQBAJ">https://play.google.com/store/books/details?id=dd0-CgAAQBAJ&amp;rdid=book-dd0-CgAAQBAJ</a> (Google Play)                                                                                                                           |
| German               | Werner Beyer                                                      | <i>Stolz und Vorurteil</i>                             | Fischer Klassik Plus (Frankfurt am Main, Germany, 2011)                                                                          | <a href="https://www.amazon.de/Stolz-Vorurteil-Roman-Fischer-Klassik-ebook/dp/B006QH3IIC/">https://www.amazon.de/Stolz-Vorurteil-Roman-Fischer-Klassik-ebook/dp/B006QH3IIC/</a> (Amazon)                                                                                                                                            |
|                      | Christian Grawe & Ursula Grawe                                    | <i>Stolz und Vorurteil</i>                             | Philipp Reclam jun. GmbH & Co. KG (Stuttgart, Germany, 2015)                                                                     | <a href="https://www.amazon.de/Stolz-Vorurteil-Roman-Reclam-Taschenbuch-ebook/dp/B01BHWFX6/">https://www.amazon.de/Stolz-Vorurteil-Roman-Reclam-Taschenbuch-ebook/dp/B01BHWFX6/</a> (Amazon)                                                                                                                                        |
|                      | Karin von Schwab                                                  | <i>Stolz und Vorurteil</i>                             | Null Papier (Düsseldorf, Germany, 2018)                                                                                          | <a href="https://www.amazon.de/Stolz-Vorurteil-Vollständige-Ausgabe-Klassiker-ebook/dp/B007506EGS/">https://www.amazon.de/Stolz-Vorurteil-Vollständige-Ausgabe-Klassiker-ebook/dp/B007506EGS/</a> (Amazon)                                                                                                                          |
| Dutch                | Margret Stevens & Trots en vooroordeel                            | <i>Trots en vooroordeel</i>                            | Athenaeum-Polak & Van Genep (Amsterdam, The Netherlands, 2014), 2nd edn.                                                         | <a href="https://www.amazon.de/Trots-vooroordeel-Dutch-Jane-Austen-ebook/dp/B00NYLD1W/">https://www.amazon.de/Trots-vooroordeel-Dutch-Jane-Austen-ebook/dp/B00NYLD1W/</a> (Amazon)                                                                                                                                                  |
|                      | Annelies Roeleveld                                                | <i>Trots en vooroordeel</i>                            | lands, 2014), 2nd edn.                                                                                                           |                                                                                                                                                                                                                                                                                                                                     |
| Spanish              | Ana M. Rodríguez                                                  | <i>Orgullo y prejuicio</i>                             | Penguin Clásicos (Barcelona, Spain, 2016)                                                                                        | <a href="https://www.amazon.com/Orgullo-prejuicio-mejores-clásicos-Spanish-ebook/dp/B00XJQ9BG/">https://www.amazon.com/Orgullo-prejuicio-mejores-clásicos-Spanish-ebook/dp/B00XJQ9BG/</a> (Amazon)                                                                                                                                  |
|                      | José de Urríes                                                    | <i>y Orgullo y prejuicio</i>                           | Biblioteca Luna (Madrid, Spain, 2017)                                                                                            | <a href="https://www.amazon.com/Orgullo-Prejuicio-Spanish-Jane-Austen-ebook/dp/B075FGRTFP/">https://www.amazon.com/Orgullo-Prejuicio-Spanish-Jane-Austen-ebook/dp/B075FGRTFP/</a> (Amazon)                                                                                                                                          |
|                      | Azara                                                             | <i>Orgullo y prejuicio</i>                             | Createspace Independent Publishing Platform (2018)                                                                               | <a href="https://www.amazon.com/Primeras-Impresiones-Orgullo-Prejuicio-Illustrated-ebook/dp/B07CMJ8S4V/">https://www.amazon.com/Primeras-Impresiones-Orgullo-Prejuicio-Illustrated-ebook/dp/B07CMJ8S4V/</a> (Amazon)                                                                                                                |
| French               | Valentine Leconte & Charlotte Benoit                              | <i>Les cinq filles de Mrs Bennet</i>                   | Librairie Plon (Paris, France, 1932)                                                                                             | * <a href="https://fr.wikisource.org/wiki/Les_Cinq_Filles_de_Mrs_Bennet/Texte_entier">https://fr.wikisource.org/wiki/Les_Cinq_Filles_de_Mrs_Bennet/Texte_entier</a> (Wikisource)                                                                                                                                                    |
| Latin                | Thomas M. Cotton                                                  | <i>Superbia Et Odium</i>                               | Phaselus Publishing (Rhosili, UK, 2015)                                                                                          | <a href="http://www.lulu.com/shop/tom-cotton/superbia-et-odium/ebook/product-22288563.html">http://www.lulu.com/shop/tom-cotton/superbia-et-odium/ebook/product-22288563.html</a> (Lulu)                                                                                                                                            |
| Polish               | Anna Trzeciakowska                                                | <i>Duma i uprzedzenie</i>                              | Prószyński Media (Warsaw, Poland, 2012)                                                                                          | * <a href="http://www.rulit.me/books/duma-i-uprzedzenie-read-270058-1.html">http://www.rulit.me/books/duma-i-uprzedzenie-read-270058-1.html</a> (Electronic Library Rulit)                                                                                                                                                          |
| Russian              | И. С. Маршак                                                      | <i>Гордость и преубеждение</i>                         | Художественная литература (Москва, СССР [Moscow, USSR], 1988)                                                                    | <a href="http://lib.ru/INOOLD/GSTEN/gord.txt">http://lib.ru/INOOLD/GSTEN/gord.txt</a> (Maxim Mashkov’s Library)                                                                                                                                                                                                                     |
| <i>Uralic</i>        |                                                                   |                                                        |                                                                                                                                  |                                                                                                                                                                                                                                                                                                                                     |
| Finnish              | O. A. Joutsen                                                     | <i>Ylpeys ja ennakkoluulo</i>                          | Werner Söderström Osakeyhtiö (Porvoo, Finland, 1922)                                                                             | * <a href="http://www.gutenberg.org/cache/epub/45186/pg45186.txt">http://www.gutenberg.org/cache/epub/45186/pg45186.txt</a> (Project Gutenberg)                                                                                                                                                                                     |
| Hungarian            | Szenci Miklós                                                     | <i>Büszkeség és bálítélet</i>                          | Európa Könyvkiadó (Budapest, Hungary, 1958)                                                                                      | * <a href="http://mek.oszk.hu/00300/00317/">http://mek.oszk.hu/00300/00317/</a> (Hungarian Electronic Library)                                                                                                                                                                                                                      |
| <i>Vasconic</i>      |                                                                   |                                                        |                                                                                                                                  |                                                                                                                                                                                                                                                                                                                                     |
| Basque               | Ana Isabel Morales                                                | <i>Harrotasuna eta aurre-juzguak</i>                   | Elkar argitaletxea (Donostia, Spain, 2013)                                                                                       | <a href="https://play.google.com/store/books/details/Austen_Jane_Harrotasuna_eta_aurrejuzguak?id=cMrNDQAQBAJ">https://play.google.com/store/books/details/Austen_Jane_Harrotasuna_eta_aurrejuzguak?id=cMrNDQAQBAJ</a> (Google Play)                                                                                                 |
| <i>Koreanic</i>      |                                                                   |                                                        |                                                                                                                                  |                                                                                                                                                                                                                                                                                                                                     |
| Korean               | 원유경 (元裕卿)                                                         | <i>오만과 편견 (傲慢과 偏見)</i>                                 | 주식회사 열린책들 (株式會社  열린冊들) (대한민국 경기도 파주시 (大韓民國 京畿道 坡州市) [Paju, A4/EB/A7/8C/EA/B3/BC_ED/8E/B8/EA/B2/AC7id=umMaGcAAQBAJ] (Google Play) | <a href="https://play.google.com/store/books/details/%EC%A0%9C%EC%9D%B8_%EC%98%A4%EC%8A%A4%ED%8B%B4_%EC%98%EA%8C%EA%B3%BC_%ED%8E%B8%EA%B2%AC7id=umMaGcAAQBAJ">https://play.google.com/store/books/details/%EC%A0%9C%EC%9D%B8_%EC%98%A4%EC%8A%A4%ED%8B%B4_%EC%98%EA%8C%EA%B3%BC_%ED%8E%B8%EA%B2%AC7id=umMaGcAAQBAJ</a> (Google Play) |
| Turkish              | Işıl Önder                                                        | <i>Gurur ve Önyargı</i>                                | İletişim Yayınları (Istanbul, Turkey, 2019)                                                                                      | <a href="https://play.google.com/store/books/details/Jane_Austen_Gurur_ve_%C3%96nyarg%C4%B1?id=EfCEDwAAQBAJ">https://play.google.com/store/books/details/Jane_Austen_Gurur_ve_%C3%96nyarg%C4%B1?id=EfCEDwAAQBAJ</a> (Google Play)                                                                                                   |
| <i>Indo-European</i> |                                                                   |                                                        |                                                                                                                                  |                                                                                                                                                                                                                                                                                                                                     |
| English              | Charlotte Brontë                                                  | <i>Jane Eyre</i>                                       | Service & Paton (London, UK, 1897)                                                                                               | * <a href="http://www.gutenberg.org/cache/epub/1260/pg1260.txt">http://www.gutenberg.org/cache/epub/1260/pg1260.txt</a> (Project Gutenberg)                                                                                                                                                                                         |
|                      | Maira Buffini                                                     | <i>Jane Eyre</i>                                       | Internet Movie Scripts Database (2008)                                                                                           | * <a href="https://www.imdb.com/scripts/Jane-Eyre.html">https://www.imdb.com/scripts/Jane-Eyre.html</a>                                                                                                                                                                                                                             |
| German               | Maria von Borch                                                   | <i>Jane Eyre</i>                                       | Jazybee Verlag (Altenmünster, Germany, 2012)                                                                                     | <a href="https://www.amazon.com/gp/product/B009XCD1D4/">https://www.amazon.com/gp/product/B009XCD1D4/</a> (Amazon)                                                                                                                                                                                                                  |
| French               | Noëmi Lesbazeilles                                                | <i>Jane Eyre ou Les mémoires d’une institutrice</i>    | Librairie Hachette (Paris, France, 1847)                                                                                         | * <a href="http://www.gutenberg.org/cache/epub/16235/pg16235.txt">http://www.gutenberg.org/cache/epub/16235/pg16235.txt</a> (Project Gutenberg)                                                                                                                                                                                     |
| Russian              | В. Станевич                                                       | <i>Джейн Эйр</i>                                       | Издательство «Правда» (Москва, СССР [Moscow, USSR], 1988)                                                                        | <a href="http://www.lib.ru/INOOLD/BRONTE/janeair.txt">http://www.lib.ru/INOOLD/BRONTE/janeair.txt</a> (Maxim Mashkov’s Library)                                                                                                                                                                                                     |
| <i>Uralic</i>        |                                                                   |                                                        |                                                                                                                                  |                                                                                                                                                                                                                                                                                                                                     |
| Finnish              | Tyne Tallgren                                                     | <i>Haapanen-Kotiapettajattaren maani</i>               | Werner Söderström Osakeyhtiö (Porvoo, Finland, 1921)                                                                             | * <a href="http://www.gutenberg.org/cache/epub/47275/pg47275.txt">http://www.gutenberg.org/cache/epub/47275/pg47275.txt</a> (Project Gutenberg)                                                                                                                                                                                     |
| Hungarian            | Ruzitska Mária                                                    | <i>Jane Eyre</i>                                       | Európa Könyvkiadó (Budapest, Hungary, 1972)                                                                                      | * <a href="http://mek.oszk.hu/05600/05680/">http://mek.oszk.hu/05600/05680/</a> (Hungarian Electronic Library)                                                                                                                                                                                                                      |
| <i>Indo-European</i> |                                                                   |                                                        |                                                                                                                                  |                                                                                                                                                                                                                                                                                                                                     |
| English              | Charles Darwin                                                    | <i>Origin of Species</i>                               | John Murray (London, UK, 1873), 6th edn.                                                                                         | * <a href="http://www.gutenberg.org/cache/epub/2009/pg2009.txt">http://www.gutenberg.org/cache/epub/2009/pg2009.txt</a> (Project Gutenberg)                                                                                                                                                                                         |
| French               | Edmond Barbier                                                    | <i>L’origine des espèces</i>                           | Schleicher Frères éditeurs (Paris, France, 1906)                                                                                 | * <a href="http://www.gutenberg.org/cache/epub/14158/pg14158.txt">http://www.gutenberg.org/cache/epub/14158/pg14158.txt</a> (Project Gutenberg)                                                                                                                                                                                     |
| Polish               | Szymon Dickstein & Józef Niusbaum                                 | <i>O powstawaniu gatunków drogą doboru naturalnego</i> | Przełęcz Tygodniowy (Warsaw, Poland, 1884)                                                                                       | * <a href="https://wcnlektury.pl/katalog/lektura/darwin-o-powstawaniu-gatunkow/">https://wcnlektury.pl/katalog/lektura/darwin-o-powstawaniu-gatunkow/</a> (Polish Free Reading)                                                                                                                                                     |
| Russian              | К. А. Тимирязев & М. А. Мензбир & А. П. Павлов & П. А. Петровский | <i>Происхождение видов</i>                             | Наука (Санкт-Петербург, СССР [Saint Petersburg, USSR], 1991)                                                                     | * <a href="http://darwin-online.org.uk/content/frameset?itemID=F763b&amp;viewtype=text&amp;pageseq=1">http://darwin-online.org.uk/content/frameset?itemID=F763b&amp;viewtype=text&amp;pageseq=1</a> (Darwin Online)                                                                                                                 |
| <i>Uralic</i>        |                                                                   |                                                        |                                                                                                                                  |                                                                                                                                                                                                                                                                                                                                     |
| Finnish              | Aarno Rafael                                                      | <i>Kos-Lajien synti</i>                                | Arvi A. Karisto (Hämeenlinna, Finland, 1913)                                                                                     | * <a href="http://www.gutenberg.org/cache/epub/52187/pg52187.txt">http://www.gutenberg.org/cache/epub/52187/pg52187.txt</a> (Project Gutenberg)                                                                                                                                                                                     |
| Hungarian            | Kampis György                                                     | <i>A fajok eredete</i>                                 | Neumann Kht. (Budapest, Hungary, 2004)                                                                                           | * <a href="http://mek.oszk.hu/05000/05011/">http://mek.oszk.hu/05000/05011/</a> (Hungarian Electronic Library)                                                                                                                                                                                                                      |

Notes:

(1) Translators’ names are given in native script and native order (surnames go first for Hungarian and Korean translators). Names of collaborating translators are separated by an & sign, irrespective of native practices. Books’ titles and publishers’ names are printed in their original languages. Publishers’ addresses are translated into English if originally written in the Latin script. Otherwise, English translations (in brackets) accompany the original addresses in non-Latin script.

(2) Freely available electronic resources are marked with an asterisk. Descriptions of websites are translated into English, wherever applicable.

(3) The German (resp. Spanish) version of *Pride and Prejudice* used in the preparation of Table S2 is translated by Christian Grawe & Ursula Grawe (resp. Ana M. Rodríguez). The same will also apply to Fig. S5 (resp. Fig. S7).

<sup>8</sup>We do not consider questions or dependent clauses, whose word orders might differ from those of the declarative sentences as independent clauses.

<sup>9</sup>Both French and Spanish switch to SOV order when the object is a pronoun. Since we ignore pronouns (which belong to function words, as opposed to content words) in our Markov model, we can regard both French and Spanish as fully SVO languages.

<sup>10</sup>Here, the (optionally present) second verb (V<sub>2</sub>) is in a non-finite form, such as an infinitive or a participle. In addition, Danish, Dutch and German are V2 (verb-second, not to be confused with the aforementioned V<sub>2</sub> notation) languages, placing the conjugated verb in the second position of a sentence, even when its preceding constituent is not the subject.

<sup>11</sup>In principle, one can freely switch word orders in Latin without affecting the meaning of a sentence: “Darcy loves Elizabeth” can be translated by all the six possible permutations of the words *Darceius*, *amat* and *Elizabetham*. In practice, the SOV order (such as *Darceius Elizabetham amat*) is dominant. The situation of Basque is similar to that of Latin. Korean and Turkish are both strictly SOV.

<sup>12</sup>Like Latin, these languages mark overtly subjects and objects through declensions, so word order is not important. It is arguable whether these languages should be classified as (predominantly) SVO, just as Latin is classified as SOV (by default).

Table S2. Statistical dictionary generated from bipartite matching of semantic fingerprints, using Jane Austen's *Pride and Prejudice*, and its translation into an Indo-European language

| (en) English    | (da) Danish | (de) German  | (nl) Dutch  | (es) Spanish | (fr) French   | (la) Latin    | (pl) Polish | (ru) Russian | (en) English | (da) Danish    | (de) German | (nl) Dutch  | (es) Spanish | (fr) French   | (la) Latin    | (pl) Polish | (ru) Russian |         |
|-----------------|-------------|--------------|-------------|--------------|---------------|---------------|-------------|--------------|--------------|----------------|-------------|-------------|--------------|---------------|---------------|-------------|--------------|---------|
| absence         |             |              | afwezigheid | absence      |               |               |             |              | laugh        | lachen         | lachen      |             | rire         |               |               |             |              |         |
| admire          | beundrede   | Bewunderung  |             |              |               |               |             |              | letter       | Brief          | brief       | carta       | lettre       | litteras      | list          | писмо       |              |         |
| agreeable       | behagelig   |              |             |              |               |               |             |              | library      | biblioteket    | Bibliothek  | bibliotheek | biblioteca   | bibliotheca   | biblioteki    | библиотека  |              |         |
| asked           |             |              |             | preguntó     |               |               |             |              | Lizzy        | Lizzy          | Lizzy       | Lizzy       | Lizula       | Lizula        | Lizy          | Лиззи       |              |         |
| aunt            | tante       | Tante        | tante       | tia          | tante         | matertera     | ciotka      | тетяшка      | London       | London         | London      | London      | Londres      | Londini       |               | Лондон      |              |         |
| ball            | bal         | Ball         | bal         |              |               |               | balu        | бал          | long         | lång           | lang        | lang        |              | longum        |               |             |              |         |
| beauty          | smukke      |              |             | hermosa      |               |               |             | красоты      | looked       | onske          | bliek       | lang        | miró         |               |               |             |              |         |
| believe         | tror        |              | geloven     |              |               |               |             |              | Lucas        | Lucas          | Lucas       | Lucas       | Lucas        | Lucas         | Lucas         | Лукас       |              |         |
| Bennet          | Bennet      | Bennet       | Bennet      | Bennet       | Bennet        | Bennet        | Bennet      | Беннет       | Lydia        | Lydia          | Lydia       | Lydia       | Lydia        | Lydia         | Lydia         | Лидия       |              |         |
| Bingley         | Bingley     | Bingley      | Bingley     | Bingley      | Bingley       | Bingleius     | Bingley     | Бингли       | madam        |                |             |             |              |               |               |             |              |         |
| book            | bog         | Buch         | boek        |              |               |               | Bourgh      | де           | man          | mand           | Mann        | man         | bombre       |               | homo          |             | человек      |         |
| Bourgh          |             |              |             |              |               |               | Bourgh      | де           | marriage     | gift           |             |             |              | marriage      | matrimonium   | matrimony   | замуж        |         |
| breakfast       |             |              |             |              |               |               |             |              | Mary         | Mary           | Mary        | Mary        | Mary         | Mary          | Mary          | Mary        | Мэри         |         |
| Brighton        | Brighton    | Brighton     | Brighton    | Brighton     | Brighton      | Britoniam     | Brighton    | Брайтон      | means        | Mary           | Mary        | Mary        | Mary         | Mary          | Mary          | Mary        | Мэри         |         |
| brother         | morbror     | Bruder       | broer       | hermano      | frère         | fratris       | brata       | брат         | Meryton      | Meryton        |             | Meryton     | Meryton      | Merytonae     | Meryton       | Merytone    |              |         |
| carriage        | vognen      | Kutsche      | rijtuig     | coche        | voiture       |               | powóz       | экипаж       | miles        | Meryton        | Meryton     |             | Meryton      | Meryton       | Merytonae     | Meryton     | Merytone     |         |
| case            | tilfelde    |              |             |              |               |               |             |              | Miss         | Miss           | missvrouw   | Miss        | Miss         | hera          | pama          | мисс        |              |         |
| Catherine       | lady        | Lady         | lady        | Catherine    | Catherine     | Caterina      | Katarzyna   | Катерина     | money        | penge          | Geld        | linero      | Miss         | pecunia       | pecunia       | денег       |              |         |
| character       |             |              | arakter     |              |               |               |             |              | mother       | mor            | Mutter      | moeder      | madre        | mère          | matrem        | matka       | матери       |         |
| Charlotte       | Charlotte   | Charlotte    | Charlotte   | Charlotte    | Charlotte     | Carlotta      | Charlotta   | Шарлотта     | motive       | bevæggrund     |             | moeder      | madre        | mère          | motif         |             |              |         |
| children        | børn        | Kind         | kinderen    |              |               |               |             | дети         | Mr           | Mr             | Mr          | mijnheer    | Mr           | Mr            | Mra           |             | Мистер       |         |
| choose          | valgte      |              |             |              |               |               |             |              | Mrs          | Mrs            | Mrs         | mevrouw     | Mrs          | Mrs           | Mra           |             | Миссис       |         |
| civility        |             |              |             | cortesia     |               |               |             | почтено      | neighborhood | nabolaget      |             |             |              |               |               |             | соседство    |         |
| Collins         | Collins     | Collins      | Collins     | Collins      | Collins       | Collina       | Collins     | Коллинз      | nephew       | nevø           | Neffen      |             | neveu        | Infrapatensum | Netherfield   | Netherfield | нефрпуде     |         |
| colony          | oberst      | Oberst       | kolonel     | coronel      | colonel       | praefectus    | pułkownik   | полковник    | Netherfield  | Netherfield    | Netherfield | Netherfield | Netherfield  | Netherfield   | Infrapatensum | Netherfield | Netherfield  |         |
| comfort         | trost       | Trost        |             |              |               |               |             | полкомы      | niece        |                |             |             | nièce        | sobrina       | niece         | племянница  |              |         |
| compliment      | kompliment  |              | compliment  | cumplido     |               |               |             |              | officers     | officererne    | Offiziere   | officieren  | oficiales    | officiers     | subpraefectos | oficerów    | офицеров     |         |
| congratulations |             |              |             | complido     | felicitations | gratulor      |             |              | oh           | oh             |             |             |              |               |               |             |              |         |
| consolation     |             |              | troost      | consuelo     |               |               |             |              | pain         | smerte         |             |             |              |               |               |             |              |         |
| cousin          | Cousine     |              |             | cousin       | consobrina    |               | Kuzyna      | кузина       | park         | parken         | Park        | park        | parque       | pare          |               | park        | парк         |         |
| cried           | udbrød      |              | hep         | exclamó      | ecría         |               |             |              | Pemberley    | Pemberley      | Pemberley   | Pemberley   | Pemberley    | Pemberley     | Pemberleianam | Pemberley   | Pemberley    |         |
| dance           | danse       | tanzen       | dansen      |              |               |               |             | танцевать    | people       |                |             |             |              |               |               | ludzi       | люди         |         |
| Darcy           | Darcy       | Darcy        | Darcy       | Darcy        | Darcy         | Darcetus      | Darcy       | Дарси        | Philips      | Philips        | Philips     | Philips     | Philips      | Philips       | Philips       | Philips     | Филипс       |         |
| datter          | Tochter     | dochter      |             | hija         | filia         |               |             | дочери       | plan         |                |             |             |              |               |               |             |              |         |
| day             | dag         | Nachricht    | dag         | dia          | die           |               |             | день         | pleased      |                |             |             |              |               | bonestores    |             |              |         |
| de              | Bourgh      | Bourgh       | Bourgh      |              |               |               |             | де           | politeness   |                |             |             |              |               |               |             |              |         |
| dear            | kære        | Bourgh       | Bourgh      |              | chère         | carissima     |             | дорогая      | poor         | stakkels       | arme        | arme        | pobre        | pauvre        |               |             |              |         |
| deceived        |             |              |             | engaño       |               |               |             |              | pounds       | pund           | Pfund       | pond        |              |               |               | funto       | тысяч        |         |
| Derbyshire      | Derbyshire  | Derbyshire   | Derbyshire  |              | Derbyshire    | Derventiano   |             | Дербишайр    | pride        | stolthed       | Stolz       | trots       | orgullo      |               |               | huma        | гордость     |         |
| deserve         | fortjent    |              |             | comer        | coenam        |               |             |              | promised     |                |             |             | prometido    | promesse      |               |             |              |         |
| dinner          | middag      | Essen        | dineren     |              | diner         |               |             |              | read         | leste          | las         | las         | leer         |               |               | czytać      |              |         |
| disappointment  | skuffelse   | Enttäuschung |             |              |               |               |             |              | refuse       |                |             |             | rechazar     | refus         | recusare      |             |              |         |
| dislike         |             |              |             |              |               |               |             | непринять    | regiment     | regimentet     | Regiment    | regiment    | regimiento   | régiment      |               |             | полк         |         |
| distance        |             |              |             | distance     |               |               |             |              | relations    | fortalte       |             |             |              |               |               |             |              |         |
| door            | døren       | Tür          |             | puerta       |               |               |             |              | respect      |                |             |             | respeto      |               |               | szacunku    | уважения     |         |
| elegant         |             |              | elegante    |              |               |               |             | wytworna     | room         |                | Zimmer      | kamer       |              |               |               | pokoiu      | комнаты      |         |
| Elizabeth       | Elizabeth   | Elizabeth    | Elizabeth   | Lizy         | Elizabeth     | Elizabetha    | Elzbieta    | Элизабет     | Rosings      | Rosings        | Rosings     | Rosings     | Rosings      | Rosings       | Rosarium      | Rosings     | Розингсе     |         |
| entered         | intrit      |              |             | ingressus    |               |               |             |              | said         | said           |             |             |              |               |               |             | сказала      |         |
| estate          | gods        | Erbe         |             |              |               |               |             | наследство   | see          |                |             | zien        |              |               |               |             | видела       |         |
| evening         | aftenen     | Abend        | avond       | velada       | sor           | vesperem      |             | вечер        | seemed       |                |             | leek        |              |               |               |             |              |         |
| eyes            | øjen        |              | ogen        | oculos       |               |               |             |              | send         | sendt          |             |             | enviado      | envoyer       |               |             |              |         |
| father          | far         | Vater        | vader       | padre        | père          | pater         | ojciec      | отец         | serious      | alvorligt      | ernst       | serius      |              |               |               |             |              |         |
| felt            |             |              | gevoelens   | sentiments   | sententias    |               | uczucia     |              | servant      |                | Diener      |             | criado       |               | ministris     | slużącego   |              |         |
| Fitzwilliam     | Fitzwilliam | Fitzwilliam  | Fitzwilliam | Fitzwilliam  | Fitzwilliam   | Fitzwilliamus | Fitzwilliam | Фитцвиллиам  | Sir          | sir            | Sir         | William     | sir          | sir           | Senior        | sir         | сэр          |         |
| five            | fem         | fiuf         | vijf        | cinco        |               |               |             | пять         | society      |                |             |             |              | société       |               |             |              |         |
| forget          |             |              |             |              |               | oblivisci     |             |              | sorry        | ked            |             | spijt       |              |               |               |             |              |         |
| Forster         | Forster     | Forster      | Forster     | Forster      | Forster       |               | Forster     | Форстер      | speak        | tale           |             | sprecken    |              |               | loqui         |             |              |         |
| fortnight       | uger        |              |             |              |               |               |             |              | surprise     | overrasket     | überrascht  |             | sorprendida  |               | attonita      |             |              |         |
| fortune         | formue      | Vermögen     |             | fortuna      | fortune       |               |             |              | table        | bordet         | Tisch       | tafel       |              | table         |               | sole        | столом       |         |
| four            | fire        | vier         | vier        | cuatro       |               |               |             |              | talking      | talte          |             |             |              |               | colloqui      |             |              |         |
| Gardiner        | Gardiner    | Gardiner     | Gardiner    | Gardiner     | Gardiner      |               | Gardiner    | Гардинер     | tell         |                |             | vertellen   |              |               |               |             |              |         |
| gentlemen       | herre       |              | heer        | caballero    |               |               |             |              | ten          | ti             |             | tien        | diez         | dix           |               |             | десять       |         |
| girls           | pige        | Mädchen      | meisjes     |              |               |               |             | dzieczęta    | thank        |                |             |             |              | merceriements |               |             |              |         |
| glad            |             |              |             |              |               |               |             |              | thousand     | lustinde       |             | henduizend  | mil          | mille         | libarum       | тысячу      | тысяч        |         |
| good            | godt        | gut          |             | mejor        | mieux         |               |             |              | town         | London         |             |             | capital      | Londres       |               | Londynu     | Лондон       |         |
| hand            |             |              | hand        |              |               |               |             |              | turned       | vendte         |             |             |              |               |               |             |              |         |
| handsome        |             | hübsch       | knap        |              |               |               |             |              | to           |                |             | wee         |              | deus          | avunculus     | wuja        | дядя         |         |
| happy           |             | Glück        | geluk       | felicidad    |               |               |             | szczęścia    | uncle        | morbror        | Onkel       | oom         | tio          | oncle         | avunculus     | wuja        | дядя         |         |
| honour          | ære         | Ehre         | eer         | honor        |               | honore        |             | шести        | vain         | forfængelighed |             |             | vanidad      |               | vano          |             | нищеславие   |         |
| house           | huset       | Haus         | huis        |              | domum         |               |             |              | visit        | besøg          | Besuch      | bezoek      |              | visite        |               |             | визит        |         |
| Hurst           |             |              |             | Hurst        |               |               | Hurst       |              | walk         |                |             |             |              |               | ambulare      |             |              |         |
| husband         | agtemand    |              |             | marido       | mari          |               |             | мужа         | want         | mangel         |             |             |              |               |               |             |              |         |
| ignorant        | uvildende   |              |             | ignoro       | ignore        |               |             |              | week         | uge            |             | weken       | semana       | semaine       | septimanis    | tygodnie    | неделю       |         |
| impossible      | umuligt     | ummöglich    |             | imposible    |               |               |             |              | Wickham      | Wickham        | Wickham     | Wickham     | Wickham      | Wickham       | Wickham       | Wickham     | Уикхем       |         |
| intended        | hensigt     |              |             | imposible    |               |               |             |              | wife         |                |             |             | uxor         |               |               | żony        |              |         |
| invitation      |             | Einladung    | uitnodiging | invitación   | invitation    |               |             | zaproszenie  | William      | William        | William     | William     | William      | William       | Gulielmus     | William     | Уильям       |         |
| Jane            | Jane        | Jane         | Jane        | Jane         | Ioanna        |               | Jane        | Джейн        | window       | vinduet        | Jane        |             | ventana      |               | Gulielmus     | Jane        | окна         |         |
| journey         |             |              |             |              |               |               |             | podróży      | woman        | skvnde         |             | yrouw       | mujer        | escribir      | écrire        | scripsit    | kobieta      | женщина |
| Kitty           | Kitty       | Kitty        | Kitty       | Kitty        | Kitty         | Kitteia       | Kitty       | Китти        | write        | skrive         | schreiben   | schrijven   | escribir     | écrire        | scripsit      | psac        | писать       |         |
| know            |             | weiß         | weet        |              |               |               |             | wiad         | years        | år             | Jahr        | jaar        | años         | ans           | annos         |             | лет          |         |
| lady            |             |              |             |              |               |               |             | lady         | young        | unge           | jungen      | jongedames  | jovent       | jeune         | paru          |             |              |         |

Notes:  
 (1) See Table S1 for provenances of texts.  
 (2) This table is sorted alphabetically according to the English entries.  
 (3) For clarity, only the most frequent word within a word pattern is tabulated. See Figs. S4–S11 for details of bipartite matching.  
 (4) Color encoding follows [1, Fig. 5c]: green = correct match; amber = close match; red = incorrect match.  
 (5) Column separator demarcates different subgroups (Germanic, Romance & Latin, Slavic) of the Indo-European language family. A Germanic compound noun (such as Danish *morbror*) may appear as the translation of more than one word.

Table S3. Statistical dictionary generated from bipartite matching of semantic fingerprints, using Jane Austen's *Pride and Prejudice*, and its translation into a non-Indo-European language

| (en) English    | (fi) Finnish | (hu) Hungarian | (eu) Basque | (ko) Korean     | (tr) Turkish | (en) English | (fi) Finnish  | (hu) Hungarian  | (eu) Basque   | (ko) Korean                    | (tr) Turkish   |
|-----------------|--------------|----------------|-------------|-----------------|--------------|--------------|---------------|-----------------|---------------|--------------------------------|----------------|
| admire          |              |                |             | 모략(謀略)화         | havranlık    | know         | nauraa        |                 | jakin         |                                |                |
| arrival         |              |                |             |                 |              | laugh        | kirjeen       | levelet         |               |                                | mektubu        |
| attachment      | läti         | bál            | atxikimendu |                 |              | letter       | kirjastoon    | könyvtárszobába | liburutegira  | 책재(書齋)로                        | kütüphaneye    |
| aunt            |              |                | zeko        | 무도회(舞踏會)에       | balo         | like         | Lizzy         | Lizzy           | antziun       | 리지(Lizzy)야                     | Lizzy          |
| ball            | uskoa        | Bennet         | Bennet      | 베넷(Bennet)      | Bennet       | Lizzy London | akarta        | Londonban       | Londonren     | long                           | Londra'ya      |
| believe         | Bennet       | Bennet         | Bennet      | 빙글리(Bingley)    | Bingley      | Lucas        | Lucas         | Lucas           | Lucas         | 부커스(Lucas)                     | Lucas          |
| Bennet          | Bingley      | Bennet         | Bennet      | 빙글리(Bingley)    | Bingley      | Lydia        | Lydia         | Lydia           | Lydia         | Lydia                          | Lydia          |
| Bingley         | Bingley      | Bennet         | Bennet      | 빙글리(Bingley)    | Bingley      | man          | mes           | ember           | ezkontza      | 결혼(結婚)을                        | evlenme        |
| book            | Bourghin     |                |             | 브라이튼(Brighton)에 | Brighton'a   | marriage     | Mary          | Mary            | Maryk         | 메리(Mary)는                      | Mary           |
| Bourgh          | Bourghin     |                |             | 캐서린(Catherine)  | Lady         | Mary         | Mary          | uzazaba         |               |                                |                |
| breakfast       | veijensä     | Brightonba     | Brightonera | 캐서린(Catherine)  | Lady         | means        | tehen         |                 | Merytonen     | 메리톤(Meryton)에                  | Meryton'a      |
| Brighton        | vaunut       | batyja         | neba        | 캐서린(Catherine)  | Lady         | master       | tehen         |                 | Merytonen     | 메리톤(Meryton)에                  | Meryton'a      |
| brother         | Charlotte    | Charlotte      | Charlotte   | 샬롯(Charlotte)이  | Charlotte    | master       | tehen         |                 | Merytonen     | 메리톤(Meryton)에                  | Meryton'a      |
| carriage        | Charlotte    | Charlotte      | Charlotte   | 샬롯(Charlotte)이  | Charlotte    | means        | tehen         |                 | Merytonen     | 메리톤(Meryton)에                  | Meryton'a      |
| Catherine       | Charlotte    | Charlotte      | Charlotte   | 샬롯(Charlotte)이  | Charlotte    | money        | rahoja        | Miss            | Merytonban    | 미스(Meryton)에                   | Miss           |
| character       | Charlotte    | Charlotte      | Charlotte   | 샬롯(Charlotte)이  | Charlotte    | mother       | aihi          | anya            | anyja         | 어머니가                           | para           |
| Charlotte       | Charlotte    | Charlotte      | Charlotte   | 샬롯(Charlotte)이  | Charlotte    | niece        | tyttö         | tyttö           | tyttö         | 아가씨가                           | animesi        |
| children        | Charlotte    | Charlotte      | Charlotte   | 샬롯(Charlotte)이  | Charlotte    | Mr           | herra         | herra           | herra         | 미인(夫人)은                        | Mr             |
| Charlotte       | Charlotte    | Charlotte      | Charlotte   | 샬롯(Charlotte)이  | Charlotte    | Mrs          | rouva         | rouva           | rouva         | 미부                             | Mrs            |
| civilty         | Charlotte    | Charlotte      | Charlotte   | 샬롯(Charlotte)이  | Charlotte    | neighborhood | naapuruston   | naapurusto      | naapurusto    | 이웃                             |                |
| Collins         | Charlotte    | Charlotte      | Charlotte   | 샬롯(Charlotte)이  | Charlotte    | nephew       | veljekset     | veljekset       | veljekset     | 형제(兄弟)들                        |                |
| Collins         | Charlotte    | Charlotte      | Charlotte   | 샬롯(Charlotte)이  | Charlotte    | Netherfield  | Netherfieldin | Netherfieldin   | Netherfieldin | 네더필드(Netherfield)에서            | Netherfield'da |
| colonel         | Charlotte    | Charlotte      | Charlotte   | 샬롯(Charlotte)이  | Charlotte    | officers     | herrat        | herrat          | herrat        | 장교(將校)들                        | subay          |
| come            | Charlotte    | Charlotte      | Charlotte   | 샬롯(Charlotte)이  | Charlotte    | oh           | oh            | oh              | oh            | 아                              | acı            |
| complement      | Charlotte    | Charlotte      | Charlotte   | 샬롯(Charlotte)이  | Charlotte    | pain         | kipinä        | kipinä          | kipinä        | 아픔                             |                |
| congratulations | Charlotte    | Charlotte      | Charlotte   | 샬롯(Charlotte)이  | Charlotte    | Pemberley    | Pemberleyin   | Pemberleyin     | Pemberleyin   | 페머블리(Pemberley)에               | Pemberley'e    |
| consolation     | Charlotte    | Charlotte      | Charlotte   | 샬롯(Charlotte)이  | Charlotte    | poor         | puuri         | puuri           | puuri         | 빈(貧)한                          | Phillips       |
| country         | Charlotte    | Charlotte      | Charlotte   | 샬롯(Charlotte)이  | Charlotte    | pounds       | raha          | raha            | raha          | 파운드(pound)를                    | Phillips       |
| cousin          | Charlotte    | Charlotte      | Charlotte   | 샬롯(Charlotte)이  | Charlotte    | pretty       | hieno         | hieno           | hieno         | 예쁜                             | round          |
| cried           | Charlotte    | Charlotte      | Charlotte   | 샬롯(Charlotte)이  | Charlotte    | pride        | hienous       | hienous         | hienous       | 자부심                            | zururu         |
| Darcy           | Charlotte    | Charlotte      | Charlotte   | 샬롯(Charlotte)이  | Charlotte    | promised     | lupaus        | lupaus          | lupaus        | 약속                             |                |
| Darcy           | Charlotte    | Charlotte      | Charlotte   | 샬롯(Charlotte)이  | Charlotte    | read         | lukea         | lukea           | lukea         | 읽다                             | okumaya        |
| daughter        | Charlotte    | Charlotte      | Charlotte   | 샬롯(Charlotte)이  | Charlotte    | refuse       | hyllyä        | hyllyä          | hyllyä        | 거절(拒絕)하다                       | reddetti       |
| day             | Charlotte    | Charlotte      | Charlotte   | 샬롯(Charlotte)이  | Charlotte    | relations    | suhteet       | suhteet         | suhteet       | 관계(關係)들                        | akrabaları     |
| de              | Charlotte    | Charlotte      | Charlotte   | 샬롯(Charlotte)이  | Charlotte    | respect      | arab          | arab            | arab          | 존경(尊敬)하다                       | saygı          |
| dear            | Charlotte    | Charlotte      | Charlotte   | 샬롯(Charlotte)이  | Charlotte    | room         | huone         | huone           | huone         | 방                              | Rosings'leki   |
| Derbyshire      | Charlotte    | Charlotte      | Charlotte   | 샬롯(Charlotte)이  | Charlotte    | Rosings said | Rosingsissa   | Rosingsissa     | Rosingsissa   | 로징스(Rosings)에서                 | dedi           |
| different       | Charlotte    | Charlotte      | Charlotte   | 샬롯(Charlotte)이  | Charlotte    | sat          | sat           | sat             | sat           | 사                              | gördü          |
| dine            | Charlotte    | Charlotte      | Charlotte   | 샬롯(Charlotte)이  | Charlotte    | see          | nähdä         | nähdä           | nähdä         | 만나다                            | görü           |
| dinner          | Charlotte    | Charlotte      | Charlotte   | 샬롯(Charlotte)이  | Charlotte    | send         | post          | post            | post          | 편지(信件)를                        | çiddi          |
| disappointment  | Charlotte    | Charlotte      | Charlotte   | 샬롯(Charlotte)이  | Charlotte    | serious      | vakava        | vakava          | vakava        | 진지(眞摯)하게                       | hizmetçi       |
| door            | Charlotte    | Charlotte      | Charlotte   | 샬롯(Charlotte)이  | Charlotte    | servant      | huljant       | huljant         | huljant       | 하인(下人)이                        | William        |
| elegant         | Charlotte    | Charlotte      | Charlotte   | 샬롯(Charlotte)이  | Charlotte    | suffer       | kärsiä        | kärsiä          | kärsiä        | 경(卿)이                          | William        |
| Elizabeth       | Charlotte    | Charlotte      | Charlotte   | 샬롯(Charlotte)이  | Charlotte    | surprise     | yllyttää      | yllyttää        | yllyttää      | 놀라게 하다                         | masaya         |
| evening         | Charlotte    | Charlotte      | Charlotte   | 샬롯(Charlotte)이  | Charlotte    | table        | pöytä         | pöytä           | pöytä         | 탁자(卓子) 를</td <td>tegekkür</td> | tegekkür       |
| eyes            | Charlotte    | Charlotte      | Charlotte   | 샬롯(Charlotte)이  | Charlotte    | thank        | kiittää       | kiittää         | kiittää       | 고맙게 말하다                        | masaya         |
| face            | Charlotte    | Charlotte      | Charlotte   | 샬롯(Charlotte)이  | Charlotte    | thousand     | tuhat         | tuhat           | tuhat         | 천(千)을                          | tegekkür       |
| father          | Charlotte    | Charlotte      | Charlotte   | 샬롯(Charlotte)이  | Charlotte    | town         | kaupunki      | kaupunki        | kaupunki      | 마을                             | masaya         |
| felt            | Charlotte    | Charlotte      | Charlotte   | 샬롯(Charlotte)이  | Charlotte    | turned       | muuttua       | muuttua         | muuttua       | 바뀌다                            | tegekkür       |
| fine            | Charlotte    | Charlotte      | Charlotte   | 샬롯(Charlotte)이  | Charlotte    | two          | kuusi         | kuusi           | kuusi         | 두(二)                           | masaya         |
| Fitzwilliam     | Charlotte    | Charlotte      | Charlotte   | 샬롯(Charlotte)이  | Charlotte    | uncle        | onkka         | onkka           | onkka         | 숙부(叔父)와                        | dayısı         |
| five            | Charlotte    | Charlotte      | Charlotte   | 샬롯(Charlotte)이  | Charlotte    | vain         | kuoli         | kuoli           | kuoli         | 사망(死)하다                        | ziyaret        |
| forget          | Charlotte    | Charlotte      | Charlotte   | 샬롯(Charlotte)이  | Charlotte    | visit        | käydä         | käydä           | käydä         | 방문(訪問)하다                       | ziyaret        |
| Forster         | Charlotte    | Charlotte      | Charlotte   | 샬롯(Charlotte)이  | Charlotte    | way          | tie           | tie             | tie           | 길                              | hafia          |
| four            | Charlotte    | Charlotte      | Charlotte   | 샬롯(Charlotte)이  | Charlotte    | weck         | herätyksiä    | herätyksiä      | herätyksiä    | 깨우다                            | Wickham        |
| Gardiner        | Charlotte    | Charlotte      | Charlotte   | 샬롯(Charlotte)이  | Charlotte    | Wickham      | Wickham       | Wickham         | Wickham       | 윅햄(Wickham)                    | Wickham        |
| gentlemen       | Charlotte    | Charlotte      | Charlotte   | 샬롯(Charlotte)이  | Charlotte    | wife         | vaimonsa      | vaimonsa        | vaimonsa      | 아내가                            | karısı         |
| girls           | Charlotte    | Charlotte      | Charlotte   | 샬롯(Charlotte)이  | Charlotte    | William      | William       | William         | William       | 윌리엄(William)                   | sir            |
| good            | Charlotte    | Charlotte      | Charlotte   | 샬롯(Charlotte)이  | Charlotte    | window       | ikkuna        | ikkuna          | ikkuna        | 창(窗)이                          | sir            |
| hand            | Charlotte    | Charlotte      | Charlotte   | 샬롯(Charlotte)이  | Charlotte    | woman        | nainen        | nainen          | nainen        | 여자                             | yaz            |
| happy           | Charlotte    | Charlotte      | Charlotte   | 샬롯(Charlotte)이  | Charlotte    | write        | kirjoittaa    | kirjoittaa      | kirjoittaa    | 쓰다                             | yl             |
| honour          | Charlotte    | Charlotte      | Charlotte   | 샬롯(Charlotte)이  | Charlotte    | years        | vuotta        | vuotta          | vuotta        | 년(年)                           | genç           |
| house           | Charlotte    | Charlotte      | Charlotte   | 샬롯(Charlotte)이  | Charlotte    | young        | nuori         | nuori           | nuori         | 젊은                             |                |
| Hurst           | Charlotte    | Charlotte      | Charlotte   | 샬롯(Charlotte)이  | Charlotte    |              |               |                 |               |                                |                |
| husband         | Charlotte    | Charlotte      | Charlotte   | 샬롯(Charlotte)이  | Charlotte    |              |               |                 |               |                                |                |
| impossible      | Charlotte    | Charlotte      | Charlotte   | 샬롯(Charlotte)이  | Charlotte    |              |               |                 |               |                                |                |
| intended        | Charlotte    | Charlotte      | Charlotte   | 샬롯(Charlotte)이  | Charlotte    |              |               |                 |               |                                |                |
| interest        | Charlotte    | Charlotte      | Charlotte   | 샬롯(Charlotte)이  | Charlotte    |              |               |                 |               |                                |                |
| introduction    | Charlotte    | Charlotte      | Charlotte   | 샬롯(Charlotte)이  | Charlotte    |              |               |                 |               |                                |                |
| invitation      | Charlotte    | Charlotte      | Charlotte   | 샬롯(Charlotte)이  | Charlotte    |              |               |                 |               |                                |                |
| Jane            | Charlotte    | Charlotte      | Charlotte   | 샬롯(Charlotte)이  | Charlotte    |              |               |                 |               |                                |                |
| Kitty           | Charlotte    | Charlotte      | Charlotte   | 샬롯(Charlotte)이  | Charlotte    |              |               |                 |               |                                |                |

Notes:  
 (1) See Table S1 for provenances of texts.  
 (2) This table is sorted alphabetically according to the English entries.  
 (3) For clarity, only the most frequent word within a word pattern is tabulated. See Figs. S12-S16 for details of bipartite matching.  
 (4) Color encoding follows [1, Fig. 5c]: green = correct match; amber = close match; red = incorrect match.  
 (5) Column separator demarcates different language families.  
 (6) Korean stems that derive from Chinese or English are accompanied by their etymologies in parentheses.

Table S4. Statistical dictionary generated from bipartite matching of semantic fingerprints, using Charlotte Brontë's *Jane Eyre*, and its translation into a European language

| (en)         | (de)         | (fr)         | (ru)          | (fi)         | (hu)         | (en)      | (de)        | (fr)        | (ru)       | (fi)                    | (hu)        | (en)       | (de)        | (fr)        | (ru)      | (fi)      | (hu)       |
|--------------|--------------|--------------|---------------|--------------|--------------|-----------|-------------|-------------|------------|-------------------------|-------------|------------|-------------|-------------|-----------|-----------|------------|
| English      | German       | French       | Russian       | Finnish      | Hungarian    | English   | German      | French      | Russian    | Finnish                 | Hungarian   | English    | German      | French      | Russian   | Finnish   | Hungarian  |
| Abbot        |              | Abbot        | Аббат         | Abbot        | Abbot        | garden    | Garten      | jardin      | сад        |                         | kertbe      | poor       |             | pauvre      | бедный    |           | szegény    |
| accompany    | begleiten    |              |               |              |              | Gateshead | Gateshead   | Gateshead   | Гейтсхэд   | Gatesheadista           | Georgiana   | prayers    |             |             |           |           | rukoukset  |
| Adele        | Adele        | Adele        | Адель         | Adele        | Adele        | girl      | Georgina    | Eliza       | Джорджана  | Georgiana               | Georgiana   | pride      | Stolz       |             | гордость  |           | büszke     |
| admiration   | Bewunderung  | admiration   |               |              |              | go        | Madchen     |             |            |                         | menjen      | principle  |             | principes   |           |           |            |
| afternoon    | Nachmittag   |              |               | Huopäivällä  | délután      | god       | gothen      | aller       |            |                         | isten       | promise    | versprechen | promesse    |           |           |            |
| angel        | Engel        | ange         |               | otta         | angyalok     | gold      | gott        | dieu        |            |                         | arany       | prove      | beweisen    |             |           |           |            |
| answer       |              |              |               | käsivartensa |              | good      |             | meux        |            |                         |             | rain       |             | pluie       |           |           |            |
| arms         |              | bras         |               | läti         | nemi         | governess | Gouvernante | губернантка |            | kotiopettajatarnevelöna |             | ran        |             |             |           |           | hizza      |
| aunt         | tante        | tante        | тетя          | ägi          | grace        | grace     | grace       |             |            |                         | becsukta    | read       | lesen       | comprendre  | читать    | työta     | olvasni    |
| bed          | Bette        | Bessie       |               | Bessie       | Bessie       | ground    |             |             |            |                         |             | reed       | Reed        | reed        | рид       | reed      |            |
| Bessie       |              | Bessie       |               | Bessie       | Bessie       | hair      | Haar        | Cheveux     | волосы     | hukka                   |             | relations  |             | parents     |           |           |            |
| birds        | Vögel        | oiseaux      | птицы         | musla        | fekete       | half      | halb        |             |            |                         | helyes      | remember   |             |             |           | muistin   |            |
| black        | schwarzen    | noir         | чёрные        |              |              | hall      | Hall        |             |            |                         |             | returned   | kehrte      | silence     |           |           | visszajött |
| blood        | Blut         | sang         | кровь         |              |              | hand      | Worte       | main        | руку       | mennä                   | kezét       | right      |             |             | нисто     |           |            |
| blue         | blauen       | bleu         |               |              | kek          | Hannah    | Hannah      | Anna        | чаштирна   | onnellinen              | gytölöletel | Rochester  | Rochester   | Rochester   | Роучестер | Rochester | Rochester  |
| book         | Buch         | livres       | книгу         | kirjan       | konyvet      | happy     | Hannah      | Anna        | счастлирна | onhellen                | gytölöletel | roof       | Dache       | Zimmer      | chambre   | комнате   |            |
| bread        | Brot         |              |               | kenyeret     |              | hate      |             |             |            | sydämeni                | szivem      | room       |             |             | комнате   |           |            |
| breakfast    | Frühstück    | déjeuner     | завтрака      | ajamiaista   | Brocklehurst | head      | Kopf        | gesund      | здоров     | entendre                | coeur       | rose       | Opfer       | sacrifice   | разговор  | istui     | engedje    |
| Brocklehurst | Brocklehurst | Brocklehurst | Брокльхерст   | Brocklehurst | Brocklehurst | health    | Kopf        | gesund      | здоров     | entendre                | coeur       | sacrifice  | Opfer       | sacrifice   | разговор  | istui     | engedje    |
| brother      | Bruder       | frère        | брат          | veljensä     | bátyja       | heard     | Herz        | coeur       | душтва     | sydämeni                | szivem      | sat        | Scatcherd   | Scatcherd   | Скечерд   | kouluun   | Scatcherd  |
| Burns        | Burns        | Burns        | Бернс         | Burns        | Burns        | heard     | Herz        | coeur       | душтва     | sydämeni                | szivem      | school     | Scatcherd   | Scatcherd   | Скечерд   | kouluun   | Scatcherd  |
| called       | licht        | appelait     |               | lumin        | magas        | heart     | Helen       | Helen       | Элен       | hallottam               | szivem      | schoolroom | Schulzimmer | Schulzimmer | школе     | kouluun   | Scatcherd  |
| candle       |              |              | свечу         | nyttöitä     | gyertyát     | Helen     | Helen       | Helen       | Элен       | hallottam               | szivem      | secret     | Schulzimmer | Schulzimmer | школе     | kouluun   | Scatcherd  |
| chair        | Stuhl        |              | кресло        | nyttöitä     | gyertyát     | home      | Hügel       | Hügel       | Хюгел      | hallottam               | szivem      | secret     | Schulzimmer | Schulzimmer | школе     | kouluun   | Scatcherd  |
| change       | Stuhl        | siège        |               | nyttöitä     | gyertyát     | hope      | Hügel       | Hügel       | Хюгел      | hallottam               | szivem      | secret     | Schulzimmer | Schulzimmer | школе     | kouluun   | Scatcherd  |
| child        | Kind         | enfant       | ребенок       | lapsi        | gyermek      | horse     | Pferd       | cheval      | лошадь     | hallottam               | szivem      | secret     | Schulzimmer | Schulzimmer | школе     | kouluun   | Scatcherd  |
| Christian    | Christen     | Chretien     |               | kirkon       |              | hour      | Stunde      | heure       | час        | hallottam               | szivem      | secret     | Schulzimmer | Schulzimmer | школе     | kouluun   | Scatcherd  |
| church       | Kirche       | église       | церковь       | kirkon       |              | house     | Hause       | maison      |            | hallottam               | szivem      | secret     | Schulzimmer | Schulzimmer | школе     | kouluun   | Scatcherd  |
| class        | Klasse       | classe       |               | kirkon       |              | human     | Menschliche |             |            | hallottam               | szivem      | secret     | Schulzimmer | Schulzimmer | школе     | kouluun   | Scatcherd  |
| clergyman    |              |              |               | pappi        |              | hungry    | Hunger      |             |            | hallottam               | szivem      | secret     | Schulzimmer | Schulzimmer | школе     | kouluun   | Scatcherd  |
| cloak        | Mantel       | manteau      | мантия        | pappi        |              | husband   | Gatten      | mar         |            | hallottam               | szivem      | secret     | Schulzimmer | Schulzimmer | школе     | kouluun   | Scatcherd  |
| cloud        | Wolken       | nuages       |               | pappi        |              | husband   | Gatten      | mar         |            | hallottam               | szivem      | secret     | Schulzimmer | Schulzimmer | школе     | kouluun   | Scatcherd  |
| cold         | helen        | retirer      | холодно       | pappi        |              | husband   | Gatten      | mar         |            | hallottam               | szivem      | secret     | Schulzimmer | Schulzimmer | школе     | kouluun   | Scatcherd  |
| come         | kam          | venir        | прийти        | pappi        |              | husband   | Gatten      | mar         |            | hallottam               | szivem      | secret     | Schulzimmer | Schulzimmer | школе     | kouluun   | Scatcherd  |
| cousins      | Locken       | boucles      | кудри         | pappi        |              | husband   | Gatten      | mar         |            | hallottam               | szivem      | secret     | Schulzimmer | Schulzimmer | школе     | kouluun   | Scatcherd  |
| curls        | Locken       | boucles      | кудри         | pappi        |              | husband   | Gatten      | mar         |            | hallottam               | szivem      | secret     | Schulzimmer | Schulzimmer | школе     | kouluun   | Scatcherd  |
| curtain      | Locken       | boucles      | кудри         | pappi        |              | husband   | Gatten      | mar         |            | hallottam               | szivem      | secret     | Schulzimmer | Schulzimmer | школе     | kouluun   | Scatcherd  |
| danger       | Gefahr       | danger       | опасность     | pappi        |              | husband   | Gatten      | mar         |            | hallottam               | szivem      | secret     | Schulzimmer | Schulzimmer | школе     | kouluun   | Scatcherd  |
| dark         | dunkel       | lumière      |               | pappi        |              | husband   | Gatten      | mar         |            | hallottam               | szivem      | secret     | Schulzimmer | Schulzimmer | школе     | kouluun   | Scatcherd  |
| daughter     | Zeit         | grande       | день          | pappi        |              | husband   | Gatten      | mar         |            | hallottam               | szivem      | secret     | Schulzimmer | Schulzimmer | школе     | kouluun   | Scatcherd  |
| day          | Zeit         | grande       | день          | pappi        |              | husband   | Gatten      | mar         |            | hallottam               | szivem      | secret     | Schulzimmer | Schulzimmer | школе     | kouluun   | Scatcherd  |
| dead         | tot          | mort         | смерть        | pappi        |              | husband   | Gatten      | mar         |            | hallottam               | szivem      | secret     | Schulzimmer | Schulzimmer | школе     | kouluun   | Scatcherd  |
| dear         | chère        | chère        |               | pappi        |              | husband   | Gatten      | mar         |            | hallottam               | szivem      | secret     | Schulzimmer | Schulzimmer | школе     | kouluun   | Scatcherd  |
| deep         | hef          |              |               | pappi        |              | husband   | Gatten      | mar         |            | hallottam               | szivem      | secret     | Schulzimmer | Schulzimmer | школе     | kouluun   | Scatcherd  |
| Dent         | Eshton       |              | Дэнт          | pappi        |              | husband   | Gatten      | mar         |            | hallottam               | szivem      | secret     | Schulzimmer | Schulzimmer | школе     | kouluun   | Scatcherd  |
| Diana        | Diana        | Diana        | Диана         | pappi        |              | husband   | Gatten      | mar         |            | hallottam               | szivem      | secret     | Schulzimmer | Schulzimmer | школе     | kouluun   | Scatcherd  |
| dinner       | Diana        | diner        | обед          | pappi        |              | husband   | Gatten      | mar         |            | hallottam               | szivem      | secret     | Schulzimmer | Schulzimmer | школе     | kouluun   | Scatcherd  |
| discovered   | entdeckt     |              |               | pappi        |              | husband   | Gatten      | mar         |            | hallottam               | szivem      | secret     | Schulzimmer | Schulzimmer | школе     | kouluun   | Scatcherd  |
| dog          | Hund         | chien        | собака        | pappi        |              | husband   | Gatten      | mar         |            | hallottam               | szivem      | secret     | Schulzimmer | Schulzimmer | школе     | kouluun   | Scatcherd  |
| door         | Thür         |              | дверь         | pappi        |              | husband   | Gatten      | mar         |            | hallottam               | szivem      | secret     | Schulzimmer | Schulzimmer | школе     | kouluun   | Scatcherd  |
| doubt        | Zweifel      |              |               | pappi        |              | husband   | Gatten      | mar         |            | hallottam               | szivem      | secret     | Schulzimmer | Schulzimmer | школе     | kouluun   | Scatcherd  |
| drawing-room |              |              |               | pappi        |              | husband   | Gatten      | mar         |            | hallottam               | szivem      | secret     | Schulzimmer | Schulzimmer | школе     | kouluun   | Scatcherd  |
| dream        | Traum        | rêve         |               | pappi        |              | husband   | Gatten      | mar         |            | hallottam               | szivem      | secret     | Schulzimmer | Schulzimmer | школе     | kouluun   | Scatcherd  |
| dressed      | Kleider      |              |               | pappi        |              | husband   | Gatten      | mar         |            | hallottam               | szivem      | secret     | Schulzimmer | Schulzimmer | школе     | kouluun   | Scatcherd  |
| eat          |              |              |               | pappi        |              | husband   | Gatten      | mar         |            | hallottam               | szivem      | secret     | Schulzimmer | Schulzimmer | школе     | kouluun   | Scatcherd  |
| Edward       | Edward       | Edouard      |               | pappi        |              | husband   | Gatten      | mar         |            | hallottam               | szivem      | secret     | Schulzimmer | Schulzimmer | школе     | kouluun   | Scatcherd  |
| eight        | Eliza        |              | восемь        | pappi        |              | husband   | Gatten      | mar         |            | hallottam               | szivem      | secret     | Schulzimmer | Schulzimmer | школе     | kouluun   | Scatcherd  |
| Eliza        | Eliza        |              | Элиза         | pappi        |              | husband   | Gatten      | mar         |            | hallottam               | szivem      | secret     | Schulzimmer | Schulzimmer | школе     | kouluun   | Scatcherd  |
| England      | Angletterre  | Angleterre   | Англия        | pappi        |              | husband   | Gatten      | mar         |            | hallottam               | szivem      | secret     | Schulzimmer | Schulzimmer | школе     | kouluun   | Scatcherd  |
| Eshton       | Dent         |              | Дэнт          | pappi        |              | husband   | Gatten      | mar         |            | hallottam               | szivem      | secret     | Schulzimmer | Schulzimmer | школе     | kouluun   | Scatcherd  |
| evening      |              | soir         | вечер         | pappi        |              | husband   | Gatten      | mar         |            | hallottam               | szivem      | secret     | Schulzimmer | Schulzimmer | школе     | kouluun   | Scatcherd  |
| event        |              | existence    | существование | pappi        |              | husband   | Gatten      | mar         |            | hallottam               | szivem      | secret     | Schulzimmer | Schulzimmer | школе     | kouluun   | Scatcherd  |
| existence    |              | existence    | существование | pappi        |              | husband   | Gatten      | mar         |            | hallottam               | szivem      | secret     | Schulzimmer | Schulzimmer | школе     | kouluun   | Scatcherd  |
| eyes         | Fuhr         | soule        | глаз          | pappi        |              | husband   | Gatten      | mar         |            | hallottam               | szivem      | secret     | Schulzimmer | Schulzimmer | школе     | kouluun   | Scatcherd  |
| Eyre         | Eyre         | Eyre         | Эйр           | pappi        |              | husband   | Gatten      | mar         |            | hallottam               | szivem      | secret     | Schulzimmer | Schulzimmer | школе     | kouluun   | Scatcherd  |
| face         | Gesicht      |              |               | pappi        |              | husband   | Gatten      | mar         |            | hallottam               | szivem      | secret     | Schulzimmer | Schulzimmer | школе     | kouluun   | Scatcherd  |
| Fairfax      | Fairfax      | Fairfax      | Фэйрфакс      | pappi        |              | husband   | Gatten      | mar         |            | hallottam               | szivem      | secret     | Schulzimmer | Schulzimmer | школе     | kouluun   | Scatcherd  |
| family       | Familie      | famille      | семья         | pappi        |              | husband   | Gatten      | mar         |            | hallottam               | szivem      | secret     | Schulzimmer | Schulzimmer | школе     | kouluun   | Scatcherd  |
| father       | Vater        | père         | отец          | pappi        |              | husband   | Gatten      | mar         |            | hallottam               | szivem      | secret     | Schulzimmer | Schulzimmer | школе     | kouluun   | Scatcherd  |
| fear         | Furcht       | crainte      |               | pappi        |              | husband   | Gatten      | mar         |            | hallottam               | szivem      | secret     | Schulzimmer | Schulzimmer | школе     | kouluun   | Scatcherd  |
| feet         | füßen        |              |               | pappi        |              | husband   | Gatten      | mar         |            | hallottam               | szivem      | secret     | Schulzimmer | Schulzimmer | школе     | kouluun   | Scatcherd  |
| felt         | fast         | tomber       |               | pappi        |              | husband   | Gatten      | mar         |            | hallottam               | szivem      | secret     | Schulzimmer | Schulzimmer | школе     | kouluun   | Scatcherd  |
| field        |              | champs       |               | pappi        |              | husband   | Gatten      | mar         |            | hallottam               | szivem      | secret     | Schulzimmer | Schulzimmer | школе     | kouluun   | Scatcherd  |
| figure       | Speisezimmer |              |               | pappi        |              | husband   | Gatten      | mar         |            | hallottam               | szivem      | secret     | Schulzimmer | Schulzimmer | школе     | kouluun   | Scatcherd  |
| fine         |              |              | прекрасно     | pappi        |              | husband   | Gatten      | mar         |            | hallottam               | szivem      | secret     | Schulzimmer | Schulzimmer | школе     | kouluun   | Scatcherd  |
| fingers      | Finger       | doigts       |               | pappi        |              | husband   | Gatten      | mar         |            | hallottam               | szivem      | secret     | Schulzimmer | Schulzimmer | школе     | kouluun   | Scatcherd  |
| fire         | Feuer        | assis        | представитель | pappi        |              | husband   | Gatten      | mar         |            | hallottam               | szivem      | secret     | Schulzimmer | Schulzimmer | школе     | kouluun   | Scatcherd  |
| first        | bringen      | sortir       | удалось       | pappi        |              | husband   | Gatten      | mar         |            | hallottam               | szivem      | secret     | Schulzimmer | Schulzimmer | школе     | kouluun   | Scatcherd  |
| five         | funf         | cinq         | пять          | pappi        |              | husband   | Gatten      | mar         |            | hallottam               | szivem      | secret     | Schulzimmer | Schulzimmer | школе     | kouluun   | Scatcherd  |
| flesh        | fleisch      |              |               | pappi        |              | husband   | Gatten      | mar         |            | hallottam               | szivem      | secret     | Schulzimmer | Schulzimmer | школе     | kouluun   | Scatcherd  |
| flowers      | Blumen       | fleurs       |               | pappi        |              | husband   | Gatten      | mar         |            | hallottam               | szivem      | secret     | Schulzimmer | Schulzimmer | школе     | kouluun   | Scatcherd  |
| forget       | vergessen    | oublié       | забыл         | pappi        |              | husband   | Gatten      | mar         |            | hallottam               | szivem      | secret     | Schulzimmer | Schulzimmer | школе     | kouluun   | Scatcherd  |
| forgive      | ardon        | pardonne     |               | pappi        |              | husband   | Gatten      | mar         |            | hallottam               | szivem      | secret     | Schulzimmer | Schulzimmer | школе     | kouluun   | Scatcherd  |
| four         | vier         | quatre       | четыре        |              |              |           |             |             |            |                         |             |            |             |             |           |           |            |

Table S5. Statistical dictionary generated from bipartite matching of semantic fingerprints, using Charles Darwin's *Origin of Species*, and its translation into a European language

| (en) English  | (fr) French   | (pl) Polish     | (ru) Russian | (fi) Finnish | (hu) Hungarian       | (en) English   | (fr) French    | (pl) Polish | (ru) Russian  | (fi) Finnish | (hu) Hungarian | (en) English   | (fr) French  | (pl) Polish  | (ru) Russian | (fi) Finnish | (hu) Hungarian |
|---------------|---------------|-----------------|--------------|--------------|----------------------|----------------|----------------|-------------|---------------|--------------|----------------|----------------|--------------|--------------|--------------|--------------|----------------|
| accumulated   | accumulation  |                 |              |              |                      | extent         | reste          |             |               |              |                | order          | ordres       |              |              |              |                |
| acquired      | acquis        |                 |              |              |                      | external       | extérieures    |             |               |              |                | organisation   |              |              |              |              | szervezet      |
| adapted       | adaptation    |                 | адаптация    |              |                      | extinct        | extinctes      |             |               |              |                | Owen           |              |              | Оуэн         | Owen         | Owen           |
| adjoining     |               |                 |              |              | szomszédos           |                |                |             |               |              |                | parallelism    | parallélisme | równoległość |              |              | párhuzam       |
| adult         |               |                 |              |              | ájszike-<br>lityneen | extraordinary  | extraordinaire |             |               |              |                | parts          |              |              |              |              | részek         |
| affinities    | affinités     |                 |              |              |                      | eye            |                |             | szem          |              |                | period         |              |              | periódus     |              |                |
| Africa        | Afrique       | Afrika          | Африка       | Afrikan      | Afrika               | F              |                |             | F             |              |                | perish         | perissent    |              |              |              | galamb         |
| air           |               | powietrze       |              |              |                      | families       | familles       |             | család        |              |                | pigeons        | pigeons      |              | golyócska    |              |                |
| allied        |               | spokrewnione    |              |              |                      | faunas         | faunes         |             | fauna         |              |                | place          | place        |              |              |              |                |
| America       | Amérique      | Amerikai        | Америка      | Amerikan     | Amerikai             | favourable     | favorables     |             |               |              |                | plants         | plantes      |              | растения     |              | sittepolya     |
| analogous     |               | analogiczne     |              |              |                      | feathers       | plumes         |             |               |              |                | pollen         | pollen       |              | porózka      |              | siitepelimistö |
| animals       | animaux       |                 |              |              |                      | females        | féelles        |             |               |              |                | principle      | vertu        |              | принцип      |              | alkuperää      |
| answer        |               |                 | ответ        |              |                      | fertility      | fécondité      |             | plodność      |              |                | probably       |              |              |              |              |                |
| ants          |               |                 | рабочих      |              | dolgozók             | fishes         |                |             | ryb           |              |                |                |              |              |              |              |                |
| archipelago   | archipel      | archipelago     | архипелаг    |              |                      | flight         |                |             |               |              |                | process        | process      |              | процесс      |              | professor      |
| arctic        | arctiques     | strefy          |              |              |                      | flowers        | flours         |             | kwiaty        |              |                | Professor      | professeur   |              | проф         |              | professor      |
| asked         | demande       |                 |              |              |                      | follow         |                |             |               |              |                | progenitor     | ancêtre      |              |              |              | professor      |
| attributed    |               |                 | невероятно   |              |                      | formerly       |                |             | korábban      |              |                | purpose        |              |              |              |              | professor      |
| Australia     |               | Australi        | Австралия    | Australian   | Ausztrália           | forms          |                |             | formák        |              |                | quadrupeds     |              |              |              |              | professor      |
| authors       |               |                 | авторы       |              |                      | fossil         | ossiles        |             | foszlatok     |              |                | range          |              |              |              |              | professor      |
| base          |               |                 | базис        |              |                      | found          | trouvés        |             | találtak      |              |                | reciprocal     |              |              | obustronnyy  |              | professor      |
| bats          | chauves       | ietorperza      | летучих      | erakon       | denevérek            | fresh          | douce          |             | frissen       |              |                | remains        |              |              | открыты      |              | professor      |
| beak          | bec           |                 |              |              |                      | fruit          | fruits         |             | gyümölcs      |              |                | remote         |              |              |              |              | professor      |
| beautiful     | beau          | szép            |              |              |                      | function       | fonctions      |             | funkció       |              |                | resemble       |              |              | reverber     |              | professor      |
| beds          |               |                 |              |              |                      | future         | future         |             | előre         |              |                | reversion      |              |              | reverber     |              | professor      |
| bees          |               | pszczoly        | пчелы        | mehiläiset   | méhek                | Gärtner        | Gärtner        |             | Mézőgazdák    |              |                | rock-pigeon    |              |              | revers       |              | professor      |
| beetles       |               | chrząszcze      | жуки         | bogarak      |                      | genera         | genres         |             | genusok       |              |                |                |              |              |              |              | professor      |
| believe       | croire        |                 |              |              |                      | generally      |                |             | általában     |              |                | rudimentary    |              |              | rudimentar   |              | professor      |
| belonging     | sait          |                 |              |              |                      | geographical   | geographiques  |             | geografikus   |              |                | rule           | régle        |              |              |              | professor      |
| birds         | oiseaux       | ptaków          | птицы        | madarak      |                      | geological     | géologiques    |             | geológiai     |              |                | said           |              |              |              |              | professor      |
| bones         |               |                 |              |              |                      | germinated     | germèrent      |             | prorastali    |              |                | sea            |              |              | meren        |              | professor      |
| botanists     | botanistes    |                 | ботаниками   |              |                      | glacial        | glaciaire      |             | jégkor        |              |                | secondary      |              |              | szekundárius |              | professor      |
| breeds        |               |                 |              |              |                      | gradations     | gradations     |             | lépcsős       |              |                | sediment       |              |              | leületem     |              | professor      |
| Britain       |               | Britanni        |              |              |                      | grafted        | greffe         |             | átültetés     |              |                | selection      |              |              | választás    |              | professor      |
| called        |               | nazywać         |              |              |                      | groups         | groupes        |             | csoporthoz    |              |                | seeds          |              |              | magok        |              | professor      |
| Cambrian      | Cambrienne    | Kambryjskim     |              | Kambrieni    | Kambriumi            | groups         | groupes        |             | csoporthoz    |              |                | separated      |              |              | elválasztás  |              | professor      |
| Candolle      | Candolle      |                 | Декадоло     |              |                      | habits         | habitudes      |             | szokások      |              |                | sexual         |              |              | szexuális    |              | professor      |
| carefully     |               |                 | тщательно    |              |                      | hand           |                |             | kez           |              |                | sexes          |              |              | szex         |              | professor      |
| case          | cause         |                 | случаев      |              |                      | head           |                |             | fej           |              |                | moutons        |              |              | juhok        |              | professor      |
| cattle        |               |                 |              |              |                      | hemisphere     | hémisphère     |             | félsziget     |              |                | courte         |              |              | rövid        |              | professor      |
| cause         |               |                 | причины      |              |                      | hermaphrodites | hermaphrodites |             | hermafroditák |              |                | simple         |              |              | egyszerű     |              | professor      |
| caves         | cellules      | komorok         |              |              |                      | homologous     | homologues     |             | homológusok   |              |                | simultaneously |              |              | szimultán    |              | professor      |
| cells         | centre        |                 | центры       |              |                      | Hooker         | Hooker         |             | Hooker        |              |                | simultaneously |              |              | szimultán    |              | professor      |
| central       |               |                 | центры       |              |                      | Hooker         | Hooker         |             | Hooker        |              |                | simultaneously |              |              | szimultán    |              | professor      |
| certain       | change        |                 | változások   |              |                      | homologous     | homologues     |             | homológusok   |              |                | simultaneously |              |              | szimultán    |              | professor      |
| change        | chapter       | rozdziale       |              |              |                      | Hooker         | Hooker         |             | Hooker        |              |                | simultaneously |              |              | szimultán    |              | professor      |
| chapter       | characters    | cechy           |              |              |                      | Hooker         | Hooker         |             | Hooker        |              |                | simultaneously |              |              | szimultán    |              | professor      |
| characters    | cirripèdes    | wasonogich      |              |              |                      | Hooker         | Hooker         |             | Hooker        |              |                | simultaneously |              |              | szimultán    |              | professor      |
| cirripèdes    |               |                 |              |              |                      | Hooker         | Hooker         |             | Hooker        |              |                | simultaneously |              |              | szimultán    |              | professor      |
| class         | classe        |                 | классы       |              |                      | Hooker         | Hooker         |             | Hooker        |              |                | simultaneously |              |              | szimultán    |              | professor      |
| climate       | climat        | klimate         |              |              |                      | Hooker         | Hooker         |             | Hooker        |              |                | simultaneously |              |              | szimultán    |              | professor      |
| climbing      | grimpanes     |                 | балуны       |              |                      | Hooker         | Hooker         |             | Hooker        |              |                | simultaneously |              |              | szimultán    |              | professor      |
| cold          |               |                 | холодных     |              |                      | Hooker         | Hooker         |             | Hooker        |              |                | simultaneously |              |              | szimultán    |              | professor      |
| colour        |               |                 | краска       |              |                      | Hooker         | Hooker         |             | Hooker        |              |                | simultaneously |              |              | szimultán    |              | professor      |
| compared      |               |                 | конкуренция  |              |                      | Hooker         | Hooker         |             | Hooker        |              |                | simultaneously |              |              | szimultán    |              | professor      |
| competition   |               |                 |              |              |                      | Hooker         | Hooker         |             | Hooker        |              |                | simultaneously |              |              | szimultán    |              | professor      |
| complex       | complexes     |                 |              |              |                      | Hooker         | Hooker         |             | Hooker        |              |                | simultaneously |              |              | szimultán    |              | professor      |
| conditions    | conditions    |                 | условия      |              |                      | Hooker         | Hooker         |             | Hooker        |              |                | simultaneously |              |              | szimultán    |              | professor      |
| continent     | continent     |                 |              |              |                      | Hooker         | Hooker         |             | Hooker        |              |                | simultaneously |              |              | szimultán    |              | professor      |
| correlated    | correlation   | współzależności | корреляция   |              |                      | Hooker         | Hooker         |             | Hooker        |              |                | simultaneously |              |              | szimultán    |              | professor      |
| corresponding | correspondant |                 |              |              |                      | Hooker         | Hooker         |             | Hooker        |              |                | simultaneously |              |              | szimultán    |              | professor      |
| creation      | creation      | stworzenia      |              |              |                      | Hooker         | Hooker         |             | Hooker        |              |                | simultaneously |              |              | szimultán    |              | professor      |
| crossed       |               | krzyżowania     |              |              |                      | Hooker         | Hooker         |             | Hooker        |              |                | simultaneously |              |              | szimultán    |              | professor      |
| crustaceans   |               |                 |              |              |                      | Hooker         | Hooker         |             | Hooker        |              |                | simultaneously |              |              | szimultán    |              | professor      |
| cuckoo        | coucou        | kukule          | кукушки      |              |                      | Hooker         | Hooker         |             | Hooker        |              |                | simultaneously |              |              | szimultán    |              | professor      |
| de            | de            |                 |              |              |                      | Hooker         | Hooker         |             | Hooker        |              |                | simultaneously |              |              | szimultán    |              | professor      |
| depth         | de            |                 |              |              |                      | Hooker         | Hooker         |             | Hooker        |              |                | simultaneously |              |              | szimultán    |              | professor      |
| described     | de            |                 |              |              |                      | Hooker         | Hooker         |             | Hooker        |              |                | simultaneously |              |              | szimultán    |              | professor      |
| developed     | de            |                 |              |              |                      | Hooker         | Hooker         |             | Hooker        |              |                | simultaneously |              |              | szimultán    |              | professor      |
| deviations    | de            |                 |              |              |                      | Hooker         | Hooker         |             | Hooker        |              |                | simultaneously |              |              | szimultán    |              | professor      |
| diagram       | diagram       | схематич        | диаграммы    |              |                      | Hooker         | Hooker         |             | Hooker        |              |                | simultaneously |              |              | szimultán    |              | professor      |
| different     | différent     |                 |              |              |                      | Hooker         | Hooker         |             | Hooker        |              |                | simultaneously |              |              | szimultán    |              | professor      |
| difficulty    | difficulté    |                 | трудности    |              |                      | Hooker         | Hooker         |             | Hooker        |              |                | simultaneously |              |              | szimultán    |              | professor      |
| direct        | direct        |                 |              |              |                      | Hooker         | Hooker         |             | Hooker        |              |                | simultaneously |              |              | szimultán    |              | professor      |
| discovered    | direct        |                 |              |              |                      | Hooker         | Hooker         |             | Hooker        |              |                | simultaneously |              |              | szimultán    |              | professor      |
| dispersal     | direct        |                 |              |              |                      | Hooker         | Hooker         |             | Hooker        |              |                | simultaneously |              |              | szimultán    |              | professor      |
| distinct      | direct        |                 |              |              |                      | Hooker         | Hooker         |             | Hooker        |              |                | simultaneously |              |              | szimultán    |              | professor      |
| disuse        | direct        |                 |              |              |                      | Hooker         | Hooker         |             | Hooker        |              |                | simultaneously |              |              | szimultán    |              | professor      |
| diverse       | direct        |                 |              |              |                      | Hooker         | Hooker         |             | Hooker        |              |                | simultaneously |              |              | szimultán    |              | professor      |
| diversity     | direct        |                 |              |              |                      | Hooker         | Hooker         |             | Hooker        |              |                | simultaneously |              |              | szimultán    |              | professor      |
| division      | direct        |                 |              |              |                      | Hooker         | Hooker         |             | Hooker        |              |                | simultaneously |              |              | szimultán    |              | professor      |
| dogs          | direct        |                 |              |              |                      | Hooker         | Hooker         |             | Hooker        |              |                | simultaneously |              |              | szimultán    |              | professor      |
| domestic      | direct        |                 |              |              |                      | Hooker         | Hooker         |             | Hooker        |              |                | simultaneously |              |              | szimultán    |              | professor      |
| dominant      | direct        |                 |              |              |                      | Hooker         | Hooker         |             | Hooker        |              |                | simultaneously |              |              | szimultán    |              | professor      |
| doubt         | direct        |                 |              |              |                      | Hooker         | Hooker         |             | Hooker        |              |                | simultaneously |              |              | szimultán    |              | professor      |
| Dr            | direct        |                 |              |              |                      | Hooker         | Hooker         |             | Hooker        |              |                | simultaneously |              |              | szimultán    |              | professor      |
| dry           | direct        |                 |              |              |                      | Hooker         | Hooker         |             | Hooker        |              |                | simultaneously |              |              | szimultán    |              | professor      |
| duck          | direct        |                 |              |              |                      | Hooker         | Hooker         |             | Hooker        |              |                | simultaneously |              |              | szimultán    |              | professor      |
| duration      | direct        |                 |              |              |                      | Hooker         | Hooker         |             | Hooker        |              |                | simultaneously |              |              | szimultán    |              | professor      |
| economy       | direct        |                 |              |              |                      | Hooker         | Hooker         |             | Hooker        |              |                | simultaneously |              |              | szimultán    |              | professor      |
| effects       | direct        |                 |              |              |                      | Hooker         | Hooker         |             | Hooker        |              |                | simultaneously |              |              | szimultán    |              | professor      |
| eggs          | direct        |                 |              |              |                      | Hooker         | Hooker         |             | Hooker        |              |                | simultaneously |              |              | szimultán    |              | professor      |
| element       | direct        |                 |              |              |                      | Hooker         | Hooker         |             | Hooker        |              |                | simultaneously |              |              | szimultán    |              | professor      |
| embryo        | direct        |                 |              |              |                      | Hooker         | Hooker         |             | Hooker        |              |                | simultaneously |              |              | szimultán    |              | professor      |
| enemies       | direct        |                 |              |              |                      | Hooker         | Hooker         |             | Hooker        |              |                | simultaneously |              |              | szimultán    |              | professor      |
| equator       | direct        |                 |              |              |                      | Hooker         | Hooker         |             | Hooker        |              |                | simultaneously |              |              | szimultán    |              | professor      |
| Europe        | direct        |                 |              |              |                      | Hooker         | Hooker         |             | Hooker        |              |                | simultaneously |              |              | szimultán    |              | professor      |
| evidence      | direct        |                 |              |              |                      |                |                |             |               |              |                |                |              |              |              |              |                |

Table S6. Statistical dictionaries compiled from *Pride and Prejudice* and its translations into French and Korean, with different thresholds for Ruzička similarities

| (en) English                       | (fr) French   | (en) English                       | (fr) French   | (en) English                       | (ko) Korean        | (en) English                       | (ko) Korean       |
|------------------------------------|---------------|------------------------------------|---------------|------------------------------------|--------------------|------------------------------------|-------------------|
| $s_R(v_i^{en}, v_j^{fr}) \geq 0.7$ | $\geq 0$      | $s_R(v_i^{en}, v_j^{fr}) \geq 0.7$ | $\geq 0$      | $s_R(v_i^{en}, v_j^{ko}) \geq 0.7$ | $\geq 0$           | $s_R(v_i^{en}, v_j^{ko}) \geq 0.7$ | $\geq 0$          |
| absence                            | absence       | absence                            | Lucas         | amiable                            | 상냥한                | Jane                               | 제인(Jane)이         |
| aunt                               | tante         | Lydia                              | Lucas         | arrival                            | 도착(到着)한            | Kitty                              | 키티(Kitty)가        |
| ball                               | bal           | Lydia                              | Lucas         | aunt                               | 숙모(叔母)가            | laugh                              | 웃음                |
| Bennet                             | Bennet        | Mary                               | Mary          | ball                               | 무도회(舞臺會)에          | lighy                              | 서재(書齋)로           |
| Bingley                            | Bingley       | master                             | Meryton       | Bennet                             | 베넷(Bennet)         | Lizzy                              | 리지(Lizzy)아        |
| Bourgh                             | Bourgh        | Meryton                            | Meryton       | Bingley                            | 빙리(Bingley)        | long                               | 고 장어              |
| Brighton                           | Brighton      | Miss                               | Miss          | book                               | 책(冊)을              | love                               | 사랑하는              |
| brother                            | frère         | mother                             | mère          | Bourgh                             | 드(de)              | Lucas                              | 루카스(Lucas)        |
| carriage                           | voiture       | motive                             | motif         | Brighton                           | 브라이톤(Brighton)에    | marriage                           | 결혼(結婚)을           |
| Catherine                          | Catherine     | Mr                                 | Mr            | brother                            | 오빠가                | Mary                               | 메리(Mary)는         |
| Charlotte                          | Charlotte     | Mrs                                | Mrs           | carriage                           | 마차(馬車)를            | Meryton                            | 메리(Mary)턴에        |
| children                           | enfants       | nephew                             | neveu         | Catherine                          | 캐서린(Catherine)     | Miss                               | 미스(嬢)이            |
| Collins                            | Collins       | Netherfield                        | Netherfield   | Charlotte                          | 샬럿(Charlotte)이     | money                              | 돈을                |
| colonel                            | colonel       | niece                              | niece         | Collins                            | 콜린스(Collins)       | mother                             | 어머니가              |
| congratulations                    | félicitations | officers                           | officiers     | colonel                            | 대령(大領)이            | Mr                                 | 씨(氏)가             |
| cousin                             | cousin        | park                               | parc          | come                               | 오느                 | Mrs                                | 부인(夫人)은           |
| cried                              | écria         | Pemberley                          | Pemberley     | congratulations                    | 축하(祝賀)해            | neighborhood                       | 이웃                |
| dance                              | danser        | Phillips                           | Phillips      | cousin                             | 사촌(四寸)             | Netherfield                        | 네더필드(Netherfield) |
| Darcy                              | Darcy         | politeness                         | politesse     | dance                              | 춤                  | officers                           | 장교(將校)들           |
| dear                               | chère         | poor                               | pauvre        | Darcy                              | 다시(Darcy)          | oh                                 | 아                 |
| Derbyshire                         | Derbyshire    | promised                           | promesse      | daughter                           | 딸                  | Pemberley                          | 캠벌리(Pemberley)에   |
| dinner                             | dîner         | refus                              | refus         | day                                | 시간(時間)을            | Phillips                           | 필립스(Phillips)     |
| distance                           | distance      | regiment                           | régiment      | de                                 | 버그(Bourgh)         | pounds                             | 파운드(鎊)            |
| Elizabeth                          | Elizabeth     | Rosings                            | Rosings       | Derbyshire                         | 디버셔(Derbyshire)에   | pretty                             | 예쁜                |
| evening                            | soir          | said                               | dit           | disappointment                     | 실망(失望)을            | promised                           | 약속(約束)을           |
| eyes                               | yeux          | send                               | envoyer       | door                               | 문(門)을              | read                               | 읽어                |
| father                             | père          | Sir                                | sir           | elegant                            | 우아(優雅)한            | refuse                             | 거절(拒絕)하는          |
| felt                               | sentiments    | society                            | société       | estate                             | 상속(相続)에            | regiment                           | 연대(聯隊)가           |
| Fitzwilliam                        | Fitzwilliam   | stranger                           | étranger      | eyes                               | 외초(微笑)를            | resolved                           | 결심(決心)을           |
| Forster                            | Forster       | table                              | table         | father                             | 아버지가               | room                               | 방(房)을             |
| fortune                            | fortune       | ten                                | dix           | fear                               | 두려워서               | Rosings                            | 로징스(Rosings)에서    |
| Gardiner                           | Gardiner      | thank                              | remerciements | Fitzwilliam                        | 피츠윌리엄(Fitzwilliam) | sat                                | 앉아                |
| good                               | mieux         | thousand                           | mille         | five                               | 다섯                 | serious                            | 진지(眞摯)하게          |
| Hurst                              | Hurst         | town                               | Londres       | forget                             | 잊지                 | servant                            | 하인(下人)이           |
| husband                            | mari          | two                                | deux          | Forster                            | 포스터(Forster)       | Sir                                | 경(卿)이             |
| ignorant                           | ignore        | uncle                              | oncle         | Gardiner                           | 가디너(Gardiner)      | thousand                           | 파운드(pound)를       |
| impossible                         | impossible    | visit                              | visite        | gentlemen                          | 신사(紳士)들이           | uncle                              | 숙부(叔父)와           |
| invitation                         | invitation    | way                                | voie          | happy                              | 행복(幸福)한            | vain                               | 허영심(虛榮心)을         |
| Jane                               | Jane          | week                               | semaine       | Hurst                              | 허스트(Hurst)         | visit                              | 방문(訪問)을           |
| Kitty                              | Kitty         | Wickham                            | Wickham       | husband                            | 남편(男便)이            | Wickham                            | 윌킴(Wickham)       |
| lady                               | lady          | write                              | écrire        | inquiries                          | 물었다                | wife                               | 아내가               |
| laugh                              | rire          | years                              | ans           | introduction                       | 소개(紹介)해            | William                            | 윌리엄(William)      |
| letter                             | lettre        | young                              | jeune         | invitation                         | 초대(招待)를            | young                              | 젊은                |

## 1.4 Automated question answering based on Markov semantics

When we are given a document (of moderate length) and a natural language question as input, we rate and rank the sentences within the document by their relevance to the question, containing topical patterns  $\mathcal{Q} = \{W_{q_1}, \dots, W_{q_K}\}$ . We expand the query into  $\mathcal{Q} \cup \mathcal{Q}'$ , a union of semantic cliques:  $\mathcal{Q} \cup \mathcal{Q}' = \bigcup_{k=1}^K \mathcal{S}_{q_k}$ . We build a localized Markov matrix  $\mathbf{P} = (p_{ij})_{1 \leq i, j \leq N}$  on  $\mathcal{Q} \cup \mathcal{Q}'$ . We further use the Brin–Page damping [15] to form an ergodic Markov matrix  $\tilde{\mathbf{P}} = (\tilde{p}_{ij})_{1 \leq i, j \leq N}$ , where  $\tilde{p}_{ij} = 0.85p_{ij} + \frac{0.15}{N}$ .

If our question  $Q$  contains words from  $W_{Q_1}, \dots, W_{Q_m} \in \mathcal{Q}$  and a candidate answer  $A$  contains words  $W_{A_1}, \dots, W_{A_n} \in \mathcal{Q} \cup \mathcal{Q}'$  (counting multiplicities, but excluding function words and patterns with fewer than 3 occurrences in the reference document), then we assign the following entropy production score [1, (11) and Footnote 4]

$$\mathcal{F}[Q, A] := - \sum_{i=1}^m \sum_{j=1}^n \tilde{\pi}_{Q_i} \tilde{p}_{Q_i A_j} \log \tilde{p}_{Q_i A_j} \quad (1.14)$$

to this question-answer pair.

In [1, Fig. 7a,b], we test our Markov language model on the WikiQA dataset. The distribution of average precisions (AP) and reciprocal ranks (RR) for individual questions in the WikiQA dataset is summarized in Fig. S2. One may wish to check Tables S11–S12 in §4 and see how our algorithm performs on each of the 1242 questions.

## 2 What our software does not

### 2.1 Non-universal statistics on short time scales

As recapitulated in §1.1, we reject text fragments shorter than or equal to the lengths of the flanking words. This is because we find such short-range features highly sensitive to grammatical rules that are specific to certain languages, thus lacking universality.

In [1, Footnote 2], we have already alluded to the highly versatile reduplications (or lack of) in different languages: German *liebe Studentinnen und Studenten* “dear (female and male) students”, Malay *orang-orang* “people” (vs. *orang* “person”), and Hawaiian *wiki wiki* “very quick” (vs. *wiki* “quick”). We choose to ignore such short-range recurrence statistics in our current study, which are typically not transferrable across languages and cultures.

The numerical instability of short-range textual features can be further illustrated by a comparison of Turkish and English morphemes (adapted from [17, p. 61]):

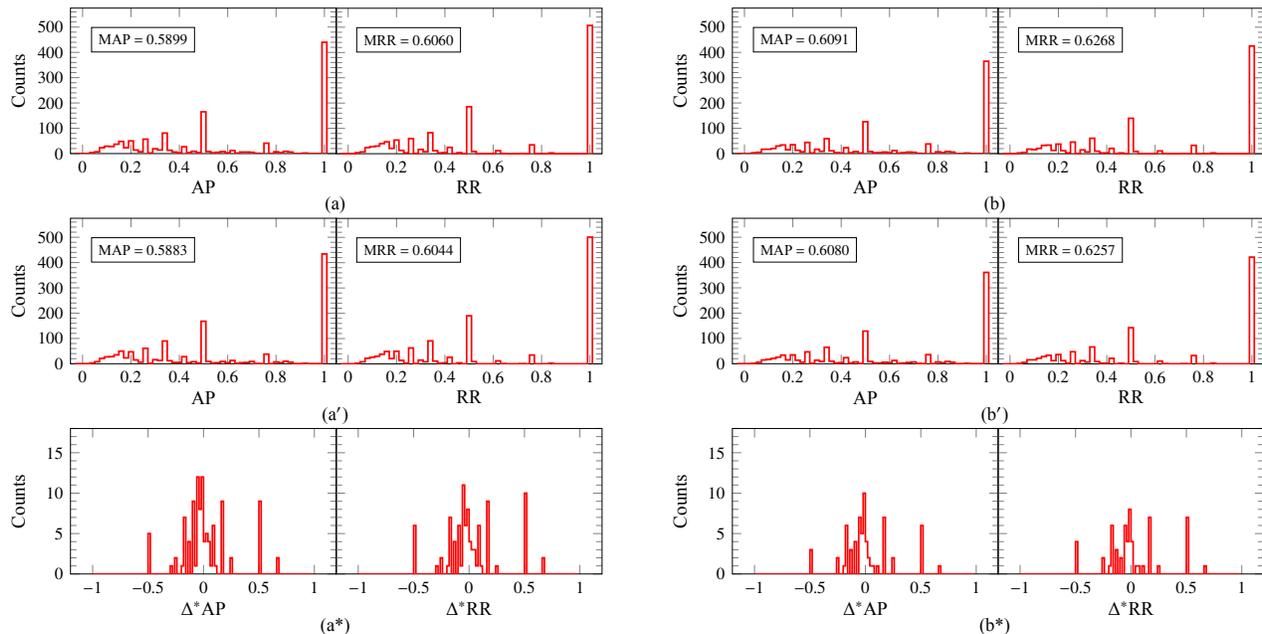

Fig. S2. Score distributions in WikiQA tests. (a) Test results on 1242 answerable questions the WikiQA dataset: histograms for average precisions (AP) and reciprocal ranks (RR) of correct answers, with their respective means displayed as *inset*. Tied scores are resolved by the McSherry–Najork algorithm [14], which effectively averages AP and RR over all possible permutations of tied entries. (b) Test results on a subset of 990 WikiQA questions (see Algorithm 3.12 in §3 for detailed screening criteria) that do not require logic inference beyond associative reasoning. (The Brin–Page damping factor 0.85 [15] is used in both panels a and b.) (a′)–(b′) Control experiments using the Bressan–Peserico damping factor 0.5 [16]. (a\*)–(b\*), Non-zero differences between Brin–Page and Bressan–Peserico values (upper panel minus lower panel).

Avrupaılaŝtırlamayacaklardansınız

You (all) are among those who will not be able to be caused to become Europeanized  $\approx$  You (all) are among those who will not be made Europeanizable

Here, in both languages, the relevance of a morpheme roughly decays monotonically with respect to the distance from the central morpheme (Avrupa/Europe). The distance correspondence is generally stabler for larger separations, but is highly unstable when we count distances between nearest (or next-to-nearest) neighboring morphemes.

Table S7. Length/time scales in natural language processing (NLP)

| Scale       | Friederici’s hierarchy [18] | Jakobson’s metaphor        | Rôle in NLP         | Evolutionary susceptibility                |
|-------------|-----------------------------|----------------------------|---------------------|--------------------------------------------|
| short-range | phonological level          | “elementary particle” [19] | acoustic encoding   | climatic/environmental [20, 21, 22]        |
|             | lexical level               | “atom”                     | concept tagging     | cognitive/cultural/social [23, 24, 25, 26] |
|             | sentence level              | “molecule”                 | syntactic computing | cognitive/cultural/social [23, 24, 25, 26] |
| ↓           |                             |                            |                     |                                            |
| long-range  | text/discourse level        | “bulk material”            | semantic processing | —                                          |

In our current work, we mainly concern ourselves with theories and applications for the recurrence statistics of word patterns that exhibit universal behavior, with a focus on semantic processing [27] rather than syntactic computation [28]. Practically, this means that we will suppress the fine structures in the three short scales in Friederici’s hierarchy (Table S7), which vary by language typology. Similar exclusions of short-range word contacts are also implemented in the  $n$ -gram language model of Brown *et al.* [29].

## 2.2 Word disambiguation and stylistic adaptability

In theory, we expect that each Markov state corresponds to exactly one concept (a family of words that are related to each other by inflection and derivation). In practice, there are homographs (words with the identical spelling but unrelated meanings), whose denotations must be resolved through careful examination of context (either by experienced human readers, or by sophisticated algorithms in supervised learning). In numerical implementations of our model, we do not make any attempt to solve the polysemy puzzle, so we do run the risk of conflating homographs into one Markov state. In languages like Danish and Dutch, this conflation is serious enough to affect the performance of certain computational tasks related to the following

Table S8. Parallel versions for a conversation in Chapter 1 of *Pride and Prejudice*

| English                                                                                                            | French                                                                                                        | Russian                                                                                                                                              | Finnish                                                                                                                                                                 |
|--------------------------------------------------------------------------------------------------------------------|---------------------------------------------------------------------------------------------------------------|------------------------------------------------------------------------------------------------------------------------------------------------------|-------------------------------------------------------------------------------------------------------------------------------------------------------------------------|
| “My dear Mr. Bennet,” <u>said his lady to him one day</u> , “have you heard that Netherfield Park is let at last?” | — Savez-vous, mon cher ami, <u>dit un jour Mrs. Bennet à son mari</u> , que Netherfield Park est enfin loué ? | — Дорогой мистер Беннет, — <u>сказала как-то раз миссис Беннет своему мужу</u> , — слышали вы, что Незерфилд-парк наконец больше не будет пустовать? | “Rakas Bennet”, <u>sanoi tämän arvon herran puolisio miehelleen eräänä päivänä</u> , “oletko kuullut, että Netherfield Parkin kartano on vihdoinkin saanut vuokraajan?” |
| Mr. Bennet replied that he <b>had not</b> .                                                                        | <b>L’ignorait.</b>                                                                                            | Мистер Беннет ответил, что он этого <b>не слышал</b> .                                                                                               | Hra Bennet vastasi, ettei hän <b>ollut kuullut</b> .                                                                                                                    |

Notes:

(1) See Table S1 for provenances.

(2) The underlined texts are roughly equivalent across four versions; the same can be said for the texts in **boldface**.Table S9. Parallel translations of the opening line in *Pride and Prejudice*

| German<br>(Werner Beyer)                                                                                                                    | (Christian Grawe & Ursula Grawe)                                                                                                                                       | (Karin von Schwab)                                                                                                                                                         |
|---------------------------------------------------------------------------------------------------------------------------------------------|------------------------------------------------------------------------------------------------------------------------------------------------------------------------|----------------------------------------------------------------------------------------------------------------------------------------------------------------------------|
| In der ganzen Welt gilt es als ausgemachte Wahrheit, daß ein begüterter Junggeselle unbedingt nach <b>einer Frau</b> Ausschau halten muß.   | Es ist eine allgemein anerkannte Tatsache, dass ein alleinstehender Mann im Besitz eines hübschen Vermögens angeblich nichts dringender braucht als <b>eine Frau</b> . | Es ist eine Wahrheit, über die sich alle Welt einig ist, daß ein unbeweibter Mann von einigem Vermögen unbedingt auf der Suche nach <b>einer Lebensgefährtin</b> sein muß. |
| Spanish<br>(Ana M. Rodríguez)                                                                                                               | (José de Urries y Azara)                                                                                                                                               | (Marciano Guerrero)                                                                                                                                                        |
| Es una verdad reconocida por todo el mundo que un soltero dueño de una gran fortuna siente un día u otro la necesidad de <b>una mujer</b> . | Es verdad universalmente admitida que un soltero poseedor de buena fortuna tiene que necesitar <b>una mujer</b> .                                                      | Es una verdad mundialmente reconocida que un hombre soltero y poseedor de una buena fortuna, debe estar en busca de <b>una esposa</b> .                                    |

Notes:

(1) See Table S1 for provenances.

(2) The underlined texts are roughly equivalent across four versions; the same can be said for the texts in **boldface**.(common but ambiguous) words:<sup>13</sup>

| Dutch        | English gloss                  | (German cognate)                   | Danish     | English gloss                                                      |
|--------------|--------------------------------|------------------------------------|------------|--------------------------------------------------------------------|
| <i>meer</i>  | { <i>more</i><br><i>lake</i>   | ( <i>mehr</i> )<br>( <i>Meer</i> ) | <i>så</i>  | { <i>saw</i> (past of <i>see</i> )<br><i>so</i><br>(to) <i>sow</i> |
| <i>vroeg</i> | { <i>asked</i><br><i>early</i> | ( <i>frug</i> )<br>( <i>früh</i> ) | <i>ved</i> | { <i>at</i><br><i>knows</i><br><i>wood</i>                         |

We refer our readers to §9.2 for a discussion of homographs in Korean.

Besides homographs, there are three more subtler noise sources that may negatively impact the translational invariance of the Markov spectrum, hence our automated word translation via cross-lingual matching of semantic fingerprints.

The first kind of noise is attributed to free variations of translators (Tables S8 and S9). As shown in Table S8, translators may take the liberty of using free (as opposed to literal) interpretations: the underlined texts in the three translations essentially read “Mrs. Bennet said to her husband one day”, which paraphrases the interpersonal relationship expressed in the original English text; the bold texts in the three translations all explicitly supply the negated verb (“had not known”/“had not heard”), which is omitted in the English original. In Table S9, all the underlined texts correspond to “a truth universally acknowledged” in the English original and all the phrases in boldface mean “a wife”, despite nuances in their wording and phrasing.

The second kind of noise is due to algorithmic imperfection in morphological classifications of words into word patterns. There are irregularities in word morphologies that cannot be fully covered by our automated word clustering algorithms described in Part III. Furthermore, the heterogeneous etymological origins<sup>14</sup> of the English language may bring us additional challenges. For example, our programs do not recognize *heart* and *cordial* as morphologically related in English, even though their German or Hungarian translations display such relationship manifestly:

| English                    | German          | Hungarian       |
|----------------------------|-----------------|-----------------|
| <i>heart</i>               | <i>Herz</i>     | <i>szív</i>     |
| <i>hearty, cordial</i>     | <i>herzlich</i> | <i>szíves</i>   |
| <i>heartily, cordially</i> | <i>herzlich</i> | <i>szívesen</i> |

The third kind of noise is due to our insufficient treatment of space, time and causality in the lexico semantics of verbs (see [30, Chap. 4] or [31, Chap. 5]). For the time being, we have swept all prepositions (which are vital to the space component of verbs) into the class of function words, and have ignored them in our text mining tasks. Thus, our numerical translation algorithm cannot handle polysemic verbs like *go*, *make*, *take*, *turn*, whose meanings are best clarified by subsequent prepositions<sup>13</sup>In modern German, *Meer* means “sea”. In archaic German, *Meer* means “lake”. In modern German, the strong conjugation *frug* for first- or third-person singular preterite is rare, while the weak conjugation *fragte* is common. We have included these German cognates, to serve as visual aids to their Dutch counterparts.<sup>14</sup>English lexicon possesses a native Germanic stock (exemplified by *hearty*, *heartily* and so forth), but is simultaneously under strong Latinate influence (shown in near-synonyms of the aforementioned words *cordial*, *cordially*), via Norman French. A more challenging scenario appears in Korean word families with disparate (Chinese/English/Korean) origins. See §9.2 for a discussion.

(if present). We have chosen to ignore prepositions (in either isolated form or as separable prefixes<sup>15</sup>) in our numerical text analysis, because they do not exhibit universal behavior, in at least two senses: (1) Short-range relations between verbs and prepositions (like *takes up*) in English may translate into long-range relations in certain Germanic languages (like *nimmt ... auf* in German and *neemt ... op* in Dutch, where the written space occupied by the ellipsis can be arbitrarily long). (2) The rôles of locative prepositions (like *on*, *in* and *from*) are largely subsumed by certain case endings in Uralic languages (such as Finnish and Hungarian). In our work, we not only ignore prepositions, but also strip away case endings in a stemming procedure (Part III). We believe that such simultaneous treatments of prepositions and case endings are consistent: they generate similar levels of coarse-graining in words across different language families. In addition to neglecting prepositions, we have designed our stemming procedure so as to merge verb forms in different tenses and aspects (time component), but it may also conflate causative and non-causative forms (causality component), in a fashion that is not necessarily consistent across all languages. For example, our stemming algorithm treats Finnish *syödä*/Korean 먹다 “(to) eat” (non-causative) and Finnish *syöttää*/Korean 먹이다 “(to) feed” (causative) as the same verb in their respective language, but not so for their English counterparts.

The language-specific usage of function words is another practical hindrance to lossless translation, but this hindrance does not contribute to our Markov spectrum (if we can ignore effects from pronominal coreferences, as discussed below) for content words. As a glance of the highly diverse typologies of function words found in different languages, we say a few more words about the gender agreement of pronouns. All the 8 modern Indo-European languages under our consideration in Part III distinguish “he” from “she” when referring to humans as subjects in a sentence, while the 5 non-Indo-European languages do not.<sup>16</sup> Gender agreement of possessive pronouns is a subtler issue for Indo-European languages. Expanding the example given by Willim and Chomsky [32, p. 100], we have

|          |                                                    |                                                   |
|----------|----------------------------------------------------|---------------------------------------------------|
| English: | <i>John told Mary about his father.</i>            | <i>John told Mary about her father.</i>           |
| French:  | <i>Jean a parlé de son père à Marie.</i>           | <i>Jean a parlé de son père à Marie.</i>          |
| German:  | <i>Johann hat Maria von seinem Vater erzählt.</i>  | <i>Johann hat Maria von ihrem Vater erzählt.</i>  |
| Polish:  | <i>Jan opowiadał Marii o swoim ojcu.</i>           | <i>Jan opowiadał Marii o jej ojcu.</i>            |
| English: | <i>John told Mary about his mother.</i>            | <i>John told Mary about her mother.</i>           |
| French:  | <i>Jean a parlé de sa mère à Marie.</i>            | <i>Jean a parlé de sa mère à Marie.</i>           |
| German:  | <i>Johann hat Maria von seiner Mutter erzählt.</i> | <i>Johann hat Maria von ihrer Mutter erzählt.</i> |
| Polish:  | <i>Jan opowiadał Marii o swojej matce.</i>         | <i>Jan opowiadał Marii o jej matce.</i>           |

Here, the pronouns *his*, *her*, *seinem*, *seiner*, *ihrem*, *ihrer* and *jej* agree with the gender of the possessor; meanwhile the pronouns *son*, *sa*, *seinem*, *seiner*, *ihrem*, *ihrer*, *swoim* and *swojej* agree with the gender of the possessed. Automated resolution of such agreements is beyond the scope of our current research, as this language-specific problem occurs on a different neuro-linguistic scale from that of our concern. However, if pronominal coreferences become ambiguous enough after literal translation, then the translator might choose to supply personal names in place of pronouns, and such rephrasing may partly affect the performance of our Markov algorithms. (See Example 4.15.2 and Fig. S3e.)

### 2.3 Causal inference and deductive reasoning

Admittedly, our semantic cliques (see [1, §2.3.2] and §1.2 above) have some limitations. At relatively low computational cost, our criterion for semantic dependence [see (1.5)] does not distinguish between causal [33, 34] and non-causal relations, nor does it generate semantic webs with hierarchical topologies [35, 36]. For comprehension tasks requiring high-precision causal inference and relationship mining, Bayesian networks [33, 34] and persistent homologies [35, 36] offer more reliable guidance than our approach.

The lack of causal inference and deductive reasoning in our question-answering machine places a cap on its MAP and MRR scores ([1, Fig. 7b] and Fig. S2). No matter how we improve the stemming/clustering algorithms for English (§4), there are certain fractions of WikiQA questions that our method cannot handle properly (Table S12). Typical failures include, but are not limited to the following categories (see Table S10 for evaluations of our performance):

- Our semantic cliques do not always enable us to address causation questions (like *What causes ...?*) correctly, with only about a fifty-fifty chance of hitting the right answer. These cliques indicate association and connection between concepts, which may or may not be of causal nature.
- Our semantic cliques do not automatically sieve answers with numbers (spelt out in English or Arabic numerals), even if the question (such as *How big ...? How long ...? How many ...? How old ...? What year ...?*) elicits one. Perhaps

<sup>15</sup>For example, the prefixes (*ab/af*, *auf/op*, and *zu/toe*) in German *abnehmen*/Dutch *afnemen* “(to) decrease”, German *aufnehmen*/Dutch *opnemen* “(to) take up”, and German *zunehmen*/Dutch *toenemen* “(to) increase” must be separated from the verb stems in certain conjugated forms. Note however, that the prefixes in English words “decrease” and “increase” are not separable as prepositions.

<sup>16</sup>In some rare circumstances, the lack of gender-specific pronouns may also hamper topic analysis in our numerical experiments. (See Example 4.15.2 and Fig. S3e.)

Table S10. Distributions of hits and misses in certain types of questions in our WikiQA experiments

| Question type              | #Hits | #Misses | Question type                | #Hits | #Misses |
|----------------------------|-------|---------|------------------------------|-------|---------|
| <i>What caused ...?</i>    | 1     | 1       | <i>How much ...?</i>         | 5     | 9       |
| <i>What causes ...?</i>    | 4     | 4       | <i>How often ...?</i>        | 0     | 2       |
| <i>What is caused ...?</i> | 1     | 0       | <i>How old ...?</i>          | 4     | 5       |
| <i>How big ...?</i>        | 0     | 2       | <i>What became of ...?</i>   | 0     | 1       |
| <i>How deep ...?</i>       | 0     | 1       | <i>What happened to ...?</i> | 0     | 4       |
| <i>How long ...?</i>       | 3     | 5       | <i>What year ...?</i>        | 7     | 14      |
| <i>How many ...?</i>       | 19    | 51      | <i>When ...?</i>             | 46    | 67      |

the statistical behavior of recurring numbers in a text document does not neatly fit into our Markov model for word patterns, so the semantic cliques do not easily detect numbers as synonyms to certain question words.

- Our semantic cliques stumble over questions that ask for superlatives, either explicitly or implicitly. Some of these questions (*What became of...? What happened to ...?*) can be very subtle, as they require finding the most recent date out of a list, going beyond the reach of our Markov model.

## Part II

# Protocols for text cleansing

After a brief summary of notations (§3.1), we present in this Part cleansing protocols for certain articles in the the English Wikipedia (§3.2) and electronic books written in 14 languages spoken in Europe and Asia (§3.3), in preparation for word clustering and word translation experiments in Part III.

Hereafter in Parts II and III, aside from English (§4), we pick Danish, German and Dutch as representative Germanic languages (§5); Spanish, French and Latin<sup>17</sup> as representative Romance languages (§6); Polish and Russian as representative Slavic languages (§7); Finnish and Hungarian as representative Uralic languages (§8); Basque, Korean and Turkish as representatives from various other language families (§9). A putative evolutionary history of these languages is sketched below:

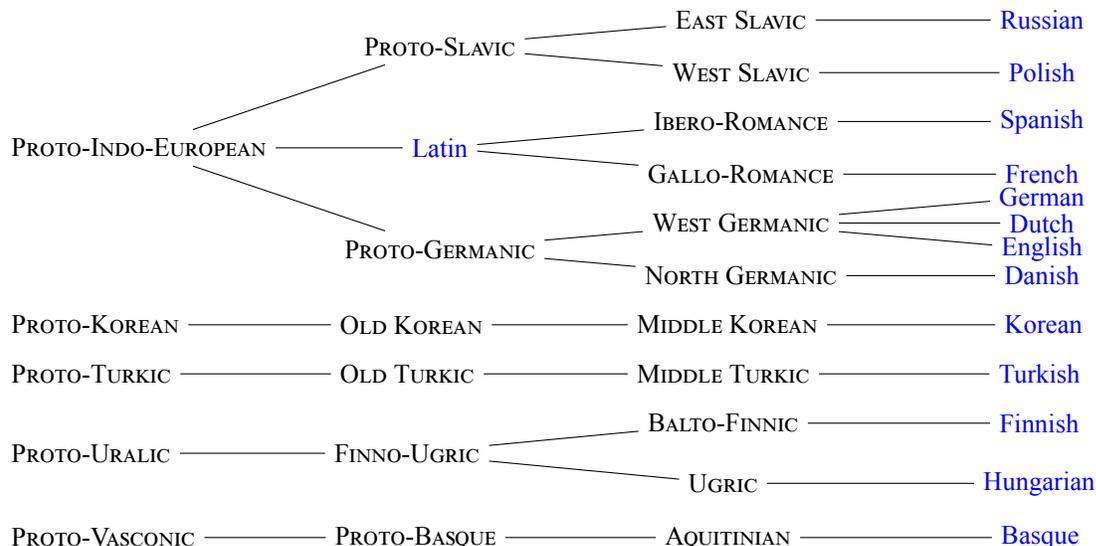

From now on, the languages other than English are first sorted alphabetically according to their genealogical affiliation (Germanic, Romance, Slavic, Uralic, “Various”), and then sorted within their respective affiliation according to their ISO codes [e.g. Spanish (es) precedes French (fr)]<sup>18</sup>.

All these Asian and European languages under investigation have clearly defined word boundaries (typically marked by spaces and punctuation marks, and additionally by apostrophes and hyphens in the case of French) and rich word morphologies

<sup>17</sup>Strictly speaking, Latin is not a Romance language, but an ancestor to all the modern Romance languages. Since a modern Romance language, Romanian, still shares a lot of conservative features with Latin, it may not hurt to label Latin as a Romance language.

<sup>18</sup>The individual sections from §5 to §9 can be read in any order, depending on need. To help our readers navigate through these protocols, we have reproduced certain explanatory texts from one section to another.

(e.g. adjective comparisons, noun declensions and verb conjugations). Inspired by the sequence alignment procedure [37, 38] in bioinformatics, we devise algorithms that employ string matching to find affinity between words, with a limited amount of input for grammatical rules.

The Germanic, Romance and Slavic languages all belong to the Indo-European family, which distinguishes from the other language families under consideration, both lexically and syntactically. The languages within the same affiliation share a lot of common features in vocabulary and syntax. We note however that English, though officially a Germanic language, has borrowed extensively from Latin and (Norman) French, so it has blended characteristics of both Germanic and Romance subgroups. In the light of this, we have singled out the algorithmic treatment of English texts in §4.

Our word clustering algorithms are based on Porter stemming [39, 40], along with extensive additions that accommodate to irregularities in word morphologies. Since regular and irregular word morphologies are handled by different neurobiological mechanisms in the human brain [41, 42], we are not going to unify their treatment under a single algorithmic framework. Regular morphologies will be identified by substitution rules (as in Porter stemming), while irregular morphologies in each language will be accommodated by a finite (though sometimes long) list of exceptions. It has been observed that grammatical irregularities tend to be associated with highly common words [43]: the frequent uses of these words make their peculiarities harder to be forgotten. It is our hope that, via many explicitly coded “exceptions to general rules”, we can achieve higher precision in text mining tasks related to those highly frequent yet highly irregular words.

### 3 String manipulations and text normalizations

#### 3.1 Notational conventions

In the source codes accompanying this work, we have implemented our text mining algorithms in *Mathematica* (including both the cleansing procedures in Part II and the clustering procedures in Part III). However, we hope that readers of this document could easily adapt our algorithms to other programming languages. Towards this end, we will present our methods of text processing using some standard notations in linguistic analysis (applicable to both Parts II and III), as declared below.

**Definition 3.1** (String length). The length of a text string  $\hat{\sigma}$  is a non-negative integer that equals the number of Unicode characters used to write out the string, denoted by  $\ell(\hat{\sigma})$ .

The empty string  $\emptyset$  (not to be confused the Danish letter  $\emptyset/\emptyset$ ) is the only text string with length zero:  $\ell(\emptyset) = 0$ .

For a positive integer  $n$  less than or equal to  $\ell(\hat{\sigma})$ , the  $n$ th position in string  $\hat{\sigma}$  is denoted by  $\hat{\sigma}^{[n]}$ , and the first  $n$  characters in string  $\hat{\sigma}$  is denoted by  $\hat{\sigma}^{[n]}$ . For a non-empty string  $\hat{\sigma}$ , its “first character” is  $\hat{\sigma}^{[1]}$  and its “last character” is  $\hat{\sigma}^{[\ell(\hat{\sigma})]}$ . For the empty string, its “first character” and “last character” are both defined as the empty string. In general, the last character of a string  $\hat{\sigma}$  is denoted by  $\Omega(\hat{\sigma})$ .

The notation  $\hat{\sigma}^{-1}$  stands for the reverse of the string  $\hat{\sigma}$ . In particular, we have  $\emptyset^{-1} = \emptyset$ ; when  $\ell(\hat{\sigma}) > 0$ , we have  $(\hat{\sigma}^{-1})^{[n]} = \hat{\sigma}^{[\ell(\hat{\sigma})+1-n]}$  for all integers in the range  $1 \leq n \leq \ell(\hat{\sigma})$ .  $\square$

**Definition 3.2** (String spelling and string alternatives). For all the languages written in either the Latin or the Cyrillic script, letters (including apostrophes and hyphens) within a text string in an algorithm is always spelt out in slant typeface, such as *word* (English) and *слово* (Russian). Boxed characters set in the typewriter typeface are taken verbatim. A boxed expression in red, in the form of U+xxxx, refers to the Unicode character with hexadecimal code xxxx. The expression  $\hat{\sigma}^+$  (resp.  $\hat{\sigma}_-$ ) results from converting  $\hat{\sigma}$  to upper (resp. lower) case.

The notation for “alternatives”  $\hat{\sigma}_1 | \dots | \hat{\sigma}_n$  refers to an arbitrary text string in the set  $\{\hat{\sigma}_1, \dots, \hat{\sigma}_n\}$ . Parentheses in string spellings, usually in the form of  $\hat{\sigma}(\hat{\sigma}_1 | \dots | \hat{\sigma}_n)$ , are used to enclose alternative portions that are not shared by a group of words.

The rules above also apply to algorithms for the Korean language, except that slant typefaces will not be used, and the native Korean alphabet does not distinguish upper and lower cases.  $\square$

*Example 3.2.1.* The boxed pattern , is interpreted literally, as a comma followed by a white space. The pattern (a|b) is a concatenation of five Unicode characters, while  $(a|b)$  refers to either member of the set  $\{a, b\}$ .

*Example 3.2.2.* For English, the string pattern  $word(\emptyset|s|s's')$  refers to any text string in the set  $\{word, words, word's, words'\}$ . For Russian, the string pattern  $слово(o|a|\emptyset)$  refers to any text string in the set  $\{слово, слова, слов\}$ . The expression  $(word(\emptyset|s|s's'))^+$  has the same effect as  $WORD(\emptyset|S|'S'S')$ , while  $((CJOB(O|A|\emptyset))_-)$  is equivalent to  $слов(o|a|\emptyset)$ .

**Definition 3.3** (Multiple occurrences of string patterns). For a string pattern  $(\hat{\sigma}_1 | \dots | \hat{\sigma}_n)$ , the notation  $(\hat{\sigma}_1 | \dots | \hat{\sigma}_n)_m$  (resp.  $(\hat{\sigma}_1 | \dots | \hat{\sigma}_n)_{m_0}$ ) denotes one (resp. zero) or more successive occurrences of the same pattern in a text string, and the notation  $(\hat{\sigma}_1 | \dots | \hat{\sigma}_n)_{[n_1, n_2]}$  refers to between  $n_1$  and  $n_2$  (inclusive) consecutive appearances of the pattern  $(\hat{\sigma}_1 | \dots | \hat{\sigma}_n)$ .<sup>19</sup> When  $v = n_1 = n_2$ , we also write  $(\hat{\sigma}_1 | \dots | \hat{\sigma}_n)_{[v, v]}$  as  $(\hat{\sigma}_1 | \dots | \hat{\sigma}_n)_{\times v}$ , to denote exactly  $v$  repeats of the pattern  $(\hat{\sigma}_1 | \dots | \hat{\sigma}_n)$ .  $\square$

<sup>19</sup>In *Mathematica* codes,  $(\hat{\sigma})_m$  is represented by  $(\sigma) \dots$  or `Repeated[ $\sigma$ ]`,  $(\hat{\sigma})_{m_0}$  by  $(\sigma) \dots$  or `RepeatedNull[ $\sigma$ ]`, and  $(\hat{\sigma})_{[n_1, n_2]}$  by `Repeated[ $\sigma$ , {n1, n2}]`.

*Example 3.3.1.* The pattern  $(d|e)_m$  may be matched by strings  $d, e, dd, de, ed, ee, ddd, dde, ded, dee, edd, ede, eed, eee$  and so on. If we consider the pattern  $(d|e)_{m_0}$ , then the empty string  $\emptyset$  also forms a match. The pattern  $(d|e)_{[0,2]}$  is only matched by the strings  $\emptyset, d, e, dd, de, ed, ee$ .

**Definition 3.4** (Wildcard symbols). We write  $\mathbf{X}$  for a generic text string of zero or positive length. At times, we may restrict  $\mathbf{X}$  to a specific set, or may use subscripts (like  $\mathbf{X}_1$  and  $\mathbf{X}_2$ ) to put the generic string in context.

We write  $\mathbf{V}$  and  $\mathbf{C}$  for generic vowels and consonants, respectively. The classification schemes for vowels and consonants may depend on language and context. Like the case of  $\mathbf{X}$ , the exact identity of the wildcard symbol  $\mathbf{V}$  or  $\mathbf{C}$  may vary from entry to entry, line to line.

The symbol  $\hat{\chi}$  denotes a single letter character (a Unicode character other than digit or punctuation<sup>20</sup>). When we repeat it  $n$  times (as in  $\underbrace{\hat{\chi}\cdots\hat{\chi}}_{n \text{ times}}$ ), we mean exactly  $n$  letter characters (not necessarily identical) appearing successively in a text string.

The symbol  $\hat{\xi}$  stands for a single letter character (which serves the same function as  $\hat{\chi}$  when used alone). However, whenever  $\hat{\xi}$  is repeated, it always stands for the same character.  $\square$

*Example 3.4.1.* The string pattern  $\mathbf{Xaint}$  ( $\mathbf{X} \in \{rt, mpl, tr\}$ ) is synonymous with the notation  $(rt|mpl|tr)aint$ , denoting any member among  $\{rtaint, mplaint, traint\}$ . For succinctness, we also abbreviate  $\mathbf{Xaint}$  ( $\mathbf{X} \in \{rt, mpl, tr\}$ ) in a superscript notation, as  $\mathbf{X}^{\in} (rt|mpl|tr)aint$ . It is sometimes useful to specify the identity of a wildcard symbol by the set it does not belong to, such as  $\hat{\chi}e$  ( $\hat{\chi} \notin \{e, i\}$ ) denotes a string pattern where the letter  $e$  does not follow a letter  $e$  or  $i$ . In such cases, we will introduce a shorthand using subscript:  $\hat{\chi}_{\notin\{e|i\}}e$ , or use an overline<sup>21</sup> for the negation of a parenthesized string pattern:  $\hat{\chi}^{\in}(\overline{e|i})e$ .

*Example 3.4.2.* The multiplicity notation (introduced in Definition 3.3) also applies to negated string patterns. For instance, in the notation  $\mathbf{X}^{\in}(\overline{(e|i)_{m_0}})e$ , the wildcard  $\mathbf{X}$  is restricted to zero or more repeated occurrences of any letter other than  $e$  or  $i$ . When  $n$  repetitions of the same letter character are intended, we write  $\hat{\chi}_{\times n}$ . Thus  $\hat{\chi}_{\times 2}$  refers to double letters, which contrasts with  $\hat{\chi}\hat{\chi}$  (two letter characters, either identical or distinct).

*Example 3.4.3.* In Finnish, there are word endings in the form of  $(ahan|ehen|ihin|ohon|\ddot{a}h\ddot{a}n|\ddot{o}h\ddot{o}n)$ . Such patterns can be represented by  $\hat{\xi}h\hat{\xi}n$  for  $\hat{\xi} \in \{a|e|i|o|\ddot{a}|\ddot{o}\}$ .

*Example 3.4.4.* The string pattern  $\mathbf{CVC}e$  in English, when  $\mathbf{V}$  and  $\mathbf{C}$  are appropriately defined, usually implies that the  $\mathbf{V}$  in question is pronounced as a long vowel.

*Example 3.4.5.* We write  $\hat{\alpha} = \hat{\beta}$  if the two strings in question match exactly. With string alternatives and wildcard symbols, we can interpret many other string equations and string inequalities. For example,  $\hat{\beta} = \hat{\alpha}\mathbf{X}$  means that string  $\hat{\beta}$  can be constructed from string  $\hat{\alpha}$ , together with zero or more trailing characters (which is usually a linguistically meaningful scenario, where  $\hat{\beta}$  is a morphological derivative of  $\hat{\alpha}$ ); the equation  $\hat{\beta} = \hat{\alpha}(\hat{\sigma}_1|\cdots|\hat{\sigma}_n)$  means that at least one of the  $n$  statements  $\hat{\beta} = \hat{\alpha}\hat{\sigma}_1, \dots, \hat{\beta} = \hat{\alpha}\hat{\sigma}_n$  holds (where  $\hat{\sigma}_1, \dots, \hat{\sigma}_n$  can be regarded as  $n$  candidate suffixes); the string inequality  $\hat{\beta} \neq \hat{\alpha}(\hat{\sigma}_1|\cdots|\hat{\sigma}_n)$  means that none of the  $n$  statements  $\hat{\beta} = \hat{\alpha}\hat{\sigma}_1, \dots, \hat{\beta} = \hat{\alpha}\hat{\sigma}_n$  is true.

**Definition 3.5** (Partial and full matches). A string  $\hat{\sigma}$  written in the plain may occur anywhere in a word. The underlined notation  $\underline{\hat{\sigma}}$  refers to a string that matches the entire word exactly.

The notation  $\hat{\sigma}\sim$  (resp.  $\sim\hat{\sigma}$ ) refers to any word that “starts” (resp. “ends”) with the string  $\hat{\sigma}$ . Here, an isolated word may “start” or “end” at external and internal word boundaries. The external word boundaries are the two ends of the text string representing the isolated word, while the internal word boundaries occur at any non-letter character (apostrophe, digit, hyphen, etc.) in the string.<sup>22</sup>  $\square$

**Definition 3.6** (Substitution rules). When we say “do  $\hat{\sigma} \rightarrow \hat{\sigma}'$ ”, we mean to replace any occurrence(s) of the string  $\hat{\sigma}$  in a word by a new string  $\hat{\sigma}'$ . Here in the substitution rule, the string  $\hat{\sigma}$  may also be augmented with wildcard symbols and partial/full match notations. The letters behind the wildcard symbols are left intact in substitutions, if  $\hat{\sigma}'$  contains the respective wildcard symbols.

When we say “do  $\hat{\sigma}_1 \rightarrow \hat{\sigma}'_1, \dots, \hat{\sigma}_n \rightarrow \hat{\sigma}'_n$ ” on a particular word, we mean to perform  $n$  types of substitution tasks in a single sweep — there might be multiple replacements in a single word, but the replacements do not overlap each other.

Instead of saying “do  $\hat{\sigma}_1 \rightarrow \hat{\sigma}'_1, \dots, \hat{\sigma}_n \rightarrow \hat{\sigma}'_n$ ”, we may also tabulate the substitution rules as follows:

$$\begin{array}{ccc} \hat{\sigma}_1 & \cdots & \hat{\sigma}_n \\ \hat{\sigma}'_1 & \cdots & \hat{\sigma}'_n \end{array}$$

<sup>20</sup>Roughly speaking, this corresponds to `LetterCharacter` in *Mathematica* for versions 10.3 and higher. Earlier versions of *Mathematica* did not treat some symbols in non-Latin writing systems as `LetterCharacter`.

<sup>21</sup>In general, we avoid applying the overline directly to letters, such as  $\bar{e}$ , because this may be confused with the macron diacritic (as in the long vowel markings  $\bar{a}, \bar{e}, \bar{i}, \bar{o}, \bar{u}, \bar{y}$  employed in Latin dictionaries). When  $\hat{\chi}_{\notin\{e\}}$  is intended, we write  $\hat{\chi}^{\in}(\overline{e})$ .

<sup>22</sup>Both external and internal word boundaries are represented by `WordBoundary` in *Mathematica*.

where the strings in the shaded entries are replaced by their counterparts that lie immediately below. The tabulation is particularly helpful when  $n$  is large and/or some structures in the substitution rules are better visualized in table form.  $\square$

*Example 3.6.1.* Application of the substitution rule “do  $\sim s \rightarrow \emptyset$ ” will remove the plural markers in the word *daughters* as well as the compound *daughters-in-law*. If we “do  $r \sim \rightarrow R$ ” on the word *rock-and-roll*, we obtain *Rock-and-Roll*. If we “do  $ass \rightarrow \emptyset$ ,  $sas \rightarrow \emptyset$ ” on the word *assassinate*, we obtain *inate*, as a result of *assassinate*  $\xrightarrow{\text{remove sas}}$  *assinate*  $\xrightarrow{\text{remove ass}}$  *inate*.<sup>23</sup>

*Example 3.6.2.* The following tabulated substitution rules

|                       |              |                                                                   |
|-----------------------|--------------|-------------------------------------------------------------------|
| ~(go(es ing ne) went) | taught       | $X \in (\emptyset   in   mis   off   out   over   p   under) led$ |
| <i>go</i>             | <i>teach</i> | <b>X</b> <i>lead</i>                                              |

regularize some verb forms in English.

**Definition 3.7** (NW and SW). For two text strings  $\hat{\sigma}_1$  and  $\hat{\sigma}_2$ , the output of the function  $NW(\hat{\sigma}_1, \hat{\sigma}_2)$  [resp.  $SW(\hat{\sigma}_1, \hat{\sigma}_2)$ ] is a string pattern that results from the sequence alignment from  $\hat{\sigma}_1$  to  $\hat{\sigma}_2$  according to the Needleman–Wunsch (resp. Smith–Waterman) algorithm.  $\square$

*Example 3.7.1.*  $NW(keep, kept) = SW(keep, kept) = k[e, \emptyset]ep[\emptyset, t]$ , where the bracketed portions show mismatches of the two strings. Here, in the presentation of the output string pattern, we have used  $[e, \emptyset]$  and  $[\emptyset, t]$  to show the respective contributions from the string  $\hat{\sigma}_1 = keep$  and  $\hat{\sigma}_2 = kept$ . Unlike the situation in notation for “alternatives” ( $\hat{\sigma}'_1 | \dots | \hat{\sigma}'_n$ ), the arguments within the square brackets no longer commute, and must reflect the order in the input arguments of the functions  $NW(\hat{\sigma}_1, \hat{\sigma}_2)$  and  $SW(\hat{\sigma}_1, \hat{\sigma}_2)$ .

*Example 3.7.2.* The outputs of the functions  $NW(\hat{\sigma}_1, \hat{\sigma}_2)$  and  $SW(\hat{\sigma}_1, \hat{\sigma}_2)$  may not necessarily be identical. For example,  $NW(infer, inferior) = infe[\emptyset, rio]r$  while  $SW(infer, inferior) = infer[\emptyset, ior]$ .

## 3.2 Normalizations of Wikipedia pages and WikiQA dataset

Each question in the WikiQA dataset [44] is associated with a unique Wikipedia page. We need to pick a sentence from a small subset (usually just the opening paragraph, as provided by the WikiQA dataset) of this Wikipedia page that best answers the question. In the main text of this research, we use the single Wikipedia page (in full, not just the opening paragraph) as the sole training source of our artificial neural network, before we score and screen individual sentences in the candidate answer pool.

To construct the knowledge base used in this work, we downloaded the static dump of English Wikipedia dated Sept. 1, 2015 (file name: `enwiki-20150901-pages-articles-xml.bz2`) from the URL [https://meta.wikimedia.org/wiki/Data\\_dump\\_torrents#enwiki](https://meta.wikimedia.org/wiki/Data_dump_torrents#enwiki) and saved it as an XML file. We chose this static dump because its time stamp is close to the publication date of the WikiQA dataset [44].

Once we have located the exact Wikipedia page suitable for a particular WikiQA task, we need to process the raw XML code of such a page, to generate (nearly human-readable) plain text strings. This normalization procedure is described below.

**Algorithm 3.8** (Normalization of English Wikipedia Articles). *Let  $\mathbf{D} = (0|1|2|3|4|5|6|7|8|9)$  be any one of the digit characters, and  $\mathbf{W} = (\hat{\chi}|\mathbf{D})$  be either a letter character or a digit character. The XML codes of a page from the filtered knowledge base are normalized by sequential applications of the following substitution rules, where all the boxed portions are spelt out in verbatim mode.*

(1) Do  $\boxed{\&amp;}; \rightarrow \boxed{\&}$ .

(2) Replace the shaded patterns by their respective counterparts that lie immediately below:

|                         |                       |                       |                         |                  |
|-------------------------|-----------------------|-----------------------|-------------------------|------------------|
| <code>&amp;nbsp;</code> | <code>&amp;lt;</code> | <code>&amp;gt;</code> | <code>&amp;quot;</code> | <code>]]</code>  |
| $\emptyset$             | $<$                   | $>$                   | $" = \boxed{U+0022}$    | $\boxed{U+2712}$ |

(3) Replace

<sup>23</sup>Written in *Mathematica* codes, these statements amount to the following results:

```
StringReplace["daughters", "s"~~WordBoundary :> ""] yields "daughter";
StringReplace["daughters-in-law", "s"~~WordBoundary :> ""] yields "daughter-in-law";
StringReplace["rock-and-roll", WordBoundary~~"r" :> "R"] yields "Rock-and-Roll";
StringReplace["assassinate", {"ass" :> "", "sas" :> ""}] yields "inate".
```

Note in particular that in the last example, the substitution rules  $\{"ass" :> "", "sas" :> ""\}$  and  $\{"sas" :> "", "ass" :> ""\}$  will generate the same output.



(= U+2013) | &ndash; | (U+00E2 U+0080 U+0093) &mdash; | (U+00E2 U+0080 U+0094)  
-- = U+002D x2 — = U+2014

(10) Do  $\mathbf{W}$  U+0027  $\rightarrow$  .

(11) If the text string so far ends with  $\mathbf{W}$ , then append . to it; otherwise, leave it as is.

(12) Call the result so far as string  $P_0$ . Denote the input WikiQA question by  $Q$  and the Wikipedia page title by  $T$  (both of which must be “corrected” by Algorithm 3.11 below). If  $P_0 = \emptyset$ , then send  $P = \text{.}$  as output; otherwise send  $P = Q$  U+000A x2  $T$  U+000A x2  $P_0$  U+000A x2  $Q$  . as output.

Here, in the algorithm above, we have tried our best to eliminate structured data (infoboxes, references, as well as hyperlinks to other pages and external files) from the XML file, and restore all clickable links to normal text. Some replacements are done in multiple sweeps to accommodate to nested structures in Wikipedia XML files. However, we note that due to the versatility of Wikipedia XML files, our cleansing algorithm may still have some blind spots. In practice, this heuristic algorithm handles most Wikipedia pages well, so long as there are no special characters in hyperlinks and there is no extensive coverage of  $\text{\TeX}$  content.

The WikiQA dataset contains some Wikipedia pages that are simply lists or tables. If we process such Wikipedia pages with Algorithm 3.8, then we will end up with (almost) an empty string. To compensate for this, we generate backup versions of Wikipedia pages, using the algorithm below.

**Algorithm 3.9** (Backup version of Wikipedia pages). Define  $B = Q$  U+000A x2  $T$  U+000A x2  $A$  U+000A x2  $Q$  ., where  $A$  is the concatenation of all the candidate answers ( $\approx$  the opening section of the accompanying Wikipedia page, by design of the WikiQA dataset), riffled by .. If  $\ell(P) < \ell(B)$ , then redefine  $P$  as the backup version  $B$ . If  $T$  matches List of X, regardless of letter case, then redefine  $P$  as  $B$  .  $B$  .  $B$ .

After processing a Wikipedia page by Algorithms 3.8 and 3.9, we arrive at a text string  $P$ , which will be suitable for sentence extractions later. To facilitate the measurement of gaps between words, we need to regularize spacing, punctuation and capitalization, as indicated below.

**Algorithm 3.10** (Regularization of text string). Let  $\mathbf{D} = (0|1|2|3|4|5|6|7|8|9)$  be any one of the digit characters, and  $\mathbf{W} = (\hat{x}|\mathbf{D})$  be either a letter character or a digit character. A processed Wikipedia page must be regularized by the following substitution rules before temporal statistics are computed.

(1) Replace

(( | U+000A) m = (=) m ... = U+002E x3 x  $\in ((\hat{x}|\text{'}'|\text{'-'})_m)$   
. = U+0020 . U+002E U+000A x3 = U+0020 x3  $\mathbf{X}$  if  $\ell(\mathbf{X}) = 1$ ;  $\mathbf{X}^{(1)}(\mathbf{X}^{[2,\ell(\mathbf{X})]})_-$  if  $\ell(\mathbf{X}) > 1$ .  
.  $\mathbf{D}$  = U+002E  $\mathbf{D}$  ,  $\mathbf{D}$  = U+002C  $\mathbf{D}$  :  $\mathbf{D}$  = U+003A  $\mathbf{D}$   
.  $\mathbf{D}$  = U+00B7  $\mathbf{D}$   $\mathbf{D}$  h  $\mathbf{D}$

where  $\mathbf{X}^{(1)}(\mathbf{X}^{[2,\ell(\mathbf{X})]})_-$  reduces  $\mathbf{X}$  to lower case except the initial character.<sup>25</sup>

(2) Replace

, ; : ( ) | U+000A U+2012 . ? ! " U+2014 (U+2013 U+002D)  
. = U+0020 x2 = U+0020 x2 x3 = U+0020 x3

(3) Prepend a single white space character U+0020 to the entire text string.

(4) Record the positions of all the U+0020  $_m$  patterns.

(5) Split the text string at U+0020  $_m$ , to obtain an ordered list of separate words.

Upon conclusion of the aforementioned algorithm, we have effectively obtained the start and end positions of every word appearing in the normalized Wikipedia page  $P$ .

After scrutinizing the WikiQA dataset, we have detected a few typographical flaws:

<sup>25</sup>This means that the capitalization status of a word is determined by its initial character: *eBay*  $\rightarrow$  *ebay*, *ELIZABETH*  $\rightarrow$  *Elizabeth*, *McDonald*  $\rightarrow$  *Mcdonald* etc.

- A few Wikipedia page names listed in WikiQA do not match our record.
- There are non-standard uses of capitalizations and diacritics.
- There are non-standard abbreviations that cannot be inferred from the related Wikipedia pages.
- There are other kinds of misspellings (including unnecessary use of foreign language) in the questions that do not match the information available from the related Wikipedia pages.

Since our purpose in the current research is to test a numerical question answering machine, rather than an automated spell checker, we decide to normalize the WikiQA dataset according to the following *ad hoc* procedures.

**Algorithm 3.11** (Normalization of WikiQA page names and questions). *We normalize the reference Wikipedia page names by the following replacements:*

|                                       |                                 |                               |                                             |
|---------------------------------------|---------------------------------|-------------------------------|---------------------------------------------|
| <i>Automatic Document Feeder</i>      | <i>High-Sticking</i>            | <i>Judas (song)</i>           | <i>Julius caesar</i>                        |
| <i>Automatic document feeder</i>      | <i>High-sticking</i>            | <i>Judas (Lady Gaga song)</i> | <i>Julius Caesar</i>                        |
| <i>What It Takes (song)</i>           | <i>World Trade Center</i>       |                               |                                             |
| <i>What It Takes (Aerosmith song)</i> | <i>World Trade Center (2001</i> | <i>U+00E2</i>                 | <i>U+0080</i> <i>U+0093</i> <i>present)</i> |

We use the following heuristics to determine the correct capitalizations and diacritics in a question  $Q$ , by checking it against all the candidate answers ( $\approx$  the opening section of the accompanying Wikipedia page, by design of the WikiQA dataset)  $A$ :

- (1) Take the union of all the words in  $A$ , and call it  $\mathcal{A}$ . Remove diacritics from  $\mathcal{A}$ , and call it  $\mathcal{A}'$ . Use set-theoretic complements to define  $\mathcal{D} = \mathcal{A}' \setminus \mathcal{A}$  and  $\mathcal{D}_0 = \mathcal{A} \setminus \mathcal{A}'$ .<sup>26</sup> Define  $\mathcal{A}_-$  (resp.  $\mathcal{D}_-$ ) as the lowercase form of  $\mathcal{A}$  (resp.  $\mathcal{D}$ ).
- (2) For each word in  $Q$ , convert it to lower case, remove diacritics if any, call the result  $\hat{q}^*$ , and then do the following:
  - (2.1) If  $\hat{q}^*$  matches  $\mathcal{A}_-(\emptyset|s|s|s')$  and does not match  $\mathcal{A}(\emptyset|s|s|s')$ , then capitalize  $\hat{q}^*$  and quit. Otherwise, go to next step.
  - (2.2) If  $\hat{q}^*$  matches  $\mathcal{D}_-(\emptyset|s|s|s')$ , landing on the  $n$ -th member of alphabetized  $\mathcal{D}$  upon its first hit, then determine the correct spelling by the  $n$ -th member of alphabetized  $\mathcal{D}_0$ . Otherwise, leave  $\hat{q}^*$  as is and quit.

Furthermore, we correct misspelt questions by the following replacements:

|                        |                                                              |                                                             |                                                                |                              |
|------------------------|--------------------------------------------------------------|-------------------------------------------------------------|----------------------------------------------------------------|------------------------------|
| <i>a full job time</i> | <i>cono sur</i>                                              | <i>Điện Chí Minh</i>                                        | <input type="checkbox"/> fy <input type="checkbox"/>           | <i>general chu chicken</i>   |
| <i>a full-time job</i> | <i>Southern Cone</i>                                         | <i>Hồ Chí Minh</i>                                          | <input type="checkbox"/> fiscal year <input type="checkbox"/>  | <i>General Tso's Chicken</i> |
| <i>Google in math</i>  | <i>jagger bomb</i>                                           | <i>st patty</i>                                             | <i>ti 82</i>                                                   | <i>trinity 5 7</i>           |
| <i>googol in math</i>  | <i>Jägerbomb</i>                                             | <i>Saint Patrick</i>                                        | <i>TI-82</i>                                                   | <i>Trin-i-tee 5:7</i>        |
| <i>tri tip</i>         | <input type="checkbox"/> ua's <input type="checkbox"/>       | <input type="checkbox"/> ww <input type="checkbox"/>        | <input type="checkbox"/> wwii <input type="checkbox"/>         |                              |
| <i>tri-tip</i>         | <input type="checkbox"/> urinalysis <input type="checkbox"/> | <input type="checkbox"/> World War <input type="checkbox"/> | <input type="checkbox"/> World War II <input type="checkbox"/> |                              |

In Table 2 and Fig. S2, we showed that our numerical question answering machine had better performance on a subset of the WikiQA questions. Our criteria for defining such a subset (via its complement) are stated below.

**Algorithm 3.12** (Heuristic classification of WikiQA questions). *We classify a WikiQA question as “quantitative” (requiring rule-based reasoning), if it matches one of the following string patterns (regardless of letter case):*

*how*(<sub>m</sub>)(big|deep|far|frequent|high|long|many|much|often|old|tall)**X**,  
*when***X**,  
**X**(#|number|percentage|proportion)**X**,  
*what*()(bec|happen|year)**X**.

Otherwise, we classify a WikiQA question as “qualitative” (requiring only associative reasoning).

<sup>26</sup>Note that if the reference page uses diacritics consistently and we alphabetize both  $\mathcal{D}$  and  $\mathcal{D}_0$ , then the corresponding positions are occupied by the same words, without and with diacritics. For example, set  $A = \text{Estée Lauder and Eva Perón}$  and  $Q = \text{péron esTee lauder}$ , then we have  $\mathcal{D} = \{\text{Estee, Peron}\}$  and  $\mathcal{D}_0 = \{\text{Estée, Perón}\}$ . After going through the remaining procedures in Step (2), we will end up with a corrected version of  $Q$  as  $\text{Perón Estée Lauder}$ . Our heuristic algorithm will malfunction, however, if  $P$  contains both *Estée* and *Estee* (i.e. the reference page uses diacritics inconsistently), or if alphabetic ordering is seriously affected by diacritics. In practice, the only glitch occurs in WikiQA-Q2158, where *Ho Chi Minh* becomes misspelt as *Điện Chí Minh*, due to unexpected alphabetic ordering of Vietnamese characters in *Mathematica* v11.3 (which brought us  $\mathcal{D} = \{\text{Ai, Bien, Chi, Cong, Dien, Ho, Nguyen, Phu, Quoc, Tat, Thanh, Viet}\}$  and  $\mathcal{D}_0 = \{\text{Ai, Biên, Chí, Cộng, Hồ, Điện, Nguyễn, Phú, Quốc, Thành, Tát, Việt}\}$ ). This is subsequently corrected by a substitution rule.

### 3.3 Normalizations of ebooks for text mining

For the topic extraction and word translation experiments (Figs. S3–S16), we use the following algorithms for cleansing electronic books written in 12 European languages and 2 Asian languages, sorted in the same order as the remaining sections of this document. Hereafter, in accordance with *Mathematica* terminology, we use the word character  $\mathbf{W} = (\hat{\chi}|\mathbf{D})$  to refer to either a letter or a digit.

**Algorithm 3.13** (Text cleansing for English ebooks). *We process our text (ebooks from Gutenberg Project and elsewhere<sup>27</sup>) according to the following procedures:*

(1) Do  $\overline{\mathbf{W}}^{\text{U+0027}} \rightarrow \square_{\times 2}$ .

(2) Replace

$$\left( \square_m \text{U+000A} \square_m \text{--} \square_m * \square_m \text{ ( } \square_m \text{ ) } \right) \xrightarrow{\mathbf{X} \in \left( (\hat{\chi} | \square_m \text{--}) \right)} \square$$

$\mathbf{X}$  if  $\ell(\mathbf{X}) = 1$ ;  $\mathbf{X}^{(1)}(\mathbf{X}^{[2, \ell(\mathbf{X})]})_-$  if  $\ell(\mathbf{X}) > 1$ .

where  $\mathbf{X}^{(1)}(\mathbf{X}^{[2, \ell(\mathbf{X})]})_-$  reduces  $\mathbf{X}$  to lower case except the initial character.

**Algorithm 3.14** (Text cleansing for Danish ebooks). *We normalize our text by doing*

$$\left( \square_m \text{U+000A} \square_m \text{--} \square_m * \square_m \text{U+002D} \text{U+2013} \text{U+2014} \text{U+201E} \text{ ( } \square_m \text{ ) } \text{U+00AB} \text{U+00BB} \text{U+2026} \right) \rightarrow \square.$$

**Algorithm 3.15** (Text cleansing for German ebooks). *We normalize our text by doing*  $\left( \text{U+0027} \text{U+2019} \right) \rightarrow \square$ ,  $\left( \text{U+2039} \text{U+203A} \right) \rightarrow \square$ ,  $\left( \square_m \text{U+000A} \square_m \text{--} \square_m * \square_m \text{U+002D} \text{U+2013} \text{U+2014} \text{U+201E} \text{ ( } \square_m \text{ ) } \text{U+00AB} \text{U+00BB} \text{U+2026} \right) \rightarrow \square$ ,  $\text{u. s. w.} \rightarrow \square_{\times 6}$ .

**Algorithm 3.16** (Text cleansing for Dutch ebooks). *We normalize our text by doing*  $\left( \text{U+0027} \text{U+2019} \right) \rightarrow \square$ ,  $\left( \text{U+2039} \text{U+203A} \right) \rightarrow \square$ ,  $\left( \square_m \text{U+000A} \square_m \text{--} \square_m * \square_m \text{U+002D} \text{U+2013} \text{U+2014} \text{U+201E} \text{ ( } \square_m \text{ ) } \text{U+00AB} \text{U+00BB} \text{U+2026} \right) \rightarrow \square$ .

**Algorithm 3.17** (Text cleansing for Spanish ebooks). *We normalize our text by doing*  $\left( \dot{\square} \square_i \right) \rightarrow \emptyset$ ,  $\left( \square_m \text{U+000A} \square_m \text{--} \square_m * \square_m \text{U+002D} \text{U+2013} \text{U+2014} \text{U+201E} \text{ ( } \square_m \text{ ) } \text{U+00AB} \text{U+00BB} \text{U+2026} \right) \rightarrow \square$ .

**Algorithm 3.18** (Text cleansing for French ebooks). *We normalize our text (ebooks from Wikisource and Gutenberg Project) according to the following procedures:*

(1) Do  $\text{M.} \rightarrow \text{Mr}$ .

(2) Do  $\left( \square_m \text{U+000A} \square_m \text{--} \square_m * \square_m \text{U+002D} \text{U+2013} \text{U+2014} \text{U+201E} \text{ ( } \square_m \text{ ) } \text{U+00AB} \text{U+00BB} \text{U+2026} \right) \rightarrow \square$ ,  $\left( \text{U+0027} \text{U+2019} \right) \rightarrow \square$ .

**Algorithm 3.19** (Text cleansing for Latin ebooks). *We normalize our text by doing*

$$\left( \square_m \text{U+000A} \square_m \text{--} \square_m * \square_m \text{U+002D} \text{U+2013} \text{U+2014} \text{U+201E} \text{ ( } \square_m \text{ ) } \text{U+00AB} \text{U+00BB} \text{U+2026} \right) \rightarrow \square.$$

**Algorithm 3.20** (Text cleansing for Polish ebooks). *We normalize our text according to the following procedures:*

(1) Do  $(\emptyset \text{U+002D} \text{U+2014})(\text{U+0020} \text{U+000A})_{m_0} [\mathbf{D}_{m_0}] (\text{U+0020} \text{U+000A})_{m_0} \rightarrow \emptyset$ ,  $\hat{\chi}_1(\text{U+0027} \text{U+2019})\hat{\chi}_2 \rightarrow \hat{\chi}_1\#\hat{\chi}_2$ .

(2) Do  $\left( \square_m \text{U+000A} \square_m \text{--} \square_m * \square_m \text{U+002D} \text{U+2013} \text{U+2014} \text{U+201E} \text{ ( } \square_m \text{ ) } \text{U+00AB} \text{U+00BB} \text{U+2026} \right) \rightarrow \square$ ,  $\left( \text{U+0027} \text{U+2019} \right) \rightarrow \square$ .

**Algorithm 3.21** (Text cleansing for Russian ebooks). *We normalize our text according to the following procedures:*

(1) Do  $(\emptyset \text{U+002D} \text{U+2014})(\text{U+0020} \text{U+000A})_{m_0} [\overline{(\square)}]_{m_0} [\text{U+0020} \text{U+000A}]_{m_0} \rightarrow \emptyset$ ,  $\text{BookTitle}(\square \text{--})_{m_0} \mathbf{D}_{m_0} / \mathbf{D}_{m_0} (\square \text{--})_{m_0} \rightarrow \square$ .

(2) Do  $\hat{\chi}_1[\text{?}]\hat{\chi}_2 \rightarrow \hat{\chi}_1\text{y}\hat{\chi}_2$ .

<sup>27</sup>It is always understood that the front and back matters (publisher's boilerplate, table of contents, introductory chapter, glossary, index, endnotes, etc.) in ebooks are manually removed. Footnotes that scatter in a few pages are left intact.

(3) Do  $(\square_m \text{U+000A} \square_m \text{--} \square_m * \square_m \text{U+002D} \text{U+2013} \text{U+2014} \text{U+201E} \square_m \text{(} \square_m \text{)} \text{U+00AB} \text{U+00BB} \text{U+2026}) \rightarrow \square_m$ ,  
 $(\text{U+0027} \text{U+2019}) \rightarrow \square_m$ .

**Algorithm 3.22** (Text cleansing for Finnish ebooks). *We normalize our text (ebooks from the Gutenberg Project) according to the following procedures:*

(1) Do  $(\square_m \text{U+000A} \square_m \text{--} \square_m * \square_m \text{U+002D} \text{U+2013} \text{U+2014} \text{U+201E} \square_m \text{(} \square_m \text{)} \text{U+00AB} \text{U+00BB} \text{U+2026}) \rightarrow \square_m$ ,  
 $(\text{U+201C} \text{U+201D}) \rightarrow \square_m$ ,  $[\text{D}_{m_0}] \rightarrow \emptyset$ ,  $\mathbf{W}[:\hat{\chi}] \rightarrow \mathbf{W}\#\hat{\chi}$ .

(2) Do  $\text{U+0027} \mathbf{W} \rightarrow \square_m$ ,  $\mathbf{W} \text{U+0027} \rightarrow \square_m$ .

**Algorithm 3.23** (Text cleansing for Hungarian ebooks). *We normalize our text (ebooks from <http://mek.oszk.hu>) according to the following procedures:*

(1) Do  $(\emptyset \text{U+002D} \text{U+2014})(\text{U+0020} \text{U+000A})_{m_0} [\text{D}_{m_0}] (\text{U+0020} \text{U+000A})_{m_0} \rightarrow \emptyset$ ,  
 $\text{BookTitle}(\square_m \text{--})_{m_0} \text{D}_{m_0} / \text{D}_{m_0} (\square_m \text{--})_{m_0} \rightarrow \square_m$ .

(2) Do  $(\square_m \text{U+000A} \square_m \text{--} \square_m * \square_m \text{U+002D} \text{U+2013} \text{U+2014} \text{U+201E} \square_m \text{(} \square_m \text{)} \text{U+00AB} \text{U+00BB} \text{U+2026}) \rightarrow \square_m$ ,  
 $(\text{U+0027} \text{U+2019} \text{U+201C} \text{U+201D}) \rightarrow \square_m$ .

**Algorithm 3.24** (Text cleansing for Basque ebooks). *We normalize our text according to the following procedures:*

(1) Do  $(\emptyset \text{U+002D} \text{U+2014})(\text{U+0020} \text{U+000A})_{m_0} [\text{D}_{m_0}] (\text{U+0020} \text{U+000A})_{m_0} \rightarrow \emptyset$ .

(2) Do  $\text{eliz} \rightarrow \text{ēliz}$ .<sup>28</sup>

(3) Do  $(\square_m \text{U+000A} \square_m \text{--} \square_m * \square_m \text{U+002D} \text{U+2013} \text{U+2014} \text{U+201E} \square_m \text{(} \square_m \text{)} \text{U+00AB} \text{U+00BB} \text{U+2026}) \rightarrow \square_m$ ,  
 $(\text{U+0027} \text{U+2018} \text{U+2019} \text{U+201C} \text{U+201D}) \rightarrow \square_m$ .

**Algorithm 3.25** (Text cleansing for Korean ebooks). *We normalize our text according to the following procedures:*

(1) Do  $(\emptyset \text{U+002D} \text{U+2014})(\text{U+0020} \text{U+000A})_{m_0} [\text{D}_{m_0}] (\text{U+0020} \text{U+000A})_{m_0} \rightarrow \emptyset$ .

(2) Do  $\text{체} \text{D}_m(\text{권}|\text{장}) \rightarrow \square_m$ .

(3) Do  $(\square_m \text{U+000A} \square_m \text{--} \square_m * \square_m \text{U+002D} \text{U+2013} \text{U+2014} \text{U+201E} \square_m \text{(} \square_m \text{)} \text{U+00AB} \text{U+00BB} \text{U+2026}) \rightarrow \square_m$ ,  
 $(\text{U+0027} \text{U+2018} \text{U+2019} \text{U+201C} \text{U+201D} \text{U+2500} \text{U+25CB} \text{U+3008} \text{U+3009} \text{U+300C} \text{U+300D}) \rightarrow \square_m$ .

(4) Adjust spacing in the text as follows:<sup>29</sup>

(4.1) Do  $\mathbf{D}\text{백} \rightarrow \mathbf{D}\square\text{백}$ ,  $\mathbf{D}\text{천} \rightarrow \mathbf{D}\square\text{천}$ ,  $\mathbf{D}\text{만} \rightarrow \mathbf{D}\square\text{만}$ ,  $\mathbf{D}\text{일} \rightarrow \mathbf{D}\square\text{일}$ ,  $\text{지}\text{난}\mathbf{W} \rightarrow \text{지}\text{난}\square\mathbf{W}$ ,  $\text{다}\text{음}\mathbf{W} \rightarrow \text{다}\text{음}\square\mathbf{W}$ ,  
 $\square\text{다}\text{시}\square_{\hat{\chi} \notin \{\text{씨}\text{양}\}} \rightarrow \square\text{다}\text{시}\square_{\hat{\chi}}$ ;

(4.2) Do  $\hat{\chi} \in (\text{가}\text{나})\square\text{싶} \rightarrow \square\hat{\chi}\text{싶}$ ,  $\text{고}\square\text{나}(\sim \hat{\chi} \in (\emptyset|\text{고}\text{기}\text{는}\text{니}\text{래}\text{면}\text{서}\text{서}\text{신}\text{실}\text{심}\text{야}\text{요}\text{자})) \rightarrow \square\text{꼭}\text{나}\mathbf{X}$ ,  
 $\text{고}\square(\sim \hat{\chi} \in (\text{난}\text{단}\text{날}\text{남})) \rightarrow \square\text{꼭}\hat{\chi}$ ,  $\text{고}\square_{\hat{\chi} \in (\text{나}\text{겠}\text{나}\text{느}\text{나}\text{는}\text{나}\text{니}\text{나}\text{더}\text{나}\text{려}\text{나}\text{세}\text{나}\text{셔}\text{나}\text{셨}\text{나}\text{시}\text{나}\text{신}\text{나}\text{십}\text{나}\text{자}\text{나}\text{지}\text{남}\text{니}\text{답}\text{시}\text{냈}\text{보}\text{(이)}|\text{본}\text{불}\text{봄}\text{봄}\text{봐}\text{봤}\text{(자)})} \rightarrow \square\text{꼭}\hat{\chi}$ ,  $\text{고}\square_{\hat{\chi} \in (\text{말}\text{싶})} \rightarrow \square\text{고}\hat{\chi}$ ,  
 $\hat{\chi} \in (\text{과}\text{엔}\text{와})\square\text{다}\text{시}\square \rightarrow \square\text{다}\text{시}\square$ ,  $\text{까}\square_{\hat{\chi} \in (\text{말}\text{보}\text{(이)}|\text{본}\text{불}\text{봄}\text{봄}\text{봐}\text{봤}\text{(자)}|\text{싶})} \rightarrow \square\text{까}\mathbf{X}$ ,  
 $\hat{\chi}_1 \in (\text{대}\text{아}\text{어})\square\hat{\chi}_2 \in (\text{보}\text{(이)}|\text{본}\text{불}\text{봄}\text{봄}\text{봐}\text{봤}\text{(자)}) \rightarrow \square\hat{\chi}_1\hat{\chi}_2$ ,  $\hat{\chi}_1 \in (\text{년}\text{단}\text{란}\text{잔})\square\text{말}\hat{\chi}_2 \in (\text{슴}\text{이}) \rightarrow \square\hat{\chi}_1\text{말}\hat{\chi}_2$ ,  
 $\text{지}\square_{\hat{\chi} \in (\text{마}\text{느}\text{마}\text{세}\text{마}\text{셨}\text{마}\text{시}\text{마}\text{십}\text{말}\text{했}\text{말}\text{데}\text{말}\text{려}\text{말}\text{았}\text{말}\text{지}\text{맙}\text{니}\text{맙}\text{시})} \rightarrow \square\text{지}\mathbf{X}$ ,  $\text{지}\square(\sim \hat{\chi} \in (\text{마}\text{는}\text{마}\text{니}\text{마}\text{셔}\text{마}\text{신}\text{마}\text{실}\text{마}\text{십}\text{만}\text{말}\text{말}\text{고}\text{말}\text{기}\text{말}\text{면}\text{말}\text{아}\text{말}\text{자}\text{맙})) \rightarrow \square\text{지}\mathbf{X}$ .

**Algorithm 3.26** (Text cleansing for Turkish ebooks). *We normalize our text according to the following procedures:*

(1) Do  $(\emptyset \text{U+002D} \text{U+2014})(\text{U+0020} \text{U+000A})_{m_0} [\text{D}_{m_0}] (\text{U+0020} \text{U+000A})_{m_0} \rightarrow \emptyset$ ,  $\hat{\chi}_1(\text{U+2019})\hat{\chi}_2 \rightarrow \hat{\chi}_1\#\hat{\chi}_2$ ,  $I \rightarrow i$ ,  $\dot{I} \rightarrow i$ ,  $\text{BÖLÜM}(\square_m) \text{D}_m \rightarrow \text{BÖLÜM}(\square_m)$ .

(2) Do  $(\square_m \text{U+000A} \square_m \text{--} \square_m * \square_m \text{U+002D} \text{U+2013} \text{U+2014} \text{U+201E} \square_m \text{(} \square_m \text{)} \text{U+00AB} \text{U+00BB} \text{U+2026}) \rightarrow \square_m$ ,  
 $(\text{U+0027} \text{U+2018} \text{U+2019} \text{U+201C} \text{U+201D}) \rightarrow \square_m$ .

<sup>28</sup>The Basque word *eliza* “church” should not be confused with the proper name *Eliza*.

<sup>29</sup>Some Korean words are best disambiguated by their immediate neighbors, such as  $\sim\text{고}\square\text{싶}\sim$  “want to do” [45, p. 251] and  $\sim(\text{가}\text{나})\square\text{싶}\sim$  “think it might” [45, p. 256]. This is the main reason why we reassign spaces to our text.

To obtain individual words from a normalized text, we split the text string at (`[ , | . ? ! : ; U+0022 ]`) (for French, also apostrophe `'` and hyphen `-`). To measure gaps between words in a normalized text, we further substitute spaces and punctuation marks according to the rules: (`[ , | : ; ]`) $\rightarrow$ , (`[ . ? ! U+0022 ]`) $\rightarrow$  $\times 2$ .

## Part III

# Protocols for word clustering

All the word clustering algorithms in this Part are available as *Mathematica* source codes (English.nb for word clustering and analysis of English texts, etc.), posted to Github

<https://github.com/yajun-zhou/linguae-naturalis-principia-mathematica>

To reproduce all the figures in this Part from these source codes, the readers need to download and/or purchase text corpora (not posted to our Github repository), following the instructions in Table S1.

Additionally, a separate source code `WikiQA.nb` is available, which implements our word clustering algorithm for English to the WikiQA dataset [44]. Based on the list of page titles in the WikiQA dataset, we extract `WikiSelecta.XML` (deposited as a zipped file `WikiSelecta.zip` in our Github folder) from the static dump of English Wikipedia dated Sept. 1, 2015 (file name: `enwiki-20150901-pages-articles-xml.bz2`). This subset of 1242 Wikipedia pages forms the only training source and knowledge base for our question-answering machine.

## 4 Approximate word clustering in English

In this section, we describe an automatic algorithm to cluster English words according to their morphologies. Due to the complicated linguistic history of English that derives from both Germanic heritage and Latin/Romance influence, the English language is rich in both inflectional complexity (such as vowel alternations in verb forms, a feature common to Germanic languages) and derivational complexity (such as many Latinate suffixes that distinguish words within the same word family). Our English word clustering algorithm thus involves methods that will be later used in the studies of Germanic (§5) and Romance (§6) languages.

### 4.1 Capitalization and stop words

Before presenting our algorithms in detail, we need to briefly discuss the capitalization problem in English and the list of English stop words.

English orthography requires capitalization of proper nouns and their derivatives.<sup>30</sup> It turns out that proper nouns and common nouns in English tend to have different etymological sources, and consequently, different morphological structures. Thus, it is helpful to single out “intrinsically capitalized words” used in an English text before performing word clustering algorithms. The precise identification of the capitalization status of a particular word is a non-trivial task: words that start any sentence are always capitalized; some authors may occasionally choose to use ALL CAPS for emphasis; some “intrinsically capitalized words” may share the same spelling with other ordinary words, up to capitalization (such as *Miss* and *miss*). For our text mining purposes, we adhere to the following heuristic determination of the capitalization status.

**Definition 4.1** (Heuristic capitalization). We say that a word is “heuristically capitalized” in a given text, if its all-lowercase form never appears in the same document. Otherwise, we consider the word’s spelling “heuristically uncapitalized”.<sup>31</sup>  $\square$

A small collection of English words perform important grammatical/logical functions, but transmit very little information on their own. These words need to be excluded in most natural language processing tasks, and are thus referred to as “stop words”. There is not a universal standard for the list of English stop words. We state our empirical list in the definition below.

<sup>30</sup>Among the major European languages, this capitalization rule perhaps only applies to English. In all the other European languages studied in this work, adjectives derived from proper nouns are spelt in lower case forms. In modern German and pre-1948 Danish, all nouns are capitalized. In Modern Turkish (which we regard as an Asian language), derivatives of proper nouns are also capitalized, as in English. However, we do not find it particularly helpful to treat Turkish proper nouns differently from other nouns in word clustering. Therefore, we will restrict Definition 4.1 to English only.

<sup>31</sup>According to this definition, a word’s spelling must be either “heuristically capitalized” or “heuristically uncapitalized”. If *Miss* and *miss* both appear in the same text, then they will be regarded as the same word, in the “heuristically uncapitalized” status of our classification scheme. On the other hand, if a text contains *Elizabeth* and *ELIZABETH*, but does not contain *elizabeth*, then we merge *Elizabeth* and *ELIZABETH* to the same word, in the “heuristically capitalized” status.

**Definition 4.2** (English stop words). If a word belongs to the following list<sup>32</sup>:

–, &c, a, about, above, across, after, afterward, afterwards, again, against, ago, ahead, albeit, all, almost, alone, along, already, also, although, always, am, amid, amidst, among, amongst, an, and, another, any, anybody, anybody's, anyhow, anyone, anything, anyway, anywhere, apart, are, aren't, around, as, aside, at, away, back, be, became, because, become, becomes, becoming, been, before, behind, being, below, beneath, beside, besides, between, beyond, both, but, by, can, can't, cannot, could, couldn't, did, didn't, do, does, doesn't, doing, don't, done, down, during, each, either, else, elsewhere, enough, etc, even, ever, every, everybody, everybody's, everyone, everyone's, everything, everywhere, except, few, for, from, front, full, further, furthermore, get, gets, getting, got, gotten, had, hadn't, hardly, has, hasn't, have, haven't, having, he, he'd, he'll, he's, hence, her, here, here's, hereabout, hereabouts, hereafter, hereby, herein, hereinafter, hereof, hereon, hereto, heretofore, hereunder, hereunto, hereupon, herewith, hers, herself, him, himself, his, hither, how, how's, however, howsoever, i, I, i'd, I'd, i'll, I'll, i'm, I'm, i've, I've, if, in, inside, instead, into, is, isn't, it, it's, its, itself, just, last, least, less, let, let's, letting, likewise, many, may, me, mere, merely, might, more, moreover, most, mostly, much, must, mustn't, my, myself, neither, never, next, no, nobody, nobody's, none, nor, not, nothing, now, nowhere, of, off, often, on, once, one, one's, ones, ones', oneself, only, or, other, others, otherwise, ought, our, ours, ourselves, out, outside, over, own, per, perhaps, quite, rather, same, several, shall, shan't, she, she'd, she'll, she's, should, shouldn't, since, so, some, somebody, somebody's, somehow, someone, someone's, something, sometimes, somewhat, somewhere, soon, sooner, still, such, than, that, that's, the, thee, their, theirs, them, themselves, then, there, there's, thereabout, thereabouts, thereafter, thereat, thereby, therefor, therefore, therefrom, therein, thereof, thereon, thereto, theretofore, thereunder, thereunto, thereupon, therewith, these, they, they'd, they'll, they're, they've, thine, this, those, thou, though, through, thus, thy, thyself, till, to, together, too, toward, towards, under, unless, until, up, upon, us, versus, very, via, was, wasn't, we, we'd, we'll, we're, we've, well, were, weren't, what, what's, whatever, whatsoever, when, whenever, when's, where, where's, whereabouts, whereas, whereat, whereby, wherefore, wherein, whereof, whereon, wheresoever, whereto, whereupon, wherever, wherewith, wherewithal, whether, which, whichever, whichsoever, while, who, who's, whoever, whole, whom, whomever, whomsoever, whose, whosoever, why, why's, whyever, whysoever, will, with, within, without, won't, would, wouldn't, yes, yet, you, you'd, you'll, you're, you've, your, yours, yourself, yourselves,

then we consider it an English stop word.<sup>33</sup> All the English stop words that appear in a particular document need to be ignored before we perform word clustering on the rest of the vocabulary list. □

## 4.2 Modified Porter stemming algorithm for English

The Porter stemming algorithm is a very useful word clustering tool for information retrieval in English [39] and many other European languages [40]. Through a series of string manipulations, the Porter stemming algorithm generates a token (known as “Porter stem”) for an arbitrary word in a given language, without consulting a dictionary. Words sharing the same token are identified with each other in the Porter stemming procedure. While this procedure correctly lumps together morphologically related words in many scenarios, it ignores morphological irregularities that prevail in the vocabularies of many European languages, including English.

In this work, we modify Porter’s stemming algorithm so that it works more accurately on realistic vocabulary lists generated from text mining tasks. Our modification has two aspects. First, instead of associating each word with a unique Porter stem, we construct the token in two stages: a longer stem called *effective spelling*, and a shorter stem called *essential root* (§4.2.1). Second, instead of using exact matching of tokens as a criterion for word clustering, we add some *admissible mutation* rules to accommodate to morphological irregularities, and build an *approximate clustering* algorithm thereupon (§4.2.2).

In English, there are about two hundred irregular verbs in common use. A limited subset of these verbs are highly irregular, and they need to be handled by explicitly written exceptions to rules during the stemming procedure (§4.2.1). The remaining

<sup>32</sup>Our list of English stop words differ from the built-in list in *Mathematica* v11.0 in the following aspects:

- (1) Our list includes – (two hyphens joined together), which accommodates to vintage encoding in certain ebooks;
- (2) Our list includes *shall* and *towards*, to accommodate to British English;
- (3) Our list includes some common function words: *afterward, afterwards, ago, ahead, albeit, amid, amidst, amongst, anyhow, anyway, apart, aside, away, beneath, beside, besides, beyond, else, elsewhere, everybody, everybody's, everyone's, except, front, hardly, hence, hither, inside, instead, just, likewise, neither, oneself, otherwise, outside, somebody, somebody's, someone's, sometimes, somewhat, soon, sooner, thereafter, therein, thereof, thereupon, unless, versus, via* and *yes*;
- (4) Our list includes *thee, thine, thou, thy* and *thyself*, to accommodate to Early Modern English (such as in the works of Shakespeare);
- (5) Our list excludes *find, first, give, go, interest, keep, made, noone, part, put, see, seem, seemed, seeming, seems, show, side* and *take*—while some of these words might appear disposable in certain rudimentary information retrieval tasks, we find it harmful to regard them as stop words for machine comprehension of English texts.

<sup>33</sup>In the list above (and also the substitution rules below), the apostrophe refers to either APOSTROPHE U+0027 or RIGHT SINGLE QUOTATION MARK

U+2019, as is appropriate for the particular text mining task.

majority of these irregular verbs, however, do exhibit systematic vowel/consonant alternation patterns, such as *keep/kept*, *sleep/slept*, *sweep/swept*, *weep/wept*, *break/broke/broken*, *speak/spoke/spoken*, *steal/stole/stolen*. These systematic irregularities are reflexes of historical Germanic vowel mutations, which are also found in modern Danish, German and Dutch (§5). We will treat these vowel alternations with an *admissible mutation* mechanism (§4.2.2).

#### 4.2.1 Effective spelling and essential root

Before deducing analogs of the Porter stem as the *effective spelling* and the *essential root*, we need to regularize some English verbs (Algorithm 4.3) and normalize the vowel lengths in English spelling (Algorithm 4.4). It should be noted that our purpose is to deduce a token for an English word that is suitable for morphological studies, so the token itself does not have to resemble the word's etymological stem (as was in the Porter stemming algorithm): in fact, we are going to exploit a wide assortment of special Latin characters (like the German *ä*, *ö*, *ü*, *ß*, the Spanish *ñ*, and various accented vowels appearing in Romance languages) as well as some Greek letters<sup>34</sup> to construct the effective spelling and essential root of an English word.

**Algorithm 4.3** (Regularization of English verbs). *For an English word  $\hat{\sigma}$ , its “regularized verb form”  $\text{RegVb}(\hat{\sigma})$  is deduced by the following four steps:*<sup>35</sup>

- (1) Do  $X^\infty(a|i)bilitX \rightarrow Xble$ ,  $\hat{\chi}ful(ler|lest|ness)X \rightarrow \hat{\chi}$ , *feet*  $\rightarrow$  *foot*, *heaven*  $\rightarrow$   $\eta\varepsilon ave\tilde{\nu}$ , *ificatX*  $\rightarrow$  *ify*, *ili(s|z)(e|ing)X*  $\rightarrow$  *ility*, *inabilX*  $\rightarrow$  *unable*, *inalien*  $\rightarrow$  *unalien*, *isticX*  $\rightarrow$  *ist*, *positiv*  $\rightarrow$   $\rho\sigma\tau iv$ , *reciprocal*  $\rightarrow$  *reciprocity*, *toricX*  $\rightarrow$  *tory*,  $\sim X^\infty(\text{barb|hil})arit(ies|y) \rightarrow Xarious$ ,  $\sim X^\infty(c|d|g|n)uit(ies|y) \rightarrow Xuous$ ,  $\sim alit(ies|y) \rightarrow al$ ,  $\sim arit(ies|y) \rightarrow ar$ ,  $\sim charit(ies|y) \rightarrow charitable$ ,  $\sim circuit(ies|y) \rightarrow circuitous$ ,  $\sim enmit(ies|y) \rightarrow enemy$ ,  $\sim femini(\emptyset|ni)t(ies|y) \rightarrow feminine$ ,  $\sim idit(ies|y) \rightarrow id$ ,  $\sim lar(hy|s) \rightarrow lar$ ,  $\sim necessit(ies|y) \rightarrow necessary$ ,  $\sim ntit(ies|y) \rightarrow ntify$ ,  $\sim simplicit(ies|y) \rightarrow simple$ ,  $\sim tricit(ies|y) \rightarrow tric$ ,  $\sim vanit(ies|y) \rightarrow vain$ ,  $\sim virgin(\emptyset|s) \rightarrow virginity$ .
- (2) In a single sweep, perform replacements according to the following substitution rules:

|                                                   |                                                           |                       |                                          |
|---------------------------------------------------|-----------------------------------------------------------|-----------------------|------------------------------------------|
| $\hat{\chi}\notin(i)aris(m t)X$                   | $\hat{\chi}\notin(s t)tress$                              | (Us Usa)              | $X^\infty(\emptyset un)dece(it pt)X\sim$ |
| $\hat{\chi}ial$                                   | $\hat{\chi}tor$                                           | American              | Xdeceive                                 |
| $X^\infty(\text{alchem narch})is(m t)X$           | $X^\infty(\text{ap im multi})pl(y)(ieX)$                  |                       | $X^\infty(\text{at g ic it iv nt})ious$  |
| $Xy$                                              | Xplication                                                |                       | Xion                                     |
| $X^\infty(b h)ang(ed ing)\sim$                    | $X^\infty(\text{cent cloist integ neut sepulch spect})er$ |                       |                                          |
| Xang                                              | Xre                                                       |                       |                                          |
| $X^\infty(\text{con miskon per precon})ceptX\sim$ | $a(c n)eousX$                                             | <i>ancestress</i>     | <i>avuncularX</i>                        |
| Xceive                                            | al                                                        | ancestor              | uncle                                    |
| <i>Belgium</i>                                    | <i>breadth</i>                                            | <i>buri</i>           | <i>bury</i>                              |
| <i>capric</i>                                     | <i>Belgian</i>                                            | <i>broad</i>          | $\beta upi$                              |
| <i>children</i>                                   | <i>choice</i>                                             | <i>clar</i>           | <i>comic</i>                             |
| <i>child</i>                                      | <i>choose</i>                                             | <i>clear</i>          | <i>comedic</i>                           |
| <i>condition</i>                                  | <i>contemporX</i>                                         | <i>crash</i>          | <i>demptX</i>                            |
| <i>Denmark</i>                                    | <i>earn</i>                                               | <i>ength</i>          |                                          |
| <i>child</i>                                      | <i>choose</i>                                             | <i>clear</i>          | <i>comedic</i>                           |
| <i>condition</i>                                  | <i>contempor</i>                                          | <i>krash</i>          | <i>deem</i>                              |
| <i>Danish</i>                                     | <i>earn</i>                                               | <i>ong</i>            |                                          |
| $\text{flect}(on ve)X$                            | <i>flower</i>                                             | $\text{focusX}$       | <i>France</i>                            |
| <i>fraternX</i>                                   | <i>grove</i>                                              | <i>hall</i>           | <i>homage</i>                            |
| <i>hour</i>                                       | $\text{iaris}(m t)X$                                      |                       |                                          |
| <i>flect</i>                                      | $\varphi lower$                                           | <i>focus</i>          | <i>French</i>                            |
| <i>brother</i>                                    | $\gamma rove$                                             | $\zeta al$            | <i>homage</i>                            |
| <i>ora</i>                                        | <i>iary</i>                                               |                       |                                          |
| <i>idiot</i>                                      | <i>inguish</i>                                            | <i>instab</i>         | <i>Ireland</i>                           |
| <i>ironi(c es)X</i>                               | <i>ironing</i>                                            | <i>irony</i>          | <i>Italy</i>                             |
| <i>Korean</i>                                     | <i>iron</i>                                               | <i>irony</i>          | <i>Italy</i>                             |
| <i>idiot</i>                                      | <i>inct</i>                                               | <i>unstab</i>         | <i>Irish</i>                             |
| <i>irony</i>                                      | <i>irony</i>                                              | <i>irony</i>          | <i>Italian</i>                           |
| <i>Korea</i>                                      |                                                           |                       |                                          |
| $\text{langu}(id or)X\sim$                        | <i>laughter</i>                                           | <i>leg</i>            | <i>lesson</i>                            |
| $\text{ma}(\uparrow d)am$                         | $\text{maritX}\sim$                                       | $\text{maternX}\sim$  | $\text{matrimonX}\sim$                   |
| <i>membran</i>                                    | <i>languish</i>                                           | <i>laugh</i>          | <i>ley</i>                               |
| <i>lekcion</i>                                    | $\varphi ru$                                              | <i>marry</i>          | <i>mother</i>                            |
| <i>marry</i>                                      | <i>mother</i>                                             | <i>marry</i>          | <i>membrañ</i>                           |
| <i>menace</i>                                     | $\text{mentalitX}$                                        | <i>Mexico</i>         | <i>mistress</i>                          |
| $\text{mound}$                                    | $\text{mourn}\sim$                                        | $\text{pacifX}\sim$   | $\text{paternX}\sim$                     |
| <i>polite</i>                                     | <i>promis</i>                                             | <i>prophetX</i>       |                                          |
| <i>meñace</i>                                     | <i>mental</i>                                             | <i>Mexican</i>        | <i>master</i>                            |
| <i>mound</i>                                      | $\mu ound$                                                | $\mu ounn$            | <i>peace</i>                             |
| <i>father</i>                                     | $\pi lite$                                                | $\pi rowmis$          | <i>prophetic</i>                         |
| <i>publish</i>                                    | <i>rash</i>                                               | $\text{rebellionX}$   | $\text{rece}(ipt pt)X\sim$               |
| <i>roof</i>                                       | <i>salar</i>                                              | <i>satin</i>          | <i>satir</i>                             |
| <i>publication</i>                                | <i>pash</i>                                               | <i>rebel</i>          | <i>receive</i>                           |
| $\rho ooof$                                       | $\sigma alar$                                             | $\sigma atin$         | $\sigma batir$                           |
| $\text{scienti}(fic st)X$                         | <i>Scotland</i>                                           | <i>severed</i>        | $\text{sororX}\sim$                      |
| <i>sow</i>                                        | <i>Spain</i>                                              | <i>species</i>        | $\text{sticitX}$                         |
| <i>tenab</i>                                      | <i>tenacX</i>                                             | <i>tenant</i>         |                                          |
| <i>science</i>                                    | <i>Scottish</i>                                           | <i>sever</i>          | <i>sister</i>                            |
| $\sigma ow$                                       | <i>Spanish</i>                                            | $\sigma piece\sigma$  | <i>stic</i>                              |
| $\tau e\tilde{\nu}ab$                             | <i>tenac</i>                                              | $\tau e\tilde{\nu}ab$ | <i>tenac</i>                             |
| $\tau e\tilde{\nu}ant$                            |                                                           |                       |                                          |
| <i>tender</i>                                     | <i>tenet</i>                                              | <i>tenta</i>          | $\text{theoriX}\sim$                     |
| <i>ticianX</i>                                    | <i>town</i>                                               | <i>traged</i>         | <i>Ukraine</i>                           |
| <i>usur</i>                                       | <i>Wales</i>                                              |                       |                                          |
| $\tau e\tilde{\nu}der$                            | $\tau en\epsilon\tau$                                     | $\tau ent\alpha$      | <i>theory</i>                            |
| <i>tical</i>                                      | <i>town</i>                                               | <i>tragic</i>         | <i>Ukrainian</i>                         |
| <i>usur</i>                                       | <i>Wales</i>                                              |                       |                                          |

<sup>34</sup>The Greek letter  $\beta$  should not be confused with German  $\beta$ .

<sup>35</sup>Not all these substitutions operate on verbs, yet most of them are conducive to correct clustering of certain verbs. For example, *missile* and *mission* should not be merged with *miss*( $\emptyset|ed|es|ing$ ), and *passion* should be separated from *pass*( $\emptyset|ed|es|ing$ ). The word family *attent*(*ion|ive|ive|ly*) was indeed etymologically related to the verb *attend*, but their modern meanings are well separated. To avoid such a conflation, while guaranteeing the correct grouping of *inten*(*d|t*), *exten*(*d|t*) and so on, we need to alter the spelling *attend*-. A diligent reader may find the rationale behind the other entries in our substitution rules.

|                                                                         |                                                   |                                                                           |                      |                                      |                                               |                                                                          |                                             |                    |                     |                |
|-------------------------------------------------------------------------|---------------------------------------------------|---------------------------------------------------------------------------|----------------------|--------------------------------------|-----------------------------------------------|--------------------------------------------------------------------------|---------------------------------------------|--------------------|---------------------|----------------|
| $weari_{\hat{x}\notin(n)}\mathbf{X}$<br>$\omega\epsilon\alpha\pi$       | $weary\mathbf{X}$<br>$\omega\epsilon\alpha\pi$    | $woke$<br>$wake$                                                          | $worr$<br>$wopr$     | $chagrin(\emptyset s)$<br>$chagrine$ | $conic(\emptyset al)(\emptyset ly)$<br>$cone$ | $good$<br>$\gamma\omega\delta$                                           | $hung$<br>$hang$                            | $made$<br>$make$   | $radii$<br>$radius$ | $ran$<br>$run$ |
| $sis$<br>$sister$                                                       | $ten(\emptyset s)(th\mathbf{X})$<br>$l\theta ten$ | $\sim\hat{x}\notin(a e i o u)ar(\emptyset ies ily ize y)$<br>$\hat{x}ial$ |                      |                                      | $\sim\hat{x}\notin(p)lus$<br>$\hat{x}li$      |                                                                          |                                             |                    |                     |                |
| $\sim(is iz)(ab able ation e ed ement er ing)(\emptyset ly s)$<br>$ize$ |                                                   |                                                                           |                      |                                      |                                               | $\sim\mathbf{X}^\epsilon(atr fer prec)ocit(ies y)$<br>$\mathbf{X}ocious$ |                                             |                    |                     |                |
| $\sim acit(ies y)$<br>$acious$                                          | $\sim antal$<br>$ance$                            | $\sim antas(ies y)$<br>$antasize$                                         | $\sim ics$<br>$ical$ | $\sim istry$<br>$ister$              | $\sim monopol(ies y)$<br>$monopolize$         | $\sim nness$<br>$n$                                                      | $\sim radical(\emptyset s)$<br>$radicalize$ | $\sim uum$<br>$ua$ |                     |                |

- (3)  $Do$   $\epsilon\alpha rnest \rightarrow \epsilon\alpha\alpha\rho n\epsilon\sigma\tau$ ,  $\mathbf{X}^\epsilon(a|i|o|u)si(on|ve)\mathbf{X} \rightarrow \mathbf{X}de$ ,  $abdomen \rightarrow ab\delta\alpha\mu\iota n$ ,  $beautical \rightarrow beauty$ ,  $began \rightarrow begin$ ,  $caus\mathbf{X}^\epsilon(a|e|i) \rightarrow \kappa\omega\zeta\mathbf{X}$ ,  $comedo \rightarrow \kappa\omicron\mu\epsilon\delta\omicron$ ,  $criti(c|que)(\emptyset|al)(\emptyset|ly) \sim \rightarrow criticize$ ,  $deer \rightarrow d\epsilon\epsilon r$ ,  $hung \sim \rightarrow \varphi\alpha\iota\mu$ ,  $pretent \sim \rightarrow pretend$ ,  $repeat\mathbf{X} \rightarrow repetition$ ,  $savage \rightarrow \sigma\alpha\beta\alpha\gamma\epsilon$ ,  $serious \rightarrow \sigma\epsilon rious$ ,  $sever(e|it) \rightarrow \sigma\epsilon\omega\epsilon r\epsilon$ ,  $suffer \rightarrow \sigma\omega\upsilon\phi\epsilon r$ ,  $suspici \rightarrow suspect$ ,  $tent \sim \rightarrow tent$ ,  $tranquil(\emptyset|l)iz\mathbf{X} \rightarrow tranquil$ ,  $weariness\mathbf{X} \rightarrow \omega\epsilon\alpha\pi$ ,  $\sim(risen|rose) \rightarrow rize$ ,  $\sim\hat{x}tic(\emptyset|al)(\emptyset|ly)(iz\mathbf{X}) \rightarrow \hat{x}sis$ ,  $\sim s \rightarrow \emptyset$ .

(4) *Replace*

|                                                                                                                   |                                                                                     |                                                         |                                                       |                                                                      |                                                           |                                               |                                        |                         |                               |                        |
|-------------------------------------------------------------------------------------------------------------------|-------------------------------------------------------------------------------------|---------------------------------------------------------|-------------------------------------------------------|----------------------------------------------------------------------|-----------------------------------------------------------|-----------------------------------------------|----------------------------------------|-------------------------|-------------------------------|------------------------|
| $\sim$<br>$\emptyset$                                                                                             | $\mathbf{X}^\epsilon(ab pre)sence$<br>$\mathbf{X}sent$                              | $\mathbf{X}^\epsilon(ad de)vi(c z)$<br>$\mathbf{X}vis$  | $\mathbf{X}^\epsilon(col e)lid$<br>$\mathbf{X}lis$    | $\mathbf{X}^\epsilon(de of)fen(c s)$<br>$\mathbf{X}fend$             | $\mathbf{X}^\epsilon(di pro)vid$<br>$\mathbf{X}vis$       |                                               |                                        |                         |                               |                        |
| $\mathbf{X}^\epsilon(dissatis lique petri putre rare satis stupe vitri)ff(ielied ies y ying)$<br>$\mathbf{X}fact$ |                                                                                     |                                                         |                                                       |                                                                      |                                                           |                                               |                                        |                         |                               |                        |
| $\mathbf{X}^\epsilon(g i r s)onal(\emptyset i ly)\mathbf{X}$<br>$\mathbf{X}on$                                    | $\mathbf{X}^\epsilon(k K)ing\sim$<br>$\mathbf{X}oenig$                              | $\mathbf{X}^\epsilon(mpl rt tr)aint$<br>$\mathbf{X}ain$ | $attend\sim$<br>$attenzd$                             | $aur$<br>$a\omega r$                                                 | $automation$<br>$automasis$                               |                                               |                                        |                         |                               |                        |
| $begg(ar ed)\sim$<br>$beg$                                                                                        | $counten$<br>$kouten$                                                               | $de\mathbf{X}^\epsilon(c r)id$<br>$de\mathbf{X}is$      | $duct(\emptyset ion)$<br>$duce$                       | $dye$<br>$dzye$                                                      | $expence$<br>$expense$                                    | $explain\sim$<br>$explan$                     | $flatter$<br>$flatter$                 |                         |                               |                        |
| $forg(e o)t(\emptyset ten)\mathbf{X}$<br>$vye\beta$                                                               | $former\sim$<br>$\varphi\omicron rmer$                                              | $four$<br>$\varphi our$                                 | $inal(\emptyset i ly)\mathbf{X}$<br>$in$              | $licen(c s)\sim$<br>$licent$                                         | $listen$<br>$lisztzn$                                     | $mad$<br>$\mu\varphi\alpha\delta$             | $mention$<br>$menzzion$                | $migrant$<br>$migrate$  | $missile$<br>$missle$         |                        |
| $mission$<br>$mit$                                                                                                | $passion$<br>$patzion$                                                              | $pool$<br>$powl$                                        | $possess$<br>$pozzezz$                                | $preceden(c t)$<br>$precezz\beta$                                    | $prett$<br>$pr\epsilon\epsilon t$                         | $prevail\sim$<br>$preval$                     | $prevent\sim$<br>$prezvent$            | $rouse$<br>$rzouse$     | $solde\sim$<br>$soldq$        | $soldi\sim$<br>$soldw$ |
| $sump$<br>$sume$                                                                                                  | $temper$<br>$temp\epsilon r$                                                        | $thought$<br>$think$                                    | $typ\sim$<br>$zyp$                                    | $warn\sim$<br>$wxarn$                                                | $(flew flown)$<br>$fly$                                   | $(mete meted metes meting metings)$<br>$mzet$ |                                        |                         |                               |                        |
| $(ridden rode)$<br>$ride$                                                                                         | $\mathbf{X}^\epsilon(\emptyset in mis off out over p under)led$<br>$\mathbf{X}lead$ |                                                         |                                                       | $\mathbf{X}^\epsilon(\emptyset s)lain$<br>$\mathbf{X}lay$            | $\mathbf{X}^\epsilon(b br c l r)ook$<br>$\mathbf{X}ooked$ |                                               |                                        |                         |                               |                        |
| $brought$<br>$bring$                                                                                              | $caught$<br>$catch$                                                                 | $eat(\emptyset en ing s)$<br>$ate$                      |                                                       | $lad(\emptyset die dish hood)(\emptyset s)$<br>$\lambda\alpha\delta$ |                                                           | $meant$<br>$mean$                             | $sought$<br>$seek$                     | $taught$<br>$teach$     | $won$<br>$win$                |                        |
| $(\sim sis siz)$<br>$ses$                                                                                         | $\sim(did does doing done)$<br>$do$                                                 |                                                         |                                                       | $\sim(goes going gone went)$<br>$go$                                 |                                                           |                                               | $\sim bought$<br>$buy$                 | $\sim came$<br>$come$   |                               |                        |
| $\sim ced(e ed es ing)$<br>$cez\beta$                                                                             | $\sim ered$<br>$er$                                                                 | $\sim gave$<br>$give$                                   | $\sim\mathbf{X}$ -in-law<br>$\lambda\omega\mathbf{X}$ | $\sim heard$<br>$hear$                                               | $\sim itten$<br>$iten$                                    | $\sim rnt$<br>$rn$                            | $\sim see(\emptyset ing n s)$<br>$saw$ | $\sim stood$<br>$stand$ | $\sim visor$<br>$vis\epsilon$ |                        |

The silent *e* in English spelling may affect the length of the immediately preceding vowel. Pairs of words like *hat/hate* and *rat/rate* are etymologically unrelated. Motivated by modern Dutch orthography (§5.3.1), we will introduce a heuristic procedure to mark the vowel lengths in English words explicitly. This procedure not only detects long vowels in **CVCe** patterns, but also words derived therefrom. (For example, the vowel *o* in *devote*, *devoting* and *devotion* should all be consistently marked as long.)

**Algorithm 4.4** (Normalization of English vowel lengths). *For a text string  $\hat{\sigma}$ , its “normalized English vowel length form”  $\text{NormVL}(\hat{\sigma})$  is determined through the following procedure:*

- (1) *If  $\hat{\sigma}$  comes from a word that is “heuristically capitalized” (Definition 4.1), then  $\text{NormVL}(\hat{\sigma}) = z\hat{\sigma}'$  where  $\hat{\sigma}'$  results from doing  $\sim ean(\emptyset|s) \rightarrow \emptyset$  on  $\hat{\sigma}$ .<sup>36</sup>*

<sup>36</sup>Here, the prefix “zx” push the word down to the end of an alphabetized list later. In English, the ending  $\sim ean$  is found mainly in adjectives (and nouns) deriving from proper nouns. The procedure here ensures that words like *Argentine*( $\emptyset|an$ )( $\emptyset|s$ ), *Boole*( $\emptyset|an$ ) and *Euclid*( $\emptyset|ean$ ) *Europe*( $\emptyset|an$ )( $\emptyset|s$ ) are clustered properly.

(2) Otherwise, perform the following substitutions, in five sequential sweeps:

(2.1) Do  $\sim\text{osit}(\text{ies|y}) \rightarrow \text{ous}$ ,  $\sim\hat{\chi}\hat{\chi}\text{oe}(\emptyset|\text{d|s}) \rightarrow \hat{\chi}\hat{\chi}\text{o}$ .

(2.2) Replace<sup>37</sup>

| (lose loss)                                   | $\hat{\chi}tr$  | $X^\infty(\text{dis ex pre})\text{tens}$ | $X^\infty(\text{ex sus})\text{pens}$                               |
|-----------------------------------------------|-----------------|------------------------------------------|--------------------------------------------------------------------|
| lost                                          | $\hat{\chi}ter$ | Xtend                                    | Xpend                                                              |
| $X^\infty(\hat{\chi}(\text{a o})\text{tion})$ | au capab~       | deep( $\emptyset \text{eX}$ )            | earl(i y)~ eed fer fine~                                           |
| Xtiv                                          | aau kapab       | depth                                    | earzli ezß fér fizne free gazß jenerat gjenero ll                  |
| manner mere~ mode~                            | neer oe oo      | pre~ puls                                | quiet rough side~ some- soul ss static stel~                       |
| mazzner mzere modz                            | ne oue ú        | pré pel                                  | cquiet rouffgh szide somz szoul zß sztatic sztel                   |
| sudden~ summer                                | ton~ water~     | women                                    | idl(est y) genera gently singly ski( $\emptyset \text{ed ing s}$ ) |
| swudden suzmmmer                              | twon wazter     | woman                                    | idle genus gentle single szki                                      |

(2.3) Replace every occurrence of double letter by a corresponding single capital letter (i.e.  $ee \rightarrow E$  etc.).

(2.4) Set  $C_1$  as any lowercase English letter<sup>38</sup> other than  $\{a, e, i, o, u, y\}$ ,  $V$  as any one among  $\{a, e, i, o, u\}$ , and  $C_2$  as any lowercase English letter other than  $\{a, e, i, o, u, w, y\}$ . Define  $V^+$  as the capital form of the vowel  $V$ . Replace<sup>39</sup>

| $C_1 V (X^\infty((C_2(\text{ag al a}\lambda \text{at e ing ion ish it iv ous})))\text{ck gh nd}))$ | ang(e ing) |
|----------------------------------------------------------------------------------------------------|------------|
| $C_1 V^+ X$                                                                                        | Ange       |

(2.5) Replace<sup>40</sup>

| A  | E  | é | I | lezß  | O  | T  | ú  | U | λ  | gOv~ | inter~ | be(Ter st) |
|----|----|---|---|-------|----|----|----|---|----|------|--------|------------|
| aa | ee | e | í | zlezß | óó | tt | oo | u | ll | góv  | jntr   | γowδ       |

before converting the string to lowercase.

With the preparations above, we can derive the effective spelling of an English word. The effective spelling (to be derived in Algorithm 4.5) is a conservative estimate for the (etymologically correct) word stem, which usually has longer string length than the essential root (to be derived in Algorithm 4.8).

**Algorithm 4.5** (English effective spelling). For an English word  $\hat{\sigma}$ , its effective spelling  $\text{EffSpell}(\hat{\sigma})$  is constructed in seven sequential steps:

(1) Take  $\text{NormVL}(\text{RegVb}(\hat{\sigma}))$ , and perform the following replacements in a single sweep:

|                  |    |         |     |        |                                         |          |                                |            |       |     |            |    |    |    |      |
|------------------|----|---------|-----|--------|-----------------------------------------|----------|--------------------------------|------------|-------|-----|------------|----|----|----|------|
| $\hat{\chi}aid$  | ck | clamat  | emn | enten  | family                                  | gral     | ióón                           | iv         | la    | ld  | lóó        | ng | oi | ou | ply  |
| $\hat{\chi}ayed$ | c  | claimat | μn  | entzen | families                                | graation | ion                            | ív         | lóa   | llz | lo         | zñ | zö | í  | plie |
| rd               | sh | tim     | ui  | ye     | $\sim'(\emptyset \text{s}) \emptyset '$ | ~ant     | ~ble( $\emptyset \text{d s}$ ) | ~hie(r st) | ~ook  | ~s  | - (hyphen) |    |    |    |      |
| rzd              | š  | ztim    | zü  | yme    | ∅                                       | ance     | bly                            | hy         | aaken | ∅   | ∅          |    |    |    |      |

(2) Replace

|                     |                               |           |                                                       |      |                           |                           |      |                                  |                  |
|---------------------|-------------------------------|-----------|-------------------------------------------------------|------|---------------------------|---------------------------|------|----------------------------------|------------------|
| $\hat{\chi}ied\sim$ | $C_1^\infty(\text{c w})a\sim$ | $ba\sim$  | $C_2^\infty(\text{s t w})X^\infty(\text{e o óó})\sim$ | dóó~ | $f^{N_1}(\text{a e})\sim$ | $f^{N_2}(\text{i í})\sim$ | móó~ | $\text{dad}(\emptyset \text{y})$ | $m(\text{o u})m$ |
| $\hat{\chi}ieed$    | $C_1\beta a$                  | $\beta a$ | $C_2zX$                                               | δo   | $\varphi V_1$             | $ff V_2$                  | μo   | φαther                           | mother           |

(3) Do  $\sim f(\emptyset|e) \rightarrow ve$ ,  $\sim xe \rightarrow x$ ,  $\sim\hat{\chi}\hat{\chi}\hat{\chi}ly \rightarrow \hat{\chi}\hat{\chi}\hat{\chi}$  (i.e. remove final "ly" if it is preceded by at least three letters).

(4) Do  $h(i|i) \rightarrow h\acute{i}$ ,  $lu \rightarrow lvu$ ,  $y \rightarrow ie$ .

(5) Do  $\sim\hat{\chi}\hat{\chi}\hat{\chi}(\text{tic|tion}) \rightarrow \hat{\chi}\hat{\chi}\hat{\chi}t$ ,  $\sim\hat{\chi}\hat{\chi}\hat{\chi}(\text{age|ed|ful|ical|izñ|izñ|ment|nezß}) \rightarrow \hat{\chi}\hat{\chi}\hat{\chi}$ .

<sup>37</sup>As we do  $\text{deep}(\emptyset|\text{eX}) \rightarrow \text{depth}$  to the words *deep*, *deeper*, *deepest*, *deeply*, we obtain *depth*, *depth*, *depth*, *depthly*. (In *Mathematica*, the command `StringReplace[{"deep", "deeper", "deepest", "deeply"}, {"deep"~~~|"e"~~~} :> "depth"]` results in `{"depth", "depth", "depth", "depthly"}`.) Here, the wildcard symbol  $X \in \{r, st\}$  is deleted after replacement, because  $X$  does not reappear in the destination string  $\hat{\sigma}' = \text{depth}$  (cf. Definition 3.6).

<sup>38</sup>A letter is an English letter if and only if it is one of the 26 members in the ISO basic Latin alphabet.

<sup>39</sup>For readers' benefit, we point out that the corresponding *Mathematica* substitution rules are `{(C1: Except["e"|"i"|"o"|"u"|"y", CharacterRange["b", "z"]])~(V: "a"|"e"|"i"|"o"|"u"~(X: (Except["e"|"i"|"o"|"u"|"w"|"x"|"y", CharacterRange["b", "z"]])~"ag"|"al"|"aλ"|"at"|"e"|"ing"|"ish"|"it"|"ous")|"ck"|"gh"|"nd") :> C1 <> ToUpperCase[V] <> X, "ang"~~"e"|"ing" :> "Ange"}`. As our substitutions disallow overlaps, the letter *e* in patterns like *ndering* (as in *plundering*, *pondering*) will not be marked as a long vowel.

<sup>40</sup>Note that during a single sweep, the longer matches take priority over shorter matches. Therefore, the result  $\text{NormVL}(\text{government}) = \text{góvnerment}$  does not contain *óó*.

## (6) Replace

|                 |                     |           |           |           |           |            |                  |           |                                          |                           |                                     |           |            |
|-----------------|---------------------|-----------|-----------|-----------|-----------|------------|------------------|-----------|------------------------------------------|---------------------------|-------------------------------------|-----------|------------|
| $(eft iev iev)$ | $(o ó)X^{\in}(p r)$ | <i>ch</i> | <i>ea</i> | <i>ir</i> | <i>ll</i> | <i>mi~</i> | <i>ph</i>        | <i>th</i> | $\sim\hat{x}\notin(d)ent(\emptyset ive)$ | $\sim X^{\in}(pell s)ion$ | $\sim\hat{x}\hat{x}\hat{x}i\hat{s}$ | $\sim lt$ | $\sim own$ |
| <i>äive</i>     | $\hat{o}X$          | <i>č</i>  | <i>ää</i> | <i>ir</i> | $\lambda$ | <i>mi</i>  | $\varphi\varphi$ | $\theta$  | $\hat{x}eend$                            | $Xiv$                     | $\hat{x}\hat{x}\hat{x}$             | <i>l</i>  | <i>ow</i>  |

(7) Replace<sup>41</sup>

|             |                             |                                                                                            |                                                                                             |
|-------------|-----------------------------|--------------------------------------------------------------------------------------------|---------------------------------------------------------------------------------------------|
| <i>beg</i>  | $d\hat{a}\hat{a}(d \theta)$ | $\hat{x}_1X_1\hat{x}_2\notin(e i)e$                                                        | $zxX_3$                                                                                     |
| <i>bbeg</i> | <i>die</i>                  | $\hat{x}_1X_1\hat{x}_2ae$ , if $\hat{x}_1X_1 = zxX_2$ ; $\hat{x}_1X_1\hat{x}_2$ otherwise. | $zx\tilde{X}_3$ , where $\tilde{X}_3$ results from doing $\sim ie \rightarrow y$ on $X_3$ . |

Here, “ $\hat{x}_1X_1 = zxX_2$ ” means that the string  $\hat{x}_1X_1$  begins with two letters “zx”.

Up to the current stage, we have introduced many non-English letters into the tokens assigned to English words. Some of these non-English letters will be regarded as extensions to the set of English vowels.

**Definition 4.6** (English Vowel Extensions). Hereafter in §4, the symbol  $V^*$  stands for any member from the list  $\{a, \hat{a}, e, i, \hat{i}, \hat{l}, \hat{o}, \hat{o}, \hat{u}, \hat{u}\}$ , the so-called English vowel extensions. In line with the multiplicity notations introduced in Definition 3.3, the symbol  $V_m^*$  stands for a text string formed by consecutive appearance of one or more (not necessarily identical or distinct) members from the set of English vowel extensions.

Dual to the notations above, the symbol  $C^*$  stands for any character that does not belong to the list  $\{a, \hat{a}, e, i, \hat{i}, \hat{l}, \hat{o}, \hat{o}, \hat{u}, \hat{u}\}$ , and  $C_{m_0}^*$  stands for a text string formed by consecutive appearance of zero or more (not necessarily identical or distinct) characters that do not belong to the same list.  $\square$

As mentioned before, the conservative effective spelling algorithm assigns a long token to an English word, while the aggressive essential root algorithm will produce a short token, removing as many final letters as “appropriate”. To ensure “appropriateness” during the short token generation, we need to explicitly label some part of an English word as unremovable. The string length of this unremovable part is called the English protected range, as defined below.

**Definition 4.7** (English protected range). Let  $\hat{\sigma}$  be the effective spelling of an English word, its protected range  $\text{ProtRg}(\hat{\sigma})$  is an integer determined as follows:<sup>42</sup>

- Look for the string pattern  $(\emptyset|be|cinter|co|c\hat{o}|dee|di|\hat{f}|\hat{h}|\hat{m}|\hat{p}|\hat{p}|\hat{r}\hat{o}\hat{o}|rV_m^*|ster|su|te|V_m^*)C_{m_0}^*V_m^*\sim$  in the string  $\hat{\sigma}$ ;
- If the string pattern above is found, the last position occupied by such a string defines  $\text{ProtRg}(\hat{\sigma})$ ; otherwise, set  $\text{ProtRg}(\hat{\sigma}) = 0$ .  $\square$

*Example 4.7.1.* Let  $\hat{\sigma} = TNT$ , then  $\text{EffSpell}(\hat{\sigma}) = zTNT$ , and  $\text{ProtRg}(\text{EffSpell}(\hat{\sigma})) = 0$ ; let  $\hat{\sigma} = trinitrotoluene$  (the IUPAC name for TNT), then  $\text{EffSpell}(\hat{\sigma}) = tr\hat{i}n\hat{i}t\hat{e}r\hat{o}l\hat{u}e\hat{n}$ , and  $\text{ProtRg}(\text{EffSpell}(\hat{\sigma})) = 3$ .

*Example 4.7.2.* Let  $\hat{\sigma} = DDT$ , then  $\text{EffSpell}(\hat{\sigma}) = zxDDT$ , and  $\text{ProtRg}(\text{EffSpell}(\hat{\sigma})) = 0$ ; let  $\hat{\sigma} = 1,1'-(2,2,2\text{-trichloroethane-1,1-diyl})bis(4\text{-chlorobenzene})$  (the IUPAC name for DDT), then

$$\text{EffSpell}(\hat{\sigma}) = 1,1(2,2,2\text{tri}\hat{c}\hat{l}\hat{o}\hat{r}\hat{i}\hat{e}\hat{\theta}aane1,1\hat{d}i\hat{e}l)bi(4\hat{c}\hat{l}\hat{o}\hat{r}\hat{o}\hat{b}enzeen),$$

and  $\text{ProtRg}(\text{EffSpell}(\hat{\sigma})) = 39$ . Here is how the effective spelling looks like with its first 39 characters underlined:

$$1,1(2,2,2\text{tri}\hat{c}\hat{l}\hat{o}\hat{r}\hat{i}\hat{e}\hat{\theta}aane1,1\hat{d}i\hat{e}l)bi(4\hat{c}\hat{l}\hat{o}\hat{r}\hat{o}\hat{b}enzeen).$$

We note that the string pattern of interest here is counted from an internal word boundary (the numerical digit 4).

**Algorithm 4.8** (English essential root). Let  $\hat{\sigma}$  be the effective spelling of an English word, then its corresponding essential root  $\text{EssRoot}(\hat{\sigma})$  is constructed in the following steps:

- (1) Break down  $\hat{\sigma} = \hat{\sigma}_1\hat{\sigma}_2$  into the concatenation of two strings  $\hat{\sigma}_1 = \hat{\sigma}^{[\text{ProtRg}(\hat{\sigma})]}$  (see the notation in Definition 3.1) and  $\hat{\sigma}_2$ , where the length of the first string  $\ell(\hat{\sigma}_1) = \text{ProtRg}(\hat{\sigma})$  is equal to the protected range of  $\hat{\sigma}$ .
- (2) On  $\hat{\sigma}_2$ , perform the following substitutions in a sequel:<sup>43</sup>

<sup>41</sup>Here, the status of heuristic capitalization affects our final treatments. If a word is heuristically capitalized, its final *e* (not preceded by *e* or *i*) will be altered to *ae*; if a word is heuristically uncapitalized, its final *e* (not preceded by *e* or *i*) will be removed. Furthermore, if a word is heuristically capitalized, its final *ie* will be changed to *y*.

<sup>42</sup>Roughly speaking, we want to protect an English word up to its first vowel (or vowel cluster) counting from an internal or external word boundary, bypassing some common prefixes.

<sup>43</sup>In other words, the core algorithm for essential root extraction runs as follows: keep the last “strong” vowel *a*, *i*, *o* or *u* in non-final position, plus one subsequent letter; delete final *a*; erase the final appearance of *e* and all the letters thereafter.

(2.1) Do  $\sim \hat{\chi}^{\in}(a|\hat{i}|o|u)^{\mathbf{X}^{\in}(a|\hat{i}|o|u)_m} \rightarrow \hat{\chi}\mathbf{X}_1$ , where  $\mathbf{X}_1$  is the first character in  $\mathbf{X}$ .

(2.2) Do  $\sim a \rightarrow \emptyset$ .

(2.3) Do  $\sim e(\overline{e})_{m_0} \rightarrow \emptyset$ .

The result after these three steps of operations is called  $\hat{\sigma}'_2$ .

(3) Concatenate  $\hat{\sigma}_1$  and  $\hat{\sigma}'_2$ .

(4) Do  $\sim pel \rightarrow pel$ ,  $\underline{reebel} \rightarrow reebel$ .

*Example 4.8.1.* Let  $\hat{\sigma}$  be the IUPAC name for TNT, then  $\text{EssRoot}(\text{EffSpell}(\hat{\sigma})) = \textit{tr\~{i}n\~{i}t\~{e}r\~{o}t\~{o}l\~{v}u}$ . Let be the IUPAC name for DDT, then  $\text{EssRoot}(\text{EffSpell}(\hat{\sigma})) = 1,1(2,2,\textit{2tri\~{c}l\~{o}r\~{i}e\~{t}h\~{a}a\~{n}e\~{1},\textit{1di\~{e}l})\textit{bi}(4\~{c}l\~{o}r\~{o}b\~{e}n\~{z}e)$ . Note, in particular, that in the latter example, the last internal word boundary (closing parenthesis) is preserved in the essential root.

*Example 4.8.2.* Here are more examples showing how the functions  $\text{RegVb}$ ,  $\text{NormVL}$ ,  $\text{EffSpell}$ ,  $\text{EssRoot}$  act on some etymologically related words.

| $\hat{\sigma}$          | $\text{RegVb}(\hat{\sigma})$ | $\text{NormVL}(\text{RegVb}(\hat{\sigma}))$ | $\text{EffSpell}(\hat{\sigma})$        | $\text{EssRoot}(\text{EffSpell}(\hat{\sigma}))$ |
|-------------------------|------------------------------|---------------------------------------------|----------------------------------------|-------------------------------------------------|
| <i>environment</i>      | <i>environment</i>           | <i>environment</i>                          | <i>env\~{i}ron</i>                     | <i>env\~{i}ron</i>                              |
| <i>environmental</i>    | <i>environmental</i>         | <i>environmental</i>                        | <i>env\~{i}ron\~{m}ental</i>           | <i>env\~{i}ron\~{m}</i>                         |
| <i>environmentalist</i> | <i>environmentalist</i>      | <i>environmentalist</i>                     | <i>env\~{i}ron\~{m}ental\~{i}st</i>    | <i>env\~{i}ron\~{m}</i>                         |
| <i>protect</i>          | <i>protect</i>               | <i>pr\~{o}t\~{e}ct</i>                      | <i>pr\~{o}t\~{e}ct</i>                 | <i>pr\~{o}t\~{e}ct</i>                          |
| <i>protection</i>       | <i>protection</i>            | <i>pr\~{o}t\~{e}ct\~{i}o\~{n}</i>           | <i>pr\~{o}t\~{e}ct</i>                 | <i>pr\~{o}t\~{e}ct</i>                          |
| <i>protector</i>        | <i>protector</i>             | <i>pr\~{o}t\~{e}ct\~{o}r</i>                | <i>pr\~{o}t\~{e}ct\~{o}\~{r}</i>       | <i>pr\~{o}t\~{e}ct\~{o}\~{r}</i>                |
| <i>protectorate</i>     | <i>protectorate</i>          | <i>pr\~{o}t\~{e}ct\~{o}r\~{a}t\~{e}</i>     | <i>pr\~{o}t\~{e}ct\~{o}\~{r}\~{a}t</i> | <i>pr\~{o}t\~{e}ct\~{o}\~{r}\~{a}t</i>          |

We note that the vowel *e* in *protect* had not been deleted in the construction of essential root. In fact, it remains in the unremovable  $\hat{\sigma}_1$  in Algorithm 4.8(1).

#### 4.2.2 Admissible mutation and approximate clustering

Unlike the Porter stemming algorithm, we shall not use the exact match of tokens as the sole criterion for word clustering. Instead, we shall sort words by their tokens, and compare consecutive neighbors in such an alphabetized list. Roughly speaking, our clustering algorithm (see Algorithm 4.15) runs as follows: if the tokens of two neighbors in such a list fail certain “approximate matching criteria”, we add a demarcation line between them; after comparisons between all the consecutive neighbors, we split the alphabetized list into word clusters.

As noted before, some English irregular verbs exhibit systematic patterns of vowel alternations, such as *drink/drank/drunk* and *sing/sang/sung*. However, the tokens for the separate forms of an irregular verb may not sit next to each other in an alphabetized list. To resolve this issue in token sorting order, we need to blot certain vowels (more precisely, the extended vowels prescribed by Definition 4.6) occurring in our token, by the following algorithm.

**Algorithm 4.9** (English vowel blotting). *For a token string  $\hat{\sigma}$ , its blotted form  $\text{BlotV}_1(\hat{\sigma})$  is constructed as follows:*

- If the first appearance of pattern  $\mathbf{V}_m^*$  occurs neither word-initially nor word-finally (as measured by external word boundaries of  $\hat{\sigma}$ ), then replace the aforementioned pattern with a single letter “a”.
- Otherwise, leave the string  $\hat{\sigma}$  intact.

*Example 4.9.1.* As a continuation of Example 4.8.2, one can append one more column  $\text{BlotV}_1(\text{EssRoot}(\text{EffSpell}(\hat{\sigma})))$  with entries *env\~{i}ron*, *env\~{i}ron\~{m}*, *env\~{i}ron\~{m}*, *pr\~{a}t\~{e}ct*, *pr\~{a}t\~{e}ct*, *pr\~{a}t\~{e}ct\~{o}\~{r}*, *pr\~{a}t\~{e}ct\~{o}\~{r}\~{a}t*.

*Example 4.9.2.* A few more examples:

| $\hat{\sigma}$                                                  | <i>automatic</i>     | <i>bee</i> | <i>find</i>  | <i>join</i> | <i>solo</i>  |
|-----------------------------------------------------------------|----------------------|------------|--------------|-------------|--------------|
| $\text{BlotV}_1(\text{EssRoot}(\text{EffSpell}(\hat{\sigma})))$ | <i>aaut\~{o}omat</i> | <i>bee</i> | <i>ffand</i> | <i>jzan</i> | <i>szalo</i> |

Our “approximate matching criteria” are encoded in a bivariate Boolean-valued function  $\text{HrdTest}(\hat{\alpha}, \hat{\beta})$ , which tests whether string  $\hat{\beta}$  is a “legitimate heir” to string  $\hat{\alpha}$ . Before stating this “heredity test function” in its entirety (Algorithm 4.14), we shall describe a “simple heredity test function” in Algorithm 4.10, which judges similarities between two strings, without worrying about the problems associated with irregular verbs.

**Algorithm 4.10** (Simple heredity test). *Let  $\hat{\alpha}'$  be the result of doing  $\sim e \rightarrow \emptyset$ ,  $\hat{\chi} \text{lie}(er|st) \rightarrow \hat{\chi}$  on  $\hat{\alpha}$ . The Boolean-valued function  $\text{SimpHrdTest}(\hat{\alpha}, \hat{\beta})$  returns **TRUE** if the lowercase form of  $\hat{\alpha}$  contains at least one instance of  $\mathbf{V}^*$  (Definition 4.6) **AND** at least one of the following 12 conditions holds:<sup>44</sup>*

- (i)  $\hat{\alpha} = \hat{\beta}$ ;
- (ii)  $\hat{\alpha} = \hat{\beta}^\circ$ , where  $\hat{\beta}^\circ$  results from doing  $\sim_{\hat{\chi} \notin (a|e|i|o|u)ster} \rightarrow \hat{\chi}$  on  $\hat{\beta}$ .
- (iii)  $\hat{\alpha} = \hat{\beta}^*$ , where  $\hat{\beta}^*$  results from doing  $\hat{\chi} \text{lie}(er|st) \rightarrow \hat{\chi}$  on  $\hat{\beta}$ ;
- (iv)  $\hat{\alpha} = \hat{\beta}^\dagger$ , where  $\hat{\beta}^\dagger$  results from doing  $\sim ie \rightarrow i$  on  $\hat{\beta}$ ;
- (v)  $\hat{\alpha} = \hat{\beta}^\ddagger$ , where  $\hat{\beta}^\ddagger$  results from doing  $\sim us \rightarrow u$  on  $\hat{\beta}$ ;
- (vi) Appending the last letter of string  $\hat{\alpha}$  to itself, one obtains  $\hat{\beta}$ ;
- (vii)  $\hat{\beta} = \hat{\alpha}'i$ ;
- (viii)  $\hat{\beta} = \hat{\alpha}'v$ ;
- (ix)  $\hat{\beta} = \hat{\alpha}n$ ;
- (x)  $\hat{\beta} = (\hat{\alpha}|\hat{\alpha}')sip$ ;
- (xi)  $\hat{\beta} = \hat{\alpha}\theta$ ;
- (xii)  $\ell(\hat{\beta}) - 1 > \ell(\hat{\alpha}') \geq \frac{\ell(\hat{\beta})}{2}$  **AND**  $\hat{\alpha} = \hat{\beta}^{\lfloor \ell(\hat{\alpha}') \rfloor}(\emptyset|e)$  **AND**  $\hat{\alpha}'\mathbf{X}_1(gu|i\acute{o}|ow|z|\beta)\mathbf{X}_2 \neq \hat{\beta}$  **AND**  $\hat{\beta}^{\ell(\hat{\alpha}')+1} = (a|e|h|i|o|\acute{o}|\acute{o}|r|u)$ . (See Definition 3.1 for the notations  $\hat{\beta}^{\lfloor n \rfloor}$  and  $\hat{\beta}^{\lfloor n \rfloor}$ .)

When  $\text{SimpHrdTest}(\hat{\alpha}, \hat{\beta}) = \mathbf{FALSE}$ , it is still possible that the two underlying words are etymologically related. To detect affinity between words in such scenarios, we need to invoke the Needleman–Wunsch (NW) and Smith–Waterman (SW) algorithms for more detailed string comparisons (cf. Definition 3.7).

**Algorithm 4.11** (Roots and suffixes by NW and SW). *For two strings  $\hat{\alpha}$  and  $\hat{\beta}$ , the function values  $\text{RootNW}(\hat{\alpha}, \hat{\beta})$ ,  $\text{SuffixNW}(\hat{\alpha}, \hat{\beta})$  and  $\text{NW}^*(\hat{\alpha}, \hat{\beta})$  are determined through the following procedure:*

- Use the Needleman–Wunsch algorithm to align the sequences as  $\text{NW}(\hat{\alpha}, \hat{\beta})$ .
- If  $\text{NW}(\hat{\alpha}, \hat{\beta})$  ends with a mismatch (shown in brackets in Examples 3.7.1 and 3.7.2), use this mismatch to define  $\text{SuffixNW}(\hat{\alpha}, \hat{\beta})$ ; otherwise, define  $\text{SuffixNW}(\hat{\alpha}, \hat{\beta}) = [\emptyset, \emptyset]$ .
- If  $\text{NW}(\hat{\alpha}, \hat{\beta})$  starts with a matching string, define  $\text{RootNW}(\hat{\alpha}, \hat{\beta})$  as the concatenation of all the (not necessarily contiguous) matching string portions in  $\text{NW}(\hat{\alpha}, \hat{\beta})$ , and define  $\text{NW}^*(\hat{\alpha}, \hat{\beta})$  by dropping the first matching string from  $\text{NW}(\hat{\alpha}, \hat{\beta})$  as well as its contribution (if non-void) to  $\text{SuffixNW}(\hat{\alpha}, \hat{\beta})$ ; otherwise, define  $\text{RootNW}(\hat{\alpha}, \hat{\beta}) = \boxed{\#\%} = \boxed{\text{U+0023}} \boxed{\text{U+0025}}$  (a nonsensical string containing two characters) and define  $\text{NW}^*(\hat{\alpha}, \hat{\beta})$  by deleting from  $\text{NW}(\hat{\alpha}, \hat{\beta})$  the contribution (if non-void) to  $\text{SuffixNW}(\hat{\alpha}, \hat{\beta})$ ;

The function values  $\text{RootSW}(\hat{\alpha}, \hat{\beta})$ ,  $\text{SuffixSW}(\hat{\alpha}, \hat{\beta})$  and  $\text{SW}^*(\hat{\alpha}, \hat{\beta})$  are determined similarly, through the SW function.

**Algorithm 4.12** (Admissible suffix mismatch). *For two strings  $\hat{\alpha}$  and  $\hat{\beta}$ , the Boolean-valued function*

$$\text{AdmSM}(\text{RootNW}(\hat{\alpha}, \hat{\beta}), \text{SuffixNW}(\hat{\alpha}, \hat{\beta}), \text{NW}^*(\hat{\alpha}, \hat{\beta}))$$

*returns **TRUE** if the lowercase form of  $\text{RootNW}(\hat{\alpha}, \hat{\beta})$  contains at least one instance of  $\mathbf{V}^*$  (Definition 4.6) **AND**  $\text{NW}^*(\hat{\alpha}, \hat{\beta})$  is void **AND**  $\text{SuffixNW}(\hat{\alpha}, \hat{\beta}) \neq [(nd|ow|z|\beta), (nd|ow)]$ <sup>45</sup> **AND** at least one of the following four conditions holds:*

- (i)  $\text{SuffixNW}(\hat{\alpha}, \hat{\beta}) = [i, n]$ ;
- (ii)  $\text{SuffixNW}(\hat{\alpha}, \hat{\beta}) = [i, u]$ ;
- (iii)  $\text{SuffixNW}(\hat{\alpha}, \hat{\beta}) = [\emptyset, s]$  **AND**  $\mathcal{Q}(\text{RootNW}(\hat{\alpha}, \hat{\beta})) = i$ ;
- (iv)  $\text{SuffixNW}(\hat{\alpha}, \hat{\beta}) = [(\emptyset|i|((a|e|h)\mathbf{X}))]$ ,  $(en|i|z|iz\mathbf{X}|(i|ia|i\acute{o}|i\acute{o}|iv|m|r|\hat{\chi}')\hat{\chi}\mathbf{X})$  where  $\hat{\chi}' = \text{RootNW}(\hat{\alpha}, \hat{\beta})^{\ell(\text{RootNW}(\hat{\alpha}, \hat{\beta}))}$  is the last character in  $\text{RootNW}(\hat{\alpha}, \hat{\beta})$ .

<sup>44</sup>As a general rule in this document, the truth values of items labeled with Roman numerals are connected to each other with logical **OR**.

<sup>45</sup>Hereafter,  $[\hat{\sigma}_1, \hat{\sigma}_2] \neq [\hat{\tau}_1, \hat{\tau}_2]$  means  $(\hat{\sigma}_1 \neq \hat{\tau}_1 \text{ AND } \hat{\sigma}_2 \neq \hat{\tau}_2)$ , while  $[\hat{\sigma}_1, \hat{\sigma}_2] = [\hat{\tau}_1, \hat{\tau}_2]$  means  $(\hat{\sigma}_1 = \hat{\tau}_1 \text{ AND } \hat{\sigma}_2 = \hat{\tau}_2)$ .

Similarly, one can evaluate another Boolean-valued function

$$\text{AdmSM}(\text{RootSW}(\hat{\alpha}, \hat{\beta}), \text{SuffixSW}(\hat{\alpha}, \hat{\beta}), \text{SW}^*(\hat{\alpha}, \hat{\beta}))$$

by trading all the occurrences of NW in the statements above with SW.

**Algorithm 4.13** (Admissible vowel alternation). For two strings  $\hat{\alpha}$  and  $\hat{\beta}$ , the Boolean-valued function

$$\text{AdmVA}(\text{RootNW}(\hat{\alpha}, \hat{\beta}), \text{SuffixNW}(\hat{\alpha}, \hat{\beta}), \text{NW}^*(\hat{\alpha}, \hat{\beta}))$$

returns **TRUE** if  $\text{SuffixNW}(\hat{\alpha}, \hat{\beta}) = [(\emptyset | (e|i|n)\mathbf{X}), (\emptyset | (e|i|n|t|z)\mathbf{X})]$  **AND**  $\text{NW}^*(\hat{\alpha}, \hat{\beta})$  consists of one mutation bracket and one non-void matching string **AND**  $\text{RootNW}(\hat{\alpha}, \hat{\beta}) \neq \mathbf{X}_1(i|u)\mathbf{X}_2$  **AND** at least one of the following three conditions holds:

- (i)  $\text{NW}^*(\hat{\alpha}, \hat{\beta}) = ([a, e]||[a, i]||[a, u]||[\ddot{a}\ddot{a}, \acute{o}\acute{o}]||[e, \emptyset]||[e, o]||[ee, oo]||[ee, \acute{o}\acute{o}]||[i, u]||[i, \acute{o}]||[i, \acute{o}\acute{o}]||[oo, \acute{o}\acute{o}])\mathbf{X}$
- (ii)  $\text{NW}^*(\hat{\alpha}, \hat{\beta}) = [\emptyset, \hat{\chi}']\mathbf{X}$  where  $\hat{\chi}' = \text{RootNW}(\hat{\alpha}, \hat{\beta})^{\ell(\text{RootNW}(\hat{\alpha}, \hat{\beta}))}$  is the last character in  $\text{RootNW}(\hat{\alpha}, \hat{\beta})$ ;
- (iii)  $\text{NW}^*(\hat{\alpha}, \hat{\beta}) = [\emptyset, e]e$ .

Similarly, one can evaluate  $\text{AdmVA}(\text{RootSW}(\hat{\alpha}, \hat{\beta}), \text{SuffixSW}(\hat{\alpha}, \hat{\beta}), \text{SW}^*(\hat{\alpha}, \hat{\beta}))$ .

**Algorithm 4.14** (Heredity test function). Let  $\hat{\alpha}'$  be the result of performing a substitution  $\sim e \rightarrow \emptyset$  on  $\hat{\alpha}$ . For two strings  $\hat{\alpha}$  and  $\hat{\beta}$ , the Boolean-valued function  $\text{HrdTest}(\hat{\alpha}, \hat{\beta})$  returns **TRUE** if at least one of the following three conditions holds:

- (i)  $\text{SimpHrdTest}(\hat{\alpha}, \hat{\beta}) = \mathbf{TRUE}$ ;
- (ii)  $\ell(\text{RootNW}(\hat{\alpha}, \hat{\beta})) \geq \frac{1}{2} \max\{\ell(\hat{\alpha}'), \ell(\hat{\beta})\}$  **AND**  $(\text{AdmSM}(\text{RootNW}(\hat{\alpha}, \hat{\beta}), \text{SuffixNW}(\hat{\alpha}, \hat{\beta}), \text{NW}^*(\hat{\alpha}, \hat{\beta})) = \mathbf{TRUE} \text{ OR } \text{AdmVA}(\text{RootNW}(\hat{\alpha}, \hat{\beta}), \text{SuffixNW}(\hat{\alpha}, \hat{\beta}), \text{NW}^*(\hat{\alpha}, \hat{\beta})) = \mathbf{TRUE})$ ;
- (iii)  $\ell(\text{RootSW}(\hat{\alpha}, \hat{\beta})) \geq \frac{1}{2} \max\{\ell(\hat{\alpha}'), \ell(\hat{\beta})\}$  **AND**  $(\text{AdmSM}(\text{RootSW}(\hat{\alpha}, \hat{\beta}), \text{SuffixSW}(\hat{\alpha}, \hat{\beta}), \text{SW}^*(\hat{\alpha}, \hat{\beta})) = \mathbf{TRUE} \text{ OR } \text{AdmVA}(\text{RootSW}(\hat{\alpha}, \hat{\beta}), \text{SuffixSW}(\hat{\alpha}, \hat{\beta}), \text{SW}^*(\hat{\alpha}, \hat{\beta})) = \mathbf{TRUE})$ .

**Algorithm 4.15** (Approximate clustering of English words). The approximate clustering of a list of English words  $\{\hat{\alpha}_1, \dots, \hat{\alpha}_N\}$  is completed in two stages:

- (1) We sort the list  $\{(\hat{\alpha}_1, \text{EffSpell}(\hat{\alpha}_1)), \dots, (\hat{\alpha}_N, \text{EffSpell}(\hat{\alpha}_N))\}$  alphabetically according to the second component (effective spelling) of each entry. If two consecutive neighbors in the alphabetized list  $\{(\hat{\alpha}_{(1)}, \text{EffSpell}(\hat{\alpha}_{(1)})), \dots, (\hat{\alpha}_{(N)}, \text{EffSpell}(\hat{\alpha}_{(N)}))\}$  satisfy  $\text{HrdTest}(\text{EffSpell}(\hat{\alpha}_{(n)}), \text{EffSpell}(\hat{\alpha}_{(n+1)})) = \mathbf{FALSE}$ , where  $n \in \mathbb{Z} \cap [1, N)$ , then add a demarcation line between these two entries. In this way, the alphabetized list is divided into separate groups of words tagged with their effective spellings:  $\{g_1 = \{(\hat{\alpha}_{(1,1)}, \text{EffSpell}(\hat{\alpha}_{(1,1)})), \dots, (\hat{\alpha}_{(1,n_1)}, \text{EffSpell}(\hat{\alpha}_{(1,n_1)}))\}, \dots, g_M = \{(\hat{\alpha}_{(M,1)}, \text{EffSpell}(\hat{\alpha}_{(M,1)})), \dots, (\hat{\alpha}_{(M,n_M)}, \text{EffSpell}(\hat{\alpha}_{(M,n_M)}))\}$ , where each sublist also preserves alphabetic order. In particular, we have  $\hat{\alpha}_{(1,1)} = \hat{\alpha}_{(1)}$  and  $\hat{\alpha}_{(M,n_M)} = \hat{\alpha}_{(N)}$ .
- (2) For each group of words  $g_m = \{(\hat{\alpha}_{(m,1)}, \text{EffSpell}(\hat{\alpha}_{(m,1)})), \dots, (\hat{\alpha}_{(m,n_m)}, \text{EffSpell}(\hat{\alpha}_{(m,n_m)}))\}$  where  $m \in \mathbb{Z} \cap [1, M]$ , we augment it into a tagged entry  $G_m = (g_m, \text{EffSpell}(\hat{\alpha}_{(m,1)}), \text{EssRoot}(\text{EffSpell}(\hat{\alpha}_{(m,1)})), \text{BlotV}_1(\text{EssRoot}(\text{EffSpell}(\hat{\alpha}_{(m,1)}))))$ . The list  $\{G_1, \dots, G_M\}$  is sorted alphabetically, with respect to  $\text{BlotV}_1(\text{EssRoot}(\text{EffSpell}(\hat{\alpha}_{(m,1)})))$  (with highest priority),  $\text{EssRoot}(\text{EffSpell}(\hat{\alpha}_{(m,1)}))$  (with medium priority), and  $\text{EffSpell}(\hat{\alpha}_{(m,1)})$  (with lowest priority). If two consecutive neighbors in the alphabetized list  $\{G_{(1)} = (g_{(1)}, \hat{\gamma}'_{(1)}, \hat{\gamma}''_{(1)}, \hat{\gamma}'''_{(1)}), \dots, G_{(M)} = (g_{(M)}, \hat{\gamma}'_{(M)}, \hat{\gamma}''_{(M)}, \hat{\gamma}'''_{(M)})\}$  satisfy

$$\text{HrdTest}(\hat{\gamma}''_{(m)}, \hat{\gamma}''_{(m+1)}) = \mathbf{FALSE}$$

**AND**

$$\text{HrdTest}(\hat{\gamma}'_{(m)}, \hat{\gamma}'_{(m+1)}) = \mathbf{FALSE}$$

where  $m \in \mathbb{Z} \cap [1, M)$ , then add a demarcation line between these two entries. In this manner, the alphabetized list  $\{G_{(1)}, \dots, G_{(M)}\}$  is divided into separate groups of tagged clusters  $\{\Gamma_1 = \{G_{(1,1)}, \dots, G_{(1,m_1)}\}, \dots, \Gamma_K = \{G_{(K,1)}, \dots, G_{(1,m_K)}\}\}$ . Finally, the output list of word clusters  $\{\tilde{\Gamma}_1, \dots, \tilde{\Gamma}_K\}$  is constructed by discarding all the tags (effective spellings, essential roots, vowel blotted forms) from each  $\Gamma_k$ , where  $k \in \mathbb{Z} \cap [1, K]$ .

*Example 4.15.1.* To partially demonstrate the capabilities of our clustering algorithm, we pick the following list of English words:

*abolish, abolished, abolishes, abolishing, abolishment, abolition, abolitionism, abolitionist, abolitionists, admonish, admonishable, admonisher, admonishes, admonishing, admonishingly, admonishment, admonition, admonitory, aid, aided, aids, America, American, analyses, analysis, analytic, analytically, analyze, analyzed, ant, antenna, antennae, anterior, anxieties, anxiety, anxious, anxiously, arise, arisen, arose, automatic, automatically, bad, bat, beauties, beautiful, beautifully, beauty, bed, bedding, beds, beg, began, beggar, begged, begin, beginning, begun, belie, belied, belief, beliefs, belie, believe, believed, believes, believing, bereave, bereft, best, bestow, bestowed, bet, better, bid, bit, bitten, break, breaking, breaks, Britain, British, broke, broken, brow, brows, browse, browsed, browses, browsing, brutal, brutality, brutalize, brutally, brute, brutish, child, childhood, children, children's, child's, conquer, conquered, conquest, cycle, cylinder, dance, danced, dances, dancing, dead, deal, dealt, death, destroy, destroyed, destruction, die, died, dies, differ, difference, different, difficult, difficulty, dosage, dose, drain, drainage, dried, dries, dry, dryly, dye, dyed, dyeing, dyes, dying, elect, elected, election, elections, electoral, emphases, emphasis, emphasize, emphasized, emphasizes, emphatic, employ, employed, employee, employer, employment, England, English, enjoy, enjoyed, enjoying, enjoyment, enjoys, environment, environmental, environmentalist, establish, established, establishes, establishing, establishment, estimate, estimated, estimates, estimation, fall, fallen, falling, falls, fame, family, famous, fat, feel, feeling, feels, fell, fellow, fellows, fellowship, felt, fight, fighting, fill, find, fit, fold, follow, fond, fought, found, fret, fretting, full, fund, funding, gentleman, gentlemen, German, Germany, good, happen, happened, happening, happens, happier, happiest, happily, happiness, happy, hat, hate, hated, hating, hatred, hats, heavy, heft, held, hell, hill, hillside, hit, hits, hitting, hold, increase, increased, increases, increasing, incredible, incredulity, incredulous, infer, inference, inferior, inferiority, inferred, infers, insist, insisted, insistence, integral, integrally, integrate, integration, interfere, interference, interfering, introduce, introduced, introduces, introduction, introductory, lack, lacking, ladies, ladies', lady, lady's, law, lawyer, leave, leaves, leaving, left, lick, lie, lied, lies, life, life's, lift, lived, lives, living, lock, love, loved, lovely, loves, loving, low, lower, lowest, lowing, lowly, luck, luckily, lucky, lying, maid, maiden, maids, male, man, manage, manipulate, mankind, manner, manners, man's, mansion, mansions, marriage, married, marries, marrow, marry, marrying, men, mend, men's, merry, mile, mind, mole, mule, natural, naturally, nature, nature's, paid, pain, painful, painfully, pay, paying, payment, payments, pays, plan, planned, planning, plans, plant, plantation, play, played, player, players, playing, plays, presidency, president, presidential, presidents, prince, princes, princess, princesses, protect, protection, protector, protectoral, protectorate, ran, rang, range, ranged, ranges, ranging, rank, rant, rate, rated, rates, rating, real, realization, realize, refer, reference, referral, rid, ridden, ride, ring, ringing, rings, road, rode, rude, ruin, ruined, ruins, run, rung, running, runs, Russell, Russia, Russian, sad, sadden, saddened, sadly, said, sang, sat, say, saying, says, secede, seceded, secedes, seceding, secession, secessionist, secessionists, secessions, sell, selling, send, sending, sent, sentence, sentences, sentiment, sentimental, sentiments, set, sets, setting, sing, singing, sit, sits, sitting, slain, slave, slave-holder, slaveholding, slavery, slavery-restricting, slaves, slay, slow, slowly, sold, solution, solutions, solve, solved, solves, son, song, sons, sore, sorely, sorrow, sorry, sort, speak, speaker, speaking, speaks, speech, speeches, spoke, spoken, spokesman, strata, stratum, strife, strifes, strive, strived, striven, strove, sun, sung, swam, swear, swell, swelled, swelling, swells, swim, swimming, swims, swollen, swoon, swooned, swoons, sword, sworn, swum, tall, tame, tamed, tax, taxes, teeth, tell, telling, thank, thanking, thanks, theft, thief, thief, thieved, thieves, thin, thing, things, think, thinking, thrift, thrifty, thrive, thrived, thriven, thrives, thrive, time, times, timing, told, tooth, traffic, trafficking, transfer, transference, transferral, want, wear, weave, weep, weeping, weeps, weft, wept, wet, wife, wife's, winter, wipe, wiped, wipes, wit, wives, woman, woman's, women, women's, word, words, wore, world, worn, woven.*

Applying Algorithm 4.15 to the list above, we arrive at the following result

{*abolish, abolished, abolishes, abolishing, abolishment, abolition, abolitionism, abolitionist, abolitionists*}, {*admonish, admonishable, admonisher, admonishes, admonishing, admonishingly, admonishment*}, {*admonition, admonitory*}, {*aid, aided, aids*}, {*America, American*}, {*analyses, analysis, analytic, analytically, analyze, analyzed*}, {*ant*}, {*antenna, antennae*}, {*anterior*}, {*anxieties, anxiety, anxious, anxiously*}, {*arise, arisen, arose*}, {*automatic, automatically*}, {*bad*}, {*bat*}, {*beauties, beautiful, beautifully, beauty*}, {*bed, bedding, beds*}, {*beg, begged*}, {*began, begin, beginning, begun*}, {*beggar*}, {*belie, belied, belie*}, {*belief, beliefs, believe, believed, believes, believing*}, {*bereave, bereft*}, {*best, better, good*}, {*bestow, bestowed*}, {*bet*}, {*bid*}, {*bit*}, {*bitten*}, {*break, breaking, breaks, broke, broken*}, {*Britain, British*}, {*brow, brows*}, {*browse, browsed, browses, browsing*}, {*brutal, brutality, brutalize, brutally, brute, brutish*}, {*child, child's, childhood, children, children's*}, {*conquer, conquered*}, {*conquest*}, {*cycle*}, {*cylinder*}, {*dance, danced, dances, dancing*}, {*dead, death, die, died, dies, dying*}, {*deal, dealt*}, {*destroy, destroyed, destruction*}, {*differ, difference, different*}, {*difficult, difficulty*}, {*dosage, dose*}, {*drain, drainage*}, {*dried, dries, dry, dryly*}, {*dye, dyed, dyeing, dyes*}, {*elect, elected, election, elections, electoral*}, {*emphases, emphasis, emphasize, emphasized, emphasizes, emphatic*}, {*employ, employed, employee, employer, employment*}, {*England, English*}, {*enjoy, enjoyed, enjoying, enjoyment, enjoys*}, {*environ-*

ment, environmental, environmentalist}, {establish, established, establishes, establishing, establishment}, {estimate, estimated, estimates, estimation}, {fall, fallen, falling, falls, fell}, {fame, famous}, {family}, {fat}, {feel, feeling, feels, felt}, {fellow, fellows, fellowship}, {fight, fighting, fought}, {fill}, {find, found}, {fit}, {fold}, {follow}, {fond}, {fret, fretting}, {full}, {fund, funding}, {gentleman, gentlemen}, {German, Germany}, {happen, happened, happening, happens}, {happier, happiest, happily, happiness, happy}, {hat, hats}, {hate, hated, hating, hatred}, {heavy, heft}, {held, hold}, {hell}, {hill}, {hillside}, {hit, hits, hitting}, {increase, increased, increases, increasing}, {incredible}, {incredulity, incredulous}, {infer, inference, inferred, infers}, {inferior, inferiority}, {insist, insisted, insistence}, {integral, integrally, integrate, integration}, {interfere, interference, interfering}, {introduce, introduced, introduces, introduction, introductory}, {lack, lacking}, {ladies, ladies', lady, lady's}, {law}, {lawyer}, {leave, leaves, leaving, left}, {lick}, {lie, lied, lies, lying}, {life, life's, lived, lives, living}, {lift}, {lock}, {love, loved, lovely, loves, loving}, {low, lower, lowest, lowing, lowly}, {luck, luckily, lucky}, {maid, maiden, maids}, {male}, {man, man's, men, men's}, {manage}, {manipulate}, {mankind}, {manner, manners}, {mansion, mansions}, {marriage, married, marries, marry, marrying}, {marrow}, {mend}, {merry}, {mile}, {mind}, {mole}, {mule}, {natural, naturally, nature, nature's}, {paid, pay, paying, payment, payments, pays}, {pain, painful, painfully}, {plan, planned, planning, plans}, {plant, plantation}, {play, played, player, players, playing, plays}, {presidency, president, presidential, presidents}, {prince, princes, princess, princesses}, {protect, protection, protector, protectoral, protectorate}, {ran, run, running, runs}, {rang, ring, ringing, rings, rung}, {range, ranged, ranges, ranging}, {rank}, {rant}, {rate, rated, rates, rating}, {real, realization, realize}, {refer, reference, referral}, {rid}, {ridden, ride, rode}, {road}, {rude}, {ruin, ruined, ruins}, {Russell, Russia, Russian}, {sad, sadden, saddened, sadly}, {said, say, saying, says}, {sang, sing, singing, sung}, {sat, sit, sits, sitting}, {secede, seceded, secedes, seceding, secession, secessionist, secessionists, secessions}, {sell, selling, sold}, {send, sending, sent}, {sentence, sentences}, {sentiment, sentimental, sentiments}, {set, sets, setting}, {slain, slay}, {slave, slave-holder, slave-holding, slavery, slavery-restricting, slaves}, {slow, slowly}, {solution, solutions, solve, solved, solves}, {son, sons}, {song}, {sore, sorely, sorry}, {sorrow}, {sort}, {speak, speaker, speaking, speaks, spoke, spoken, spokesman}, {speech, speeches}, {strata, stratum}, {strife, strifes, strive, strived, striven, strove}, {sun}, {swam, swim, swimming, swims, swum}, {swear, sworn}, {swell, swelled, swelling, swells, swollen}, {swoon, swooned, swoons}, {sword}, {tall}, {tame, tamed}, {tax, taxes}, {teeth, tooth}, {tell, telling, told}, {thank, thanking, thanks}, {theft, thief, thieve, thieved, thieves}, {thin}, {thing, things}, {think, thinking}, {thrift, thrifty}, {thrive, thrived, thriven, thrives, thrive}, {time, times, timing}, {traffic, trafficking}, {transfer, transference, transferral}, {want}, {wear, wore, worn}, {weave, weft, woven}, {weep, weeping, weeps, wept}, {wet}, {wife, wife's, wives}, {winter}, {wipe, wiped, wipes}, {wit}, {woman, woman's, women, women's}, {word, words}, {world},

which contains only very few errors. For such a list of test words, the time cost of our algorithm is only twice as long as conventional Porter stemming<sup>46</sup>, the latter of which yields the following clustering result:

{abolish, abolished, abolishes, abolishing, abolishment}, {abolition}, {abolitionism}, {abolitionist, abolitionists}, {admonish, admonishable, admonisher, admonishes, admonishing, admonishment}, {admonishingly}, {admonition}, {admonitory}, {aid, aided, aids}, {America}, {American}, {analyses}, {analysis}, {analytic, analytically}, {analyze, analyzed}, {ant}, {antenna, antennae}, {anterior}, {anxieties, anxiety}, {anxious}, {anxiously}, {arise}, {arisen}, {arose}, {automatic, automatically}, {bad}, {bat}, {beauties, beautiful, beauty}, {beautifully}, {bed, bedding, beds}, {beg, begged}, {began}, {beggar}, {begin, beginning}, {begun}, {belie, belied, belies}, {belief, beliefs}, {believe, believed, believes, believing}, {bereave}, {bereft}, {best}, {bestow, bestowed}, {bet}, {better}, {bid}, {bit}, {bitten}, {break, breaking, breaks}, {Britain}, {British}, {broke}, {broken}, {brow, brows}, {browse, browsed, browses, browsing}, {brutal, brutality, brutalize, brutally}, {brute}, {brutish}, {child}, {childhood}, {children}, {children's}, {child's}, {conquer, conquered}, {conquest}, {cycle}, {cylinder}, {dance, danced, dances, dancing}, {dead}, {deal}, {dealt}, {death}, {destroy, destroyed}, {destruction}, {die}, {died, dies}, {differ, difference, different}, {difficult}, {difficulty}, {dosage}, {dose}, {drain}, {drainage}, {dried, dries}, {dry}, {dryly}, {dye, dyeing, dyes}, {dyed, dying}, {elect, elected, election, elections}, {electoral}, {emphases, emphasize, emphasized, emphasizes}, {emphasis}, {emphatic}, {employ, employed}, {employee}, {employer, employment}, {England}, {English}, {enjoy, enjoyed, enjoying, enjoys}, {enjoyment}, {environment}, {environmental}, {environmentalist}, {establish, established, establishes, establishing, establishment}, {estimate, estimated, estimates, estimation}, {fall, falling, falls}, {fallen}, {fame}, {family}, {famous}, {fat}, {feel, feeling, feels}, {fell}, {fellow, fellows}, {fellowship}, {felt}, {fight, fighting}, {fill}, {find}, {fit}, {fold}, {follow}, {fond}, {fought}, {found}, {fret, fretting}, {full}, {fund, funding}, {gentleman}, {gentlemen}, {German}, {Germany}, {good}, {happen, happened, happening, happens}, {happier}, {happiest}, {happily}, {happiness, happy}, {hat, hats}, {hate, hated, hating}, {hatred}, {heavy}, {heft}, {held}, {hell},

<sup>46</sup>We use the Porter stemming functionality built in *Mathematica* v11.0 for this numerical experiment. Certain variations on the Porter stemming algorithm may have better performances in word clustering.

{hill}, {hillside}, {hit, hits, hitting}, {hold}, {increase, increased, increases, increasing}, {incredible}, {incredulity, incredulous}, {infer, inference, inferred, infers}, {inferior, inferiority}, {insist, insisted, insistence}, {integral, integrally, integrate, integration}, {interfere, interference}, {interfering}, {introduce, introduced, introduces}, {introduction}, {introductory}, {lack, lacking}, {ladies, lady}, {ladies' }, {lady's}, {law}, {lawyer}, {leave, leaves, leaving}, {left}, {lick}, {lie}, {lied, lies}, {life}, {life's}, {lift}, {lived, lives, living}, {lock}, {love, loved, lovely, loves, loving}, {low, lowing}, {lower}, {lowest}, {lowly}, {luck}, {luckily}, {lucky}, {lying}, {maid, maids}, {maiden}, {male}, {man}, {manage}, {manipulate}, {mankind}, {manner, manners}, {man's}, {mansion, mansions}, {marriage}, {married, marries, marry, marrying}, {marrow}, {men}, {mend}, {men's}, {merry}, {mile}, {mind}, {mole}, {mule}, {natural, naturally, nature}, {nature's}, {paid}, {pain, painful}, {painfully}, {pay, paying, pays}, {payment, payments}, {plan, planned, planning, plans}, {plant}, {plantation}, {play, played, playing, plays}, {player, players}, {presidency, president, presidents}, {presidential}, {prince, princes}, {princess, princesses}, {protect, protection}, {protector, protectoral, protectorate}, {ran}, {rang, range, ranged, ranges, ranging}, {rank}, {rant}, {rate, rated, rates, rating}, {real}, {realization, realize}, {refer, reference}, {referral}, {rid}, {ridden}, {ride}, {ring, ringing, rings}, {road}, {rode}, {rude}, {ruin, ruined, ruins}, {run, running, runs}, {rung}, {Russell}, {Russia}, {Russian}, {sad}, {sadden, saddened}, {sadly}, {said}, {sang}, {sat}, {say, saying, says}, {secede, seceded, secedes, seceding}, {secession, secessions}, {secessionist, secessionists}, {sell, selling}, {send, sending}, {sent}, {sentence, sentences}, {sentiment, sentimental, sentiments}, {set, sets, setting}, {sing, singing}, {sit, sits, sitting}, {slain}, {slave, slaves}, {slave-holder, slaveholding}, {slavery}, {slavery-restricting}, {slay}, {slow}, {slowly}, {sold}, {solution, solutions}, {solve, solved, solves}, {son, sons}, {song}, {sore, sorely}, {sorrow}, {sorry}, {sort}, {speak, speaking, speaks}, {speaker}, {speech, speeches}, {spoke}, {spoken}, {spokesman}, {strata}, {stratum}, {strife, strifes}, {strive, strived}, {striven}, {strove}, {sun}, {sung}, {swam}, {swear}, {swell, swelled, swelling, swells}, {swim, swimming, swims}, {swollen}, {swoon, swooned, swoons}, {sword}, {sworn}, {swum}, {tall}, {tame, tamed}, {tax, taxes}, {teeth}, {tell, telling}, {thank, thanking, thanks}, {theft}, {thief}, {thieve, thieved, thieves}, {thin}, {thing, things}, {think, thinking}, {thrift}, {thrifty}, {thrive, thrived, thrives}, {thriven}, {throve}, {time, times, timing}, {told}, {tooth}, {traffic}, {trafficking}, {transfer, transference}, {transferral}, {want}, {wear}, {weave}, {weep, weeping, weeps}, {weft}, {wept}, {wet}, {wife}, {wife's}, {winter}, {wipe, wiped, wipes}, {wit}, {wives}, {woman}, {woman's}, {women}, {women's}, {word, words}, {wore}, {world}, {worn}, {woven},

containing more errors than our output.

*Example 4.15.2.* In Fig. S3, we apply our modified Porter stemming algorithm to topic mining from three English masterpieces (see Table S1 for provenances), and compare the results with ground truths.

According to our stochastic model for recurrence time statistics, word patterns should stay either around the critical line of Poissonian banality (colored gray in Fig. S3) or below it (colored red in Fig. S3). The pattern *Eliza*( $\emptyset$ |*beth*)( $\emptyset$ |'s) in Fig. S3a is a prominent counterexample to this general rule. Our explanation for this is the aliasing of “Elizabeth” by pronouns and nicknames.

Furthermore, if a language lacks gender distinction in third-person pronouns, then its speaker might sometimes spell out a specific person’s name to avoid confusion. This practice also complicates the statistical behavior of *Eliza*( $\emptyset$ |*beth*)( $\emptyset$ |'s) in translations of *Pride and Prejudice*. In Fig. S3e, we see that in four versions (Hungarian, Basque, Korean and Turkish), our statistical algorithm fails to identify the equivalent of *Eliza*( $\emptyset$ |*beth*)( $\emptyset$ |'s) as a topic, and the corresponding word counts also deviate significantly from the English original. These four languages, together with Finnish, do not have separate words for “he” and “she”.<sup>47</sup> The use of pronouns (or possessive suffixes, or personal verb markers, or explicit names) in these five languages can be demonstrated by the following excerpt (see Table S1 for provenances) from Chapter 43 of *Pride and Prejudice*:

English

*Mrs. Gardiner was standing a little behind; and on her pausing, he asked her if she would do him the honour of introducing him to her friends.*

Finnish

*Gardinerit olivat jääneet vähän taemmaksi; ja kun Elizabethilta puhe juuttui, pyysi Darcy tulla esitetyksi hänen ystävilleen.*

Hungarian

*Mrs. Gardiner kissé hátrább maradt, és amikor Elizabeth elhallgatott, Darcy megkérte, legyen szíves bemutatni őt ismerőseinek.*

<sup>47</sup>This statement is true for colloquial Korean, where  $\sphericalangle$  means both “he” and “she”. In written Korean texts that are translations of certain European languages, the word  $\sphericalangle$  is sometimes used for “she”. This explains why the Korean word count statistics conform to the English original for *Eliza*( $\emptyset$ |*beth*)( $\emptyset$ |'s) better than Hungarian, Basque and Turkish.

## Basque

*Gardiner anderea atzeratxoago zegoen; eta Elizabeth isildu zelarik, Darcy jaunak galde egin zion ea ez al zion egingo lagun horien aurrean bera aurkezteko ohorea.*

## Korean

가디너 부인은 조금 뒤에 서 있었다. 엘리자베스가 말을 멈추자 다시 씨는 그녀에게 친구 분들을 소개하는 영광을 베풀어 주지 않겠냐고 물었다.

## Turkish

*Mrs. Gardiner biraz arkada duruyordu; Elizabeth'in duraklamasıyla Mr. Darcy, arkadaşlarıyla tanışma şerefine erişmeyi rica etti.*

Here, in the parallel texts given above, the magenta parts point to Elizabeth herself, either in name or by coreference; the blue parts refer to Mr. Darcy. Agglutinative case prefixes/suffixes (other than those personal markers) are not shown in color. To avoid potential misinterpretations of pronominal coreferences, all the non-Indo-European translations above explicitly mentioned the names Elizabeth and Darcy as antecedents, and the subsequent pronouns (or personal markers) referred to these antecedents, according to their order of appearance in the translated texts.



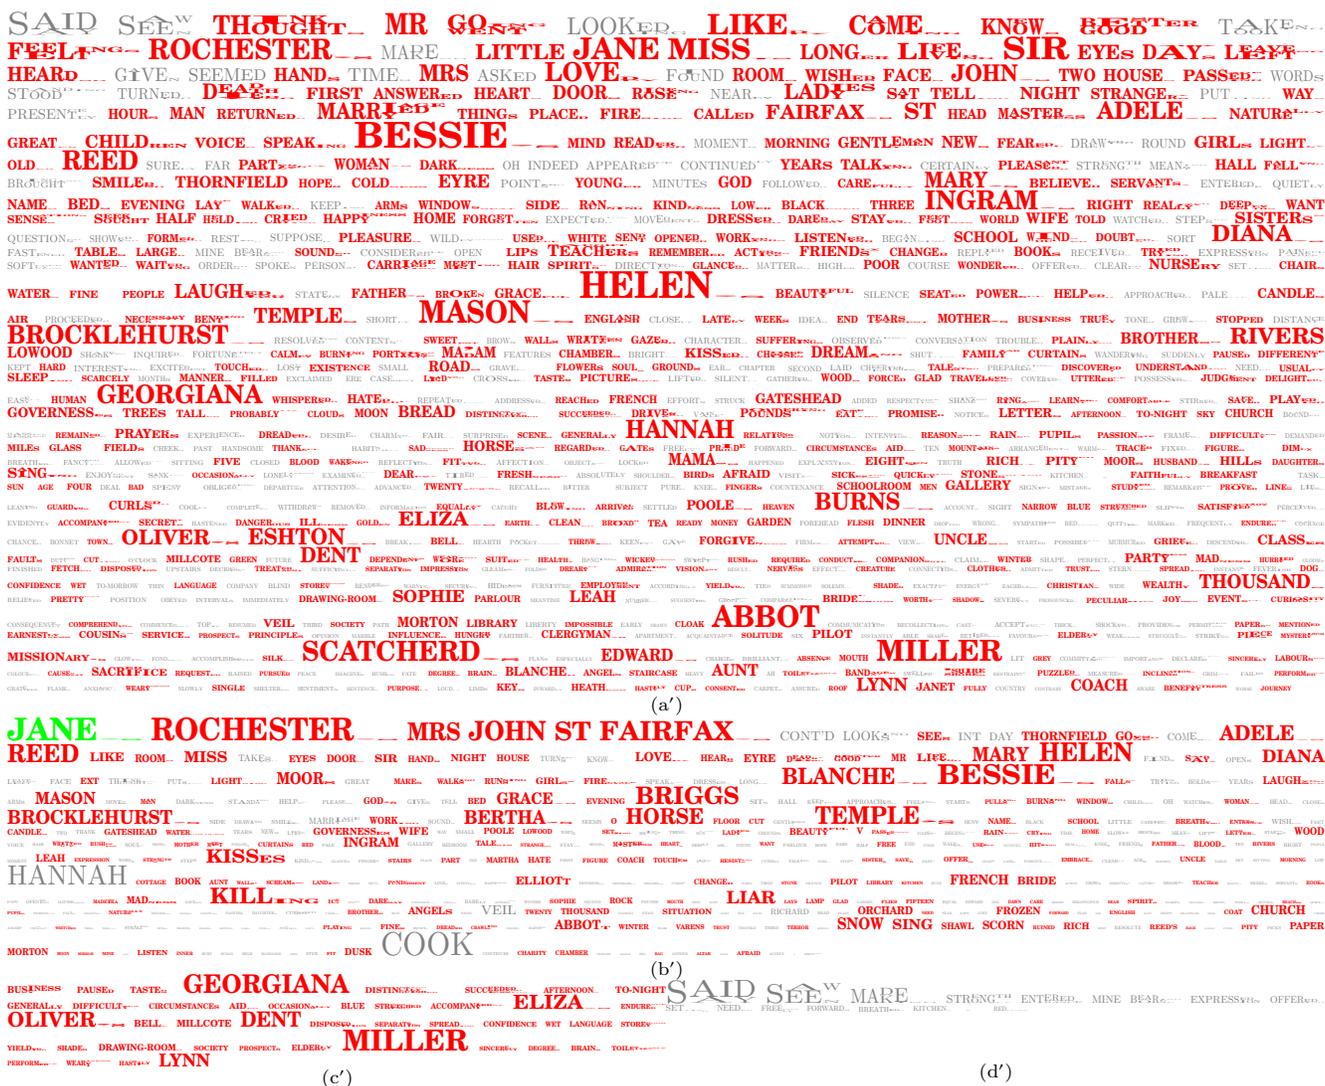

Fig. S3. Text mining in English. (Continued) A similar service on Charlotte Brontë's *Jane Eyre*. Moira Buffini's screenplay adaptation is chosen as the ground truth for topic extraction.



*Example 4.15.3.* We use exactly the same clustering algorithm to automatically generate words related to a particular question, in our WikiQA experiments. In Table S11 below, we list all the questions whose top-scoring answers (according to our algorithm) contain at least one sentence that has been officially labeled as correct by the WikiQA team. All the tabulated entries take the form of

[WikiQA-Q#]: [WikiQA question]

[Reference Wikipedia page]

[Sentence(s) bearing the highest score in our algorithm.]

Here, while tabulating our results, we make no attempt to correct the spelling or capitalization in the question (see however, Algorithm 3.11), and the punctuation marks in the candidate answer(s) are kept in the same form as the original WikiQA dataset, such as

26: how did anne frank die

Anne Frank

**Anne Frank** and her sister, Margot, were eventually transferred to the **Bergen-Belsen concentration camp**, where they **died** of **typhus** in March **1945**.

In the example above, the words related to the question (including the place of death “Bergen-Belsen concentration camp”, cause of death “typhus” and year of death “1945”, all discovered by our automated text mining) are highlighted in red.

Some (85 out of 580 total) question numbers in Table S11 are prefixed with †, because the corresponding questions are classified as “quantitative”, by Algorithm 3.12. Intuitively speaking, one might answer such “quantitative” questions better by focusing on candidate sentences that mention numbers, dates and so on. However, in our current work, we have made no effort to treat “quantitative” questions with special screening procedures for the answers.

**Table S11. List of WikiQA hits**

|                                                                                                                                                                                                                                                                                                                                                                                                                                                                                                                                                                                                                                                                                                                                                                                                                                                                                                                                                                                                                                    |                                                 |
|------------------------------------------------------------------------------------------------------------------------------------------------------------------------------------------------------------------------------------------------------------------------------------------------------------------------------------------------------------------------------------------------------------------------------------------------------------------------------------------------------------------------------------------------------------------------------------------------------------------------------------------------------------------------------------------------------------------------------------------------------------------------------------------------------------------------------------------------------------------------------------------------------------------------------------------------------------------------------------------------------------------------------------|-------------------------------------------------|
| 0: HOW AFRICAN AMERICANS WERE IMMIGRATED TO THE US                                                                                                                                                                                                                                                                                                                                                                                                                                                                                                                                                                                                                                                                                                                                                                                                                                                                                                                                                                                 | <i>African immigration to the United States</i> |
| As such, <b>African immigrants</b> are to be distinguished from <b>African American</b> people, the latter of whom are descendants of mostly West and <b>Central Africans</b> who were involuntarily brought to the United States by means of the historic Atlantic slave trade.                                                                                                                                                                                                                                                                                                                                                                                                                                                                                                                                                                                                                                                                                                                                                   |                                                 |
| 1: how are glacier caves formed?                                                                                                                                                                                                                                                                                                                                                                                                                                                                                                                                                                                                                                                                                                                                                                                                                                                                                                                                                                                                   | <i>Glacier cave</i>                             |
| A <b>glacier cave</b> is a <b>cave formed</b> within the ice of a <b>glacier</b> .                                                                                                                                                                                                                                                                                                                                                                                                                                                                                                                                                                                                                                                                                                                                                                                                                                                                                                                                                 |                                                 |
| †16: how much is 1 tablespoon of water                                                                                                                                                                                                                                                                                                                                                                                                                                                                                                                                                                                                                                                                                                                                                                                                                                                                                                                                                                                             | <i>Tablespoon</i>                               |
| In the USA one <b>tablespoon</b> (measurement unit) is approximately 15 mL; the capacity of an actual <b>tablespoon</b> (dining utensil) ranges from 7 mL to 14 mL.                                                                                                                                                                                                                                                                                                                                                                                                                                                                                                                                                                                                                                                                                                                                                                                                                                                                |                                                 |
| In countries where a <b>tablespoon</b> is a serving spoon, the nearest equivalent to the US <b>tablespoon</b> is either the dessert spoon or the soup spoon.                                                                                                                                                                                                                                                                                                                                                                                                                                                                                                                                                                                                                                                                                                                                                                                                                                                                       |                                                 |
| A <b>tablespoonful</b> , nominally the capacity of one <b>tablespoon</b> , is commonly used as a measure of volume in cooking.                                                                                                                                                                                                                                                                                                                                                                                                                                                                                                                                                                                                                                                                                                                                                                                                                                                                                                     |                                                 |
| 18: how a rocket engine works                                                                                                                                                                                                                                                                                                                                                                                                                                                                                                                                                                                                                                                                                                                                                                                                                                                                                                                                                                                                      | <i>Rocket engine</i>                            |
| A <b>rocket engine</b> , or simply “ <b>rocket</b> ”, is a <b>jet engine</b> that uses only stored propellant mass for <b>forming</b> its high speed propulsive <b>jet</b> .                                                                                                                                                                                                                                                                                                                                                                                                                                                                                                                                                                                                                                                                                                                                                                                                                                                       |                                                 |
| 26: how did anne frank die                                                                                                                                                                                                                                                                                                                                                                                                                                                                                                                                                                                                                                                                                                                                                                                                                                                                                                                                                                                                         | <i>Anne Frank</i>                               |
| <b>Anne Frank</b> and her sister, Margot, were eventually transferred to the <b>Bergen-Belsen concentration camp</b> , where they <b>died</b> of <b>typhus</b> in March <b>1945</b> .                                                                                                                                                                                                                                                                                                                                                                                                                                                                                                                                                                                                                                                                                                                                                                                                                                              |                                                 |
| †31: how old was monica lewinsky during the affair                                                                                                                                                                                                                                                                                                                                                                                                                                                                                                                                                                                                                                                                                                                                                                                                                                                                                                                                                                                 | <i>Monica Lewinsky</i>                          |
| <b>Monica Samille Lewinsky</b> (born July 23, 1973) is an American woman with whom United States President Bill Clinton admitted to having had an “improper relationship” while she worked at the White House in 1995 and 1996.                                                                                                                                                                                                                                                                                                                                                                                                                                                                                                                                                                                                                                                                                                                                                                                                    |                                                 |
| 33: how are antibodies used in                                                                                                                                                                                                                                                                                                                                                                                                                                                                                                                                                                                                                                                                                                                                                                                                                                                                                                                                                                                                     | <i>antibody</i>                                 |
| An <b>antibody</b> (Ab), also known as an immunoglobulin (Ig), is a large Y-shaped <b>protein produced</b> by B-cells that is <b>used</b> by the immune system to <b>identify</b> and neutralize foreign objects such as bacteria and viruses.                                                                                                                                                                                                                                                                                                                                                                                                                                                                                                                                                                                                                                                                                                                                                                                     |                                                 |
| †45: how old is kirk douglas, the actor?                                                                                                                                                                                                                                                                                                                                                                                                                                                                                                                                                                                                                                                                                                                                                                                                                                                                                                                                                                                           | <i>Kirk Douglas</i>                             |
| <b>Kirk Douglas</b> (born Issur Danielovitch, † December 9, 1916) is an American <b>stage</b> and film <b>actor</b> , film producer and author.                                                                                                                                                                                                                                                                                                                                                                                                                                                                                                                                                                                                                                                                                                                                                                                                                                                                                    |                                                 |
| †50: how long was richard nixon a president                                                                                                                                                                                                                                                                                                                                                                                                                                                                                                                                                                                                                                                                                                                                                                                                                                                                                                                                                                                        | <i>Richard Nixon</i>                            |
| <b>Richard Milhous Nixon</b> (January 9, 1913 – <b>April 22, 1994</b> ) was the 37th <b>President</b> of the United States, <b>serving</b> from 1969 to 1974, when he became the only <b>president</b> to resign the office.                                                                                                                                                                                                                                                                                                                                                                                                                                                                                                                                                                                                                                                                                                                                                                                                       |                                                 |
| †64: How long was Mickie James with WWE?                                                                                                                                                                                                                                                                                                                                                                                                                                                                                                                                                                                                                                                                                                                                                                                                                                                                                                                                                                                           | <i>Mickie James</i>                             |
| <b>James</b> appeared in <b>Wickie Wrestling Entertainment (WWE)</b> in October 2005 and was placed in a storyline with <b>Trish Stratus</b> , in which <b>James’</b> gimmick was that of <b>Stratus’</b> biggest fan turned obsessed stalker, an angle which lasted almost a year.                                                                                                                                                                                                                                                                                                                                                                                                                                                                                                                                                                                                                                                                                                                                                |                                                 |
| 77: how are the # of electrons in each shell determined                                                                                                                                                                                                                                                                                                                                                                                                                                                                                                                                                                                                                                                                                                                                                                                                                                                                                                                                                                            | <i>Electron shell</i>                           |
| Each <b>shell</b> can <b>contain</b> only a fixed number of <b>electrons</b> : The 1st <b>shell</b> can hold up to two <b>electrons</b> , the 2nd <b>shell</b> can hold up to eight <b>electrons</b> , the 3rd <b>shell</b> can hold up to 18, and 4th <b>shell</b> can hold up to 32 and so on.                                                                                                                                                                                                                                                                                                                                                                                                                                                                                                                                                                                                                                                                                                                                   |                                                 |
| †94: how old is beatrice arthur                                                                                                                                                                                                                                                                                                                                                                                                                                                                                                                                                                                                                                                                                                                                                                                                                                                                                                                                                                                                    | <i>Bea Arthur</i>                               |
| <b>Beatrice</b> “Bea” Arthur (May 13, 1922 – April 25, 2009) was an American actress, comedienne, and singer whose career spanned seven decades.                                                                                                                                                                                                                                                                                                                                                                                                                                                                                                                                                                                                                                                                                                                                                                                                                                                                                   |                                                 |
| 98: how are public schools funded                                                                                                                                                                                                                                                                                                                                                                                                                                                                                                                                                                                                                                                                                                                                                                                                                                                                                                                                                                                                  | <i>state school</i>                             |
| <b>State schools</b> (also known as <b>public schools</b> or <b>government schools</b> ) generally <b>refer</b> to primary or secondary <b>schools</b> mandated for or offered to all children without charge paid for, in whole or in part, by taxation.                                                                                                                                                                                                                                                                                                                                                                                                                                                                                                                                                                                                                                                                                                                                                                          |                                                 |
| 102: how does interlibrary loan work                                                                                                                                                                                                                                                                                                                                                                                                                                                                                                                                                                                                                                                                                                                                                                                                                                                                                                                                                                                               | <i>Interlibrary loan</i>                        |
| <b>Interlibrary loan</b> (abbreviated ILL, and sometimes called interloan, document delivery, or document supply) is a service whereby a user of one library can borrow books or receive photocopies of documents that are owned by another library. In many cases, nominal fees accompany <b>interlibrary loan</b> services.                                                                                                                                                                                                                                                                                                                                                                                                                                                                                                                                                                                                                                                                                                      |                                                 |
| 104: what did mia hamn do his work                                                                                                                                                                                                                                                                                                                                                                                                                                                                                                                                                                                                                                                                                                                                                                                                                                                                                                                                                                                                 | <i>Mia Hamm</i>                                 |
| Mariel Margaret “ <b>Mia</b> ” <b>Hamm</b> (born March 17, 1972) is a retired American professional soccer player.                                                                                                                                                                                                                                                                                                                                                                                                                                                                                                                                                                                                                                                                                                                                                                                                                                                                                                                 |                                                 |
| 105: what bacteria grow on macconkey agar                                                                                                                                                                                                                                                                                                                                                                                                                                                                                                                                                                                                                                                                                                                                                                                                                                                                                                                                                                                          | <i>MacConkey agar</i>                           |
| <b>MacConkey agar</b> is a culture medium designed to <b>grow</b> Gram-negative <b>bacteria</b> and differentiate them for lactose fermentation.                                                                                                                                                                                                                                                                                                                                                                                                                                                                                                                                                                                                                                                                                                                                                                                                                                                                                   |                                                 |
| 110: how do forensic auditors examine financial reporting                                                                                                                                                                                                                                                                                                                                                                                                                                                                                                                                                                                                                                                                                                                                                                                                                                                                                                                                                                          | <i>Financial audit</i>                          |
| The purpose of an audit is provide and objective independent <b>examination</b> of the <b>financial statements</b> , which <b>increases</b> the value and credibility of the <b>financial statements</b> produced by management, thus <b>increase</b> user confidence in the <b>financial statement</b> , reduce investor <b>risk</b> and consequently reduce the cost of capital of the preparer of the <b>financial statements</b> .                                                                                                                                                                                                                                                                                                                                                                                                                                                                                                                                                                                             |                                                 |
| 127: What committees are joint committees                                                                                                                                                                                                                                                                                                                                                                                                                                                                                                                                                                                                                                                                                                                                                                                                                                                                                                                                                                                          | <i>Joint committee</i>                          |
| A <b>Joint Committee</b> is a term in politics that is used to refer to a <b>committee</b> made up of members of both chambers of a bicameral legislature.                                                                                                                                                                                                                                                                                                                                                                                                                                                                                                                                                                                                                                                                                                                                                                                                                                                                         |                                                 |
| †130: How many states and territories are within India?                                                                                                                                                                                                                                                                                                                                                                                                                                                                                                                                                                                                                                                                                                                                                                                                                                                                                                                                                                            | <i>States and territories of India</i>          |
| <b>India</b> is a federal union of <b>states</b> comprising twenty-eight <b>states</b> and seven union <b>territories</b> .                                                                                                                                                                                                                                                                                                                                                                                                                                                                                                                                                                                                                                                                                                                                                                                                                                                                                                        |                                                 |
| 140: how is single malt scotch made                                                                                                                                                                                                                                                                                                                                                                                                                                                                                                                                                                                                                                                                                                                                                                                                                                                                                                                                                                                                | <i>Single malt Scotch</i>                       |
| <b>Single Malt Scotch</b> is <b>single malt</b> whisky <b>made</b> in Scotland using a pot still distillation process at a <b>single</b> distillery, with <b>malted</b> barley as the only grain ingredient.                                                                                                                                                                                                                                                                                                                                                                                                                                                                                                                                                                                                                                                                                                                                                                                                                       |                                                 |
| 164: what county in texas is conroe located in                                                                                                                                                                                                                                                                                                                                                                                                                                                                                                                                                                                                                                                                                                                                                                                                                                                                                                                                                                                     | <i>Conroe, Texas</i>                            |
| <b>Conroe</b> is the seat of <b>Montgomery County</b> and falls within the metropolitan area.                                                                                                                                                                                                                                                                                                                                                                                                                                                                                                                                                                                                                                                                                                                                                                                                                                                                                                                                      |                                                 |
| 178: how does a dredge work?                                                                                                                                                                                                                                                                                                                                                                                                                                                                                                                                                                                                                                                                                                                                                                                                                                                                                                                                                                                                       | <i>Dredging</i>                                 |
| A <b>dredger</b> (or “dredge” as is the general usage in the Americas) is any device, <b>machine</b> , or vessel that is used to <b>excavate</b> and remove material from the bottom of a body of water.                                                                                                                                                                                                                                                                                                                                                                                                                                                                                                                                                                                                                                                                                                                                                                                                                           |                                                 |
| †181: how many world series did curt schilling have                                                                                                                                                                                                                                                                                                                                                                                                                                                                                                                                                                                                                                                                                                                                                                                                                                                                                                                                                                                | <i>Curt Schilling</i>                           |
| He helped lead the Philadelphia <b>Phillies</b> to the <b>World Series</b> in and <b>won World Series</b> championships in with the <b>Arizona Diamondbacks</b> and in and with the Boston Red Sox.                                                                                                                                                                                                                                                                                                                                                                                                                                                                                                                                                                                                                                                                                                                                                                                                                                |                                                 |
| 188: what area code is 479                                                                                                                                                                                                                                                                                                                                                                                                                                                                                                                                                                                                                                                                                                                                                                                                                                                                                                                                                                                                         | <i>Area code 479</i>                            |
| <b>Area code 479</b> serves Benton, Carroll (split with <b>area code 870</b> ), Crawford, Franklin, Johnson, Logan, Madison, Polk, Pope, Scott, Sebastian, Washington and Yell Counties in Arkansas.                                                                                                                                                                                                                                                                                                                                                                                                                                                                                                                                                                                                                                                                                                                                                                                                                               |                                                 |
| <b>Area code 479</b> is the telephone <b>area code</b> serving thirteen counties in northwest Arkansas, including the cities of Fort Smith, Fayetteville, Springdale, Rogers and Bentonville: the second, third, fourth, eighth and tenth-largest cities in the state, respectively.                                                                                                                                                                                                                                                                                                                                                                                                                                                                                                                                                                                                                                                                                                                                               |                                                 |
| 189: what does arraignment mean                                                                                                                                                                                                                                                                                                                                                                                                                                                                                                                                                                                                                                                                                                                                                                                                                                                                                                                                                                                                    | <i>Arraignment</i>                              |
| During the second <b>arraignment</b> , a post-indictment <b>arraignment</b> or PIA, the defendant is allowed to enter a plea. The first is called the initial <b>arraignment</b> and must take place within 48 hours of an individual’s arrest, 72 hours if the individual was arrested on the weekend and not able to go before a judge until Monday. In response to <b>arraignment</b> , the accused is expected to enter a plea. In federal courts of the United States, <b>arraignment</b> takes place in two stages. In England, Wales, Northern Ireland and Australia, <b>arraignment</b> is the first of eleven stages in a criminal trial, and involves the clerk of the court reading out the indictment. During this <b>arraignment</b> the defendant is informed of the pending legal charges and is informed of his or her right to retain counsel. <b>Arraignment</b> is a formal reading of a criminal charging document in the presence of the defendant to inform the defendant of the charges against him or her. |                                                 |
| 190: what did chaucer do                                                                                                                                                                                                                                                                                                                                                                                                                                                                                                                                                                                                                                                                                                                                                                                                                                                                                                                                                                                                           | <i>Geoffrey Chaucer</i>                         |
| While he achieved fame during his lifetime as an author, philosopher, alchemist and astronomer, composing a scientific treatise on the astrolabe for his ten year-old son Lewis, <b>Chaucer</b> also maintained an active career in the civil service as a bureaucrat, courtier and diplomat. Geoffrey <b>Chaucer</b> (c. 1343 – 25 October 1400), known as the Father of English literature, is widely considered the greatest English poet of the Middle Ages and was the first poet to have been buried in Poet’s Corner of Westminster Abbey                                                                                                                                                                                                                                                                                                                                                                                                                                                                                   |                                                 |
| <b>Chaucer</b> is a crucial figure in developing the legitimacy of the vernacular, Middle English, at a time when the dominant literary languages in England were French and Latin.                                                                                                                                                                                                                                                                                                                                                                                                                                                                                                                                                                                                                                                                                                                                                                                                                                                |                                                 |
| 193: what does am and pm stand for                                                                                                                                                                                                                                                                                                                                                                                                                                                                                                                                                                                                                                                                                                                                                                                                                                                                                                                                                                                                 | <i>12-hour clock</i>                            |
| The 12-hour <b>clock</b> was developed over time from the mid-second millennium BC to the 16th century AD. The 12-hour <b>clock</b> is a time convention in which the 24 hours of the day are divided into two periods: a.m. (from the Latin ante meridiem, meaning “before midday”) and p.m. (post meridiem, “after midday”).                                                                                                                                                                                                                                                                                                                                                                                                                                                                                                                                                                                                                                                                                                     |                                                 |
| 203: how do pineapples grow                                                                                                                                                                                                                                                                                                                                                                                                                                                                                                                                                                                                                                                                                                                                                                                                                                                                                                                                                                                                        | <i>Pineapple</i>                                |
| The <b>Pineapple</b> ( <i>Ananas comosus</i> ) is a tropical plant with edible multiple fruit consisting of coalesced berries, and the most economically significant plant in the Bromeliaceae family. <b>Pineapples</b> may be cultivated from a crown cutting of the fruit, possibly flowering in 20–24 months and fruiting in the following six months. <b>Pineapples</b> are consumed fresh, cooked, juiced, and preserved, and are found in a wide array of cuisines. <b>Pineapple</b> does not ripen significantly post-harvest.                                                                                                                                                                                                                                                                                                                                                                                                                                                                                             |                                                 |
| 221: what does righteousness mean                                                                                                                                                                                                                                                                                                                                                                                                                                                                                                                                                                                                                                                                                                                                                                                                                                                                                                                                                                                                  | <i>Righteousness</i>                            |
| <b>Righteousness</b> (also called rectitude) is an important theological concept in Christianity, Judaism, Islam, Hinduism (dharma), and Zoroastrianism.                                                                                                                                                                                                                                                                                                                                                                                                                                                                                                                                                                                                                                                                                                                                                                                                                                                                           |                                                 |
| 241: what does the universal law of gravitation state                                                                                                                                                                                                                                                                                                                                                                                                                                                                                                                                                                                                                                                                                                                                                                                                                                                                                                                                                                              | <i>Newton’s law of universal gravitation</i>    |
| <b>Newton’s law of universal gravitation states</b> that every point <b>mass</b> in the <b>universe</b> attracts every other point <b>mass</b> with a force that is directly proportional to the <b>product</b> of their <b>masses</b> and inversely proportional to the square of the distance between them.                                                                                                                                                                                                                                                                                                                                                                                                                                                                                                                                                                                                                                                                                                                      |                                                 |
| 242: how does a dim sum restaurant work                                                                                                                                                                                                                                                                                                                                                                                                                                                                                                                                                                                                                                                                                                                                                                                                                                                                                                                                                                                            | <i>Dim sum</i>                                  |
| <b>Dim sum</b> is also well known for the unique way it is served in some <b>restaurants</b> , wherein fully cooked and ready-to-serve <b>dim sum dishes</b> are carted around the <b>restaurant</b> for customers to choose their <b>orders</b> while seated at their tables.                                                                                                                                                                                                                                                                                                                                                                                                                                                                                                                                                                                                                                                                                                                                                     |                                                 |
| †253: how many planets is jupiter away from the sun?                                                                                                                                                                                                                                                                                                                                                                                                                                                                                                                                                                                                                                                                                                                                                                                                                                                                                                                                                                               | <i>Jupiter</i>                                  |
| <b>Jupiter</b> is the fifth <b>planet</b> from the <b>Sun</b> and the largest <b>planet</b> in the Solar <b>System</b> .                                                                                                                                                                                                                                                                                                                                                                                                                                                                                                                                                                                                                                                                                                                                                                                                                                                                                                           |                                                 |
| 254: what city was the convention when gerald ford was nominated                                                                                                                                                                                                                                                                                                                                                                                                                                                                                                                                                                                                                                                                                                                                                                                                                                                                                                                                                                   | <i>1976 Republican National Convention</i>      |
| Held in Kemper Arena in Kansas <b>City</b> , Missouri, the <b>convention</b> nominated President <b>Gerald Ford</b> for a full term, but only after narrowly defeating a strong challenge from former California Governor Ronald Reagan.                                                                                                                                                                                                                                                                                                                                                                                                                                                                                                                                                                                                                                                                                                                                                                                           |                                                 |
| 261: what county is northville mi                                                                                                                                                                                                                                                                                                                                                                                                                                                                                                                                                                                                                                                                                                                                                                                                                                                                                                                                                                                                  | <i>Northville, Michigan</i>                     |
| Most of the <b>city</b> is in Oakland <b>County</b> , and is surrounded by the <b>city</b> of <b>Novi</b> .                                                                                                                                                                                                                                                                                                                                                                                                                                                                                                                                                                                                                                                                                                                                                                                                                                                                                                                        |                                                 |
| 289: what do porcupines eat                                                                                                                                                                                                                                                                                                                                                                                                                                                                                                                                                                                                                                                                                                                                                                                                                                                                                                                                                                                                        | <i>Porcupine</i>                                |
| It <b>eats</b> leaves, herbs, twigs and green plants like skunk cabbage and clover and in the winter it may <b>eat</b> bark.                                                                                                                                                                                                                                                                                                                                                                                                                                                                                                                                                                                                                                                                                                                                                                                                                                                                                                       |                                                 |
| 290: what did elijah mccooy invent                                                                                                                                                                                                                                                                                                                                                                                                                                                                                                                                                                                                                                                                                                                                                                                                                                                                                                                                                                                                 | <i>Elijah McCoy</i>                             |
| <b>Elijah J. McCoy</b> (May 2, 1844 – October 10, 1929) was a black Canadian-American inventor and engineer, who was notable for his 57 U.S. patents, most to do with lubrication of steam engines.                                                                                                                                                                                                                                                                                                                                                                                                                                                                                                                                                                                                                                                                                                                                                                                                                                |                                                 |
| 299: What does the idea of effective nuclear charge tell us                                                                                                                                                                                                                                                                                                                                                                                                                                                                                                                                                                                                                                                                                                                                                                                                                                                                                                                                                                        | <i>Effective nuclear charge</i>                 |
| The term “ <b>effective</b> ” is used because the shielding <b>effect</b> of negatively <b>charged</b> electrons prevents higher orbital electrons from experiencing the full <b>nuclear charge</b> by the repelling <b>effect</b> of inner-layer electrons.                                                                                                                                                                                                                                                                                                                                                                                                                                                                                                                                                                                                                                                                                                                                                                       |                                                 |
| 303: what domain is eu                                                                                                                                                                                                                                                                                                                                                                                                                                                                                                                                                                                                                                                                                                                                                                                                                                                                                                                                                                                                             | <i>.eu</i>                                      |
| <b>.eu</b> is the country code top-level <b>domain</b> (ccTLD) for the European Union (EU).                                                                                                                                                                                                                                                                                                                                                                                                                                                                                                                                                                                                                                                                                                                                                                                                                                                                                                                                        |                                                 |
| 304: What does the name “Meister” mean in German                                                                                                                                                                                                                                                                                                                                                                                                                                                                                                                                                                                                                                                                                                                                                                                                                                                                                                                                                                                   | <i>Meister</i>                                  |
| <b>Meister</b> means master in <b>German</b> (as in master craftsman, or as an honorific title such as <b>Meister</b> Eckhart).                                                                                                                                                                                                                                                                                                                                                                                                                                                                                                                                                                                                                                                                                                                                                                                                                                                                                                    |                                                 |
| 309: what did tycho brahe do                                                                                                                                                                                                                                                                                                                                                                                                                                                                                                                                                                                                                                                                                                                                                                                                                                                                                                                                                                                                       | <i>Tycho Brahe</i>                              |
| <b>Tycho Brahe</b> (14 December 1546/24 October 1601), born Tyge Ottesen <b>Brahe</b> , was a <b>Danish</b> nobleman known for his accurate and comprehensive astronomical and planetary observations.                                                                                                                                                                                                                                                                                                                                                                                                                                                                                                                                                                                                                                                                                                                                                                                                                             |                                                 |
| 317: what holiday is first weekend of september                                                                                                                                                                                                                                                                                                                                                                                                                                                                                                                                                                                                                                                                                                                                                                                                                                                                                                                                                                                    | <i>Labor day</i>                                |
| Labor Day is an American federal <b>holiday</b> observed on the <b>first</b> Monday in <b>September</b> , that celebrates the economic and social contributions of workers.                                                                                                                                                                                                                                                                                                                                                                                                                                                                                                                                                                                                                                                                                                                                                                                                                                                        |                                                 |
| 320: what does life insurance cover?                                                                                                                                                                                                                                                                                                                                                                                                                                                                                                                                                                                                                                                                                                                                                                                                                                                                                                                                                                                               | <i>Life insurance</i>                           |
| <b>Life insurance</b> is a contract between an <b>insured</b> ( <b>insurance</b> policy holder) and an <b>insurer</b> , where the <b>insurer</b> promises to pay a designated <b>beneficiary</b> a sum of money (the “ <b>benefits</b> ”) upon the <b>death</b> of the <b>insured person</b> .                                                                                                                                                                                                                                                                                                                                                                                                                                                                                                                                                                                                                                                                                                                                     |                                                 |
| 327: how is a backpack made                                                                                                                                                                                                                                                                                                                                                                                                                                                                                                                                                                                                                                                                                                                                                                                                                                                                                                                                                                                                        | <i>Backpack</i>                                 |
| The bag itself was <b>made</b> up of different <b>animal</b> hide and skin (depending on what sorts of animals were in the area) and sewn together by the intestines of said animals, which were woven together tightly to <b>make</b> a sturdy thread-like material.                                                                                                                                                                                                                                                                                                                                                                                                                                                                                                                                                                                                                                                                                                                                                              |                                                 |

- 331: what day is st. patricks day  
Saint **Patrick's Day** or the Feast of Saint **Patrick** (, "the **Day** of the Festival of **Patrick**") is a cultural and religious holiday celebrated on 17 March. *Saint Patrick's Day*
- 334: what cheese is made from goat's milk  
**Goat cheese**, or chèvre (from the French word for goat), is **cheese made out of the milk of goats** . *Goat cheese*
- 338: what country is belize in  
**Belize** , is a **country** located on the northeastern **coast** of Central **America**. *Belize*
- 342: how does a cat purr  
However, using a strict definition of **purring** that continuous sound production must alternate between pulmonic egressive and ingressive airstream (and usually go on for minutes), Peters (2002), in an exhaustive review of the scientific literature, reached the conclusion that until then only "**purring cats**" (Felidae) and two species of genets , Genetta tigrina, and most likely also Genetta genetta, had been documented to **purr**. *Purr*
- 346: what county is St. Elizabeth MO in  
**St. Elizabeth** is a village in Miller **County** , Missouri , United States . *St. Elizabeth, Missouri*
- 348: what county is wilton ca in  
**Wilton** is a census-designated place (CDP) in Sacramento **County** , California , United States . *Wilton, California*
- #354: how many gold gloves does barry larkin have  
**Larkin** is considered one of the top players of his era , winning nine Silver Slugger **awards** and three **Gold Glove awards** . *Barry Larkin*
- 361: how did women's role change during the war  
Whether it was on the home front or the front-lines, for civilian or enlisted **women**, the World Wars started a new era for **women's opportunities to contribute in war** and be recognized for efforts outside of the home. *Women's roles in the World Wars*
- 366: how does lsd impact the human body  
Lysergic acid diethylamide, abbreviated **LSD** or LSD-25, also known as lysergide ( INN ) and colloquially as acid, is a semisynthetic **psychedelic** drug of the ergoline family, well known for its psychological effects which can include altered thinking processes, closed and open eye visuals, synesthesia, an altered sense of time and spiritual experiences , as well as for its key role in 1960s counterculture . *Lysergic acid diethylamide*
- Currently, a number of organizations—including the Beckley Foundation , MAPS , Heffter Research Institute and the Albert Hofmann Foundation—exist to fund, encourage and coordinate research into the medicinal and spiritual uses of **LSD** and related **psychedelics** .
- 374: what county is orono maine in  
**Orono** is a town in Penobscot **County** , **Maine** , United States . *Orono, Maine*
- 377: what it is a pilot study  
A **pilot** experiment, also called a **pilot study** , is a small scale preliminary **study** conducted in order to evaluate feasibility, time, cost, adverse events, and effect size (statistical variability) in an attempt to predict an appropriate sample size and improve upon the **study** design prior to performance of a full-scale research project. *Pilot experiment*
- #383: how many humps on a camel  
The two surviving species of **camel** are the dromedary , or one-humped **camel**, which is native to the Middle East and the Horn of Africa ; and the Bactrian , or two-humped **camel**, which **inhabits** Central Asia . *Camel*
- 384: what can be powered by wind  
**Wind power** is the conversion of **wind** energy into a useful form of energy, such as using **wind** turbines to make electrical **power** , windmills for mechanical **power**, **wind** pumps for water pumping or drainage , or sails to propel ships. *Wind power*
- 389: what chili wants wiki  
What Chili **Wants** is an American reality series on VH1 starring Chili , one-third of the Grammy Award -winning R&B trio TLC . *What Chili Wants*
- 398: what division is boise state football  
The **Boise State Broncos football** program represents **Boise State University** in college **football** and compete in the **Football** Bowl Subdivision (FBS) of **Division I** as a member of the Mountain West Conference . *Boise State Broncos football*
- #409: how much caffeine is in a shot of espresso  
**Espresso** has more **caffeine** per unit **volume** than most beverages, but the usual serving **size** is smaller—a typical **60 mL** (2 US fluid ounce ) of **espresso** has 80 to 150 mg of **caffeine**, **little** less than the 95 to 200 mg of a **standard 240 mL** (8 US fluid ounces ) **cup** of drip-brewed coffee. *Espresso*
- 417: what does add my two cents mean  
"My **two cents** " (2¢) and its longer version "put my **two cents** in" is an United States (US) idiomatic expression, taken from the original English idiom expression: to put in "my **two pennies** worth" or "my tuppence worth." *My two cents*
- 447: what does bruce jenner do  
William **Bruce Jenner** (born October 28, 1949) is a former U.S. track and field athlete , motivational speaker , socialite , television personality and businessman . *Bruce Jenner*
- 448: what does alkali do to liquids?  
In chemistry , an **alkali** (, from Arabic : **الْقَالِي** **الْقَالِي**) is a basic , ionic salt of an **alkali** metal or alkaline earth metal element . *Alkali*
- This broad use of the term is likely to have come about because **alkalis** were the first bases known to obey the Arrhenius definition of a base and are still among the more common bases.  
Some authors also define an **alkali** as a base that dissolves in water .
- 450: what area code is 217  
**Area code 217** is the North American telephone **area code** for much of western and central Illinois . *Area code 217*
- 462: what does gloria in excelsis deo mean  
"**Gloria in excelsis Deo**" ( Latin for "**Glor**y to God in the highest") is a hymn known also as the Greater Dooxology (as distinguished from the "Minor Dooxology" or **Gloria Patri**) and the Angelic Hymn. *Gloria in Excelsis Deo*
- #463: how many grams in a Troy ounce of gold  
The **Troy ounce** is 480 **grains**, compared with the avoirdupois **ounce**, which is <sup>480</sup>/<sub>14</sub> **grains**. *Troy weight*
- #473: how much does united states spend on health care  
According to the **World Health** Organization (WHO), the **United States** spent more on **health care** per **capita** (\$7,146), and more on **health care** as percentage of its GDP (15.2%), than any other **nation** in 2008. *Health care in the United States*
- #488: how many died in Hiroshima and Nagasaki  
Within the first two to four months of the **bombings**, the acute **effects** killed 90,000–166,000 people in **Hiroshima** and 60,000–80,000 in **Nagasaki**, with roughly half of the **deaths** in each **city** occurring on the first day. *Atomic bombings of Hiroshima and Nagasaki*
- 490: what county is Holly Ridge nc in?  
**Holly Ridge** is a town in Onslow **County** , North Carolina , United States . *Holly Ridge, North Carolina*
- 503: what kind of books does debbie macomber writes  
**Debbie Macomber** (born October 22, 1948 in Yakima, Washington) is a best-selling American author of over 150 romance novels and contemporary women's fiction. *Debbie Macomber*
- 504: what county is catonsville md in  
**Catonsville** is the home of the University of Maryland, Baltimore **County** (UMBC), a public research university with over 12,000 students. *Catonsville, Maryland*
- Catonsville** is a census-designated place (CDP) in Baltimore **County** , Maryland , United States.
- 509: what kind of literature did john steinbeck writing  
As the author of twenty-seven **books**, including sixteen novels, six non-fiction **books**, and five collections of short stories, **Steinbeck** received the **Nobel Prize for Literature** in 1962. *John Steinbeck*
- 510: whatever happened clint walker  
Norman Eugene **Walker**, known as **Clint Walker** (born May 30, 1927), is a retired American actor . *Clint Walker*
- 512: what does the family leave act  
The **Family and Medical Leave Act** of 1993 (FMLA) is a United States federal law requiring covered employers to provide employees job-protected and unpaid **leave** for qualified **medical** and **family reasons**. *Family and Medical Leave Act of 1993*
- 515: How is the pothole formed  
A **pothole** (sometimes called a kettle and known in parts of the Western United States as a chuckhole) is a type of disruption in the surface of a roadway where a portion of the road material has broken away, leaving a hole.  
A deep **pothole** on New York City's Second Avenue *Pothole*
- 517: what does este lauder do  
**Estée Lauder** Companies, Inc. is a manufacturer and marketer of prestige skincare, makeup, fragrance and hair care products. *Estée Lauder Companies*
- 534: what creates sonic boom  
A **sonic boom** is the **sound** associated with the shock waves **created** by an object traveling through the air faster than the **speed of sound**. *Sonic boom*
- 551: what city is oregon state university in  
**Oregon State University** (OSU) is a coeducational , public **research university** located in Corvallis , **Oregon** , United States . *Oregon State University*
- #561: how many bones are in the skeletal system is composed of 306 bones  
*Human skeleton*
- Humans are born with over 270 **bones**, some of which fuse together into a longitudinal axis, the axial **skeleton** , to which the appendicular **skeleton** is attached.
- 564: What county is North Myrtle Beach in SC  
**North Myrtle Beach** is a coastal resort city in **Horry County** , **South Carolina** , United States . *North Myrtle Beach, South Carolina*
- #568: how much of our universe does plasma make up  
In the **universe**, **plasma** is the most common state of **matter** for ordinary **matter** , most of which is in the rarefied intergalactic **plasma** (particularly intracluster medium ) and in stars. *Plasma (physics)*
- 571: what does barefoot and pregnant mean  
The phrase "**barefoot** and **pregnant**" was probably first used sometime before 1950.  
The only way to keep a woman happy," he said, "is to keep her **barefoot** and **pregnant**."  
"**Barefoot** and **pregnant**" is a phrase most commonly associated with the controversial idea that women should not work outside the home and should have many children during their reproductive years. *Barefoot and pregnant*
- 572: what county is oakhurst, nj in  
**Oakhurst**, **New Jersey** is a census-designated place and unincorporated community within Ocean Township , in Monmouth **County** , **New Jersey** , United States. *Oakhurst, New Jersey*
- 574: What did Lawrence Joshua Chamberlain do?  
**Joshua Lawrence Chamberlain** (September 8, 1828 – February 24, 1914), born as **Lawrence Joshua Chamberlain**, was an American **college** professor from the State of Maine , who volunteered during the American Civil War to join the Union Army . *Joshua Chamberlain*
- 575: what circuit court is maryland  
The **Circuit Courts of Maryland** are the state trial **courts** of general jurisdiction in **Maryland**. *Maryland Circuit Courts*
- 577: what causes a deficiency in adenosine deaminase  
**Adenosine deaminase deficiency**, also called **ADA deficiency** or ADA-SCID, is an autosomal recessive metabolic disorder that **causes immunodeficiency** . *Adenosine deaminase deficiency*
- 582: how is human height measured  
**Human height** is the distance from the bottom of the feet to the top of the head in a **human** body , standing erect. *Human height*
- Human height** is the distance from the bottom of the feet to the top of the head in a **human** body , standing erect.  
A **timing belt** is a non-slipping mechanical drive **belt** and the term may refer to either:  
**Timing belt** (camshaft), a toothed **belt** used to drive the camshaft(s) within an internal combustion engine  
**A timing belt** is a non-slipping mechanical drive **belt** and the term may refer to either: *Timing belt*
- 604: what channel is shopnbc on  
**ShopNBC** is an American broadcast and cable home shopping network, owned and operated by ValueVision Media , which is in turn 30% owned by GE Equity and NBC Universal. *ShopNBC*
- 606: how post and lintels are used  
**Post and lintel**, "prop and **lintel**" or "trabeated" is a simple construction method using a **lintel** , header, or architrave as the horizontal member over a building void supported at its ends by two vertical columns , or . *Post and lintel*
- 616: what county is Cambria WI in  
**Cambria** is a village in Columbia **County** , Wisconsin , United States . *Cambria, Wisconsin*
- #622: HOW MANY STRIPES ARE ON THE AMERICAN FLAG  
The national **flag** of the United States of **America** , often simply referred to as the **American flag**, consists of **thirteen** equal horizontal **stripes** of **red** (**top** and **bottom**) **alternating** with **white**, with a **blue** rectangle in the canton (referred to specifically as the "union") bearing fifty small, **white**, **five-pointed stars** arranged in nine offset horizontal rows of **six stars** (**top** and **bottom**) **alternating** with rows of **five stars**. *Flag of the United States*
- 625: what do biologists do  
**Biologists** involved in basic research attempt to discover underlying mechanisms that govern how organisms work. *Biologist*
- Biologists** involved in applied research attempt to develop or improve medical, industrial or agricultural processes.  
A **biologist** is a scientist who studies living organisms and their relationship to their environment.
- 626: what does base jumping stand for  
**BASE jumping**, also sometimes written as B.A.S.E. **jumping**, is an activity where participants **jump** from **fixed** objects and use a **parachute** to break their fall. *BASE jumping*
- 631: What country is the largest stalagmite  
The **largest stalagmite** in the world is high and is located in the cave of Cueva Martin Inferno, Cuba. *Stalagmite*
- 633: what does Gringo mean  
Roger Axtell, a travel etiquette expert, notes that "[t]he word **gringo** is not necessarily a bad word.  
**Gringo** ( , ) is a slang Spanish and Portuguese word used in Ibero-America , to denote foreigners, often from the United States . *Gringo*
- 638: what does hair testing show  
A drug **test** is a technical analysis of a biological specimen – for example urine, **hair**, blood, sweat, or oral fluid / saliva – to determine the presence or absence of specified parent drugs or their metabolites . *Drug test*
- 644: what hormones produce thyroid  
The **thyroid hormones**, triiodothyronine (T3) and thyroxine (T4), are tyrosine -based **hormones produced by the thyroid gland** that are primarily responsible for regulation of metabolism. *Thyroid hormone*
- 645: what does automatic paper feeder on printers mean  
In multifunction or all-in-one **printers**, fax machines , photocopiers and scanners , an **automatic document feeder** or ADF is a feature which takes several pages and **feeds** the **paper** one page at a time into a scanner or copier, allowing the user to scan , and thereby copy , **print** , or fax , multiple-page documents without having to manually replace each page. *Automatic Document Feeder*
- #660: how old a child pedophile crime  
As a medical diagnosis, **pedophilia** or paedophilia is a psychiatric **disorder** in persons 16 years of **age** or **older** typically characterized by a primary or exclusive sexual interest toward **prepubescent children** (generally **age** 11 years or **younger**, though specific diagnosis criteria for the **disorder** extends the cut-off point for prepubescence to **age** 13). *Pedophilia*
- #662: how many people were killed in the holocaust  
Over one **million** Jewish children were **killed** in the **Holocaust**, as were **approximately** two **million** Jewish women and three **million** Jewish men. *The Holocaust*
- 679: what channel is letterman on  
Late Show with David **Letterman** is an American late-night talk show **hosted** by David **Letterman** on CBS . *Late Show with David Letterman*
- 683: what does karma mean in buddhism  
**Karma** ( Sanskrit, also **karmān**, Pāli : Kamma) **means** "action" or "doing"; whatever one does, says, or thinks is a **karma**. *Karma in Buddhism*
- 687: what kind is a tilapia  
**Tilapia** ( ) is the common name for nearly a hundred species of cichlid fish from the **tilapine** cichlid tribe . *Tilapia*
- #695: how many grape farms in united states  
As of the last census of agriculture in 2007, there were 2.2 **million farms**, covering an area of , an average of per **farm**. *Agriculture in the United States*
- 696: what freezes faster? hot or cold water?  
The Mpemba effect, named after Tanzanian student Erasto Mpemba , is the assertion that warmer **water** can **freeze faster** than **colder water**. *Mpemba effect*
- 698: what causes a small bowel obstruction  
**Bowel obstruction** (or intestinal **obstruction**) is a mechanical or functional **obstruction** of the intestines, preventing the normal transit of the products of digestion. *Bowel obstruction*
- #699: how many qfc stores are there  
Quality Food Centers (**QFC**) is a supermarket chain based in Bellevue, Washington , with 64 **stores** in the Puget Sound region of Washington state and in the Portland, Oregon metropolitan area. *QFC*
- 705: What Causes Brain Freezing  
It is **caused** by having something cold touch the roof of the mouth ( palate ), and is believed to result from a nerve response **causing** rapid constriction and swelling of blood vessels or a "referring " of pain from the roof of the mouth to the head. *Ice-cream headache*
- 708: what does leeroy jenkins mean  
**Leeroy Jenkins**, sometimes misspelled **Leroy Jenkins** and often elongated with numerous additional letters, is an Internet meme named for a player character created by Ben Schulz in Blizzard Entertainment's MMORPG , World of Warcraft . *Leeroy Jenkins*
- #722: how many episodes of Lost were there  
A total of 121 **episodes** of **Lost** were produced, the last of which aired on May 23, 2010.  
ABC announced that **Lost** would end after six seasons, having produced a total of 121 **episodes**. *List of Lost episodes*
- #742: how much does a gold bar weigh  
The standard **gold bar** held as **gold** reserves by central banks and traded among bullion dealers is the 400-troy-ounce (12.4 kg or 438.9 ounces) Good Delivery **gold bar**. *Gold bar*
- 743: what county is bolingbrook il in?  
**Bolingbrook** is a large village in Will and DuPage **Counties** in the U.S. state of Illinois . *Bolingbrook, Illinois*
- #745: how many kids does archie manning have  
He is the father of current Denver Broncos quarterback Peyton **Manning** , current New York Giants **starting** quarterback Eli **Manning** , and former Ole Miss receiver **Cooper Manning** . *Archie Manning*

|                                                                                                                                                                                                                                                                                                                                                                                                                                                                                                                                                                                                                                                                                                                                                                                                                                                                                                                                                                                                                                                                                                                                                                                                                                                                                                                                                                                                                                                                                                                                                                                                                                                                                                                                                                                                                                                                                                                                                                                                                                                                                                                                                                                                                                                                                                                                                                                                                                                                                                                                                                                                                                                                                                                                                                                                                                                                                                                                                                                                                                                                                                                                                                                                                                                                                                                                                                                                                                                                                                                                                                                                                                                                                                                                                                                                                                                                                                                                                                                                                                                                                                                                                                                                                                                                                                                                                                                                                                                                                                                                                                                                                                                                                                                                                                                                                                                                                                                                                                                                                                                                                                                                                                                                                                                                                                                                                                                                                                                                                                                                                                                                                                                                                                                                                                                                                                                                                                                                                                                                                                                                                                                                                                                                                                                                                                                                                                                                                                                                                                                                                                                                                                                                                                                                                                                                                                                                                                                                                                                                                                                                                                                                                                                                                                                                                                                                                                                                                                                                                                                                                                                                                                                                                                                                                                                                                                                                                                                                                                                                                                                                                                                                                                                                                                                                                                                                                                                                                                                                                                                                                                                                                                                                                                                                                                                                                                                                                                                                                                                                                                                                                                                                                                                                                                                                                                                                                                                                                                                                                                                                                                                                                                                                                                                                                                                                                                                                                |                                                                                                                                                                                                                                                                                                                                                                                                                                                                                                                                                                                                                                                                                                                                                                                                                                |
|--------------------------------------------------------------------------------------------------------------------------------------------------------------------------------------------------------------------------------------------------------------------------------------------------------------------------------------------------------------------------------------------------------------------------------------------------------------------------------------------------------------------------------------------------------------------------------------------------------------------------------------------------------------------------------------------------------------------------------------------------------------------------------------------------------------------------------------------------------------------------------------------------------------------------------------------------------------------------------------------------------------------------------------------------------------------------------------------------------------------------------------------------------------------------------------------------------------------------------------------------------------------------------------------------------------------------------------------------------------------------------------------------------------------------------------------------------------------------------------------------------------------------------------------------------------------------------------------------------------------------------------------------------------------------------------------------------------------------------------------------------------------------------------------------------------------------------------------------------------------------------------------------------------------------------------------------------------------------------------------------------------------------------------------------------------------------------------------------------------------------------------------------------------------------------------------------------------------------------------------------------------------------------------------------------------------------------------------------------------------------------------------------------------------------------------------------------------------------------------------------------------------------------------------------------------------------------------------------------------------------------------------------------------------------------------------------------------------------------------------------------------------------------------------------------------------------------------------------------------------------------------------------------------------------------------------------------------------------------------------------------------------------------------------------------------------------------------------------------------------------------------------------------------------------------------------------------------------------------------------------------------------------------------------------------------------------------------------------------------------------------------------------------------------------------------------------------------------------------------------------------------------------------------------------------------------------------------------------------------------------------------------------------------------------------------------------------------------------------------------------------------------------------------------------------------------------------------------------------------------------------------------------------------------------------------------------------------------------------------------------------------------------------------------------------------------------------------------------------------------------------------------------------------------------------------------------------------------------------------------------------------------------------------------------------------------------------------------------------------------------------------------------------------------------------------------------------------------------------------------------------------------------------------------------------------------------------------------------------------------------------------------------------------------------------------------------------------------------------------------------------------------------------------------------------------------------------------------------------------------------------------------------------------------------------------------------------------------------------------------------------------------------------------------------------------------------------------------------------------------------------------------------------------------------------------------------------------------------------------------------------------------------------------------------------------------------------------------------------------------------------------------------------------------------------------------------------------------------------------------------------------------------------------------------------------------------------------------------------------------------------------------------------------------------------------------------------------------------------------------------------------------------------------------------------------------------------------------------------------------------------------------------------------------------------------------------------------------------------------------------------------------------------------------------------------------------------------------------------------------------------------------------------------------------------------------------------------------------------------------------------------------------------------------------------------------------------------------------------------------------------------------------------------------------------------------------------------------------------------------------------------------------------------------------------------------------------------------------------------------------------------------------------------------------------------------------------------------------------------------------------------------------------------------------------------------------------------------------------------------------------------------------------------------------------------------------------------------------------------------------------------------------------------------------------------------------------------------------------------------------------------------------------------------------------------------------------------------------------------------------------------------------------------------------------------------------------------------------------------------------------------------------------------------------------------------------------------------------------------------------------------------------------------------------------------------------------------------------------------------------------------------------------------------------------------------------------------------------------------------------------------------------------------------------------------------------------------------------------------------------------------------------------------------------------------------------------------------------------------------------------------------------------------------------------------------------------------------------------------------------------------------------------------------------------------------------------------------------------------------------------------------------------------------------------------------------------------------------------------------------------------------------------------------------------------------------------------------------------------------------------------------------------------------------------------------------------------------------------------------------------------------------------------------------------------------------------------------------------------------------------------------------------------------------------------------------------------------------------------------------------------------------------------------------------------------------------------------------------------------------------------------------------------------------------------------------------------------------------------------------------------------------------------------------------------------------------------------------------------------------------------------------------------------------------------------------------------------------------------------------------------------------------------------------------------------------------------------------------------------------------------------------------------------------------------------------------------------------------------------------------------------------------------------------------------------------------------------------------------------------------------------------------------------------------------------------------------------------------------------------------|--------------------------------------------------------------------------------------------------------------------------------------------------------------------------------------------------------------------------------------------------------------------------------------------------------------------------------------------------------------------------------------------------------------------------------------------------------------------------------------------------------------------------------------------------------------------------------------------------------------------------------------------------------------------------------------------------------------------------------------------------------------------------------------------------------------------------------|
| 746: what does an advocacy website promote?<br>Research is beginning to explore how <b>advocacy</b> groups in the U.S. and Canada are using social media to facilitate civic engagement and collective action.<br>Lobbying (often by lobby groups) is a form of <b>advocacy</b> where a direct approach is made to legislators on an issue which plays a significant role in modern politics.<br><b>Advocacy</b> is a political process by an individual or group which aims to influence public-policy and resource allocation decisions within political, economic, and social systems and institutions.<br><b>Advocacy</b> can include many activities that a person or organization undertakes including media campaigns, public speaking, commissioning and publishing research or polls or the filing of an amicus brief .                                                                                                                                                                                                                                                                                                                                                                                                                                                                                                                                                                                                                                                                                                                                                                                                                                                                                                                                                                                                                                                                                                                                                                                                                                                                                                                                                                                                                                                                                                                                                                                                                                                                                                                                                                                                                                                                                                                                                                                                                                                                                                                                                                                                                                                                                                                                                                                                                                                                                                                                                                                                                                                                                                                                                                                                                                                                                                                                                                                                                                                                                                                                                                                                                                                                                                                                                                                                                                                                                                                                                                                                                                                                                                                                                                                                                                                                                                                                                                                                                                                                                                                                                                                                                                                                                                                                                                                                                                                                                                                                                                                                                                                                                                                                                                                                                                                                                                                                                                                                                                                                                                                                                                                                                                                                                                                                                                                                                                                                                                                                                                                                                                                                                                                                                                                                                                                                                                                                                                                                                                                                                                                                                                                                                                                                                                                                                                                                                                                                                                                                                                                                                                                                                                                                                                                                                                                                                                                                                                                                                                                                                                                                                                                                                                                                                                                                                                                                                                                                                                                                                                                                                                                                                                                                                                                                                                                                                                                                                                                                                                                                                                                                                                                                                                                                                                                                                                                                                                                                                                                                                                                                                                                                                                                                                                                                                                                                                                                                                                                                                                               | <i>Advocacy</i>                                                                                                                                                                                                                                                                                                                                                                                                                                                                                                                                                                                                                                                                                                                                                                                                                |
| #750: how many amendments in us<br>The Constitution has been <b>amended</b> seventeen <b>additional</b> times (for a total of <b>twenty-seven</b> amendments).                                                                                                                                                                                                                                                                                                                                                                                                                                                                                                                                                                                                                                                                                                                                                                                                                                                                                                                                                                                                                                                                                                                                                                                                                                                                                                                                                                                                                                                                                                                                                                                                                                                                                                                                                                                                                                                                                                                                                                                                                                                                                                                                                                                                                                                                                                                                                                                                                                                                                                                                                                                                                                                                                                                                                                                                                                                                                                                                                                                                                                                                                                                                                                                                                                                                                                                                                                                                                                                                                                                                                                                                                                                                                                                                                                                                                                                                                                                                                                                                                                                                                                                                                                                                                                                                                                                                                                                                                                                                                                                                                                                                                                                                                                                                                                                                                                                                                                                                                                                                                                                                                                                                                                                                                                                                                                                                                                                                                                                                                                                                                                                                                                                                                                                                                                                                                                                                                                                                                                                                                                                                                                                                                                                                                                                                                                                                                                                                                                                                                                                                                                                                                                                                                                                                                                                                                                                                                                                                                                                                                                                                                                                                                                                                                                                                                                                                                                                                                                                                                                                                                                                                                                                                                                                                                                                                                                                                                                                                                                                                                                                                                                                                                                                                                                                                                                                                                                                                                                                                                                                                                                                                                                                                                                                                                                                                                                                                                                                                                                                                                                                                                                                                                                                                                                                                                                                                                                                                                                                                                                                                                                                                                                                                                                                 | <i>United States Constitution</i>                                                                                                                                                                                                                                                                                                                                                                                                                                                                                                                                                                                                                                                                                                                                                                                              |
| 751: what city is george washington university<br>The <b>George Washington University</b> (GW, <b>GWU</b> , or <b>George Washington</b> ) is a comprehensive private , coeducational research <b>university</b> located in <b>Washington, D.C.</b> .                                                                                                                                                                                                                                                                                                                                                                                                                                                                                                                                                                                                                                                                                                                                                                                                                                                                                                                                                                                                                                                                                                                                                                                                                                                                                                                                                                                                                                                                                                                                                                                                                                                                                                                                                                                                                                                                                                                                                                                                                                                                                                                                                                                                                                                                                                                                                                                                                                                                                                                                                                                                                                                                                                                                                                                                                                                                                                                                                                                                                                                                                                                                                                                                                                                                                                                                                                                                                                                                                                                                                                                                                                                                                                                                                                                                                                                                                                                                                                                                                                                                                                                                                                                                                                                                                                                                                                                                                                                                                                                                                                                                                                                                                                                                                                                                                                                                                                                                                                                                                                                                                                                                                                                                                                                                                                                                                                                                                                                                                                                                                                                                                                                                                                                                                                                                                                                                                                                                                                                                                                                                                                                                                                                                                                                                                                                                                                                                                                                                                                                                                                                                                                                                                                                                                                                                                                                                                                                                                                                                                                                                                                                                                                                                                                                                                                                                                                                                                                                                                                                                                                                                                                                                                                                                                                                                                                                                                                                                                                                                                                                                                                                                                                                                                                                                                                                                                                                                                                                                                                                                                                                                                                                                                                                                                                                                                                                                                                                                                                                                                                                                                                                                                                                                                                                                                                                                                                                                                                                                                                                                                                                                                           | <i>George Washington University</i>                                                                                                                                                                                                                                                                                                                                                                                                                                                                                                                                                                                                                                                                                                                                                                                            |
| #755: How many Muslims live in the United Kingdom?<br>The vast majority of <b>Muslims</b> in the <b>United Kingdom</b> live in England and Wales : of 1,591,000 <b>Muslims</b> recorded at the 2001 Census, 1,536,015 were <b>living</b> in England and Wales , where they formed 3% of the <b>population</b> in 2001; 42,557 were <b>living</b> in Scotland , forming 0.84% of the <b>population</b> ; and 1,943 were <b>living</b> in Northern Ireland .                                                                                                                                                                                                                                                                                                                                                                                                                                                                                                                                                                                                                                                                                                                                                                                                                                                                                                                                                                                                                                                                                                                                                                                                                                                                                                                                                                                                                                                                                                                                                                                                                                                                                                                                                                                                                                                                                                                                                                                                                                                                                                                                                                                                                                                                                                                                                                                                                                                                                                                                                                                                                                                                                                                                                                                                                                                                                                                                                                                                                                                                                                                                                                                                                                                                                                                                                                                                                                                                                                                                                                                                                                                                                                                                                                                                                                                                                                                                                                                                                                                                                                                                                                                                                                                                                                                                                                                                                                                                                                                                                                                                                                                                                                                                                                                                                                                                                                                                                                                                                                                                                                                                                                                                                                                                                                                                                                                                                                                                                                                                                                                                                                                                                                                                                                                                                                                                                                                                                                                                                                                                                                                                                                                                                                                                                                                                                                                                                                                                                                                                                                                                                                                                                                                                                                                                                                                                                                                                                                                                                                                                                                                                                                                                                                                                                                                                                                                                                                                                                                                                                                                                                                                                                                                                                                                                                                                                                                                                                                                                                                                                                                                                                                                                                                                                                                                                                                                                                                                                                                                                                                                                                                                                                                                                                                                                                                                                                                                                                                                                                                                                                                                                                                                                                                                                                                                                                                                                                     | <i>Islam in the United Kingdom</i>                                                                                                                                                                                                                                                                                                                                                                                                                                                                                                                                                                                                                                                                                                                                                                                             |
| #763: how long to take iwo jima<br>The Battle of <b>Iwo Jima</b> (19 February – 26 March 1945), or <b>Operation Detachment</b> , was a major battle in which the <b>United States Armed Forces</b> fought for and captured the island of <b>Iwo Jima</b> from the Japanese Empire .                                                                                                                                                                                                                                                                                                                                                                                                                                                                                                                                                                                                                                                                                                                                                                                                                                                                                                                                                                                                                                                                                                                                                                                                                                                                                                                                                                                                                                                                                                                                                                                                                                                                                                                                                                                                                                                                                                                                                                                                                                                                                                                                                                                                                                                                                                                                                                                                                                                                                                                                                                                                                                                                                                                                                                                                                                                                                                                                                                                                                                                                                                                                                                                                                                                                                                                                                                                                                                                                                                                                                                                                                                                                                                                                                                                                                                                                                                                                                                                                                                                                                                                                                                                                                                                                                                                                                                                                                                                                                                                                                                                                                                                                                                                                                                                                                                                                                                                                                                                                                                                                                                                                                                                                                                                                                                                                                                                                                                                                                                                                                                                                                                                                                                                                                                                                                                                                                                                                                                                                                                                                                                                                                                                                                                                                                                                                                                                                                                                                                                                                                                                                                                                                                                                                                                                                                                                                                                                                                                                                                                                                                                                                                                                                                                                                                                                                                                                                                                                                                                                                                                                                                                                                                                                                                                                                                                                                                                                                                                                                                                                                                                                                                                                                                                                                                                                                                                                                                                                                                                                                                                                                                                                                                                                                                                                                                                                                                                                                                                                                                                                                                                                                                                                                                                                                                                                                                                                                                                                                                                                                                                                            | <i>Battle of Iwo Jima</i>                                                                                                                                                                                                                                                                                                                                                                                                                                                                                                                                                                                                                                                                                                                                                                                                      |
| 764: What a Margarita contains<br>The <b>margarita</b> is a Mexican cocktail consisting of tequila mixed with Cointreau or similar orange -flavoured liqueur and lime or lemon juice , often served with salt on the glass rim.<br>The drink is served shaken with ice (on the rocks), blended with ice (frozen margarita), or without ice (straight up).                                                                                                                                                                                                                                                                                                                                                                                                                                                                                                                                                                                                                                                                                                                                                                                                                                                                                                                                                                                                                                                                                                                                                                                                                                                                                                                                                                                                                                                                                                                                                                                                                                                                                                                                                                                                                                                                                                                                                                                                                                                                                                                                                                                                                                                                                                                                                                                                                                                                                                                                                                                                                                                                                                                                                                                                                                                                                                                                                                                                                                                                                                                                                                                                                                                                                                                                                                                                                                                                                                                                                                                                                                                                                                                                                                                                                                                                                                                                                                                                                                                                                                                                                                                                                                                                                                                                                                                                                                                                                                                                                                                                                                                                                                                                                                                                                                                                                                                                                                                                                                                                                                                                                                                                                                                                                                                                                                                                                                                                                                                                                                                                                                                                                                                                                                                                                                                                                                                                                                                                                                                                                                                                                                                                                                                                                                                                                                                                                                                                                                                                                                                                                                                                                                                                                                                                                                                                                                                                                                                                                                                                                                                                                                                                                                                                                                                                                                                                                                                                                                                                                                                                                                                                                                                                                                                                                                                                                                                                                                                                                                                                                                                                                                                                                                                                                                                                                                                                                                                                                                                                                                                                                                                                                                                                                                                                                                                                                                                                                                                                                                                                                                                                                                                                                                                                                                                                                                                                                                                                                                                      | <i>Margarita</i>                                                                                                                                                                                                                                                                                                                                                                                                                                                                                                                                                                                                                                                                                                                                                                                                               |
| 766: what color is burgundy<br><b>Burgundy</b> is a dark red <b>color</b> associated with the <b>Burgundy</b> wine of the same name, which in turn is named after the <b>Burgundy</b> region of France .                                                                                                                                                                                                                                                                                                                                                                                                                                                                                                                                                                                                                                                                                                                                                                                                                                                                                                                                                                                                                                                                                                                                                                                                                                                                                                                                                                                                                                                                                                                                                                                                                                                                                                                                                                                                                                                                                                                                                                                                                                                                                                                                                                                                                                                                                                                                                                                                                                                                                                                                                                                                                                                                                                                                                                                                                                                                                                                                                                                                                                                                                                                                                                                                                                                                                                                                                                                                                                                                                                                                                                                                                                                                                                                                                                                                                                                                                                                                                                                                                                                                                                                                                                                                                                                                                                                                                                                                                                                                                                                                                                                                                                                                                                                                                                                                                                                                                                                                                                                                                                                                                                                                                                                                                                                                                                                                                                                                                                                                                                                                                                                                                                                                                                                                                                                                                                                                                                                                                                                                                                                                                                                                                                                                                                                                                                                                                                                                                                                                                                                                                                                                                                                                                                                                                                                                                                                                                                                                                                                                                                                                                                                                                                                                                                                                                                                                                                                                                                                                                                                                                                                                                                                                                                                                                                                                                                                                                                                                                                                                                                                                                                                                                                                                                                                                                                                                                                                                                                                                                                                                                                                                                                                                                                                                                                                                                                                                                                                                                                                                                                                                                                                                                                                                                                                                                                                                                                                                                                                                                                                                                                                                                                                                       | <i>Burgundy (color)</i>                                                                                                                                                                                                                                                                                                                                                                                                                                                                                                                                                                                                                                                                                                                                                                                                        |
| 773: what day is the feast of st joseph's?<br>Saint <b>Joseph's Day</b> , March 19, the <b>Feast of St. Joseph</b> is in Western Christianity the principal <b>feast day</b> of Saint <b>Joseph</b> , Spouse of the Blessed Virgin Mary .                                                                                                                                                                                                                                                                                                                                                                                                                                                                                                                                                                                                                                                                                                                                                                                                                                                                                                                                                                                                                                                                                                                                                                                                                                                                                                                                                                                                                                                                                                                                                                                                                                                                                                                                                                                                                                                                                                                                                                                                                                                                                                                                                                                                                                                                                                                                                                                                                                                                                                                                                                                                                                                                                                                                                                                                                                                                                                                                                                                                                                                                                                                                                                                                                                                                                                                                                                                                                                                                                                                                                                                                                                                                                                                                                                                                                                                                                                                                                                                                                                                                                                                                                                                                                                                                                                                                                                                                                                                                                                                                                                                                                                                                                                                                                                                                                                                                                                                                                                                                                                                                                                                                                                                                                                                                                                                                                                                                                                                                                                                                                                                                                                                                                                                                                                                                                                                                                                                                                                                                                                                                                                                                                                                                                                                                                                                                                                                                                                                                                                                                                                                                                                                                                                                                                                                                                                                                                                                                                                                                                                                                                                                                                                                                                                                                                                                                                                                                                                                                                                                                                                                                                                                                                                                                                                                                                                                                                                                                                                                                                                                                                                                                                                                                                                                                                                                                                                                                                                                                                                                                                                                                                                                                                                                                                                                                                                                                                                                                                                                                                                                                                                                                                                                                                                                                                                                                                                                                                                                                                                                                                                                                                                      | <i>Saint Joseph's Day</i>                                                                                                                                                                                                                                                                                                                                                                                                                                                                                                                                                                                                                                                                                                                                                                                                      |
| 791: what does a laboratory in a gynecologist office consist of<br>A <b>medical laboratory</b> or clinical <b>laboratory</b> is a <b>laboratory</b> where tests are done on clinical specimens in order to get information about the health of a patient as pertaining to the diagnosis, treatment, and prevention of disease.                                                                                                                                                                                                                                                                                                                                                                                                                                                                                                                                                                                                                                                                                                                                                                                                                                                                                                                                                                                                                                                                                                                                                                                                                                                                                                                                                                                                                                                                                                                                                                                                                                                                                                                                                                                                                                                                                                                                                                                                                                                                                                                                                                                                                                                                                                                                                                                                                                                                                                                                                                                                                                                                                                                                                                                                                                                                                                                                                                                                                                                                                                                                                                                                                                                                                                                                                                                                                                                                                                                                                                                                                                                                                                                                                                                                                                                                                                                                                                                                                                                                                                                                                                                                                                                                                                                                                                                                                                                                                                                                                                                                                                                                                                                                                                                                                                                                                                                                                                                                                                                                                                                                                                                                                                                                                                                                                                                                                                                                                                                                                                                                                                                                                                                                                                                                                                                                                                                                                                                                                                                                                                                                                                                                                                                                                                                                                                                                                                                                                                                                                                                                                                                                                                                                                                                                                                                                                                                                                                                                                                                                                                                                                                                                                                                                                                                                                                                                                                                                                                                                                                                                                                                                                                                                                                                                                                                                                                                                                                                                                                                                                                                                                                                                                                                                                                                                                                                                                                                                                                                                                                                                                                                                                                                                                                                                                                                                                                                                                                                                                                                                                                                                                                                                                                                                                                                                                                                                                                                                                                                                                 | <i>Medical laboratory</i>                                                                                                                                                                                                                                                                                                                                                                                                                                                                                                                                                                                                                                                                                                                                                                                                      |
| 812: what countries allow gays to openly serve in the military<br>Nations that permit <b>gay</b> people to <b>serve openly</b> in the <b>military</b> include the 4 of the 5 members of the UN Security Council (United States, United Kingdom, France, and Russia), the Republic of China (Taiwan), Australia , <b>Israel</b> , <b>South Africa</b> , Argentina , and all NATO members excluding Turkey .                                                                                                                                                                                                                                                                                                                                                                                                                                                                                                                                                                                                                                                                                                                                                                                                                                                                                                                                                                                                                                                                                                                                                                                                                                                                                                                                                                                                                                                                                                                                                                                                                                                                                                                                                                                                                                                                                                                                                                                                                                                                                                                                                                                                                                                                                                                                                                                                                                                                                                                                                                                                                                                                                                                                                                                                                                                                                                                                                                                                                                                                                                                                                                                                                                                                                                                                                                                                                                                                                                                                                                                                                                                                                                                                                                                                                                                                                                                                                                                                                                                                                                                                                                                                                                                                                                                                                                                                                                                                                                                                                                                                                                                                                                                                                                                                                                                                                                                                                                                                                                                                                                                                                                                                                                                                                                                                                                                                                                                                                                                                                                                                                                                                                                                                                                                                                                                                                                                                                                                                                                                                                                                                                                                                                                                                                                                                                                                                                                                                                                                                                                                                                                                                                                                                                                                                                                                                                                                                                                                                                                                                                                                                                                                                                                                                                                                                                                                                                                                                                                                                                                                                                                                                                                                                                                                                                                                                                                                                                                                                                                                                                                                                                                                                                                                                                                                                                                                                                                                                                                                                                                                                                                                                                                                                                                                                                                                                                                                                                                                                                                                                                                                                                                                                                                                                                                                                                                                                                                                                     | <i>Sexual orientation and military service</i>                                                                                                                                                                                                                                                                                                                                                                                                                                                                                                                                                                                                                                                                                                                                                                                 |
| 813: How Works Diaphragm Pump<br>A <b>diaphragm pump</b> (also known as a Membrane <b>pump</b> , Air Operated Double <b>Diaphragm Pump</b> (AODD) or Pneumatic <b>Diaphragm Pump</b> ) is a positive displacement <b>pump</b> that uses a combination of the reciprocating action of a rubber , thermoplastic or teflon <b>diaphragm</b> and suitable valves either side of the <b>diaphragm</b> ( check valve , butterfly valves, flap valves, or any other form of shut-off valves) to <b>pump</b> a fluid .                                                                                                                                                                                                                                                                                                                                                                                                                                                                                                                                                                                                                                                                                                                                                                                                                                                                                                                                                                                                                                                                                                                                                                                                                                                                                                                                                                                                                                                                                                                                                                                                                                                                                                                                                                                                                                                                                                                                                                                                                                                                                                                                                                                                                                                                                                                                                                                                                                                                                                                                                                                                                                                                                                                                                                                                                                                                                                                                                                                                                                                                                                                                                                                                                                                                                                                                                                                                                                                                                                                                                                                                                                                                                                                                                                                                                                                                                                                                                                                                                                                                                                                                                                                                                                                                                                                                                                                                                                                                                                                                                                                                                                                                                                                                                                                                                                                                                                                                                                                                                                                                                                                                                                                                                                                                                                                                                                                                                                                                                                                                                                                                                                                                                                                                                                                                                                                                                                                                                                                                                                                                                                                                                                                                                                                                                                                                                                                                                                                                                                                                                                                                                                                                                                                                                                                                                                                                                                                                                                                                                                                                                                                                                                                                                                                                                                                                                                                                                                                                                                                                                                                                                                                                                                                                                                                                                                                                                                                                                                                                                                                                                                                                                                                                                                                                                                                                                                                                                                                                                                                                                                                                                                                                                                                                                                                                                                                                                                                                                                                                                                                                                                                                                                                                                                                                                                                                                                 | <i>Diaphragm pump</i>                                                                                                                                                                                                                                                                                                                                                                                                                                                                                                                                                                                                                                                                                                                                                                                                          |
| #815: how many percent is a basis point<br>The relationship between percentage changes and <b>basis points</b> can be summarized as follows: 1 percentage <b>point</b> change = 100 <b>basis points</b> , and 0.01 percentage <b>points</b> = 1 <b>basis point</b> .                                                                                                                                                                                                                                                                                                                                                                                                                                                                                                                                                                                                                                                                                                                                                                                                                                                                                                                                                                                                                                                                                                                                                                                                                                                                                                                                                                                                                                                                                                                                                                                                                                                                                                                                                                                                                                                                                                                                                                                                                                                                                                                                                                                                                                                                                                                                                                                                                                                                                                                                                                                                                                                                                                                                                                                                                                                                                                                                                                                                                                                                                                                                                                                                                                                                                                                                                                                                                                                                                                                                                                                                                                                                                                                                                                                                                                                                                                                                                                                                                                                                                                                                                                                                                                                                                                                                                                                                                                                                                                                                                                                                                                                                                                                                                                                                                                                                                                                                                                                                                                                                                                                                                                                                                                                                                                                                                                                                                                                                                                                                                                                                                                                                                                                                                                                                                                                                                                                                                                                                                                                                                                                                                                                                                                                                                                                                                                                                                                                                                                                                                                                                                                                                                                                                                                                                                                                                                                                                                                                                                                                                                                                                                                                                                                                                                                                                                                                                                                                                                                                                                                                                                                                                                                                                                                                                                                                                                                                                                                                                                                                                                                                                                                                                                                                                                                                                                                                                                                                                                                                                                                                                                                                                                                                                                                                                                                                                                                                                                                                                                                                                                                                                                                                                                                                                                                                                                                                                                                                                                                                                                                                                           | <i>Basis point</i>                                                                                                                                                                                                                                                                                                                                                                                                                                                                                                                                                                                                                                                                                                                                                                                                             |
| 819: what genre is bloody beetroots<br>The <b>Bloody Beetroots</b> is well-known for the black Venom mask he wears during performances.<br>The <b>Bloody Beetroots</b> is the pseudonym of Sir Bob Cornelius Rifo, the Italian electro house and dance-punk music producer , DJ and photographer .<br>"The <b>Bloody Beetroots DJ set</b> " contains Sir Bob Cornelius Rifo and Tommy Tea.                                                                                                                                                                                                                                                                                                                                                                                                                                                                                                                                                                                                                                                                                                                                                                                                                                                                                                                                                                                                                                                                                                                                                                                                                                                                                                                                                                                                                                                                                                                                                                                                                                                                                                                                                                                                                                                                                                                                                                                                                                                                                                                                                                                                                                                                                                                                                                                                                                                                                                                                                                                                                                                                                                                                                                                                                                                                                                                                                                                                                                                                                                                                                                                                                                                                                                                                                                                                                                                                                                                                                                                                                                                                                                                                                                                                                                                                                                                                                                                                                                                                                                                                                                                                                                                                                                                                                                                                                                                                                                                                                                                                                                                                                                                                                                                                                                                                                                                                                                                                                                                                                                                                                                                                                                                                                                                                                                                                                                                                                                                                                                                                                                                                                                                                                                                                                                                                                                                                                                                                                                                                                                                                                                                                                                                                                                                                                                                                                                                                                                                                                                                                                                                                                                                                                                                                                                                                                                                                                                                                                                                                                                                                                                                                                                                                                                                                                                                                                                                                                                                                                                                                                                                                                                                                                                                                                                                                                                                                                                                                                                                                                                                                                                                                                                                                                                                                                                                                                                                                                                                                                                                                                                                                                                                                                                                                                                                                                                                                                                                                                                                                                                                                                                                                                                                                                                                                                                                                                                                                                     | <i>The Bloody Beetroots</i>                                                                                                                                                                                                                                                                                                                                                                                                                                                                                                                                                                                                                                                                                                                                                                                                    |
| #838: how many asian indians live in usa<br><b>Indian Americans</b> are citizens of the United States of <b>Indian</b> ancestry and comprise about 3.18 million <b>people</b> , or ~1.0% of the U.S. <b>population</b> , the <b>country's</b> third largest self-reported <b>Asian</b> ancestral <b>group</b> after Chinese <b>Americans</b> and Filipino <b>Americans</b> according to <b>American</b> Community Survey of 2010 data.                                                                                                                                                                                                                                                                                                                                                                                                                                                                                                                                                                                                                                                                                                                                                                                                                                                                                                                                                                                                                                                                                                                                                                                                                                                                                                                                                                                                                                                                                                                                                                                                                                                                                                                                                                                                                                                                                                                                                                                                                                                                                                                                                                                                                                                                                                                                                                                                                                                                                                                                                                                                                                                                                                                                                                                                                                                                                                                                                                                                                                                                                                                                                                                                                                                                                                                                                                                                                                                                                                                                                                                                                                                                                                                                                                                                                                                                                                                                                                                                                                                                                                                                                                                                                                                                                                                                                                                                                                                                                                                                                                                                                                                                                                                                                                                                                                                                                                                                                                                                                                                                                                                                                                                                                                                                                                                                                                                                                                                                                                                                                                                                                                                                                                                                                                                                                                                                                                                                                                                                                                                                                                                                                                                                                                                                                                                                                                                                                                                                                                                                                                                                                                                                                                                                                                                                                                                                                                                                                                                                                                                                                                                                                                                                                                                                                                                                                                                                                                                                                                                                                                                                                                                                                                                                                                                                                                                                                                                                                                                                                                                                                                                                                                                                                                                                                                                                                                                                                                                                                                                                                                                                                                                                                                                                                                                                                                                                                                                                                                                                                                                                                                                                                                                                                                                                                                                                                                                                                                         | <i>Indian American</i>                                                                                                                                                                                                                                                                                                                                                                                                                                                                                                                                                                                                                                                                                                                                                                                                         |
| 843: what caused the world war 2<br>The main <b>causes of World War II</b> were nationalistic issues, unresolved issues, and resentments resulting from <b>World War I</b> and the interwar period in Europe, in addition to the effects of the Great Depression in the 1930s.                                                                                                                                                                                                                                                                                                                                                                                                                                                                                                                                                                                                                                                                                                                                                                                                                                                                                                                                                                                                                                                                                                                                                                                                                                                                                                                                                                                                                                                                                                                                                                                                                                                                                                                                                                                                                                                                                                                                                                                                                                                                                                                                                                                                                                                                                                                                                                                                                                                                                                                                                                                                                                                                                                                                                                                                                                                                                                                                                                                                                                                                                                                                                                                                                                                                                                                                                                                                                                                                                                                                                                                                                                                                                                                                                                                                                                                                                                                                                                                                                                                                                                                                                                                                                                                                                                                                                                                                                                                                                                                                                                                                                                                                                                                                                                                                                                                                                                                                                                                                                                                                                                                                                                                                                                                                                                                                                                                                                                                                                                                                                                                                                                                                                                                                                                                                                                                                                                                                                                                                                                                                                                                                                                                                                                                                                                                                                                                                                                                                                                                                                                                                                                                                                                                                                                                                                                                                                                                                                                                                                                                                                                                                                                                                                                                                                                                                                                                                                                                                                                                                                                                                                                                                                                                                                                                                                                                                                                                                                                                                                                                                                                                                                                                                                                                                                                                                                                                                                                                                                                                                                                                                                                                                                                                                                                                                                                                                                                                                                                                                                                                                                                                                                                                                                                                                                                                                                                                                                                                                                                                                                                                                 | <i>Causes of World War II</i>                                                                                                                                                                                                                                                                                                                                                                                                                                                                                                                                                                                                                                                                                                                                                                                                  |
| 867: how is root beer made?<br><b>Root beer</b> is a carbonated , sweetened beverage , originally <b>made</b> using the <b>root</b> of a sassafras plant (or the bark of a sassafras tree) as the primary flavor.                                                                                                                                                                                                                                                                                                                                                                                                                                                                                                                                                                                                                                                                                                                                                                                                                                                                                                                                                                                                                                                                                                                                                                                                                                                                                                                                                                                                                                                                                                                                                                                                                                                                                                                                                                                                                                                                                                                                                                                                                                                                                                                                                                                                                                                                                                                                                                                                                                                                                                                                                                                                                                                                                                                                                                                                                                                                                                                                                                                                                                                                                                                                                                                                                                                                                                                                                                                                                                                                                                                                                                                                                                                                                                                                                                                                                                                                                                                                                                                                                                                                                                                                                                                                                                                                                                                                                                                                                                                                                                                                                                                                                                                                                                                                                                                                                                                                                                                                                                                                                                                                                                                                                                                                                                                                                                                                                                                                                                                                                                                                                                                                                                                                                                                                                                                                                                                                                                                                                                                                                                                                                                                                                                                                                                                                                                                                                                                                                                                                                                                                                                                                                                                                                                                                                                                                                                                                                                                                                                                                                                                                                                                                                                                                                                                                                                                                                                                                                                                                                                                                                                                                                                                                                                                                                                                                                                                                                                                                                                                                                                                                                                                                                                                                                                                                                                                                                                                                                                                                                                                                                                                                                                                                                                                                                                                                                                                                                                                                                                                                                                                                                                                                                                                                                                                                                                                                                                                                                                                                                                                                                                                                                                                              | <i>Root beer</i>                                                                                                                                                                                                                                                                                                                                                                                                                                                                                                                                                                                                                                                                                                                                                                                                               |
| 872: what does informal logic mean<br><b>Informal logic</b> , intuitively, refers to the principles of <b>logic</b> and <b>logical</b> thought outside of a formal setting.                                                                                                                                                                                                                                                                                                                                                                                                                                                                                                                                                                                                                                                                                                                                                                                                                                                                                                                                                                                                                                                                                                                                                                                                                                                                                                                                                                                                                                                                                                                                                                                                                                                                                                                                                                                                                                                                                                                                                                                                                                                                                                                                                                                                                                                                                                                                                                                                                                                                                                                                                                                                                                                                                                                                                                                                                                                                                                                                                                                                                                                                                                                                                                                                                                                                                                                                                                                                                                                                                                                                                                                                                                                                                                                                                                                                                                                                                                                                                                                                                                                                                                                                                                                                                                                                                                                                                                                                                                                                                                                                                                                                                                                                                                                                                                                                                                                                                                                                                                                                                                                                                                                                                                                                                                                                                                                                                                                                                                                                                                                                                                                                                                                                                                                                                                                                                                                                                                                                                                                                                                                                                                                                                                                                                                                                                                                                                                                                                                                                                                                                                                                                                                                                                                                                                                                                                                                                                                                                                                                                                                                                                                                                                                                                                                                                                                                                                                                                                                                                                                                                                                                                                                                                                                                                                                                                                                                                                                                                                                                                                                                                                                                                                                                                                                                                                                                                                                                                                                                                                                                                                                                                                                                                                                                                                                                                                                                                                                                                                                                                                                                                                                                                                                                                                                                                                                                                                                                                                                                                                                                                                                                                                                                                                                    | <i>Informal logic</i>                                                                                                                                                                                                                                                                                                                                                                                                                                                                                                                                                                                                                                                                                                                                                                                                          |
| 874: what country is turkey in<br><b>Turkey</b> ( ), officially the Republic of <b>Turkey</b> , is a transcontinental <b>country</b> , <b>located</b> mostly on Anatolia in Western Asia and on East Thrace in Southeastern Europe .                                                                                                                                                                                                                                                                                                                                                                                                                                                                                                                                                                                                                                                                                                                                                                                                                                                                                                                                                                                                                                                                                                                                                                                                                                                                                                                                                                                                                                                                                                                                                                                                                                                                                                                                                                                                                                                                                                                                                                                                                                                                                                                                                                                                                                                                                                                                                                                                                                                                                                                                                                                                                                                                                                                                                                                                                                                                                                                                                                                                                                                                                                                                                                                                                                                                                                                                                                                                                                                                                                                                                                                                                                                                                                                                                                                                                                                                                                                                                                                                                                                                                                                                                                                                                                                                                                                                                                                                                                                                                                                                                                                                                                                                                                                                                                                                                                                                                                                                                                                                                                                                                                                                                                                                                                                                                                                                                                                                                                                                                                                                                                                                                                                                                                                                                                                                                                                                                                                                                                                                                                                                                                                                                                                                                                                                                                                                                                                                                                                                                                                                                                                                                                                                                                                                                                                                                                                                                                                                                                                                                                                                                                                                                                                                                                                                                                                                                                                                                                                                                                                                                                                                                                                                                                                                                                                                                                                                                                                                                                                                                                                                                                                                                                                                                                                                                                                                                                                                                                                                                                                                                                                                                                                                                                                                                                                                                                                                                                                                                                                                                                                                                                                                                                                                                                                                                                                                                                                                                                                                                                                                                                                                                                           | <i>Turkey</i>                                                                                                                                                                                                                                                                                                                                                                                                                                                                                                                                                                                                                                                                                                                                                                                                                  |
| 876: what county is Augusta,GA located in?<br><b>Augusta</b> is the principal city of the <b>Augusta – Richmond County</b> Metropolitan Statistical Area , which as of 2010 had an estimated population of 556,877, making it both the second-largest city and the second-largest metro area in the <b>state</b> after Atlanta .                                                                                                                                                                                                                                                                                                                                                                                                                                                                                                                                                                                                                                                                                                                                                                                                                                                                                                                                                                                                                                                                                                                                                                                                                                                                                                                                                                                                                                                                                                                                                                                                                                                                                                                                                                                                                                                                                                                                                                                                                                                                                                                                                                                                                                                                                                                                                                                                                                                                                                                                                                                                                                                                                                                                                                                                                                                                                                                                                                                                                                                                                                                                                                                                                                                                                                                                                                                                                                                                                                                                                                                                                                                                                                                                                                                                                                                                                                                                                                                                                                                                                                                                                                                                                                                                                                                                                                                                                                                                                                                                                                                                                                                                                                                                                                                                                                                                                                                                                                                                                                                                                                                                                                                                                                                                                                                                                                                                                                                                                                                                                                                                                                                                                                                                                                                                                                                                                                                                                                                                                                                                                                                                                                                                                                                                                                                                                                                                                                                                                                                                                                                                                                                                                                                                                                                                                                                                                                                                                                                                                                                                                                                                                                                                                                                                                                                                                                                                                                                                                                                                                                                                                                                                                                                                                                                                                                                                                                                                                                                                                                                                                                                                                                                                                                                                                                                                                                                                                                                                                                                                                                                                                                                                                                                                                                                                                                                                                                                                                                                                                                                                                                                                                                                                                                                                                                                                                                                                                                                                                                                                               | <i>Augusta, Georgia</i>                                                                                                                                                                                                                                                                                                                                                                                                                                                                                                                                                                                                                                                                                                                                                                                                        |
| 893: what does a cutter do<br>In baseball , a <b>cutter</b> , or <b>cut</b> fastball, is a type of fastball which breaks slightly toward the pitcher 's glove side as it reaches home plate.<br>When a batter is able to hit a <b>cutter</b> pitch, it often results in soft contact and an easy out, due to the pitch's movement keeping the ball away from the bat's sweet spot.<br>The <b>cutter</b> is typically 2–5 mph slower than a pitcher's four-seam fastball.<br>Some pitchers use a <b>cutter</b> as a way to prevent hitters from expecting their regular fastballs.<br>In 2010, the average pitch classified as a <b>cutter</b> by PITCHfx thrown by a right-handed pitcher was 88.6 mph; the average four-seamer was 92.1 mph.<br>An animated diagram of a <b>cutter</b><br>A common technique used to throw a <b>cutter</b> is to use a four-seam fastball grip with the baseball set slightly off center in the hand.                                                                                                                                                                                                                                                                                                                                                                                                                                                                                                                                                                                                                                                                                                                                                                                                                                                                                                                                                                                                                                                                                                                                                                                                                                                                                                                                                                                                                                                                                                                                                                                                                                                                                                                                                                                                                                                                                                                                                                                                                                                                                                                                                                                                                                                                                                                                                                                                                                                                                                                                                                                                                                                                                                                                                                                                                                                                                                                                                                                                                                                                                                                                                                                                                                                                                                                                                                                                                                                                                                                                                                                                                                                                                                                                                                                                                                                                                                                                                                                                                                                                                                                                                                                                                                                                                                                                                                                                                                                                                                                                                                                                                                                                                                                                                                                                                                                                                                                                                                                                                                                                                                                                                                                                                                                                                                                                                                                                                                                                                                                                                                                                                                                                                                                                                                                                                                                                                                                                                                                                                                                                                                                                                                                                                                                                                                                                                                                                                                                                                                                                                                                                                                                                                                                                                                                                                                                                                                                                                                                                                                                                                                                                                                                                                                                                                                                                                                                                                                                                                                                                                                                                                                                                                                                                                                                                                                                                                                                                                                                                                                                                                                                                                                                                                                                                                                                                                                                                                                                                                                                                                                                                                                                                                                                                                                                                                                                                                                                                         | <i>Cutter (baseball)</i>                                                                                                                                                                                                                                                                                                                                                                                                                                                                                                                                                                                                                                                                                                                                                                                                       |
| 895: what it takes aerosmith album<br>"What It <b>Takes</b> " is a power ballad by American hard rock band <b>Aerosmith</b> .                                                                                                                                                                                                                                                                                                                                                                                                                                                                                                                                                                                                                                                                                                                                                                                                                                                                                                                                                                                                                                                                                                                                                                                                                                                                                                                                                                                                                                                                                                                                                                                                                                                                                                                                                                                                                                                                                                                                                                                                                                                                                                                                                                                                                                                                                                                                                                                                                                                                                                                                                                                                                                                                                                                                                                                                                                                                                                                                                                                                                                                                                                                                                                                                                                                                                                                                                                                                                                                                                                                                                                                                                                                                                                                                                                                                                                                                                                                                                                                                                                                                                                                                                                                                                                                                                                                                                                                                                                                                                                                                                                                                                                                                                                                                                                                                                                                                                                                                                                                                                                                                                                                                                                                                                                                                                                                                                                                                                                                                                                                                                                                                                                                                                                                                                                                                                                                                                                                                                                                                                                                                                                                                                                                                                                                                                                                                                                                                                                                                                                                                                                                                                                                                                                                                                                                                                                                                                                                                                                                                                                                                                                                                                                                                                                                                                                                                                                                                                                                                                                                                                                                                                                                                                                                                                                                                                                                                                                                                                                                                                                                                                                                                                                                                                                                                                                                                                                                                                                                                                                                                                                                                                                                                                                                                                                                                                                                                                                                                                                                                                                                                                                                                                                                                                                                                                                                                                                                                                                                                                                                                                                                                                                                                                                                                                  | <i>What It Takes (song)</i>                                                                                                                                                                                                                                                                                                                                                                                                                                                                                                                                                                                                                                                                                                                                                                                                    |
| 898: what county is erie colorado<br><b>Erie</b> is a Statutory Town in Boulder and Weld <b>counties</b> in the U.S. <b>state</b> of <b>Colorado</b> .                                                                                                                                                                                                                                                                                                                                                                                                                                                                                                                                                                                                                                                                                                                                                                                                                                                                                                                                                                                                                                                                                                                                                                                                                                                                                                                                                                                                                                                                                                                                                                                                                                                                                                                                                                                                                                                                                                                                                                                                                                                                                                                                                                                                                                                                                                                                                                                                                                                                                                                                                                                                                                                                                                                                                                                                                                                                                                                                                                                                                                                                                                                                                                                                                                                                                                                                                                                                                                                                                                                                                                                                                                                                                                                                                                                                                                                                                                                                                                                                                                                                                                                                                                                                                                                                                                                                                                                                                                                                                                                                                                                                                                                                                                                                                                                                                                                                                                                                                                                                                                                                                                                                                                                                                                                                                                                                                                                                                                                                                                                                                                                                                                                                                                                                                                                                                                                                                                                                                                                                                                                                                                                                                                                                                                                                                                                                                                                                                                                                                                                                                                                                                                                                                                                                                                                                                                                                                                                                                                                                                                                                                                                                                                                                                                                                                                                                                                                                                                                                                                                                                                                                                                                                                                                                                                                                                                                                                                                                                                                                                                                                                                                                                                                                                                                                                                                                                                                                                                                                                                                                                                                                                                                                                                                                                                                                                                                                                                                                                                                                                                                                                                                                                                                                                                                                                                                                                                                                                                                                                                                                                                                                                                                                                                                         | <i>Erie, Colorado</i>                                                                                                                                                                                                                                                                                                                                                                                                                                                                                                                                                                                                                                                                                                                                                                                                          |
| 902: what classes are considered humanities<br>The <b>humanities</b> that are also regarded as social <b>sciences</b> include history , anthropology , area <b>studies</b> , communication <b>studies</b> , cultural <b>studies</b> , law , economics and linguistics .                                                                                                                                                                                                                                                                                                                                                                                                                                                                                                                                                                                                                                                                                                                                                                                                                                                                                                                                                                                                                                                                                                                                                                                                                                                                                                                                                                                                                                                                                                                                                                                                                                                                                                                                                                                                                                                                                                                                                                                                                                                                                                                                                                                                                                                                                                                                                                                                                                                                                                                                                                                                                                                                                                                                                                                                                                                                                                                                                                                                                                                                                                                                                                                                                                                                                                                                                                                                                                                                                                                                                                                                                                                                                                                                                                                                                                                                                                                                                                                                                                                                                                                                                                                                                                                                                                                                                                                                                                                                                                                                                                                                                                                                                                                                                                                                                                                                                                                                                                                                                                                                                                                                                                                                                                                                                                                                                                                                                                                                                                                                                                                                                                                                                                                                                                                                                                                                                                                                                                                                                                                                                                                                                                                                                                                                                                                                                                                                                                                                                                                                                                                                                                                                                                                                                                                                                                                                                                                                                                                                                                                                                                                                                                                                                                                                                                                                                                                                                                                                                                                                                                                                                                                                                                                                                                                                                                                                                                                                                                                                                                                                                                                                                                                                                                                                                                                                                                                                                                                                                                                                                                                                                                                                                                                                                                                                                                                                                                                                                                                                                                                                                                                                                                                                                                                                                                                                                                                                                                                                                                                                                                                                        | <i>Humanities</i>                                                                                                                                                                                                                                                                                                                                                                                                                                                                                                                                                                                                                                                                                                                                                                                                              |
| 910: what food is in afghan<br>Accompanying these staples are dairy products ( yogurt and whey ) , various <b>nuts</b> , and native vegetables, as well as fresh and dried <b>fruits</b> ; <b>Afghanistan</b> is well known for its grapes .                                                                                                                                                                                                                                                                                                                                                                                                                                                                                                                                                                                                                                                                                                                                                                                                                                                                                                                                                                                                                                                                                                                                                                                                                                                                                                                                                                                                                                                                                                                                                                                                                                                                                                                                                                                                                                                                                                                                                                                                                                                                                                                                                                                                                                                                                                                                                                                                                                                                                                                                                                                                                                                                                                                                                                                                                                                                                                                                                                                                                                                                                                                                                                                                                                                                                                                                                                                                                                                                                                                                                                                                                                                                                                                                                                                                                                                                                                                                                                                                                                                                                                                                                                                                                                                                                                                                                                                                                                                                                                                                                                                                                                                                                                                                                                                                                                                                                                                                                                                                                                                                                                                                                                                                                                                                                                                                                                                                                                                                                                                                                                                                                                                                                                                                                                                                                                                                                                                                                                                                                                                                                                                                                                                                                                                                                                                                                                                                                                                                                                                                                                                                                                                                                                                                                                                                                                                                                                                                                                                                                                                                                                                                                                                                                                                                                                                                                                                                                                                                                                                                                                                                                                                                                                                                                                                                                                                                                                                                                                                                                                                                                                                                                                                                                                                                                                                                                                                                                                                                                                                                                                                                                                                                                                                                                                                                                                                                                                                                                                                                                                                                                                                                                                                                                                                                                                                                                                                                                                                                                                                                                                                                                                   | <i>Afghan cuisine</i>                                                                                                                                                                                                                                                                                                                                                                                                                                                                                                                                                                                                                                                                                                                                                                                                          |
| 922: what kind of cut is tri tip<br>The <b>tri-tip</b> is a <b>cut</b> of beef from the bottom sirloin primal <b>cut</b> .                                                                                                                                                                                                                                                                                                                                                                                                                                                                                                                                                                                                                                                                                                                                                                                                                                                                                                                                                                                                                                                                                                                                                                                                                                                                                                                                                                                                                                                                                                                                                                                                                                                                                                                                                                                                                                                                                                                                                                                                                                                                                                                                                                                                                                                                                                                                                                                                                                                                                                                                                                                                                                                                                                                                                                                                                                                                                                                                                                                                                                                                                                                                                                                                                                                                                                                                                                                                                                                                                                                                                                                                                                                                                                                                                                                                                                                                                                                                                                                                                                                                                                                                                                                                                                                                                                                                                                                                                                                                                                                                                                                                                                                                                                                                                                                                                                                                                                                                                                                                                                                                                                                                                                                                                                                                                                                                                                                                                                                                                                                                                                                                                                                                                                                                                                                                                                                                                                                                                                                                                                                                                                                                                                                                                                                                                                                                                                                                                                                                                                                                                                                                                                                                                                                                                                                                                                                                                                                                                                                                                                                                                                                                                                                                                                                                                                                                                                                                                                                                                                                                                                                                                                                                                                                                                                                                                                                                                                                                                                                                                                                                                                                                                                                                                                                                                                                                                                                                                                                                                                                                                                                                                                                                                                                                                                                                                                                                                                                                                                                                                                                                                                                                                                                                                                                                                                                                                                                                                                                                                                                                                                                                                                                                                                                                                     | <i>Tri-tip</i>                                                                                                                                                                                                                                                                                                                                                                                                                                                                                                                                                                                                                                                                                                                                                                                                                 |
| 923: what county is willmar mn in?<br><b>Willmar</b> is a city in, and the <b>county</b> seat of, Kandiyohi <b>County</b> , Minnesota , United States .                                                                                                                                                                                                                                                                                                                                                                                                                                                                                                                                                                                                                                                                                                                                                                                                                                                                                                                                                                                                                                                                                                                                                                                                                                                                                                                                                                                                                                                                                                                                                                                                                                                                                                                                                                                                                                                                                                                                                                                                                                                                                                                                                                                                                                                                                                                                                                                                                                                                                                                                                                                                                                                                                                                                                                                                                                                                                                                                                                                                                                                                                                                                                                                                                                                                                                                                                                                                                                                                                                                                                                                                                                                                                                                                                                                                                                                                                                                                                                                                                                                                                                                                                                                                                                                                                                                                                                                                                                                                                                                                                                                                                                                                                                                                                                                                                                                                                                                                                                                                                                                                                                                                                                                                                                                                                                                                                                                                                                                                                                                                                                                                                                                                                                                                                                                                                                                                                                                                                                                                                                                                                                                                                                                                                                                                                                                                                                                                                                                                                                                                                                                                                                                                                                                                                                                                                                                                                                                                                                                                                                                                                                                                                                                                                                                                                                                                                                                                                                                                                                                                                                                                                                                                                                                                                                                                                                                                                                                                                                                                                                                                                                                                                                                                                                                                                                                                                                                                                                                                                                                                                                                                                                                                                                                                                                                                                                                                                                                                                                                                                                                                                                                                                                                                                                                                                                                                                                                                                                                                                                                                                                                                                                                                                                                        | <i>Willmar, Minnesota</i>                                                                                                                                                                                                                                                                                                                                                                                                                                                                                                                                                                                                                                                                                                                                                                                                      |
| #943: how many innings makes an official game<br>Since most professional baseball <b>games</b> are nine <b>innings</b> long, the fifth <b>inning</b> is used as the threshold for an <b>official game</b> .                                                                                                                                                                                                                                                                                                                                                                                                                                                                                                                                                                                                                                                                                                                                                                                                                                                                                                                                                                                                                                                                                                                                                                                                                                                                                                                                                                                                                                                                                                                                                                                                                                                                                                                                                                                                                                                                                                                                                                                                                                                                                                                                                                                                                                                                                                                                                                                                                                                                                                                                                                                                                                                                                                                                                                                                                                                                                                                                                                                                                                                                                                                                                                                                                                                                                                                                                                                                                                                                                                                                                                                                                                                                                                                                                                                                                                                                                                                                                                                                                                                                                                                                                                                                                                                                                                                                                                                                                                                                                                                                                                                                                                                                                                                                                                                                                                                                                                                                                                                                                                                                                                                                                                                                                                                                                                                                                                                                                                                                                                                                                                                                                                                                                                                                                                                                                                                                                                                                                                                                                                                                                                                                                                                                                                                                                                                                                                                                                                                                                                                                                                                                                                                                                                                                                                                                                                                                                                                                                                                                                                                                                                                                                                                                                                                                                                                                                                                                                                                                                                                                                                                                                                                                                                                                                                                                                                                                                                                                                                                                                                                                                                                                                                                                                                                                                                                                                                                                                                                                                                                                                                                                                                                                                                                                                                                                                                                                                                                                                                                                                                                                                                                                                                                                                                                                                                                                                                                                                                                                                                                                                                                                                                                                    | <i>Official game</i>                                                                                                                                                                                                                                                                                                                                                                                                                                                                                                                                                                                                                                                                                                                                                                                                           |
| 963: how tennessee became a state<br><b>Tennessee</b> was the last <b>state</b> to leave the <b>Union</b> and join the <b>Confederacy</b> at the outbreak of the U.S. Civil War in 1861, and the first <b>state</b> to be readmitted to the <b>Union</b> at the end of the war.<br>767: what county is coatesville indiana located in<br><b>Coatesville</b> is a town in Clay Township , Hendricks <b>County</b> , <b>Indiana</b> , United States .                                                                                                                                                                                                                                                                                                                                                                                                                                                                                                                                                                                                                                                                                                                                                                                                                                                                                                                                                                                                                                                                                                                                                                                                                                                                                                                                                                                                                                                                                                                                                                                                                                                                                                                                                                                                                                                                                                                                                                                                                                                                                                                                                                                                                                                                                                                                                                                                                                                                                                                                                                                                                                                                                                                                                                                                                                                                                                                                                                                                                                                                                                                                                                                                                                                                                                                                                                                                                                                                                                                                                                                                                                                                                                                                                                                                                                                                                                                                                                                                                                                                                                                                                                                                                                                                                                                                                                                                                                                                                                                                                                                                                                                                                                                                                                                                                                                                                                                                                                                                                                                                                                                                                                                                                                                                                                                                                                                                                                                                                                                                                                                                                                                                                                                                                                                                                                                                                                                                                                                                                                                                                                                                                                                                                                                                                                                                                                                                                                                                                                                                                                                                                                                                                                                                                                                                                                                                                                                                                                                                                                                                                                                                                                                                                                                                                                                                                                                                                                                                                                                                                                                                                                                                                                                                                                                                                                                                                                                                                                                                                                                                                                                                                                                                                                                                                                                                                                                                                                                                                                                                                                                                                                                                                                                                                                                                                                                                                                                                                                                                                                                                                                                                                                                                                                                                                                                                                                                                                            | <i>Tennessee</i>                                                                                                                                                                                                                                                                                                                                                                                                                                                                                                                                                                                                                                                                                                                                                                                                               |
| 968: how does Delaware support its claim to being the first state?<br><b>Delaware</b> was one of the 13 <b>colonies</b> participating in the <b>American</b> Revolution and on December 7, 1787, became the <b>first state</b> to ratify the Constitution of the United States , thereby becoming known as The <b>First State</b> .                                                                                                                                                                                                                                                                                                                                                                                                                                                                                                                                                                                                                                                                                                                                                                                                                                                                                                                                                                                                                                                                                                                                                                                                                                                                                                                                                                                                                                                                                                                                                                                                                                                                                                                                                                                                                                                                                                                                                                                                                                                                                                                                                                                                                                                                                                                                                                                                                                                                                                                                                                                                                                                                                                                                                                                                                                                                                                                                                                                                                                                                                                                                                                                                                                                                                                                                                                                                                                                                                                                                                                                                                                                                                                                                                                                                                                                                                                                                                                                                                                                                                                                                                                                                                                                                                                                                                                                                                                                                                                                                                                                                                                                                                                                                                                                                                                                                                                                                                                                                                                                                                                                                                                                                                                                                                                                                                                                                                                                                                                                                                                                                                                                                                                                                                                                                                                                                                                                                                                                                                                                                                                                                                                                                                                                                                                                                                                                                                                                                                                                                                                                                                                                                                                                                                                                                                                                                                                                                                                                                                                                                                                                                                                                                                                                                                                                                                                                                                                                                                                                                                                                                                                                                                                                                                                                                                                                                                                                                                                                                                                                                                                                                                                                                                                                                                                                                                                                                                                                                                                                                                                                                                                                                                                                                                                                                                                                                                                                                                                                                                                                                                                                                                                                                                                                                                                                                                                                                                                                                                                                                            | <i>Delaware</i>                                                                                                                                                                                                                                                                                                                                                                                                                                                                                                                                                                                                                                                                                                                                                                                                                |
| 973: what does fidelity do<br>FMR LLC ( <b>Fidelity</b> Management and Research) or <b>Fidelity</b> Investments is an American multinational financial services corporation.<br><b>Fidelity</b> Ventures is its venture capital arm.<br><b>Fidelity</b> Investments manages a large family of mutual funds , provides fund distribution and investment advice services, as well as providing discount brokerage services , retirement services, wealth management , securities execution and clearance, life insurance and a number of other services.<br><b>Fidelity</b> International Limited (FIL), was an international affiliate founded in 1969, serving most countries in the rest of the world.<br>976: what causes thunder sound<br>In turn, this expansion of air creates a sonic shock wave, similar to a sonic boom , which produces the <b>sound</b> of <b>thunder</b> , often referred to as a clap, crack, or peal of <b>thunder</b> .<br>990: what does continuous improvement mean<br>A <b>continual improvement</b> process, also often called a <b>continuous improvement</b> process (abbreviated as CIP or CI), is an ongoing effort to <b>improve</b> products, services, or processes.<br>993: what area code is 810<br><b>Area code 810</b> is the telephone <b>area code</b> serving eastern Michigan .<br>996: what kind of earthquake was haiti<br>The <b>2010 Haiti earthquake</b> was a catastrophic magnitude 7.0 Mw <b>earthquake</b> , with an epicenter near the town of L'Éogâne ( Ouest Department ) , <b>approximately</b> west of Port-au-Prince , <b>Haiti's</b> capital.<br>997: what kind of horse was mister ed<br>The stars of the show were Mister <b>Ed</b> , a palomino <b>horse</b> who could "talk", played by gelding Bamboo Harvester and voiced by former Western star Allan Lane (who went uncredited for the entire length of the series), and his owner, an eccentric and enormously klutzy , yet friendly, architect <b>named</b> Wilbur Post ( Alan Young ) .<br>999: who does chris humphries play for<br>Kris Nathan <b>Humphries</b> (born February 6, 1985) is an American professional basketball <b>player</b> with the Brooklyn Nets .<br>#1010: what year was the 8 track invented<br>Stereo <b>8</b> was created in 1964 by a consortium led by Bill Lear of Lear Jet Corporation, along with Ampex , Ford Motor <b>Company</b> , General Motors , Motorola , and RCA Victor Records (RCA).<br>1012: what are points on a mortgage<br>The longer you keep the property financed under the loan with purchased <b>points</b> , the more the money spent on the <b>points</b> will pay off.<br>Keeping the property or refinancing prior to this break-even <b>point</b> will result in a net financial loss for the buyer while selling the loan for longer than this break-even <b>point</b> will result in a net financial savings for the buyer.<br><b>Points</b> , sometimes also called a "discount <b>point</b> ", are a form of pre-paid interest .<br>1015: what are the official languages of nigeria<br>The <b>official language</b> of <b>Nigeria</b> , English , the former colonial <b>language</b> , was chosen to facilitate the cultural and linguistic unity of the country.<br>1020: who played guitar on the kiss album, creatures of the night<br>It is also the band's last <b>album</b> <b>recorded</b> with Ace Frehley credited as an official member (until 1998's Psycho Circus ), and its first <b>album</b> with Vinnie Vincent as the initially uncredited lead <b>guitarist</b> (Vincent would later be credited, but not featured primarily on the cover, of 1985's reissue of the <b>album</b> ).<br>1025: what are the different types of cross country skiing<br>Cross-country <b>skiing</b> is part of the Nordic <b>skiing</b> sport family, which includes <b>ski</b> jumping , Nordic combined (cross-country <b>skiing</b> and <b>ski</b> jumping), Biathlon ( <b>skiing</b> and rifle marksmanship ) and ski-orientation (which includes map navigation along snow trails and tracks).<br>1026: what are use taxes?<br>A <b>use tax</b> in United States is complementary to sales <b>tax</b> which means, if you buy a <b>Taxable</b> product/services without paying any Sales <b>tax</b> to vendor, you owe <b>use tax</b> .<br>1030: what is an array in programming<br>In computer science , <b>array programming languages</b> (also known as vector or multidimensional <b>languages</b> ) generalize operations on scalars to apply transparently to vectors , matrices , and higher dimensional <b>arrays</b> .<br>1032: who wrote a rose is a rose is a rose<br>The sentence " <b>Rose is a rose is a rose is a rose</b> " was <b>written</b> by Gertrude Stein as part of the 1913 poem Sacred Emily, which appeared in the 1922 book Geography and Plays.<br>1043: what state is jakarta in?<br><b>Jakarta</b> ( ), officially known as the Special <b>Capital Region</b> of <b>Jakarta</b> ( ), is the <b>capital</b> and largest <b>city</b> of <b>Indonesia</b> .<br>1046: what song is sung in 6 foot 7 foot<br>"6 Foot 7 Foot" (also styled as "6'7") is a <b>song</b> by American rapper Lil Wayne featuring label mate, Cory Gunz .<br>1052: who can file suspicious activity report<br>In United States financial regulation , a <b>suspicious activity report</b> (or SAR) is a <b>report</b> made by a financial institution to the Financial Crimes Enforcement Network (FinCEN), an <b>agency</b> of the United States Department of the Treasury , regarding <b>suspicious</b> or potentially <b>suspicious activity</b> .<br>1054: what are the sulfaas<br>The original antibacterial sulfonamides (sometimes called <b>sulfa</b> drugs or sulpha drugs) are synthetic antimicrobial agents that contain the sulfonamide <b>group</b> .<br>It is important to make a distinction between <b>sulfa</b> drugs and other sulfur-containing drugs and additives, such as sulfates and sulfites, which are chemically unrelated to the sulfonamide <b>group</b> , and do not cause the same hypersensitivity reactions seen in the sulfonamides.<br>1060: who owns joe's crab shack<br><b>Joe's Crab Shack</b> is an American chain of beach-themed seafood casual dining restaurants <b>owned</b> by Ignite Restaurant Group .<br>1063: what is a right wing christian<br><b>Christian right</b> is a term used in the United <b>States</b> to describe right-wing <b>Christian political</b> groups that are characterized by their strong support of socially conservative policies.<br>1072: what is an assist in basketball<br>In <b>basketball</b> , an <b>assist</b> is attributed to a player who passes the ball to a teammate in a way that leads to a score by field goal , meaning that he or she was " <b>assisting</b> " in the <b>basket</b> .<br>1088: what school district is alvin in?<br><b>Alvin Independent School District</b> is a <b>school district</b> based in <b>Alvin</b> , Texas ( USA ) .<br>1091: what are the houses of hogwarts<br><b>Hogwarts School</b> of Witchcraft and Wizardry, shortened <b>Hogwarts</b> , is a fictional British <b>school</b> of <b>magic</b> for <b>students</b> aged eleven to eighteen, and is the primary setting for the first six books in J.K. Rowling 's Harry Potter series.<br>1094: What kind of personality test is the MBTI<br>The Myers-Briggs Type <b>Indicator</b> ( <b>MBTI</b> ) <b>assessment</b> is a psychometric <b>questionnaire</b> designed to measure <b>psychological</b> preferences in how people perceive the world and make decisions.<br>1100: where does a flea live<br><b>Fleas</b> are external parasites , <b>living</b> by hematophagy off the blood of mammals and birds .<br>1108: who wrote rhymer of the ancient mariner<br>The <b>Rime of the Ancient Mariner</b> (originally The <b>Rime</b> of the Ancyent Mariner) is the longest major poem by the English poet Samuel Taylor Coleridge , <b>written</b> in 1797–98 and published in 1798 in the first <b>edition</b> of Lyrical Ballads .<br>#1109: when did freddie mercury die<br><b>Freddie Mercury</b> (born Farrokh Bulsara; Gujarati : ફરૃહ બલસૃરા, Phārōkh Bālāsāra); 5 September 1946 – 24 November 1991) was a British musician, singer and songwriter, best known as the lead vocalist and lyricist of the <b>rock</b> band Queen .<br>1111: what is a PAC file<br>The URL of the <b>PAC file</b> is either configured manually or determined automatically by the Web Proxy Autodiscovery Protocol.<br>The browser fetches this <b>PAC file</b> before requesting other URLs.<br>A proxy auto-config ( <b>PAC file</b> ) defines how web browsers and other user agents can automatically choose the appropriate proxy server (access method) for fetching a given URL .<br>A <b>PAC file</b> contains a JavaScript function "FindProxyForURL(url, host)".<br>1117: what are spoilers for<br><b>Spoilers</b> on the front of a vehicle are often called air dams, because in addition to directing air flow they also reduce the amount of air flowing underneath the vehicle which generally reduces aerodynamic lift and drag.<br><b>Spoilers</b> for cars are often incorrectly confused with, or the term used interchangeably with, wings.<br><b>Spoilers</b> are often fitted to race and high-performance sports cars , although they have become common on passenger vehicles as well.<br>Some <b>spoilers</b> are added to cars primarily for styling purposes and have either little aerodynamic benefit or even make the aerodynamics worse.<br>A <b>spoiler</b> is an automotive aerodynamic device whose intended design function is to " <b>spoil</b> " unfavorable air movement across a body of a vehicle in motion, usually described as turbulence or drag. | <i>Thunder</i><br><i>Continual improvement process</i><br><i>Area code 810</i><br><i>2010 Haiti earthquake</i><br><i>Mister Ed</i><br><i>Kris Humphries</i><br><i>8-track tape</i><br><i>Point (mortgage)</i><br><i>Languages of Nigeria</i><br><i>Creatures of the Night</i><br><i>Cross-country skiing</i><br><i>Use tax</i><br><i>Array programming</i><br><i>Rose is a rose is a rose is a rose</i><br><i>Jakarta</i><br><i>6 Foot 7 Foot</i><br><i>Suspicious activity report</i><br><i>Sulfonamide (medicine)</i><br><i>Joe's Crab Shack</i><br><i>Christian right</i><br><i>Assist (basketball)</i><br><i>Alvin Independent School District</i><br><i>Hogwarts</i><br><i>Myers-Briggs Type Indicator</i><br><i>Flea</i><br><i>The Rime of the Ancient Mariner</i><br><i>Freddie Mercury</i><br><i>Proxy auto-config</i> |

|                                                                                                                                                                                                                                                                                                                                                                                                                                                                                                                                                                                                                                                                                                                                                                                                                                                         |                                                             |
|---------------------------------------------------------------------------------------------------------------------------------------------------------------------------------------------------------------------------------------------------------------------------------------------------------------------------------------------------------------------------------------------------------------------------------------------------------------------------------------------------------------------------------------------------------------------------------------------------------------------------------------------------------------------------------------------------------------------------------------------------------------------------------------------------------------------------------------------------------|-------------------------------------------------------------|
| 1120: who sings i am a man of constant sorrow<br>"Man of Constant Sorrow" (also known as "I Am A Man of Constant Sorrow") is a traditional American folk song first recorded by Dick Burnett, a partially blind fiddler from Kentucky.                                                                                                                                                                                                                                                                                                                                                                                                                                                                                                                                                                                                                  | <i>Man of Constant Sorrow</i>                               |
| 1123: who kill franz ferdinand wwl<br>On 28 June 1914, Archduke <b>Franz Ferdinand</b> of Austria, heir presumptive to the Austro-Hungarian throne, and his wife, Sophie, Duchess of Hohenberg, were shot <b>dead</b> in Sarajevo, by Gavrilo Princip, one of a group of six Bosnian Serb assassins coordinated by Danilo Ilić.                                                                                                                                                                                                                                                                                                                                                                                                                                                                                                                         | <i>Assassination of Archduke Franz Ferdinand of Austria</i> |
| 1140: what is a mms message<br>Multimedia <b>Messaging Service (MMS)</b> is a standard way to send <b>messages</b> that include multimedia content to and from mobile phones.                                                                                                                                                                                                                                                                                                                                                                                                                                                                                                                                                                                                                                                                           | <i>Multimedia Messaging Service</i>                         |
| 1150: who sang proud mary<br>"Proud Mary" is a rock song written by American singer-songwriter and multi-instrumentalist John Fogerty, and <b>recorded</b> by his band Creedence Clearwater Revival.                                                                                                                                                                                                                                                                                                                                                                                                                                                                                                                                                                                                                                                    | <i>Proud Mary</i>                                           |
| 1154: where do crocodiles live<br><b>Crocodiles (subfamily Crocodylinae)</b> or <b>true crocodiles</b> are large aquatic tetrapods that <b>live</b> throughout the tropics in Africa, Asia, the Americas and Australia.                                                                                                                                                                                                                                                                                                                                                                                                                                                                                                                                                                                                                                 | <i>Crocodile</i>                                            |
| 1157: what relates to erosion<br>Water and wind <b>erosion</b> are now the two primary causes of land degradation; combined, they are responsible for 84% of degraded acreage, making excessive <b>erosion</b> one of the most significant global <b>environmental</b> problems.                                                                                                                                                                                                                                                                                                                                                                                                                                                                                                                                                                        | <i>Erosion</i>                                              |
| 1159: where in oregon is albany<br><b>Albany</b> is the 11th largest city in the U.S. state of <b>Oregon</b> , and is the <b>county</b> seat of <b>Linn County</b> .                                                                                                                                                                                                                                                                                                                                                                                                                                                                                                                                                                                                                                                                                    | <i>Albany, Oregon</i>                                       |
| #1168: when did abraham lincoln write the emancipation proclamation??<br>The <b>Emancipation Proclamation</b> was an <b>order</b> issued to all segments of the <b>Executive</b> branch (including the Army and Navy) of the United States by President <b>Abraham Lincoln</b> on January 1, 1863, during the American Civil War.                                                                                                                                                                                                                                                                                                                                                                                                                                                                                                                       | <i>Emancipation Proclamation</i>                            |
| 1172: what part of the pre-world war I arms race was the most intense?<br>The <b>causes of World War I</b> , which <b>began</b> in central Europe in late <b>July</b> 1914 and finished in 1918, included many factors, such as the conflicts and hostility of the four decades leading up to the <b>war</b> .                                                                                                                                                                                                                                                                                                                                                                                                                                                                                                                                          | <i>Causes of World War I</i>                                |
| #1182: when president nixon resigns<br>Richard Milhous <b>Nixon</b> (January 9, 1913 – April 22, 1994) was the 37th <b>President</b> of the United States, <b>serving</b> from 1969 to 1974, when he became the only <b>president to resign</b> the office.                                                                                                                                                                                                                                                                                                                                                                                                                                                                                                                                                                                             | <i>Richard Nixon</i>                                        |
| 1184: where fourth of july came from<br>Independence Day, commonly known as the <b>Fourth of July</b> , is a federal <b>holiday</b> in the United States commemorating the adoption of the Declaration of Independence on <b>July 4, 1776</b> , declaring independence from the Kingdom of Great Britain.                                                                                                                                                                                                                                                                                                                                                                                                                                                                                                                                               | <i>Independence Day (United States)</i>                     |
| 1194: what people used mayan numeral system<br><b>Maya numerals</b> are a vigesimal (base - twenty) <b>numeral system used</b> by the Pre-Columbian Maya civilization.                                                                                                                                                                                                                                                                                                                                                                                                                                                                                                                                                                                                                                                                                  | <i>Maya numerals</i>                                        |
| 1196: what is a newsgroup message<br><b>A Usenet newsgroup</b> is a usually within the <b>Usenet</b> system, for <b>messages</b> posted from many users in different locations.                                                                                                                                                                                                                                                                                                                                                                                                                                                                                                                                                                                                                                                                         | <i>Usenet newsgroup</i>                                     |
| 1204: who accompanied King louis the VII of France on the second crusade<br>The <b>Second Crusade</b> was announced by <b>Pope Eugene III</b> , and was the <b>first of the crusades</b> to be led by <b>European kings</b> , namely <b>Louis VII of France</b> and <b>Conrad III of Germany</b> , with help from a number of other <b>European nobles</b> .                                                                                                                                                                                                                                                                                                                                                                                                                                                                                            | <i>Second Crusade</i>                                       |
| #1207: when did gary moore die<br>Robert William <b>Gary Moore</b> (4 April 1952 – 6 February 2011), was a Northern Irish musician, most widely recognised as a singer and guitarist.                                                                                                                                                                                                                                                                                                                                                                                                                                                                                                                                                                                                                                                                   | <i>Gary Moore</i>                                           |
| 1209: what is a hosting company on a website<br>A web <b>hosting service</b> is a type of <b>Internet hosting service</b> that allows individuals and organizations to make their <b>website</b> accessible via the World Wide Web.                                                                                                                                                                                                                                                                                                                                                                                                                                                                                                                                                                                                                     | <i>Web hosting service</i>                                  |
| 1218: who owns Exxon Mobil<br>It is a direct descendant of John D. Rockefeller's Standard Oil company, and was formed on November 30, 1999, by the <b>merger of Exxon and Mobil</b> .                                                                                                                                                                                                                                                                                                                                                                                                                                                                                                                                                                                                                                                                   | <i>ExxonMobil</i>                                           |
| 1222: what is a rock quarry<br><b>A quarry</b> is a type of open-pit mine from which <b>rock</b> or minerals are extracted.                                                                                                                                                                                                                                                                                                                                                                                                                                                                                                                                                                                                                                                                                                                             | <i>Quarry</i>                                               |
| 1223: what kind of school is MIT<br>The <b>MIT Sloan School of Management</b> (also known as <b>MIT Sloan</b> or <b>Sloan</b> ) is the business <b>school of the Massachusetts Institute of Technology</b> , in Cambridge, <b>Massachusetts</b> , USA.                                                                                                                                                                                                                                                                                                                                                                                                                                                                                                                                                                                                  | <i>MIT Sloan School of Management</i>                       |
| 1225: what are banana plugs for<br>A <b>banana connector</b> (commonly <b>banana plug</b> for the male, <b>banana socket</b> or <b>banana jack</b> for the female) is a single-wire (one conductor) electrical connector used for joining wires to equipment.                                                                                                                                                                                                                                                                                                                                                                                                                                                                                                                                                                                           | <i>Banana connector</i>                                     |
| #1229: when did the trojan war take place<br>The ancient <b>Greeks thought</b> that the <b>Trojan War</b> was a <b>historical event</b> that had <b>taken place</b> in the 13th or 12th <b>century BC</b> , and <b>believed</b> that Troy was <b>located</b> in modern-day Turkey near the Dardanelles.                                                                                                                                                                                                                                                                                                                                                                                                                                                                                                                                                 | <i>Trojan War</i>                                           |
| 1230: what is a letterbox movie<br>The term refers to the shape of a <b>letter box</b> , a slot in a wall or door through which mail is delivered, being rectangular and wider than it is high.<br><b>Letterboxing</b> is the practice of transferring film shot in a widescreen aspect ratio to standard-width video formats while preserving the film's original aspect ratio.<br>A 2.35:1 widescreen image <b>letterboxed</b> in a 1.33:1 screen                                                                                                                                                                                                                                                                                                                                                                                                     | <i>Letterboxing (filming)</i>                               |
| #1243: when did the civil war start and where<br>The <b>American Civil War (ACW)</b> , also known as the <b>War</b> between the States or <b>simply the Civil War</b> (see naming), was a <b>civil war fought</b> from 1861 to 1865 between the United States (the "Union" or the "North") and several Southern <b>slave</b> states that declared their secession and formed the Confederate States of <b>America</b> (the "Confederacy" or the "South").                                                                                                                                                                                                                                                                                                                                                                                               | <i>American Civil War</i>                                   |
| 1244: What are the busiest airports in the world<br>The definition of the <b>world's busiest airport</b> has been specified by the <b>Airports Council International</b> in Geneva, Switzerland.                                                                                                                                                                                                                                                                                                                                                                                                                                                                                                                                                                                                                                                        | <i>World's busiest airport</i>                              |
| 1248: where the streets have no name filming location<br>The song was notably performed on a Los Angeles <b>rooftop</b> for the <b>filming</b> of its music <b>video</b> , which won a Grammy Award for Best Performance Music <b>Video</b> . Recently the song has been used by the NFL's Baltimore Ravens as their entrance song in Super Bowl XLVII.                                                                                                                                                                                                                                                                                                                                                                                                                                                                                                 | <i>Where the Streets Have No Name</i>                       |
| 1253: where did the mayflower land<br>The <b>Mayflower</b> was the ship that in 1620 transported 102 English Pilgrims, including a core group of Separatists, to New England.                                                                                                                                                                                                                                                                                                                                                                                                                                                                                                                                                                                                                                                                           | <i>Mayflower</i>                                            |
| 1257: what languages are spoken in south africa<br>The English version of the <b>South African</b> constitution refers to the <b>languages</b> by the names in those <b>languages</b> : isiZulu, isiXhosa, Afrikaans, Sepedi (referring to Northern Sotho), Setswana, English, Sesotho (referring to Southern Sotho), Xitsonga, Siswati, Tshivenda and isiNdebele (referring to <b>Southern Ndebele</b> ).                                                                                                                                                                                                                                                                                                                                                                                                                                              | <i>Languages of South Africa</i>                            |
| 1262: Who controlled Alaska before US?<br>The name " <b>Alaska</b> " (Аляска) was already introduced in the <b>Russian</b> colonial period, when it was used only for the peninsula and is derived from the Aleut <b>alaxsxaq</b> , meaning "the mainland" or, more literally, "the object towards which the action of the sea is directed".<br><b>Alaska</b> was purchased from <b>Russia</b> on March 30, 1867, for \$7.2 million (\$ adjusted for inflation) at approximately two cents per acre (\$4.74/km <sup>2</sup> ).<br><b>Alaska</b> () is a state in the United States, situated in the northwest extremity of the North American continent, with the international boundary with Canada to the east, the Arctic Ocean to the north, and the Pacific Ocean to the west and south, with <b>Russia</b> further west across the Bering Strait. | <i>Alaska</i>                                               |
| 1268: who sang black velvet<br>"Black Velvet" is a blues verse with a rock chorus written by Canadian songwriters Christopher Ward and David Tyson, recorded by Canadian <b>singer</b> songwriter Alannah Myles.                                                                                                                                                                                                                                                                                                                                                                                                                                                                                                                                                                                                                                        | <i>Black Velvet (song)</i>                                  |
| 1274: who produced loyal to the game?<br>Released in the United States on December 14, 2004 (December 12 in the United Kingdom), <b>Loyal to the Game</b> was <b>produced</b> by Eminem.                                                                                                                                                                                                                                                                                                                                                                                                                                                                                                                                                                                                                                                                | <i>Loyal to the Game</i>                                    |
| 1275: WHAT ARE HERITABLE TRAITS<br><b>heritability of a trait</b> within a population is the proportion of observable differences in a <b>trait</b> between individuals within a population that is due to genetic differences.                                                                                                                                                                                                                                                                                                                                                                                                                                                                                                                                                                                                                         | <i>Heritability</i>                                         |
| 1284: who does afge represent<br>The American Federation of Government Employees ( <b>AFGE</b> ) is an American labor union <b>representing</b> over 650,000 employees of the federal government, about 5,000 employees of the District of Columbia, and a few hundred private sector employees, mostly in and around federal facilities.                                                                                                                                                                                                                                                                                                                                                                                                                                                                                                               | <i>American Federation of Government Employees</i>          |
| 1292: who wrote puff the magic dragon<br>"Puff, the Magic Dragon" is a song <b>written</b> by Leonard Lipton and Peter Yarrow, and made popular by Yarrow's daughter Peter, Paul and Mary in a 1963 recording.                                                                                                                                                                                                                                                                                                                                                                                                                                                                                                                                                                                                                                          | <i>Puff, the Magic Dragon</i>                               |
| 1301: what is a vetting process<br><b>Vetting</b> is the <b>process</b> of performing a background check on someone before offering them employment, conferring an award, etc.                                                                                                                                                                                                                                                                                                                                                                                                                                                                                                                                                                                                                                                                          | <i>Vetting</i>                                              |
| #1303: when did the free soilers party start?<br>The <b>Free Soil Party</b> was a short-lived political <b>party</b> in the United States active in the 1848 and 1852 presidential elections, and in some state elections.                                                                                                                                                                                                                                                                                                                                                                                                                                                                                                                                                                                                                              | <i>Free Soil Party</i>                                      |
| 1308: where does the expression "knocking on wood" come from<br><b>Knocking on wood</b> , or to touch <b>wood</b> , refers to the apotropaic tradition in western folklore of literally touching <b>knocking on wood</b> , or merely stating that you are doing or intend same, in order to avoid "tempting fate" after making a favourable observation, a boast, or declaration concerning one's own death.                                                                                                                                                                                                                                                                                                                                                                                                                                            | <i>Knocking on wood</i>                                     |
| 1310: who sang the nights the lights went out<br>"The Night the <b>Lights Went Out</b> in Georgia" is a Southern Gothic song written by songwriter Bobby Russell and performed in 1972 by his then-wife Vicki Lawrence.                                                                                                                                                                                                                                                                                                                                                                                                                                                                                                                                                                                                                                 | <i>The Night the Lights Went Out in Georgia</i>             |
| 1315: what is a synthetic conduit<br>A <b>nerve guidance conduit</b> (also referred to as an <b>artificial nerve conduit</b> or <b>artificial nerve graft</b> , as opposed to an autograft) is an <b>artificial</b> means of guiding axonal regrowth to facilitate <b>nerve</b> regeneration and is one of several clinical <b>treatments for nerve injuries</b> .                                                                                                                                                                                                                                                                                                                                                                                                                                                                                      | <i>Nerve guidance conduit</i>                               |
| 1316: what is a wwII theater<br>The <b>European Theatre of World War II</b> , also known as the <b>European War</b> , was a huge area of heavy fighting across <b>Europe</b> from Germany's invasion of Poland on <b>September 1, 1939</b> until the end of the <b>war</b> with the German unconditional surrender on May 8, 1945 ( V-E Day ).                                                                                                                                                                                                                                                                                                                                                                                                                                                                                                          | <i>European Theatre of World War II</i>                     |
| 1318: what is amoxicillin for?<br><b>Amoxicillin</b> is susceptible to degradation by $\beta$ -lactamase -producing bacteria, which are resistant to a broad spectrum of $\beta$ -lactam antibiotics, such as penicillin.<br><b>Amoxicillin</b> is one of the most common antibiotics prescribed for children.<br><b>Amoxicillin</b> (INN), formerly amoxycillin (BAN), and abbreviated amox, is a moderate-spectrum, bacteriolytic, $\beta$ -lactam antibiotic used to treat bacterial infections caused by susceptible microorganisms.                                                                                                                                                                                                                                                                                                                | <i>Amoxicillin</i>                                          |
| 1321: what state was the civil war in<br>The <b>American Civil War (ACW)</b> , also known as the <b>War</b> between the States or <b>simply the Civil War</b> (see naming), was a <b>civil war fought</b> from 1861 to 1865 between the United States (the "Union" or the "North") and several Southern <b>slave</b> states that declared their secession and formed the Confederate States of <b>America</b> (the "Confederacy" or the "South").                                                                                                                                                                                                                                                                                                                                                                                                       | <i>American Civil War</i>                                   |
| 1322: where did the early humans live?<br>According to the Recent African Ancestry theory, modern <b>humans evolved</b> in Africa possibly from <b>Homo heidelbergensis</b> , <b>Homo rhodesiensis</b> or <b>Homo antecessor</b> and migrated out of the continent some 50,000 to 100,000 years ago, replacing local populations of <b>Homo erectus</b> , <b>Homo denisova</b> , <b>Homo floresiensis</b> and <b>Homo neanderthalensis</b> .                                                                                                                                                                                                                                                                                                                                                                                                            | <i>Human evolution</i>                                      |
| 1325: who invaded north africa during ww2<br><b>Operation Torch</b> (initially called <b>Operation Gymnast</b> ) was the British – American <b>invasion</b> of French <b>North Africa</b> in World War II during the <b>North Africa Campaign</b> , <b>started</b> on 8 November 1942.                                                                                                                                                                                                                                                                                                                                                                                                                                                                                                                                                                  | <i>Operation Torch</i>                                      |
| #1326: WHAT YEARS WAS THE CS VETTE PRODUCED<br>The <b>Chevrolet Corvette (C5)</b> is a sports car <b>produced</b> by the <b>Chevrolet</b> division of General Motors for the 1997 through 2004 model years.                                                                                                                                                                                                                                                                                                                                                                                                                                                                                                                                                                                                                                             | <i>Chevrolet Corvette (C5)</i>                              |
| 1328: What U.S. President's head has been featured on the nickel (five-cent coin) since 1938?<br>The <b>Buffalo nickel</b> was <b>introduced</b> in 1913 as part of a drive to increase the beauty of American <b>coinage</b> ; in 1938, the <b>Jefferson nickel</b> followed.                                                                                                                                                                                                                                                                                                                                                                                                                                                                                                                                                                          | <i>Nickel (United States coin)</i>                          |
| 1329: who sings stand by me<br>"Stand by Me" is a song originally performed by Ben E. King and written by King, Jerry Leiber, and Mike Stoller, inspired by the spiritual "Lord <b>Stand</b> by Me," plus two lines rooted in Psalms 46:2–3.                                                                                                                                                                                                                                                                                                                                                                                                                                                                                                                                                                                                            | <i>Stand by Me (song)</i>                                   |
| #1331: When did F15s first fly<br>The <b>Eagle first flew</b> in July 1972, and entered service in 1976.                                                                                                                                                                                                                                                                                                                                                                                                                                                                                                                                                                                                                                                                                                                                                | <i>McDonnell Douglas F-15 Eagle</i>                         |
| 1336: what are the arb medications<br>Angiotensin receptor blocker (antagonist), a <b>medication</b> for treating high blood pressure                                                                                                                                                                                                                                                                                                                                                                                                                                                                                                                                                                                                                                                                                                                   | <i>ARB</i>                                                  |
| 1341: what are SATA Power Connector<br>Serial ATA (SATA) is a computer bus interface that <b>connects</b> host bus adapters to mass storage <b>devices</b> such as hard disk <b>drives</b> and optical drives.                                                                                                                                                                                                                                                                                                                                                                                                                                                                                                                                                                                                                                          | <i>Serial ATA</i>                                           |
| 1344: What kind of poem is "This Is Just to Say"<br>"This Is Just To Say" (1934) is a famous imagist <b>poem</b> by William Carlos Williams.                                                                                                                                                                                                                                                                                                                                                                                                                                                                                                                                                                                                                                                                                                            | <i>This Is Just To Say</i>                                  |
| 1347: who played dumbledore in harry potter<br><b>Dumbledore</b> is portrayed by Richard <b>Harris</b> in the film adaptations of <b>Harry Potter</b> and the Philosopher's Stone and <b>Harry Potter</b> and the Chamber of Secrets.                                                                                                                                                                                                                                                                                                                                                                                                                                                                                                                                                                                                                   | <i>Albus Dumbledore</i>                                     |
| 1348: what produces calcitonin<br><b>Calcitonin</b> (also known as thyrocalcitonin) is a 32-amino <b>acid</b> linear polypeptide hormone that is <b>produced</b> in humans primarily by the parafollicular cells (also known as C-cells) of the thyroid, and in many other animals in the ultimobranchial body.                                                                                                                                                                                                                                                                                                                                                                                                                                                                                                                                         | <i>Calcitonin</i>                                           |
| 1351: who hit the first home run at riverfront stadium?<br>On <b>June 30, 1970</b> , the Reds hosted the Atlanta Braves in their grand opening, with Hank Aaron <b>hitting the first ever home run</b> at <b>Riverfront</b> .                                                                                                                                                                                                                                                                                                                                                                                                                                                                                                                                                                                                                           | <i>Riverfront Stadium</i>                                   |
| 1352: Who Makes Nexen Tires<br><b>Nexen Tire</b> is a <b>tire</b> manufacturer, headquartered in Yangsan, South Gyeongsang Province, and Seoul, both in South Korea.                                                                                                                                                                                                                                                                                                                                                                                                                                                                                                                                                                                                                                                                                    | <i>Nexen Tire</i>                                           |
| 1353: who did richard nixon refer to as the silent majority<br>The term was popularized (though not first used) by U.S. President <b>Richard Nixon</b> in a November 3, 1969, speech in which he said, "And so tonight—to you, the great <b>silent majority</b> of my fellow Americans—I ask for your support."                                                                                                                                                                                                                                                                                                                                                                                                                                                                                                                                         | <i>Silent majority</i>                                      |
| 1355: What are the lateral and median apertures of the brain?<br>It is an opening in each <b>lateral</b> extremity of the <b>lateral</b> recess of the fourth ventricle of the human <b>brain</b> , which also has a single <b>median aperture</b> .                                                                                                                                                                                                                                                                                                                                                                                                                                                                                                                                                                                                    | <i>Lateral aperture</i>                                     |
| 1358: what part of the pig do pork chops come from<br><b>A pork chop</b> is a <b>chop</b> of <b>pork</b> (a meat <b>chop</b> ) cut perpendicularly to the spine of the <b>pig</b> and usually containing a rib or <b>part</b> of a vertebra, served as an individual portion.                                                                                                                                                                                                                                                                                                                                                                                                                                                                                                                                                                           | <i>Pork chop</i>                                            |
| 1362: what are grits made from<br>Modern <b>grits</b> are commonly <b>made</b> of alkali-treated corn known as hominy.                                                                                                                                                                                                                                                                                                                                                                                                                                                                                                                                                                                                                                                                                                                                  | <i>Grits</i>                                                |
| 1367: what state is new england in<br><b>New England</b> is a region in the northeastern corner of the United States consisting of the six <b>states of Maine, New Hampshire, Vermont, Massachusetts, Rhode Island, and Connecticut</b> .                                                                                                                                                                                                                                                                                                                                                                                                                                                                                                                                                                                                               | <i>New England</i>                                          |
| 1378: what are stanzas in poetry<br>A <b>stanza</b> consists of a grouping of two or more lines, set off by a space, that usually has a set pattern of meter and rhyme. The <b>stanza</b> in <b>poetry</b> is analogous with the paragraph that is seen in prose, related thoughts are grouped into units.                                                                                                                                                                                                                                                                                                                                                                                                                                                                                                                                              | <i>Stanza</i>                                               |
| 1382: who shot franz ferdinand<br>On 28 June 1914, <b>Archduke Franz Ferdinand</b> of Austria, heir presumptive to the Austro-Hungarian throne, and his wife, Sophie, Duchess of Hohenberg, were <b>shot dead</b> in Sarajevo, by Gavrilo <b>Princip</b> , one of a group of six Bosnian Serb assassins coordinated by Danilo Ilić.                                                                                                                                                                                                                                                                                                                                                                                                                                                                                                                     | <i>Assassination of Archduke Franz Ferdinand of Austria</i> |
| 1386: what are the three ossicles<br>The <b>ossicles</b> (also called auditory <b>ossicles</b> ) are the <b>three</b> smallest bones in the human body, the malleus, the incus and the stapes.                                                                                                                                                                                                                                                                                                                                                                                                                                                                                                                                                                                                                                                          | <i>Ossicles</i>                                             |
| 1391: what is an army specialist<br><b>Specialist</b> (abbreviated "SPC") is one of the four junior enlisted ranks in the U.S. <b>Army</b> , just above Private First Class and equivalent in pay grade to <b>Corporal</b> .                                                                                                                                                                                                                                                                                                                                                                                                                                                                                                                                                                                                                            | <i>Specialist (rank)</i>                                    |
| 1399: what to make with linen<br>Many products are <b>made of linen</b> : aprons, bags, towels (swimmers, bath, beach, <b>body</b> and wash towels), napkins, <b>bed linens</b> , <b>linen</b> tablecloths, runners, chair covers, and men's & women's wear.                                                                                                                                                                                                                                                                                                                                                                                                                                                                                                                                                                                            | <i>Linen</i>                                                |
| 1404: what south dakota county is wakonda in<br><b>Wakonda</b> is a town in Clay <b>County, South Dakota</b> , United States.                                                                                                                                                                                                                                                                                                                                                                                                                                                                                                                                                                                                                                                                                                                           | <i>Wakonda, South Dakota</i>                                |
| 1408: what are american people of japanese descent called<br><b>Japanese Americans</b> have historically been among the three largest Asian <b>American</b> communities, but in recent decades, it has become the sixth largest group at roughly 1,304,286, including those of mixed-race or mixed-ethnicity.                                                                                                                                                                                                                                                                                                                                                                                                                                                                                                                                           | <i>Japanese American</i>                                    |
| 1420: what is a bus adapter in a computer?<br>In <b>computer</b> hardware, a host controller, host <b>adapter</b> , or host <b>bus adapter</b> (HBA) connects a host system (the <b>computer</b> ) to other network and storage devices.                                                                                                                                                                                                                                                                                                                                                                                                                                                                                                                                                                                                                | <i>Host adapter</i>                                         |
| 1421: where does cashmere come from<br><i>Cashmere wool</i>                                                                                                                                                                                                                                                                                                                                                                                                                                                                                                                                                                                                                                                                                                                                                                                             | <i>Cashmere wool</i>                                        |

**Cashmere wool**, usually simply known as **cashmere**, is a fiber obtained from **Cashmere** goats and other types of goat .

1423: Who invented egg rolls Egg roll  
 2 Egg roll Varieties of **egg rolls** are found in mainland China , many Chinese-speaking regions of Asia, and Chinese immigrant communities around the world.

1424: what westerners include in pain and suffering Pain and suffering  
**Pain and suffering** is the legal term for the physical and emotional stress caused from an injury (see also **pain and suffering**).

1429: who won the 2010 world cup 2010 FIFA World Cup  
 In the **final**, **Spain**, the **European** champions , **defeated** third-time **finalists** the **Netherlands** 1-0 after extra **time** , with Andrés Iniesta 's **goal** in the 116th minute giving **Spain** their **first world title**, becoming the eighth nation to **win** the tournament, and the **first European** nation to **win** the tournament outside its home continent.

1431: who wrote the song in the mood In the Mood  
 "In the **Mood**" is a big band era #1 hit recorded by American bandleader Glenn Miller .

1434: what is active learning strategies Active learning  
**Active learning** is an umbrella term that refers to several models of instruction that focus the responsibility of **learning on learners**.

1442: who sang I want to dance with somebody I Wanna Dance with Somebody (Who Loves Me)  
 "I **Wanna Dance** with Somebody (Who **Loves Me**)" is the first single from Whitney Houston 's second studio album **Whitney** .

1456: who sung the banana boat song Day-O (The Banana Boat Song)  
 "Day-O (**The Banana Boat Song**)" is a traditional Jamaican mento folk **song**, the best-known version of which was **sung** by Harry Belafonte and an alternate version interspersed with another Jamaican folksong , Hill and Gully Rider, by Dame Shirley Bassey .

#1459: what year did keeping up with the Kardashians begin Keeping Up with the Kardashians  
**Keeping Up with the Kardashians** (often referred to simply as **The Kardashians**) is an American reality television series that premiered on October 14, 2007, on E! .

1464: what is a store confectioner Confectionery store  
 A **confectionery store** (more commonly referred to as a sweet shop in the United Kingdom, a candy **store** in the North America, or a lolly shop in Australia) sells **confectionery** and is usually targeted to children.

#1465: when did qing dynasty begin Qing Dynasty  
 The **Qing Dynasty**, also **Empire of the Great Qing** or **Great Qing**, was the last imperial **dynasty of China** , ruling from 1644 to 1912 with a brief, abortive restoration in 1917.

1489: who wrote serenity prayer Serenity Prayer  
 The **Serenity Prayer** is the common name for an originally untitled **prayer** by the American theologian Reinhold Niebuhr (1892-1971).

1490: what are the Declaration and Resolves of the First Continental Congress about Declaration and Resolves of the First Continental Congress  
 The **Declaration and Resolves of the First Continental Congress** (also known as the **Declaration** of Colonial Rights, or the **Declaration** of Rights), was a statement adopted by the **First Continental Congress** on October 14, 1774, in response to the **Intolerable Acts** passed by the British Parliament .

1499: who created massey ferguson Massey Ferguson  
 The company was formed by a merger between **Massey Harris** and the **Ferguson** Company farm machinery manufacturer in 1953, **creating** the company **Massey Harris Ferguson**.

1506: where do the mohawks live Mohawk people  
 Their traditional homeland stretched southward of the **Mohawk River** , eastward to the Green Mountains of Vermont , westward to the border with the Oneida **Nation** 's traditional homeland **territory**, and northward to the St Lawrence River.

#1511: when did proof die Proof (rapper)  
 In 2006, **Proof** was shot and killed during an altercation at the CCC nightclub in Detroit.  
 DeShaun Dupree Holton (October 2, 1973 – April 11, 2006), better known by his stage name **Proof**, was an American rapper and actor from Detroit, Michigan .

1524: what are social security taxes Social Security (United States)  
**Tax** deposits are formally entrusted to the **Federal Old-Age and Survivors Insurance Trust Fund**, the **Federal Disability Insurance Trust Fund**, the **Federal Hospital Insurance Trust Fund**, or the **Federal Supplementary Medical Insurance Trust Fund** which comprise the **Social Security Trust Fund** .

1527: what town is laurel hollow ny Laurel Hollow, New York  
**Laurel Hollow** is a village in the **Town** of Oyster Bay in Nassau County, New York in the United States .

1530: who won fifa world cup 2010 2010 FIFA World Cup  
 In the **final**, **Spain**, the **European** champions , **defeated** third-time **finalists** the **Netherlands** 1-0 after extra **time** , with Andrés Iniesta 's **goal** in the 116th minute giving **Spain** their **first world title**, becoming the eighth nation to **win** the tournament, and the **first European** nation to **win** the tournament outside its home continent.

#1531: when did egg McMuffin get invented McMuffin  
 The **Egg McMuffin** is the signature breakfast sandwich; it was **invented** by the late McDonald's franchisee Herb Peterson in the late 1960s and was introduced nationwide in 1972.

1544: what the names of destiny's child Destiny's Child  
 Formed in 1990 in Houston, Texas, **Destiny's Child** members began their musical endeavors as Girl's Tyne comprising, among others, Knowles, Rowland, LaTavia Roberson and LeToya Luckett.  
**Destiny's Child** was launched into mainstream recognition following the release of their best-selling second album, *The Writing's on the Wall*, which contained the number-one singles " Bills, Bills, Bills " and " Say My Name " .  
**Destiny's Child** was an American R&B girl group whose final, and perhaps most recognizable, line-up comprised Beyoncé Knowles , Kelly Rowland and Michelle Williams .  
**Destiny's Child** has sold more than 50 million records worldwide to date.  
 After years of limited success, they were signed to Columbia Records as **Destiny's Child**.

1551: What are procedure codes terms in coding? Procedure codes  
**Procedure codes** are numbers or alphanumeric **codes** used to identify specific health interventions taken by medical professionals.

1562: what is a duvet cover used for Duvet  
 A **duvet** ( or ; ; from the French **duvet** "down"), also known as a doona in Australian English or a continental **quilt** (or simply **quilt**) in British English, but this usage is no longer common, is a type of bedding , a soft flat bag filled with down , feathers , wool , silk or a synthetic alternative, and protected with a removable **cover**, analogous to a pillow and pillow case.

1563: who did mr bojangles Mr. Bojangles (song)  
 "**Mr. Bojangles**" is the title of a song originally written and recorded by American country music artist Jerry Jeff Walker for his 1968 album of the same title.

1574: what is an agents job role in film Talent agent  
 A **talent agent**, or booking **agent**, is a person who finds **jobs** for **actors** , authors , **film** directors , musicians , models , producers, professional athletes , writers and other people in various entertainment **businesses**.

1576: WHAT IS A LAW ENFORCEMENT MURDER BOOK Murder book  
 In **law enforcement** parlance, the term **murder book** refers to the case file of a **murder** investigation.

#1581: when album love always released Love Always  
**Love Always** is the debut **album** of American R&B duo K-Ci & JoJo , **released** on June 17, 1997, by MCA Records .

1583: who wrote west side story West Side Story  
**West Side Story** is an American **musical** with a book by Arthur **Laurents** , **music** by Leonard **Bernstein** , lyrics by Stephen **Sondheim** , and conception and choreography by Jerome Robbins .

1600: what states does interstate 70 travel through Interstate 70  
**Interstate 70** (I-70) is an **Interstate** Highway in the United **States** that runs from **Interstate 15** near Cove Fort, **Utah** , to a Park and Ride near **Baltimore**, Maryland .

1604: where do mangos come from Mango  
 The **mango** is native to **South** Asia , from where it has been distributed worldwide to become one of the most cultivated fruits in the tropics .

1607: what video format will play in a DVD player DVD-Video  
 Discs **using** the DVD-Video specification **require** a **DVD drive** and an H.262/MPEG-2 Part 2 **decoder** (e.g., a **DVD player**, or a computer **DVD drive** with a **software DVD** player).

1610: what part of the government governs the US post office? United States Postal Service  
 The **United States Postal Service** (USPS), also known as the **Post Office** and U.S. Mail, is an independent **agency** of the **United States federal government** responsible for **providing postal** service in the **United States**.

1614: what motor does a 2001 monte carlo Chevrolet Monte Carlo  
 The **Monte Carlo SS** was **revived** from 2000 to 2007 and initially powered by 3.8-liter **V6** (supercharged in 2004-2005), later to be replaced by a 5.3-liter **V8** for 2006-2007.

#1619: what year was President Kennedy president? John F. Kennedy

John Fitzgerald "Jack" **Kennedy** (May 29, 1917 – **November** 22, 1963), often referred to by his initials JFK, was the 35th **President** of the United States , serving from 1961 until his **death** in 1963.

1620: who owns popeyes chicken Popeyes Louisiana Kitchen  
 Often referred to as **Popeyes** and sometimes as **Popeyes Chicken & Biscuits** or **Popeyes Chicken & Seafood**, it was acquired by Sandy Springs, Georgia-based AFC Enterprises , originally America's Favorite **Chicken** Company, in 1993 .

1624: who said give me liberty or give me death Give me Liberty, or give me Death!  
 "Give me **liberty**, or give me death!" is a quotation attributed to Patrick Henry from a speech he made to the Virginia Convention .

1630: what are the most known sports in america Sports in the United States  
 Four of the nation's five most **popular** team **sports** were developed in North **America**: **American football** , baseball , **basketball** and ice hockey , whereas **soccer** was developed in England.

1639: what is aden disease Acute disseminated encephalomyelitis  
**Acute disseminated encephalomyelitis** (**ADEM**) is an immune mediated **disease** of the brain .

#1642: what year did john adams become president? John Adams  
**John Adams** (**October** 30, 1735 ( O.S. **October** 19, 1735) – July 4, 1826) was the second **president** of the **United States** (1797-1801), having earlier served as the **first vice president** of the **United States** .

1648: who created bing Bing  
**Bing** (known previously as **Live Search**, Windows **Live Search**, and MSN **Search**) is a web **search** engine (advertised as a " decision engine " ) from Microsoft .

1653: what are anti inflammatory Anti-inflammatory  
 Anti-inflammatory refers to the property of a substance or treatment that reduces **inflammation** .  
 Anti-inflammatory drugs make up about half of analgesics , remedying pain by reducing **inflammation** as opposed to opioids , which affect the central nervous system .

1656: who sang mamma told me not to come Mama Told Me Not to Come  
 "Mama **Told Me** (Not to Come)" is a song by Randy Newman written for Eric Burdon 's first solo album in 1966.

1660: what are dialysis tubes Dialysis tubing  
**Dialysis tubing** is a type of semi- or partially permeable membrane **tubing** made from regenerated cellulose or cellophane

1662: who designed the statue of liberty Statue of Liberty  
 The **Statue of Liberty** (**Liberty** Enlightening the World; French: **La Liberté** éclairant le monde) is a neoclassical **sculpture** on **Liberty Island** in New York Harbor , **designed** by Frédéric Bartholdi and dedicated on **October** 28, 1886.

1667: what is am 2201 AM-2201  
 The toxicity of **AM-2201** is still a matter of debate and there may be long term side effects.  
 Reputed recreational use of **AM-2201** in the United States has led to it being specifically listed in a proposed 2011 amendment to the Controlled Substances Act , aiming to add a number of synthetic drugs into Schedule I .  
**AM-2201** (1-(5-fluoropentyl)-3-(1-naphthyl)indole) is a research chemical that acts as a potent but nonselective full agonist for the cannabinoid receptor .

#1677: when did george washington die? George Washington  
**George Washington** ( – 1799) was the **first President** of the **United States** (1789-1797), the commander-in-chief of the **Continental Army** during the American Revolutionary War , and one of the Founding Fathers of the **United States** .

1683: what are four thirds camera Four Thirds system  
 The **Four Thirds** system is a standard created by Olympus and Kodak for digital single-lens reflex **camera** (DSLR) design and development.<ref name="DPReview.com 2001-02-13">

1691: who wrote nature boy Nature Boy  
 "**Nature Boy**" is a song by Eden Ahbez , published in 1947.  
 Nat King Cole 's 1948 recording of the song was a major hit and "**Nature Boy**" has since become a pop and jazz standard , with dozens of major artists interpreting the song.

#1698: when did playstation 3 first launch PlayStation 3 launch  
 The **launch** of the **PlayStation 3** into the **Japanese market** on 10 **November** 2006 **marked** the second major seventh generation entertainment system to be released.

1708: who wrote the song cocaine Cocaine (song)  
 "**Cocaine**" is a **song written** and recorded by JJ Cale in 1976, but also known as a cover version recorded by Eric Clapton .

#1710: when did pearl harbor get bombed Attack on Pearl Harbor  
 The attack on **Pearl Harbor** (called Hawaii Operation or Operation AI by the Japanese Imperial General Headquarters (Operation Z in planning) and the Battle of **Pearl Harbor**) was a surprise military strike conducted by the Imperial Japanese Navy against the United States naval base at **Pearl Harbor** , Hawaii, on the morning of December 7, 1941 (December 8 in Japan).

#1714: when did marlins start Miami Marlins  
 The Miami **Marlins** began play in the 1993 season as the Florida **Marlins**.  
 Per agreement with the city and Miami-Dade County (which owns the park), the **Marlins** officially changed their name to the "Miami **Marlins**" on November 11, 2011.

1716: where do dungeness crab live Dungeness crab  
 The **Dungeness crab**, *Metacarcinus magister* (formerly  *Cancer magister*), is a species of **crab** that inhabits eelgrass beds and water bottoms on the west coast of North America .

1720: who plays mary poppins in the movie Mary Poppins (film)  
**Mary Poppins** is a 1964 musical film starring Julie Andrews , Dick **Van Dyke** , David Tomlinson , and Glynis Johns , **produced** by **Walt Disney** , and based on the **Mary Poppins books** series by P. L. **Travers** .

1722: What are the different translations for the Bible Bible translations  
 The full **Bible** has been **translated** into 518 **languages**, and 2798 **languages** have at least some portion of the **Bible**.

#1723: when does black friday start for christmas Black Friday (shopping)  
**Black Friday** is the **day** following **Thanksgiving Day** in the United States , often regarded as the beginning of the **Christ**-mas shopping **season**.

#1730: when did Emperor Justinian die Justinian I  
**Justinian I** ( , ) (c. 482 – 14 November 565), commonly known as **Justinian the Great**, was Byzantine **Emperor** from 527 to 565.

1734: what movement was elizabeth cady stanton a part of Elizabeth Cady Stanton  
**Elizabeth Cady Stanton** (November 12, 1815 – October 26, 1902) was an American social activist , abolitionist, and leading figure of the early women's rights **movement** .

1738: what radio station are the boston bruins on? Boston Bruins Radio Network  
 The **Boston Bruins Radio Network** is a 25-station (17 A.M., 8 F.M. plus 2 F.M. translators) CBS **Radio network** which carries live broadcasts of the **Boston Bruins** .

#1739: when did ms drgs go into effect Diagnosis-related group  
 The system is also referred to as "the **DRGs**", and its intent was to identify the "products" that a hospital provides.  
**DRGs** may be further grouped into Major Diagnostic Categories (MDCs).  
**DRGs** have been used in the US since 1982 to determine how much Medicare pays the hospital for each "product", since patients within each category are clinically similar and are expected to use the same level of hospital resources.  
**DRGs** are assigned by a "groupor" program based on ICD (International Classification of Diseases) diagnoses, procedures, age, sex, discharge status, and the presence of complications or comorbidities .  
**DRGs** are also standard practice for establishing reimbursements for other Medicare related reimbursements such as to home healthcare providers.

1741: what are the characteristics of an ethnic group Ethnic group  
**Ethnic** identity is constantly reinforced through common **characteristics** which set the **group** apart from other **groups**.

1746: what mountains are on appalachian trail Appalachian Trail  
 The **Appalachian National Scenic Trail**, generally known as the **Appalachian Trail** or simply the A.T., is a marked hiking **trail** in the eastern United States **extending** between Springer Mountain in **Georgia** and Mount **Katahdin** in Maine .

1748: what are add ons Add-on  
**Add-ons** for Firefox (addons.mozilla.org), the official Mozilla Foundation web site which serves as a repository of **add-ons** for Mozilla-based applications  
**Add-on** (Mozilla), a piece of software that enhances and customizes Mozilla-based applications  
**Add-on** might mean:

1749: what would be the deliverables Deliverable  
 A **deliverable** also differs from a project document in that project document is typically part of a project **deliverable**, or a project **deliverable** may contain number of documents and physical things.  
 It may be either an outcome to be achieved (as in "The corporation says that becoming profitable this year is a deliverable.") or an output to be provided (as in "The **deliverable** for the completed project consists of a special-purpose electronic device and its controlling software.")  
**Deliverable** is a term used in project management to describe a tangible or intangible object produced as a result of the project that is intended to be **delivered** to a customer (either internal or external).

A **deliverable** may be composed of multiple smaller **deliverables**.

A **deliverable** differs from a project milestone in that a milestone is a measurement of progress toward an output whereas the **deliverable** is the result of the process.

In technical projects, **deliverables** can further be classified as hardware, software, or design documents.

In contracted efforts, **deliverable** may refer to an item specifically required by contract documents, such as an item on a Contract Data Requirements List or mentioned in the Statement Of Work.

For a typical project, a milestone might be the completion of a product design while the **deliverable** might be the technical diagram of the product.

A **deliverable** could be a report, a document, a server upgrade or any other building block of an overall project.

1754: what school did oprah winfrey help *Oprah Winfrey Leadership Academy for Girls*  
The **Oprah Winfrey Leadership Academy for Girls** - South Africa is a female boarding **school** founded in January 2007 and located in Henley on Klip near Meyerton, south of Johannesburg, South Africa.

#1757: when did scott pilgrim come out *Scott Pilgrim vs. the World*  
**Scott Pilgrim vs. the World** is a 2010 American **comedy** film directed by Edgar Wright, based on the graphic novel series **Scott Pilgrim** by Bryan Lee O'Malley.

1760: what is a google in math *Googol*  
In the binary numeral system, one would need 333 bits to represent a **googol**, i.e., 1 **googol** ≈ 2332.19, or exactly.

Other names for **googol** include ten duotrigintillion on the short scale, ten thousand sexdecillion on the long scale, or ten sexdecillion on the Peletier long scale.

It is also the namesake of the internet company Google, with the name "Google" being a misspelling of "googol" by the company's founders.

A **googol** is the large number 10100; that is, the digit 1 followed by 100 zeroes:

A **googol** is approximately 70!

A **googol** has no particular significance in mathematics, but is useful when comparing with other very large quantities such as the number of subatomic particles in the visible universe or the number of hypothetically possible chess games.

1 **Googol** (1E100) is a small fraction more, than the biggest number a usual hand-held calculator can display and handle, which is 9.999...

1763: what structure is disulfide bonds *Disulfide bond*  
In chemistry, a **disulfide bond** (Br.E. disulphide **bond**) is a covalent **bond**, usually derived by the coupling of two thiol groups.

1768: who rules communism government *Communist state*  
It has a form of **government** characterized by single-party **rule** or dominant-party **rule** of a communist party (referred as Dictatorship of the Proletariat by its proponents) and a professed allegiance to a Leninist or Marxist-Leninist ideology as the guiding principle of the state.

1772: who makes skittles? *Skittles (confectionery)*  
**Skittles** is a brand of fruit-flavoured sweets, currently produced and marketed by the Wm. Wrigley Jr. Company, a division of Mars, Inc.

1778: what is a discipline of study *List of academic disciplines*  
An academic **discipline**, or field of **study**, is a branch of knowledge that is taught and researched at the college or university level.

1783: who wrote stand by me *Stand by Me (song)*  
"**Stand by Me**" is a song originally performed by Ben E. King and **written** by King, Jerry Leiber, and Mike Stoller, inspired by the spiritual "Lord **Stand** by Me," thus two lines rooted in Psalms 46:2–3.

1784: what are metaphors used for *Metaphor*  
This quote is a **metaphor** because the world is not literally a stage.

One of the most prominent examples of a **metaphor** in English literature is the All the world's a stage monologue from As You Like It:

**Metaphor** is a type of analogy and is closely related to other rhetorical figures of speech that achieve their effects via association, comparison or resemblance including allegory, hyperbole, and simile.

In simpler terms, a **metaphor** compares two objects or things without using the words "like" or "as".

A **metaphor** is a figure of speech that describes a subject by asserting that it is, on some point of comparison, the same as another otherwise unrelated object.

1788: what are the names of the ll divos *Il Divo*  
Il **Divo** is an English multinational operatic pop vocal group created by music manager, executive, and reality TV star Simon Cowell.

Il **Divo** is a group of four male singers: French pop singer Sébastien Izambard, Spanish baritone Carlos Marin, American tenor David Miller, and Swiss tenor Urs Bühler.

1792: What is a 28 day cycle? *Menstrual cycle*  
This article focuses on the human menstrual **cycle**, a "monthly" **cycle** that can vary around an average of ~28 days per cycle.

1797: what is a llc company? *Limited liability company*  
An **LLC** is a legal form of **company** that provides limited liability to its owners in the vast majority of **United States jurisdictions**.

1798: what are k cups *K-Cup*  
K-Cup portion packs are used with Keurig or other single **cup brewing systems** to **brew a cup** of coffee, tea, or hot chocolate.

1800: what is a chronograph watch *Chronograph*  
A **chronograph** is a specific type of **watch** that is used as a stopwatch combined with a display **watch**.

1801: what is a PCI port used for *Conventional PCI*  
**Conventional PCI (PCI)** is an initialism formed from Peripheral Component Interconnect, part of the **PCI Local Bus standard** and often shortened to just **PCI** is a local **computer bus** for attaching hardware devices in a **computer**.

#1813: when did the movie deep blue sea come out *Deep Blue Sea*  
**Deep Blue Sea** is a 1999 science fiction horror film that stars Saffron Burrows, Thomas Jane, LL Cool J, Michael Rapaport, Stellan Skarsgård and Samuel L. Jackson.

1818: what are a and r reps *Artists and repertoire*  
**Artists and repertoire** (A&R) is the division of a record label or music publishing company that is responsible for talent scouting and overseeing the **artistic** development of recording **artists** and/or songwriters.

1819: what measurement is a furlong *Furlong*  
A **furlong** is a **measure** of distance in imperial units and U.S. customary units equal to one-eighth of a mile, equivalent to 220 yards, 660 feet, 40 rods, or 10 chains.

#1825: when the wind blows james patterson *When the Wind Blows (James Patterson novel)*  
When the **Wind Blows** is a novel by **James Patterson**.

1829: what are the catholic gifts of the holy spirit *Seven gifts of the Holy Spirit*  
The **seven gifts of the Holy Spirit** is an enumeration of **seven spiritual gifts** originating with patristic authors, later elaborated by five intellectual **virtues** and four other groups of ethical characteristics.

1832: what are lobbying groups *Lobbying*  
**Lobbying** is done by many different types of people and organized **groups**, including individuals in the private sector, corporations, fellow legislators or government officials, or advocacy **groups** (interest groups).

1840: what nationality is kris jenner *Kris Jenner*  
Kristen Mary "**Kris Jenner**" (née Houghton, previously Kardashian; born November 5, 1955) is an American socialite, author and television personality.

#1850: when did lucy stone died *Lucy Stone*  
**Lucy Stone** (August 13, 1818 – October 19, 1893) was a prominent American abolitionist and suffragist, and a vocal advocate and organizer promoting rights for women.

1851: what are stocks and bonds *Bond (finance)*  
**Bonds** and **stocks** are both securities, but the major **difference** between the two is that (capital) stockholders have an equity stake in the **company** (i.e. they are owners), whereas **bondholders** have a creditor stake in the **company** (i.e. they are lenders).

1852: what are the boundaries of the pelvic outlet *Pelvic outlet*  
The lower circumference of the lesser pelvis is very irregular; the space enclosed by it is named the inferior aperture or **pelvic outlet**.

#1858: when did germans enter paris in ww2 *Liberation of Paris*  
The Liberation of **Paris** (also known as the Battle for **Paris**) took place during World War II from 19 **August** 1944 until the surrender of the occupying **German** garrison on **25 August**.

1859: who wrote the song feelin alright *Feelin' Alright*  
"**Feelin' Alright**?" also known as "**Feelin' Alright**" is a **song written** by Dave Mason of the English rock band Traffic from their eponymous 1968 album, Traffic.

1860: what is a neuro tract *Neural pathway*

A neural **pathway**, **neural tract**, or neural face, connects one part of the nervous system with another and usually consists of bundles of elongated, myelin-insulated neurons, known collectively as white matter.

#1863: when did dr.carter g woodson die *Carter G. Woodson*  
**Carter Godwin Woodson** (December 19, 1875April 3, 1950) was an African-American historian, author, journalist and the founder of the Association for the Study of African American Life and History.

1864: what are loan originations *Loan origination*  
**Loan origination** is the **process** by which a borrower **applies** for a new **loan**, and a lender **processes** that **application**.

#1872: what year did aeromsmith i dont want to miss a thing *I Don't Want to Miss a Thing*  
"I Don't **Want to Miss a Thing**" is a song performed by American rock **band Aerosmith** for the 1998 film Armageddon.

1886: who makes triumph motorcycles *Triumph Motorcycles*  
**Triumph Motorcycles** Ltd., a current British **motorcycle** manufacturer

1894: what produces primary xylem? *Xylem*  
The word **xylem** is derived from the Greek word ξύλον (xylon), meaning "wood"; the best-known **xylem** tissue is **wood**, though it is **found** throughout the plant.

1897: what is a ti 82? *TI-82*  
The **TI-82** was designed in 1993 as a stripped down, more user friendly version of the TI-85, and as a replacement for the TI-81.

The **TI-82** is a graphing calculator made by Texas Instruments.

Like the TI-81, the **TI-82** features a 96x64 pixel display, and the core feature set of the TI-81 with many new features.

1899: what makes of the united states *United States*  
The **United States** of America (USA or U.S.A.), commonly called the **United States** (US or U.S.) or America, is a **federal** republic consisting of fifty **states** and a **federal district**.

#1919: when did thomas jefferson become president *Thomas Jefferson*  
**Thomas Jefferson** (April 13, 1743 (April 2, 1743 O.S.) – July 4, 1826) was an **American** Founding **Father**, the principal author of the Declaration of Independence (1776) and the third **President** of the United States (1801–1809).

1920: who sang sun city *Sun City (song)*  
"**Sun City**" is a 1985 protest song written by Steven Van Zandt, produced by Van Zandt and Arthur Baker and recorded by Artists United Against **Apartheid** to convey opposition to the South African policy of **apartheid**.

1931: who wrote the song hallelujah *Hallelujah (Leonard Cohen song)*  
"**Hallelujah**" is a **song written** by **Canadian** singer-songwriter Leonard **Cohen**, originally released on his album Various Positions (1984).

1932: what are garnishments *Garnishment*  
A **garnishment** is a means of collecting a **monetary** judgment against a defendant by ordering a third party (the **garnishee**) to pay **money**, otherwise owed to the defendant, directly to the plaintiff.

1944: what are land parcels *Parcel*  
**land** lot, a piece of **land**;

1945: what state is mn *Minnesota*  
Minnesota () is a U.S. **state** located in the Midwestern United **States**.

1947: what naturally occurring isotopes does cobalt have *Isotopes of cobalt*  
**Naturally occurring cobalt** (Co) is composed of 1 stable **isotope**, <sup>59</sup>Co. 28 radioisotopes have been characterized with the most stable being <sup>60</sup>Co with a half-life of 5.2714 years, <sup>57</sup>Co with a half-life of 271.79 days, <sup>56</sup>Co with a half-life of 77.27 days, and <sup>58</sup>Co with a half-life of 70.86 days.

1948: Who Moved My Cheese Synopsis *Who Moved My Cheese?*  
It describes **change** in one's work and life, and four typical reactions to said **change** by two mice and two "littlepeople", during their hunt for **cheese**.

1949: who replaced nikita khrushchev *Nikita Khrushchev*  
**Khrushchev's party colleagues** removed him from power in 1964, **replacing** him with **Leonid Brezhnev** as First Secretary and Alexei Kosygin as Premier.

1953: What Are Mnemonic Devices *Mnemonic*  
A **mnemonic** (, with a silent "m"), or **mnemonic device**, is any **learning** technique that aids **information** retention.

1962: What is a surveyor's wheel *Surveyor's wheel*  
A **surveyor's wheel**, also called a clickwheel, hodometer, waywiser, trundle **wheel**, measuring **wheel**, or perambulator is a device for measuring distance.

#1967: what year was girls just want to have fun release *Girls Just Want to Have Fun*  
"**Girls Just Want to Have Fun**" is a 1979 song originally written by Robert Hazard and made famous by singer Cyndi Lauper.

1972: what are the players in Quidditch? *Quidditch*  
Matches are **played** between two teams of seven **players** riding flying broomsticks, using four balls and six elevated ring-shaped goals, three on each side of the **Quidditch** pitch (field).

1975: who wrote the song a little more country than that? *A Little More Country Than That*  
"A **Little More Country Than That**" is the title of a **song written** by Joey + Rory 's Rory Lee Feek, Wynn Varble, and Don Poythress, and recorded by American **country** artist Easton Corbin.

1976: who makes blackberry *BlackBerry*  
The **BlackBerry** is a line of wireless handheld devices and services designed and marketed by Research In Motion **Limited** (RIM) operating as **BlackBerry**.

1979: what are arizona's symbols *List of Arizona state symbols*  
The newest adopted **symbol of Arizona** is the Colt Single Action Army in 2011.

The following is a list of **symbols** of the U.S. state of **Arizona**.

The first **symbol** was the motto, which was made official in 1864 for the **Arizona** Territory.

Fifteen of the state **symbols** are on display on the **Arizona** Capitol Museum.

1983: what is adoration catholic church *Eucharistic adoration*  
Eucharistic **adoration** is a practice in the Roman **Catholic Church**, and in a few Anglican and Lutheran **churches**, in which the Blessed Sacrament is exposed and **adored** by the faithful.

#1984: when the body is systemic *Systemic*  
**Systemic** refers to something that is spread throughout, **system-wide**, affecting a group or **system** such as a **body**, economy, market or society as a whole.

1985: what are SLR cameras *Single-lens reflex camera*  
A single-lens reflex (**SLR**) **camera** is a **camera** that typically uses a mirror and prism system (hence "reflex", from the mirror's reflection) that permits the photographer to view through the lens and see exactly what will be captured, contrary to viewfinder **cameras** where the image could be significantly different from what will be captured.

1986: what is a vm server *Virtual machine*  
A virtual machine (**VM**) is a software implemented **abstraction** of the underlying hardware, which is presented to the application layer of the **system**.

#1998: when did the titanic sink *RMS Titanic*  
RMS **Titanic** was a British passenger liner that **sank** in the North Atlantic Ocean on 15 April 1912 after colliding with an **iceberg** during her **maiden voyage** from **Southampton**, UK to **New York City**, US.

1999: where is the human thigh located? *Human leg*  
The **human leg** is the entire **lower extremity** or **limb** of the **human** body, including the foot, **thigh** and even the hip or gluteal region; however, the precise definition in **human** anatomy refers only to the section of the **lower limb** extending from the **knee** to the **ankle**.

2001: what is considered a large car *Full-size car*  
A full-size **car** is a marketing term used in North America for an automobile **larger** than a mid-size **car**.

2004: who is flo from progressive *Flo (Progressive Insurance)*  
In 2011, **Progressive** introduced an Australian counterpart to **Flo**, named Kitty, played by Australian actress Holly Austin.

**Flo** is a fictional character who appears in commercials for **Progressive Insurance**.

2009: what is petit lemans *Petit Le Mans*  
The **Petit Le Mans** (French for little Le Mans) is a sports car endurance race held annually at Road Atlanta in Braselton, Georgia, USA.

The **Petit Le Mans** covers a maximum of (which is approximately 394 laps) or a maximum of 10 hours, whichever comes first; only once, in the rain-stopped 2009 race, has the leading team failed to complete.

2015: what is considered to be a disaster *Disaster*  
Developing countries suffer the greatest costs when a **disaster** hits – more than 95 percent of all deaths caused by **disasters** occur in developing countries, and losses due to natural **disasters** are 20 times greater (as a percentage of GDP) in developing countries than in industrialized countries.

Ruins from the 1906 San Francisco earthquake, remembered as one of the worst natural **disasters** in United States history in contemporary academia, **disasters** are seen as the consequence of inappropriately managed risk.

Hazards that strike in areas with low vulnerability will never become **disasters**, as is the case in uninhabited regions.

A **disaster** is a natural or man-made (or technological) hazard resulting in an event of substantial extent causing significant physical damage or destruction, loss of life, or drastic change to the environment.

A **disaster** can be extensively defined as any tragic event stemming from events such as earthquakes, floods, catastrophic accidents, fires, or explosions.

2017: What is firebird server *Firebird (database server)*  
The database forked from Borland's open source edition of InterBase in 2000, but since **Firebird 1.5** the code has been largely rewritten.

**Firebird** is an open source SQL relational database management system that runs on Linux, Windows, and a variety of Unix.

2019: What is caused by the human immunodeficiency virus? *HIV*  
**Human immunodeficiency virus** (HIV) is a lentivirus (slowly replicating retrovirus) that **causes** acquired **immunodeficiency** syndrome (AIDS), a condition in **humans** in which progressive failure of the immune system **allows** life-threatening opportunistic infections and cancers to thrive.

2026: what is the function of the vas deferens? *Vas deferens*  
The **vas deferens** (plural: vasa deferentia), also called ductus **deferens** (Latin: "carrying-away vessel"; plural: ductus deferentes), is part of the male anatomy of many vertebrates; they transport sperm from the epididymis in anticipation of ejaculation.

2027: What is Ischemia or infarction? *Ischemia*  
Vascular **ischemia** of the toes with characteristic cyanosis.  
**Ischemia** is generally caused by problems with blood vessels, with resultant damage to or dysfunction of tissue. In medicine, **ischemia**, also spelled as ischaemia or ischæmia, (; from Greek language ισχαιμία, ischaimia; isch- root denoting a restriction or thinning or to make or grow thin/lean, haema blood) is a restriction in blood supply to tissues, causing a shortage of oxygen and glucose needed for cellular metabolism (to keep tissue alive).

2035: where is humboldt ks *Humboldt, Kansas*  
**Humboldt** is a city situated along the Neosho River in the southwest part of Allen County, located in southeast Kansas, in the Central United States.

2036: what was nixon accused of *Watergate scandal*  
The Watergate **scandal** was a political **scandal** that occurred in the United States in the 1970s as a result of the June 17, 1972 break-in at the Democratic National Committee headquarters at the Watergate office complex in Washington, D.C., and the **Nixon administration's** attempted cover-up of its involvement.

2043: who is victoria jackson from saturday night live *Victoria Jackson*  
**Victoria Jackson** (born August 2, 1959) is an American comedian, actress, satirist, singer and internet blogger best known as a cast member of the NBC television sketch comedy series **Saturday Night Live** (SNL) from 1986 to 1992.

2044: what was the post modernist era in literature? *Postmodern literature*  
Postmodern **literature** is **literature** characterized by heavy reliance on techniques like **fragmentation**, paradox, and questionable narrators, and is often (though not exclusively) defined as a style or **trend** which emerged in the post–World War II era.

2045: who is the group enigma *Enigma (musical project)*  
The Romanian-born Cretu conceived the **Enigma** project while working in Germany, but based his recording studio A.R.T. Studios in Ibiza, Spain, from the early 1990s until May 2009, where he has recorded all of **Enigma's** studio releases to date.

2049: what is the federal death tax *Estate tax in the United States*  
The estate **tax** in the United States is a **tax** imposed on the **transfer** of the "taxable estate" of a deceased **person**, whether such **property** is **transferred** via a will, according to the **state** laws of intestacy or otherwise made as an incident of the **death** of the owner, such as a **transfer** of **property** from an intestate estate or trust, or the payment of **certain** life insurance benefits or financial account sums to beneficiaries.

#2052: when was raphael born *Raphael*  
Raffaello Sanzio da **Urbino** (April 6 or March 28, 1483 – April 6, 1520), better known simply as **Raphael**, was an Italian painter and architect of the High Renaissance.

2059: where is the seed located in an artichoke *Artichoke*  
The edible matter is **buds** that form within the **flower** heads before the **flowers** come into bloom.

2065: WHAT IS PARESTHESIAS OF HANDS *Paresthesia*  
The manifestation of **paresthesia** may be transient or chronic.  
**Paresthesia** ( ), is a sensation of tickling, tingling, burning, pricking, or numbness of a person's skin with no apparent long-term physical effect.

2072: who is paul avery to the zodiac killings *Paul Avery*  
**Paul Avery** (April 2, 1934December 10, 2000) was an American police reporter, best known for his stories on the infamous serial **killer** known as the **Zodiac**, and later for his work on the Patricia Hearst kidnapping.

2074: what is sump pump used for *Sump pump*  
A **sump pump** is a **pump** used to remove water that has accumulated in a water collecting **sump** basin, commonly found in the basement of homes.

#2075: when was bloody kansas in *Bleeding Kansas*  
Bleeding **Kansas**, **Bloody Kansas** or the Border War, was a series of violent political confrontations involving anti-slavery Free-Staters and pro-slavery "Border Ruffian" elements, that took place in the **Kansas** Territory and the neighboring towns of Missouri between 1854 and 1861.

2076: What Is Benzene Used For *Benzene*  
It is mainly **used** as a precursor to heavy **chemicals**, such as **ethylbenzene** and cumene, which are **produced** on a billion kilogram scale.

2079: what is homebrew for wii? *Wii homebrew*  
**Wii homebrew** refers to the reuse of Nintendo's **Wii** game console to run software that has not been authorized by Nintendo.

In more general terms, **Wii Homebrew** refers to the use of the **Wii**'s hardware, accessories and software for purposes outside those intended by the manufacturer.

2081: who was bush's national security advisor *Stephen Hadley*  
**Stephen John Hadley** (born February 13, 1947) was the 21st U.S. Assistant to the President for **National Security** Affairs (commonly referred as **National Security Advisor**), serving under President George W. **Bush**.

2088: what is another name for the large intestine *Large intestine*  
The **large intestine** (or bowel, colon) is the last part of the digestive system in vertebrate animals.  
The **large intestine** is about long, which is about one-fifth of the whole length of the intestinal canal.  
The **large intestine** consists of the cecum, rectum and anal canal.  
In Terminologia Anatomica the **large intestine** includes the cecum, colon, rectum, and anal canal.

2090: where is the valley at in los angeles *San Fernando Valley*  
The San Fernando **Valley** (locally known as "The Valley") is an urbanized **valley** located in the **Los Angeles** metropolitan area of southern California, United States, defined by the mountains of the Transverse Ranges circling it.

#2094: when is susan smith eligible for parole *Susan Smith*  
According to the South Carolina Department of Corrections, **Smith** will be **eligible** for **parole** on November 4, 2024, after serving a minimum of thirty years.

#2098: when was everybody hates chris made *Everybody Hates Chris*  
Everybody **Hates Chris** is an American television period sitcom that depicts the teenage experiences of comedian **Chris Rock** (who is also the narrator) while growing up in the Bedford-Stuyvesant neighborhood of Brooklyn, New York.

2099: what is lung effusion *Pleural effusion*  
Pleural **effusion** is excess fluid that accumulates between the two pleural layers, the fluid-filled **space** that surrounds the **lungs**.

2104: who is shem in the bible *Shem*  
**Shem** (; Sēm; Arabic: Sām, Ge'ez: ሩባ, Sēm; "renown; prosperity; name") was one of the sons of Noah in the Hebrew **Bible** as well as in Islamic literature.  
However, the New American Standard **Bible** gives, "Also to **Shem**, the father of all the children of Eber, and the older brother of Japheth, children were born."

2105: what is go daddy.com? *Go Daddy*  
**Go Daddy** or **Go Daddy Group Inc.** is a privately held **company** that is primarily an internet domain **registrar** and web hosting **company**.

2106: where is andy whitfield from? *Andy Whitfield*  
**Andy Whitfield** (died 11 September 2011) was a Welsh Australian actor and model.

2107: where is the country andorra located *Andorra*  
**Andorra** (; ), officially the Principality of **Andorra** (), also called the Principality of the Valleys of **Andorra** (), is a landlocked microstate in Southwestern Europe, **located** in the eastern Pyrenees mountains and bordered by **Spain** and France.

2110: what is the highest point in oahu *Oahu*  
The **highest point** is Mt. Ka'ala in the Waianae Range, rising to above sea level.

2113: what is spelt flour *Spelt*

**Spelt** was an important staple in parts of Europe from the Bronze Age to medieval times; it now survives as a relict crop in Central Europe and northern Spain and has found a new market as a health food.

**Spelt** is sometimes considered a subspecies of the closely related species common wheat (*T. aestivum*), in which case its botanical name is considered to be *Triticum aestivum* subsp. *spelta*.

**Spelt**, also known as dinkel wheat, or hulled wheat, is an ancient species of wheat from the fifth millennium BC.

2118: where is kennywood in pittsburgh *Kennywood*  
**Kennywood** is an amusement park located in West Mifflin, **Pennsylvania**, a suburb of **Pittsburgh**.

2125: Who is the rap singer in right round with kesha in the background? \*(dancer)\* *Right Round*  
"**Right Round**" is a song performed by **American rapper** Flo Rida, **released** as the lead **single** from his second studio album, R.O.O.T.S. (2009).

2128: what is rock of ages about *Rock of Ages (musical)*  
**Rock of Ages** is a **rock** / jukebox **musical**, with a book by Chris D'Arienzo, built around classic **rock** hits from the 1980s, especially from the famous glam metal bands of the decade.

2134: what is the singer Stevie Wonders full name *Stevie wonder*  
**Stevland Hardaway Morris** (born May 13, 1950 as **Stevland Hardaway** Judkins), **known** by his stage **name** **Stevie Wonder**, is an American **singer**, songwriter, and multi-instrumentalist, a child prodigy who developed into one of the most creative **musical** figures of the late 20th century.

2140: what is general chu chicken *General Tso's chicken*  
**General Tso's chicken** (sometimes Governor **Tso's chicken**, **General** Gau's **chicken**, **General** Tao's **chicken**, **General** Tsao's **chicken**, **General** Tong's **chicken**, **General** Tang's **chicken** or simply **General's Chicken**) is a sweet, slightly spicy, deep-fried **chicken** dish that is popularly served in North American Chinese restaurants.

2142: where is david ortiz from *David Ortiz*  
**David Americo Ortiz** Arias (born November 18, 1975, nicknamed "Big Papi") is a Dominican-American professional baseball designated hitter with the Boston Red Sox of Major League Baseball (MLB).

2143: what is an irregular heartbeat pvc *Premature ventricular contraction*  
A premature ventricular contraction (PVC), also known as a premature ventricular **complex**, ventricular premature contraction (or **complex** or **complexes**) (VPC), ventricular premature beat (VPB), or ventricular extrasystole (VES), is a relatively common event where the **heartbeat** is initiated by Purkinje fibres in the ventricles rather than by the sinoatrial node, the normal **heartbeat** initiator.

2150: what is flour made from *Flour*  
**Flour** is a powder which is **made** by grinding cereal grains, or other seeds or roots (like **Cassava**).

2156: what is cubic ft *Cubic foot*  
To calculate **cubic** feet multiply length X width X height.  
The term **cubic** foot is an Imperial and US customary (non-metric) unit of volume, used in the United States and the United Kingdom.  
It is defined as the volume of a **cube** with sides of one foot (0.3048 m) in length.

#2157: when was kirstie alley on cheers *Kirstie Alley*  
**Kirstie Louise Alley** (born January 12, 1951) is an American actress and comedian known for her role in the TV series **Cheers**, in which she played Rebecca Howe from 1987–1993, winning an Emmy Award and a Golden Globe Award as the Outstanding Lead Actress in a Comedy Series in 1991.

2161: what is another name for cpu *Central processing unit*  
A central processing unit (CPU), also referred to as a central processor unit, is the **hardware** within a computer that carries out the instructions of a computer program by performing the basic arithmetical, logical, and input/output operations of the system.

2169: what was the city of Mithridates *Mithridates VI of Pontus*  
**Mithridates VI** or Mithradates VI ( ), from Old Persian Mithradatha, "gift of Mithra"; 134–63 BC, also known as Mithradates the Great (Megas) and Eupator Dionysius, was king of Pontus and Armenia Minor in northern Anatolia (now Turkey) from about 120–63 BC.

**Mithridates** is remembered as one of the Roman Republic's most formidable and successful enemies, who engaged three of the prominent generals from the late Roman Republic in the Mithridatic Wars: Lucius Cornelius Sulla, Lucullus and Pompey.

2174: what is extreme right wing *Far-right politics*  
The **far right** is commonly associated with persons or groups who hold **extreme** nationalist, xenophobic, racist, religious fundamentalist or reactionary views.  
The far-right (also known as the **extreme right**) refers to the highest degree of rightism in right-wing politics.

2177: what is high emotional intelligence? *Emotional intelligence*  
**Emotional intelligence** (EI) is the ability to identify, assess, and control the **emotions** of oneself, of others, and of groups.

2178: what is the role of heredity *Heredity*  
**Heredity** is the passing of **traits** to offspring from its parents or ancestor.

#2186: what is prefix phone number *Telephone prefix*  
A telephone **prefix** is the first set of digits of a telephone **number**; in the North American Numbering Plan countries (country code 1), it is the first three digits of a seven-digit **phone number**.

2187: what is metformin used for *Metformin*  
**Metformin** ( **BM**, pronounced , ; originally sold as **Glucophage**) is an **oral** antidiabetic drug in the biguanide class.

2190: what is it like at mount rushmore? *Mount Rushmore*  
The **Mount Rushmore** National Memorial is a sculpture carved into the granite face of **Mount Rushmore** near Keystone, South Dakota, in the United States.

2195: where is keith whitely from *Keith Whitley*  
Jackie **Keith Whitley** (July 1, 1954Stambler, Irwin, and Grelun Landon (2000). - Country Music: The Encyclopedia. - New York: St. Martin's Press. - p.533. - ISBN 978-0-312-26487-1.—Carlin, Richard (2003). - Country Music: A Biographical Dictionary. - New York: Routledge - p.427. - ISBN 978-0-415-93802-0.—Larkin, Colin (1995). - The Guinness Encyclopedia of Popular Music. - New York: Stockton Press - P.462. - ISBN 978-0-85112-662-3.—Stanton, Scott (2003). - The Tombstone Tourist: Musicians. - New York: Pocket Books. - p.395. - ISBN 978-0-7434-6330-0.—Hicks, Jack. - "Singer **Keith Whitley's** Memory Alive Through Songs, Love in Home Town". - The Kentucky Post. - September 25, 1991.—"Country Music Star **Keith Whitley** Dead at 33". - Lexington Herald-Leader. - May 10, 1989.—Hurst, Jack. - "Whitley's Last Days". - Chicago Tribune. - May 14, 1989.—"Alcohol Kills Country Singer **Keith Whitley**". - United Press International. - (c/o The San Francisco Chronicle). - May 10, 1989. — May 9, 1989), known professionally as **Keith Whitley**, was an American country music singer.

2200: who is basketball star antoine walker *Antoine Walker*  
**Antoine Devon Walker** (born August 12, 1976) is an American former professional **basketball** player.

2202: where are the internal and external iliac arteries *External iliac artery*  
The **external iliac arteries** are two major **arteries** which bifurcate off the common **iliac arteries** anterior to the sacroiliac joint of the pelvis.

2207: where is the Rhine river located on a map *Rhine*  
The **Rhine** (; ) is a European **river** that runs from the Swiss canton of Grisons in the southeastern Swiss Alps through **Germany** and eventually flows into the North Sea coast in the **Netherlands** and is the twelfth longest **river** in Europe, at about, with an average discharge of more than.

2208: what is sanskrit shri *Sri*  
Sri (Devanagari: श्री, IAST: Śrī; Śrī), also transliterated as Sree or **Shri** or Shree is a word of **Sanskrit** origin, used in the Indian subcontinent as polite form of address equivalent to the English "Mr." in written and spoken language, or as a title of veneration for deities (usually translated as "Holy").

2214: Where is a famous alluvial plain *Mississippi Alluvial Plain*  
The Mississippi River **Alluvial Plain** is an **alluvial plain** created by the Mississippi River on which lies parts of seven U.S. states, from southern Louisiana to southern Illinois.

2215: Where is South Beach in Miami *South Beach*  
**South Beach**, also nicknamed **SoBe**, is a neighborhood in the city of **Miami Beach**, Florida, United States, located due east of **Miami** city proper between Biscayne Bay and the Atlantic Ocean.

2233: what is bones job *Bones (TV series)*  
The show is based on forensic anthropology and forensic archaeology, with each **episode** focusing on an FBI case file concerning the mystery behind human remains brought by FBI Special Agent Seeley Booth ( David **Boreanaz**) to the forensic anthropologist Dr. Temperance "**Bones**" Brennan ( **Emily Deschanel** ).

#2235: when was malcolm x assassinated *Malcolm X*  
**Malcolm X** (; May 19, 1925February 21, 1965), born **Malcolm Little** and also **known** as El-Hajj Malik El-Shabazz ( ), was an African-American Muslim minister and human rights activist.

2239: where is penn state stadium *Beaver Stadium*  
**Beaver Stadium** is an outdoor college football **stadium** in University Park, Pennsylvania, United States, on the campus of The Pennsylvania **State University**.

2240: what is in a tequila sunrise? *Tequila Sunrise (cocktail)*  
The **Tequila Sunrise** is a cocktail made in two different ways, the original (**tequila**, crème de cassis, lime juice and soda water) and the more popular concoction (**tequila**, orange juice, and grenadine syrup).

|                                                                                                                                                                                                                                                                                                                                                                                                                                                                                                                                                                                                                                                                                                                                                                                                                                                                                                                                                                                                                                                                                                                                                                                                                                                                                                                                                       |                                                       |
|-------------------------------------------------------------------------------------------------------------------------------------------------------------------------------------------------------------------------------------------------------------------------------------------------------------------------------------------------------------------------------------------------------------------------------------------------------------------------------------------------------------------------------------------------------------------------------------------------------------------------------------------------------------------------------------------------------------------------------------------------------------------------------------------------------------------------------------------------------------------------------------------------------------------------------------------------------------------------------------------------------------------------------------------------------------------------------------------------------------------------------------------------------------------------------------------------------------------------------------------------------------------------------------------------------------------------------------------------------|-------------------------------------------------------|
| 2244: where are facial sinuses                                                                                                                                                                                                                                                                                                                                                                                                                                                                                                                                                                                                                                                                                                                                                                                                                                                                                                                                                                                                                                                                                                                                                                                                                                                                                                                        | <i>Paranasal sinuses</i>                              |
| Paranasal <b>sinuses</b> are a group of four paired air-filled spaces that surround the nasal cavity ( maxillary <b>sinuses</b> ), above the eyes ( frontal <b>sinuses</b> ), between the eyes ( ethmoid <b>sinuses</b> ), and behind the ethmoids ( sphenoid <b>sinuses</b> ).                                                                                                                                                                                                                                                                                                                                                                                                                                                                                                                                                                                                                                                                                                                                                                                                                                                                                                                                                                                                                                                                       |                                                       |
| 2246: what is lean manufacturing and who developed                                                                                                                                                                                                                                                                                                                                                                                                                                                                                                                                                                                                                                                                                                                                                                                                                                                                                                                                                                                                                                                                                                                                                                                                                                                                                                    | <i>Lean manufacturing</i>                             |
| <b>Lean manufacturing</b> , <b>lean enterprise</b> , or <b>lean production</b> , often simply, "Lean," is a production practice that considers the expenditure of resources for any goal other than the creation of value for the end customer to be wasteful, and thus a target for elimination.                                                                                                                                                                                                                                                                                                                                                                                                                                                                                                                                                                                                                                                                                                                                                                                                                                                                                                                                                                                                                                                     |                                                       |
| 2253: what is the capital city of California.                                                                                                                                                                                                                                                                                                                                                                                                                                                                                                                                                                                                                                                                                                                                                                                                                                                                                                                                                                                                                                                                                                                                                                                                                                                                                                         | <i>Sacramento, California</i>                         |
| Sacramento is the <b>capital city</b> of the U.S. state of <b>California</b> and the seat of <b>government</b> of Sacramento <b>County</b> .                                                                                                                                                                                                                                                                                                                                                                                                                                                                                                                                                                                                                                                                                                                                                                                                                                                                                                                                                                                                                                                                                                                                                                                                          |                                                       |
| 2255: What was "Freedom Summer"?                                                                                                                                                                                                                                                                                                                                                                                                                                                                                                                                                                                                                                                                                                                                                                                                                                                                                                                                                                                                                                                                                                                                                                                                                                                                                                                      | <i>Freedom Summer</i>                                 |
| <b>Freedom Summer</b> (also known as the Mississippi <b>Summer Project</b> ) was a campaign in the United States launched in June 1964 to attempt to register as many African American voters as possible in Mississippi , which had historically excluded most blacks from voting.                                                                                                                                                                                                                                                                                                                                                                                                                                                                                                                                                                                                                                                                                                                                                                                                                                                                                                                                                                                                                                                                   |                                                       |
| 2264: what was the Name the first electronic handheld calculator                                                                                                                                                                                                                                                                                                                                                                                                                                                                                                                                                                                                                                                                                                                                                                                                                                                                                                                                                                                                                                                                                                                                                                                                                                                                                      | <i>Sumlock ANITA calculator</i>                       |
| The ANITA Mark VII and ANITA Mark VIII <b>calculators</b> were launched simultaneously in late 1961 as the world's <b>first all-electronic desktop calculators</b> .                                                                                                                                                                                                                                                                                                                                                                                                                                                                                                                                                                                                                                                                                                                                                                                                                                                                                                                                                                                                                                                                                                                                                                                  |                                                       |
| 2265: when was Washington elected president                                                                                                                                                                                                                                                                                                                                                                                                                                                                                                                                                                                                                                                                                                                                                                                                                                                                                                                                                                                                                                                                                                                                                                                                                                                                                                           | <i>George Washington</i>                              |
| <b>George Washington</b> (–, 1799) was the <b>first President of the United States</b> (1789–1797), the commander-in-chief of the <b>Continental Army</b> during the American Revolutionary War , and one of the Founding Fathers of the <b>United States</b> .                                                                                                                                                                                                                                                                                                                                                                                                                                                                                                                                                                                                                                                                                                                                                                                                                                                                                                                                                                                                                                                                                       |                                                       |
| 2279: what is customary at Shiva                                                                                                                                                                                                                                                                                                                                                                                                                                                                                                                                                                                                                                                                                                                                                                                                                                                                                                                                                                                                                                                                                                                                                                                                                                                                                                                      | <i>Shiva (Judaism)</i>                                |
| This state lasts for seven <b>days</b> , during which family members traditionally gather in one home (preferably the home of the deceased) and receive visitors.                                                                                                                                                                                                                                                                                                                                                                                                                                                                                                                                                                                                                                                                                                                                                                                                                                                                                                                                                                                                                                                                                                                                                                                     |                                                       |
| 2281: who is the guy in the wheelchair who is smart                                                                                                                                                                                                                                                                                                                                                                                                                                                                                                                                                                                                                                                                                                                                                                                                                                                                                                                                                                                                                                                                                                                                                                                                                                                                                                   | <i>Stephen Hawking in popular culture</i>             |
| Professor Stephen Hawking , known for being a theoretical physicist , has appeared in many works of popular culture.                                                                                                                                                                                                                                                                                                                                                                                                                                                                                                                                                                                                                                                                                                                                                                                                                                                                                                                                                                                                                                                                                                                                                                                                                                  |                                                       |
| 2283: what is in a hot toddy                                                                                                                                                                                                                                                                                                                                                                                                                                                                                                                                                                                                                                                                                                                                                                                                                                                                                                                                                                                                                                                                                                                                                                                                                                                                                                                          | <i>Hot toddy</i>                                      |
| A <b>hot toddy</b> , also <b>hot totty</b> , and <b>hot tottie</b> , is typically a mixed drink made of liquor and water with sugar and spices and served <b>hot</b> .                                                                                                                                                                                                                                                                                                                                                                                                                                                                                                                                                                                                                                                                                                                                                                                                                                                                                                                                                                                                                                                                                                                                                                                |                                                       |
| 2284: what is honey bee propolis                                                                                                                                                                                                                                                                                                                                                                                                                                                                                                                                                                                                                                                                                                                                                                                                                                                                                                                                                                                                                                                                                                                                                                                                                                                                                                                      | <i>Propolis</i>                                       |
| <b>Propolis</b> is a resinous mixture that <b>honey bees</b> collect from tree buds, sap flows, or other botanical sources.                                                                                                                                                                                                                                                                                                                                                                                                                                                                                                                                                                                                                                                                                                                                                                                                                                                                                                                                                                                                                                                                                                                                                                                                                           |                                                       |
| 2285: when was Steven Tyler born                                                                                                                                                                                                                                                                                                                                                                                                                                                                                                                                                                                                                                                                                                                                                                                                                                                                                                                                                                                                                                                                                                                                                                                                                                                                                                                      | <i>Steven Tyler</i>                                   |
| <b>Steven Tyler</b> (born <b>Steven Victor Tallarico</b> ; March 26, 1948) is an American <b>singer</b> , songwriter, and multi-instrumentalist, best known as the frontman and lead <b>singer</b> of the <b>Boston</b> -based rock band Aerosmith , in which he also plays the harmonica, and occasional piano and percussion.                                                                                                                                                                                                                                                                                                                                                                                                                                                                                                                                                                                                                                                                                                                                                                                                                                                                                                                                                                                                                       |                                                       |
| 2286: what is name of national anthem song of Switzerland                                                                                                                                                                                                                                                                                                                                                                                                                                                                                                                                                                                                                                                                                                                                                                                                                                                                                                                                                                                                                                                                                                                                                                                                                                                                                             | <i>Swiss Psalm</i>                                    |
| The Swiss Psalm ( , , ) is the <b>national anthem of Switzerland</b> .                                                                                                                                                                                                                                                                                                                                                                                                                                                                                                                                                                                                                                                                                                                                                                                                                                                                                                                                                                                                                                                                                                                                                                                                                                                                                |                                                       |
| 2287: what is blood urea                                                                                                                                                                                                                                                                                                                                                                                                                                                                                                                                                                                                                                                                                                                                                                                                                                                                                                                                                                                                                                                                                                                                                                                                                                                                                                                              | <i>Blood urea nitrogen</i>                            |
| Normal human <b>adult blood</b> should contain between 7 to 21 mg of <b>urea</b> nitrogen per 100 ml (7–21 mg/dL ) of <b>blood</b> .                                                                                                                                                                                                                                                                                                                                                                                                                                                                                                                                                                                                                                                                                                                                                                                                                                                                                                                                                                                                                                                                                                                                                                                                                  |                                                       |
| 2291: what is corpus christi holiday                                                                                                                                                                                                                                                                                                                                                                                                                                                                                                                                                                                                                                                                                                                                                                                                                                                                                                                                                                                                                                                                                                                                                                                                                                                                                                                  | <i>Corpus Christi (feast)</i>                         |
| The Feast of <b>Corpus Christi</b> (Latin for Body of <b>Christ</b> ), also known as <b>Corpus Domini</b> , is a Latin Rite liturgical solemnity celebrating the tradition and belief in the body and blood of Jesus <b>Christ</b> and his Real Presence in the Eucharist .                                                                                                                                                                                                                                                                                                                                                                                                                                                                                                                                                                                                                                                                                                                                                                                                                                                                                                                                                                                                                                                                           |                                                       |
| 2296: what is the difference between multistage and cluster sampling                                                                                                                                                                                                                                                                                                                                                                                                                                                                                                                                                                                                                                                                                                                                                                                                                                                                                                                                                                                                                                                                                                                                                                                                                                                                                  | <i>Cluster sampling</i>                               |
| In this technique, the total population is divided into these groups (or <b>clusters</b> ) and a <b>simple random sample</b> of the groups is selected.                                                                                                                                                                                                                                                                                                                                                                                                                                                                                                                                                                                                                                                                                                                                                                                                                                                                                                                                                                                                                                                                                                                                                                                               |                                                       |
| <b>Cluster sampling</b> is a <b>sampling</b> technique used when "natural" but relatively homogeneous groupings are evident in a statistical population .                                                                                                                                                                                                                                                                                                                                                                                                                                                                                                                                                                                                                                                                                                                                                                                                                                                                                                                                                                                                                                                                                                                                                                                             |                                                       |
| 2297: where is Jamestown north carolina                                                                                                                                                                                                                                                                                                                                                                                                                                                                                                                                                                                                                                                                                                                                                                                                                                                                                                                                                                                                                                                                                                                                                                                                                                                                                                               | <i>Jamestown, North Carolina</i>                      |
| <b>Jamestown</b> is a town in Guilford County , <b>North Carolina</b> , United States , and is a suburb of the nearby cities of Greensboro and High Point.                                                                                                                                                                                                                                                                                                                                                                                                                                                                                                                                                                                                                                                                                                                                                                                                                                                                                                                                                                                                                                                                                                                                                                                            |                                                       |
| 2302: what is stepwise linear regression                                                                                                                                                                                                                                                                                                                                                                                                                                                                                                                                                                                                                                                                                                                                                                                                                                                                                                                                                                                                                                                                                                                                                                                                                                                                                                              | <i>Stepwise regression</i>                            |
| In statistics , <b>stepwise regression</b> includes <b>regression</b> models in which the choice of predictive variables is carried out by an automatic procedure.                                                                                                                                                                                                                                                                                                                                                                                                                                                                                                                                                                                                                                                                                                                                                                                                                                                                                                                                                                                                                                                                                                                                                                                    |                                                       |
| 2314: when was Andy Griffith born                                                                                                                                                                                                                                                                                                                                                                                                                                                                                                                                                                                                                                                                                                                                                                                                                                                                                                                                                                                                                                                                                                                                                                                                                                                                                                                     | <i>Andy Griffith</i>                                  |
| <b>Andy Samuel Griffith</b> (June 1, 1926 – July 3, 2012) was an American actor, television producer, Grammy Award-winning Southern-gospel singer, and writer.                                                                                                                                                                                                                                                                                                                                                                                                                                                                                                                                                                                                                                                                                                                                                                                                                                                                                                                                                                                                                                                                                                                                                                                        |                                                       |
| 2315: what is the definition of a hung jury                                                                                                                                                                                                                                                                                                                                                                                                                                                                                                                                                                                                                                                                                                                                                                                                                                                                                                                                                                                                                                                                                                                                                                                                                                                                                                           | <i>Hung jury</i>                                      |
| A <b>hung jury</b> or deadlocked <b>jury</b> is a <b>jury</b> that cannot, by the required voting threshold, agree upon a verdict after an extended period of deliberation and is unable to change its votes.                                                                                                                                                                                                                                                                                                                                                                                                                                                                                                                                                                                                                                                                                                                                                                                                                                                                                                                                                                                                                                                                                                                                         |                                                       |
| 2321: what is the capacity of the cowboy stadium                                                                                                                                                                                                                                                                                                                                                                                                                                                                                                                                                                                                                                                                                                                                                                                                                                                                                                                                                                                                                                                                                                                                                                                                                                                                                                      | <i>Cowboys Stadium</i>                                |
| The <b>stadium</b> seats 85,000, making it the third <b>largest stadium</b> in the NFL by seating <b>capacity</b> .                                                                                                                                                                                                                                                                                                                                                                                                                                                                                                                                                                                                                                                                                                                                                                                                                                                                                                                                                                                                                                                                                                                                                                                                                                   |                                                       |
| 2326: what is the color puce                                                                                                                                                                                                                                                                                                                                                                                                                                                                                                                                                                                                                                                                                                                                                                                                                                                                                                                                                                                                                                                                                                                                                                                                                                                                                                                          | <i>Puce</i>                                           |
| The <b>colors</b> in the boxes at right are two of the various shades and varieties of <b>puce</b> .<br><b>Puce</b> (often misspelled as "puse", "peuse" or "peuce") is defined in the United States as a brownish-purple <b>color</b> .                                                                                                                                                                                                                                                                                                                                                                                                                                                                                                                                                                                                                                                                                                                                                                                                                                                                                                                                                                                                                                                                                                              |                                                       |
| 2333: where was JFK buried                                                                                                                                                                                                                                                                                                                                                                                                                                                                                                                                                                                                                                                                                                                                                                                                                                                                                                                                                                                                                                                                                                                                                                                                                                                                                                                            | <i>State funeral of John F. Kennedy</i>               |
| After the Requiem Mass at St. Matthew's Cathedral , the late president was <b>buried</b> at <b>Arlington National Cemetery</b> in Virginia.                                                                                                                                                                                                                                                                                                                                                                                                                                                                                                                                                                                                                                                                                                                                                                                                                                                                                                                                                                                                                                                                                                                                                                                                           |                                                       |
| 2337: what is renaissance english                                                                                                                                                                                                                                                                                                                                                                                                                                                                                                                                                                                                                                                                                                                                                                                                                                                                                                                                                                                                                                                                                                                                                                                                                                                                                                                     | <i>English Renaissance</i>                            |
| The <b>English Renaissance</b> was a cultural and <b>artistic</b> movement in <b>England</b> dating from the late 15th and early 16th centuries to the early 17th century.                                                                                                                                                                                                                                                                                                                                                                                                                                                                                                                                                                                                                                                                                                                                                                                                                                                                                                                                                                                                                                                                                                                                                                            |                                                       |
| 2338: Who is the husband of Betty Ford                                                                                                                                                                                                                                                                                                                                                                                                                                                                                                                                                                                                                                                                                                                                                                                                                                                                                                                                                                                                                                                                                                                                                                                                                                                                                                                | <i>Betty Ford</i>                                     |
| Elizabeth Ann Bloomer Warren "Betty" <b>Ford</b> (April 8, 1918 – July 8, 2011), was First Lady of the United States from 1974 to 1977 during the presidency of her <b>husband Gerald Ford</b> .                                                                                                                                                                                                                                                                                                                                                                                                                                                                                                                                                                                                                                                                                                                                                                                                                                                                                                                                                                                                                                                                                                                                                      |                                                       |
| 2344: what was Coco Chanel's real first name?                                                                                                                                                                                                                                                                                                                                                                                                                                                                                                                                                                                                                                                                                                                                                                                                                                                                                                                                                                                                                                                                                                                                                                                                                                                                                                         | <i>Coco Chanel</i>                                    |
| Gabrielle "Coco" Bonheur <b>Chanel</b> (August 19, 1883 – January 10, 1971) was a French fashion designer and founder of the <b>Chanel</b> brand.                                                                                                                                                                                                                                                                                                                                                                                                                                                                                                                                                                                                                                                                                                                                                                                                                                                                                                                                                                                                                                                                                                                                                                                                     |                                                       |
| 2345: what is grist mill stone                                                                                                                                                                                                                                                                                                                                                                                                                                                                                                                                                                                                                                                                                                                                                                                                                                                                                                                                                                                                                                                                                                                                                                                                                                                                                                                        | <i>Gristmill</i>                                      |
| A <b>gristmill</b> (also: <b>grist mill</b> , <b>corn mill</b> or <b>flour mill</b> ) grinds grain into flour .                                                                                                                                                                                                                                                                                                                                                                                                                                                                                                                                                                                                                                                                                                                                                                                                                                                                                                                                                                                                                                                                                                                                                                                                                                       |                                                       |
| 2352: where is Big Pokey from                                                                                                                                                                                                                                                                                                                                                                                                                                                                                                                                                                                                                                                                                                                                                                                                                                                                                                                                                                                                                                                                                                                                                                                                                                                                                                                         | <i>Big Pokey</i>                                      |
| Milton Powell (born December 4, 1977), better known by his stage name <b>Big Pokey</b> , is a rap artist from Houston, Texas and is one of the original members of the Screwed Up Click .<br><b>Big Pokey</b> joined up with DJ Screw in the early 1990s and started releasing songs on DJ Screw's many mixtapes .                                                                                                                                                                                                                                                                                                                                                                                                                                                                                                                                                                                                                                                                                                                                                                                                                                                                                                                                                                                                                                    |                                                       |
| 2353: what is baklava recipe                                                                                                                                                                                                                                                                                                                                                                                                                                                                                                                                                                                                                                                                                                                                                                                                                                                                                                                                                                                                                                                                                                                                                                                                                                                                                                                          | <i>Baklava</i>                                        |
| <b>Baklava</b> ( , or ; also Baklawa) is a rich, sweet pastry made of layers of phyllo pastry filled with chopped nuts and sweetened with syrup or honey .                                                                                                                                                                                                                                                                                                                                                                                                                                                                                                                                                                                                                                                                                                                                                                                                                                                                                                                                                                                                                                                                                                                                                                                            |                                                       |
| 2354: what is the rule of the 9s                                                                                                                                                                                                                                                                                                                                                                                                                                                                                                                                                                                                                                                                                                                                                                                                                                                                                                                                                                                                                                                                                                                                                                                                                                                                                                                      | <i>Total body surface area</i>                        |
| In adults, the " <b>rule of nines</b> " is used to determine the total percentage of area burned for each major section of the body.                                                                                                                                                                                                                                                                                                                                                                                                                                                                                                                                                                                                                                                                                                                                                                                                                                                                                                                                                                                                                                                                                                                                                                                                                  |                                                       |
| 2357: what is the sign for degrees                                                                                                                                                                                                                                                                                                                                                                                                                                                                                                                                                                                                                                                                                                                                                                                                                                                                                                                                                                                                                                                                                                                                                                                                                                                                                                                    | <i>Degree symbol</i>                                  |
| The <b>degree symbol</b> (°) is a typographical symbol that is used, among other things, to represent <b>degrees</b> of arc (e.g. in geographic coordinate systems ), hours (in the medical field), or <b>degrees</b> of temperature .                                                                                                                                                                                                                                                                                                                                                                                                                                                                                                                                                                                                                                                                                                                                                                                                                                                                                                                                                                                                                                                                                                                |                                                       |
| 2361: who is carlos pena on big time rush                                                                                                                                                                                                                                                                                                                                                                                                                                                                                                                                                                                                                                                                                                                                                                                                                                                                                                                                                                                                                                                                                                                                                                                                                                                                                                             | <i>Big Time Rush</i>                                  |
| <b>Big Time Rush</b> (BTR) is an American television series created by Scott Fellows about the Hollywood misadventures of four hockey players from Minnesota —Kendall, James, <b>Carlos</b> , and Logan, after they are selected to form a boy band .                                                                                                                                                                                                                                                                                                                                                                                                                                                                                                                                                                                                                                                                                                                                                                                                                                                                                                                                                                                                                                                                                                 |                                                       |
| 2370: WHO IS HENRY SAMPSON JR.                                                                                                                                                                                                                                                                                                                                                                                                                                                                                                                                                                                                                                                                                                                                                                                                                                                                                                                                                                                                                                                                                                                                                                                                                                                                                                                        | <i>Henry Sampson (inventor)</i>                       |
| <b>Henry T. Thomas Sampson, Jr.</b> (born in <b>Jackson, Mississippi</b> in 1934) is an African-American inventor.                                                                                                                                                                                                                                                                                                                                                                                                                                                                                                                                                                                                                                                                                                                                                                                                                                                                                                                                                                                                                                                                                                                                                                                                                                    |                                                       |
| 2383: what is the fundamental theorem of calculus used for                                                                                                                                                                                                                                                                                                                                                                                                                                                                                                                                                                                                                                                                                                                                                                                                                                                                                                                                                                                                                                                                                                                                                                                                                                                                                            | <i>Fundamental theorem of calculus</i>                |
| The <b>fundamental theorem of calculus</b> is a <b>theorem</b> that links the concept of the derivative of a <b>function</b> with the concept of the <b>integral</b> .                                                                                                                                                                                                                                                                                                                                                                                                                                                                                                                                                                                                                                                                                                                                                                                                                                                                                                                                                                                                                                                                                                                                                                                |                                                       |
| 2385: what is nicki minaj real name                                                                                                                                                                                                                                                                                                                                                                                                                                                                                                                                                                                                                                                                                                                                                                                                                                                                                                                                                                                                                                                                                                                                                                                                                                                                                                                   | <i>Nicki Minaj</i>                                    |
| Onika Tanya Maraj (born December 8, 1982), known by her stage <b>name Nicki Minaj</b> ( ), is a Trinidadian-born American rapper, <b>singer</b> , songwriter and <b>television</b> personality.                                                                                                                                                                                                                                                                                                                                                                                                                                                                                                                                                                                                                                                                                                                                                                                                                                                                                                                                                                                                                                                                                                                                                       |                                                       |
| 2390: what is the disease osteonecrosis of the jaw?                                                                                                                                                                                                                                                                                                                                                                                                                                                                                                                                                                                                                                                                                                                                                                                                                                                                                                                                                                                                                                                                                                                                                                                                                                                                                                   | <i>Osteonecrosis of the jaw</i>                       |
| <b>Osteonecrosis of the jaw</b> (ONJ) is a <b>severe bone disease</b> that affects the maxilla and the mandible .                                                                                                                                                                                                                                                                                                                                                                                                                                                                                                                                                                                                                                                                                                                                                                                                                                                                                                                                                                                                                                                                                                                                                                                                                                     |                                                       |
| 2395: who is suicide trn                                                                                                                                                                                                                                                                                                                                                                                                                                                                                                                                                                                                                                                                                                                                                                                                                                                                                                                                                                                                                                                                                                                                                                                                                                                                                                                              | <i>Suicide (character)</i>                            |
| <b>Suicide</b> is a fictional character from <b>TNA Impact!</b>                                                                                                                                                                                                                                                                                                                                                                                                                                                                                                                                                                                                                                                                                                                                                                                                                                                                                                                                                                                                                                                                                                                                                                                                                                                                                       |                                                       |
| 2397: where is hickory located ne                                                                                                                                                                                                                                                                                                                                                                                                                                                                                                                                                                                                                                                                                                                                                                                                                                                                                                                                                                                                                                                                                                                                                                                                                                                                                                                     | <i>Hickory; North Carolina</i>                        |
| <b>Hickory</b> is the principal city in the Hickory-Lenoir-Morganton MSA , in which the population at the 2010 Census was 365,497.<br><b>Hickory</b> is a city in Catawba County , with parts also in Burke County and Caldwell County .                                                                                                                                                                                                                                                                                                                                                                                                                                                                                                                                                                                                                                                                                                                                                                                                                                                                                                                                                                                                                                                                                                              |                                                       |
| 2398: what is Polyester in packaging PET                                                                                                                                                                                                                                                                                                                                                                                                                                                                                                                                                                                                                                                                                                                                                                                                                                                                                                                                                                                                                                                                                                                                                                                                                                                                                                              | <i>Polyethylene terephthalate</i>                     |
| <b>Polyethylene terephthalate</b> (sometimes written poly( <b>ethylene</b> terephthalate)), commonly abbreviated <b>PET</b> , <b>PETE</b> , or the obsolete PETP or PET-P, is a thermoplastic <b>polymer resin</b> of the <b>polyester</b> family and is used in synthetic <b>fibers</b> ; beverage, food and other liquid containers ; thermoforming applications; and engineering <b>resins</b> often in combination with glass <b>fiber</b> .                                                                                                                                                                                                                                                                                                                                                                                                                                                                                                                                                                                                                                                                                                                                                                                                                                                                                                      |                                                       |
| 2403: who is director Jack Smight                                                                                                                                                                                                                                                                                                                                                                                                                                                                                                                                                                                                                                                                                                                                                                                                                                                                                                                                                                                                                                                                                                                                                                                                                                                                                                                     | <i>Jack Smight</i>                                    |
| <b>Jack Smight</b> (March 9, 1925 - September 1, 2003) was an American theatre and film <b>director</b> .                                                                                                                                                                                                                                                                                                                                                                                                                                                                                                                                                                                                                                                                                                                                                                                                                                                                                                                                                                                                                                                                                                                                                                                                                                             |                                                       |
| 2404: what is dmitri mendelev 4                                                                                                                                                                                                                                                                                                                                                                                                                                                                                                                                                                                                                                                                                                                                                                                                                                                                                                                                                                                                                                                                                                                                                                                                                                                                                                                       | <i>Dmitri Mendeleev</i>                               |
| <b>Dmitri</b> Ivanovich <b>Mendeleev</b> (; 8 February 1834 – 2 February 1907 O.S. 27 January 1834 – 20 January 1907) was a Russian chemist and inventor.                                                                                                                                                                                                                                                                                                                                                                                                                                                                                                                                                                                                                                                                                                                                                                                                                                                                                                                                                                                                                                                                                                                                                                                             |                                                       |
| 2405: where is Modesto California                                                                                                                                                                                                                                                                                                                                                                                                                                                                                                                                                                                                                                                                                                                                                                                                                                                                                                                                                                                                                                                                                                                                                                                                                                                                                                                     | <i>Modesto, California</i>                            |
| <b>Modesto</b> ( Spanish for " <b>modest</b> " ), officially the <b>City of Modesto</b> , is the county seat and largest <b>city</b> of Stanislaus County , <b>California</b> , United States .                                                                                                                                                                                                                                                                                                                                                                                                                                                                                                                                                                                                                                                                                                                                                                                                                                                                                                                                                                                                                                                                                                                                                       |                                                       |
| 2407: what is the female symbol called                                                                                                                                                                                                                                                                                                                                                                                                                                                                                                                                                                                                                                                                                                                                                                                                                                                                                                                                                                                                                                                                                                                                                                                                                                                                                                                | <i>Gender symbol</i>                                  |
| The two standard gender <b>symbols</b> denoting male ♂ and <b>female</b> ♀ are derived from astrological <b>symbols</b> , denoting the classical planets Mars and Venus , respectively.                                                                                                                                                                                                                                                                                                                                                                                                                                                                                                                                                                                                                                                                                                                                                                                                                                                                                                                                                                                                                                                                                                                                                               |                                                       |
| 2409: what is leasehold; real estate                                                                                                                                                                                                                                                                                                                                                                                                                                                                                                                                                                                                                                                                                                                                                                                                                                                                                                                                                                                                                                                                                                                                                                                                                                                                                                                  | <i>Leasehold estate</i>                               |
| A <b>leasehold estate</b> is an ownership of a temporary <b>right to hold land</b> or <b>property</b> in which a lessee or a tenant <b>holds rights of real property</b> by some form of title from a lessor or landlord .                                                                                                                                                                                                                                                                                                                                                                                                                                                                                                                                                                                                                                                                                                                                                                                                                                                                                                                                                                                                                                                                                                                            |                                                       |
| 2425: when was Mary Anderson born                                                                                                                                                                                                                                                                                                                                                                                                                                                                                                                                                                                                                                                                                                                                                                                                                                                                                                                                                                                                                                                                                                                                                                                                                                                                                                                     | <i>Mary Anderson (inventor)</i>                       |
| <b>Mary Anderson</b> (1866–1953) was a real estate developer, rancher, viticulturist and inventor of the windshield wiper blade.                                                                                                                                                                                                                                                                                                                                                                                                                                                                                                                                                                                                                                                                                                                                                                                                                                                                                                                                                                                                                                                                                                                                                                                                                      |                                                       |
| 2426: WHO WAS IN THE MOVIE I CONFESS WITH MONTGOMERY CLIFT                                                                                                                                                                                                                                                                                                                                                                                                                                                                                                                                                                                                                                                                                                                                                                                                                                                                                                                                                                                                                                                                                                                                                                                                                                                                                            | <i>I Confess (film)</i>                               |
| <b>I Confess</b> is a 1953 drama <b>film</b> directed by Alfred <b>Hitchcock</b> , and starring <b>Montgomery Clift</b> as Fr. Michael William Logan, a Catholic priest , Anne Baxter as Ruth Grandfort, and Karl Malden as Inspector Larrue.                                                                                                                                                                                                                                                                                                                                                                                                                                                                                                                                                                                                                                                                                                                                                                                                                                                                                                                                                                                                                                                                                                         |                                                       |
| 2430: what is black hairy tongue disease                                                                                                                                                                                                                                                                                                                                                                                                                                                                                                                                                                                                                                                                                                                                                                                                                                                                                                                                                                                                                                                                                                                                                                                                                                                                                                              | <i>Black hairy tongue</i>                             |
| <b>Black hairy tongue</b> (BHT, also termed lingua villosa nigra) refers to a condition of the <b>tongue</b> where the filiform papillae elongate with <b>black</b> or brown discoloration, giving a <b>black</b> and <b>hairy</b> appearance.                                                                                                                                                                                                                                                                                                                                                                                                                                                                                                                                                                                                                                                                                                                                                                                                                                                                                                                                                                                                                                                                                                        |                                                       |
| 2434: what is ethernet gigabit                                                                                                                                                                                                                                                                                                                                                                                                                                                                                                                                                                                                                                                                                                                                                                                                                                                                                                                                                                                                                                                                                                                                                                                                                                                                                                                        | <i>Gigabit Ethernet</i>                               |
| In computer networking , <b>gigabit Ethernet</b> (GbE or 1 GbE) is a term describing various technologies for transmitting <b>Ethernet</b> frames at a rate of a <b>gigabit</b> per second (1,000,000,000 bits per second), as defined by the IEEE 802.3-2008 standard.                                                                                                                                                                                                                                                                                                                                                                                                                                                                                                                                                                                                                                                                                                                                                                                                                                                                                                                                                                                                                                                                               |                                                       |
| 2438: where is the tibia location                                                                                                                                                                                                                                                                                                                                                                                                                                                                                                                                                                                                                                                                                                                                                                                                                                                                                                                                                                                                                                                                                                                                                                                                                                                                                                                     | <i>Tibia</i>                                          |
| The <b>tibia</b> is named for the Greek aulos flute, also known as a <b>tibia</b> .<br>The <b>tibia</b> ( ), shinbone or shankbone, is the larger and stronger of the two bones in the leg below the knee in vertebrates (the other being the fibula ), and connects the knee with the ankle bones .<br>The <b>tibia</b> is found next to the fibula on the medial side of the leg, closer to center-line.<br>The <b>tibia</b> is connected to the fibula by an interosseous membrane , forming a type of joint called a syndesmosis with very little movement.                                                                                                                                                                                                                                                                                                                                                                                                                                                                                                                                                                                                                                                                                                                                                                                       |                                                       |
| 2442: where is bloemfontein in africa                                                                                                                                                                                                                                                                                                                                                                                                                                                                                                                                                                                                                                                                                                                                                                                                                                                                                                                                                                                                                                                                                                                                                                                                                                                                                                                 | <i>Bloemfontein</i>                                   |
| <b>Bloemfontein</b> ( ; Dutch for "fountain of flowers") is the capital city of the Free State Province of South <b>Africa</b> ; and, as the judicial capital of the nation, one of South <b>Africa's</b> three national capitals – the other two being Cape Town , the legislative capital, and Pretoria , the administrative capital.                                                                                                                                                                                                                                                                                                                                                                                                                                                                                                                                                                                                                                                                                                                                                                                                                                                                                                                                                                                                               |                                                       |
| 2447: What is the prostate for?                                                                                                                                                                                                                                                                                                                                                                                                                                                                                                                                                                                                                                                                                                                                                                                                                                                                                                                                                                                                                                                                                                                                                                                                                                                                                                                       | <i>Prostate</i>                                       |
| The <b>prostate</b> (from Greek προσαρτήρ – <b>prostates</b> , literally "one who stands before", "protector", "guardian") is a compound tubuloalveolar exocrine <b>gland</b> of the male reproductive system in most mammals .                                                                                                                                                                                                                                                                                                                                                                                                                                                                                                                                                                                                                                                                                                                                                                                                                                                                                                                                                                                                                                                                                                                       |                                                       |
| 2450: what is in the preamble of the constitution                                                                                                                                                                                                                                                                                                                                                                                                                                                                                                                                                                                                                                                                                                                                                                                                                                                                                                                                                                                                                                                                                                                                                                                                                                                                                                     | <i>Preamble to the United States Constitution</i>     |
| The <b>Preamble</b> to the United States <b>Constitution</b> is a brief introductory statement of the <b>Constitution's</b> fundamental purposes and guiding principles.                                                                                                                                                                                                                                                                                                                                                                                                                                                                                                                                                                                                                                                                                                                                                                                                                                                                                                                                                                                                                                                                                                                                                                              |                                                       |
| 2462: where is the sermon on the mount in the bible                                                                                                                                                                                                                                                                                                                                                                                                                                                                                                                                                                                                                                                                                                                                                                                                                                                                                                                                                                                                                                                                                                                                                                                                                                                                                                   | <i>Sermon on the Mount</i>                            |
| to most believers in Jesus, the <b>Sermon on the Mount</b> contains the central tenets of Christian discipleship .<br>The <b>Sermon on the Mount</b> ( anglicized from the Matthean Vulgate Latin section title: Sermo in monte) is a collection of sayings and teachings of Jesus , which emphasizes his moral teaching found in the Gospel of Matthew (chapters 5 , 6 and 7 ) .                                                                                                                                                                                                                                                                                                                                                                                                                                                                                                                                                                                                                                                                                                                                                                                                                                                                                                                                                                     |                                                       |
| <b>Sermon on the Mount</b> by Carl Bloch                                                                                                                                                                                                                                                                                                                                                                                                                                                                                                                                                                                                                                                                                                                                                                                                                                                                                                                                                                                                                                                                                                                                                                                                                                                                                                              |                                                       |
| 2468: what is article 5 about                                                                                                                                                                                                                                                                                                                                                                                                                                                                                                                                                                                                                                                                                                                                                                                                                                                                                                                                                                                                                                                                                                                                                                                                                                                                                                                         | <i>Article Five of the United States Constitution</i> |
| <b>Article Five</b> of the United States Constitution describes the process whereby the Constitution may be altered.                                                                                                                                                                                                                                                                                                                                                                                                                                                                                                                                                                                                                                                                                                                                                                                                                                                                                                                                                                                                                                                                                                                                                                                                                                  |                                                       |
| 2471: what is the political tea party                                                                                                                                                                                                                                                                                                                                                                                                                                                                                                                                                                                                                                                                                                                                                                                                                                                                                                                                                                                                                                                                                                                                                                                                                                                                                                                 | <i>Tea Party movement</i>                             |
| The <b>Tea Party</b> movement is an American <b>political</b> movement that advocates strict adherence to the United States Constitution , reducing U.S. government spending and taxes , and reduction of the U.S. <b>national</b> debt and federal budget deficit .                                                                                                                                                                                                                                                                                                                                                                                                                                                                                                                                                                                                                                                                                                                                                                                                                                                                                                                                                                                                                                                                                  |                                                       |
| 2474: What is the function of albumin?                                                                                                                                                                                                                                                                                                                                                                                                                                                                                                                                                                                                                                                                                                                                                                                                                                                                                                                                                                                                                                                                                                                                                                                                                                                                                                                | <i>Human serum albumin</i>                            |
| <b>Albumin</b> transports hormones, fatty acids, and other compounds, buffers pH, and maintains osmotic pressure , among other <b>functions</b> .                                                                                                                                                                                                                                                                                                                                                                                                                                                                                                                                                                                                                                                                                                                                                                                                                                                                                                                                                                                                                                                                                                                                                                                                     |                                                       |
| 2476: who is ezeziel in the bible                                                                                                                                                                                                                                                                                                                                                                                                                                                                                                                                                                                                                                                                                                                                                                                                                                                                                                                                                                                                                                                                                                                                                                                                                                                                                                                     | <i>Book of Ezekiel</i>                                |
| The Book of <b>Ezekiel</b> is the third of the Latter Prophets in the Hebrew <b>Bible</b> , following the books of Isaiah and Jeremiah and preceding the Book of the Twelve .                                                                                                                                                                                                                                                                                                                                                                                                                                                                                                                                                                                                                                                                                                                                                                                                                                                                                                                                                                                                                                                                                                                                                                         |                                                       |
| 2483: where are the ten commandments in the bible                                                                                                                                                                                                                                                                                                                                                                                                                                                                                                                                                                                                                                                                                                                                                                                                                                                                                                                                                                                                                                                                                                                                                                                                                                                                                                     | <i>Ten Commandments</i>                               |
| The <b>Ten Commandments</b> appear twice in the Hebrew <b>Bible</b> , in the books of <b>Exodus</b> and Deuteronomy .                                                                                                                                                                                                                                                                                                                                                                                                                                                                                                                                                                                                                                                                                                                                                                                                                                                                                                                                                                                                                                                                                                                                                                                                                                 |                                                       |
| 2504: where is loxahatchee fl at                                                                                                                                                                                                                                                                                                                                                                                                                                                                                                                                                                                                                                                                                                                                                                                                                                                                                                                                                                                                                                                                                                                                                                                                                                                                                                                      | <i>Loxahatchee, Florida</i>                           |
| <b>Loxahatchee</b> is located within the Indian Trails Improvement District and the <b>Loxahatchee</b> Groves Water Control District. In 2006, the state of Florida approved incorporation of part of <b>Loxahatchee</b> as the Town of <b>Loxahatchee</b> Groves to become the 38th municipality in Palm Beach County.<br>The name <b>Loxahatchee</b> means "turtle river".<br><b>Loxahatchee</b> is also the name of the Post Office that serves this area, which is under the zip code of 33470.<br><b>Loxahatchee</b> is a community located in Palm Beach County, Florida, United States .<br>Lion Country Safari, a drive-through safari park , is located in <b>Loxahatchee</b> .                                                                                                                                                                                                                                                                                                                                                                                                                                                                                                                                                                                                                                                              |                                                       |
| 2506: what is chow mein                                                                                                                                                                                                                                                                                                                                                                                                                                                                                                                                                                                                                                                                                                                                                                                                                                                                                                                                                                                                                                                                                                                                                                                                                                                                                                                               | <i>Chow mein</i>                                      |
| <b>Chow mein</b> ( ; Chinese : 炒麵, " <b>fried</b> noodles") is a <b>Chinese</b> term for a dish of stir-fried noodles , of which there are many varieties.                                                                                                                                                                                                                                                                                                                                                                                                                                                                                                                                                                                                                                                                                                                                                                                                                                                                                                                                                                                                                                                                                                                                                                                            |                                                       |
| 2511: what is the oath of allegiance of the united states                                                                                                                                                                                                                                                                                                                                                                                                                                                                                                                                                                                                                                                                                                                                                                                                                                                                                                                                                                                                                                                                                                                                                                                                                                                                                             | <i>Oath of Allegiance (United States)</i>             |
| The <b>United States Oath of Allegiance</b> (officially referred to as the " <b>Oath of Allegiance</b> ," 8 C.F.R. Part 337 (2008)) is an <b>oath</b> that must be taken by all immigrants who wish to become <b>United States</b> citizens .                                                                                                                                                                                                                                                                                                                                                                                                                                                                                                                                                                                                                                                                                                                                                                                                                                                                                                                                                                                                                                                                                                         |                                                       |
| 2512: what is that dot on the forehead of indian women                                                                                                                                                                                                                                                                                                                                                                                                                                                                                                                                                                                                                                                                                                                                                                                                                                                                                                                                                                                                                                                                                                                                                                                                                                                                                                | <i>hifil Bindi (decoration)</i>                       |
| A <b>bindi</b> (, from Sanskrit bindu, meaning "a drop, small particle, <b>dot</b> "), or a pottu/bottu (in Tamil, Telugu, and Malayalam) is a <b>forehead</b> decoration worn in South Asia (particularly India , Bangladesh, Nepal , Sri Lanka and Mauritius ) and Southeast Asia .                                                                                                                                                                                                                                                                                                                                                                                                                                                                                                                                                                                                                                                                                                                                                                                                                                                                                                                                                                                                                                                                 |                                                       |
| 2524: where is Desmanthus illinoensis found                                                                                                                                                                                                                                                                                                                                                                                                                                                                                                                                                                                                                                                                                                                                                                                                                                                                                                                                                                                                                                                                                                                                                                                                                                                                                                           | <i>Desmanthus illinoensis</i>                         |
| <b>Desmanthus illinoensis</b> (commonly known as Illinois bundleflower, prairie-mimosa or pricklegweed) is a plant in many areas of the south central US.                                                                                                                                                                                                                                                                                                                                                                                                                                                                                                                                                                                                                                                                                                                                                                                                                                                                                                                                                                                                                                                                                                                                                                                             |                                                       |
| 2531: what is the origin of fiona                                                                                                                                                                                                                                                                                                                                                                                                                                                                                                                                                                                                                                                                                                                                                                                                                                                                                                                                                                                                                                                                                                                                                                                                                                                                                                                     | <i>Fiona</i>                                          |
| The name <b>Fiona</b> has been particularly popular for girls of Asian or Pacific Islander descent in New York City , where <b>Fiona</b> ranked as the ninth most popular name for girls from those groups in 2007.<br>There is also a modern tendency to equate the authentic Scottish Gaelic feminine name Fionnghal with <b>Fiona</b> .<br>The name was subsequently used as a pseudonym by William Sharp (1855–1905), who authored several romantic works under the name " <b>Fiona Macleod</b> ".<br>The name <b>Fiona</b> was invented, and first used, by the Scottish poet James Macpherson (1736–96), author of the Ossian poems, which he claimed were translations from ancient Gaelic sources (sources, when challenged, he never produced).<br>The name <b>Fiona</b> is rising in popularity particularly in German-speaking countries.<br>The name <b>Fiona</b> is also sometimes used as an Anglicisation of the Irish-language name Fiona, although these names are otherwise unrelated (as Fiona is derived from an element meaning "vine").<br><b>Fiona</b> was tied for third place in the ranking of most popular names for baby girls born in the tiny principality of Liechtenstein in 2008.<br><b>Fiona</b> was the 49th most popular name for baby girls born in 2008 in Germany .<br><b>Fiona</b> is a feminine given name . |                                                       |
| 2533: what is auto quarter panel                                                                                                                                                                                                                                                                                                                                                                                                                                                                                                                                                                                                                                                                                                                                                                                                                                                                                                                                                                                                                                                                                                                                                                                                                                                                                                                      | <i>Quarter panel</i>                                  |
| On an <b>automobile</b> , a <b>quarter panel</b> (or rear wing as it is known in British English ) is usually considered the body <b>panel</b> which goes between the rear door and the trunk and typically wraps around the wheel well; however, the similar front section (vehicle), between the door and the hood, is sometimes incorrectly referred to as a <b>quarter panel</b> .                                                                                                                                                                                                                                                                                                                                                                                                                                                                                                                                                                                                                                                                                                                                                                                                                                                                                                                                                                |                                                       |
| 2536: when was pearl harbor bombed                                                                                                                                                                                                                                                                                                                                                                                                                                                                                                                                                                                                                                                                                                                                                                                                                                                                                                                                                                                                                                                                                                                                                                                                                                                                                                                    | <i>Attack on Pearl Harbor</i>                         |
| The attack on <b>Pearl Harbor</b> (called Hawaii Operation or Operation AI by the Japanese Imperial General Headquarters (Operation Z in planning) and the Battle of <b>Pearl Harbor</b> ) was a surprise military strike conducted by the Imperial Japanese                                                                                                                                                                                                                                                                                                                                                                                                                                                                                                                                                                                                                                                                                                                                                                                                                                                                                                                                                                                                                                                                                          |                                                       |

|                                                                                                                                                                                                                                                                                                                                                          |                                               |
|----------------------------------------------------------------------------------------------------------------------------------------------------------------------------------------------------------------------------------------------------------------------------------------------------------------------------------------------------------|-----------------------------------------------|
| Navy against the United States naval base at <b>Pearl Harbor</b> , Hawaii, on the morning of December 7, 1941 (December 8 in Japan).                                                                                                                                                                                                                     |                                               |
| 2537: what is the la tour de france                                                                                                                                                                                                                                                                                                                      | <i>Tour de France</i>                         |
| The <b>Tour de France</b> ( ) is an annual multiple stage bicycle race primarily held in <b>France</b> , while also occasionally making passes through nearby countries.                                                                                                                                                                                 |                                               |
| 2540: what is associates arts degree                                                                                                                                                                                                                                                                                                                     | <i>Associate degree</i>                       |
| An <b>associate degree</b> is an undergraduate academic <b>degree</b> awarded by community colleges, junior colleges, technical colleges, and bachelor's <b>degree</b> -granting colleges and universities upon completion of a course of study usually lasting two years.                                                                               |                                               |
| 2543: what is vat tax?                                                                                                                                                                                                                                                                                                                                   | <i>Value added tax</i>                        |
| A <b>VAT</b> is like a sales <b>tax</b> in that ultimately only the end <b>consumer</b> is <b>taxed</b> .                                                                                                                                                                                                                                                |                                               |
| A value added <b>tax (VAT)</b> is a form of <b>consumption tax</b> .                                                                                                                                                                                                                                                                                     |                                               |
| 2544: what is high sticking in hockey                                                                                                                                                                                                                                                                                                                    | <i>High-Sticking</i>                          |
| -sticking is the name of two infractions in the sport of ice <b>hockey</b> that may occur when a player intentionally or inadvertently plays with his or her <b>stick</b> above the height of the shoulders or above the cross bar of a <b>hockey</b> goal.                                                                                              |                                               |
| #2553: when was the trojan war                                                                                                                                                                                                                                                                                                                           | <i>Trojan War</i>                             |
| The ancient <b>Greeks</b> <b>thought</b> that the Trojan <b>War</b> was a <b>historical event</b> that had taken <b>place</b> in the 13th or 12th <b>century BC</b> , and <b>believed</b> that Troy was <b>located</b> in modern-day Turkey near the Dardanelles.                                                                                        |                                               |
| 2556: where is the palatine canal                                                                                                                                                                                                                                                                                                                        | <i>Greater palatine canal</i>                 |
| The greater <b>palatine canal</b> (or pterygopalatine <b>canal</b> ) is a passage in the skull that transmits the greater <b>palatine</b> artery, vein, and nerve between the pterygopalatine fossa and the oral cavity.                                                                                                                                 |                                               |
| 2557: what is the lowest temperature ever recorded in antarctica                                                                                                                                                                                                                                                                                         | <i>Climate of Antarctica</i>                  |
| <b>Antarctica</b> has the <b>lowest</b> naturally occurring <b>temperature</b> ever <b>recorded</b> on the ground on Earth: $-89.2^{\circ}\text{C}$ ( $-128.6^{\circ}\text{F}$ ) at Vostok Station.                                                                                                                                                      |                                               |
| 2560: what is oregon institute of technology like                                                                                                                                                                                                                                                                                                        | <i>Oregon Institute of Technology</i>         |
| <b>Oregon Institute of Technology</b> , also known as <b>Oregon Tech</b> or <b>OIT</b> , is one of seven Universities in the <b>Oregon</b> University System, and the only public <b>institute of technology</b> in the Pacific Northwest.                                                                                                               |                                               |
| #2563: When Is Passover Over                                                                                                                                                                                                                                                                                                                             | <i>Passover</i>                               |
| In Judaism, a <b>day</b> commences at dusk and lasts until the following dusk, thus the first <b>day of Passover</b> only begins after dusk of the 14th of Nisan and ends at dusk of the 15th <b>day</b> of the month of Nisan.                                                                                                                          |                                               |
| 2580: WHERE IS ROUGH AND READY, CA                                                                                                                                                                                                                                                                                                                       | <i>Rough and Ready, California</i>            |
| <b>Rough</b> and <b>Ready</b> is a census-designated place in Nevada County, California, United States.                                                                                                                                                                                                                                                  |                                               |
| 2584: where is rashard lewis from???                                                                                                                                                                                                                                                                                                                     | <i>Rashard Lewis</i>                          |
| <b>Rashard</b> Quovon <b>Lewis</b> (born August 8, 1979 in Pineville, Louisiana) is an American professional basketball player who currently plays for the Miami Heat of the NBA.                                                                                                                                                                        |                                               |
| 2590: what is doxycycline hyclate used for                                                                                                                                                                                                                                                                                                               | <i>Doxycycline</i>                            |
| <b>Doxycycline</b> is a member of the tetracycline antibiotics group, and is commonly <b>used</b> to treat a variety of infections.                                                                                                                                                                                                                      |                                               |
| 2592: what is sodium hypochlorite solution                                                                                                                                                                                                                                                                                                               | <i>Sodium hypochlorite</i>                    |
| <b>Sodium hypochlorite solution</b> , commonly known as bleach or liquid bleach, is frequently used as a disinfectant or a bleaching agent.                                                                                                                                                                                                              |                                               |
| #2597: when was jacques cousteau born                                                                                                                                                                                                                                                                                                                    | <i>Jacques Cousteau</i>                       |
| Jacques-Yves <b>Cousteau</b> (, commonly known in English as <b>Jacques Cousteau</b> ; 11 June 1910 – 25 June 1997) was a French naval officer, explorer, <b>conservationist</b> , filmmaker, innovator, scientist, photographer, author and researcher who studied the sea and all forms of life in water.                                              |                                               |
| 2607: where was the fugitive slave law made                                                                                                                                                                                                                                                                                                              | <i>Fugitive Slave Act of 1850</i>             |
| The <b>Fugitive Slave Law</b> or <b>Fugitive Slave Act</b> was passed by the United States Congress on September 18, 1850, as part of the Compromise of 1850 between Southern <b>slave-holding</b> interests and Northern Free-Soilers.                                                                                                                  |                                               |
| 2612: what is eic earned income credit                                                                                                                                                                                                                                                                                                                   | <i>Earned Income Tax Credit</i>               |
| The United States <b>federal earned income tax credit</b> or <b>earned income credit (EITC or EIC)</b> is a refundable tax <b>credit</b> for low- and medium-income individuals and couples, primarily for those who have qualifying children.                                                                                                           |                                               |
| 2620: where is valley village ca                                                                                                                                                                                                                                                                                                                         | <i>Valley Village, Los Angeles</i>            |
| <b>Village</b> is a district in the San Fernando <b>Valley</b> region of Los Angeles, California.                                                                                                                                                                                                                                                        |                                               |
| <b>Valley Village</b> ParkValley                                                                                                                                                                                                                                                                                                                         |                                               |
| 2630: What is sign of cancer                                                                                                                                                                                                                                                                                                                             | <i>Cancer (astrology)</i>                     |
| <b>Cancer (♋)</b> is an astrological <b>sign</b> , which is associated with the constellation <b>Cancer</b> .                                                                                                                                                                                                                                            |                                               |
| 2643: what is a gsm cell phone                                                                                                                                                                                                                                                                                                                           | <i>GSM</i>                                    |
| <b>GSM</b> (Global System for Mobile Communications, originally ), is a <b>standard</b> set developed by the European Telecommunications <b>Standards</b> Institute (ETSI) to describe protocols for second generation ( 2G ) digital cellular networks used by mobile <b>phones</b> .                                                                   |                                               |
| 2644: what was the cash and carry lend lease                                                                                                                                                                                                                                                                                                             | <i>Lend-Lease</i>                             |
| The <b>Lend Lease</b> act was an act where the United States had supported its allies.                                                                                                                                                                                                                                                                   |                                               |
| 2646: what is el morro in puerto rico                                                                                                                                                                                                                                                                                                                    | <i>Castillo San Felipe del Morro</i>          |
| Castillo San <b>Felipe del Morro</b> also known as Fort San <b>Felipe del Morro</b> or <b>Morro</b> Castle, is a 16th-century citadel located in San Juan, <b>Puerto Rico</b> .                                                                                                                                                                          |                                               |
| 2651: where are poison dart frog seen                                                                                                                                                                                                                                                                                                                    | <i>Poison dart frog</i>                       |
| <b>Poison dart frog</b> (also dart-poison <b>frog</b> , <b>poison frog</b> or formerly <b>poison</b> arrow <b>frog</b> ) is the common name of a group of <b>frogs</b> in the family Dendrobatidae which are native to Central and South America.                                                                                                        |                                               |
| 2659: where were the Winter Olympics in 2006                                                                                                                                                                                                                                                                                                             | <i>2006 Winter Olympics</i>                   |
| The <b>2006 Winter Olympics</b> , officially known as the XX <b>Olympic Winter</b> Games, was a <b>winter</b> multi-sport event which was celebrated in Turin, Italy from February 10, <b>2006</b> , through February 26, <b>2006</b> .                                                                                                                  |                                               |
| 2671: WHAT IS NON BINDING?                                                                                                                                                                                                                                                                                                                               | <i>Non-binding arbitration</i>                |
| Subsequent to a non-binding arbitration, the parties remain free to pursue their claims either through the courts, or by way of a <b>binding</b> arbitration, although in practice a settlement is the most common outcome.                                                                                                                              |                                               |
| Non-binding arbitration is a type of arbitration in which the arbitrator makes a determination of the rights of the parties to the dispute, but this determination is not <b>binding</b> upon them, and no enforceable arbitration award is issued.                                                                                                      |                                               |
| 2675: who was mr big on sex and the city                                                                                                                                                                                                                                                                                                                 | <i>Mr. Big (Sex and the City)</i>             |
| <b>John</b> James "Mr. <b>Big</b> " Preston is a recurring fictional <b>character</b> in the HBO <b>series</b> <b>Sex</b> and the <b>City</b> , portrayed by Chris Noth.                                                                                                                                                                                 |                                               |
| 2682: what is the actresses name that played in walk that line?                                                                                                                                                                                                                                                                                          | <i>Walk the Line</i>                          |
| The <b>film</b> was nominated for five Academy Awards including <b>Best Actor</b> (Joaquin Phoenix), <b>Best Actress</b> (Reese Witherspoon, which she won), and <b>Best Costume Design</b> (Ariane Phillips).                                                                                                                                           |                                               |
| 2686: where is university of nelson mandela metropolitan located                                                                                                                                                                                                                                                                                         | <i>Nelson Mandela Metropolitan University</i> |
| <b>Nelson Mandela Metropolitan University</b> (NMMU) is a South African tertiary education institution with its main administration in the coastal city of Port Elizabeth.                                                                                                                                                                               |                                               |
| #2687: when was How the west was won filmed?                                                                                                                                                                                                                                                                                                             | <i>How the West Was Won (film)</i>            |
| How the <b>West Was Won</b> is a 1962 American epic - <b>Western film</b> .                                                                                                                                                                                                                                                                              |                                               |
| #2703: when was the great fire in chicago                                                                                                                                                                                                                                                                                                                | <i>Great Chicago Fire</i>                     |
| The <b>Great Chicago Fire</b> was a conflagration that burned from Sunday, <b>October</b> 8, to early Tuesday, <b>October</b> 10, 1871, killing hundreds and destroying about in <b>Chicago</b> , Illinois.                                                                                                                                              |                                               |
| 2717: what is pci interface                                                                                                                                                                                                                                                                                                                              | <i>Conventional PCI</i>                       |
| <b>Conventional PCI (PCI)</b> is an initialization formed from Peripheral Component Interconnect, part of the <b>PCI Local Bus standard</b> and often shortened to just <b>PCI</b> is a local <b>computer</b> bus for attaching hardware devices in a <b>computer</b> .                                                                                  |                                               |
| 2718: what is jagger bombs                                                                                                                                                                                                                                                                                                                               | <i>Jägerbomb</i>                              |
| The <b>Jägerbomb</b> ( ) is a bomb shot cocktail that was originally mixed by dropping a shot of Jägermeister into a glass of beer and in recent years evolved by the Bagheri brothers (UK) with Red Bull or other energy drinks.                                                                                                                        |                                               |
| A long drink mixed with Jägermeister and Red Bull is called "JägerBull" as it is adopted from Jägermeister and RedBull.                                                                                                                                                                                                                                  |                                               |
| 2724: what is the name of mountains along califonia                                                                                                                                                                                                                                                                                                      | <i>California Coast Ranges</i>                |
| The other three coastal <b>California mountain</b> ranges are the Transverse Ranges, Peninsular Ranges and the Klamath <b>Mountains</b> .                                                                                                                                                                                                                |                                               |
| 2733: who is the author of tree grows in brooklyn                                                                                                                                                                                                                                                                                                        | <i>A Tree Grows in Brooklyn (novel)</i>       |
| A <b>Tree Grows in Brooklyn</b> is a 1943 <b>novel</b> written by Betty Smith.                                                                                                                                                                                                                                                                           |                                               |
| 2734: where is al Jazeera based                                                                                                                                                                                                                                                                                                                          | <i>Al Jazeera</i>                             |
| <b>Al Jazeera</b> ( , literally "The Island", abbreviating "The [Arabian] Peninsula " ), also known as Aljazeera and JSC ( <b>Jazeera Satellite</b> Channel), is a broadcaster owned by the privately held <b>Al Jazeera Media Network</b> and headquartered in Doha, Qatar.                                                                             |                                               |
| 2756: what is the location of coldwater ms                                                                                                                                                                                                                                                                                                               | <i>Coldwater, Mississippi</i>                 |
| <b>Coldwater</b> is a small town in Tate County, Mississippi.                                                                                                                                                                                                                                                                                            |                                               |
| 2757: what is the function of the hard palate                                                                                                                                                                                                                                                                                                            | <i>Hard palate</i>                            |
| The <b>hard palate</b> is a thin horizontal bony plate of the skull, located in the roof of the mouth.                                                                                                                                                                                                                                                   |                                               |
| Also on the anterior portion of the roof of the <b>hard palate</b> is the Rugae which are the irregular ridges in the mucous membrane that help facilitate the movement of food backwards towards the pharynx.                                                                                                                                           |                                               |
| 2761: where is Chayanne from?                                                                                                                                                                                                                                                                                                                            | <i>Chayanne</i>                               |
| Elmer Figueroa Arce (born June 28, 1968), best known under the stage name <b>Chayanne</b> , is a Puerto Rican Latin pop singer and actor.                                                                                                                                                                                                                |                                               |
| As a solo artist, <b>Chayanne</b> has released 21 solo albums and sold over 15 million albums worldwide.                                                                                                                                                                                                                                                 |                                               |
| 2768: what is eggnog made of                                                                                                                                                                                                                                                                                                                             | <i>Eggnog</i>                                 |
| <b>Eggnog</b> , or egg nog, is a sweetened dairy -based beverage traditionally <b>made</b> with milk and/or cream, sugar, and whipped eggs (which gives it a frothy texture).                                                                                                                                                                            |                                               |
| 2773: what is gravy made of                                                                                                                                                                                                                                                                                                                              | <i>Gravy</i>                                  |
| The <b>gravy</b> may be further colored and flavored with <b>gravy</b> salt (a simple mix of salt and caramel food coloring) or <b>gravy</b> browning ( <b>gravy</b> salt dissolved in water) or ready-made cubes and powders can be used as a substitute for natural meat or <b>vegetable</b> extracts.                                                 |                                               |
| 2786: what is cta used for                                                                                                                                                                                                                                                                                                                               | <i>Computed tomography angiography</i>        |
| Computed tomography angiography ( <b>CTA</b> ) is a computed tomography technique <b>used</b> to visualize arterial and venous vessels throughout the body.                                                                                                                                                                                              |                                               |
| 2795: what is vitamin b12 used for                                                                                                                                                                                                                                                                                                                       | <i>Vitamin B12</i>                            |
| <b>Vitamin B12</b> , <b>vitamin B12</b> or <b>vitamin</b> B-12, also <b>called</b> cobalamin, is a water-soluble <b>vitamin</b> with a key role in the normal functioning of the brain and nervous system, and for the formation of blood.                                                                                                               |                                               |
| 2797: What is the North American Free Trade Agreement?                                                                                                                                                                                                                                                                                                   | <i>North American Free Trade Agreement</i>    |
| The <b>North American Free Trade Agreement</b> (NAFTA) is an <b>agreement</b> signed by Canada, Mexico, and the United States, creating a trilateral <b>trade bloc</b> in <b>North America</b> .                                                                                                                                                         |                                               |
| 2798: what is tmz stand for                                                                                                                                                                                                                                                                                                                              | <i>TMZ (website)</i>                          |
| The name <b>TMZ stands</b> for the historic " studio zone " or 30-mile zone radius from the intersection of West Beverly Boulevard and North La Cienega Boulevard in Los Angeles.                                                                                                                                                                        |                                               |
| 2800: what is impingement of the shoulder                                                                                                                                                                                                                                                                                                                | <i>Impingement syndrome</i>                   |
| <b>Shoulder impingement</b> syndrome, also called painful arc syndrome, supraspinatus syndrome, swimmer's <b>shoulder</b> , and thrower's <b>shoulder</b> , is a clinical syndrome which occurs when the tendons of the rotator cuff muscles become irritated and inflamed as they pass through the subacromial space, the passage beneath the acromion. |                                               |
| 2818: who was the first one to invent medicine                                                                                                                                                                                                                                                                                                           | <i>History of medicine</i>                    |
| The ancient Egyptians had a system of <b>medicine</b> that was very advanced for its time and influenced <b>later</b> medical <b>traditions</b> .                                                                                                                                                                                                        |                                               |
| 2822: Who was Daniel J Daly?                                                                                                                                                                                                                                                                                                                             | <i>Daniel Daly</i>                            |
| Sergeant Major <b>Daniel</b> Joseph "Dan" <b>Daly</b> (November 11, 1873 – April 27, 1937) was a United States Marine and one of only nineteen men (including seven Marines) to have received the Medal of Honor twice.                                                                                                                                  |                                               |
| 2829: what is the plot of the shawshank redemption?                                                                                                                                                                                                                                                                                                      | <i>The Shawshank Redemption</i>               |
| Adapted from the Stephen <b>King</b> novella Rita Hayworth and <b>Shawshank Redemption</b> , the film tells the story of Andy Dufresne, a banker who spends nearly two decades in <b>Shawshank</b> State Prison for the murder of his wife and her lover <b>despite</b> his claims of innocence.                                                         |                                               |
| 2830: what is an information technology manager                                                                                                                                                                                                                                                                                                          | <i>Information technology management</i>      |
| Managing this responsibility within a company entails many of the basic management functions, like budgeting, staffing, and organizing and controlling, along with other aspects that are unique to <b>technology</b> , like change management, software design, network planning, tech support etc.                                                     |                                               |
| IT management is the discipline whereby all of the <b>technology</b> resources of a firm are managed in accordance with its needs and priorities.                                                                                                                                                                                                        |                                               |
| 2832: what is the scientific name of a cardinal bird                                                                                                                                                                                                                                                                                                     | <i>Northern Cardinal</i>                      |
| The Northern <b>Cardinal (Cardinalis cardinalis)</b> is a North American <b>bird</b> in the genus <b>Cardinalis</b> ; it is also known colloquially as the redbird or common <b>cardinal</b> .                                                                                                                                                           |                                               |
| 2838: where are kenworth trucks built                                                                                                                                                                                                                                                                                                                    | <i>Kenworth</i>                               |
| <b>Kenworth</b> is an American manufacturer of medium and heavy-duty Class 8 <b>trucks</b> based in Kirkland, <b>Washington, United States</b> , a suburb of Seattle, <b>Washington</b> .                                                                                                                                                                |                                               |
| #2844: when is the feast of St. Rita                                                                                                                                                                                                                                                                                                                     | <i>Rita of Cascia</i>                         |
| The Roman Catholic <b>Church</b> , under the pontificate of Pope Leo XIII officially <b>canonized</b> <b>Rita</b> on May 24, 1900, while her <b>feast day</b> is celebrated every May 22.                                                                                                                                                                |                                               |
| 2846: where is j cole from                                                                                                                                                                                                                                                                                                                               | <i>J. Cole</i>                                |
| Jermaine Lamar <b>Cole</b> (born January 28, 1985), better known by his stage name <b>J. Cole</b> , is an American hip-hop recording artist and record producer from Fayetteville, North Carolina.                                                                                                                                                       |                                               |
| 2856: what is the gdp for greenland 2010?                                                                                                                                                                                                                                                                                                                | <i>Economy of Greenland</i>                   |
| <b>GDP</b> per capita is similar to the average European economies but the economy is critically dependent upon substantial support from the Danish government, which supplies about half the revenues of the home rule government who in turn employ about 8,000 <b>Greenlanders</b> out of a labor force of 40,156 (Jan. 2012).                        |                                               |
| 2857: What is hydrogen in                                                                                                                                                                                                                                                                                                                                | <i>Hydrogen</i>                               |
| Most of the <b>hydrogen</b> on Earth is in molecules such as water and organic compounds because <b>hydrogen</b> readily forms covalent compounds with most non-metallic elements.                                                                                                                                                                       |                                               |
| In 1766–81, Henry Cavendish was the first to recognize that <b>hydrogen</b> gas was a discrete substance, and that it produces water when burned, a property which later gave it its name: in Greek, <b>hydrogen</b> means "water-former".                                                                                                               |                                               |
| 2858: where is UWA on world list of universities                                                                                                                                                                                                                                                                                                         | <i>University of Western Australia</i>        |
| One of <b>Australia's</b> best and most prestigious <b>universities</b> , <b>UWA</b> is highly ranked <b>internationally</b> in various <b>publications</b> ; the 2011 QS <b>World University</b> Rankings <b>placed UWA</b> at 73rd <b>internationally</b> .                                                                                            |                                               |
| #2878: when was purple haze by jimi hendrix made?                                                                                                                                                                                                                                                                                                        | <i>Purple haze</i>                            |
| " <b>Purple Haze</b> " is a song written and <b>recorded</b> by <b>Jimi Hendrix</b> in 1967, released as the second single by The <b>Jimi Hendrix</b> Experience in both the United Kingdom and the United States.                                                                                                                                       |                                               |
| 2880: where was martin luther born                                                                                                                                                                                                                                                                                                                       | <i>Martin Luther</i>                          |
| <b>Martin Luther</b> ( ; 10 November 1483 – 18 <b>February</b> 1546) was a German monk, former Catholic priest, <b>professor</b> of theology and seminal figure of a reform movement in sixteenth century Christianity, <b>subsequently</b> known as the <b>Protestant</b> Reformation.                                                                  |                                               |
| 2891: what is the mortality rate of sepsis                                                                                                                                                                                                                                                                                                               | <i>Septic shock</i>                           |
| The <b>mortality rate</b> from <b>septic</b> shock is approximately 25–50%.                                                                                                                                                                                                                                                                              |                                               |
| 2893: where is kos from?                                                                                                                                                                                                                                                                                                                                 | <i>K-os</i>                                   |
| The alias " <b>k-os</b> ", spelled with a lower case "k", was intended to be less aggressive than the pseudonyms of other rappers whose names were all upper case, such as KRS-One.                                                                                                                                                                      |                                               |
| <b>k-os</b> usually performs with a live band, something that is uncommon in the hip hop genre.                                                                                                                                                                                                                                                          |                                               |
| <b>k-os</b> received his first musical exposure with the single "Musical Essence", released in 1993.                                                                                                                                                                                                                                                     |                                               |
| Kevin Brereton (born February 20, 1972), better known by his stage name <b>k-os</b> (; "chaos"), is a Canadian rapper, singer, songwriter and record producer.                                                                                                                                                                                           |                                               |
| It is an acronym for " Knowledge of Self," although in a later interview he said that it originally stood for "Kevin's Original Sound." <b>k-os'</b> music incorporates a wide variety of music genres, including rap, funk, rock, and reggae.                                                                                                           |                                               |
| A musician as well as a producer, <b>k-os</b> has written and produced nearly every part of all four of his albums.                                                                                                                                                                                                                                      |                                               |
| 2904: what is the sign called?                                                                                                                                                                                                                                                                                                                           | <i>At sign</i>                                |
| The <b>at sign</b> is also commonly <b>called</b> the at symbol, ampersat, apetail or commercial at in <b>English</b> —and less <b>commonly</b> a wide range of other terms.                                                                                                                                                                             |                                               |
| 2905: who is the book the catcher in the rye by?                                                                                                                                                                                                                                                                                                         | <i>The Catcher in the Rye</i>                 |
| The <b>Catcher in the Rye</b> is a 1951 novel by J. D. <b>Salinger</b> .                                                                                                                                                                                                                                                                                 |                                               |
| 2910: what is prince williams last name                                                                                                                                                                                                                                                                                                                  | <i>Prince William, Duke of Cambridge</i>      |
| <b>Prince William, Duke of Cambridge</b> ( <b>William</b> Arthur Philip Louis; <b>born</b> 21 June 1982), is the elder son of Charles, <b>Prince</b> of Wales, and Diana, <b>Princess</b> of Wales, and third-eldest grandchild of <b>Queen Elizabeth II</b> and <b>Prince</b> Philip, <b>Duke</b> of Edinburgh.                                         |                                               |
| 2914: what is IBRIX                                                                                                                                                                                                                                                                                                                                      | <i>IBRIX Fusion</i>                           |
| The software was produced, sold, and supported by <b>IBRIX</b> Incorporated of Billerica, Massachusetts.                                                                                                                                                                                                                                                 |                                               |
| Subsequent to the acquisition, the software components of <b>IBRIX</b> have been combined with ProLiant servers to form the X9000 series of storage systems.                                                                                                                                                                                             |                                               |
| <b>IBRIX</b> Fusion is a scalable parallel file system combined with integrated logical volume manager, availability features and a management interface.                                                                                                                                                                                                |                                               |
| HP announced on July 17, 2009 that it had reached a definitive agreement to acquire <b>IBRIX</b> .                                                                                                                                                                                                                                                       |                                               |
| 2915: what is bilirubin total                                                                                                                                                                                                                                                                                                                            | <i>Bilirubin</i>                              |
| <b>Bilirubin</b> is excreted in bile and urine, and elevated levels may indicate certain diseases.                                                                                                                                                                                                                                                       |                                               |
| <b>Bilirubin</b> (formerly referred to as hematinidin) is the yellow breakdown product of normal heme catabolism.                                                                                                                                                                                                                                        |                                               |
| 2918: what is quasi judicial agency                                                                                                                                                                                                                                                                                                                      | <i>Quasi-judicial body</i>                    |

A quasi-judicial body is an entity such as an arbitrator or tribunal board, generally of a public administrative **agency**, which has powers and procedures resembling those of a court of law or judge, and which is obligated to objectively determine facts and draw conclusions from them so as to provide the basis of an official action.

|                                                                   |                                           |
|-------------------------------------------------------------------|-------------------------------------------|
| 2924: who is the founder of twitter                               | <i>Twitter</i>                            |
| 2925: what is the name of the wizard of oz                        | <i>Wizard of Oz (character)</i>           |
| 2932: what is bj's wholesale club                                 | <i>BJ's Wholesale Club</i>                |
| 2936: what is the name of the wizard of oz                        | <i>Wizard of Oz (character)</i>           |
| 2940: what is homebrew for wii                                    | <i>Wii homebrew</i>                       |
| 2952: what is korean money called                                 | <i>South Korean won</i>                   |
| 2955: what is three phase electrical                              | <i>Three-phase electric power</i>         |
| 2957: what is the significance of Good Friday?                    | <i>Good Friday</i>                        |
| 2959: where is the great basin located on a us map                | <i>Great Basin</i>                        |
| 2966: what was the date of pearl harbor                           | <i>Attack on Pearl Harbor</i>             |
| 2969: what is disney's magic kingdom                              | <i>Magic Kingdom</i>                      |
| 2972: what is the kanji for language                              | <i>Kanji</i>                              |
| 2973: what is in fruitcake                                        | <i>Fruit cake</i>                         |
| 2978: who was the congressman who was caught with an escort in ny | <i>Eliot Spitzer prostitution scandal</i> |

On March 10, 2008, The New York Times reported that New York Governor Eliot Spitzer had patronized an elite **escort** service run by Emperors Club VIP.

|                                                                  |                                                          |
|------------------------------------------------------------------|----------------------------------------------------------|
| 2982: what is lockton affinity                                   | <i>Lockton Companies</i>                                 |
| 2991: what is the name of chris cornell's band?                  | <i>Chris Cornell</i>                                     |
| 2994: what is preciosa crystal?                                  | <i>Preciosa (corporation)</i>                            |
| 2998: where is the chupacabra found                              | <i>Chupacabra</i>                                        |
| 2999: what is the purpose of North American Free Trade Agreement | <i>North American Free Trade Agreement</i>               |
| 3004: what are all of the jonas brothers                         | <i>Jonas Brothers</i>                                    |
| 3012: what is the brisket from                                   | <i>Brisket</i>                                           |
| 3021: what is busiest airport in US                              | <i>List of the busiest airports in the United States</i> |
| 3027: where is osaka japan                                       | <i>Osaka</i>                                             |
| 3030: what is surname and given name                             | <i>Given name</i>                                        |
| 3037: What is an economic feature?                               | <i>Economics</i>                                         |
| 3043: what is section eight housing                              | <i>Section 8 (housing)</i>                               |

**Example 4.15.4.** In Table S12 below, we list the questions where our top-scoring answers have all been officially labeled as incorrect by the WikiQA team, including 167 “quantitative” questions, out of 662 total. It should be noted that some questions in this table are simply too tricky to be handled by literal interpretations. For example, our top-scoring answer to Q1838 differs from the official one (shown in blue):

1838: who sang cool jerk *Cool Jerk*  
 In the feature film Home Alone 2: Lost in New York, Uncle Frank ( Gerry Bamman ) **sings “Cool Jerk”** in the shower. “Cool Jerk” is a popular song written by Donald Storbball and originally performed by The Capitols.

Since our algorithm fails to reinterpret “who sang” as “who originally performed”, our answer is outshone by the official correct answer. Doubtlessly, this particular entry in Table S12 illustrates the limitations of our automated question comprehension.

**Example 4.15.5.** It is still arguable whether dozens of entries in Table S12 represent miscarriage of justice by the WikiQA team. In the cases selected below, we believe that our top-scoring answers are not any worse than the official ones (painted in blue):

#129: how many stripes on the flag *Flag of the United States*  
 The national **flag** of the United States of America, often simply referred to as the American **flag**, consists of **thirteen** equal horizontal **stripes** of **red (top) and bottom) alternating with white**, with a **blue** rectangle in the canton (referred to specifically as the “union”) bearing fifty small, **white, five-pointed stars** arranged in nine offset horizontal rows of **six stars (top and bottom) alternating with rows of five stars**.

The 50 stars on the flag represent the 50 states of the United States of America and the 13 stripes represent the thirteen British colonies that declared independence from the Kingdom of Great Britain and became the first states in the Union.

214: what does salesforce.com do? *Salesforce.com*  
**Salesforce.com** Inc. is a global enterprise software company **headquartered** in San Francisco, California. **Though best known for its customer relationship management (CRM) product, Salesforce has also expanded into the “social enterprise arena” through acquisitions.**

#557: how many spanish speaking people are there in the us *Spanish language in the United States*  
 There are 45 million Hispanophones who **speak Spanish** as a first or second **language**, as well as six million **Spanish language** students, composing the **largest** national Spanish-speaking community outside of **Mexico** and making **Spanish** the Romance **language** and the Indo-European **language** with **largest** number of **native speakers** in the world. According to the 2010 American Community Survey conducted by the U.S. Census Bureau, Spanish is the primary language spoken at home by almost 37 million people aged five or older, a figure more than double that of 1990.

1831: where do you find iodine *Iodine*  
 Because of this function, radioisotopes of **iodine** are concentrated in the thyroid gland along with nonradioactive **iodine**. **Iodine is found on Earth mainly as the highly water-soluble iodide ion, I<sup>-</sup>, which concentrates it in oceans and brine pools.**

2463: who is E from entourage *Eric Murphy*  
 Murphy is a fictional **character** on the comedy-drama television series **Entourage**. **Eric “E.”**

2532: what is the official language of america? *Languages of the United States*  
 The situation is quite varied at the state and territorial levels, with some states mirroring the federal policy of **adopting no official language** in a **de jure** capacity, others **adopting English** alone, others **officially adopting English** as well as local **languages**, and still others **adopting** a policy of **de facto** bilingualism. **The most commonly used language is English.**

2841: what is the type of democracy in which all citizens have the right to make government decisions *Democracy*  
 One **form** of **democracy** is **direct democracy**, in which all eligible **citizens** have **direct** and **active** participation in the **decision making** of the **government**. **Democracy is a form of government in which all eligible citizens have an equal say in the decisions that affect their lives.**

In particular, the penultimate official answer listed above (accompanying Q2532) is logically irrelevant,<sup>48</sup> if not factually misleading; the last official answer listed above (accompanying Q2841) does not even address the “type of democracy” in the question (*i.e.* direct, representative *etc.*) at all. Despite our disagreement over certain judgements made by the WikiQA team, we are not going to alter their official labels for correct/incorrect answers, so as to ensure a fair comparison in [1, Fig. 7b] and Fig. S2.

Table S12. List of WikiQA misses

|                                                                                                                                                                                                                                                                                                                                                                                                                                                                                                                                                                        |                                                                       |
|------------------------------------------------------------------------------------------------------------------------------------------------------------------------------------------------------------------------------------------------------------------------------------------------------------------------------------------------------------------------------------------------------------------------------------------------------------------------------------------------------------------------------------------------------------------------|-----------------------------------------------------------------------|
| 4: how a water pump works                                                                                                                                                                                                                                                                                                                                                                                                                                                                                                                                              | Pump                                                                  |
| 4: how a water pump works                                                                                                                                                                                                                                                                                                                                                                                                                                                                                                                                              | Pump                                                                  |
| <b>Pumps</b> can be classified into three major groups according to the method they use to move the fluid: direct lift, displacement, and gravity pumps.                                                                                                                                                                                                                                                                                                                                                                                                               |                                                                       |
| #11: how big is bmc software in houston, tx                                                                                                                                                                                                                                                                                                                                                                                                                                                                                                                            | BMC Software                                                          |
| Headquartered in <b>Houston</b> , Texas, <b>BMC</b> develops, markets and sells <b>software</b> used for multiple functions, including IT service management, data center <b>automation</b> , <b>performance</b> management, virtualization lifecycle management and cloud computing management.                                                                                                                                                                                                                                                                       |                                                                       |
| #17: how much are the harry potter movies worth                                                                                                                                                                                                                                                                                                                                                                                                                                                                                                                        | Harry Potter                                                          |
| Also due to the <b>success</b> of the books and films, <b>Harry Potter</b> has been used for a theme <b>park</b> , the <b>Wizarding World of Harry Potter</b> in <b>Universal Parks &amp; Resorts</b> 's Islands of Adventure.                                                                                                                                                                                                                                                                                                                                         |                                                                       |
| #20: how old was sue lyon when she made lolita                                                                                                                                                                                                                                                                                                                                                                                                                                                                                                                         | Lolita (1962 film)                                                    |
| The film stars <b>James Mason</b> as Humbert Humbert, <b>Sue Lyon</b> as Dolores Haze ( <b>Lolita</b> ) and Shelley Winters as Charlotte Haze with Peter Sellers as Clare Quilty.                                                                                                                                                                                                                                                                                                                                                                                      |                                                                       |
| 21: how are cholera and typhus transmitted and prevented                                                                                                                                                                                                                                                                                                                                                                                                                                                                                                               | Cholera                                                               |
| <b>Cholera</b> is an infection in the small intestine caused by the bacterium <i>Vibrio cholerae</i> .                                                                                                                                                                                                                                                                                                                                                                                                                                                                 |                                                                       |
| 28: how are aircraft radial engines built                                                                                                                                                                                                                                                                                                                                                                                                                                                                                                                              | Radial engine                                                         |
| The <b>radial</b> configuration was very commonly used in <b>aircraft engines</b> before turbine <b>engines</b> became predominant.                                                                                                                                                                                                                                                                                                                                                                                                                                    |                                                                       |
| #30: how deep can be drill for deep underwater                                                                                                                                                                                                                                                                                                                                                                                                                                                                                                                         | Deepwater drilling                                                    |
| There are basically two kinds of mobile <b>deepwater drilling</b> rigs: semi-submersible <b>drilling</b> rigs and <b>drillships</b> .                                                                                                                                                                                                                                                                                                                                                                                                                                  |                                                                       |
| #32: how long was frank sinatra famous                                                                                                                                                                                                                                                                                                                                                                                                                                                                                                                                 | Frank Sinatra                                                         |
| <b>Sinatra</b> left Capitol to found his own record label, Reprise Records in 1961 (finding success with albums such as Ring-a-Ding-Ding!, <b>Sinatra</b> at the Sands and <b>Francis Albert Sinatra &amp; Antonio Carlos Jobim</b> ), toured internationally, was a founding member of the Rat Pack and fraternized with celebrities and statesmen, including John F. <b>Kennedy</b> .                                                                                                                                                                                |                                                                       |
| #42: how much is jk rowling worth                                                                                                                                                                                                                                                                                                                                                                                                                                                                                                                                      | J. K. Rowling                                                         |
| Joanne "Jo" <b>Rowling</b> ( <span></span> , (born 31 July 1965), pen name <b>J. K. Rowling</b> , is a British novelist, best known as the author of the <b>Harry Potter</b> fantasy <b>series</b> .                                                                                                                                                                                                                                                                                                                                                                   |                                                                       |
| #43: how big is auburndale florida                                                                                                                                                                                                                                                                                                                                                                                                                                                                                                                                     | Auburndale, Florida                                                   |
| <b>Auburndale</b> is a city in Polk County, <b>Florida</b> , United States.                                                                                                                                                                                                                                                                                                                                                                                                                                                                                            |                                                                       |
| #46: how old is the singer bob seger                                                                                                                                                                                                                                                                                                                                                                                                                                                                                                                                   | Bob Seger                                                             |
| As a locally successful Detroit-area artist, he performed and recorded as <b>Bob Seger</b> and the Last Heard and <b>Bob Seger</b> System throughout the 1960s.                                                                                                                                                                                                                                                                                                                                                                                                        |                                                                       |
| #48: how long was i love lucy on the air                                                                                                                                                                                                                                                                                                                                                                                                                                                                                                                               | I Love Lucy                                                           |
| <b>I Love Lucy</b> is an American <b>television sitcom</b> starring Lucille Ball, Desi Arnaz, Vivian Vance, and William <b>Frawley</b> .                                                                                                                                                                                                                                                                                                                                                                                                                               |                                                                       |
| #59: HOW MUCH IS CENTAVOS IN MEXICO                                                                                                                                                                                                                                                                                                                                                                                                                                                                                                                                    | Mexican peso                                                          |
| The name was originally used in reference to <b>peso oro</b> (gold weights) or <b>peso plata</b> (silver weights).                                                                                                                                                                                                                                                                                                                                                                                                                                                     |                                                                       |
| 66: how did armando christian perez become famous                                                                                                                                                                                                                                                                                                                                                                                                                                                                                                                      | Pitbull (entertainer)                                                 |
| In 2004, he released his debut album titled M.I.A.M.I. (short for Money Is A Major Issue) underTVT Records.                                                                                                                                                                                                                                                                                                                                                                                                                                                            |                                                                       |
| #75: how old were the twin towers when destroyed                                                                                                                                                                                                                                                                                                                                                                                                                                                                                                                       | World Trade Center                                                    |
| At the time of their completion, the original 1 World Trade Center (the North <b>Tower</b> ) and 2 World Trade Center (the South Tower), known collectively as the " <b>Twin Towers</b> ", were the <b>tallest buildings</b> in the world.                                                                                                                                                                                                                                                                                                                             |                                                                       |
| #89: how many presidents of the us                                                                                                                                                                                                                                                                                                                                                                                                                                                                                                                                     | List of Presidents of the United States                               |
| Upon the death, resignation, or removal from <b>office</b> of an incumbent <b>President</b> , the Vice <b>President</b> assumes the <b>office</b> .                                                                                                                                                                                                                                                                                                                                                                                                                    |                                                                       |
| #100: what happens to the light independent reactions of photosynthesis?                                                                                                                                                                                                                                                                                                                                                                                                                                                                                               | Light-independent reactions                                           |
| This <b>process happens</b> when <b>light</b> is available <b>independent</b> of the kind of <b>photosynthesis</b> (C3 carbon fixation, C4 carbon fixation, and Crassulacean Acid Metabolism); CAM plants store malic acid in their vacuoles every night and release it by day in order to make this <b>process</b> work.                                                                                                                                                                                                                                              |                                                                       |
| 107: what countries are under the buddhism religion                                                                                                                                                                                                                                                                                                                                                                                                                                                                                                                    | Buddhism by country                                                   |
| Government policies in these <b>countries</b> may encourage the under-reporting or non-reporting of <b>religious</b> adherence, resulting in official totals that may drastically underestimate the number of <b>religious</b> practitioners in these <b>countries</b> .                                                                                                                                                                                                                                                                                               |                                                                       |
| 108: how did wild bill's father die                                                                                                                                                                                                                                                                                                                                                                                                                                                                                                                                    | Wild Bill Hickok                                                      |
| James Butler Hickok (May 27, 1837 – August 2, 1876), better known as <b>Wild Bill</b> Hickok, was a folk hero of the American Old West.                                                                                                                                                                                                                                                                                                                                                                                                                                |                                                                       |
| #109: how many land rovers have landed on mars                                                                                                                                                                                                                                                                                                                                                                                                                                                                                                                         | Mars rover                                                            |
| It currently manages the <b>Mars</b> Exploration <b>Rover</b> mission's active Opportunity <b>rover</b> and inactive Spirit, and, as part of the <b>Mars</b> Science Laboratory mission, the Curiosity <b>rover</b> .                                                                                                                                                                                                                                                                                                                                                  |                                                                       |
| 112: what bird family is the owl                                                                                                                                                                                                                                                                                                                                                                                                                                                                                                                                       | Owl                                                                   |
| <b>Owls</b> hunt mostly small mammals, insects, and other <b>birds</b> , although a few species specialize in <b>hunting</b> fish.                                                                                                                                                                                                                                                                                                                                                                                                                                     |                                                                       |
| 113: how did harmon killebrew get strong                                                                                                                                                                                                                                                                                                                                                                                                                                                                                                                               | Harmon Killebrew                                                      |
| <b>Harmon Clayton Killebrew</b> (; June 29, 1936 – May 17, 2011), nicknamed " <b>Killer</b> " and "Hammerin' <b>Harmon</b> ", was an American professional baseball first baseman, third baseman, and left fielder.                                                                                                                                                                                                                                                                                                                                                    |                                                                       |
| 116: What did the augurs use to interpret the will of the gods?                                                                                                                                                                                                                                                                                                                                                                                                                                                                                                        | Augur                                                                 |
| An <b>augur</b> holding a lituus, the curved wand often <b>used</b> as a symbol of <b>augury</b> on Roman coins                                                                                                                                                                                                                                                                                                                                                                                                                                                        |                                                                       |
| #117: How much did Waterboy grossed                                                                                                                                                                                                                                                                                                                                                                                                                                                                                                                                    | The Waterboy                                                          |
| The <b>Waterboy</b> is a 1998 American sports/comedy film directed by Frank Coraci (who played Robert 'Robert' Boucher, Sr.), starring Adam <b>Sandler</b> , Kathy Bates, Fairuza Balk, Henry Winkler, Jerry Reed, Larry Gilliard, Jr., Blake Clark, Peter Dante and Jonathan Loughran, and produced by Robert Simonds and Jack Giarraputo.                                                                                                                                                                                                                            |                                                                       |
| 118: What country is Farmington Hills, MI in?                                                                                                                                                                                                                                                                                                                                                                                                                                                                                                                          | Farmington Hills, Michigan                                            |
| Although the two cities have separate services and addresses, <b>Farmington</b> and <b>Farmington Hills</b> are often thought of as the same community.                                                                                                                                                                                                                                                                                                                                                                                                                |                                                                       |
| 121: what does a groundhog look for on groundhog day                                                                                                                                                                                                                                                                                                                                                                                                                                                                                                                   | Groundhog Day                                                         |
| <b>Groundhog Day</b> , already a widely recognized and popular tradition, received widespread attention as a result of the 1993 film <b>Groundhog Day</b> , which was set in Punxsutawney, PA (though filmed primarily in Woodstock, IL) and portrayed Punxsutawney Phil.                                                                                                                                                                                                                                                                                              |                                                                       |
| #129: how many stripes on the flag                                                                                                                                                                                                                                                                                                                                                                                                                                                                                                                                     | Flag of the United States                                             |
| The national <b>flag</b> of the United States of America, often simply referred to as the American <b>flag</b> , consists of <b>thirteen</b> equal horizontal <b>stripes</b> of <b>red</b> ( <b>top</b> and <b>bottom</b> ) <b>alternating</b> with <b>white</b> , with a <b>blue</b> rectangle in the canton (referred to specifically as the "union") bearing fifty small, <b>white</b> , <b>five-pointed stars</b> arranged in nine offset horizontal rows of <b>six stars</b> ( <b>top</b> and <b>bottom</b> ) <b>alternating</b> with rows of <b>five stars</b> . |                                                                       |
| 132: how is whooping cough distinguished from similar diseases                                                                                                                                                                                                                                                                                                                                                                                                                                                                                                         | Pertussis                                                             |
| In some countries, this <b>disease</b> is called the 100 days' <b>cough</b> or <b>cough</b> of 100 days.                                                                                                                                                                                                                                                                                                                                                                                                                                                               |                                                                       |
| 136: what county is galveston in texas                                                                                                                                                                                                                                                                                                                                                                                                                                                                                                                                 | Galveston County, Texas                                               |
| League City is the largest city in <b>Galveston County</b> in terms of population; URL_http between 2000 and 2005 it surpassed <b>Galveston</b> as the <b>county's</b> largest city.                                                                                                                                                                                                                                                                                                                                                                                   |                                                                       |
| 137: what cities are in the bahamas                                                                                                                                                                                                                                                                                                                                                                                                                                                                                                                                    | List of cities in the Bahamas                                         |
| This is a list of <b>cities</b> in the <b>Bahamas</b> .                                                                                                                                                                                                                                                                                                                                                                                                                                                                                                                |                                                                       |
| #139: how many schools are in the big ten                                                                                                                                                                                                                                                                                                                                                                                                                                                                                                                              | Big Ten Conference                                                    |
| The <b>Big Ten Conference</b> , formerly Western <b>Conference</b> and <b>Big Nine Conference</b> , is the oldest <b>Division I</b> college athletic conference in the United States.                                                                                                                                                                                                                                                                                                                                                                                  |                                                                       |
| 141: what composer used sound mass                                                                                                                                                                                                                                                                                                                                                                                                                                                                                                                                     | Sound mass                                                            |
| In contrast to more traditional musical textures, <b>sound mass composition</b> "minimizes the importance of individual pitches in preference for texture, timbre, and dynamics as primary shapers of gesture and impact."                                                                                                                                                                                                                                                                                                                                             |                                                                       |
| 144: How Do You Play Spades                                                                                                                                                                                                                                                                                                                                                                                                                                                                                                                                            | Spades                                                                |
| Its major difference as compared to other <b>Whist</b> variants is that, instead of <b>trump</b> being decided by the <b>highest</b> bidder or at random, the <b>Spade suit</b> is always <b>trump</b> , hence the name.                                                                                                                                                                                                                                                                                                                                               |                                                                       |
| 145: what continent is australia                                                                                                                                                                                                                                                                                                                                                                                                                                                                                                                                       | Australia (continent)                                                 |
| The <b>continent</b> of <b>Australia</b> lies on a continental shelf overlain by shallow seas which divide it into several landmasses — the Arafura Sea and Torres Strait between <b>mainland Australia</b> and New Guinea, and Bass Strait between <b>mainland Australia</b> and Tasmania.                                                                                                                                                                                                                                                                            |                                                                       |
| 146: what causes heart disease                                                                                                                                                                                                                                                                                                                                                                                                                                                                                                                                         | Cardiovascular disease                                                |
| Cardiovascular <b>disease</b> refers to any <b>disease</b> that affects the cardiovascular system, principally <b>cardiac disease</b> , vascular <b>diseases</b> of the brain and kidney, and peripheral <b>arterial disease</b> .                                                                                                                                                                                                                                                                                                                                     |                                                                       |
| 147: what countries did immigrants come from during the immigration                                                                                                                                                                                                                                                                                                                                                                                                                                                                                                    | History of immigration to the United States                           |
| During the nation's history, the growing <b>country</b> experienced successive waves of <b>immigration</b> which rose and fell over time, particularly from Europe, with the cost of transoceanic transportation sometimes paid by travelers becoming indentured servants after their arrival in the New World.                                                                                                                                                                                                                                                        |                                                                       |
| #150: how many people live in atlanta georgia                                                                                                                                                                                                                                                                                                                                                                                                                                                                                                                          | Atlanta                                                               |
| <b>Atlanta</b> is the primary transportation hub of the Southeastern United States, via highway, railroad, and air, with Hartsfield–Jackson <b>Atlanta</b> International Airport being the world's <b>busiest</b> airport since 1998.                                                                                                                                                                                                                                                                                                                                  |                                                                       |
| 159: what does it mean to be a commonwealth state                                                                                                                                                                                                                                                                                                                                                                                                                                                                                                                      | Commonwealth                                                          |
| Most notably, the <b>Commonwealth</b> of Nations, an association primarily of former members of the British Empire, is often referred to as simply "the <b>Commonwealth</b> ".                                                                                                                                                                                                                                                                                                                                                                                         |                                                                       |
| #163: how long can you be in the supreme court                                                                                                                                                                                                                                                                                                                                                                                                                                                                                                                         | Supreme Court of the United States                                    |
| It has ultimate (and largely discretionary) appellate <b>jurisdiction</b> over all <b>federal courts</b> and over <b>state court cases</b> involving issues of <b>federal law</b> , and original <b>jurisdiction</b> over a small range of <b>cases</b> .                                                                                                                                                                                                                                                                                                              |                                                                       |
| 165: what can sql 2005 do                                                                                                                                                                                                                                                                                                                                                                                                                                                                                                                                              | Microsoft SQL Server                                                  |
| There are at least a dozen different <b>editions</b> of <b>Microsoft SQL</b> Server aimed at different audiences and for different workloads (ranging from small applications that store and retrieve <b>data</b> on the same computer, to millions of users and computers that access huge amounts of <b>data</b> from the Internet at the same time).                                                                                                                                                                                                                |                                                                       |
| #167: how many people were killed in the oklahoma city bombing                                                                                                                                                                                                                                                                                                                                                                                                                                                                                                         | Oklahoma City bombing                                                 |
| The <b>Oklahoma City bombing</b> was a domestic terrorist <b>bomb</b> attack on the Alfred P. Murrah <b>Federal Building</b> in downtown <b>Oklahoma City</b> on April 19, 1995.                                                                                                                                                                                                                                                                                                                                                                                       |                                                                       |
| 172: What group took home the award for best rock album at the Australian Recording Industry Association (ARIA) Music Awards?                                                                                                                                                                                                                                                                                                                                                                                                                                          | ARIA Music Awards                                                     |
| The <b>Australian Recording Industry Association Music Awards</b> (commonly known as <b>ARIA Music Awards</b> or <b>ARIA Awards</b> ) is an annual series of awards nights celebrating the <b>Australian music industry</b> , put on by the <b>Australian Recording Industry Association</b> (ARIA).                                                                                                                                                                                                                                                                   |                                                                       |
| 180: what did benedict arnold die                                                                                                                                                                                                                                                                                                                                                                                                                                                                                                                                      | Benedict arnold                                                       |
| In the winter of 1782, <b>Arnold</b> moved to London with his second wife, <b>Margaret "Peggy" Shippen Arnold</b> .                                                                                                                                                                                                                                                                                                                                                                                                                                                    |                                                                       |
| #185: how many ports are there in networking                                                                                                                                                                                                                                                                                                                                                                                                                                                                                                                           | Port (computer networking)                                            |
| In the client-server model of application architecture, <b>ports</b> are used to provide a multiplexing service on each server-side <b>port</b> number that <b>network</b> clients connect to for service initiation, after which communication can be reestablished on other connection-specific <b>port</b> numbers.                                                                                                                                                                                                                                                 |                                                                       |
| 195: how is canada's health care                                                                                                                                                                                                                                                                                                                                                                                                                                                                                                                                       | Comparison of the health care systems in Canada and the United States |
| Total <b>government spending</b> per capita in the U.S. on <b>health care</b> was 23% <b>higher</b> than <b>Canadian government spending</b> , and U.S. <b>government expenditure</b> on <b>health care</b> was just under 83% of total <b>Canadian spending</b> (public and private) though these statistics don't take into account population <b>differences</b> .                                                                                                                                                                                                  |                                                                       |
| #197: how many xbox 360 games are there                                                                                                                                                                                                                                                                                                                                                                                                                                                                                                                                | List of Xbox 360 games                                                |
| For a list of downloadable <b>Xbox Live Arcade games</b> , see the List of <b>Xbox Live Arcade games</b> .                                                                                                                                                                                                                                                                                                                                                                                                                                                             |                                                                       |
| 207: what country did wine originate in                                                                                                                                                                                                                                                                                                                                                                                                                                                                                                                                | History of wine                                                       |
| Following the decline of Rome and its industrial-scale <b>wine</b> production for <b>export</b> , the Christian Church in medieval Europe also became a firm supporter of <b>wine</b> , necessary for celebration of the Catholic Mass. Whereas <b>wine</b> was forbidden in medieval Islamic cultures, its use in Christian libation was widely tolerated.                                                                                                                                                                                                            |                                                                       |
| #208: how many district are in west bengal                                                                                                                                                                                                                                                                                                                                                                                                                                                                                                                             | List of districts of West Bengal                                      |
| Geographically, <b>West Bengal</b> is divided into a variety of <b>regions</b> —Darjeeling Himalayan hill <b>region</b> , Terai and Doers <b>region</b> , North <b>Bengal plains</b> , Rarh <b>region</b> , <b>Western</b> plateau and high lands, coastal <b>plains</b> , Sunderbans and the Ganges Delta.                                                                                                                                                                                                                                                            |                                                                       |
| #210: how many towns in new hampshire                                                                                                                                                                                                                                                                                                                                                                                                                                                                                                                                  | List of cities and towns in New Hampshire                             |
| However, <b>towns</b> currently are able to change their form of government by simple voter approval of a <b>new</b> municipal charter, with several of the more populous <b>towns</b> having already done so.                                                                                                                                                                                                                                                                                                                                                         |                                                                       |
| 214: what does salesforce.com do?                                                                                                                                                                                                                                                                                                                                                                                                                                                                                                                                      | Salesforce.com                                                        |
| <b>Salesforce.com</b> Inc. is a global enterprise software company <b>headquartered</b> in San Francisco, California.                                                                                                                                                                                                                                                                                                                                                                                                                                                  |                                                                       |
| 217: what does 1 year mean to the planet                                                                                                                                                                                                                                                                                                                                                                                                                                                                                                                               | Earth                                                                 |
| The Earth's <b>axis</b> of <b>rotation</b> is <b>tilted</b> 23.4° away from the perpendicular of its orbital <b>plane</b> , producing <b>seasonal</b> variations on the <b>planet's</b> surface with a <b>period</b> of one tropical <b>year</b> (365.24 solar days).                                                                                                                                                                                                                                                                                                  |                                                                       |
| 219: what is feedback mechanism in plants during respiration                                                                                                                                                                                                                                                                                                                                                                                                                                                                                                           | Cellular respiration                                                  |
| While the overall <b>reaction</b> is a combustion <b>reaction</b> , no single <b>reaction</b> that comprises it is a combustion <b>reaction</b> .                                                                                                                                                                                                                                                                                                                                                                                                                      |                                                                       |
| 220: how fire extinguisher works                                                                                                                                                                                                                                                                                                                                                                                                                                                                                                                                       | Fire extinguisher                                                     |
| A <b>fire extinguisher</b> , flame <b>extinguisher</b> , or simply an <b>extinguisher</b> , is an active <b>fire</b> protection device used to <b>extinguish</b> or control small <b>fires</b> , often in emergency situations.                                                                                                                                                                                                                                                                                                                                        |                                                                       |
| 225: what countries are in central america?                                                                                                                                                                                                                                                                                                                                                                                                                                                                                                                            | Central america                                                       |
| <b>Central America</b> () is the <b>central</b> geographic region of the <b>Americas</b> .                                                                                                                                                                                                                                                                                                                                                                                                                                                                             |                                                                       |
| 227: how does a steam engine work                                                                                                                                                                                                                                                                                                                                                                                                                                                                                                                                      | Steam engine                                                          |
| In general usage, the term <b>steam engine</b> can <b>refer</b> to either the integrated <b>steam</b> plants (including boilers etc.) such as railway <b>steam</b> locomotives and portable <b>engines</b> , or may <b>refer</b> to the piston or turbine machinery alone, as in the beam <b>engine</b> and stationary <b>steam engine</b> .                                                                                                                                                                                                                           |                                                                       |
| 237: what county is tacoma washington in                                                                                                                                                                                                                                                                                                                                                                                                                                                                                                                               | Tacoma, Washington                                                    |
| Since the 1990s, developments in the downtown core include the <b>University of Washington Tacoma</b> ; <b>Tacoma Link</b> , the first modern electric light rail service in the <b>state</b> ; the <b>state's highest</b> density of <b>art</b> and <b>history museums</b> ; and a restored urban waterfront, the <b>Thea Foss Waterway</b> .                                                                                                                                                                                                                         |                                                                       |
| 238: what county is chula vista ca in                                                                                                                                                                                                                                                                                                                                                                                                                                                                                                                                  | Chula Vista, California                                               |
| Located in the city is one of America's few year-round United States Olympic Training <b>centers</b> and popular tourist destinations include Cricket Wireless Amphitheater, the <b>Chula Vista</b> marina, and the <b>Chula Vista Nature Center</b> .                                                                                                                                                                                                                                                                                                                 |                                                                       |
| 240: what did isaac newton do                                                                                                                                                                                                                                                                                                                                                                                                                                                                                                                                          | Isaac Newton                                                          |
| In addition to his work on the calculus, as a <b>mathematician</b> <b>Newton</b> contributed to the study of power series, generalised the binomial theorem to non-integer exponents, and developed <b>Newton's</b> method for approximating the roots of a function                                                                                                                                                                                                                                                                                                   |                                                                       |
| #244: how many US soldiers killed in iraq war                                                                                                                                                                                                                                                                                                                                                                                                                                                                                                                          | Casualties of the Iraq War                                            |
| <b>Casualties</b> of the conflict in <b>Iraq</b> since 2003 (beginning with the <b>2003 invasion of Iraq</b> , and continuing with the ensuing occupation of <b>Iraq</b> , as well as the activities of the various <b>armed</b> groups operating in the country) have come in many forms, and the accuracy of the information available on different types of <b>Iraq War casualties</b> varies greatly.                                                                                                                                                              |                                                                       |

<sup>48</sup>Think about this: Punjabi is the most commonly used language in Pakistan, whose official languages are English and Urdu.

- #255: how many professional hockey teams in canada  
The **National Hockey League (NHL)** is an "unincorporated not-for-profit **association**" which operates a **major professional ice hockey league** of 30 franchised **member clubs**, of which **seven** are **currently located in Canada** and 23 in the **United States**.  
*National Hockey League*
- #267: how many games did brett favre start in a row  
Favre became the Packers' **starting** quarterback in the fourth **game** of the **1992 season**, stepping in for injured quarterback Don **Majkowski**, and **started every game** through the 2007 **season**.  
*Brett Favre*
- 273: what does a vote to table a motion mean?  
In the rest of the English-speaking **world** such as the United Kingdom, to **table means** to move to **place** (the topic) upon the **table** (or to move to **place** on a **proposal**) to begin consideration (or reconsideration) of a **proposal**.  
*Table (parliamentary procedure)*
- 276: What does the class mean for SDHC cards?  
Host devices that comply with newer **versions** of the specification provide backward **compatibility** and accept older SD **cards**, but this article explains several factors that can prevent the use of a newer SD **card**.  
*Secure Digital*
- #295: how many apple store are there in total?  
The **Apple Store** is a chain of retail **stores** owned and operated by **Apple Inc.**, dealing in computers and consumer electronics.  
*Apple Store*
- 300: how is jerky made  
Some makers still use just salt and sun-dry fresh sliced meat to **make jerky**.  
*Jerky*
- #305: what happened on the moon during the period of Late Heavy Bombardment?  
The **Late Heavy Bombardment** (commonly referred to as the **lunar cataclysm**, or **LHB**) is a **hypothetical** event around 4.1 to 3.8 billion years ago (Ga).  
*Late Heavy Bombardment*
- 307: How did Edgar Allan Poe die?  
**Edgar Allan Poe** (born **Edgar Poe**; January 19, 1809 – October 7, 1849) was an American author, poet, editor and literary critic, considered part of the American Romantic Movement.  
*Edgar allan poe*
- #311: how many seasons heroes  
The second **season** of **Heroes** attracted an average of 13.1 **million viewers** in the U.S., and marked NBC's sole series among the top 20 ranked programs in total **viewership** for the 2007–2008 **season**.  
*Heroes (TV series)*
- #318: how old r Dylan and Cole Sprouse  
They are twins and are collectively referred to as **Dylan and Cole Sprouse** or the **Sprouse** brothers, usually abbreviated as **Sprouse** Bros.  
*Dylan and Cole Sprouse*
- #321: how many days does the chinese new year last  
**Chinese New Year**  
*Chinese New Year*
- 324: what does s.h.i.e.l.d stand for  
S.H.I.E.L.D. is a fictional **espionage** and law-enforcement agency in the **Marvel Comics** Universe.  
*S.H.I.E.L.D.*
- #326: how many consoles has xbox 360 sold  
Several major features of the **Xbox 360** are its integrated **Xbox Live service** that allows players to compete **online**; **download** arcade **games**, **game** demos, trailers, TV shows, music and movies; and its Windows Media Center multimedia capabilities.  
*Xbox 360*
- 328: WHAT COUNTRY IS MEXICO IN  
**Mexico** ranks sixth in the **world** and first in the Americas by **number** of UNESCO **World Heritage Sites** with 31, and in 2007 was the **tenth** most **visited country** in the **world** with 21.4 million international arrivals per year.  
*Mexico*
- #330: how is slugging percentage calculated  
The next year he **slugged** .846, and these records went unbroken until 2001, when Barry Bonds achieved 411 bases in 476 at-bats, bringing his **slugging percentage** to .863, unmatched since.  
*Slugging percentage*
- 335: what does the federal reserve do  
The **Federal Reserve System's** structure is composed of the presidentially appointed Board of **Governors** (or **Federal Reserve Board**), the **Federal Open Market Committee** (FOMC), twelve **regional Federal Reserve Banks** located in major cities throughout the nation, numerous **privately owned U.S. member banks** and various advisory councils.  
*Federal Reserve System*
- #340: how many books are included in the protestant Bible?  
The first part of Christian **Bibles** is the Old Testament, which contains, at minimum, the twenty-four **books** of the Hebrew **Bible** divided into thirty-nine **books** and **ordered** differently from the Hebrew **Bible**.  
*Books of the Bible*
- #341: how many stars on the first american flag  
Although the Betsy Ross story is accepted by most **Americans**, some **flag** historians and revisionists do not accept the Betsy Ross design as the **first American flag**.  
*Betsy Ross flag*
- #345: what became of rich on price is right  
**Richard Wayne "Rich" Fields** is an American broadcaster, spokesman, announcer and meteorologist, best known for being the announcer of the American version of **The Price Is Right** from 2004–2010.  
*Rich Fields*
- #352: what happened to stevie ray vaughan  
As the younger **brother** of **Jimmie Vaughan**, **Vaughan** started playing the **guitar** at age seven and formed several bands that **occasionally** performed in local nightclubs.  
*Stevie Ray Vaughan*
- 358: what caused ww  
Most **historians** and popular commentators include **causes** from more than one category of **explanation** to provide a rounded account of the **causes** of the war.  
*Causes of World War I*
- #362: how many seasons were there of the wire  
Despite only **receiving** modest **ratings** and never **winning** major **television awards**, **The Wire** has been **described** by many **critics** as one of the greatest **TV dramas** of all time.  
*The Wire*
- 364: what kind of legal remedy is it to ask someone to fulfill their promise  
Contract **law** varies **greatly** from one **jurisdiction** to another, including differences in **common law** compared to **civil law**, the impact of received **law**, particularly from England in **common law** countries, and of **law** codified in regional legislation.  
*Contract*
- 365: how is ASP.NET different from .NET  
ASP.NET is built on the Common Language Runtime (CLR), allowing programmers to write ASP.NET code using any supported **.NET** language.  
*ASP.NET*
- #370: how many people live in memphis tennessee  
A resident of **Memphis** is referred to as a **Memphian**, and the **Memphis** region is known, particularly to **media** outlets, as "**Memphis & The Mid-South**".  
*Memphis, Tennessee*
- #372: how many muscles in the human body  
The **muscles** of the **human body** can be categorized into a number of groups which include **muscles** relating to the head and neck, **muscles** of the torso or trunk, **muscles** of the upper limbs, and **muscles** of the lower limbs.  
*List of muscles of the human body*
- 373: how did seminoles war end  
The **Seminole Wars**, also known as the **Florida Wars**, were three **conflicts** in **Florida** between the **Seminole** — the collective name given to the amalgamation of various groups of native **Americans** and Black people who settled in **Florida** in the early 18th century — and the United States **Army**.  
*Seminole Wars*
- #385: how many nature oceans are on earth  
This animation uses **Earth** science data from a variety of sensors on NASA **Earth** observing satellites to measure physical oceanography parameters such as **ocean currents**, **ocean winds**, **sea surface height** and **sea surface temperature**.  
*Ocean*
- 388: what county is jacksonville florida in  
**Jacksonville** is the principal **city** in the **Jacksonville metropolitan area**, with a population of 1,345,596 in 2010.  
*Jacksonville, Florida*
- 391: what does a liquid oxygen plant look like  
**Liquid oxygen** — abbreviated LOx, LOX or Lox in the aerospace, submarine and gas **industries** — is one of the physical forms of elemental **oxygen**.  
*Liquid oxygen*
- 402: What does the term "mens rea" mean  
Therefore, **mens rea** refers to the mental element of the **offence** that accompanies the **actus reus**.  
*Mens rea*
- In Australia, for example, the elements of the federal **offences** are now designated as "fault elements" or "mental elements" (**mens rea**) and "physical elements" or "external elements" (**actus reus**).
- 406: what do UA's detect  
Major uses of drug testing are to **detect** the **presence** of performance enhancing **steroids** in **sport** or for drugs prohibited by laws, such as cannabis, cocaine and heroin.  
*Drug test*
- 414: What does Human sperm consist of?  
The process that results in the discharge of semen is called **ejaculation**.  
*Semen*
- 416: how did the penguins acquire sidney crosby  
The **Penguins** returned to the Finals against Detroit the following year and won in seven **games**; **Crosby** became the youngest captain in NHL history to win the Stanley Cup.  
*Sidney Crosby*
- #420: how much total wealth in USA  
*Wealth in the United States*
- In addition, **wealth** is unevenly distributed, with the **wealthiest** 25% of US households **owning** 87% of the **wealth** in the **United States**, which was \$54.2 **trillion** in 2009.  
*Plus-minus sign*
- 429: what does a plus-minus sign mean  
The **sign** is normally pronounced "**plus** or **minus**".  
*Plus-minus sign*
- The **plus-minus sign** ( ) is a mathematical symbol commonly used either
- 433: how was the moon formed  
Red and orange tinted **Moon**, as seen from Earth during a **lunar eclipse**, where the Earth comes between the **Moon** and **Sun**  
*Moon*
- 435: what did ronald reagan do as president  
**Ronald Wilson Reagan** (; February 6, 1911 – **June 5, 2004**) was the 40th **President** of the United States (1981–1989).  
*Ronald Reagan*
- 439: what does judgment as a matter of law mean  
JML motions may also be made after the verdict is returned, where they are called "renewed" motions for **judgment** as a **matter of law** (RJMOL), but the motion is still commonly known by its former name, **judgment** notwithstanding verdict, or j.n.o.v. (from the English **judgment** and the Latin non obstante veredicto).  
*Judgment as a matter of law*
- #441: how many presidents have been assassinated  
**Assassination** attempts and **plots** on **Presidents** of the United States have been numerous: more than 20 attempts to kill sitting and former **presidents**, as well as the Presidents-elect, are known.  
*List of United States presidential assassination attempts and plots*
- 443: what does oklahoma produce  
**Oklahoma City** and **Tulsa** serve as **Oklahoma's** primary **economic** anchors, with nearly two thirds of **Oklahomans** living within their metropolitan statistical areas.  
*Oklahoma*
- #444: how many redwall books are there  
It is the title of the first **book** of the series, published in 1986, as well as the name of the Abbey featured in the **book** and the name of an animated TV series **based** on three of the novels (**Redwall**, **Mattimeo**, and **Martin the Warrior**), which first aired in 1999.  
*Redwall*
- 446: what date did the american civil war start  
The **American Civil War** (ACW), also known as the **War** between the States or **simply the Civil War** (see naming), was a **civil war** fought from 1861 to 1865 between the United States (the "Union" or the "North") and several Southern **slave** states that declared their secession and formed the Confederate States of **America** (the "Confederacy" or the "South").  
*American Civil War*
- 452: how jameson irish whiskey is made  
With annual sales of over 31 million bottles, **Jameson** is by far the best selling **Irish whiskey** in the world, as it has been sold internationally since the early 19th century when **John Jameson** along with his son (also named John) was producing more than a million gallons annually.  
*Jameson Irish Whiskey*
- #464: How many consecutive games did Ken Jennings win?  
**Jennings** is noted for holding the record for the longest **winning** streak on the U.S. syndicated **game show Jeopardy!**  
*Ken Jennings*
- 468: what county is jennings, la  
**Jennings** is the principal city of the **Jennings** Micropolitan Statistical Area, which includes all of **Jefferson Davis Parish**.  
*Jennings, Louisiana*
- 469: how does nanotechnology affect health  
A more generalized description of **nanotechnology** was subsequently established by the National **Nanotechnology** Initiative, which defines **nanotechnology** as the manipulation of matter with at least one dimension sized from 1 to 100 nanometers.  
*Nanotechnology*
- 476: what does it take to start a lodge in freemason  
By exception the three surviving **lodges** that formed the world's first known **Grand Lodge** in London (today called the United **Grand Lodge** of England) have the unique privilege to operate as time immemorial i.e. without such warrant, only one other **lodge** operates without a warrant - this is the **Grand Stewards' Lodge** in London, although it is not also entitled to the "time immemorial" title.  
*Masonic Lodge*
- 480: how does black pepper grow  
**Peppercorns**, and the ground **pepper** derived from them, may be described simply as **pepper**, or more precisely as **black pepper** (cooked and **dried** unripe fruit), **green pepper** (**dried** unripe fruit) and **white pepper** (**dried** ripe seeds).  
*Black pepper*
- 482: how south african leaders are elected  
The President of the Republic of **South Africa** is the head of state and head of government under **South Africa's** Constitution.  
*President of South Africa*
- 485: how was the phone invented  
This article covers the early years from 1844 to 1898, from conception of the **idea** of an electric voice-transmission device, to failed attempts to use "make-and-break" current, to successful experiments with electromagnetic telephones by Alexander Graham Bell and **Thomas Watson**, and finally to commercially successful telephones in the late 19th century.  
*Invention of the telephone*
- 491: what forms seasons  
Hot regions have two or three **seasons**; the **rainy** (or wet, or monsoon) **season** and the **dry season**, and in some **tropical** areas, a cool or mild **season**.  
*Season*
- 492: how did mohammed gandhi die  
**Mohandas Karamchand Gandhi** (; 2 October 1869 – 30 January 1948), commonly known as **Mahatma Gandhi**, was the preeminent leader of **Indian** nationalism in British-ruled **India**.  
*Mahatma Gandhi*
- #495: how many users do twitter have  
**Twitter** is an online social networking **service** and microblogging **service** that enables its **users** to **send** and read text-based **messages** of up to 140 characters, known as "**tweets**".  
*Twitter*
- 513: how did the vietnam war end  
They viewed the **conflict** as a colonial war, **fought** initially against France, backed by the U.S., and later against **South Vietnam**, which it regarded as a **U.S. puppet state**.  
*Vietnam War*
- #516: how much more time does chemo give to people with renal cancer  
**Renal cell carcinoma** (RCC, also known as **hypernephroma**) is a **kidney cancer** that originates in the lining of the proximal convoluted tubule, the very small tubes in the **kidney** that transport GF (glomerular filtrate) from the glomerulus to the descending limb of the nephron.  
*Renal cell carcinoma*
- 521: how does a solid state drive work  
Hybrid **drives** or **solid state** hybrid **drives** (SSHD) combine the features of SSDs and HDDs in the same unit, containing a large **hard disk drive** and an SSD cache to improve performance of frequently accessed data.  
*Solid-state drive*
- #529: how long did the roman empire last  
The **Roman Empire** ( ) was the post-**Republican** period of the ancient **Roman** civilization, characterised by an autocratic form of government and large territorial **holdings** around the Mediterranean in **Europe**, **Africa**, and **Asia**.  
*Roman Empire*
- #533: how much does U.S. pay on health care per person  
**Total government spending** per capita in the U.S. on **health care** was 23% higher than Canadian **government spending**, and **U.S. government expenditure** on **health care** was just under 83% of **total** Canadian **spending** (**public** and **private**) though these statistics don't take into account population differences.  
*Comparison of the health care systems in Canada and the United States*
- 537: how is rfid tag powered  
Radio-frequency **identification** (RFID) is the wireless non-contact use of radio-frequency electromagnetic fields to transfer data, for the purposes of automatically **identifying** and **tracking tags** attached to objects.  
*Radio-frequency identification*
- #556: how long have kanab ambersnail been endangered?  
The **Kanab ambersnail**, scientific name *Oxyloma haydeni* kanabensis or *Oxyloma kanabense*, is a critically **endangered** subspecies or species of small, air-breathing land snail, a terrestrial pulmonate gastropod mollusc in the family Succineidae, the amber snails.  
*Kanab ambersnail*
- Now considered a Critically **Endangered** species on the IUCN Red List of Threatened Species due to a series of factors (including influence), the **Kanab ambersnail** has been reintroduced to three springs above the historic high water level along the Colorado River.
- #557: how many spanish speaking people are there in the us  
There are 45 million Hispanophones who **speak Spanish** as a first or second **language**, as well as six million **Spanish** language students, composing the **largest** national Spanish-speaking community **outside** of **Mexico** and making **Spanish** the Romance **language** and the Indo-European **language** with **largest** number of **native speakers** in the world.  
*Spanish language in the United States*
- 558: what does (sic) mean?  
**Sic** (noise artist), styled as [sic], stage name of Jennifer Morris, a Canadian noise artist  
*Sic*
- 560: how does sedimentary rock form  
The **sedimentary rock** cover of the continents of the **Earth's crust** is extensive, but the **total** contribution of **sedimentary rocks** is estimated to be only 8% of the **total volume** of the **crust**.  
*Sedimentary rock*
- 562: what did st patrick do  
The text, however, distinguishes between "Old **Patrick**" (thought to mean Palladius) and "**Patrick**, archbishop of the Scots," who died in 492.  
*Saint Patrick*
- 563: how do you know if something is the golden ratio  
Many 20th century artists and architects have **proportioned** their works to approximate the **golden ratio**—especially in the form of the **golden** rectangle, in which the **ratio** of the longer side to the shorter is the **golden ratio**—believing this **proportion** to be aesthetically pleasing (see Applications and observations below).  
*Golden ratio*
- 570: How is a computer used?  
*Computer*

Simple **computers** are small enough to fit into mobile devices, and mobile **computers** can be powered by small batteries. Personal **computers** in their various forms are icons of the Information Age and are what most people think of as "computers."

#581: how often does ham station need to ID? *Station identification*  
**Station** identification (ident or channel **ID**) is the **practice** of radio or television **stations** or networks identifying themselves on air, typically by means of a call sign or brand name (sometimes known, particularly in the United States, as a "sounder" or "stinger", more generally as a **station** or network ID).

#583: how many days are in a leap year *Leap year*  
The term **leap year** gets its name from the fact that while a fixed **date** in the Gregorian calendar normally advances one **day** of the **week** from one year to the next, in a **leap year** the **day** of the **week** will advance two **days** (from March onwards) due to the year's extra **day** inserted at the end of **February** (thus "leaping over" one of the **days** in the week).

597: what county is Bethlehem pa in *Bethlehem, Pennsylvania*  
There are three general sections of the city: North **Bethlehem**, South **Bethlehem** and West **Bethlehem**.

598: what countries legalize marijuana *Legality of cannabis*  
While **federal law** in the **United States** bans all sale and **possession** of **cannabis**, enforcement varies widely at the **state** level and some **states** have established medicinal **marijuana** programs in that contradict **federal law**; two **states** ( Colorado and **Washington** ) have repealed their **laws** prohibiting the recreational **use** of **cannabis** and replaced them with a regulatory regime, also contrary to **federal** statute.

#603: how many albums has dmX sold to this date *DMX (rapper)*  
In 1999, **DMX** released his best-selling **album** ...And Then There Was **X**, which featured the hit **single** "Party Up (Up in Here)".

610: what do mucous membranes secrete *Mucous membrane*  
The term **mucous membrane** refers to where they are found in the body and not every **mucous membrane** secretes mucus.

611: what company is cricket wireless by *Cricket Wireless*  
**Cricket Communications, Inc.** ( d.b.a. **Cricket Wireless**) founded in 1999, provides **wireless** services to over 7 million customers in the United States.

#615: how many numbers on a credit card *Bank card number*  
**Payment card numbers** are found on **payment cards**, such as **credit cards** and debit **cards**, as well as stored-value **cards**, **gift cards** and other similar **cards**.

617: how is public policy created *Public policy*  
The U.S. professional association of **public policy** practitioners, researchers, scholars, and students is the Association for **Public Policy** Analysis and Management.  
As an academic discipline, **public policy** is studied by professors and students at **public policy** schools of major universities throughout the country.

#619: how many wives did Henry the 8th have *Henry VIII of England*  
**Henry's** struggles with Rome led to the separation of the **Church of England** from **papal** authority, the Dissolution of the Monasteries, and his own establishment as the Supreme Head of the **Church of England**.

620: what country are bongo drums from? *Bongo drum*  
The **drums** are of different size: the larger **drum** is called in Spanish the hembra ( female ) and the smaller the macho ( male ).

#621: how many books in bible *Books of the Bible*  
The first part of Christian **Bibles** is the Old Testament, which contains, at minimum, the twenty-four **books** of the Hebrew **Bible** divided into thirty-nine **books** and **ordered** differently from the Hebrew **Bible**.

639: what does freedom of speech cover *Freedom of speech*  
The right to **freedom** of expression is recognized as a **human right** under **Article 19** of the Universal Declaration of **Human Rights** and recognized in international **human rights law** in the International Covenant on Civil and Political **Rights** (ICCPR).

647: what county is san jose in? *San Jose, California*  
**San Jose** was founded on **November 29, 1777**, as El Pueblo de **San José** de Guadalupe, the **first** civilian town in the **Spanish** colony of Nueva **California**, which later became Alta **California**.

651: what cars have smart key systems *Smart key*  
A **smart key** is an electronic **access** and authorization **system** which is available as an option or standard in several **cars**.

676: how did John F. Kennedy die? *John F. Kennedy*  
**John Fitzgerald** "Jack" **Kennedy** (May 29, 1917 – **November 22, 1963**), often referred to by his initials JFK, was the 35th President of the United States, serving from 1961 until his **death** in 1963.

#677: how many members are in the house of representatives *United States House of Representatives*  
The Speaker of the **United States House of Representatives**, who **presides** over the chamber, is elected by the **members** of the **House**, and is therefore traditionally the leader of the **House** Democratic **Caucus** or the **House** Republican **Conference**, whichever party has more voting **members**.

678: what can silk be used for *Silk*  
Many **silks** are mainly **produced** by the **larvae** of **insects** undergoing complete metamorphosis, but some adult **insects** such as web-spinners **produce silk**, and some **insects** such as raspy crickets **produce silk** throughout their lives.

682: what does uncle sam represent to the american people *Uncle Sam*  
The first use of **Uncle Sam** in literature was in the 1816 allegorical book "The Adventures of **Uncle Sam** in Search After His Lost Honor" by Frederick Augustus Fiddady, Esq. An **Uncle Sam** is mentioned as early as 1775, in the original "Yankee Doodle" lyrics of the Revolutionary War.

684: what do cyberstalkers do *Cyberstalking*  
**Cyberstalking** is a criminal offense that comes into play under state anti-stalking **laws**, slander **laws**, and harassment **laws**.

685: how do insulin syringes work *Syringe*  
The word "**syringe**" is derived from the Greek **συριγγή** syrix = "tube" via back-formation of a new singular from its Greek-type plural "**syringes**" (**συριγγές** syringes).

692: how did david carradine die *David Carradine*  
**David Carradine** (born John Arthur **Carradine**; **December 8, 1936** – June 3, 2009) was an American actor and martial artist, best known for his leading role as a warrior monk, Kwai Chang Caine, in the 1970s television series **Kung Fu**.

700: what affects the money supply *Money supply*  
Second, if the velocity of **money**, i.e., the ratio between **nominal GDP** and **money supply**, changes, an **increase** in the **money supply** could have either no **effect**, an exaggerated **effect**, or an unpredictable **effect** on the growth of **nominal GDP**.

703: how is today special? *Today's Special*  
It was **set** in a department store, based on the flagship location of the now defunct Simpson's in Toronto.

707: what does auld lang syne mean *Auld Lang Syne*  
Consequently "For **auld lang syne**", as it appears in the first line of the chorus, might be loosely translated as "for (the sake of) **old times**".

715: how was the president involved in the gulf war *Gulf War*  
The **war** is also known under other **names**, such as the Persian **Gulf War**, First **Gulf War**, **Gulf War I**, or the First **Iraq War**, before the **term** "Iraq **War**" became identified instead with the 2003 **Iraq War** (also referred to in the U.S. as "Operation **Iraqi Freedom**").

#716: how many times has a player hit for the cycle *Hitting for the cycle*  
One **NPB player** has also **hit** for the **cycle** in an **NPB All-Star game**.

723: what does it mean if i'm flat footed? *Flat foot*  
Three studies (see citations below in military section) of military recruits have shown no evidence of later increased **injury**, or **foot** problems, due to **flat feet**, in a population of people who reach military service age without prior **foot** problems.

726: what age group is generation X *Generation X*  
**Generation X**, commonly abbreviated to **Gen X**, is the **generation** born after the Western post-World War II baby boom.

729: how did James Dean die? *James Dean*  
**James Byron Dean** (February 8, 1931 – September 30, 1955) was an American actor.

734: what glows in the dark *Glow-in-the-dark*  
Glow in the **Dark Tour**, a 2008 concert tour by Kanye West

737: what did sparta do around 650 bc *Sparta*  
**Sparta** ( Doric **Greek** ; ; Attic **Greek** ; , or Lacedaemon, was a **prominent** city-state in **ancient Greece**, situated on the banks of the Eurotas River in Laconia, in south-eastern Peloponnese.

738: what fantasy american football means *Fantasy football (American)*  
Due to the growth of the Internet, **Fantasy football** has vastly increased in **popularity**, particularly because **Fantasy football** providers such as ESPN, Yahoo, CBS, and the NFL itself are able to keep track of statistics entirely online, eliminating the need to check box scores and newspapers regularly to keep track of players.

#741: how many muscles in the body *List of muscles of the human body*

The **muscles** of the human **body** can be categorized into a number of groups which include **muscles** relating to the head and neck, **muscles** of the torso or trunk, **muscles** of the upper limbs, and **muscles** of the lower limbs.

747: what does the green mean on the mexican flag *Flag of Mexico*  
While the **meaning** of the **colors** has changed over time, these three **colors** were adopted by **Mexico** following **independence** from Spain during the country's War of **Independence**, and subsequent First **Mexican Empire**.

#749: how often do elk have sex *Elk*  
**Male elk** have large antlers which are shed each year.

#757: how many players on a side for a football game *American football*  
**American football** is the most **popular sport** in the **United States** today, and the **National Football League** (NFL) is its most **popular league**.

760: what does the temporal lobe part of the brain do *Temporal lobe*  
The **temporal lobe** is a region of the cerebral cortex that is located beneath the lateral fissure on both cerebral hemispheres of the mammalian **brain**.

#761: how many lungs does a human have *Human lung*  
The right **lung** consists of three **lobes** while the left **lung** is slightly smaller consisting of only two **lobes** (the left **lung** has a "cardiac notch" allowing space for the heart within the chest).

768: what is the population of center tx *Center, Texas*  
The Rio Theater in **Center**  
It is named for its location near the **center** of Shelby County, not for its location in Texas as it is located near the Louisiana border.  
First Christian Church at 124 Cora Street in **Center** is one of the oldest congregations in the community.  
First Baptist Church at 117 Cora Street in **Center** is located next to the downtown section.  
Chamber of Commerce Building in **Center**.  
**Center** is a city in Shelby County, Texas, United States.

770: what causes photo red eye *Red-eye effect*  
The red-eye **effect** in photography is the common appearance of **red** pupils in color photographs of **eyes**.

771: what creates a cloud *Cloud*  
These include strato- for low **clouds** with limited convection that form mostly in uneven layers, cumulo- for complex high-convective storm **clouds**, nimbo- for thick layered **clouds** of some complexity that can produce moderate to heavy precipitation, alto- for middle **clouds**, and cirro- for high **clouds**; the latter two of which may be of simple or moderately complex structure.

#772: how many students go to santa barbara *University of California, Santa Barbara*  
The **University of California, Santa Barbara** (commonly referred to as UC **Santa Barbara** or UCSB) is a public research **university** and one of the ten general campuses of the **University of California system**.

774: what culture is mariah carey *Mariah Carey*  
Under the guidance of Columbia Records executive Tommy Mottola, **Carey** released her self-titled debut studio album **Mariah Carey** in 1990; it went multi-platinum and spawned four consecutive number one singles on the U.S. Billboard Hot 100 chart.

779: how was color introduced in film? *Color motion picture film*  
**Color motion picture film** refers both to unexposed **color** photographic **film** in a format suitable for use in a **motion picture camera**, and to finished **motion picture film**, ready for use in a **projector**, which bears images in **color**.

781: what artist have song with ashanti? *Ashanti (entertainer)*  
**Ashanti** is most famous for her eponymous debut album, which **featured** the hit **song** " Foolish ", and sold over 503,000 copies in its first week of release throughout the U.S. in April 2002.

783: what came first army or air force *United States Army Air Forces*  
Although other **nations** already had separate **air forces independent** of the **army** or navy (such as the British Royal **Air Force** and the German **Luftwaffe** ), the AAF remained a part of the **United States Army** until the **United States Air Force** came into being in September 1947.

784: what day is 2011 super bowl? *Super Bowl XLV*  
Unlike other matchups, this game featured two title-brand franchises: coming into the game, the **Packers** held the most NFL **championships** with 12 (9 league **championships** prior to the **Super Bowl** era and 3 **Super Bowl** championships), while the **Steelers** held the most **Super Bowl championships** with 6.

785: what does the FOIA apply to *Freedom of Information Act (United States)*  
The Federal Government's Freedom of Information Act should not be confused with the different and varying Freedom of Information **Acts** passed by the individual states.  
Many of those state **acts** may be similar but not identical to the **federal act**.

#786: how many countries are member of the eu? *European Union*  
With a combined **population** of over 500 **million** inhabitants, or 7.3% of the **world population**, the **EU**, in 2012, generated a nominal gross domestic product (GDP) of 16.584 **trillion** US dollars, representing approximately 20% of the global GDP when measured in terms of purchasing power parity, and represents the **largest** nominal GDP and GDP PPP in the world.

#790: how many vehicles are registered in the us *Passenger vehicles in the United States*  
This number, along with the average age of **vehicles**, has increased steadily since 1960, indicating a growing number of **vehicles** per capita.

792: what cards do you need in poker to get a royal flush *List of poker hands*  
The ranking of a particular hand is increased by including multiple **cards** of the same **card rank**, by all five **cards** being from the same suit, or by all five **cards** being of consecutive rank.

799: what does xylem transport *Xylem*  
The word **xylem** is derived from the Greek word ξύλον (xylon), meaning "wood"; the best-known **xylem** tissue is **wood**, though it is **found** throughout the plant.

#800: how many mvp's has kobe bryant won *Kobe Bryant*  
In 2006, **Bryant scored** a career-high 81 points against the Toronto Raptors, the second most points **scored** in a **single game** in **NBA** history, second only to Wilt Chamberlain's 100-point **game** in 1962.

804: what do Jehovah witnesses believe *Jehovah's Witnesses*  
**Jehovah's Witnesses** is a millenarian restorationist Christian denomination with nontrinitarian **beliefs** distinct from mainstream Christianity. Sources for descriptors: • Millenarian: • Restorationist: • Christian: • Denomination: The organization reports worldwide membership of over 7.78 million adherents involved in evangelism, convention attendance of over 12 million, and annual Memorial attendance of over 19 million.

806: how old old is xp operating system *Windows XP*  
According to web analytics **data generated** by Net Applications, Windows **XP** was the most **widely used operating system** until August 2012, when Windows 7 overtook it.

#811: how many pawns in chess *Pawn (chess)*  
It is also **common** to refer to a rook **pawn**, meaning any **pawn** on the a- or h-file, a knight **pawn** (on the b- or g-file), a bishop **pawn** (on the c- or f-file), a queen **pawn** (on the d-file), a king **pawn** (on the e-file), and a central **pawn** (on either the d- or e-file).

814: how is hydrogen produced *Hydrogen production*  
**Hydrogen production** is the family of industrial methods for generating **hydrogen**.

833: what country is madrid spain in *Madrid*  
As the **capital city** of **Spain**, seat of government, and **residence** of the **Spanish** monarch, **Madrid** is also the political, **economic** and cultural centre of **Spain**.

835: What causes rogue waves *Rogue wave*  
**Rogue waves** (also known as freak **waves**, monster **waves**, killer **waves**, extreme **waves**, and abnormal **waves**) are relatively large and spontaneous ocean surface **waves** that occur far out at sea, and are a threat even to large ships and ocean liners.

#837: what happened to montgomery clift *Montgomery Clift*  
Edward **Montgomery Clift** (October 17, 1920July 23, 1966) was an American film and stage actor The New York Times' obituary noted his portrayal of "moody, sensitive young men".

#850: what happened to george o'malley on grey's anatomy? *George O'Malley*  
Introduced as a **surgical** intern at the fictional Seattle Grace Hospital, **O'Malley** worked his way up to resident level, while his **relationships** with his colleagues Meredith **Grey** ( Ellen Pompeo ), Cristina Yang ( Sandra Oh ), Izzie **Stevens** ( Katherine Heigl ) and Alex Karev ( Justin Chambers ) formed a focal point of the series.

#852: how many people die from myasthenia gravis per year *Myasthenia Gravis*  
**Myasthenia gravis** (from Greek μῦς "muscle", "weakness", and "serious"; abbreviated MG) is an autoimmune neuromuscular **disease** leading to fluctuating muscle weakness and fatigability.

#854: how many rooms in borgata hotel *The Borgata*  
The **Borgata Hotel** Casino and **Spa** is a luxury **hotel**, casino, and **spa** in Atlantic City, New Jersey, United States.

859: what country has the most muslims in the world *Islam by country*

In the Middle East, the non-Arab **countries** of Turkey and Iran are the largest **Muslim-majority countries**; in Africa, Egypt and Nigeria have the most populous **Muslim** communities.

861: what country is dubai in *Dubai*  
The Sheikdom of **Dubai** was formally established in 1833 by Sheikh Maktoum bin Butti Al-Maktoum when he persuaded around 800 members of his tribe of the Bani Yas, living in what was then the Second Saudi State and now part of Saudi Arabia, to follow him to the **Dubai** Creek by the Abu Falasa clan of the Bani Yas.

863: how much of earth is covered ocean water *Ocean*  
The Mars **ocean** hypothesis **suggests** that nearly a third of the surface of Mars was once **covered** by **water**, though the **water** on Mars is no longer **oceanic**, and a runaway greenhouse effect may have boiled away the global **ocean** of Venus.

870: how much did yankee stadium cost *Yankee Stadium*  
The **first** game at the new **Yankee Stadium** was a pre-season exhibition game against the Chicago Cubs **played** on **April 3, 2009**, which the **Yankees won 7-4**.

879: What happened to "The Glades" tv series *The Glades (TV series)*  
The **Glades** was renewed by A&E for a **third season** on October 18, 2011, which aired from June 3 to August 12, 2012.

887: how many albums has eminem sold in his career *Eminem*  
His next two records The **Marshall Mathers LP**, and The **Eminem Show**, also **won** Best Rap **Album Grammy Awards**, making **Eminem** the **first artist to win Best Rap Album** for **three consecutive LPs**.

891: what do pigs eat *Pig*  
**Pigs** include the domestic **pig**, its ancestor the wild boar, and several other wild relatives.

900: What happened during the Starving Time in Jamestown? *Starving Time*  
The **Starving Time** at **Jamestown** in the Colony of Virginia was a period of **starvation** during the winter of 1609–1610 in which all but **60** of 500 colonists died.

905: what does the president of the usa do *President of the United States*  
It also prohibits a **person** from being elected to the **presidency** more than once if that **person** previously had **served** as **president**, or acting **president**, for more than two years of another **person's** term as **president**.

911: how kimberlite pipes form *Volcanic pipe*  
Volcanic **pipes** are geological structures **formed** by the violent, supersonic eruption of deep-origin volcanoes.

913: how many sections of grey's anatomy are there *Grey's Anatomy*  
**Dr. Preston Burke** (Isaiah Washington) **departs** at the conclusion of the third **season**, and is **replaced** by **Dr. Erica Hahn** (Brooke Smith), who leaves the show during the fifth **season**, and later **Dr. Teddy Altman** (Kim Raver), who **departs** at the **end** of the eighth **season**.

914: how is schizophrenia diagnosed? *Schizophrenia*  
Despite the etymology of the term from the Greek roots skhizein (σχίζω, "to split") and phrēn, phrēn- (φρήν, φρέν-, "mind"), **schizophrenia** does not imply a "**split personality**", or "**multiple personality disorder**" (which is known these days as dissociative identity disorder)—a condition with which it is often confused in public perception.

931: what kind of company is Microsoft? *Microsoft*  
As of 2013, **Microsoft** is market dominant in both the PC operating **system** and office suite markets (the latter with **Microsoft Office**).

938: how does weather happen *Weather*  
Studying how the **weather works** on other planets has been helpful in understanding how **weather works** on Earth.

940: how many countries have english as an official language *List of countries where English is an official language*  
According to the Constitution of India, "Hindi in the Devanagari script" is the **official language** of the union; and **English** the "subsidiary **official language**"; however, **English** is mandated for the authoritative texts of all federal laws and Supreme Court decisions and (along with Hindi) is one of the two **languages** of the Indian Parliament.

941: what countries are in cono sur *Southern Cone*  
**High** life expectancy, the **highest** Human Development Index of Latin America, **high Standard** of living, significant participation in the global markets and the emerging economy of its members make the **Southern Cone** the most prosperous macro-region in **South America**.

949: what branch of the military is delta force *Delta Force*  
The Central Intelligence Agency's highly secretive Special Activities Division (SAD) and more **specifically** its elite Special **Operations Group (SOG)** often works with – and recruits – **operators** from **Delta Force**.

957: what takes the seasons *Season*  
Hot regions have two or three **seasons**; the **rainy** (or wet, or monsoon) **season** and the **dry season**, and in some **tropical** areas, a cool or mild **season**.

959: what does 3g network mean *3G*  
**3G** finds application in **wireless voice telephony**, mobile Internet access, fixed **wireless** Internet access, video calls and mobile TV.

960: what does Mazel tov! mean *Mazel tov*  
"**Mazel tov**" or "**mazal tov**" ( Hebrew / Yiddish : מַזֵּל טוֹב, Hebrew: "**mazal tov**"; Yiddish: "**mazel tov**"; lit. "good luck").

961: How Do You Get Hepatitis C *Hepatitis C*  
**Hepatitis C** is an infectious disease affecting primarily the liver, caused by the **hepatitis C** virus (HCV).

962: how does flexible spending account work *Flexible spending account*  
The most common **type** of **flexible spending account**, the medical expense FSA (also medical FSA or **health FSA**), is similar to a **health savings account (HSA)** or a **health reimbursement account (HRA)**.

966: how many baseball teams usa *Major league baseball*  
Major **League Baseball (MLB)** is a professional **baseball league**, consisting of **teams** that play in the **National League** and the **American League**.

972: how many amendments in the US constitution *List of amendments to the United States Constitution*  
To date, no convention for proposing **amendments** has been called by the states, and only once—in 1933 for the ratification of the twenty-first **amendment**—has the convention method of ratification been employed.

979: what day is the federal holiday for Martin Luther King Jr. *Martin Luther King, Jr. Day*  
**Martin Luther King, Jr. Day** is a United States **federal holiday** marking the birthday of Rev. Dr. **Martin Luther King, Jr.**

985: what area code is 949 *Area code 949*  
The **area code** in red is **Area Code 949**; all others in blue are California **area codes**.

994: how many babies are in a typical raccoon litter *Raccoon*  
The **raccoon** (, Procyon lotor), sometimes spelled **raccoon**, also known as the common **raccoon**, North **American raccoon**, northern **raccoon** and colloquially as **coon**, is a medium-sized mammal **native** to **North America**.

998: What does Rapture meaning in a theological sense? *Rapture*  
Denominations such as Roman Catholics, Orthodox **Christians**, Lutheran **Christians**, and Reformed **Christians** believe in a **rapture** only in the **sense** of a **general final resurrection**, when **Christ** returns a single time.

1002: what are corporation balance *Balance sheet*  
In financial accounting, a **balance** sheet or statement of financial position is a summary of the financial **balances** of a sole proprietorship, a business partnership, a **corporation** or other business organization, such as an LLC or an LLP.

1003: what is .17 hmr caliber *.17 HMR*  
It descended from the .22 Magnum by necking down the .22 Magnum case to take a **.17 caliber** (4.5 mm) bullet, and it is more costly to shoot than traditional **.22 caliber** rimfire cartridges.

1007: what made the civil war different from others *American Civil War*  
The **American Civil War** (ACW), also known as the **War** between the States or **simply the Civil War** (see naming), was a **civil war** fought from 1861 to 1865 between the United States (the "Union" or the "**North**") and several **Southern slave** states that declared their secession and formed the Confederate States of **America** (the "Confederacy" or the "**South**").

1008: where to buy potato bread made without wheat *Potato bread*  
**Potato bread** is a form of **bread** in which **potato** replaces a portion of the regular **wheat** flour.

1014: who killed julius caesar *Julius caesar*  
**Gaius Julius Caesar** (, July 100 BC – 15 March 44 BC) was a Roman general, statesman, Consul and notable author of Latin prose.

1024: who wrote white christmas *White Christmas (song)*  
I just **wrote** the best **song** I've ever **written** — heck, I just **wrote** the best **song** that anybody's ever written!"

1027: WHAT IS A FY QUARTER *Fiscal year*  
Many universities have a **fiscal year** which ends during the summer, both to align the **fiscal year** with the school year (and, in some cases involving public universities, with the state government's **fiscal** year), and because the school is normally less **busy** during the summer months.

1028: who pulmonary hypertension *Pulmonary hypertension*  
In medicine, **pulmonary hypertension** (PH) is an increase of **blood pressure** in the **pulmonary** artery, **pulmonary** vein, or **pulmonary** capillaries, together known as the **lung** vasculature, leading to shortness of breath, dizziness, fainting, and other symptoms, all of which are exacerbated by exertion.

1033: what is a notary for *Notary public*  
With the exceptions of Louisiana, Puerto Rico, Quebec, whose private law is based on civil law, and British Columbia, whose notarial tradition stems from scrivener **notary** practice, a **notary** public in the rest of the **United States** and most of Canada has powers that are far more limited than those of civil-law or other **common-law notaries**, both of whom are qualified lawyers admitted to the bar: such **notaries** may be referred to as notaries-at-law or lawyer **notaries**.

1038: when did the cold war start *Cold War*  
The tensest times were during the **Berlin Blockade** (1948–1949), the **Korean War** (1950–1953), the Suez Crisis (1956), the **Berlin Crisis** of 1961, the Cuban missile crisis (1962), the Vietnam War (1959–1975), the Yom Kippur War (1973), the Soviet war in **Afghanistan** (1979–1989), the Soviet downing of **Korean Air Lines Flight 007** (1983), and the "Able Archer" NATO military exercises (1983).

1039: what state is pike's peak in? *Pikes Peak State Park*  
It gets its name from the Iowa incarnation of **Pikes Peak**, a particularly high point overlooking the gorge of the Upper Mississippi, and like **Pikes Peak** in Colorado, is named for Zebulon **Pike**.

1049: what is a book index *Index (publishing)*  
In a traditional back-of-the-book **index** the headings will include names of people, places and events, and concepts selected by a person as being relevant and of interest to a possible reader of the **book**.

1050: who sings the song never ending story *The NeverEnding Story (song)*  
"The **NeverEnding Story**" (titled "The **NeverEnding Story** (L'histoire sans fin)" in the French version) is the title **song** from the English version of the 1984 film **The NeverEnding Story**.

1053: who created facebook *Facebook*  
**Facebook** is an online social networking service, whose **name** stems from the colloquial **name** for the book given to **students** at the start of the academic year by some **university** administrations in the United States to help **students** get to know each other.

1057: what are risk for infections *Risk of infection*  
Although any one can become **infected** by a pathogen, patients with this diagnosis are at an elevated **risk** and **extra infection** controls should be considered.

1061: where do cruises dock in new york city *New York Passenger Ship Terminal*  
With an upsurge in **cruise** ship traffic and the terminal's ability to handle comfortably only three large ships at a time, two **new** terminals have been opened in the harbor — the Cape Liberty **Cruise** Port opened in 2004 in Bayonne, **New Jersey** (used by Royal Caribbean **Cruise** Line, **Celebrity Cruises** and Azamara **Cruises**), and the Brooklyn **Cruise** Terminal (used by the Queen Mary 2 and other ships of the Carnival Corporation **cruise** brands) opened in 2006 in Brooklyn, **New York**.

1064: who played the lead roles in the movie leaving las vegas *Leaving Las Vegas*  
After limited **release** in the United States on October 27, 1995, **Leaving Las Vegas** made its nationwide **release** on February 9, 1996, receiving strong praise from critics and audiences.

1065: what is a CMM machine *Coordinate-measuring machine*  
A **machine** which takes readings in six degrees of freedom and displays these readings in mathematical form is known as a **CMM**.

1067: what percentage of water in the body *Body water*  
In physiology, **body water** is the **water** content of the human **body**.

1068: what type of batteries are 357 (LR44) *LR44 battery*  
Silver-oxide **batteries** type SR44 may provide extra capacity compared to **LR44 types** but have slightly different voltage characteristics.

1069: where did hurricane katrina begin *Hurricane Katrina*  
The **hurricane strengthened** to a Category **5 hurricane** over the warm Gulf water, but weakened before making its second landfall as a Category **3 hurricane** on the morning of Monday, **August 29** in southeast **Louisiana**.

1073: what are 1 mil guaranies in united states dollars *Mill (currency)*  
In the **United States**, it is a notional unit equivalent to of a **United States dollar** (a tenth of a cent).

1075: where did the persian war take place *Greco-Persian Wars*  
The **allied Greeks** followed up their success by destroying the rest of the **Persian fleet** at the **Battle** of Mycale, before expelling **Persian garrisons** from **Sestos** (479 BC) and **Byzantium** (478 BC).

1078: what is a day care for? *Day care*  
Some childminders **care** for children from several **families** at the same time, either in their own **home** (commonly known as "**family day care**" in Australia) or in a **specialized child care** facility.

1079: who discovered neptune the planet *Discovery of Neptune*  
Unfortunately, Le Verrier's triumph also led to a tense international dispute over priority, as, shortly after the **discovery**, George Airy, at the time British Astronomer **Royal**, announced that Adams had also predicted the **discovery of the planet**.

1081: what separates me from you album *What Separates Me from You*  
The **album** debuted on the US Billboard 200 at **number 11** with 58,000 first week sales, becoming A Day to Remember's personal best, as Homesick peaked at **number 21**.

1084: when did thomson make the plum-pudding model *Plum pudding model*  
Still, **Thomson's model** (along with a similar Saturnian ring **model** for atomic electrons, also put forward in 1904 by Nagaoka after James Clerk Maxwell's **model** of Saturn's rings), were earlier harbingers of the later and more successful solar-system-like Bohr **model** of the atom.

1085: what part of the pig is bacon *Bacon*  
Meat from other animals, such as beef, lamb, chicken, goat, or turkey, may also be cut, cured, or otherwise prepared to resemble **bacon**, and may even be referred to as "**bacon**".

1086: where did erisa come from *Employee Retirement Income Security Act*  
**ERISA** is sometimes used to refer to the full body of **laws** regulating employee benefit plans, which are found mainly in the Internal Revenue Code and **ERISA** itself.

1087: what percent of illegal immigrants are from mexico and europe *Illegal immigration to the United States*  
**Illegal immigration** to the **United States** is the act of foreign **nationals** entering the **United States**, without **government** permission and in violation of **United States** nationality law, or staying beyond the termination date of a visa, also in violation of the law.

1092: when us subprime mortgage market collapse *Subprime mortgage crisis*  
As **adjustable-rate mortgages** began to reset at **higher interest** rates (causing **higher monthly** payments), **mortgage delinquencies** soared.

1098: what type of game is heavy rain *Heavy Rain*  
It won 2010's **Game of the Year** from CNN and **Gaming** Union, and Best PS3 **Game of 2010** by GameSpy and IGN.

1099: what are superannuation contributions? *Superannuation in Australia*  
For example, **employers** are required to pay a proportion of an **employee's** salaries and wages (currently 9%) into a **super-annuation** fund, but people are encouraged to put aside **additional** funds into **superannuation**.

1102: what is a group of deer called *Deer*  
Species in the Cervidae family include white-tailed **deer**, mule **deer** such as black-tailed **deer**, **elk**, moose, red **deer**, **reindeer** (caribou), **fallow deer**, **roe deer** and chital.

1103: what state was john mccain a senator in during the 2008 election *United States presidential election, 2008*  
This **election** was also notable for being the first time in U.S. history that both **major party** candidates were sitting **U.S. Senators**, only the third time (after 1920 and 1960) that any sitting **U.S. Senator** was **elected president**, and only the second time that the **winning President** and **Vice President** (Obama and Biden) were both sitting **U.S. Senators**.

1104: when does the electoral college votes *Electoral College (United States)*  
Maine and Nebraska use the "**congressional district** method", selecting one **elector** within each **congressional** district by **popular vote** and selecting the remaining **two electors** by a statewide **popular vote**.

1105: when barack obama was born *Barack Obama*  
He began his **presidential campaign** in 2007, and in 2008, after a close **primary campaign** against Hillary Rodham Clinton, he won sufficient delegates in the Democratic Party **primaries** to receive the **presidential** nomination.

1112: what year did disney's animal kingdom lodge open *Disney's Animal Kingdom Lodge*  
**Disney's Animal Kingdom Lodge** is located in the **Animal Kingdom** Resort Area, adjacent to **Disney's Animal Kingdom**

1130: what are two languages in Nigeria? *Languages of Nigeria*  
**Nigeria's** linguistic diversity is a microcosm of Africa as a whole, encompassing three major African **languages** families: Afroasiatic, Nilo-Saharan, and Niger-Congo.

1133: what war led to Pearl Harbor *Events leading to the attack on Pearl Harbor*  
Rather than seize and fortify the islands, and wait for the inevitable US counterattack, Japan's military **leaders** instead decided on the pre-emptive **Pearl Harbor** attack, which they assumed would negate the American forces needed for the liberation and reconquest of the islands.  
A series of events led to the attack on **Pearl Harbor**.

1141: where in the world are smallpox common *Smallpox*  
The disease was originally known in English as the "pox" or "red **plague**"; the term "**smallpox**" was first used in **Britain** in the 15th century to distinguish **variola** from the "great pox" (syphilis).

|                                                                                                                                                                                                                                                                                                                                                                                                                                                                                                                  |                                             |
|------------------------------------------------------------------------------------------------------------------------------------------------------------------------------------------------------------------------------------------------------------------------------------------------------------------------------------------------------------------------------------------------------------------------------------------------------------------------------------------------------------------|---------------------------------------------|
| #1142: what year did the beatles came out with the song i wanna hold your hand<br>"I Want to <b>Hold Your Hand</b> " is a <b>song</b> by the English rock band the <b>Beatles</b> .                                                                                                                                                                                                                                                                                                                              | <i>I Want to Hold Your Hand</i>             |
| 1143: what is a gasser car<br>The <b>gasser</b> is the predecessor of the modern Funny <b>Car</b> .                                                                                                                                                                                                                                                                                                                                                                                                              | <i>Gasser (car)</i>                         |
| 1145: what tensions preceded the berlin blockade<br>During the multinational <b>occupation</b> of post-World War II <b>Germany</b> , the <b>Soviet</b> Union <b>blocked</b> the <b>Western Allies</b> ' railway, road, and canal access to the sectors of <b>Berlin</b> under <b>Allied control</b> .                                                                                                                                                                                                            | <i>Berlin Blockade</i>                      |
| 1153: who sang that song-a change is going to come<br>The <b>song</b> has gained in popularity and critical acclaim in the decades since its release, and is #12 on Rolling Stone 's 500 Greatest <b>Songs</b> of All Time .                                                                                                                                                                                                                                                                                     | <i>A Change Is Gonna Come</i>               |
| #1155: what percentage of the human body is water<br>In physiology , <b>body water</b> is the <b>water</b> content of the <b>human body</b> .                                                                                                                                                                                                                                                                                                                                                                    | <i>Body water</i>                           |
| 1158: what is a form of legal ownership<br>Given a short-sighted <b>owner</b> , however, a <b>private</b> property system can make these <b>tragedies</b> worse—for example, a <b>private owner</b> of a piece of oil-rich property, depending on his worldview, might be more interested in short-term financial gain than incremental use with an eye toward other 's concerns (e.g., those of future generations, the disenfranchised, etc.).                                                                 | <i>Ownership</i>                            |
| 1162: who wrote what's my name rhanna<br>An accompanying music <b>video</b> , directed by Philip Andelman, portrays a romantic encounter between <b>Rihanna</b> and Drake in a grocery store along with romantic <b>scenes</b> between the pair and <b>Rihanna walking</b> through Manhattan 's <b>Lower East Side</b> .                                                                                                                                                                                         | <i>What's My Name? (Rihanna song)</i>       |
| #1163: what year did isaac newton die<br>In addition to his work on the <b>calculus</b> , as a <b>mathematician</b> <b>Newton</b> contributed to the study of power series , generalised the binomial <b>theorem</b> to non-integer exponents, and developed <b>Newton's</b> method for approximating the roots of a function                                                                                                                                                                                    | <i>Isaac Newton</i>                         |
| 1164: what is a constant in math?<br>What it means for a <b>constant</b> to arise "naturally", and what makes a <b>constant</b> "interesting", is ultimately a matter of taste, and some <b>mathematical constants</b> are notable more for historical reasons than for their intrinsic mathematical interest.                                                                                                                                                                                                   | <i>Mathematical constant</i>                |
| 1178: who owns land rover<br>The ongoing commercial success of the original <b>Land Rover</b> series models, and latterly the Range <b>Rover</b> in the 1970s in the midst of BL's well documented business troubles prompted the establishment of a separate <b>Land Rover company</b> but still under the BL umbrella, remaining part of the subsequent <b>Rover Group</b> in 1988, under the <b>ownership</b> of British Aerospace after the remains of British <b>Leyland</b> were broken up and privatised. | <i>Land Rover</i>                           |
| 1180: what states have legalized prostitution<br>As with other countries, <b>prostitution</b> in the <b>United States</b> can be divided into three broad categories: <b>street prostitution</b> , <b>brothel prostitution</b> , and escort <b>prostitution</b> .                                                                                                                                                                                                                                                | <i>Prostitution in the United States</i>    |
| 1181: what states are on the east coast<br>The <b>East Coast</b> of the <b>United States</b> , also known as the <b>Eastern</b> Seaboard or the Atlantic Seaboard and commonly shortened to <b>East Coast</b> , refers to the easternmost <b>coast</b> of the <b>United States</b> along the Atlantic Ocean .                                                                                                                                                                                                    | <i>East Coast of the United States</i>      |
| #1183: when did sertraline come on the market<br><b>Sertraline</b> is primarily <b>prescribed</b> for major <b>depressive</b> disorder in adult outpatients as well as obsessive-compulsive , panic , and social anxiety disorders in both adults and children.                                                                                                                                                                                                                                                  | <i>Sertraline</i>                           |
| #1186: when did secretariat win<br><b>Secretariat's</b> grandsire, Nasrullah , is also the great-great-grandsire of 1977 Triple Crown <b>winner</b> Seattle Slew .                                                                                                                                                                                                                                                                                                                                               | <i>Secretariat (horse)</i>                  |
| 1187: what are batteries made up of<br><b>Battery</b> recycling of <b>automotive batteries</b> reduces the need for resources required for manufacture of new <b>batteries</b> , diverts toxic <b>lead</b> from landfills, and prevents risk of improper disposal.                                                                                                                                                                                                                                               | <i>Automotive battery</i>                   |
| 1189: what is a full job time?<br><b>Full-time jobs</b> are often considered careers .                                                                                                                                                                                                                                                                                                                                                                                                                           | <i>Full-time</i>                            |
| 1190: what are the three primary colors in the subtractive color model<br>A <b>subtractive color model</b> explains the mixing of a limited set of dyes , inks , paint pigments or natural <b>colorants</b> to create a wider range of <b>colors</b> , each the result of partially or completely <b>subtracting</b> (that is, absorbing) some wavelengths of light and not others.                                                                                                                              | <i>Subtractive color</i>                    |
| 1191: what are layers of the ionosphere<br>It is distinguished because it is <b>ionized</b> by solar radiation.                                                                                                                                                                                                                                                                                                                                                                                                  | <i>Ionosphere</i>                           |
| 1201: who plays as big bird<br><b>Big Bird</b> is a protagonist of the children's television show Sesame Street .                                                                                                                                                                                                                                                                                                                                                                                                | <i>Big Bird</i>                             |
| 1205: who founded walmart<br><b>Walmart</b> remains a family-owned <b>business</b> , as the company is controlled by the Walton family , who own a 48 percent stake in <b>Walmart</b> .                                                                                                                                                                                                                                                                                                                          | <i>Walmart</i>                              |
| 1206: what are some legal uses of meth<br>Both dextromethamphetamine and racemic methamphetamine are <b>Schedule II controlled substances</b> in the <b>United States</b> , and similarly the production, distribution, sale, and possession of methamphetamine is restricted or <b>illegal</b> in many jurisdictions .                                                                                                                                                                                          | <i>Methamphetamine</i>                      |
| 1208: what is 6 pin din connector<br>Mini-DIN is similar to the larger, older <b>DIN connector</b> .                                                                                                                                                                                                                                                                                                                                                                                                             | <i>Mini-DIN connector</i>                   |
| 1211: where does the word baptism come from<br>While <b>John</b> the Baptist 's <b>use</b> of a deep river for his <b>baptism</b> suggests <b>immersion</b> , pictorial and archaeological evidence of <b>Christian baptism</b> from the 3rd century onward indicates that a normal form was to have the candidate stand in <b>water</b> while <b>water</b> was poured over the upper body.                                                                                                                      | <i>Baptism</i>                              |
| 1212: what school did Zach Thomas play for before making it in the NFL<br>Zachary Michael <b>Thomas</b> (born September 1, 1973) is a former American college and professional football <b>player</b> who was a linebacker in the National Football League ( <b>NFL</b> ) for thirteen seasons.                                                                                                                                                                                                                  | <i>Zach Thomas</i>                          |
| 1213: what order is the moth<br>Most of this <b>order</b> are <b>moths</b> ; there are thought to be approximately 160,000 species of <b>moth</b> (nearly ten times the number of species of butterfly), with thousands of species yet to be described.                                                                                                                                                                                                                                                          | <i>Moth</i>                                 |
| 1215: what are the uses for gui<br>The term <b>GUI</b> is restricted to the scope of two-dimensional display screens with display resolutions able to describe generic information, in the tradition of the computer <b>science</b> research at the PARC (Palo Alto Research Center).                                                                                                                                                                                                                            | <i>Graphical user interface</i>             |
| 1217: who won antm cycle 12<br><b>America's Next Top Model, Cycle 12</b> is the twelfth <b>cycle</b> of <b>America's Next Top Model</b> and the sixth <b>season</b> to air on The CW network.                                                                                                                                                                                                                                                                                                                    | <i>America's Next Top Model, Cycle 12</i>   |
| 1219: who built the globe<br>A modern reconstruction of the <b>Globe</b> , named "Shakespeare's <b>Globe</b> ", opened in 1997 approximately from the site of the original theatre.                                                                                                                                                                                                                                                                                                                              | <i>Globe Theatre</i>                        |
| 1221: what are warehouse spreadsheets used for<br>In computing , a data <b>warehouse</b> or enterprise data <b>warehouse</b> ( <b>DW</b> , <b>DWH</b> , or <b>EDW</b> ) is a database <b>used</b> for <b>reporting</b> and data <b>analysis</b> .                                                                                                                                                                                                                                                                | <i>Data warehouse</i>                       |
| 1224: Who Started the Mormon Church<br>Today <b>Mormons</b> are understood to be <b>members</b> of The <b>Church</b> of Jesus <b>Christ</b> of <b>Latter-day Saints</b> ( <b>LDS Church</b> ).                                                                                                                                                                                                                                                                                                                   | <i>Mormons</i>                              |
| 1226: what part of the earth's structure is believed to consist of tectonic plates<br><b>Plate tectonics</b> (from the Late Latin <b>tectonicus</b> , from the "pertaining to building") is a scientific theory that describes the large-scale <b>motions</b> of <b>Earth's lithosphere</b> .                                                                                                                                                                                                                    | <i>Plate tectonics</i>                      |
| 1232: who won the 2009 super bowl<br>The club became an unexpected <b>winner</b> during the regular <b>season</b> , compiling a 9–7 <b>record</b> , and the playoffs with the aid of head coach Ken Whisenand , who was the Steelers' offensive coordinator in <b>Super Bowl</b> XL , and the re-emergence of <b>quarterback</b> Kurt <b>Warner</b> , who was the <b>Super Bowl</b> MVP in <b>Super Bowl</b> XXXIV with his former <b>team</b> , St. Louis Rams.                                                 | <i>Super Bowl XLIII</i>                     |
| 1233: what is a popular people meter<br>The <b>People Meter</b> is an electronic method of television measurement that moved from active and diary-based to passive and <b>meter-monitored</b> .<br>Finally in 1986, Nielsen developed an electronic <b>meter</b> , <b>People Meter</b> , to solve the problem.                                                                                                                                                                                                  | <i>People meter</i>                         |
| 1235: what are the characteristics of bryophytes<br><b>Bryophytes</b> produce enclosed <b>reproductive</b> structures ( <b>gametangia</b> and sporangia), but they produce neither flowers nor seeds, <b>reproducing</b> via spores .                                                                                                                                                                                                                                                                            | <i>Bryophyte</i>                            |
| #1236: when to use semicolon<br>The <b>semicolon</b> (;) is a punctuation mark with several <b>uses</b> .<br>The modern <b>uses</b> of the <b>semicolon</b> relate either to the listing of items or to the linking of related clauses .<br>Ben Jonson was the first notable English writer to <b>use</b> the <b>semicolon</b> systematically.                                                                                                                                                                   | <i>Semicolon</i>                            |
| #1238: when did xbox release                                                                                                                                                                                                                                                                                                                                                                                                                                                                                     | <i>Xbox</i>                                 |
| Although these two are free while <b>Xbox</b> Live required a subscription, as well as broadband-only connection which was not completely adopted yet, <b>Xbox</b> Live was a success due to better servers , features such as a buddy list, and milestone titles like Halo 2 <b>released</b> in November 2004, which is the best-selling <b>Xbox</b> video game and was by far the most popular online game for years.                                                                                          |                                             |
| 1242: what is a roll play games<br>Role-playing <b>games</b> also <b>include</b> <b>single-player</b> offline role-playing video <b>games</b> in which players <b>control</b> a character or team who undertake quests, and may <b>include</b> capabilities that advance using statistical mechanics.                                                                                                                                                                                                            | <i>Role-playing game</i>                    |
| 1254: what is a forward in soccer<br>Modern team formations usually <b>include</b> one to three <b>forwards</b> ; <b>two</b> is the most common.                                                                                                                                                                                                                                                                                                                                                                 | <i>Forward (association football)</i>       |
| 1255: WHO QUALIFIES AS A DOMESTIC PARTNER IN CA<br>Initially, <b>domestic partnerships</b> enjoyed very few privileges—principally just hospital-visitation <b>rights</b> and the <b>right</b> to be claimed as a next of kin of the estate of a deceased <b>partner</b> .                                                                                                                                                                                                                                       | <i>Domestic partnership in California</i>   |
| 1256: where did mark jackson play pro basketball?<br><b>Mark A. Jackson</b> (born April 1, 1965) is an American <b>basketball coach</b> , and former player who is the current head <b>coach</b> of the Golden State Warriors of the NBA .                                                                                                                                                                                                                                                                       | <i>Mark Jackson (basketball)</i>            |
| 1267: what are stink bombs made of<br>A <b>stink bomb</b> is a device designed to create an unpleasant smell .                                                                                                                                                                                                                                                                                                                                                                                                   | <i>Stink bomb</i>                           |
| 1270: who said "A picture is worth a thousand words"?<br>The discussion of "One <b>Picture Worth Thousand Words</b> " versus "One <b>Picture Worth Ten Thousand Words</b> " Wan yen i hua and 10,000 miles worth 10,000 books is cited in Information graphics where the concept of many in different disciplines and cultures.                                                                                                                                                                                  | <i>A picture is worth a thousand words</i>  |
| 1287: what teams won super bowl<br><b>Super Bowl</b> III in 1969 was the first such game that carried the " <b>Super Bowl</b> " moniker, the names " <b>Super Bowl I</b> " and " <b>Super Bowl II</b> " were retroactively applied to the first two games.                                                                                                                                                                                                                                                       | <i>List of Super Bowl champions</i>         |
| #1288: what year was christianity introduced to sub-saharan africa<br>However, the most recent December 18, 2012 <b>Pew Forum</b> research <b>estimates</b> that in 2010, 6,010 <b>million Christians</b> , 3,270 <b>million traditional African religion</b> followers, 610,000 Muslims and 50,000 unaffiliated (no known <b>religion</b> ) people lived in South Sudan.                                                                                                                                        | <i>Christianity in Africa</i>               |
| #1295: when did expos become national<br>In the, <b>Expos</b> won a division <b>championship</b> , won their first-ever playoff series by defeating the Philadelphia Phillies, 3–2, and advanced to the <b>National League Championship Series</b> , where they would go on to lose to the Los Angeles Dodgers 3–2, in their only postseason appearance during the strike-shortened season.                                                                                                                      | <i>Washington Nationals</i>                 |
| 1296: what is a contingent fee with an attorney<br>A <b>contingent fee</b> (in the <b>United States</b> ) or conditional <b>fee</b> (in England and Wales ) is any <b>fee</b> for services provided where the <b>fee</b> is payable only if there is a favourable result.                                                                                                                                                                                                                                        | <i>Contingent fee</i>                       |
| 1297: what is a D.O. stand for medical doctor<br>Many <b>D.O.</b> physicians attend the same graduate <b>medical</b> education programs as their <b>M.D.</b> counterparts, and then take <b>M.D.</b> specialty <b>board</b> exams, while other <b>D.O.</b> graduates enter osteopathic programs and take <b>D.O.</b> specialty <b>board</b> examinations.                                                                                                                                                        | <i>Doctor of Osteopathic Medicine</i>       |
| 1307: who reports the consumer price index<br>A <b>consumer price index</b> ( <b>CPI</b> ) measures changes in the <b>price</b> level of a market basket of <b>consumer</b> goods and services purchased by households.                                                                                                                                                                                                                                                                                          | <i>Consumer Price Index</i>                 |
| 1309: what are rocker arms?<br>The effective leverage of the <b>arm</b> (and thus the force it can exert on the valve stem) is determined by the <b>rocker arm</b> ratio, the ratio of the distance from the <b>rocker arm's</b> center of rotation to the tip divided by the distance from the center of rotation to the point acted on by the camshaft or pushrod.                                                                                                                                             | <i>Rocker arm</i>                           |
| 1313: where does the return address go on mail<br>Should the <b>return address</b> be of a different state or country, the <b>mail</b> may be routed through that location for ease of <b>return</b> .                                                                                                                                                                                                                                                                                                           | <i>Return address</i>                       |
| #1314: when did steven adler play for guns and roses<br>During the 2000s, <b>Adler</b> was the drummer of the band <b>Adler's</b> Appetite , and since 2012, he has held the same position in the band <b>Adler</b> .                                                                                                                                                                                                                                                                                            | <i>Steven Adler</i>                         |
| #1327: what year was gulf war<br>The <b>war</b> is also known under other <b>names</b> , such as the Persian <b>Gulf War</b> , First <b>Gulf War</b> , <b>Gulf War</b> I, or the First Iraq <b>War</b> , before the term " <b>Iraq War</b> " became identified instead with the 2003 Iraq <b>War</b> (also referred to in the U.S. as " <b>Operation Iraqi Freedom</b> ").                                                                                                                                       | <i>Gulf War</i>                             |
| #1335: what year was elvis born<br>In 1968, after seven years away from the stage, he returned to live performance in a celebrated comeback television <b>special</b> that led to an extended <b>Las Vegas</b> concert residency and a string of profitable tours.                                                                                                                                                                                                                                               | <i>Elvis Presley</i>                        |
| 1339: where did columbus really land in 1492?<br>Though <b>Columbus</b> was not the first European explorer to reach the Americas (having been preceded by the Norse expedition led by Leif Ericson in the 11th century), <b>Columbus's</b> voyages led to the first <b>lasting</b> European contact with the Americas, inaugurating a period of European exploration, conquest, and colonization that <b>lasted</b> for several <b>centuries</b> .                                                              | <i>Christopher Columbus</i>                 |
| 1340: what is a brindle boxer<br>Boxers were <b>first</b> exhibited in a dog show for St. Bernards in Munich in 1895, the <b>first Boxer</b> club being founded during the next year.                                                                                                                                                                                                                                                                                                                            | <i>Boxer (dog)</i>                          |
| 1342: who invented the internet<br>Since the mid-1990s, the <b>Internet</b> has had a revolutionary impact on culture and <b>commerce</b> , including the rise of near-instant communication by electronic mail , instant messaging , Voice over <b>Internet</b> Protocol (VoIP) "phone calls", two-way interactive video calls , and the World <b>Wide Web</b> with its discussion forums , blogs , social networking , and online shopping sites.                                                              | <i>History of the Internet</i>              |
| #1345: when does the royal standard fly?<br>If the ancient <b>Royal Standard</b> of Scotland is flying above Holyrood <b>Palace</b> or Balmoral Castle , instead of the <b>Royal Standard</b> of the United Kingdom used in Scotland, it also indicates that the Queen is not in residence.                                                                                                                                                                                                                      | <i>Royal Standard of the United Kingdom</i> |
| 1354: what is the atmosphere on mercury<br>The existence of a <b>atmosphere</b> had been contentiously before 1974, although by that time a consensus had formed that <b>Mercury</b> , like the Moon, lacked any substantial <b>atmosphere</b> .                                                                                                                                                                                                                                                                 | <i>Atmosphere of Mercury</i>                |
| #1356: what year did the last monkeys go into space<br>Before humans <b>went</b> into <b>space</b> , several animals were <b>launched</b> into <b>space</b> , including numerous <b>monkeys</b> , so that scientists could investigate the biological effects of <b>space</b> travel .                                                                                                                                                                                                                           | <i>Monkeys in space</i>                     |
| 1364: what religion is westminster abbey<br><b>Westminster Abbey</b> is a collegiate <b>church</b> governed by the <b>Dean</b> and Chapter of <b>Westminster</b> , as established by Royal charter of Queen Elizabeth I in 1560, which <b>created</b> it as the Collegiate <b>Church</b> of St Peter <b>Westminster</b> and a Royal Peculiar under the personal jurisdiction of the Sovereign.                                                                                                                   | <i>Westminster Abbey</i>                    |
| #1365: when did coca cola first come out<br>The most common of these is Diet <b>Coke</b> , with others including <b>Caffeine-Free Coca-Cola</b> , Diet <b>Coke Caffeine-Free</b> , <b>Coca-Cola</b> Cherry , <b>Coca-Cola</b> Zero , <b>Coca-Cola</b> Vanilla , and special versions with lemon, <b>lime</b> or coffee.                                                                                                                                                                                          | <i>Coca-Cola</i>                            |
| 1366: what role do ombudsman play in the swedish government?<br>In many countries the <b>ombudsman's</b> remit extends beyond dealing with alleged maladministration to promoting and protecting <b>human rights</b> , the <b>ombudsman</b> is recognised as the national <b>human rights</b> institution .                                                                                                                                                                                                      | <i>Ombudsman</i>                            |
| 1372: who played batman in dark knight<br>Considered one of the <b>best films</b> of the 2000s and one of the <b>best superhero films</b> ever made , the <b>film</b> received <b>highly</b> positive <b>reviews</b> and <b>set</b> numerous records during its <b>theatrical</b> run.                                                                                                                                                                                                                           | <i>The Dark Knight (film)</i>               |
| 1384: who won the super in xli<br><b>Super Bowl</b> XLI was an <b>American football</b> game between the <b>American Football Conference</b> (AFC) <b>champion</b> Indianapolis <b>Colts</b> and the <b>National Football Conference</b> (NFC) <b>champion</b> Chicago Bears to decide the <b>National Football</b> League (NFL) <b>champion</b> for the 2006 <b>season</b> .                                                                                                                                    | <i>Super Bowl XLI</i>                       |
| 1389: what are the parts of plant stems?<br>In most <b>plants</b> stems are located above the soil surface but some <b>plants</b> have underground <b>stems</b> .                                                                                                                                                                                                                                                                                                                                                | <i>Plant stem</i>                           |
| #1394: what year did martin luther king die<br><b>Martin Luther King, Jr. Day</b> was established as a U.S. federal <b>holiday</b> in 1986.                                                                                                                                                                                                                                                                                                                                                                      | <i>Martin Luther King, Jr.</i>              |
| 1400: what spanish speaking countries have the most world cup titles<br>The <b>World Cup</b> is the <b>world's</b> most widely <b>viewed</b> sporting event; an <b>estimated</b> 715.1 <b>million</b> people <b>watched</b> the final match of the 2006 <b>FIFA World Cup</b> held in <b>Germany</b> .                                                                                                                                                                                                           | <i>FIFA World Cup</i>                       |
| 1402: who composed the singapore national anthem<br><b>Singaporeans</b> are especially encouraged to sing the <b>national anthem</b> on occasions of <b>national</b> celebration or <b>national</b> significance such as at the <b>National Day</b> Parade , at <b>National Day</b> observance ceremonies conducted by educational institutions and government departments, and at sporting events at which <b>Singapore</b> teams are participating.                                                            | <i>Majulah Singapura</i>                    |

|                                                                                                                                                                                                                                                                                                                                                                                                                                                                                                                                                       |                                                  |
|-------------------------------------------------------------------------------------------------------------------------------------------------------------------------------------------------------------------------------------------------------------------------------------------------------------------------------------------------------------------------------------------------------------------------------------------------------------------------------------------------------------------------------------------------------|--------------------------------------------------|
| #1411: when does v start                                                                                                                                                                                                                                                                                                                                                                                                                                                                                                                              | <i>V (2009 TV series)</i>                        |
| <b>V</b> stars Morena Baccarin , Lourdes Benedicto , Morris Chestnut , Joel Gretsch , Logan Huffman , Charles Mesure , Elizabeth Mitchell , Laura Vandervoort and <b>Scott Wolf</b> , and was executive produced by <b>Scott Rosenbaum</b> , Yves Simoneau , <b>Scott Peters</b> , and Jace Hall .                                                                                                                                                                                                                                                    |                                                  |
| #1416: when did spongebob first air                                                                                                                                                                                                                                                                                                                                                                                                                                                                                                                   | <i>SpongeBob SquarePants</i>                     |
| He teamed up with several <b>Nickelodeon</b> veterans and Rocko crew members, including creative director Derek Drymon ( Action League Now! , Hey Arnold! , and Rocko's Modern Life) writers and directors Sherm Cohen , and Dan Povenmire , writer Tim Hill , actor and writer Martin Olson , animation director Alan Smart (all from Rocko's Modern Life), and story editor Merriwether Williams ( The Angry Beavers ), who worked on the <b>series</b> for its <b>first</b> few seasons and switched to <b>SpongeBob SquarePants</b> in July 1999. |                                                  |
| 1418: what are d.o. of medicine                                                                                                                                                                                                                                                                                                                                                                                                                                                                                                                       | <i>Doctor of Osteopathic Medicine</i>            |
| Many <b>D.O. physicians</b> attend the same graduate medical education programs as their <b>M.D.</b> counterparts, and then take <b>M.D.</b> specialty <b>board</b> exams, while other <b>D.O.</b> graduates enter osteopathic programs and take <b>D.O.</b> specialty <b>board</b> examinations.                                                                                                                                                                                                                                                     |                                                  |
| 1425: what is a medallion guarantee                                                                                                                                                                                                                                                                                                                                                                                                                                                                                                                   | <i>Medallion signature guarantee</i>             |
| The United States and Canada , a <b>medallion</b> signature <b>guarantee</b> is a special signature <b>guarantee</b> for the transfer of securities .                                                                                                                                                                                                                                                                                                                                                                                                 |                                                  |
| A <b>medallion</b> signature <b>guarantee</b> is not the same as an acknowledgment by a notary public , in the sense that a "signature <b>guarantee</b> " is a certification by the institution that the signature is authentic, and an acknowledgment is a certification by a notary public attesting that the signer signed a document voluntarily.                                                                                                                                                                                                 |                                                  |
| 1438: what is "thin film" technology                                                                                                                                                                                                                                                                                                                                                                                                                                                                                                                  | <i>Thin film</i>                                 |
| <b>Thin films</b> are also used in dye-sensitized <b>solar cells</b> .                                                                                                                                                                                                                                                                                                                                                                                                                                                                                |                                                  |
| 1443: what zones are tropical                                                                                                                                                                                                                                                                                                                                                                                                                                                                                                                         | <i>Tropics</i>                                   |
| The <b>tropics</b> are also referred to as the <b>tropical zone</b> and the torrid <b>zone</b> (see geographical <b>zone</b> ) .                                                                                                                                                                                                                                                                                                                                                                                                                      |                                                  |
| 1444: what type of business is walmart                                                                                                                                                                                                                                                                                                                                                                                                                                                                                                                | <i>Walmart</i>                                   |
| <b>Walmart</b> remains a family-owned <b>business</b> , as the company is controlled by the Walton family , who own a 48 percent stake in <b>Walmart</b> .                                                                                                                                                                                                                                                                                                                                                                                            |                                                  |
| 1445: what part of the plant are avocados                                                                                                                                                                                                                                                                                                                                                                                                                                                                                                             | <i>Avocado</i>                                   |
| The <b>avocado</b> (Persea americana) is a <b>tree</b> native to Central Mexico, classified in the <b>flowering plant</b> family Lauraceae along with cinnamon , camphor and bay laurel .                                                                                                                                                                                                                                                                                                                                                             |                                                  |
| #1449: when does air bag deploy                                                                                                                                                                                                                                                                                                                                                                                                                                                                                                                       | <i>Airbag</i>                                    |
| Modern vehicles may contain multiple airbag <b>modules</b> in various side and frontal locations of the <b>passenger</b> seating positions, and sensors may <b>deploy</b> one or more airbags in an impact zone at variable rates based on the type, angle and severity of impact; the airbag is designed to only inflate in moderate to severe frontal <b>crashes</b> .                                                                                                                                                                              |                                                  |
| 1452: what are some chinese inventions                                                                                                                                                                                                                                                                                                                                                                                                                                                                                                                | <i>List of Chinese inventions</i>                |
| For the purposes of this list, <b>inventions</b> are regarded as technological firsts developed in <b>China</b> , and as such does not include foreign technologies which the <b>Chinese</b> acquired through contact, such as the windmill from the Middle East or the telescope from Early modern Europe .                                                                                                                                                                                                                                          |                                                  |
| #1457: when did ww1 begin                                                                                                                                                                                                                                                                                                                                                                                                                                                                                                                             | <i>World War I</i>                               |
| It was predominantly called the <b>World War</b> or the <b>Great War</b> from its occurrence until the start of <b>World War II</b> in 1939, and the <b>First World War</b> or <b>World War I</b> thereafter.                                                                                                                                                                                                                                                                                                                                         |                                                  |
| 1461: what two empires fought to control afghanistan                                                                                                                                                                                                                                                                                                                                                                                                                                                                                                  | <i>Afghanistan</i>                               |
| <b>Afghanistan</b> ( ; ), officially the <b>Islamic Republic of Afghanistan</b> , is a landlocked sovereign state forming part of South <b>Asia</b> , <b>Central Asia</b> , and to some extent <b>Western Asia</b> .                                                                                                                                                                                                                                                                                                                                  |                                                  |
| 1462: what triggered the civil war                                                                                                                                                                                                                                                                                                                                                                                                                                                                                                                    | <i>American Civil War</i>                        |
| The <b>American Civil War</b> (ACW), also known as the <b>War</b> between the States or <b>simply the Civil War</b> (see naming ), was a <b>civil war</b> fought from 1861 to 1865 between the United States (the "Union" or the " <b>North</b> ") and several Southern <b>slave</b> states that declared their secession and formed the Confederate States of <b>America</b> (the "Confederacy" or the "South") .                                                                                                                                    |                                                  |
| 1466: who owns youtube                                                                                                                                                                                                                                                                                                                                                                                                                                                                                                                                | <i>Youtube</i>                                   |
| Most of the content on <b>YouTube</b> has been uploaded by individuals, although media corporations including CBS , the BBC , Vevo , Hulu , and other organizations offer some of their material via the site, as part of the <b>YouTube</b> partnership program.                                                                                                                                                                                                                                                                                     |                                                  |
| 1468: what are tires made of                                                                                                                                                                                                                                                                                                                                                                                                                                                                                                                          | <i>Tire</i>                                      |
| Metal <b>tires</b> are still used on locomotives and railcars , and solid rubber (or other polymer) <b>tires</b> are still used in various non-automotive applications, such as some casters , carts , lawnmowers , and wheelbarrows .                                                                                                                                                                                                                                                                                                                |                                                  |
| 1469: who killed general warren in bunker hill                                                                                                                                                                                                                                                                                                                                                                                                                                                                                                        | <i>Joseph Warren</i>                             |
| <b>Warren</b> had been commissioned a Major <b>General</b> in the colony's militia shortly before the June 17, 1775 Battle of <b>Bunker Hill</b> .                                                                                                                                                                                                                                                                                                                                                                                                    |                                                  |
| His death, immortalized in John Trumbull's painting, The Death of <b>General Warren</b> at the Battle of <b>Bunker's Hill</b> , June 17, 1775, galvanized the rebel forces, and he has been memorialized in many place names in the United States.                                                                                                                                                                                                                                                                                                    |                                                  |
| 1472: where do women ejaculation exactly coming from                                                                                                                                                                                                                                                                                                                                                                                                                                                                                                  | <i>Female ejaculation</i>                        |
| The <b>exact</b> source and nature of the fluid continue to be a topic of debate among medical professionals, which is also related to doubts over the existence of the G-Spot.                                                                                                                                                                                                                                                                                                                                                                       |                                                  |
| 1473: who won the women's world cup                                                                                                                                                                                                                                                                                                                                                                                                                                                                                                                   | <i>FIFA Women's World Cup</i>                    |
| The first <b>Women's World Cup</b> tournament, named the <b>Women's World Championship</b> , was held in 1991, sixty-one years after the men's first <b>FIFA World Cup</b> tournament in 1930.                                                                                                                                                                                                                                                                                                                                                        |                                                  |
| #1478: when did texas become a state                                                                                                                                                                                                                                                                                                                                                                                                                                                                                                                  | <i>Texas</i>                                     |
| <b>Houston</b> is the <b>largest</b> city in <b>Texas</b> and the fourth-largest in the United <b>States</b> , while San Antonio is the <b>second largest</b> in the state and seventh <b>largest</b> in the United <b>States</b> .                                                                                                                                                                                                                                                                                                                   |                                                  |
| 1484: who owns smirnoff                                                                                                                                                                                                                                                                                                                                                                                                                                                                                                                               | <i>Smirnoff</i>                                  |
| <b>Smirnoff</b> products include vodka , <b>flavoured vodka</b> , and <b>malt beverages</b> .                                                                                                                                                                                                                                                                                                                                                                                                                                                         |                                                  |
| 1485: who made the matrix                                                                                                                                                                                                                                                                                                                                                                                                                                                                                                                             | <i>The Matrix</i>                                |
| The success of the film led to the <b>release</b> of two feature film sequels, both <b>written</b> and directed by the Wachowskis, <b>The Matrix Reloaded</b> and <b>The Matrix Revolutions</b> .                                                                                                                                                                                                                                                                                                                                                     |                                                  |
| 1486: what are some six sigma tools used                                                                                                                                                                                                                                                                                                                                                                                                                                                                                                              | <i>Six sigma</i>                                 |
| A <b>six sigma</b> process is one in which 99.99966% of the products manufactured are <b>statistically</b> expected to be free of defects (3.4 defects per million), although, as discussed below , this defect level corresponds to only a 4.5 <b>sigma</b> level.                                                                                                                                                                                                                                                                                   |                                                  |
| 1493: what is a bad beat in poker                                                                                                                                                                                                                                                                                                                                                                                                                                                                                                                     | <i>Bad beat</i>                                  |
| There is no consensus among <b>poker</b> players as to what exactly constitutes a <b>bad beat</b> and often players will disagree about whether a particular hand was a <b>bad beat</b> .                                                                                                                                                                                                                                                                                                                                                             |                                                  |
| 1495: what part of beef are rouladen cut from?                                                                                                                                                                                                                                                                                                                                                                                                                                                                                                        | <i>Rouladen</i>                                  |
| <b>Rouladen</b> (or Rinderroulade, singular: <b>roulade</b> ) is a German meat <b>roulade</b> usually consisting of bacon, onions, mustard and pickles wrapped in thinly sliced <b>beef</b> which is then cooked.                                                                                                                                                                                                                                                                                                                                     |                                                  |
| 1497: where does cellular respiration occur                                                                                                                                                                                                                                                                                                                                                                                                                                                                                                           | <i>Cellular respiration</i>                      |
| While the overall <b>reaction</b> is a combustion <b>reaction</b> , no single <b>reaction</b> that comprises it is a combustion <b>reaction</b> .                                                                                                                                                                                                                                                                                                                                                                                                     |                                                  |
| 1500: what is a lapping machine                                                                                                                                                                                                                                                                                                                                                                                                                                                                                                                       | <i>Lapping</i>                                   |
| The other form of <b>lapping</b> involves a softer <b>material</b> such as pitch or a ceramic for the <b>lap</b> , which is "charged" with the abrasive.                                                                                                                                                                                                                                                                                                                                                                                              |                                                  |
| The first type of <b>lapping</b> (traditionally called grinding ), typically involves rubbing a brittle <b>material</b> such as glass against a surface such as iron or glass itself (also known as the " <b>lap</b> " or grinding tool) with an abrasive such as aluminum oxide , jeweller's rouge , optician's rouge , emery , silicon carbide , diamond , etc., in between them.                                                                                                                                                                   |                                                  |
| 1502: who plays ethan in my babysitter's a vampire                                                                                                                                                                                                                                                                                                                                                                                                                                                                                                    | <i>My Babysitter's a Vampire (TV series)</i>     |
| <b>My Babysitter's a Vampire</b> ( French : Ma gardienne est un <b>vampire</b> ) is a 2011 Canadian <b>television</b> series, based on the <b>television</b> film of the same name .                                                                                                                                                                                                                                                                                                                                                                  |                                                  |
| 1513: what is a base SI unit                                                                                                                                                                                                                                                                                                                                                                                                                                                                                                                          | <i>SI base unit</i>                              |
| The International System of <b>Units (SI)</b> defines seven <b>units</b> of measure as a basic set from which all other <b>SI units</b> are derived .                                                                                                                                                                                                                                                                                                                                                                                                 |                                                  |
| #1516: when did ww1 end?                                                                                                                                                                                                                                                                                                                                                                                                                                                                                                                              | <i>World War I</i>                               |
| It was predominantly called the <b>World War</b> or the <b>Great War</b> from its occurrence until the start of <b>World War II</b> in 1939, and the <b>First World War</b> or <b>World War I</b> thereafter.                                                                                                                                                                                                                                                                                                                                         |                                                  |
| 1519: what state is area code 419                                                                                                                                                                                                                                                                                                                                                                                                                                                                                                                     | <i>Area codes 419 and 567</i>                    |
| The main <b>area code</b> , <b>419</b> , was created as one of the original <b>area codes</b> in October 1947; the overlay <b>area code</b> <b>567</b> was created on January 1, 2002.                                                                                                                                                                                                                                                                                                                                                                |                                                  |
| 1521: what is 9/11 bombings                                                                                                                                                                                                                                                                                                                                                                                                                                                                                                                           | <i>September 11 attacks</i>                      |
| The <b>fourth plane</b> , United <b>Airlines Flight</b> 93 , was targeted at the United States Capitol in Washington, D.C., but <b>crashed</b> into a field near Shanksville, Pennsylvania , after its <b>passengers</b> tried to overcome the <b>hijackers</b> .                                                                                                                                                                                                                                                                                     |                                                  |
| #1528: when did charles dickens live                                                                                                                                                                                                                                                                                                                                                                                                                                                                                                                  | <i>Charles dickens</i>                           |
| Born in <b>Portsmouth</b> , England, <b>Dickens</b> left <b>school</b> to work in a factory after his father was thrown into <b>debtors' prison</b> .                                                                                                                                                                                                                                                                                                                                                                                                 |                                                  |
| #1529: when did the civil rights movement begin                                                                                                                                                                                                                                                                                                                                                                                                                                                                                                       | <i>Civil rights movement</i>                     |
| <b>Civil rights movements</b> ranging from the global LGBT <b>rights movement</b> to the global Women's <b>rights movement</b> to various racial minority <b>rights movements</b> around the <b>world</b> continue.                                                                                                                                                                                                                                                                                                                                   |                                                  |
| 1532: who shot john lennon?                                                                                                                                                                                                                                                                                                                                                                                                                                                                                                                           | <i>Death of John Lennon</i>                      |
| <b>John Lennon</b> was an English musician who gained worldwide fame as one of the founders of The Beatles , for his subsequent solo career, and for his political activism and pacifism .                                                                                                                                                                                                                                                                                                                                                            |                                                  |
| 1534: what state is new orleans in                                                                                                                                                                                                                                                                                                                                                                                                                                                                                                                    | <i>New Orleans</i>                               |
| The <b>New Orleans metropolitan area</b> ( <b>New Orleans–Metairie–Kenner Metropolitan Statistical Area</b> ) had a population of 1,167,764 in 2010 and was the 46th largest in the United <b>States</b> .                                                                                                                                                                                                                                                                                                                                            |                                                  |
| 1535: what where the most important factors that led to the defeat of the democrates in 1968?                                                                                                                                                                                                                                                                                                                                                                                                                                                         | <i>United States presidential election, 1968</i> |
| This was the last <b>election</b> in which <b>New York</b> had the most <b>votes</b> in the <b>electoral</b> college (43 votes).                                                                                                                                                                                                                                                                                                                                                                                                                      |                                                  |
| #1537: when did kurt cobain kill himself                                                                                                                                                                                                                                                                                                                                                                                                                                                                                                              | <i>Kurt Cobain</i>                               |
| <b>Kurt Donald Cobain</b> (February 20, 1967 – <b>April 5</b> , 1994) was an American musician and <b>artist</b> , best known as the lead singer , guitarist and primary songwriter of the grunge band Nirvana .                                                                                                                                                                                                                                                                                                                                      |                                                  |
| 1538: who starred in the original true grit                                                                                                                                                                                                                                                                                                                                                                                                                                                                                                           | <i>True Grit (1969 film)</i>                     |
| <b>True Grit</b> is a 1969 American western <b>film</b> written by Marguerite Roberts and directed by Henry Hathaway .                                                                                                                                                                                                                                                                                                                                                                                                                                |                                                  |
| 1539: what is a millwright worker                                                                                                                                                                                                                                                                                                                                                                                                                                                                                                                     | <i>Milwright</i>                                 |
| Modern <b>millwrights work</b> with steel and other materials in addition to wood and must often combine the skills of several skilled trades in order to successfully fabricate industrial machinery or to assemble machines from pre-fabricated parts.                                                                                                                                                                                                                                                                                              |                                                  |
| 1548: who created the tourbillon movement?                                                                                                                                                                                                                                                                                                                                                                                                                                                                                                            | <i>Tourbillon</i>                                |
| Stuhling <b>Tourbillon Movement</b> () .                                                                                                                                                                                                                                                                                                                                                                                                                                                                                                              |                                                  |
| 1549: what is an .msi file                                                                                                                                                                                                                                                                                                                                                                                                                                                                                                                            | <i>Windows Installer</i>                         |
| The installation information, and often the <b>files</b> themselves, are packaged in installation packages , loosely relational databases structured as COM Structured Storages and <b>commonly</b> known as " <b>MSI files</b> ", from their default <b>file extension</b> .                                                                                                                                                                                                                                                                         |                                                  |
| #1550: what year did mexico gain independence from spain                                                                                                                                                                                                                                                                                                                                                                                                                                                                                              | <i>Mexican War of Independence</i>               |
| The movement, which became known as the <b>Mexican War of Independence</b> , was led by Mexican-born <b>Spaniards</b> , <b>Mestizos</b> and Amerindians who sought <b>independence from Spain</b> .                                                                                                                                                                                                                                                                                                                                                   |                                                  |
| 1553: what is a Four Lokos                                                                                                                                                                                                                                                                                                                                                                                                                                                                                                                            | <i>Four Loko</i>                                 |
| The name " <b>Four</b> " is derived from the original energy drink's <b>four</b> main ingredients: alcohol, caffeine, taurine, and guarana                                                                                                                                                                                                                                                                                                                                                                                                            |                                                  |
| 1555: what is a fret on a guitar                                                                                                                                                                                                                                                                                                                                                                                                                                                                                                                      | <i>Fret</i>                                      |
| The neck of a <b>guitar</b> showing the nut (in the background, coloured white) and first four metal <b>frets</b> .                                                                                                                                                                                                                                                                                                                                                                                                                                   |                                                  |
| #1559: what year was smokey the bear invented                                                                                                                                                                                                                                                                                                                                                                                                                                                                                                         | <i>Smokey Bear</i>                               |
| <b>Smokey Bear</b> (often called <b>Smokey the Bear</b> or <b>Smokey</b> ) is a mascot of the United States Forest Service created to educate the public about the dangers of forest fires .                                                                                                                                                                                                                                                                                                                                                          |                                                  |
| 1561: who said tv is a vast wasteland                                                                                                                                                                                                                                                                                                                                                                                                                                                                                                                 | <i>Newton N. Minow</i>                           |
| His speech referring to television as a " <b>vast wasteland</b> " is cited even as the speech has passed its 50th anniversary.                                                                                                                                                                                                                                                                                                                                                                                                                        |                                                  |
| 1575: who discovered the 2 moons of mars,Phobos and Deimos                                                                                                                                                                                                                                                                                                                                                                                                                                                                                            | <i>Moons of Mars</i>                             |
| It is possible that <b>Mars</b> may have <b>moons</b> smaller than 50 - 100 meters and a dust ring between <b>Phobos</b> and <b>Deimos</b> may be present but none have been <b>discovered</b> .                                                                                                                                                                                                                                                                                                                                                      |                                                  |
| 1580: where does angela davis currently work                                                                                                                                                                                                                                                                                                                                                                                                                                                                                                          | <i>Angela Davis</i>                              |
| <b>Angela Yvonne Davis</b> (born January 26, 1944) is an American political activist , scholar, and author.                                                                                                                                                                                                                                                                                                                                                                                                                                           |                                                  |
| 1587: who killed robert kennedy                                                                                                                                                                                                                                                                                                                                                                                                                                                                                                                       | <i>Assassination of Robert F. Kennedy</i>        |
| The <b>assassination of Robert Francis "Bobby" Kennedy</b> , a United States Senator and brother of <b>assassinated</b> President John Fitzgerald " <b>Jack</b> " <b>Kennedy</b> , took place shortly after midnight on June 5, 1968, in Los Angeles , California , during the campaign season for the United States Presidential election, 1968 .                                                                                                                                                                                                    |                                                  |
| #1589: when Harry met Sally case                                                                                                                                                                                                                                                                                                                                                                                                                                                                                                                      | <i>When Harry Met Sally...</i>                   |
| When <b>Harry Met Sally...</b> is a 1989 American romantic comedy film written by Nora Ephron and directed by Rob Reiner .                                                                                                                                                                                                                                                                                                                                                                                                                            |                                                  |
| 1590: who owns hamburger helper                                                                                                                                                                                                                                                                                                                                                                                                                                                                                                                       | <i>Hamburger Helper</i>                          |
| The <b>Hamburger Helper</b> mascot is the " <b>Helping Hand</b> ", an anthropomorphic animated , four fingered left-hand glove, which appears in the product's television commercials and on the packages.                                                                                                                                                                                                                                                                                                                                            |                                                  |
| 1591: what makes a dwarf planet                                                                                                                                                                                                                                                                                                                                                                                                                                                                                                                       | <i>Dwarf planet</i>                              |
| The exclusion of <b>dwarf planets</b> from the roster of <b>planets</b> by the IAU has been both praised and criticized; it was said to be the "right decision" by Mike Brown , who <b>discovered</b> and other new <b>dwarf planets</b> , but has been rejected by Alan Stern , who had coined the term <b>dwarf planet</b> in 1990.                                                                                                                                                                                                                 |                                                  |
| #1593: when did jack lalanne die                                                                                                                                                                                                                                                                                                                                                                                                                                                                                                                      | <i>Jack LaLanne</i>                              |
| On the occasion of <b>LaLanne's death</b> , Schwarzenegger <b>credited LaLanne</b> for being "an apostle for fitness" by inspiring "billions all over the world to <b>live</b> healthier lives," and, as governor of California , had earlier placed him on his Governor's Council on Physical Fitness.                                                                                                                                                                                                                                               |                                                  |
| 1598: who made the original care bears                                                                                                                                                                                                                                                                                                                                                                                                                                                                                                                | <i>Care Bears</i>                                |
| The <b>Care Bears</b> appeared in their own TV <b>specials</b> called <b>The Care Bears</b> in the Land Without Feelings (1983) and <b>The Care Bears</b> Battle the Freeze Machine (1984).                                                                                                                                                                                                                                                                                                                                                           |                                                  |
| #1601: when do solar eclipses happen?                                                                                                                                                                                                                                                                                                                                                                                                                                                                                                                 | <i>Solar eclipse</i>                             |
| <b>Earth's</b> orbit is called the <b>ecciptic plane</b> as the Moon's orbit must cross this <b>plane</b> in order for an <b>eclipse</b> (both <b>solar</b> as well as lunar ) to occur.                                                                                                                                                                                                                                                                                                                                                              |                                                  |
| 1606: what latitude is tropic of cancer                                                                                                                                                                                                                                                                                                                                                                                                                                                                                                               | <i>Tropic of cancer</i>                          |
| The <b>Tropic of Cancer</b> , also referred to as the Northern <b>tropic</b> , is the circle of <b>latitude</b> on the Earth that marks the most northerly position at which the Sun may appear directly overhead at its zenith .                                                                                                                                                                                                                                                                                                                     |                                                  |
| 1611: what state is the capital in                                                                                                                                                                                                                                                                                                                                                                                                                                                                                                                    | <i>List of capitals in the United States</i>     |
| In addition, each of the 50 U.S. <b>states</b> and the five principal territories of the United <b>States</b> maintains its own <b>capital</b> .                                                                                                                                                                                                                                                                                                                                                                                                      |                                                  |
| 1612: what are square diamonds called?                                                                                                                                                                                                                                                                                                                                                                                                                                                                                                                | <i>Princess cut</i>                              |
| The <b>square</b> princess cut <b>diamond</b> is usually slightly cheaper than round brilliant cut <b>diamonds</b> of the same carat weight because it retains about 80% of the rough <b>diamond</b> , as opposed to the round brilliant which retains only about 50% of the rough.                                                                                                                                                                                                                                                                   |                                                  |
| 1615: where scottsdale?                                                                                                                                                                                                                                                                                                                                                                                                                                                                                                                               | <i>Scottsdale, Arizona</i>                       |
| <b>Scottsdale</b> is bordered to the west by <b>Phoenix</b> and <b>Paradise Valley</b> , to the north by <b>Carefree</b> , to the south by <b>Tempe</b> , and to the east by Fountain Hills and the Salt River Pima-Maricopa Indian Community .                                                                                                                                                                                                                                                                                                       |                                                  |
| 1616: who has brad pitt dated                                                                                                                                                                                                                                                                                                                                                                                                                                                                                                                         | <i>Brad Pitt</i>                                 |
| In addition, <b>Pitt</b> owns a <b>production</b> company, Plan B Entertainment , whose <b>productions</b> include The Departed (2006), which won the Academy <b>Award</b> for Best Picture , and Moneyball, which garnered a Best Picture nomination.                                                                                                                                                                                                                                                                                                |                                                  |
| 1617: what is a dogs classification                                                                                                                                                                                                                                                                                                                                                                                                                                                                                                                   | <i>Dog</i>                                       |
| MDNA evidence shows an evolutionary split between the <b>modern dog's</b> lineage and the <b>modern wolf's</b> lineage around 100,000 years ago but , the oldest fossil specimens genetically linked to the <b>modern dog's</b> lineage date to approximately 33,000-36,000 years ago.                                                                                                                                                                                                                                                                |                                                  |
| 1622: what nationality is wendy williams                                                                                                                                                                                                                                                                                                                                                                                                                                                                                                              | <i>Wendy Williams</i>                            |
| She hosts a syndicated television <b>talk show</b> , <b>The Wendy Williams Show</b> .                                                                                                                                                                                                                                                                                                                                                                                                                                                                 |                                                  |
| 1626: what president was theodore roosevelt                                                                                                                                                                                                                                                                                                                                                                                                                                                                                                           | <i>Theodore Roosevelt</i>                        |
| <b>Roosevelt</b> was 42 years old when sworn in as <b>President of the United States</b> in 1901, making him the youngest <b>president</b> ever; he beat out the youngest elected <b>president</b> , John F. Kennedy , by only one year.                                                                                                                                                                                                                                                                                                              |                                                  |
| 1628: who starred in webster                                                                                                                                                                                                                                                                                                                                                                                                                                                                                                                          | <i>Webster (TV series)</i>                       |
| <b>Webster</b> is an American situation comedy that aired on ABC from <b>September</b> 16, 1983 until May 8, 1987, and in first-run syndication from <b>September</b> 21, 1987 until <b>March</b> 10, 1989.                                                                                                                                                                                                                                                                                                                                           |                                                  |
| 1633: what is a monarch to a monarchy                                                                                                                                                                                                                                                                                                                                                                                                                                                                                                                 | <i>Monarchy</i>                                  |
| The <b>monarchs of Cambodia</b> , <b>Japan</b> , Jordan, Malaysia and <b>Morocco</b> " <b>reign</b> ", but do not rule" although there is considerable variation in the amount of authority they wield.                                                                                                                                                                                                                                                                                                                                               |                                                  |
| 1637: what is an "N.M?"                                                                                                                                                                                                                                                                                                                                                                                                                                                                                                                               | <i>Newton metre</i>                              |
| The symbolic form is <b>N m</b> or <b>N·m</b> .                                                                                                                                                                                                                                                                                                                                                                                                                                                                                                       |                                                  |
| 1652: who made hubble telescope                                                                                                                                                                                                                                                                                                                                                                                                                                                                                                                       | <i>Hubble Space Telescope</i>                    |
| Although not the first space <b>telescope</b> , <b>Hubble</b> is one of the <b>largest</b> and most versatile, and is well known as both a vital research <b>tool</b> and a <b>public</b> relations boon for astronomy .                                                                                                                                                                                                                                                                                                                              |                                                  |
| #1659: when did andrea doria sink                                                                                                                                                                                                                                                                                                                                                                                                                                                                                                                     | <i>SS Andrea Doria</i>                           |
| <b>Named</b> after the 16th-century <b>Genoese</b> admiral <b>Andrea Doria</b> , the ship had a gross register tonnage of 29,100 and a capacity of about 1,200 passengers and 500 crew.                                                                                                                                                                                                                                                                                                                                                               |                                                  |
| 1673: who wrote second corinthians                                                                                                                                                                                                                                                                                                                                                                                                                                                                                                                    | <i>Second Epistle to the Corinthians</i>         |
| The <b>Second Epistle to the Corinthians</b> , often referred to as <b>Second Corinthians</b> (and <b>written</b> as 2 Corinthians), is the eighth book of the New Testament of the Bible.                                                                                                                                                                                                                                                                                                                                                            |                                                  |
| 1675: who first synthesized heroin                                                                                                                                                                                                                                                                                                                                                                                                                                                                                                                    | <i>Heroin</i>                                    |

Mexican cartels are also known to **produce** a third type of illicit **heroin**, commonly called black tar , which results from a simplified, **quicker** synthesis procedure and contains a high percentage of **morphine** derivatives other than **heroin**, such as 6-monoacetylmorphine (6-MAM).

1678: what is a wiki platform *Wiki*  
**Wikis** are powered by **wiki** software .

1686: who plays dumbledore in harry potter *Albus Dumbledore*  
**Dumbledore** is **portrayed** by Richard Harris in the **film** adaptions of **Harry Potter** and the Philosopher's **Stone** and **Harry Potter** and the **Chamber of Secrets** .

1689: what type of land is savannah *Savanna*  
**Typical tropical savanna** in Northern Australia demonstrating the high tree density and regular spacing characteristic of many **savannas**.

1695: who set the world record for women for high jump *High jump*  
 Javier Sotomayor ( Cuba ) is the current men's **record** holder with a **jump** of **set** in 1993, the longest standing **record** in the history of the men's **high jump**.

1701: where does ground pepper come from *Black pepper*  
**Peppercorns**, and the **ground pepper** derived from them, may be described simply as **pepper**, or more precisely as black **pepper** (cooked and **dried** unripe fruit), **green pepper** (**dried** unripe fruit) and **white pepper** (**dried** ripe seeds).

1707: what type of ecosystem does stingrays live in *Stingray*  
 They are classified in the suborder Myliobatoidae of the order Myliobatiformes , and consist of eight families: Hexatrygonidae (sixgill stingray), Plesiobatidae (deep water stingray), Urotrygonidae (stingarees), Urotrygonidae (round rays), Dasyatidae (whiptail stingrays), Potamotrygonidae (river stingrays), Gymnuridae (butterfly rays), and Myliobatidae (eagle rays).

1712: what religion is primary in Africa? *Religion in Africa*  
**Religious** distribution in **Africa**  
**Religion** in **Africa** is multifaceted and has been a major influence on art , culture and philosophy .

1713: who won season 2 of project runway *Project Runway (season 2)*  
**Project Runway Season 2** was the second **season** of Bravo 's successful **Project Runway** , a reality competition for fashion designers.

1715: what is a mule in coins *Mule (coin)*  
 The name derives from the **mule** , the hybrid offspring of a horse and a donkey, due to such a **coin** having two sides intended for different **coins**, much as a **mule** has parents of two different species.

1721: what is an arc in a story plot *Story arc*  
 Although **story arcs** have existed for decades, the term "**story arc**" was coined in 1988 in relation to the television series **Wiseguy** , and was quickly adapted for other uses.

1727: who sang what a wonderful world *What a Wonderful World*  
 "What a **Wonderful World**" is a song written by Bob Thiele (as "George Douglas") and George David Weiss .

1728: what month is the president inaugurated *United States presidential inauguration*  
 (Prior to the Twentieth Amendment , the **date** was **March 4**, the **day** of the year on which the Constitution of the United States first took effect in 1789; the last **inauguration** to take place on the older **date** was Franklin D. Roosevelt 's first one on **March 4**, 1933.)

1751: what are club seats *Club seating*  
**Club level seating** is a special section of **seating** in modern sports stadiums .

1766: what is a redshirt freshman football player *Redshirt (college sports)*  
 For example, a coach may choose to **redshirt a player** who is then referred to as a **redshirt freshman** or simply a **redshirt**.

1776: what year did South Africa become a team in rugby *South Africa national rugby union team*  
 The **South Africa national rugby union team** (known as the Springboks) represents **South Africa in rugby union** .

1782: who did john f kennedy run against? *John F. Kennedy*  
 After military service as **commander** of the Motor Torpedo Boats PT-109 and PT-59 during **World War II** in the **South Pacific** , **Kennedy** represented Massachusetts' 11th congressional district in the U.S. House of Representatives from 1947 to **1953** as a Democrat.

1785: what season is dexter on *Dexter (TV series)*  
 Set in Miami , the show's first **season** was largely based on the **novel** Darkly Dreaming **Dexter** , the first of the **Dexter** series novels by Jeff Lindsay .

1786: What are context effects of memory? *Context-dependent memory*  
 However, the research **literature** on context-dependent **memory** **describes** a number of different types of contextual information that may affect recall such as environmental context-dependent **memory**, state-dependent learning , **cognitive** context-dependent **memory** and **mood-congruent memory**.

1789: who won the 1998 world cup *1998 FIFA World Cup*  
 The **1998 FIFA World Cup** was the 16th **FIFA World Cup** , the **world** championship for men's national association football teams.

1791: where did the vietnamese settle in america *Vietnamese American*  
 A **Vietnamese American** ( ) is an American of **Vietnamese descent**.

1793: when did hitler kill himself *Death of Adolf Hitler*  
 Accounts differ as to the cause of **death**; one that he **died** by poison only and another that he **died** by a self-inflicted gunshot, while biting down on a cyanide capsule.

1796: when did world war 2 end *World War II*  
 With an invasion of the **Japanese** archipelago imminent, and the Soviet **Union** having declared **war** on **Japan** by invading **Manchuria** , **Japan** surrendered on 15 August **1945**, **ending the war** in Asia and cementing the total **victory** of the Allies over the Axis.

1805: who won the 1967 nba championship *1967 NBA Finals*  
 The **1967 NBA World Championship Series** was the **championship** series of the 1966-67 National Basketball Association season , and was the conclusion of the **1967 NBA Playoffs** .

1806: who make airbus *Airbus*  
**Airbus** began as a consortium of **aerospace manufacturers**, **Airbus Industrie**.

1809: who invented the television *History of television*  
 As **electronic camera** and **display tubes** were perfected, electromechanical **television** gave way to all-electronic systems in nearly all **applications**.

1812: what are the side effects for lyme disease *Lyme disease*  
**Lyme disease**, **Lyme borreliosis** is an infectious **disease** caused by at least three species of bacteria belonging to the genus **Borrelia**.

1814: who wrote the song for star wars *Star Wars music*  
 Additionally, music for **Star Wars**: The Clone **Wars** was **written** by Kevin Kiner, and further music has been composed for **Star Wars** video **games** and **works** in other media.

1822: where does ray lamontagne live *Ray lamontagne*  
 Raymond "Ray" Charles Jack **LaMontagne** ( ; born June 18, 1973) is an American singer-songwriter .

1827: who made facebook *Facebook*  
 Critics , such as **Facebook** Detox , state that **Facebook** has turned into a national obsession in the United States, resulting in vast amounts of time lost and encouraging narcissism.

1831: where do you find iodine *Iodine*  
 Because of this function, radioisotopes of **iodine** are concentrated in the thyroid gland along with nonradioactive **iodine**.

1833: what kind of people are on the show skins *Skins (UK TV series)*  
 Other ventures to expand the brand have included a failed North **American** adaptation , which **aired** on MTV in **2011** but it was **cancelled** after one season after **advertisers** abandoned the **series** in response to low **ratings** and the **significant** controversy which arose over its depiction of **teen** sexuality.

1834: who played the drums in the band cream back in 1968 *Cream (band)*  
**Cream** were inducted into the Rock and Roll **Hall of Fame** in 1993.

1837: what president made decision to buy louisiana *Louisiana Purchase*  
 The **Louisiana Purchase** ( "Sale of Louisiana" ) was the acquisition by the United States of America in 1803 of France 's claim to the territory of **Louisiana** .

1838: who sang cool jerk *Cool Jerk*  
 In the feature film Home Alone 2: Lost in New York , Uncle Frank ( Gerry Bamman ) **sings** "**Cool Jerk**" in the shower.

1839: what is a league in the sea *League (unit)*  
 A **league** is a **unit** of length (or, rarely, area ) .

1845: when will ie9 be released *Internet Explorer 9*  
 The system requirements for **Internet Explorer 9** are **Windows 7** , **Windows Server 2008 R2** , **Windows Vista Service Pack 2** or **Windows Server 2008 SP2** with the **Platform Update** .

1849: when did classification of races begin *Race (human classification)*  
 While **biologists** sometimes **use** the **concept** of **race** to make **distinctions** among fuzzy sets of traits, others in the **scientific** community suggest that the idea of **race** often is used in a naive or simplistic way, i.e. that among humans, **race** has

no taxonomic significance: all living humans belong to the same **species**, **Homo sapiens** and **subspecies**, **Homo sapiens sapiens**.

1855: what states has the electric chair *Electric chair*  
 Execution by **electrocution**, usually performed using an **electric chair**, is an execution **method** originating in the **United States** in which the condemned person is strapped to a specially built wooden **chair** and **electrocuted** through **electrodes** placed on the body.

1857: what are private labels *Private label*  
 McBride plc is an example of a European based provider of **private label** household and **personal** care products.

1866: When did the New Deal start *New Deal*  
 The **New Deal** produced a **political** realignment, making the Democratic **Party** the majority (as well as the **party** that held the White House for seven out of nine Presidential terms from 1933 to 1969), with its base in **liberal ideas**, the white **South**, traditional **Democrats**, big city machines, and the **newly** empowered labor unions and ethnic minorities.

1873: when did daylight savings time start *Daylight saving time*  
**Daylight saving time** (DST)—also summer **time** in British **English** —is the practice of advancing clocks during the lighter months so that evenings have more **daylight** and mornings have less.

1874: What region of France is Montargis in? *Montargis*  
**Montargis** is a commune in the Loiret department in north-central **France** on the Loing river.

1877: what year lord of rings made? *The Lord of the Rings*  
 The enduring **popularity** of **The Lord of the Rings** has led to numerous references in **popular culture**, the founding of many societies by fans of **Tolkien's works** , and the **publication** of many **books** about **Tolkien** and his **works**.

1878: what time will the world end on may 21 *2011 end times prediction*  
 The **2011 end times** prediction made by American Christian radio **host** Harold Camping stated that the Rapture and Judgment Day would take **place** on May **21, 2011**, and that the **end of the world** would take **place** five months later on **October 21, 2011**.

1885: what is file based system *File system*  
 Some **file systems** are "virtual", in that the "**files**" supplied are **computed** on request (e.g. procsfs) or are merely a mapping into a **different file system** used as a backing store.

1887: What political conflicts marked the presidency of William Howard Taft? *William Howard Taft*  
**William Howard Taft** (September 15, 1857 – **March 8**, 1930) was the 27th **President of the United States** (1909–1913) and later the tenth **Chief Justice of the United States** (1921–1930).

1890: what temperature is a salt ice bath *Cooling bath*  
 Cooling **baths** are generally one of two types: (a) a cold fluid (particularly liquid nitrogen , water , or even air ) — but most commonly the term refers to (b) a mixture of 3 components: (1) a cooling agent (such as **dry ice** or water **ice** ); (b) a liquid "carrier" (such as liquid water, ethylene glycol, acetone, etc.), which transfers heat between the **bath** and the vessel; ; and (c) an additive to depress the melting-point of the solid/liquid system.

1893: when slavery abolished *Slavery in the United States*  
 However, by 1804, all **states north** of the Mason and Dixon Line had either **abolished slavery** outright or **passed laws** for the gradual **abolition of slavery**.

1905: what are circumpolar constellations *Circumpolar constellation*  
 In the northern hemisphere, we will always be able to see stars and **constellations** in the northern **circumpolar** sky, while in the southern hemisphere, we will always be able to see stars and **constellations** in the southern **circumpolar** sky.

1906: where do sesame seeds come from *Sesame*  
 The world's **largest** exporter of **sesame seeds** was India, and Japan the **largest** importer.

1912: who owned kansas before it became a state *Kansas*  
 When officially opened to **settlement** by the U.S. **government** in 1854, abolitionist Free-Staters from New England and pro-slavery **settlers** from neighboring **Missouri** rushed to the territory to determine if **Kansas** would become a free **state** or a **slave state**.

1915: where did the olmecs come from *Olmec*  
 Among other "firsts", the **Olmec** appeared to practice ritual bloodletting and played the **Mesoamerican** ballgame , hallmarks of nearly all subsequent **Mesoamerican** societies.

1918: what states allow same sex marriage *Same-sex marriage in the United States*  
 The Defense of **Marriage Act** (DOMA), enacted in 1996, prevents the **federal** government from **recognizing same-sex marriages** and allows each **state** to refuse recognition of **same-sex marriages** performed in other **states**.

1923: who won the most nba championships *List of NBA players with most championships*  
 Saul **won** consecutive **championships** with the Rochester Royals and the Minneapolis Lakers in the 1950s, while **Kerr won** consecutive **championships** with the Bulls and the Spurs in the 1990s, **Horry won** seven **championships** with the Houston Rockets , the Los Angeles Lakers and the San Antonio Spurs , while **Salley won** four **championships** with the Detroit Pistons , the Bulls and the Lakers.

1925: when did the word fuck begin *Fuck*  
 In modern usage, **fuck** and its derivatives (such as **fucker** and **fucking**) can be used in the position of a noun , a verb , an adjective or an adverb .

1926: what are the 7 continents *Continent*  
 Depending on the convention and model , some **continents** may be consolidated or subdivided: for example, Eurasia is most often subdivided into Europe and Asia (red shades), while North and South America are sometimes recognized as one **American continent** (green shades).

1930: what state is milwaukee in *Milwaukee*  
 Known for its brewing traditions, major new additions to the city include the **Milwaukee** Riverwalk , the Delta Center (formerly "Frontier Airlines Center"), Miller Park , an internationally renowned addition to the **Milwaukee** Art Museum , **Milwaukee** Repertory Theater , and Pier **Wisconsin** , as well as major **renovations** to the U.S. Cellular **Arena** .

1935: what years was the 18th century *18th century*  
 To **historians** who expand the **century** to include larger **historical** movements, the "long" **18th century** may run from the Glorious **Revolution** of 1688 to the battle of Waterloo in 1815 or even later.

1937: what year was the eiffel tower made *Eiffel Tower*  
 The **Eiffel Tower** ( . ) is an **iron lattice tower** located on the Champ de Mars in Paris , **named** after the **engineer** Gustave **Eiffel** , whose company designed and built the **tower**.

1942: when monopoly came out *History of the board game Monopoly*  
 Also in the 1970s, Professor Ralph Anspach , who had himself published a board game intended to illustrate the principles of both **monopolies** and trust busting , fought Parker Brothers and its then parent company, General Mills , over the trademarks of the **Monopoly** board game.

1954: who passed no child left behind *No Child Left Behind Act*  
 The **No Child Left Behind Act of 2001** (NCLB) is a United States **Act** of Congress that is a **reauthorization of the Elementary and Secondary Education Act** , which included Title I , the government's flagship aid program for disadvantaged students.

1956: what are the charges against Casey Anthony *Death of Caylee Anthony*  
**Caylee Marie Anthony** (August 9, 2005 – **2008**) was a two-year-old American girl who **lived** in Orlando, Florida with her **mother**, **Casey Marie Anthony**, and her **maternal** grandparents, **George** and **Cindy Anthony**.

1965: where did world war I start *World War I*  
 It was predominantly called the **World War** or the **Great War** from its occurrence until the **start of World War II** in 1939, and the **First World War** or **World War I** thereafter.

1966: what species is a spider *Spider*  
 It now appears that the spiral orb **web** may be one of the earliest forms, and **spiders** that produce **tangled** cobwebs are more abundant and diverse than **orb-web spiders** .

1968: when can you use a defibrillator *Defibrillation*  
 Some external units, known as **automated** external defibrillators (AEDs), **automate** the diagnosis of treatable rhythms, meaning that lay responders or bystanders are able to **use** them successfully with little, or in some cases no training at all.

1969: who created the cato institute *Cato Institute*  
 According to the 2011 **Global Go To Think Tank** Index, **Cato** is the 6th most influential US based think **tank** , ranking 3rd in Economic Policy and 2nd in Social Policy.

1977: when does a demand curve shift? *Demand curve*  
 The **demand curve** for all consumers together follows from the **demand curve** of every individual consumer: the individual **demands** at each price are added together.

1992: Where Elephants Live *Elephant*  
 Traditionally, two species are recognised, the **African elephant** (*Loxodonta africana*) and the **Asian elephant** (*Elephas maximus*), although some evidence **suggests** that **African bush elephants** and **African forest elephants** are separate species (L. africana and L. cyclotis respectively).

1997: what are the quad muscles *Quadriceps femoris muscle*

The **quadriceps** femoris ( Latin for "four-headed **muscle** of the femur"), also called simply the **quadriceps**, **quadriceps** extensor, **quads**, is a large **muscle** group that includes the four prevailing **muscles** on the front of the thigh .

2005: when was james madison in the house of representatives  
James Madison, Jr. (March 16, 1751 (O.S. March 5) – June 28, 1836) was an American statesman and political theorist, the fourth **President** of the United States (1809–1817).  
James Madison

2007: What is and where is hydraulic fluid found and used for  
Hydraulic fluid  
**Hydraulic fluids**, also called **hydraulic liquids**, are the medium by which power is transferred in **hydraulic** machinery .

2008: Where Are Mahindra Tractors Made  
Mahindra Tractors  
**Mahindra Tractors**, the farm equipment division of **Mahindra & Mahindra** , builds and sources **tractors** that are sold worldwide across six continents.

2012: what is middle class in the us  
American middle class  
One of the first major studies of the **middle class** in **America** was White Collar: The **American Middle Classes**, published in 1951 by sociologist C. Wright Wright Mills Mills Wright Mills .

2013: what is the scientific name of the eastern tiger salamander?  
Tiger Salamander  
The proper common **name** is the **eastern tiger salamander**, to differentiate it from other closely related species.

2020: what was the steelworkers strike  
Steel strike of 1919  
The **strike** began on September 21, 1919, and **collapsed** on January 8, 1920.

2022: When was the first Mary Poppins book written  
Mary Poppins  
**Mary Poppins** is the title character of a **series** of children's **books** written by P. L. Traversers .

2024: what is sims language  
Simlish  
Initially, inspired by the Native American code talkers of World War II , **Sims** creator Will Wright and **language** expert Marc Gimpel suggested experimenting with the Navajo **language** to create Simlish.

2037: who is elizabeth from general hospital who are the boys fathers  
Elizabeth Webber  
**Elizabeth** is part of two supercouple pairings, Lucky Spencer and **Elizabeth Webber** and **Jason Morgan** and **Elizabeth Webber**.

2038: what is reagan known for  
Presidency of Ronald Reagan  
The **United States presidency** of Ronald **Reagan** , also **known** as the **Reagan** administration, was a Republican administration headed by Ronald **Reagan** from **January 20**, 1981, to **January 20**, 1989.

2040: what is evoked otoacoustic emissions  
Otoacoustic emission  
Broadly speaking, there are two types of **otoacoustic emissions**: spontaneous **otoacoustic emissions** (SOAEs), which can occur without external stimulation, and **evoked otoacoustic emissions** (EOAEs), which require an **evoking** stimulus.

2041: what is chep pallet  
CHEP  
**CHEP** offers wooden and plastic **pallets**, small display **pallets**, crates and IBC containers.

2046: when was scooby doo created  
Scooby-Doo  
This Saturday morning **cartoon** series featured four teenagers— Fred Jones , Daphne Blake , Velma Dinkley , and Norville "Shaggy" Rogers — and their talking brown Great Dane **dog** named **Scooby-Doo** , who solve **mysteries** involving supposedly **supernatural** creatures through a series of antics and missteps.

2054: who is the CEO of FACEBOOK  
Mark Zuckerberg  
In **2007**, at the age of twenty-three years, Zuckerberg became a billionaire as a result of **Facebook** and the number of **Facebook** users worldwide reached a total of one billion in 2012.

2057: What Is the Largest Whale  
Blue whale  
The blue **whale** (Balaenoptera musculus) is a marine mammal belonging to the suborder of baleen **whales** (called Mysticeti ) .

2058: What Is Range in Math  
Range (mathematics)  
This is the current usage for **range** in computer science .  
Sometimes "**range**" refers to the codomain and sometimes to the image.  
Some books say that **range** of this function is its codomain, the set of all real numbers, reflecting that the function is real-valued.  
Other books say that the **range** is the function's image, the set of non-negative real numbers, reflecting that a number can be the output of this function if and only if it is a non-negative real number.  
In this case, the larger set containing the **range** is called the codomain.  
In mathematics, the **range** of a function refers to either the codomain or the image of the function, depending upon usage.

2060: who is on the hundred dollar bill  
United States one hundred-dollar bill  
The **United States one hundred-dollar bill** (\$100) is a **denomination** of **United States** currency .

2061: what is the ingredient in mustard  
Mustard (condiment)  
The other four **mustards** pictured are a simple table **mustard** with turmeric coloring (center left), a Bavarian **swast** **mustard** (center-right), a Dijon **mustard** (lower-left), and a coarse French **mustard** made mainly from black **seed** **mustard** (lower-right).

2062: who are the members of the climax blues band?  
Climax Blues Band  
The **Climax Blues Band** (originally known as the **Climax Chicago Blues Band**) were formed in Stafford , England in 1968.

2064: when was the web invented  
World Wide Web  
With a **web browser** , one can view **web** pages that may contain text, images, videos, and other multimedia , and navigate between them via hyperlinks .

2066: what is kathmandu known for  
Kathmandu  
**Kathmandu**'s sister cities ( Lalitpur Patan ) and Bhaktapur are integral to **Kathmandu**'s cultural heritage, **tourism** industry, and **economy**; therefore UNESCO's World Heritage Site lists all three cities' monuments and attractions together under one heading, "**Kathmandu Valley**-UNESCO World Heritage Site" .

2071: where is mark sanchez from  
Mark Sanchez  
Despite a subpar performance, **Sanchez** led the Jets to the AFC **Championship Game** , a losing effort to the Indianapolis Colts , becoming the fourth rookie quarterback in NFL history to win his first playoff **game** and the second to win two playoff **games**.

2080: where is cougar town filmed  
Cougar Town  
The **show** was created by **Bill Lawrence** and Kevin **Biegel** and is **produced** by Doozer (Lawrence's company) and Coquette **Productions** in association with **ABC Studios** .

2089: where is green bay packers from  
Green Bay Packers  
The **Green Bay Packers** have won 13 league **championships** (more than any other team in the NFL), including nine NFL **championships** prior to the **Super Bowl** era and four **Super Bowl** victories—in **1967** ( **Super Bowl** I ), **1968** ( **Super Bowl** II ), **1997** ( **Super Bowl** XXXI ) and **2011** ( **Super Bowl** XLV ) .

2091: when was the world of coca cola built  
World of Coca-Cola  
Its well-known advertising as well as a host of entertainment areas and attractions, and is **located** in Atlanta , Georgia (where the company's headquarters are **located**) at Pemberton Place (named in honor of John Pemberton , the inventor of Coca-Cola ) .

2096: what is the highest mountain in america and where is it located?  
Mount McKinley  
**Mount McKinley** (also known as Denali taken from the Inuit Koyukon Athabaskan language meaning "The Great One") is the **highest mountain** peak in the United States and in North **America** with a summit **elevation** of above sea level .

2097: what was the first honda car  
Honda S600  
Available as a roadster – bearing strong resemblance to the **Honda S500** – and as a fastback coupé – introduced in March 1965 – the S600 was the **first Honda** available in two trim levels.

2100: what is the population of san francisco  
San Francisco  
**San Francisco** ( ), officially the City and County of **San Francisco**, is the leading financial and cultural center of Northern California and the **San Francisco** Bay Area .

2102: who is the writer of the beowulf poem?  
Beowulf  
**Beowulf** ( , in **Old English** or ) is the conventional title of an **Old English** heroic epic **poem** consisting of 3182 alliterative long lines , set in **Scandinavia** , commonly cited as one of the most important **works** of **Anglo-Saxon literature** .

2114: what is sherlock holmes job  
Sherlock Holmes  
The **character** grew tremendously in popularity with the first **series** of **short** stories in The Strand Magazine , beginning with A Scandal in Bohemia in 1891; further **series** of **short** stories and two novels **published** in **serial** form appeared between then and 1927.

2119: what is social security card used for  
Social Security number  
A **Social Security** number may be obtained by applying on Form SS-5, "Application for A **Social Security** Number **Card**".

2120: what is the minimalist trend  
Minimalism  
**Minimalism** is any design or **style** in which the simplest and fewest elements are used to create the maximum effect.

2126: who is the current Chief Justice of the U.S. supreme court?  
Chief Justice of the United States  
The **Chief Justice** of the United States is the **head** of the **United States** federal **court** system (the judicial branch of the federal government of the United States ) and the **chief** judge of the **Supreme Court** of the United States .

2129: when was the american labor union formed  
Labor unions in the United States  
The economist Joseph Stiglitz has asserted that, "Strong **unions** have **helped** to reduce inequality, whereas weaker **unions** have made it easier for CEOs , sometimes **working** with market forces that they have **helped** shape, to increase it."

2132: what is the largest credit union  
Navy Federal Credit Union  
Navy Federal **Credit Union** (or Navy Federal) is a **credit union** headquartered in Vienna, Virginia , chartered and regulated under the authority of the National **Credit Union** Administration (NCUA) of the U.S. federal government.

2135: what is definition of psychotic  
Psychosis  
Despite this, "**psychosis**" is generally given to noticeable deficits in normal behavior (negative signs) and more commonly to diverse **types** of **hallucinations** or **delusional beliefs** (e.g. grandiosity, **delusions** of persecution).

2136: Who is General Grievous of Star Wars  
General Grievous  
**General Grievous** is a fictional **character** in the **Star Wars** universe .

2139: where is scotty mcCreery from  
Scotty McCreery  
He also released a **Christmas album**, **Christmas** with **Scotty McCreery** , which has been certified gold.

2151: what is my resting heart rate at age 24  
Heart rate  
**Tachycardia** is defined as a **resting heart rate** above 100 **bpm**, though persistent **rest rates** between 80-100 **bpm**, mainly if they are present during sleep, may be signs of hyperthyroidism or anemia (see below).

2152: what is the name for an old horse-drawn vehicle  
Carriage  
**Working vehicles** such as the (four-wheeled) wagon and (**two-wheeled**) **cart** share important parts of the **history** of the carriage, as is the fast (**two-wheeled**) chariot .

2154: where was the tsunami in 2005  
2004 Indian Ocean earthquake and tsunami  
The resulting **tsunami** was given various **names**, including the **2004 Indian Ocean tsunami**, **South Asian tsunami**, **Indonesian tsunami**, and the **Boxing Day tsunami**.

2155: what is the source of geothermal energy  
Geothermal energy  
The **geothermal** gradient , which is the difference in temperature between the core of the **planet** and its **surface**, drives a continuous conduction of thermal **energy** in the form of heat from the core to the **surface**.

2158: who was ho chi minh in vietnam war  
Ho chi minh  
**Hồ Chí Minh** (**Northern Vietnamese** pronunciation : , Southern **Vietnamese** pronunciation : ); 19 May 1890 – 2 **September** 1969), born **Nguyễn Sinh Cung** and also known as **Nguyễn Tất Thành** and **Nguyễn Ái Quốc**, was a **Vietnamese** communist **revolutionary** leader who was prime minister (1945–1955) and president (1945–1969) of the **Democratic Republic of Vietnam** (North Vietnam).

2167: who was charged with murder after the massacre at My lai  
My Lai Massacre  
The **My Lai Massacre** ( , , , or ) was the Vietnam **War** **mass murder** of between 347 and 504 unarmed civilians in South Vietnam on **March 16**, 1968, by United States Army soldiers of "Charlie" Company of 1st **Battalion**, 20th **Infantry** Regiment , 11th Brigade of the Americal Division .

2173: what is metal music about  
Heavy metal music  
Underground scenes produced an array of more extreme, aggressive styles: thrash **metal** broke into the mainstream with bands such as Metallica , Megadeth , **Slayer** , and Anthrax , while other styles of the most extreme **subgenres** of **metal** like death **metal** and black **metal** remain subcultural phenomena.

2175: what is the title of Hobbes main work  
Thomas Hobbes  
Thomas **Hobbes** of Malmesbury (5 April 1588 – 4 December 1679), in some older texts Thomas **Hobbs** of Malmesbury, was an English philosopher, best known today for his **work** on political philosophy .

2188: what is the cabin pressure of the outflow  
Cabin pressurization  
The **cabin pressure** is regulated by the outflow **valve**.

2191: what is buttoned-down shirt?  
Dress shirt  
A **shirt**, **dress shirt**, button-front **shirt**, or button-up **shirt** is a garment with a collar , a full-length opening at the front from the collar to the hem, and sleeves with cuffs .

2192: when is administrative assistant day  
Administrative Professionals' Day  
**Administrative Professionals Day** (also known as Secretaries **Day** or Admin **Day**) is an unofficial secular holiday observed in several countries to recognize the work of secretaries , **administrative assistants**, receptionists , and other **administrative** support professionals.

2204: what is steam by valve corporation  
Steam (software)  
The **Steam** logo is a stylised left-side fly-crank and rod from the Walschaerts **valve** gear of a **steam** locomotive .

2209: what is civil engineering aBOU  
Civil engineering  
It is traditionally broken into several sub-disciplines including environmental **engineering** , geotechnical **engineering** , geophysics , geodesy , control **engineering** , structural **engineering** , biomechanics , nanotechnology , transportation **engineering** , earth science , atmospheric sciences , forensic **engineering** , municipal or urban **engineering** , water resources **engineering** , materials **engineering** , coastal **engineering** , surveying , and construction **engineering** .

2217: who was john f kennedy up against  
United States presidential election, 1960  
This election is notable as being the first time in U.S. history that two sitting U.S. Senators (**Kennedy** and **Johnson**) were elected as **president** and **vice-president**, a phenomenon that has been repeated once, by Barack **Obama** and Joe Biden in 2008 (in both cases, the **president** was the younger, more junior senator).

2221: what is the controlled substance act known as  
Controlled Substances Act  
Two **federal** agencies, the Drug Enforcement Administration and the Food and Drug Administration , determine which **substances** are added to or removed from the various **schedules**, though the **statute passed** by Congress created the initial listing, and Congress has sometimes **scheduled** other **substances** through legislation such as the Hillory J. Farias and Samantha Reid Date-Rape **Prevention Act** of 2000, which placed gamma hydroxybutyrate in **Schedule** 1. Classification decisions are **required** to be made on criteria including potential for **abuse** (an undefined term), currently accepted medical use in treatment in the United States, and international treaties.

2226: what is the si unit of pressure  
Pressure  
While **pressure** may be **measured** in any **unit** of force divided by any **unit** of area, the **SI unit** of **pressure** (the newton per square **metre** ) is called the pascal (Pa) after the seventeenth-century philosopher and scientist Blaise Pascal .

2227: what is the great basin area  
Great Basin  
It is noted for both its **arid** conditions and its **Basin** and **range** topography that varies from the North American low point at Badwater **Basin** to the highest point of the contiguous United States , less than away at the summit of Mount **White** .

2230: when was fdr elected as president  
Franklin D. Roosevelt  
A dominant leader of the **Democratic Party** and the only **American** president **elected** to more than two **terms**, he built a **New Deal** coalition that realigned **American politics** after 1932, as his domestic policies defined **American** liberalism for the middle third of the 20th century.

2231: where was ms-13 originally from  
MS-13  
In the U.S., the **MS-13** has an especially heavy presence in Los Angeles County and the San Francisco Bay Area in Northern California; of the Washington, D.C. metropolitan areas of Fairfax County, Virginia, Montgomery County, Maryland, and Prince George's County, Maryland; Long Island, **New York**; the Boston, Massachusetts area; Charlotte, North **Carolina**; and Houston, Texas.

2234: where was the super bowl in 1991  
Super Bowl XXI  
The Bills and their explosive no-huddle offense were making their first **Super Bowl** appearance after finishing the regular **season** with a 13-3 record, and leading the league in total points scored with 428.

2235: **Super Bowl** XXV was an American football game between the American Football Conference (AFC) champion Buffalo Bills and the National Football Conference (NFC) champion New York Giants to decide the National Football League (NFL) champion for the 1990 **season** .  
In advancing to their second **Super Bowl**, the Giants also posted a 13-3 regular **season** record, but with a ball-control offense and a defense that allowed a league low 211 points.

2237: who are the characters in 90210 in season 3  
90210 (season 3)  
Christmas-themed episode "Holiday Madness", hit **season** highs in all key **demos** with 2.1 in The CW's target **demo** of women 18–34, a 1.4 in **adults** 18–34 and a 1.1 in **adults** 18–49.

2238: when was queen elizabeth ii married  
Elizabeth II  
There have been times of **personal** sorrow for her which include the **death** of her **father** at 56, the assassination of **Prince Philip**'s uncle, Lord Mountbatten, the breakdown of her **children's marriages** in 1992 (a year deemed her annus horribilis ) , the **death** in 1997 of her former daughter-in-law, Diana, **Princess** of Wales , and the **deaths** of her **mother** and sister in **2002**.

2249: who is the singer westlife  
Westlife  
**Westlife** sold over 50 **million** records **worldwide**, a **total** that **included** studio albums, singles, video releases, and compilation albums.

2250: what is vitamin a for  
Vitamin A  
The associated acid (retinoic acid), a metabolite that can be irreversibly synthesized from **vitamin** A, has only partial **vitamin** A activity, and does not function in the retina for the visual cycle.

2254: when is it memorial day  
Memorial Day  
**Memorial Day** is not to be confused with Veterans **Day** ; **Memorial Day** is a **day** of remembering the men and women who died while serving, while Veterans **Day** celebrates the service of all U.S. military veterans, living or dead.

2259: what is the function of the liver  
Liver  
The **liver** is necessary for survival; there is currently no way to compensate for the absence of **liver function** in the long **term**, although new **liver** dialysis techniques can be used in the short **term**.

2261: what is the formula for calcium nitrate  
Calcium nitrate

A variety of related salts are known including **calcium ammonium nitrate** decahydrate and **calcium potassium nitrate** decahydrate.

2262: where is día de los muertos celebrated *Day of the Dead*  
The holiday has spread throughout the world. In Brazil, **Dia de Finados** is a public holiday that many Brazilians **celebrate** by visiting cemeteries and **churches**.

2263: where is the 2011 mlb all star game location *2011 Major League Baseball All-Star Game*  
The **2011 Major League Baseball All-Star Game** was the 82nd in-season exhibition **game** between the All-Stars of the National **League** (NL) and the American **League** (AL); the **leagues** composing **Major League Baseball**.

2267: where is the island New Guinea? *New Guinea*  
The Germans **annexed** the northern coast of the **eastern** half of the **island** as German **New Guinea** in their pre-World War I effort to establish themselves as a **colonial** power, whilst the south **eastern** portion was reluctantly **claimed** by Britain.

2272: what is in milk *Milk*  
New Zealand, the European Union's 27 member states, Australia, and the **United States** are the world's largest exporters of **milk** and **milk** products.

2273: What is motorcycle speedway racing *Motorcycle speedway*  
On average, in adult human males, the plasma concentration of **testosterone** is about 7–8 times as great as the concentration in adult human females' plasma, but as the metabolic consumption of **testosterone** in males is greater, the daily **production** is about 20 times greater in men.

2289: where are the most concentration of jews living *Jews*  
Converts to Judaism, whose status as **Jews** within the **Jewish** ethnos is equal to those born into it, have been absorbed into the **Jewish** people throughout the millennia.

2293: who was the first european in the americas *European colonization of the Americas*  
In 1497, sailing from the **north** on behalf of England, John Cabot landed on the **North American coast**, and a year later, **Columbus's** third voyage **reached** the South **American coast**.

2295: where is testosterone produced *Testosterone*  
Its **compounds** are commonly encountered as copper(II) **salts**, which often impart **blue** or green colors to minerals such as azurite and turquoise and have been widely used historically as pigments.

2301: what was the parthenon used for *Parthenon*  
In the 5th century AD, the **Parthenon** was converted into a **Christian church** dedicated to the **Virgin Mary**.

2307: when was jamestown colonized *Jamestown, Virginia*  
**Historic Jamestowne**, the archaeological **site** on **Jamestown Island**, is a cooperative effort by **Jamestown National Historic Site** (part of Colonial National **Historical Park**), and **Preservation Virginia**.

2308: what was the first year of kentucky derby *Kentucky Derby*  
The **Kentucky Derby** ( ) is a Grade I **stakes** race for three-year-old Thoroughbreds, held annually in Louisville, **Kentucky, United States**, on the **first Saturday** in May, capping the two-week-long **Kentucky Derby Festival**.

2311: who is on the \$10. bill *United States ten-dollar bill*  
The source of the face on the **\$10 bill** is John Trumbull's 1805 portrait of **Hamilton** that belongs to the portrait collection of New York City Hall.

2318: who is norah jones parents *Norah Jones*  
**Norah Jones** (born Geetali **Norah Jones Shankar**; **March 30, 1979**) is an **American** singer-songwriter, pianist, and actress.

2325: what is Carbon 14 dating is a type of? *Carbon-14*  
There are three naturally occurring isotopes of **carbon** on Earth: 99% of the **carbon** is **carbon-12**, 1% is **carbon-13**, and **carbon-14** occurs in trace amounts, i.e., making up about 1 part per trillion (0.000000001%) of the **carbon** in the atmosphere.

2331: when was the battle at tombstone fought *Gunfight at the O.K. Corral*  
The gunfight, believed to have lasted only about thirty seconds, was **fought** between the **outlaw** Cowboys **Billy Clabberne**, **Ike** and **Billy Clanton**, and Tom and Frank McLary, and the opposing town **Marshal** Virgil Earp and his brothers Assistant Town **Marshal** Morgan and temporary lawman Wyatt, aided by Doc **Holliday** designated as a temporary **marshal** by Virgil.

2335: what is the population of algoma wi for 2010 *Algoma, Wisconsin*  
**See** also the **Town of Algoma** in **Winnebago County, Wisconsin**.

2349: who is Dr. JB Danquah *J. B. Danquah*  
During his political career, he was one of the primary opposition **leaders** to Ghanaian president and independence leader Kwame Nkrumah.

2356: where is kj 52 from *KJ-52*  
The "**KJ**" part of his **name** refers to his old rap alias, "King J. Mac," a **name** which he later described in one of his podcasts as "horribly cheesy."

2360: what is the prognosis of stomach cancer *Stomach cancer*  
**Stomach cancer**, or **gastric cancer**, refers to **cancer** arising from any part of the **stomach**.

2367: what is el mate *Mate (beverage)*  
"Tea-bag" type infusions of **mate** (**mate cocido**) have been on the market in Argentina, Paraguay and Uruguay for many years under such trade names as "Taragüi Vitality" in Argentina, "Pajarito" and "Kurupi" in Paraguay, and in Brazil under the name "**Mate Leão**".

2369: what is dave batista doing now *Dave Batista*  
David Michael "**Dave**" Bautista, Jr. (born January 18, 1969), is an American mixed martial artist, bodybuilder, actor, and former professional wrestler best known for his time in World Wrestling Entertainment competing under the ring name **Batista**.

2371: where is the arctic circle located on the earth *Arctic circle*  
In fact, because of atmospheric refraction and mirages, and because the sun appears as a disk and not a point, part of the midnight sun may be seen on the night of the northern summer solstice up to about 50' ( ) south of the **Arctic Circle**; similarly, on the day of the northern winter solstice, part of the sun may be seen up to about 50' north of the **Arctic Circle**.

2375: what is the erb/heart *Erb's point (cardiology)*  
**Heart** valves are labeled with "B", "T", "A", and "P". First **heart** sound: caused by atrioventricular valves - Bicuspid/Mitral (B) and Tricuspid (T).  
Second **heart** sound caused by semilunar valves - Aortic (A) and Pulmonary/Pulmonic (P).  
Front of thorax, showing surface relations of bones, lungs (purple), pleura (blue), and **heart** (red outline).

2377: when was pokemon first started *Pokémon*  
The term **Pokémon**, in addition to referring to the **Pokémon franchise** itself, also collectively refers to the 649 fictional species that have made appearances in **Pokémon** media as of the **release** of the fifth generation titles **Pokémon Black 2** and **White 2**; with the upcoming **releases** of **Pokémon X** and **Y**, **6 new Pokémon** have been featured in promotions for the **games**.

2379: where are colors on stoplight *Traffic light*  
Traffic lights alternate the right of way accorded to road users by displaying lights of a standard **color** (**red**, **yellow/amber**, and **green**) following a universal **color** code.

2392: what is mincemeat made of *Mincemeat*  
Variants of **mincemeat** are found in Australia, Brittany, Canada, northern Europe, Ireland, South Africa, the **United Kingdom** and the **United States**.

2399: what was the GE building in rockefeller plaza called before *GE Building*  
The **GE Building** is an Art Deco skyscraper that forms the centerpiece of **Rockefeller Center** in Midtown Manhattan, New York City, USA.

2400: who are the two senators of louisiana *List of United States Senators from Louisiana*  
**Louisiana** was admitted to the Union on April 30, 1812, and elects **senators** to Classes 2 and Class 3.

2408: who is st patry? *Saint Patrick's Day*  
**Saint Patrick's Day** or the Feast of **Saint Patrick** (, "the Day of the Festival of **Patrick**") is a cultural and religious holiday celebrated on 17 March.

2427: WHAT IS THE LENGTH OF A NAUTICAL MILE *Nautical mile*  
The **nautical mile** is nearly equal to a minute of latitude on a chart, so a distance measured with a chart divider can be roughly converted to **nautical miles** using the chart's latitude scale.

2431: what is firewire used for *IEEE 1394*  
Apple first included **FireWire** in some of its 1999 models, and most Apple computers since the year 2000 have included **FireWire** ports, though, as of 2013, nothing beyond the 800 version (IEEE-1394b).

2432: when was srb born *Stevie Ray Vaughan*  
As the younger **brother** of **Jimmie** Vaughan, Vaughan started playing the guitar at age seven and formed several bands that **occasionally** performed in local nightclubs.

2433: what is stent surgery *Stent*

The term may also refer to a tube used to temporarily hold such a natural conduit open to allow access for **surgery**.

2439: what is tofu made of *Tofu*  
There are many different varieties of **tofu**, including fresh **tofu** and **tofu** that has been processed in some way.

2440: Where is Bubbles the Chimp now *Bubbles (chimpanzee)*  
In 2003 the public learned that, like all captive chimpanzees, **Bubbles** had matured into a large and aggressive adult **chimp**, unsuitable as a companion animal.

2441: what is muse's lead singer's name *Muse (band)*  
**Muse** are known for their energetic and extravagant live performances and their fusion of many music genres, including space **rock**, **progressive rock**, **alternative rock**, heavy metal, classical music and electronica.

2451: when was the internet started *History of the Internet*  
The **Internet** was commercialized in 1995 when **NSFNET** was decommissioned, removing the last restrictions on the use of the **Internet** to carry **commercial** traffic.

2455: where is rolling rock brewed *Rolling Rock*  
**Rolling Rock** is a 4.6% abv pale lager launched in 1939 by the Latrobe **Brewing Company**.

2456: when was Pope Benedict XVI elected? *Pope Benedict XVI*  
Prior to becoming **pope**, he was "a major figure on the **Vatican stage** for a quarter of a century" as "one of the most respected, influential and controversial members of the College of **Cardinals**"; he had an influence "second to none when it came to **setting church priorities and directions**" as one of **Pope John Paul II**'s closest confidants.

2458: Who was John Adam's children *John Adams*  
**John Adams** (**October 30, 1735** ( O.S. **October 19, 1735**) – July 4, 1826) was the second president of the **United States** (1797–1801), having earlier served as the **first** vice president of the **United States**.

2459: who was on the 10 dollar bill *United States ten-dollar bill*  
The **\$10 bill** is the only U.S. paper currency in circulation in which the portrait faces to the left (the \$100,000 **bill** featured a portrait of Woodrow Wilson facing to the left, but was used only for intra-government transactions).

2460: what is water jet propulsion *Jetboat*  
Unlike these previous **waterjet** developments, such as Campini's and the Hanley Hydrojet, Hamilton had a specific need for a **propulsion system** to operate in very-shallow **water**, and the **waterjet** proved to be the ideal solution.

2463: who is E from entourage *Eric Murphy*  
Murphy is a fictional **character** on the comedy-drama television series **Entourage**.

2472: what is puerto rico currency *Currencies of Puerto Rico*  
The Banco Español de **Puerto Rico** was renamed **Bank of Porto Rico** and issued bills equivalent to the **United States dollar**, creating the **Puerto Rican dollar**.

2486: what is endodontic dentistry *Endodontics*  
Endodontists perform a variety of procedures including **endodontic** therapy (commonly known as "root canal therapy"), **endodontic** retreatment, **surgery**, treating cracked teeth, and treating dental trauma.

2491: who is the junior senator of ne *Kay Hagan*  
When Hagan defeated Republican **incumbent** Elizabeth Dole in the 2008 United States **Senate** election, she was the first woman to defeat an **incumbent** woman in a **Senate** election.

2492: who is heisman trophy named after *Heisman Trophy*  
The **Heisman Memorial Trophy Award** (usually known colloquially as the **Heisman Trophy** or the Heisman), is awarded annually to the player deemed the most outstanding player in collegiate **football**.

2498: what is sado masochism *Sadomasochism*  
Similarly, **sexual sadism** within the context of mutual consent should not be mistaken for acts of **sexual violence** or aggression.

2501: where are Giant Panda Bears found? *Giant Panda*  
"black and white cat-foot", also known as the **giant panda** to distinguish it from the unrelated **red panda**, is a **bear** native to central-western and south western China.

2505: what is the format of the canadian citizenship test *Canadian Citizenship Test*  
The **Canadian Citizenship Test** is a **test**, administered by **Citizenship** and Immigration **Canada** (CIC), that is required for all applicants for **Canadian citizenship** who are aged between 18 and 54 and who meet the basic requirements for **citizenship**.

2510: What is up with Kent Hovind *Kent Hovind*  
Since January 2007, **Hovind** has been serving a ten-year **prison** sentence after being convicted of 58 **federal** counts, including 12 tax offenses, one count of obstructing **federal** agents, and 45 counts of structuring **cash** transactions.

2518: where is good morning america studio *Times Square Studios*  
The **studio** is best known as the production home of ABC News' **Good Morning America** (GMA), a **morning** news and talk program and segments for GMA on ABC News Now.

2523: what is primary medicine *Primary care*  
Such a professional can be a **primary** care physician, such as a general **practitioner** or family physician, or depending on the locality, health system organization, and patient's discretion, they may see a pharmacist, a physician assistant, a **nurse practitioner**, a **nurse** (such as in the United Kingdom), a clinical officer (such as in **parts** of Africa), or an Ayurvedic or other traditional **medicine** professional (such as in **parts** of Asia).

2530: when was the first super bowl *Super Bowl*  
**Super Bowl XLV**, played in 2011, became the most-watched American television program in history, drawing an average audience of 111 million viewers and taking over the spot held by the previous year's **Super Bowl**, which itself had taken over the #1 spot held for twenty-eight **years** by the final episode of M\*A\*S\*H.

2532: what is the official language of america? *Languages of the United States*  
The situation is quite varied at the state and territorial levels, with some states mirroring the federal policy of **adopting no official language** in a **de jure** capacity, others **adopting English** alone, others **officially adopting English** as well as local **languages**, and still others **adopting** a policy of **de facto** bilingualism.

2534: where is shropshire, uk *Shropshire*  
The two **Shropshire** unitary areas (covering all of the ceremonial county), together with the authorities covering the ceremonial county of Staffordshire, comprise the "**Shropshire** and Staffordshire" NUTS 2 region.  
**Shropshire** is one of England's most rural and sparsely populated counties, with the population density of the **Shropshire** Council area being just 91/km2 (237/sq mi).

2539: what is the social norm approach? *Social Norms Approach*  
Despite the fact that college drinking is at elevated levels, the perceived amount almost always exceeds actual behavior. The **social norms approach** has shown signs of countering misperceptions, however research on **resulting changes** in behavior **resulting from changed** perceptions varies between mixed to conclusively nonexistent.

2545: what is an sd memory card reader *Memory card reader*  
There are three categories of **card readers** sorted by the type and quantity of the **card** slots: single **card reader** (e.g. 1x SD-only), multi **card reader** (e.g. 9-in-1) and series **card reader** (e.g. 4x SD only).

2547: What was Captain Ahab's Ship in the novel "Moby Dick" *Moby-Dick*  
**Ishmael** soon learns that **Ahab** has one purpose on this **voyage**: to seek out **Moby Dick**, a ferocious, enigmatic white sperm **whale**.

2563: when is halley's comet next *Halley's Comet*  
**Halley's Comet** or **Comet Halley** ( or ), officially designated 1P/**Halley**, is the best-known of the short-period **comets** and is visible from Earth every 75–76 years.

2566: what is soy made from *Soybean*  
Fat-free (**defatted**) soybean meal is a significant and cheap source of **protein** for animal feeds and many prepackaged meals; **soy vegetable oil** is another **product** of processing the soybean crop.

2569: what is linkedin used for *LinkedIn*  
**LinkedIn** reports more than 200 million acquired **users** in more than 200 countries and territories.

2596: what is captcha code *CAPTCHA*  
Although most **CAPTCHAs** are letter pictures randomly generated, many of them have become difficult even for a human to read, so picture **CAPTCHAs** were created in which a human is shown a simple test to show a picture of a certain animal (given few animal pictures), which is simple for a human being to process, and therefore easy to pick, while a bot cannot process and solve the question because although it can analyze the picture, it cannot easily guess the animal.

2611: who is in the group trinity 5 7 *Trin-i-tee 5:7*  
In 1998, the **group** released their first album entitled **Trin-i-tee 5:7** which debut at #1 on the Top Gospel charts.

2619: when is international men's day *International Men's Day*  
**International Men's Day** is celebrated in over 60 countries, including Trinidad and Tobago, Jamaica, Australia, India, China, United States, Romania, Singapore, Malta, United Kingdom, South Africa, Tanzania, **Zimbabwe**, Botswana, Seychelles, **Burundi**, Hungary, Ireland, **Isle of Man**, Ghana, **Canada**, Denmark, Norway, Austria, **Bosnia** and Herzegovina, Ukraine, France, **Italy**, Pakistan, **Cuba**, Antigua and Barbuda, **St. Kitts and Nevis**, **St. Lucia**, **Grenada** and Cayman Islands, on 19 November, and global support for the celebration is broad.

2635: when was the patriot act enacted *Patriot Act*

On May 26, 2011, President **Barack Obama** used an Autopen to **sign** the **PATRIOT Sunsets Extension Act of 2011**, a four-year extension of three key provisions in the USA **PATRIOT Act** while he was in France: **roving wiretaps**, **searches of business records** (the "library records provision"), and conducting **surveillance of "lone wolves"** — individuals suspected of terrorist-related activities not linked to terrorist groups.

#2637: when was the **tacoma bridge collapse**? *Tacoma Narrows Bridge*  
Historically, the name "**Tacoma Narrows Bridge**" has applied to the original **bridge** nicknamed "Galloping **Gertie**", which opened in July 1940 but **collapsed** because of aeroelastic flutter four months later, as well as the replacement of the original **bridge** which opened in 1950 and still stands today as the **westbound lanes** of the present-day twin **bridge** complex.

2640: what is **brown flax** *Flax*  
**Flax** (also known as **common flax** or **linseed**) (binomial name: *Linum usitatissimum*) is a member of the genus *Linum* in the family *Linaceae*.

#2669: when was the **lady gaga judas** song released *Judas (song)*  
**Gaga** has performed "**Judas**" on a **number of television shows**, including *The Graham Norton Show*, *Saturday Night Live*, *Good Morning America's "Summer Concert Series"*, the *French X Factor* as well as on *The Ellen DeGeneres Show*.

2670: what is **mpeg4 avc or sp/asp** *H.264/MPEG-4 AVC*  
The **ITU-T H.264 standard** and the **ISO/IEC MPEG-4 AVC standard (formally, ISO/IEC 14496-10 – MPEG-4 Part 10, Advanced Video Coding)** are jointly maintained so that they have identical technical content.

2685: what is the definition of a **map** *Map*  
Although most commonly used to depict geography, **maps** may represent any space, real or imagined, without regard to context or scale; e.g. **brain mapping**, **DNA mapping** and **extraterrestrial mapping**.

2688: who is on **blink 182** album cover *Enema of the State*  
Produced by **Jerry Finn**, the **album** was released on June 1, 1999 in the **United States** on **MCA Records**.

2691: What is the name of the late **Major League** old professor *Casey Stengel*  
After his **major league** career began, he acquired the **nickname "Casey"**, which originally came from the initials of his hometown ("K. C."), which evolved into "**Casey**", influenced by the wide popularity of the poem **Casey at the Bat**.

#2693: when was the **constitution written** *Constitution*  
The **Constitution** of India is the longest **written constitution** of any sovereign **country** in the world, **containing** 448 articles, 12 schedules and 100 amendments, with 117,369 words in its English language version, while the **United States Constitution** is the shortest **written constitution**, at 7 articles and 27 amendments.

2697: what is the use of a **sales invoice**? *Invoice*  
In English, the context of the term **invoice** is usually **used** to clarify its meaning, such as "We sent them an **invoice**" (they owe us money) or "We received an **invoice** from them" (we owe them money).

2698: what was the actress who played the **pink power ranger** *Kimberly Hart*  
Kimberly is best remembered as the first **Pink Ranger** and first **Pink Ninja Ranger** from the first entry of the **franchise** **Mighty Morphin Power Rangers**.

2700: what is **squash** the sport *Squash (sport)*  
The **game** was formerly called **squash racquets**, a reference to the "**squashable**" soft ball used in the **game** (compared with the fatter ball used in its parent **game racquets** or rackets).

2702: where is the **world cup in 2010** *2010 FIFA World Cup*  
The **2010 FIFA World Cup** was the 19th **FIFA World Cup**, the **world championship** for men's national association football teams.

2707: what is hosting a **website** *Web hosting service*  
The most basic is web page and small-scale **file hosting**, where **files** can be uploaded via **File Transfer Protocol (FTP)** or a Web interface.

#2708: when was the first **nfl madden** game released *Madden NFL*  
**Madden NFL** (known as **John Madden Football** before 1993) is an American **football** video **game series** developed by Electronic Arts Tiburon for **EA Sports**.

2738: what is the purpose of **child support**? *Child support*  
The 1992 United Nations Convention on the Rights of the **Child**, a binding convention signed by every member nation of the United Nations and formally ratified by all but Somalia and the United States, declares that the upbringing and development of **children** and a standard of **living** adequate for the **children's** development is a common responsibility of both parents and a fundamental human right for **children**, and asserts that the primary responsibility to provide such for the **children** rests with their parents.

2741: where was **martin luther king** shot? *Martin Luther King, Jr.*  
**Martin Luther King, Jr.** **Day** was established as a U.S. federal **holiday** in **1986**.

2747: who is the mayor of **chicago** 2011 *Chicago mayoral election, 2011*  
The city of **Chicago**, Illinois held a nonpartisan **mayoral** election on Tuesday, February 22, **2011**.

#2749: when is the **wv state fair** *State Fair of West Virginia*  
The **State Fair of West Virginia** is an **annual state fair** for **West Virginia**.

#2755: when was the **state of utah** established *Utah*  
Approximately 80% of **Utah's** 2,817,222 people live along the Wasatch Front, centering on Salt **Lake City**, leaving vast expanses of the **state** nearly uninhabited and making the **population** the sixth most urbanized in the U.S. **Utah** is bordered by **Colorado** on the east, **Wyoming** on the northeast, **Idaho** on the north, **Arizona** on the south, and **Nevada** on the west.

#2762: when is **world war hulk** movie come *World War Hulk*  
The **series** consists of five main issues titled **World War Hulk**, with Greg Pak as writer and John Romita, Jr. as penciller, and three other limited **series**: **World War Hulk: Front Line**, **World War Hulk: Gamma Corps**, and **World War Hulk: X-Men**.

2763: WHERE WAS JOHN WAYNE BORN *John Wayne*  
Marion Mitchell Morrison (**born** Marion **Robert** Morrison; May 26, 1907 – June 11, 1979), better known by his stage name **John Wayne**, was an American film **actor**, director and producer.

2765: what is the difference between **alpha lipoic acid** and **lipoic acid** *Lipoic acid*  
The carbon atom at C6 is chiral and the molecule exists as two enantiomers (R)-(+)-lipoic **acid** (RLA) and (S)-(-)-lipoic **acid** (SLA) and as a racemic mixture (R/S)-lipoic **acid** (R/S-LA).

2767: what is the organic layer in an amoled screen *OLED*  
An OLED (**organic light-emitting diode**) is a **light-emitting diode (LED)** in which the emissive **electroluminescent layer** is a film of **organic** compound which **emits light** in response to an **electric** current.

2783: what is **bourbon** made of *Bourbon whiskey*  
The name of the spirit derives from its historical association with an area known as Old **Bourbon**, around which is now **Bourbon County**, Kentucky (which, in turn, was named after the French House of **Bourbon** royal family).

2802: where is **La Palma** africa *La Palma*  
It was as a result of his visit to **La Palma** and Tenerife where he visited the **Las Cañadas** and Taburiente calderas, that the Spanish word for cauldron - "Caldera" - was introduced into the English language geological vocabulary.

2810: where was **hillary clinton** born *Hillary Rodham Clinton*  
That **election** marked the **first time** an American **First Lady** had **run** for public office; **Clinton** was also the **first** female senator to represent the **state**.

#2819: When was 27th amendment proposed *Twenty-seventh Amendment to the United States Constitution*  
The Twenty-seventh **Amendment (Amendment XXVII)** prohibits any law that increases or decreases the salary of members of the Congress from taking effect until the start of the next set of terms of office for Representatives.

2821: what is **singapore's** currency *Singapore dollar*  
The Monetary Authority of **Singapore** and the **Brunei Currency** and Monetary Board still maintain the historic exchangeability of their two **currencies**, the **Singaporean** dollar and the **Brunei** dollar, respectively.

2828: where was **paul revere** born *Paul Revere*  
Following the **war**, **Revere** returned to his **silversmith** trade and used the profits from his expanding business to finance his work in iron **casting**, bronze bell and cannon **casting**, and the forging of copper bolts and spikes.

2841: what is the type of democracy in which all citizens have the right to make government decisions *Democracy*  
One **form of democracy** is **direct democracy**, in which all eligible **citizens** have **direct** and **active** participation in the **decision making of the government**.

2847: what is ratchet from ratchet and clank *Ratchet & Clank*

The franchise was created and developed by Insomniac Games and published by Sony Computer Entertainment for many different **PlayStation** consoles, such as **PlayStation 2** and **PlayStation 3** with the exclusion of **Size Matters** and **Secret Agent Clank**, which were developed by High Impact Games for the **PlayStation Portable**.

2848: where was the first real roller coaster *roller coaster*  
Some **roller coasters**, notably wild mouse **roller coasters**, run with single cars.

2849: what is in a will *Will and testament*  
In the strictest sense, a "will" has historically been limited to **real property** while "**testament**" applies only to dispositions of **personal property** (thus giving rise to the popular title of the document as "Last Will and **Testament**"), though this distinction is seldom observed today.

2862: what is bracketing in photography *Bracketing*  
Autobracketing is automatic **bracketing** by using a setting on the camera to take several **bracketed** shots (in contrast to the **photographer** altering the settings by hand between each shot).

2869: what is the disk defragmenter tool *Defragmentation*  
**Defragmentation** is advantageous and relevant to file systems on electromechanical **disk** drives.

2870: what is level of agreement mean *Service-level agreement*  
As an example, **internet** service providers will commonly include service **level agreements** within the **terms** of their **contracts** with customers to define the level(s) of service being sold in plain language **terms**.

2883: who is the actor that plays **harry potter** *List of Harry Potter cast members*  
She **announced** that she could never have dreamt of the talented **actors** and **actresses** who have appeared in all the **Harry Potter** movies.

2884: what is the concept of "wellness"? *Wellness (alternative medicine)*  
**Wellness** grew as a popular **concept** starting in the 19th century, just as the middle class began emerging in the industrialized world, and a time when a newly prosperous public had the time and the resources to pursue **wellness** and other forms of self-improvement.

2899: what is the defensive line in football called *American football positions*  
This has resulted in the development of three "platoons" of players, the offense (the team with the ball, who is **trying** to score), the **defense** (the team **trying** to prevent the other team from scoring, and to take the ball from them), and the special teams (who play in kicking situations).

2903: what is the measurements of saturn's moons *Moons of Saturn*  
They include the seven major satellites, four small **moons** which exist in a **trojan orbit** with larger **moons**, two mutually co-orbital **moons** and two **moons** which act as shepherds of **Saturn's F Ring**.

2907: who are the girls from the bad girls club? *Bad Girls Club*  
If a "**bad girl**" breaks a rule, she is evicted from the show and, if it is early in the **season**, replaced by a new "**bad girl**".

2916: what was bernie madoff selling *Bernard Madoff*  
**Madoff** founded the Wall Street firm **Bernard L. Madoff** Investment Securities **LLC** in 1960, and was its chairman until his arrest on December 11, 2008.

2923: who is inventor of the radio *Invention of radio*  
Others, notably Guglielmo **Marconi**, were concerned with practical improvements and the commercial application of **radio** to wireless telegraphy.

2925: what is scurvy disease *Scurvy*  
Other epynoms for **scurvy** include Moeller's **disease** and Cheadle's **disease**.

2931: what is google openID *OpenID*  
An extension to the standard (the **OpenID** Attribute **Exchange**) facilitates the transfer of user attributes, such as name and gender, from the **OpenID** identity provider to the relying party (each relying party may request a different set of attributes, depending on its requirements).

2933: what is atherosclerotic heart disease *Atherosclerosis*  
Arteriosclerosis is a **general term** describing any hardening (and loss of elasticity) of medium or large **arteries** (from the Greek *arteria*, meaning **artery**, and , meaning hardening); arteriosclerosis is any hardening (and loss of elasticity) of **arteries** (small arteries); **atherosclerosis** is a hardening of an **artery** specifically due to an atheromatous plaque.

2935: what was the name of the uss john kennedy before *USS John F. Kennedy (CV-67)*  
The ship is **named** after the 35th President of the United States, **John F. Kennedy**, and is nicknamed "Big John."

2939: what were 3 important things that douglas macarthur did? *Douglas MacArthur*  
**General of the Army Douglas MacArthur** (26 January 1880s April 1964) was an American **general** and field marshal of the Philippine **Army** who was Chief of Staff of the **United States Army** during the 1930s and played a prominent **role** in the Pacific theater during World War II.

2946: what is santa's wife's name *Mrs. Claus*  
Mrs. Claus is the **wife of Santa Claus**, the Christmas gift-bringer in North American and European Christmas tradition.

#2949: when was Saddle Creek founded *Saddle Creek Records*  
**Saddle Creek** first appeared in print on a show flyer, offering to "Spend an evening with **Saddle Creek**" (later to be the title of the label's DVD).

2958: Who is the highest scoring NBA player *List of National Basketball Association season scoring leaders*  
The National **Basketball** Association's (**NBA**) **scoring** title is awarded to the **player** with the **highest** points per game average in a given season.

2961: what is direct marketing channel *Direct Marketing*  
**Direct marketing** relies on being able to **address** the members of a target **market**.

2974: what is the name of the family who own the billmore estates in nc *Billmore Estate*  
**Billmore Estate** is a large private **estate** and tourist attraction in Asheville, North Carolina.

2979: where are the kidneys in your body *Kidney*  
**Common** clinical conditions involving the **kidney** include the nephritic and nephrotic syndromes, renal cysts, acute **kidney** injury, **chronic kidney** disease, urinary tract infection, nephrolithiasis, and urinary tract obstruction.

2983: what is white chocolate made of *White chocolate*  
**White chocolate** is a **chocolate** derivative.

2986: what is the latest season of psych *Psych*  
USA renewed the series for a seventh **season**, to include 16 episodes, on January 10, **2012**, and again for an **eighth season**, to include eight episodes, on December 19, **2012**.

2990: what is the main component of vaccines *vaccine*  
**Vaccines** may be prophylactic (example: to **prevent** or ameliorate the effects of a future infection by any natural or "wild" pathogen), or therapeutic (e.g. **vaccines** against cancer are also being investigated; see cancer **vaccine**).

3005: what is in the alpine mountain systems *Alps*  
The Alps are one of the great **mountain** range **systems** of Europe stretching approximately across eight **Alpine** countries from Austria and Slovenia in the **east**, Switzerland, Liechtenstein, Germany, **France** to the **west** and Italy and Monaco to the **south**.

3008: who is mary matalin married to *Mary Matalin*  
She appears in the award-winning documentary film *Boogie Man: The Lee Atwater Story* and also played herself, opposite her husband, James **Carville**, John Slattery, and **Mary McCormack** in the short **lived** HBO series *K Street*.

3010: where is basque spoken *Basque language*  
These **provinces** and many **areas** of **Navarre** are heavily populated by ethnic Basques, but **Basque** was, at least until the 1990s, not **spoken** as a native language in most of Álava, western parts of Biscay and central and southern **areas** of **Navarre**, either because it had been replaced by **Spanish** along the centuries, in some **areas**, or because it had never been **spoken** there, in **other areas**.

3020: where is dear john filmed at *Dear John (2010 film)*  
**Dear John** is a **2010** American romantic drama - war **film** starring Amanda Seyfried and Channing Tatum.

3034: what is melissa and joey about *Melissa & Joey*  
**Melissa & Joey** is an **ABC Family** original television series starring **Melissa** Joan Hart and **Joey** Lawrence.

3039: what is the average american income *Household income in the United States*  
**Income** includes wages and salaries, unemployment insurance, disability payments, child support payments received, regular rental receipts, as well as any personal business, investment, or other kinds of **income** received routinely. As households tend to share a similar economic context, the use of household **income** remains among the most widely accepted measures of **income**.

#3042: When was Apple Computer founded *Apple Inc.*  
**Apple Inc.**, formerly **Apple Computer**, Inc., is an American **multinational corporation** headquartered in Cupertino, California that designs, **develops**, and **sells** consumer **electronics**, **computer software** and personal **computers**.

## 5 Approximate word clustering in selected Germanic languages

In this section, we present the approximate clustering algorithms for three representative Germanic languages: Danish, Dutch and German. All these three languages underwent orthographic reforms at certain points in the 20th century. We devise algorithms that accommodate to both the new and old orthographies.

It is worth mentioning that the three aforementioned Germanic languages contain some morphological features not found in English (an atypical Germanic language):

- Both Danish and German have highly inflected nouns and adjectives, and the same is true for the written standard of pre-1946 Dutch.
- Both Dutch and German verbs conjugate in the persons, and both these languages have verbs with separable prefixes.
- All these three languages allow/require a compound to be written as a single word without spaces or hyphens.

Up to minor changes, these descriptions for Dutch extend to Afrikaans (a variety of Dutch spoken in South Africa), while the features of Danish are also found in Norwegian and Swedish (two Scandinavian languages that share the same ancestor with Danish). Therefore, the algorithms presented here can be generalized to these languages with minimal modifications. We note, however, that Old Norse (the ancestral language of modern Scandinavian languages) and its conservative modern descendants (Faroese and Icelandic) have much higher morphological complexity, not yet fully captured by our current algorithms.

Like English, the Germanic strong verbs conjugate in a wide variety of “irregular” patterns. Our algorithms address the majority of these strong verbs, but do not cover all the irregularities in verb conjugation.

We will not impose the “heuristic capitalization” procedure (Definition 4.1) on any of the non-English languages treated in this document. Accordingly, all the words in a vocabulary list must be reduced to lowercase form before they are submitted to any one of our modified Porter stemming algorithm for languages other than English.

### 5.1 Modified Porter stemming algorithm for Danish

Some adverbs, articles, prepositions and pronouns occur frequently in Danish texts, while conveying very little information in their own right. They are regarded as stop words.

**Definition 5.1** (Danish stop words). If a word belongs to the following list<sup>49</sup>:

*ad, af, al, aldrig, alle, allerede, alligevel, alt, altfor, altid, anden, andet, andre, andres, at, atter, bag, bagved, bare, blandt, blev, blevet, bliv, blive, bliver, blot, bort, borte, burde, burdet, bør, både, baade, da, de, dem, den, denne, dennelunde, dens, der, deres, derfor, derfra, derhenne, derpå, derpaa, dersom, dertil, des, desto, det, dets, dette, dig, din, dine, disse, dit, dog, du, efter, efterhånden, efterhaanden, eftersom, egen, eget, egne, eller, en, én, end, endnu, endvidere, ene, eneste, enhver, enhver, ens, enten, er, et, ethvert, flere, flest, fleste, for, foran, forbi, fordi, forudsat, fra, før, førend, ganske, gennem, gjorde, gjort, gør, gøre, ham, han, hans, har, havde, have, heller, hellere, hen, hende, hendes, henne, her, herfra, herhen, herhenne, hermed, hertil, hinanden, hinsides, hos, hun, hvad, hvadenten, hvem, hver, hverken, hvert, hvilke, hvilken, hvilket, hvis, hvor, hvordan, hvorfor, hvorhen, hvorhenne, hvormed, hvorvidt, i, iblandt, idet, iflad, ifølge, igen, igennem, ihvorvel, ikke, imellem, imens, imod, ind, inde, inden, indtil, ingen, intet, ja, jeg, jer, jeres, jo, kan, kun, kunde, kunne, kunnet, langs, lidt, ligesom, ligeså, ligesaa, man, mange, mangen, med, medens, megen, meget, mellem, men, mens, mere, mest, mig, min, mine, mit, mod, må, maa, måske, maaske, måtte, maatte, måttet, maattet, ned, nede, nej, nemlig, nogen, noget, nogle, nok, nu, næmlich, nær, nærved, næsten, når, naar, nårsomhelst, naarsomhelst, ofte, oftere, oftest, ofteste, og, også, ogsaa, om, omend, omkring, omme, op, oppe, os, osv, over, overfor, ovre, på, paa, selv, selvom, siden, sidst, sidste, sig, sikken, sin, sine, sit, skal, skulde, skulle, snart, som, sommetider, straks, så, saa, sådan, saadan, sådanne, saadanne, sådant, saadant, såfremt, saafremt, således, saaledes, såvel, saavel, thi, til, tilbage, tit, trods, uagtet, ud, ude, uden, under, undertiden, undtagen, var, vi, vil, vilde, ville, villet, vor, vore, vores, vort, vær, være, været,*

then we consider it a Danish stop word. All the Danish stop words that appear in a particular document need to be ignored before we perform word clustering on the rest of the vocabulary list. □

<sup>49</sup>Our list of Danish stop words is based on [snowball.tartarus.org/algorithms/danish/stop.txt](http://snowball.tartarus.org/algorithms/danish/stop.txt), together with forms derived from substitutions  $\acute{a} \rightarrow aa$  (accommodating to pre-1948 Danish orthography).

## 5.1.1 Effective spelling and essential root

**Algorithm 5.2** (Danish effective spelling). Set  $\mathbf{V} = (a|e|i|o|u)$ . For a Danish word  $\hat{\sigma}$ , its effective spelling  $\text{EffSpell}(\hat{\sigma})$  is constructed in the following steps:

(1) Convert to lowercase, and replace<sup>50</sup>

|                |                |                |               |               |                |               |              |               |                 |              |                |
|----------------|----------------|----------------|---------------|---------------|----------------|---------------|--------------|---------------|-----------------|--------------|----------------|
| <i>dug</i>     | <i>dvikl</i>   | <i>elizaX~</i> | <i>fattig</i> | <i>formue</i> | <i>forster</i> | <i>fætter</i> | <i>hoved</i> | <i>jone</i>   | <i>klæd</i>     |              |                |
| <i>duy</i>     | <i>dbikl</i>   | <i>ελιζ</i>    | <i>πριμργ</i> | <i>φορτῦ</i>  | <i>φορστρ</i>  | <i>ῥεφθε</i>  | <i>ηεαδ</i>  | <i>γοῦε</i>   | <i>κλαδδ</i>    |              |                |
| <i>kone</i>    | <i>langsom</i> | <i>læk~</i>    | <i>mund</i>   | <i>mål</i>    | <i>ordn~</i>   | <i>peg</i>    | <i>rolig</i> | <i>sidde~</i> | <i>sider</i>    |              |                |
| <i>κοῦε</i>    | <i>σλοωm</i>   | <i>δlak</i>    | <i>μυῖδ</i>   | <i>σμαλ</i>   | <i>ωordn</i>   | <i>ποιῦτ</i>  | <i>ρωλιg</i> | <i>σιτε</i>   | <i>παγερ</i>    |              |                |
| <i>sl(og)å</i> | <i>soldat</i>  | <i>stolt</i>   | <i>sukk</i>   | <i>sum~</i>   | <i>sund</i>    | <i>synd</i>   | <i>sød</i>   | <i>tur</i>    | <i>uværdig~</i> | <i>miss</i>  | <i>s(a i)d</i> |
| <i>ζληα</i>    | <i>σολδατ</i>  | <i>στοιτζ</i>  | <i>συκκ</i>   | <i>συμm</i>   | <i>γσυῖδ</i>   | <i>τσυῖ</i>   | <i>σωιτ</i>  | <i>τυρσ</i>   | <i>ωοθλοσ</i>   | <i>ζμιοσ</i> | <i>σιτε</i>    |

(2) Replace

|                                               |                   |                                |             |              |               |             |             |              |                  |             |             |             |                             |
|-----------------------------------------------|-------------------|--------------------------------|-------------|--------------|---------------|-------------|-------------|--------------|------------------|-------------|-------------|-------------|-----------------------------|
| <i>'</i>                                      | <i>χ̂(u)fuldX</i> | <i>X<sup>ε</sup>(g l v)ent</i> | <i>ee</i>   | <i>gods~</i> | <i>guv</i>    | <i>hær</i>  | <i>hår</i>  | <i>janu~</i> | <i>kon~</i>      | <i>kær~</i> | <i>land</i> | <i>lind</i> | <i>mis<sub>χ̂</sub>(t)~</i> |
| <i>∅</i>                                      | <i>χ̂</i>         | <i>Xent</i>                    | <i>eê</i>   | <i>γοδσ</i>  | <i>γυv</i>    | <i>ηοστ</i> | <i>χαρ</i>  | <i>jnu</i>   | <i>con</i>       | <i>kær</i>  | <i>lanδ</i> | <i>lind</i> | <i>μsχ̂</i>                 |
| <i>mæssig</i>                                 | <i>part</i>       | <i>præ~</i>                    | <i>ros~</i> | <i>sol~</i>  | <i>sonet~</i> | <i>ss</i>   | <i>uge</i>  | <i>varm~</i> | <i>χ̂værdigX</i> | <i>yv</i>   | <i>ø~</i>   |             |                             |
| <i>∅</i>                                      | <i>part</i>       | <i>πρæ</i>                     | <i>ρoσ</i>  | <i>σoλ</i>   | <i>σoнет</i>  | <i>β</i>    | <i>ωeк</i>  | <i>varμ</i>  |                  | <i>χ̂</i>   | <i>oγ</i>   | <i>zxo</i>  |                             |
| <i>(liden mindre mindst mindste smaa små)</i> |                   |                                |             |              |               |             |             |              |                  |             |             |             |                             |
|                                               | <i>lille</i>      |                                |             |              |               |             |             |              |                  |             |             |             |                             |
|                                               |                   |                                |             | <i>ρωλιg</i> | <i>σσaw</i>   |             | <i>χ̂es</i> |              | <i>e</i>         |             |             | <i>e</i>    |                             |
| <i>ro(∅ en)</i>                               |                   |                                |             |              |               |             |             |              |                  |             |             |             |                             |
| <i>seen(∅ de)</i>                             |                   |                                |             |              |               |             |             |              |                  |             |             |             |                             |
| <i>~χ̂(a e i o u)tes</i>                      |                   |                                |             |              |               |             |             |              |                  |             |             |             |                             |
| <i>~isme(∅ en)</i>                            |                   |                                |             |              |               |             |             |              |                  |             |             |             |                             |
| <i>~ist(∅ en er erne)(∅ s)</i>                |                   |                                |             |              |               |             |             |              |                  |             |             |             |                             |

(3) Replace

|                                                  |                                             |                            |                                       |                                          |                  |                       |                       |                              |                                  |              |               |             |              |              |             |             |
|--------------------------------------------------|---------------------------------------------|----------------------------|---------------------------------------|------------------------------------------|------------------|-----------------------|-----------------------|------------------------------|----------------------------------|--------------|---------------|-------------|--------------|--------------|-------------|-------------|
| <i>f(a æ)d</i>                                   | <i>(here herre)~</i>                        | <i>(ond værrer værst)~</i> | <i>X<sup>ε</sup>(tagg tigg tigg)~</i> |                                          |                  |                       |                       |                              |                                  |              |               |             |              |              |             |             |
| <i>faδ</i>                                       | <i>zherre</i>                               | <i>onxved</i>              | <i>bX</i>                             |                                          |                  |                       |                       |                              |                                  |              |               |             |              |              |             |             |
| <i>X<sup>ε</sup>lege(∅ d r t)~</i>               | <i>ald~</i>                                 | <i>b(o ø)g~</i>            | <i>bild</i>                           | <i>bill~</i>                             | <i>bland~</i>    | <i>bord~</i>          | <i>bragt~</i>         | <i>bu</i>                    | <i>bøde~</i>                     | <i>dam~</i>  | <i>dans~</i>  | <i>dig~</i> | <i>dum~</i>  |              |             |             |
| <i>zzX</i>                                       | <i>gamle</i>                                | <i>kbog</i>                | <i>βild</i>                           | <i>tbill</i>                             | <i>mbland</i>    | <i>ebord</i>          | <i>bring</i>          | <i>βu</i>                    | <i>fbode</i>                     | <i>ldam</i>  | <i>danzts</i> | <i>δich</i> | <i>s dum</i> |              |             |             |
| <i>dyd~</i>                                      | <i>d(â aa)r~</i>                            | <i>fald~</i>               | <i>far~</i>                           | <i>for~</i>                              | <i>frugt~</i>    | <i>først~</i>         | <i>før~</i>           | <i>glim~</i>                 | <i>god~</i>                      | <i>grad~</i> | <i>grød~</i>  | <i>gud~</i> | <i>gæst~</i> | <i>hils~</i> |             |             |
| <i>vdyd</i>                                      | <i>δcar</i>                                 | <i>efald</i>               | <i>r far</i>                          | <i>vfor</i>                              | <i>fruct</i>     | <i>l st</i>           | <i>zxfor</i>          | <i>γlim</i>                  | <i>γod</i>                       | <i>kgrad</i> | <i>rgrød</i>  | <i>hgud</i> | <i>hgast</i> | <i>ghils</i> |             |             |
| <i>hind~</i>                                     | <i>hum</i>                                  | <i>hund~</i>               | <i>hus</i>                            | <i>hør~</i>                              | <i>iv~</i>       | <i>kald~</i>          | <i>kend~</i>          | <i>kold~</i>                 | <i>komp~</i>                     | <i>kone~</i> | <i>kun~</i>   | <i>kør~</i> | <i>lav~</i>  | <i>luk~</i>  | <i>lys~</i> | <i>løb~</i> |
| <i>χind</i>                                      | <i>hυμ</i>                                  | <i>δχund</i>               | <i>hυσs</i>                           | <i>χχor</i>                              | <i>xiv</i>       | <i>ckald</i>          | <i>kend</i>           | <i>kold</i>                  | <i>comp</i>                      | <i>wkone</i> | <i>gkun</i>   | <i>dkor</i> | <i>lav</i>   | <i>λοk</i>   | <i>xlys</i> | <i>rlob</i> |
| <i>mind~</i>                                     | <i>mini~</i>                                | <i>mørk~</i>               | <i>m(â aa)d~</i>                      | <i>ny(∅ e ere est et t)~</i>             | <i>nâ~</i>       | <i>rede~</i>          | <i>r(y ø)g~</i>       | <i>sag<sub>χ̂</sub>(d t)</i> | <i>se~</i>                       | <i>sir</i>   |               |             |              |              |             |             |
| <i>mind</i>                                      | <i>μini</i>                                 | <i>dmork</i>               | <i>wmad</i>                           |                                          | <i>wnu</i>       | <i>rna</i>            | <i>pede</i>           | <i>ρyg</i>                   | <i>zsagχ̂</i>                    | <i>zse</i>   | <i>σιρ</i>    |             |              |              |             |             |
| <i>skænd~</i>                                    | <i>smal~</i>                                | <i>smul~</i>               | <i>som~</i>                           | <i>svær</i>                              | <i>syg~</i>      | <i>søg</i>            | <i>søn</i>            | <i>til~</i>                  | <i>tro(∅ edelen ens et r s)~</i> | <i>tung~</i> |               |             |              |              |             |             |
| <i>zskand</i>                                    | <i>zmal</i>                                 | <i>xmul</i>                | <i>zom</i>                            | <i>dfsvar</i>                            | <i>σyg</i>       | <i>soeek</i>          | <i>ζon</i>            | <i>zil</i>                   | <i>gθtro</i>                     | <i>wtung</i> |               |             |              |              |             |             |
| <i>ty~</i>                                       | <i>undre~</i>                               | <i>v(â aa)gn~</i>          | <i>yngre~</i>                         | <i>(â aa)b~</i>                          | <i>(â aa)r~</i>  | <i>(gik g(â aa)r)</i> | <i>bed(re st ste)</i> | <i>f(â aa)(∅ et r)</i>       | <i>fik</i>                       |              |               |             |              |              |             |             |
| <i>θy</i>                                        | <i>wundre</i>                               | <i>wvagn</i>               | <i>ung</i>                            | <i>oabp</i>                              | <i>jår</i>       | <i>ga</i>             | <i>γod</i>            | <i>zfa</i>                   | <i>zfa</i>                       |              |               |             |              |              |             |             |
| <i>mr</i>                                        | <i>mrs</i>                                  | <i>mød(∅ t te tes)</i>     | <i>møde(∅ r rne rnes r s t ts)</i>    | <i>sag</i>                               | <i>sagtens</i>   | <i>se(∅ r s t)</i>    |                       |                              |                                  |              |               |             |              |              |             |             |
| <i>zηερpe</i>                                    | <i>zφυρ</i>                                 | <i>μod</i>                 | <i>μod</i>                            | <i>zsag</i>                              | <i>zssagtens</i> | <i>σσaw</i>           |                       |                              |                                  |              |               |             |              |              |             |             |
| <i>s(â aa)(∅ s)</i>                              | <i>ti</i>                                   | <i>ved</i>                 | <i>æld(re st ste)</i>                 | <i>~st(od (â aa)(∅ elig(∅ e t et r))</i> |                  |                       |                       |                              |                                  |              |               |             |              |              |             |             |
| <i>σσaw</i>                                      | <i>lθti</i>                                 | <i>vid</i>                 | <i>gammel</i>                         | <i>stand</i>                             |                  |                       |                       |                              |                                  |              |               |             |              |              |             |             |
| <i>~X<sup>ε</sup>(br m)(oder or)(∅ en ens s)</i> | <i>~X<sup>ε</sup>(br m)ødre(∅ ne nes s)</i> | <i>~far(∅ en ens s)</i>    | <i>~l(â aa)</i>                       |                                          |                  |                       |                       |                              |                                  |              |               |             |              |              |             |             |
| <i>Xoδ</i>                                       | <i>Xoδ</i>                                  | <i>faδ</i>                 | <i>ligger</i>                         |                                          |                  |                       |                       |                              |                                  |              |               |             |              |              |             |             |

(4) Do  $st_{\hat{\chi}}(o|\emptyset) \rightarrow sz\hat{\chi}$ ,  $vi \rightarrow vzi$ ,  $y \rightarrow u$ ,  $\text{æ} \rightarrow a$ ,  $\emptyset \rightarrow o$ ,  $(\hat{a}|aa) \rightarrow a$  and undouble characters (i.e. do  $mm \rightarrow m$  etc.);

(5) If the result so far is an empty string, stop here. Otherwise, break down the result into  $\hat{\sigma}_1\hat{\sigma}_2$ , where  $\ell(\hat{\sigma}_1) = 1$ , and work on  $\hat{\sigma}_2$  in four sequential steps:

(5.1) Do  $el \rightarrow l$ ,  $\hat{e} \rightarrow e$ ,  $riv \rightarrow irv$ ;

(5.2) Do  $\hat{\chi}_{\neq} \mathbf{V}re \rightarrow \hat{\chi}er$ ;

<sup>50</sup>To avoid confusion of Greek nu with Latin vee, we write the former as  $\tilde{\nu}$  in substitution rules.

(5.3) *Do*  $inter \rightarrow inter;$

(5.4) *Call the result so far as*  $\hat{\sigma}'_2$ . *Concatenate*  $\hat{\sigma}_1$  and  $\hat{\sigma}'_2$ .

**Definition 5.3** (Danish protected range). Set  $\mathbf{V} = (a|e|i|o|u)$ ,  $\mathbf{V}_m^* = (a|i|o|u)_m$  and  $\mathbf{C}_{m_0} = \overline{(a|e|i|o|u)}_{m_0}$ . Let  $\hat{\sigma}$  be the effective spelling of a Danish word, its protected range  $\text{ProtRg}(\hat{\sigma}) = \max\{\lambda_1(\hat{\sigma}), \lambda_2(\hat{\sigma})\}$  is determined by two non-negative integers  $\lambda_1(\hat{\sigma})$  and  $\lambda_2(\hat{\sigma})$  specified through the following procedures:

- Look for the string pattern  $(\emptyset|ab|af|be|in|\pi pa)\mathbf{C}_{m_0}(e|\mathbf{V}_m^*)(a|e|i|o|r|u)_{[0,1]}\sim$  in the string  $\hat{\sigma}$ ;<sup>51</sup>
  - If the string pattern above is found, the last position occupied by such a string defines  $\lambda_1(\hat{\sigma})$ ; otherwise, set  $\lambda_1(\hat{\sigma}) = 0$ ;
  - Do  $\sim(\emptyset|t)(\emptyset|s) \rightarrow \emptyset$  on  $\hat{\sigma}$ , and call the result  $\hat{\sigma}'$ ;
  - Look for the pattern  $(a|o|s|\beta|t|u)$  in the string  $\hat{\sigma}'$ ;
  - If a letter in the pattern above is found, the last position occupied by such a letter defines  $\lambda_2(\hat{\sigma})$ ; otherwise, set  $\lambda_2(\hat{\sigma}) = 0$ .
- 

**Algorithm 5.4** (Danish essential root). *Let*  $\hat{\sigma}$  *be the effective spelling of a Danish word, then its corresponding essential root*  $\text{EssRoot}(\hat{\sigma})$  *is constructed in the following steps:*

(1) *Break down*  $\hat{\sigma} = \hat{\sigma}_1\hat{\sigma}_2$  *into the concatenation of two strings*  $\hat{\sigma}_1 = \hat{\sigma}^{[\text{ProtRg}(\hat{\sigma})]}$  *(see the notation in Definition 3.1) and*  $\hat{\sigma}_2$ , *where the length of the first string*  $\ell(\hat{\sigma}_1) = \text{ProtRg}(\hat{\sigma})$  *is equal to the protected range of*  $\hat{\sigma}$ .

(2) *On*  $\hat{\sigma}_2$ , *perform the following substitutions in a sequel:*<sup>52</sup>

(2.1) *Do*  $\sim ne(\emptyset|s) \rightarrow \emptyset$ ;

(2.2) *Do*  $\sim e(d|e|n|r|s|t)_{m_0} \rightarrow \emptyset$ .

*The result after these two steps of operations is called*  $\hat{\sigma}'_2$ .

(3) *Concatenate*  $\hat{\sigma}_1$  and  $\hat{\sigma}'_2$ , *before doing*  $\sim s(\emptyset|t) \rightarrow \emptyset$ ;

(4) *Do*  $\sim \hat{x}^\epsilon(b|d|g|k)t \rightarrow \hat{x}$ ,  $\sim er \rightarrow e$ ,  $\sim gd \rightarrow g$ .

*Example 5.4.1.* In many cases, the essential root of a Danish word is already a very close approximation to its etymological stem. For instance, we may consider the inflected forms of two Danish nouns *datter* “daughter” and *mand* “man”, as tabulated below:

| $\hat{\sigma}$   | $\text{EffSpell}(\hat{\sigma})$ | $\text{EssRoot}(\text{EffSpell}(\hat{\sigma}))$ | $\hat{\sigma}$  | $\text{EffSpell}(\hat{\sigma})$ | $\text{EssRoot}(\text{EffSpell}(\hat{\sigma}))$ |
|------------------|---------------------------------|-------------------------------------------------|-----------------|---------------------------------|-------------------------------------------------|
| <i>datter</i>    | <i>dater</i>                    | <i>dat</i>                                      | <i>mand</i>     | <i>mand</i>                     | <i>mand</i>                                     |
| <i>datteren</i>  | <i>dateren</i>                  | <i>dat</i>                                      | <i>manden</i>   | <i>manden</i>                   | <i>mand</i>                                     |
| <i>datterens</i> | <i>daterens</i>                 | <i>dat</i>                                      | <i>mandens</i>  | <i>mandens</i>                  | <i>mand</i>                                     |
| <i>datters</i>   | <i>daters</i>                   | <i>dat</i>                                      | <i>mands</i>    | <i>mands</i>                    | <i>mand</i>                                     |
| <i>døtre</i>     | <i>doter</i>                    | <i>dot</i>                                      | <i>mænd</i>     | <i>mand</i>                     | <i>mand</i>                                     |
| <i>døtrene</i>   | <i>doterne</i>                  | <i>dot</i>                                      | <i>mændene</i>  | <i>mandene</i>                  | <i>mand</i>                                     |
| <i>døtrenes</i>  | <i>doternes</i>                 | <i>dot</i>                                      | <i>mændenes</i> | <i>mandenes</i>                 | <i>mand</i>                                     |
| <i>døtres</i>    | <i>doters</i>                   | <i>dot</i>                                      | <i>mænds</i>    | <i>mands</i>                    | <i>mand</i>                                     |

The declensions of *datter* “daughter” exhibit vowel alternations in their essential roots. This phenomenon, together with the vowel alternations in Danish irregular verbs, will be handled in §5.1.2.

### 5.1.2 Admissible mutation and approximate clustering

The Danish vowel blotting mechanism is slightly different from the English counterpart (Algorithm 4.9).

**Algorithm 5.5** (Danish vowel blotting). *Set*  $\mathbf{V} = (a|e|i|o|u)$  and  $\mathbf{C}_{m_0} = \overline{(a|e|i|o|u)}_{m_0}$ . *For a token string*  $\hat{\sigma}$ , *its blotted form*  $\text{BlotV}_1(\hat{\sigma})$  *is constructed as follows:*

- *If the string pattern*  $(\emptyset|ab|af|be)\mathbf{C}_{m_0}\mathbf{V}\sim$  *can be found in the string*  $\hat{\sigma}$ , *then the last position occupied by such a pattern is replaced by the letter “a”.*
- *Otherwise, leave the string*  $\hat{\sigma}$  *intact.*

<sup>51</sup>See Definition 3.3 for the multiplicity notation  $(\hat{\sigma}_1|\dots|\hat{\sigma}_n)_{[0,1]}$ .

<sup>52</sup>In other words, the core algorithm for essential root extraction runs as follows: keep the last “strong” vowel *a, i, o* or *u* in non-final position, plus one subsequent letter; delete final *a*; erase the final appearance of *e* and all the letters thereafter.

*Example 5.5.1.* As a continuation of Example 5.4.1, we point out that  $\text{BlotV}_1(\text{EssRoot}(\text{EffSpell}(\hat{\sigma})))$  evaluates to *dat* (resp. *mand*) for all the declensions of *datter* (resp. *mand*). If we consider  $\text{BlotV}_1(\text{EffSpell}(\hat{\sigma}))$  instead, the output is identical to  $\text{EffSpell}(\hat{\sigma})$  for every declined form of *mand*, but involves a substitution  $o \rightarrow a$  for the case of *datter*.

*Example 5.5.2.* A few more examples involving inflected forms of the Danish irregular verb *finde* “find”:

| $\hat{\sigma}$                                                  | <i>fandt</i> | <i>find</i> | <i>finder</i> | <i>funden</i> | <i>fundet</i> | <i>fundne</i> |
|-----------------------------------------------------------------|--------------|-------------|---------------|---------------|---------------|---------------|
| $\text{EffSpell}(\hat{\sigma})$                                 | <i>fandt</i> | <i>find</i> | <i>finder</i> | <i>funden</i> | <i>fundet</i> | <i>fundne</i> |
| $\text{BlotV}_1(\text{EffSpell}(\hat{\sigma}))$                 | <i>fandt</i> | <i>fand</i> | <i>fander</i> | <i>fanden</i> | <i>fandet</i> | <i>fandne</i> |
| $\text{EssRoot}(\text{EffSpell}(\hat{\sigma}))$                 | <i>fand</i>  | <i>find</i> | <i>find</i>   | <i>fund</i>   | <i>fund</i>   | <i>fund</i>   |
| $\text{BlotV}_1(\text{EssRoot}(\text{EffSpell}(\hat{\sigma})))$ | <i>fand</i>  | <i>fand</i> | <i>fand</i>   | <i>fand</i>   | <i>fand</i>   | <i>fand</i>   |

Similar to what we did in §4.2.2 for the case of English, we will construct a “heredity test function”  $\text{HrdTest}(\hat{\alpha}, \hat{\beta})$  from a “simple heredity test function” in Algorithm 5.6 and a set of “admissible suffix mismatch and vowel alternation” rules in Algorithm 5.8.

**Algorithm 5.6** (Simple heredity test). *Suppose that  $\hat{\alpha}$  and  $\hat{\beta}$  are both lowercase strings. Set  $\mathbf{V} = (a|e|i|o|u)$ . The Boolean-valued function  $\text{SimpHrdTest}(\hat{\alpha}, \hat{\beta})$  returns **TRUE** if  $\hat{\alpha}$  contains at least one instance of  $\mathbf{V}$ , **AND** at least one of the following three conditions holds:<sup>53</sup>*

- (i)  $\hat{\alpha} = \hat{\beta}$ ;
- (ii)  $\hat{\beta} = \hat{\alpha}t$ ;
- (iii)  $\ell(\hat{\beta}) > \ell(\hat{\alpha}) > \frac{\ell(\hat{\beta})}{2}$  **AND**  $\hat{\alpha} = \hat{\beta}^{[\ell(\hat{\alpha})]}$  **AND**  $\hat{\beta}^{\ell(\hat{\alpha})+1} = (e|s)$ . (See Definition 3.1 for the notations  $\hat{\beta}^{[n]}$  and  $\hat{\beta}^{(n)}$ .)

In what follows, we shall define  $\text{SuffixNW}(\hat{\alpha}, \hat{\beta})$  and  $\text{SuffixSW}(\hat{\alpha}, \hat{\beta})$  as what is done in the English case (Algorithm 4.11), but the definitions of  $\text{RootNW}(\hat{\alpha}, \hat{\beta})$ ,  $\text{NW}^*(\hat{\alpha}, \hat{\beta})$  and  $\text{SuffixSW}(\hat{\alpha}, \hat{\beta})$ ,  $\text{SW}^*(\hat{\alpha}, \hat{\beta})$  will be subtly different.

**Algorithm 5.7** (Roots and Suffixes by NW and SW). *For two strings  $\hat{\alpha}$  and  $\hat{\beta}$ , the function values  $\text{RootNW}(\hat{\alpha}, \hat{\beta})$ ,  $\text{SuffixNW}(\hat{\alpha}, \hat{\beta})$  and  $\text{NW}^*(\hat{\alpha}, \hat{\beta})$  are determined through the following procedure:*

- Use the Needleman–Wunsch algorithm to align the sequences as  $\text{NW}(\hat{\alpha}, \hat{\beta})$ .
- If  $\text{NW}(\hat{\alpha}, \hat{\beta})$  ends with a mismatch (shown in brackets in Examples 3.7.1 and 3.7.2), use this mismatch to define  $\text{SuffixNW}(\hat{\alpha}, \hat{\beta})$ ; otherwise, define  $\text{SuffixNW}(\hat{\alpha}, \hat{\beta}) = [\emptyset, \emptyset]$ .
- Construct  $\text{RootNW}(\hat{\alpha}, \hat{\beta})$  from all the (not necessarily contiguous) matching string portions in  $\text{NW}(\hat{\alpha}, \hat{\beta})$ , joined together by  $\# = \text{U+0023}$ :
- If the first mutation bracket in  $\text{NW}(\hat{\alpha}, \hat{\beta})$  does not appear at the end [which in turn, makes a non-void contribution to  $\text{SuffixNW}(\hat{\alpha}, \hat{\beta})$ ], then define  $\text{NW}^*(\hat{\alpha}, \hat{\beta})$  as this first mismatch; otherwise, define  $\text{NW}^*(\hat{\alpha}, \hat{\beta}) = \emptyset$ ;

The function values  $\text{RootSW}(\hat{\alpha}, \hat{\beta})$ ,  $\text{SuffixSW}(\hat{\alpha}, \hat{\beta})$  and  $\text{SW}^*(\hat{\alpha}, \hat{\beta})$  are determined similarly, through the SW function.

*Example 5.7.1.* Let  $\hat{\alpha} = \textit{fandt}$ ,  $\hat{\beta} = \textit{find}$ , then we have  $\text{NW}(\hat{\alpha}, \hat{\beta}) = \text{SW}(\hat{\alpha}, \hat{\beta}) = f[a, i]nd[t, \emptyset]$ , leading to  $\text{SuffixNW}(\hat{\alpha}, \hat{\beta}) = \text{SuffixSW}(\hat{\alpha}, \hat{\beta}) = [t, \emptyset]$ ,  $\text{RootNW}(\hat{\alpha}, \hat{\beta}) = \text{RootSW}(\hat{\alpha}, \hat{\beta}) = f\#nd$ ,  $\text{NW}^*(\hat{\alpha}, \hat{\beta}) = \text{SW}^*(\hat{\alpha}, \hat{\beta}) = [a, i]$ .

**Algorithm 5.8** (Admissible suffix mismatch and vowel alternation). *For two strings  $\hat{\alpha}$  and  $\hat{\beta}$ , the Boolean-valued function*

$$\text{AdmMut}(\text{RootNW}(\hat{\alpha}, \hat{\beta}), \text{SuffixNW}(\hat{\alpha}, \hat{\beta}), \text{NW}^*(\hat{\alpha}, \hat{\beta}))$$

returns **TRUE** if

$$\text{SuffixNW}(\hat{\alpha}, \hat{\beta}) = [(\emptyset|(e|nd|t)_m)((\textit{bar|dom|hed|ig|lig|skab})\mathbf{X}), (\emptyset|(e|nd|t)_m)((\textit{bar|dom|hed|ig|lig|skab})\mathbf{X})]$$

**AND** at least one of the following two conditions holds:

- (i)  $\text{NW}^*(\hat{\alpha}, \hat{\beta}) = \emptyset$  **AND**  $\text{RootNW}(\hat{\alpha}, \hat{\beta})$  contains at least one instance of  $\mathbf{V} = (a|e|i|o|u)$ ;
- (ii)  $\text{NW}^*(\hat{\alpha}, \hat{\beta}) = ([a, i][a, o][a, u][e, i][i, u][o, u])$ .

<sup>53</sup>As a general rule in this document, the truth values of items labeled with Roman numerals are connected to each other with logical **OR**.

Similarly, one can evaluate another Boolean-valued function

$$\text{AdmMut}(\text{RootSW}(\hat{\alpha}, \hat{\beta}), \text{SuffixSW}(\hat{\alpha}, \hat{\beta}), \text{SW}^*(\hat{\alpha}, \hat{\beta}))$$

by trading all the occurrences of NW in the statements above with SW.

**Algorithm 5.9** (Heredity test function). For two strings  $\hat{\alpha}$  and  $\hat{\beta}$ , the Boolean-valued function  $\text{HrdTest}(\hat{\alpha}, \hat{\beta})$  returns **TRUE** if at least one of the following three conditions holds:

- (i)  $\text{SimpHrdTest}(\hat{\alpha}, \hat{\beta}) = \mathbf{TRUE}$ ;
- (ii)  $\ell(\text{RootNW}(\hat{\alpha}, \hat{\beta})) \geq \frac{\max\{\ell(\hat{\alpha}), \ell(\hat{\beta})\}}{2}$  **AND**  $\text{AdmMut}(\text{RootNW}(\hat{\alpha}, \hat{\beta}), \text{SuffixNW}(\hat{\alpha}, \hat{\beta}), \text{NW}^*(\hat{\alpha}, \hat{\beta})) = \mathbf{TRUE}$ ;
- (iii)  $\ell(\text{RootSW}(\hat{\alpha}, \hat{\beta})) \geq \frac{\max\{\ell(\hat{\alpha}), \ell(\hat{\beta})\}}{2}$  **AND**  $\text{AdmMut}(\text{RootSW}(\hat{\alpha}, \hat{\beta}), \text{SuffixSW}(\hat{\alpha}, \hat{\beta}), \text{SW}^*(\hat{\alpha}, \hat{\beta})) = \mathbf{TRUE}$ .

Our approximate clustering algorithm for Danish differs from the English counterpart (Algorithm 4.15) in one specific detail: in Algorithm 5.10 below, vowel blotting is applied to both the effective spelling and the essential root in two stages, while Algorithm 4.15 has restricted the use of vowel blotting to the essential root.

**Algorithm 5.10** (Approximate clustering of Danish words). The approximate clustering of a list of Danish words  $\{\hat{\alpha}_1, \dots, \hat{\alpha}_N\}$  is completed in two stages:

- (1) We sort the list  $\{(\hat{\alpha}_1, \text{EffSpell}(\hat{\alpha}_1), \text{BlotV}_1(\text{EffSpell}(\hat{\alpha}_1))), \dots, (\hat{\alpha}_N, \text{EffSpell}(\hat{\alpha}_N), \text{BlotV}_1(\text{EffSpell}(\hat{\alpha}_N)))\}$  alphabetically according to the third component (with higher priority) and the second component (with lower priority). If two consecutive neighbors in the alphabetized list  $\{(\hat{\alpha}_{(1)}, \text{EffSpell}(\hat{\alpha}_{(1)}), \text{BlotV}_1(\text{EffSpell}(\hat{\alpha}_{(1)}))), \dots, (\hat{\alpha}_{(N)}, \text{EffSpell}(\hat{\alpha}_{(N)}), \text{BlotV}_1(\text{EffSpell}(\hat{\alpha}_{(N)})))\}$  satisfy  $\text{HrdTest}(\text{EffSpell}(\hat{\alpha}_{(n)}), \text{EffSpell}(\hat{\alpha}_{(n+1)})) = \mathbf{FALSE}$ , where  $n \in \mathbb{Z} \cap [1, N)$ , then add a demarcation line between these two entries. In this way, the alphabetized list is divided into separate groups of words tagged with their effective spellings:  $\{g_1 = \{(\hat{\alpha}_{(1,1)}, \text{EffSpell}(\hat{\alpha}_{(1,1)}), \text{BlotV}_1(\text{EffSpell}(\hat{\alpha}_{(1,1)}))), \dots, (\hat{\alpha}_{(1,n_1)}, *, *)\}, \dots, g_M = \{(\hat{\alpha}_{(M,1)}, *, *), \dots, (\hat{\alpha}_{(M,n_M)}, *, *)\}$ ,<sup>54</sup> where each sublist also preserves alphabetic order. In particular, we have  $\hat{\alpha}_{(1,1)} = \hat{\alpha}_{(1)}$  and  $\hat{\alpha}_{(M,n_M)} = \hat{\alpha}_{(N)}$ .
- (2) For each group of words  $g_m = \{(\hat{\alpha}_{(m,1)}, *, *), \dots, (\hat{\alpha}_{(m,n_m)}, *, *)\}$  where  $m \in \mathbb{Z} \cap [1, M]$ , we augment it into a tagged entry  $G_m = (g_m, \text{EffSpell}(\hat{\alpha}_{(m,1)}), \text{EssRoot}(\text{EffSpell}(\hat{\alpha}_{(m,1)})), \text{BlotV}_1(\text{EssRoot}(\text{EffSpell}(\hat{\alpha}_{(m,1)}))))$ . The list  $\{G_1, \dots, G_M\}$  is sorted alphabetically, with respect to  $\text{BlotV}_1(\text{EssRoot}(\text{EffSpell}(\hat{\alpha}_{(m,1)})))$  (with highest priority),  $\text{EssRoot}(\text{EffSpell}(\hat{\alpha}_{(m,1)}))$  (with medium priority), and  $\text{EffSpell}(\hat{\alpha}_{(m,1)})$  (with lowest priority). If two consecutive neighbors in the alphabetized list  $\{G_{(1)} = (g_{(1)}, \hat{\gamma}'_{(1)}, \hat{\gamma}''_{(1)}, \hat{\gamma}'''_{(1)}), \dots, G_{(M)} = (g_{(M)}, \hat{\gamma}'_{(M)}, \hat{\gamma}''_{(M)}, \hat{\gamma}'''_{(M)})\}$  satisfy

$$\text{HrdTest}(\hat{\gamma}''_{(m)}, \hat{\gamma}''_{(m+1)}) = \mathbf{FALSE}$$

**AND**

$$\text{HrdTest}(\hat{\gamma}'_{(m)}, \hat{\gamma}'_{(m+1)}) = \mathbf{FALSE}$$

where  $m \in \mathbb{Z} \cap [1, M)$ , then add a demarcation line between these two entries. In this manner, the alphabetized list  $\{G_{(1)}, \dots, G_{(M)}\}$  is divided into separate groups of tagged clusters  $\{\Gamma_1 = \{G_{(1,1)}, \dots, G_{(1,m_1)}\}, \dots, \Gamma_K = \{G_{(K,1)}, \dots, G_{(1,m_K)}\}\}$ . Finally, the output list of word clusters  $\{\tilde{\Gamma}_1, \dots, \tilde{\Gamma}_K\}$  is constructed by discarding all the tags (effective spellings, essential roots, vowel blotted forms) from each  $\Gamma_k$ , where  $k \in \mathbb{Z} \cap [1, K]$ .

*Example 5.10.1.* As an illustration of our clustering algorithm, we pick the following families of Danish words, where an “approximate translation” in English, enclosed in quotation marks, is appended to the end of each family:<sup>55</sup>

*and, anden, andens, ands, ænder, ænderne, ændernes, ænders* — “duck”;  
*Anders, Andersen, Andersens* — “Andrew”;  
*barn, barnet, barnets, barns, børn, børnene, børnenes, børns* — “child”;  
*bonde, bonden, bondens, bondes, bønder, bønderne, bøndernes, bønders* — “farmer”;  
*datter, datteren, datterens, datters, døtre, døtrene, døtrenes, døtres* — “daughter”;  
*ferie, ferien, feriens, ferier, ferierne, ferienes, feriers, ferier* — “holiday”;  
*fængsel, fængslerne, fængselet, fængselets, fængsels, fængsler, fængslernes, fængslers, fængslet, fængslets* — “jail”;  
*himle, himlen, himlene, himlenes, himlens, himles, himmel, himmelen, himmelens, himmels* — “heaven”;  
*hus, hus', huse, husende, husene, husenes, huser, huses, huset, husets, hust, huste* — “house”;

<sup>54</sup>Hereafter, we use an asterisk (\*) to abbreviate components that are clear from context.

<sup>55</sup>We note that within each family, words may be related to each other through both inflections (adjective comparisons, noun declensions, verb conjugations) and derivations (such as compound nouns formed from several components, verbs derived from nouns, etc.). Therefore, the “approximate translation” only matches certain members in the specified word family.

*husven, husvennen, husvennens, husvenner, husvennerne, husvennernes, husvenners, husvens* — “family friend”;  
*hænder, hænderne, hændernes, hænders, Haand, hånd, hånden, hånds* — “hand”;  
*kø, køen, køens, køer, køerne, køernes, køers, køs* — “queue”;  
*køb, købene, købenes, køber, købet, købets, købs, købt, købte, købtes* — “purchase”;  
*København, Københavns* — “Copenhagen”;  
*mand, manden, mandens, mands, mænd, mændene, mændenes, mænds* — “man”;  
*prins, prinse, prinselig, prinsen, prinsens, prinser, prinserne, prinsernes, prinsers, prinses* — “prince”;  
*prinsesse, prinsessekrone, prinsessen, prinsessens, prinsesser, prinsesserne, prinsessernes, prinsessers, prinsesses* — “princess”;  
*ske, skeen, skeens, skeer, skeerne, skeernes, skeers, skes* — “spoon”;  
*ske, sker, sket, skete* — “happen”;  
*stor, store, stort, større, størst* — “big”;  
*ung, ungdom, unge, ungt, yngre, yngst* — “young”;  
*ven, vennen, vennens, venner, vennerne, vennernes, venners, vens* — “friend”;  
*venlig, venligere, venligst, venligste, venligt* — “friendly”;  
*vent, vente, ventede, ventedes, venter, ventes, ventet* — “wait”;  
*vin, vine, vinen, vinene, vinenes, vinens, vines, vins* — “wine”;  
*vinter, vinteren, vinterens, vinters, vintre, vintrene, vintrenes, vintres* — “winter”;  
*vinterferie, vinterferien, vinterferiens, vinterferier, vinterferierne, vinterferiernes, vinterferiers, vinterferies* — “winter holiday”;  
*ø, øen, øens, øer, øerne, øernes, øers, øs* — “island”;  
*å, åen, åens, åer, åerne, åernes, åers, ås* — “creek”;  
*år, årene, årenes, året, årets, års* — “year”.

Applying Algorithm 5.10 to this list of words, we obtain the following clustering results:

{*and, anden, andens, Anders, Andersen, Andersens, ands, ænder, ænderne, ændernes, ænders*}, {*barn, barnet, barnets, barns, børn, børnene, børnenes, børns*}, {*bonde, bonden, bondens, bondes, bønder, bønderne, bøndernes, bønders*}, {*datter, datteren, datterens, datters, døtre, døtrene, døtrenes, døtres*}, {*ferie, ferien, feriens, ferier, ferierne, feriernes, feriers, feris*}, {*fængsel, fængselerne, fængselet, fængselets, fængsels, fængsler, fængslernes, fængslers, fængslet, fængslets*}, {*himle, himlen, himlene, himlenes, himlens, himles, himmel, himmelen, himmelens, himmels*}, {*hus, hus', huse, husende, husene, husenes, huser, huses, huset, husets, hust, huste, husven, husvennen, husvennens, husvenner, husvennerne, husvennernes, husvenners, husvens*}, {*hænder, hænderne, hændernes, hænders, Haand, hånd, hånden, hånds*}, {*kø, køen, køens, køer, køerne, køernes, køers, køs*}, {*køb, købene, købenes, køber, købet, købets, købs, købt, købte, købtes*}, {*København, Københavns*}, {*mand, manden, mandens, mands, mænd, mændene, mændenes, mænds*}, {*prins, prinse, prinsen, prinsens, prinser, prinserne, prinsernes, prinsers, prinses, prinselig*}, {*ske, skeen, skeens, skeer, skeerne, skeernes, skeers, skes, sket, skete*}, {*stor, store, stort, større, størst*}, {*ung, ungdom, unge, ungt, yngre, yngst*}, {*ven, veninde, veninden, venindens, veninder, veninderne, venindernes, venindes, venner, vennen, vennens, venners, venter, venterne, venternes, venteres, venteret*}, {*venlig, venligere, venligst, venligste, venligt*}, {*vent, vente, ventede, ventedes, venter, ventes, ventet*}, {*vin, vine, vinen, vinene, vinenes, vinens, vines, vins*}, {*vinter, vinteren, vinterens, vinters, vintre, vintrene, vintrenes, vintres*}, {*vinterferie, vinterferien, vinterferiens, vinterferier, vinterferierne, vinterferiernes, vinterferiers, vinterferies*}, {*ø, øen, øens, øer, øerne, øernes, øers, øs*}, {*å, åen, åens, åer, åerne, åernes, åers, ås*}, {*år, årene, årenes, året, årets, års*}.

Example 5.10.2. To further test our algorithm against Danish irregular verbs, we throw the following list:

*afbrudt, afbryd, afbryde, afbryder, afbrød* — “interrupt”;  
*bar, bær, bære, bærer, båret* — “carry”;  
*besat, besatte, besæt, besætte, besætter* — “occupy”;  
*beskrev, beskreven, beskrevet, beskrevne, beskriv, beskriver* — “describe”;  
*blotlagde, blotlagt, blotlæg, blotlægge, blotlægger* — “expose”;  
*bræk, brække, brækkede, brækker, brækket* — “break”;  
*drak, drik, drikker, drukken, drukket, drukne* — “drink”;  
*fandt, find, finder, funden, fundet, fundne* — “find”;  
*fik, få, fået, får* — “get”;  
*flyv, flyve, flyver, fløj, fløjte* — “fly”;  
*gav, gavs, giv, give, givende, givendes, giver, gives, givet, givets* — “give”;  
*gentag, gentagen, gentager, gentaget, gentagne, gentog* — “repeat”;

*græd, græde, græder, grædt* — “weep”;  
*hjalp, hjulpen, hjulpet, hjulpne, hjælp, hjælpe, hjælper* — “help”;  
*kom, komme, kommen, kommende, kommer, kommet, komme* — “come”;  
*lad, lader, ladet, ladt, lod* — “allow”;  
*lig, ligge, ligger, ligget, lå* — “lie (be in horizontal position)”;  
*løb, løbe, løber, løbet* — “run”;  
*optræd, optræde, optræder, optrådt, optrådte* — “appear”;  
*ryg, ryge, ryger, røg, røget* — “smoke”;  
*sang, sunget, syng, syngende, synger* — “sing”;  
*trak, trukken, trukket, trukne, træk, trækkende, trækker* — “pull”;  
*æd, æde, æder, ædt, åd* — “eat (like an animal)”

into our algorithm, and obtain

{*afbrudt, afbryd, afbryde, afbryder, afbrød*}, {*bar, bær, bære, bærer, båret*}, {*besat, besatte, besæt, besætte, besætter*}, {*beskrev, beskreven, beskrevet, beskrevne, beskriv, beskriver*}, {*blotlagde, blotlagt, blotlæg, blotlægge, blotlægger*}, {*bræk, brække, brækkede, brækker, brækket*}, {*drak, drik, drikker, drukken, drukket, drukne*}, {*fandt, find, finder, funden, fundet, fundne*}, {*fik, få, fået, får*}, {*flyv, flyve, flyver, fløj, fløjjet*}, {*gav, gavs, giv, give, givende, givendes, giver, gives, givet, givets*}, {*gentag, gentagen, gentager, gentaget, gentagne, gentog*}, {*græd, græde, græder, grædt*}, {*hjalp, hjulpen, hjulpet, hjulpne, hjælp, hjælpe, hjælper*}, {*kom, komme, kommen, kommende, kommer, kommet, komme*}, {*lad, lader, ladet, ladt, lod*}, {*lig, ligge, ligger, ligget, lå*}, {*løb, løbe, løber, løbet*}, {*optræd, optræde, optræder, optrådt, optrådte*}, {*ryg, ryge, ryger, røg, røget*}, {*sang, sunget, syng, syngende, synger*}, {*trak, trukken, trukket, trukne, træk, trækkende, trækker*}, {*æd, æde, æder, ædt, åd*}.

Example 5.10.3. Combining the inputs from the last two examples, we obtain the following output:

{*afbrudt, afbryd, afbryde, afbryder, afbrød*}, {*and, anden, andens, Anders, Andersen, Andersens, ands, ænder, ænderne, ændernes, ænders*}, {*bar, bær, bære, bærer, båret*}, {*barn, barnet, barnets, barns, børn, børnene, børnenes, børns*}, {*besat, besatte, besæt, besætte, besætter*}, {*beskrev, beskreven, beskrevet, beskrevne, beskriv, beskriver*}, {*blotlagde, blotlagt, blotlæg, blotlægge, blotlægger*}, {*bonde, bonden, bondens, bondes, bønder, bønderne, bøndernes, bonders*}, {*bræk, brække, brækkede, brækker, brækket*}, {*datter, datteren, datterens, datters, døtre, døtrene, døtrenes, døtres*}, {*drak, drik, drikker, drukken, drukket, drukne*}, {*fandt, find, finder, funden, fundet, fundne*}, {*ferie, ferien, feriens, ferier, ferierne, feriernes, feriers, feris*}, {*fik, få, fået, får*}, {*flyv, flyve, flyver, fløj, fløjjet*}, {*fængsel, fængselerne, fængselet, fængselets, fængsels, fængsler, fængslernes, fængsleres, fængslet, fængslets*}, {*gav, gavs, giv, give, givende, givendes, giver, gives, givet, givets*}, {*gentag, gentagen, gentager, gentaget, gentagne, gentog*}, {*græd, græde, græder, grædt*}, {*himle, himlen, himlene, himlenes, himlens, himles, himmel, himmelen, himmelens, himmels*}, {*hjalp, hjulpen, hjulpet, hjulpne, hjælp, hjælpe, hjælper*}, {*hus, hus', huse, husende, husene, husenes, huser, huses, huset, husets, hust, huste, husven, husvennen, husvennens, husvenner, husvennerne, husvennernes, husvenners, husvens*}, {*hænder, hænderne, hændernes, hænderes, Haand, hånd, hånden, hånds*}, {*kom, komme, kommen, kommende, kommer, kommet, komme*}, {*kø, køen, køens, køer, køerne, køernes, køers, køs*}, {*køb, købene, købenes, køber, købet, købets, købs, købt, købte, købtes*}, {*København, Københavns*}, {*lad, lader, ladet, ladt, lod*}, {*lig, ligge, ligger, ligget, lå*}, {*løb, løbe, løber, løbet*}, {*mand, manden, mandens, mands, mænd, mændene, mændenes, mænds*}, {*optræd, optræde, optræder, optrådt, optrådte*}, {*prins, prinse, prinsen, prinsens, prinser, prinserne, prinsernes, prinsers, prinses, prinsesse, prinsessekroner, prinsessen, prinsessens, prinsesser, prinsesserne, prinsessernes, prinsessers, prinsesses*}, {*prinselig*}, {*ryg, ryge, ryger, røg, røget*}, {*sang, sunget, syng, syngende, synger*}, {*ske, skeen, skeens, skeer, skeerne, skeernes, skeers, sker, skes, sket, skete*}, {*stor, store, stort, større, størst*}, {*trak, trukken, trukket, trukne, træk, trækkende, trækker*}, {*ung, ungdom, unge, ungt, yngre, yngst*}, {*ven, veninde, veninden, venindens, veninder, veninderne, venindernes, veninders, venindes, vennen, vennens, venner, vennerne, vennernes, venners, vens*}, {*venlig, venligere, venligst, venligste, venligt*}, {*vent, vente, ventede, ventedes, venter, ventes, ventet*}, {*vin, vine, vinen, vinene, vinenes, vinens, vines, vins*}, {*vinter, vinteren, vinterens, vinters, vintre, vintrene, vintrenes, vintres*}, {*vinterferie, vinterferien, vinterferiens, vinterferier, vinterferierne, vinterferiernes, vinterferiers, vinterferies*}, {*æd, æde, æder, ædt, åd*}, {*ø, øen, øens, øer, øerne, øernes, øers, øs*}, {*å, åen, åens, åer, åerne, åernes, åers, ås*}, {*år, årene, årenes, året, årets, års*}.

### 5.1.3 Heuristic detection of compounds

In Danish (as well as German and Dutch), compounds are usually spelt as a single word, without spaces or hyphens between the constituting components. For example, the Danish compound *vinterferie* “winter holiday” is formed by joining *vinter*

“winter” and *ferie* “holiday”. Aside from direct concatenation, Danish compounds may also involve an intervening letter *e* or *s* [46, §12.2.2.2].

Automatic detection of the “hidden word boundaries” within Germanic compounds is a non-trivial task. However, if we limit our scope to compounds with only two constituting components that both appear in isolations in a vocabulary list, there are heuristic methods to break down these binary compound words. We will integrate such a heuristic compound detection method with Danish word clustering, later in Algorithm 5.13 (which is a variation on Algorithm 5.10), where any detected binary compound is “dissolved” into its two constituting components (“head” and “tail”) and filed as two copies, one clustered with the “head” word, the other with the “tail” word.

Before stating Algorithm 5.13 in full, we need some preparations (Definition 5.11 and 5.12) to sort out potential binary compounds and their constituting components.

**Definition 5.11** (String minus operation). Suppose that  $\ell(\hat{\beta}) \geq \ell(\hat{\alpha})$  and  $\hat{\beta} = \hat{\beta}^{\ell(\hat{\alpha})} \hat{\tau}$ , then  $\hat{\beta} \ominus \hat{\alpha} = \hat{\tau}$  defines the the “string minus operation”. In other words,  $\hat{\beta} \ominus \hat{\alpha}$  is a string that leaves out the first  $\ell(\hat{\alpha})$  characters in  $\hat{\beta}$ .  $\square$

**Algorithm 5.12** (Heuristic identification of Danish binary compounds). Let  $\Lambda^{\hat{\rho}} = \{\hat{\rho}_1, \dots, \hat{\rho}_Q\}$  be a list of distinct Danish essential roots (without vowel blotting) that contain at least one instance of  $\mathbf{V} = (a|e|i|o|u)$  and DO NOT match the following string patterns:

$$(\pi\rho a|a|af|ag|ak|al|an\mathbf{X}|ar|at|be|ben|dag|du|frem|lo|mi|mod|na|nar|ned|om|op|ot|ov|rak|re|rig|rod|ru|sam|tag|u|ud|und|vfor\mathbf{X}|Xant|zil\mathbf{X}).$$

The output of the function  $\text{CpdDet}(\Lambda^{\hat{\rho}})$  is obtained through the following procedures:

- (1) Construct a list  $\{(\hat{\rho}_1, \lambda_1^{\hat{\rho}}), \dots, (\hat{\rho}_Q, \lambda_Q^{\hat{\rho}})\}$  where  $\lambda_q^{\hat{\rho}} = \{\hat{\rho}_{(q,1)}, \dots, \hat{\rho}_{(q,n_q)}\}$  is a subset of  $\Lambda^{\hat{\rho}}$  whose members all match the string pattern  $\hat{\rho}_q \sim$ , for  $q \in \mathbb{Z} \cap [1, Q]$ .
- (2) Expand the aforementioned entry  $(\hat{\rho}_q, \lambda_q^{\hat{\rho}})$  into a list of triplets  $\{(\hat{\rho}_{(q,1)}, \hat{\rho}_q, \hat{\rho}_{(q,1)} \ominus \hat{\rho}_q), \dots, (\hat{\rho}_{(q,n_q)}, \hat{\rho}_q, \hat{\rho}_{(q,n_q)} \ominus \hat{\rho}_q)\}$  for every  $q \in \mathbb{Z} \cap [1, Q]$  such that  $\lambda_q^{\hat{\rho}} \neq \emptyset$ . Collect all these triplets as one runs through the list  $\{(\hat{\rho}_1, \lambda_1^{\hat{\rho}}), \dots, (\hat{\rho}_Q, \lambda_Q^{\hat{\rho}})\}$ . The list of these triplets  $\{(\hat{\rho}_{(1)}, \hat{\eta}_{(1)}, \hat{\rho}_{(1)} \ominus \hat{\eta}_{(1)}), \dots, (\hat{\rho}_{(Q')}, \hat{\eta}_{(Q')}, \hat{\rho}_{(Q')} \ominus \hat{\eta}_{(Q')})\}$  contains potentially valid decompositions of compounds.
- (3) Screen the aforementioned list of triplets as follows: for every  $q' \in \mathbb{Z} \cap [1, Q']$ , if  $(\hat{\rho}_{(q')}, \hat{\eta}_{(q')}, \hat{\tau}_{(q')} = \hat{\rho}_{(q')} \ominus \hat{\eta}_{(q')})$  satisfies

$$\ell(\hat{\rho}_{(q')} \ominus \hat{\eta}_{(q')}) \geq 2 \quad \text{AND} \quad \hat{\rho}_{(q')} \ominus \hat{\eta}_{(q')} = \mathbf{X}_1(a|e|i|o|u)\mathbf{X}_2,$$

then construct  $\hat{\tau}_{(q')}^*$  by performing  $(e|s|t) \sim \rightarrow \emptyset$  on  $\hat{\tau}_{(q')}$  and  $\hat{\tau}_{(q')}^{**}$  by doing  $(e|r|e)s \sim \rightarrow \emptyset$  on  $\hat{\tau}_{(q')}$ , before generating a list  $\lambda_{(q')}^{\hat{\tau}}$  by members of  $\Lambda^{\hat{\rho}}$  that match the pattern  $(\hat{\tau}_{(q')}) | \hat{\tau}_{(q')}^* | \hat{\tau}_{(q')}^{**}$ ; otherwise, set  $\lambda_{(q')}^{\hat{\tau}} = \emptyset$ .

- (4) Collect all the triplets  $(\hat{\rho}_{(q')}, \hat{\eta}_{(q')}, \lambda_{(q')}^{\hat{\tau}})$  where  $\lambda_{(q')}^{\hat{\tau}}$  is non-void and  $\hat{\tau}_{(q')}$  DOES NOT match the following string patterns:

$$(dom\mathbf{X}|hed\mathbf{X}|lig\mathbf{X}|om).$$

This list of triplets  $\text{CpdDet}(\Lambda_{\hat{\rho}})$  contains the heuristic decompositions of all the identified binary compounds.

**Algorithm 5.13** (Approximate clustering of Danish words with heuristic detection of compounds). The approximate clustering of a list of Danish words  $\{\hat{\alpha}_1, \dots, \hat{\alpha}_N\}$  respecting compounding is completed in four stages:

- (1) Do as in Algorithm 5.10(1).
- (2) Do as in Algorithm 5.10(2). Save both the tagged clusters  $\{\Gamma_1 = \{G_{(1,1)}, \dots, G_{(1,m_1)}\}, \dots, \Gamma_K = \{G_{(K,1)}, \dots, G_{(1,m_K)}\}\}$  and the list of word clusters  $\{\check{\Gamma}_1, \dots, \check{\Gamma}_K\}$  for further use.
- (3) Construct a tagged list of word clusters  $\{(\check{\Gamma}_1, \Lambda_1^{\hat{\rho}}), \dots, (\check{\Gamma}_K, \Lambda_K^{\hat{\rho}})\}$  where  $\Lambda_k^{\hat{\rho}}$  is the union of all Danish essential roots (without vowel blotting) available to  $\Gamma_k$ , for  $k \in \mathbb{Z} \cap [1, K]$ . Set  $\Lambda^{\hat{\rho}} = \Lambda_1^{\hat{\rho}} \cup \dots \cup \Lambda_K^{\hat{\rho}}$ , and evaluate  $\text{CpdDet}(\Lambda^{\hat{\rho}})$ .
- (4) The first component  $\hat{\rho}_{(q')}$  of each triplet  $(\hat{\rho}_{(q')}, \hat{\eta}_{(q')}, \lambda_{(q')}^{\hat{\tau}})$  in  $\text{CpdDet}(\Lambda^{\hat{\rho}})$  is called a “dissolvable compound”, the second component  $\hat{\eta}_{(q')}$  a “heuristic head”, and the first member in the third component  $\lambda_{(q')}^{\hat{\tau}}$  a “heuristic tail”. In the tagged list  $\{(\check{\Gamma}_1, \Lambda_1^{\hat{\rho}}), \dots, (\check{\Gamma}_K, \Lambda_K^{\hat{\rho}})\}$ , every entry containing a “dissolvable compound” is removed, and regrouped with the entries matching its “heuristic head” and “heuristic tail”. Finally, remove all tags.

*Example 5.13.1.* We may revisit Example 5.10.3 with the algorithm above. The results are given below:

{*afbrudt, afbryd, afbryde, afbryder, afbrød*}, {*and, anden, andens, Anders, Andersen, Andersens, ands, ænder, ænderne, ændernes, ænders*}, {*bar, bær, bære, bærer, båret*}, {*barn, barnet, barnets, barns, børn, børnene, børnenes, børns*}, {*besat, besatte, besæt, besætte, besætter*}, {*beskrev, beskreven, beskrevet, beskrevne, beskriv, beskriver*}, {*blotlagde, blotlagt, blotlæg, blotlægge, blotlægger*}, {*bonde, bonden, bondens, bondes, bønder, bønderne, bøndernes, bønders*}, {*bræk, brække, brækkede, brækker, brækket*}, {*datter, datteren, datterens, datters, døtre, døtrene, døtrenes, døtres*}, {*drak, drik, drikker, drukken, drukket, drukne*}, {*fundt, find, finder, funden, fundet, fundne*}, {*ferie, ferien, feriens, ferier, ferierne, ferienes, feriers, feris, vinterferie, vinterferien, vinterferiens, vinterferier, vinterferierne, vinterferiernes, vinterferiers, vinterferies*}, {*fik, få, fået, får*}, {*flyv, flyve, flyver, fløj, fløjet*}, {*fængsel, fængselerne, fængselet, fængselets, fængsels, fængsler, fængslernes, fængslers, fængslet, fængslets*}, {*gav, gavs, giv, give, givende, givendes, giver, gives, givet, givets*}, {*gentag, gentagen, gentager, gentaget, gentagne, gentog*}, {*græd, græde, græder, grædt*}, {*himle, himlen, himlene, himlenes, himlens, himles, himmel, himmelen, himmelens, himmels*}, {*hjalp, hjælpe, hjulpet, hjulpne, hjælp, hjælpe, hjælper*}, {*hus, hus', huse, husende, husene, husenes, huser, huses, huset, husets, hust, huste, husven, husvennen, husvennens, husvenner, husvennerne, husvennernes, husvenners, husvens*}, {*hænder, hænderne, hændernes, hænders, Haand, hånd, hånden, hånds*}, {*kom, komme, kommen, kommende, kommer, kommet, komme*}, {*kø, køen, køens, køer, køerne, køernes, køers, køs*}, {*køb, købene, købenes, køber, købet, købets, købs, købt, købte, købtes*}, {*København, Københavns*}, {*lad, lader, ladet, ladt, lod*}, {*lig, ligge, ligger, ligget, lå*}, {*løb, løbe, løber, løbet*}, {*mand, manden, mandens, mands, mænd, mændene, mændenes, mænds*}, {*optræd, optræde, optræder, optrådt, optrådte*}, {*prins, prinse, prinselig, prinsen, prinsens, prinser, prinserne, prinsernes, prinsers, prinses, prinsesse, prinsessekrone, prinsessen, prinsessens, prinsesser, prinsesserne, prinsessernes, prinsessers, prinsesses*}, {*ryg, ryge, ryger, røg, røget*}, {*sang, sunget, syng, syngende, synger*}, {*ske, skeen, skeens, skeer, skeerne, skeernes, skeers, sker, skes, sket, skete*}, {*stor, store, stort, større, størst*}, {*trak, trukken, trukket, trukne, træk, trækker, trækker*}, {*ung, ungdom, unge, ungt, yngre, yngst*}, {*ven, veninde, veninden, venindens, veninder, veninderne, venindernes, veninders, venindes, venlig, venligere, venligst, venligste, venligt, vennen, vennens, venner, vennerne, vennernes, venners, vens*}, {*vent, vente, ventede, ventedes, venter, ventes, ventet*}, {*vin, vine, vinen, vinene, vinenes, vinens, vines, vins*}, {*vinter, vinteren, vinterens, vinterferie, vinterferien, vinterferiens, vinterferier, vinterferierne, vinterferiernes, vinterferiers, vinterferies, vinters, vintre, vintrene, vintrenes, vintres*}, {*æd, æde, æder, ædt, åd*}, {*ø, øen, øens, øer, øerne, øernes, øers, øs*}, {*å, åen, åens, åer, åerne, åernes, åers, ås*}, {*år, årene, årenes, året, årets, års*}.

Here, the word family generated by *vinterferie* “winter holiday” is correctly redistributed to the constituting components *vinter* “winter” and *ferie* “holiday”. In the meantime, there are no inappropriate compound detections, such as grouping *bære* “carry” with *barn* “child”.

*Example 5.13.2.* In Fig. S4, we further apply the aforementioned word clustering algorithm to topic extraction and machine translation (see Table S1 for text source).

The Danish word *ved* can mean “at” or “know” (present tense), which can be either a function word or a highly frequent content word (from the English perspective). We have chosen not to include *ved* in our list of Danish stop words (Definition 5.1), but have made no efforts to resolve its polysemy. Thus, in the second cluster of Fig. S4a, we have conflated several concepts that are spelt as *ved* (“at” or “know”) and *vide* (“know” or “wide”).

Moreover, the English topic *de* (part of the proper name “de Bourgh”) cannot be correctly translated by our algorithm, because the list of Danish stop words (Definition 5.1) includes *de* “the (plural), they, those”. Nevertheless, we consider a link between English *de* and Danish *Bourgh* an excusable error (marked in amber color in Fig. S4b, since these two words always stay together in the entire text—with nearly identical kinetic behavior).

It should be noted that Jane Austen used the word *related* mostly in the sense of *told* in her novel, which is correctly translated into *fortalte* in Danish.



## 5.2 Modified Porter stemming algorithm for German

**Definition 5.14** (German stop words). If the lowercase<sup>56</sup> form of a word belongs to the following list<sup>57</sup>:

*ab, aber, all, alle, allein, allem, allen, aller, alles, als, also, am, an, ander, andere, anderem, anderen, anderer, anderes, anderm, andern, anders, aneinander, auch, auf, aufeinander, aufs, aus, auseinander, ausser, außer, ausserdem, außerdem, bei, beide, beidem, beiden, beider, beides, beieinander, beim, bevor, bin, binnen, bis, bisher, bislang, bist, da, dabei, dafür, dagegen, dahin, damit, danach, dann, daran, darauf, darf, darfst, darin, darüber, darum, das, dass, daß, dasselbe, davon, dazu, dein, deine, deinem, deinen, deiner, deines, deins, dem, deme, demselben, den, denen, denn, dennoch, denselben, der, deren, derer, dern, dero, derselbe, derselben, des, deshalb, deß, desselben, dessen, desto, dich, die, dies, diese, dieselbe, dieselben, diesem, diesen, dieser, dieses, dir, doch, dort, dorthier, dorthin, du, durch, durcheinander, dürfe, dürfen, dürfend, dürfest, dürfet, dürft, durfte, dürfte, durften, dürften, durftest, dürftest, durftet, dürftet, ebenso, ein, einander, eine, einem, einen, einer, eines, einig, einige, einigem, einigen, einiger, einiges, einmal, empor, er, es, etwas, euch, euer, eure, eurem, euren, eurer, eures, falls, für, füreinander, ganz, ganze, ganzem, ganzen, ganzer, ganzes, gar, gedurft, gegen, gegeneinander, gegenüber, gehabt, gekonnt, gemocht, gemusst, gemußt, genug, gerade, geradezu, gesollt, getan, gewesen, gewollt, geworden, hab, habe, haben, habend, habest, habet, habt, hast, hat, hatte, hätte, hatten, hätten, hattest, hättest, hattet, hättet, her, herab, heran, herauf, heraus, herbei, herein, herüber, hervor, hier, hierher, hierhin, hin, hinab, hinauf, hinaus, hindurch, hinein, hingegen, hinten, hinter, hintereinander, hinüber, hinunter, hinweg, hinzu, ich, ihm, ihn, ihnen, ihr, ihre, ihrem, ihren, ihrer, ihres, im, immer, immerhin, in, indem, indes, indessen, ineinander, ins, iregendetwas, iregendwo, irgend, irgendein, irgendeine, irgendeinem, irgendeinen, irgendeiner, irgendeines, irgendjemand, irgendjemandem, irgendjemanden, irgendjemandes, irgendwann, irgendwas, irgendwelche, irgendwelchem, irgendwelchen, irgendwelcher, irgendwelches, irgendwer, irgendwie, irgendwohin, ist, ja, je, jede, jedem, jeden, jeder, jedes, jedoch, jemand, jemandem, jemanden, jemandes, jemand, jene, jenem, jenen, jener, jenes, jetzt, kann, kannst, kaum, kein, keine, keinem, keinen, keiner, keines, könne, können, könnend, könntest, könntet, könnt, konnte, könnte, konnten, könntest, könntest, konntet, konntet, los, machen, mag, magst, man, manche, manchem, manchen, mancher, manches, manchmal, mehr, mehre, mehrere, mehreres, mehres, mein, meine, meinem, meinen, meiner, meines, meins, mich, mir, mit, miteinander, mochte, möchte, mochten, möchten, mochtest, möchtest, mochtet, möchte, mögen, mögend, mögest, möget, mögt, muss, muß, müsse, müssen, müssend, müssest, müsst, müßt, mußte, mußte, müsst, müßt, mußten, mußten, müsstest, müßttest, müsstest, müßttest, musstest, müßttest, musstest, müßttest, na, nach, nachdem, nacheinander, nebeneinander, nein, nicht, nichts, nie, niemals, niemand, niemandem, niemanden, niemandes, niemands, nimmer, noch, nun, nur, ob, oben, obgleich, obwohl, obzwar, oder, oft, öfter, öftesten, ohne, pro, schon, sehr, sei, seien, seiet, sein, seine, seinem, seinen, seiner, seines, seins, seist, seit, seitdem, selbst, sich, sie, sind, so, sobald, sogar, solange, solch, solche, solchem, solchen, solcher, solches, soll, solle, sollen, sollend, sollest, sollet, sollst, sollt, sollte, sollten, solltest, solltet, sondern, sonst, soviel, soweit, sowie, sowohl, stets, tat, täte, taten, täten, tatest, tätest, tatet, tätet, trotz, trotzdem, tu, tue, tuen, tuend, tuest, tuet, tun, ture, tust, tut, über, überdies, übereinander, um, umsonst, und, uns, unse, unsem, unsen, unser, unsere, unserem, unseren, unserer, unseres, unserm, unsern, unses, unsre, unsrem, unsren, unsrer, unsres, unter, untereinander, usw, viel, viele, vielen, vieles, vielleicht, vielmehr, vom, von, voneinander, vor, vorbei, vordem, voreinander, vorüber, während, wann, war, wär, ward, warden, wardest, wardet, wardst, wäre, waren, wären, wärest, wäret, warst, wärst, wart, warum, was, weg, weil, weiter, welche, welchem, welchen, welcher, welches, wem, wen, wenig, wenige, wenigen, weniger, wenigsten, wenigstens, wenn, wenngleich, wer, werd, werde, werden, werdend, werdest, werdet, weshalb, wessen, weswegen, wie, wieder, wieso, wieviel, wiewohl, will, willst, wir, wird, wirst, wo, woher, wohin, wohl, wolle, wollen, wollend, wolltest, wollest, wollt, wollte, wollten, wolltest, wolltet, worden, wurde, würde, wurden, würden, würdest, würdest, würdet, würdet, ziemlich, zu, zudem, zueinander, zum, zur, zusammen, zurück, zuvor, zwar, zwischen,*

then we consider it a German stop word. All the German stop words that appear in a particular document need to be ignored before we perform word clustering on the rest of the vocabulary list. □

The post-1996 German orthography requires writing *ss* in place of *ß* in certain words. This new rule affects the stop word *daß*, whose new spelling *dass* has been added to our stop word list. We need to add *schon* “already” to the list of stop words, to avoid conflation with *schön* “beautiful” during approximate clustering (which ignores all umlauts). Although the words *schon* and *schön* were indeed etymologically related (reminiscent of the adverbial and adjectival uses of the word *pretty* in English), their current meanings are well separated.

<sup>56</sup>For the matching of German stop words, lowercase forms are enforced before comparison. Therefore, both *sie* “she, they” and *Sie* “you (polite form)” appearing in a German text are considered stop words, even though the capitalized form *Sie* does not appear in our list.

<sup>57</sup>Our list of German stop words is based on [snowball.tartarus.org/algorithms/german/stop.txt](http://snowball.tartarus.org/algorithms/german/stop.txt), with extensive additions that roughly match their counterparts in English.

For clustering German words, it is necessary that we ignore umlauts, so that *Apfel* “apple” is clustered with *Äpfel* “apples” etc. We also need to convert all the occurrences of  $\beta$  to *ss* (which matches the orthographic practice for German spelling in Switzerland), in order to accommodate to texts written before the German spelling reform in 1996: *Kuß* “kiss” (noun, pre-1996), *Kuss* “kiss” (noun, post-1996), *Küsse* “kisses” (noun, pre- and post-1996). This necessarily carries certain risk, as *Buße* “penance” (pre- and post-1996) will be conflated with *Busse* “buses” (pre- and post-1996).

All German nouns are capitalized, while adjectives and verbs derived from nouns are not: cf. *Deutsch* “German” (noun, “the German language”) and *deutsch* “German” (adjective). It is thus advisable to ignore capitalization during clustering, contrary to the practice in English.

### 5.2.1 Effective spelling and essential root

**Algorithm 5.15** (German effective spelling). Set  $\mathbf{V} = (a|e|\varepsilon|i|i|o|u)$  and  $\mathbf{V}^* = (a|\varepsilon|i|i|o|u)$ . For a German word  $\hat{\sigma}$ , its effective spelling  $\text{EffSpell}(\hat{\sigma})$  is constructed in the following steps:<sup>58</sup>

(1) Convert to lowercase, and replace

|                                             |                                              |                                         |                                             |                                                |                                    |                                          |                                          |                                          |                                                     |                                           |                                          |                         |
|---------------------------------------------|----------------------------------------------|-----------------------------------------|---------------------------------------------|------------------------------------------------|------------------------------------|------------------------------------------|------------------------------------------|------------------------------------------|-----------------------------------------------------|-------------------------------------------|------------------------------------------|-------------------------|
| $(\emptyset \text{ver})st(a e i o ü)rb\sim$ | $\hat{\chi}kunft$                            | $\hat{\chi}sicht$                       | $\hat{\chi}tr(\ddot{a} a)cht$               | $abwesen(d h)\mathbf{X}$                       |                                    |                                          |                                          |                                          |                                                     |                                           |                                          |                         |
| $\sigma\tau\epsilon\rho b$                  | $\hat{\chi}\hat{\chi}^+kunft$                | $\hat{\chi}\times_2s\hat{\chi}t$        | $\hat{\chi}^+\hat{\chi}tracht$              | $\alpha\beta\sigma\epsilon nt$                 |                                    |                                          |                                          |                                          |                                                     |                                           |                                          |                         |
| <i>acht</i> ~                               | <i>ähn</i>                                   | <i>anwesen(d h)\mathbf{X}</i>           | <i>b(ü u)ch</i>                             | <i>bald</i> ~                                  | <i>benn</i> ~                      | <i>bessie</i> ~                          | <i>blut</i> ~                            | <i>born</i> ~                            | <i>brot</i>                                         | <i>dame</i>                               | <i>dämmer</i>                            |                         |
| <i>de</i>                                   | <i>\sigma\mu\ddot{a}hn</i>                   | <i>\pi\rho\epsilon\sigma\epsilon nt</i> | <i>\beta\upsilon k</i>                      | <i>\beta\alpha\lambda\delta</i>                | <i>\beta\epsilon nn</i>            | <i>\beta\epsilon\sigma\theta ie</i>      | <i>\beta\lambda\omega\delta</i>          | <i>brunn</i>                             | <i>\beta\rho\tau</i>                                | <i>\delta\alpha\mu\epsilon</i>            | <i>\delta\alpha\omega\mu\epsilon\rho</i> |                         |
| <i>dent</i> ~                               | <i>diana</i> ~                               | <i>dicht</i>                            | <i>ehe</i> ~                                | <i>erinn</i> ~                                 | <i>f(ü u)(ss \beta)</i>            | <i>fessel</i>                            | <i>fessl</i>                             | <i>fest</i> ~                            | <i>feuer</i>                                        | <i>gardi</i> ~                            |                                          |                         |
| <i>de\ddot{v}tt</i>                         | <i>\delta i\ddot{a}\nu\ddot{a}</i>           | <i>\theta ikt</i>                       | <i>\mu\epsilon\epsilon</i>                  | <i>\mu\ddot{v}\epsilon\mu\eta n</i>            | <i>\phi\upsilon\tau\sigma\zeta</i> | <i>\phi\epsilon\sigma\epsilon l</i>      | <i>\phi\epsilon\sigma l</i>              | <i>\phi\epsilon\sigma\tau</i>            | <i>\phi\epsilon\upsilon\epsilon\rho</i>             | <i>\gamma\alpha\rho\delta i</i>           |                                          |                         |
| <i>gef(\ddot{a} a)hr</i>                    | <i>gegenwart</i> ~                           | <i>geheim</i>                           | <i>gestalt</i>                              | <i>gewalt</i> ~                                | <i>gott</i> ~                      | <i>h(\ddot{a} a ie)lt</i>                | <i>h(\ddot{o} o)he</i>                   | <i>hall</i>                              |                                                     |                                           |                                          |                         |
| <i>\delta\alpha\ddot{\nu}\gamma\rho r</i>   | <i>\pi\rho\epsilon\sigma\epsilon nt</i>      | <i>\sigma\epsilon k\rho\epsilon t</i>   | <i>\sigma\eta\alpha i\pi</i>                | <i>\phi\sigma\rho ct</i>                       | <i>\gamma\sigma\tau\tau</i>        | <i>\chi\sigma\lambda\delta</i>           | <i>hoche</i>                             | <i>h\sigma\alpha all</i>                 |                                                     |                                           |                                          |                         |
| <i>hannah</i> ~                             | <i>helen</i> ~                               | <i>hell</i>                             | <i>hüll</i>                                 | <i>inne</i> ~                                  | <i>irr</i>                         | <i>jone</i> ~                            | <i>leah</i> ~                            | <i>ledig</i>                             | <i>liebst</i>                                       | <i>lied</i>                               | <i>lond</i> ~                            |                         |
| <i>\chi\alpha\ddot{\nu}\nu\alpha\chi</i>    | <i>\epsilon\lambda\epsilon\ddot{\nu}\eta</i> | <i>h\chi\epsilon\lambda\lambda</i>      | <i>\omega\rho\alpha\pi</i>                  | <i>i\ddot{\nu}ne</i>                           | <i>i\upsilon\rho r</i>             | <i>\gamma i\sigma ne</i>                 | <i>\lambda\epsilon\alpha\alpha\eta</i>   | <i>\sigma i\ddot{\nu}\gamma</i>          | <i>lieb</i>                                         | <i>lie\delta</i>                          | <i>\lambda\sigma\eta\delta</i>           |                         |
| <i>m(ama utti)~</i>                         | <i>m(ü u)nd</i> ~                            | <i>meile</i>                            | <i>minut</i>                                | <i>müd</i>                                     | <i>oa</i> ~                        | <i>oberst</i>                            | <i>ort</i> ~                             | <i>pferd</i>                             | <i>plötz</i>                                        | <i>porträt</i>                            | <i>quell</i>                             |                         |
| <i>mutter</i>                               | <i>\mu i\ddot{\nu}\delta</i>                 | <i>\mu\epsilon i\lambda\epsilon</i>     | <i>\mu i\ddot{\nu}\omega\tau</i>            | <i>\mu\tau i\rho\delta</i>                     | <i>\omega\alpha</i>                | <i>\sigma\beta\epsilon\rho\sigma\tau</i> | <i>\omega\sigma\tau</i>                  | <i>\chi\sigma\rho\sigma</i>              | <i>\sigma\upsilon\delta\delta\epsilon\ddot{\nu}</i> | <i>\rho\sigma\rho\tau\rho\ddot{a}t</i>    | <i>q\upsilon\epsilon\lambda l</i>        |                         |
| <i>r(\ddot{o} o)t</i> ~                     | <i>recht</i>                                 | <i>ree</i> ~                            | <i>reich</i>                                | <i>reis</i>                                    | <i>relig</i>                       | <i>ri(ss \beta)~</i>                     | <i>robert</i>                            | <i>roches</i> ~                          | <i>s(a \ddot{a})(ss \beta)</i>                      |                                           |                                          |                         |
| <i>ro\theta</i>                             | <i>\rho i\gamma\chi\tau</i>                  | <i>\rho\epsilon\epsilon</i>             | <i>\rho\rho\epsilon i\chi</i>               | <i>\rho\epsilon\epsilon i\sigma s</i>          | <i>\rho\epsilon\lambda i\gamma</i> | <i>\rho i\phi\tau</i>                    | <i>\rho\sigma\beta\epsilon\rho\tau</i>   | <i>\rho\rho\omega\zeta\epsilon\sigma</i> | <i>sitz</i>                                         |                                           |                                          |                         |
| <i>schulter</i> ~                           | <i>sommer</i> ~                              | <i>spiel</i>                            | <i>still</i>                                | <i>talent</i>                                  | <i>them</i>                        | <i>tot</i> ~                             | <i>versuch</i> ~                         | <i>weg</i>                               | <i>welk</i>                                         | <i>well</i> ~                             | <i>wohl</i>                              | <i>ach</i>              |
| <i>schul\delta\epsilon r</i>                | <i>\sigma\sigma\mu\epsilon\rho r</i>         | <i>\pi\lambda\lambda\alpha l</i>        | <i>\sigma\tau i\lambda\lambda</i>           | <i>\tau\alpha\lambda\epsilon\ddot{\nu}\tau</i> | <i>\theta\epsilon\mu</i>           | <i>\sigma\tau\epsilon\rho b</i>          | <i>\nu\epsilon\rho\sigma\upsilon\chi</i> | <i>\omega\epsilon\gamma</i>              | <i>\omega i\theta\rho k</i>                         | <i>\omicron\ddot{\delta}\alpha\lambda</i> | <i>whol</i>                              | <i>\alpha\alpha\chi</i> |
| <i>besessen</i>                             | <i>de</i>                                    | <i>gatte(\emptyset n)</i>               | <i>gattin(\emptyset nen)</i>                | <i>gesessen</i>                                | <i>gibt</i>                        | <i>mrs</i>                               | <i>tod(\emptyset e en es s)</i>          | <i>~leute(\emptyset n)</i>               |                                                     |                                           |                                          |                         |
| <i>besitzen</i>                             | <i>\delta\epsilon\epsilon</i>                | <i>\epsilon\eta\mu\alpha\eta n</i>      | <i>\epsilon\eta\epsilon\phi\rho\alpha u</i> | <i>sitzen</i>                                  | <i>geben</i>                       | <i>z\phi\rho\alpha u</i>                 | <i>\sigma\tau\epsilon\rho b</i>          | <i>mann</i>                              |                                                     |                                           |                                          |                         |

(2) Replace

|                                         |                                              |                                 |                                          |                                                             |                                                 |                                         |                                              |                                  |                               |                                    |                           |             |                                  |
|-----------------------------------------|----------------------------------------------|---------------------------------|------------------------------------------|-------------------------------------------------------------|-------------------------------------------------|-----------------------------------------|----------------------------------------------|----------------------------------|-------------------------------|------------------------------------|---------------------------|-------------|----------------------------------|
| '                                       | $(\emptyset \text{ge})g\ddot{o}nn\sim$       | $(\emptyset \text{ge})hind\sim$ | $(b\ddot{o}s bosheit boshaft)\mathbf{X}$ | $\hat{\chi}^\epsilon(a e i k n o p s t u y)tisch\mathbf{X}$ |                                                 |                                         |                                              |                                  |                               |                                    |                           |             |                                  |
| $\emptyset$                             | <i>goenn</i>                                 | <i>\chi ind</i>                 | <i>bboes</i>                             | <i>\hat{\chi} ik</i>                                        |                                                 |                                         |                                              |                                  |                               |                                    |                           |             |                                  |
| $\mathbf{X}^\epsilon(a i)list$          | $\mathbf{X}^\epsilon(ge k sch ss \beta)ling$ | <i>\ddot{a}</i>                 | <i>absent</i>                            | <i>bek</i> ~                                                | <i>best<math>\hat{\chi}^\epsilon(e)</math>~</i> | <i>bett</i>                             | <i>brannt</i> ~                              | <i>ch</i>                        | <i>eb</i> ~                   | <i>ei</i>                          |                           |             |                                  |
| $\mathbf{X}l$                           | $\mathbf{X}lang$                             | <i>a</i>                        | $\alpha\beta\sigma\epsilon nt$           | <i>bek</i>                                                  | <i>bst<math>\hat{\chi}</math></i>               | <i>zbett</i>                            | <i>brenn</i>                                 | <i>\zeta</i>                     | <i>xeb</i>                    | <i>\acute{e}</i>                   |                           |             |                                  |
| <i>ernst</i> ~                          | <i>finger</i>                                | <i>fünf</i>                     | <i>gegess</i>                            | <i>gesund</i> ~                                             | <i>hübe</i>                                     | <i>janu</i> ~                           | <i>langsam</i> ~                             | <i>leb</i>                       | <i>leib</i> ~                 | <i>leist</i>                       | <i>lös</i>                | <i>mäd</i>  | <i>manier</i>                    |
| <i>er\ddot{\nu}\sigma\tau</i>           | <i>\phi i\eta\gamma\epsilon r</i>            | <i>\delta\epsilon</i>           | <i>\epsilon\sigma s</i>                  | <i>\gamma\epsilon s\upsilon nd</i>                          | <i>hebe</i>                                     | <i>jnu</i>                              | <i>\gamma\lambda\alpha\eta\sigma\alpha m</i> | <i>\lambda\epsilon\beta</i>      | <i>\lambda\epsilon i\beta</i> | <i>\lambda\epsilon i\sigma\tau</i> | <i>\lambda\sigma\zeta</i> | <i>makd</i> | <i>\mu\alpha\eta i\epsilon r</i> |
| <i>monat</i>                            | <i>\ddot{o}</i>                              | <i>ob</i> ~                     | <i>passag</i>                            | <i>ruh</i>                                                  | <i>schlecht</i>                                 | <i>schock</i>                           | <i>setz</i>                                  | <i>sitz</i>                      |                               |                                    |                           |             |                                  |
| <i>\mu\sigma\eta\alpha t</i>            | <i>\sigma</i>                                | <i>\omega b</i>                 | <i>\rho\alpha\sigma\sigma\alpha g</i>    | <i>\rho\upsilon h</i>                                       | <i>schlecht</i>                                 | <i>schok</i>                            | <i>\zeta\epsilon t\zeta</i>                  | <i>\sigma i\tau\zeta</i>         |                               |                                    |                           |             |                                  |
| <i>sonn</i>                             | <i>\beta</i>                                 | <i>trän</i>                     | <i>tz</i>                                | <i>ü</i>                                                    | <i>über</i>                                     | <i>überred</i> ~                        | <i>verkünd</i>                               | <i>vier</i> ~                    | <i>vulg</i>                   |                                    |                           |             |                                  |
| <i>\sigma\sigma\ddot{\nu}\ddot{\nu}</i> | <i>ss</i>                                    | <i>\tau\epsilon\alpha\rho</i>   | <i>z\tau\zeta</i>                        | <i>u</i>                                                    | <i>xüber</i>                                    | <i>\pi\epsilon\sigma\beta</i>           | <i>\pi\rho\sigma\ddot{\nu}\sigma</i>         | <i>4\epsilon</i>                 | <i>xvulg</i>                  |                                    |                           |             |                                  |
| <i>wahr</i>                             | <i>wasser</i>                                | <i>welt</i>                     | <i>wert</i>                              | <i>wünsch\mathbf{X}</i>                                     | <i>zoll</i>                                     | <i>gebrochen</i>                        | <i>labe</i>                                  | <i>last</i>                      | <i>miss(\emptyset es)</i>     | <i>~is(mus tisch)\mathbf{X}</i>    |                           |             |                                  |
| <i>v\omega\eta\rho r</i>                | <i>\omega\alpha\sigma\epsilon r</i>          | <i>xw\epsilon l\tau</i>         | <i>f\omega\epsilon r\tau</i>             | <i>w\upsilon n\sigma\zeta</i>                               | <i>\tau\sigma\lambda\lambda</i>                 | <i>\beta\rho\epsilon\zeta\epsilon n</i> | <i>\lambda\alpha\beta</i>                    | <i>\lambda\epsilon\sigma\eta</i> | <i>\mu i\sigma</i>            | $\emptyset$                        |                           |             |                                  |

(3) Replace

<sup>58</sup>To avoid confusion of Greek nu with Latin vee, we write the former as  $\ddot{\nu}$  in substitution rules.

|                              |                                                    |                      |                            |                                  |                                                       |                                  |                                |                         |                             |                |                 |                   |             |                 |               |            |
|------------------------------|----------------------------------------------------|----------------------|----------------------------|----------------------------------|-------------------------------------------------------|----------------------------------|--------------------------------|-------------------------|-----------------------------|----------------|-----------------|-------------------|-------------|-----------------|---------------|------------|
| (∅ be)str~<br>σtr            | (∅ ge)last~<br>xlast                               | (∅ ge)lieb~<br>lxieb | (braçte gebraçt)<br>bringe | (lass liess)<br>lass             | abend~<br>azbend                                      | ahn~<br>xzahn                    |                                |                         |                             |                |                 |                   |             |                 |               |            |
| alt~<br>a.lt                 | anz <sub>χ̂</sub> (u)<br>antχ̂                     | arb<br>αrb           | besitz<br>φορτυβ̄          | bes <sub>χ̂</sub> (s)t~<br>gesχ̂ | bet~<br>βbet                                          | bild<br>βild                     | bitter~<br>βitter              | bus~<br>zbus            | çs <sub>χ̂</sub> (t)<br>xχ̂ | daçt<br>denk   | dank<br>thank   | dien<br>dien      |             |                 |               |            |
| dumm<br>δumm                 | erb<br>εrb̄e                                       | fass<br>φass         | fê~<br>fvê                 | folg<br>vfolg                    | froh<br>vroh                                          | fund <sub>χ̂</sub> (e)<br>φundχ̂ | gast<br>γast                   | gel(a i u)ng~<br>geling | gew(a i o)nn<br>wiṽ         | grund<br>grunδ | gruss<br>kgruss |                   |             |                 |               |            |
| gut<br>besser                | hand<br>hanδ                                       | hart<br>xhart        | hu~<br>shu                 | ie<br>î                          | in <sup>X</sup> <sub>(d g k)</sub><br>în <sup>X</sup> | kind<br>gkind                    | klag<br>klag                   | komi<br>komi            | komp<br>comp                | kumm<br>xkumm  | kund<br>xkund   | kuns<br>gkuns     | lêd<br>lêd  | lês~<br>σοφτ    | list<br>ylist | lob<br>lob |
| lock<br>lock                 | lub<br>lub                                         | lust<br>zlust        | mutter<br>μuther           | nahr<br>vahr                     | name<br>vame                                          | nummer<br>xnnummer               | ohr~<br>ohρ                    | ort~<br>ort             | platz<br>pplatz             | raf~<br>ρaf    | reçn<br>peçn    | rest~<br>pest     | saç<br>xsaç | satz<br>xσatz   | sçon<br>zçon  |            |
| sçl<br>sçl                   | segn<br>szegn                                      | setz<br>zsetz        | siçt<br>σiçt               | sieg<br>sxieg                    | sohn<br>szohn                                         | stamm<br>σtamm                   | stand<br>steh                  | stemm<br>σztemm         | suç<br>zsuç                 | tanz<br>tavz   | tisç<br>tisç    | tugend<br>xtugend | uhr~<br>unρ | verg~<br>verzug | vett<br>vwett |            |
| voll<br>ffoll                | w(ê ie)s <sub>χ̂</sub> (s)<br>zxwê <sub>s</sub> χ̂ | wên<br>xvên          | wind<br>wind               | winter<br>wvinter                | wort<br>wvort                                         | wusst<br>wiss                    | zêt<br>zzêt                    |                         |                             |                |                 |                   |             |                 |               |            |
| geh(∅ e en est st t)<br>ging | bat(∅ en est et)<br>bitten                         | gebeten<br>bitten    | herr(∅ en n)<br>hherr      | kam(∅ e en est et st t)<br>komm  | mr<br>hherr                                           |                                  |                                |                         |                             |                |                 |                   |             |                 |               |            |
| oh<br>zxoh                   | sass(∅ en est et t)<br>sitz                        | segen(∅ s)<br>szegn  | tante(∅ n)<br>tante        | ~çs<br>x                         | ~ement(∅ s)<br>îren                                   | ~enz(∅ en)<br>∅                  | ~w(ê ie)s<br>zxwê <sub>s</sub> |                         |                             |                |                 |                   |             |                 |               |            |

(4) If the result so far is an empty string, stop here. Otherwise, break down the result into  $\hat{\sigma}_1\hat{\sigma}_2$ , where  $\ell(\hat{\sigma}_1) = \max\{3, \ell(\hat{\sigma})\}$ , obtain  $\hat{\sigma}'_1$  by doing  $kam\sim \rightarrow zkam$  on  $\hat{\sigma}_1$  before deducing  $\hat{\sigma}'_2$  from  $\hat{\sigma}_2$  in two sequential steps:

(3.1) Do  $el \rightarrow l$ ;

(3.2) Do  $kation\mathbf{X} \rightarrow zîren$ ,  $\sim ln \rightarrow l$ ,  $(ffol|haft|ist|massig)\mathbf{X} \rightarrow \emptyset$ .

Concatenate  $\hat{\sigma}'_1$  and  $\hat{\sigma}'_2$ .

(5) Do  $sç\lambda oç\sim \rightarrow sç\lambda os$ ,  $\sim\chî(a|e|ê|i|i|o|s|u)s \rightarrow \chî$ ,  $\sim\chî\mathbf{V}(çen|ling)(\emptyset|e|en|s) \rightarrow \chî$ ,  $\sim(h|k)êt(\emptyset|en) \rightarrow \emptyset$ ,  $\sim ik(\emptyset|en|er(\emptyset|n|s)) \rightarrow \emptyset$ ,  $\sim lèn(\emptyset|s) \rightarrow \emptyset$ ,  $\sim\mathbf{VX}\chî\mathbf{V}^*st \rightarrow \mathbf{VX}\chî$  on  $\hat{\sigma}'_1\hat{\sigma}'_2$ .

**Definition 5.16** (German protected range). Set  $\mathbf{V}^* = (a|ê|i|i|o|u)$ ,  $\mathbf{C}_{m_0} = \overline{(a|e|ê|i|i|o|u)}_{m_0}$  and  $\mathbf{C}_m = \overline{(a|e|i|o|u|ê|i)}_m$ . Let  $\hat{\sigma}$  be the effective spelling of a German word, its protected range  $\text{ProtRg}(\hat{\sigma}) = \max\{\lambda_1(\hat{\sigma}), \lambda_2(\hat{\sigma})\}$  is determined by two non-negative integers  $\lambda_1(\hat{\sigma})$  and  $\lambda_2(\hat{\sigma})$  specified through the following procedures:

- Look for the string pattern  $((\emptyset|a|b|e|e|ê|ê|r|g|e|i|i|mit|naç|u|vor|xüber|zer|zu)\mathbf{C}_{m_0}\mathbf{V}^*|\mathbf{C}_me)\overline{(a|e|ê|i|i|r|u)}_{m_0}\sim$  in the string  $\hat{\sigma}$ ;
  - If the string pattern above is found, the last position occupied by such a string defines  $\lambda_1(\hat{\sigma})$ ; otherwise, set  $\lambda_1(\hat{\sigma}) = 0$ ;
  - Look for the pattern  $(a|o|u)$  in the string  $\hat{\sigma}$ ;
  - If a letter in the pattern above is found, the last position occupied by such a letter defines  $\lambda_2(\hat{\sigma})$ ; otherwise, set  $\lambda_2(\hat{\sigma}) = 0$ .
- 

Unlike Danish, but similar to Dutch, our German essential root is free from common separable verb prefixes (see step (3) in the algorithm below).

**Algorithm 5.17** (German essential root). Set  $\mathbf{V} = (a|e|ê|i|i|o|u)$  and  $\mathbf{C} = \overline{(a|e|ê|i|i|o|u)}$ . Let  $\hat{\sigma}$  be the effective spelling of a German word, then its corresponding essential root  $\text{EssRoot}(\hat{\sigma})$  is constructed in the following steps:

- (1) Break down  $\hat{\sigma} = \hat{\sigma}_1\hat{\sigma}_2$  into the concatenation of two strings  $\hat{\sigma}_1 = \hat{\sigma}^{[\text{ProtRg}(\hat{\sigma})]}$  (see the notation in Definition 3.1) and  $\hat{\sigma}_2$ , where the length of the first string  $\ell(\hat{\sigma}_1) = \text{ProtRg}(\hat{\sigma})$  is equal to the protected range of  $\hat{\sigma}$ .
- (2) On  $\hat{\sigma}_2$ , perform the following substitutions in a sequel:<sup>59</sup>

(2.1) Do  $\sim s \rightarrow \emptyset$ ;

(2.2) Do  $\sim e(d|e|m|n|r|st|t)_{m_0} \rightarrow \emptyset$ .

<sup>59</sup>In other words, the core algorithm for essential root extraction runs as follows: keep the last “strong” vowel  $a$ ,  $i$ ,  $o$  or  $u$  in non-final position, plus one subsequent letter; delete final  $a$ ; erase the final appearance of  $e$  and all the letters thereafter.

The result after these two steps of operations is called  $\hat{\sigma}'_2$ .

(3) Concatenate  $\hat{\sigma}_1$  and  $\hat{\sigma}'_2$ , before doing

$$(\emptyset|ab|an|auf|aus|b\acute{e}|dur|ç|én|h(er)|in)(\emptyset|ab|an|auf|aus|én|xü|ber)|mit|naç|um|vor|wé|ter|w(i|i)|der|xü|ber|zu(\emptyset|ruck))(\emptyset|ge|zu)\mathbf{XV}\sim\rightarrow\mathbf{XV};$$

(4) Do  $(\hat{\chi}_{\times 2}t|\sim\hat{\chi}_{\times 2})\rightarrow\hat{\chi}$ ,<sup>60</sup> (Check Example 3.4.2 to see the notation  $\hat{\chi}_{\times 2}$  for double letters.)

(5) Do  $\sim Ct\rightarrow C$ ,  $nd\rightarrow\check{v}d$ .

### 5.2.2 Admissible mutation and approximate clustering

Like English, German has hundreds of irregular verbs in daily use. Unlike English, these German verbs may not only have irregular past tense and past participles, but also have irregular present tense conjugations.

The German vowel blotting mechanism is similar to the Danish version (Algorithm 5.5).

**Algorithm 5.18** (German vowel blotting). Set  $\mathbf{V}_m = (a|e|\acute{e}|i|\check{i}|o|u)_m$  and  $\mathbf{C}_{m_0} = \overline{(a|e|\acute{e}|i|\check{i}|o|u)}_{m_0}$ . For a token string  $\hat{\sigma}$ , its blotted form  $\text{BlotV}_1(\hat{\sigma})$  is constructed as follows:

- If the string pattern  $(\emptyset|a|b|e|\acute{e}|i|\check{i}|o|u)\mathbf{C}_{m_0}\mathbf{V}_m\sim$  can be found in the string  $\hat{\sigma}$ , then the last position occupied by such a pattern is replaced by the letter “a”.
- Otherwise, leave the string  $\hat{\sigma}$  intact.

Similar to what we did in §5.1.2 for the case of Danish, we will construct a bivariate Boolean-valued function  $\text{HrdTest}(\hat{\alpha},\hat{\beta})$  on a “simple heredity test function” in Algorithm 5.19, and a set of “admissible suffix mismatch and vowel alternation” rules in Algorithm 5.20.

**Algorithm 5.19** (Simple heredity test). Suppose that  $\hat{\alpha}$  and  $\hat{\beta}$  are both lowercase strings. Set  $\mathbf{V} = (a|e|\acute{e}|i|\check{i}|o|u)$ . The Boolean-valued function  $\text{SimpHrdTest}(\hat{\alpha},\hat{\beta})$  returns **TRUE** if  $\hat{\alpha}$  contains at least one instance of  $\mathbf{V}$ , **AND** at least one of the following four conditions holds.<sup>61</sup>

- $\hat{\alpha} = \hat{\beta}$ ;
- $\hat{\beta} = \hat{\alpha}d$ ;
- $\hat{\beta} = \hat{\alpha}t$ ;
- Appending the last character of  $\hat{\alpha}$  to itself, one obtains  $\hat{\beta}$ , i.e.  $\hat{\alpha}\Omega(\hat{\alpha}) = \hat{\beta}$ ;
- $\ell(\hat{\beta}) > \ell(\hat{\alpha}) \geq \frac{\ell(\hat{\beta})}{2}$  **AND**  $\hat{\alpha} = \hat{\beta}^{[\ell(\hat{\alpha})]}$  **AND**  $\hat{\beta}^{\ell(\hat{\alpha})+1} = (e|n|s)$ . (See Definition 3.1 for the notations  $\hat{\beta}^{[n]}$  and  $\hat{\beta}^{\{n\}}$ .)

In what follows, we define  $\text{SuffixNW}(\hat{\alpha},\hat{\beta})$ ,  $\text{RootNW}(\hat{\alpha},\hat{\beta})$ ,  $\text{NW}^*(\hat{\alpha},\hat{\beta})$  and  $\text{SuffixSW}(\hat{\alpha},\hat{\beta})$ ,  $\text{SuffixSW}(\hat{\alpha},\hat{\beta})$ ,  $\text{SW}^*(\hat{\alpha},\hat{\beta})$  as what is done in the Danish case (Algorithm 5.7).

**Algorithm 5.20** (Admissible suffix mismatch and vowel alternation). For two strings  $\hat{\alpha}$  and  $\hat{\beta}$ , the Boolean-valued function

$$\text{AdmMut}(\text{RootNW}(\hat{\alpha},\hat{\beta}), \text{SuffixNW}(\hat{\alpha},\hat{\beta}), \text{NW}^*(\hat{\alpha},\hat{\beta}))$$

returns **TRUE** if<sup>62</sup>

$$(\text{SuffixNW}(\hat{\alpha},\hat{\beta}) = [(\emptyset|(d|e|n|t)_m|(\Omega(\text{RootNW}(\hat{\alpha},\hat{\beta}))|bar|er|ig|in|\acute{r}|is|ç|li|ç|sam|st|tum|ung)\mathbf{X}), \\ (\emptyset|(d|e|n|t)_m|(\Omega(\text{RootNW}(\hat{\alpha},\hat{\beta}))|bar|er|ig|in|\acute{r}|is|ç|li|ç|sam|st|tum|ung)\mathbf{X})])$$

$$\text{OR } \text{SuffixNW}(\hat{\alpha},\hat{\beta}) = [ih,og] \text{ OR } \text{SuffixNW}(\hat{\alpha},\hat{\beta}) = [og,ih]$$

**AND** at least one of the following three conditions holds:<sup>63</sup>

- $\text{NW}^*(\hat{\alpha},\hat{\beta}) = \emptyset$  **AND**  $\text{RootNW}(\hat{\alpha},\hat{\beta})$  contains at least one instance of  $(a|e|\acute{e}|i|\check{i}|o|u|z)$ ;

<sup>60</sup>In *Mathematica* codes, the substitution rule reads  $\{\mathbf{x}_\sim\sim\mathbf{x}_\sim\sim\mathbf{t} \mid \text{WordBoundary} \rightarrow \mathbf{x}\}$ .

<sup>61</sup>As a general rule in this document, the truth values of items labeled with Roman numerals are connected to each other with logical **OR**.

<sup>62</sup>Depending on the programming language chosen, the string *ih* may be sorted before or after *og*.

<sup>63</sup>We note that  $\text{NW}^*(\hat{\alpha},\hat{\beta})$  and  $\text{NW}^*(\hat{\beta},\hat{\alpha})$  differ only in the order of the two components in the bracket.

- (ii)  $NW^*(\hat{\alpha}, \hat{\beta}) = ([a, e][a, i][a, \hat{i}][a, \hat{i}][a, o][a, u][ah, i][ah, o][au, \hat{i}][au, o][e, \hat{i}][e, \hat{i}][e, o][\hat{e}, \hat{i}][\hat{e}, \hat{i}][eh, i][eh, o][i, o][\hat{i}, \hat{i}][\hat{i}, o][\hat{i}, u][o, u]);$
- (iii)  $NW^*(\hat{\beta}, \hat{\alpha}) = ([a, e][a, \hat{i}][a, \hat{i}][a, \hat{i}][a, o][a, u][ah, i][ah, o][au, \hat{i}][au, o][e, \hat{i}][e, \hat{i}][e, o][\hat{e}, \hat{i}][\hat{e}, \hat{i}][eh, i][eh, o][i, o][\hat{i}, \hat{i}][\hat{i}, o][\hat{i}, u][o, u]).$

Similarly, one can evaluate another Boolean-valued function

$$\text{AdmMut}(\text{RootSW}(\hat{\alpha}, \hat{\beta}), \text{SuffixSW}(\hat{\alpha}, \hat{\beta}), \text{SW}^*(\hat{\alpha}, \hat{\beta}))$$

by trading all the occurrences of NW in the statements above with SW.

**Algorithm 5.21** (Heredity test function). *In what follows,  $\ell([\hat{\sigma}, \hat{\tau}]) = \min\{\ell(\hat{\sigma}), \ell(\hat{\tau})\}$ . For two strings  $\hat{\alpha}$  and  $\hat{\beta}$ , the Boolean-valued function  $\text{HrdTest}(\hat{\alpha}, \hat{\beta})$  returns **TRUE** if at least one of the following three conditions holds:*

- (i)  $\text{SimpHrdTest}(\hat{\alpha}, \hat{\beta}) = \text{TRUE};$
- (ii)  $\ell(\text{RootNW}(\hat{\alpha}, \hat{\beta})) + \ell(\text{SuffixNW}(\hat{\alpha}, \hat{\beta})) + \ell(\text{NW}^*(\hat{\alpha}, \hat{\beta})) \geq \frac{\max\{\ell(\hat{\alpha}), \ell(\hat{\beta})\}}{2}$  **AND**  $\text{AdmMut}(\text{RootNW}(\hat{\alpha}, \hat{\beta}), \text{SuffixNW}(\hat{\alpha}, \hat{\beta}), \text{NW}^*(\hat{\alpha}, \hat{\beta})) = \text{TRUE};$
- (iii)  $\ell(\text{RootSW}(\hat{\alpha}, \hat{\beta})) + \ell(\text{SuffixSW}(\hat{\alpha}, \hat{\beta})) + \ell(\text{SW}^*(\hat{\alpha}, \hat{\beta})) \geq \frac{\max\{\ell(\hat{\alpha}), \ell(\hat{\beta})\}}{2}$  **AND**  $\text{AdmMut}(\text{RootSW}(\hat{\alpha}, \hat{\beta}), \text{SuffixSW}(\hat{\alpha}, \hat{\beta}), \text{SW}^*(\hat{\alpha}, \hat{\beta})) = \text{TRUE}.$

**Algorithm 5.22** (Approximate clustering of German words). *The algorithm is essentially the same as Algorithm 5.10, except that German rules (instead of Danish rules) apply to all the tags (effective spelling, essential root, vowel blotting etc.).*

*Example 5.22.1.* As an illustration of our clustering algorithm, we pick the following families of German words, where an “approximate translation” in English, enclosed in quotation marks, is appended to the end of each family:

*Apfel, Äpfel, Äpfelchen, Äpfeln, Apfels — “apple”;*  
*Arbeit, arbeite, arbeiten, Arbeiten, arbeitest, arbeitet, arbeitete, arbeiteten, gearbeitet — “work”;*  
*Arbeiter, Arbeitern, Arbeiters — “worker”;*  
*Arbeitsplatz, Arbeitsplatze, Arbeitsplätze, Arbeitsplätzen, Arbeitsplatzes — “workplace”;*  
*Arbeitstag, Arbeitstage, Arbeitstagen, Arbeitstages, Arbeitstags — “workday”;*  
*Bus, Busse, Bussen, Busses — “bus”;*  
*Buße, Bußen — “penance”;*  
*dunkel, dunkelste, dunkelstem, dunkelsten, dunkelster, dunkelstes, dunkle, dunklem, dunklen, dunkler, dunklere, dunklerem, dunkleren, dunklerer, dunkleres, dunkles — “dark”;*  
*Ei, Eie, Eier, Eiern, Eies, Eis — “egg”;*  
*Eigelb, Eigelbe, Eigelben, Eigelbs — “egg yolk”;*  
*Eis, Eise, Eises — “ice”;*  
*frei, freie, freiem, freien, freier, freiere, freierem, freieren, freierer, freieres, freies, freiste, freistem, freisten, freisten, freister, freistes — “free”;*  
*Freiheit, Freiheiten — “freedom”;*  
*gehaust, haus, Haus, Häuschen, hause, Hause, hausen, hausend, Häuser, Hauses, haust, hauste, hauste, haustest — “house”;*  
*geküsst, Kuss, Kuß, Küsschen, Kusse, küsse, Küsse, küssen, Küssen, Kusses, küssest, küsst, küsste, küsstest, küsstet — “kiss”;*  
*gelb, gelbe, gelbem, gelben, gelber, gelbere, gelberem, gelberen, gelberer, gelberes, gelbes, gelbste, gelbstem, gelbsten, gelbster, gelbstes — “yellow”;*  
*gross, groß, große, großem, großen, größer, größere, größerem, größeren, größerer, größeres, großes, größte, größtem, größten, größter, größtes — “big”;*  
*Öl, Öle, Ölen, Öles, Öls — “oil”;*  
*Platz, Platze, Plätze, Plätzen, Platzes — “place”;*  
*studier, studiere, studiere, studiere, studieren, studierend, studierest, studieret, studierst, studiert, studiert, studierte, studierte, studierten, studiertest, studiertest, studiertet — “study”;*  
*Tag, Tage, Tagen, Tages, Tags — “day”.*

Applying Algorithm 5.22 to this list of words, we obtain the following clustering results:

{*Apfel, Äpfel, Äpfelchen, Äpfeln, Apfels*}, {*Arbeit, arbeite, arbeiten, Arbeiten, Arbeiter, Arbeitern, Arbeiters, arbeitest, arbeitest, arbeitete, arbeiteten, gearbeitet*}, {*Arbeitsplatz, Arbeitsplatze, Arbeitsplätze, Arbeitsplätzen, Arbeitsplatzes*}, {*Arbeitstag, Arbeitstage, Arbeitstagen, Arbeitstages, Arbeitstags*}, {*Bus, Busse, Buße, Bussen, Bußen, Busses*}, {*dunkel, dunkelste, dunkelstem, dunkelsten, dunkelster, dunkelstes, dunkle, dunklem, dunklen, dunkler, dunklere, dunklerem, dunkleren, dunklerer, dunkleres, dunkles*}, {*Ei, Eie, Eier, Eiern, Eies*}, {*Eigelb, Eigelbe, Eigelben, Eigelbs*}, {*Eis, Eise, Eises*}, {*frei, freie, freiem, freien, freier, freiere, freierem, freieren, freierer, freieres, freies, Freiheit, Freiheiten, freiste, freistem, freisten, freister, freistes*}, {*gehaust, haus, Haus, Häuschen, hause, Hause, hausen, hausend, Häuser, Hauses, haust, hauste, haustest*}, {*geküsst, Kuss, Kuß, Küsschen, Kusse, küsse, Küsse, küssen, Küssen, Kusses, küssest, küsst, küsste, küsstest, küsstet*}, {*gelb, gelbe, gelbem, gelben, gelber, gelbere, gelberem, gelberen, gelberer, gelberes, gelbes, gelbste, gelbstem, gelbsten, gelbster, gelbstes*}, {*gross, groß, große, großem, großen, größer, größere, größerem, größeren, größerer, größeres, großes, größte, größtem, größten, größter, größtes*}, {*Öl, Öle, Ölen, Öles, Öls*}, {*Platz, Platze, Plätze, Plätzen, Platzes*}, {*studier, studiere, studieren, studierend, studierest, studieret, studierst, studiert, studierte, studierten, studiertest, studiertet*}, {*Tag, Tage, Tagen, Tages, Tags*}.

*Example 5.22.2.* To further test our algorithm against German irregular verbs with various vowel alternation patterns across different tenses and moods, we throw the following list:

*befahl, befähle, befahlen, befählen, befählest, befählet, befahlst, befahlt, befehle, befehlen, befehlend, befehlest, befehlet, befehlt, befiehlst, befiehlt, befohlen* — “command”;

*begann, begänne, begannen, begännen, begännest, begännet, begannst, begannt, beginn, beginne, beginnen, beginnend, beginnest, beginnet, beginnst, beginnt, begönne, begonnen, begönnen, begönnest, begönnet* — “begin”;

*beiß, beiße, beißen, beißend, beißest, beißet, beißt, biss, bisse, bissen, bisset, bisst, gebissen* — “bite”;

*blas, blase, blasen, blasend, blasest, blaset, blast, bläst, blies, bliese, bliesen, bliesest, blieset, bliest, geblasen* — “blow”;

*brach, bräche, brachen, brächen, brächest, brächet, brachst, bracht, breche, brechen, brechend, brechest, brechet, brecht, brich, brichst, bricht, gebrochen* — “break”;

*brät, brate, braten, bratend, bratest, bratet, brätst, briet, briete, brieten, brietest, brietet, gebraten* — “fry”;

*fahr, fahre, fahren, fahrend, fahrest, fahret, fährst, fahrt, fährt, fuhr, führe, fahren, führen, führest, führet, fuhrst, fuhrt, gefahren* — “drive”;

*fall, falle, fallen, fallend, fallest, fallet, fällt, fallt, fällt, fiel, fiele, fielen, fielest, fielet, fielst, fielt, gefallen* — “fall”;

*fand, fände, fanden, fänden, fandest, fändest, fandet, fändet, finde, finden, findend, findest, findet, gefunden* — “find”;

*fechte, fechten, fechtend, fechtest, fechtet, ficht, fichtst, focht, föchte, fochten, föchten, fochtest, föchtest, fochtet, föchtet, gefochten* — “fence”;

*flieg, fliege, fliegen, fliegend, fliegest, flieget, fliegst, fliegt, flog, flöge, flogen, flögen, flögest, flöget, flogst, flogt, geflogen* — “fly”;

*fraß, fräße, fraßen, fräßen, fräbest, fräbet, fraßt, fresse, fressen, fressend, fressest, fresset, frisst, friss, frisst, gefressen* — “feed”;

*galt, gälte, galten, gälten, galtest, gältest, galtet, gältet, gegolten, gelte, gelten, geltend, geltest, geltet, gilt, giltst, gölte, gölten, göltest, göltet* — “count”;

*geglichen, gleich, gleiche, gleichen, gleichend, gleichest, gleichet, gleichst, gleicht, glich, gliche, glichen, glichest, glichet, glichst, glicht* — “resemble”;

*gegriffen, greif, greife, greifen, greifend, greifest, greifet, greifst, greift, griff, griffe, griffen, griffest, griffet, griffst, grifft* — “grab”;

*gehangen, häng, hänge, hängen, hängend, hängest, hänget, hängst, hängt, hing, hinge, hingen, hingest, hinget, hingst, hingt* — “hang”;

*gehoben, haben, heb, hebe, heben, hebend, hebest, hebet, hebst, hebt, hob, höbe, hoben, höben, höbest, höbet, hobst, hobt, hübe, hüben, hübest, hübet* — “heave”;

*gekrochen, krieche, kriechen, kriechend, kriechest, kriechet, kriechst, kriecht, kroch, kröche, krochen, kröchen, kröchest, kröchet, krochst, krocht* — “creep”;

*gelaufen, lauf, laufe, laufen, laufend, laufest, laufet, läufst, läuft, läuft, lief, liefe, liefen, liefest, liefet, liefst, lieft* — “walk”;

*gelesen, las, läse, lasen, läsen, läsest, läset, last, lese, lesen, lesend, lesest, leset, lest, lies, liest* — “read”;

*genommen, nahm, nähme, nahmen, nähmen, nähmest, nähmet, nahmst, nimmt, nehme, nehmen, nehmend, nehmet, nehmet, nehmt, nimm, nimmst, nimmt* — “take”;

*geritten, reite, reiten, reitend, reitest, reitet, ritt, ritte, ritten, rittest, rittet* — “ride”;

*gerufen, rief, riefe, riefen, riefest, riefet, riefst, rief, ruf, rufe, rufen, rufend, rufest, rufet, rufst, ruft* — “shriek”;



### 5.2.3 Heuristic detection of compounds

The following algorithm for heuristic detection of German compounds differs from the Danish version (Algorithm 5.12) only in some specific details. To make the context clear, we still state the algorithm in full. (In what follows, the string minus operation  $\hat{\beta} \ominus \hat{\alpha}$  is prescribed by Definition 5.11.)

**Algorithm 5.23** (Heuristic identification of German binary compounds). *Let  $\Lambda^{\hat{\rho}} = \{\hat{\rho}_1, \dots, \hat{\rho}_Q\}$  be a list of distinct German essential roots (without vowel blotting) that contain at least one instance of  $\mathbf{V} = (a|e|\acute{e}|i|\acute{i}|o|u)$  and DO NOT match the following string patterns:*

*(ab|al|am|ar|arg|bar|be|beg|bek|bek|ên|fal|gel|gros|isç|los|mal|man|miss|naç|nis|sam|sçaf|sçaf|tal|u|un|ung|ver|vers|xüber).*

*The the output of the function  $\text{CpdDet}(\Lambda^{\hat{\rho}})$  is obtained through the following procedures:*

- (1) *Construct a list  $\{(\hat{\rho}_1, \lambda_1^{\hat{\rho}}), \dots, (\hat{\rho}_Q, \lambda_Q^{\hat{\rho}})\}$  where  $\lambda_q^{\hat{\rho}} = \{\hat{\rho}_{(q,1)}, \dots, \hat{\rho}_{(q,n_q)}\}$  is a subset of  $\Lambda^{\hat{\rho}}$  whose members all match the string pattern  $\hat{\rho}_{q\sim}$ , for  $q \in \mathbb{Z} \cap [1, Q]$ .*
- (2) *Expand the aforementioned entry  $(\hat{\rho}_q, \lambda_q^{\hat{\rho}})$  into a list of triplets  $\{(\hat{\rho}_{(q,1)}, \hat{\rho}_q, \hat{\rho}_{(q,1)} \ominus \hat{\rho}_q), \dots, (\hat{\rho}_{(q,n_q)}, \hat{\rho}_q, \hat{\rho}_{(q,n_q)} \ominus \hat{\rho}_q)\}$  for every  $q \in \mathbb{Z} \cap [1, Q]$  such that  $\lambda_q^{\hat{\rho}} \neq \emptyset$ . Collect all these triplets as one runs through the list  $\{(\hat{\rho}_1, \lambda_1^{\hat{\rho}}), \dots, (\hat{\rho}_Q, \lambda_Q^{\hat{\rho}})\}$ . The list of these triplets  $\{(\hat{\rho}_{(1)}, \hat{\eta}_{(1)}, \hat{\rho}_{(1)} \ominus \hat{\eta}_{(1)}), \dots, (\hat{\rho}_{(Q)}, \hat{\eta}_{(Q)}, \hat{\rho}_{(Q)} \ominus \hat{\eta}_{(Q)})\}$  contains potentially valid decompositions of compounds.*
- (3) *Screen the aforementioned list of triplets as follows: for every  $q' \in \mathbb{Z} \cap [1, Q']$ , if  $(\hat{\rho}_{(q')}, \hat{\eta}_{(q')}, \hat{\tau}_{(q')} = \hat{\rho}_{(q')} \ominus \hat{\eta}_{(q')})$  satisfies*

$$\ell(\hat{\rho}_{(q')} \ominus \hat{\eta}_{(q')}) \geq 2 \quad \text{AND} \quad \hat{\rho}_{(q')} \ominus \hat{\eta}_{(q')} = \mathbf{X}_1(a|e|\acute{e}|i|\acute{i}|o|u)\mathbf{X}_2,$$

*then construct  $\hat{\tau}_{(q')}$  by performing  $(e|n|s)\sim \rightarrow \emptyset$  on  $\hat{\tau}_{(q')}$  and  $\hat{\tau}_{(q')}^*$  by doing  $(e|n|e|s|g|e)\sim \rightarrow \emptyset$  on  $\hat{\tau}_{(q')}$ , before generating a list  $\lambda_{(q')}^{\hat{\tau}}$  by members of  $\Lambda^{\hat{\rho}}$  that match the pattern  $(\hat{\tau}_{(q')}|\hat{\tau}_{(q')}^*|\hat{\tau}_{(q')}^*)$ ; otherwise, set  $\lambda_{(q')}^{\hat{\tau}} = \emptyset$ .*

- (4) *Collect all the triplets  $(\hat{\rho}_{(q')}, \hat{\eta}_{(q')}, \lambda_{(q')}^{\hat{\tau}})$  where  $\lambda_{(q')}^{\hat{\tau}}$  is non-void and  $\hat{\tau}_{(q')}$  DOES NOT match the following string patterns:*

*(hêtX|liçX|kêtX|um|ungX).*

*This list of triplets  $\text{CpdDet}(\Lambda_{\hat{\rho}})$  contains the heuristic decompositions of all the identified binary compounds.*

**Algorithm 5.24** (Approximate clustering of German words with heuristic detection of compounds). *The procedure runs essentially the same way as Algorithm 5.24, except that German rules replace Danish rules.*

*Example 5.24.1.* Testing the algorithm above against the combined inputs from Examples 5.22.1 and 5.22.2, we obtain the following result:

*{Apfel, Äpfel, Äpfelchen, Äpfeln, Apfels}, {Arbeit, arbeite, arbeiten, Arbeiten, Arbeiter, Arbeitern, Arbeiters, arbeitest, arbeitet, arbeitete, arbeiteten, Arbeitsplatz, Arbeitsplatze, Arbeitsplätze, Arbeitsplätzen, Arbeitsplatzes, Arbeitstag, Arbeitstage, Arbeitstagen, Arbeitstages, Arbeitstags, gearbeitet}, {Arbeitsplatz, Arbeitsplatze, Arbeitsplätze, Arbeitsplätzen, Arbeitsplatzes, Platz, Platze, Plätze, Plätzen, Platzes}, {Arbeitstag, Arbeitstage, Arbeitstagen, Arbeitstages, Arbeitstags, Tag, Tage, Tagen, Tages, Tags}, {befahl, befähle, befahlen, befählen, befählest, befählet, befahlst, befahlt, befehle, befehlen, befehlend, befehlest, befehlet, befiehlt, befiehst, befiehlt, befohlen}, {begann, begänne, begannen, begännen, begännest, begännet, begannst, begannt, beginn, beginne, beginnen, beginnend, beginnest, beginnet, beginnst, beginnt, begönne, begonnen, begönnen, begönnest, begönnet}, {beiß, beiße, beißen, beißend, beißest, beißet, beißt, biss, bisse, bissen, bissest, bisset, bisst, gebissen}, {blas, blase, blasen, blasend, blasest, blaset, blast, bläst, blies, bliese, bliesen, bliesest, blieset, bliest, geblasen}, {brach, brä- che, brachen, brächen, brächest, brächet, brachst, bracht, breche, brechen, brechend, brechest, brechet, brecht, brich, brichst, bricht, gebrochen}, {brät, brate, braten, bratend, bratest, bratet, brätst, briet, briete, brieren, brie- test, brieret, gebraten}, {Bus, Busse, Buße, Bussen, Bußen, Busses}, {dunkel, dunkelste, dunkelstem, dunkelsten, dunkelster, dunkelstes, dunkle, dunklem, dunklen, dunkler, dunklere, dunklerem, dunkleren, dunklerer, dunkleres, dunkles}, {Ei, Eie, Eier, Eiern, Eies, Eigelb, Eigelbe, Eigelben, Eigelbs}, {Eigelb, Eigelbe, Eigelben, Eigelbs, gelb, gelbe, gelbem, gelben, gelber, gelbere, gelberem, gelberer, gelberes, gelbes, gelbste, gelbstem, gelbsten, gelbster, gelbstes}, {Eis, Eise, Eises}, {fahr, fahre, fahren, fahrend, fahrest, fahret, fährt, fährt, fährt, führt, führe, führen, führen, führest, führet, fuhrst, fuhrt, gefahren}, {fall, falle, fallen, fallend, fallest, fallet, fällt, fällt, fällt, fiel, fielen, fielen, fielest, fielet, fielt, fiel, gefallen}, {fand, fände, fanden, fänden, fandest, fandest, fandet, fändet, finde, finden, findend, findest, findet, gefunden}, {fechte, fechten, fechtend, fechtest, fechtet, ficht, fichtst, focht, föchte, fochten, föchten, fochtest, föchtest, fochtet, föchtet, gefochten}, {flieg, fliege, fliegen, flie- gend, fliegest, flieget, fliegst, fliegt, flog, flöge, flogen, flögen, flögest, flöget, flogst, flogt, geflogen}, {fraß, fräße,*

*fraßen, fräßen, fräßest, fräßet, fraßt, fresse, fressen, fressend, fressest, fresset, fressst, friss, frisst, gefressen*}, {*frei, freiem, freien, freier, freiere, freierem, freieren, freierer, freieres, freies, Freiheit, Freiheiten*}, {*freie, freiste, freistem, freisten, freister, freistes*}, {*galt, gälte, galten, gälten, galtest, gältest, galtet, gältet, gegolten, gelte, gelten, geltend, geltest, geltet, gilt, giltst, gölte, gölten, göltest, göltet*}, {*geglichen, gleich, gleiche, gleichen, gleichend, gleichest, gleichet, gleichst, gleich, glich, gliche, glichen, gleichst, glichet, glichst, glicht*}, {*gegriffen, greif, greife, greifen, greifend, greifest, greifet, greifst, greift, griff, griffe, griffen, griffest, griffet, griffst, griffst, griffst*}, {*gehangen, häng, hänge, hängen, hängend, hängest, hängst, hängst, hängst, hing, hinge, hingen, hingest, hingst, hingst, hingst*}, {*gehaust, haus, Haus, Häuschen, hause, Hause, hausen, hausend, Häuser, Hauses, haust, hauste, haustest*}, {*gehoben, haben, heb, hebe, heben, hebend, hebest, hebet, hebst, hebt, hob, höbe, hoben, höben, höbest, höbet, hobst, hobt, hübe, hüben, hübest, hübet*}, {*gekrochen, krieche, kriechen, kriechend, kriechest, kriechet, kriechst, kriecht, kroch, kröche, krochen, kröchen, kröchest, kröchet, krochst, krocht*}, {*geküsst, Kuss, Kuß, Küsschen, Kusse, küsse, Küsse, küssen, Küssen, Kusses, küssest, küsst, küsste, küsstest, küsstet*}, {*gelaufen, lauf, laufe, laufen, laufend, laufest, laufet, läufst, läuft, lief, liefe, liefen, liefest, liefet, liefst, lieft*}, {*gelesen, las, läse, lasen, läsen, läsest, läset, last, lese, lesen, lesend, lesest, leset, lest, lies, liest*}, {*genommen, nahm, nähme, nahmen, nähmen, nähmest, nähmet, nahmst, nimmt, nehme, nehmen, nehmend, nehmest, nehmet, nehmt, nimm, nimmst, nimmt*}, {*geritten, reite, reiten, reitend, reitest, reitet, ritt, ritte, ritten, rittest, rittet*}, {*gerufen, rief, riefte, riefen, riefest, riefet, riefst, riefst, ruf, rufe, rufen, rufend, rufest, rufet, rufst, ruft*}, {*geschlafen, schlaf, schlafe, schlafen, schlafend, schlafest, schlafet, schläfst, schläft, schlief, schliefte, schliefen, schliefest, schliefet, schliefst, schliefst*}, {*geschlossen, schließ, schließe, schließen, schließend, schließest, schließet, schließt, schloss, schlösse, schlossen, schlössen, schlossest, schlössest, schlosset, schlösset, schlosst*}, {*geschrieben, schreibe, schreiben, schreibend, schreibest, schreibet, schreibst, schreibt, schrieb, schriebe, geschrieben, schriebest, schriebet, schriebst, schriebst*}, {*gesoffen, sauf, saufe, saufen, saufend, saufest, saufet, säufst, sauft, säuft, soff, söffe, sofften, söffen, söffest, söffet, soffst, soffst*}, {*gestoßen, stieß, stieße, stießen, stießest, stießet, stießt, stoß, stoße, stoßen, stoßend, stoßest, stoßet, stoßt, stößt*}, {*getroffen, traf, trafe, trafen, träfen, träfest, träfet, trafst, traf, treffe, treffen, treffend, treffest, treffet, trifft, trifft, trifftst, trifftst*}, {*gezogen, zieh, ziehe, ziehen, ziehend, ziehest, ziehet, ziehst, zieht, zog, zöge, zogen, zögen, zögest, zöget, zogst, zogt*}, {*gross, groß, große, großem, großen, großer, größere, größerem, größeren, größerer, größeres, großes, größte, größtem, größten, größter, größtes*}, {*Öl, Öle, Ölen, Öles, Öls*}, {*studier, studiere, studieren, studierend, studierest, studieret, studierst, studiert, studierte, studierten, studiertest, studiertet*}.

Here, the compounds *Arbeitsplatz* “workplace”, *Arbeitstag* “workday” and *Eigelb* “egg yolk” are correctly dissolved into their respective constituting components. In the meantime, we note that *bisse* “bite (a subjunctive form)” is not confused with the noun *Busse* “buses (nominative, genitive or accusative)”, because the vowel alternation pattern [i, u] is disallowed in German tags (effective spellings or essential roots), unlike the case in English. Actual German verb conjugations do exhibit alternations between the vowels *i* and *u*, when the vowel in question is followed by *nd*, *ng* or *nk*. Our Algorithm 5.15(3) takes care of this by relabeling *i* in such scenarios as  $\hat{i}$ , so that the vowel alternation pattern [i, u] will be later permitted in Algorithm 5.20.

*Example 5.24.2.* In Fig. S5, we further apply the aforementioned word clustering algorithm to topic extraction and machine translation (see Table S1 for text sources).

According to German orthography, diacritical marks in the letters *ä*, *ö*, *ü* are ignored during alphabetical sorting. This rule, if implemented literally, sometimes reduces readability of certain stacked vowels in our word clusters. Therefore, in Fig. S5, we make a compromise: the letters *ä*, *ö*, *ü* are sorted after *z* during alphabetization, as in Swedish orthography.

It should be noted that we have used a German version for *Jane Eyre* that contains pre-1902 spellings. For example, in Fig. S5a'–B', we see *Thee* “tea” and *Thür* “door” instead of their modern counterparts *Tee* and *Tür*. Fortunately, our stemming algorithm is not adversely affected by such archaic orthography.

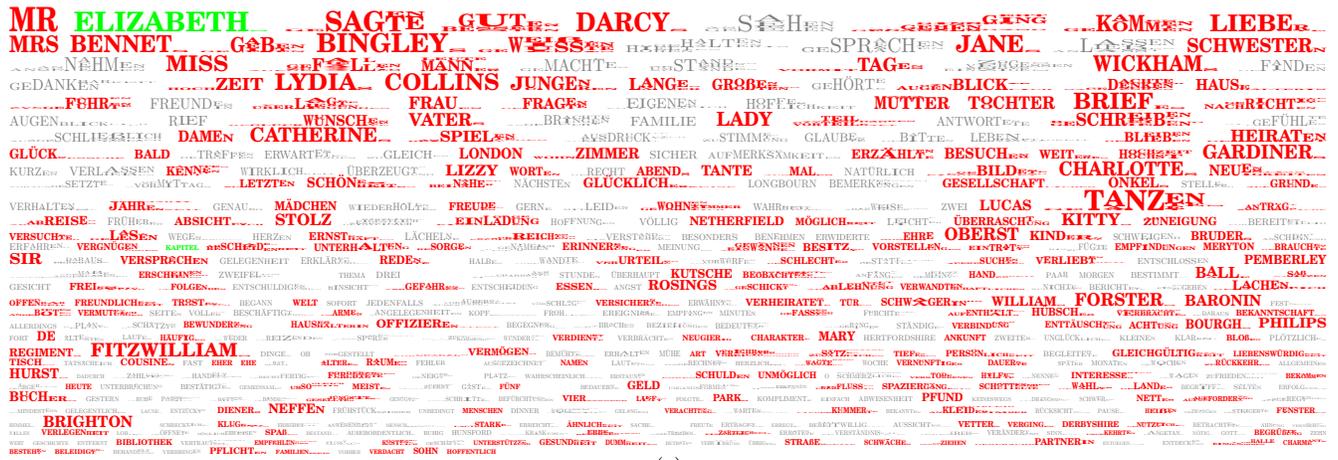

(a)

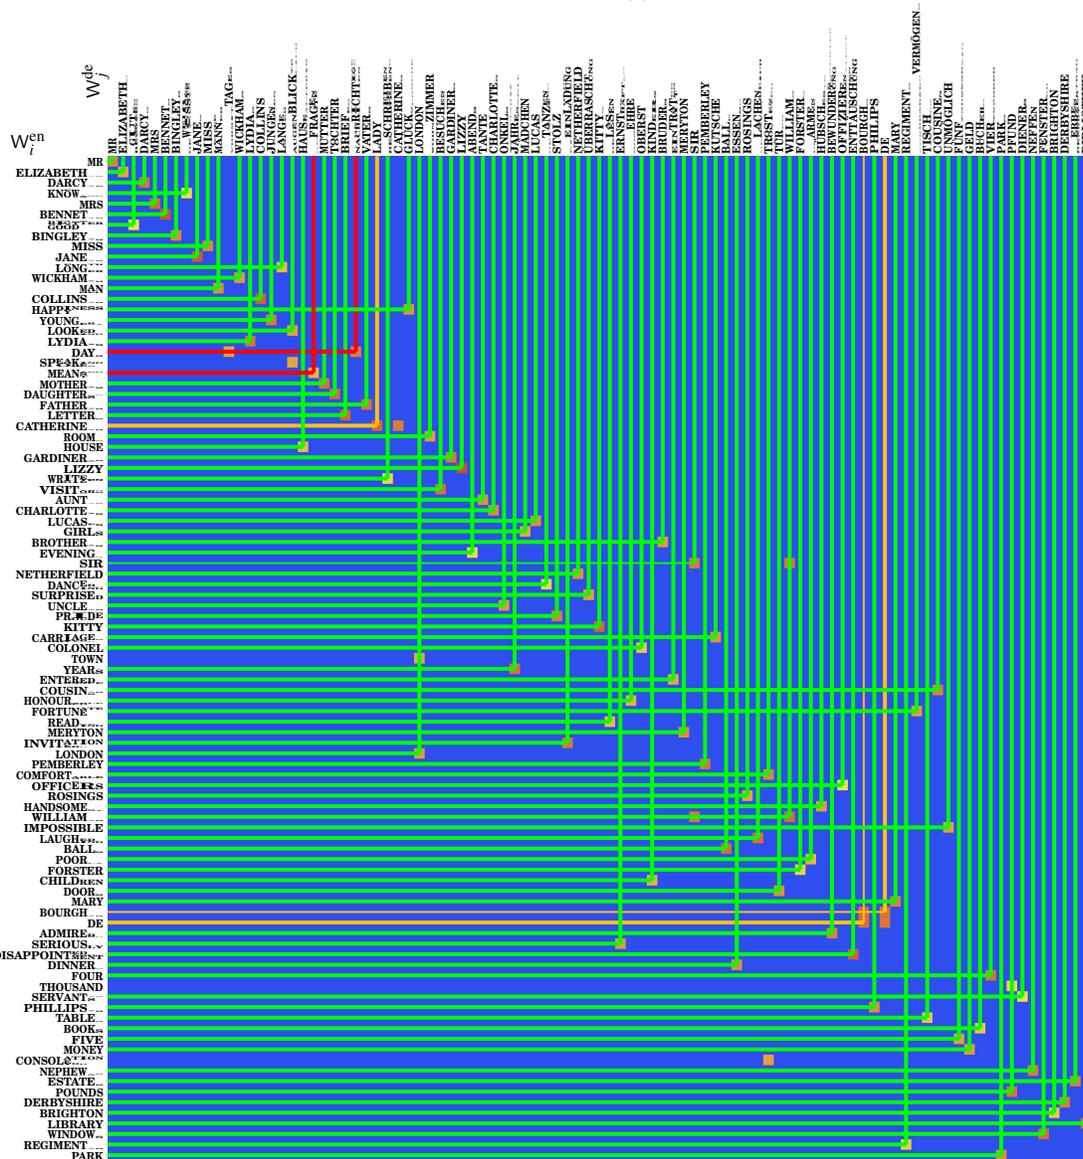

(b)

Fig. S5. Text mining in German. (a) Statistically identified topics ( $n_{ii} \geq 20$ ) in a German version of *Pride and Prejudice*, with the same color encoding scheme as Fig. S3. (b) Semantic similarities  $s(W_i^{en}, W_j^{de})$  between selected topics in English and German versions of *Pride and Prejudice*. Cross-hairs meet at optimal nodes that solve the bipartite matching problem. The thickness of each horizontal (resp. vertical) cross-hair is inversely proportional to the row-wise (resp. column-wise) ranking of the similarity score for the optimal node. *Green* (resp. *red*) cross-hair indicates a correct (resp. incorrect) match. *Amber* cross-hair marks a link between distinct concepts that share the same hypernyms.



### 5.3 Modified Porter stemming algorithm for Dutch

**Definition 5.25** (Dutch stop words). If a word belongs to the following list<sup>64</sup>:

'k, 'n, 'ne, 'ns, 's, aan, achter, achteruit, af, al, allang, alle, allebei, allemaal, allen, alles, als, altijd, ander, andere, anders, behalve, beide, beiden, ben, beneden, bent, boven, bovendien, bij, bijna, d'n, daar, daardoor, daarin, daarmee, daarna, daarnaast, daarom, daaronder, daarop, daartoe, daarvan, dan, dat, datgene, datgenen, de, deden, deed, deedt, degene, degenen, den, der, dergelijk, dergelijke, dergelijks, des, desondanks, deze, dezelfde, dezen, dezer, dezes, die, diegene, diegenen, dien, diens, dier, dikwijls, dit, doch, doe, doen, doend, doet, door, dus, echt, echter, een, eenieder, eenmaal, eens, eigenlijk, elders, elk, elkaar, elkaars, elke, en, ene, enen, ener, enig, enige, enkel, enkele, enkels, er, erg, ergens, erin, ermee, ernaast, erom, eronder, erop, ertoe, ervan, even, eveneens, evengoed, evenmin, eventjes, eventueel, evenwel, evenzeer, ge, gedaan, geen, gehad, gekund, ontmoeten, gemogen, genoeg, geweest, geworden, gij, haar, had, hadden, hadt, hare, heb, hebbe, hebben, hebbend, hebt, heeft, heel, heen, hele, helemaal, hem, hen, het, hetgeen, hetwelk, hetzelfde, hier, hierin, hiermee, hiernaast, hierom, hieronder, hierop, hiertoe, hiervan, hiervoor, hoe, hoelang, hoeveel, hoewel, hun, hunne, hunner, hij, ieder, iedere, iedereen, iemand, iets, ik, in, intussen, is, ja, je, jezelf, jou, jouw, jouwe, jouwer, jullie, jij, jijzelf, k, kan, kon, konden, kondt, kunnen, kunnend, kunt, later, luttel, luttele, maar, mag, me, mee, meer, meest, meeste, men, menig, menige, met, meteen, minder, mindere, minderen, minst, minste, minstens, misschien, mocht, mochte, mochten, moest, moeste, moesten, moet, moete, moeten, moetend, moge, mogen, mogend, moogt, mij, mijn, mijne, mijner, mijzelf, n, na, naar, naartoe, naast, nauwelijks, nee, neen, nen, nergens, net, niemand, niet, niets, niettemin, noch, nog, nooit, nou, nu, of, om, omdat, onder, onmiddellijk, ons, onszelf, onze, onzer, ooit, ook, op, over, per, reeds, sindsdien, sint, sommige, sommigen, soms, straks, t, te, tegen, ten, tenminste, tenslotte, ter, terug, tevens, toch, toe, toen, tot, trouwens, u, uit, uw, uwe, uwer, uzelf, vaak, vaak, vaakst, vake, vaker, van, vanaf, vandaan, vanwaar, veel, vele, voor, vooral, vooruit, vroeger, waar, waarheen, waarin, waarmee, waarnaast, waarom, waaronder, waarop, waart, waartoe, waarvandaan, wanneer, want, waren, was, wat, we, weer, wees, weest, weinig, weinige, wel, welk, welke, wellicht, werd, werden, werdt, wezen, wie, wil, word, worden, wordend, wordt, wij, zal, ze, zeer, zelden, zelf, zich, zichzelf, zo, zoals, zojuist, zolang, zonder, zou, zoude, zouden, zoudt, zoveel, zulk, zulke, zulks, zulle, zullen, zullend, zult, zij, zijn, zijnd, zijne, zijner, zijt,

then we consider it a Dutch stop word. All the Dutch stop words that appear in a particular document need to be ignored before we perform word clustering on the rest of the vocabulary list.  $\square$

To accommodate to pre-1946 (Flanders)/pre-1947 (Netherlands) Dutch written standard, which employed a sophisticated case system as in modern German (see [https://en.wikipedia.org/wiki/Archaic\\_Dutch\\_declension](https://en.wikipedia.org/wiki/Archaic_Dutch_declension)), we need to add inflected forms of the definite and indefinite articles, as well as those of the demonstratives to the list of stop words. It should be noted that archaic Dutch declensions still survive in some stock phrases in modern Dutch, such as the genitive construction in *het Koninkrijk der Nederlanden* “the Kingdom of Netherlands”.

The 1946/1947 orthography reform changed the endings of certain words: *bosch* “forest”, *mensch* “human” and *visch* “fish” (singular noun) are now spelt *bos*, *mens* and *vis*, respectively [47, §2.1]. Meanwhile, the spellings of adjectival endings in *mathematisch* “mathematical” and *typisch* “typical” are not affected, despite having the same silent *ch* at word final positions. So long as a document consistently employs an orthographical standard, we do not need to worry about these changes in our clustering algorithm, and we will not forcibly change all word final *sch* to *s*.

#### 5.3.1 Effective spelling and essential root

Vowel lengths are indicated in Dutch spellings according to certain rules. For example, all these three words *boom* “tree”, *boomen* “trees (pre-1946/pre-1947)” and *bomen* “trees (post-1946/post-1947)” contain the same long vowel in their first syllable [47, §2.1]. The penultimate step in the following algorithm helps us detect the vowel length in a Dutch spelling heuristically.

**Algorithm 5.26** (Dutch effective spelling). Set  $\mathbf{V} = (a|A|e|ē|ē|E|i|ī|ō|ō|O|u|ū|ū|U|y)$ ,  $\mathbf{V}_* = (a|e|o|u)$  and  $\mathbf{V}_0 = (a|e|i|o|u)$ . Set

$$\mathbf{c} = (b|c|d|f|g|h|i|k|l|m|n|p|q|r|s|t|v|w|x|z) \text{ and } \mathbf{C} = (B|C|D|F|G|H|J|K|L|M|N|P|Q|R|S|T|V|W|X|Z).$$

For a Dutch word  $\hat{\sigma}$ , its effective spelling  $\text{EffSpell}(\hat{\sigma})$  is constructed in the following steps:

(1) Convert to lowercase, and replace

<sup>64</sup>Our list of Dutch stop words is based on [snowball.tartarus.org/algorithms/dutch/stop.txt](http://snowball.tartarus.org/algorithms/dutch/stop.txt), with extensive additions that roughly match their counterparts in English. We have also included these words: *d'n, den, der, des, deze, dezen, dezer, dezes, dien, diens, dier, eens, eens, ene, enen, ener, 'n, 'ne, nen, 'ns, 's*, which are involved in archaic Dutch declensions and records of colloquial speech.

|                                     |                              |                    |                             |                             |                  |                 |                   |                           |                    |                      |             |
|-------------------------------------|------------------------------|--------------------|-----------------------------|-----------------------------|------------------|-----------------|-------------------|---------------------------|--------------------|----------------------|-------------|
| (Ø ge)zegen~<br>βλεσπ               | aanwezigX<br>πρεσεντ         | afwezigX<br>αβσεντ | bezet~<br>βζετ              | compl~<br>κμλ               | diner<br>δινερ   | eerb~<br>ehrβ   | eerder~<br>vroeg  | ellend<br>μισρβδ          | forst~<br>φορστ    | gardiner<br>φαρδινερ |             |
| gelo <sup>Xε</sup> (of v)~<br>βλλοX | genegen~<br>nijgen           | gezag<br>αυτργ     | gezicht<br>φαστ             | jone~<br>γοñε               | kilo~<br>κιλο    | kind~<br>κιλδδ  | langza~<br>σλωωza | ma(Ø m)ma(Ø a)~<br>moeder | manier~<br>μαñiepr |                      |             |
| meester<br>μειστερ                  | negen~<br>9e                 | o(or re)~<br>εαρ   | pappa(Ø a)~<br>vader        | ped~<br>πεδ                 | plant<br>πλαντ   | schok<br>σχοκ   | schoonh~<br>mooih | tafel<br>ταβλλ            | triest~<br>τριεσττ | vier~<br>4er         | wit<br>ωιττ |
| wonder<br>wonder                    | (Ø ge)rend(Ø e en)<br>rennen | jane<br>γιοñα      | ma(ʒ ʒ atje)(Ø s)<br>moeder | mamme(n tje)(Ø s)<br>moeder | oom(Ø s)<br>oñκλ | ~mooieX<br>mooi |                   |                           |                    |                      |             |

(2) Replace<sup>65</sup>

|                     |                   |                                   |                                  |                          |                           |                    |                                        |                               |                            |                            |                |                        |                  |                     |                        |                          |
|---------------------|-------------------|-----------------------------------|----------------------------------|--------------------------|---------------------------|--------------------|----------------------------------------|-------------------------------|----------------------------|----------------------------|----------------|------------------------|------------------|---------------------|------------------------|--------------------------|
| (Ø ge)hoor<br>χoor  | (Ø ge)zegd<br>zeg | X <sup>ε</sup> (bra(af v))~<br>pX | X <sup>ε</sup> (do(d od))~<br>tX | á<br>a                   | ä<br>a                    | bruik<br>bruik     | docht~<br>dtocht                       | é<br>e                        | è<br>e                     | ë<br>e                     | geëe~<br>geE   | geget<br>et            | georg~<br>jgeorg |                     |                        |                          |
| gezond<br>jgezond   | hor<br>χor        | i<br>i                            | i<br>i                           | janu~<br>jnu             | koning<br>koning          | leraar<br>leren    | lie <sup>Xε</sup> (f v)(Ø st)~<br>xliX | lof<br>lof                    | loof<br>λοοφ               | los<br>xlos                | lov<br>λον     | moe(Ø ie)~<br>μμmoe    | ó<br>o           | ö<br>o              |                        |                          |
| oe<br>ô             | ou<br>û           | placht<br>pleeg                   | su~<br>xsu                       | tien<br>tzien            | tuin<br>tuin              | ú<br>u             | ü<br>u                                 | voeld<br>fól                  | ij<br>y                    | zicht<br>zien              | ziek~<br>xziek | zom~<br>ζom            | zoon~<br>xxzoon  | best(Ø e)<br>gód    |                        |                          |
| beter(Ø e s)<br>gód | sir<br>ssir       | ~(ismelist)(Ø en tje)(Ø s)<br>e   | ~dje(Ø s)<br>d                   | ~ga(Ø an and at)<br>ging | ~ga(af f ve ven)<br>geven | ~kom(Ø t)<br>komen | ~kwa(amt m me men)<br>komen            | ~la(agt gl gel gen)<br>liggen | ~la(ast s ze zen)<br>lezen | ~sta(Ø an and at)<br>stond | ~uk<br>ukk     | ~wist(Ø e en)<br>weten | ~zaagt<br>zñn    | ~zag(Ø e en)<br>zñn | ~zat(Ø e en)<br>zitten | ~zei(Ø de den dt)<br>zeg |

(3) Do  $ei \rightarrow \hat{e}$ ,  $list \rightarrow \hat{list}$ ,  $ui \rightarrow \hat{u}$ ;(4) Do  $ie \rightarrow \hat{i}$ ,  $aan(\Ø|ge)n \rightarrow n$ ,  $door(\Ø|ge)r \rightarrow r$ ,  $dwars(\Ø|ge)s \rightarrow s$ ,  $om(\Ø|ge)m \rightarrow m$ ,  $op(\Ø|ge)p \rightarrow p$ ,  $vort(\Ø|ge)t \rightarrow t$ ,  $weg(\Ø|ge)g \rightarrow g$ ;(5) Do  $\sim end \rightarrow e$ ,  $\sim_{\hat{x}_1 \neq} \mathbf{V}s \rightarrow \hat{x}_1$ ,  $\hat{x}_2(dom|vol)(e|l|r|s|t)_{m_0} \rightarrow \hat{x}_2$ ,  $\hat{x}_3(ery|vaardig)\mathbf{X} \rightarrow \hat{x}_3$ ;(6) Do  $\hat{x}_1v \rightarrow \hat{x}_1f$ ,  $\hat{x}_2z \rightarrow \hat{x}_2s$  before turning double letters into the capital form of the same letter (i.e.  $ee \rightarrow E$  etc.);(7) Do  $\sim en \rightarrow e$ ;(8) Do  $\sim \mathbf{V}_*ce \rightarrow \mathbf{V}_*^+c$ ,  $\sim \mathbf{V}_0C_e \rightarrow \mathbf{V}_0C_-$ , where  $\mathbf{V}_*^+$  is the upper case form of  $\mathbf{V}_*$  and  $C_-$  is the lower case form of  $C$ ;(9) Do  $lerares \rightarrow lEr$ ,  $vrE \rightarrow \beta rE$ ,  $\sim \hat{r}(\Ø|es|s|tje)(Ø|s) \rightarrow \emptyset$ ,  $\sim An(\Ø|en|tje)(Ø|s) \rightarrow a$ ,  $\sim sje(\Ø|s) \rightarrow s$ ,  $\sim tje(\Ø|s) \rightarrow \emptyset$ ,  $\sim Tje(\Ø|s) \rightarrow t$ .

**Definition 5.27** (Dutch protected range). Set  $\mathbf{V}^* = (a|A|\hat{e}|E|i|\hat{i}|o|\hat{o}|O|u|\hat{u}|\hat{u}|U|y)$ , and write  $\bar{\mathbf{V}}_m$  (resp.  $\bar{\mathbf{V}}_{m_0}$ ) for one (resp. zero) or more repeats of any character other than  $\mathbf{V} = (a|A|e|\hat{e}|E|i|\hat{i}|o|\hat{o}|O|u|\hat{u}|\hat{u}|U|y)$ . Define  $\mathbf{C}_{m_0}^{**} = (\bar{a}|\bar{A}|\bar{e}|\bar{\hat{e}}|\bar{E}|\bar{i}|\bar{\hat{i}}|\bar{o}|\bar{\hat{o}}|\bar{O}|\bar{u}|\bar{\hat{u}}|\bar{\hat{u}}|\bar{U})_{m_0}$ . Let  $\hat{\sigma}$  be the effective spelling of a Dutch word, its protected range  $\text{ProtRg}(\hat{\sigma}) = \max\{\lambda_1(\hat{\sigma}), \lambda_2(\hat{\sigma})\}$  is determined by two non-negative integers  $\lambda_1(\hat{\sigma})$  and  $\lambda_2(\hat{\sigma})$  specified through the following procedures:

- Look for the string pattern  $((\Ø|a|A|b|e|e|E|g|e|h|e|r|i|m|e|d|e|n|a|O|\hat{o}|u|U|\hat{u}|\hat{u}|v|e|r)\bar{\mathbf{V}}_{m_0}\mathbf{V}^*|\bar{\mathbf{V}}_m(e|E))\mathbf{C}_{m_0}^{**}$  in the string  $\hat{\sigma}$ ;
- If the string pattern above is found, the last position occupied by such a string defines  $\lambda_1(\hat{\sigma})$ ; otherwise, set  $\lambda_1(\hat{\sigma}) = 0$ ;
- Look for the pattern  $(a|A|o|\hat{o}|O|u|\hat{u}|U)$  in the string  $\hat{\sigma}$ ;
- If a letter in the pattern above is found, the last position occupied by such a letter defines  $\lambda_2(\hat{\sigma})$ ; otherwise, set  $\lambda_2(\hat{\sigma}) = 0$ .

□

Unlike Danish, but similar to German, our Dutch essential root is free from common separable verb prefixes (see step (3) in the algorithm below).

<sup>65</sup>Here, the string pattern  $ij$  may refer to two Latin letters  $i$  and  $j$  sitting next to each other, or a single Unicode character LATIN SMALL LIGATURE IJ U+0133.

**Algorithm 5.28** (Dutch essential root). Set  $\mathbf{V} = (a|A|e|\hat{e}|E|i|\hat{i}|o|\hat{o}|O|u|\hat{u}|U|y)$  and  $\mathbf{C} = \overline{(a|A|e|\hat{e}|E|i|\hat{i}|o|\hat{o}|O|u|\hat{u}|U|y)}$ . Let  $\hat{\sigma}$  be the effective spelling of a Dutch word, then its corresponding essential root  $\text{EssRoot}(\hat{\sigma})$  is constructed in the following steps:

(1) Break down  $\hat{\sigma} = \hat{\sigma}_1\hat{\sigma}_2$  into the concatenation of two strings  $\hat{\sigma}_1 = \hat{\sigma}^{[\text{ProtRg}(\hat{\sigma})]}$  (see the notation in Definition 3.1) and  $\hat{\sigma}_2$ , where the length of the first string  $\ell(\hat{\sigma}_1) = \text{ProtRg}(\hat{\sigma})$  is equal to the protected range of  $\hat{\sigma}$ .

(2) On  $\hat{\sigma}_2$ , perform the following substitutions in a sequel:<sup>66</sup>

(2.1) Do  $\sim(Er|s) \rightarrow \emptyset$ ;

(2.2) Do  $\sim e(d|e|m|n|r|st|t)_{m_0} \rightarrow \emptyset$ .

The result after these two steps of operations is called  $\hat{\sigma}'_2$ .

(3) Concatenate  $\hat{\sigma}_1$  and  $\hat{\sigma}'_2$ , before doing  $(\emptyset|af|An|by|dOr|dwars|mE|mede|na|om|op|t\hat{o}|vOrt|weg)(\emptyset|ge)\mathbf{XV}\sim \rightarrow \mathbf{XV}$ ;

(4) Do  $\sim\mathbf{Ct} \rightarrow \mathbf{C}$ ;

(5) Do  $v \rightarrow f, z \rightarrow s$ ;

(6) Do  $\sim\hat{\chi} \rightarrow \hat{\chi}_-$  (i.e. reduce final letter to lowercase);

(7) Do  $ag \rightarrow Ag, ak \rightarrow Ak, al \rightarrow Al, at \rightarrow At, breng \rightarrow brach, denk \rightarrow dach, Ef \rightarrow ef, ep \rightarrow Ep, kOp \rightarrow koch, nam \rightarrow nAm, s\hat{o}k \rightarrow soch$ .

### 5.3.2 Admissible mutation and approximate clustering

The Dutch vowel blotting mechanism is similar to the Danish version (Algorithm 5.5).

**Algorithm 5.29** (Dutch vowel blotting). Set  $\mathbf{V}_m = (a|A|e|\hat{e}|E|i|\hat{i}|o|\hat{o}|O|u|\hat{u}|\hat{u}|U|y)_m$  and  $\mathbf{C}_{m_0} = \overline{(a|A|e|\hat{e}|E|i|\hat{i}|o|\hat{o}|O|u|\hat{u}|\hat{u}|U|y)_{m_0}}$ . For a token string  $\hat{\sigma}$ , its blotted form  $\text{BlotV}_1(\hat{\sigma})$  is constructed as follows:

- If the string pattern  $(\emptyset|a|be|e|\hat{e}|i|o|u|\hat{u})\mathbf{C}_{m_0}\mathbf{V}_m\sim$  can be found in the string  $\hat{\sigma}$ , then the last position occupied by such a pattern is replaced by the letter “a”.
- Otherwise, leave the string  $\hat{\sigma}$  intact.

Similar to what we did in §5.1.2 for the case of Danish, we will construct a bivariate Boolean-valued function  $\text{HrdTest}(\hat{\alpha}, \hat{\beta})$  on a “simple heredity test function” in Algorithm 5.30, and a set of “admissible suffix mismatch and vowel alternation” rules in Algorithm 5.31.

**Algorithm 5.30** (Simple heredity test). Set  $\mathbf{V} = (a|A|e|\hat{e}|E|i|\hat{i}|o|\hat{o}|O|u|\hat{u}|\hat{u}|U|y)$ . The Boolean-valued function  $\text{SimpHrdTest}(\hat{\alpha}, \hat{\beta})$  returns **TRUE** if  $\hat{\alpha}$  contains at least one instance of  $\mathbf{V}$ , **AND** at least one of the following six conditions holds:<sup>67</sup>

(i)  $\hat{\alpha} = \hat{\beta}$ ;

(ii)  $\hat{\beta} = \hat{\alpha}d$ ;

(iii)  $\hat{\beta} = \hat{\alpha}Er$ ;

(iv)  $\hat{\beta} = \hat{\alpha}s$ ;

(v)  $\hat{\beta} = \hat{\alpha}t$ ;

(vi)  $\ell(\hat{\beta}) > \ell(\hat{\alpha}) \geq \ell(\hat{\beta}) - 2$  **AND**  $\hat{\alpha} = \hat{\beta}^{[\ell(\hat{\alpha})]}$  **AND**  $\hat{\beta}^{\{\ell(\hat{\alpha})+1\}} = (e|n|s)$ . (See Definition 3.1 for the notations  $\hat{\beta}^{[n]}$  and  $\hat{\beta}^{\{n\}}$ .)

In what follows, we define  $\text{SuffixNW}(\hat{\alpha}, \hat{\beta}), \text{RootNW}(\hat{\alpha}, \hat{\beta}), \text{NW}^*(\hat{\alpha}, \hat{\beta})$  and  $\text{SuffixSW}(\hat{\alpha}, \hat{\beta}), \text{SuffixSW}(\hat{\alpha}, \hat{\beta}), \text{SW}^*(\hat{\alpha}, \hat{\beta})$  as what is done in the Danish case (Algorithm 5.7).

<sup>66</sup>In other words, the core algorithm for essential root extraction runs as follows: keep the last “strong” vowel  $a, i, o$  or  $u$  in non-final position, plus one subsequent letter; delete final  $a$ ; erase the final appearance of  $e$  and all the letters thereafter.

<sup>67</sup>As a general rule in this document, the truth values of items labeled with Roman numerals are connected to each other with logical **OR**.

**Algorithm 5.31** (Admissible suffix mismatch and vowel alternation). For two strings  $\hat{\alpha}$  and  $\hat{\beta}$ , the Boolean-valued function

$$\text{AdmMut}(\text{RootNW}(\hat{\alpha}, \hat{\beta}), \text{SuffixNW}(\hat{\alpha}, \hat{\beta}), \text{NW}^*(\hat{\alpha}, \hat{\beta}))$$

returns **TRUE** if

$$\begin{aligned} & \text{SuffixNW}(\hat{\alpha}, \hat{\beta}) \\ = & [(\emptyset|(e|E|n|t)_m|((\text{acht|haft|mat})\text{ig}|(\emptyset|b)\text{Ar}|e(\text{ling|lyk|nis|r})|h(e|\hat{e})d|i(n|ng|sch)|je|l(\text{ing|yk})|nis|s(\text{Am}|e|t)|t(\hat{e}t|je)|\text{yk})\mathbf{X})), \\ & (\emptyset|(e|E|n|t)_m|((\text{acht|haft|mat})\text{ig}|(\emptyset|b)\text{Ar}|e(\text{ling|lyk|nis|r})|h(e|\hat{e})d|i(n|ng|sch)|je|l(\text{ing|yk})|nis|s(\text{Am}|e|t)|t(\hat{e}t|je)|\text{yk})\mathbf{X}))] \end{aligned}$$

**AND** at least one of the following three conditions holds:<sup>68</sup>

- (i)  $\text{NW}^*(\hat{\alpha}, \hat{\beta}) = \emptyset$  **AND** the lowercase form of  $\text{RootNW}(\hat{\alpha}, \hat{\beta})$  contains at least one instance of  $(a|e|\hat{e}|i|\hat{i}|o|\hat{o}|u)$ ;
- (ii)  $\text{NW}^*(\hat{\alpha}, \hat{\beta}) = ([A, E][A, \hat{i}][A, \hat{i}][A, \hat{o}][A, O][e, \hat{i}][e, o][E, \hat{i}][E, O][E, y][i, o][\hat{i}, O][O, \hat{u}])$ ;
- (iii)  $\text{NW}^*(\hat{\beta}, \hat{\alpha}) = ([A, E][A, \hat{i}][A, \hat{i}][A, \hat{o}][A, O][e, \hat{i}][e, o][E, \hat{i}][E, O][E, y][i, o][\hat{i}, O][O, \hat{u}])$ .

Similarly, one can evaluate another Boolean-valued function

$$\text{AdmMut}(\text{RootSW}(\hat{\alpha}, \hat{\beta}), \text{SuffixSW}(\hat{\alpha}, \hat{\beta}), \text{SW}^*(\hat{\alpha}, \hat{\beta}))$$

by trading all the occurrences of NW in the statements above with SW.

**Algorithm 5.32** (Heredity test function). The structure of the Dutch heredity test function  $\text{HrdTest}(\hat{\alpha}, \hat{\beta})$  is identical to the German version (Algorithm 8.1.2), except that the functions  $\text{SimpHrdTest}$ ,  $\text{RootNW}$ ,  $\text{SuffixNW}$ ,  $\text{NW}^*$ ,  $\text{RootSW}$ ,  $\text{SuffixSW}$ ,  $\text{SW}^*$  must follow the Dutch rules stated above.

**Algorithm 5.33** (Approximate clustering of Dutch words). The algorithm is essentially the same as Algorithm 5.10, except that Dutch rules (instead of Danish rules) apply to all the tags (effective spelling, essential root, vowel blotting etc.).

*Example 5.33.1.* As an illustration of our clustering algorithm, we pick the following families of Dutch words, where an “approximate translation” in English, enclosed in quotation marks, is appended to the end of each family:<sup>69</sup>

*best, beste, beter, betere, beters, goed, goede, goeden, goeder, goeds* — “good”;  
*daad, daden* — “deed”;  
*dooier, dooiers, dooiertje* — “yolk”;  
*ei, eieren, eitje, eitjes* — “egg”;  
*eidooier, eidooiers, eidooiertje, eierdooier, eierdooiers, eierdooiertje* — “egg yolk”;  
*eiwit, eiwitten, eiwittje* — “egg white”;  
*geleerd, leer, leerde, leerden, leert, lere, leren, lerend* — “learn”;  
*gelost, los, losse, lossen, lossend, lost, loste, losten* — “dump”;  
*geraasd, raas, raasde, raasden, raast, raze, razen, razend* — “rage”;  
*gewerkt, werk, werke, werken, werkend, werkt, werkte, werkten* — “work”;  
*klein, kleine, kleinen, kleiner, kleinere, kleineren, kleins, kleinst, kleinste* — “small”;  
*maan, manen, maantje* — “moon”;  
*man, manne, mannen, mans* — “man”;  
*vrouw, vrouwe, vrouwen* — “woman”;  
*wit, wits, witst, witste, witte, witter, wittere, witters* — “white”.

Applying Algorithm 5.33 to this list of words, we obtain the following clustering results:

{*best, beste, beter, betere, beters, goed, goede, goeden, goeder, goeds*}, {*daad, daden*}, {*dooier, dooiers, dooiertje*}, {*ei, eieren, eitje, eitjes*}, {*eidooier, eidooiers, eidooiertje*}, {*eierdooier, eierdooiers, eierdooiertje*}, {*eiwit, eiwitten, eiwittje*}, {*geleerd, leer, leerde, leerden, leert, lere, leren, lerend*}, {*gelost, los, losse, lossen, lossend, lost, loste, losten*}, {*geraasd, raas, raasde, raasden, raast, raze, razen, razend*}, {*gewerkt, werk, werke, werken, werkend, werkt, werkte, werkten*}, {*klein, kleine, kleinen, kleiner, kleinere, kleineren, kleins, kleinst, kleinste*}, {*maan, maantje, man, manen, manne, mannen, mans*}, {*vrouw, vrouwe, vrouwen*}, {*wit, wits, witst, witste, witte, witter, wittere, witters*}.

<sup>68</sup>We note that  $\text{NW}^*(\hat{\alpha}, \hat{\beta})$  and  $\text{NW}^*(\hat{\beta}, \hat{\alpha})$  differ only in the order of the two components in the bracket.

<sup>69</sup>This list includes archaic declension forms found in the paradigms on the following web-page: [en.wikipedia.org/wiki/Archaic\\_Dutch\\_declension](http://en.wikipedia.org/wiki/Archaic_Dutch_declension).

We note that two alternative forms of “egg yolk” *eidooier* and *eierdooier* are split into two different clusters in this method.

*Example 5.33.2.* To further test our algorithm against Dutch irregular verbs with various vowel alternation patterns across different tenses and moods, we throw the following list:

*bak, bakke, bakken, bakkend, bakt, bakte, bakten, gebakken* — “bake”;  
*ban, bande, banden, banne, bannen, bannend, bant, gebannen* — “expel”;  
*bederf, bederft, bederve, bederven, bedervend, bedierf, bedierft, bedorve, bedorven* — “spoil”;  
*bedrieg, bedriege, bedriegen, bedriegend, bedriegt, bedroge, bedrogen, bedroog, bedroogt* — “deceive”;  
*beet, bete, beten, bijt, bijte, bijten, bijtend, gebeten* — “bite”;  
*begin, beginne, beginnen, beginnend, begint, begon, begonne, begonnen, begont* — “begin”;  
*bied, biede, bieden, biedend, biedt, bode, boden, bood, boodt, geboden* — “bid”;  
*bind, binde, binden, bindend, bindt, bond, bonde, bonden, bondt, gebonden* — “tie”;  
*blaas, blaast, blaze, blazen, blazend, blies, bliest, blieze, bliezen, geblazen* — “blow”;  
*bleek, bleekt, bleke, bleken, blijkt, blijke, blijken, blijktend, blijktt, gebleken* — “appear”;  
*boge, bogen, boog, boogt, buig, buige, buigen, buigend, buigt, gebogen* — “bend”;  
*braakt, brak, brake, braken, breek, breekt, breke, breken, brekend, gebroken* — “break”;  
*bracht, brachte, brachten, breng, brenge, brengen, brengend, brengt, gebracht* — “bring”;  
*dacht, dachte, dachten, denk, denke, denken, denkend, denkt, gedacht* — “think”;  
*draag, draagt, drage, dragen, dragend, droeg, droege, droegen, droegt, gedragen* — “carry”;  
*droop, droopt, drope, dropen, druip, druipe, druipen, druipend, druipt, gedropen* — “drip”;  
*gegolden, geld, gelde, gelden, geldend, geldt, gold, golde, golden, goldt* — “apply”;  
*geheven, hef, heffe, heffen, heffend, heft, hief, hieft, hieve, hieven* — “heave”;  
*geholpen, help, helpe, helpen, helpend, helpt, hielp, hielpe, hielpen, hielpt* — “help”;  
*gekocht, kocht, kochte, kochten, koop, koopt, kope, kopen, kopend* — “buy”;  
*gelegen, laag, lag, lage, lagen, lig, ligge, liggen, liggend, ligt* — “lie”;  
*genomen, naamt, nam, name, namen, neem, neemt, neme, nemen, nemend* — “take”;  
*geschapen, schep, scheppe, scheppen, scheppend, schept, schiep, schiepe, schiepen, schiept* — “create”;  
*gescholden, scheld, schelde, schelden, scheldend, scheldt, schold, scholde, scholden, scholdt* — “scold”;  
*gevraagd, vraag, vraagde, vraagde, vraagden, vraagt, vrage, vragen, vragend, vroeg, vroeger, vroegen, vroegt* — “ask”;  
*gewogen, weeg, weegt, wege, wegen, wegend, woge, wogen, woog, woogt* — “weigh”;  
*gezetten, zat, zate, zaten, zit, zitte, zitten, zittend* — “sit”;  
*gezocht, zocht, zochte, zochten, zoek, zoekte, zoeken, zoekend, zoekt* — “seek”

into our algorithm, and obtain

{*bak, bakke, bakken, bakkend, bakt, bakte, bakten, gebakken*}, {*ban, bande, banden, banne, bannen, bannend, bant, gebannen*}, {*bederf, bederft, bederve, bederven, bedervend, bedierf, bedierft, bedorve, bedorven*}, {*bedrieg, bedriege, bedriegen, bedriegend, bedriegt, bedroge, bedrogen, bedroog, bedroogt*}, {*beet, bete, beten, bijt, bijte, bijten, bijtend, gebeten*}, {*begin, beginne, beginnen, beginnend, begint, begon, begonne, begonnen, begont*}, {*bied, biede, bieden, biedend, biedt, bode, boden, bood, boodt, geboden*}, {*bind, binde, binden, bindend, bindt, bond, bonde, bonden, bondt, gebonden*}, {*blaas, blaast, blaze, blazen, blazend, blies, bliest, blieze, bliezen, geblazen*}, {*bleek, bleekt, bleke, bleken, blijkt, blijke, blijken, blijktend, blijktt, gebleken*}, {*boge, bogen, boog, boogt, buig, buige, buigen, buigend, buigt, gebogen*}, {*braakt, brak, brake, braken, breek, breekt, breke, breken, brekend, gebroken*}, {*bracht, brachte, brachten, breng, brenge, brengen, brengend, brengt, gebracht*}, {*dacht, dachte, dachten, denk, denke, denken, denkend, denkt, gedacht*}, {*draag, draagt, drage, dragen, dragend, droeg, droege, droegen, droegt, gedragen*}, {*droop, droopt, drope, dropen, druip, druipe, druipen, druipend, druipt, gedropen*}, {*gegolden, geld, gelde, gelden, geldend, geldt, gold, golde, golden, goldt*}, {*geheven, hef, heffe, heffen, heffend, heft, hief, hieft, hieve, hieven*}, {*geholpen, help, helpe, helpen, helpend, helpt, hielp, hielpe, hielpen, hielpt*}, {*gekocht, kocht, kochte, kochten, koop, koopt, kope, kopen, kopend*}, {*gelegen, laag, lag, lage, lagen, lig, ligge, liggen, liggend, ligt*}, {*genomen, naamt, nam, name, namen, neem, neemt, neme, nemen, nemend*}, {*geschapen, schep, scheppe, scheppen, scheppend, schept, schiep, schiepe, schiepen, schiept*}, {*gescholden, scheld, schelde, schelden, scheldend, scheldt, schold, scholde, scholden, scholdt*}, {*gevraagd, vraag, vraagde, vraagde, vraagden, vraagt, vrage, vragen, vragend, vroeg, vroeger, vroegen, vroegt*}, {*gewogen, weeg, weegt, wege, wegen, wegend, woge, wogen, woog, woogt*}, {*gezetten, zat, zate, zaten, zit, zitte, zitten, zittend*}, {*gezocht, zocht, zochte, zochten, zoek, zoekte, zoeken, zoekend, zoekt*}.

### 5.3.3 Heuristic detection of compounds

The following algorithm for heuristic detection of Dutch compounds differs from the Danish version (Algorithm 5.12) only in some specific details. To make the context clear, we still state the algorithm in full. (In what follows, the string minus operation  $\hat{\beta} \ominus \hat{\alpha}$  is prescribed by Definition 5.11.)

**Algorithm 5.34** (Heuristic identification of Dutch binary compounds). *Let  $\Lambda^{\hat{\rho}} = \{\hat{\rho}_1, \dots, \hat{\rho}_Q\}$  be a list of distinct Dutch essential roots (without vowel blotting) that contain at least one instance of  $\mathbf{V} = (a|A|e|ē|E|i|ī|o|ō|O|u|ū|ü|U|y)$  and DO NOT match the following string patterns:*

$(acht\mathbf{X}|al|an|At|bar|be\mathbf{X}|con|el|en|Er|fer\mathbf{X}|fol|fOr\mathbf{X}|ge|ging|grOt|kOm|le|man|me|o|of|on|ond|ongel|per|ū|üt|wAr|xlos).$

The output of the function  $\text{CpdDet}(\Lambda^{\hat{\rho}})$  is obtained through the following procedures:

- (1) Construct a list  $\{(\hat{\rho}_1, \lambda_1^{\hat{\rho}}), \dots, (\hat{\rho}_Q, \lambda_Q^{\hat{\rho}})\}$  where  $\lambda_q^{\hat{\rho}} = \{\hat{\rho}_{(q,1)}, \dots, \hat{\rho}_{(q,n_q)}\}$  is a subset of  $\Lambda^{\hat{\rho}}$  whose members all match the string pattern  $\hat{\rho}_q \sim$ , for  $q \in \mathbb{Z} \cap [1, Q]$ .
- (2) Expand the aforementioned entry  $(\hat{\rho}_q, \lambda_q^{\hat{\rho}})$  into a list of triplets  $\{(\hat{\rho}_{(q,1)}, \hat{\rho}_q, \hat{\rho}_{(q,1)} \ominus \hat{\rho}_q), \dots, (\hat{\rho}_{(q,n_q)}, \hat{\rho}_q, \hat{\rho}_{(q,n_q)} \ominus \hat{\rho}_q)\}$  for every  $q \in \mathbb{Z} \cap [1, Q]$  such that  $\lambda_q^{\hat{\rho}} \neq \emptyset$ . Collect all these triplets as one runs through the list  $\{(\hat{\rho}_1, \lambda_1^{\hat{\rho}}), \dots, (\hat{\rho}_Q, \lambda_Q^{\hat{\rho}})\}$ . The list of these triplets  $\{(\hat{\rho}_{(1)}, \hat{\eta}_{(1)}, \hat{\rho}_{(1)} \ominus \hat{\eta}_{(1)}), \dots, (\hat{\rho}_{(Q)}, \hat{\eta}_{(Q)}, \hat{\rho}_{(Q)} \ominus \hat{\eta}_{(Q)})\}$  contains potentially valid decompositions of compounds.
- (3) Screen the aforementioned list of triplets as follows: for every  $q' \in \mathbb{Z} \cap [1, Q']$ , if  $(\hat{\rho}_{(q')}, \hat{\eta}_{(q')}, \hat{\tau}_{(q')} = \hat{\rho}_{(q')} \ominus \hat{\eta}_{(q')})$  satisfies

$$\ell(\hat{\rho}_{(q')} \ominus \hat{\eta}_{(q')}) \geq 2 \quad \text{AND} \quad \hat{\rho}_{(q')} \ominus \hat{\eta}_{(q')} = \mathbf{X}_1(a|A|e|ē|E|i|ī|o|ō|O|u|ū|ü|U|y)\mathbf{X}_2,$$

then construct  $\hat{\tau}_{(q')}$  by performing  $(e|n|s) \sim \rightarrow \emptyset$  on  $\hat{\tau}_{(q')}$  and  $\hat{\tau}_{(q')}^{**}$  by doing  $(e|n|e|r|e|s|g|e) \sim \rightarrow \emptyset$  on  $\hat{\tau}_{(q')}$ , before generating a list  $\lambda_{(q')}^{\hat{\tau}}$  by members of  $\Lambda^{\hat{\rho}}$  that match the pattern  $(\hat{\tau}_{(q')}|\hat{\tau}_{(q')}^{*}|\hat{\tau}_{(q')}^{**})$ ; otherwise, set  $\lambda_{(q')}^{\hat{\tau}} = \emptyset$ .

- (4) Collect all the triplets  $(\hat{\rho}_{(q')}, \hat{\eta}_{(q')}, \lambda_{(q')}^{\hat{\tau}})$  where  $\lambda_{(q')}^{\hat{\tau}}$  is non-void and  $\hat{\tau}_{(q')}$  DOES NOT match the following string patterns:

$(h(e|ē)d\mathbf{X}|ing\mathbf{X}|lyk\mathbf{X}|tēt\mathbf{X}|um).$

This list of triplets  $\text{CpdDet}(\Lambda_{\hat{\rho}})$  contains the heuristic decompositions of all the identified binary compounds.

**Algorithm 5.35** (Approximate clustering of Dutch words with heuristic detection of compounds). *The procedure runs essentially the same way as Algorithm 5.35, except that Dutch rules replace Danish rules.*

*Example 5.35.1.* Testing the algorithm above against the combined inputs from Examples 5.33.1 and 5.33.2, we obtain the following result:

$\{bak, bakke, bakken, bakkend, bakt, bakte, bakten, gebakken\}$ ,  $\{ban, bande, banden, banne, bannen, bannend, bant, gebannen\}$ ,  $\{bederf, bederft, bederve, bederven, bedervend, bedierf, bedierft, bedorve, bedorven\}$ ,  $\{bedrieg, bedriege, bedriegen, bedriegend, bedriegt, bedroge, bedrogen, bedroog, bedroogt\}$ ,  $\{beet, bete, beten, bijt, bijte, bijten, bijtend, gebeten\}$ ,  $\{begin, beginne, beginnen, beginnend, begint, begon, begonne, begonnen, begont\}$ ,  $\{best, beste, beter, betere, beters, goed, goede, goeden, goeder, goeds\}$ ,  $\{bied, biede, bieden, biedend, biedt, bode, boden, bood, boodt, geboden\}$ ,  $\{bind, binde, binden, bindend, bindt, bond, bonde, bonden, bondt, gebonden\}$ ,  $\{blaas, blaast, blaze, blazen, blazend, blies, bliest, blieze, bliezen, geblazen\}$ ,  $\{bleek, bleekt, bleke, bleken, blijkt, blijke, blijken, blijktend, blijktt, gebleken\}$ ,  $\{boge, bogen, boog, boogt, buig, buige, buigen, buigend, buigt, gebogen\}$ ,  $\{braakt, brak, brake, braken, breek, breekt, breke, breken, brekend, gebroken\}$ ,  $\{bracht, brachte, brachten, breng, bringe, brengen, brengend, brengt, gebracht\}$ ,  $\{daad, daden\}$ ,  $\{dacht, dachte, dachten, denk, denke, denken, denkend, denkt, gedacht\}$ ,  $\{dooier, dooiers, dooiertje, eidooier, eidooiers, eidooiertje, eierdooier, eierdooiers, eierdooiertje\}$ ,  $\{draag, draagt, drage, dragen, dragend, droeg, droege, droegen, droegt, gedragen\}$ ,  $\{droop, droopt, drope, dropen, druip, druipe, druipen, druipend, druipt, gedropen\}$ ,  $\{ei, eidooier, eidooiers, eidooiertje, eierdooier, eierdooiers, eierdooiertje, eieren, eitje, eitjes, eiwit, eiwitten, eiwittje\}$ ,  $\{eiwit, eiwitten, eiwittje, wit, wits, witst, witste, witte, witter, wittere, witters\}$ ,  $\{gegouden, geld, gelde, gelden, geldend, geldt, gold, golde, golden, goldt\}$ ,  $\{geheven, hef, heffe, heffen, heffend, heft, hief, hieft, hieve, hieven\}$ ,  $\{geholpen, help, helpe, helpen, helpend, helpt, hielp, hielpje, hielpen, hielpt\}$ ,  $\{gekocht, kocht, kochte, kochten, koop, koopt, kope, kopen, kopens, geleerd, leer, leerde, leerden, leert, lere, leren, lerend\}$ ,  $\{gelegen, laag, lage, lagen, lig, ligge, liggen, liggend, ligt\}$ ,  $\{gelost, los, losse, lossen, lossend, lost, loste, losten\}$ ,  $\{genomen, naamt, nam, name, namen, neem, neemt, neme, nemen, nemend\}$ ,  $\{geraasd, raas, raasde, raasden, raast, raze, razen, razend\}$ ,  $\{geschapen, schep, scheppe, scheppen, scheppend, schept, schiepe, schiepen, schiept\}$ ,  $\{gescholden, scheld,$

*schelde, schelden, scheldend, scheldt, schold, scholde, scholden, scholdt*}, {*gevraagd, vraag, vraagd, vraagde, vraagden, vraagt, vrage, vragen, vragend, vroeg, vroege, vroegen, vroegt*}, {*gewerkt, werk, werke, werken, werkend, werkt, werkte, werkten*}, {*gewogen, weeg, weegt, wege, wegen, wegend, woge, wogen, woog, woogt*}, {*gezeten, zat, zate, zaten, zit, zitte, zitten, zittend*}, {*gezocht, zocht, zochte, zochten, zoek, zoeke, zoeken, zoekend, zoekt*}, {*klein, kleine, kleinen, kleiner, kleinere, kleiner, kleins, kleinst, kleinste*}, {*maan, maantje, man, manen, manne, mannen, mans*}, {*vrouw, vrouwe, vrouwen*}.

Here, the compounds *ei(Ø|er)dooier* “egg yolk” and *eiwit* “egg white” are correctly dissolved into their respective constituting components.

*Example 5.35.2.* In Fig. S6, we further apply the aforementioned word clustering algorithm to topic extraction and machine translation (see Table S1 for text source).

Note that *de* “the” is a Dutch stop word, so the English *de* cannot be translated exactly by our algorithm.

The co-occurring words in *Lady Catherine (de Bourgh)* and *Sir William (Lucas)* also make it difficult to resolve them exactly in our numerical experiments. These pairs of mismatches are indicated by amber cross-hairs in Fig. S6b.



## 6 Approximate word clustering in selected Romance languages

In this section, we present the approximate clustering algorithms for two representative modern Romance languages with a large number of speakers: Spanish and French. Their ancestral language, Latin, is also treated in this section.

Due to heavy loads of Latinate loanwords in English (borrowed either directly from Latin, or through Norman French), the word formation of English shares a lot of features with modern Romance languages. However, some critical differences must be noted:

- Unlike English, apostrophes and hyphens are used extensively in French to mark word boundaries.
- Unlike English, verbs in all these three languages conjugate in all persons for all tenses and aspects, thus making the verb morphology highly complicated.
- Unlike English, adjectives in all these three languages inflect in both gender and number.
- The classical language Latin additionally have declensions of nouns and adjectives in six cases.

The descriptions above (except the case declension of Latin) also extend to modern Italian, together with some Romance languages spoken in the Iberian Peninsula other than Spanish (namely, Catalan, Galician, Portuguese and Valencian), with minor modifications. Romanian, a Romance language spoken in Eastern Europe, has more conservative morphological structures (such as three genders and five cases), which are closer to the complexity of Latin (which has three genders and six cases) than all the other modern Romance languages.

### 6.1 Modified Porter stemming algorithm for Spanish

Before defining Spanish stop words, we need to define Spanish vowel extensions, and construct an algorithm to stress the penultimate vowel in a Spanish word, by heuristics.

**Definition 6.1** (Spanish Vowel Extensions). Hereafter in §6.1, the symbol  $\mathbf{V}^*$  stands for any member from the list  $\{a, e, i, \hat{i}, o, u\}$ , the so-called Spanish vowel extensions. In line with the multiplicity notations introduced in Definition 3.3, the symbol  $\mathbf{V}_m^*$  stands for a text string formed by consecutive appearance of one or more (not necessarily identical or distinct) members from the set of Spanish vowel extensions.

Dual to the notations above, the symbol  $\mathbf{C}^*$  stands for any character that does not belong to the list  $\{a, e, i, \hat{i}, o, u\}$ , and  $\mathbf{C}_{m_0}^*$  stands for a text string formed by consecutive appearance of zero or more (not necessarily identical or distinct) characters that do not belong to the same list.  $\square$

**Algorithm 6.2** (Penultimate Stress). *We define  $\text{StrPenult}(\hat{\sigma})$  through the following operations on  $\hat{\sigma}$ :*

- (1) *Remove diacritic marks from  $\hat{\sigma}$ , except that the Spanish letter  $\tilde{n}$  must be kept intact.*
- (2) *Do  $\sim(\mathbf{V}^*)^{\mathbf{X}\epsilon}(\mathbf{C}_m^* \mathbf{V}_m^* \mathbf{C}_{m_0}^*) \rightarrow \mathbf{V}'\mathbf{X}$ , where one derives  $\mathbf{V}'$  from  $\mathbf{V}^*$  by adding stress marks to  $(a|e|i|\hat{o}|u)$ . The result so far is called  $\hat{\sigma}'$ .*
- (3) *If  $\Omega(\hat{\sigma}') = (d|r)$  or  $\hat{\sigma}' = \text{está}$ , then perform the operation in Step (1) on  $\hat{\sigma}'$  and output  $\text{StrPenult}(\hat{\sigma})$ . Otherwise, check whether  $\hat{\sigma}' = \mathbf{X}\epsilon a$ . If so,  $\text{StrPenult}(\hat{\sigma})$  results from doing  $\sim ea \rightarrow \acute{e}a$  on  $\hat{\sigma}'$ ; if not,  $\text{StrPenult}(\hat{\sigma}) = \hat{\sigma}'$ .*

**Definition 6.3** (Spanish stop words). If a word belongs to the following list<sup>70</sup>:

*a, abajo, acá, acaso, adentro, afuera, ahí, ahora, al, algo, alguien, algun, algún, alguna, algunas, alguno, algunos, allá, allí, alrededor, ambas, ambos, ante, antes, aquel, aquél, aquella, aquélla, aquellas, aquéllas, aquello, aquellos, aquéllos, aquí, arriba, así, atrás, aun, aún, aunque, bajo, bien, cada, casi, cerca, como, cómo, con, conmigo, conosco, consigo, contigo, contra, convusco, cual, cuál, cuales, cualesquier, cualesquiera, cualquier, cualquiera, cuan, cuán, cuando, cuándo, cuanta, cuánta, cuantas, cuántas, cuanto, cuánto, cuantos, cuántos, cuya, cuya, cuyas, cuyo, cuyos, de, debajo, del, delante, dentro, desde, después, detrás, donde, dónde, durante, durea, e, el, él, ella, ellas, ello, ellos, empero, en, encima, enfrente, entonces, entre, esa, ésa, esas, ésas, ese, ése, éses, eso, esos, esta, ésta, estas, éstas, este, éste, éstos, esto, estos, frente, hacia, hasta, jamás, junto, la, las, le, lejos, les, lo, los, luego, mas, más, me, mediante, menos, mi, mí, mía, mías, mío, míos, mis, misma, mismas, mismísima, mismísimas, mismísimo, mismísimos, mismo, mismos, mucha, muchas, mucho, muchos, muy, nada, nadie, ni, ningún, ninguna, ningunas, ninguno, ningunos, no, nos, nosotras, nosotros, nuestra, nuestras, nuestro, nuestros, nunca, o, os, otra, otras, otro, otros, para, pero, poco, por, porque, pronto, pues, que, qué, quien, quién, quienes, quizá, según, si, sí, siempre, sin, sino, siquiera, so, sobre, su, sus, suya, suyas, suyo, suyos,*

<sup>70</sup>Our list of Spanish stop words is based on `snowball.tartarus.org/algorithms/spanish/stop.txt`, with extensive additions.



## (1) Replace

|                    |                |                     |                           |                    |               |               |              |                 |                        |                    |             |
|--------------------|----------------|---------------------|---------------------------|--------------------|---------------|---------------|--------------|-----------------|------------------------|--------------------|-------------|
| <i>af</i>          | <i>ag</i>      | <i>amab</i> (∅ i)l~ | <i>ami</i> (g stad stos)~ | <i>año</i>         | <i>at</i>     | <i>biblio</i> | <i>caus</i>  | <i>charlott</i> | <i>cinc</i>            | <i>com</i> (ú u)n~ |             |
| <i>αf</i>          | <i>αg</i>      | <i>φρεῦδ</i>        | <i>φρεῦδ</i>              | <i>ηαρο</i>        | <i>αt</i>     | <i>βιβλιω</i> | <i>καουσ</i> | <i>šarlotτ</i>  | <i>qi5</i>             | <i>κωτιῦ</i>       |             |
| <i>coment</i>      | <i>comprom</i> | <i>contr</i>        | <i>dis</i>                | <i>feli</i> (c z)~ | <i>gard</i>   | <i>inter</i>  | <i>list</i>  | <i>long</i>     | <i>mer</i> (a o)(∅ s)~ | <i>mili</i> (c t)~ | <i>mir</i>  |
| <i>κομεντ</i>      | <i>κπρομ</i>   | <i>κτρ</i>          | <i>δ</i>                  | <i>φελιζ</i>       | <i>γαρδ</i>   | <i>ι</i>      | <i>λιστ</i>  | <i>λοῦγ</i>     | <i>πιρ</i>             | <i>ααρμ</i>        | <i>μιρ</i>  |
| <i>pare</i> (∅ z)c | <i>posib</i>   | <i>posic</i>        | <i>positiv</i>            | <i>primaver</i>    | <i>primit</i> | <i>puerta</i> | <i>vener</i> | <i>vino</i>     | <i>carta</i> (∅ s)     | <i>jueves</i>      | <i>mary</i> |
| <i>πεαρ</i>        | <i>ποσιβ</i>   | <i>πωσιζ</i>        | <i>ρωσιτιβ</i>            | <i>σπριῦγ</i>      | <i>πριμιτ</i> | <i>ργορτ</i>  | <i>βεῦερ</i> | <i>ωῖνε</i>     | <i>λεττρ</i>           | <i>j4ue4</i>       | <i>μαρη</i> |

## (2) Replace

|                           |                                    |                                                 |                                               |                  |                      |            |           |               |                                       |                |               |             |           |             |
|---------------------------|------------------------------------|-------------------------------------------------|-----------------------------------------------|------------------|----------------------|------------|-----------|---------------|---------------------------------------|----------------|---------------|-------------|-----------|-------------|
| (á a)nim~                 | (di díga)                          | <b>Spanish Verb Combo</b>                       | (dia día)~                                    | (ie ié)          | (ndr ng)             | (zc zg)    | á         | <i>abuelo</i> | <i>ac</i>                             |                |               |             |           |             |
| <i>ανιμ</i>               |                                    | <i>decir</i>                                    | <i>δια</i>                                    | <i>ί</i>         | <i>n</i>             | <i>z</i>   | <i>a</i>  | <i>abuelω</i> | <i>αc</i>                             |                |               |             |           |             |
| <i>dece</i>               | <i>dif</i>                         | <i>dij</i>                                      | <i>diremos</i>                                | <i>dire</i>      | <i>edad</i>          | <i>edu</i> | <i>en</i> | <i>es</i>     | <i>ex</i>                             | <i>hermano</i> | <i>hermos</i> | <i>hijo</i> | <i>in</i> | <i>lady</i> |
| <i>δεce</i>               | <i>διf</i>                         | <i>διχ</i>                                      | <i>decir</i>                                  | <i>διρε</i>      | <i>εδαδ</i>          | <i>εδυ</i> | <i>εῦ</i> | <i>εs</i>     | <i>εξ</i>                             | <i>hermanω</i> | <i>hermωσ</i> | <i>hijω</i> | <i>ιῦ</i> | <i>lady</i> |
| <i>ldr</i>                | <i>marid</i>                       | <i>mejor</i> (∅ es)~                            | <i>oc</i>                                     | <i>ón</i>        | <i>par</i> (e ie)nt~ | <i>qu</i>  | <i>sg</i> | <i>sir</i>    | <i>su</i> <sup>Xε</sup> ((f g p r)χ)~ |                |               |             |           |             |
| <i>l</i>                  | <i>μαριδ</i>                       | <i>bueno</i>                                    | <i>ωc</i>                                     | <i>one</i>       | <i>παριεντ</i>       | <i>k</i>   | <i>s</i>  | <i>σιρ</i>    | <i>σωX</i>                            |                |               |             |           |             |
| <i>tío</i>                | <i>ye</i>                          | <b>StrPenult(giveSpanish)Spanish Verb Combo</b> | <b>StrPenult(goSpanish)Spanish Verb Combo</b> |                  |                      |            |           |               |                                       |                |               |             |           |             |
| <i>τίω</i>                | <i>e</i>                           | <i>σγιβσ</i>                                    | <i>σγοσ</i>                                   |                  |                      |            |           |               |                                       |                |               |             |           |             |
| (miss señorita srta)(∅ s) | (mr señor)(∅ es)                   | (mrs señora sra)(∅ s)                           | <b>giveSpanish</b>                            | <b>goSpanish</b> |                      |            |           |               |                                       |                |               |             |           |             |
| <i>mdseñorita</i>         | <i>mrseñor</i>                     | <i>fseñora</i>                                  | <i>σγιβσ</i>                                  | <i>σγοσ</i>      |                      |            |           |               |                                       |                |               |             |           |             |
| <i>mam</i> (a á i)(∅ s)   | <i>pap</i> (a á acito aito i)(∅ s) | ~χ̂(i i)s(mo ta tica tico)(∅ s)                 | ~dos                                          | ~tri(ces z)      |                      |            |           |               |                                       |                |               |             |           |             |
| <i>madre</i>              | <i>padre</i>                       | <i>χ̂e</i>                                      | <i>das</i>                                    | <i>tor</i>       |                      |            |           |               |                                       |                |               |             |           |             |

## (3) Replace

|             |          |                        |            |          |
|-------------|----------|------------------------|------------|----------|
| (∅ h)(u ü)e | c(c t)   | co <sup>Xε</sup> (g j) | én         | i        |
| <i>o</i>    | <i>z</i> | <i>racoX</i>           | <i>ena</i> | <i>i</i> |

(4) Do  $\acute{e} \rightarrow e$ ,  $\tilde{n} \rightarrow n$ ,  $\acute{o} \rightarrow o$ ,  $(\acute{u}|\ddot{u}) \rightarrow u$ .

(5) Do  $c^{V\epsilon}(a|o|u) \rightarrow k\mathbf{V}$ ,  $c^{V\epsilon}(e|i|\acute{i}) \rightarrow z\mathbf{V}$ ,  $g^{V\epsilon}(e|i|\acute{i}) \rightarrow j\mathbf{V}$ ,  $gu \rightarrow g$ .

(6) Do  $\underline{ven} \rightarrow vis$ ,  $\sim(d|mo|mos|n|r)\mathbf{SpanishVerbCombo} \rightarrow \emptyset$ ,  $\sim idad(\emptyset|es) \rightarrow \emptyset$ .

**Definition 6.5** (Spanish protected range). Let  $\hat{\sigma}$  be a text string derived from a Spanish word, its protected range  $\text{ProtRg}(\hat{\sigma})$  is an integer determined as follows:

- Try to find the string pattern  $(\emptyset|al|des|es|ko|pre|pro|ra|re|tran|tras)\mathbf{C}_m^* \mathbf{V}^*(\emptyset|(b|d|g|m|n|r|s|t|v|z)_m)~$  in the string  $\hat{\sigma}$ ;
- If the string pattern above is found, the last position occupied by such a string defines  $\text{ProtRg}(\hat{\sigma})$ ; otherwise, set  $\text{ProtRg}(\hat{\sigma}) = 0$ .  $\square$

**Algorithm 6.6** (Spanish essential root). Let  $\hat{\sigma}$  be the effective spelling of a Spanish word, then its corresponding essential root  $\text{EssRoot}(\hat{\sigma})$  is constructed in the following steps:

- (1) Do  $kom\mathbf{V}^* \sim \rightarrow kkom\mathbf{V}^*$  on  $\hat{\sigma}$  and call the result  $\hat{\sigma}_*$ .
- (2) Break down  $\hat{\sigma}_* = \hat{\sigma}_1\hat{\sigma}_2$  into the concatenation of two strings  $\hat{\sigma}_1 = \hat{\sigma}_*^{[\text{ProtRg}(\hat{\sigma}_*)]}$  (see the notation in Definition 3.1) and  $\hat{\sigma}_2$ , where the length of the first string  $\ell(\hat{\sigma}_1) = \text{ProtRg}(\hat{\sigma}_*)$  is equal to the protected range of  $\hat{\sigma}_*$ .
- (3) On  $\hat{\sigma}_2$ , perform the following substitutions in a sequel:
  - (3.1) Do  $\sim(d|t)(a|o)(\emptyset|s)(\emptyset|\mathbf{SpanishVerbCombo}) \rightarrow \emptyset$ ,  $\sim d(\emptyset|es) \rightarrow \emptyset$ .
  - (3.2) Do  $(ba|(b(\emptyset|i)(\emptyset|l))|nt|(r\mathbf{V}^*|\sim r)|st|\sim n)(\emptyset|\mathbf{SpanishVerbCombo}) \rightarrow \emptyset$ .
  - (3.3) Do  $(dor|g|ion|ka|ko|log|m|s|tiv|uv|y|z) \rightarrow \emptyset$ .<sup>71</sup>
  - (3.4) Do  $\sim\mathbf{V}_m^* \rightarrow \emptyset$ .

<sup>71</sup>We note that longer matches take priority over shorter matches: if *log* is found, then delete these three letters altogether, instead of just a single letter *g*.

The result after these four steps of operations is called  $\hat{\sigma}'_2$ .

(4) Concatenate  $\hat{\sigma}_1$  and  $\hat{\sigma}'_2$ .

(5) Perform the following replacements on  $\hat{\sigma}_1\hat{\sigma}'_2$ :

|                                                              |                   |                  |                                                                                                                      |                  |                  |                                           |                   |                  |                                      |
|--------------------------------------------------------------|-------------------|------------------|----------------------------------------------------------------------------------------------------------------------|------------------|------------------|-------------------------------------------|-------------------|------------------|--------------------------------------|
| $\text{X}^\epsilon(\emptyset \text{kon} \text{re})\text{di}$ | $\text{durm}$     | $\text{o}$       | $\sim\text{d}(\text{ez} \text{ich} \text{ig} \text{ij} \text{iz})$                                                   | $\sim\text{duj}$ | $\sim\text{jog}$ | $\sim\text{k}(\text{e} \text{u})\text{p}$ | $\sim\text{kerr}$ | $\sim\text{kis}$ | $\sim\text{p}(\text{ost} \text{us})$ |
| $\text{Xdir}$                                                | $\text{dorm}$     | $\text{oxx}$     | $\text{dir}$                                                                                                         | $\text{duz}$     | $\text{jug}$     | $\text{kab}$                              | $\text{ker}$      | $\text{kir}$     | $\text{pon}$                         |
| $\sim\text{pud}$                                             | $\sim\text{traj}$ | $\sim\text{tuv}$ | $\sim\text{v}(\text{e} \text{ed} \text{em} \text{er} \text{es} \text{im} \text{ind} \text{ir} \text{is} \text{ist})$ |                  |                  |                                           |                   |                  | $\sim\text{yaz}$                     |
| $\text{pod}$                                                 | $\text{tra}$      | $\text{ten}$     |                                                                                                                      | $\text{vis}$     |                  |                                           |                   |                  | $\text{yag}$                         |

### 6.1.2 Admissible mutation and approximate clustering

**Algorithm 6.7** (Spanish vowel blotting). Set  $\mathbf{V}_m^*$  and  $\mathbf{C}_{m_0}^*$  as in Definition 6.1. For a token string  $\hat{\sigma}$ , its blotted form  $\text{BlotV}_1(\hat{\sigma})$  is constructed as follows:

- If the string pattern  $(\emptyset|a|des|e|es|i|i|ko|o|pre|pro|ra|re|tran|tras|u)\mathbf{C}_{m_0}^*\mathbf{V}_m^*\sim$  can be found in the string  $\hat{\sigma}$ , then the last position occupied by such a pattern is replaced by the letter “a”.
- Otherwise, leave the string  $\hat{\sigma}$  intact.

Similar to what we did in §5 for three representative Germanic languages, we will construct a bivariate Boolean-valued function  $\text{HrdTest}(\hat{\alpha}, \hat{\beta})$  on a “simple heredity test function” in Algorithm 6.8, and a set of “admissible suffix mismatch and vowel alternation” rules in Algorithm 6.9.

**Algorithm 6.8** (Simple heredity test). The Boolean-valued function  $\text{SimpHrdTest}(\hat{\alpha}, \hat{\beta})$  returns **TRUE** if the lowercase form of  $\hat{\alpha}$  contains at least one instance of  $\mathbf{V}^*$  (Definition 6.1) **AND** at least one of the following four conditions holds:<sup>72</sup>

- After doing  $\sim s \rightarrow \emptyset$  on  $\hat{\beta}$ , we obtain  $\hat{\alpha}$ ;
- After doing  $\sim a(\emptyset|s) \rightarrow o$  on  $\hat{\alpha}$ , we obtain  $\hat{\beta}$ ;
- $\hat{\beta} = \hat{\alpha}k$ ;
- $\ell(\hat{\beta}) > \ell(\hat{\alpha}) \geq \frac{\ell(\hat{\beta})}{2}$  **AND**  $\hat{\alpha} = \hat{\beta}^{\ell(\hat{\alpha})}$  **AND**  $\hat{\beta}^{\ell(\hat{\alpha}'+1)} = \mathbf{V}^*$ . (See Definition 3.1 for the notations  $\hat{\beta}^{[n]}$  and  $\hat{\beta}^{[n]}$ .)

In what follows, we define  $\text{SuffixNW}(\hat{\alpha}, \hat{\beta})$ ,  $\text{RootNW}(\hat{\alpha}, \hat{\beta})$ ,  $\text{NW}^*(\hat{\alpha}, \hat{\beta})$  and  $\text{SuffixSW}(\hat{\alpha}, \hat{\beta})$ ,  $\text{SuffixSW}(\hat{\alpha}, \hat{\beta})$ ,  $\text{SW}^*(\hat{\alpha}, \hat{\beta})$  as what is done in the Danish case (Algorithm 5.7), which was also applied to two other Germanic languages treated in §5.

**Algorithm 6.9** (Admissible suffix mismatch and vowel alternation). For two strings  $\hat{\alpha}$  and  $\hat{\beta}$ , the Boolean-valued function

$$\text{AdmMut}(\text{RootNW}(\hat{\alpha}, \hat{\beta}), \text{SuffixNW}(\hat{\alpha}, \hat{\beta}), \text{NW}^*(\hat{\alpha}, \hat{\beta}))$$

returns **TRUE** if

$$\text{SuffixNW}(\hat{\alpha}, \hat{\beta}) = [(\emptyset|\mathbf{V}^*\mathbf{X}(d|t)|(r|s)\mathbf{X}|tiv\mathbf{X}), (\emptyset|\mathbf{V}^*\mathbf{X}(d|t)|(r|s)\mathbf{X}|tiv\mathbf{X})]$$

**AND** at least one of the following two conditions holds:

- $\text{NW}^*(\hat{\alpha}, \hat{\beta}) = \emptyset$  **AND**  $\text{RootNW}(\hat{\alpha}, \hat{\beta})$  contains at least one instance of  $\mathbf{V}^*$ ;
- $\text{NW}^*(\hat{\alpha}, \hat{\beta}) = ([e, i][[e, i][[i, i][[i, i]$ .

Similarly, one can evaluate another Boolean-valued function

$$\text{AdmSM}(\text{RootSW}(\hat{\alpha}, \hat{\beta}), \text{SuffixSW}(\hat{\alpha}, \hat{\beta}), \text{SW}^*(\hat{\alpha}, \hat{\beta}))$$

by trading all the occurrences of **NW** in the statements above with **SW**.

**Algorithm 6.10** (Heredity test function). The structure of the Spanish heredity test function  $\text{HrdTest}(\hat{\alpha}, \hat{\beta})$  is identical to the German version (Algorithm 8.1.2), except that the functions  $\text{SimpHrdTest}$ ,  $\text{RootNW}$ ,  $\text{SuffixNW}$ ,  $\text{NW}^*$ ,  $\text{RootSW}$ ,  $\text{SuffixSW}$ ,  $\text{SW}^*$  must follow the Spanish rules stated above.

<sup>72</sup>As a general rule in this document, the truth values of items labeled with Roman numerals are connected to each other with logical **OR**.



*hablaras, hablarás, hablare, hablaré, hablareis, hablaréis, hablaremos, habláremos, hablaren, hablares, hablaría, hablaríais, hablaríamos, hablarían, hablarías, hablaron, hablas, hablás, hablase, hablaseis, hablásemos, hablasen, hablaste, hablasteis, hable, hablé, habléis, hablemos, hablen, hables, hablés, hablo, habló* — “speak”;

*viva, viváis, vivamos, vivan, vivas, vivás, vive, viven, vives, viví, vivía, vivíais, vivíamos, vivían, vivías, vivid, vivida, vividas, vivido, vividos, viviendo, viviera, vivierais, viviéramos, vivieran, vivieras, viviere, viviereis, viviéremos, vivieren, vivieres, vivieron, viviese, vivieseis, viviésemos, viviesen, vivieses, vivimos, vivió, vivir, vivirá, vivirán, vivirás, viviré, viviréis, viviremos, viviría, viviríais, viviríamos, vivirían, vivirías, vivís, viviste, vivisteis, vivo* — “live”.

Without exceptions, the conjugated forms of these regular verbs follow the pattern **root + ending**, where the root remains invariant, while the ending starts with a vowel, and consists of at most two syllables (discounting final *~mos*). We shall refer to this pattern as the “canonical root-ending dichotomy” hereafter.

Applying the clustering algorithm to the conjugated forms of the three Spanish verbs above, we obtain

{*coma, comáis, comamos, coman, comas, comás, come, comé, comed, coméis, comemos, comen, comer, comerá, comerán, comerás, comeré, comeréis, comeremos, comería, comeríais, comeríamos, comerían, comerías, comes, comés, comí, comía, comíais, comíamos, comían, comías, comida, comidas, comido, comidos, comiendo, comiera, comierais, comiéramos, comieran, comieras, comiere, comiereis, comiéremos, comieren, comieres, comieron, comiese, comieseis, comiésemos, comiesen, comieses, comimos, comió, comiste, comisteis, como*}.

{*habla, habló, hablaba, hablabais, hablábamos, hablaban, hablabas, hablad, hablada, habladas, hablado, hablados, habláis, hablamos, hablan, hablando, hablar, hablara, hablará, hablarais, habláramos, hablaran, hablarán, hablaras, hablarás, hablare, hablaré, hablareis, hablaréis, hablaremos, habláremos, hablaren, hablares, hablaría, hablaríais, hablaríamos, hablarían, hablarías, hablaron, hablas, hablás, hablase, hablaseis, hablásemos, hablasen, hablaste, hablasteis, hable, hablé, habléis, hablemos, hablen, hables, hablés, hablo, habló*}.

{*viva, viváis, vivamos, vivan, vivas, vivás, vive, viven, vives, viví, vivía, vivíais, vivíamos, vivían, vivías, vivid, vivida, vividas, vivido, vividos, viviendo, viviera, vivierais, viviéramos, vivieran, vivieras, viviere, viviereis, viviéremos, vivieren, vivieres, vivieron, viviese, vivieseis, viviésemos, viviesen, vivieses, vivimos, vivió, vivir, vivirá, vivirán, vivirás, viviré, viviréis, viviremos, viviría, viviríais, viviríamos, vivirían, vivirías, vivís, viviste, vivisteis, vivo*}.

*Example 6.11.3.* Our typology for irregular Spanish verbs is largely based on Wiktionary ([https://en.wiktionary.org/wiki/Wiktionary:Spanish\\_verb\\_inflection-table\\_templates](https://en.wiktionary.org/wiki/Wiktionary:Spanish_verb_inflection-table_templates)). There are about one hundred different types of irregularities on this official template list. We are not going to exhaust all of them in our sample words.

In our clustering test in this example, we ignore some “trivially irregular verbs”, whose roots are at most off by a stress mark (which will be dropped in the effective spelling, anyway) in conjugated forms. We also ignore irregular types whose conjugation template follows the “canonical root-ending dichotomy”, even though the detailed endings may deviate from the three aforementioned regular types (for example, the conjugations of *distinguir* and *plañir*). Some highly irregular verbs in common use are also excluded from our test.

The typology on the aforementioned Wiktionary page regards [*o, ue*]**Xar**, [*o, ue*]**Xer** ending and [*o, ue*]**Xir** ending as three separate cases. We pick only one of these three scenarios for our test below, because our algorithm treats vowel alternations and endings independently. The same principle applies to other types of vowel alternations and consonant changes. What remain in our sample pool are the irregular verbs exhibiting systematic vowel alternation and/or consonant changes, which account for the overwhelming majority of irregular factors in Spanish verbs.

Concretely speaking, we send the following verbs

*adquiera, adquirieran, adquirieras, adquiere, adquieren, adquieres, adquiero, adquirirás, adquiramos, adquirí, adquiriría, adquiriríais, adquiríamos, adquirirían, adquirirías, adquiririd, adquirida, adquiridas, adquirido, adquiridos, adquiriendo, adquiriera, adquirierais, adquiriéramos, adquirieran, adquirieras, adquiriere, adquiriereis, adquiriéremos, adquirieren, adquirieres, adquirieron, adquiriese, adquirieseis, adquiriésemos, adquiriesen, adquirieses, adquirimos, adquirió, adquirir, adquirirá, adquirirán, adquirirás, adquiriré, adquiriréis, adquiriremos, adquiriría, adquiriríais, adquiriríamos, adquirirían, adquirirías, adquirirís, adquiriste, adquiristeis* — “acquire”;

*anda, andá, andaba, andabais, andábamos, andaban, andabas, andad, andada, andadas, andado, andados, andáis, andamos, andan, andando, andar, andarás, andarán, andarás, andaré, andaréis, andaremos, andaría, andaríaais, andaríaamos, andaríaan, andaríaas, andas, andás, ande, andéis, andemos, anden, andes, ando, anduve, anduviera, anduvierais, anduviéramos, anduvieran, anduvieras, anduviere, anduviereis, anduviéremos, anduvieren, anduvieres, anduvieron, anduviese, anduvieseis, anduviésemos, anduviesen, anduvieses, anduvimos, anduviste, anduvisteis, anduvo* — “walk”;





*prevén, prevendrá, prevendrán, prevendrás, prevendré, prevendréis, prevendremos, prevendría, prevendríaís, prevendríamos, prevendrían, prevendrían, prevenga, prevengáis, prevengamos, prevengan, prevengas, prevengo, prevenía, preveníaís, preveníamos, prevenían, prevenías, prevenid, prevenida, prevenidas, prevenido, prevenidos, prevenimos, prevenir, prevenís, previene, previenen, previenes, previne, previniendo, previniera, previnierais, previniéramos, previnieran, previnieras, previniere, previniereis, previniéremos, previnieren, previnieres, previniéron, previniése, previniéseis, previniésemos, previniesen, previnieses, previnimos, previniste, previnisteis, previno* — “prevent”;

*produce, producen, produces, producí, producía, producíaís, producíamos, producían, producías, producid, producida, producidas, producido, producidos, produciendo, producimos, producir, producirá, producirán, producirás, produciré, produciréis, produciremos, produciría, produciríaís, produciríamos, producirían, producirías, producis, produjo, produjera, produjeraís, produjéramos, produjeran, produjeras, produjere, produjereis, produjéremos, produjeren, produjeres, produjeron, produjese, produjeseis, produjésemos, produjesen, produjeses, produjimos, produjiste, produjisteis, produjo, produzca, produzcaís, produzcamos, produzcan, produzcas, produzcas, produzco* — “produce”;

*queráis, queramos, querás, queré, quered, queréis, queremos, querer, querés, quería, queríaís, queríamos, querían, querías, querida, queridas, querido, queridos, queriendo, querrá, querrán, querrás, querré, querréis, querramos, querría, querríaís, querríamos, querrían, querrías, quiera, quieran, quieras, quiere, quieren, quieres, quiero, quise, quisiera, quisierais, quisiéramos, quisieran, quisieras, quisiere, quisiereis, quisiéremos, quisieren, quisieres, quisieron, quisiese, quisieseis, quisiésemos, quisiesen, quisieses, quisimos, quisiste, quisisteis, quiso* — “desire”;

*rehuí, rehuía, rehuíaís, rehuíamos, rehuían, rehuías, rehuid, rehuida, rehuidas, rehuido, rehuidos, rehuimos, rehuir, rehuirá, rehuirán, rehuirás, rehuiré, rehuiréis, rehuiremos, rehuiría, rehuiríaís, rehuiríamos, rehuirían, rehuirías, rehúis, rehúiste, rehúisteis, rehuya, rehuyaís, rehuyamos, rehúyan, rehúyas, rehúye, rehúyen, rehuyendo, rehuyera, rehuyeraís, rehuyéramos, rehuyeran, rehuyeras, rehuyere, rehuyereis, rehuyéremos, rehuyeren, rehuyeres, rehuyeron, rehúyes, rehuyese, rehuyeseis, rehuyésemos, rehuyesen, rehuyeses, rehuyó, rehúyo* — “avoid”;

*repón, repondrá, repondrán, repondrás, repondré, repondréis, repondremos, repondría, repondríaís, repondríamos, repondrían, repondrían, reponed, reponed, reponéis, reponemos, reponen, reponer, repones, reponga, repongáis, repongamos, repongán, repongás, repongo, reponía, reponíaís, reponíamos, reponían, reponías, reponiendo, repuesta, repuestas, repuesto, repuestos, repuse, repusiera, repusierais, repusiéramos, repusieran, repusieras, repusiere, repusiereis, repusiéremos, repusieren, repusieres, repusieron, repusiese, repusieseis, repusiésemos, repusiesen, repusieses, repusimos, repusiste, repusisteis, repuso* — “replace”;

*retén, retendrá, retendrán, retendrás, retendré, retendréis, retendremos, retendría, retendríaís, retendríamos, retendrían, retendrían, retened, retened, retenéis, retenemos, retener, retenga, retengáis, retengamos, retengan, retengas, retengo, retenía, reteníaís, reteníamos, retenían, retenías, retenida, retenidas, retenido, retenidos, reteniendo, retiene, retienen, retienes, retuve, retuviera, retuvierais, retuviéramos, retuvieran, retuvieras, retuviere, retuviereis, retuviéremos, retuvieren, retuvieres, retuviese, retuvieseis, retuviésemos, retuviesen, retuvieses, retuvimos, retuviste, retuvisteis, retuvo* — “retain”;

*sal, saldrá, saldrán, saldrás, saldré, saldréis, saldremos, saldría, saldríaís, saldríamos, saldrían, saldrías, sale, salen, sales, salga, salgáis, salgamos, salgan, salgas, salgo, salí, salía, salíaís, salíamos, salían, salías, salid, salida, salidas, salido, salidos, saliendo, saliera, salierais, saliéramos, salieran, salieras, saliere, saliereis, saliéremos, salieren, salieres, salieron, saliese, salieseis, saliésemos, saliesen, salieses, salimos, salió, salir, salís, saliste, salisteis* — “leave”;

*trae, traed, traéis, traemos, traen, traer, traerá, traerán, traerás, traeré, traeréis, traeremos, traería, traeríaís, traeríamos, traerían, traerías, traes, traía, traíaís, traíamos, traían, traías, traída, traídas, traído, traídos, traiga, traigáis, traigamos, traigan, traigas, traigo, traje, trajera, trajeraís, trajéramos, trajeran, trajeras, trajere, trajereis, trajéremos, trajeren, trajeres, trajeron, trajese, trajeseis, trajésemos, trajesen, trajeses, trajimos, trajiste, trajisteis, trajo, trayendo* — “bring”;

*ve, vea, veáis, veamos, vean, veas, ved, veía, veíaís, veíamos, veían, veías, veis, vemos, ven, veo, ver, verá, verán, verás, veré, veréis, veremos, vería, veríaís, veríamos, verían, verías, ves, vi, viendo, viera, vierais, viéramos, vieran, vieras, viere, viereis, viéremos, vieren, vieres, vieron, viese, vieseis, viésemos, vieses, vieses, vimos, vio, vista, vistas, viste, visteis, visto, vistos* — “see”;

*yace, yaced, yacéis, yacemos, yacen, yacer, yacerá, yacerán, yacerás, yaceré, yaceréis, yaceremos, yacería, yaceríais, yaceríamos, yacerían, yacerías, yaces, yací, yacía, yacíais, yacíamos, yacían, yacías, yacida, yacidas, yacido, yacidos, yaciendo, yaciera, yacierais, yaciéramos, yacieran, yacieras, yaciere, yaciereis, yaciéremos, yacieren, yacieres, yacieron, yaciese, yacieseis, yaciésemos, yaciesen, yacieses, yacimos, yació, yaciste, yacisteis, yaga, yagáis, yagamos, yagan, yagas, yago, yaz, yazca, yazcáis, yazcamos, yazcan, yazcas, yazco, yazga, yazgáis, yazgamos, yazgan, yazgas, yazgo* — “recline”

as input, and receive

{*adquiera, adquieran, adquieras, adquiere, adquieren, adquieres, adquiero, adquiráis, adquiramos, adquirí, adquiría, adquiríais, adquiríamos, adquirirían, adquirirías, adquiririd, adquirida, adquiridas, adquirido, adquiridos, adquiriendo, adquiriera, adquirierais, adquiriéramos, adquirieran, adquirieras, adquiriere, adquiriereis, adquiriéremos, adquirieren, adquirieres, adquirieron, adquiriese, adquirieseis, adquiriésemos, adquiriesen, adquirieses, adquirimos, adquirió, adquirir, adquirirá, adquirirán, adquirirás, adquiriré, adquiriréis, adquiriremos, adquiriría, adquiriríais, adquiriríamos, adquirirían, adquirirías, adquirirís, adquiriste, adquiristeis*}

{*anda, andá, andaba, andabais, andábamos, andaban, andabas, andad, andada, andadas, andado, andados, andáis, andamos, andan, andando, andar, andaré, andarán, andarás, andaré, andaréis, andaremos, andaría, andaríaís, andaríamos, andarian, andaríaís, andas, andás, ande, andéis, andemos, anden, andes, ando, anduve, anduviera, anduvierais, anduviéramos, anduvieran, anduvieras, anduviere, anduviereis, anduviéremos, anduvieren, anduvieres, anduvieron, anduviese, anduvieseis, anduviésemos, anduviesen, anduvieses, anduvimos, anduviste, anduvisteis, anduvo*}

{*argüí, argüía, argüíais, argüíamos, argüían, argüías, argüid, argüida, argüidas, argüido, argüidos, argüimos, argüir, argüiré, argüirán, argüirás, argüiré, argüiréis, argüiremos, argüiría, argüiríais, argüiríamos, argüirían, argüirías, argüís, argüiste, argüisteis, arguya, arguyáis, arguyamos, arguyan, arguyas, arguye, arguyen, arguyendo, arguyera, arguyerais, arguyéramos, arguyeran, arguyeras, arguyere, arguyereis, arguyéremos, arguyeren, arguyeres, arguyeron, arguyes, arguyese, arguyeseis, arguyésemos, arguyesen, arguyeses, arguyo, arguyó*}

{*ase, asen, ases, asga, asgáis, asgamos, asgan, asgas, asgo, así, asia, asíais, asíamos, asían, asías, asid, asida, asidas, asido, asidos, asiendo, asiera, asierais, asiéramos, asieran, asieras, asiere, asiereis, asiéremos, asieren, asieres, asieron, asiese, asieseis, asiésemos, asiesen, asieses, asimos, asió, asir, asirá, asirán, asirás, asiré, asiréis, asiremos, asiría, asiríais, asiríamos, asirían, asirías, asís, asiste, asisteis*}

{*avergoncé, avergoncéis, avergoncemos, avergonzaba, avergonzabais, avergonzábamos, avergonzaban, avergonzabas, avergonzad, avergonzada, avergonzadas, avergonzado, avergonzados, avergonzáis, avergonzamos, avergonzando, avergonzar, avergonzara, avergonzaré, avergonzarais, avergonzáríamos, avergonzaran, avergonzarán, avergonzaras, avergonzarás, avergonzare, avergonzaré, avergonzareis, avergonzaréis, avergonzaremos, avergonzáríamos, avergonzaren, avergonzares, avergonzaría, avergonzaríais, avergonzaríamos, avergonzarían, avergonzarías, avergonzaron, avergonzase, avergonzaseis, avergonzásemos, avergonzasen, avergonzases, avergonzaste, avergonzasteis, avergonzó, avergüence, avergüencen, avergüences, avergüenza, avergüenzan, avergüenzas, avergüenzo*}

{*cabe, cabed, cabéis, cabemos, caben, caber, cabes, cabía, cabíais, cabíamos, cabían, cabías, cabida, cabidas, cabido, cabidos, cabiendo, cabrá, cabrán, cabrás, cabré, cabréis, cabremos, cabría, cabríaís, cabríamos, cabrían, cabrias, cupe, cupiera, cupierais, cupiéramos, cupieran, cupieras, cupiere, cupiereis, cupiéremos, cupieren, cupieres, cupieron, cupiese, cupieseis, cupiésemos, cupiesen, cupieses, cupimos, cupiste, cupisteis, cupo, quepa, quepáis, quepamos, quepan, quepas, quepo*}

{*cae, caed, caéis, caemos, caen, caer, caerá, caerán, caerás, caeré, caeréis, caeremos, caería, caeríaís, caeríamos, caerían, caerías, caes, caí, caía, caíaís, caíamos, caían, caías, caida, caidas, caído, caídos, caiga, caigáis, caigamos, caigan, caigas, caigo, caímos, caiste, caisteis, cayendo, cayera, cayerais, cayéramos, cayeran, cayeras, cayere, cayeréis, cayéremos, cayeren, cayeres, cayeron, cayese, cayeseis, cayésemos, cayesen, cayeses, cayó*}

{*coge, coged, cogéis, cogemos, cogen, coger, cogerá, cogerán, cogerás, cogeré, cogeréis, cogereamos, cogería, cogeriaís, cogeriíamos, cogieran, cogieras, coges, cogí, cogía, cogíaís, cogíamos, cogían, cogías, cogida, cogidas, cogido, cogidos, cogiendo, cogiera, cogierais, cogiéramos, cogieran, cogieras, cogiere, cogiereis, cogiéremos, cogieren, cogieres, cogieron, cogiese, cogieseis, cogiésemos, cogiesen, cogieses, cogimos, cogió, cogiste, cogisteis, coja, cojáis, cojamos, cojan, cojas, cojo*}

{*conoce, conocé, conoced, conocéis, conocemos, conocen, conocer, conocerá, conocerán, conocerás, conoceré, conoceréis, conoceremos, conocería, conoceríais, conoceríamos, conocerían, conocerías, conoces, conocés, conocí, conocía, conocíais, conocíamos, conocían, conocías, conocida, conocidas, conocido, conocidos, conociendo, conociera, conocierais, conociéramos, conocieran, conocieras, conociere, conociereis, conociéremos, conocieren, conocieres, conocieron, conociese, conocieseis, conociésemos, conociesen, conocieses, conocimos, conoció, conociste, conocisteis, conozca, conozcáis, conozcamos, conozcan, conozcas, conozco*},

{*cruce, crucé, crucéis, crucemos, crucen, cruces, crucés, cruza, cruzá, cruzaba, cruzabais, cruzábamos, cruzaban, cruzabas, cruzad, cruzada, cruzadas, cruzado, cruzados, cruzáis, cruzamos, cruzan, cruzando, cruzar, cruzara, cruzará, cruzarais, cruzáramos, cruzaran, cruzarán, cruzaras, cruzarás, cruzare, cruzaré, cruzareis, cruzaréis, cruzaremos, cruzáremos, cruzaren, cruzares, cruzaría, cruzaríais, cruzaríamos, cruzarían, cruzarías, cruzaron, cruzas, cruzás, cruzase, cruzaseis, cruzásemos, cruzasen, cruzases, cruzaste, cruzasteis, cruzo, cruzó*},

{*decía, decíais, decíamos, decían, decías, decid, decidimos, decir, decís, dice, dicen, dices, dicha, dichas, dicho, dichos, diciendo, diga, digáis, digamos, digan, digas, digo, dije, dijera, dijerais, dijéramos, dijeran, dijeras, dijere, dijereis, dijéremos, dijeren, dijeres, dijeron, dijese, dijeseis, dijésemos, dijesen, dijeses, dijimos, dijiste, dijisteis, dijo, dirá, dirán, dirás, diré, diréis, diremos, diría, diríais, diríamos, dirían, dirías, discernáis*},

{*delinca, delincáis, delincamos, delincan, delincas, delinco, delinque, delinquen, delinques, delinquí, delinquía, delinquíais, delinquíamos, delinquíán, delinquíás, delinquíad, delinquíada, delinquíadas, delinquíado, delinquíados, delinquíando, delinquíara, delinquíerais, delinquíéramos, delinquíeran, delinquíeras, delinquíere, delinquíereis, delinquíéremos, delinquíeren, delinquíeres, delinquíeron, delinquíese, delinquíeseis, delinquíésemos, delinquíesiesen, delinquíeses, delinquíemos, delinquíó, delinquir, delinquirá, delinquirán, delinquirás, delinquiré, delinquiréis, delinquiremos, delinquiría, delinquiríais, delinquiríamos, delinquirían, delinquirías, delinquíis, delinquistes, delinquisteis*},

{*deshuesa, deshuesa, deshuesan, deshuesas, deshuese, deshuesen, deshueses, deshueso, desosaba, desosabais, desosábamos, desosaban, desosabas, desosad, desosada, desosadas, desosado, desosados, desosáis, desosamos, desosando, desosar, desosara, desosará, desosarais, desosáramos, desosaran, desosarán, desosaras, desosará, desosare, desosaré, desosareis, desosaréis, desosaremos, desosáremos, desosaren, desosares, desosaría, desosaríais, desosaríamos, desosarían, desosarías, desosaron, desosás, desosase, desosaseis, desosásemos, desosasen, desosases, desosaste, desosasteis, desosé, desoséis, desosemos, desosó*},

{*di*},

{*discernamos, discerní, discernía, discerníais, discerníamos, discernían, discernías, discernid, discernida, discernidas, discernido, discernidos, discerniendo, discerniera, discernierais, discerniéramos, discernieran, discernieras, discerniere, discerniereis, discerniéremos, discernieren, discernieres, discernieron, discerniese, discernieseis, discerniésemos, discerniesen, discernieses, discernimos, discernió, discernir, discernirá, discernirán, discernirás, discerniré, discerniréis, discerniremos, discerniría, discerniríais, discerniríamos, discernirían, discernirías, discernís, discerniste, discernisteis, discierna, disciernan, disciernas, discierne, disciernen, disciernes, discierno*},

{*erra, erraba, errabais, errábamos, erraban, errabas, errad, errada, erradas, errado, errados, erráis, erramos, erran, errando, errar, errara, errará, errarais, erráramos, erraran, errarán, erraras, errarás, errare, erraré, errareis, erraréis, erraremos, erráremos, erraren, errares, erraría, erraríais, erraríamos, errarían, errarías, erraron, erras, errase, erraseis, errásemos, errasen, errases, erraste, errasteis, erre, erré, erréis, erremos, erren, erres, erro, erró, yerra, yerran, yerras, yerre, yerren, yerres, yerro*},

{*juega, juegan, juegas, juego, juegue, jueguen, juegues, jugá, jugaba, jugabais, jugábamos, jugaban, jugabas, jugad, jugada, jugadas, jugado, jugados, jugáis, jugamos, jugando, jugar, jugara, jugará, jugarais, jugaráramos, jugaran, jugarán, jugaras, jugarás, jugare, jugaré, jugareis, jugaréis, jugaremos, jugáremos, jugaren, jugares, jugaría, jugaríais, jugaríamos, jugarían, jugarías, jugaron, jugás, jugase, jugaseis, jugásemos, jugasen, jugases, jugaste, jugasteis, jugó, jugué, juguéis, juguemos, jugués*},

{*lea, leáis, leamos, lean, leas, lee, leé, leed, leéis, leemos, leen, leer, leerá, leerán, leerás, leeré, leeréis, leeremos, leería, leeríais, leeríamos, leerían, leerías, lees, leés, leí, leía, leíais, leíamos, leían, leías, leída, leídas, leído, leídos, leímos, leíste, leísteis, leo, leyendo, leyera, leyerais, leyéramos, leyeran, leyeras, leyere, leyereis, leyéremos, leyeren, leyeres, leyeron, leyese, leyeseis, leyésemos, leyesen, leyeses, leyó*},

{*oí, oía, oíais, oíamos, oían, oías, oíd, oída, oídas, oído, oídos, oiga, oigáis, oigamos, oigan, oigas, oigo, oímos, oír, oirá, oirán, oirás, oiré, oiréis, oiremos, oiría, oiríais, oiríamos, oirían, oirías, oís, oíste, oísteis, oye, oyen, oyendo, oyerá, oyeráis, oyéramos, oyeran, oyeras, oyere, oyeréis, oyéremos, oyeren, oyeres, oyeron, oyes, oyese, oyeseis, oyésemos, oyesen, oyeses, oyó*},

{*pedí, pedía, pedíais, pedíamos, pedían, pedías, pedid, pedida, pedidas, pedido, pedidos, pedimos, pedir, pedirá, pedirán, pedirás, pediré, pediréis, pediremos, pediría, pediríais, pediríamos, pedirían, pedirías, pedís, pediste, pedisteis, pida, pidáis, pidamos, pidan, pidas, pide, piden, pides, pidiendo, pidiera, pidierais, pidiéramos, pidieran, pidieras, pidiere, pidiereis, pidiéremos, pidieren, pidieres, pidieron, pidiese, pidieseis, pidiésemos, pidiesen, pidieses, pidió, pido*},

{*pervetí, pervetía, pervetíais, pervetíamos, pervetían, pervetías, pervetid, pervetida, pervetidas, pervetido, pervetidos, pervetimos, pervetir, pervetirá, pervetirán, pervetirás, pervetiré, pervetiréis, pervetiremos, pervetiría, pervetiríais, pervetiríamos, pervetirían, pervetirías, pervetís, pervetiste, pervetisteis, pervierta, perviertan, perviertas, pervierte, pervierten, perviertes, pervierto, pervirtáis, pervirtamos, pervirtás, pervirtiende, pervirtiera, pervirtierais, pervirtiéramos, pervirtieran, pervirtieras, pervirtiere, pervirtiereis, pervirtiéremos, pervirtieren, pervirtieres, pervirtieron, pervirtiese, pervirtieseis, pervirtiésemos, pervirtiesen, pervirtieses, pervirtió*},

{*podáis, podamos, poded, podéis, podemos, poder, podía, podíais, podíamos, podían, podías, podida, podidas, podido, podidos, podrá, podrán, podrás, podré, podréis, podremos, podría, podríais, podríamos, podrían, podrías, pude, pudiendo, pudiera, pudierais, pudiéramos, pudieran, pudieras, pudiere, pudiereis, pudiéremos, pudieren, pudieres, pudieron, pudiese, pudieseis, pudiésemos, pudiesen, pudieses, pudimos, pudiste, pudisteis, pudo, pueda, puedan, puedan, puede, pueden, puedes, puedo*},

{*prevén, prevendrá, prevendrán, prevendrás, prevendré, prevendréis, prevendremos, prevendría, prevendríais, prevendríamos, prevendrían, prevendrías, prevenga, prevengáis, prevengamos, prevengan, prevengas, prevengo, prevenía, preveníais, preveníamos, prevenían, prevenías, prevenid, prevenida, prevenidas, prevenido, prevenidos, prevenimos, prevenir, prevenís, previene, previenen, previenes, previne, previniendo, previniera, previnierrais, previniéramos, previnieran, previnieras, previniere, previniereis, previniéremos, previnieren, previnieres, previnieron, previniere, previniereis, previniésemos, previniesen, previnieses, previnimos, previniste, previnisteis, previno*},

{*produce, producen, produces, producí, producía, producíais, producíamos, producían, producías, producid, producida, producidas, producido, producidos, produciendo, producimos, producir, producirá, producirán, producirás, produciré, produciréis, produciremos, produciría, produciríais, produciríamos, producirían, producirías, producí, produce, produjera, produjeráis, produjéramos, produjeran, produjeras, produjere, produjereis, produjéremos, produjeren, produjeres, produjeron, produjese, produjeseis, produjésemos, produjesen, produjeses, produjimos, produjiste, produjisteis, produjo, produzca, produzcaís, produzcamos, produzcan, produzcas, produzcas, produzco*},

{*queráis, queramos, querás, queré, quered, queréis, queremos, querer, querés, quería, queríais, queríamos, querían, querías, querida, queridas, querido, queridos, queriendo, querrá, querrán, querrás, querré, querréis, querramos, querría, querríais, querríamos, querrían, querrías, quiera, quieran, quieras, quiere, quieren, quieres, quiero, quise, quisiera, quisierais, quisiéramos, quisieran, quisieras, quisiere, quisiereis, quisiéremos, quisieren, quisieres, quisieron, quisiese, quisieseis, quisiésemos, quisiesen, quisieses, quisimos, quisiste, quisisteis, quiso*},

{*rehuí, rehuía, rehuíais, rehuíamos, rehuían, rehuías, rehuíd, rehuida, rehuidas, rehuido, rehuidos, rehuimos, rehuir, rehuirá, rehuirán, rehuirás, rehuiré, rehuiréis, rehuiremos, rehuiría, rehuiríais, rehuiríamos, rehuirían, rehuirías, rehuís, rehuiste, rehuisteis, rehúya, rehuyáis, rehuyamos, rehúyan, rehúyas, rehúye, rehúyen, rehuyendo, rehuyera, rehuyerais, rehuyéramos, rehuyeran, rehuyeras, rehuyere, rehuyereis, rehuyéremos, rehuyeren, rehuyeres, rehuyeron, rehúyes, rehuyese, rehuyeseis, rehuyésemos, rehuyesen, rehuyeses, rehuyó, rehúyo*},

{*repón, repondrá, repondrán, repondrás, repondré, repondréis, repondremos, repondría, repondríais, repondríamos, repondrían, repondrías, repone, reponed, reponéis, reponemos, reponen, reponer, repones, reponga, repongáis, repongamos, repongán, repongás, repongo, reponía, reponíais, reponíamos, reponían, reponías, reponiendo, repuesta, repuestas, repuesto, repuestos, repuse, repusiera, repusierais, repusiéramos, repusieran, repusieras, repusiere, repusiereis, repusiéremos, repusieren, repusieres, repusieron, repusiese, repusieseis, repusiésemos, repusiesen, repusieses, repusimos, repusiste, repusisteis, repuso*},

{*retén, retendrá, retendrán, retendrás, retendré, retendréis, retendremos, retendría, retendríaís, retendríamos, retendrían, retendrían, retened, retenéis, retenemos, retener, retenga, retengáis, retengamos, retengan, retengas, retengo, retenía, reteníaís, reteníamos, retenían, retenías, retenida, retenidas, retenido, retenidos, reteniendo, retiene, retienen, retienes, retuve, retuviera, retuvierais, retuviéramos, retuvieran, retuvieras, retuviere, retuviereis, retuviéremos, retuvieren, retuvieres, retuvieron, retuviere, retuviereis, retuviésemos, retuviesen, retuvieses, retuvimos, retuviste, retuvisteis, retuvo*},

{*sal, saldrá, saldrán, saldrás, saldré, saldréis, saldremos, saldría, saldríaís, saldríamos, saldrían, saldrías, sale, salen, sales, salga, salgáis, salgamos, salgan, salgas, salgo, salt, salía, salíaís, salíamos, salían, salías, salid, salida, salidas, salido, salidos, saliendo, saliera, salierais, saliéramos, salieran, salieras, saliere, saliereis, saliéremos, salieren, salieres, salieron, saliese, salieseis, saliésemos, saliesen, salieses, salimos, salió, salir, salís, saliste, salisteis*},

{*trae, traed, traéis, traemos, traen, traer, traerá, traerán, traerás, traeré, traeréis, traeremos, traería, traeríaís, traeríamos, traerían, traerías, traes, traía, traíaís, traíamos, traían, traías, traída, traídas, traído, traídos, traiga, traigáis, traigamos, traigan, traigas, traigo, traje, trajera, trajerais, trajéramos, trajeran, trajeras, trajere, trajereis, trajéremos, trajeren, trajeres, trajeron, trajese, trajeseis, trajésemos, trajesen, trajeses, trajimos, trajiste, trajisteis, trajo, trayendo*},

{*ve*}},

{*vea, veáis, veamos, vean, veas, ved, veía, veíaís, veíamos, veían, veías, veis, vemos, ven, veo, ver, verá, verán, verás, veré, veréis, veremos, vería, veríaís, veríamos, verían, verías, ves, vi, viendo, viera, vierais, viéramos, vieran, vieras, viere, viereis, viéremos, vieren, vieres, vieron, viere, viereis, viésemos, vieses, vieses, vimos, vio, vista, vistas, viste, visteis, visto, vistos*},

{*yace, yaced, yacéis, yacemos, yacen, yacer, yacerá, yacerán, yacerás, yaceré, yaceréis, yaceremos, yacería, yaceríaís, yaceríamos, yacerían, yacerías, yaces, yací, yacía, yacíaís, yacíamos, yacían, yacías, yacida, yacidas, yacido, yacidos, yaciendo, yaciera, yacierais, yaciéramos, yacieran, yacieras, yaciere, yaciereis, yaciéremos, yacieren, yacieres, yacieron, yaciese, yacieseis, yaciésemos, yaciesen, yacieses, yacimos, yació, yaciste, yacisteis, yaga, yagáis, yagamos, yagan, yagas, yago, yaz, yazca, yazcáis, yazcamos, yazcan, yazcas, yazco, yazga, yazgáis, yazgamos, yazgan, yazgas, yazgo*}

as output. Here, the ambiguous words *di* and *ve* become orphans in our algorithm: *di* is a conjugated form of both *dar* “give” and *decir* “say”; *ve* is a conjugated form of both *ir* “go” and *ver* “see”.

*Example 6.11.4.* In Fig. S7, we further apply the aforementioned word clustering algorithm to topic extraction and machine translation (see Table S1 for text source).

Note that the machine translation task is particularly challenging in the example shown, for at least two reasons: (1) The translator has merged the name *Elizabeth* and the nickname *Lizzy* of the protagonist into one; (2) The Spanish noun *casa* “house” is spelt the same way as a conjugated form of the Spanish verb *casar* “marry”. Despite these disadvantages, the topics that are unrelated to these challenges are correctly translated.

In Fig. S7b, we consider the Spanish word *capital* “capital (city)” an exact match to the English word *town*, because the latter refers to London in *Pride and Prejudice*.

In Spanish, both *bella* and *hermosa* mean “beautiful” and modify feminine nouns. It thus comes to no surprise that the row for “beautiful” in Fig. S7b contains two hot spots that correspond to these two Spanish adjectives.



## 6.2 Modified Porter stemming algorithm for French

The French verbs for “to be” and “to have” are highly irregular. These verbs are also used as auxiliaries in various tenses and moods of arbitrary verbs, similar to their counterparts in English. All their conjugated forms (including the infinitive forms) are treated as stop words.

*a, ai, aie, aient, aies, ait, as, aura, aurai, auraient, aurais, aurait, auras, aurez, auriez, aurions, aurons, auront, avaient, avais, avait, avez, aviez, avons, avoir, avons, ayant, ayez, ayons, eu, eûmes, eurent, eus, eusse, eussent, eusses, eussiez, eussions, eut, eût, eûtes, ont* — “have”;

*es, est, étaient, étais, était, étant, été, êtes, étiez, étions, être, fûmes, furent, fus, fusse, fussent, fusses, fussiez, fussions, fut, fût, fûtes, sera, serai, seraient, serais, serait, seras, serez, seriez, serions, serons, seront, soient, sois, soit, sommes, sont, soyez, soyons, suis* — “be”.

In addition, we treat the following verbs as stop words.

*faire, fais, faisaient, faisais, faisait, faisant, faisiez, faisons, faisons, fait, faites, fasse, fassent, fasses, fassiez, fassions, fera, ferai, feraient, ferais, ferait, feras, ferez, feriez, ferions, ferons, feront, fîmes, firent, fis, fisse, fissent, fisses, fissiez, fissions, fit, fit, fîtes, font* — “do”;

*fallait, falloir, fallu, fallut, faudra, faudrait, faut* — “be necessary”;

*peut, peuvent, peux, pourra, pourrai, pourraient, pourrais, pourrait, pourras, pourrez, pourriez, pourrions, pourrons, pourront, pouvaient, pouvais, pouvait, pouvant, pouvez, pouviez, pouvions, pouvoir, pouvons, pu, puisse, puissent, puisses, puissiez, puissions, pûmes, purent, pus, pusse, pussent, pusses, pussiez, pussions, put, pût, pûtes* — “can”.

**Definition 6.12** (French stop words). If a word belongs to the following list<sup>73</sup>:

*a, à, afin, ai, aie, aient, aies, ainsi, ait, alors, après, arrière, as, assez, au, aucun, aucune, aucunes, aucuns, aura, aurai, auraient, aurais, aurait, auras, aurez, auriez, aurions, aurons, auront, aussi, autant, autour, autre, autrefois, autres, aux, avaient, avais, avait, avant, avec, avez, aviez, avions, avoir, avons, ayant, ayez, ayons, beaucoup, bien, bientôt, c, ça, çà, car, ce, ceci, cela, celà, celle, celles, celui, cependant, ces, cet, cette, ceux, chacun, chacune, chaque, chez, ci, combien, comme, comment, contre, d, dans, de, dedans, dehors, déjà, depuis, dernier, dernière, dernières, derniers, derrière, des, dès, dessous, dessus, devaient, devais, devait, devant, devez, deviez, devons, devoir, devons, devra, devrai, devraient, devrais, devrait, devras, devrez, devriez, devrions, devrons, devront, dois, doit, doive, doivent, doives, donc, dont, du, dû, dûmes, durant, durent, dus, dusse, dussent, dusses, dussiez, dussions, dut, dût, dûtes, elle, elles, en, encore, envers, es, est, et, étaient, étais, était, étant, été, êtes, étiez, étions, être, eu, eue, eues, eûmes, eurent, eus, eusse, eussent, eusses, eussiez, eussions, eut, eût, eûtes, eux, faire, fais, faisaient, faisais, faisait, faisant, faisiez, faisons, faisons, fait, faite, faites, faits, fallait, falloir, fallu, fallut, fasse, fassent, fasses, fassiez, fassions, faudra, faudrait, faut, fera, ferai, feraient, ferais, ferait, feras, ferez, feriez, ferions, ferons, feront, fîmes, firent, fis, fisse, fissent, fisses, fissiez, fissions, fit, fit, fîtes, fois, font, fûmes, furent, fus, fusse, fussent, fusses, fussiez, fussions, fut, fût, fûtes, hors, ici, il, ils, j, jamais, je, jusqu, jusque, juste, justement, l, la, là, laquelle, le, lequel, les, lesquelles, lesquels, leur, leurs, lors, lorsqu, lorsque, lui, m, ma, maintenant, mais, malgré, me, même, mêmes, mes, mien, mienne, miennes, miens, moi, moindre, moins, mon, n, ne, ni, non, nos, notre, nôtre, nôtres, nous, nul, nulle, nulles, nuls, on, ont, ou, où, oui, par, parce, parfois, parmi, partout, pas, pendant, personne, peu, peut, peuvent, peux, plupart, plus, plusieurs, plutôt, pour, pourquoi, pourra, pourrai, pourraient, pourrais, pourrait, pourras, pourrez, pourriez, pourrions, pourrons, pourront, pourtant, pouvaient, pouvais, pouvait, pouvant, pouvez, pouviez, pouvions, pouvoir, pouvons, presque, presque, prochain, prochaine, prochaines, prochains, propos, pu, puis, puisque, puisse, puissent, puisses, puissiez, puissions, pûmes, purent, pus, pusse, pussent, pusses, pussiez, pussions, put, pût, pûtes, qu, quand, quant, que, quel, quelconque, quelle, quelles, quelque, quelquefois, quelques, quels, qui, quiconque, quoi, quoique, rien, s, sa, sans, sauf, se, selon, sera, serai, seraient, serais, serait, seras, serez, seriez, serions, serons, seront, ses, si, sien, sienne, siennes, siens, sitôt, soi, soient, sois, soit, sommes, son, sont, sous, souvent, soyez, soyons, suis, sur, surtout, t, ta, tandis, tant, tantôt, te, tel, telle, tellement, telles, tels, tes, tien, tienne, tiennes, tiens, toi, ton, toujours, tous, tout, toute, toutefois, toutes, travers, très, trop, tu, un, une, unes, uns, vers, voici, voilà, vos, votre, vôtre, vôtres, vous, y,*

then we consider it a French stop word. All the French stop words that appear in a particular document need to be ignored before we perform word clustering on the rest of the vocabulary list. □

<sup>73</sup>Our list of French stop words is based on [snowball.tartarus.org/algorithms/french/stop.txt](http://snowball.tartarus.org/algorithms/french/stop.txt), with extensive modifications that roughly match their counterparts in English.

The French verbs for “to come” and “to go” also have highly irregular conjugations:<sup>74</sup>

*aille, aillent, ailles, alla, allai, allaient, allais, allait, allâmes, allant, allas, allasse, allassent, allasses, allassiez, allassions, allât, allâtes, allé, allés, aller, allèrent, allez, allez, allions, allons, ira, irai, iraient, irais, irait, iras, irez, iriez, irions, irons, iront, va, vais, vas, vont* — “go”;

*venaient, venais, venait, venant, venez, venez, venions, venir, venons, venu, venus, viendra, viendrai, viendraient, viendrais, viendrait, viendras, viendrez, viendriez, viendrions, viendrons, viendront, vienne, viennent, viennes, viens, vient, vîmmes, vinrent, vins, vinsse, vînsent, vînses, vînsiez, vînsions, vint, vînt, vîntes* — “come”.

We are not going to treat them as stop words in French, so as to be consistent with their counterparts in other languages. However, to prepare for clustering of content words, we will refer to these two groups of strings as **goFrench** and **comeFrench**, respectively.

## 6.2.1 Effective spelling and essential root

**Definition 6.13** (French Vowel Extensions). Hereafter in §6.2, the symbol  $\mathbf{V}^*$  stands for any member from the list  $\{a, \hat{a}, e, \hat{e}, i, \hat{i}, o, u, \hat{u}\}$ , the so-called French vowel extensions. In line with the multiplicity notations introduced in Definition 3.3, the symbol  $\mathbf{V}_m^*$  stands for a text string formed by consecutive appearance of one or more (not necessarily identical or distinct) members from the set of French vowel extensions.

Dual to the notations above, the symbol  $\mathbf{C}^*$  stands for any character that does not belong to the list  $\{a, \hat{a}, e, \hat{e}, i, \hat{i}, o, u, \hat{u}\}$ , and  $\mathbf{C}_{m_0}^*$  stands for a text string formed by consecutive appearance of zero or more (not necessarily identical or distinct) characters that do not belong to the same list.  $\square$

**Algorithm 6.14** (French effective spelling). For a French word  $\hat{\sigma}$ , its effective spelling  $\text{EffSpell}(\hat{\sigma})$  is constructed in six sequential steps:

(1) *Replace*<sup>75</sup>

|                                       |                                                |                                       |                                                                 |                                      |                                        |                                 |                           |                            |                               |                               |                 |                 |                                  |
|---------------------------------------|------------------------------------------------|---------------------------------------|-----------------------------------------------------------------|--------------------------------------|----------------------------------------|---------------------------------|---------------------------|----------------------------|-------------------------------|-------------------------------|-----------------|-----------------|----------------------------------|
| $ab\mathbf{C}^*\sim$                  | $amabilit\hat{e}\sim$                          | $chance\sim$                          | $charlotte$                                                     | $d\acute{e}f\mathbf{X}\sim$          | $d\acute{e}mi\sim$                     | $d\acute{e}tect\mathbf{X}\sim$  | $d\acute{e}tei\sim$       |                            |                               |                               |                 |                 |                                  |
| $b\alpha a\mathbf{C}^*$               | $ami$                                          | $\beta ance$                          | $char\lambda\omega\tau$                                         | $\delta\phi$                         | $d\epsilon mi$                         | $\tau\delta\epsilon\kappa\tau$  | $\tau\beta\tau\epsilon i$ |                            |                               |                               |                 |                 |                                  |
| $d\acute{e}tend\sim$                  | $d\acute{e}test\mathbf{X}\sim$                 | $diab(\emptyset o)l\sim$              | $discour\sim$                                                   | $foyer\sim$                          | $fr\acute{e}m\sim$                     | $guet\sim$                      | $guid\sim$                | $imposs\sim$               | $inct\mathbf{X}$              | $lisi\acute{e}r\sim$          |                 |                 |                                  |
| $\rho\lambda\xi$                      | $\eta\alpha\tau\epsilon$                       | $\delta i\alpha\beta\lambda$          | $\delta\sigma\kappa\omega\upsilon r$                            | $\phi\omega\kappa\alpha\rho\epsilon$ | $\phi\tau\mu$                          | $\gamma\omega\epsilon\tau$      | $\gamma\omega i\delta$    | $\mu\tau\omega\sigma$      | $i\eta\gamma\upsilon\epsilon$ | $\lambda i\sigma\epsilon\rho$ |                 |                 |                                  |
| $list\sim$                            | $litan\sim$                                    | $litt\sim$                            | $livr\mathbf{X}\sim$                                            | $louis\sim$                          | $message\sim$                          | $muet\sim$                      | $muf\sim$                 | $musi\sim$                 | $mutu\sim$                    | $ndit\acute{e}\mathbf{X}$     | $nom\sim$       | $\hat{o}\sim$   | $partag\sim$                     |
| $\lambda i\sigma\tau$                 | $\lambda i\tau\alpha\tilde{\nu}$               | $\lambda i\tau\tau$                   | $\lambda i\beta\rho$                                            | $\lambda u i\sigma$                  | $\mu\epsilon\beta\alpha\gamma\epsilon$ | $\mu\omega\upsilon\tau\tau$     | $m\acute{f}$              | $\mu\omega\sigma i$        | $m\tau\upsilon$               | $nd$                          | $\eta\omega\mu$ | $\omega\hat{o}$ | $\rho\alpha\rho\tau\alpha\gamma$ |
| $pr\acute{e}sen(c t)\sim$             | $quotidien\mathbf{X}$                          | $r\acute{e}cemment$                   | $r\acute{e}gim\sim$                                             | $r\acute{e}gion\sim$                 | $remerc\sim$                           | $rou(sse x)\sim$                | $salad\sim$               | $s\acute{e}r\sim$          |                               |                               |                 |                 |                                  |
| $pr\acute{e}\nu\tau$                  | $j\omega\upsilon r$                            | $r\acute{e}c\epsilon\tau$             | $\rho\epsilon\gamma\mu$                                         | $\epsilon\rho\gamma\tilde{\nu}$      | $\rho\mu\epsilon\rho\kappa$            | $r\omega\upsilon\gamma\epsilon$ | $s\alpha\lambda\delta$    | $\rho\sigma\epsilon\sigma$ |                               |                               |                 |                 |                                  |
| $sommet\sim$                          | $tableau$                                      | $taill$                               | $t\acute{e}m\acute{e}r\sim$                                     | $term\sim$                           | $triste\sim$                           | $trois\sim$                     | $uni(cit q)$              | $volt\sim$                 | $volu\sim$                    |                               |                 |                 |                                  |
| $\sigma\omega\mu\epsilon\tau$         | $\tau\alpha\beta\lambda\epsilon\alpha\upsilon$ | $tail$                                | $\tau\epsilon\mu\epsilon\rho$                                   | $ter\mu$                             | $tr i\sigma\tau\epsilon$               | $\acute{z}trois$                | $u\tilde{\nu}i\kappa$     | $\beta\omega\lambda\tau$   | $\omega\nu\omega\lambda$      |                               |                 |                 |                                  |
| $(\emptyset ma mes)dame(\emptyset s)$ | $(\emptyset ma mes)demoiselle(\emptyset s)$    | $bessie$                              | $hui$                                                           | $joyau(\emptyset x)$                 | $mlle(\emptyset s)$                    | $mme(\emptyset s)$              |                           |                            |                               |                               |                 |                 |                                  |
| $lady$                                | $mi\beta$                                      | $\beta\epsilon\sigma\theta i\epsilon$ | $\alpha\upsilon\eta\omega\upsilon r\delta$                      | $joaillerie$                         | $mi\beta$                              | $lady$                          |                           |                            |                               |                               |                 |                 |                                  |
| $nu(\emptyset e)(\emptyset s)$        | $rite(\emptyset s)$                            | $vie(\emptyset s)$                    | $\sim^{X\in(\mathbf{V}^*\mathbf{C}_{m_0}^*)}ement(\emptyset s)$ | $\sim an(ce t)$                      |                                        |                                 |                           |                            |                               |                               |                 |                 |                                  |
| $\tilde{\nu}u\delta\epsilon$          | $\rho i\tau$                                   | $v i\upsilon r\epsilon$               | $\mathbf{X}u$                                                   | $ants$                               |                                        |                                 |                           |                            |                               |                               |                 |                 |                                  |

(2) *Replace*

|                                                    |                                                 |                                         |                                  |                                         |                        |                           |                 |                                     |                                      |                   |
|----------------------------------------------------|-------------------------------------------------|-----------------------------------------|----------------------------------|-----------------------------------------|------------------------|---------------------------|-----------------|-------------------------------------|--------------------------------------|-------------------|
| $(maman matern m\acute{e}r\epsilon)\mathbf{X}\sim$ | $(meilleur mieux)\sim$                          | $\mathbf{C}^*y$                         |                                  |                                         |                        |                           |                 |                                     |                                      |                   |
| $\mu\alpha\mu\alpha$                               | $\mu\epsilon i\lambda\lambda\epsilon\upsilon r$ | $\mathbf{C}^*\eta$                      |                                  |                                         |                        |                           |                 |                                     |                                      |                   |
| $X^{\in}(\text{aper con per})cept\mathbf{X}\sim$   | $a^{X^{\in}}(cc ss tt)\sim$                     | $accr\acute{u}\mathbf{X}\sim$           | $accus\sim$                      | $ad\sim$                                | $aff\sim$              | $aim\sim$                 | $air\sim$       | $anv$                               | $avuncula i\mathbf{r}\mathbf{X}\sim$ |                   |
| $\mathbf{X}ce\upsilon$                             | $x\mathbf{X}^{[1]}$                             | $x\kappa r\omega i\sigma\sigma\omega s$ | $acc\upsilon\sigma$              | $z\delta$                               | $\varphi$              | $am\omega\upsilon r$      | $a i\mathbf{r}$ | $at\upsilon$                        | $\omega n\kappa\lambda\epsilon$      |                   |
| $bon(\emptyset n\acute{e})(\emptyset s)\sim$       | $cess\sim$                                      | $choi(s x)\sim$                         | $concl(u \acute{u})\sim$         | $courage\sim$                           | $ction$                | $dame\sim$                | $dat\sim$       | $d\acute{e}cept\mathbf{X}\sim$      | $d\acute{e}te\sim$                   | $d\acute{e}t\sim$ |
| $\mu\epsilon i\lambda\lambda\epsilon\upsilon r$    | $\xi\epsilon\sigma\sigma$                       | $ch\omega i\zeta$                       | $q\omega n\kappa\lambda\upsilon$ | $k\omega\upsilon r\alpha\gamma\epsilon$ | $ct i\upsilon\epsilon$ | $\delta\alpha\mu\epsilon$ | $dat$           | $d\epsilon\upsilon\epsilon\upsilon$ | $\delta\tau$                         | $d\epsilon\tau$   |

<sup>74</sup>We have chosen not to include the feminine forms of past participles (*allée, allées, venue, venues*) in the lists below, because their functions as nouns deviate from the original verbs. Similarly, when the present participles *allant* and *venant* are used as adjectives, their meanings no longer align perfectly with the respective verbs. Therefore, we do not include the feminine and plural forms of these adjectives (such as *allante* and *allants*) in our lists of verb forms.

<sup>75</sup>To avoid confusion of Greek nu with Latin vee, we write the former as  $\tilde{\nu}$  in substitution rules.



(3.3)  $Do(ion|ke|log|s|tif|y) \rightarrow \emptyset$ .<sup>76</sup>

(3.4)  $Do \sim \mathbf{V}_m^* \rightarrow \emptyset$ .

The result after these four steps of operations is called  $\hat{\sigma}'_2$ .

(3) Concatenate  $\hat{\sigma}'_1$  and  $\hat{\sigma}'_2$ .

(4) Perform the following replacements on  $\hat{\sigma}'_1 \hat{\sigma}'_2$ :

|                                            |                                                    |                                                                         |                                               |                                             |                                  |                             |                   |
|--------------------------------------------|----------------------------------------------------|-------------------------------------------------------------------------|-----------------------------------------------|---------------------------------------------|----------------------------------|-----------------------------|-------------------|
| $mo(\rho\tau w\rho)\mathbf{X}\sim$<br>mowp | $mow(dr l)\mathbf{X}\sim$<br>mowd                  | $dekh(err u(\emptyset s ss t))$<br>dekhoyr                              | $di(\emptyset r s ss t)$<br>dict              | $ekrif$<br>ekris                            | $kkows$<br>kkowd                 |                             |                   |
| $lu(\emptyset r s ss t)$<br>lis            | $p(ow(\emptyset frr t) u(\emptyset y ss))$<br>puss | $ri$<br>rir                                                             | $s(a(f kh w\rho y s y t) u)$<br>suss          | $v(is(\emptyset s))(\emptyset err)$<br>voyr |                                  |                             |                   |
| $va(wdr y ll)$<br>val                      | $vow(\emptyset dr t y ll)$<br>vowl                 | $xs(e(\emptyset y) i(\emptyset r s ss t) oy(\emptyset r s t))$<br>xsied |                                               |                                             |                                  |                             |                   |
| $\sim ce(ofw(\emptyset r s ss t))$<br>cef  | $\sim enferr$<br>enfoy                             | $\sim na(k y(\emptyset s t))$<br>nayss                                  | $\sim pr(i(\emptyset r s ss t) en)$<br>prendr | $\sim sol(\emptyset f)$<br>sowd             | $\sim ti(\emptyset en)$<br>tendr | $\sim v(en i ien)$<br>vendr | $\sim vek$<br>vif |

## 6.2.2 Admissible mutation and approximate clustering

Unlike the three representative Germanic languages and Spanish, we do not need vowel blotting for French, because vowel alternation is not found systematically in French verb conjugations.

In what follows, we will construct a bivariate Boolean-valued function  $\text{HrdTest}(\hat{\alpha}, \hat{\beta})$  on a “simple heredity test function” in Algorithm 6.17, and a set of “admissible suffix mismatch” rules in Algorithm 6.18.

**Algorithm 6.17** (Simple heredity test). *Let  $\hat{\alpha}'$  be the result from doing  $\sim(\emptyset|e)s \rightarrow \emptyset$  on  $\hat{\alpha}$ , and define  $\hat{\beta}'$  similarly. The Boolean-valued function  $\text{SimpHrdTest}(\hat{\alpha}, \hat{\beta})$  returns **TRUE** if the lowercase form of  $\hat{\alpha}$  contains at least one instance of  $\mathbf{V}^*$  (Definition 6.13) **AND** at least one of the following three conditions holds:<sup>77</sup>*

- (i)  $\hat{\alpha}' = \hat{\beta}'$ ;
- (ii) After doing  $\sim(d|f|fr|t) \rightarrow \emptyset$  on  $\hat{\beta}$ , we obtain  $\hat{\alpha}$ ;
- (iii)  $\ell(\hat{\beta}) > \ell(\hat{\alpha}) \geq \frac{\ell(\hat{\beta})}{2}$  **AND**  $\hat{\alpha} = \hat{\beta}^{\ell(\hat{\alpha})}$  **AND**  $\hat{\beta}^{\ell(\hat{\alpha}'+1)} = \mathbf{V}^*$ . (See Definition 3.1 for the notations  $\hat{\beta}^{[n]}$  and  $\hat{\beta}^{\{n\}}$ .)

In what follows, we define  $\text{SuffixNW}(\hat{\alpha}, \hat{\beta})$ ,  $\text{RootNW}(\hat{\alpha}, \hat{\beta})$ ,  $\text{NW}^*(\hat{\alpha}, \hat{\beta})$  and  $\text{SuffixSW}(\hat{\alpha}, \hat{\beta})$ ,  $\text{SuffixSW}(\hat{\alpha}, \hat{\beta})$ ,  $\text{SW}^*(\hat{\alpha}, \hat{\beta})$  as what is done in the Danish case (Algorithm 5.7), which was also applied to two other Germanic languages treated in §5.

**Algorithm 6.18** (Admissible suffix mismatch). *For two strings  $\hat{\alpha}$  and  $\hat{\beta}$ , the Boolean-valued function*

$$\text{AdmSM}(\text{RootNW}(\hat{\alpha}, \hat{\beta}), \text{SuffixNW}(\hat{\alpha}, \hat{\beta}), \text{NW}^*(\hat{\alpha}, \hat{\beta}))$$

returns **TRUE** if

$$\text{SuffixNW}(\hat{\alpha}, \hat{\beta}) = [(\emptyset|\mathbf{V}^*\mathbf{X}r|(m|r|s|t|y)\mathbf{X}|tif\mathbf{X}), (\emptyset|\mathbf{V}^*\mathbf{X}r|(m|r|s|t|y)\mathbf{X}|tif\mathbf{X})]$$

**AND**  $\text{NW}^*(\hat{\alpha}, \hat{\beta}) = \emptyset$  **AND**  $\text{RootNW}(\hat{\alpha}, \hat{\beta})$  contains at least one instance of  $\mathbf{V}^*$ .

Similarly, one can evaluate another Boolean-valued function

$$\text{AdmSM}(\text{RootSW}(\hat{\alpha}, \hat{\beta}), \text{SuffixSW}(\hat{\alpha}, \hat{\beta}), \text{SW}^*(\hat{\alpha}, \hat{\beta}))$$

by trading all the occurrences of **NW** in the statements above with **SW**.

**Algorithm 6.19** (Heredity test function). *The structure of the French heredity test function  $\text{HrdTest}(\hat{\alpha}, \hat{\beta})$  is identical to the German version (Algorithm 8.1.2), except that the functions  $\text{SimpHrdTest}$ ,  $\text{RootNW}$ ,  $\text{SuffixNW}$ ,  $\text{NW}^*$ ,  $\text{RootSW}$ ,  $\text{SuffixSW}$ ,  $\text{SW}^*$  must follow the French rules stated above.*

**Algorithm 6.20** (Approximate clustering of French words). *The algorithm is essentially the same as Algorithm 5.10, except that French rules (instead of Danish rules) apply to all the tags (effective spelling, essential root etc.), and vowel blotting is not used.*

Concretely speaking, the approximate clustering of a list of French words  $\{\hat{\alpha}_1, \dots, \hat{\alpha}_N\}$  is completed in two stages:

<sup>76</sup>We note that longer matches take priority over shorter matches: if *log* is found, then delete these three letters altogether, instead of just a single letter *g*.

<sup>77</sup>As a general rule in this document, the truth values of items labeled with Roman numerals are connected to each other with logical **OR**.



*paie, paient, paiera, paierai, paieraient, paierais, paierait, paieras, paieriez, paierions, paierons, paieront, paies, paya, payai, payaient, payais, payait, payâmes, payant, payas, payasse, payassent, payasses, payassiez, payassions, payât, payâtes, paye, payé, payent, payer, payera, payerai, payeraient, payerais, payerait, payeras, payèrent, payerez, payeriez, payerions, payerons, payeront, payes, payez, payiez, payions, payons* — “pay”;

*plaça, plaçai, plaçaient, plaçais, plaçait, plaçâmes, plaçant, plaças, plaçasse, plaçassent, plaçasses, plaçassiez, plaçassions, plaçât, plaçâtes, place, placé, placent, placer, placera, placerai, placeraient, placerais, placerait, placeras, placèrent, placerez, placeriez, placerions, placerons, placeront, places, placez, placiez, placions, plaçons* — “place”.

and obtain the following results:

{*aima, aimai, aimaient, aimais, aimait, aimâmes, aimant, aimas, aimasse, aimassent, aimasses, aimassiez, aimassions, aimât, aimâtes, aime, aimé, aiment, aimer, aimera, aimerai, aimeraient, aimerais, aimerait, aimeras, aimèrent, aimerez, aimeriez, aimerions, aimerons, aimeront, aimes, aimez, aimez, aimions, aimons*} ,

{*appela, appelle, appelaient, appelleis, appelleait, appelleâmes, appelant, appelas, appelleasse, appelleassent, appelleasses, appelleassiez, appelleassions, appelleât, appelleâtes, appelé, appeler, appelèrent, appelez, appelez, appellions, appelle, appellent, appellera, appellerai, appelleraient, appellerais, appellerait, appelleras, appellerez, appelleriez, appellerions, appellerons, appelleront, appelle, appellons*} ,

{*créa, créai, créaient, créais, créait, créâmes, créant, créas, créasse, créassent, créasses, créassiez, créassions, créât, créâtes, crée, créé, créent, créer, créera, créerai, créeraient, créerais, créerait, créeras, créèrent, créez, créeriez, créerions, créerons, créeront, créés, créez, créez, créions, créons*} ,

{*fini, finîmes, finir, finira, finirai, finiraient, finirais, finirait, finiras, finirent, finirez, finiriez, finirions, finirons, finiront, finis, finissaient, finissais, finissait, finissant, finisse, finissent, finisses, finissez, finissiez, finissions, finissons, finit, finît, finîtes*} ,

{*haï, haïmes, haïr, haïra, haïrai, haïraient, haïrais, haïrait, haïras, haïrent, haïrez, haïriez, haïrions, haïrons, haïront, hais, haïs, haïssaient, haïssais, haïssait, haïssant, haïsse, haïssent, haïsses, haïssiez, haïssions, haïssions, hait, haît, haïtes*} ,

{*mange, mangé, mangea, mangeai, mangeaient, mangeais, mangeait, mangeâmes, mangeant, mangeas, mangeasse, mangeassent, mangeasses, mangeassiez, mangeassions, mangeât, mangeâtes, mangent, mangeons, manger, mangera, mangerai, mangeraient, mangerais, mangerait, mangeras, mangèrent, mangez, mangeriez, mangerions, mangerons, mangeront, manges, mangez, mangiez, mangions*} ,

{*noie, noient, noiera, noierai, noieraient, noierais, noierait, noieras, noierez, noieriez, noierions, noierons, noieront, noies, noya, noyai, noyaient, noyais, noyait, noyâmes, noyant, noyas, noyasse, noyassent, noyasses, noyassiez, noyassions, noyât, noyâtes, noyé, noyer, noyèrent, noyez, noyiez, noyions, noyons*} ,

{*paie, paient, paiera, paierai, paieraient, paierais, paierait, paieras, paieriez, paierions, paierons, paieront, paies, paya, payai, payaient, payais, payait, payâmes, payant, payas, payasse, payassent, payasses, payassiez, payassions, payât, payâtes, paye, payé, payent, payer, payera, payerai, payeraient, payerais, payerait, payeras, payèrent, payerez, payeriez, payerions, payerons, payeront, payes, payez, payiez, payions, payons*} ,

{*plaça, plaçai, plaçaient, plaçais, plaçait, plaçâmes, plaçant, plaças, plaçasse, plaçassent, plaçasses, plaçassiez, plaçassions, plaçât, plaçâtes, place, placé, placent, placer, placera, placerai, placeraient, placerais, placerait, placeras, placèrent, placerez, placeriez, placerions, placerons, placeront, places, placez, placiez, placions, plaçons*} .

*Example 6.20.2.* Unlike Spanish, French verb conjugations do not exhibit systematic vowel alternations. In fact, the vowels in almost all French verb stems are invariant. There are a few dozen commonly used French verbs that are irregular in their own unique ways. They are treated by dedicated exceptions to rules in our clustering algorithm. Similar to the sampling of Spanish verbs, we ignore cases where the French verb root is different by at most a diacritic mark on the letter *e* (as both *é* and *è* will be converted to *e* in the effective spelling) in conjugated forms.

We use the following representative irregular verbs in French as our input:

*accrois, accroissaient, accroissais, accroissait, accroissant, accroisse, accroissent, accroisses, accroissez, accroissiez, accroissions, accroissons, accroît, accroîtra, accroîtrai, accroîtraient, accroîtrais, accroîtrait, accroîtras, accroître, accroîtrez, accroîtriez, accroîtrions, accroîtrons, accroîtront, accrû, accrûmes, accrûrent, accrûs, accrûsse, accrûssent, accrûsses, accrûssiez, accrûssions, accrût, accrûtes* — “increase”;





*moud, moudra, moudrai, moudraient, moudrais, moudrait, moudras, moudre, moudrez, moudriez, moudrions, moudrons, moudront, mouds, moulaient, moulais, moulait, moulant, moule, moulent, moules, moulez, mouliez, moulions, moulons, moulu, moulûmes, mouluent, moulus, moulusse, moulussent, moulusses, moulussiez, moulussions, moulut, moulût, moulûtes* — “grind” ;

*nais, naissaient, naissais, naissait, naissant, naisse, naissent, naisses, naissez, naissiez, naissions, naissons, naît, naîtra, naîtrai, naîtraient, naîtrais, naîtrait, naîtras, naître, naîtrez, naîtriez, naîtrions, naîtrons, naîtront, naquîmes, naquîrent, naquîs, naquîsse, naquîssent, naquîsses, naquîssiez, naquîssions, naquît, naquît, naquîtes, né* — “be born” ;

*nui, nuira, nuirai, nuiraient, nuirais, nuirait, nuiras, nuire, nuirez, nuiriez, nuirions, nuirons, nuiront, nuis, nuisaient, nuisais, nuisait, nuisant, nuise, nuisent, nuises, nuisez, nuisiez, nuisîmes, nuisions, nuisirent, nuisis, nuisisse, nuisissent, nuisisses, nuisissiez, nuisissions, nuisit, nuisît, nuisîtes, nuisons, nuit* — “spoil” ;

*offert, offraient, offrais, offrait, offrant, offre, offrent, offes, offrez, offiez, offîmes, offrions, offrir, offrira, offrirai, offriraient, offrirais, offrirait, offriras, offriront, offririez, offririez, offririons, offrirons, offriront, offris, offrîsse, offrissent, offrisses, offrissiez, offrissions, offrit, offrit, offrites, offrons* — “offer” ;

*peignaient, peignais, peignait, peignant, peigne, peignent, peignes, peignez, peigniez, peignîmes, peignons, peignirent, peignis, peignisse, peignissent, peignisses, peignissiez, peignissions, peignit, peignît, peignîtes, peignons, peindra, peindrai, peindraient, peindraîs, peindrait, peindras, peindre, peindrez, peindriez, peindrions, peindrons, peindront, peins, peint* — “paint” ;

*plaira, plairai, plairaient, plairais, plairait, plairas, plaire, plairez, plairiez, plairions, plairons, plairont, plais, plaisaient, plaisais, plaisait, plaisant, plaise, plaisent, plaies, plaisez, plaissiez, plaissions, plaions, plait, plaît, plu, plûmes, plurent, plus, plusse, plussent, plusses, plussiez, plussions, plut, plût, plûtes* — “please” ;

*prenaient, prenais, prenait, prenant, prend, prendra, prendrai, prendraient, prendrais, prendrait, prendras, prendre, prendrez, prendriez, prendrions, prendrons, prendront, prends, prenez, prenez, prenions, prenne, prennent, prennent, prenons, primes, prirent, pris, prisse, prissent, prisses, prissiez, prissions, prit, prît, prîtes* — “take” ;

*recevaient, recevais, recevait, recevant, recevez, receviez, recevions, recevoir, recevons, recevra, recevrai, recevraient, recevrais, recevrait, recevras, recevrez, recevriez, recevriers, recevrons, recevront, reçois, reçoit, reçoive, reçoivent, reçoives, reçu, reçûmes, reçurent, reçus, reçusse, reçussent, reçusses, reçussiez, reçussions, reçut, reçût, reçûtes* — “receive” ;

*riaient, riais, riait, riant, rie, rient, ries, riez, rîez, riions, rîmes, rions, rira, rirai, riraient, rirais, rirait, riras, rire, rirent, rirez, ririez, ririons, rirons, riront, ris, risse, rissent, risses, rissiez, rissions, rit, rît, rîtes* — “laugh” ;

*sachant, sache, sachent, saches, sachez, sachiez, sachions, sachons, sais, sait, saura, saurai, sauraient, saurais, saurait, sauras, saurez, sauriez, saurions, saurons, sauront, savaient, savais, savait, savent, savez, saviez, savions, savoir, savons, su, sûmes, surent, sus, susse, sussent, susses, sussiez, sussions, sut, sût, sûtes* — “know” ;

*suffi, suffîmes, suffira, suffirai, suffiraient, suffirais, suffirait, suffiras, suffire, suffirent, suffirez, suffiriez, suffirions, suffirons, suffiront, suffis, suffisaient, suffisais, suffisait, suffisant, suffise, suffisent, suffises, suffisez, suffissiez, suffissions, suffisons, suffisse, suffissent, suffisses, suffissiez, suffissions, suffit, suffit, suffîtes* — “suffice” ;

*traie, traient, traies, traïra, traïrai, traïraient, traïrais, traïrait, traïras, traïre, traïrez, traïriez, traïrions, traïrons, traïront, trais, trait, traya, trayai, trayaient, trayais, trayait, trayâmes, trayant, trayas, trayasse, trayassent, trayasses, trayassiez, trayassions, trayât, trayâtes, trayèrent, trayez, trayiez, trayions, trayons* — “milk” ;

*vaille, vaillent, vailles, valaient, valais, valait, valant, valent, valez, valiez, valions, valoir, valons, valu, valûmes, valurent, valus, valusse, valussent, valusses, valussiez, valussions, valut, valût, valûtes, vaudra, vaudrai, vaudraient, vaudrais, vaudrait, vaudras, vaudrez, vaudriez, vaudrions, vaudrons, vaudront, vaut, vaux* — “earn” ;

*vainc, vaincra, vaincrai, vaincraient, vaincrais, vaincrait, vaincras, vaincre, vaincrez, vaincriez, vaincrons, vaincrons, vaincront, vaincs, vaincu, vainquaient, vainquais, vainquait, vainquant, vainque, vainquent, vainques, vainquez, vainquiez, vainquîmes, vainquions, vainquirent, vainquis, vainquîsse, vainquissent, vainquisses, vainquissiez, vainquissions, vainquit, vainquît, vainquîtes, vainquons* — “win” ;

*vécu, vécûmes, vécurent, vécus, vécusse, vécussent, vécusses, vécussiez, vécussions, vécut, vécût, vécûtes, vis, vit, vivaient, vivais, vivait, vivant, vive, vivent, vives, vivez, viviez, vivions, vivons, vivra, vivrai, vivraient, vivrais, vivrait, vivras, vivre, vivez, vivriez, vivrions, vivrons, vivront* — “live” ;







{*vaille, vailent, vailles, valaient, valais, valait, valant, valent, valez, valiez, valions, valoir, valons, valu, valûmes, valurent, valus, valusse, valussent, valusses, valussiez, valussions, valut, valût, valûtes, vaudra, vaudrai, vaudraient, vaudrais, vaudrait, vaudras, vaudrez, vaudriez, vaudrions, vaudrons, vaudront, vaut, vaux*},

{*vainc, vaincra, vaincrai, vaincraient, vaincrais, vaincrait, vaincras, vaincre, vaincrez, vaincriez, vaincrions, vaincrons, vaincront, vaincs, vaincu, vainquaient, vainquais, vainquait, vainquant, vainque, vainquent, vainques, vainquez, vainquiez, vainquûmes, vainquions, vainquirent, vainquis, vainquisse, vainquissent, vainquisses, vainquissiez, vainquissions, vainquit, vainquît, vainquîtes, vainquons*},

{*vécu, vécûmes, vécurent, vécus, vécusse, vécussent, vécusses, vécussiez, vécussions, vécut, vécût, vécûtes, vivaient, vivais, vivait, vivant, vive, vivent, vives, vivez, viviez, vivions, vivons, vivra, vivrai, vivraient, vivrais, vivrait, vivras, vivre, vivrez, vivriez, vivrions, vivrons, vivront*},

{*vêt, vêtaient, vêtai, vêtait, vêtant, vête, vêtent, vêtes, vêtez, vêtiez, vêtîmes, vêtions, vêtir, vêtira, vêtirai, vêtiraient, vêtirais, vêtirait, vêtiras, vêtirent, vêtirez, vêtiriez, vêtirions, vêtirons, vêtiront, vêtis, vêtisse, vêtissent, vêtisses, vêtissiez, vêtissions, vêtit, vêtît, vêtîtes, vêtions, vêts, vêtû*},

{*veuille, veuillent, veuilles, veulent, veut, veux, voudra, voudrai, voudraient, voudrais, voudrait, voudras, voudrez, voudriez, voudrions, voudrons, voudront, voulaient, voulais, voulait, voulant, voulez, vouliez, voulions, vouloir, voulons, voulu, voulûmes, voulurent, voulus, voulusse, voulussent, voulusses, voulussiez, voulussions, voulut, voulût, voulûtes*},

{*vis, vit*},

Here, some verb conjugations are not clustered as expected, because we want to accommodate to inherent ambiguities of certain French verb forms. For example, both *vis* and *vit* may be conjugated forms of *vivre* “live” or *voir* “see”, and the infinitive form of *plu* may be either *plaire* “please” or *pleuvoir* “rain”.

*Example 6.20.3.* In [1, Figs. 3c, 6] and Fig. S8, we further apply the aforementioned word clustering algorithm to topic extraction and machine translation (see Table S1 for text sources).

It should be noted that the performance of machine translation is affected by polysemy of certain commonly occurring French words. For example, *livre* “book, pound” and *livres* “books, pounds” can also be conjugated forms of the verb *livrer* “deliver”. Furthermore, a word in English may correspond to a phrase in French, such as *jeune fille* “girl” (in contrast with *fille* “daughter”). This explains why our algorithm does not identify French translations for such common words like “girl” and “daughter”.

Topicality (non-Poissonian behavior) plays an essential rôle in our algorithms. If a word pattern generates a significantly non-Poissonian trajectory, then it will have distinguishing features in its time structure ([1, Figs. 3c, 6] and Fig. S8c), which allow better semantic resolution than nearly Poissonian trajectories (Fig. S8b and Fig. S8d). The recurrence kinetics of non-topics are very close to single exponential decays, so the vector embedding of recurrence eigenvalues ([1, Figs. 3c, 6] and Fig. S8c) will not help here.

In French, “bat” (a kind of flying mammal) is called *chauve-souris* (literally “bald mouse”), so we consider *bat* an exact match to *chauve* “bald” in Fig. S8b”. (Also note that the row for *bat* in Fig. S8b” indeed contains two hot spots, one for *chauve* and one for *souris*.) In Darwin’s *Origin of Species*, the adjective *fresh* is mostly used in the context of *fresh water*, which is *eau douce* in French. Therefore, we consider *fresh* an exact match to *douce* (meaning “sweet” in general) in Fig. S8b”.

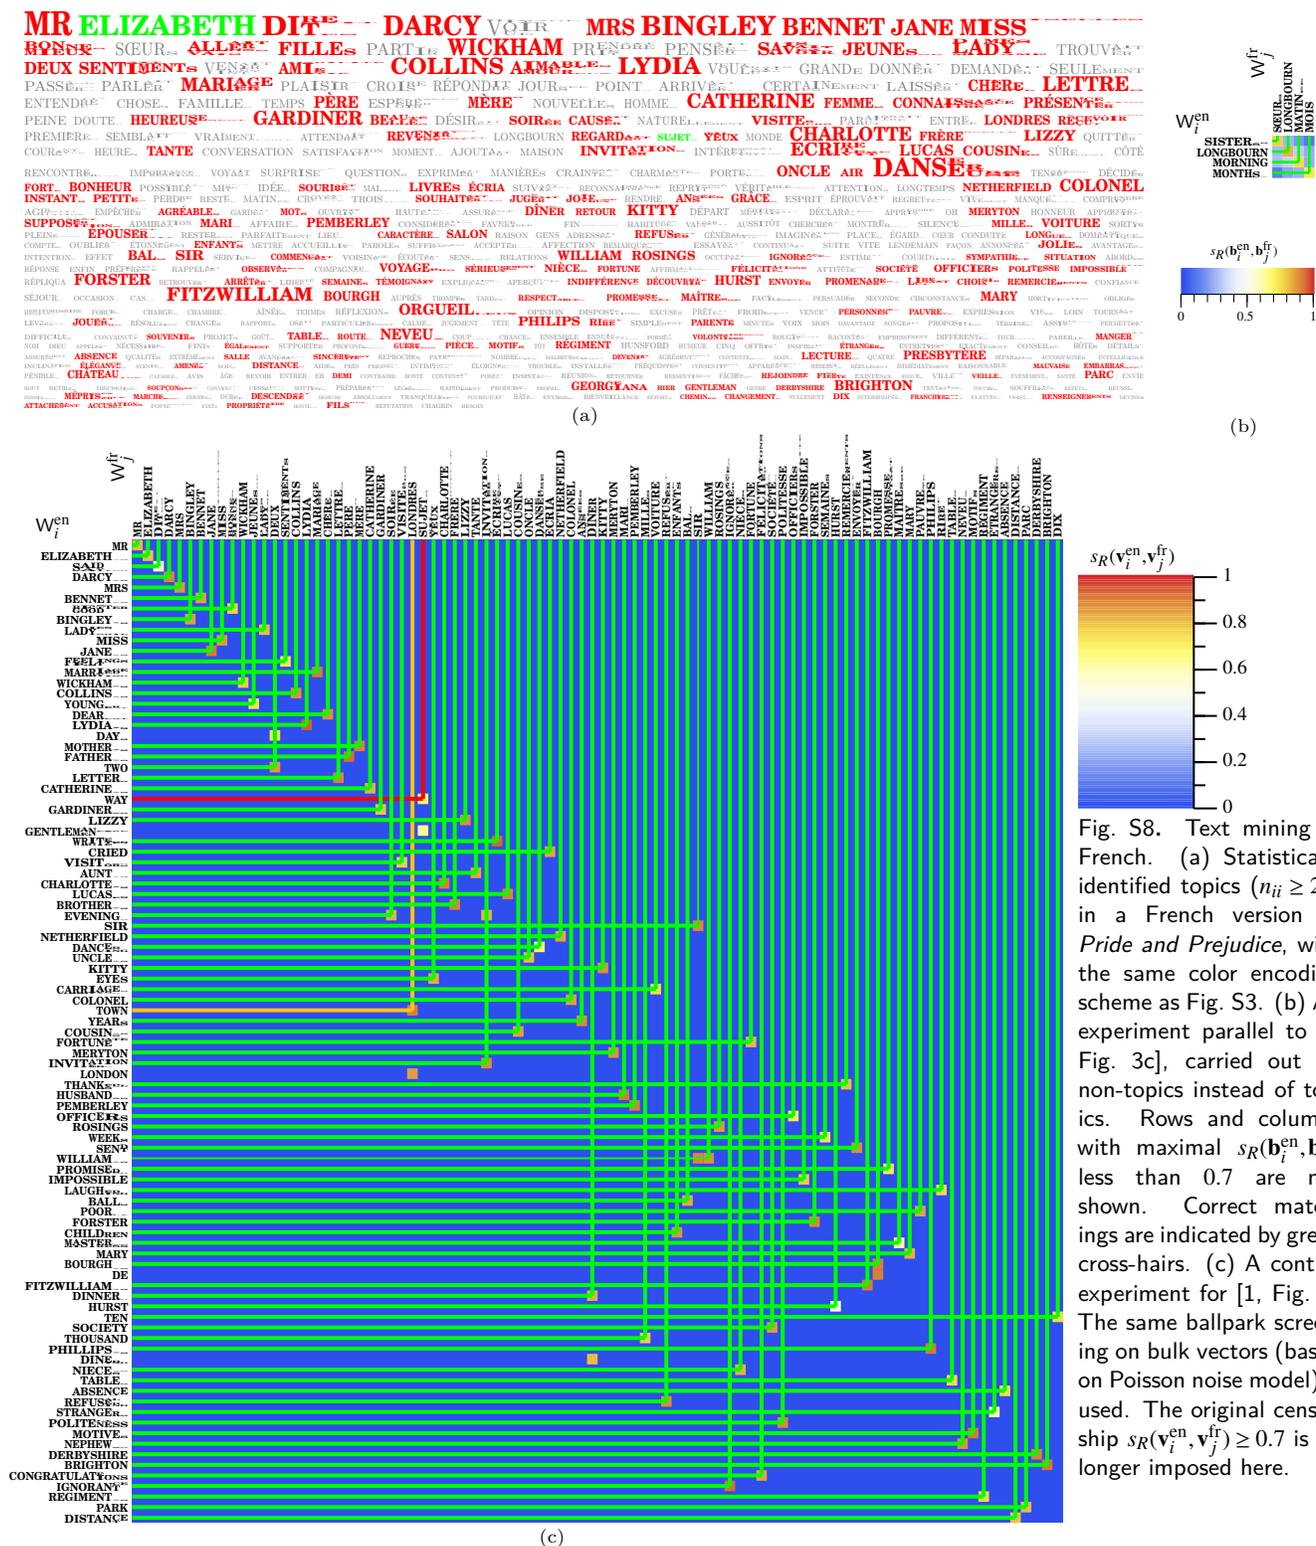

Fig. S8. Text mining in French. (a) Statistically identified topics ( $n_{ii} \geq 20$ ) in a French version of *Pride and Prejudice*, with the same color encoding scheme as Fig. S3. (b) An experiment parallel to [1, Fig. 3c], carried out on non-topics instead of topics. Rows and columns with maximal  $s_R(\mathbf{b}_i^{\text{en}}, \mathbf{b}_j^{\text{fr}})$  less than 0.7 are not shown. Correct matchings are indicated by green cross-hairs. (c) A control experiment for [1, Fig. 6]. The same ballpark screening on bulk vectors (based on Poisson noise model) is used. The original censorship  $s_R(\mathbf{v}_i^{\text{en}}, \mathbf{v}_j^{\text{fr}}) \geq 0.7$  is no longer imposed here.

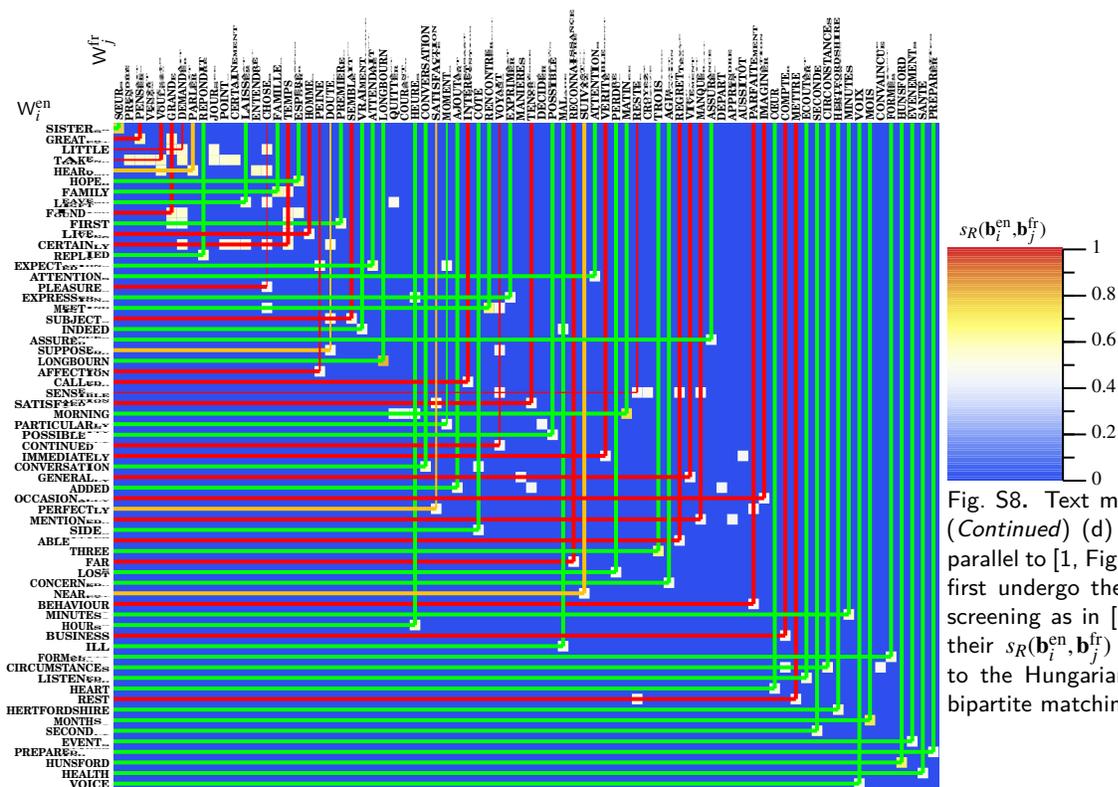

(d)

Fig. S8. Text mining in French. (Continued) (d) An experiment parallel to [1, Fig. 6]. Non-topics first undergo the same ballpark screening as in [1, Fig. 6], then their  $s_R(\mathbf{b}_i^{\text{en}}, \mathbf{b}_j^{\text{fr}})$  scores are sent to the Hungarian algorithm for bipartite matching.





### 6.3 Modified Porter stemming algorithm for Latin

**Definition 6.21** (Latin stop words). If a word belongs to the following list<sup>79</sup>:

*a, ab, abhinc, absque, abusque, ac, acta, actu, actum, acturus, actus, ad, adaeque, adhuc, adusque, adversum, adversus, agam, agamini, agamur, agamus, agant, agantur, agar, agare, agaris, agas, agat, agatis, agatur, age, agebam, agebamini, agebamur, agebamus, agebant, agebantur, agebar, agebare, agebaris, agebas, agebat, agebatis, agebatur, agemini, agemur, agemus, agendi, agendo, agendum, agendus, agens, agent, agentur, agere, agerem, ageremini, ageremur, ageremus, agerent, agerentur, agerer, agerere, agereris, ageres, ageret, ageretis, ageretur, ageris, ages, aget, agetis, agetur, agi, agimini, agimur, agimus, agis, agit, agite, agitis, agito, agitor, agitote, agitur, ago, agor, agunt, agunto, aguntor, aguntur, alia, aliae, aliam, aliarum, alias, alicui, alicuius, alicujus, alie, alii, aliis, alio, aliorum, alios, aliquae, aliquando, aliquantum, aliquarum, aliquas, aliquem, aliqui, aliquibus, aliquid, aliquis, aliquo, aliquorum, aliquos, aliquot, aliquotiens, aliter, aliud, alium, alius, alter, altera, alterae, alteram, alterarum, alteras, alteri, alteris, alterius, altero, alterorum, alteros, alterum, an, ante, antea, apud, at, atque, atorque, aut, autem, caetera, caetera, caeterae, caeterae, caeteram, caeteram, caeterarum, caeterarum, caeteras, caeteras, caetere, caetere, caeteri, caeteri, caeteris, caeteris, caetero, caetero, caeterorum, caeterorum, caeteros, caeteros, caeterum, caeterum, caeterus, caeterus, causa, cetera, ceterae, ceterae, ceteram, ceterarum, ceteras, ceteras, ceteri, ceteri, ceteris, ceteris, cetero, cetero, ceterorum, ceterorum, ceteros, ceteros, ceterum, ceterum, ceterus, ceterus, circa, circum, cis, citra, com, concoque, contorque, contra, coque, coram, cui, cuidam, cuiquam, cuique, cuius, cuiusdam, cuiusquam, cuiusque, cuiusvis, cuiusvis, cum, cur, de, decoque, dein, deinde, denique, denuo, deque, detorque, dum, e, ea, eadem, eae, eaedem, eam, eandem, earum, earundem, eadem, ecquando, egeram, egeramus, egerant, egeras, egerat, egeratis, egere, egerim, egerimus, egerint, egeris, egerit, egeritis, egero, egerunt, egi, egimus, egisse, egissem, egissemus, egissent, egisses, egisset, egissetis, egisti, egistis, egit, ego, ei, eidem, eis, eisdem, eius, eiusdem, ejus, ejusdem, en, enim, eo, eodem, eorum, eorundem, eos, eosdem, eram, eramus, erant, eras, erat, eratis, ere, erga, ergo, erimus, eris, erit, eritis, ero, erunt, es, esse, essem, essemus, essent, esses, esset, essetis, est, este, estis, esto, estote, et, etiam, etiamsi, etsi, eum, eundem, ex, excoque, extorque, extra, fac, face, facere, facerem, faceremus, facerent, faceres, faceret, faceretis, faciam, faciamus, faciant, facias, faciat, faciatis, faciebam, faciebamur, faciebant, faciebas, faciebat, faciebatis, faciemus, faciendi, faciendo, faciendum, faciendus, faciens, facient, facies, faciet, facietis, facimus, facio, facis, facit, facite, facitis, facito, facitote, faciunt, faciunt, facta, factae, factam, factarum, factas, facte, facti, factis, factio, factorum, factos, factu, factum, facturus, factus, feceram, feceramur, fecerant, feceras, fecerat, feceratis, fecere, fecerim, fecerimus, fecerint, feceris, fecerit, feceritis, fecero, fecerunt, feci, fecimus, fecisse, fecissem, fecissemus, fecissent, fecisses, fecisset, fecissetis, fecisti, fecistis, fecit, fi, fiam, fiamus, fiant, fias, fiat, fiat, fiat, fiamus, fiebam, fiebamur, fiebant, fiebas, fiebat, fiebatis, fiamus, fiendi, fiendo, fiendum, fient, fierem, fieremus, fierent, fieres, fieret, fieretis, fieri, fies, fiet, fietis, fimus, fio, fis, fit, fite, fitis, fito, fitote, fiunt, fiunt, fore, forem, foremus, forent, fores, foret, foretis, forms, forsan, forsitan, fortasse, fortassis, frequenter, frequentissime, frequentius, fueram, fueramus, fuerant, fueras, fuerat, fueratis, fuere, fuerim, fuerimus, fuerint, fueris, fuerit, fueritis, fuero, fuerunt, fui, fuimus, fuisse, fuissem, fuissemus, fuissent, fuisses, fuisset, fuissetis, fuisti, fuistis, fuit, futura, futurae, futuram, futurarum, futuras, future, futuri, futuris, futuro, futurorum, futuros, futurum, futurus, habe, habeam, habeamini, habeamur, habeamus, habeant, habeantur, habear, habere, habearis, habeas, habeat, habeatis, habeatur, habebam, habebamini, habebamur, habebamus, habebant, habebantur, habebat, habebare, habebaris, habebas, habebat, habebatis, habebatur, habebere, habeberis, habebimini, habebimus, habebis, habebit, habebitis, habebitur, habebo, habebor, habebunt, habebuntur, habemini, habemur, habemus, habenda, habendae, habendam, habendarum, habendas, habende, habendi, habendis, habendo, habendorum, habendos, habendum, habendus, habens, habent, habente, habentem, habentes, habenti, habentia, habentibus, habentis, habentium, habento, habentor, habentur, habeo, habeor, habere, haberem, haberemini, haberemur, haberemus, haberent, haberentur, haberer, haberere, habereris, haberes, haberet, haberetis, haberetur, haberi, haberier, haberis, habes, habet, habete, habetis, habeto, habetor, habetote, habetur, habita, habitae, habitam, habitarum, habitas, habite, habiti, habitis, habito, habitorum, habitos, habitu, habitum, habitura, habiturae, habituram, habiturorum, habituras, habiture, habituri, habituris, habituro, habiturorum, habituros, habiturum, habiturus, habitus, habueram, habueramus, habuerant, habueras, habuerat, habueratis, habuere, habuerim, habuerimus, habuerint, habueris, habuerit, habueritis, habuero, habuerunt, habui, habuimus, habuisse, habuissem, habuissemus, habuissent, habuisses, habuisset, habuissetis, habuisti, habuistis, habuit, hac, hae, haec, hanc, harum, has, haud, hi, hic, hinc, his, hoc, horum, hos, huc, huic, huius, hujus, hunc, iam, ibi, id, idem, igitur, iis, illa, illae, illam, illarum, illas, ille, illi, illis, illius, illo, illorum, illos, illud, illum, immo, in, incoque, inde, infra, infrequenter,*

<sup>79</sup>Our list of Latin stop words is based on [https://wiki.digitalclassicist.org/Stopwords\\_for\\_Greek\\_and\\_Latin](https://wiki.digitalclassicist.org/Stopwords_for_Greek_and_Latin) and <http://snowball.tartarus.org/otherapps/schinke/intro.html>, with extensive additions to roughly match their counterparts in English. In particular, we have included all the conjugated forms of *faciō* “make”, *fiō* “become”, *sum* “be” and *possum* “can”. It is worth noting that the conjugation tables for *faciō* and *fiō* partially overlap.



*super, supra, susque, suum, suus, tale, talem, tales, tali, talia, talibus, talis, talium, tam, tamen, tametsi, tandem, tanta, tantae, tantam, tantarum, tantas, tante, tanti, tantis, tanto, tantorum, tantos, tantum, tantus, te, tecum, tenus, tibi, torque, tot, tota, totae, totam, totarum, totas, tote, toti, totis, totius, toto, totorum, totos, totum, totus, trans, tu, tua, tuae, tuam, tuarum, tuas, tue, tui, tuis, tum, tuo, tuorum, tuos, tuum, tuus, ubi, ubicumque, ubinam, ubique, ubiubi, uel, uero, ultra, umquam, una, unae, unam, unarum, unas, unde, undique, une, uni, unis, unius, uno, unorum, unos, unquam, unum, unus, usquam, usque, ut, uter, uterque, utique, utra, utrae, utram, utrarum, utras, utri, utribique, utris, utrius, utro, utroque, utrorum, utros, utrum, valde, vel, versum, versus, vester, vestra, vestrae, vestram, vestrarum, vestras, vestri, vestris, vestro, vestrorum, vestros, vestrum, vix, vobis, vobiscum, vos, voster,*

or is spelt as a word from the list above, followed by suffix *que*, then we consider it a Latin stop word. All the Latin stop words that appear in a particular document need to be ignored before we perform word clustering on the rest of the vocabulary list.  $\square$

Similar to what we did in the algorithm for French, we need to define string patterns **goLatin**, **goodLatin**, **betterLatin**, **bestLatin** to cover some irregular inflections:

*eam, eamus, eant, eas, eat, eatis, eatur, eo, eundi, eundo, eundum, eundus, eunt, eunto, i, ibam, ibamus, ibant, ibas, ibat, ibatis, ibatur, ibimus, ibis, ibit, ibitis, ibitur, ibo, ibunt, iens, ieram, ieramus, ierant, ieras, ierat, ieratis, iere, ierim, ierimus, ierint, ieris, ierit, ieritis, iero, ierunt, ii, iimus, iit, imus, ire, irem, iremus, irent, ires, iret, iretis, iretur, iri, is, isse, issem, issemus, issent, isses, isset, issetis, isti, istis, it, ite, itis, ito, itote, itu, itum, itur, iturus, itus, ivi, ivisti, ivit* — “go”;

*bona, bonae, bonam, bonarum, bonas, bone, boni, bonis, bono, bonorum, bonos, bonum, bonus* — “good”;

*melior, meliora, meliore, meliorem, meliores, meliori, melioribus, melioris, meliorum, melius* — “better”;

*optima, optimae, optimam, optimarum, optimas, optime, optimi, optimis, optimo, optimorum, optimos, optimum, optimus, optuma, optumae, optumam, optumarum, optimas, optume, optumi, optimis, optimo, optimorum, optumos, optimum, optumus* — “best”.

However, we are not going to treat these strings as stop words<sup>80</sup>, so as to be consistent with their counterparts in other languages.

### 6.3.1 Effective spelling and essential root

**Definition 6.22** (Latin Vowel Extensions). Hereafter in §6.3, the symbol  $\mathbf{V}^*$  stands for any member from the list  $\{a, e, i, o, u, y\}$ , the so-called Latin vowel extensions. In line with the multiplicity notations introduced in Definition 3.3, the symbol  $\mathbf{V}_m^*$  stands for a text string formed by consecutive appearance of one or more (not necessarily identical or distinct) members from the set of Latin vowel extensions.

Dual to the notations above, the symbol  $\mathbf{C}^*$  stands for any character that does not belong to the list  $\{a, e, i, o, u, y\}$ , and  $\mathbf{C}_{m_0}^*$  stands for a text string formed by consecutive appearance of zero or more (not necessarily identical or distinct) characters that do not belong to the same list.  $\square$

**Definition 6.23** (Latin protected range). Let  $\hat{\sigma}$  be a text string derived from a Latin word, its protected range  $\text{ProtRg}(\hat{\sigma})$  is an integer determined as follows:

- Try to find the string pattern  $(\emptyset|a(b|d|mb)|circum|co(m|\mu|n|rr)|de(f|l|t)|i|jnter|o(b|f)|per|pr(ae|e|o)|re|su|tran)\mathbf{C}_{m_0}^*\mathbf{V}^*\mathbf{C}_{m_0}^*\sim$  in the string  $\hat{\sigma}$ ;
- If the string pattern above is found, the last position occupied by such a string defines  $\text{ProtRg}(\hat{\sigma})$ ; otherwise, set  $\text{ProtRg}(\hat{\sigma}) = 0$ .  $\square$

**Algorithm 6.24** (Latin effective spelling). For a Latin word  $\hat{\sigma}$ , its effective spelling  $\text{EffSpell}(\hat{\sigma})$  is constructed in sequential steps:

- (1)  $Do^{\text{81}} \bar{a} \rightarrow a, \bar{ae} \rightarrow ae, \bar{e} \rightarrow e, \bar{i} \rightarrow i, \bar{o} \rightarrow o, \bar{ae} \rightarrow oe, \bar{u} \rightarrow u, \bar{y} \rightarrow y$ .
- (2) Do *carolin* $\sim \rightarrow \kappa\alpha\text{p}\text{o}\text{l}\text{i}\text{v}$ , *emi(s|s|t|tt)*  $\rightarrow \varepsilon\mu\text{i}\sigma$ , *impr* $\sim \rightarrow \text{mpp}$ , *pass*  $\rightarrow \text{pand}$ , *pater* $\sim \rightarrow \text{patre}$ , *separ* $\sim \rightarrow \sigma\text{e}\text{t}\alpha\text{p}$ , *vac*  $\rightarrow \beta\text{e}\alpha\text{c}$ .

<sup>80</sup>Nevertheless, we have included *eam, eo, is, iste* and *istis* in our list of Latin stop words, because they not only function as conjugated forms of the Latin verb for “to go”, but also as pronouns.

<sup>81</sup>Note that the italic forms of  $\bar{ae}$  ( $\bar{a}$ ) and  $\bar{e}$  ( $\bar{e}$ ) are very similar.

## (3) Replace

|                                                             |                                              |                                                       |                       |                         |                      |                         |                      |                              |                  |                |                 |             |                 |
|-------------------------------------------------------------|----------------------------------------------|-------------------------------------------------------|-----------------------|-------------------------|----------------------|-------------------------|----------------------|------------------------------|------------------|----------------|-----------------|-------------|-----------------|
| $(\emptyset con)sobrinX$<br>κουσῖ                           | $(\emptyset cu)cur^{X\epsilon}(r s)$<br>kurX | $(ami materer)^{X\epsilon}(a e i o u y)\sim$<br>αυῖτX |                       |                         |                      | $(m p)atruelX$<br>κουσῖ |                      |                              |                  |                |                 |             |                 |
| aestim~<br>αστιμ                                            | ami(s t)(\emptyset s)~<br>αμισ               | amicissX~<br>amica                                    | asp~<br>αspa          | camer~<br>ριμ           | car(a i o)~<br>δεαρι | collin~<br>κολλιῖ       | color~<br>φαρβρ      | delect~<br>δλιγτ             | dign~<br>διγν    |                |                 |             |                 |
| divid~<br>diviδ                                             | divin~<br>divῖ                               | er(ect ex ig)~<br>ερεξῖτ                              | fem(ell in)~<br>φεμλν | haer~<br>ηαερ           | here(d s)~<br>ηειρ   | hestern~<br>ηεστ        | honest~<br>ηονεστ    | horta~<br>ηορτα              |                  |                |                 |             |                 |
| hr~<br>μωστερ                                               | ingenu~<br>ινγεῖνυ                           | laet~<br>χαπτ                                         | lisul~<br>λιζζ        | locut<br>λλοquor        | loq<br>λλοq          | lucas~<br>λυξσ          | marit~<br>μαρτ       | materi~<br>ματρι             | matron~<br>λαδη  | matur~<br>μτυρ | matut~<br>ματιῖ |             |                 |
| memin~<br>μῖν                                               | met~<br>φεαρ                                 | mra~<br>μρσα                                          | nupt~<br>ῖνυπτ        | opin~<br>ωπιν           | pact~<br>παγγ        | pag~<br>παγ             | pet~<br>πετ          | pig~<br>πιγ                  | rheda~<br>ωογῖνα | saltX~<br>δαῖσ | salut~<br>σαλυτ | san~<br>σαῖ | sapien~<br>ωισπ |
| scri(b ps pt)~<br>ωπιτρ                                     | senior~<br>σγῖορ                             | sign~<br>σιγν                                         | soror~<br>σορορ       | tem~<br>τμε             | van~<br>βαῖ          | ven(a o)~<br>νεῖνα      | vene(m t)~<br>νεῖνατ | vidu~<br>βιδο                |                  |                |                 |             |                 |
| $d(e e i i s o o orum os um us)i(\emptyset i i s s)$<br>γoδ |                                              | $amic(i u)(\emptyset m s)$<br>amica                   |                       | $car(e um us)$<br>δεαρι |                      | die<br>diebus           | heri<br>ηεστ         | vener(\emptyset e)<br>νεῖνατ |                  |                |                 |             |                 |

## (4) Replace

|                                                                                                |                                                                                                     |                           |                      |                                       |                                                    |                         |                            |                       |              |
|------------------------------------------------------------------------------------------------|-----------------------------------------------------------------------------------------------------|---------------------------|----------------------|---------------------------------------|----------------------------------------------------|-------------------------|----------------------------|-----------------------|--------------|
| δεαπιλ<br>καρλ                                                                                 | χῖtri(c x)<br>χῖτορ                                                                                 | a(dfer lat tul)~<br>affer | ab(lat tul)~<br>aufe | amic(i(a e m r te to) u t)~<br>αμβιcu |                                                    |                         |                            |                       |              |
| bib~<br>βιβ                                                                                    | co(lla ntul)~<br>confer                                                                             | complement<br>compler     | concors<br>concord   | creat~<br>crear                       | dea~<br>δεαυ                                       | di(lat stul)~<br>differ | diurn~<br>δι               |                       |              |
| domin(a)~<br>δομῖνο                                                                            | domina~<br>δομῖναα                                                                                  | e(lat x tul)~<br>effe     | expos~<br>expon      | filia~<br>φιλαα                       | hort~<br>γαρδτ                                     | ira(sc t)~<br>ιρ        | latrin~<br>λαβ             | matrimon~<br>ματριμον |              |
| memor~<br>μεμ                                                                                  | mens <sup>Xε</sup> (a e i o u y)~<br>μενσX                                                          | ob(lat tul)~<br>offer     | onerosX~<br>oneris   | patrimon~<br>πατριμον                 | patru <sub>χ</sub> (m)X~<br>αβυγκυλυς              | pin(g x)~<br>πικτ       | reg~<br>ρεγ                |                       |              |
| sci(am ar eb em en es et m o re r sc t un v)X<br>sci                                           |                                                                                                     |                           |                      | str<br>starr                          | su(blat stul)~<br>suffer                           |                         | terter<br>τερτερ           |                       |              |
| truculentX~<br>τρυκυμ                                                                          | tutel~<br>τυταρ                                                                                     | us(i u)~<br>υτο           | via~<br>βιαα         | xt<br>x                               | <b>(bestLatin betterLatin goodLatin)</b><br>λγoοδλ |                         |                            |                       |              |
| $X\epsilon(\emptyset ab ad amb circum co de in inter ob prod red suss trans)goLatin$<br>Xλγoολ |                                                                                                     |                           |                      |                                       |                                                    |                         |                            |                       |              |
| cor<br>κορδισ                                                                                  | $d(ee ei eis eo eorum eos eum eus ia iae iam iarum ias ie ii iis io iorum ios is ium ius)$<br>divus |                           |                      |                                       |                                                    |                         |                            |                       |              |
| lux<br>λυκυμ                                                                                   | mens<br>μεντις                                                                                      | mos<br>μορις              | nix<br>νιβις         | ops<br>οπυμ                           | re<br>ρεβυς                                        | trux<br>τρυκυμ          | vi(\emptyset m)<br>βιριβυς | ~que<br>'que          | ~scis<br>sci |

(5) Do  $a^{X\epsilon}(cc|dd|ff|gg|rr|ss|tt)\sim \rightarrow \alpha X$ ,  $x \rightarrow \check{c}$ .

## (6) Replace

|                             |                                        |                                                |                   |                |                  |                              |               |           |                    |                |            |                   |                |
|-----------------------------|----------------------------------------|------------------------------------------------|-------------------|----------------|------------------|------------------------------|---------------|-----------|--------------------|----------------|------------|-------------------|----------------|
| $\hat{x}\notin(m)om$<br>χoμ | $X\epsilon(a e i o r u y)p(s t)$<br>Xp | $X\epsilon(\hat{x}(a e i o r u y))r$<br>Xerque | cantor~<br>κανερε | dele~<br>ddele |                  |                              |               |           |                    |                |            |                   |                |
| mpt<br>m                    | osχ<br>οσχ                             | patr~<br>πατρ                                  | puls<br>πελλ      | tang~<br>τακτ  | tarrid<br>ταρριζ | tr <sub>χ</sub> (a)~<br>τερχ | trah<br>τρακτ | ult<br>ολ | ire(m mus s)<br>εο | pater<br>πατερ | vis<br>βολ | ~emen(dX s)<br>εμ | ~starr<br>σταρ |

(7) Do  $\sim rs \rightarrow rt$ ,  $\sim \hat{x}\epsilon(a|e|i|o|r|t|u)er \rightarrow \hat{x}erquei$ ,  $inter\sim \rightarrow jnter$ ,  $super\sim \rightarrow suzp$ .(8) Remove apostrophe, and call the string obtained so far as  $\hat{\sigma}_\#$ .

- (9) Break down  $\hat{\sigma}_{\#} = \hat{\sigma}_1\hat{\sigma}_2$  into the concatenation of two strings  $\hat{\sigma}_1 = \hat{\sigma}_{\#}^{[\text{ProtRg}(\hat{\sigma}_{\#})]}$  (see the notation in Definition 3.1) and  $\hat{\sigma}_2$ , where the length of the first string  $\ell(\hat{\sigma}_1) = \text{ProtRg}(\hat{\sigma}_{\#})$  is equal to the protected range of  $\hat{\sigma}_{\#}$ .
- (10) Do  $act \rightarrow ag$ ,  $erb \rightarrow erv$ ,  $eg\sim \rightarrow ag$ ,  $X^{\epsilon}(i|o|u)v \rightarrow \mathbf{X}t$ ,  $ub \rightarrow uss$  on  $\hat{\sigma}_1$  and call the result  $\hat{\sigma}'_1$ .
- (11) Do  $\sim que \rightarrow 'que$  on  $\hat{\sigma}_2$  and call the result  $\hat{\sigma}'_2$ .
- (12) If the pattern  $\sim \mathbf{C}^*\mathbf{V}^*\mathbf{C}^*$  is found in  $\hat{\sigma}'_1$  and the two occurrences of  $\mathbf{C}^*$  represent the same letter, then remove the last letter from  $\hat{\sigma}'_1$ , and do  $\mathbf{V}^*\sim \rightarrow \emptyset$  on  $\hat{\sigma}'_2$ .<sup>82</sup> Call the results after these operations  $\hat{\sigma}''_1$  and  $\hat{\sigma}''_2$ , respectively.
- (13) On  $\hat{\sigma}''_2$ , perform the following substitutions in a sequel:
- (10.1) Do  $\hat{x}_{\neq}(c|t)ul \rightarrow \hat{x}$ ,  $(cul|lent|mon) \rightarrow \emptyset$ ,  $(errim|issim) \rightarrow \emptyset$ ,  $men(\emptyset|t) \rightarrow \emptyset$ .
- (10.2) Do  $\sim(m|ni|nt(\emptyset|\mathbf{V}^*)(\emptyset|r)|r\mathbf{V}^*|s) \rightarrow \emptyset$ .
- (10.3) Do  $\sim\hat{x}(mi|mul|mur|ntur|sti|ri) \rightarrow \hat{x}$ ,  $\hat{x}_{\neq}(r)t \rightarrow \hat{x}$ .
- The result after these three steps of operations is called  $\hat{\sigma}''_2$ .
- (14) Concatenate  $\hat{\sigma}'_1$  and  $\hat{\sigma}''_2$ .
- (15) Do  $die(bu|m|ru|s) \rightarrow dieque$ ,  $ign \rightarrow en$ ,  $re(bu|m|rum|s) \rightarrow reque$ ,  $ct \rightarrow \check{c}$ ,  $pro\sigma\sim \rightarrow pros$ ,  $\mathbf{V}^*men(\emptyset|t) \rightarrow \mathbf{V}^*$ ,  $' \rightarrow \emptyset$ .

**Algorithm 6.25** (Latin essential root). Let  $\hat{\sigma}$  be the effective spelling of a Latin word, then its corresponding essential root  $\text{EssRoot}(\hat{\sigma})$  is constructed in the following steps:

- (1) Break down  $\hat{\sigma} = \hat{\sigma}_1\hat{\sigma}_2$  into the concatenation of two strings  $\hat{\sigma}_1 = \hat{\sigma}^{[\text{ProtRg}(\hat{\sigma})]}$  (see the notation in Definition 3.1) and  $\hat{\sigma}_2$ , where the length of the first string  $\ell(\hat{\sigma}_1) = \text{ProtRg}(\hat{\sigma})$  is equal to the protected range of  $\hat{\sigma}$ .
- (2) Do  $\mathbf{C}^*(a|ae)\mathbf{C}^* \rightarrow \mathbf{C}^*e\mathbf{C}^*$  on  $\hat{\sigma}_1$ ,<sup>83</sup> and call the result  $\hat{\sigma}'_1$ .
- (3) On  $\hat{\sigma}_2$ , perform the following substitutions in a sequel:
- (3.1) Do  $\sim que \rightarrow \emptyset$ .
- (3.2) Do  $(b|id|nd|t|v)\mathbf{V}^*(\emptyset|m|n|r|(s)_m|t) \rightarrow \emptyset$ .
- (3.3) Do  $\sim(a|e|i|in|o|r|ss|u)_m \rightarrow \emptyset$ .
- The result after these three steps of operations is called  $\hat{\sigma}'_2$ .
- (4) Concatenate  $\hat{\sigma}'_1$  and  $\hat{\sigma}'_2$ .
- (5) Replace<sup>84</sup>

|                                                                  |                                                                                                                                          |                                                |                           |                                               |                 |
|------------------------------------------------------------------|------------------------------------------------------------------------------------------------------------------------------------------|------------------------------------------------|---------------------------|-----------------------------------------------|-----------------|
| $sens\sim$                                                       | $X^{\epsilon}(\emptyset a circum con di e\check{c} in jnter ob per prae re suzp st a ae ans ant e eb em end ens ent er es ess est et o)$ |                                                |                           |                                               |                 |
| sent                                                             | $\mathbf{X}stand$                                                                                                                        |                                                |                           |                                               |                 |
|                                                                  | $X^{\epsilon}(\emptyset ab ad con in per prae pro red suss)d(a and ans ant e eb em end ens ent er er g es ess est et etis etur o or)$    |                                                |                           |                                               |                 |
|                                                                  | $\mathbf{X}datt$                                                                                                                         |                                                |                           |                                               |                 |
|                                                                  | $X^{\epsilon}(\emptyset ad af au circum con de di fin jnter(\emptyset queo) of prae pro re suf trans)fer(q r t)$                         |                                                |                           |                                               |                 |
|                                                                  | $\mathbf{X}fer$                                                                                                                          |                                                |                           |                                               |                 |
|                                                                  | $X^{\epsilon}(\emptyset ad circum com de di e im jnter(\emptyset queo) o per prae pro re suss suzp trans)mis(\emptyset s)$               |                                                |                           | $X^{\epsilon}(\emptyset co \mu prae pro)pass$ |                 |
|                                                                  | $\mathbf{X}mitt$                                                                                                                         |                                                |                           | $\mathbf{X}Xet$                               |                 |
| $ci(e eam eant ear eas eat eb em end ens ent eo eor er es et t)$ | $es(\emptyset s t)$                                                                                                                      | $i(\check{c} c)\mathbf{V}^*\mathbf{C}^*_{m_0}$ | $m(all el ev)$            | $noll$                                        | $v(el ell olt)$ |
| cit                                                              | ed                                                                                                                                       | ic                                             | mevol                     | nol                                           | vol             |
| $\sim(lev lit)$                                                  | $\sim(aper ien)$                                                                                                                         | $\sim(cur r ren s)$                            | $\sim(fund(\emptyset en)$ | $\sim(ges(s t)$                               | $\sim(mess$     |
| lin                                                              | ap                                                                                                                                       | cur                                            | fus                       | ger                                           | met             |
| $\sim(lev lit)$                                                  | $\sim(aper ien)$                                                                                                                         | $\sim(cur r ren s)$                            | $\sim(fund(\emptyset en)$ | $\sim(ges(s t)$                               | $\sim(mess$     |
| lin                                                              | ap                                                                                                                                       | cur                                            | fus                       | ger                                           | met             |
| $\sim(p ast ev)$                                                 | $\sim(pel)$                                                                                                                              | $\sim(port an)$                                | $\sim(se t v)$            | $\sim(starr(\emptyset d)$                     | $\sim(vent$     |
| pasc                                                             | pell                                                                                                                                     | por                                            | ser                       | stern                                         | ven             |
|                                                                  |                                                                                                                                          |                                                |                           |                                               | vert            |
|                                                                  |                                                                                                                                          |                                                |                           |                                               | vic             |
|                                                                  | $X^{\epsilon}(\emptyset ab abs al at circum con de dis in jnter(\emptyset queo) ob prae pro re sub trans)(let tul)$                      |                                                |                           |                                               |                 |
|                                                                  | $\mathbf{X}'fer$                                                                                                                         |                                                |                           |                                               |                 |

<sup>82</sup>This peculiar step is tailored for reduplications in the perfect forms of certain Latin verbs. Such reduplications are not attested in most modern Indo-European languages, with Greek being a notable exception.

<sup>83</sup>Here, the two occurrences of  $\mathbf{C}^*$  may or may not represent the same letter.

<sup>84</sup>All the patches below are devoted to some common verbs that exhibit highly irregular conjugations.

where in the last step, one constructs  $\mathbf{X}'$  from  $\mathbf{X}$  by doing  $\sim ab(\emptyset|s) \rightarrow au$ ,  $\sim(\check{c}|l|t) \rightarrow f$ ,  $dis \rightarrow dif$ ,  $ob \rightarrow of$ ,  $suss \rightarrow suf$ .

(6) Set

$$\mathbf{X}_1 = (eam|eant|eas|eat|eo|eund|eunt|i|ib|ibant|ibem|ibes|ibet|ibim|ibis|ibit|ibo|ibunt|iens|ieq|ier|i|im|iit|im|imus|ir|ire|irent|ireq|iret|iri|is|isse|issem|issent|isser|ist|isti|istis|it|ite|iti|itis|itist|ito|itu|itum|itur|itus),$$

and

$$\mathbf{X}_2 = (er|es|ess|est|for|fuer|fui|fuim|fuiss|fuist|fuit|fut|si|sim|sint|sit|sum|sumus|sunt|sunto).$$

Replace<sup>85</sup>

$$\frac{\mathbf{X}^\infty(\emptyset|ab|ad|amb|circum|co|de|in|jnter(\emptyset|queo)|ob|prod|red|suss|trans)\mathbf{X}_1}{\mathbf{X}_{eo}}$$

$$\frac{\mathbf{X}^\infty(ab|ad|de|in|jnter|ob|prae|pro|suss|suzp)\mathbf{X}_2}{\mathbf{X}_{sum}}$$

### 6.3.2 Admissible mutation and approximate clustering

Like the case of French, vowel blotting is unnecessary for Latin. The only significant pattern of vowel alternation in Latin verb conjugations has already been taken care of by Algorithm 6.25(2).

In what follows, we will construct a bivariate Boolean-valued function  $\text{HrdTest}(\hat{\alpha}, \hat{\beta})$  on a “simple heredity test function” in Algorithm 6.26, and a set of “admissible suffix mismatch” rules in Algorithm 6.27.

**Algorithm 6.26** (Simple heredity test). *Let  $\hat{\alpha}'$  be the result from doing  $\sim \mathbf{V}_{m_0}^*(\emptyset|er|que|que|s|st) \rightarrow \emptyset$  on  $\hat{\alpha}$ , and define  $\hat{\beta}'$  similarly. The Boolean-valued function  $\text{SimpHrdTest}(\hat{\alpha}, \hat{\beta})$  returns **TRUE** if the lowercase form of  $\hat{\alpha}$  contains at least one instance of  $\mathbf{V}^*$  (Definition 6.22) **AND** at least one of the following three conditions holds.<sup>86</sup>*

- (i)  $\hat{\alpha}' = \hat{\beta}'$ ;
- (ii)  $\hat{\beta} = \hat{\alpha}t$ ;
- (iii)  $\ell(\hat{\beta}) > \ell(\hat{\alpha}) \geq \frac{\ell(\hat{\beta})}{2}$  **AND**  $\hat{\alpha} = \hat{\beta}^{\lfloor \ell(\hat{\alpha}) \rfloor}$  **AND**  $\hat{\beta}^{\lfloor \ell(\hat{\alpha}') + 1 \rfloor} = \mathbf{V}^*$ . (See Definition 3.1 for the notations  $\hat{\beta}^{\lfloor n \rfloor}$  and  $\hat{\beta}^{\lfloor n \rfloor}$ .)

In what follows, we define  $\text{SuffixNW}(\hat{\alpha}, \hat{\beta})$ ,  $\text{RootNW}(\hat{\alpha}, \hat{\beta})$ ,  $\text{NW}^*(\hat{\alpha}, \hat{\beta})$  and  $\text{SuffixSW}(\hat{\alpha}, \hat{\beta})$ ,  $\text{SuffixSW}(\hat{\alpha}, \hat{\beta})$ ,  $\text{SW}^*(\hat{\alpha}, \hat{\beta})$  as what is done in the Danish case (Algorithm 5.7), which was also applied to two other Germanic languages treated in §5.

**Algorithm 6.27** (Admissible suffix mismatch). *For two strings  $\hat{\alpha}$  and  $\hat{\beta}$ , the Boolean-valued function*

$$\text{AdmSM}(\text{RootNW}(\hat{\alpha}, \hat{\beta}), \text{SuffixNW}(\hat{\alpha}, \hat{\beta}), \text{NW}^*(\hat{\alpha}, \hat{\beta}))$$

*returns **TRUE** if  $\text{NW}^*(\hat{\alpha}, \hat{\beta}) = \emptyset$  **AND**  $\text{RootNW}(\hat{\alpha}, \hat{\beta})$  contains at least one instance of  $\mathbf{V}^*$  **AND** at least one of the following four conditions holds:*

- (i)  $\text{SuffixNW}(\hat{\alpha}, \hat{\beta}) = [(\emptyset|(a|e|i|o|u)_m(\emptyset|n)), (\emptyset|(a|e|i|o|u)_m(\emptyset|n))]$ ;
- (ii)  $\text{SuffixNW}(\hat{\alpha}, \hat{\beta}) = [c, \check{c}][[\check{c}, g]][[c, q]][[d, s]][[den, s]]$ ;
- (iii)  $\text{SuffixNW}(\hat{\alpha}, \hat{\beta}) = [d, t]$  **AND**  $\mathcal{Q}(\text{RootNW}(\hat{\alpha}, \hat{\beta})) = r$ ;
- (iv)  $\text{SuffixNW}(\hat{\alpha}, \hat{\beta}) = [\check{c}, c\mathbf{V}^*\mathbf{X}]$ .

*Similarly, one can evaluate another Boolean-valued function*

$$\text{AdmSM}(\text{RootSW}(\hat{\alpha}, \hat{\beta}), \text{SuffixSW}(\hat{\alpha}, \hat{\beta}), \text{SW}^*(\hat{\alpha}, \hat{\beta}))$$

*by trading all the occurrences of NW in the statements above with SW.*

**Algorithm 6.28** (Heredity test function). *The structure of the Latin heredity test function  $\text{HrdTest}(\hat{\alpha}, \hat{\beta})$  is identical to the German version (Algorithm 8.1.2), except that the functions  $\text{SimpHrdTest}$ ,  $\text{RootNW}$ ,  $\text{SuffixNW}$ ,  $\text{NW}^*$ ,  $\text{RootSW}$ ,  $\text{SuffixSW}$ ,  $\text{SW}^*$  must follow the Latin rules stated above.*

<sup>85</sup>All the patches below are devoted to suppletive verbs derived from  $e\check{o}$  “go” and  $sum$  “be”.

<sup>86</sup>As a general rule in this document, the truth values of items labeled with Roman numerals are connected to each other with logical **OR**.

**Algorithm 6.29** (Approximate clustering of Latin words). *The algorithm is essentially the same as Algorithm 6.20, except that Latin rules (instead of French rules) apply to all the tags (effective spelling, essential root etc.).*

*Example 6.29.1.* There are five declensions in Latin. The first three declensions cover both nouns and adjectives, while the last two are reserved for nouns only. We extract sample nouns and adjectives from the following Wiktionary and Wikipedia pages:

[https://en.wiktionary.org/wiki/Appendix:Latin\\_first\\_declension](https://en.wiktionary.org/wiki/Appendix:Latin_first_declension)

*comētae, comētārum, comētās, comētē, comētem, comētēn, comētēs, comētīs* — “comet”;

*dynastae, dynastārum, dynastās, dynastē, dynastēn, dynastēs, dynastīs* — “ruler”;

*nauta, nautā, nautae, nautam, nautārum, nautās, nautīs* — “sailor”;

*nymphae, nymphārum, nymphās, nymphē, nymphēn, nymphēs, nymphīs* — “bride”;

*Rōma, Rōmā, Rōmae, Rōmam* — “Rome”;

*rosa, rosā, rosae, rosam, rosārum, rosās, rosīs* — “rose”;

*stēlla, stēllā, stēllae, stēllam, stēllārum, stēllās, stēllīs* — “star”;

*xiphīa, xiphīae, xiphīān, xiphīārum, xiphīās, xiphīūs* — “swordfish”.

[https://en.wiktionary.org/wiki/Appendix:Latin\\_second\\_declension](https://en.wiktionary.org/wiki/Appendix:Latin_second_declension)

*ager, agrī, agrīs, agrō, agrōrum, agrōs, agrum* — “field”;

*ampele, ampelī, ampelīs, ampelō, ampelon, ampelōrum, ampelos, ampelōs, ampelum* — “vine”;

*atome, atomī, atomīs, atomō, atomōrum, atomōs, atomum, atomus* — “atom”;

*bella, bellī, bellīs, bellō, bellōrum, bellum* — “war”;

*fīlī, fīlīi, fīlīis, fīliō, fīliōrum, fīliōs, fīlium, fīlius* — “son”;

*magister, magistrī, magistrīs, magistrō, magistrōrum, magistrōs, magistrum* — “teacher”;

*mūre, mūrī, mūrīs, mūrō, mūrōrum, mūrōs, mūrum, mūrus* — “wall”;

*mūthe, mūthī, mūthīs, mūthō, mūthon, mūthōrum, mūthos, mūthōs, mūthum* — “myth”;

*phaenomena, phaenomenī, phaenomenīs, phaenomenō, phaenomenon, phaenomenōrum* — “phenomenon”;

*puer, puerī, puerīs, puerō, puerōrum, puerōs, puerum* — “child”;

*templa, templī, templīs, templō, templōrum, templum* — “temple”.

[https://en.wiktionary.org/wiki/Appendix:Latin\\_third\\_declension](https://en.wiktionary.org/wiki/Appendix:Latin_third_declension)

*āēr, āera, āere, āerem, āerēs, āerī, āeribus, āeris, āeros, āerum* — “air”;

*animal, animālī, animālia, animālibus, animālis, animālium* — “animal”;

*base, basem, basēs, basī, basibus, basim, basis, basīs, basium* — “pedestal”;

*haerese, haerese, haeresēs, haeresī, haeresibus, haeresim, haeresis, haeresīs, haeresium* — “sect”;

*homine, hominem, hominēs, hominī, hominibus, hominis, hominum, homō* — “human”;

*nocte, noctem, noctēs, noctī, noctibus, noctis, noctium, nox* — “night”;

*nōmen, nōmina, nōmine, nōminī, nōminibus, nōminis, nōminum* — “name”;

*tigre, tigrem, tigrēs, tigrī, tigribus, tigrīde, tigrīdem, tigrīdēs, tigrīdī, tigrīdibus, tigrīdis, tigrīdum, tigrīm, tigrīs, tigrīs, tigrīs, tigrīum* — “tiger”;

*turre, turrem, turrēs, turrī, turribus, turrim, turris, turris, turrium* — “tower”.

[https://en.wiktionary.org/wiki/Appendix:Latin\\_fourth\\_declension](https://en.wiktionary.org/wiki/Appendix:Latin_fourth_declension)

*cornibus, cornū, cornua, cornūs, cornuum* — “horn”;

*Dīdō, Dīdōne, Dīdōnem, Dīdōnēs, Dīdōnī, Dīdōnibus, Dīdōnis, Dīdōnum* — “Dido”;

*ēchibus, ēcho, ēchū, ēchuī, ēchum, ēchūs, ēchuum* — “echo”;

*manibus, manū, manuī, manum, manus, manūs, manuum* — “hand”.

[https://en.wiktionary.org/wiki/Appendix:Latin\\_fifth\\_declension](https://en.wiktionary.org/wiki/Appendix:Latin_fifth_declension)

*diē, diēbus, diēi, diem, diērum, diēs* — “day”;

*fidē, fidēbus, fideī, fidem, fidērum, fidēs* — “faith”;

*rē, rēbus, reī, rem, rērum, rēs* — “thing”;

*speciē, speciēbus, speciēi, speciem, speciērum, speciēs* — “view”.

[https://en.wikipedia.org/wiki/Latin\\_declension#Adjectives](https://en.wikipedia.org/wiki/Latin_declension#Adjectives)

Here are some Latin adjectives whose positive forms belong to the first and second declensions. (We also incorporate, in our list below, comparative and superlative forms of certain sample adjectives, which may or may not share the same declension pattern with the original adjectives in positive forms.)

*alta, altā, altae, altam, altārum, altās, alte, altī, altior, altiōra, altiōre, altiōrem, altiōrēs, altiōrī, altiōribus, altiōris, altiōrum, altīs, altissima, altissimā, altissimae, altissimam, altissimārum, altissimās, altissime, altissimī, altissimīs, altissimō, altissimōrum, altissimōs, altissimum, altissimus, altius, altō, altōrum, altōs, altum, altus* — “tall”;

*atoma, atomā, atomae, atomam, atomārum, atomās, atome, atomī, atomīs, atomō, atomōrum, atomōs, atomum, atomus* — “indivisible”;

*miser, misera, miserā, miserae, miseram, miserārum, miserās, miserī, miserior, miseriōra, miseriōre, miseriōrem, miseriōrēs, miseriōrī, miseriōribus, miseriōris, miseriōrum, miserīs, miserius, miserō, miserōrum, miserōs, miserrima, miserrimā, miserrimae, miserrimam, miserrimārum, miserrimās, miserrime, miserrimī, miserrimīs, miserrimō, miserrimōrum, miserrimōs, miserrimum, miserrimus, miserum* — “poor”;

*sacer, sacra, sacrā, sacrae, sacram, sacrārum, sacrās, sacrī, sacrīs, sacrō, sacrōrum, sacrōs, sacrum* — “sacred”;

*ūlla, ūllā, ūllae, ūllam, ūllārum, ūllās, ūlle, ūllī, ūllīs, ūllius, ūllō, ūllōrum, ūllōs, ūllum, ūllus* — “any”.

Here are some Latin adjectives whose positive forms belong to the third declension.

*agile, agilem, agilēs, agilī, agilia, agilibus, agilis, agilium* — “agile”;

*alacer, alacre, alacrem, alacrēs, alacrī, alacria, alacribus, alacris, alacrium* — “lively”;

*atrōcem, atrōcēs, atrōcī, atrōcia, atrōcibus, atrōcior, atrōciōra, atrōciōre, atrōciōrem, atrōciōrēs, atrōciōrī, atrōciōribus, atrōciōris, atrōciōrum, atrōcis, atrōcissima, atrōcissimā, atrōcissimae, atrōcissimam, atrōcissimārum, atrōcissimās, atrōcissime, atrōcissimī, atrōcissimīs, atrōcissimō, atrōcissimōrum, atrōcissimōs, atrōcissimum, atrōcissimus, atrōcium, atrōcius, atrōx* — “fierce”;

*celer, celere, celerem, celerēs, celerī, celeria, celeribus, celerior, celeriōra, celeriōre, celeriōrem, celeriōrēs, celeriōrī, celeriōribus, celeriōris, celeriōrum, celeris, celerium, celerius, celerrima, celerrimā, celerrimae, celerrimam, celerrimārum, celerrimās, celerrime, celerrimī, celerrimīs, celerrimō, celerrimōrum, celerrimōs, celerrimum, celerrimus* — “fast”;

*melior, meliōra, meliōre, meliōrem, meliōrēs, meliōrī, meliōribus, meliōris, meliōrum, melius* — “better”;

*trīste, trīstem, trīstēs, trīstī, trīstia, trīstibus, trīstior, trīstiōra, trīstiōre, trīstiōrem, trīstiōrēs, trīstiōrī, trīstiōribus, trīstiōris, trīstiōrum, trīstis, trīstissima, trīstissimā, trīstissimae, trīstissimam, trīstissimārum, trīstissimās, trīstissime, trīstissimī, trīstissimīs, trīstissimō, trīstissimōrum, trīstissimōs, trīstissimum, trīstissimus, trīstium, trīstius* — “unhappy”;

*vetera, vetere, veterem, veterēs, veterī, veteribus, veteris, veterrima, veterrimā, veterrimae, veterrimam, veterrimārum, veterrimās, veterrime, veterrimī, veterrimīs, veterrimō, veterrimōrum, veterrimōs, veterrimum, veterrimus, veterum, vetus, vetustior, vetustiōra, vetustiōre, vetustiōrem, vetustiōrēs, vetustiōrī, vetustiōribus, vetustiōris, vetustiōrum, vetustissima, vetustissimā, vetustissimae, vetustissimam, vetustissimārum, vetustissimās, vetustissime, vetustissimī, vetustissimīs, vetustissimō, vetustissimōrum, vetustissimōs, vetustissimum, vetustissimus, vetustius* — “old”.

Our clustering algorithm yields the following result:

{*āēr, āera, āere, āerem, āerēs, āerī, āeribus, āeris, āeros, āerum*} ,

{*ager, agrī, agrīs, agrō, agrōrum, agrōs, agrum*} ,

{*agile, agilem, agilēs, agilī, agilia, agilibus, agilis, agiliūm*} ,

{*alacer, alacre, alacrem, alacrēs, alacrī, alacria, alacribus, alacris, alacriūm*} ,

{*alta, altā, altae, altam, altārum, altās, alte, altī, altior, altiōra, altiōre, altiōrem, altiōrēs, altiōrī, altiōribus, altiōris, altiōrum, altīs, altissima, altissimā, altissimae, altissimam, altissimārum, altissimās, altissime, altissimī, altissimīs, altissimō, altissimōrum, altissimōs, altissimum, altissimus, altius, altō, altōrum, altōs, altum, altus*} ,

{*ampele, ampelī, ampelīs, ampelō, ampelon, ampelōrum, ampelos, ampelōs, ampelum*} ,

{*animal, animālī, animālia, animālibus, animālis, animāliūm*} ,

{*atoma, atomā, atomae, atomam, atomārum, atomās, atome, atomī, atomīs, atomō, atomōrum, atomōs, atomum, atomus*} ,

{*atrōcem, atrōcēs, atrōcī, atrōcia, atrōcibus, atrōcior, atrōciōra, atrōciōre, atrōciōrem, atrōciōrēs, atrōciōrī, atrōciōribus, atrōciōris, atrōciōrum, atrōcis, atrōcissima, atrōcissimā, atrōcissimae, atrōcissimam, atrōcissimārum, atrōcissimās, atrōcissime, atrōcissimī, atrōcissimīs, atrōcissimō, atrōcissimōrum, atrōcissimōs, atrōcissimum, atrōcissimus, atrōcium, atrōcius, atrōx*} ,

{*base, basem, basēs, basī, basibus, basim, basis, basīs, basium*} ,

{*bella, bellī, bellīs, bellō, bellōrum, bellum*} ,

{*celer, celere, celerem, celerēs, celerī, celeria, celeribus, celerior, celeriōra, celeriōre, celeriōrem, celeriōrēs, celeriōrī, celeriōribus, celeriōris, celeriōrum, celeris, celerium, celerius, celerrima, celerrimā, celerrimae, celerrimam, celerrimārum, celerrimās, celerrime, celerrimī, celerrimīs, celerrimō, celerrimōrum, celerrimōs, celerrimum, celerrimus*} ,

{*comētae, comētārum, comētās, comētē, comētem, comētēn, comētēs, comētīs*} ,

{*cornibus, cornū, cornua, cornūs, cornuum*} ,

{*Dīdō, Dīdōne, Dīdōnem, Dīdōnēs, Dīdōnī, Dīdōnibus, Dīdōnis, Dīdōnum, diē, diēbus, diēī, diem, diērum, diēs*} ,

{*dynastae, dynastārum, dynastās, dynastē, dynastēn, dynastēs, dynastīs*} ,

{*ēchibus, ēcho, ēchū, ēchuī, ēchum, ēchūs, ēchuūm*} ,

{*fidē, fidēbus, fideī, fidem, fidērum, fidēs*} ,

{*fīlī, fīlīū, fīlīs, fīliō, fīliōrum, fīliōs, fīliūm, fīlius*} ,

- {*haerese, haeresem, haeresēs, haeresī, haeresibus, haeresim, haeresis, haeresīs, haeresium*},
- {*homine, hominem, hominēs, hominī, hominibus, hominis, hominum, homō*},
- {*magister, magistrī, magistrīs, magistrō, magistrōrum, magistrōs, magistrum*},
- {*manibus, manū, manuī, manum, manus, manūs, manuum*},
- {*melior, melius*},
- {*meliōra, meliōre, meliōrem, meliōrēs, meliōrī, meliōribus, meliōris, meliōrum*},
- {*miser, misera, miserā, miserae, miseram, miserārum, miserās, miserī, miserior, miseriōra, miseriōre, miseriōrem, miseriōrēs, miseriōrī, miseriōribus, miseriōris, miseriōrum, miserīs, miserius, miserō, miserōrum, miserōs, miserrima, miserrimā, miserrimae, miserrimam, miserrimārum, miserrimās, miserrime, miserrimī, miserrimīs, miserrimō, miserrimōrum, miserrimōs, miserrimum, miserrimus, miserum*},
- {*mūre, mūrī, mūrīs, mūrō, mūrōrum, mūrōs, mūrum, mūrus*},
- {*mȳthe, mȳthī, mȳthīs, mȳthō, mȳthon, mȳthōrum, mȳthos, mȳthōs, mȳthum*},
- {*nauta, nautā, nautae, nautam, nautārum, nautās, nautīs*},
- {*nocte, noctem, noctēs, noctī, noctibus, noctis, noctium, nox*},
- {*nōmen, nōmina, nōmine, nōminī, nōminibus, nōminis, nōminum*},
- {*nymphae, nymphārum, nymphās, nymphē, nymphēn, nymphēs, nymphīs*},
- {*phaenomena, phaenomenī, phaenomenīs, phaenomenō, phaenomenon, phaenomenōrum*},
- {*puer, puerī, puerīs, puerō, puerōrum, puerōs, puerum*},
- {*rē, rēbus, reī, rem, rērum, rēs*},
- {*Rōma, Rōmā, Rōmae, Rōmam*},
- {*rosa, rosā, rosae, rosam, rosārum, rosās, rosīs*},
- {*sacer, sacra, sacrā, sacrae, sacram, sacrārum, sacrās, sacrī, sacrīs, sacrō, sacrōrum, sacrōs, sacrum*},
- {*speciē, speciēbus, speciēi, speciem, speciērum, speciēs*},
- {*stēlla, stēllā, stēllae, stēllam, stēllārum, stēllās, stēllīs*},
- {*templa, templī, templīs, templō, templōrum, templum*},
- {*tigre, tigrem, tigrēs, tigrī, tigribus, tigrīde, tigridem, tigridēs, tigrīdī, tigrīdibus, tigrīdis, tigrīdum, tigrim, tigris, tigrīs, tigris, tigrīum*},
- {*trīste, trīstem, trīstēs, trīstī, trīstia, trīstibus, trīstior, trīstiōra, trīstiōre, trīstiōrem, trīstiōrēs, trīstiōrī, trīstiōribus, trīstiōris, trīstiōrum, trīstis, trīstissima, trīstissimā, trīstissimae, trīstissimam, trīstissimārum, trīstissimās, trīstissime, trīstissimī, trīstissimīs, trīstissimō, trīstissimōrum, trīstissimōs, trīstissimum, trīstissimus, trīstium, trīstius*},
- {*turre, turrem, turrēs, turrī, turribus, turrim, turris, turris, turrium*},
- {*ūlla, ūllā, ūllae, ūllam, ūllārum, ūllās, ūlle, ūllī, ūllīs, ūllīus, ūllō, ūllōrum, ūllōs, ūllum, ūllus*},
- {*vetera, vetere, veterem, veterēs, veterī, veteribus, veteris, veterrima, veterrimā, veterrimae, veterrimam, veterrimārum, veterrimās, veterrime, veterrimī, veterrimīs, veterrimō, veterrimōrum, veterrimōs, veterrimum, veterimus, veterum, vetus, vetustior, vetustiōra, vetustiōre, vetustiōrem, vetustiōrēs, vetustiōrī, vetustiōribus, vetustiōris, vetustiōrum, vetustissima, vetustissimā, vetustissimae, vetustissimam, vetustissimārum, vetustissimās, vetustissime, vetustissimī, vetustissimīs, vetustissimō, vetustissimōrum, vetustissimōs, vetustissimum, vetustissimus, vetustius*},

{*xiphiā, xiphiae, xiphiān, xiphiārum, xiphiās, xiphiīs*}.

Example 6.29.2. Latin verbs are divided into four conjugation groups. We test our algorithm on the following selections of verbs, based primarily on the Wikipedia links below:

[https://en.wikipedia.org/wiki/Latin\\_conjugation#First\\_conjugation](https://en.wikipedia.org/wiki/Latin_conjugation#First_conjugation)

*amā, amābam, amābāminī, amābāmur, amābāmus, amābant, amābantur, amābar, amābāre, amābāris, amābās, amābat, amābātis, amābātur, amābere, amāberis, amābiminī, amābimur, amābimus, amābis, amābit, amābitis, amābitur, amābō, amābor, amābunt, amābuntur, amāminī, amāmur, amāmus, amandī, amandō, amandum, amandus, amāns, amant, amantō, amantor, amantur, amāre, amārem, amārēminī, amārēmur, amārēmus, amārent, amārentur, amārer, amārēre, amārēris, amārēs, amāret, amārētis, amārētur, amārī, amāris, amās, amat, amāta, amātā, amātae, amātam, amātārum, amātās, amāte, amātī, amātis, amātīs, amātō, amātor, amātōrum, amātōs, amātōte, amātū, amātum, amātur, amātūrus, amātus, amāveram, amāverāmus, amāverant, amāverās, amāverat, amāverātis, amāvēre, amāverim, amāverimus, amāverīmus, amāverint, amāveris, amāverīs, amāverit, amāveritis, amāverītis, amāverō, amāvērunt, amāvī, amāvimus, amāvisse, amāvissēmus, amāvissem, amāvissēmus, amāvisset, amāvissētis, amāvissētis, amāvistī, amāvistis, amāvit, amem, amēminī, amēmur, amēmus, ament, amentur, amer, amēre, amēris, amēs, amet, amētis, amētur, amō, amor* — “love”;

*dā, dabam, dabāminī, dabāmur, dabāmus, dabant, dabantur, dabar, dabāre, dabāris, dabās, dabat, dabātis, dabātur, dabere, daberis, dabiminī, dabimur, dabimus, dabis, dabit, dabitur, dabō, dabor, dabunt, dabuntur, daminī, damur, damus, dandī, dandō, dandum, dandus, dāns, dant, dantō, dantor, dantur, dare, darem, darēminī, darēmur, darēmus, darent, darentur, darer, darēre, darēris, darēs, daret, darētis, darētur, darī, daris, dās, dat, data, datā, datae, datam, datārum, datās, date, datī, datis, datīs, datō, dator, datōrum, datōs, datōte, datū, datum, datur, datūrus, datus, dederam, dederāmus, dederant, dederās, dederat, dederātis, dedēre, dederim, dederimus, dederīmus, dederint, dederis, dederīs, dederit, dederitis, dederītis, dederō, dedērunt, dedī, dedimus, dedisse, dedissem, dedissēmus, dedissent, dedissēs, dedisset, dedissētis, dedistī, dedistis, dedit, dem, dēminī, dēmur, dēmus, dent, dentur, der, dēre, dēris, dēs, det, dētis, dētur, dō, dor* — “give”;

*fricā, fricābam, fricābāminī, fricābāmur, fricābāmus, fricābant, fricābantur, fricābar, fricābāre, fricābāris, fricābās, fricābat, fricābātis, fricābātur, fricābere, fricāberis, fricābiminī, fricābimur, fricābimus, fricābis, fricābit, fricābitis, fricābitur, fricābō, fricābor, fricābunt, fricābuntur, fricāminī, fricāmur, fricāmus, fricandī, fricandō, fricandum, fricandus, fricāns, fricant, fricantō, fricantor, fricantur, fricāre, fricārem, fricārēminī, fricārēmur, fricārēmus, fricārent, fricārentur, fricārer, fricārēre, fricārēris, fricārēs, fricāret, fricārētis, fricārētur, fricārī, fricāris, fricās, fricat, fricāte, fricātibus, fricātis, fricātō, fricātor, fricātōte, fricātū, fricātū, fricātum, fricātur, fricātūrus, fricātus, fricātūs, fricātuum, fricem, fricēminī, fricēmur, fricēmus, fricent, fricentur, fricer, fricēre, fricēris, fricēs, fricet, fricētis, fricētur, fricō, fricor, fricueram, fricuerāmus, fricuerant, fricuerās, fricuerat, fricuerātis, fricuēre, fricuerim, fricuerimus, fricuerīmus, fricuerint, fricueris, fricuerīs, fricuerit, fricueritis, fricuerītis, fricuerō, fricuērunt, fricuī, fricuimus, fricuisse, fricuissem, fricuissemus, fricuissemus, fricuisset, fricuissetis, fricuisstī, fricuisstis, fricuīt* — “rub”;

*iūta, iūtā, iūtae, iūtā, iūtārum, iūtās, iūte, iūtī, iūtīs, iūtō, iūtōrum, iūtōs, iūtū, iūtum, iūtūrus, iūtus, iuvā, iuvābam, iuvābāminī, iuvābāmur, iuvābāmus, iuvābant, iuvābantur, iuvābar, iuvābāre, iuvābāris, iuvābās, iuvābat, iuvābātis, iuvābātur, iuvābere, iuvāberis, iuvābiminī, iuvābimur, iuvābimus, iuvābis, iuvābit, iuvābitis, iuvābitur, iuvābō, iuvābor, iuvābunt, iuvābuntur, iuvāminī, iuvāmur, iuvāmus, iuvandī, iuvandō, iuvandum, iuvandus, iuvāns, iuvant, iuvantō, iuvantor, iuvantur, iuvāre, iuvārem, iuvārēminī, iuvārēmur, iuvārēmus, iuvārent, iuvārentur, iuvārer, iuvārēre, iuvārēris, iuvārēs, iuvāret, iuvārētis, iuvārētur, iuvārī, iuvāris, iuvās, iuvat, iuvāte, iuvātis, iuvātō, iuvātor, iuvātōte, iuvātur, iuvem, iuvēminī, iuvēmur, iuvēmus, iuvent, iuventur, iuver, iūveram, iūverāmus, iūverant, iūverās, iūverat, iūverātis, iuvēre, iūvēre, iūverim, iūverimus, iūverīmus, iūverint, iūveris, iūverīs, iūverit, iūveritis, iūverītis, iūverō, iūvērunt, iuvēs, iuvet, iuvētis, iuvētur, iūvī, iūvimus, iūvisse, iūvissem, iūvissemus, iūvisset, iūvissetis, iūvistī, iūvistis, iūvit, iuvō, iuvor* — “help”;

*lavā, lavābam, lavābāminī, lavābāmur, lavābāmus, lavābant, lavābantur, lavābar, lavābāre, lavābāris, lavābās, lavābat, lavābātis, lavābātur, lavābere, lavāberis, lavābiminī, lavābimur, lavābimus, lavābis, lavābit, lavābitis, lavābitur, lavābō, lavābor, lavābunt, lavābuntur, lavāminī, lavāmur, lavāmus, lavandī, lavandō, lavandum, lavandus, lavāns, lavant, lavantō, lavantor, lavantur, lavāre, lavārem, lavārēminī, lavārēmur, lavārēmus, lavārent, lavārentur, lavārer, lavārēre, lavārēris, lavārēs, lavāret, lavārētis, lavārētur, lavārī, lavāris, lavās, lavat, lavāta, lavātā, lavātae, lavātā, lavātārum, lavātās, lavāte, lavātī, lavātis, lavātīs, lavātō, lavātor, lavātōrum, lavātōs, lavātōte, lavātū, lavātum, lavātur, lavātūrus, lavātus, lavem, lavēminī, lavēmur, lavēmus, lavent, laventur, laver, lavēre, lavēris, lavēs, lavet, lavētis, lavētur, lavō, lavar* — “wash”;





*fōveritis, fōverītis, fōverō, fōvērunt, fōvēs, fōvet, fōvēte, fōvētis, fōvētō, fōvētor, fōvētōte, fōvētur, fōvī, fōvimus, fōvisse, fōvissem, fōvissemus, fōvisissent, fōvisseēs, fōvisset, fōvissetis, fōvistī, fōvistis, fōvit* — “caress”;

*iubē, iubeam, iubeāminī, iubeāmur, iubeāmus, iubeant, iubeantur, iubeat, iubeāre, iubeāris, iubeās, iubeat, iubeātis, iubeātur, iubēbam, iubēbāminī, iubēbāmur, iubēbāmus, iubēbant, iubēbantur, iubēbar, iubēbāre, iubēbāris, iubēbās, iubēbat, iubēbātis, iubēbātur, iubēbere, iubēberis, iubēbiminī, iubēbimur, iubēbimus, iubēbis, iubēbit, iubēbitis, iubēbitur, iubēbō, iubēbor, iubēbunt, iubēbuntur, iubēminī, iubēmur, iubēmus, iubendī, iubendō, iubendum, iubendus, iubēns, iubent, iubentō, iubentor, iubentur, iubeō, iubeor, iubēre, iubērem, iubērēminī, iubērēmur, iubērēmus, iubērent, iubērentur, iubērer, iubērere, iubērēris, iubērēs, iubēret, iubērētis, iubērētur, iubērī, iubēris, iubēs, iubet, iubēte, iubētis, iubētō, iubētor, iubētōte, iubētur, iussa, iussā, iussae, iussam, iussārum, iussās, iusse, iusseram, iusserāmus, iusserant, iusserās, iusserat, iusserātis, iussēre, iusserim, iusserimus, iusserīmus, iusserint, iusseris, iusserīs, iusserit, iusseritis, iusserītis, iusserō, iussērunt, iussī, iussimus, iussīs, iussisse, iussissem, iussissēmus, iussissent, iussissēs, iussisset, iussissētis, iussistī, iussistis, iussit, iussō, iussōrum, iussōs, iussū, iussum, iussūrus, iussus* — “order”;

*momorderam, momorderāmus, momorderant, momorderās, momorderat, momorderātis, momordēre, momorderim, momorderimus, momorderīmus, momorderint, momorderis, momorderīs, momorderit, momorderitis, momorderītis, momorderō, momordērunt, momordī, momordimus, momordisse, momordissem, momordissēmus, momordissent, momordissēs, momordisset, momordissētis, momordistī, momordistis, momordit, mordē, mordeam, mordeāminī, mordeāmur, mordeāmus, mordeant, mordeantur, mordeat, mordeāre, mordeāris, mordeās, mordeat, mordeātis, mordeātur, mordēbam, mordēbāminī, mordēbāmur, mordēbāmus, mordēbant, mordēbantur, mordēbar, mordēbāre, mordēbāris, mordēbās, mordēbat, mordēbātis, mordēbātur, mordēbere, mordēberis, mordēbiminī, mordēbimur, mordēbimus, mordēbis, mordēbit, mordēbitis, mordēbitur, mordēbō, mordēbor, mordēbunt, mordēbuntur, mordēminī, mordēmur, mordēmus, mordendī, mordendō, mordendum, mordendus, mordēns, mordent, mordentō, mordentor, mordentur, mordeō, mordeor, mordēre, mordērem, mordērēminī, mordērēmur, mordērēmus, mordērent, mordērentur, mordērer, mordērere, mordērēris, mordērēs, mordēret, mordērētis, mordērētur, mordērī, mordēris, mordēs, mordet, mordēte, mordētis, mordētō, mordētor, mordētōte, mordētur, morsa, morsā, morsae, morsam, morsārum, morsās, morse, morsī, morsīs, morsō, morsōrum, morsōs, morsū, morsum, morsūrus, morsus* — “bite”;

*monē, moneam, moneāminī, moneāmur, moneāmus, moneant, moneantur, moneat, moneāre, moneāris, moneās, moneat, moneātis, moneātur, monēbam, monēbāminī, monēbāmur, monēbāmus, monēbant, monēbantur, monēbar, monēbāre, monēbāris, monēbās, monēbat, monēbātis, monēbātur, monēbere, monēberis, monēbiminī, monēbimur, monēbimus, monēbis, monēbit, monēbitis, monēbitur, monēbō, monēbor, monēbunt, monēbuntur, monēminī, monēmur, monēmus, monendī, monendō, monendum, monendus, monēns, monent, monentō, monentor, monentur, moneō, moneor, monēre, monērem, monērēminī, monērēmur, monērēmus, monērent, monērentur, monērer, monērere, monērēris, monērēs, monēret, monērētis, monērētur, monērī, monēris, monēs, monet, monēte, monētis, monētō, monētor, monētōte, monētur, monitū, monitum, monitūrus, monitus, monueram, monuerāmus, monuerant, monuerās, monuerat, monuerātis, monuēre, monuerim, monuerimus, monuerīmus, monuerint, monueris, monuerīs, monuerit, monueritis, monuerītis, monuerō, monuērunt, monuī, monuimus, monuisse, monuissem, monuissēmus, monuissent, monuissēs, monuisset, monuissētis, monuistī, monuistis, monuit* — “warn”;

*polliceāminī, polliceāmur, polliceantur, polliceat, polliceāre, polliceāris, polliceātur, pollicēbāminī, pollicēbāmur, pollicēbantur, pollicēbar, pollicēbāre, pollicēbāris, pollicēbātur, pollicēbere, pollicēberis, pollicēbiminī, pollicēbimur, pollicēbitur, pollicēbor, pollicēbuntur, pollicēminī, pollicēmur, pollicendī, pollicendō, pollicendum, pollicendus, pollicēns, pollicentor, pollicentur, polliceor, pollicēre, pollicērēminī, pollicērēmur, pollicērentur, pollicērer, pollicērere, pollicērēris, pollicērētur, pollicērī, pollicēris, pollicētor, pollicētur, pollicita, pollicitā, pollicitae, pollicitam, pollicitārum, pollicitās, pollicite, polliciti, pollicitīs, pollicitō, pollicitōrum, pollicitōs, pollicitū, pollicitum, pollicitūrus, pollicitus* — “promise”;

*spondē, spondeam, spondeāminī, spondeāmur, spondeāmus, spondeant, spondeantur, spondeat, spondeāre, spondeāris, spondeās, spondeat, spondeātis, spondeātur, spondēbam, spondēbāminī, spondēbāmur, spondēbāmus, spondēbant, spondēbantur, spondēbar, spondēbāre, spondēbāris, spondēbās, spondēbat, spondēbātis, spondēbātur, spondēbere, spondēberis, spondēbiminī, spondēbimur, spondēbimus, spondēbis, spondēbit, spondēbitis, spondēbitur, spondēbō, spondēbor, spondēbunt, spondēbuntur, spondēminī, spondēmur, spondēmus, spondendī, spondendō, spondendum, spondendus, spondēns, spondent, spondentō, spondentor, spondentur, spondeō, spondeor, spondēre, spondērem, spondērēminī, spondērēmur, spondērēmus, spondērent, spondērentur, spondērer,*

*spondērēre, spondērēris, spondērēs, spondēret, spondērētis, spondērētur, spondērī, spondēris, spondēs, spondet, spondēte, spondētis, spondētō, spondētor, spondētōte, spondētur, spōnse, spōnsī, spōnsis, spōnsō, spōnsōrum, spōnsōs, spōnsū, spōnsum, spōnsūrus, spōnsus, sponponderam, sponponderāmus, sponponderant, sponponderās, sponponderat, sponponderātis, sponpondēre, sponponderim, sponponderimus, sponponderīmus, sponponderint, sponponderis, sponponderīs, sponponderit, sponponderitis, sponponderītis, sponponderō, sponpondērunt, sponpondī, sponpondimus, sponpondisse, sponpondissem, sponpondissēmus, sponpondissent, sponpondissēs, sponpondisset, sponpondissētis, sponpondistī, sponpondistis, sponpondit* — “vow”;

*stridē, strideam, strideāminī, strideāmur, strideāmus, strideant, strideantur, stridear, strideāre, strideāris, strideās, strideat, strideātis, strideātur, stridēbam, stridēbāminī, stridēbāmur, stridēbāmus, stridēbant, stridēbantur, stridēbar, stridēbāre, stridēbāris, stridēbās, stridēbat, stridēbātis, stridēbātur, stridēbere, stridēberis, stridēbiminī, stridēbimur, stridēbimus, stridēbis, stridēbit, stridēbitis, stridēbitur, stridēbō, stridēbor, stridēbunt, stridēbuntur, stridēminī, stridēmur, stridēmus, stridendī, stridendō, stridendum, stridendus, stridēns, strident, stridentō, stridentor, stridentur, strideō, strideor, stridēre, stridērem, stridērēminī, stridērēmur, stridērēmus, stridērent, stridērentur, stridērer, stridērēre, stridērēris, stridērēs, stridēret, stridērētis, stridērētur, stridērī, stridēris, stridēs, stridet, stridēte, stridētis, stridētō, stridētor, stridētōte, stridētur, stridū, stridum, stridūrus* — “hiss”;

*tenē, teneam, teneāminī, teneāmur, teneāmus, teneant, teneantur, tenear, teneāre, teneāris, teneās, teneat, teneātis, teneātur, tenēbam, tenēbāminī, tenēbāmur, tenēbāmus, tenēbant, tenēbantur, tenēbar, tenēbāre, tenēbāris, tenēbās, tenēbat, tenēbātis, tenēbātur, tenēbere, tenēberis, tenēbiminī, tenēbimur, tenēbimus, tenēbis, tenēbit, tenēbitis, tenēbitur, tenēbō, tenēbor, tenēbunt, tenēbuntur, tenēminī, tenēmur, tenēmus, tenendī, tenendō, tenendum, tenendus, tenēns, tenent, tenentō, tenentor, tenentur, teneō, teneor, tenēre, tenērem, tenērēminī, tenērēmur, tenērēmus, tenērent, tenērentur, tenērer, tenērēre, tenērēris, tenērēs, tenēret, tenērētis, tenērētur, tenērī, tenēris, tenēs, tenet, tenēte, tenētis, tenētō, tenētor, tenētōte, tenētur, tenueram, tenuerāmus, tenuerant, tenuerās, tenuerat, tenuerātis, tenuēre, tenuerim, tenuerimus, tenuerīmus, tenuerint, tenueris, tenuerīs, tenuerit, tenueritis, tenuerītis, tenuerō, tenuērunt, tenuī, tenuimus, tenuisse, tenuissem, tenuissēmus, tenuissent, tenuissēs, tenuisset, tenuissētis, tenuistī, tenuistis, tenuit* — “hold”;

*terrē, terream, terreāminī, terreāmur, terreāmus, terreat, terreatur, terrear, terreāre, terreāris, terreās, terreat, terreātis, terreātur, terrēbam, terrēbāminī, terrēbāmur, terrēbāmus, terrēbant, terrēbantur, terrēbar, terrēbāre, terrēbāris, terrēbās, terrēbat, terrēbātis, terrēbātur, terrēbere, terrēberis, terrēbiminī, terrēbimur, terrēbimus, terrēbis, terrēbit, terrēbitis, terrēbitur, terrēbō, terrēbor, terrēbunt, terrēbuntur, terrēminī, terrēmur, terrēmus, terrendī, terrendō, terrendum, terrendus, terrēns, terrent, terrentō, terrentor, terrentur, terreō, terreor, terrēre, terrērem, terrērēminī, terrērēmur, terrērēmus, terrērent, terrērentur, terrērer, terrērēre, terrērēris, terrērēs, terrēret, terrērētis, terrērētur, terrērī, terrēris, terrēs, terret, terrēte, terrētis, terrētō, terrētor, terrētōte, terrētur, territa, territā, territae, territam, territārum, territās, territe, territī, territīs, territō, territōrum, territōs, territū, territum, territūrus, territus, terrueram, terruerāmus, terruerant, terruerās, terruerat, terruerātis, terruēre, terruerim, terruerimus, terruerīmus, terruerint, terrueris, terruerīs, terruerit, terrueritis, terruerītis, terruerō, terruērunt, terruī, terruimus, terruisse, terruissem, terruissēmus, terruissent, terruissēs, terruisset, terruissētis, terruistī, terruistis, terruit* — “frighten”;

*vidē, videam, videāminī, videāmur, videāmus, videant, videantur, videar, videāre, videāris, videās, videat, videātis, videātur, vidēbam, vidēbāminī, vidēbāmur, vidēbāmus, vidēbant, vidēbantur, vidēbar, vidēbāre, vidēbāris, vidēbās, vidēbat, vidēbātis, vidēbātur, vidēbere, vidēberis, vidēbiminī, vidēbimur, vidēbimus, vidēbis, vidēbit, vidēbitis, vidēbitur, vidēbō, vidēbor, vidēbunt, vidēbuntur, vidēminī, vidēmur, vidēmus, videndī, videndō, videndum, videndus, vidēns, vident, videntō, videntor, videntur, videō, videor, videram, viderāmus, viderant, viderās, viderat, viderātis, vidēre, vidēre, vidērem, vidērēminī, vidērēmur, vidērēmus, vidērent, vidērentur, vidērer, vidērēre, vidērēris, vidērēs, vidēret, vidērētis, vidērētur, vidērī, viderim, viderimus, viderīmus, viderint, vidēris, videris, viderīs, viderit, videritis, viderītis, viderō, viderunt, vidēs, videt, vidēte, vidētis, vidētō, vidētor, vidētōte, vidētur, vīdī, vīdimus, vīdisse, vīdissem, vīdissēmus, vīdissent, vīdissēs, vīdisset, vīdissētis, vīdistī, vīdistis, vīdit, vīsa, vīsā, vīsae, vīsam, vīsarum, vīsās, vīse, vīsī, vīsīs, vīsō, vīsōrum, vīsōs, vīsū, vīsum, vīsūrus, vīsus* — “see”.

[https://en.wikipedia.org/wiki/Latin\\_conjugation#Third\\_conjugation](https://en.wikipedia.org/wiki/Latin_conjugation#Third_conjugation)

*ācta, āctā, āctae, āctam, āctārum, āctās, ācte, āctī, āctīs, āctō, āctōrum, āctōs, āctū, āctum, āctūrus, āctus, agam, agāminī, agāmur, agāmus, agant, agantur, agar, agāre, agāris, agās, agat, agātis, agātur, age, agēbam, agēbāminī, agēbāmur, agēbāmus, agēbant, agēbantur, agēbar, agēbāre, agēbāris, agēbās, agēbat, agēbātis, agēbātur, agēminī, agēmur, agēmus, agendī, agendō, agendum, agendus, agēns, agent, agentur, agere, agēre, agerem, agerēminī, agerēmur, agerēmus, agerent, agerentur, agerer, agerēre, agerēris, agerēs, ageret, agerētis,*

*ageretur, ageris, agēris, agēs, aget, agētis, agētur, agī, agiminī, agimur, agimus, agis, agit, agite, agitis, agitō, agitor, agitōte, agitur, agō, agor, agunt, aguntō, aguntor, aguntur, ēgeram, ēgerāmus, ēgerant, ēgerās, ēgerat, ēgerātis, ēgēre, ēgerim, ēgerimus, ēgerīmus, ēgerint, ēgeris, ēgerīs, ēgerit, ēgeritis, ēgerītis, ēgerō, ēgerunt, ēgī, ēgimus, ēgisse, ēgisse, ēgissēmus, ēgissent, ēgissēs, ēgisset, ēgissētis, ēgistī, ēgistis, ēgit* — “drive”;

*adhaerēscam, adhaerēscāminī, adhaerēscāmur, adhaerēscāmus, adhaerēscant, adhaerēscantur, adhaerēscar, adhaerēscāre, adhaerēscāris, adhaerēscās, adhaerēscat, adhaerēscātis, adhaerēscātur, adhaerēsce, adhaerēscēbam, adhaerēscēbāminī, adhaerēscēbāmur, adhaerēscēbāmus, adhaerēscēbant, adhaerēscēbantur, adhaerēscēbar, adhaerēscēbāre, adhaerēscēbāris, adhaerēscēbās, adhaerēscēbat, adhaerēscēbātis, adhaerēscēbātur, adhaerēscēminī, adhaerēscēmur, adhaerēscēmus, adhaerēscendī, adhaerēscendō, adhaerēscendum, adhaerēscendus, adhaerēscēns, adhaerēscēt, adhaerēscētur, adhaerēscere, adhaerēscēre, adhaerēscerem, adhaerēscerēminī, adhaerēscerēmur, adhaerēscerēmus, adhaerēscerent, adhaerēscerentur, adhaerēscerer, adhaerēscerēre, adhaerēscerēris, adhaerēscerēs, adhaerēsceret, adhaerēscerētis, adhaerēscerētur, adhaerēsceris, adhaerēscēris, adhaerēscēs, adhaerēscet, adhaerēscētis, adhaerēscētur, adhaerēscī, adhaerēsciminī, adhaerēscimur, adhaerēscimus, adhaerēscis, adhaerēscit, adhaerēscite, adhaerēscitis, adhaerēscitō, adhaerēscitor, adhaerēscitōte, adhaerēscitur, adhaerēscō, adhaerēscor, adhaerēscunt, adhaerēscuntō, adhaerēscuntor, adhaerēscuntur* — “adhere”;

*adolēscam, adolēscāminī, adolēscāmur, adolēscāmus, adolēscant, adolēscantur, adolēscar, adolēscāre, adolēscāris, adolēscās, adolēscat, adolēscātis, adolēscātur, adolēsce, adolēscēbam, adolēscēbāminī, adolēscēbāmur, adolēscēbāmus, adolēscēbant, adolēscēbantur, adolēscēbar, adolēscēbāre, adolēscēbāris, adolēscēbās, adolēscēbat, adolēscēbātis, adolēscēbātur, adolēscēminī, adolēscēmur, adolēscēmus, adolēscendī, adolēscendō, adolēscendum, adolēscendus, adolēscēns, adolēscēt, adolēscētur, adolēscere, adolēscēre, adolēscerem, adolēscerēminī, adolēscerēmur, adolēscerēmus, adolēscerent, adolēscerentur, adolēscerer, adolēscerēre, adolēscerēris, adolēscerēs, adolēsceret, adolēscerētis, adolēscerētur, adolēsceris, adolēscēris, adolēscēs, adolēscet, adolēscētis, adolēscētur, adolēscī, adolēsciminī, adolēscimur, adolēscimus, adolēscis, adolēscit, adolēscite, adolēscitis, adolēscitō, adolēscitor, adolēscitōte, adolēscitur, adolēscō, adolēscor, adolēscunt, adolēscuntō, adolēscuntor, adolēscuntur, adolēveram, adolēverāmus, adolēverant, adolēverās, adolēverat, adolēverātis, adolēvēre, adolēverim, adolēverimus, adolēverīmus, adolēverint, adolēveris, adolēverīs, adolēverit, adolēveritis, adolēverītis, adolēverō, adolēverunt, adolēvī, adolēvimus, adolēvisse, adolēvissem, adolēvissēmus, adolēvissent, adolēvissēs, adolēvisset, adolēvissētis, adolēvistī, adolēvistis, adolēvit, adulta, adultā, adultae, adultam, adultārum, adultās, adulte, adultī, adultīs, adultō, adultōrum, adultōs, adultū, adultum, adultūrus, adultus* — “mature”;

*caedam, caedāminī, caedāmur, caedāmus, caedant, caedantur, caedar, caedāre, caedāris, caedās, caedat, caedātis, caedātur, caede, caedēbam, caedēbāminī, caedēbāmur, caedēbāmus, caedēbant, caedēbantur, caedēbar, caedēbāre, caedēbāris, caedēbās, caedēbat, caedēbātis, caedēbātur, caedēminī, caedēmur, caedēmus, caedendī, caedendō, caedendum, caedendus, caedēns, caedent, caedentur, caedere, caedēre, caederem, caederēminī, caederēmur, caederēmus, caederent, caederentur, caederer, caederēre, caederēris, caederēs, caederet, caederētis, caederētur, caederis, caedēris, caedēs, caedet, caedētis, caedētur, caedī, caediminī, caedimur, caedimus, caedis, caedit, caedite, caeditis, caeditō, caeditor, caeditōte, caeditur, caedō, caedor, caedunt, caeduntō, caeduntor, caeduntur, caesa, caesā, caesae, caesam, caesārum, caesās, caese, caesī, caesīs, caesō, caesōrum, caesōs, caesū, caesum, caesūrus, caesus, cecīderam, cecīderāmus, cecīderant, cecīderās, cecīderat, cecīderātis, cecīdēre, cecīderim, cecīderimus, cecīderīmus, cecīderint, cecīderis, cecīderīs, cecīderit, cecīderitis, cecīderītis, cecīderō, cecīderunt, cecīdī, cecīdimus, cecīdisse, cecīdissem, cecīdissēmus, cecīdissent, cecīdissēs, cecīdisset, cecīdissētis, cecīdistī, cecīdistis, cecīdit* — “kill”;

*carpam, carpāminī, carpāmur, carpāmus, carpant, carpantur, carpar, carpāre, carpāris, carpās, carpat, carpātis, carpātur, carpe, carpēbam, carpēbāminī, carpēbāmur, carpēbāmus, carpēbant, carpēbantur, carpēbar, carpēbāre, carpēbāris, carpēbās, carpēbat, carpēbātis, carpēbātur, carpēminī, carpēmur, carpēmus, carpendī, carpendō, carpendum, carpendus, carpēns, carper, carperentur, carpere, carpēre, carperem, carperēminī, carperēmur, carperēmus, carperent, carperentur, carperer, carperēre, carperēris, carperēs, carperet, carperētis, carperētur, carperis, carpēris, carpēs, carpet, carpētis, carpētur, carpī, carpiminī, carpimur, carpimus, carpis, carpit, carpite, carpitis, carpitō, carpitōte, carpitur, carpō, carpor, carpseram, carpsērāmus, carpsērant, carpsērās, carpsērat, carpsērātis, carpsēre, carpsērim, carpsērimus, carpsērīmus, carpsērīnt, carpsēris, carpsērīs, carpsērit, carpsēritis, carpsērītis, carpsērō, carpsērunt, carpsī, carpsīmus, carpsisse, carpsissem, carpsissēmus, carpsissent, carpsissēs, carpsisset, carpsissētis, carpsistī, carpsistis, carpsit, carpta, carptā, carptae, carptam, carptārum, carptās, carpte, carptī, carptīs, carptō, carptōrum, carptōs, carptū, carptum, carptūrus, carptus, carpunt, carpuntō, carpuntor, carpuntur* — “pluck”;

*colam, colāminī, colāmur, colāmus, colant, colantur, colar, colāre, colāris, colās, colat, colātis, colātur, cole, colēbam, colēbāminī, colēbāmur, colēbāmus, colēbant, colēbantur, colēbar, colēbāre, colēbāris, colēbās, colēbat, colēbātis, colēbātur, colēminī, colēmur, colēmus, colendī, colendō, colendum, colendus, colēns, colent, colentur, colere, colēre, colerem, colerēminī, colerēmur, colerēmus, colerent, colerentur, colerer, colerēre, colerēris, colerēs, coleret, colerētis, colerētur, coleris, colēris, colēs, colet, colētis, colētur, colī, coliminī, colimur, colimus, colis, colit, colite, colitis, colitō, colitor, colitōte, colitur, colō, color, colueram, coluerāmus, coluerant, coluerās, coluerat, coluerātis, coluēre, coluerim, coluerimus, coluerīmus, coluerint, colueris, colueris, coluerit, colueritis, coluerītis, coluerō, coluērunt, coluī, coluimus, coluisse, coluissem, coluissēmus, coluissent, coluissēs, coluisset, coluissētis, coluistī, coluistis, coluit, colunt, coluntō, coluntor, coluntur, culta, cultā, cultae, cultam, cultārum, cultās, culte, cultī, cultis, cultō, cultōrum, cultōs, cultū, cultum, cultūrus, cultus* — “cultivate”;

*cucurreram, cucurrerāmus, cucurrerant, cucurrerās, cucurrerat, cucurrerātis, cucurrēre, cucurrerim, cucurrerimus, cucurrerīmus, cucurrerint, cucurreris, cucurrerīs, cucurrerit, cucurreritis, cucurrerītis, cucurrerō, cucurrērunt, cucurrī, cucurrimus, cucurrisse, cucurrissem, cucurrissēmus, cucurrissent, cucurrissēs, cucurrisset, cucurrissētis, cucurristī, cucurristis, cucurrit, curram, currāminī, currāmur, currāmus, currant, currantur, currar, currāre, currāris, currās, currat, currātis, currātur, curre, currēbam, currēbāminī, currēbāmur, currēbāmus, currēbant, currēbantur, currēbar, currēbāre, currēbāris, currēbās, currēbat, currēbātis, currēbātur, currēminī, currēmur, currēmus, currendī, currendō, currendum, currendus, currēns, current, currentur, currere, currēre, currerem, currerēminī, currerēmur, currerēmus, currerent, currerentur, currerer, currerēre, currerēris, currerēs, curreret, currerētis, currerētur, curreris, currēris, currēs, curret, currētis, currētur, currī, curriminī, currimur, currimus, curris, currit, currite, curritis, curritō, curritor, curritōte, curritur, currō, curror, currunt, curruntō, curruntor, curruntur, cursa, cursā, cursae, cursam, cursārum, cursās, curse, cursī, cursīs, cursō, cursōrum, cursōs, cursū, cursum, cursūrus, cursus* — “run”;

*emam, emāminī, emāmur, emāmus, emant, emantur, emar, emāre, emāris, emās, emat, emātis, emātur, eme, emēbam, emēbāminī, emēbāmur, emēbāmus, emēbant, emēbantur, emēbar, emēbāre, emēbāris, emēbās, emēbat, emēbātis, emēbātur, emēminī, emēmur, emēmus, emendī, emendō, emendum, emendus, emēns, ement, ementur, ēmeram, ēmerāmus, ēmerant, ēmerās, ēmerat, ēmerātis, emere, emēre, emēre, emerem, emerēminī, emerēmur, emerēmus, emerent, emerentur, emerer, emerēre, emerēris, emerēs, emeret, emerētis, emerētur, ēmerim, ēmerimus, ēmerīmus, ēmerint, emeris, emēris, ēmeris, ēmeris, ēmerit, ēmeritis, ēmerītis, ēmerō, emērunt, emēs, emet, emētis, emētur, emī, emī, emiminī, emimur, emimus, emimus, emīs, emisse, emissem, emissēmus, emissent, emissēs, emisset, emissētis, emistī, emistis, emit, emīt, emite, emitis, emitō, emitō, emitō, emitō, emitō, emitō, emō, emor, empta, emptā, emptae, emptam, emptārum, emptās, empte, emptī, emptīs, emptō, emptōrum, emptōs, emptū, emptum, emptum, emptūrus, emptus, emptus, emunt, emuntō, emuntor, emuntur* — “buy”;

*flectam, flectāminī, flectāmur, flectāmus, flectant, flectantur, flectar, flectāre, flectāris, flectās, flectat, flectātis, flectātur, flecte, flectēbam, flectēbāminī, flectēbāmur, flectēbāmus, flectēbant, flectēbantur, flectēbar, flectēbāre, flectēbāris, flectēbās, flectēbat, flectēbātis, flectēbātur, flectēminī, flectēmur, flectēmus, flectendī, flectendō, flectendum, flectendus, flectēns, flectent, flectentur, flectere, flectēre, flecterem, flecterēminī, flecterēmur, flecterēmus, flecterent, flecterentur, flecterer, flecterēre, flecterēris, flecterēs, flecteret, flecterētis, flecterētur, flecteris, flectēris, flectēs, flectet, flectētis, flectētur, flectī, flectiminī, flectimur, flectimus, flectis, flectit, flectite, flectitis, flectitō, flectitor, flectitōte, flectitur, flectō, flector, flectunt, flectuntō, flectuntor, flectuntur, flexa, flexā, flexae, flexam, flexārum, flexās, flexe, flexeram, flexerāmus, flexerant, flexerās, flexerat, flexerātis, flexēre, flexerim, flexerimus, flexerīmus, flexerint, flexeris, flexeris, flexerit, flexeritis, flexerītis, flexerō, flexērunt, flexī, fleximus, flexis, flexisse, flexissem, flexissēmus, flexissent, flexissēs, flexisset, flexissētis, flexistī, flexistis, flexit, flexō, flexōrum, flexōs, flexū, flexum, flexūrus, flexus* — “bend”;

*flōrēscam, flōrēscāminī, flōrēscāmur, flōrēscāmus, flōrēscant, flōrēscantur, flōrēscar, flōrēscāre, flōrēscāris, flōrēscās, flōrēscat, flōrēscātis, flōrēscātur, flōrēsce, flōrēscēbam, flōrēscēbāminī, flōrēscēbāmur, flōrēscēbāmus, flōrēscēbant, flōrēscēbantur, flōrēscēbar, flōrēscēbāre, flōrēscēbāris, flōrēscēbās, flōrēscēbat, flōrēscēbātis, flōrēscēbātur, flōrēscēminī, flōrēscēmur, flōrēscēmus, flōrēscendī, flōrēscendō, flōrēscendum, flōrēscendus, flōrēscēns, flōrēscēnt, flōrēscēntur, flōrēscere, flōrēscēre, flōrēscerem, flōrēscerēminī, flōrēscerēmur, flōrēscerēmus, flōrēscerent, flōrēscerentur, flōrēscerer, flōrēscerēre, flōrēscerēris, flōrēscerēs, flōrēsceret, flōrēscerētis, flōrēscerētur, flōrēsceris, flōrēscēris, flōrēscēs, flōrēscet, flōrēscētis, flōrēscētur, flōrēscī, flōrēsciminī, flōrēscimur, flōrēscimus, flōrēscis, flōrēscit, flōrēscite, flōrēscitis, flōrēscitō, flōrēscitor, flōrēscitōte, flōrēscitur, flōrēscō, flōrēscor, flōrēscunt, flōrēscuntō, flōrēscuntor, flōrēscuntur* — “blossom”;

*fūderam, fūderāmus, fūderant, fūderās, fūderat, fūderātis, fūdēre, fūderim, fūderimus, fūderīmus, fūderint, fūderis, fūderis, fūderit, fūderitis, fūderītis, fūderō, fūderunt, fūdī, fūdīmus, fūdisse, fūdissem, fūdissēmus, fūdisset,*

*fūdissēs, fūdisset, fūdissētis, fūdistī, fūdistis, fūdit, fundam, fundāmus, fundant, fundantur, fundās, fundat, fundātis, fundātur, funde, fundēbam, fundēbāmus, fundēbant, fundēbantur, fundēbās, fundēbat, fundēbātis, fundēbātur, fundēmus, fundendī, fundendō, fundendum, fundendus, fundēns, fundent, fundentur, fundere, funderem, funderēmus, funderent, funderentur, funderēs, funderet, funderētis, funderētur, fundēs, fundet, fundētis, fundētur, fundī, fundīmus, fundis, fundit, fundite, funditis, funditō, fundiōte, funditur, fundō, fundunt, funduntō, funduntur, fūsa, fūsā, fūsae, fūsam, fūsārum, fūsās, fūse, fūsi, fūsis, fūsō, fūsōrum, fūsōs, fūsū, fūsūm, fūsūrus, fūsus* — “pour”;

*genita, genitā, genitae, genitam, genitārum, genitās, genite, geniū, genitīs, genitō, genitōrum, genitōs, genitū, genitum, geniūrus, genitus, genueram, genuerāmus, genuerant, genuerās, genuerat, genuerātis, genuēre, genuerim, genuerimus, genuerīmus, genuerint, genueris, genuerīs, genuerit, genueritis, genuerītis, genuerō, genuerunt, genuī, genuimus, genuisse, genuissem, genuissēmus, genuissent, genuissēs, genuisset, genuissētis, genuistī, genuistis, genuit, gignam, gignāminī, gignāmur, gignāmus, gignant, gignantur, gignar, gignāre, gignāris, gignās, gignat, gignātis, gignātur, gigne, gignēbam, gignēbāminī, gignēbāmur, gignēbāmus, gignēbant, gignēbantur, gignēbar, gignēbare, gignēbāris, gignēbās, gignēbat, gignēbātis, gignēbātur, gignēminī, gignēmur, gignēmus, gignendī, gignendō, gignendum, gignendus, gignēns, gignent, gignentur, gignere, gignēre, gignerem, gignerēminī, gignerēmur, gignerēmus, gignerent, gignerentur, gignerer, gignerēre, gignerēris, gignerēs, gigneret, gignerētis, gignerētur, gigneris, gignēris, gignēs, gignet, gignētis, gignētur, gignī, gigniminī, gignimur, gignimus, gignis, gignit, gignite, gignitis, gignitō, gignitor, gignitōte, gignitur, gignō, gignor, gignunt, gignuntō, gignuntor, gignuntur* — “beget”;

*geram, gerāminī, gerāmur, gerāmus, gerant, gerantur, gerar, gerāre, gerāris, gerās, gerat, gerātis, gerātur, gere, gerēbam, gerēbāminī, gerēbāmur, gerēbāmus, gerēbant, gerēbantur, gerēbar, gerēbare, gerēbāris, gerēbās, gerēbat, gerēbātis, gerēbātur, gerēminī, gerēmur, gerēmus, gerendī, gerendō, gerendum, gerendus, gerēns, gerent, gerentur, gerere, gerēre, gererem, gererēminī, gererēmur, gererēmus, gererent, gererentur, gererer, gererēre, gererēris, gererēs, gereret, gererētis, gererētur, gereris, gerēris, gerēs, geret, gerētis, gerētur, gerī, geriminī, gerimur, gerimus, geris, gerit, gerite, geritis, geritō, geritor, geritōte, geritur, gerō, geror, gerunt, geruntō, geruntor, geruntur, gesseram, gesserāmus, gesserant, gesserās, gesserat, gesserātis, gessēre, gesserim, gesserimus, gesserīmus, gesserint, gesseris, gesserīs, gesserit, gesseritis, gesserītis, gesserō, gesserunt, gessī, gessimus, gessisse, gessissem, gessissēmus, gessissent, gessissēs, gessisset, gessissētis, gessistī, gessistis, gessit, gesta, gestā, gestae, gestam, gestārum, gestās, geste, gestī, gestīs, gestō, gestōrum, gestōs, gestū, gestum, gestūrus, gestus* — “wear”;

*īcam, īcāminī, īcāmur, īcāmus, īcant, īcantur, īcar, īcāre, īcāris, īcās, īcat, īcātis, īcātur, īce, īcēbam, īcēbāminī, īcēbāmur, īcēbāmus, īcēbant, īcēbantur, īcēbar, īcēbare, īcēbāris, īcēbās, īcēbat, īcēbātis, īcēbātur, īcēminī, īcēmur, īcēmus, īcendī, īcendō, īcendum, īcendus, īcēns, īcent, īcentur, īceram, īcerāmus, īcerant, īcerās, īcerat, īcerātis, īcere, īcēre, īcerem, īcerēminī, īcerēmur, īcerēmus, īcerent, īcerentur, īcerer, īcerēre, īcerēris, īcerēs, īceret, īcerētis, īcerētur, īcerim, īcerimus, īcerīmus, īcerint, īceris, īcerīs, īcēris, īcerit, īceritis, īcerītis, īcerō, īcērunt, īcēs, īcet, īcētis, īcētur, īcī, īciminī, īcimur, īcimus, īcis, īcisse, īcissem, īcissēmus, īcissent, īcissēs, īcisset, īcissētis, īcistī, īcistis, īcit, īcite, īcitis, īcitō, īcitor, īcitōte, īcitur, īcō, īcor, īcta, īctā, īctae, īctam, īctārum, īctās, īcte, īctī, īctīs, īctō, īctōrum, īctōs, īctū, īctum, īctūrus, īctus, īcunt, īcuntō, īcuntor, īcuntur* — “strike”;

*lēcta, lēctā, lēctae, lēctam, lēctārum, lēctās, lēcte, lēctī, lēctīs, lēctō, lēctōrum, lēctōs, lēctū, lēctum, lēctūrus, lēctus, legam, legāminī, legāmur, legāmus, legant, legantur, legar, legāre, legāris, legās, legat, legātis, legātur, lege, legēbam, legēbāminī, legēbāmur, legēbāmus, legēbant, legēbantur, legēbar, legēbare, legēbāris, legēbās, legēbat, legēbātis, legēbātur, legēminī, legēmur, legēmus, legendī, legendō, legendum, legendus, legēns, legent, legentur, lēgeram, lēgerāmus, lēgerant, lēgerās, lēgerat, lēgerātis, legere, legēre, lēgēre, legerem, legerēminī, legerēmur, legerēmus, legerent, legerentur, legerer, legerēre, legerēris, legerēs, legeret, legerētis, legerētur, lēgerim, lēgerimus, lēgerīmus, lēgerint, legeris, legēris, lēgeris, lēgerīs, lēgerit, lēgeritis, lēgerītis, lēgerō, lēgērunt, legēs, leget, legētis, legētur, legī, lēgī, legiminī, legimur, legimus, lēgimus, legis, lēgisse, lēgisse, lēgissēmus, lēgissent, lēgissēs, lēgisset, lēgissētis, lēgistī, lēgistis, legit, lēgit, legite, legitis, legitō, legitor, legitōte, legitur, legō, legor, legunt, leguntō, leguntor, leguntur* — “read”;

*lēveram, lēverāmus, lēverant, lēverās, lēverat, lēverātis, lēvēre, lēverim, lēverimus, lēverīmus, lēverint, lēveris, lēverīs, lēverit, lēveritis, lēverītis, lēverō, lēvērunt, lēvī, lēvimus, lēvisse, lēvissem, lēvissēmus, lēvissent, lēvissēs, lēvisset, lēvissētis, lēvistī, lēvistis, lēvit, linam, lināminī, lināmur, lināmus, linant, linantur, linar, lināre, lināris, linās, linat, linātis, linātur, line, linēbam, linēbāminī, linēbāmur, linēbāmus, linēbant, linēbantur, linēbar, linēbare, linēbāris, linēbās, linēbat, linēbātis, linēbātur, linēminī, linēmur, linēmus, linendī, linendō, linendum, linendus, linēns, linent, linentur, linere, linēre, linerem, linerēminī, linerēmur, linerēmus, linerent, linerentur, linerer, linerēre, linerēris, linerēs, lineret, linerētis, linerētur, lineris, linēris, linēs, linet, linētis, linētur, linī, līnīminī, līnimur, līnimus, līnis, līnit, līnite, līnitis, līnitō, līnitor, līnitōte, līnitur, līnō, līnor, līnunt, līnuntō, līnuntor, līnuntur, litū, litum, litūrus, litus* — “smear”;

*locūta, locūtā, locūtae, locūtam, locūtārum, locūtās, locūte, locūī, locūtīs, locūtō, locūtōrum, locūtōs, locūtū, locūtum, locūtūrus, locūtus, loquāminī, loquāmur, loquantur, loquar, loquāre, loquāris, loquātur, loquēbāminī, loquēbāmur, loquēbantur, loquēbar, loquēbāre, loquēbāris, loquēbātur, loquēminī, loquēmur, loquendī, loquendō, loquendum, loquendus, loquēns, loquentur, loquere, loquēre, loquerēminī, loquerēmur, loquerentur, loquerer, loquerēre, loquerēris, loquerētur, loqueris, loquēris, loquētur, loquī, loquiminī, loquimur, loquitur, loquitur, loquor, loquuntur, loquuntur* — “speak”;

*messa, messā, messae, messam, messārum, messās, messe, messī, messīs, messō, messōrum, messōs, messū, messueram, messuerāmus, messuerant, messuerās, messuerat, messuerātis, messuēre, messuerim, messuerimus, messuerīmus, messuerint, messueris, messuerīs, messuerit, messueritis, messuerītis, messuerō, messuērunt, messuī, messuimus, messuisse, messuisse, messuissēmus, messuissent, messuissēs, messuisset, messuissētis, messuistī, messuistis, messuīt, messum, messūrus, messus, metam, metāminī, metāmur, metāmus, metant, metantur, metar, metāre, metāris, metās, metat, metātis, metātur, mete, metēbam, metēbāminī, metēbāmur, metēbāmus, metēbant, metēbantur, metēbar, metēbāre, metēbāris, metēbās, metēbat, metēbātis, metēbātur, metēminī, metēmur, metēmus, metendī, metendō, metendum, metendus, metēns, metent, metentur, metere, metēre, meterem, meterēminī, meterēmur, meterēmus, meterent, meterentur, meterer, meterēre, meterēris, meterēs, meteret, meterētis, meterētur, meteris, metēris, metēs, metet, metētis, metētur, metī, metiminī, metimur, metimus, metis, metit, metite, metitis, metitō, metitor, metitōte, metitur, metō, metor, metunt, metuntō, metuntor, metuntur* — “reap”;

*mīseram, mīserāmus, mīserant, mīserās, mīserat, mīserātis, mīserē, mīserim, mīserimus, mīserīmus, mīserint, mīseris, mīserīs, mīserit, mīseritis, mīserītis, mīserō, mīserunt, mīsi, mīsimus, mīsisse, mīsissem, mīsissemus, mīsisissent, mīsisissēs, mīsisisset, mīsissettis, mīsisstī, mīsisstis, mīsit, missa, missā, missae, missam, missārum, missās, misse, missī, missīs, missō, missōrum, missōs, missū, missum, missūrus, missus, mittam, mittāminī, mittāmur, mittāmus, mittant, mittantur, mittar, mittāre, mittāris, mittās, mittat, mittātis, mittātur, mitte, mittēbam, mittēbāminī, mittēbāmur, mittēbāmus, mittēbant, mittēbantur, mittēbar, mittēbāre, mittēbāris, mittēbās, mittēbat, mittēbātis, mittēbātur, mittēminī, mittēmur, mittēmus, mittendī, mittendō, mittendum, mittendus, mittēns, mittent, mittentur, mittere, mittēre, mitterem, mitterēminī, mitterēmur, mitterēmus, mitterent, mitterentur, mitterer, mitterēre, mitterēris, mitterēs, mitteret, mitterētis, mitterētur, mitteris, mittēris, mittēs, mittet, mittētis, mittētur, mittī, mittiminī, mittimur, mittimus, mittis, mittit, mittite, mittitis, mittitō, mittitor, mittitōte, mittitur, mittō, mittor, mittunt, mittuntō, mittuntor, mittuntur* — “send”;

*nōscam, nōscāminī, nōscāmur, nōscāmus, nōscant, nōscantur, nōscar, nōscāre, nōscāris, nōscās, nōscat, nōscātis, nōscātur, nōsce, nōscēbam, nōscēbāminī, nōscēbāmur, nōscēbāmus, nōscēbant, nōscēbantur, nōscēbar, nōscēbāre, nōscēbāris, nōscēbās, nōscēbat, nōscēbātis, nōscēbātur, nōscēminī, nōscēmur, nōscēmus, nōscendī, nōscendō, nōscendum, nōscendus, nōscēns, nōscēt, nōscētur, nōscere, nōscēre, nōscerem, nōscerēminī, nōscerēmur, nōscerēmus, nōscerent, nōscerentur, nōscerer, nōscerēre, nōscerēris, nōscerēs, nōsceret, nōscerētis, nōscerētur, nōsceris, nōscēris, nōscēs, nōscet, nōscētis, nōscētur, nōscī, nōsciminī, nōscimur, nōscimus, nōscis, nōscit, nōscite, nōscitis, nōscitō, nōscitor, nōscitōte, nōscitur, nōscō, nōscor, nōscunt, nōscuntō, nōscuntor, nōscuntur, nōta, nōtā, nōtae, nōtam, nōtārum, nōtās, nōte, nōtī, nōtīs, nōtō, nōtōrum, nōtōs, nōtū, nōtum, nōtūrus, nōtus, nōveram, nōverāmus, nōverant, nōverās, nōverat, nōverātis, nōvēre, nōverim, nōverimus, nōverīmus, nōverint, nōveris, nōverīs, nōverit, nōveritis, nōverītis, nōverō, nōvērunt, nōvī, nōvimus, nōvisse, nōvissem, nōvissemus, nōvisissent, nōvisissēs, nōvisisset, nōvissettis, nōvistī, nōvistis, nōvit* — “know”;

*pāscam, pāscāminī, pāscāmur, pāscāmus, pāscant, pāscantur, pāscar, pāscāre, pāscāris, pāscās, pāscat, pāscātis, pāscātur, pāsce, pāscēbam, pāscēbāminī, pāscēbāmur, pāscēbāmus, pāscēbant, pāscēbantur, pāscēbar, pāscēbāre, pāscēbāris, pāscēbās, pāscēbat, pāscēbātis, pāscēbātur, pāscēminī, pāscēmur, pāscēmus, pāscendī, pāscendō, pāscendum, pāscendus, pāscēns, pāscēt, pāscētur, pāscere, pāscēre, pāscerem, pāscerēminī, pāscerēmur, pāscerēmus, pāscerent, pāscerentur, pāscerer, pāscerēre, pāscerēris, pāscerēs, pāsceret, pāscerētis, pāscerētur, pāsceris, pāscēris, pāscēs, pāscet, pāscētis, pāscētur, pāscī, pāsciminī, pāscimur, pāscimus, pāscis, pāscit, pāscite, pāscitis, pāscitō, pāscitor, pāscitōte, pāscitur, pāscō, pāscor, pāscunt, pāscuntō, pāscuntor, pāscuntur, pasta, pastā, pastae, pastam, pastārum, pastās, paste, pastī, pastīs, pastō, pastōrum, pastōs, pastū, pastum, pastūrus, pastus, pāveram, pāverāmus, pāverant, pāverās, pāverat, pāverātis, pāvēre, pāverim, pāverimus, pāverīmus, pāverint, pāveris, pāverīs, pāverit, pāveritis, pāverītis, pāverō, pāvērunt, pāvī, pāvimus, pāvisse, pāvissēmus, pāvissēmus, pāvissent, pāvissēs, pāvisset, pāvissētis, pāvistī, pāvistis, pāvīt* — “feed”;

*pellam, pellāminī, pellāmur, pellāmus, pellant, pellantur, pellar, pellāre, pellāris, pellās, pellat, pellātis, pellātur, pelle, pellēbam, pellēbāminī, pellēbāmur, pellēbāmus, pellēbant, pellēbantur, pellēbar, pellēbāre, pellēbāris, pellēbās, pellēbat, pellēbātis, pellēbātur, pellēminī, pellēmur, pellēmus, pellendī, pellendō, pellendum, pellendus, pellēns, pellent, pellentur, pellere, pellēre, pellerem, pellerēminī, pellerēmur, pellerēmus, pellerent, pellerentur,*



*trītam, trītārum, trītās, trīte, trīti, trītis, trītō, trītōrum, trītōs, trītū, trītum, trītūrus, trītus, trīveram, trīverāmus, trīverant, trīverās, trīverat, trīverātis, trīvēre, trīverim, trīverimus, trīverīmus, trīverint, trīveris, trīverīs, trīverit, trīveritīs, trīverītis, trīverō, trīvērunt, trīvī, trīvimus, trīvisse, trīvissem, trīvissēmus, trīvissent, trīvissēs, trīvisset, trīvissētis, trīvistī, trīvistis, trīvit* — “triture”;

*texam, texāminī, texāmur, texāmus, texant, texantur, texar, texāre, texāris, texās, texat, texātis, texātur, texe, texēbam, texēbāminī, texēbāmur, texēbāmus, texēbant, texēbantur, texēbar, texēbāre, texēbāris, texēbās, texēbat, texēbātis, texēbātur, texēminī, texēmur, texēmus, texendī, texendō, texendum, texendus, texēns, texent, texentur, texere, texēre, texerem, texerēminī, texerēmur, texerēmus, texerent, texerentur, texerer, texerēre, texerēris, texerēs, texeret, texerētis, texerētur, texeris, texēris, texēs, texet, texētis, texētur, texī, teximinī, teximur, teximus, texis, textit, textite, textitis, textitō, textitor, textitōte, textitur, texō, texor, texta, textā, textae, textam, textārum, textās, texte, textī, textīs, textō, textōrum, textōs, textū, textum, textūrus, textus, texueram, texuerāmus, texuerant, texuerās, texuerat, texuerātis, texuēre, texuerim, texuerimus, texuerīmus, texuerint, texueris, texuerīs, texuerit, texueritīs, texuerītis, texuerō, texuērunt, texuī, texuimus, texuuisse, texuissēmus, texuissent, texuissēs, texuisset, texuissētis, texuistī, texuistis, texuīt, texunt, texuntō, texuntor, texuntur* — “weave”;

*tracta, tractā, tractae, tractam, tractārum, tractās, tracte, tractī, tractīs, tractō, tractōrum, tractōs, tractū, tractum, tractūrus, tractus, traham, trahāminī, trahāmur, trahāmus, trahant, trahantur, trahar, trahāre, trahāris, trahās, trahat, trahātis, trahātur, trahe, trahēbam, trahēbāminī, trahēbāmur, trahēbāmus, trahēbant, trahēbantur, trahēbar, trahēbāre, trahēbāris, trahēbās, trahēbat, trahēbātis, trahēbātur, trahēminī, trahēmur, trahēmus, trahendī, trahendō, trahendum, trahendus, trahēns, trahent, trahentur, trahere, trahēre, traherem, traherēminī, traherēmur, traherēmus, traherent, traherentur, traherer, traherēre, traherēris, traherēs, traheret, traherētis, traherētur, traheris, trahēris, trahēs, trahet, trahētis, trahētur, trahī, trahiminī, trahimur, trahimus, trahis, trahit, trahite, trahitis, trahitō, trahitor, trahitōte, trahitur, trahō, trahor, trahunt, trahuntō, trahuntor, trahuntur* — “drag”;

*versa, versā, versae, versam, versārum, versās, verse, versī, versīs, versō, versōrum, versōs, versū, versum, versūrus, versus, vertam, vertāminī, vertāmur, vertāmus, vertant, vertantur, vertar, vertāre, vertāris, vertās, vertat, vertātis, vertātur, verte, vertēbam, vertēbāminī, vertēbāmur, vertēbāmus, vertēbant, vertēbantur, vertēbar, vertēbāre, vertēbāris, vertēbās, vertēbat, vertēbātis, vertēbātur, vertēminī, vertēmur, vertēmus, vertendī, vertendō, vertendum, vertendus, vertēns, vertent, vertentur, verteram, verterāmus, verterant, verterās, verterat, verterātis, vertere, vertēre, verterem, verterēminī, verterēmur, verterēmus, verterent, verterentur, verterer, verterēre, verterēris, verterēs, verteret, verterētis, verterētur, verterim, verterimus, verterīmus, verterint, verteris, verterīs, vertēris, verterit, verteritīs, verterītis, verterō, vertērunt, vertēs, vertet, vertētis, vertētur, vertī, vertiminī, vertimur, vertimus, vertis, vertisse, vertissem, vertissēmus, vertissent, vertissēs, vertisset, vertissētis, vertistī, vertistis, vertit, vertite, vertitis, vertitō, vertitor, vertitōte, vertitur, vertō, vertor, vertunt, vertuntō, vertuntor, vertuntur* — “turn”;

*vīceram, vīcerāmus, vīcerant, vīcerās, vīcerat, vīcerātis, vīcēre, vīcerim, vīcerimus, vīcerīmus, vīcerint, vīceris, vīcerīs, vīcerit, vīceritīs, vīcerītis, vīcerō, vīcērunt, vīcī, vīcimus, vīcisse, vīcissem, vīcissēmus, vīcissent, vīcissēs, vīcisset, vīcissētis, vīcistī, vīcistis, vīcit, vīcta, vīctā, vīctae, vīctam, vīctārum, vīctās, vīcte, vīctī, vīctīs, vīctō, vīctōrum, vīctōs, vīctū, victum, vīctum, vīctūrus, victus, vīctus, vincam, vincāminī, vincāmur, vincāmus, vincant, vincantur, vincar, vincāre, vincāris, vincās, vincat, vincātis, vincātur, vince, vincēbam, vincēbāminī, vincēbāmur, vincēbāmus, vincēbant, vincēbantur, vincēbar, vincēbāre, vincēbāris, vincēbās, vincēbat, vincēbātis, vincēbātur, vincēminī, vincēmur, vincēmus, vincendī, vincendō, vincendum, vincendus, vincēns, vincent, vincentur, vincere, vincēre, vincerem, vincerēminī, vincerēmur, vincerēmus, vincerent, vincerentur, vincerer, vincerēre, vincerēris, vincerēs, vinceret, vincerētis, vincerētur, vinceris, vincēris, vincēs, vincet, vincētis, vincētur, vincī, vinciminī, vincimur, vincimus, vincis, vincit, vincite, vincitīs, vincitō, vincitor, vincitōte, vincitur, vincō, vincor, vincunt, vincuntō, vincuntor, vincuntur* — “conquer”;

*vīsa, vīsā, vīsaie, vīsam, vīsāminī, vīsāmur, vīsāmus, vīsant, vīsantur, vīsar, vīsāre, vīsāris, vīsārum, vīsās, vīsat, vīsātis, vīsātur, vīse, vīsēbam, vīsēbāminī, vīsēbāmur, vīsēbāmus, vīsēbant, vīsēbantur, vīsēbar, vīsēbāre, vīsēbāris, vīsēbās, vīsēbat, vīsēbātis, vīsēbātur, vīsēminī, vīsēmur, vīsēmus, vīsēndī, vīsēndō, vīsēndum, vīsēndus, vīsēns, vīsēnt, vīsēntur, vīseram, vīserāmus, vīserant, vīserās, vīserat, vīserātis, vīserē, vīsēre, vīserem, vīserēminī, vīserēmur, vīserēmus, vīserent, vīserentur, vīserer, vīserēre, vīserēris, vīserēs, vīseret, vīserētis, vīserētur, vīserim, vīserimus, vīserīmus, vīserint, vīseris, vīserīs, vīserit, vīseritīs, vīserītis, vīserō, vīserunt, vīsēs, vīset, vīsētis, vīsētur, vīsī, vīsiminī, vīsimur, vīsimus, vīsīs, vīsīs, vīsisse, vīsisse, vīsissēmus, vīsissent, vīsissēs, vīsisset, vīsissētis, vīsistī, vīsistis, vīsīt, vīsīte, vīsītis, vīsītō, vīsitor, vīsītōte, vīsitur, vīsō, vīsor, vīsōrum, vīsōs, vīsū, vīsum, vīsunt, vīsuntō, vīsuntor, vīsuntur, vīsūrus, vīsus* — “visit”;

*vomam, vomāminī, vomāmur, vomāmus, vomant, vomantur, vomar, vomāre, vomāris, vomās, vomat, vomātis, vomātur, vome, vomēbam, vomēbāminī, vomēbāmur, vomēbāmus, vomēbant, vomēbantur, vomēbar, vomēbāre, vomēbāris, vomēbās, vomēbat, vomēbātis, vomēbātur, vomēminī, vomēmur, vomēmus, vomendī, vomendō, vomendum, vomendus, vomēns, voment, vomentur, vomere, vomēre, vomerem, vomerēminī, vomerēmur, vomerēmus, vomerent, vomerentur, vomerer, vomerēre, vomerēris, vomerēs, vomeret, vomerētis, vomerētur, vomeris, vomēris, vomēs, vomet, vomētis, vomētur, vomī, vomīminī, vomīmur, vomīmus, vomīs, vomit, vomita, vomitā, vomitae, vomitam, vomitārum, vomitās, vomite, vomitī, vomitis, vomitīs, vomitō, vomitor, vomitōrum, vomitōs, vomitōte, vomitū, vomitum, vomitur, vomitūrus, vomitus, vomō, vomor, vomueram, vomuerāmus, vomuerant, vomuerās, vomuerat, vomuerātis, vomuēre, vomuerim, vomuerimus, vomuerīmus, vomuerint, vomueris, vomuerīs, vomuerit, vomueritis, vomuerītis, vomuerō, vomuērunt, vomuī, vomuīmus, vomuisse, vomuissem, vomuissēmus, vomuis-sent, vomuissēs, vomuisset, vomuissētis, vomuistī, vomuistis, vomuīt, vomunt, vomuntō, vomuntor, vomuntur* — “vomit”.

[https://en.wikipedia.org/wiki/Latin\\_conjugation#Fourth\\_conjugation](https://en.wikipedia.org/wiki/Latin_conjugation#Fourth_conjugation)

*aperī, aperiam, aperīāminī, aperīāmur, aperīāmus, aperiant, aperiantur, aperiar, aperīāre, aperīāris, aperīās, aperiat, aperīātis, aperīātur, aperīēbam, aperīēbāminī, aperīēbāmur, aperīēbāmus, aperīēbant, aperīēbantur, aperīēbar, aperīēbāre, aperīēbāris, aperīēbās, aperīēbat, aperīēbātis, aperīēbātur, aperīēminī, aperīēmur, aperīēmus, aperīendī, aperīendō, aperīendum, aperīendus, aperīēns, aperient, aperientur, aperīēre, aperīēris, aperīēs, aperiet, aperīētis, aperīētur, aperīminī, aperīmur, aperīmus, aperīō, aperior, aperīre, aperīrem, aperīrēmi-nī, aperīrēmur, aperīrēmus, aperīrent, aperīrentur, aperīrer, aperīrēre, aperīrēris, aperīrēs, aperīret, aperīrētis, aperīrētur, aperīrī, aperīris, aperīs, aperit, aperīte, aperītis, aperītō, aperītor, aperītōte, aperītur, aperīunt, ape-riuntō, aperīuntor, aperīuntur, aperta, apertā, apertae, apertam, apertārum, apertās, aperte, apertī, apertīs, apertō, apertōrum, apertōs, apertū, apertum, apertūrus, apertus, aperueram, aperuerāmus, aperuerant, aperuerās, aperuerat, aperuerātis, aperuēre, aperuerim, aperuerimus, aperuerīmus, aperuerint, aperueris, aperuerīs, aperuerit, aperueritis, aperuerītis, aperuerō, aperuērunt, aperuī, aperuīmus, aperuisse, aperuissem, aperuissēmus, aperuissent, aperuissēs, aperuisset, aperuissētis, aperuistī, aperuistis, aperuīt* — “open”;

*audī, audiam, audiāminī, audiāmur, audiāmus, audiant, audiantur, audiar, audiāre, audiāris, audiās, audiat, audiātis, audiātur, audiēbam, audiēbāminī, audiēbāmur, audiēbāmus, audiēbant, audiēbantur, audiēbar, audiēbāre, audiēbāris, audiēbās, audiēbat, audiēbātis, audiēbātur, audiēminī, audiēmur, audiēmus, audiendī, audien-dō, audiendum, audiendus, audiēns, audient, audientur, audiēre, audiēris, audiēs, audiet, audiētis, audiētur, audīminī, audīmur, audīmus, audīō, audior, audīre, audīrem, audīrēminī, audīrēmur, audīrēmus, audīrent, au-dīrentur, audīrer, audīrēre, audīrēris, audīrēs, audīret, audīrētis, audīrētur, audīrī, audīris, audīs, audit, audīta, audītā, audītae, audītam, audītārum, audītās, audīte, audītī, audītis, audītīs, audītō, audītor, audītōrum, audītōs, audītōte, audītū, audītum, audītur, audītūrus, audītus, audiunt, audiuntō, audiuntor, audiuntur, audīveram, audīverāmus, audīverant, audīverās, audīverat, audīverātis, audīvēre, audīverim, audīverimus, audīverīmus, au-dīverint, audīveris, audīverīs, audīverit, audīveritis, audīverītis, audīverō, audīvērunt, audīvī, audīvimus, audī-visse, audīvissem, audīvissēmus, audīvissent, audīvissēs, audīvisset, audīvissētis, audīvistī, audīvistis, audīvit* — “hear”;

*mūnī, mūniam, mūniāminī, mūniāmur, mūniāmus, mūniant, mūniantur, mūniar, mūniāre, mūniāris, mūniās, mū-niat, mūniātis, mūniātur, mūniēbam, mūniēbāminī, mūniēbāmur, mūniēbāmus, mūniēbant, mūniēbantur, mūniē-bar, mūniēbāre, mūniēbāris, mūniēbās, mūniēbat, mūniēbātis, mūniēbātur, mūniēminī, mūniēmur, mūniēmus, mūniendī, mūniendō, mūniendum, mūniendus, mūniēns, mūnient, mūnientur, mūniēre, mūniēris, mūniēs, mūniet, mūniētis, mūniētur, mūnīminī, mūnīmur, mūnīmus, mūniō, mūnior, mūnīre, mūnīrem, mūnīrēminī, mūnīrēmur, mūnīrēmus, mūnīrent, mūnīrentur, mūnīrer, mūnīrēre, mūnīrēris, mūnīrēs, mūnīret, mūnīrētis, mūnīrētur, mūnīrī, mūnīris, mūnīs, mūnit, mūnita, mūnitā, mūnitae, mūnitam, mūnitārum, mūnitās, mūnite, mūnīte, mūnitī, mūnitīs, mūnitō, mūnitō, mūnitō, mūnitōrum, mūnitōs, mūnitōte, mūnitū, mūnitum, mūnitum, mūnitur, mūnitū-rus, mūnitus, mūnītus, mūniunt, mūniuntō, mūniuntor, mūniuntur, mūnīveram, mūnīverāmus, mūnīverant, mū-nīverās, mūnīverat, mūnīverātis, mūnīvēre, mūnīverim, mūnīverimus, mūnīverīmus, mūnīverint, mūnīveris, mū-nīverīs, mūnīverit, mūnīveritis, mūnīverītis, mūnīverō, mūnīvērunt, mūnīvī, mūnīvimus, mūnīvisse, mūnīvissem, mūnīvissēmus, mūnīvissent, mūnīvissēs, mūnīvisset, mūnīvissētis, mūnīvistī, mūnīvistis, mūnīvit* — “fortify”;

*oriāminī, oriāmur, oriantur, oriar, oriāre, oriāris, oriātur, oriēbāminī, oriēbāmur, oriēbantur, oriēbar, oriēbāre, oriēbāris, oriēbātur, oriēminī, oriēmur, oriendī, oriendō, oriendum, oriendus, oriēns, orientur, oriēre, oriēris, oriētur, oriēminī, oriēmur, orior, oriēre, oriēminī, oriēmur, oriērentur, oriērer, oriērēre, oriērēris, oriērētur, oriērī, oriēris, oriētor, oriētur, oriētūrus, oriēuntor, oriēuntur, orta, ortā, ortae, ortam, ortārum, ortās, orte, ortī, ortīs, ortō, ortōrum, ortōs, ortū, ortum, ortus* — “rise”;

*saepī, saepiam, saepiāminī, saepiāmur, saepiāmus, saepiant, saepiantur, saepiar, saepiāre, saepiāris, saepiās, saepiat, saepiātis, saepiātur, saepiēbam, saepiēbāminī, saepiēbāmur, saepiēbāmus, saepiēbant, saepiēbantur, saepiēbar, saepiēbare, saepiēbāris, saepiēbās, saepiēbat, saepiēbātis, saepiēbātur, saepiēminī, saepiēmur, saepiēmus, saepiendī, saepiendō, saepiendum, saepiendus, saepiēns, saepient, saepientur, saepiēre, saepiēris, saepiēs, saepiet, saepiētis, saepiētur, saepīminī, saepīmur, saepīmus, saepiō, saepior, saepīre, saepīrem, saepīrēminī, saepīrēmur, saepīrēmus, saepīrent, saepīrentur, saepīrer, saepīrēre, saepīrēris, saepīrēs, saepīret, saepīrētis, saepīrētur, saepīrī, saepīris, saepīs, saepit, saepīte, saepītis, saepītō, saepītor, saepītōte, saepītur, saepiunt, saepiuntō, saepiuntor, saepiuntur, saepseram, saepserāmus, saepserant, saepserās, saepserat, saepserātis, saepserē, saepserim, saepserimus, saepserimus, saepserint, saepseris, saepserīs, saepserit, saepseritis, saepserītis, saepserō, saepserunt, saepsī, saepsimus, saepsisse, saepsissem, saepsissēmus, saepsissent, saepsissēs, saepsisset, saepsissētis, saepsistī, saepsistis, saepsit, saepta, saeptā, saeptae, saeptam, saeptārum, saeptiās, saepte, saeptī, saeptīs, saeptō, saeptōrum, saeptōs, saeptū, saeptum, saeptūrus, saeptus* — “surround”;

*sancī, sanciam, sancīāminī, sancīāmur, sancīāmus, sanciant, sanciantur, sanciar, sancīāre, sancīāris, sancīās, sanciat, sancīātis, sancīātur, sancīēbam, sancīēbāminī, sancīēbāmur, sancīēbāmus, sancīēbant, sancīēbantur, sancīēbar, sancīēbare, sancīēbāris, sancīēbās, sancīēbat, sancīēbātis, sancīēbātur, sancīēminī, sancīēmur, sancīēmus, sancīendī, sancīendō, sancīendum, sancīendus, sancīēns, sancient, sancientur, sancīēre, sancīēris, sancīēs, sanciet, sancīētis, sancīētur, sancīminī, sancīmur, sancīmus, sancīō, sancior, sancīre, sancīrem, sancīrēminī, sancīrēmur, sancīrēmus, sancīrent, sancīrentur, sancīrer, sancīrēre, sancīrēris, sancīrēs, sancīret, sancīrētis, sancīrētur, sancīrī, sancīris, sancīs, sancit, sancīte, sancītis, sancītō, sancītor, sancītōte, sancītur, sancīunt, sancīuntō, sancīuntor, sancīuntur, sāncta, sānctā, sānctae, sānctam, sānctārum, sānctās, sāncte, sānctī, sānctīs, sānctō, sānctōrum, sānctōs, sānctū, sānctum, sānctūrus, sānctus, sānxeram, sānxerāmus, sānxerant, sānxerās, sānxerat, sānxerātis, sānxēre, sānixerim, sānixerimus, sānixerimus, sānixerint, sānixeris, sānixerīs, sānixerit, sānixeritis, sānixerītis, sānixerō, sānxērunt, sānxī, sānximus, sānxisse, sānxissem, sānxissēmus, sānxissent, sānxissēs, sānxisset, sānxissētis, sānxistī, sānxistis, sānxit* — “confirm”;

*sēnsa, sēnsā, sēnsae, sēnsam, sēnsārum, sēnsās, sēnse, sēnseram, sēnserāmus, sēnserant, sēnserās, sēnserat, sēnserātis, sēnsere, sēnserim, sēnserimus, sēnserimus, sēnserint, sēnseris, sēnserīs, sēnserit, sēnseritis, sēnserītis, sēnserō, sēnsērunt, sēnsī, sēnsimus, sēnsīs, sēnsisse, sēnsissem, sēnsissēmus, sēnsissent, sēnsissēs, sēnsisset, sēnsissētis, sēnsistī, sēnsistis, sēnsit, sēnsō, sēnsōrum, sēnsōs, sēnsū, sēnsūm, sēnsūrus, sēnsus, sentī, sentiam, sentiāminī, sentiāmur, sentiāmus, sentiant, sentiantur, sentiar, sentiāre, sentiāris, sentiās, sentiat, sentiātis, sentiātur, sentiēbam, sentiēbāminī, sentiēbāmur, sentiēbāmus, sentiēbant, sentiēbantur, sentiēbar, sentiēbare, sentiēbāris, sentiēbās, sentiēbat, sentiēbātis, sentiēbātur, sentiēminī, sentiēmur, sentiēmus, sentiendī, sentiendō, sentiendum, sentiendus, sentiēns, sentient, sentiēre, sentiēris, sentiēs, sentiet, sentiētis, sentiētur, sentiīminī, sentiīmur, sentiīmus, sentiō, sentior, sentiēre, sentiērem, sentiērēminī, sentiērēmur, sentiērēmus, sentiērent, sentiērentur, sentiērer, sentiērēre, sentiērēris, sentiērēs, sentiēret, sentiērētis, sentiērētur, sentiērī, sentiēris, sentiēs, sentiit, sentiīte, sentiītis, sentiītō, sentiītor, sentiītōte, sentiītur, sentiunt, sentiuntō, sentiuntor, sentiuntur* — “feel”;

*vēneram, vēnerāmus, vēnerant, vēnerās, vēnerat, vēnerātis, vēnēre, vēnerim, vēnerimus, vēnerimus, vēnerint, vēneris, vēnerīs, vēnerit, vēneritis, vēnerītis, vēnerō, vēnērunt, venī, venī, veniam, veniāmus, veniant, veniās, veniat, veniātis, veniātur, veniēbam, veniēbāmus, veniēbant, veniēbās, veniēbat, veniēbātis, veniēbātur, veniēmus, veniendī, veniendō, veniendum, veniendus, veniēns, venient, veniēs, veniet, veniētis, veniētur, venimus, vēnimus, veniō, venīre, venīrem, venīrēmus, venīrent, venīrēs, venīret, venīrētis, venīrētur, venīrī, venīs, vēnisse, vēnissem, vēnissēmus, vēnissent, vēnissēs, vēnisset, vēnissētis, vēnistī, vēnistis, venit, vēnit, venīte, venītis, venītō, venītōte, venītur, veniunt, veniuntō, venta, ventā, ventae, ventam, ventārum, ventās, vente, ventī, ventīs, ventō, ventōrum, ventōs, ventū, ventum, ventūrus, ventus* — “come”.

As we throw each group of test verbs into our algorithm, the verb forms from the same conjugation groups are clustered correctly.

We note, however, that the inflected forms of *vetus* “old” and *vetō* “forbid” will be partly conflated if they appear simultaneously:

{*vetā, vetābam, vetābāminī, vetābāmur, vetābāmus, vetābant, vetābantur, vetābar, vetābare, vetābāris, vetābās, vetābat, vetābātis, vetābātur, vetābere, vetāberis, vetābiminī, vetābimur, vetābimus, vetābis, vetābit, vetābitis, vetābitur, vetābō, vetābor, vetābunt, vetābuntur, vetāminī, vetāmur, vetāmus, vetandī, vetandō, vetandum, vetandus, vetāns, vetant, vetantō, vetantor, vetantur, vetāre, vetārem, vetārēminī, vetārēmur, vetārēmus, vetārent, vetārentur, vetārēr, vetārēre, vetārēris, vetārēs, vetāret, vetārētis, vetārētur, vetārī, vetāris, vetās, vetat, vetāte, vetātis, vetātō, vetātor, vetātōte, vetātur, vetem, vetēminī, vetēmur, vetēmus, vetent, vetentur, veter, vetera, veterere, vetēre, veterem, veterēs, veterī, veteribus, veteris, vetēris, veterima, veterimā, veterimae, veterimam,*

*veterrimārum, veterrimās, veterrime, veterrimī, veterrimīs, veterrimō, veterrimōrum, veterrimōs, veterrimum, veterrimus, veterum, vetēs, vetet, vetētis, vetētur, vetita, vetitā, vetitae, vetitam, vetitārum, vetitās, vetite, vetitī, vetitīs, vetitō, vetitōrum, vetitōs, vetitū, vetitum, vetitūrus, vetitus, vetō, vetor, vetueram, vetuerāmus, vetuerant, vetuerās, vetuerat, vetuerātis, vetuēre, vetuerim, vetuerimus, vetuerīmus, vetuerint, vetueris, vetuerīs, vetuerit, vetueritis, vetuerītis, vetuerō, vetuērunt, vetuī, vetuimus, vetuisse, vetuissem, vetuissēmus, vetuissent, vetuissēs, vetuisset, vetuissētis, vetuistī, vetuistis, vetuit, vetus, vetustissimī, vetustissimīs},*

{*vetustior, vetustiōra, vetustiōre, vetustiōrem, vetustiōrēs, vetustiōrī, vetustiōribus, vetustiōris, vetustiōrum, vetustissima, vetustissimā, vetustissimae, vetustissimam, vetustissimārum, vetustissimās, vetustissime, vetustissimō, vetustissimōrum, vetustissimōs, vetustissimum, vetustissimus, vetustius*}.

Such unfortunate confluences seem unavoidable. Observe that *veteris* is the genitive singular form of *vetus*, while *vetēris* is the second-person singular present passive subjunctive of *vetō*. Both *veteris* and *vetēris* share the same essential root *vet*, and they are practically indistinguishable without context, if the document in question does not employ the diacritical mark for long vowels. Some other Latin words also behave similarly: *portā* is both the ablative singular of *porta* “gate” and the singular present active imperative of *portō* “convey”.

Example 6.29.3. We pick a list of typical irregular verbs from the Wikipedia links indicated below.

[https://en.wikipedia.org/wiki/Latin\\_conjugation#Irregular\\_verbs](https://en.wikipedia.org/wiki/Latin_conjugation#Irregular_verbs)

[https://en.wikipedia.org/wiki/Latin\\_conjugation#Third\\_conjugation\\_.E2.80.93i.C5.8D\\_verbs](https://en.wikipedia.org/wiki/Latin_conjugation#Third_conjugation_.E2.80.93i.C5.8D_verbs)

*cape, capere, caperem, caperēminī, caperēmur, caperēmus, caperent, caperentur, caperer, caperēre, caperēris, caperēs, caperet, caperētis, caperētur, caperis, capī, capiam, capiāminī, capiāmur, capiāmus, capiant, capiantur, capiar, capiāre, capiāris, capiās, capiat, capiātis, capiātur, capiēbam, capiēbāminī, capiēbāmur, capiēbāmus, capiēbant, capiēbantur, capiēbar, capiēbāre, capiēbāris, capiēbās, capiēbat, capiēbātis, capiēbātur, capiēmīnī, capiēmur, capiēmus, capiendī, capiendō, capiendum, capiendus, capiēns, capient, capientur, capiēre, capiēris, capiēs, capiet, capiētis, capiētur, capiminī, capimur, capimus, capiō, capior, capis, capit, capite, capitis, capitō, capitor, capitōte, capitur, capiunt, capiuntō, capiuntur, capta, captā, captae, captam, captārum, captās, capte, captī, captīs, captō, captōrum, captōs, captū, captum, captūrus, captus, cēperam, cēperāmus, cēperant, cēperās, cēperat, cēperātis, cēpēre, cēperim, cēperimus, cēperīmus, cēperint, cēperis, cēperīs, cēperit, cēperitis, cēperītis, cēperō, cēpērunt, cēpī, cēpimus, cēpisse, cēpisse, cēpissēmus, cēpissent, cēpissēs, cēpisset, cēpissētis, cēpistī, cēpistis, cēpit — “capture”;*

*cupe, cupere, cuperem, cuperēminī, cuperēmur, cuperēmus, cuperent, cuperentur, cuperer, cuperēre, cuperēris, cuperēs, cuperet, cuperētis, cuperētur, cuperis, cupī, cupiam, cupiāminī, cupiāmur, cupiāmus, cupiant, cupiantur, cupiar, cupiāre, cupiāris, cupiās, cupiat, cupiātis, cupiātur, cupiēbam, cupiēbāminī, cupiēbāmur, cupiēbāmus, cupiēbant, cupiēbantur, cupiēbar, cupiēbāre, cupiēbāris, cupiēbās, cupiēbat, cupiēbātis, cupiēbātur, cupiēmīnī, cupiēmur, cupiēmus, cupiendī, cupiendō, cupiendum, cupiendus, cupiēns, cupient, cupientur, cupiēre, cupiēris, cupiēs, cupiet, cupiētis, cupiētur, cupiminī, cupimur, cupimus, cupiō, cupior, cupis, cupit, cupīta, cupītā, cupītae, cupītam, cupītārum, cupītās, cupite, cupīte, cupītī, cupītis, cupītīs, cupitō, cupītō, cupitor, cupītōrum, cupītōs, cupitōte, cupītū, cupītum, cupitur, cupītūrus, cupītus, cupiunt, cupiuntō, cupiuntur, cupīveram, cupīverāmus, cupīverant, cupīverās, cupīverat, cupīverātis, cupīvēre, cupīverim, cupīverimus, cupīverīmus, cupīverint, cupīveris, cupīverīs, cupīverit, cupīveritis, cupīverītis, cupīverō, cupīvērunt, cupīvī, cupīvimus, cupīvisse, cupīvissem, cupīvissēmus, cupīvissent, cupīvissēs, cupīvisset, cupīvissētis, cupīvistī, cupīvistis, cupīvit — “desire”;*

*eam, eamus, eant, eas, eat, eatis, eatur, eo, eundi, eundo, eundum, eundus, eunt, eunto, i, ibam, ibamus, ibant, ibas, ibat, ibatis, ibatur, ibimus, ibis, ibit, ibitis, ibitur, ibo, ibunt, iens, ieram, ieramus, ierant, ieras, ierat, ieratis, iere, ierim, ierimus, ierint, ieris, ierit, ieritis, iero, ierunt, ii, iimus, iit, imus, ire, irem, iremus, irent, ires, iret, iretis, iretur, iri, is, isse, issem, issemus, issent, isses, isset, issetis, isti, istis, it, ite, itis, ito, itote, itu, itum, itur, iturus, itus, ivi, ivisti, ivit — “go”;*

*edam, edāminī, edāmur, edāmus, edant, edantur, edar, edāre, edāris, edās, edat, edātis, edātur, ede, edēbam, edēbāminī, edēbāmur, edēbāmus, edēbant, edēbantur, edēbar, edēbāre, edēbāris, edēbās, edēbat, edēbātis, edēbātur, edēmīnī, edēmur, edēmus, edendī, edendō, edendum, edendus, edēns, edent, edentur, ēderam, ēderāmus, ēderant, ēderās, ēderat, ēderātis, edere, edēre, ēdēre, ederem, ederēminī, ederēmur, ederēmus, ederent, ederentur, ederer, ederēre, ederēris, ederēs, ederet, ederētis, ederētur, ēderim, ēderimus, ēderīmus, ēderint, ederis, edēris, ēderis, ēderīs, ēderit, ēderitis, ēderītis, ēderō, ēdērunt, edēs, edet, edētis, edētur, edī, ēdī, edim, ediminī, edimur, edimus,*

*edimus, ēdimus, edint, edis, edīs, ēdisse, ēdissem, ēdissemus, ēdisissent, ēdisēs, ēdisset, ēdissetis, ēdistī, ēdistis, edit, edit, edite, editis, editis, editō, editor, editōte, editur, edō, edor, edunt, eduntō, eduntor, eduntur, ēs, ēsa, ēsā, ēsae, ēsam, ēsārum, ēsās, ēse, ēsī, ēsīs, ēsō, ēsōrum, ēsōs, esse, ēsse, ēssem, ēssēmus, ēssent, ēssēs, ēsset, ēssētis, ēst, ēste, ēstis, ēstō, ēstōte, ēstur, ēsū, ēsum, ēsūrus, ēsus* — “eat”;

*fer, feram, ferāminī, ferāmur, ferāmus, ferant, ferantur, ferar, ferāre, ferāris, ferās, ferat, ferātis, ferātur, ferēbam, ferēbāminī, ferēbāmur, ferēbāmus, ferēbant, ferēbantur, ferēbar, ferēbāre, ferēbāris, ferēbās, ferēbat, ferēbātis, ferēbātur, ferēminī, ferēmur, ferēmus, ferendī, ferendō, ferendum, ferendus, ferēns, ferent, ferentur, ferēre, ferēris, ferēs, feret, ferētis, ferētur, feriminī, ferimur, ferimus, ferō, feror, ferre, ferrem, ferrēminī, ferrēmur, ferrēmus, ferrent, ferrentur, ferrer, ferrēre, ferrēris, ferrēs, ferret, ferrētis, ferrētur, ferrī, ferris, fers, fert, ferte, fertis, fertō, fertor, fertōte, fertur, ferunt, feruntō, feruntor, feruntur, lāta, lātā, lātae, lātam, lātārum, lātās, lāte, lātī, lātīs, lātō, lātōrum, lātōs, lātū, lātum, lātūrus, lātus, tuleram, tulerāmus, tulerant, tulerās, tulerat, tulerātis, tulēre, tulerim, tulerimus, tulerīmus, tulerint, tuleris, tulerīs, tulerit, tuleritis, tulerītis, tulerō, tulērunnt, tulī, tulimus, tulisse, tulissem, tulissēmus, tulissent, tulissēs, tulisset, tulissētis, tulistī, tulistis, tulit* — “carry”;

*mālam, mālēbam, mālēbāmus, mālēbant, mālēbās, mālēbat, mālēbātis, mālēmus, mālent, mālēns, mālet, mālētis, mālim, mālimus, mālint, mālis, mālit, mālītis, mālle, māllem, māllēmus, māllent, māllēs, māllet, māllētis, mālo, mālueram, māluerāmus, māluerant, māluerās, māluerat, māluerātis, māluēre, māluerim, māluerimus, māluerīmus, māluerint, mālueris, māluerīs, māluerit, mālueritis, māluerītis, māluerō, māluērunt, māluī, māluimus, māluisse, māluissem, māluissēmus, māluissent, māluissēs, māluisset, māluissētis, māluistī, māluistis, māluit, mālumus, mālunt, māvīs, māvult, māvultis* — “prefer”;

*morere, morerēminī, morerēmur, morerentur, morerer, morerēre, morerēris, morerētur, moreris, morī, moriāminī, moriāmur, moriantur, moriar, moriāre, moriāris, moriātur, moriēbāminī, moriēbāmur, moriēbantur, moriēbar, moriēbāre, moriēbāris, moriēbātur, moriēminī, moriēmur, moriendī, moriendō, moriendum, moriendus, moriēns, morientur, moriēre, moriēris, moriētur, moriminī, morimur, morior, moritor, moritur, moritūrus, moriuntor, moriuntur, mortua, mortuā, mortuae, mortuam, mortuārum, mortuās, mortue, mortuī, mortuīs, mortuō, mortuōrum, mortuōs, mortuū, mortuum, mortuus* — “die”;

*nōlam, nōlēbam, nōlēbāmus, nōlēbant, nōlēbās, nōlēbat, nōlēbātis, nōlēmus, nōlēns, nōlent, nōlēns, nōlet, nōlētis, nōlī, nōlim, nōlīmus, nōlint, nōlīs, nōlit, nōlīte, nōlītis, nōlitō, nōlitōte, nōlle, nōllem, nōllēmus, nōllent, nōllēs, nōllet, nōllētis, nōlō, nōlueram, nōluerāmus, nōluerant, nōluerās, nōluerat, nōluerātis, nōluēre, nōluerim, nōluerimus, nōluerīmus, nōluerint, nōlueris, nōluerīs, nōluerit, nōlueritis, nōluerītis, nōluerō, nōluērunt, nōluī, nōluimus, nōluisse, nōluissem, nōluissēmus, nōluissent, nōluissēs, nōluisset, nōluissētis, nōluistī, nōluistis, nōluit, nōlumus, nōlunt, nōluntō* — “refuse”;

*passa, passā, passae, passam, passārum, passās, passe, passī, passīs, passō, passōrum, passōs, passū, passum, passūrus, passus, patere, paterēminī, paterēmur, paterentur, paterer, paterēre, paterēris, paterētur, pateris, patī, patiāminī, patiāmur, patiantur, patiar, patiāre, patiāris, patiātur, patiēbāminī, patiēbāmur, patiēbantur, patiēbar, patiēbāre, patiēbāris, patiēbātur, patiēminī, patiēmur, patiendī, patiendō, patiendum, patiendus, patiēns, patientur, patiēre, patiēris, patiētur, patiminī, patimur, patior, patitor, patitur, patiuntor, patiuntur* — “suffer”;

*rape, rapere, raperem, raperēminī, raperēmur, raperēmus, raperent, raperentur, raperer, raperēre, raperēris, raperēs, raperet, raperētis, raperētur, raperis, rapī, rapiam, rapiāminī, rapiāmur, rapiāmus, rapiant, rapiantur, rapiar, rapiāre, rapiāris, rapiās, rapiat, rapiātis, rapiātur, rapiēbam, rapiēbāminī, rapiēbāmur, rapiēbāmus, rapiēbant, rapiēbantur, rapiēbar, rapiēbāre, rapiēbāris, rapiēbās, rapiēbat, rapiēbātis, rapiēbātur, rapiēminī, rapiēmur, rapiēmus, rapiendī, rapiendō, rapiendum, rapiendus, rapiēns, rapient, rapientur, rapiēre, rapiēris, rapiēs, rapiet, rapiētis, rapiētur, rapiminī, rapimur, rapimus, rapiō, rapior, rapis, rapit, rapite, rapitis, rapitō, rapitor, rapitōte, rapitur, rapiunt, rapiuntō, rapiuntor, rapiuntur, rapta, raptā, raptae, raptam, raptārum, raptās, rapte, raptī, raptīs, raptō, raptōrum, raptōs, raptū, raptum, raptūrus, raptus, rapueram, rapuerāmus, rapuerant, rapuerās, rapuerat, rapuerātis, rapuēre, rapuerim, rapuerimus, rapuerīmus, rapuerint, rapueris, rapuerīs, rapuerit, rapueritis, rapuerītis, rapuerō, rapuērunt, rapuī, rapuimus, rapuisse, rapuissem, rapuissēmus, rapuissent, rapuissēs, rapuisset, rapuissētis, rapuistī, rapuistis, rapuit* — “snatch”;

*velim, velīmus, velint, velīs, velit, velītis, velle, vellem, vellēmus, vellent, vellēs, vellet, vellētis, vīs, volam, volēbam, volēbāmus, volēbant, volēbās, volēbat, volēbātis, volēmus, volēns, volent, volēs, volet, volētis, volō, volt, voltis, volueram, voluerāmus, voluerant, voluerās, voluerat, voluerātis, voluēre, voluerim, voluerimus, voluerīmus, voluerint, volueris, voluerīs, voluerit, volueritis, voluerītis, voluerō, voluērunt, voluī, voluimus, voluisse, voluissem, voluissēmus, voluissent, voluissēs, voluisset, voluissētis, voluistī, voluistis, voluit, volumus, volunt, vult, vultis* — “want”.

The clustering result is satisfactory:

{*cape, capere, caperem, caperēminī, caperēmur, caperēmus, caperent, caperentur, caperer, caperēre, caperēris, caperēs, caperet, caperētis, caperētur, caperis, capī, capiam, capiāminī, capiāmur, capiāmus, capiant, capiantur, capiar, capiāre, capiāris, capiās, capiat, capiātis, capiātur, capiēbam, capiēbāminī, capiēbāmur, capiēbāmus, capiēbant, capiēbantur, capiēbar, capiēbāre, capiēbāris, capiēbās, capiēbat, capiēbātis, capiēbātur, capiēminī, capiēmur, capiēmus, capiendī, capiendō, capiendum, capiendus, capiēns, capient, capientur, capiēre, capiēris, capiēs, capiet, capiētis, capiētur, capiminī, capimur, capimus, capiō, capior, capis, capit, capite, capitis, capitō, capitor, capitōte, capitur, capiunt, capiuntō, capiuntor, capiuntur, capta, captā, captae, captam, captārum, captās, capte, captī, captīs, captō, captōrum, captōs, captū, captum, captūrus, captus, cēperam, cēperāmus, cēperant, cēperās, cēperat, cēperātis, cēpēre, cēperim, cēperimus, cēperīmus, cēperint, cēperis, cēperīs, cēperit, cēperitis, cēperītis, cēperō, cēpērunt, cēpī, cēpimus, cēpisse, cēpissē, cēpissēm, cēpissent, cēpissēs, cēpisset, cēpissētis, cēpistī, cēpistis, cēpit*},

{*cupe, cupere, cuperem, cuperēminī, cuperēmur, cuperēmus, cuperent, cuperentur, cuperer, cuperēre, cuperēris, cuperēs, cuperet, cuperētis, cuperētur, cuperis, cupī, cupiam, cupiāminī, cupiāmur, cupiāmus, cupiant, cupiantur, cupiar, cupiāre, cupiāris, cupiās, cupiat, cupiātis, cupiātur, cupiēbam, cupiēbāminī, cupiēbāmur, cupiēbāmus, cupiēbant, cupiēbantur, cupiēbar, cupiēbāre, cupiēbāris, cupiēbās, cupiēbat, cupiēbātis, cupiēbātur, cupiēminī, cupiēmur, cupiēmus, cupiendī, cupiendō, cupiendum, cupiendus, cupiēns, cupient, cupientur, cupiēre, cupiēris, cupiēs, cupiet, cupiētis, cupiētur, cupiminī, cupimur, cupimus, cupiō, cupior, cupis, cupit, cupīta, cupītā, cupītae, cupītam, cupītārum, cupītās, cupite, cupīte, cupītī, cupītis, cupītō, cupītō, cupitor, cupītōrum, cupītōs, cupītōte, cupītū, cupītum, cupitur, cupītūrus, cupītus, cupiunt, cupiuntō, cupiuntor, cupiuntur, cupīveram, cupīverāmus, cupīverant, cupīverās, cupīverat, cupīverātis, cupīvēre, cupīverim, cupīverimus, cupīverīmus, cupīverint, cupīveris, cupīverīs, cupīverit, cupīveritis, cupīverītis, cupīverō, cupīvērunt, cupīvī, cupīvimus, cupīvisse, cupīvissem, cupīvissemus, cupīvissent, cupīvisēs, cupīvisset, cupīvisētis, cupīvistī, cupīvistis, cupīvit*},

{*eam, eamus, eant, eas, eat, eatis, eatur, eo, ēs, ēsa, ēsā, ēsae, ēsam, ēsī, ēsō, ēsū, eundi, eundo, eundum, eundus, eunt, eunto, i, ibam, ibamus, ibant, ibas, ibat, ibatis, ibatur, ibimus, ibis, ibit, ibitis, ibitur, ibo, ibunt, iens, ieram, ieramus, ierant, ieras, ierat, ieratis, iere, ierim, ierimus, ierint, ieris, ierit, ieritis, iero, ierunt, ii, iimus, iit, imus, ire, irem, iremus, irent, ires, iret, iretis, iretur, iri, is, isse, issem, issemus, issent, isses, isset, issetis, isti, istis, it, ite, itis, ito, itote, itu, itum, itur, iturus, itus, ivi, ivisti, ivit*},

{*edam, edāminī, edāmur, edāmus, edant, edantur, edar, edāre, edāris, edās, edat, edātis, edātur, ede, edēbam, edēbāminī, edēbāmur, edēbāmus, edēbant, edēbantur, edēbar, edēbāre, edēbāris, edēbās, edēbat, edēbātis, edēbātur, edēminī, edēmur, edēmus, edendī, edendō, edendum, edendus, edēns, edent, edentur, ēderam, ēderāmus, ēderant, ēderās, ēderat, ēderātis, edere, edēre, ēdēre, ederem, ederēminī, ederēmur, ederēmus, ederent, ederentur, ederer, ederēre, ederēris, ederēs, ederet, ederētis, ederētur, ēderim, ēderimus, ēderīmus, ēderint, ēderis, ēderīs, ēderit, ēderitis, ēderītis, ēderō, ēdērunt, edēs, edet, edētis, edētur, edī, edī, edim, ediminī, edimus, edimus, edimus, edint, edīs, edīs, edisse, edissem, edissēm, edissent, edissēs, edisset, edissētis, edistī, edistis, edit, edit, edite, editis, edītis, editō, editor, editōte, editur, edō, edor, edunt, eduntō, eduntor, eduntur, ēsārum, ēsās, ēse, ēsīs, ēsōrum, ēsōs, esse, ēsse, ēssem, ēssēm, ēssēt, ēssēs, ēsset, ēssētis, ēst, ēste, ēstis, ēstō, ēstōte, ēstur, ēsum, ēsūrus, ēsus*},

{*fer, feram, ferāminī, ferāmur, ferāmus, ferant, ferantur, ferar, ferāre, ferāris, ferās, ferat, ferātis, ferātur, ferēbam, ferēbāminī, ferēbāmur, ferēbāmus, ferēbant, ferēbantur, ferēbar, ferēbāre, ferēbāris, ferēbās, ferēbat, ferēbātis, ferēbātur, ferēminī, ferēmur, ferēmus, ferendī, ferendō, ferendum, ferendus, ferēns, ferent, ferentur, ferēre, ferēris, ferēs, feret, ferētis, ferētur, feriminī, ferimur, ferimus, ferō, feror, ferre, ferrem, ferrēminī, ferrēmur, ferrēmus, ferrent, ferrentur, ferrer, ferrēre, ferrēris, ferrēs, ferret, ferrētis, ferrētur, ferrī, ferris, fers, fert, ferte, fertis, fertō, fertor, fertōte, fertur, ferunt, feruntō, feruntor, feruntur, lāta, lātā, lātae, lātam, lātārum, lātās, lāte, lātī, lātīs, lātō, lātōrum, lātōs, lātū, lātum, lātūrus, lātus, tuleram, tulerāmus, tulerant, tulerās, tulerat, tulerātis, tulēre, tulerim, tulerimus, tulerīmus, tulerint, tuleris, tulerīs, tulerit, tuleritis, tulerītis, tulerō, tulērunt, tulī, tulimus, tulisse, tulussem, tulissēm, tulissent, tulissēs, tulisset, tulissētis, tulistī, tulistis, tulit*},

{*mālam, mālēbam, mālēbāmus, mālēbant, mālēbās, mālēbat, mālēbātis, mālēm, mālent, mālēs, mālet, mālētis, mālim, mālīmus, mālint, mālīs, mālit, mālītis, mälle, mällem, mällēm, mällent, mällēs, mället, mällētis, mālō, mālueram, māluerāmus, māluerant, māluerās, māluerat, māluerātis, māluēre, māluerim, māluerimus, māluerīmus, māluerint, mālueris, māluerīs, māluerit, mālueritis, māluerītis, māluerō, māluērunt, māluī, māluimus, māluisse, māluissem, māluissēm, māluissent, māluissēs, māluisset, māluissētis, māluistī, māluistis, māluit, mālum, mālunt, māvīs, māvult, māvultis*},

{*morere, morerēminī, morerēmur, morerentur, morerer, morerēre, morerēris, morerētur, moreris, morī, moriāminī, moriāmur, moriantur, moriar, moriāre, moriāris, moriātur, moriēbāminī, moriēbāmur, moriēbantur, moriēbar, moriēbāre, moriēbāris, moriēbātur, moriēmīnī, moriēmur, moriendī, moriendō, moriendum, moriendus, moriēns, morientur, moriēre, moriēris, moriētur, moriminī, morimur, morior, moritor, moritur, moritūrus, moriuntor, moriuntur, mortua, mortuā, mortuae, mortuam, mortuārum, mortuās, mortue, mortuī, mortuīs, mortuō, mortuōrum, mortuōs, mortuū, mortuum, mortuus*}},

{*nōlam, nōlēbam, nōlēbāmus, nōlēbant, nōlēbās, nōlēbat, nōlēbātis, nōlēmus, nōlēns, nōlent, nōlēs, nōlet, nōlētis, nōlī, nōlim, nōlīmus, nōlint, nōlīs, nōlit, nōlīte, nōlītis, nōlitō, nōlitōte, nōlle, nōllem, nōllēmus, nōllent, nōllēs, nōllet, nōllētis, nōlō, nōlueram, nōluerāmus, nōluerant, nōluerās, nōluerat, nōluerātis, nōluēre, nōluerim, nōluerimus, nōluerīmus, nōluerint, nōlueris, nōluerīs, nōluerit, nōlueritis, nōluerītis, nōluerō, nōluērunt, nōluī, nōluimus, nōluisse, nōluissem, nōluissēmus, nōluissent, nōluissēs, nōluisset, nōluissētis, nōluistī, nōluistis, nōluit, nōlumus, nōlunt, nōluntō*}},

{*passa, passā, passae, passam, passārum, passās, passe, passī, passīs, passō, passōrum, passōs, passū, passum, passūrus, passus, patere, paterēminī, paterēmur, paterentur, paterer, paterēre, paterēris, paterētur, pateris, patī, patiāminī, patiāmur, patiantur, patiar, patiāre, patiāris, patiātur, patiēbāminī, patiēbāmur, patiēbantur, patiēbar, patiēbāre, patiēbāris, patiēbātur, patiēmīnī, patiēmur, patiendī, patiendō, patiendum, patiendus, patiēns, patientur, patiēre, patiēris, patiētur, patiminī, patimur, patior, patitor, patitur, patiuntor, patiuntur*}},

{*rape, rapere, raperem, raperēminī, raperēmur, raperēmus, raperent, raperentur, raperer, raperēre, raperēris, raperēs, raperet, raperētis, raperētur, raperis, rapī, rapiam, rapiāminī, rapiāmur, rapiāmus, rapiant, rapiantur, rapiar, rapiāre, rapiāris, rapiās, rapiat, rapiātis, rapiātur, rapiēbam, rapiēbāminī, rapiēbāmur, rapiēbāmus, rapiēbant, rapiēbantur, rapiēbar, rapiēbāre, rapiēbāris, rapiēbās, rapiēbat, rapiēbātis, rapiēbātur, rapiēmīnī, rapiēmur, rapiēmus, rapiendī, rapiendō, rapiendum, rapiendus, rapiēns, rapient, rapientur, rapiēre, rapiēris, rapiēs, rapiet, rapiētis, rapiētur, rapiminī, rapimur, rapimus, rapīō, rapior, rapis, rapit, rapite, rapitis, rapitō, rapitor, rapitōte, rapitur, rapiunt, rapiuntō, rapiuntor, rapiuntur, rapta, raptā, raptae, raptam, raptārum, raptās, rapte, raptī, raptīs, raptō, raptōrum, raptōs, raptū, raptum, raptūrus, raptus, rapueram, rapuerāmus, rapuerant, rapuerās, rapuerat, rapuerātis, rapuēre, rapuerim, rapuerimus, rapuerīmus, rapuerint, rapueris, rapuerīs, rapuerit, rapueritis, rapuerītis, rapuerō, rapuērunt, rapuī, rapuimus, rapuisse, rapuissem, rapuissēmus, rapuissent, rapuissēs, rapuisset, rapuissētis, rapuistī, rapuistis, rapuīt*}},

{*velim, velīmus, velint, velīs, velit, velītis, velle, vellem, vellēmus, vellent, vellēs, vellet, vellētis, vīs, volam, volēbam, volēbāmus, volēbant, volēbās, volēbat, volēbātis, volēmus, volēns, volent, volēs, volet, volētis, volō, volt, voltis, volueram, voluerāmus, voluerant, voluerās, voluerat, voluerātis, voluēre, voluerim, voluerimus, voluerīmus, voluerint, volueris, voluerīs, voluerit, volueritis, voluerītis, voluerō, voluērunt, voluī, voluimus, voluisse, voluissem, voluissēmus, voluissent, voluissēs, voluisset, voluissētis, voluistī, voluistis, voluit, volumus, volunt, vult, vultis*}},

*Example 6.29.4.* In Fig. S9, we further apply the aforementioned word clustering algorithm to topic extraction and machine translation (see Table S1 for text source). Since vowel lengths are usually not marked in written Latin, confluations of certain concepts are unavoidable in our algorithm. For example, we have *mēnsis* “month” (nominative/genitive/vocative singular) vs. *mēnsīs* “tables” (dative/ablative plural), *miserīs* “poor” (masculine/feminine/neuter ablative plural) vs. *miseris* “you will have sent” (second person singular, future perfect).
