# Supplementary material for: A mathematical model for universal semantics
Source: arXiv:1907.12293 ancillary file (2020-07-12)
Supplement: Supplementary file 2 [file SoftwareManualPartB.pdf]

## 7 Approximate word clustering in selected Slavic languages

In this section, we present the approximate clustering algorithms for two representative Slavic languages: Polish and Russian.

Despite differences in the writing systems (Polish uses the Latin script while Russian employs the Cyrillic alphabet), both these languages share some morphological features in common:

- Polish nouns decline in seven cases, Russian six (in singular and plural forms).
- Adjectives are declined in three genders and in all the cases available to nouns.
- The same verb in imperfective and perfective aspects often differ by a prefix or an alternation of consonant/vowel. A limited amount of verbs have etymologically unrelated stems in their imperfective and perfective aspects.
- Both Polish and Russian have a handful of “verbs of motion” that contrast multidirectional and unidirectional forms.

These characterizations also apply to other Slavic languages (Croatian, Czech, Slovak and Slovene written in the Latin script; Belarusian, Bulgarian, Macedonian, Serbian and Ukrainian written in the Cyrillic script), more or less. In addition, the two modern Baltic languages, Latvian and Lithuanian, are similar to Slavic languages at the morphological level.

Some common words in Polish and Russian have very short (even vowelless) stems, and the short stems themselves may allow vowel and/or consonant alternations. At times, words with very different meanings have nearly identical stems. Thus it is highly challenging to design approximate clustering algorithms for these languages, while avoiding confusions of unrelated words. In the methods developed in this section, we make a compromise between a workable algorithm and error-free clustering.

### 7.1 Modified Porter stemming algorithm for Polish

**Definition 7.1** (Polish stop words). If a word belongs to the following list<sup>87</sup>:

*a, aby, ach, acz, aczkolwiek, aj, albo, albowiem, ale, ależ, ani, aż, bardziej, bardzo, bądź, bądźcie, bądźmy, bez, będą, będąc, będąca, będące, będący, będą, będzie, będziecie, będziemy, będziesz, bo, bowiem, by, bycie, być, byli, byliby, bylibyście, bylibyśmy, byliście, byliśmy, był, była, byłaby, byłabym, byłabyś, byłaś, byłby, byłbym, byłbyś, byłem, byłeś, było, byłoby, były, byłyby, byłybyście, byłybyśmy, byłyście, byłyśmy, bym, bynajmniej, byś, byście, byśmy, bywszy, cali, cała, cały, chociaż, choć, choćby, chyba, ci, ciebie, cię, co, cokolwiek, coraz, coś, cóż, czasami, czasem, czego, czegokolwiek, czegoś, czemu, czemukolwiek, czemuś, często, czy, czyjś, czyli, czym, czymkolwiek, czymś, czyż, czyżby, czyżbym, czyżbyś, czyżbyście, czyżbyśmy, daleko, dla, dlaczego, dlatego, do, dobrze, dokąd, dokądś, doń, dopóki, doprawdy, dosyć, dość, dużo, dwa, dwaj, dwie, dwoje, dzięki, dzisiaj, dziś, gdy, gdyby, gdybym, gdybyś, gdybyście, gdybyśmy, gdyż, gdzie, gdziekolwiek, gdzieś, go, i, ich, ile, ileś, iloma, ilu, im, inna, inną, inne, innego, innej, innemu, inni, inny, innych, innym, innymi, iż, ja, jacy, jacyś, jak, jaka, jakaś, jaką, jakąś, jakby, jaki, jakich, jakichś, jakie, jakiego, jakiegoś, jakiej, jakiejś, jakiemu, jakiemuś, jakież, jakim, jakimi, jakimiś, jakimś, jakiś, jakiz, jakkolwiek, jako, jakoś, ją, je, jeden, jedna, jednak, jednakże, jedną, jedne, jednego, jednej, jednemu, jedni, jedno, jednych, jednym, jednymi, jedyna, jedyną, jedyne, jedyne, jedynej, jedynemu, jedyni, jedynie, jedyny, jedynych, jedynym, jedynymi, jego, jej, jemu, jest, jestem, jesteś, jesteście, jesteśmy, jeszcze, jeśli, jeżeli, już, każda, każdą, każde, każdego, każdej, każdemu, każdy, każdym, każdymi, kiedy, kiedyś, kilka, kim, kimkolwiek, kimś, kogo, kogokolwiek, kogoś, koło, komu, komukolwiek, komuś, kto, ktokolwiek, ktoś, która, którą, które, którego, której, któremu, który, których, którym, którymi, któryś, którzy, ku, lat, lecz, lub, ma, macie, mają, mając, mająca, mające, mający, mało, mam, mamy, masz, mą, me, mego, mej, memu, mi, miał, miałł, miała, miałaby, miałabym, miałabyś, miałam, miałaś, miałby, miałbym, miałbyś, miałem, miałeś, miało, miały, miałyby, miałybyście, miałybyśmy, miałyście, miałyśmy, miano, mieć, miej, miejcie, miejmy, mieli, mieliby, mielibyście, mielibyśmy, mieliście, mieliśmy, mię, między, mimo, mną, mnie, mogą, mogąc, mogąca, mogące, mogący, mogą, mogli, mogliby, moglibyście, moglibyśmy, mogliście, mogliśmy, mogła, mogłaby, mogłabym, mogłabyś, mogłam, mogłaś, mogłem, mogłeś, mogło, mogłoby, mogłobym, mogłobyś, mogłom, mogłoś, mogły, mogłyby, mogłybyście, mogłybyśmy, mogłyście, mogłyśmy, moi, moich, moim, moimi, moja, moją, moje, mojego, mojej, mojemu, może, możecie, możemy, możesz, możliwe, można, móc, mógł, mógłby, mógłbym, mógłbyś, mój, mu, musi, musiał, musiała, musiałaby, musiałabym, musiałabyś, musiałam, musiałaś, musiałby, musiałbym, musiałbyś, musiałem, musiałeś, musiało, musiałoby, musiałobym, musiałobyś, musiałom, musiałoś, musiały, musiałyby, musiałybyście, musiałybyśmy, musiałyście, musiałyśmy, musicie, musicie, musieli, musieliby, musielibyście, musielibyśmy, musieliście, musieliśmy, musimy, musisz, muszq, muszqca, muszqce, muszqcy, muszq, my, mych, mym, mymi, na, nad, najbardziej, nam, nami, nań, naokoło, naprzeciw, nas,*

<sup>87</sup>Our list of Polish stop words is based on <https://pl.wikipedia.org/wiki/Wikipedia:Stopwords>, with extensive additions to roughly match their counterparts in English. In particular, we have included all the inflected forms of *co* “what”, *każdy* “every”, *kto* “who”, *nikt* “nobody”, *nic* “nothing”, *wszyscy*, *wszystek*, *wszystkie*, *wszystko* “all (in various genders)” and all the personal pronouns.

*nasí, nasz, nasza, naszą, nasze, naszego, naszej, naszemu, naszych, naszym, naszymi, natomiast, natychmiast, nawet, nią, nic, nich, niczego, niczemu, niczym, nie, niech, niechaj, nieco, niego, niej, niektóre, niektórych, niektórym, niektórymi, niektóryzy, niemu, nigdy, nikim, nikogo, nikomu, nikt, nim, nimi, niż, no, o, oba, obaj, obie, obiema, oboje, obojga, obojgiem, obojgu, obok, oboma, obu, oby, obym, obys, obyscie, obysmy, od, około, on, ona, one, oni, ono, oprócz, oraz, oto, owa, ową, owe, owego, owej, owemu, owi, owo, owszem, owych, owym, owymi, ów, pan, pana, pani, po, pod, podczas, pomiędzy, pomimo, ponad, ponieważ, poprzez, potem, powinien, powinieniem, powinienes, powinna, powinnam, powinnaś, powinni, powinniście, powinniśmy, powinno, powinny, powinnyście, powinnyśmy, poza, później, prawie, przeciw, przeciw, przeciwko, przed, przede, przedtem, przez, przy, razem, roku, również, sam, sama, samą, same, samego, samej, samemu, sami, samo, samych, samym, samymi, są, siebie, się, skąd, skądś, skoro, sobą, sobie, spomiędzy, sponad, sposób, spośród, spoza, swa, swą, swe, swego, swej, swemu, swoi, swoich, swoim, swoimi, swoja, swoją, swoje, swojego, swojej, swojemu, swój, swych, swym, swymi, ta, tacy, tak, taka, taką, taki, takich, takie, takiego, takiej, takiemu, takim, takimi, także, tam, tamci, tamta, tamtą, tamte, tamtego, tamtej, tamtemu, tamten, tamto, tamtych, tamtym, tamtymi, tą, te, tego, tej, temu, ten, teraz, też, tę, to, tobą, tobie, toteż, trzeba, tu, tutaj, twa, twą, twe, twego, twej, twemu, twoi, twoich, twoim, twoimi, twoja, twoją, twoje, twojego, twojej, twojemu, twój, twych, twym, twymi, ty, tych, tyle, tylko, tyloma, tylu, tym, tymi, tyś, u, w, wam, wami, was, wasi, wasz, wasza, waszą, wasze, waszego, waszej, waszemu, waszych, waszym, waszymi, wbrew, we, wedlug, wiele, wieloma, wielu, więc, więcej, wkrótce, właśnie, wobec, wszak, wszakże, wszyscy, wszystek, wszystka, wszystką, wszystkich, wszystkie, wszystkiego, wszystkiej, wszystkimu, wszystkim, wszystkimi, wszystko, wśród, wtedy, wy, z, za, zapewne, zaraz, zaś, zawsze, zbyt, ze, zł, znowu, znów, został, zza, ż, żaden, żadna, żadne, żadnych, że, żeby,*

then we consider it a Polish stop word. All the Polish stop words that appear in a particular document need to be ignored before we perform word clustering on the rest of the vocabulary list. □

In addition, we define string patterns **eatPolish**, **givePolish**, **MissPolish**, **MrsPolish** through inflected forms of four Polish words:

*jada, jadać, jadaj, jadają, jadając, jadająca, jadające, jadający, jadal, jadał, jadała, jadale, jadało, jadały, jadana, jadane, jadani, jadanie, jadano, jadany, jadasz, jadł, jadła, jadle, jadło, jady, je, jedli, jedz, jedzą, jedząc, jedząca, jedzące, jedzący, jedzeni, jedzenie, jedzona, jedzone, jedzono, jedzony, jesz, jeść* — “eat”;

*da, dacie, dać, dadzą, daj, dają, dając, dająca, dające, dający, dajcie, daje, dajecie, dajemy, dajesz, daję, dajmy, dali, daliby, dalibyście, dalibyśmy, daliście, daliśmy, dał, dała, dałaby, dałabym, dałabyś, dałam, dałaś, dalby, dalbym, dalbyś, dałem, dales, dało, dałoby, dały, dałyby, dałybyście, dałybyśmy, dałyście, dałyśmy, dam, damy, dana, dane, dani, danie, dano, dany, dasz, dawać, dawaj, dawajcie, dawajmy, dawali, dawaliby, dawalibyście, dawalibyśmy, dawaliście, dawaliśmy, dawal, dawala, dawalaby, dawalabym, dawalabyś, dawalam, dawalaś, dawalby, dawalbym, dawalbyś, dawalem, dawales, dawalo, dawalo1, dawaloby, dawaly, dawalyby, dawalybyście, dawalybyśmy, dawalyście, dawalyśmy, dawana, dawane, dawani, dawanie, dawano, dawany, dawszy* — “give”;

*panna, pannach, pannami, panną, pannę, pannie, panno, pannom, panny* — “Miss”;

*paniach, paniami, panią, panie, paniom, pań* — “Mrs”.

In order to stay consistent with their counterparts in English, we are not going to treat these string patterns as stop words in Polish. Instead, we will exploit them in clustering of Polish content words.

### 7.1.1 Effective spelling and essential root

It is assumed that all Polish words are converted to lowercase<sup>88</sup> before going through any of the procedures below.

**Definition 7.2** (Polish Vowels and Verb Prefixes). Hereafter in §7.1, the symbol **V** stands for any member from the list of Polish vowels {*a, q, e, ę, i, o, ó, u, y*}. In line with the multiplicity notations introduced in Definition 3.3, the symbol **V<sub>m</sub>** stands for a text string formed by consecutive appearance of one or more (not necessarily identical or distinct) members from the set of Polish vowels.

Dual to the notations above, the symbol **C** stands for any character that does not belong to the list {*a, q, e, ę, i, o, ó, u, y*}, and **C<sub>m<sub>0</sub></sub>** stands for a text string formed by consecutive appearance of zero or more (not necessarily identical or distinct) characters that do not belong to the same list.

The symbol **P** = ( $\emptyset$ |*do|na|nad|o|ob|obe|po|pod|pode|prze|przed|przy|roz|s|sj|u|w|we|wy|z|za|ze*) represents the possible prefix of a Polish verb. □

<sup>88</sup>As of v11.0, *Mathematica* does not produce conversions  $A \rightarrow a, E \rightarrow e, \acute{N} \rightarrow n, \acute{S} \rightarrow s, \acute{Z} \rightarrow z, \acute{Z} \rightarrow z$  upon invoking the `ToLowerCase` operation. Therefore, case conversions for these special Polish letters need to be hand-coded if one implements our algorithm in *Mathematica*.

**Algorithm 7.3** (Polish effective spelling). For a Polish word  $\hat{\sigma}$ , its effective spelling  $\text{EffSpell}(\hat{\sigma})$  is constructed in sequential steps:

(1) Replace

|                                        |                                                                         |          |                                  |                     |                                   |                         |                            |            |            |         |
|----------------------------------------|-------------------------------------------------------------------------|----------|----------------------------------|---------------------|-----------------------------------|-------------------------|----------------------------|------------|------------|---------|
| <b>Prze(cz k)</b>                      | $(\emptyset co)dzienn\sim$                                              |          | $(\emptyset naj)czarn\sim$       |                     | $(\emptyset naj)koniecz\sim$      |                         |                            |            |            |         |
| <b>Přvĕk</b>                           | dni                                                                     |          | βlak                             |                     | v̄secz                            |                         |                            |            |            |         |
| $(\emptyset naj)wyżs(\emptyset z)\sim$ | $(\emptyset naj)zim\sim$                                                |          | $(\emptyset o)żeni\sim$          |                     | $(\emptyset o po)(ślub żen)i\sim$ |                         | $(\emptyset prze)czyt\sim$ |            |            |         |
| ηwyκη                                  | ωiv̄τ                                                                   |          | małżeństwo                       |                     | małżeństwi                        |                         | pczytō                     |            |            |         |
| $(\emptyset wy)marz\sim$               | $(mężat zameżn żonat)\sim$                                              |          | $(ojcz tat)ul(\emptyset e)k\sim$ |                     | $(s ś)piesz$                      |                         | $(u z)mar(l l)X\sim$       |            |            |         |
| δριμ                                   | małżeństw                                                               |          | ojc                              |                     | χυρ                               |                         | μoρτ                       |            |            |         |
| bogat~                                 | bram~                                                                   | dłu(g ż) | dziewię~                         | dzwo~               | idea(l ł)~                        | ident~                  | iii                        | imi~       | karol~     | katarz~ |
| ρbkit                                  | βραμ                                                                    | λογ      | 9e                               | δζwo                | ιδεαλ                             | ιδεv̄τ                  | 3                          | v̄αμ       | καρλ       | καταρζ  |
| kieli(ch sz)~                          | ksi(qżecz ędz ęg)                                                       |          | marc~                            | martw               | milicj~                           | odC~                    |                            | opl~       | pami(q ę)~ |         |
| καλx                                   | książ                                                                   |          | μ3αρ                             | μoρτ                | μιλτ                              | qC                      |                            | opλ        | μpεμy      |         |
| panowie                                | plan                                                                    | plac     | pocz                             | poje~               | pok(o ó)i                         | pok(o ó)j               | poka(z ż)~                 | popul~     | ptaX~      | robi~   |
| panach                                 | πλαv̄                                                                   | placn    | ποξ                              | je                  | ρyμoi                             | ρyμoj                   | σxοω                       | ποπυλ      | βipδ       | zrobi   |
| rozpracz~                              | rób~                                                                    | skr~     | sp(o ó)C~                        | stan(o ó)w          |                                   | stos                    | str~                       | sześ(c ć)~ |            | świad~  |
| δεσπp                                  | zrob                                                                    | σkp      | sCp                              | koiv̄τw             |                                   | stoσ                    | σtp                        | 6          |            | ωiv̄σ   |
| świat~                                 | tajemnicz~                                                              |          | trz(y e(ch j m ma))~             |                     | tysi(q ę)c~                       |                         | uczū                       |            | ujemn~     |         |
| ωświlō                                 | μyσticz                                                                 |          | 3e                               |                     | mIil                              |                         | φily                       |            | ωjemn      |         |
| um(∅ a ie)r(∅ z)X~                     | upły~                                                                   | v        | wiejsk~                          | wizj~               | woln                              | wy(s ł sy ł ście ł śl)~ |                            | wymien~    | wynajd~    |         |
| μoρτ                                   | ωpły                                                                    | 5        | ρyρλ                             | ωisj                | φipn                              | σeiv̄δ                  |                            | ξmien      | βynajd     |         |
| wynal(a e)(z ż)~                       | wyso(c k)~                                                              | wzmian~  | x                                | zaw(∅ a ie)r(∅ z)X~ |                                   | zię(c ć)~               |                            | zi~        | zna(cz k)~ |         |
| βynajdo                                | ηwyκη                                                                   | μmeiv̄τn | 10                               | iv̄κλ               |                                   | iv̄λαω                  |                            | ζi         | ζv̄ak      |         |
| zna(a e)(z ż)~                         | zys(k zcz)~                                                             |          | ży(j ł łt)~                      |                     | <b>MissPolish</b>                 |                         |                            |            |            |         |
| znajdo                                 | γav̄                                                                    |          | živ̄ć                            |                     | miβ                               |                         |                            |            |            |         |
| <b>MrsPolish</b>                       | $(\emptyset z)eatPolish(\emptyset by)(\emptyset ś)(\emptyset cie m my)$ |          |                                  |                     | $(i ś szli)$                      |                         |                            |            |            |         |
| μipσ                                   | εατ                                                                     |          |                                  |                     | idż                               |                         |                            |            |            |         |
| $czu(j ł łt ~ć)$                       | de                                                                      | l        | lady                             | rzec                | ta(cie tach)                      | tat(V m w) <sub>m</sub> |                            | ~Cze       |            |         |
| φilyć                                  | δeε                                                                     | 50       | damskich                         | rzekl               | ojcu                              | ojcu                    |                            | C          |            |         |

(2) Replace

|                                        |             |             |                                       |             |                    |                                   |          |         |         |        |
|----------------------------------------|-------------|-------------|---------------------------------------|-------------|--------------------|-----------------------------------|----------|---------|---------|--------|
| <b>Pmieszaz~</b>                       | <b>Ptrz</b> |             | $(do na o od po roz wy za)(łoz łóž)~$ |             |                    |                                   |          |         |         |        |
| mixa                                   | Ptp         |             | kład                                  |             |                    |                                   |          |         |         |        |
| $X^E((poj przyj)(q ę m))~$             | brać~       | chud(l łn)~ | cie(ni ń)~                            | ciesz~      | czc                | dba~                              | domyst~  | domys~  | doskon  | drzew~ |
| σX                                     | wziąć       | ωoτ         | oμβ                                   | ξeσ         | czτ                | δyβa                              | myst     | mys     | πεpφ    | δrzew  |
| licz(∅ b)~                             | list~       | łamχ        | łaśc                                  | maj(q ę)t~  | mal~               | miejsc~                           | miesiąc~ | mieszk~ | miękkko | milcz~ |
| v̄yμα                                  | λιστ        | μλαμχ       | σλαśc                                 | φοpτ        | μαλ                | miejστ                            | μoiv̄sc  | mieszκ  | miękkej | qit    |
| opin~                                  | op~         | os(o ó)b~   | pan(ow uj)~                           | pi(s sz ś)X |                    | piecz(q ę)~                       |          | piosenk |         | praw   |
| ωpiv̄n                                 | ωp          | oσoβ        | κοτpλ                                 | πισ         |                    | σilya                             |          | śpiewać |         | pραβ   |
| przedmio(c t)X~                        | przekon~    | qm(a o ó)w  | rze(cz kq kę)~                        | serc~       | slab               | straż~                            | szczęś   | szedł   | ślicz~  | ślub   |
| θiy                                    | βλιφ        | δεiv̄η      | rzekl                                 | serdecz     | sβlaβ              | φip                               | ηαπ      | chodz   | βur     | σlub   |
| uszy $X^E(c ć j k ł łt)~$              | will~       | zach~       | zna~                                  | zobacz~     | życz~              | $(i ście i ś szli szłobym szłom)$ |          |         |         |        |
| szyX                                   | βily        | Ξ           | zna                                   | widzi       | ωis                | szedlem                           |          |         |         |        |
| $przyjaci(e o ó)(l ł)(\emptyset c k)X$ | ś(ś w)      |             | ~#χ <sub>m0</sub>                     |             | $\sim X^E(k ł)ach$ |                                   | ~kich    | ~oce    |         |        |
| przyjak                                | święta      |             | ∅                                     |             | Xa                 |                                   | ki       | oc      |         |        |

(3) Do dom~ → δομ, pie(c|cz|k) → βακ, **givePolish**(∅|by)(∅|ś)(∅|cie|m|my) → dar, ~kacie → ka.

## (4) Replace

|                                                |                                                |                                                        |                                               |                                                          |                                                     |                                |                               |                          |                            |                            |                         |                  |
|------------------------------------------------|------------------------------------------------|--------------------------------------------------------|-----------------------------------------------|----------------------------------------------------------|-----------------------------------------------------|--------------------------------|-------------------------------|--------------------------|----------------------------|----------------------------|-------------------------|------------------|
| $(\mathbf{P} \emptyset naj)t\sim$<br>$\lambda$ | $(\emptyset naj)gors(i z)\sim$<br>$\acute{z}l$ | $(\emptyset naj)gorzej\sim$<br>$\acute{z}le$           | $(\emptyset naj)lepiej\sim$<br>$\delta obrze$ | $(\emptyset naj)leps(i z)\sim$<br>$\delta obr$           |                                                     |                                |                               |                          |                            |                            |                         |                  |
| $(\emptyset naj)mniej(s i z)\sim$<br>$mał$     | $(\emptyset naj)więks(i z)\sim$<br>$duż$       | $(\emptyset za)ta(niec ńc)(\emptyset z)\sim$<br>$tańc$ | $(mów powie)\sim$<br>$\pi owie$               | $(my umy)\sim$<br>$u\mu y$                               |                                                     |                                |                               |                          |                            |                            |                         |                  |
| $(wiad wiedz)\sim$<br>$wie$                    | $X^{\in}(s z)t$<br>$Xjł$                       | $bra(c ć t)\sim$<br>$\beta bra$                        | $chc\sim$<br>$choc$                           | $cioc\sim$<br>$tsioc$                                    | $cioc\sim$<br>$tsioci$                              | $ciot(c ek k)\sim$<br>$tsioci$ | $dam\sim$<br>$d\delta a\mu m$ | $dar\sim$<br>$tdarc$     | $dobr\sim$<br>$\delta obr$ | $dumier$<br>$\delta umien$ | $dzieck\sim$<br>$dziec$ |                  |
| $ksi(q ę)dz\sim$<br>$księż$                    | $mam\sim$<br>$\mu am$                          | $mat(c ek k)\sim$<br>$\mu am$                          | $mył\sim$<br>$\tilde{y}\mu y$                 | $naj(\hat{x})_m X_1^{\in}(e j sz)X$<br>$(\hat{x})_m X_1$ | $nara X^{\in}(z ż)\sim$<br>$\tilde{y}araX$          | $od\sim$<br>$odz$              |                               |                          |                            |                            |                         |                  |
| $orz(e \emptyset ek k)\sim$<br>$orł$           | $pi(ą ł ę ć ć)\sim$<br>$\acute{s}a$            | $pies\sim$<br>$psa$                                    | $piln\sim$<br>$\pi iln$                       | $\acute{s}n$<br>$sn$                                     | $tydzień\sim$<br>$tygodni$                          | $wielk\sim$<br>$duż$           | $wuj(ek k)\sim$<br>$wuj$      | $zł\sim$<br>$\acute{z}l$ | $zdum\sim$<br>$z\delta um$ | $zmi\sim$<br>$\zeta mi$    | $znał\sim$<br>$znaj$    | $dzień$<br>$dni$ |
| $(ojciec ojcze)$<br>$ojcach$                   | $kwiecień$<br>$kwietni$                        | $oj$<br>$yoj$                                          | $pić$<br>$pici$                               | $tatu(s \sim\acute{s})$<br>$ojc$                         | $uch((\emptyset V)(\emptyset ch m mi))$<br>$uszach$ | $wielce$<br>$duż$              |                               |                          |                            |                            |                         |                  |

(5) Do  $ch \rightarrow s\chi$ ,  $cz \rightarrow \acute{c}$ ,  $ł \rightarrow l$ ,  $ó \rightarrow o$ ,  $sz \rightarrow \acute{s}$ ,  $\sim del \rightarrow \emptyset$ ,  $\sim i \rightarrow j$ .(6) Do  $wi(ad|edz) \rightarrow wie$ ,  $Ci \rightarrow Cji$ ,  $X^{\in}(\mathbf{P}mow)\sim \rightarrow X\mathbf{maw}$ , and call the result  $\hat{\sigma}'$ .(7) Break down  $\hat{\sigma}' = \hat{\sigma}'_1 \hat{\sigma}'_2$  into the concatenation of two strings  $\hat{\sigma}'_1 = \hat{\sigma}'^{[\min\{\lambda(\hat{\sigma}'), \ell(\hat{\sigma}')\}]}$  (see the notation in Definition 3.1) and  $\hat{\sigma}'_2$ , where  $\lambda(\hat{\sigma}') - 1$  equals either the last position occupied by the string pattern  $(\mathbf{P}|bez(\emptyset|e)|n|jie|pa|st(\emptyset|r))\hat{x}\sim$  in the non-void  $\hat{\sigma}'$ , or  $-1$  if  $\hat{\sigma}' = \emptyset$ .(8) On  $\hat{\sigma}'_2$ , perform the following substitutions in a sequel:

## (8.1) Replace

|                                             |                                                    |                  |                             |                                                                                 |                                                                                                                                                                                                                                                                      |
|---------------------------------------------|----------------------------------------------------|------------------|-----------------------------|---------------------------------------------------------------------------------|----------------------------------------------------------------------------------------------------------------------------------------------------------------------------------------------------------------------------------------------------------------------|
| $X^{\in}(g k l)j$<br>$X$                    | $ck$<br>$c$                                        | $dzk$<br>$d$     | $\acute{n}c$<br>$\acute{n}$ | $ow(\emptyset \acute{c} ji \acute{c} ec) nji(\emptyset c k) sk)$<br>$\emptyset$ | $(a(c st t) l jiw (\emptyset aw nji)\acute{c}(\emptyset y k \sim ycy) njisk (a(l r)n(\emptyset ji))$<br>$(a\acute{c}(\emptyset celk) a(\emptyset \acute{n}s) k ar(ce k z) by dl icie ł i(st \acute{s}ci w) kac j s(k tw) y (cie ł st \acute{s}ci w))$<br>$\emptyset$ |
| $\sim a(\acute{c}ek cy rek)$<br>$\emptyset$ | $\sim X^{\in}(nt st)(ce ek k)\hat{x}_{m_0}$<br>$X$ | $\sim ij$<br>$i$ | $\sim mjię$<br>$mjienj$     |                                                                                 |                                                                                                                                                                                                                                                                      |

(8.2) Do  $kV \rightarrow V$ ,  $\sim(ce|k) \rightarrow \emptyset$ ,  $\sim((a|ily)s\chi|e|ego|em|emu|im|mj|ow(\emptyset|j)V_{m_0}|om|um|ym|V\acute{c}) \rightarrow \emptyset$ .The result after these two steps of operations is called  $\hat{\sigma}'_2$ .(9) Concatenate  $\hat{\sigma}'_1$  and  $\hat{\sigma}'_2$ .(10) Do  $\acute{c} \rightarrow cj$ ,  $\acute{n} \rightarrow nj$ ,  $\acute{s} \rightarrow sj$ ,  $\acute{z} \rightarrow zj$ .**Definition 7.4** (Polish protected range). Let  $\hat{\sigma}$  be a text string derived from a Polish word, its protected range  $\text{ProtRg}(\hat{\sigma}) = \min\{\lambda_1(\hat{\sigma}), \lambda_2(\hat{\sigma})\}$  is determined by two non-negative integers  $\lambda_1(\hat{\sigma})$  and  $\lambda_2(\hat{\sigma})$  specified through the following procedures:

- Look for the string pattern  $(na|u|we|wy)_{m_0} C_{m_0} V(j|\acute{s})_{m_0}\sim$  in the string  $\hat{\sigma}$ ;
- If the string pattern above is found, the last position occupied by such a string defines  $\lambda_1(\hat{\sigma})$ ; otherwise, set  $\lambda_1(\hat{\sigma}) = 0$ ;
- Look for the pattern  $(na|po|prze|przy|roz|s|w|wy|z)V_{m_0} CV_{m_0} C\sim$  in the string  $\hat{\sigma}$ ;
- If the pattern above is found, the last position occupied by such a pattern defines  $\lambda_2(\hat{\sigma})$ ; otherwise, set  $\lambda_2(\hat{\sigma}) = \ell(\hat{\sigma})$ .  $\square$

**Algorithm 7.5** (Polish essential root). Let  $\hat{\sigma}$  be the effective spelling of a Polish word, then its corresponding essential root  $\text{EssRoot}(\hat{\sigma})$  is constructed in the following steps:(1) Break down  $\hat{\sigma} = \hat{\sigma}'_1 \hat{\sigma}'_2$  into the concatenation of two strings  $\hat{\sigma}'_1 = \hat{\sigma}^{[\text{ProtRg}(\hat{\sigma})]}$  (see the notation in Definition 3.1) and  $\hat{\sigma}'_2$ , where the length of the first string  $\ell(\hat{\sigma}'_1) = \text{ProtRg}(\hat{\sigma})$  is equal to the protected range of  $\hat{\sigma}$ .(2) On  $\hat{\sigma}'_2$ , perform the following substitutions in a sequel:(2.1) Do  $\sim V_m \rightarrow \emptyset$ .

(2.2)  $Do \sim \mathbf{V}_m(m|n(\emptyset|j)|w\delta) \rightarrow \mathbf{V}_m, \sim \mathbf{V}_{m_0}\delta \rightarrow \mathbf{V}_{m_0}, \sim(ac|qt|ęc|j|ęt) \rightarrow \emptyset.$

(2.3)  $Do \sim \mathbf{V}_m \rightarrow \emptyset.$

The result after these three steps of operations is called  $\hat{\sigma}'_2$ .

(3) Concatenate  $\hat{\sigma}_1$  and  $\hat{\sigma}'_2$ .

In Polish (as well as Russian and many other Slavic languages), the imperfect and perfect aspects of the same verb may differ by a prefix. To improve the performance of verb clustering, we need the following extensions to Definition 7.4 and Algorithm 7.5.

**Definition 7.6** (Polish verbal protected range). Let  $\hat{\sigma}$  be a text string derived from a Polish word, its verbal protected range  $\text{VbProtRg}(\hat{\sigma})$  is an integer determined as follows:

- Try to find the string pattern  $(do|na|o|odz|po|prze|we|wy)_{m_0} \mathbf{C}_{m_0} \mathbf{V}(j|l)_{m_0} \sim$  in the string  $\hat{\sigma}$ ;
- If the string pattern above is found, the last position occupied by such a string defines  $\text{VbProtRg}(\hat{\sigma})$ ; otherwise, set  $\text{VbProtRg}(\hat{\sigma}) = 0.$   $\square$

**Algorithm 7.7** (Polish verbal essential root). Let  $\hat{\sigma}$  be the token string associated with a Polish word, then its corresponding verbal essential root  $\text{VbEssRoot}(\hat{\sigma})$  is constructed in the following steps:

- (1) Break down  $\hat{\sigma} = \hat{\sigma}_1 \hat{\sigma}_2$  into the concatenation of two strings  $\hat{\sigma}_1 = \hat{\sigma}^{[\text{VbProtRg}(\hat{\sigma})]}$  (see the notation in Definition 3.1) and  $\hat{\sigma}_2$ , where the length of the first string  $\ell(\hat{\sigma}_1) = \text{VbProtRg}(\hat{\sigma})$  is equal to the verbal protected range of  $\hat{\sigma}$ .
- (2) Do  $\sim(\mathbf{V}_{m_0}(\ell(\mathbf{V}_{m_0}(\emptyset|c|s|m)(\emptyset|j)(\emptyset|m))))_{m_0} \rightarrow \emptyset$  on  $\hat{\sigma}_2$ , and call the result  $\hat{\sigma}'_2$ .
- (3) Concatenate  $\hat{\sigma}_1$  and  $\hat{\sigma}'_2$ .
- (4) Do  $\sim \hat{\chi}^{\in}(d|m|n|r|s|w|z)j \rightarrow \hat{\chi}, \sim c(\emptyset|j) \rightarrow t, \sim z \rightarrow z.$
- (5) Replace

|                                          |           |              |                      |             |
|------------------------------------------|-----------|--------------|----------------------|-------------|
| $(bjierz bjior br bra bran wez wz wzji)$ | $\sim dn$ | $l(a al ej)$ | $pji(\emptyset j t)$ | $\sim zdz$  |
| <i>bral</i>                              | <i>d</i>  | <i>lan</i>   | <i>pjil</i>          | <i>zjdz</i> |

(6) Replace

|                                                                          |                                   |                                                                    |  |  |
|--------------------------------------------------------------------------|-----------------------------------|--------------------------------------------------------------------|--|--|
| $(\emptyset do na o odz po roz wy za)kla(\emptyset d dd dz)$             |                                   |                                                                    |  |  |
| <i>klad</i>                                                              |                                   |                                                                    |  |  |
| $(\emptyset w)(i id idz s\chi odz s\chi la s\chi lo s\chi ly s\chi ji)$  | $(\emptyset w)(jad jedz jes\chi)$ | $\mathbf{X}_1^{\in}(do ob odz po przy wy)(jad jedz jes\chi jezdz)$ |  |  |
| <i>s\chi odz</i>                                                         | <i>jes\chi</i>                    | $\mathbf{X}'_1 jes\chi$                                            |  |  |
| $\mathbf{X}_2^{\in}(do odz odze po przy we wy)(j j d jdz s\chi odz sed)$ | $obejrz$                          | $odze(d j l s\chi odz)$                                            |  |  |
| $\mathbf{X}''_2 s\chi odz$                                               | <i>oglad</i>                      | <i>odz s\chi odz</i>                                               |  |  |

where  $\mathbf{X}'_1$  results from doing  $przy \rightarrow \pi rzy$  on  $\mathbf{X}_1$  and  $\mathbf{X}''_2$  results from doing  $odze \rightarrow odz, przy \rightarrow \pi rzy$  on  $\mathbf{X}_2$ .

### 7.1.2 Admissible mutation and approximate clustering

In Polish (as well as Russian and many other Slavic languages), fleeting vowels may appear or disappear in inflected forms of the same word. We need to heuristically detect and remove these fleeting vowels to achieve better clustering results. Meanwhile, in Polish (as well as Russian and many other Slavic languages), one encounters vowel alternations in verb conjugations, as in Spanish or the Germanic languages.

**Algorithm 7.8** (Polish vowel blotting). For a token string  $\hat{\sigma}$ , its blotted form  $\text{BlotFltV}(\hat{\sigma})$  is constructed as follows:

- (1) Do  $\sim \mathbf{C}(e|jie|jio)\hat{\chi}^{\in}(c|k|l|n|r|s|w) \rightarrow \mathbf{C}\hat{\chi}.$
- (2) Do  $\sim \hat{\chi}kier \rightarrow \hat{\chi}kr.$
- (3) Do  $q \rightarrow e, i(a|o) \rightarrow ie.$

In what follows, we will construct a bivariate Boolean-valued function  $\text{HrdTest}(\hat{\alpha}, \hat{\beta})$  on a “simple heredity test function” in Algorithm 7.9, and a set of “admissible suffix mismatch” rules in Algorithm 7.10.

**Algorithm 7.9** (Simple heredity test). Let  $\hat{\alpha}'$  be a string obtained from  $\hat{\alpha}$  by the following steps:

(1) Break down  $\hat{\alpha} = \hat{\alpha}_1\hat{\alpha}_2$  into the concatenation of two strings  $\hat{\alpha}_1 = \hat{\alpha}^{\lfloor \min\{3, \ell(\hat{\alpha})\} \rfloor}$  (see the notation in Definition 3.1) and  $\hat{\alpha}_2$ , where the length of the first string  $\ell(\hat{\alpha}_1) = \min\{3, \ell(\hat{\alpha})\}$  is equal to 3 or the length of  $\hat{\alpha}$ , whichever is shorter.

(2) On  $\hat{\alpha}_2$ , perform the following substitutions in a sequel:

(2.1) Do  $\sim\mathbf{C}_m \rightarrow \mathbf{X}'$ , where  $\mathbf{X}'$  is obtained from  $\mathbf{C}_m$  by deleting all the occurrences of the letter “j”.

(2.2) Do  $\sim(n|(\mathbf{V}_{m_0}(l|n|\tilde{s}|t|w)_{m_0})_m) \rightarrow \emptyset$ .

The result after these two steps of operations is called  $\hat{\alpha}'_2$ .

(3) Construct  $\hat{\alpha}' = \text{BlotFltV}(\hat{\alpha}_1\hat{\alpha}'_2)$ .

Define  $\hat{\beta}'$  similarly. The Boolean-valued function  $\text{SimpHrdTest}(\hat{\alpha}, \hat{\beta})$  returns **TRUE** if the lowercase form of  $\hat{\alpha}$  contains at least one instance of  $\{q, a, e, \acute{e}, i, l, n, o, \acute{o}, r, u, y\}$  **AND** at least one of the following six conditions holds:<sup>89</sup>

(i)  $\hat{\alpha} = \hat{\beta}$ ;

(ii)  $\hat{\beta} = \hat{\alpha}in$ ;

(iii)  $\hat{\beta} = \hat{\alpha}n$ ;

(iv)  $\hat{\beta} = \hat{\alpha}z$ ;

(v)  $\min\{\ell(\hat{\alpha}'), \ell(\hat{\beta}')\} \geq 3$  **AND** ( $\hat{\alpha} = \hat{\beta}'$  **OR**  $\hat{\alpha}' = \hat{\beta}$  **OR**  $\hat{\alpha}' = \hat{\beta}'$  **OR**  $\hat{\beta}' = \hat{\alpha}'z$ ).

(vi)  $\ell(\hat{\beta}) > \ell(\hat{\alpha}) \geq \frac{\ell(\hat{\beta})}{3}$  **AND**  $\hat{\beta} = \hat{\alpha}(a|e|o)_m(m|t)$ .

In what follows, we define  $\text{SuffixNW}(\hat{\alpha}, \hat{\beta})$ ,  $\text{RootNW}(\hat{\alpha}, \hat{\beta})$ ,  $\text{NW}^*(\hat{\alpha}, \hat{\beta})$  and  $\text{SuffixSW}(\hat{\alpha}, \hat{\beta})$ ,  $\text{SuffixSW}(\hat{\alpha}, \hat{\beta})$ ,  $\text{SW}^*(\hat{\alpha}, \hat{\beta})$  as what is done in the Danish case (Algorithm 5.7), which was also applied to two other Germanic languages treated in §5. Particular to the Polish case, we further define  $\text{SuffixNW}'(\hat{\alpha}, \hat{\beta})$  by performing the substitutions  $(e|j|ie)\sim \rightarrow \emptyset$ ,  $\sim j \rightarrow \emptyset$ ,  $\sim jc \rightarrow c$  to both components of  $\text{SuffixNW}(\hat{\alpha}, \hat{\beta})$ , in a single sweep. The notation  $\text{SuffixSW}'(\hat{\alpha}, \hat{\beta})$  is defined similarly. If  $\text{SuffixNW}'(\hat{\alpha}, \hat{\beta}) = [\hat{\tau}_1, \hat{\tau}_2]$ , then  $\text{SuffixNW}'(\hat{\beta}, \hat{\alpha}) = [\hat{\tau}_2, \hat{\tau}_1]$ .

**Algorithm 7.10** (Admissible suffix mismatch and vowel alternation). For two strings  $\hat{\alpha}$  and  $\hat{\beta}$ , the Boolean-valued function

$$\text{AdmMut}(\text{RootNW}(\hat{\alpha}, \hat{\beta}), \text{SuffixNW}(\hat{\alpha}, \hat{\beta}), \text{NW}^*(\hat{\alpha}, \hat{\beta}))$$

returns **TRUE** if  $\text{NW}^*(\hat{\alpha}, \hat{\beta}) = \emptyset|[a, e]||[a, o]||[q, \acute{e}]||[e, o]$  **AND**  $\text{RootNW}(\hat{\alpha}, \hat{\beta})$  contains at least one instance of  $\{q, a, e, \acute{e}, i, l, n, o, \acute{o}, r, u, y\}$  **AND** at least one of the following three conditions holds:

(i)  $\text{SuffixNW}'(\hat{\alpha}, \hat{\beta}) = [\emptyset, \emptyset]||[\emptyset, b]||[\emptyset, e]||[\emptyset, ie]||[c, k]||[c, t]||[\acute{c}, k]||[dz, g]||[j|c, t]||[s, \acute{s}]||[s\chi, s]||[s\chi, \acute{s}]||[z, \acute{z}]||[zd, \acute{z}d\acute{z}]||[zg, \acute{z}d\acute{z}]$ ;

(ii)  $\text{SuffixNW}'(\hat{\beta}, \hat{\alpha}) = [\emptyset, \emptyset]||[\emptyset, b]||[\emptyset, e]||[\emptyset, ie]||[c, k]||[c, t]||[\acute{c}, k]||[dz, g]||[j|c, t]||[s, \acute{s}]||[s\chi, s]||[s\chi, \acute{s}]||[z, \acute{z}]||[zd, \acute{z}d\acute{z}]||[zg, \acute{z}d\acute{z}]$ ;

(iii)  $\text{SuffixNW}(\hat{\alpha}, \hat{\beta}) = [\emptyset|(\emptyset|j|l)\mathbf{V}_{m_0}(\emptyset|m|sj)(\emptyset|m|cj), \emptyset|(\emptyset|j|l)\mathbf{V}_{m_0}(\emptyset|m|sj)(\emptyset|m|cj)]$ .

Similarly, one can evaluate another Boolean-valued function

$$\text{AdmMut}(\text{RootSW}(\hat{\alpha}, \hat{\beta}), \text{SuffixSW}(\hat{\alpha}, \hat{\beta}), \text{SW}^*(\hat{\alpha}, \hat{\beta}))$$

by trading all the occurrences of **NW** in the statements above with **SW**.

**Algorithm 7.11** (Heredity test function). For two strings  $\hat{\alpha}$  and  $\hat{\beta}$ , define  $\hat{\alpha}'$  and  $\hat{\beta}'$  as in Algorithm 7.9. The Boolean-valued function  $\text{HrdTest}(\hat{\alpha}, \hat{\beta})$  returns **TRUE** if at least one of the following three conditions holds:

(i)  $\text{SimpHrdTest}(\hat{\alpha}, \hat{\beta}) = \mathbf{TRUE}$ ;

(ii)  $\ell(\text{RootNW}(\hat{\alpha}, \hat{\beta})) \geq \frac{\max\{\ell(\hat{\alpha}'), \ell(\hat{\beta}')\}}{2}$  **AND**  $\text{AdmMut}(\text{RootNW}(\hat{\alpha}, \hat{\beta}), \text{SuffixNW}(\hat{\alpha}, \hat{\beta}), \text{NW}^*(\hat{\alpha}, \hat{\beta})) = \mathbf{TRUE}$ ;

(iii)  $\ell(\text{RootSW}(\hat{\alpha}, \hat{\beta})) \geq \frac{\max\{\ell(\hat{\alpha}'), \ell(\hat{\beta}')\}}{2}$  **AND**  $\text{AdmMut}(\text{RootSW}(\hat{\alpha}, \hat{\beta}), \text{SuffixSW}(\hat{\alpha}, \hat{\beta}), \text{SW}^*(\hat{\alpha}, \hat{\beta})) = \mathbf{TRUE}$ .

<sup>89</sup>As a general rule in this document, the truth values of items labeled with Roman numerals are connected to each other with logical **OR**.

**Algorithm 7.12** (Polish verb aspect test). *Let  $\text{NW}(\hat{\alpha}, \hat{\beta})$  be the result of performing Needleman–Wunsch alignment on strings  $\hat{\alpha}$  and  $\hat{\beta}$ . Let  $\mathbf{X}^*$  be an arbitrary non-empty string. The Boolean-valued function  $\text{VbAspTest}(\hat{\alpha}, \hat{\beta})$  returns **TRUE** if at least one of the following three conditions holds:*

- (i)  $\text{NW}(\hat{\alpha}, \hat{\beta}) = \mathbf{X}^*$  (in other words,  $\hat{\alpha} = \hat{\beta}$ );
- (ii)  $\text{NW}(\hat{\alpha}, \hat{\beta}) = [\mathbf{P}, \mathbf{P}]\mathbf{X}^*$  (in other words,  $\hat{\alpha}$  agrees with  $\hat{\beta}$  up to a pair of word initial mismatching strings, both of which are possible prefixes of Polish verbs);
- (iii)  $\text{NW}(\hat{\alpha}, \hat{\beta}) = [\mathbf{P}, \mathbf{P}]\mathbf{X}^*[[a, e]][[a, o]][[q, \varrho]][[e, o]]\mathbf{X}^*$ , where the two occurrences of  $\mathbf{X}^*$  may or may not represent the same non-empty string.

Note that Smith–Waterman alignment is not used in this test.

The first two stages in the following approximate clustering algorithm for Polish words are very similar to the English counterpart (Algorithm 4.15), while the third stage is tailored for the verb aspects in Polish.

**Algorithm 7.13** (Approximate clustering of Polish words). *The approximate clustering of a list of Polish words  $\{\hat{\alpha}_1, \dots, \hat{\alpha}_N\}$  is completed in three stages:*

- (1) *We sort the list  $\{(\hat{\alpha}_1, \text{EffSpell}(\hat{\alpha}_1)), \dots, (\hat{\alpha}_N, \text{EffSpell}(\hat{\alpha}_N))\}$  alphabetically according to the second component (effective spelling) of each entry. If two consecutive neighbors in the alphabetized list  $\{(\hat{\alpha}_{(1)}, \text{EffSpell}(\hat{\alpha}_{(1)})), \dots, (\hat{\alpha}_{(N)}, \text{EffSpell}(\hat{\alpha}_{(N)}))\}$  satisfies  $\text{HrdTest}(\text{EffSpell}(\hat{\alpha}_{(n)}), \text{EffSpell}(\hat{\alpha}_{(n+1)})) = \mathbf{FALSE}$ , where  $n \in \mathbb{Z} \cap [1, N)$ , then add a demarcation line between these two entries. In this way, the alphabetized list is divided into separate groups of words tagged with their effective spellings:  $\{g_1 = \{(\hat{\alpha}_{(1,1)}, \text{EffSpell}(\hat{\alpha}_{(1,1)})), \dots, (\hat{\alpha}_{(1,n_1)}, \text{EffSpell}(\hat{\alpha}_{(1,n_1)}))\}, \dots, g_M = \{(\hat{\alpha}_{(M,1)}, \text{EffSpell}(\hat{\alpha}_{(M,1)})), \dots, (\hat{\alpha}_{(M,n_M)}, \text{EffSpell}(\hat{\alpha}_{(M,n_M)}))\}$ , where each sublist also preserves alphabetic order. In particular, we have  $\hat{\alpha}_{(1,1)} = \hat{\alpha}_{(1)}$  and  $\hat{\alpha}_{(M,n_M)} = \hat{\alpha}_{(M)}$ .*
- (2) *For each group of words  $g_m = \{(\hat{\alpha}_{(m,1)}, \text{EffSpell}(\hat{\alpha}_{(m,1)})), \dots, (\hat{\alpha}_{(m,n_m)}, \text{EffSpell}(\hat{\alpha}_{(m,n_m)}))\}$  where  $m \in \mathbb{Z} \cap [1, M]$ , we augment it into a tagged entry  $G_m = (g_m, \text{EffSpell}(\hat{\alpha}_{(m,1)}), \text{EssRoot}(\text{EffSpell}(\hat{\alpha}_{(m,1)})), \text{BlotFltV}(\text{EssRoot}(\text{EffSpell}(\hat{\alpha}_{(m,1)}))))$ . The list  $\{G_1, \dots, G_M\}$  is sorted alphabetically, with respect to  $\text{BlotFltV}(\text{EssRoot}(\text{EffSpell}(\hat{\alpha}_{(m,1)})))$  (with highest priority),  $\text{EssRoot}(\text{EffSpell}(\hat{\alpha}_{(m,1)}))$  (with medium priority), and  $\text{EffSpell}(\hat{\alpha}_{(m,1)})$  (with lowest priority). If two consecutive neighbors in the alphabetized list  $\{G_{(1)} = (g_{(1)}, \hat{\gamma}'_{(1)}, \hat{\gamma}''_{(1)}, \hat{\gamma}'''_{(1)}), \dots, G_{(M)} = (g_{(M)}, \hat{\gamma}'_{(M)}, \hat{\gamma}''_{(M)}, \hat{\gamma}'''_{(M)})\}$  satisfy*

$$\text{SimpHrdTest}(\hat{\gamma}'''_{(m+1)}, \hat{\gamma}'''_{(m)}) = \mathbf{FALSE}$$

**AND**

$$\text{SimpHrdTest}(\hat{\gamma}'''_{(m)}, \hat{\gamma}'''_{(m+1)}) = \mathbf{FALSE}$$

**AND**

$$\text{HrdTest}(\hat{\gamma}'''_{(m+1)}, \hat{\gamma}'''_{(m)}) = \mathbf{FALSE}$$

**AND**

$$\text{HrdTest}(\hat{\gamma}'''_{(m)}, \hat{\gamma}'''_{(m+1)}) = \mathbf{FALSE}$$

**AND**

$$\text{HrdTest}(\hat{\gamma}'_{(m)}, \hat{\gamma}'_{(m+1)}) = \mathbf{FALSE}$$

where  $m \in \mathbb{Z} \cap [1, M)$ , then add a demarcation line between these two entries. In this manner, the alphabetized list  $\{G_{(1)}, \dots, G_{(M)}\}$  is divided into separate groups of tagged clusters  $\{\Gamma_1 = \{G_{(1,1)}, \dots, G_{(1,m_1)}\}, \dots, \Gamma_K = \{G_{(K,1)}, \dots, G_{(1,m_K)}\}\}$ . Generate a list of word clusters  $\{\check{\Gamma}_1 = (\check{G}_{(1,1)}, \dots), \dots, \check{\Gamma}_K = (\check{G}_{(K,1)}, \dots)\}$  by discarding all the tags (effective spellings, essential roots, vowel blotted forms) from each  $\Gamma_k$ , where  $k \in \mathbb{Z} \cap [1, K]$ .

- (3) *For each word cluster  $\check{\Gamma}_k = (\check{G}_{(k,1)}, \dots)$ , we augment it into a tagged entry*

$$\mathcal{G}_k \equiv (\check{\Gamma}_k, \check{\Gamma}'_k, \check{\Gamma}''_k) := (\check{\Gamma}_k, \text{EssRoot}(\text{EffSpell}(\check{G}_{(k,1)})), \text{VbEssRoot}(\text{EssRoot}(\text{EffSpell}(\check{G}_{(k,1)}))))$$

Recall that  $\hat{\sigma}^{-1}$  is the reverse of the string  $\hat{\sigma}$  (Definition 3.1). The list  $\{\mathcal{G}_1 = (\check{\Gamma}_1, \check{\Gamma}'_1, \check{\Gamma}''_1), \dots, \mathcal{G}_K = (\check{\Gamma}_K, \check{\Gamma}'_K, \check{\Gamma}''_K)\}$  is sorted sorted alphabetically, with respect to  $(\check{\Gamma}''_k)^{-1}$  (with higher priority) and  $\check{\Gamma}'_k$  (with lower priority). If two consecutive neighbors in the alphabetized list  $\{\mathcal{G}_{(1)} = (\check{\Gamma}_{(1)}, \check{\Gamma}'_{(1)}, \check{\Gamma}''_{(1)}), \dots, \mathcal{G}_{(K)} = (\check{\Gamma}_{(K)}, \check{\Gamma}'_{(K)}, \check{\Gamma}''_{(K)})\}$  satisfy

$$\text{VbAspTest}(\hat{\Gamma}''_{(k)}, \hat{\Gamma}''_{(k+1)}) = \mathbf{FALSE}$$

**AND**

$$\text{VbAspTest}(\hat{\Gamma}'_{(k)}, \hat{\Gamma}'_{(k+1)}) = \mathbf{FALSE}$$

where  $k \in \mathbb{Z} \cap [1, K)$ , then add a demarcation line between these two entries. In this manner, the alphabetized list  $\{\mathcal{G}_{(1)}, \dots, \mathcal{G}_{(K)}\}$  is divided into separate groups of tagged clusters  $\{\tilde{\Gamma}_1 = \{\mathcal{G}_{(1,1)}, \dots, \mathcal{G}_{(1,n_1)}\}, \dots, \tilde{\Gamma}_J = \{\mathcal{G}_{(J,1)}, \dots, \mathcal{G}_{(1,n_J)}\}\}$ , from which the output list of word clusters is generated, after removal of all the tags from each  $\tilde{\Gamma}_j$ , where  $j \in \mathbb{Z} \cap [1, J]$ .

*Example 7.13.1.* We refer to the Polish version of Wiktionary ([https://pl.wiktionary.org/wiki/Kategoria:Gramatyka\\_j%C4%99zyka\\_polskiego](https://pl.wiktionary.org/wiki/Kategoria:Gramatyka_j%C4%99zyka_polskiego)), for the divisions of declension and conjugation classes, of nouns and verbs respectively.

Here are some nouns that display the 1st masculine declension patterns:

*drani, drania, draniach, draniami, dranie, draniem, draniom, draniowi, draniów, draniu, drań* — “rascal”;

*goryl, goryla, gorylach, gorylami, goryle, gorylem, goryli, gorylom, goryłowi, goryłu* — “gorilla”;

*liści, liścia, liściach, liście, liściem, liściom, liściowi, liściu, liść, liśćmi* — “leaf”.

2nd masculine declension:

*owoc, owocach, owocami, owoce, owocem, owocom, owocowi, owoców, owocu* — “fruit”;

*stróż, stróża, stróżach, stróżami, stróżem, stróżom, stróżowi, stróżowie, stróżu, stróży* — “guard”;

*tasiemca, tasiemcach, tasiemcami, tasiemce, tasiemcem, tasiemcom, tasiemcowi, tasiemców, tasiemcu, tasiemiec* — “tapeworm”.

3rd masculine declension:

*chirurdzy, chirurg, chirurga, chirurgach, chirurgami, chirurgiem, chirurgom, chirurgowi, chirurgów, chirurgu* — “surgeon”;

*kożuch, kożucha, kożuchach, kożuchami, kożuchem, kożuchom, kożuchowi, kożuchów, kożuchu, kożuchy* — “sheepskin”;

*strażacy, strażak, strażaka, strażakach, strażakami, strażakiem, strażakom, strażakowi, strażaków, strażaku* — “fireman”.

4th masculine declension:

*chleb, chleba, chlebach, chlebami, chlebem, chlebie, chlebom, chlebowi, chlebów, chleby* — “bread”;

*doktor, doktora, doktorach, doktorami, doktorem, doktorom, doktorowi, doktorowie, doktorów, doktorze, doktorzy* — “doctor”;

*drozd, drozda, drozdach, drozdami, drozdem, drozdom, drozdowi, drozdów, drozdy, droździe* — “thrush”.

5th masculine declension:

*Marsjan, Marsjanach, Marsjanami, Marsjanie, Marsjanin, Marsjanina, Marsjaninem, Marsjaninie, Marsjaninowi, Marsjanom, Marsjany* — “Martian”.

1st neuter declension:

*pola, polach, polami, pole, polem, polom, polu, pól* — “field”;

*studia, studiach, studiami, studiem, studio, studiom, studiów, studiu* — “studio”.

2nd neuter declension:

*pluc, pluca, plucach, plucami, plucem, płuco, płucom, płucu* — “lung”.

3rd neuter declension:

*cuda, cudach, cudami, cudem, cudo, cudom, cudów, cudu, cudzie* — “wonder”;

*palcie, palt, palta, paltach, paltami, paltem, palto, paltom, paltu* — “overcoat”.

4th neuter declension:

*dziewcząt, dziewczę, dziewczęcia, dziewczęciem, dziewczęciu, dziewczęta, dziewczętach, dziewczętami, dziewczętom* — “girl”.

5th neuter declension:

*ramienia, ramieniem, ramieniu, ramię, ramion, ramiona, ramionach, ramionami, ramionom* — “shoulder”.

6th neuter declension:

*muzea, muzeach, muzeami, muzeom, muzeów, muzeum* — “museum”.

1st feminine declension:

*pani, paniach, paniami, panią, panie, paniom, pań* — “lady”;

*świni, świnia, świniach, świniami, świnią, świnie, świnię, świnio, świniom, świń* — “pig”.

2nd feminine declension:

*prac, praca, pracach, pracami, pracą, prace, pracę, praco, pracom, pracy* — “job”;

*sadza, sadzach, sadzami, sadzą, sadze, sadzę, sadzo, sadzom, sadzy* — “soot”.

3rd feminine declension:

*much, mucha, muchach, muchami, muchą, muchę, mucho, muchom, muchy, musze* — “bowtie”;

*plotce, plotek, plotka, plotkach, plotkami, plotką, plotkę, plotki, plotko, plotkom* — “rumour”.

4th feminine declension:

*form, forma, formach, formami, formą, formę, formie, formo, formom, formy* — “shape”.

5th feminine declension:

*brew, brwi, brwiach, brwiami, brwią, brwiom* — “eyebrow”;

*kolei, kolej, kolejach, kolejami, koleją, koleje, kolejom* — “rail”;

*kości, kościach, kością, kościom, kość, kośćmi* — “bone”.

6th feminine declension:

*klacz, klaczach, klaczami, klaczą, klacze, klaczom, klaczy* — “mare”;

*mysz, myszach, myszami, myszą, myszom, myszy* — “mouse”.

As we send these nouns into our clustering algorithm, we receive the following results:

{*brew, brwi, brwiach, brwiami, brwią, brwiom*}, {*chirurgi, chirurg, chirurga, chirurgach, chirurgami, chirurgiem, chirurgom, chirurgowi, chirurgów, chirurgu*}, {*chleb, chleba, chlebach, chlebami, chlebem, chlebie, chlebom, chlebowi, chlebów, chleby*}, {*cuda, cudach, cudami, cudem, cudo, cudom, cudów, cudu, cudzie*}, {*doktor, doktora, doktorach, doktorami, doktorem, doktorom, doktorowi, doktorowie, doktorów, doktorze, doktorzy*}, {*drani, drania, draniach, draniami, dranie, draniem, draniom, draniowi, draniów, draniu, drań*}, {*drozd, drozda, drozdach, drozdami, drozdem, drozdom, drozdowi, drozdów, drozdy, drożdże*}, {*dziewcząt, dziewczę, dziewczęcia, dziewczęciem, dziewczęciu, dziewczęta, dziewczętach, dziewczętami, dziewczętom*}, {*form, forma, formach, formami, formą, formę, formie, formo, formom, formy*}, {*goryl, goryla, gorylach, gorylami, goryle, gorylem, goryli, gorylom, goryłowi, gorylu*}, {*klacz, klaczach, klaczami, klaczą, klacze, klaczom, klaczy*}, {*kolei, kolej, kolejach, kolejami, koleją, koleje, kolejom*}, {*kości, kościach, kością, kościom, kość, kośćmi*}, {*kożuch, kożucha, kożuchach, kożuchami, kożuchem, kożuchom, kożuchowi, kożuchów, kożuchu, kożuchy*}, {*liści, liścia, liściach, liście, liściem, liściom, liściowi, liściu, liść, liśćmi*}, {*Marsjan, Marsjanach, Marsjanami, Marsjanie, Marsjanin, Marsjanina, Marsjaninem, Marsjaninie, Marsjaninowi, Marsjanom, Marsjany*}, {*much, mucha, muchach, muchami, muchą, muchę, mucho, muchom, muchy, musze*}, {*muzea, muzeach, muzeami, muzeom, muzeów, muzeum*}, {*mysz, myszach, myszami, myszą, myszom, myszy*}, {*owoc, owocach, owocami, owoce, owocem, owocom,*

owocowi, owoców, owocu}, {palcie, palt, palta, paltach, paltami, paltem, palto, paltom, paltu}, {pani, paniach, paniami, panią, panie, paniom, pań}, {plotce, plotek, plotka, plotkach, plotkami, plotką, plotkę, plotki, plotko, plotkom}, {płuc, płuca, płucach, płucami, płucem, płuco, płucom, płucu}, {pola, polach, polami, pole, polem, polom, polu, pól}, {prac, praca, pracach, pracami, pracem, praco, pracom, pracy}, {ramienia, ramieniem, ramieniu, ramię, ramion, ramiona, ramionach, ramionami, ramionom}, {sadza, sadzach, sadzami, sadzą, sadze, sadzę, sadzo, sadzom, sadzy}, {strażacy, strażak, strażaka, strażakach, strażakami, strażakiem, strażakom, strażakowi, strażaków, strażaku}, {stróż, stróża, stróżach, stróżami, stróżem, stróżom, stróżowi, stróżowie, stróżu, stróży}, {studia, studiach, studiami, studiem, studio, studiom, studiów, studiu}, {świni, świnią, świniach, świniami, świnią, świnię, świniom, świń}, {tasiemca, tasiemcach, tasiemcami, tasiemce, tasiemcem, tasiemcom, tasiemcowi, tasiemców, tasiemcu, tasiemiec}.

We pick the following Polish verbs, followed by their English translations (enclosed in quotation marks) and conjugation classes (enclosed in parentheses):

*czyta, czytacie, czytać, czytaj, czytają, czytając, czytająca, czytające, czytający, czytajcie, czytajmy, czytali, czytaliście, czytaliście, czytaliście, czytaliście, czytał, czytała, czytałaby, czytałabym, czytałabyś, czytałam, czytałaś, czytałby, czytałbym, czytałbyś, czytałem, czytałeś, czytało, czytałoby, czytały, czytałyby, czytałybyście, czytałybyśmy, czytałyście, czytałyśmy, czytam, czytamy, czytana, czytane, czytani, czytanie, czytano, czytany, czytasz, przeczyta, przeczytacie, przeczytać, przeczytaj, przeczytają, przeczytajcie, przeczytajmy, przeczytali, przeczytaliście, przeczytaliście, przeczytaliście, przeczytaliście, przeczytał, przeczytała, przeczytałaby, przeczytałabym, przeczytałabyś, przeczytałam, przeczytałaś, przeczytałby, przeczytałbym, przeczytałbyś, przeczytałem, przeczytałeś, przeczytało, przeczytałoby, przeczytały, przeczytałyby, przeczytałybyście, przeczytałybyśmy, przeczytałyście, przeczytałyśmy, przeczytam, przeczytamy, przeczytana, przeczytane, przeczytani, przeczytanie, przeczytano, przeczytany, przeczytasz, przeczytawszy* — “read” (1);

*umiał, umiała, umiałaby, umiałabym, umiałabyś, umiałam, umiałaś, umiałby, umiałbym, umiałbyś, umiałem, umiałeś, umiało, umiałoby, umiały, umiałyby, umiałybyście, umiałybyśmy, umiałyście, umiałyśmy, umie, umiecie, umieć, umiej, umieją, umiejąc, umiejąca, umiejące, umiejący, umiejcie, umiejmy, umieli, umieliby, umielibyście, umielibyśmy, umieliście, umieliśmy, umiem, umiemy, umiesz* — “can” (2);

*taniał, taniała, taniała, taniałaby, taniałabym, taniałabyś, taniałam, taniałaś, taniałby, taniałbym, taniałbyś, taniałem, taniałeś, taniało, taniałoby, taniałobym, taniałobyś, taniałom, taniałoś, taniały, taniałyby, taniałybyście, taniałybyśmy, taniałyście, taniałyśmy, taniano, tanieć, taniej, tanieją, taniejąc, taniejąca, taniejące, taniejący, taniejcie, tanieje, taniejecie, taniejemy, taniejesz, tanieję, taniejmy, tanieli, tanieliby, tanielibyście, tanielibyśmy, tanieliście, tanieliśmy, tanienie* — “cheapen” (3);

*malować, malowali, malowaliby, malowalibyście, malowalibyśmy, malowaliście, malowaliśmy, malował, malowała, malowałaby, malowałabym, malowałabyś, malowałam, malowałaś, malowałby, malowałbym, malowałbyś, malowałem, malowałeś, malowało, malowałoby, malowały, malowałyby, malowałybyście, malowałybyśmy, malowałyście, malowałyśmy, malowana, malowane, malowani, malowanie, malowano, malowany, maluj, malują, malując, malująca, malujące, malujący, malujcie, maluje, malujecie, malujemy, malujesz, maluję, malujemy, pomalować, pomalowali, pomalowaliby, pomalowalibyście, pomalowalibyśmy, pomalowaliście, pomalowaliśmy, pomalował, pomalowała, pomalowałaby, pomalowałabym, pomalowałabyś, pomalowałam, pomalowałaś, pomalowałby, pomalowałbym, pomalowałbyś, pomalowałem, pomalowałeś, pomalowało, pomalowałoby, pomalowały, pomalowałyby, pomalowałybyście, pomalowałybyśmy, pomalowałyście, pomalowałyśmy, pomalowana, pomalowane, pomalowani, pomalowanie, pomalowano, pomalowany, pomalowawszy, pomaluj, pomalują, pomalujcie, pomaluje, pomalujecie, pomalujemy, pomalujesz, pomaluję, pomalujemy* — “portray” (4);

*ciągną, ciągnąc, ciągnąca, ciągnące, ciągnący, ciągnąć, ciągnął, ciągnąłby, ciągnąłbym, ciągnąłbyś, ciągnąłem, ciągnąłeś, ciągnę, ciągnęli, ciągnęliby, ciągnęlibyście, ciągnęlibyśmy, ciągnęliście, ciągnęliśmy, ciągnęła, ciągnęłaby, ciągnęłabym, ciągnęłabyś, ciągnęłam, ciągnęłaś, ciągnęło, ciągnęłoby, ciągnęły, ciągnęłyby, ciągnęłybyście, ciągnęłybyśmy, ciągnęłyście, ciągnęłyśmy, ciągnie, ciągniecie, ciągniemy, ciągnieni, ciągniesz, ciągnięci, ciągnięcie, ciągnięta, ciągnięte, ciągnięto, ciągnięty, ciągnij, ciągnijcie, ciągnijmy, ciągniona, ciągnione, ciągniony* — “pull” (5a);

*płyną, płynąc, płynąca, płynące, płynący, płynąć, płynął, płynąłby, płynąłbym, płynąłbyś, płynąłem, płynąłeś, płynę, płynęli, płynęliby, płynęlibyście, płynęlibyśmy, płynęliście, płynęliśmy, płynęła, płynęłaby, płynęłabym, płynęłabyś, płynęłam, płynęłaś, płynęło, płynęłoby, płynęły, płynęłyby, płynęłybyście, płynęłybyśmy, płynęłyście, płynęłyśmy, płynię, płyniecie, płyniemy, płyniesz, płynięcie, płynięto, płyni, płynicie, płynimy* — “swim” (5b);

*chudli, chudliby, chudlibyście, chudlibyśmy, chudliście, chudliśmy, chudł, chudła, chudlaby, chudlabym, chudłabyś, chudłam, chudłaś, chudlby, chudlbym, chudłbyś, chudłem, chudleś, chudło, chudłoby, chudły, chudłyby, chudłybyście, chudłybyśmy, chudłyście, chudłyśmy, chudną, chudnąc, chudnąca, chudnące, chudnący, chudnąć, chudnąć, chudnie, chudniecie, chudniemy, chudniesz, chudnij, chudnijcie, chudnijmy* — “lose weight” (5c);

*robi, robią, robiąc, robiąca, robiące, robiący, robicie, robić, robieni, robienie, robię, robili, robiliby, robilibyście, robilibyśmy, robiliście, robiliśmy, robił, robiła, robiłaby, robiłabym, robiłabyś, robiłam, robiłaś, robiłby, robiłbym, robiłbyś, robiłem, robileś, robiło, robiłoby, robiłobym, robiłobyś, robiłom, robiłoś, robiły, robiłyby, robiłybyście, robiłybyśmy, robiłyście, robiłyśmy, robimy, robiona, robione, robiono, robiony, robisz, zrobi, zrobią, zrobicie, zrobić, zrobieni, zrobienie, zrobię, zrobili, zrobiliby, zrobilibyście, zrobilibyśmy, zrobiliście, zrobiliśmy, zrobił, zrobiła, zrobiłaby, zrobiłabym, zrobiłabyś, zrobiłam, zrobiłaś, zrobiłby, zrobiłbym, zrobiłbyś, zrobiłem, zrobileś, zrobiło, zrobiłoby, zrobiłobym, zrobiłobyś, zrobiłom, zrobiłoś, zrobiły, zrobiłyby, zrobiłybyście, zrobiłybyśmy, zrobiłyście, zrobiłyśmy, zrobimy, zrobiona, zrobione, zrobiono, zrobiony, zrobisz, zrobiwszy* — “do” (6a);

*uwierz, uwierzą, uwierzcie, uwierzenie, uwierzę, uwierzmy, uwierzono, uwierzy, uwierzycie, uwierzyć, uwierzyli, uwierzyliby, uwierzylibyście, uwierzylibyśmy, uwierzyliście, uwierzyliśmy, uwierzył, uwierzyła, uwierzyłaby, uwierzyłabym, uwierzyłabyś, uwierzyłam, uwierzyłaś, uwierzyłby, uwierzyłbym, uwierzyłbyś, uwierzyłem, uwierzyłeś, uwierzyło, uwierzyłoby, uwierzyłobym, uwierzyłobyś, uwierzyłom, uwierzyłoś, uwierzyły, uwierzyłyby, uwierzyłybyście, uwierzyłybyśmy, uwierzyłyście, uwierzyłyśmy, uwierzmy, uwierzysz, uwierzysz, uwierzysz, wierz, wierzą, wierząc, wierząca, wierzące, wierzący, wiercie, wierzenie, wierzę, wierzymy, wierzone, wierzy, wierzycie, wierzyć, wierzyli, wierzyliby, wierzylibyście, wierzylibyśmy, wierzyliście, wierzyliśmy, wierzył, wierzyła, wierzyłaby, wierzyłabym, wierzyłabyś, wierzyłam, wierzyłaś, wierzyłby, wierzyłbym, wierzyłbyś, wierzyłem, wierzyłeś, wierzyło, wierzyłoby, wierzyłobym, wierzyłobyś, wierzyłom, wierzyłoś, wierzyły, wierzyłyby, wierzyłybyście, wierzyłybyśmy, wierzyłyście, wierzyłyśmy, wierzymy, wierzysz* — “believe” (6b);

*widzą, widząc, widząca, widzące, widzący, widzenie, widzę, widzi, widział, widziała, widziałaby, widziałabym, widziałabyś, widziałam, widziałas, widziałby, widziałbym, widziałbyś, widziałem, widziałeś, widziało, widziałoby, widziałobym, widziałobyś, widziałom, widziałoś, widziały, widziałyby, widziałybyście, widziałybyśmy, widziałyście, widziałyśmy, widziana, widziane, widziani, widziano, widziany, widzicie, widzieć, widzieli, widzieliby, widzielibyście, widzielibyśmy, widzieliście, widzieliśmy, widzimy, widzisz, widz, widzicie, widzimy, zobacz, zobaczą, zobaczcie, zobaczenie, zobaczę, zobaczmy, zobaczono, zobaczy, zobaczycie, zobaczyć, zobaczyli, zobaczyliby, zobaczylibyście, zobaczylibyśmy, zobaczyliście, zobaczyliśmy, zobaczył, zobaczyła, zobaczyłaby, zobaczyłabym, zobaczyłabyś, zobaczyłam, zobaczyłaś, zobaczyłby, zobaczyłbym, zobaczyłbyś, zobaczyłem, zobaczyłeś, zobaczyło, zobaczyłoby, zobaczyły, zobaczyłyby, zobaczyłybyście, zobaczyłybyśmy, zobaczyłyście, zobaczyłyśmy, zobaczymy, zobaczysz, zobaczysz* — “see” (7a);

*leż, leżał, leżała, leżałaby, leżałabym, leżałabyś, leżałam, leżałaś, leżałby, leżałbym, leżałbyś, leżałem, leżałeś, leżało, leżałoby, leżałobym, leżałobyś, leżałom, leżałoś, leżały, leżałyby, leżałybyście, leżałybyśmy, leżałyście, leżałyśmy, leżano, leżą, leżąc, leżąca, leżące, leżący, leżcie, leżeć, leżeli, leżeliby, leżelibyście, leżelibyśmy, leżeliście, leżeliśmy, leżenie, leżę, leżmy, leży, leżycie, leżymy, leżysz* — “lie” (7b);

*odczyta, odczytacie, odczytać, odczytaj, odczytają, odczytajcie, odczytajmy, odczytali, odczytaliby, odczytalibyście, odczytalibyśmy, odczytaliście, odczytaliśmy, odczytał, odczytała, odczytałaby, odczytałabym, odczytałabyś, odczytałam, odczytałaś, odczytałby, odczytałbym, odczytałbyś, odczytałem, odczytałeś, odczytało, odczytałoby, odczytałobym, odczytałobyś, odczytałom, odczytałoś, odczytały, odczytałyby, odczytałybyście, odczytałybyśmy, odczytałyście, odczytałyśmy, odczytam, odczytamy, odczytana, odczytane, odczytani, odczytanie, odczytano, odczytany, odczytasz, odczytawszy, odczytuj, odczytują, odczytując, odczytująca, odczytujące, odczytujący, odczytujcie, odczytuje, odczytujecie, odczytujemy, odczytujesz, odczytuję, odczytujmy, odczytywać, odczytywali, odczytywaliby, odczytywalibyście, odczytywalibyśmy, odczytywaliście, odczytywaliśmy, odczytywał, odczytywała, odczytywałaby, odczytywałabym, odczytywałabyś, odczytywałam, odczytywałaś, odczytywałby, odczytywałbym, odczytywałbyś, odczytywałem, odczytywałeś, odczytywało, odczytywałoby, odczytywałobym, odczytywałobyś, odczytywałam, odczytywałoś, odczytywały, odczytywałyby, odczytywałybyście, odczytywałybyśmy, odczytywałyście, odczytywałyśmy, odczytywana, odczytywane, odczytywani, odczytywanie, odczytywano, odczytywany* — “decipher” (8a);

*zyska, zyskacie, zyskać, zyskaj, zyskają, zyskajcie, zyskajmy, zyskali, zyskaliby, zyskalibyście, zyskalibyśmy, zyskaliście, zyskaliśmy, zyskał, zyskała, zyskałaby, zyskałabym, zyskałabyś, zyskałam, zyskałaś, zyskałby, zyskałbym, zyskałbyś, zyskałem, zyskałeś, zyskało, zyskałoby, zyskałobym, zyskałobyś, zyskałom, zyskałoś, zyskały, zyskałyby, zyskałybyście, zyskałybyśmy, zyskałyście, zyskałyśmy, zyskam, zyskamy, zyskana, zyskane, zyskani, zyskanie,*



*czytałam, czytałaś, czytałby, czytałbym, czytałbyś, czytałem, czytałeś, czytało, czytałoby, czytały, czytałyby, czytałybyście, czytałybyśmy, czytałyście, czytałyśmy, czytam, czytamy, czytana, czytane, czytani, czytanie, czytano, czytany, czytasz, przeczyta, przeczytacie, przeczytać, przeczytaj, przeczytają, przeczytajcie, przeczytajmy, przeczytali, przeczytaliby, przeczytalibyście, przeczytalibyśmy, przeczytaliście, przeczytaliśmy, przeczytał, przeczytała, przeczytałaby, przeczytałabym, przeczytałabyś, przeczytałam, przeczytałaś, przeczytałby, przeczytałbym, przeczytałbyś, przeczytałem, przeczytałeś, przeczytało, przeczytałoby, przeczytały, przeczytałyby, przeczytałybyście, przeczytałybyśmy, przeczytałyście, przeczytałyśmy, przeczytam, przeczytamy, przeczytana, przeczytane, przeczytani, przeczytanie, przeczytano, przeczytany, przeczytasz, przeczytawszy*},

*{łać, lali, laliby, lalibyście, lalibyśmy, laliście, laliśmy, lał, lała, lałaby, lałabym, lałabyś, lałam, lałaś, lałby, lałbym, lałbyś, lałem, laleś, lało, lałoby, lały, lałyby, lałybyście, lałybyśmy, lałyście, lałyśmy, lana, lane, lani, lanie, lano, lany, lej, leją, lejąc, lejąca, lejące, lejący, lejcie, leje, lejecie, lejemy, lejesz, leję, lejmy}*},

*{leż, leżał, leżała, leżałaby, leżałabym, leżałabyś, leżałam, leżałaś, leżałby, leżałbym, leżałbyś, leżałem, leżałeś, leżało, leżałoby, leżałobym, leżałobyś, leżałom, leżałoś, leżały, leżałyby, leżałybyście, leżałybyśmy, leżałyście, leżałyśmy, leżano, leżą, leżąc, leżąca, leżące, leżący, leżcie, leżeć, leżeli, leżeliby, leżelibyście, leżelibyśmy, leżełiście, leżełiśmy, leżenie, leżę, leżmy, leży, leżycie, leżymy, leżysz}*},

*{malować, malowali, malowaliby, malowalibyście, malowalibyśmy, malowaliście, malowaliśmy, malował, malowała, malowałaby, malowałabym, malowałabyś, malowałam, malowałaś, malowałby, malowałbym, malowałbyś, malowałem, malowałeś, malowało, malowałoby, malowały, malowałyby, malowałybyście, malowałybyśmy, malowałyście, malowałyśmy, malowana, malowane, malowani, malowanie, malowano, malowany, maluj, malują, malując, malująca, malujące, malujący, malujcie, maluje, malujecie, malujemy, malujesz, maluję, malujemy}*},

*{mazać, mazali, mazaliby, mazalibyście, mazalibyśmy, mazaliście, mazaliśmy, mazał, mazała, mazałaby, mazałabym, mazałabyś, mazałam, mazałaś, mazałby, mazałbym, mazałbyś, mazałem, mazałeś, mazało, mazałoby, mazały, mazałyby, mazałybyście, mazałybyśmy, mazałyście, mazałyśmy, mazana, mazane, mazani, mazanie, mazano, mazany, maż, mażąc, mażąc, mażąca, mażące, mażący, mażcie, maże, mażecie, mażemy, mażesz, mażę, mażmy}*},

*{odczyta, odczytacie, odczytać, odczytaj, odczytają, odczytajcie, odczytajmy, odczytali, odczytaliby, odczytalibyście, odczytalibyśmy, odczytaliście, odczytaliśmy, odczytał, odczytała, odczytałaby, odczytałabym, odczytałabyś, odczytałam, odczytałaś, odczytałby, odczytałbym, odczytałbyś, odczytałem, odczytałeś, odczytało, odczytałoby, odczytałobym, odczytałobyś, odczytałom, odczytałoś, odczytały, odczytałyby, odczytałybyście, odczytałybyśmy, odczytałyście, odczytałyśmy, odczytam, odczytamy, odczytana, odczytane, odczytani, odczytanie, odczytano, odczytany, odczytasz, odczytawszy, odczytuj, odczytują, odczytując, odczytująca, odczytujące, odczytujący, odczytujcie, odczytuje, odczytujecie, odczytujemy, odczytujesz, odczytuję, odczytujmy, odczytywać, odczytywali, odczytywaliby, odczytywalibyście, odczytywalibyśmy, odczytywaliście, odczytywaliśmy, odczytywał, odczytywała, odczytywałaby, odczytywałabym, odczytywałabyś, odczytywałam, odczytywałaś, odczytywałby, odczytywałbym, odczytywałbyś, odczytywałem, odczytywałeś, odczytywało, odczytywałoby, odczytywałobym, odczytywałobyś, odczytywałom, odczytywałoś, odczytywały, odczytywałyby, odczytywałybyście, odczytywałybyśmy, odczytywałyście, odczytywałyśmy, odczytywana, odczytywane, odczytywani, odczytywanie, odczytywano, odczytywany}*},

*{pici, picie, pić, pij, piją, pijąc, pijąca, pijące, pijący, pijcie, pije, pijecie, pijemy, pijesz, pije, pijmy, pili, piliby, pilibyście, pilibyśmy, piliście, piliśmy, pił, piła, piłaby, piłabym, piłabyś, piłam, piłaś, piłby, piłbym, piłbyś, piłem, piłeś, pilo, piloby, pilobym, pilobyś, pilom, piloś, piły, piłyby, piłybyście, piłybyśmy, piłyście, piłyśmy, pita, pite, pito, pity}*},

*{płyną, płynąc, płynąca, płynące, płynący, płynąc, płynął, płynąłby, płynąłbym, płynąłbyś, płynąłem, płynąłeś, płynę, płynęli, płynęliby, płynęlibyście, płynęlibyśmy, płynęliście, płynęliśmy, płynęła, płynęłaby, płynęłabym, płynęłabyś, płynęłam, płynęłaś, płynęło, płynęłoby, płynęły, płynęłyby, płynęłybyście, płynęłybyśmy, płynęłyście, płynęłyśmy, płynie, płyniecie, płyniemy, płyniesz, płynięcie, płynięto, płyn, płynicie, płynimy}*},

*{pomalować, pomalowali, pomalowaliby, pomalowalibyście, pomalowalibyśmy, pomalowaliście, pomalowaliśmy, pomalował, pomalowała, pomalowałaby, pomalowałabym, pomalowałabyś, pomalowałam, pomalowałaś, pomalowałby, pomalowałbym, pomalowałbyś, pomalowałem, pomalowałeś, pomalowało, pomalowałoby, pomalowałobym, pomalowałobyś, pomalowałom, pomalowałoś, pomalowały, pomalowałyby, pomalowałybyście, pomalowałybyśmy, pomalowałyście, pomalowałyśmy, pomalowana, pomalowane, pomalowani, pomalowanie, pomalowano, pomalowany, pomalowawszy, pomaluj, pomalują, pomalujcie, pomaluje, pomalujecie, pomalujemy, pomalujesz, pomaluję, pomalujemy}*},







## 7.2 Modified Porter stemming algorithm for Russian

Our analysis mainly centers on Russian documents in the modern (post-1918) orthography.<sup>90</sup> We also assume that the Russian documents under investigation do not carry stress marks (which only appear in pedagogical contexts) on individual words. We remove the diacritical mark from *ě* in the effective spelling.

In modern Russian, the following present tense conjugations for the Russian verb “to be”

*еси, есмы, есмь, есте, есть, суть*

are no longer used as their English counterparts, but they are found in works of 19th-century Russian authors (like Dostoevsky). The word *есть* is still used modern constructions of possessions (such as *У меня есть ...* “I have ...”). We are going to include all the inflected forms of the Russian verb “to be” in our list of stop words.

**Definition 7.14** (Russian stop words). If a word belongs to the following list<sup>91</sup>:

*а, б, без, более, большие, будем, будет, будете, будешь, будто, буду, будут, будучи, будь, будьте, бы, быв, бывав, бывавши, бывавший, бываем, бывает, бываете, бываешь, бывай, бывайте, бывал, бывала, бывали, бывало, бывать, бываю, бывают, бывающий, бывая, бывшая, бывшего, бывшее, бывшей, бывшем, бывшему, бывшей, бывши, бывшие, бывший, бывшим, бывших, бывшую, был, была, были, было, быть, в, вам, вами, вас, ваш, ваша, ваше, вашего, вашей, вашим, вашему, вашей, ваши, вашим, вашими, ваших, вашу, вдоль, вдруг, ведь, весь, весьма, взад, вместе, вместо, вне, внутри, во, вовне, вовсе, возле, вокруг, вон, вопреки, вот, впереди, впрочем, все, всегда, всего, всей, всем, всеми, всему, всех, всею, всё, вскоре, вслед, всю, вся, всяк, всяка, всякая, всяки, всякие, всякий, всяким, всякими, всяких, всяко, всякого, всякое, всякой, всяком, всякому, всякою, всякую, вы, где, да, давай, давайте, даже, дай, дайте, делав, делавшая, делавшего, делавшее, делавшей, делавшем, делавшему, делавшей, делавшие, делавший, делавшим, делавшими, делавших, делавшую, делаем, делаем, делаемая, делаемо, делаемого, делаемое, делаемой, делаемом, делаемому, делаемую, делаемую, делаемы, делаемые, делаемый, делаемым, делаемыми, делаемых, делаем, делаете, делаешь, делай, делайте, делал, делала, делали, делало, делан, делана, деланная, деланного, деланное, деланной, деланном, деланному, деланною, деланную, деланные, деланный, деланным, деланными, деланных, делано, деланы, делать, делаю, делают, делающая, делающего, делающее, делающей, делающем, делающему, делающей, делающие, делающий, делающим, делающими, делающих, делающую, делая, для, до, должен, должна, должно, должны, другая, другие, другим, другими, других, другого, другое, другой, другом, другому, другую, е, его, едва, ее, её, ей, еле, ему, еси, если, есмы, есмь, есте, есть, еще, ещё, ею, ж, же, за, затем, зато, зачем, здесь, и, ибо, из, изо, или, им, именно, ими, иначе, иная, иногда, иного, иное, иной, ином, иному, иною, иную, иные, иным, иными, иных, их, к, ка, каждая, каждого, каждое, каждой, каждому, каждой, каждую, каждые, каждый, каждым, каждым, как, какая, какие, каким, какими, каких, каков, какова, каковая, каково, какового, каковое, каковой, каковом, каковому, каковою, каковую, каковы, каковые, каковым, каковыми, каковых, какого, какое, какой, каком, какому, какою, какую, кем, ко, когда, кого, кое, коего, коей, кем, коему, коею, кои, коим, коими, коих, кой, ком, кому, конечно, которая, которого, которое, которой, которм, которму, котормую, которые, который, которым, которыми, которых, кою, коя, кроме, кто, куда, ли, либо, лишь, любая, любого, любое, любой, любом, любому, любой, любую, любые, любым, любыми, любых, м, между, менее, меня, мне, мног, многа, многая, многи, многие, многий, многим, многими, многих, много, многого, многое, многой, многим, многому, многию, многию, мной, мною, мог, могли, можете, могла, могли, могло, могу, могут, могущая, могущего, могущее, могущей, могущем, могущему, могущей, могущие, могущий, могущим, могущими, могущих, могущую, могшая, могшего, могшее, могшей, могшем, могшему, могшей, могшие, могший, могшим, могшими, могших, могшую, мое, моего, моей, моем, моему, моею, моё, можем, может, можете, можешь, можно, мои, моим, моими, моих, мой, мою, моя, мы, на, навстречу, над, надо, назад, наиболее, наконец, нам, нами, напролет, напролёт, напротив, нас, насколько, настолько, наш, наша, наше, нашего, нашей, нашем, нашему, нашей, наши, нашим, нашими, наших, нашу, не, негде, него, нее, неё, ней, некем, некогда, некого, некому, некоторая, некоторого, некоторое, некоторой, некотором, некоторому, некоторую, некоторую, некоторые, некоторый, некоторым, некоторыми, некоторых, некуда, нельзя, нем, немног, немнога, немногая, немноги, немногие, немногий, немногим, немногими, немногих, немного, немногого, немногое, немногой, немногом, немногому, немногую, нему, нередко, несколькими, несколькими, нескольких, несмотря, нет, неужели, нечего, нечем, нечему, нею, нём,*

<sup>90</sup>When 19th-century Russian literature is printed and read today, the spellings therein are thoroughly modernized.

<sup>91</sup>Our list of Russian stop words is based on <http://snowball.tartarus.org/algorithms/russian/stop.txt>, with extensive modifications to roughly match their counterparts in English. In particular, we have included all the inflected forms of *быть* “to be”, *каждый* “every”, *какой* “what kind”, *кто* “who”, *чей* “whose”, *что* “what”, and all the possessive pronouns declined in six cases and three genders. Some archaic, poetic or dialectal forms are also included.



### 7.2.1 Effective spelling and essential root

It is assumed that all Russian words are converted to lowercase<sup>92</sup> before going through any of the procedures below.

**Definition 7.16** (Russian Effective Vowels and Verb Prefixes). Hereafter in §7.2, the symbol  $\mathbf{V}^*$  stands for any member from the list  $\{a, e, u, o, y, \text{ы}, \text{ь}, \text{ю}, \text{я}\}$ , the so-called Russian effective vowels.<sup>93</sup> In line with the multiplicity notations introduced in Definition 3.3, the symbol  $\mathbf{V}_m^*$  stands for a text string formed by consecutive appearance of one or more (not necessarily identical or distinct) members from the set of Russian vowel extensions.

Dual to the notations above, the symbol  $\mathbf{C}^*$  stands for any character that does not belong to the list  $\{a, e, u, o, y, \text{ы}, \text{ь}, \text{ю}, \text{я}\}$ , and  $\mathbf{C}_{m_0}^*$  stands for a text string formed by consecutive appearance of zero or more (not necessarily identical or distinct) characters that do not belong to the same list.

The symbol  $\mathbf{P} = (\emptyset|\text{е}|\text{е}|\text{з}|\text{во}|\text{во}|\text{з}|\text{е}|\text{с}|\text{в}|\text{ы}|\text{д}|\text{о}|\text{з}|\text{а}|\text{и}|\text{з}|\text{и}|\text{с}|\text{н}|\text{а}|\text{о}|\text{о}|\text{б}|\text{о}|\text{б}|\text{о}|\text{т}|\text{о}|\text{т}|\text{о}|\text{п}|\text{е}|\text{р}|\text{е}|\text{п}|\text{о}|\text{п}|\text{о}|\text{д}|\text{п}|\text{о}|\text{д}|\text{о}|\text{п}|\text{р}|\text{и}|\text{п}|\text{р}|\text{а}|\text{з}|\text{п}|\text{р}|\text{а}|\text{з}|\text{о}|\text{п}|\text{р}|\text{а}|\text{с}|\text{с}|\text{о}|\text{л}|\text{у})$  represents the possible prefix of a Russian verb.

We further define  $\mathbf{P}^* = (\text{вз}|\text{в}|\text{оз}|\text{в}|\text{е}|\text{с}|\text{ь}|\text{в}|\text{ь}|\text{и}|\text{з}|\text{ь}|\text{и}|\text{с}|\text{ь}|\text{о}|\text{б}|\text{ь}|\text{о}|\text{т}|\text{ь}|\text{п}|\text{о}|\text{д}|\text{ь}|\text{п}|\text{р}|\text{а}|\text{з}|\text{ь}|\text{п}|\text{р}|\text{а}|\text{с}|\text{ь}|\text{с}|\text{ь}|\mathbf{P})$  to account for a possible insertion of the Russian hard sign ь after a prefix ending in a consonant.  $\square$

**Algorithm 7.17** (Russian effective spelling). For a Russian word  $\hat{\sigma}$ , its effective spelling  $\text{EffSpell}(\hat{\sigma})$  is constructed in sequential steps:

(1) If  $\hat{\sigma}$  contains  $(a|e|\text{ё}|\text{u}|\text{o}|\text{y}|\text{ы}|\text{ь}|\text{э}|\text{ю}|\text{я})$ , then leave it as is; otherwise, replace it by  $\xi\hat{\sigma}\xi$ .

(2) Replace<sup>94</sup>

|                                                                                                                             |                                                                                              |                                                                                       |
|-----------------------------------------------------------------------------------------------------------------------------|----------------------------------------------------------------------------------------------|---------------------------------------------------------------------------------------|
| $(\emptyset \text{no})\text{сид}\sim$<br>сыт                                                                                | $(\emptyset \text{y})\text{с}(\text{ев} \text{еви} \text{ел} \text{яд})\sim$<br>сыт          | $\mathbf{X}^\epsilon(\emptyset \text{no} \text{y})\text{чт}\sim$<br>Хчест             |
| $\text{зр}^{\mathbf{X}^\epsilon}(\text{a} \text{e} \text{u} \text{o})\hat{\chi}\sim$<br>$\text{γr}^{\mathbf{X}\hat{\chi}'}$ | жел $\sim$ завтрак $\sim$ зву(κ ч) $\sim$ изум $\sim$ исп $\mathbf{X}^\epsilon$ (o ы) $\sim$ | каза $\sim$ камин $\sim$ кокет $\sim$<br>кажуший хеарθ фокет                          |
| колен $\sim$ корач                                                                                                          | коро(тκ тоκ ч)                                                                               | крат(κ оκ ч) кри $\sim$ кро(т тκ тоκ ц)                                               |
| колѐн                                                                                                                       | σηорт                                                                                        | σηорт кри кри мылδ                                                                    |
| кров(∅ e)л $\sim$<br>ρωφ                                                                                                    | кровать $\sim$ ββεδδ                                                                         | крыл $\sim$ крыл л(e ē)ε(∅ κ ч) $\hat{\chi}$ од(∅ и)н $\sim$<br>I                     |
| остан(a o)в $\sim$<br>остаѐв                                                                                                | отча $\sim$ рав(∅ e)н                                                                        | разговар $\sim$ разговор разум $\sim$ разум са(ди дя жу) $\sim$ солнц $\sim$<br>солце |
| ств(ова y)X                                                                                                                 | стен $\sim$ сторон $\sim$ т(e ē ь)м $\sim$ тарел $\sim$                                      | уш(a e εκ и κ н)X $\sim$ хо(т ч)<br>сть ωαλλ σайдн темδκ тарел уωρ χот                |
| холл $\sim$ холл                                                                                                            | холм $\sim$ холм чис(∅ e)л денни сент сесть стар(a ∅ я)                                      | ух(a e o a м y) старый уωρ                                                            |
| χολλ                                                                                                                        | χολμ ξиσλ δεѐνι σанкт сыт                                                                    | старый                                                                                |

where  $\hat{\chi}'$  results from doing  $\text{в} \rightarrow \beta$ ,  $\text{м} \rightarrow \mu$ ,  $\text{н} \rightarrow \tilde{\nu}$ ,  $\text{ц} \rightarrow \tau\sigma$ ,  $\text{ч} \rightarrow \xi$  on  $\hat{\chi}$ .

(3) Replace

|                                                 |                                                                                                                  |                                                                                |                                                |                                                    |
|-------------------------------------------------|------------------------------------------------------------------------------------------------------------------|--------------------------------------------------------------------------------|------------------------------------------------|----------------------------------------------------|
| $(\emptyset \text{no})\text{стара}\sim$<br>τρηα | $(\text{ε} \text{ж} \text{ε} \text{к} \text{а} \text{ж} \text{д} \text{o})\text{днeвн}^{\mathbf{X}}\sim$<br>день | $\text{γ} \text{р} \text{а} \text{ѐ} \text{и} \text{ц} \text{ч}\sim$<br>границ | $\text{б}(\text{a} \text{o})\text{лт}$<br>болт | $\text{вн} \text{и} \text{м} \text{а}\sim$<br>тτѐα |
| военн $\sim$ воен                               | вол дамV $\sim$ женат $\sim$ завтра(∅ шн) $\sim$ кров $\sim$ март $\sim$ миллион                                 | март $\sim$ март                                                               | миллион                                        | навлин                                             |
| войн                                            | βвол δдамV $\sim$ мар                                                                                            | тморω                                                                          | кροβ                                           | μратσ мξмон пикκ                                   |
| нал(e ь)ц                                       | план $\sim$ погод                                                                                                | преданн $\sim$ предел $\sim$ пред $\sim$ нт(a и)X $\sim$                       | сад $\sim$ свад $\sim$ скал                    | φиѐγу планѐ ωεθ прат лиц пр бирδ γарδ мар рокη     |
| соба(κ ч)                                       | специал                                                                                                          | странн                                                                         | стрем                                          | сударын сумм $\sim$ тон(∅ o)(κ ч ьи) $\sim$<br>θиѐ |
| доу                                             | спеξл                                                                                                            | φремδ                                                                          | риζ                                            | μαδαμ сумμ                                         |
| убе(∅ ж)δ                                       | угод $\sim$ улиц                                                                                                 | хва(т ч) $\sim$                                                                | част $\mathbf{X}^\epsilon$ (e и н ь я) $\sim$  | южX $\sim$ леди па увы                             |
| βиѐκ                                            | γѐод                                                                                                             | триτ                                                                           | χβат                                           | частX юг ледδ паασ αλασ                            |

<sup>92</sup>As of v11.0, *Mathematica* does not produce desired case conversions of Russian letters upon invoking the `ToLowerCase` or `ToUpperCase` operation. Therefore, case conversions for all the Russian letters need to be hand-coded if one implements our algorithm in *Mathematica*.

<sup>93</sup>We note that although  $\text{э}$  is indeed a vowel letter, it never appears in the ending of a Russian word. The soft sign  $\text{ь}$  was historically a short vowel, and it still occurs often in modern Russian word endings.

<sup>94</sup>Words like *кровать* “bed” and *кровли* “roofs” appear to carry commonly seen verb suffixes *-ать* and *-ли*, but are actually not related to *кровь* “blood”. We have created exceptional effective spellings to separate these words (and their inflections) into three classes. However, we note that our algorithm does not distinguish *кров* “shelter” (and its inflections) from any of the inflected forms of *кровь*. Furthermore, *кровь* “blood”, *кровоточить* “to bleed” and *кровотечение* “bleeding” are split into three different clusters by our current method.

## (4) Replace

|                                                                    |                                      |                                                         |                       |                                                   |                              |                                        |                                                                    |                 |                                |               |             |
|--------------------------------------------------------------------|--------------------------------------|---------------------------------------------------------|-----------------------|---------------------------------------------------|------------------------------|----------------------------------------|--------------------------------------------------------------------|-----------------|--------------------------------|---------------|-------------|
| (∅ вз)волн~<br>ωαβ                                                 | (∅ вы)т(е ё)(к ч)(∅ ш)~<br>тек       | (∅ по)жен <sup>Xε</sup> (у ю я)~<br>мар                 | (∅ об с)новχ~<br>ῥовχ | (∅ по)счаст~<br>счаст                             |                              |                                        |                                                                    |                 |                                |               |             |
| (∅ на по про)чит~<br>чит                                           | (∅ по)чувств<br>фул                  | (в воз по)люб~<br>люб                                   | (по про)яв~<br>яв     | <b>P*giveRussian</b> (∅ сь ся)~<br><b>P*ргывр</b> | <b>P*ник</b><br><b>P*виу</b> |                                        |                                                                    |                 |                                |               |             |
| бенн бо(к ч) бeῖῥ<br>беῖῥ                                          | брак(о у)χ<br>сиод                   | вез велик~<br>рефсχ                                     | вид вляя~<br>γвар     | втор~<br>болеш                                    | выжима~<br>βид               | выжм~<br>иῥфля                         | гад горьк~<br>2о                                                   | гост~<br>выжа   | гул<br>γад                     | гулл<br>горьк | гул<br>γост |
| дал(ек ёк ён)<br>фар                                               | дв(а е у(м мя х))<br>2e2             | девуш(∅ е)к~<br>дев                                     | девят~<br>9я          | десят<br>10e                                      | ди(к ч)~<br>дик              | див <sub>χ</sub> ϕ(ш)<br>диβχ          | добр~<br>доβр                                                      | долин~<br>долин | дол~<br>доп                    |               |             |
| дум жизн~<br>дум                                                   | заб замуж<br>ζаб                     | зл~<br>ζл                                               | зна(л н ю)~<br>зна    | июл~<br>γиюл                                      | июн~<br>ηюῥ                  | карет<br>γарет                         | кла(в л ст)(∅ ш)~<br>клад                                          | клон<br>γлоῥ    | красн~<br>руед                 |               |             |
| кон(∅ е)ц~<br>коῥζ                                                 | лид~<br>лид                          | мил~<br>μιλ                                             | мир~<br>μир           | молв~<br>μов                                      | мягк~<br>мягч                | недел~<br>нек                          | ноч~<br>ῥохт                                                       | обед<br>обд     | ок <sup>V*</sup> (∅ м)~<br>очи |               |             |
| отве(т ч)~<br>αῖσω                                                 | отлив~<br>отλιβ                      | п(е в ш л т) о(ем ет еиш ёш ём ёт ёиш ю от юц))<br>песн |                       |                                                   |                              |                                        |                                                                    |                 |                                |               |             |
| парк~<br>парк                                                      | перв~<br>1e                          | пес(∅ е)н~<br>песн                                      | пеш<br>пеξ            | письменн~<br>писат                                | подлин~<br>подлиῥ            | подол~<br>подол                        |                                                                    |                 |                                |               |             |
| поз <sup>Xε</sup> (в о)~<br>зX                                     | пойм~<br>поня                        | покл~<br>покл                                           | поко<br>рум           | полков~<br>полков                                 | поч(е ё)(∅ с)т~<br>ηоῥ       | поч <sup>V*</sup> ~<br>ч <sup>V*</sup> | пр <sup>V*</sup> <sub>м</sub> м<br>пр <sup>V*</sup> <sub>м</sub> μ |                 |                                |               |             |
| пр <sup>V*</sup> <sub>м</sub> т<br>пр <sup>V*</sup> <sub>м</sub> τ | пр <sup>Xε</sup> (у о)лив~<br>прXлиβ | приним~<br>приня                                        | приятел~<br>приятел   | прол(е ё)~<br>ле                                  |                              | прони(к ц)~<br>проῥик                  |                                                                    |                 |                                |               |             |
| разлу(к ч)~<br>спе                                                 | свет~<br>свет                        | сл(у ы)ш<br>лыс                                         | смел~<br>смел         | собы~<br>собоη                                    | сц~<br>сζ                    | счит<br>цчит                           | тан(∅ е)ц~<br>танζ                                                 | титул~<br>титул |                                |               |             |
| треб<br>треβ                                                       | трет~<br>3и                          | трон~<br>трог                                           | уи~<br>Ωи             | цел<br>ξел                                        | человек<br>люд               | шарк<br>šару                           | янв~<br>jяῥ                                                        | боже<br>бог     |                                |               |             |
| брат(∅ а е ом у ьев ья ьям ьями ьях)<br>βбратβ                     |                                      |                                                         |                       |                                                   |                              | лет(∅ а(∅ м ми х))<br>год              |                                                                    |                 |                                |               |             |
| мыл( <sup>V*</sup>  ∅)<br>мыть                                     | окон<br>окно                         | писем<br>письмо                                         | полях<br>поля         | сем(у ~ь)<br>7e                                   | сн(ах ов у ы)<br>сон         |                                        |                                                                    |                 |                                |               |             |

## (5) Replace

|                    |                                |                                  |                                   |                           |              |                   |                |                                         |
|--------------------|--------------------------------|----------------------------------|-----------------------------------|---------------------------|--------------|-------------------|----------------|-----------------------------------------|
| (по с)лож~<br>клад | <b>P*еду</b> ~<br><b>P*еха</b> | <b>P*(буд бы)</b><br><b>P*βε</b> | <b>P*(й д йт)~</b><br><b>P*ид</b> | <b>P*ле(т ч)~</b><br>флет | брак~<br>мар | звол<br>αλω       | знатн~<br>ῥовл | зна(к ч)~<br>μнаῥ                       |
| мер(и)~<br>μмер    | плать~<br>δплать               | пож~<br>ж                        | пре~<br>пре                       | прив~<br>β                | прил~<br>л   | сем(ей ь)~<br>φαμ | чет<br>кел     | <b>P*еде(м т те шь)</b><br><b>P*еха</b> |

## (6) Replace

|                                                        |                                |                            |                   |                                              |                |               |                                          |                           |                   |
|--------------------------------------------------------|--------------------------------|----------------------------|-------------------|----------------------------------------------|----------------|---------------|------------------------------------------|---------------------------|-------------------|
| (дочь доч(∅ а е)к)<br>дочер                            | (∅ наи)(высок выси)~<br>βвысок | (∅ наи)(худш хуж)~<br>плох |                   |                                              |                |               |                                          |                           |                   |
| (∅ наи)младш~<br>ммолад                                | (∅ наи)низш~<br>низк           | (∅ наи по)лучш~<br>хорош   | (∅ с)дел~<br>бдел | (тет тёт)(о у и уше)к~<br>тетя               |                |               |                                          |                           |                   |
| <b>C<sub>т</sub>*ост</b> ~<br><b>C<sub>т</sub>*озт</b> | бал~<br>ббал                   | бл~<br>жжбл                | глян<br>гляд      | де(й я)~<br>бгдея                            | джо~<br>сджо   | дом~<br>домчм | друз~<br>друг                            | дяд(е ь юш юше)к~<br>дядя |                   |
| е(з х)~<br>сье                                         | жб<br>ж                        | забет<br>за                | игр~<br>ыгр       | исъм<br>исзз                                 | крут~<br>круч  | ле~<br>ле     | м <sup>V*</sup> л~<br>мм <sup>V*</sup> л | мин~<br>мчин              | наде~<br>ннаде    |
| наиχ <sub>ми</sub> X<br>χ <sub>ми</sub>                | нест<br>нес                    | обр~<br>ччобр              | па~<br>ппа        | пол <sup>Xε</sup> (а е и о ы ь ю я)~<br>полχ | полн~<br>бполн | пра<br>бпра   | раст<br>рос                              | род~<br>ррод              | ска(ж з)<br>говор |

|                                                              |       |        |       |       |    |                                                                                                      |      |      |        |       |
|--------------------------------------------------------------|-------|--------|-------|-------|----|------------------------------------------------------------------------------------------------------|------|------|--------|-------|
| слав~                                                        | слов~ | собств | спор~ | стол~ | тз | юнош~                                                                                                | даст | де   | дорого | отцах |
| зслав                                                        | цслав | зопств | цспор | цстол | цц | юност                                                                                                | дал  | днде | дорог  | отец  |
| $\text{nan}(\mathbf{V}^* \emptyset)(\emptyset \ddot{u} m x)$ |       |        | пони  |       |    | $(\text{матв мамоч}(\emptyset a e)к\sim \text{мам}(\mathbf{V}^* \emptyset)(\emptyset \ddot{u} m x))$ |      |      |        |       |
| отец                                                         |       |        | ппони |       |    | матер                                                                                                |      |      |        |       |

(7) Replace

|                              |                                                                    |       |                  |       |       |                     |              |       |      |
|------------------------------|--------------------------------------------------------------------|-------|------------------|-------|-------|---------------------|--------------|-------|------|
| $(\emptyset n o c co)жм\sim$ | $\mathbf{C}_{m_0}^*гн\sim$                                         | да~   | $e(e \ddot{u})к$ | зв    | особ~ | певши               | пон~         | риск~ | сл~  |
| жал                          | $\mathbf{C}_{m_0}^*гюн$                                            | чдача | ееч              | зов   | ззоб  | по                  | н            | рисч  | жсл  |
| соб~                         | $\mathbf{X}_1(\emptyset в y n o y)м\mathbf{X}_2^{\infty}(o ы)\sim$ | день  | лоб              | мяжок | рот   | училищ $\mathbf{X}$ | (живи ~жить) | ~ести | ~ец  |
| зоб                          | $\mathbf{X}_1мюж\mathbf{X}_2$                                      | дни   | лба              | мягч  | рта   | скул                | жил          | ел    | ~ьца |

and call the result  $\hat{\sigma}'$ .

(8) Break down  $\hat{\sigma}' = \hat{\sigma}_1\hat{\sigma}_2$  into the concatenation of two strings  $\hat{\sigma}_1 = \hat{\sigma}'^{[\min\{\lambda(\hat{\sigma}'), \ell(\hat{\sigma}')\}]}$  (see the notation in Definition 3.1) and  $\hat{\sigma}_2$ , where  $\lambda(\hat{\sigma}') - 1$  equals either the last position occupied by the string pattern  $(\mathbf{P}^*|\text{без|безо|бес|не|нна|сmp})\hat{x}\sim$  in the non-void  $\hat{\sigma}'$ , or  $-1$  if  $\hat{\sigma}' = \emptyset$ .

(9) On  $\hat{\sigma}_2$ , perform the following substitutions in a sequel:

(4.1) Do  $(ак|виц|лиш|чек|чиш|чик|як|(тел|чк)\mathbf{X}) \rightarrow \emptyset$ ,  $(ар|ач|ник|ниц|ств|яр) \rightarrow \emptyset$ ,  $\mathbf{X}^{\infty}(e|б)б \rightarrow \mathbf{X}$ ,  $(кац|(\emptyset|ц)ир(ов|y)) \rightarrow \emptyset$ ,  $\sim(сб|с|а|ться) \rightarrow \emptyset$ ,  $\simи \rightarrow \text{мен}$ ,  $\simи\mathbf{V}^*(e|u|\ddot{u}|m|x|o|я) \rightarrow и$ .

(4.2) Do  $\sim((a|o|я)м|(a|u|ы|я)х|\mathbf{V}^*eв|(e|o)го|(e|o)му|\ddot{u}|(\ddot{u})_m\text{те|му|ов}|\mathbf{V}^*m(\emptyset|б)|шь) \rightarrow \emptyset$ ,  $(ac|a|uc|oc)m \rightarrow \emptyset$ ,  $\sim(e|ц|к) \rightarrow \emptyset$ ,  $(к|ц)\mathbf{V}^*(\emptyset|x) \rightarrow \mathbf{V}^*$ ,  $\sim(\mathbf{V}^*m|(\ddot{u})_m\text{те}) \rightarrow \emptyset$ .

The result after these two steps of operations is called  $\hat{\sigma}'_2$ .

(10) Concatenate  $\hat{\sigma}_1$  and  $\hat{\sigma}'_2$ .

(11) Do  $(\ddot{e}|\ddot{E}) \rightarrow e$ ,  $ммальч\mathbf{V}^*\mathbf{X}\sim \rightarrow ммальч$ .

**Definition 7.18** (Russian protected range). Let  $\hat{\sigma}$  be a text string derived from a Russian word, its protected range  $\text{ProtRg}(\hat{\sigma}) = \min\{\lambda_1(\hat{\sigma}), \lambda_2(\hat{\sigma})\}$  is determined by two non-negative integers  $\lambda_1(\hat{\sigma})$  and  $\lambda_2(\hat{\sigma})$  specified through the following procedures:

- Look for the string pattern  $(в|ы|н|а|y)_m\mathbf{C}_{m_0}^*\mathbf{V}^*(\ddot{u})_m\sim$  in the string  $\hat{\sigma}$ ;
- If the string pattern above is found, the last position occupied by such a string defines  $\lambda_1(\hat{\sigma})$ ; otherwise, set  $\lambda_1(\hat{\sigma}) = 0$ ;
- Look for the pattern  $(\emptyset|вз|в|н|а|н|о|н|р|о|р|а|з|р|а|с|с|c)\mathbf{V}_{m_0}^*\mathbf{C}^*\mathbf{V}_{m_0}^*\mathbf{C}^*\sim$  in the string  $\hat{\sigma}$ ;
- If the pattern above is found, the last position occupied by such a pattern defines  $\lambda_2(\hat{\sigma})$ ; otherwise, set  $\lambda_2(\hat{\sigma}) = \ell(\hat{\sigma})$ .  $\square$

**Algorithm 7.19** (Russian essential root). Let  $\hat{\sigma}$  be the effective spelling of a Russian word, then its corresponding essential root  $\text{EssRoot}(\hat{\sigma})$  is constructed in the following steps:

(1) Break down  $\hat{\sigma} = \hat{\sigma}_1\hat{\sigma}_2$  into the concatenation of two strings  $\hat{\sigma}_1 = \hat{\sigma}^{[\text{ProtRg}(\hat{\sigma})]}$  (see the notation in Definition 3.1) and  $\hat{\sigma}_2$ , where the length of the first string  $\ell(\hat{\sigma}_1) = \text{ProtRg}(\hat{\sigma})$  is equal to the protected range of  $\hat{\sigma}$ .

(2) Do  $ь \rightarrow e$  on  $\hat{\sigma}_1$ , and call the result  $\hat{\sigma}'_1$ .

(3) On  $\hat{\sigma}_2$ , perform the following substitutions in a sequel:

(3.1) Do  $\sim\mathbf{V}_m^* \rightarrow \emptyset$ ;

(3.2) Do  $\sim\mathbf{V}_{m_0}^*(в|и|\ddot{u}|(\emptyset|и)|м|н|н)_m \rightarrow \mathbf{V}_{m_0}^*$ ;

(3.3) Do  $\sim\mathbf{V}_m^* \rightarrow \emptyset$ .

The result after these three steps of operations is called  $\hat{\sigma}'_2$ .

(4) Concatenate  $\hat{\sigma}'_1$  and  $\hat{\sigma}'_2$ . If  $\ell(\hat{\sigma}'_1\hat{\sigma}'_2) = 3$ , do  $\sim(a|e|u|\ddot{u}|o|y|ы|ь|ю|я) \rightarrow \emptyset$  on  $\hat{\sigma}'_1\hat{\sigma}'_2$ , and call the result  $\hat{\sigma}'$ ; otherwise, define  $\hat{\sigma}' = \hat{\sigma}'_1\hat{\sigma}'_2$ .

(5) Do  $\sim(\ddot{u}|б)\hat{x}(\mathbf{V}^*в)_m \rightarrow e\hat{x}$  on  $\hat{\sigma}'$ .

(6) Replace

|                   |                                               |        |                     |      |                             |
|-------------------|-----------------------------------------------|--------|---------------------|------|-----------------------------|
| $\partial n \sim$ | $((\emptyset n o c co)жа(\emptyset в m) с ж)$ |        | $(реб ребен ребят)$ |      | $X \in (\partial л л n ш)e$ |
| день              | жал                                           |        | дет                 |      | Xu                          |
| краш              | ул                                            | чдачад | ~вел                | ~жив | ~ne (л л m)                 |
| красив            | услыш                                         | чдач   | вед                 | жил  | no                          |

To improve the performance of verb clustering in Russian, we need the following extension to Algorithm 7.19.

**Algorithm 7.20** (Russian verbal essential root). *Let  $\hat{\sigma}$  be the token string associated with a Russian word, then its corresponding verbal essential root  $VbEssRoot(\hat{\sigma})$  is constructed in the following steps:*

- (1) Break down  $\hat{\sigma} = \hat{\sigma}_1 \hat{\sigma}_2$  into the concatenation of two strings  $\hat{\sigma}_1 = \hat{\sigma}^{[ProtRg(\hat{\sigma})]}$  (see the notation in Definition 3.1) and  $\hat{\sigma}_2$ , where the length of the first string  $\ell(\hat{\sigma}_1) = ProtRg(\hat{\sigma})$  is equal to the protected range of  $\hat{\sigma}$ .
- (2) Do  $\sim(\mathbf{V}_{m_0}(\partial|л|л|\mathbf{V}_m m)_{m_0})_m \rightarrow \emptyset$  on  $\hat{\sigma}_2$ , and call the result  $\hat{\sigma}'_2$ .
- (3) Concatenate  $\hat{\sigma}_1$  and  $\hat{\sigma}'_2$ .
- (4) Do  $npu\partial \rightarrow npuu\partial$ .
- (5) Do  $\mathbf{P}^*(e\partial|e\partial ж) \sim \rightarrow \mathbf{P}^*ex$ ,  $(\partial p|вз|воз)(\emptyset|ем|ьм) \rightarrow бер$ ,  $\mathbf{P}^*(u\partial|хож|ш|шедш) \rightarrow \mathbf{P}^*ход$ .

## 7.2.2 Admissible mutation and approximate clustering

In Russian (as well as Polish and many other Slavic languages), fleeting vowels may appear or disappear in inflected forms of the same word. We need to heuristically detect and remove these fleeting vowels to achieve better clustering results. Meanwhile, in Russian (as well as Polish and many other Slavic languages), one encounters vowel alternations in verb conjugations, as in Spanish or the Germanic languages.

**Algorithm 7.21** (Russian vowel blotting). *For a token string  $\hat{\sigma}$ , its blotted form  $BlotFltV(\hat{\sigma})$  is constructed as follows:*

- (1) Do  $\sim \mathbf{C}^*(e|o)^{\hat{\epsilon}}(\kappa|л|л|л|л)(\mathbf{V}_{m_0}^*(\partial|л|л|m)_{m_0})_m |u) \rightarrow \mathbf{C}^* \hat{\chi}$ .
- (2) Do  $\sim \hat{\chi}^{\epsilon}(\partial|m)ep(\mathbf{V}_{m_0}^*(\partial|л|л|m)_{m_0})_m |u) \rightarrow \hat{\chi}p$ .
- (3) Do  $e \rightarrow u$ ,  $o \rightarrow a$ .

In what follows, we will construct a bivariate Boolean-valued function  $HrdTest(\hat{\alpha}, \hat{\beta})$  on a “simple heredity test function” in Algorithm 7.22, and a set of “admissible suffix mismatch” rules in Algorithm 7.23.

**Algorithm 7.22** (Simple heredity test). *Let  $\hat{\alpha}'$  be a string obtained from  $\hat{\alpha}$  by the following steps:*

- (1) Break down  $\hat{\alpha} = \hat{\alpha}_1 \hat{\alpha}_2$  into the concatenation of two strings  $\hat{\alpha}_1 = \hat{\alpha}^{[\min\{3, \ell(\hat{\alpha})\}]}$  (see the notation in Definition 3.1) and  $\hat{\alpha}_2$ , where the length of the first string  $\ell(\hat{\alpha}_1) = \min\{3, \ell(\hat{\alpha})\}$  is equal to 3 or the length of  $\hat{\alpha}$ , whichever is shorter.
- (2) Do  $\sim((\mathbf{V}_{m_0}^*(\partial|л|л|m|u)_{m_0})_m |u)$  on  $\hat{\alpha}_2$ , and call the result  $\hat{\alpha}'_2$ .
- (3) Construct  $\hat{\alpha}' = \hat{\alpha}_1 \hat{\alpha}'_2$ .

Define  $\hat{\beta}'$  similarly. The Boolean-valued function  $SimpHrdTest(\hat{\alpha}, \hat{\beta})$  returns **TRUE** if the lowercase form of  $\hat{\alpha}$  contains at least one instance of  $\{a, e, u, o, y, ы, ь, ю, я, лб, pm, ch\}$  **AND** at least one of the following five conditions holds:<sup>95</sup>

- (i)  $\hat{\alpha} = \hat{\beta}$ ;
- (ii)  $\hat{\beta} = \hat{\alpha}u$ ;
- (iii)  $\hat{\beta} = \hat{\alpha}u$ ;
- (iv)  $\min\{\ell(\hat{\alpha}'), \ell(\hat{\beta}')\} \geq 3$  **AND**  $(\hat{\alpha} = \hat{\beta}'$  **OR**  $\hat{\alpha}' = \hat{\beta}$  **OR**  $\hat{\alpha}' = \hat{\beta}')$ .
- (v)  $\ell(\hat{\beta}) > \ell(\hat{\alpha}) \geq \frac{\ell(\hat{\beta})}{3}$  **AND**  $\hat{\beta} = \hat{\alpha}(a|e|o|я)_m(\partial|л|m)$ .

In what follows, we define  $SuffixNW(\hat{\alpha}, \hat{\beta})$ ,  $RootNW(\hat{\alpha}, \hat{\beta})$ ,  $NW^*(\hat{\alpha}, \hat{\beta})$  and  $SuffixSW(\hat{\alpha}, \hat{\beta})$ ,  $SuffixSW'(\hat{\alpha}, \hat{\beta})$ ,  $SW^*(\hat{\alpha}, \hat{\beta})$  as what is done in the Danish case (Algorithm 5.7), which was also applied to two other Germanic languages treated in §5. Particular to the Russian case, we further define  $SuffixNW'(\hat{\alpha}, \hat{\beta})$  by performing the substitutions  $\sim((\mathbf{V}_{m_0}^*(\partial|л|л|\mathbf{V}_m^* m)_{m_0})_m |u) \rightarrow \emptyset$  to both components of  $SuffixNW(\hat{\alpha}, \hat{\beta})$ . The notation  $SuffixSW'(\hat{\alpha}, \hat{\beta})$  is defined similarly. If  $SuffixNW(\hat{\alpha}, \hat{\beta}) = [\hat{\tau}_1, \hat{\tau}_2]$ , then  $SuffixNW'(\hat{\beta}, \hat{\alpha}) = [\hat{\tau}_2, \hat{\tau}_1]$ .

<sup>95</sup>As a general rule in this document, the truth values of items labeled with Roman numerals are connected to each other with logical **OR**.

**Algorithm 7.23** (Admissible suffix mismatch and vowel alternation). For two strings  $\hat{\alpha}$  and  $\hat{\beta}$ , the Boolean-valued function

$$\text{AdmMut}(\text{RootNW}(\hat{\alpha}, \hat{\beta}), \text{SuffixNW}(\hat{\alpha}, \hat{\beta}), \text{NW}^*(\hat{\alpha}, \hat{\beta}))$$

returns **TRUE** if  $\text{NW}(\hat{\alpha}, \hat{\beta}) = \emptyset[[\emptyset, u][[a, o][[e, u][[u, \emptyset]]]]$  **AND** ( $\text{RootNW}(\hat{\alpha}, \hat{\beta})$  contains at least one instance of  $\{a, e, u, o, y, \mathfrak{y}, \mathfrak{b}, \mathfrak{i}, \mathfrak{o}, \mathfrak{y}\}$ ) **OR**  $\Omega(\text{RootNW}(\hat{\alpha}, \hat{\beta})) = (\kappa|\mu|\eta|\mu|p)$ ) **AND** at least one of the following three conditions holds:

- (i)  $\text{SuffixNW}'(\hat{\alpha}, \hat{\beta}) = [z, \mathfrak{x}][[z, \mathfrak{z}][[\delta, \mathfrak{x}][[\mathfrak{x}, \mathfrak{z}][[\mathfrak{x}, \mathfrak{u}][[\kappa, \mathfrak{u}][[c, \mathfrak{u}][[m, \mathfrak{u}][[x, \mathfrak{u}][[e\kappa, \mathfrak{u}][[o\kappa, \mathfrak{u}][[c\kappa, \mathfrak{u}][[cm, \delta][[cm, \mathfrak{u}]]]]]]]]]]]]];$
- (ii)  $\text{SuffixNW}'(\hat{\beta}, \hat{\alpha}) = [z, \mathfrak{x}][[z, \mathfrak{z}][[\delta, \mathfrak{x}][[\mathfrak{x}, \mathfrak{z}][[\mathfrak{x}, \mathfrak{u}][[\kappa, \mathfrak{u}][[c, \mathfrak{u}][[m, \mathfrak{u}][[x, \mathfrak{u}][[e\kappa, \mathfrak{u}][[o\kappa, \mathfrak{u}][[c\kappa, \mathfrak{u}][[cm, \delta][[cm, \mathfrak{u}]]]]]]]]]]];$
- (iii)  $\text{SuffixNW}(\hat{\alpha}, \hat{\beta}) = [\emptyset|(\mathbf{V}_m(\emptyset|\mathfrak{e}|\eta|\mu|m|\mathfrak{u}))], \emptyset|(\mathbf{V}_m(\emptyset|\mathfrak{e}|\eta|\mu|m|\mathfrak{u}))].$

Similarly, one can evaluate another Boolean-valued function

$$\text{AdmMut}(\text{RootSW}(\hat{\alpha}, \hat{\beta}), \text{SuffixSW}(\hat{\alpha}, \hat{\beta}), \text{SW}^*(\hat{\alpha}, \hat{\beta}))$$

by trading all the occurrences of NW in the statements above with SW.

**Algorithm 7.24** (Heredity test function). The structure of the Russian heredity test function  $\text{HrdTest}(\hat{\alpha}, \hat{\beta})$  is identical to the Polish version (Algorithm 7.11), except that the functions  $\text{SimpHrdTest}$ ,  $\text{RootNW}$ ,  $\text{SuffixNW}$ ,  $\text{NW}$ ,  $\text{RootSW}$ ,  $\text{SuffixSW}$ ,  $\text{SW}$  and the strings  $\hat{\alpha}'$ ,  $\hat{\beta}'$  must follow the Russian rules stated above.

**Algorithm 7.25** (Russian verb aspect test). Let  $\text{NW}(\hat{\alpha}, \hat{\beta})$  be the result of performing Needleman–Wunsch alignment on strings  $\hat{\alpha}$  and  $\hat{\beta}$ . Let  $\mathbf{X}^*$  be an arbitrary non-empty string. The Boolean-valued function  $\text{VbAspTest}(\hat{\alpha}, \hat{\beta})$  returns **TRUE** if at least one of the following four conditions holds:

- (i)  $\text{NW}(\hat{\alpha}, \hat{\beta}) = \mathbf{X}^*$  (in other words,  $\hat{\alpha} = \hat{\beta}$ );
- (ii)  $\text{NW}(\hat{\alpha}, \hat{\beta}) = [\mathbf{P}^*, \mathbf{P}^*]\mathbf{X}^*$  (in other words,  $\hat{\alpha}$  agrees with  $\hat{\beta}$  up to a pair of word initial mismatching strings, both of which are possible prefixes of Russian verbs);
- (iii)  $\text{NW}(\hat{\alpha}, \hat{\beta}) = [\mathbf{P}^*, \mathbf{P}^*]\mathbf{X}^*([\emptyset, u][[a, o][[e, u][[u, \emptyset][[u, e][[o, a]]]]]]\mathbf{X}^*$ , where the two occurrences of  $\mathbf{X}^*$  may or may not represent the same non-empty string;
- (iv)  $\text{NW}(\hat{\alpha}, \hat{\beta}) = [\mathbf{P}^*, \mathbf{P}^*]\mathbf{X}^*[\hat{\tau}_1, \hat{\tau}_2]$  so that either  $[\hat{\tau}_1', \hat{\tau}_2']$  or  $[\hat{\tau}_2', \hat{\tau}_1']$  matches  $[z, \mathfrak{x}][[z, \mathfrak{z}][[\delta, \mathfrak{x}][[\mathfrak{x}, \mathfrak{z}][[\mathfrak{x}, \mathfrak{u}][[\kappa, \mathfrak{u}][[c, \mathfrak{u}][[m, \mathfrak{u}][[x, \mathfrak{u}][[e\kappa, \mathfrak{u}][[o\kappa, \mathfrak{u}][[c\kappa, \mathfrak{u}][[cm, \delta][[cm, \mathfrak{u}]]]]]]]]]]]]$ . Here,  $\hat{\tau}_1'$  results from doing  $\sim((\mathbf{V}_{m_0}^*(\mathfrak{e}|\eta|\mu|\mathbf{V}_{m_0}^*m)_m)|u) \rightarrow \emptyset$  on  $\hat{\tau}_1$ , and  $\hat{\tau}_2'$  is similarly defined.

Note that Smith–Waterman alignment is not used in this test.

The following approximate clustering algorithm for Russian words are very similar to the Polish counterpart (Algorithm 7.13), except that Latin transliteration (Algorithm 7.15) is used before sorting the tokens. For clarity, we state the algorithm in full.

**Algorithm 7.26** (Approximate clustering of Russian words). The approximate clustering of a list of English words  $\{\hat{\alpha}_1, \dots, \hat{\alpha}_N\}$  is completed in three stages:

- (1) We sort the list  $\{(\hat{\alpha}_1, \text{EffSpell}(\hat{\alpha}_1)), \dots, (\hat{\alpha}_N, \text{EffSpell}(\hat{\alpha}_N))\}$  alphabetically according to the Latin transliteration of second component (Algorithm 7.15 applied to the effective spelling) of each entry. If two consecutive neighbors in the alphabetized list  $\{(\hat{\alpha}_{(1)}, \text{EffSpell}(\hat{\alpha}_{(1)})), \dots, (\hat{\alpha}_{(N)}, \text{EffSpell}(\hat{\alpha}_{(N)}))\}$  satisfies  $\text{HrdTest}(\text{EffSpell}(\hat{\alpha}_{(n)}), \text{EffSpell}(\hat{\alpha}_{(n+1)})) = \text{FALSE}$ , where  $n \in \mathbb{Z} \cap [1, N)$ , then add a demarcation line between these two entries. In this way, the alphabetized list is divided into separate groups of words tagged with their effective spellings:  $\{g_1 = \{(\hat{\alpha}_{(1,1)}, \text{EffSpell}(\hat{\alpha}_{(1,1)})), \dots, (\hat{\alpha}_{(1,n_1)}, \text{EffSpell}(\hat{\alpha}_{(1,n_1)}))\}, \dots, g_M = \{(\hat{\alpha}_{(M,1)}, \text{EffSpell}(\hat{\alpha}_{(M,1)})), \dots, (\hat{\alpha}_{(M,n_M)}, \text{EffSpell}(\hat{\alpha}_{(M,n_M)}))\}$ , where each sublist also preserves alphabetic order. In particular, we have  $\hat{\alpha}_{(1,1)} = \hat{\alpha}_{(1)}$  and  $\hat{\alpha}_{(M,n_M)} = \hat{\alpha}_{(N)}$ .
- (2) For each group of words  $g_m = \{(\hat{\alpha}_{(m,1)}, \text{EffSpell}(\hat{\alpha}_{(m,1)})), \dots, (\hat{\alpha}_{(m,n_m)}, \text{EffSpell}(\hat{\alpha}_{(m,n_m)}))\}$  where  $m \in \mathbb{Z} \cap [1, M]$ , we augment it into a tagged entry  $G_m = (g_m, \text{EffSpell}(\hat{\alpha}_{(m,1)}), \text{EssRoot}(\text{EffSpell}(\hat{\alpha}_{(m,1)})), \text{BlotFltV}(\text{EssRoot}(\text{EffSpell}(\hat{\alpha}_{(m,1)}))))$ . The list  $\{G_1, \dots, G_M\}$  is sorted alphabetically, with respect to  $\text{RuLat}(\text{BlotFltV}(\text{EssRoot}(\text{EffSpell}(\hat{\alpha}_{(m,1)}))))$  (with highest priority),  $\text{RuLat}(\text{EssRoot}(\text{EffSpell}(\hat{\alpha}_{(m,1)})))$  (with medium priority), and  $\text{RuLat}(\text{EffSpell}(\hat{\alpha}_{(m,1)}))$  (with lowest priority). If two consecutive neighbors in the alphabetized list  $\{G_{(1)} = (g_{(1)}, \hat{\gamma}'_{(1)}, \hat{\gamma}''_{(1)}, \hat{\gamma}'''_{(1)}), \dots, G_{(M)} = (g_{(M)}, \hat{\gamma}'_{(M)}, \hat{\gamma}''_{(M)}, \hat{\gamma}'''_{(M)})\}$  satisfy

$$\text{SimpHrdTest}(\hat{\gamma}'''_{(m+1)}, \hat{\gamma}'''_{(m)}) = \text{FALSE}$$

**AND**

$$\text{SimpHrdTest}(\hat{\gamma}''_{(m)}, \hat{\gamma}''_{(m+1)}) = \text{FALSE}$$

**AND**

$$\text{HrdTest}(\hat{\gamma}''_{(m+1)}, \hat{\gamma}''_{(m)}) = \text{FALSE}$$

**AND**

$$\text{HrdTest}(\hat{\gamma}''_{(m)}, \hat{\gamma}''_{(m+1)}) = \text{FALSE}$$

**AND**

$$\text{HrdTest}(\hat{\gamma}'_{(m)}, \hat{\gamma}'_{(m+1)}) = \text{FALSE}$$

where  $m \in \mathbb{Z} \cap [1, M)$ , then add a demarcation line between these two entries. In this manner, the alphabetized list  $\{G_{(1)}, \dots, G_{(M)}\}$  is divided into separate groups of tagged clusters  $\{\Gamma_1 = \{G_{(1,1)}, \dots, G_{(1,m_1)}\}, \dots, \Gamma_K = \{G_{(K,1)}, \dots, G_{(1,m_K)}\}\}$ . Generate a list of word clusters  $\{\check{\Gamma}_1 = (\check{G}_{(1,1)}, \dots), \dots, \check{\Gamma}_K = (\check{G}_{(K,1)}, \dots)\}$  by discarding all the tags (effective spellings, essential roots, vowel blotted forms) from each  $\Gamma_k$ , where  $k \in \mathbb{Z} \cap [1, K]$ .

(3) For each word cluster  $\check{\Gamma}_k = (\check{G}_{(k,1)}, \dots)$ , we augment it into a tagged entry

$$\mathcal{G}_k \equiv (\check{\Gamma}_k, \check{\Gamma}'_k, \check{\Gamma}''_k) := (\check{\Gamma}_k, \text{EssRoot}(\text{EffSpell}(\check{G}_{(k,1)})), \text{VbEssRoot}(\text{EssRoot}(\text{EffSpell}(\check{G}_{(k,1)})))).$$

Recall that  $\hat{\sigma}^{-1}$  is the reverse of the string  $\hat{\sigma}$  (Definition 3.1). The list  $\{\mathcal{G}_1 = (\check{\Gamma}_1, \check{\Gamma}'_1, \check{\Gamma}''_1), \dots, \mathcal{G}_K = (\check{\Gamma}_K, \check{\Gamma}'_K, \check{\Gamma}''_K)\}$  is sorted sorted alphabetically, with respect to  $(\text{RuLat}(\check{\Gamma}''_k))^{-1}$  (with higher priority) and  $\text{RuLat}(\check{\Gamma}'_k)$  (with lower priority). If two consecutive neighbors in the alphabetized list  $\{\mathcal{G}_{(1)} = (\check{\Gamma}_{(1)}, \check{\Gamma}'_{(1)}, \check{\Gamma}''_{(1)}), \dots, \mathcal{G}_{(K)} = (\check{\Gamma}_{(K)}, \check{\Gamma}'_{(K)}, \check{\Gamma}''_{(K)})\}$  satisfy

$$\text{VbAspTest}(\hat{\Gamma}''_{(k)}, \hat{\Gamma}''_{(k+1)}) = \text{FALSE}$$

**AND**

$$\text{VbAspTest}(\hat{\Gamma}'_{(k)}, \hat{\Gamma}'_{(k+1)}) = \text{FALSE}$$

where  $k \in \mathbb{Z} \cap [1, K)$ , then add a demarcation line between these two entries. In this manner, the alphabetized list  $\{\mathcal{G}_{(1)}, \dots, \mathcal{G}_{(K)}\}$  is divided into separate groups of tagged clusters  $\{\tilde{\Gamma}_1 = \{\mathcal{G}_{(1,1)}, \dots, \mathcal{G}_{(1,n_1)}\}, \dots, \tilde{\Gamma}_J = \{\mathcal{G}_{(J,1)}, \dots, \mathcal{G}_{(1,n_J)}\}\}$ , from which the output list of word clusters is generated, after removal of all the tags from each  $\tilde{\Gamma}_j$ , where  $j \in \mathbb{Z} \cap [1, J]$ .

*Example 7.26.1.* Most Russian nouns distinguish six cases (nominative, genitive, dative, accusative, instrumental, prepositional) in singular and plural. A limited number of nouns have additional forms in three more cases (vocative, locative and partitive).

The sample nouns below are chosen according to the following web pages:

[https://en.wiktionary.org/wiki/Appendix:Russian\\_nouns#Declension\\_paradigms](https://en.wiktionary.org/wiki/Appendix:Russian_nouns#Declension_paradigms)

[https://en.wiktionary.org/wiki/Template:ru-noun-table#Basic\\_examples](https://en.wiktionary.org/wiki/Template:ru-noun-table#Basic_examples)

*апреле, апрелей, апрелем, апрели, апрель, апрелю, апреля, апрелям, апрелями, апрелях* — “April”;

*блюд, блюда, блюдам, блюдами, блюдах, блюде, блюдо, блюдом, блюду* — “dish”;

*бог, бога, богам, богами, богах, боге, боги, богам, богом, богу, боже* — “god”;

*бояр, боярам, боярами, боярах, бояре, боярин, боярина, боярине, боярином, боярину* — “boyar”;

*вид, вида, видам, видами, видах, виде, видов, видом, виду, виды* — “appearance”;

*волчиц, волчица, волчицам, волчицами, волчицах, волчице, волчицей, волчищем, волчищи, волчищу* — “maturewolf”;

*воротец, воротца, воротцам, воротцами, воротцах* — “wicket”;

*времена, временам, временами, временах, временем, времени, времён, время* — “time”;

*газет, газета, газетам, газетами, газетах, газете, газетой, газетою, газету, газеты* — “newspaper”;

*герое, героев, героем, герои, герой, герою, героя, героям, героями, героях* — “hero”;

*гетеросексуальности, гетеросексуальность, гетеросексуальностью* — “heterosexuality”;

*голов, голова, головам, головами, головах, голове, головой, головою, голову, головы* — “head”;

*дверей, двери, дверь, дверьми, дверью, дверям, дверями, дверях* — “door”;

*дев, дева, девам, девами, девах, деве, дево, девой, девою, деву, девы* — “maiden”;

*день, дне, дней, днём, дни, дню, дня, дням, днями, днях* — “day”;

*детей, дети, детьми, детям, детях, ребёнка, ребёнке, ребёнком, ребёнку, ребёнок, ребят, ребята, ребята-там, ребятами, ребятах* — “child”;

*друг, друга, друге, другом, другу, дружже, друзей, друзья, друзьям, друзьями, друзьях* — “friend”;

*железа, железам, железами, железах, железе, железой, железю, железу, железы, желёз* — “gland”;

*жилиц, жилища, жилищам, жилищами, жилищах, жилище, жилищем, жилищу* — “dwelling”;

*житие, житием, житии, житий, житию, жития, житиям, житиями, житиях* — “life”;

*журнал, журнала, журналам, журналами, журналах, журнале, журналов, журналом, журналу, журналы* — “magazine”;

*искр, искра, искрам, искрами, искрах, искре, искрой, искрою, искру, искры* — “spark”;

*историей, историею, истории, историй, историю, история, историям, историями, историях* — “history”;

*камень, каменьев, каменя, каменям, каменями, каменях, камне, камней, камнем, камни, камню, камня, камням, камнями, камнях* — “stone”;

*карандаш, карандаша, карандашам, карандашами, карандашах, карандаше, карандашей, карандаши, карандашом, карандашу* — “pencil”;

*книг, книга, книгам, книгами, книгах, книге, книги, книгой, книгою, книгу* — “book”;

*колен, колена, коленам, коленами, коленах, колене, колено, коленом, колену* — “tribe”;

*колена, колене, коленей, колени, колено, коленом, колену, коленям, коленями, коленьях* — “knee”;

*колена, колене, колено, коленом, колену, коленьев, коленья, коленьям, коленьями, коленьях* — “joint”;

*копеек, копейка, копейкам, копейками, копейках, копейке, копейки, копейкой, копейкою, копейку* — “kopek”;

*лёд, льда, льдам, льдами, льдах, льде, льдов, льдом, льду, льды* — “ice”;

*лоскут, лоскута, лоскутам, лоскутами, лоскутах, лоскуте, лоскутов, лоскутом, лоскуту, лоскуты, лоскутьев, лоскутья, лоскутьям, лоскутьями, лоскутьях* — “rag”;

*лошадей, лошади, лошадь, лошадьми, лошадью, лошадям, лошадями, лошадях* — “horse”;

*мальчат, мальчата, мальчатам, мальчатами, мальчатах, мальчонка, мальчонкам, мальчонками, мальчонках, мальчонке, мальчонки, мальчонков, мальчонком, мальчонку, мальчонок* — “littleboy”;

*море, морей, морем, морю, моря, морям, морями, морях* — “sea”;

*мост, моста, мостам, мостами, мостах, мосте, мостов, мостом, мосту, мосты* — “bridge”;

*муж, мужа, муже, мужей, мужем, мужу, мужья, мужьям, мужьями, мужьях* — “husband”;

*неделе, неделей, неделю, недели, недель, неделю, неделя, неделям, неделями, неделях* — “week”;

*нож, ножа, ножам, ножами, ножах, ноже, ножей, ножи, ножом, ножу* — “knife”;

*няне, няней, нянею, няни, нянь, няню, няня, няням, нянями, нянях* — “nurse”;

- озерца, озерце, озерцо, озерцом, озерцу, озёрце, озёрца, озёрцам, озёрцами, озёрцах* — “lake”;
- окна, окнам, окнами, окнах, окне, окно, окном, окну, окон* — “window”;
- ореол, ореола, ореолам, ореолами, ореолах, ореоле, ореолов, ореолом, ореолу, ореолы* — “halo”;
- отец, отца, отцам, отцами, отцах, отце, отцов, отцом, отцу, отцы* — “father”;
- палец, пальца, пальцам, пальцами, пальцах, пальце, пальцев, пальцем, пальцу, пальцы* — “finger”;
- писем, письма, письмам, письмами, письмах, письме, письмо, письмом, письму* — “letter”;
- площадей, площади, площадь, площадью, площадям, площадями, площадях* — “square”;
- повод, повода, поводе, поводом, поводу, поводьев, поводья, поводьям, поводьями, поводьях* — “rein”;
- поле, полей, полем, полю, поля, полям, полями, полях* — “field”;
- пух, пуха, пухе, пухом, пуху* — “feather”;
- работ, работа, работам, работами, работах, работе, работой, работою, работу, работы* — “task”;
- рот, рта, рта́м, ртами, рта́х, рте, ртов, ртом, рту, рты* — “mouth”;
- сапожек, сапожка, сапожкам, сапожками, сапожках, сапожке, сапожки, сапожков, сапожком, сапожку, сапожок* — “boot”;
- сестёр, сестра, сестре, сестрой, сестрою, сестру, сестры, сёстрам, сёстрами, сёстрах, сёстры* — “sister”;
- словаре, словарей, словарём, словари, словарь, словарю, словаря, словарям, словарями, словарях* — “dictionary”;
- случае, случаев, случаем, случаи, случай, случая, случаям, случаями, случаях* — “event”;
- сна, снам, снами, снах, сне, снов, сном, сну, сны, сон* — “dream”;
- снег, снега, снегам, снегами, снегах, снеге, снегов, снегом, снегу* — “snow”;
- стол, стола, столам, столами, столах, столе, столов, столом, столу, столы* — “table”;
- сын, сына, сынам, сынами, сынах, сыне, сынов, сыновей, сыновья, сыновьям, сыновьями, сыновьях, сыном, сыну, сыны* — “son”;
- товарищ, товарища, товарищам, товарищами, товарищах, товарище, товарищей, товарищем, товарищи, товарищу* — “comrade”;
- урок, урока, урокам, уроками, уроках, уроке, уроки, уроков, уроком, уроку* — “lesson”;
- учащегося, учащемся, учащемуся, учащиеся, учащийся, учащимися, учащимся, учащихся* — “pupil”;
- учение, учением, учении, учений, учению, учения, учениям, учениями, учениях* — “learning”;
- училищ, училища, училищам, училищами, училищах, училище, училищем, училищу* — “college”;
- учителе, учителей, учителем, учителя, учитель, учителю, учителя, учителям, учителями, учителях* — “teacher”;
- феномен, феномена, феноменам, феноменами, феноменах, феномене, феноменов, феноменом, феномену, феномены* — “phenomenon”;
- хвала, хвалам, хвалами, хвалах, хвале, хвалой, хвалою, хвалу, хвалы* — “praise”;
- чае, чаем, чаёв, чаи, чай, чаю, чая, чаям, чаями, чаях* — “tea”.

It is worth noting that, unlike Polish, the consonants of the Russian noun stem mostly remain stable in all declined forms. The sample nouns given above are clustered by our algorithm as follows:

- {*апреле, апрелей, апрелем, апрели, апрель, апрелю, апреля, апрелям, апрелями, апрелях*},
- {*блюд, блюда, блюдам, блюдами, блюдах, блюде, блюдо, блюдом, блюду*},
- {*бог, бога, богам, богами, богах, боге, боги, богов, богом, богу, боже*},
- {*бояр, боярам, боярами, боярах, бояре, боярин, боярина, боярине, боярином, боярину*},
- {*вид, вида, видам, видами, видах, виде, видов, видом, виду, виды*},
- {*волчиц, волчица, волчицам, волчицами, волчицах, волчице, волчицей, волчицем, волчицы, волчицу*},
- {*воротец, воротца, воротцам, воротцами, воротцах*},
- {*времена, временам, временами, временах, временем, времени, времён, время*},
- {*газет, газета, газетам, газетами, газетах, газете, газетой, газетою, газету, газеты*},
- {*герое, героев, героем, герои, герой, герою, героя, героям, героями, героях*},
- {*гетеросексуальности, гетеросексуальность, гетеросексуальностью*},
- {*голов, голова, головам, головами, головах, голове, головой, головою, голову, головы*},
- {*дверей, двери, дверь, дверьми, дверью, дверям, дверями, дверях*},
- {*дев, дева, девам, девами, девах, деве, дево, девой, девою, деву, девы*},
- {*день, дне, дней, днём, дни, дню, дня, дням, днями, днях*},
- {*детей, дети, детьми, детям, детях, ребёнка, ребёнке, ребёнком, ребёнку, ребёнок, ребят, ребята, ребята-там, ребятами, ребятах*},
- {*друг, друга, друге, другом, другу, дружже, друзей, друзья, друзьям, друзьями, друзьях*},
- {*железа, железам, железами, железах, железе, железой, железой, железу, железы, желе́з*},
- {*жилищ, жилища, жилищам, жилищами, жилищах, жилище, жилищем, жилищу*},
- {*житие, житием, житии, житий, житию, жития, житиям, житиями, житиях*},
- {*журнал, журнала, журналам, журналами, журналах, журнале, журналов, журналом, журналу, журналы*},
- {*искр, искра, искрам, искрами, искрах, искре, искрой, искрою, искру, искры*},
- {*историей, историю, истории, историй, историю, история, историям, историями, историях*},
- {*камень, каменьев, каменья, каменьям, каменьями, каменьях, камне, камней, камнем, камни, камню, камня, камням, камнями, камнях*},
- {*карандаш, карандаша, карандашам, карандашами, карандашах, карандаше, карандашей, карандаши, карандашом, карандашу*},
- {*книг, книга, книгам, книгами, книгах, книге, книги, книгой, книгой, книгу*},
- {*колен, колена, коленам, коленами, коленах, колене, коленей, колени, колена, коленом, колена, коленев, коленья, коленьям, коленьями, коленьях, коленям, коленями, коленях*},
- {*копеек, копейка, копейкам, копейками, копейках, копейке, копейки, копейкой, копейкою, копейку*},
- {*лёд, льда, льдам, льдами, льдах, льде, льдов, льдом, льду, льды*},

{*лоскут, лоскута, лоскутам, лоскутами, лоскутах, лоскуте, лоскутов, лоскутом, лоскуту, лоскуты, лоскутьев, лоскутья, лоскутьям, лоскутьями, лоскутьях*},

{*лошадей, лошади, лошадь, лошадьми, лошадю, лошадям, лошадьями, лошадях*},

{*мальчат, мальчата, мальчатам, мальчатами, мальчатах, мальчонка, мальчонкам, мальчонками, мальчонках, мальчонке, мальчонки, мальчонков, мальчонком, мальчонку, мальчонок*},

{*море, морей, морем, морю, моря, морям, морями, морях*},

{*мост, моста, мостам, мостами, мостах, мосте, мостов, мостом, мосту, мосты*},

{*муж, мужа, муже, мужей, мужем, мужу, мужья, мужьям, мужьями, мужьях*},

{*неделе, неделей, неделю, недели, недель, неделю, неделя, неделям, неделями, неделях*},

{*нож, ножа, ножам, ножами, ножих, ноже, ножей, ножи, ножом, ножу*},

{*няне, няней, нянею, няни, нянь, няню, няня, няням, нянями, нянях*},

{*озерца, озерце, озерцо, озерцом, озерцу, озёрце, озёрца, озёрцам, озёрцами, озёрцах*},

{*окна, окнам, окнами, окнах, окне, окно, окном, окну, окон*},

{*ореол, ореола, ореолам, ореолами, ореолах, ореоле, ореолов, ореолом, ореолу, ореолы*},

{*отец, отца, отцам, отцами, отцах, отце, отцов, отцом, отцу, отцы*},

{*палец, пальца, пальцам, пальцами, пальцах, пальце, пальцев, пальцем, пальцу, пальцы*},

{*писем, письма, письмам, письмами, письмах, письме, письмо, письмом, письму*},

{*площадей, площади, площадь, площадью, площадям, площадями, площадях*},

{*повод, повода, поводе, поводом, поводу, поводьев, поводья, поводьям, поводьями, поводьях*},

{*поле, полей, полем, полю, поля, полям, полями, полях*},

{*пух, пуха, пухе, пухом, пуху*},

{*работ, работа, работам, работами, работах, работе, работой, работою, работу, работы*},

{*рот, рта, ртам, ртами, ртах, рте, ртов, ртом, рту, рты*},

{*сапожек, сапожка, сапожкам, сапожками, сапожках, сапожке, сапожки, сапожков, сапожком, сапожку, сапожок*},

{*сестёр, сестра, сестре, сестрой, сестрою, сестру, сестры, сётрам, сётрами, сёстрах, сёстры*},

{*словаре, словарей, словарём, словари, словарь, словарю, словаря, словарям, словарями, словарях*},

{*случае, случаев, случаем, случаи, случай, случию, случая, случаям, случаями, случаях*},

{*сна, снам, снами, снах, сне, снов, сном, сну, сны, сон*},

{*снег, снега, снегам, снегами, снегах, снеге, снегов, снегом, снегу*},

{*стол, стола, столам, столами, столах, столе, столов, столом, столу, столы*},

{*сын, сына, сынам, сынами, сынах, сыне, сынов, сыновей, сыновья, сыновьям, сыновьями, сыновьях, сыном, сыну, сыны*},

{*товарищ, товарища, товарищам, товарищами, товарищах, товарище, товарищей, товарищем, товарищи, товарищу*},

{урок, урока, урокам, уроками, уроках, уроке, уроки, уроков, уроком, уроку},

{учащегося, учащемся, учащемуся, учащиеся, учащийся, учащимся, учащимся, учащих, учителя, учителей, учителем, учителя, учитель, учителю, учителя, учителям, учителями, учителях},

{учение, учением, учени, учений, учению, учения, учениям, учениями, учениях},

{училищ, училища, училищам, училищами, училищах, училище, училищем, училищу},

{феномен, феномена, феноменам, феноменами, феноменах, феномене, феноменов, феноменом, феномену, феномены},

{хвала, хвалам, хвалами, хвалах, хвале, хвалой, хвалою, хвалу, хвалы},

{чае, чаем, чаёв, чаи, чай, чаю, чая, чаям, чаями, чаях},

As we send the following sample adjectives (including participles of certain verbs)

*большая, большего, большее, большей, большем, большему, большею, большие, больший, большим, большими, больших, большего, большое, большой, большом, большому, большою, большую, велик, велика, велики, велико, наибольшая, наибольшего, наибольшее, наибольшей, наибольшем, наибольшему, наибольшею, наибольшие, наибольший, наибольшим, наибольшими, наибольших, наибольшую* — “big”;

*делавшая, делавшего, делавшее, делавшей, делавшем, делавшему, делавшею, делавшие, делавший, делавшим, делавшими, делавших, делавшую* — “do (past active participles)”;

*делающая, делающего, делающее, делающей, делающем, делающему, делающею, делающие, делающий, делающим, делающими, делающих, делающую* — “do (present active participles)”;

*дорог, дорога, дорогая, дороги, дорогие, дорогим, дорогими, дорогих, дорого, дорогого, дорогое, дорогой, дорогом, дорогому, дорогою, дорогую, дороже* — “expensive”;

*красив, красива, красивая, красивее, красивейший, красиво, красивого, красивое, красивой, красивом, красивому, красивою, красивую, красивы, красивые, красивый, красивым, красивыми, красивых, краше* — “beautiful”;

*крут, крута, крутая, крутейший, круто, крутого, крутое, крутой, крутом, крутому, крутою, крутую, круты, крутые, крутым, крутыми, крутых, круче* — “steep”;

*любим, любима, любимая, любимо, любимого, любимое, любимой, любимом, любимому, любимую, любимую, любимы, любимые, любимый, любимым, любимыми, любимых* — “love (present passive participles)”;

*молод, молода, молодая, молод, молодого, молодое, молодой, молодом, молодому, молодой, молодую, молоды, молодые, молодым, молодыми, молодых, моложе* — “young”;

*мягка, мягкая, мягки, мягкие, мягкий, мягким, мягкими, мягких, мягко, мягкого, мягкое, мягкой, мягком, мягкому, мягкою, мягкую, мягко, мягчайший, мягче, наимягчайший* — “soft”;

*решена, решено, решены, решён, решённая, решённого, решённое, решённой, решённом, решённому, решённую, решённые, решённый, решёнными, решённых* — “decide (past passive perfect participles)”;

*тих, тиха, тихая, тихи, тихие, тихий, тихим, тихими, тихих, тихо, тихого, тихое, тихой, тихом, тихому, тихую, тихую, тишайший, тише* — “silent”;

*част, часта, частая, часто, частого, частое, частой, частом, частому, частую, частую, часты, частые, частый, частым, частыми, частых, чаще* — “frequent”.

to our algorithm, we receive the following results:

{большая, большего, большее, большей, большем, большему, большею, большие, больший, большим, большими, больших, большего, большое, большой, большом, большому, большою, большую, велик, велика, велики, велико, наибольшая, наибольшего, наибольшее, наибольшей, наибольшем, наибольшему, наибольшею, наибольшие, наибольший, наибольшим, наибольшими, наибольших, наибольшую},

{делавшая, делавшего, делавшее, делавшей, делавшем, делавшему, делавшиею, делавшие, делавший, делавшим, делавшими, делавших, делавшую, делающая, делающего, делающее, делающей, делающем, делающему, делающею, делающие, делающий, делающим, делающими, делающих, делающую},

{дорог, дорога, дорогая, дороги, дорогие, дорогим, дорогими, дорогих, дорого, дорогого, дорогое, дорогой, дорогом, дорогому, дорогою, дорогую, дорожке},

{красив, красива, красивая, красивее, красивейший, красиво, красивого, красивое, красивой, красивом, красивому, красивою, красивую, красивы, красивые, красивый, красивым, красивыми, красивых, краше},

{крут, крута, крутая, крутейший, круто, крутого, крутое, крутой, крутом, крутому, крутою, крутую, круты, крутые, крутым, крутыми, крутых, круче},

{любим, любима, любимая, любимо, любимого, любимое, любимой, любимом, любимому, любимую, любимую, любимы, любимые, любимый, любимым, любимыми, любимых},

{молод, молода, молодая, молодо, молодого, молодое, молодой, молодом, молодому, молодую, молодую, молоды, молодые, молодым, молодыми, молодых, моложе},

{мягка, мягкая, мягки, мягкие, мягкий, мягким, мягкими, мягких, мягко, мягкого, мягкое, мягкой, мягком, мягкому, мягкою, мягкую, мягок, мягчайший, мягче, наимягчайший},

{решена, решено, решены, решён, решённая, решённого, решённое, решённой, решённом, решённому, решённую, решённые, решённый, решённым, решёнными, решённых},

{тих, тиха, тихая, тихи, тихие, тихий, тихим, тихими, тихих, тихо, тихого, тихое, тихой, тихом, тихому, тихою, тихую, тишайший, тише},

{част, часта, частая, часто, частого, частое, частой, частом, частому, частою, частую, часты, частые, частый, частым, частыми, частых, чаще},

*Example 7.26.2.* Like Polish, a great majority of Russian verbs come in imperfective/perfective pairs. Consonant alternations still find their way into the Russian verb stems (more precisely, the end of stems) in conjugated forms. In the following, we list representative verbs from all the 16 Zaliznyak classes ([https://en.wiktionary.org/wiki/Appendix:Russian\\_verbs](https://en.wiktionary.org/wiki/Appendix:Russian_verbs)), together with their imperfective/perfective counterparts that are formed in various ways (we note that the two aspects of the same verb may not belong to the same Zaliznyak class). These verb conjugations may also involve consonant changes in the stem, or other types of irregularities. The Zaliznyak class number, which will be shown parenthetically after the English translation for each word family below, describes at least one aspect (imperfective or perfective) of the verb in question.

делав, делавши, делавший, делаем, делаемый, делает, делаете, делаешь, делай, делайте, делал, делала, делали, делало, деланный, делать, делаю, делают, делающий, деля, сделав, сделавши, сделавший, сделаем, сделает, сделаете, сделаешь, сделай, сделайте, сделал, сделала, сделали, делало, деланный, сделать, сделаю, сделают — “do” (1);

нарисовав, нарисовавши, нарисовавший, нарисовал, нарисовала, нарисовали, нарисовало, нарисованный, нарисовать, рисуем, рисует, рисуете, рисуешь, рисуй, рисуйте, рисую, рисуют, рисовав, рисовавши, рисовавший, рисовал, рисовала, рисовали, рисовало, рисованный, рисовать, рисуем, рисуемый, рисует, рисуете, рисуешь, рисуй, рисуйте, рисую, рисуют, рисующий, рисуя — “draw” (2a);

блевав, блевавши, блевавший, блевал, блевала, блевали, блевало, блеванём, блеванёт, блеванёте, блеванёшь, блевани, блеваните, блевану, блеванув, блеванувиши, блеванувиши, блеванул, блеванула, блеванули, блевануло, блеванут, блевануть, блевать, блёванный, блюём, блюёт, блюёте, блюёшь, блюй, блюйте, блюю, блюют, блюющий, блюя — “vomit” (2b);

гиб, гибла, гибли, гибло, гибнем, гибнет, гибнете, гибнешь, гибни, гибните, гибну, гибнув, гибнувши, гибнувиши, гибнул, гибнут, гибнуть, гибнущий, погиб, погибла, погибли, погибло, погибнем, погибнет, погибнете, погибнешь, погибни, погибните, погибну, погибнут, погибнуть, погибши, погибший — “die” (3a);

рискнём, рискнёт, рискнёте, рискнёшь, рискни, рискните, рискну, рискнув, рискнувши, рискнувиши, рискнул, рискнула, рискнули, рискнуло, рискнут, рискнуть, рисковав, рисковавши, рисковавший, рисковал, рисковала, рисковали, рисковало, рисковать, рискуем, рискует, рискуете, рискуешь, рискуй, рискуйте, рискую, рискуют, рискующий, рискуя — “risk” (3b);



*береги, берегите, берегла, берегли, берегло, берегу, берегут, берегущий, бережём, бережённый, бережёт, бережёте, бережёшь, беречь, берёг, берёгши, берёгший, сбереги, сберегите, сберегла, сберегли, сберегло, сберегу, сберегут, сбережём, сбережённый, сбережёт, сбережёте, сбережёшь, сберечь, сберёг, сберёгши, сберёгший, убереги, уберегите, уберегла, уберегли, уберегло, уберегу, уберегут, убережём, убережённый, убережёт, убережёте, убережёшь, уберечь, уберёг, уберёгши, уберёгший* — “guard” (8b);

*вымер, вымерев, вымереть, вымерла, вымерли, вымерло, вымерши, вымерший, вымирав, вымиравши, вымиравший, вымираем, вымирает, вымираете, вымираешь, вымирай, вымирайте, вымирал, вымирала, вымиралы, вымирало, вымирать, вымираю, вымирают, вымирающий, вымирая, вымрем, вымрет, вымрете, вымрешь, вымири, вымирите, вымру, вымрут* — “become extinct” (9a);

*потерев, потереть, потёр, потёрла, потёрли, потёрло, потёртый, потёрши, потёрший, потрём, потрёт, потрёте, потрёшь, потри, потрите, потру, потрут, тереть, тёр, тёрла, тёрли, тёрло, тёртый, тёрши, тёрший, трём, трёт, трёте, трёшь, три, трите, тру, трут, трущий* — “rub” (9b);

*выпалывав, выпалывавши, выпалывавший, выпалываем, выпалываемый, выпалывает, выпалываете, выпалываешь, выпалывай, выпалывайте, выпалывал, выпалывала, выпалывали, выпалывало, выпалывать, выпалываю, выпалывают, выпалывающий, выпалывая, выполем, выполет, выполете, выполешь, выполи, выполите, выполов, выполовши, выполовший, выполол, выполола, выпололи, выпололо, выполотый, выполоть, выполю, выполют* — “weed” (10a);

*вкалывав, вкалывавши, вкалывавший, вкалываем, вкалываемый, вкалывает, вкалываете, вкалываешь, вкалывай, вкалывайте, вкалывал, вкалывала, вкалывали, вкалывало, вкалывать, вкалываю, вкалывают, вкалывающий, вкалывая, вколем, вколет, вколете, вколешь, вколи, вколите, вколов, вколовши, вколовший, вколел, вколола, вкололи, вкололо, вколотый, вколоть, вколю, вколют* — “stick” (10c);

*вылейся, вылейтесь, выливавшийся, выливавшись, выливаемся, выливаетесь, выливается, выливаешься, выливайся, выливайтесь, выливалась, выливались, выливалось, выливался, выливаться, выливаюсь, выливаются, выливающийся, выливаясь, вылившись, вылилась, вылились, вылилось, вылился, вылиться, выльемся, выльетесь, выльется, выльешься, выльюсь, выльются* — “spill over” (11a);

*добей, добейте, добив, добивав, добивавши, добивавший, добиваем, добиваемый, добивает, добиваете, добиваешь, добивай, добивайте, добивал, добивала, добивали, добивало, добивать, добиваю, добивают, добивающий, добивая, добивши, добивший, добил, добила, добили, добило, добитый, добить, добыём, добыёт, добыёте, добыёшь, добыю, добыют* — “crush” (11b);

*вымоем, вымоет, вымоете, вымоешь, вымой, вымойте, вымою, вымоют, вымыв, вымывши, вымывший, вымыл, вымыла, вымыли, вымыло, вымытый, вымыть, моем, моемый, моет, моете, моешь, мой, мойте, мою, моют, моющий, моя, мыв, мывши, мывший, мыл, мыла, мыли, мыло, мытый, мыть, помоем, помоем, помоете, помоешь, помой, помойте, помою, помогут, помыв, помывши, помывший, помыл, помыла, помыли, помыло, помытый, помыть, умоем, умоем, умоете, умоешь, умой, умойте, умою, умоют, умыв, умывши, умывший, умыл, умыла, умыли, умыло, умытый, умыть* — “wash” (12a);

*гнив, гнивши, гнивший, гниём, гниёт, гниёте, гниёшь, гнил, гнила, гнили, гнило, гнить, гнию, гниют, гниющий, сгнив, сгнивши, сгнивший, сгниём, сгниёт, сгниёте, сгниёшь, сгнил, сгнила, сгнили, сгнило, сгнить, сгнию, сгниют* — “putrefy” (12b);

*дав, давав, дававши, дававший, даваемый, давай, давайте, давал, давала, давали, давало, давать, давая, давши, давший, дадим, дадите, дадут, даём, даёт, даёте, даёшь, дай, дайте, дал, дала, дали, дало, дам, данный, даст, дать, дашь, даю, дают, дающий* — “give” (13);

*выжав, выжавши, выжавший, выжал, выжала, выжали, выжало, выжатый, выжать, выжимав, выжимавши, выжимавший, выжимаем, выжимаемый, выжимает, выжимаете, выжимаешь, выжимай, выжимайте, выжимал, выжимала, выжимали, выжимало, выжимать, выжимаю, выжимают, выжимающий, выжимая, выжмем, выжмет, выжмете, выжмешь, выжми, выжмите, выжму, выжмут* — “wring” (14a);

*жсав, жсавши, жсавший, жсал, жсала, жсали, жсало, жсатый, жсать, жсмём, жсмёт, жсмёте, жсмёшь, жсми, жсмите, жсму, жсмут, жсмущий, жсмя, пожсав, пожсавши, пожсавший, пожсал, пожсала, пожсали, пожсало, пожсатый, пожсать, пожсмём, пожсмёт, пожсмёте, пожсмёшь, пожсми, пожсмите, пожсму, пожсмут, сжсав, сжсавши, сжсавший, сжсал, сжсала, сжсали, сжсало, сжсатый, сжсать, сожсмём, сожсмёт, сожсмёте, сожсмёшь, сожсми, сожсмите, сожсму, сожсмут* — “squeeze” (14b);

*обнимаю, обнимаешь, обнимай, обнимайте, обнимал, обнимала, обнимали, обнимало, обнимать, обнимаю, обнимают, обнимающий, обнимающая, обнимем, обнимет, обнимете, обнимешь, обними, обнимите, обниму, обнимут, обняв, обнявши, обнявший, обнял, обняла, обняли, обняло, обнятый, обнять* — “hug” (14c);

*встав, вставав, встававши, встававший, вставай, вставайте, вставал, вставала, вставали, вставало, вставать, вставая, вставши, вставший, встаём, встаёт, встаёте, встаёшь, встал, встала, встали, встало, встанем, встанет, встанете, встанешь, встану, встанут, встань, встаньте, встать, встаю, встают, встающий* — “rise” (15);

*выжив, выживав, выживавши, выживавший, выживаем, выживает, выживаете, выживаешь, выживай, выживайте, выживал, выживала, выживали, выживало, выживать, выживаю, выживают, выживающий, выживая, выживем, выживет, выживете, выживешь, выживи, выживите, выживу, выживут, выживши, выживший, выжил, выжила, выжили, выжило, выжить* — “survive” (16a);

*жив, живём, живёт, живёте, живёшь, живи, живите, живу, живут, живущий, живши, живший, живя, жил, жила, жили, жило, жить, пожив, поживём, поживёт, поживёте, поживёшь, поживи, поживите, поживу, поживут, поживши, поживший, пожил, пожила, пожили, пожило, пожить* — “live” (16b).

These verbs are clustered by our algorithms as follows:

{береги, берегите, берегла, берегли, берегло, берегу, берегут, берегущий, бережём, бережённый, бережёт, бережёте, бережёшь, беречь, берёг, берёги, берёгший, сбереги, сберегите, сберегла, сберегли, сберегло, сберегу, сберегут, сбережём, сбережённый, сбережёт, сбережёте, сбережёшь, сберечь, сберёг, сберёги, сберёгший, убереги, уберегите, уберегла, уберегли, уберегло, уберегу, уберегут, убережём, убережённый, убережёт, убережёте, убережёшь, уберечь, уберёг, уберёги, уберёгший},

{блевав, блевавши, блевавший, блевал, блевала, блевали, блевало, блеванём, блеванёт, блеванёте, блеванёшь, блевани, блеваните, блевану, блеванув, блеванувши, блеванувший, блеванул, блеванула, блеванули, блевануло, блеванут, блевануть, блевать, блёванный, блюём, блюёт, блюёте, блюёшь, блюй, блюйте, блюю, блюют, блюющий, блюя},

{бренча, бренчав, бренчавши, бренчавший, бренчал, бренчала, бренчали, бренчало, бренчат, бренчать, бренчащий, бренчи, бренчим, бренчит, бренчите, бренчишь, бренчу},

{ведём, ведённый, ведёт, ведёте, ведёшь, веди, ведите, ведомый, вежди, веждишь, веда, вела, вели, вело, вести, поведём, поведённый, поведёт, поведёте, поведёшь, поведи, поведите, поведу, поведут, поведиши, поведишь, поведа, повела, повели, повело, повести},

{веду, ведут, ведущий},

{веем, веемый, веете, веешь, вей, вейте, вею, веют, веющий, вея, веяв, веявши, веявший, веял, веяла, веяли, веяло, веянный, веять},

{веет},

{взглядывав, взглядывавши, взглядывавший, взглядываем, взглядываемый, взглядывает, взглядываете, взглядываешь, взглядывай, взглядывайте, взглядывал, взглядывала, взглядывали, взглядывало, взглядывать, взглядываю, взглядывают, взглядывающий, взглядывая, взглянем, взглянет, взглянете, взглянешь, взгляни, взгляните, взгляну, взглянув, взглянувши, взглянувший, взглянул, взглянула, взглянули, взглянуло, взглянут, взглянуть, глядев, глядевши, глядевший, глядел, глядела, глядели, глядело, глядеть, гляди, глядим, глядит, глядите, глядишь, глядя, глядят, глядящий, гляжу},

{взывав, вызывавши, вызывавший, вызываем, вызывает, вызываете, вызываешь, вызывай, вызывайте, вызывал, вызывала, вызывали, вызывало, вызывать, вызываю, вызывают, вызывающий, вызывая, вызычем, вызычет, вызычете, вызычешь, вызыци, вызыците, вызыцу, вызыцут},

{взыскав, зыскавши, зыскавший, зысканный, зыскать, зыскивав, зыскивавши, зыскивавший, зыскиваем, зыскиваемый, зыскивает, зыскиваете, зыскиваешь, зыскивай, зыскивайте, зыскивал, зыскивала, зыскивали, зыскивало, зыскивать, зыскиваю, зыскивают, зыскивающий, зыскивая},

{взыскал, зыскала, зыскали, зыскало},

{вкалывав, вкалывавиши, вкалывавиший, вкалываем, вкалываемый, вкалывает, вкалываете, вкалываешь, вкалывай, вкалывайте, вкалывал, вкалывала, вкалывали, вкалывало, вкалывать, вкалываю, вкалывают, вкалывающий, вкалывая, вколем, вколет, вколете, вколешь, вколи, вколите, вколов, вколовиши, вколовиший, вколлол, вколлола, вколлоли, вколлоло, вколлотый, вколлоть, вколлю, вколлют},

{влез, влезав, влезавиши, влезавиший, влезаем, влезает, влезаете, влезаеть, влезай, влезайте, влезал, влезала, влезали, влезало, влезать, влезая, влезем, влезет, влезете, влезешь, влезла, влезли, влезло, влезть, влезу, влезут, влезши, влезший, влезь, влезьте},

{воззвав, воззвавиши, воззвавиший, воззвал, воззвала, воззвали, воззвало, воззванный, воззвать, воззовём, воззовёт, воззовёте, воззовёшь, воззови, воззовите, воззову, воззовут},

{встав, вставав, встававиши, встававиший, вставай, вставайте, вставал, вставала, вставали, вставало, вставать, вставая, вставиши, вставиший, встаём, встаёт, встаёте, встаёшь, встал, встала, встали, встало, встанем, встанет, встанете, встанешь, встану, встанут, встань, встаньте, встать, встаю, встают, встающий},

{выжав, выжавиши, выжавиший, выжал, выжала, выжали, выжало, выжатый, выжать, выжив, выживав, выживавиши, выживавиший, выживаем, выживает, выживаете, выживаешь, выживай, выживайте, выживал, выживала, выживали, выживало, выживать, выживаю, выживают, выживающий, выживая, выживем, выживет, выживете, выживешь, выживи, выживите, выживу, выживут, выживши, выживиший, выжил, выжила, выжили, выжило, выживав, выживавиши, выживавиший, выживаем, выживаемый, выживает, выживаете, выживаешь, выживай, выживайте, выживал, выживала, выживали, выживало, выживать, выживаю, выживают, выживающий, выживая, выжить, выжмем, выжмет, выжмете, выжмешь, выжми, выжмите, выжму, выжмут},

{вылейся, вылейтесь, выливавшийся, выливавшись, выливаемся, выливаетесь, выливается, выливаешься, выливайся, выливайтесь, выливалась, выливались, выливалось, выливался, выливаться, выливаюсь, выливаются, выливающийся, выливаясь, вылившись, вылившись, вылилась, вылились, вылилось, вылился, вылиться, выльемся, выльетесь, выльется, выльешься, выльюсь, выльются},

{вымер, вымерев, вымереть, вымерла, вымерли, вымерло, вымериши, вымериший, вымирав, вымиравши, вымиравший, вымираем, вымирает, вымираете, вымираешь, вымирай, вымирайте, вымирал, вымирала, вымиралы, вымирало, вымирать, вымираю, вымирают, вымирающий, вымирая, вымрем, вымрет, вымрете, вымрешь, вымири, вымирите, вымру, вымрут},

{вымоем, вымоет, вымоете, вымоешь, вымой, вымойте, вымою, вымоют, вымыв, вымывши, вымывиший, вымыл, вымыла, вымыли, вымыло, вымытый, вымыть, моем, моемый, моет, моете, моешь, мой, мойте, мою, моют, моющий, моя, мыв, мывиши, мывиший, мыл, мыла, мыли, мыло, мытый, мыть, помоем, помоет, помоете, помоешь, помой, помойте, помою, помогут, помыв, помывши, помывиший, помыл, помыла, помыли, помыло, помытый, помыть, умоем, умоет, умоете, умоешь, умой, умойте, умою, умоют, умыв, умывши, умывиший, умыл, умыла, умыли, умыло, умытый, умыть},

{выпалывав, выпалывавиши, выпалывавиший, выпалываем, выпалываемый, выпалывает, выпалываете, выпалываешь, выпалывай, выпалывайте, выпалывал, выпалывала, выпалывали, выпалывало, выпалывать, выпалываю, выпалывают, выпалывающий, выпалывая, выподем, выполет, выполете, выполешь, выполи, выполите, выполов, выполовиши, выполовиший, выполлол, выполлола, выполлоли, выполлоло, выполлотый, выполлоть, выполлю, выполют},

{вытек, вытекав, вытекавиши, вытекавиший, вытекаем, вытекает, вытекаете, вытекаешь, вытекай, вытекайте, вытекал, вытекала, вытекали, вытекало, вытекать, вытекаю, вытекают, вытекающий, вытекающая, вытеки, вытеките, вытекла, вытекли, вытекло, вытеку, вытекут, вытекиши, вытекиший, вытечем, вытечет, вытечете, вытечешь, вытечь, теки, теките, текла, текли, текло, теку, текут, текущий, течём, течёт, течёте, течёшь, течь, тёк, тёкиши, тёкиший},

{гиб, гибла, гибли, гибло, гибнем, гибнет, гибнете, гибнешь, гибни, гибните, гибну, гибнув, гибнувши, гибнувиший, гибнул, гибнут, гибнуть, гибнущий, погиб, погибла, погибли, погибло, погибнем, погибнет, погибнете, погибнешь, погибни, погибните, погибну, погибнут, погибнуть, погибши, погибший},

{гнив, гнивши, гнивиший, гниём, гниёт, гниёте, гниёшь, гнил, гнила, гнили, гнило, гнить, гнию, гниют, гниющий, сгнив, сгнивши, сгнивиший, сгниём, сгниёт, сгниёте, сгниёшь, сгнил, сгнила, сгнили, сгнило, сгнить, сгнию, сгниют},

{дав, давав, дававши, дававший, даваемый, давай, давайте, давал, давала, давали, давало, давать, давая, давши, давший, дадим, дадите, дадут, даём, даёт, даёте, даёшь, дай, дайте, дал, дала, дали, дало, дам, данный, даст, дать, дашь, даю, дают, дающий},

{делаю, делавши, делавший, делаем, делаемый, делает, делаете, делаешь, делай, делайте, делал, делала, делали, делало, деланный, делать, делаю, делают, делающий, делая, сделав, сделавши, сделавший, сделаем, сделает, сделаете, сделаешь, сделай, сделайте, сделал, сделала, сделали, делало, сделанный, сделать, сделаю, сделают},

{добей, добейте, добив, добивав, добивавши, добивавший, добиваем, добиваемый, добивает, добиваете, добиваешь, добивай, добивайте, добивал, добивала, добивали, добивало, добивать, добиваю, добивают, добивающий, добивая, добивши, добивший, добил, добила, добили, добило, добитый, добить, добьём, добьёт, добьёте, добьёшь, добью, добьют},

{жав, жавши, жавший, жал, жала, жаленный, жали, жалив, жалил, жалила, жалили, жалило, жалим, жалимый, жалит, жалите, жалить, жалишь, жало, жаль, жальте, жालю, жаля, жалят, жалящий, жатый, жать, жмём, жмёт, жмёте, жмёшь, жми, жмите, жму, жмут, жмущий, жмя, пожав, пожавши, пожавший, пожал, пожала, пожали, пожало, пожатый, пожать, пожмём, пожмёт, пожмёте, пожмёшь, пожми, пожмите, пожму, пожмут, сжав, сжавши, сжавший, сжал, сжала, сжали, сжало, сжатый, сжать, сожмём, сожмёт, сожмёте, сожмёшь, сожми, сожмите, сожму, сожмут},

{жаливши, жаливший, ужаливши, ужаливший},

{жив, живём, живёт, живёте, живёшь, живи, живите, живу, живут, живущий, живши, живший, живя, жил, жила, жили, жило, жить, пожив, поживём, поживёт, поживёте, поживёшь, поживи, поживите, поживу, поживут, поживши, поживший, пожил, пожила, пожили, пожило, пожить},

{изгнав, изгнавши, изгнавший, изгнал, изгнала, изгнали, изгнало, изгнанный, изгнать, изгони, изгоним, изгонит, изгоните, изгонишь, изгону, изгоняв, изгонявши, изгонявший, изгоняем, изгоняемый, изгоняет, изгоняете, изгоняешь, изгоняй, изгоняйте, изгонял, изгоняла, изгоняли, изгоняло, изгонят, изгонять, изгоняю, изгоняют, изгоняющий, изгоняя},

{люби, любив, любивши, любивший, любил, любила, любили, любило, любим, любимый, любит, любите, любить, любишь, любленный, люблю, любя, любяют, любящий, полюби, полюбив, полюбивши, полюбивший, полюбил, полюбила, полюбил, полюбил, полюбил, полюбим, полюбит, полюбите, полюбить, полюбишь, полюбленный, полюблю, полюбят},

{нарисовав, нарисовавши, нарисовавший, нарисовал, нарисовала, нарисовали, нарисовало, нарисованный, нарисовать, рисуем, рисует, рисуете, рисуешь, рисуй, рисуйте, рисую, рисуют, рисовав, рисовавши, рисовавший, рисовал, рисовала, рисовали, рисовало, рисованный, рисовать, рисуем, рисуемый, рисует, рисуете, рисуешь, рисуй, рисуйте, рисую, рисуют, рисующий, рисуя},

{обнимав, обнимавши, обнимавший, обнимаем, обнимаемый, обнимает, обнимаете, обнимаешь, обнимай, обнимайте, обнимал, обнимала, обнимали, обнимало, обнимать, обнимаю, обнимают, обнимающий, обнимая, обнимем, обнимет, обнимете, обнимешь, обними, обнимите, обниму, обнимут, обняв, обнявши, обнявший, обнял, обняла, обняли, обняло, обнятый, обнять},

{потерев, потереть, потёр, потёрла, потёрли, потёрло, потёртый, потёрши, потёрший, потрём, потрёт, потрёт, потрёшь, потри, потрите, потру, потрут, тереть, тёр, тёрла, тёрли, тёрло, тёртый, тёрши, тёрший},

{пощади, пощадив, пощадивши, пощадивший, пощадил, пощадила, пощадили, пощадило, пощадим, пощадит, пощадите, пощадить, пощадишь, пощадят, пощажённый, пощажу, щади, щадив, щадивши, щадивший, щадил, щадила, щадил, щадил, щадим, щадимый, щадит, щадите, щадить, щадить, щадя, щадят, щадящий, щажённый, щажу},

{рискнём, рискнёт, рискнёте, рискнёшь, рискни, рискните, рискну, рискнув, рискнувши, рискнувший, рискнул, рискнула, рискнули, рискнуло, рискнут, рискнуть, рисковав, рисковавши, рисковавший, рисковал, рисковала, рисковали, рисковало, рисковать, рискуем, рискует, рискуете, рискуешь, рискуй, рискуйте, рискую, рискуют, рискующий, рискуя},

{*слыша, слышав, слышавши, слышавший, слышал, слышала, слышали, слышало, слышанный, слышат, слышатъ, слышаций, слышим, слышимый, слышит, слышите, слышишь, слышу, услышав, услышавши, услышавший, услышал, услышала, услышали, услышало, услышанный, слышат, слышатъ, услышим, услышит, услышите, услышишь, услышу, услышь, услышьте*},

{*трём, трёт, трёте, трёшь, три, трите, тру, трут, трущий*},

{*ужаленный, ужалив, ужалил, ужалила, ужалили, ужалило, ужалим, ужалит, ужалите, ужалить, ужалишь, ужаль, ужальте, ужалю, ужалят*},

Please beware that the verb clustering example above contains a few notable errors, partly due to interference between verbs with similar-looking stems.

*Example 7.26.3.* In Fig. S11, we further apply the aforementioned word clustering algorithm to topic extraction and machine translation (see Table S1 for text sources).

In Russian, “bat” (a kind of flying mammal) is called *летучая мышь* (literally “flying mouse”), so we consider *bat* an exact match to *летучая* “flying” in Fig. S11b’.





ВИДЫ... ФОРМЫ... РАЗЛИЧНЫЕ... ЖИВОТНЫЕ... ОБРАЗОМ... РОДА... БОЛЬШИЕ... СЛУЧАЕВ... СТРОИТЕЛЬСТВО... ВРЕМЯ... ОТБОР...  
 ЕСТЕСТВЕННЫЕ... РАЗНОВИДНОСТИ... РАСТЕНИЙ... ОСОБЕННОСТИ... ПРИЗНАКИ... РАЗВИТИЕ... МОДИФИКАЦИИ... ДВА... ОТНОШЕНИЯ... НАПРИМЕР...  
 ПРЕДСТАВЛЯЕТ... СУЩЕСТВУЮЩИЕ... ИМЕЕТ... ЧАСТИ... ПОСЛЕДОВАТЕЛЬНОСТИ... ЧИСЛА... СОВЕРШЕННО... УСЛОВИЯ... ИЗМЕНЧИВЫ... ЗНАЧИТЕЛЬНО... СЯЗАННЫМИ...  
 СТЕПЕНИ ВЕРОЯТНО... СИЛЫ... ОРГАНИЗМ... СКРЕЩИВАНИЯ... ЖИЗНИ... ДАВНО... ВАРИАЦИИ... ДЕЙСТВИЕ... ГРУППЫ... НАКЛОН... СЛЕДОВАТЕЛЬНО... ОБЪЯСНИМО...  
 ПЕРИОД... ОСНОВАНИИ... КАК... НОВЫЕ... КРАЙНЕ... СОСТОЯНИИ... РАЗМЕР... СУЩЕСТВА... МАЛО... ИЗВЕСТНО... ОУДАЧЛИВЫ... ПОЛЕЗНО... ОБЫЧНО... РАДИО... ТРУДОСТА...  
 ПРЕДСТА... ХОРОШО... ПЕРВЫ... СВЯЗНО... ПОРОД... ПТИЦ... СОХРАНЕНИЕ... ОСТАВЛЕ... ОРГАНИЗМ... ОБЛАСТИ... ДРУГ... СХОДИМО... РЕЗУЛЬТАТ...  
 СПОСОБНО... ЗАМЕЧА... ОБИТАТЕЛИ... ОБЩИИ... РАСПРОСТРАНЕНИЯ... МЕСТА... ИЗЛОЖИ... ТЕЧЕНИЕ... ВРЕМ... ВСТРЕЧАЕТСЯ... СКОЛОН... ПРОИЗВЕ... ФАКТ... СТОРОНЫ ПОДРОБНО...  
 ОТЛИЧАЕТСЯ... СТЕРИЛЬНОСТЬ... ПРИРОДЕ... ГИБРИДОВ... ДАВНО... ВНЕШНЕ НАСКОМКИ... ДАВНО... ПОТОМ... ПОЛОВА... ВОПРОС... СОМНЕВА... ИНСТИНКТ...  
 ПОДВЕРЖАЮ... ИСТИННО... СРАВНИТЕ... КЛИМАТ... ГАИ... ПРОМЕЖУТОЧНЫЕ... ОТЛИЧА... ИЗМЕН... ПОСЛА... ВСТОИ... ДОМАШНИ... ОБЛАСТИ... ИСТОРИЧЕСКИ... ВЫСТА... ЦЕЛИ... ВОЗРАСТ...  
 ДЛИН... МЕДИ... СЕМЕНА... В ВЫРАЖЕНИИ... СРЕДСТВ... ТРОИ... ЮЖНО... ЦВЕТ... ДОИ... ПОСЛА... ОТЛИЧА... КЛАСС... ЧЕЛОВЕК... ПРИРОД... ПРИРОД... ПУТЬ...  
 ПОСЛЕ... ДРУГ... ВОДЕ... ЗАКОН... ЗАКОН... ДРЕВ... ФЕРТИЛЬНОСТЬ... ПЫЛЬ... ГОЛУБИ... ПОКОЛЕНИЯ... ЗАДА... СТО...  
 РЕД... МАТЕРИ... ПЕРЕМ... НЕИЗ... УДАЧ... АДАПТИ... ПЛА... ОБИТА... ЗАМЕ... ОРАС... ПРОИЗ... НАТУРА... ДИ... ОБИ... ИВА... ВЫСО... ДА... СЕМЬИ...  
 ПРИВЫЧ... ГРАДИ... СТАДИ... ПРИРО... ДОСТИ... ПОЛУ... ПЕРЕХОД... ПОВИ... УПОТРЕБ... ПОСЛА... ПРОИЗХОЖД... ПЧЕЛ... ОБЪЯС... СТРЕ... СОС... ПРИ... ПРО... Д... ОБЪЕ... РЕ...  
 РАС... РАВ... ПОД... УДАЧ... ОБЛА... РАВНО... СМ... АМЕРИ... РАВ... ПОКО... ОБИТА... МЕКОНОТА... СЕ... СО... СЕВЕР... ДОСТА... МО... ПРЕ... НО... ПР... МО...  
 КЛИМАТ... ИСТО... СЕ... В... Р... НАСЛЕД... РУДИМЕНТАРНЫЕ... ДЕЙ... ЦВЕТКА... КЛУ... РАБОТ... РАВНО... ИСПО... РАВНО... ПОСЛО...

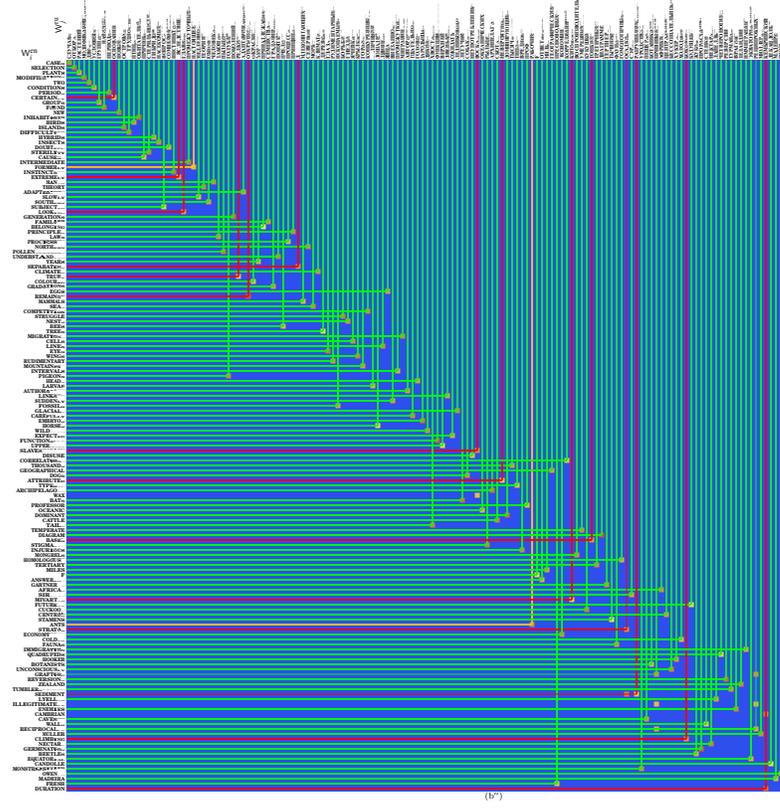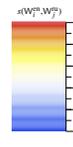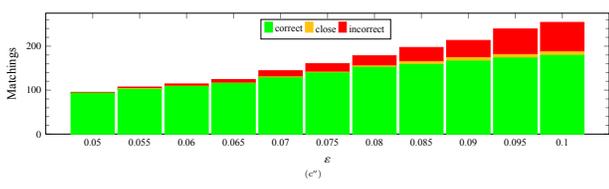

Fig. 511. Text mining in Russian. (Continued) (a'') Statistically identified topics ( $n_{ij} \geq 20$ ) in a Russian version of *Origin of Species*, with the same color encoding scheme as Fig. S3. (b'') Semantic similarities  $s(W^E, W^R)$  between selected topics in English and Russian versions of *Origin of Species*. Cross-hairs meet at optimal nodes that solve the bipartite matching problem. The thickness of each horizontal (resp. vertical) cross-hair is inversely proportional to the row-wise (resp. column-wise) rank of the similarity score for the optimal node. Green (resp. red) cross-hair indicates a correct (resp. incorrect) match. Amber cross-hair marks a link between distinct concepts that share the same hypernyms. (c'') Results from control experiments with different choices of the  $\epsilon$ -parameter in ballpark screening criteria (1.13).

## 8 Approximate word clustering in selected Uralic languages

In this section, we present the approximate clustering algorithms for two representative Uralic languages: Finnish and Hungarian.

The major challenges in information processing for Finnish and Hungarian are the following:

- Both languages have extremely complex case systems (15 for Finnish and 18 for Hungarian, not counting rarely used cases), and the situation is compounded by the fact that several case endings may attach sequentially to the same word.
- Finnish has consonant gradation (mutation of stem-final consonants) during declension. (Estonian, another Uralic language not treated here, behaves similarly.) Hungarian case endings sometimes also cause changes in the stem-final consonants.
- Their verb morphologies have a similar complexity as the Romance languages.
- Similar to the Germanic counterpart, both Finnish and Hungarian orthographies require that certain compounds be written as single words, with no spaces or hyphens between their constituents.

Finnish and Hungarian are two major agglutinative languages spoken in Europe. Basque, a language isolate spoken in France and Spain, also has agglutinative morphology. The agglutinative nature of Turkish (as well as other Turkic languages spoken in Eurasia) is similar to Finnish and Hungarian. We will cover the word clustering algorithms for Basque and Turkish in §9.

### 8.1 Modified Porter stemming algorithm for Finnish

**Definition 8.1** (Finnish stop words). If a word belongs to the following list<sup>96</sup>:

*aika, aina, ainainen, ainoa, ainoaa, ainoain, ainoan, ainoana, ainoat, ainoata, ainoiden, ainoihin, ainoiksi, ainoilla, ainoille, ainoilta, ainoin, ainoina, ainoine, ainoisiin, ainoissa, ainoista, ainoita, ainoitta, ainoitten, ainuiden, ainuihin, ainuiksi, ainuilla, ainuille, ainuilta, ainuin, ainuina, ainuineen, ainuisiin, ainuissa, ainuista, ainuita, ainuitta, ainuitten, ainut, ainutta, ainuiksi, ainuulla, ainuulle, ainuulta, ainuun, ainuuna, ainuuseen, ainuussa, ainuusta, ainuut, ainuutta, aivan, ala, alakkain, alapuolella, alas, alatusten, alhaalla, alhaalle, alhaalta, ali, alitse, alla, alle, allekkain, alta, ansiosta, asti, edelle, edellä, edeltä, edes, edessä, edestä, editse, eduksi, ehkä, ei, elati-ve, eli, ellei, emme, en, enemmän, eniten, ennen, ennenkuin, ennestä, ennestään, ensi, ensin, entä, enää, erittäin, eräiden, eräihin, eräiksi, eräille, eräillä, eräiltä, eräin, eräine, eräinä, eräisiin, eräissä, eräistä, eräitten, eräittä, eräitä, eräs, erästä, erääksi, eräälle, eräällä, eräältä, erään, eräänä, eräeseen, eräässä, eräästä, eräät, eräättä, esi, esiin, et, etemme, eteen, eteensä, etenkin, etenään, ette, ettei, etten, ettet, että, halki, he, heidän, heidät, heihin, heille, heillä, heiltä, heissä, heistä, heitä, heti, hiukan, hyvin, hän, häneen, hänelle, hänellä, häneltä, hänessä, hänestä, hänet, häntä, ihan, ikään, ilman, itse, itseemme, itseeni, itseenne, itseensä, itseesi, itseksesi, itsellesi, itselläsi, itsellään, itseltäsi, itseltään, itsen, itsenä, itsenäsi, itsenään, itsesi, itsessäsi, itsessään, itsestäsi, itsestään, itseä, itseäsi, itseään, ja, jk, jkhun, jkn, jkta, jo, johdosta, johon, johonkukseen, joiden, joidenkuiden, joihin, joihinkuihin, joiksi, joiksikuiksi, joilla, joillain, joillakuilla, joille, joillekuille, joilta, joiltain, joiltakuilta, join, joina, joinain, joinakuina, joine, joinekuine, joinkuin, joissa, joissain, joissakuissa, joista, joistain, joistakuista, joita, joitain, joitakuista, joitse, joitta, joittakuitta, joitten, joittenkuitten, jokainen, jokaiseen, jokaiseksi, jokaisella, jokaiselle, jokaiselta, jokaisen, jokaisena, jokaisessa, jokaisesta, jokaiset, jokaisetta, jokaisia, jokaisien, jokaisiin, jokaisiksi, jokaisilla, jokaisille, jokaisilta, jokaisin, jokaisina, jokaisine, jokaisissa, jokaisista, jokaisitta, jokaista, jokaisten, joksikuksi, joku, jollain, jollakulla, jollei, jollekulle, jollen, jollet, jolloin, joltain, joltakulta, jommaksikumaksi, jommallakummalla, jommallekummalle, jommaltakummalta, jommankumman, jommassakummassa, jommastakummasta, jommatkummat, jommattakummatta, jommiksikummiiksi, jommillakummilla, jommillekummille, jommiltakummilta, jomminkummin, jommissakummassa, jommistakummista, jommittakummitta, jompaa-kumpaa, jompaankumpaan, jompanakumpana, jompiakumpia, jompiinkumpiin, jompikumpi, jompinakumpina, jompinekumpine, jona, jonain, jonakuna, jonka, jonkin, jonkun, jos, joskus, jossain, jossakussa, jostain, jostakusta, jota, jotain, jotakuta, joten, jotenkuten, jotka, jotkin, jotkut, jottakutta, joukoon, joukossa, joukosta, juuri, jäljessä, jälkeen, jälleen, kai, kaikeksi, kaikella, kaikelle, kaikelta, kaiken, kaikessa, kaikesta, kaiket, kaiketta, kaikiksi, kaikilla, kaikille, kaikilta, kaikissa, kaikista, kaikitta, kaikkea, kaikkeen, kaikkein, kaikkena, kaikki, kaikkia, kaikkiin, kaikkina, kaikkine, kanssa, kautta, keiden, keihin, keiksi, keille, keillä, keiltä, keinä, keissä, keistä, keitä, keneen, keneksi, kenelle, kenellä, keneltä, kenen, kenenä, kenessä, kenestä, kenet, kenties, kerran, keskelle,*

<sup>96</sup>Our list of Finnish stop words is based on <http://snowball.tartarus.org/algorithms/finnish/stop.txt>, with extensive additions to roughly match their counterparts in English.

*keskellä, keskeltä, kesken, keskenään, keskeä, keski, keskitse, keskuudeksi, keskuudella, keskuudelle, keskuudelta, keskuuden, keskuudessa, keskuudesta, keskuudet, keskuudetta, keskuuksia, keskuuksien, keskuuksiin, keskuuksiksi, keskuuksilla, keskuuksille, keskuuksilta, keskuuksin, keskuuksina, keskuuksineen, keskuuksissa, keskuuksista, keskuuksitta, keskuus, keskuuteen, keskuutena, keskuutta, ketkä, ketä, kohdaksi, kohdalla, kohdalle, kohdalta, kohdan, kohdassa, kohdasta, kohdat, kohdatta, kohdiksi, kohdilla, kohdille, kohdilta, kohdin, kohdissa, kohdista, kohditta, kohta, kohtaa, kohtain, kohtana, kohti, kohtia, kohtiin, kohtina, kohtineen, koko, koska, kovin, kuhunkin, kuidenkin, kuihinkin, kuiksikin, kuillakin, kuillekin, kuiltakin, kuin, kuinakin, kuissakin, kuistakin, kuitakin, kuitenkin, kuittakin, kuittenkin, kuka, kukin, kuksikin, kullakin, kullekin, kulloinkin, kultakin, kummaksi, kummalla, kummalle, kummalta, kumman, kummassa, kummasta, kummat, kummatta, kummiksi, kummilla, kummille, kummilta, kummin, kummissa, kummista, kummitta, kumpaa, kumpaan, kumpain, kumpana, kumpi, kumpia, kumpiin, kumpina, kumpine, kun, kunakin, kunnekin, kunnes, kussakin, kustakin, kutakin, kuten, kutkin, kuttakin, kykene, kykenee, kykeneminen, kykenemistä, kykenemä, kykenemäisillään, kykenemän, kykenemättömien, kykenemättömiin, kykenemättömiksi, kykenemättömille, kykenemättömillä, kykenemättömillä, kykenemättömin, kykenemättömine, kykenemättöminä, kykenemättömissä, kykenemättömistä, kykenemättömittä, kykenemättömiä, kykenemättömäksi, kykenemättömälle, kykenemättömällä, kykenemättömältä, kykenemättömän, kykenemättömänä, kykenemättömissä, kykenemättömästä, kykenemättömät, kykenemättömättä, kykenemättömään, kykenemätön, kykenemätöntä, kykenemätöntä, kykenemään, kykenen, kykenet, kykenevien, kykeneviin, kykeneviksi, kykeneville, kykenevillä, kykeneviltä, kykenevin, kykenevine, kykenevinä, kykenevissä, kykenevistä, kykenevittä, kykeneviä, kykenevä, kykeneväin, kykenevän, kykenevänä, kykenevää, kykenevään, kykeni, kykenin, kykenisi, kykenisin, kykenisit, kykenit, kyllin, kyllä, lain, liene, lienee, lienen, lienet, liian, luo, luokse, luona, luota, lähekkäin, lähelle, lähellä, läheltä, lähes, lähetysten, lähi, lähitse, läpi, läsnä, lävitse, me, meidän, meidät, meihin, meille, meillä, meiltä, meissä, meistä, meitä, melko, mieluummin, mihin, miksi, mikä, mikäli, mikään, millainen, millaiseen, millaiseksi, millaisella, millaiselle, millaiselta, millaisen, millaisena, millaisessa, millaisesta, millaiset, millaisetta, millaisia, millaisien, millaisiin, millaisiksi, millaisilla, millaisille, millaisilta, millaisin, millaisina, millaisineen, millaisissa, millaisista, millaisitta, millaista, millaisten, mille, milloin, millä, millään, miltä, miltään, minkä, minkälainen, minkälaiseen, minkälaiseksi, minkälaisella, minkälaiselle, minkälaiselta, minkälaisen, minkälaisena, minkälaisessa, minkälaisesta, minkälaiset, minkälaisetta, minkälaisia, minkälaisien, minkälaisiin, minkälaisiksi, minkälaisilla, minkälaisille, minkälaisilta, minkälaisin, minkälaisina, minkälaisineen, minkälaisissa, minkälaisista, minkälaisista, minkälaista, minkälaiten, minkään, minne, minua, minulla, minulle, minulta, minun, minussa, minusta, minut, minuun, minä, minään, missä, missään, mistä, mistään, miten, mitkä, mitkään, mitä, mitään, moinen, moiseen, moiseksi, moisella, moiselle, moiselta, moisen, moisena, moisessa, moisesta, moiset, moisetta, moisia, moisien, moisiin, moisiksi, moisilla, moisille, moisilta, moisin, moisina, moisine, moisissa, moisista, moisitta, moista, moisten, molemmaksi, molemmalla, molemmalle, molemmalta, molemman, molemmassa, molemmasta, molemmat, molemmatta, molemmiksi, molemmilla, molemmille, molemmilta, molemmin, molemmissa, molemmista, molemmitta, molempaa, molempaan, molempana, molempi, molempia, molempiin, molempina, molempine, moneen, moneksi, monella, monelle, monelta, monen, monena, monessa, monesta, monesti, monet, monetta, moni, monia, moniaalla, moniaalle, moniaalta, moniin, monin, monina, monine, monna, monta, muiden, muihin, muiksi, muilla, muille, muilta, muin, muina, muine, muissa, muista, muita, muitta, muitten, mukaan, mukana, mutta, mutte, muttei, mutten, muttet, muu, muualla, muualle, muualta, muuhun, muulloin, muun, muuna, muut, muuta, muutama, muutamaa, muutamain, muutaman, muutamana, muutamat, muutamia, muutamien, muutamiin, muutamiksi, muutamalla, muutamille, muutamilta, muutamin, muutamina, muutamineen, muutamissa, muutamista, muutamitta, myös, myötä, ne, niiden, niihin, niiksi, niille, niillä, niiltä, niin, niine, niinkuin, niinä, niissä, niistä, niitten, niittä, niitä, no, noiden, noihin, noiksi, noilla, noille, noilta, noin, noina, noissa, noista, noita, nuo, nyt, näiden, näihin, näiksi, näille, näillä, näiltä, näin, näine, näinä, näissä, näistä, näittä, näitä, nämä, ohi, ohitse, oikein, oitis, ole, olema, olemaa, olemain, olemaisillaan, oleman, olemana, olemat, olematon, olematonta, olematonten, olemattomaan, olemattomaksi, olemattomalla, olemattomalle, olemattomalta, olemattoman, olemattomana, olemattomassa, olemattomasta, olemattomat, olemattomatta, olemattomia, olemattomien, olemattomiin, olemattomiksi, olemattomilla, olemattomille, olemattomilta, olemattomin, olemattomina, olemattomine, olemattomissa, olemattomista, olemattomitta, olemia, olemien, olemiin, olemiksi, olemilla, olemille, olemilta, olemien, olemineen, olemissa, olemista, olemitta, olen, olet, oleva, olevaa, olevain, olevan, olevana, olevasi, olevia, olevien, oleviin, oleviksi, olevilla, oleville, olevilta, olevin, olevina, olevine, olevissa, olevista, olevitta, oli, olin, olisi, olisin, olisit, olit, olkaa, olko, olkoon, olkoot, olla, olleeksi, olleella, olleelle, olleelta, olleen, olleena, olleeseen, olleessa, olleesta, olleet, olleetta, olleiden, olleihin, olleiksi, olleilla, olleille, olleilta, ollein, olleina, olleine, olleisiin, olleissa, olleista, olleita, olleitta, olleitten, ollen, ollessa, olлуiksi, olлуilla, olлуille, olлуilta, olлуun, olлуissa, olлуista, olлуutta, olлуksi, olhulla, ollulle, ollulta, ollun, ollussa, ollusta, ollut, ollutta, oltaessa, oltaisi, oltaisiin, oltako, oltakoon, oltaman, oltane, oltava, oltiin, oltu, oltua, oltuihin, oltuina, oltuine, oltuja, oltujen, oltuna, oltuun, oma, omaa, omain, oman, omana, omat, omia, omien, omiin, omiksi, omilla, omille, omilta, omin, omina, omina, omine, omissa, omista, omitta, on, ovat, paitsi, paljon, paljoa, paljoihin, paljoiksi, paljoilla, paljoille, paljoilta, paljoin,*

paljoina, paljoineen, paljoissa, paljoista, paljoitta, paljoja, paljojen, paljon, paljona, paljoon, paljot, pelkiksi, pelkille, pelkillä, pelkiltä, pelkin, pelkissä, pelkistä, pelkittä, pelkkien, pelkkiin, pelkkine, pelkkinä, pelkkiä, pelkkä, pelkkäin, pelkkään, pelkkää, pelkkään, pelkäksi, pelkälle, pelkällä, pelkältä, pelkän, pelkässä, pelkästä, pelkät, pelkättä, perässä, pian, pitkin, poikki, pois, poissa, pysty, pystyessä, pystyi, pystyin, pystyisi, pystyisin, pystyisit, pystyit, pystykää, pystyköön, pystykööt, pystyminen, pystymistä, pystymä, pystymäisillään, pystymän, pystymätön, pystymään, pystyn, pystyne, pystyne, pystyneenä, pystyneeseen, pystyneet, pystyneiden, pystyneihin, pystyneiksi, pystyneille, pystyneillä, pystyneiltä, pystynein, pystyneine, pystyneinä, pystyneisiin, pystyneissä, pystyneistä, pystyneitten, pystyneittä, pystyneitä, pystynet, pystynyt, pystynyttä, pystyt, pystyttiin, pystytty, pystyttäessä, pystyttäisi, pystyttäisiin, pystyttäkö, pystyttäköön, pystyttämän, pystyttäne, pystyttävä, pystyt, pystyttiin, pystytty, pystyttäessä, pystyy, pystyä, päin, rinnalla, saa, saada, saaden, saadessa, saakaa, saakka, saakoon, saakoot, saama, saamaisillaan, saaman, saamaton, saaminen, saamista, saan, saane, saanee, saaneet, saanet, saanut, saat, saataessa, saataisi, saataisiin, saatako, saatakoon, saataman, saatane, saatava, saatiin, saatu, saava, sai, sain, saisi, saisin, saisit, sait, sama, samaa, saman, samana, samat, samoihin, samoiksi, samoilla, samoille, samoilta, samoin, samoina, samoine, samoissa, samoista, samoitta, samoja, samojen, sangen, se, sellainen, sellaiseen, sellaiseksi, sellaisella, sellaiselle, sellaiselta, sellaisen, sellaisena, sellaisessa, sellaisesta, sellaiset, sellaisetta, sellaisia, sellaisien, sellaisiin, sellaisiksi, sellaisilla, sellaisille, sellaisilta, sellaisin, sellaisina, sellaisineen, sellaisissa, sellaisista, sellaisitta, sellaista, sellaiten, semmoinen, semmoiseen, semmoiseksi, semmoisella, semmoiselle, semmoiselta, semmoisen, semmoisena, semmoisessa, semmoisesta, semmoiset, semmoisetta, semmoisia, semmoisien, semmoisiin, semmoisiksi, semmoisilla, semmoisille, semmoisilta, semmoisin, semmoisina, semmoisine, semmoisissa, semmoisista, semmoisitta, semmoista, semmoisten, sen, sentään, senvuoksi, siellä, sieltä, siihen, siinä, siis, siitä, sijaan, siksi, sille, silloin, sillä, siltä, sinne, sinua, sinulla, sinulle, sinulta, sinun, sinussa, sinusta, sinut, sinuun, sinä, sisä, sisäkkäin, sisätysten, sisään, siten, sitten, sitä, taa, taakse, taannoin, taas, tahansa, tahi, tai, taitse, taka, takaa, takaisin, takana, takia, te, tee, teet, tehden, tehdessä, tehdä, tehdään, tekkää, tekkö, tekköön, tekkööt, tehne, tehnee, tehneet, tehnen, tehnet, tehnyt, tehtiin, tehty, tehtäessä, tehtäisi, tehtäisiin, tehtäkö, tehtäköön, tehtämän, tehtäne, tehtävä, teidän, teidät, teihin, teille, teillä, teiltä, teimme, tein, teissä, teistä, teit, teitte, teitä, tekee, tekeminen, tekemistä, tekemä, tekemäisillään, tekemän, tekemätön, tekemään, tekevä, tekevät, teki, tekisi, tekisin, tekisit, todella, toinen, toisaalla, toisaalle, toisaalta, toiseen, toiseksi, toisella, toiselle, toiselta, toisen, toisena, toisensa, toisessa, toisesta, toiset, toisetta, toisia, toisien, toisiensa, toisiin, toisiinsa, toisikseen, toisiksensa, toisiksi, toisilla, toisille, toisilta, toisin, toisina, toisine, toisinsa, toisissa, toisista, toisitta, toista, toisten, toistensa, tuo, tuohon, tuollainen, tuollaiseen, tuollaiseksi, tuollaisella, tuollaiselle, tuollaiselta, tuollaisen, tuollaisena, tuollaisessa, tuollaisesta, tuollaiset, tuollaisetta, tuollaisia, tuollaisien, tuollaisiin, tuollaisiksi, tuollaisilla, tuollaisille, tuollaisilta, tuollaisin, tuollaisina, tuollaisineen, tuollaisissa, tuollaisista, tuollaisitta, tuollaista, tuollaisten, tuon, tuona, tuota, tuskin, tähden, tähän, täksi, tällainen, tällaiseen, tällaiseksi, tällaisella, tällaiselle, tällaiselta, tällaisen, tällaisena, tällaisessa, tällaisesta, tällaiset, tällaisetta, tällaisia, tällaisien, tällaisiin, tällaisiksi, tällaisilla, tällaisille, tällaisilta, tällaisin, tällaisina, tällaisineen, tällaisissa, tällaisista, tällaisitta, tällaista, tällaisten, tälle, tällä, tällöin, tältä, tämä, tämän, tänne, tänä, tässä, tästä, täten, tätä, täydy, täytyi, täytyisi, täytykö, täytyköön, täytyminen, täytymistä, täytyne, täytynee, täytynyt, täytyy, täytyä, täällä, täältä, ulkoa, ulkona, ulos, usea, useaa, usein, useammaksi, useammalla, useammalle, useammalta, useamman, useammassa, useammasta, useammat, useammatta, useammiksi, useammilla, useammille, useammilta, useammin, useammissa, useammista, useammitta, useampaa, useampaan, useampain, useampana, useampi, useampia, useampiin, useampina, useampine, usean, useana, useat, useata, useiden, useihin, useiksi, useilla, useille, useilta, useimmaksi, useimmalla, useimmalle, useimmalta, useimman, useimmassa, useimmasta, useimmat, useimmatta, useimmiksi, useimmilla, useimmille, useimmilta, useimmin, useimmissa, useimmista, useimmitta, useimpaan, useimpain, useimpana, useimpia, useimpien, useimpiin, useimpina, useimpine, usein, useina, useine, useinta, useinten, useisiin, useissa, useista, useita, useitta, useitten, uudelleen, uudestaan, vaan, vai, vaikka, vaikkei, vaikkemme, vaikken, vaikket, vaikkette, vain, vallan, varsin, vasta, vastedes, vasten, vastikään, vielä, viereen, vierekkäin, vierelle, vierellä, viereltä, vieren, vieressä, vierestä, vieret, vieretysten, vieri, vieriin, vieritse, vierä, viertä, voi, voida, voiden, voidessa, voikaa, voikoon, voikoot, voima, voimaisillaan, voiman, voimaton, voiminen, voimista, voin, voine, voinee, voinet, voinet, voinut, voisi, voisin, voisit, voit, voitaessa, voitaisi, voitaisiin, voitako, voitakoon, voitaman, voitane, voitava, voitiin, voitu, voiva, vuoksi, väliin, välillä, välissä, välistä, yhdeksi, yhdelle, yhdellä, yhdeltä, yhden, yhdessä, yhdesti, yhdestä, yhdet, yhdettä, yhteen, yhtenä, yhtä, yhtäälle, yhtäällä, yhtäältä, yhtään, yhä, yksi, yksiin, yksin, yksine, yksinä, yksittäin, yksiä, ylen, yli, ylitse, yläpuolella, ylös, ympäri, ympäriinsä, ympäritse, älkää, älköön, älkööt, ällös, älä,

then we consider it a Finnish stop root (notation: **FinnishStopRoot**). A Finnish stop word matches the following string pattern:

**FinnishStopRoot**( $\emptyset$ |ksi|lla|lle|llä|lta|ltä|ssa|ssä|sta|stä|tta|ttä)( $\emptyset$ |kse)  
( $\emptyset$ |an|en|mm|nn|nsa|nsä|si|tte|vat|vät)( $\emptyset$ |han|hän|ka|kaan|kin|ko|kä|kään|kö|pa|pä)<sub>m</sub>,

or (*jok|vast*)'X.<sup>97</sup> All the Finnish stop words that appear in a particular document need to be ignored before we perform word clustering on the rest of the vocabulary list.  $\square$

Up to some modifications, our method is modeled after the Porter stemming algorithm for Finnish (<http://snowball.tartarus.org/algorithms/finnish/stemmer.html>), devised by Martin F. Porter. Our modifications of the Porter stemming algorithm aim at two goals: to fully take care of verb conjugations and to fully accommodate to consonant/vowel alternations in declensions.

### 8.1.1 Effective spelling and essential root

It is assumed that all Finnish words are converted to lowercase before going through any of the procedures below.

Unlike the situation in German, diacritical marks in Finnish can affect the meaning of a word immensely. For example, we have *rohkaista* “to encourage” vs. *röhkäistä* “to grunt”. Therefore, we are going to retain diacritical marks in the construction of Finnish effective spellings and essential roots, contrary to the practice for German.

Before we start, we recapitulate Martin F. Porter’s definition of Finnish vowels, restricted vowels and long vowels.

**Definition 8.2** (Finnish Vowels, Restricted Vowels and Long Vowels). Hereafter in §8.1, the symbol  $\mathbf{V}$  stands for any member from the list of Finnish vowels  $\{a, e, i, o, u, y, \ddot{a}, \ddot{o}\}$ . In line with the multiplicity notations introduced in Definition 3.3, the symbol  $\mathbf{V}_m$  stands for a text string formed by consecutive appearance of one or more (not necessarily identical or distinct) members from the set of Finnish vowels.

Dual to the notations above, the symbol  $\mathbf{C}$  stands for any character that does not belong to the list  $\{a, e, i, o, u, y, \ddot{a}, \ddot{o}\}$ , and  $\mathbf{C}_{m_0}$  stands for a text string formed by consecutive appearance of zero or more (not necessarily identical or distinct) characters that do not belong to the same list.

The symbol  $\mathbf{V}^*$  stands for any member from the list of Finnish restricted vowels  $\{a, e, i, o, u, \ddot{a}, \ddot{o}\}$ , while  $\mathbf{V}^{**}$  represents any one in the list of Finnish long vowels  $\{aa, ee, ii, oo, uu, \ddot{a}\ddot{a}, \ddot{o}\ddot{o}\}$ .  $\square$

In the following, we define the first and second protected ranges of a Finnish word, following Martin F. Porter’s definition of regions  $R1$  and  $R2$ .

**Definition 8.3** (Finnish First protected range). Let  $\hat{\sigma}$  be a Finnish text string, then its first protected range  $\text{ProtRg}_1(\hat{\sigma})$  is specified through the following procedures:

- Look for the string pattern  $\mathbf{C}_{m_0}\mathbf{V}_m\mathbf{C}\sim$  in the string  $\hat{\sigma}$ ;
- If the string pattern above is found, the last position occupied by such a string defines  $\text{ProtRg}_1(\hat{\sigma})$ ; otherwise, set  $\text{ProtRg}_1(\hat{\sigma}) = \ell(\hat{\sigma})$ .

Once  $\text{ProtRg}_1(\hat{\sigma})$  is determined, the text string  $\hat{\sigma}$  needs to be explicitly marked with a separator signifying the position of the first protected range. Concretely speaking, we define  $\text{MarkRg}_1(\hat{\sigma})$  by inserting a dagger symbol (“†”) at position  $\text{ProtRg}_1(\hat{\sigma}) + 1$  to the string  $\hat{\sigma}$ .  $\square$

**Definition 8.4** (Finnish Second protected range). Let  $\hat{\sigma}'$  be a Finnish text string marked explicitly with its first protected range, then its second protected range  $\text{ProtRg}_2(\hat{\sigma}')$  is determined by the following procedures:

- Look for the string pattern  $\dagger\mathbf{C}_{m_0}\mathbf{V}_m\mathbf{C}$  in the string  $\hat{\sigma}'$ ;
- If the string pattern above is found, the last position occupied by such a string defines  $\text{ProtRg}_2(\hat{\sigma}')$ ; otherwise, set  $\text{ProtRg}_2(\hat{\sigma}') = \ell(\hat{\sigma}')$ .

Once  $\text{ProtRg}_2(\hat{\sigma}')$  is determined, the text string  $\hat{\sigma}'$  needs to be further marked with a separator signifying the position of the second protected range. Concretely speaking, we define  $\text{MarkRg}_2(\hat{\sigma}')$  by inserting a double dagger symbol (“‡”) at position  $\text{ProtRg}_2(\hat{\sigma}') + 1$  to the string  $\hat{\sigma}'$ .  $\square$

*Example 8.4.1.* We use some English words to illustrate the workings of  $\text{ProtRg}_1$ ,  $\text{MarkRg}_1$ ,  $\text{ProtRg}_2$  and  $\text{MarkRg}_2$ :

| $\hat{\sigma}$                                   | <i>beau</i>   | <i>beauty</i>   | <i>beautiful</i>   | <i>beautifully</i>   |
|--------------------------------------------------|---------------|-----------------|--------------------|----------------------|
| $\text{ProtRg}_1(\hat{\sigma})$                  | 4             | 5               | 5                  | 5                    |
| $\text{MarkRg}_1(\hat{\sigma})$                  | <i>beau†</i>  | <i>beaut†y</i>  | <i>beaut†iful</i>  | <i>beaut†ifully</i>  |
| $\text{ProtRg}_2(\text{MarkRg}_1(\hat{\sigma}))$ | 5             | 7               | 8                  | 8                    |
| $\text{MarkRg}_2(\text{MarkRg}_1(\hat{\sigma}))$ | <i>beau†‡</i> | <i>beaut†y‡</i> | <i>beaut†if‡ul</i> | <i>beaut†if‡ully</i> |

<sup>97</sup>Here, the apostrophe refers to either APOSTROPHE [U+0027](#) or RIGHT SINGLE QUOTATION MARK [U+2019](#), as is appropriate for the particular text mining task.

**Algorithm 8.5** (Finnish effective spelling). For a Finnish word  $\hat{\sigma}$  (converted to lower case form), its effective spelling  $\text{EffSpell}(\hat{\sigma})$  is constructed in sequential steps:

- (1) Convert to lowercase and do  $\sim\text{ksest}(a|\ddot{a}) \rightarrow s$ ,  $\#\mathbf{X} \rightarrow \emptyset$ .
- (2) Do  $\text{uudelleen}\sim \rightarrow p\epsilon$ .
- (3) Do  $\text{nt}(\text{o}|\ddot{o})(\text{i}|\text{j})(\text{o}|\text{hi})(\text{o}|\text{n})(\text{o}|\text{a}|\text{en}|\ddot{a}) \rightarrow \text{nta}$ ,  $\sim\hat{\chi}_1\text{eeseen}\mathbf{X} \rightarrow \hat{\chi}_1\text{e}$ ,  $\sim\hat{\chi}_2\text{m}(\text{a}|\ddot{a})\text{sil}\mathbf{X} \rightarrow \hat{\chi}_2$ ,  $\sim\hat{\chi}_3\text{sest}(\text{a}|\ddot{a})\mathbf{X} \rightarrow \hat{\chi}_3\text{nen}$ ,  $\mathbf{X}\hat{\chi}\text{m}(\text{a}|\ddot{a})(\text{t}|\text{tt})(\text{o}|\ddot{o})(\text{m}|\text{n})(\text{o}|\text{a}|\text{aa}|\text{i}|\text{t}|\ddot{a}|\ddot{a}\ddot{a})(\text{o}|\text{en}|\text{in}|\text{ksi}|\text{ll}|\text{lt}|\text{n}|\text{ss}|\text{st}|\text{tt})(\text{o}|\text{a}|\text{e}|\ddot{a}) \rightarrow \text{tv}\tau\text{-}\mathbf{X}\hat{\chi}$ .
- (4) Replace

|                                                                          |                                                                                       |                                                    |                                                                                                                                                                                 |                                                                                                                     |
|--------------------------------------------------------------------------|---------------------------------------------------------------------------------------|----------------------------------------------------|---------------------------------------------------------------------------------------------------------------------------------------------------------------------------------|---------------------------------------------------------------------------------------------------------------------|
| $(\text{sisar} \text{velj})\text{enpo}(\text{i} \text{j})\mathbf{X}\sim$ | $(\text{sisar} \text{velj})\text{entyt}\mathbf{X}\sim$                                | <i>amerika</i>                                     | <i>avioliit</i> ( $\text{o} \text{t}$ ) $\sim$                                                                                                                                  | <i>etei</i> ( $\text{n} \text{s}$ ) $\sim$                                                                          |
| <i>v̄efω</i>                                                             | <i>v̄iece</i>                                                                         | <i>αμερικα</i>                                     | <i>μαρρ</i>                                                                                                                                                                     | <i>αιλς</i>                                                                                                         |
| <i>help</i> $\sim$                                                       | <i>henkilö</i>                                                                        | <i>ihme</i> $\mathbf{X}\sim$                       | <i>ihmi</i>                                                                                                                                                                     | <i>isänne</i>                                                                                                       |
| <i>ηελρ</i>                                                              | <i>περσö</i>                                                                          | <i>ωο̄öpe</i>                                      | <i>inhimi</i>                                                                                                                                                                   | <i>isä</i>                                                                                                          |
| <i>kaalli</i>                                                            | <i>kasvo</i>                                                                          | <i>kats</i> $\mathbf{X}$                           | <i>kirjasto</i>                                                                                                                                                                 | <i>koir</i>                                                                                                         |
| <i>expnsi</i>                                                            | <i>φασο</i>                                                                           | <i>kator</i>                                       | <i>λιβρο</i>                                                                                                                                                                    | <i>dog</i>                                                                                                          |
| <i>läpikotaisin</i>                                                      | <i>maine</i>                                                                          | <i>musta</i> ( <i>ank</i>   <i>sukk</i> ) $\sim$   | <i>naimis</i> $\sim$                                                                                                                                                            | <i>ou</i> ( <i>d</i>   <i>t</i> ) $\sim$                                                                            |
| <i>θυρυ</i>                                                              | <i>fame</i>                                                                           | <i>ιαλωσ</i>                                       | <i>μαρρ</i>                                                                                                                                                                     | <i>ωειρδο</i>                                                                                                       |
| <i>puolust</i>                                                           | <i>päiv</i>                                                                           | <i>selv</i> $\sim$                                 | <i>seuralai</i> ( $\text{n} \text{s}$ )                                                                                                                                         | <i>silm</i>                                                                                                         |
| <i>defens</i>                                                            | <i>πäiv</i>                                                                           | <i>celar</i>                                       | <i>σοclais</i>                                                                                                                                                                  | <i>εγε</i>                                                                                                          |
| <i>taho</i> $\sim$                                                       | <i>tall</i>                                                                           | <i>tarkoi</i> $\sim$                               | <i>tarkoi</i> $\sim$                                                                                                                                                            | <i>tullut</i> $\mathbf{X}\sim$                                                                                      |
| <i>αυθο</i>                                                              | <i>ταλλ</i>                                                                           | <i>μεᾱvi</i>                                      | <i>μεᾱvi</i>                                                                                                                                                                   | <i>tuli</i>                                                                                                         |
| <i>usko</i> $\sim$                                                       | <i>uu</i> ( <i>de</i>   <i>si</i> ) <i>m</i> ( <i>m</i>   <i>p</i> ) $\mathbf{X}\sim$ | <i>vaikut</i> ( $\text{o} \text{t}$ ) $\mathbf{X}$ | <i>val</i> ( <i>l</i>   <i>t</i> ) $\mathbf{X}^{\epsilon}$ ( <i>a</i>   <i>o</i> )                                                                                              | <i>valli</i> $\sim$                                                                                                 |
| <i>φαθο</i>                                                              | <i>uusi</i>                                                                           | <i>infl</i>                                        | <i>γawlt</i> $\mathbf{X}$                                                                                                                                                       | <i>δομ̄vi</i>                                                                                                       |
| <i>vuosi</i> ( <i>teen</i>   <i>tena</i>   <i>tt</i> )                   | <i>yh</i> ( <i>d</i>   <i>t</i> ) $\sim$                                              | <i>miss</i>                                        | <i>nai</i> ( $\text{o} \text{si} \text{va}$ )( $\text{o} \text{n} \text{t}$ )( $\text{o} \text{e} \text{ut}$ )( $\text{o} \text{e} \text{t} \text{mme} \text{tte} \text{vat}$ ) |                                                                                                                     |
| <i>jahpi</i>                                                             | <i>yks</i>                                                                            | <i>neiti</i>                                       | <i>μαρρ</i>                                                                                                                                                                     |                                                                                                                     |
| <i>uusitte</i>                                                           | <i>vuonna</i>                                                                         | <i>~aikoi</i>                                      | <i>~käyt</i> ( <i>in</i>   <i>te</i> )                                                                                                                                          | <i>~käyttäy</i> ( <i>d</i>   <i>t</i> ) $\mathbf{X}$                                                                |
| <i>uusi</i>                                                              | <i>jahr</i>                                                                           | <i>aio</i>                                         | <i>käy</i>                                                                                                                                                                      | <i>baχs</i>                                                                                                         |
|                                                                          |                                                                                       |                                                    |                                                                                                                                                                                 | <i>~vuode</i> ( <i>ksi</i>   <i>lla</i>   <i>lle</i>   <i>lta</i>   <i>n</i>   <i>ssa</i>   <i>sta</i>   <i>t</i> ) |
|                                                                          |                                                                                       |                                                    |                                                                                                                                                                                 | <i>jahr</i>                                                                                                         |

- (5) Replace

|                                                                                            |                                                                                         |                                                                                                 |
|--------------------------------------------------------------------------------------------|-----------------------------------------------------------------------------------------|-------------------------------------------------------------------------------------------------|
| $(\text{mamm} \text{muts} \ddot{a} \text{ip} \ddot{a} \text{ipp} \ddot{a} \text{isk})\sim$ | $\mathbf{X}^{\epsilon}(\mathbf{V} \text{s})\text{tapa}$                                 | $\mathbf{X}^{\epsilon}(\text{o} \text{l} \ddot{a} \text{hi})\text{omai}(\text{n} \text{s})\sim$ |
| <i>äit</i>                                                                                 | <i>Xtava</i>                                                                            | <i>Xpeltβa</i>                                                                                  |
| $\mathbf{X}^{\epsilon}(\text{o} \text{i} \text{ko})\text{lu}(\text{e} \text{i})\sim$       | <i>ahdist</i>                                                                           | <i>aiko</i> $\sim$                                                                              |
| <i>Xluki</i>                                                                               | <i>αγιστ</i>                                                                            | <i>aio</i>                                                                                      |
| <i>har</i> ( <i>r</i>   <i>t</i> ) $\sim$                                                  | <i>harm</i> $\sim$                                                                      | <i>harv</i> $\sim$                                                                              |
| <i>δowt</i>                                                                                | <i>hram</i>                                                                             | <i>παρ</i>                                                                                      |
| <i>juo</i> ( <i>ks</i>   <i>sk</i>   <i>ss</i> ) $\sim$                                    | <i>kahv</i>                                                                             | <i>kakist</i> $\sim$                                                                            |
| <i>juost</i>                                                                               | <i>kofφ</i>                                                                             | <i>kof</i>                                                                                      |
| <i>kitty</i> $\sim$                                                                        | <i>ko</i> ( <i>d</i>   <i>t</i> )( <i>e</i>   <i>i</i> )                                | <i>kohtalo</i>                                                                                  |
| <i>κιττυ</i>                                                                               | <i>κοτι</i>                                                                             | <i>φατο</i>                                                                                     |
| <i>loist</i> $\sim$                                                                        | <i>lom</i> $\sim$                                                                       | <i>luist</i> $\sim$                                                                             |
| <i>σiηiṽ</i>                                                                               | <i>ηολδ</i>                                                                             | <i>σιλδ</i>                                                                                     |
| <i>mail</i> ( <i>e</i>   <i>e</i>   <i>e</i>   <i>ja</i>   <i>i</i> ) $\sim$               | <i>mai</i> ( <i>n</i>   <i>n</i>   <i>n</i>   <i>t</i>   <i>ts</i>   <i>tt</i> ) $\sim$ | <i>mary</i> $\sim$                                                                              |
| <i>μαυλι</i>                                                                               | <i>με̄ντζιον</i>                                                                        | <i>μαρρ</i>                                                                                     |
| <i>nai</i> ( <i>d</i>   <i>k</i>   <i>m</i>   <i>t</i> ) $\sim$                            | <i>nei</i> ( <i>d</i>   <i>t</i> ) <i>o</i>                                             | <i>oiv</i> ( <i>a</i>   <i>i</i> ) $\sim$                                                       |
| <i>μαρρ</i>                                                                                | <i>μαιδο</i>                                                                            | <i>φῑva</i>                                                                                    |
| <i>pisi</i> ( <i>mm</i>   <i>mp</i>   <i>n</i>   <i>nt</i> ) $\sim$                        | <i>pitk</i> $\mathbf{X}^{\epsilon}$ ( <i>i</i>   <i>ä</i> ) $\sim$                      | <i>pitu</i> $\sim$                                                                              |
| <i>λο̄γγ</i>                                                                               | <i>λο̄γγX</i>                                                                           | <i>λο̄γγυ</i>                                                                                   |
|                                                                                            | <i>puh</i> ( <i>d</i>   <i>t</i> )                                                      | <i>puisto</i>                                                                                   |
|                                                                                            | <i>puh</i> ( <i>d</i>   <i>t</i> )                                                      | <i>puisto</i>                                                                                   |
|                                                                                            | <i>päiv</i> älli $\sim$                                                                 | <i>sa</i> ( <i>d</i>   <i>t</i> )( <i>a</i>   <i>e</i>   <i>oi</i> ) $\sim$                     |
|                                                                                            | <i>δῑvep̄lli</i>                                                                       | <i>ραῑva</i>                                                                                   |

|                                           |                                |                                   |                        |                        |                    |                            |                   |                  |              |               |
|-------------------------------------------|--------------------------------|-----------------------------------|------------------------|------------------------|--------------------|----------------------------|-------------------|------------------|--------------|---------------|
| <i>sal(e e e ja i)</i>                    | <i>seitsem~</i>                | <i>selk~</i>                      | <i>seurustel</i>       | <i>sie(d)t~</i>        | <i>siev(i ä)~</i>  | <i>suvai(n nn t ts tt)</i> |                   |                  |              |               |
| ζαλι                                      | 7em                            | sel                               | σocl                   | σotd                   | περτι              | τολpat                     |                   |                  |              |               |
| <i>säily~</i>                             | <i>sääst~</i>                  | <i>tahd</i>                       | <i>talou</i>           | <i>tapa~</i>           | <i>tapp~</i>       | <i>tee~</i>                | <i>tilan(n)t~</i> | <i>to(de si)</i> |              |               |
| rämÿy                                     | σavat                          | taht                              | εεκωu                  | tava                   | κιλ                | ξai                        | σιtyn             | totta            |              |               |
| <i>tuha(n nn nt t tt)</i>                 | <i>tulk<sub>χ̂</sub>(a o)~</i> | <i>tun(n t)(e i en ev u)(∅ u)</i> | <i>tunti(n s)</i>      | <i>turh~</i>           | <i>tyt(∅ t)är~</i> |                            |                   |                  |              |               |
| θat                                       | τυλκκχ̂                        | tuntea                            | τuntis                 | ῥιlh                   | δοχτρ              |                            |                   |                  |              |               |
| <i>tyt(∅ t)ö~</i>                         | <i>tädi~</i>                   | <i>tänään~</i>                    | <i>vapi~</i>           | <i>varh</i>            | <i>varm</i>        | <i>vel(∅ k)(a o)</i>       | <i>veli~</i>      | <i>vih(∅ k)i</i> | <i>ylell</i> | <i>ylist~</i> |
| γiρlö                                     | täti                           | τοδηan                            | vavi                   | εαrλh                  | κυσρ               | δεβτα                      | veljen            | μαρpi            | luxll        | πυραzs        |
| <i>aie(∅ tta)</i>                         | <i>eilen</i>                   | <i>enoX</i>                       | <i>huomen(issa na)</i> | <i>leskirouvX</i>      | <i>nainen</i>      |                            |                   |                  |              |               |
| aike                                      | eilinen                        | ῥοκλο                             | τομρωω                 | leski                  | naisen             |                            |                   |                  |              |               |
| <i>~aik(a aa oi ojen)(∅ in n na neen)</i> | <i>~kaunis</i>                 | <i>~käytä(∅ mmel tte)</i>         | <i>~käytös(∅ ten)</i>  | <i>~varu(ks s st)X</i> | <i>~veli</i>       |                            |                   |                  |              |               |
| aja                                       | kaunii                         | υσά                               | βαχs                   | κιβmt                  | veljen             |                            |                   |                  |              |               |

## (6) Replace

|                                  |                                            |                                |                     |                            |                     |                                                       |               |                                             |              |                |                  |
|----------------------------------|--------------------------------------------|--------------------------------|---------------------|----------------------------|---------------------|-------------------------------------------------------|---------------|---------------------------------------------|--------------|----------------|------------------|
| <i>(hyv parah paras parh)~</i>   | <b>V'</b>                                  | <b>X<sup>ε</sup>(y ö öiC)~</b> | <i>é</i>            | <i>hdeks</i>               | <i>herist~</i>      | <i>hert~</i>                                          | <i>herä~</i>  | <i>huom~</i>                                | <i>ilo~</i>  | <i>inh~</i>    |                  |
| parempi                          | <b>VQ</b>                                  | <b>qX</b>                      | e                   | hdex                       | ξak                 | σewt                                                  | ωakä          | σim                                         | ilzo         | inzh           |                  |
| <i>is(i ä)~</i>                  | <i>jano~</i>                               | <i>juo(k s)C~</i>              | <i>kirje~</i>       | <i>kuum~</i>               | <i>lm</i>           | <i>miel</i>                                           | <i>sall~</i>  | <i>sellai<sup>X<sup>ε</sup></sup>(n s)~</i> | <i>siro~</i> | <i>siskoX~</i> | <i>toi(m nt)</i> |
| faija                            | γiano                                      | qojo                           | girje               | guum                       | λμ                  | miel                                                  | sallq         | zenlaiX                                     | σiro         | sisar          | ηοβ              |
| <i>toiv~</i>                     | <i>tun(n t)(e j i)<sub>χ̂</sub>(e s)</i>   | <i>tunne(i r)</i>              | <i>tunnis(s t)a</i> | <i>tuntei(hin na neen)</i> | <i>tuom(∅ ar)i~</i> |                                                       |               |                                             |              |                |                  |
| χοπ                              | τuntiχ̂                                    | τunti                          | τunti               | τunti                      | δομι                |                                                       |               |                                             |              |                |                  |
| <i>vaj~</i>                      | <i>ystäv(∅ yks yst)(∅ i)~</i>              | <i>hra</i>                     | <i>nti</i>          | <i>rva</i>                 | <i>~(∅ si)tte</i>   | <i>~X<sup>ε</sup>(χ̂<sub>m</sub>)zχ̂<sub>m0</sub></i> | <i>~C'X</i>   |                                             |              |                |                  |
| waj                              | ystew                                      | herra                          | neiti               | rouva                      | ∅                   | χ̂z                                                   | C             |                                             |              |                |                  |
| <i>~X<sup>ε</sup>(l s)k(o ö)</i> | <i>~X<sup>ε</sup>(u y)(ksin s tta ttä)</i> | <i>~ej(a ä)</i>                | <i>~et</i>          | <i>~isk(aa ää)</i>         | <i>~lleen</i>       | <i>~mies</i>                                          | <i>~tunti</i> |                                             |              |                |                  |
| X                                | Xd                                         | e                              | etkin               | isk                        | ll                  | mieh                                                  | τunti         |                                             |              |                |                  |
| <i>(hyv parah paras parh)~</i>   | <b>V'</b>                                  | <b>X<sup>ε</sup>(y ö öiC)~</b> | <i>é</i>            | <i>hdeks</i>               | <i>herist~</i>      | <i>hert~</i>                                          | <i>herä~</i>  | <i>huom~</i>                                | <i>ilo~</i>  | <i>inh~</i>    |                  |
| parempi                          | <b>VQ</b>                                  | <b>qX</b>                      | e                   | hdex                       | ξak                 | σewt                                                  | ωakä          | σim                                         | ilzo         | inzh           |                  |
| <i>is(i ä)~</i>                  | <i>jano~</i>                               | <i>juo(k s)C~</i>              | <i>kirje~</i>       | <i>kuum~</i>               | <i>lm</i>           | <i>miel</i>                                           | <i>sall~</i>  | <i>sellai<sup>X<sup>ε</sup></sup>(n s)~</i> | <i>siro~</i> | <i>siskoX~</i> | <i>toi(m nt)</i> |
| faija                            | γiano                                      | qojo                           | girje               | guum                       | λμ                  | miel                                                  | sallq         | zenlaiX                                     | σiro         | sisar          | ηοβ              |
| <i>toiv~</i>                     | <i>tun(n t)(e j i)<sub>χ̂</sub>(e s)</i>   | <i>tunne(i r)</i>              | <i>tunnis(s t)a</i> | <i>tuntei(hin na neen)</i> | <i>tuom(∅ ar)i~</i> |                                                       |               |                                             |              |                |                  |
| χοπ                              | τuntiχ̂                                    | τunti                          | τunti               | τunti                      | δομι                |                                                       |               |                                             |              |                |                  |
| <i>vaj~</i>                      | <i>ystäv(∅ yks yst)(∅ i)~</i>              | <i>hra</i>                     | <i>nti</i>          | <i>rva</i>                 | <i>~(∅ si)tte</i>   | <i>~X<sup>ε</sup>(χ̂<sub>m</sub>)zχ̂<sub>m0</sub></i> | <i>~C'X</i>   |                                             |              |                |                  |
| waj                              | ystew                                      | herra                          | neiti               | rouva                      | ∅                   | Xz                                                    | C             |                                             |              |                |                  |
| <i>~X<sup>ε</sup>(l s)k(o ö)</i> | <i>~X<sup>ε</sup>(u y)(ksin s tta ttä)</i> | <i>~ej(a ä)</i>                | <i>~et</i>          | <i>~isk(aa ää)</i>         | <i>~lleen</i>       | <i>~mies</i>                                          | <i>~tunti</i> |                                             |              |                |                  |
| X                                | Xd                                         | e                              | etkin               | isk                        | ll                  | mieh                                                  | τunti         |                                             |              |                |                  |

- (7) If the result so far start with **C<sub>m</sub>VV~** (where the two occurrences of **V** may or may not represent the same vowel), perform the following replacements on the word initial pattern **C<sub>m</sub>VV~**.<sup>98</sup>

|                          |                               |             |             |             |
|--------------------------|-------------------------------|-------------|-------------|-------------|
| $\xi^{\in}(\mathbf{V})i$ | <b>V**</b>                    | <i>ie</i>   | <i>uo</i>   | <i>yö</i>   |
| $\xi j \xi i$            | <b>(V**)<sup>(1)</sup>iji</b> | <i>eije</i> | <i>oijo</i> | <i>öijö</i> |

If the result after step (6) does not start with **C<sub>m</sub>VV~**, leave it as is.

- (8) Mark the first protected range with †.
- (9) Replace

|                                                                                               |
|-----------------------------------------------------------------------------------------------|
| $\sim X^{\in}((a e i n o t u y ä ö)(\emptyset \dagger))(han hän kaan kään kin ko kö pa pä)_m$ |
| <b>X</b>                                                                                      |

<sup>98</sup>Here, the two instances of  $\xi$  in  $\xi j \xi i$  represent the same letter; **(V\*\*)<sup>(1)</sup>iji** stands the first letter in the long vowel **V\*\***, followed immediately by *iji*.

$$\sim(\emptyset|s)(iess(a|\ddot{a})|k(aa|\ddot{a}))(\emptyset|mme)k(oo|\ddot{o}\ddot{o})(n|t)|minen|nee(\emptyset|t)|n(e|u|y)|t|si(mme|n|t)|tt(aessa|\ddot{a}ess|\ddot{a}iss|\ddot{a}i|aman|\ddot{a}m|\ddot{a}n|ane|\ddot{a}ne|aneen|\ddot{a}neen|\ddot{a}i|u|y))v(a|\ddot{a}|at|\ddot{a}t)$$

$$\sim\ddagger\mathbf{X}(l|v)(a|\ddot{a})i(n|s)\hat{\chi}_{m_0}$$

$$\ddagger\mathbf{X}$$

$$\sim\ddagger\mathbf{X}hk\hat{\chi}_{m_0}$$

$$\ddagger\mathbf{X}$$

$$\sim\ddagger\mathbf{X}lli(n|s)\hat{\chi}_{m_0}$$

$$\ddagger\mathbf{X}$$

$$\sim\ddagger\mathbf{X}luont(a|e)\hat{\chi}_{m_0}$$

$$\ddagger\mathbf{X}$$

$$\sim\ddagger\mathbf{X}suh(d|t)\hat{\chi}_{m_0}$$

$$\ddagger\mathbf{X}$$

$$\sim\ddagger\mathbf{X}t(a|\ddot{a})r\hat{\chi}_{m_0}$$

$$\ddagger\mathbf{X}$$

(10) Mark the second protected range with  $\ddagger$ .

(11) Do  $\sim\ddagger\mathbf{X}sti \rightarrow \ddagger\mathbf{X}$ ,  $\sim\ddagger\mathbf{X}'(ks|ll|lt|s|st)\mathbf{X}'' \rightarrow \ddagger\mathbf{X}'$ ,  $(k\ddagger s|l\ddagger l|l\ddagger t|s\ddagger s|s\ddagger t)\mathbf{X}''' \rightarrow \emptyset$ .

(12) Do  $\ddagger \rightarrow \emptyset$ .

(13) Replace

$$\sim\ddagger it$$

$$i$$

$$\sim\ddagger\mathbf{X}Cit$$

$$\ddagger\mathbf{X}Ci$$

$$\sim\ddagger\mathbf{X}(mme|nne|nsa|ns\ddot{a})$$

$$\ddagger\mathbf{X}$$

$$\sim\ddagger\mathbf{X}_{\hat{\chi} \notin}(k)si$$

$$\ddagger\mathbf{X}\hat{\chi}$$

$$\sim\ddagger\mathbf{X}^{\mathbf{X}_1 \in}(\emptyset|kse)ni$$

$$\sim\ddagger\mathbf{X}\mathbf{X}'_1$$

$$\sim\mathbf{X}_2 \in ((\ddagger\mathbf{X}(in|ll))|i\ddagger n|l\ddagger l)een$$

$$\mathbf{X}_2e$$

$$\sim\mathbf{X}_3 \in ((\ddagger\mathbf{X}(ll|lt|n|s|s|st|t))|l\ddagger l|l\ddagger t|n\ddagger s\ddagger s|s\ddagger t|t\ddagger t)\mathbf{X}_4 \in (aa|\ddot{a}\ddot{a})n$$

$$\mathbf{X}_3\mathbf{X}_4^{(1)}$$

where one obtains  $\mathbf{X}'_1$  after doing  $kse \rightarrow ksi$  on  $\mathbf{X}_1$ .

(14) Do  $\ddagger \rightarrow \emptyset$ .

(15) Do  $mai\sim \rightarrow \varepsilon\alpha\rho\theta$ ,  $mm^{\hat{\chi} \in}(a|\ddot{a})(\emptyset|n) \rightarrow M\hat{\chi}$ ,  $sisar\sim \rightarrow \sigma i\sigma\alpha\rho$ ,  $\tau\nu\tau-j\mathbf{V}_m \rightarrow \tau\nu\tau-Z\mathbf{V}_m$ ,  $\tau\nu\tau-k\ddot{a}y \rightarrow \tau\nu\tau-kk\ddot{a}y$ ,  $\sim nt(a|\ddot{a}) \rightarrow nt$ ,  $\sim x(a|\ddot{a})s \rightarrow x$ ,  $\underline{kahdexi} \rightarrow kaks i$ .

**Algorithm 8.6** (Finnish essential root). Let  $\hat{\sigma}$  be the effective spelling of a Finnish word, then its corresponding essential root  $\text{EssRoot}(\hat{\sigma})$  is constructed in the following steps:

(1) Mark the first protected range with  $\ddagger$ .

(2) Do  $\sim\ddagger\mathbf{X}\hat{\xi}h\hat{\xi}n \rightarrow \ddagger\mathbf{X}\hat{\xi}^*$  if  $\hat{\xi} \in \{a, e, i, o, u, \ddot{a}, \ddot{o}\}$ . Make the following replacements in the same sweep:

$$\sim\ddagger\mathbf{X}\mathbf{V}^*i(den|siin|tten)$$

$$\ddagger\mathbf{X}\mathbf{V}^*i^*$$

$$\sim\mathbf{X}_1 \in (\ddagger\mathbf{X}(\mathbf{V}^{**}|(a|\ddot{a})k))seen$$

$$\mathbf{X}'_1^*$$

$$\sim\mathbf{X}_2 \in (\ddagger\mathbf{X}\mathbf{C}\mathbf{V}|\mathbf{C}\ddagger\mathbf{V})(\emptyset|ej)(a|\ddot{a})$$

$$\mathbf{X}_2^*$$

$$\sim\ddagger\mathbf{X}\mathbf{V}tt(a|\ddot{a})$$

$$\ddagger\mathbf{X}\mathbf{V}^*$$

$$\sim\ddagger\mathbf{X}(ine|ksi|ll(a|\ddot{a}|e)|lt(a|\ddot{a})|n(a|\ddot{a})|ss(a|\ddot{a})|st(a|\ddot{a}))$$

$$\ddagger\mathbf{X}^*$$

$$\sim\mathbf{X}_3 \in (\ddagger\mathbf{X})n$$

$$\ddagger\mathbf{X}'_3^*$$

where one constructs  $\mathbf{X}'_1$  by doing  $\sim(a|\ddot{a})k \rightarrow \emptyset$  on  $\mathbf{X}_1$ , and  $\mathbf{X}'_3$  by doing  $\sim\mathbf{X} \in (aa|ee|ie|i|oo|uu|\ddot{a}\ddot{a}|\ddot{o}\ddot{o}) \rightarrow \mathbf{X}^{(1)}$  on  $\mathbf{X}_3$ .

(3) Do  $\sim\ddagger\mathbf{X}(m(a|\ddot{a})(\emptyset|isi)|m(ato|\ddot{a}t\ddot{o})|mi|ne|t(a|\ddot{a})|tt(a|\ddot{a})i) \rightarrow \ddagger\mathbf{X}^*$ .

(4) Mark the second protected range with  $\ddagger$ .

(5) If the result so far does not end with  $*$ , append a symbol  $\#$  at the end of the string.

(6) Replace

$$\sim\ddagger\mathbf{X}i(M|mp)(a|\ddot{a})$$

$$\ddagger\mathbf{X}$$

$$\sim\ddagger\mathbf{X}(M|mp)(a|\ddot{a})$$

$$\ddagger\mathbf{X} \text{ if } \mathbf{X} \text{ does not end with } \sim po$$

(7) Replace

$$\sim\ddagger(\hat{\chi}|\ddagger)_{m_0}(i|j)^*$$

$$\ddagger(\hat{\chi}|\ddagger)_{m_0}^*$$

$$\sim\mathbf{X} \in (\ddagger(\hat{\chi}|\ddagger)_{m_0}\mathbf{V}|\mathbf{V}(\ddagger|\ddagger)_m)t(\emptyset|\ddagger)\#$$

$$\mathbf{X}_\tau$$

(8) If the pattern  $\sim\ddagger\mathbf{X}Ma\tau$  is found, replace it with  $\ddagger\mathbf{X}'$ . Here,  $\mathbf{X}'$  is obtained by removing  $\sim(\emptyset|i)Ma$  from  $\mathbf{X}Ma$  if  $\mathbf{X}$  does not end with  $\sim po$ ; otherwise, set  $\mathbf{X}'$  as  $\mathbf{X}Ma$ .

(9) Do  $(\ddagger|\#|\#|\tau) \rightarrow \emptyset$ .

(10)  $Do \sim \dagger \mathbf{XV}^{**} \rightarrow \dagger \mathbf{X}(\mathbf{V}^{**})^{[1]}$ .

(11)  $Do \sim \dagger \mathbf{XC}(a|e|i|\ddot{a}) \rightarrow \dagger \mathbf{XC}$ .

(12)  $Do \sim \dagger \mathbf{X}^{\hat{\chi} \in (o|u)}j \rightarrow \dagger \mathbf{X}\hat{\chi}$ .

(13)  $Do \sim \dagger \mathbf{X}_1 i(l)_m \mathbf{X}_2 \rightarrow \dagger \mathbf{X}_1, \sim \dagger \mathbf{XCit} \rightarrow \dagger \mathbf{XCi}, \sim \dagger \mathbf{Xjo} \rightarrow \dagger \mathbf{Xj}, \sim \dagger \mathbf{Xks} \rightarrow \dagger \mathbf{Xd}, \sim \dagger \mathbf{X}(st|ts) \rightarrow \dagger \mathbf{X}$ .

(14)  $Do \dagger \rightarrow \emptyset$ .

(15) *Replace*

|          |          |                           |                            |                                                                          |                      |                      |             |           |
|----------|----------|---------------------------|----------------------------|--------------------------------------------------------------------------|----------------------|----------------------|-------------|-----------|
| $ng$     | $nk$     | $kah(\emptyset d dest t)$ | $k\ddot{a}(v y)\mathbf{X}$ | $n\ddot{a}(e emm en et h hk\ddot{o} ht hty ij\ddot{a} ij\ddot{a} ke ki)$ | $tun(\emptyset n s)$ | $vase(\emptyset nt)$ | $\sim oi$   | $\sim ti$ |
| $\gamma$ | $\kappa$ | $kaks$                    | $k\ddot{a}y$               | $n\ddot{a}hd$                                                            | $tunt$               | $vaseM$              | $\emptyset$ | $t$       |

(16)  $Do \hat{\chi}_{\times 2} \rightarrow \hat{\chi}^+$ , that is, replace all double letters by the capital form of the corresponding single letter.

(17)  $Do U(d|t) \sim \rightarrow Usi, \sim \hat{\chi}(U|Y)(\emptyset|d|s|t) \rightarrow \hat{\chi}, \underline{Us} \rightarrow Usi$ .

For clustering purposes, we will also define an operation to undouble final consonants in the effective spelling of a Finnish word.

**Algorithm 8.7** (Reduction of Final Double Consonants). *Let  $\hat{\sigma}$  be the effective spelling of a Finnish word, then  $\text{UndCons}(\hat{\sigma})$  is defined by the following procedure:*

- Look for the pattern  $\sim \hat{\chi}_{\times 2} \mathbf{V}_{m_0}$  in  $\hat{\sigma}$ .
- If the pattern is not found or if  $\hat{\chi}$  is one of the Finnish vowels  $\{a, e, i, o, u, y, \ddot{a}, \ddot{o}\}$ , do nothing; otherwise, replace the pattern by  $\hat{\chi} \mathbf{V}_{m_0}$ .

### 8.1.2 Admissible mutation and approximate clustering

**Algorithm 8.8** (Simple heredity test). *Construct  $\hat{\alpha}'$  by doing  $\sim(d|e|i|n|t|v) \rightarrow \emptyset$  on  $\hat{\alpha}$ . Define  $\hat{\beta}'$  similarly. The Boolean-valued function  $\text{SimpHrdTest}(\hat{\alpha}, \hat{\beta})$  returns **TRUE** if the lowercase form of  $\hat{\alpha}$  contains at least one instance of  $\{a, e, i, o, u, y, \ddot{a}, \ddot{o}\}$  **AND** at least one of the following three conditions holds:<sup>99</sup>*

- $\hat{\alpha} = \hat{\beta}$ ;
- $\hat{\alpha}' = \hat{\beta}'$ ;
- $\ell(\hat{\beta}) > \ell(\hat{\alpha}) \geq \frac{\ell(\hat{\beta})}{2}$  **AND**  $\hat{\beta} = \hat{\alpha} \mathbf{VX}$ .

In what follows, we define  $\text{SuffixNW}(\hat{\alpha}, \hat{\beta}), \text{RootNW}(\hat{\alpha}, \hat{\beta}), \text{NW}^*(\hat{\alpha}, \hat{\beta})$  and  $\text{SuffixSW}(\hat{\alpha}, \hat{\beta}), \text{SuffixSW}'(\hat{\alpha}, \hat{\beta}), \text{SW}^*(\hat{\alpha}, \hat{\beta})$  as what is done in the Danish case (Algorithm 5.7), which was also applied to two other Germanic languages treated in §5.

Consonant gradations refer to consonant mutation patterns found in Finnish and its close relative, Estonian. (While Hungarian is also a Uralic language, it does not exhibit systematic consonant mutations as in Finnish.) In order to accommodate to this particular feature of Finnish, we need to define admissible consonant alternation patterns in Finnish effective spellings and essential roots.

**Definition 8.9** (Finnish consonant gradations). Define  $\mathbb{G} = [\emptyset, \emptyset][[k, \emptyset][[k, j][[k, Q][[k, v][[K, k][[L, l][[L, lt][[M, mp][[mp, nt][[N, n][[N, nt][[p, v][[P, p][[R, r][[R, rt][[s, d][[s, t][[S, s][[S, st][[t, d][[t, s][[T, s][[T, t][[\kappa, \gamma]$  as admissible Finnish consonant gradations.

**Algorithm 8.10** (Admissible suffix mismatch and vowel alternation). *For two strings  $\hat{\alpha}$  and  $\hat{\beta}$ , the Boolean-valued function*

$$\text{AdmMut}(\text{RootNW}(\hat{\alpha}, \hat{\beta}), \text{SuffixNW}(\hat{\alpha}, \hat{\beta}), \text{NW}^*(\hat{\alpha}, \hat{\beta}))$$

*returns **TRUE** if at least one of the following three conditions holds:*

- $\text{SuffixNW}(\hat{\alpha}, \hat{\beta}) = [\emptyset|h|\mathbf{V}_m, \emptyset|h|\mathbf{V}_m]$  **AND**  $(\text{NW}^*(\hat{\alpha}, \hat{\beta}) = \mathbb{G} \text{ OR } \text{NW}^*(\hat{\beta}, \hat{\alpha}) = \mathbb{G} \text{ OR } (\text{NW}^*(\hat{\alpha}, \hat{\beta}) = \emptyset \text{ AND the lowercase form of } \text{RootNW}(\hat{\alpha}, \hat{\beta}) \text{ contains at least one instance of } \mathbf{V}))$ ;
- $\text{NW}^*(\hat{\alpha}, \hat{\beta}) = \emptyset$  **AND**  $\text{SuffixNW}'(\hat{\alpha}, \hat{\beta}) = \mathbb{G}[a, o][[m, nt][[n, t]$ , where one obtains  $\text{SuffixNW}'(\hat{\alpha}, \hat{\beta})$  by doing  $\sim(h|s|\mathbf{V}_m) \rightarrow \emptyset$  on both components of  $\text{SuffixNW}(\hat{\alpha}, \hat{\beta})$ ;

<sup>99</sup>As a general rule in this document, the truth values of items labeled with Roman numerals are connected to each other with logical **OR**.

- (iii)  $NW^*(\hat{\alpha}, \hat{\beta}) = \emptyset$  **AND**  $\text{SuffixNW}''(\hat{\beta}, \hat{\alpha}) = \mathbb{G}$ , where  $\text{SuffixNW}''(\hat{\beta}, \hat{\alpha})$  results from doing  $\sim(h|\mathbf{V}_m) \rightarrow \emptyset$  on both components of  $\text{SuffixNW}(\hat{\beta}, \hat{\alpha})$ .

Similarly, one can evaluate another Boolean-valued function

$$\text{AdmMut}(\text{RootSW}(\hat{\alpha}, \hat{\beta}), \text{SuffixSW}(\hat{\alpha}, \hat{\beta}), \text{SW}^*(\hat{\alpha}, \hat{\beta}))$$

by trading all the occurrences of NW in the statements above with SW.

The following heredity test function is very similar to the German version (Algorithm ), except that we additionally require that the two strings in question must start with the same letter — constant gradations do not apply to the initial consonants.

**Algorithm 8.11** (Heredity test function). *In what follows,  $\ell([\hat{\sigma}, \hat{\tau}]) = \min\{\ell(\hat{\sigma}), \ell(\hat{\tau})\}$ . For two strings  $\hat{\alpha}$  and  $\hat{\beta}$ , the Boolean-valued function  $\text{HrdTest}(\hat{\alpha}, \hat{\beta})$  returns **TRUE** if at least one of the following three conditions holds:*

- (i)  $\text{SimpHrdTest}(\hat{\alpha}, \hat{\beta}) = \mathbf{TRUE}$ ;
- (ii)  $\ell(\text{RootNW}(\hat{\alpha}, \hat{\beta})) + \ell(\text{SuffixNW}(\hat{\alpha}, \hat{\beta})) + \ell(\text{NW}^*(\hat{\alpha}, \hat{\beta})) \geq \frac{\max\{\ell(\hat{\alpha}), \ell(\hat{\beta})\}}{2}$  **AND**  $\text{AdmMut}(\text{RootNW}(\hat{\alpha}, \hat{\beta}), \text{SuffixNW}(\hat{\alpha}, \hat{\beta}), \text{NW}^*(\hat{\alpha}, \hat{\beta})) = \mathbf{TRUE}$  **AND** both  $\hat{\alpha}$  and  $\hat{\beta}$  start with the same letter;
- (iii)  $\ell(\text{RootSW}(\hat{\alpha}, \hat{\beta})) + \ell(\text{SuffixSW}(\hat{\alpha}, \hat{\beta})) + \ell(\text{SW}^*(\hat{\alpha}, \hat{\beta})) \geq \frac{\max\{\ell(\hat{\alpha}), \ell(\hat{\beta})\}}{2}$  **AND**  $\text{AdmMut}(\text{RootSW}(\hat{\alpha}, \hat{\beta}), \text{SuffixSW}(\hat{\alpha}, \hat{\beta}), \text{SW}^*(\hat{\alpha}, \hat{\beta})) = \mathbf{TRUE}$  **AND** both  $\hat{\alpha}$  and  $\hat{\beta}$  start with the same letter.

**Algorithm 8.12** (Approximate clustering of Finnish words). *The approximate clustering of a list of Finnish words  $\{\hat{\alpha}_1, \dots, \hat{\alpha}_N\}$  is completed in two stages:*

- (1) *We sort the list  $\{(\hat{\alpha}_1, \text{EffSpell}(\hat{\alpha}_1), \text{UndCons}(\text{EffSpell}(\hat{\alpha}_1))), \dots, (\hat{\alpha}_N, \text{EffSpell}(\hat{\alpha}_N), \text{UndCons}(\text{EffSpell}(\hat{\alpha}_N)))\}$  alphabetically according to the third component (with higher priority) and the second component (with lower priority). If two consecutive neighbors in the alphabetized list  $\{(\hat{\alpha}_{(1)}, \text{EffSpell}(\hat{\alpha}_{(1)}), \text{UndCons}(\text{EffSpell}(\hat{\alpha}_{(1)}))), \dots, (\hat{\alpha}_{(N)}, \text{EffSpell}(\hat{\alpha}_{(N)}), \text{UndCons}(\text{EffSpell}(\hat{\alpha}_{(N)})))\}$  satisfies both  $\text{HrdTest}(\text{EffSpell}(\hat{\alpha}_{(n)}), \text{EffSpell}(\hat{\alpha}_{(n+1)})) = \mathbf{FALSE}$  and  $\text{HrdTest}(\text{EffSpell}(\hat{\alpha}_{(n+1)}), \text{EffSpell}(\hat{\alpha}_{(n)})) = \mathbf{FALSE}$ , where  $n \in \mathbb{Z} \cap [1, N)$ , then add a demarcation line between these two entries. In this way, the alphabetized list is divided into separate groups of words with tags:  $\{g_1 = \{(\hat{\alpha}_{(1,1)}, \text{EffSpell}(\hat{\alpha}_{(1,1)}), \dots), \dots, (\hat{\alpha}_{(1,n_1)}, \text{EffSpell}(\hat{\alpha}_{(1,n_1)}), \dots)\}, \dots, g_M = \{(\hat{\alpha}_{(M,1)}, \text{EffSpell}(\hat{\alpha}_{(M,1)}), \dots), \dots, (\hat{\alpha}_{(M,n_M)}, \text{EffSpell}(\hat{\alpha}_{(M,n_M)}), \dots)\}$ , where each sublist also preserves alphabetic order. In particular, we have  $\hat{\alpha}_{(1,1)} = \hat{\alpha}_{(1)}$  and  $\hat{\alpha}_{(M,n_M)} = \hat{\alpha}_{(N)}$ .*
- (2) *For each group of words  $g_m = \{(\hat{\alpha}_{(m,1)}, \text{EffSpell}(\hat{\alpha}_{(m,1)}), \dots, (\hat{\alpha}_{(m,n_m)}, \text{EffSpell}(\hat{\alpha}_{(m,n_m)}))\}$  where  $m \in \mathbb{Z} \cap [1, M]$ , we augment it into a tagged entry  $G_m = (g_m, \text{EffSpell}(\hat{\alpha}_{(m,1)}), \text{EssRoot}(\text{EffSpell}(\hat{\alpha}_{(m,1)})), T_m)$ , where one constructs the tag  $T_m$  from  $\text{EssRoot}(\text{EffSpell}(\hat{\alpha}_{(m,1)}))$  in two steps:*
- *Replace all capital letters (including those in the standard Latin alphabet, as well as  $\ddot{A}$  and  $\ddot{O}$ ) by double letters in lowercase form, and do  $\sim o \rightarrow a$ .*
  - *Apply  $\text{UndCons}$ .*

*The list  $\{G_1, \dots, G_M\}$  is sorted alphabetically, with respect to  $T_m$  (with highest priority),  $\text{EssRoot}(\text{EffSpell}(\hat{\alpha}_{(m,1)}))$  (with medium priority), and  $\text{EffSpell}(\hat{\alpha}_{(m,1)})$  (with lowest priority). If two consecutive neighbors in the alphabetized list  $\{G_{(1)} = (g_{(1)}, \hat{\gamma}'_{(1)}, \hat{\gamma}''_{(1)}, \hat{\gamma}'''_{(1)}), \dots, G_{(M)} = (g_{(M)}, \hat{\gamma}'_{(M)}, \hat{\gamma}''_{(M)}, \hat{\gamma}'''_{(M)})\}$  satisfy*

$$\text{HrdTest}(\hat{\gamma}''_{(m)}, \hat{\gamma}''_{(m+1)}) = \mathbf{FALSE}$$

**AND**

$$\text{HrdTest}(\hat{\gamma}'_{(m)}, \hat{\gamma}'_{(m+1)}) = \mathbf{FALSE}$$

*where  $m \in \mathbb{Z} \cap [1, M)$ , then add a demarcation line between these two entries. In this manner, the alphabetized list  $\{G_{(1)}, \dots, G_{(M)}\}$  is divided into separate groups of tagged clusters  $\{\Gamma_1 = \{G_{(1,1)}, \dots, G_{(1,m_1)}\}, \dots, \Gamma_K = \{G_{(K,1)}, \dots, G_{(1,m_K)}\}\}$ . Finally, generate a list of word clusters  $\{\check{\Gamma}_1 = (\check{G}_{(1,1)}, \dots), \dots, \check{\Gamma}_K = (\check{G}_{(K,1)}, \dots)\}$  by discarding all the tags.*

**Example 8.12.1.** There are 78 inflection classes in the Finnish language, according to the classification scheme of KOTUS ([https://en.wiktionary.org/wiki/Appendix:Finnish\\_nominal\\_inflection](https://en.wiktionary.org/wiki/Appendix:Finnish_nominal_inflection) and [https://en.wiktionary.org/wiki/Appendix:Finnish\\_conjugation](https://en.wiktionary.org/wiki/Appendix:Finnish_conjugation)). Among these classes, the first 51 classes describe nominal declensions (nouns, adjectives and numerals) while the rest are classes for verb conjugations. We pick one representative word from each inflection class, with or without gradation (consonant alternation in the stem).

The KOTUS class number will be shown parenthetically after the English translation for each word family of Finnish nominals below.

*valo, valoa, valoihin, valoiksi, valoilla, valoille, valoilta, valoin, valoina, valoineen, valoissa, valoista, valoitta, valoja, valojen, valoksi, valolla, valolle, valolta, valon, valona, valoon, valossa, valosta, valot, valotta* — “light” (1);

*palvelu, palvelua, palveluiden, palveluihin, palveluiksi, palveluilla, palveluille, palveluilta, palveluin, palveluina, palveluineen, palveluissa, palveluista, palveluita, palveluitta, palveluitten, palveluja, palvelujen, palveluksi, palvelulla, palvelulle, palvelulta, palvelun, palveluna, palvelussa, palvelusta, palvelut, palvelutta, palveluun* — “service” (2);

*valtio, valtioiden, valtioihin, valtioiksi, valtioilla, valtioille, valtioilta, valtiain, valtioina, valtioineen, valtioissa, valtioista, valtioita, valtioitta, valtioitten, valtioksi, valtiolla, valtiolle, valtiolta, valtion, valtiona, valtioon, valtiossa, valtiosta, valtiot, valtiota, valtiotta* — “government” (3);

*laatikko, laatikkoa, laatikkoihin, laatikkoina, laatikkoineen, laatikkoja, laatikkojen, laatikkona, laatikkoon, laatikoiden, laatikoihin, laatikoiksi, laatikoilla, laatikoille, laatikoilta, laatikoin, laatikoissa, laatikoista, laatikoita, laatikoitta, laatikoitten, laatikoksi, laatikolla, laatikolle, laatikolta, laatikon, laatikossa, laatikosta, laatikot, laatikotta* — “box” (4);

*risteihin, risteiksi, risteille, risteillä, risteiltä, ristein, risteineen, risteinä, risteissä, risteistä, risteittä, ristejä, risti, ristien, ristiin, ristiksi, ristille, ristillä, ristiltä, ristin, ristinä, ristissä, rististä, ristiä, ristittä, ristiä* — “cross” (5);

*papereiden, papereihin, papereiksi, papereilla, papereille, papereilta, paperein, papereina, papereineen, papereissa, papereista, papereita, papereitta, papereitten, papereja, paperi, paperia, paperien, paperiin, paperiksi, paperilla, paperille, paperilta, paperin, paperina, paperissa, paperista, paperit, paperitta* — “paper” (6);

*ovea, oveen, oveksi, ovella, ovelle, ovelta, oven, ovena, ovesta, ovesta, ovet, ovetta, ovi, ovia, ovien, oviin, oviksi, ovilla, oville, ovilta, ovin, ovina, ovineen, ovissa, ovista, ovitta* — “door” (7);

*nalle, nallea, nalleen, nalleihin, nalleiksi, nalleilla, nalleille, nalleilta, nallein, nallein, nalleina, nalleineen, nalleissa, nalleista, nalleitta, nalleja, nallejen, nalleksi, nallella, nallelle, nallelta, nallen, nalleina, nalleissa, nallesta, nallet, nalletta* — “teddy bear” (8);

*kala, kalaa, kalaan, kalain, kalaksi, kalalla, kalalle, kalalta, kalan, kalana, kalassa, kalasta, kalat, kalatta, kaloihin, kaloiksi, kaloilla, kaloille, kaloilta, kaloin, kaloina, kaloineen, kaloissa, kaloista, kaloitta, kaloja, kalojen* — “fish” (9);

*koira, koiraa, koiraan, koirain, koiraksi, koiralla, koiralle, koiralta, koiran, koirana, koirassa, koirasta, koirat, koiratta, koiria, koirien, koiriin, koiriksi, koirilla, koirille, koirilta, koirin, koirina, koirineen, koirissa, koirista, koiritta* — “dog” (10);

*omena, omenaa, omenaan, omenain, omenaksi, omenalla, omenalle, omenalta, omenan, omenana, omenassa, omenasta, omenat, omenatta, omenia, omenien, omeniin, omeniksi, omenilla, omenille, omenilta, omenin, omenina, omenineen, omenissa, omenista, omeniitta, omenoiden, omenoihin, omenoiksi, omenoilla, omenoille, omenoilta, omenoin, omenoina, omenoineen, omenoissa, omenoista, omenoita, omenoitta, omenoitten, omenoja, omenojen* — “apple” (11);

*kulkija, kulkijaa, kulkijaan, kulkijain, kulkijaksi, kulkijalla, kulkijalle, kulkijalta, kulkijan, kulkijana, kulkijassa, kulkijasta, kulkijat, kulkijatta, kulkijoiden, kulkijoihin, kulkijoiksi, kulkijoilla, kulkijoille, kulkijoilta, kulkijoin, kulkijoina, kulkijoineen, kulkijoissa, kulkijoista, kulkijoita, kulkijoitta, kulkijoitten* — “traveller” (12);

*katiska, katiskaa, katiskaan, katiskain, katiskaksi, katiskalla, katiskalle, katiskalta, katiskan, katiskana, katiskassa, katiskasta, katiskat, katiskatta, katiskoiden, katiskoihin, katiskoiksi, katiskoilla, katiskoille, katiskoilta, katiskoin, katiskoina, katiskoineen, katiskoissa, katiskoista, katiskoita, katiskoitta, katiskoitten, katiskoja, katiskojen* — “fishtrap” (13);

*solakaksi, solakalla, solakalle, solakalta, solakan, solakassa, solakasta, solakat, solakatta, solakka, solakkaa, solakkaan, solakkain, solakkana, solakkoihin, solakkoina, solakkoineen, solakkoja, solakkojen, solakoiden, solakoihin, solakoiksi, solakoilla, solakoille, solakoilta, solakoin, solakoissa, solakoista, solakoita, solakoitta, solakoitten* — “slender” (14);

*korkea, korkeaa, korkeaan, korkeain, korkeaksi, korkealla, korkealle, korkealta, korkean, korkeana, korkeassa, korkeasta, korkeat, korkeata, korkeatta, korkeiden, korkeihin, korkeiksi, korkeilla, korkeille, korkeilta, korkein, korkeina, korkeine, korkeisiin, korkeissa, korkeista, korkeita, korkeitta, korkeitten* — “tall” (15);

*vanhemaksi, vanhemmalla, vanhemmalle, vanhemmalta, vanhemman, vanhemmassa, vanhemmasta, vanhemmat, vanhemmatta, vanhemmiksi, vanhemmilla, vanhemmille, vanhemmilta, vanhemmin, vanhemmissa, vanhemmista, vanhemmitta, vanhempaa, vanhempaan, vanhempain, vanhempana, vanhempi, vanhempia, vanhempien, vanhempisiin, vanhempina, vanhempine* — “senior” (16);

*vapaa, vapaaksi, vapaalla, vapaalle, vapaalta, vapaan, vapaana, vapaaseen, vapaassa, vapaasta, vapaat, vapaata, vapaatta, vapaiden, vapaihin, vapaiksi, vapailla, vapaille, vapailta, vapain, vapaina, vapaine, vapaisiin, vapaissa, vapaista, vapaita, vapaitta, vapaitten* — “free” (17);

*maa, maahan, maaksi, maalla, maalle, maalta, maan, maana, maassa, maasta, maat, maata, maatta, maiden, maihin, maiksi, mailla, maille, mailta, main, maina, maineen, maissa, maista, maita, maitta, maitten* — “earth” (18);

*soiden, soihin, soiksi, soilla, soille, soilta, soin, soina, soineen, soissa, soista, soita, soitta, soitten, suo, suohon, suoksi, suolla, suolle, suolta, suon, suona, suossa, suosta, suot, suota, suotta* — “swamp” (19);

*filee, fileehen, fileeksi, fileelle, fileellä, fileeltä, fileen, fileenä, fileeseen, fileessä, fileestä, fileet, fileettä, fileetä, fileiden, fileihin, fileiksi, fileille, fileillä, fileiltä, filein, fileineen, fileinä, fileisiin, fileissä, fileistä, fileitten, fileittä, fileitä* — “fillet” (20);

*rosé, roséhen, roséiden, roséihin, roséiksi, roséilla, roséille, roséilta, roséin, roséina, roséineen, roséissa, roséista, roséita, roséitta, roséitten, roséksi, rosélla, rosélle, roséлта, rosén, roséna, roséssa, rosésta, rosét, roséta, roséta* — “pinkwine” (21);

*parfait, parfait'hen, parfait'iden, parfait'ihin, parfait'iksi, parfait'illa, parfait'ille, parfait'ilta, parfait'in, parfait'ina, parfait'ineen, parfait'issa, parfait'ista, parfait'ita, parfait'itta, parfait'itten, parfait'ksi, parfait'lla, parfait'lle, parfait'lta, parfait'n, parfait'na, parfait'ssa, parfait'sta, parfait't, parfait'ta, parfait'ta* — “parfait” (22);

*tiileen, tiileksi, tiilelle, tiilellä, tiileltä, tiilen, tiilenä, tiilessä, tiilestä, tiilet, tiilettä, tiili, tiilien, tiiliin, tiiliksi, tiilille, tiilillä, tiililtä, tiilin, tiilineen, tiilinä, tiilissä, tiilistä, tiilittä, tiiliä, tiiltä* — “brick” (23);

*uneen, uneksi, unella, unelle, unelta, unen, unena, unessa, unesta, unet, unetta, uni, unia, unien, uniin, uniksi, unilla, unille, unilta, unin, unina, unineen, unissa, unista, unitta, unta, unten* — “dream” (24);

*toimea, toimeen, toimeksi, toimella, toimelle, toimelta, toimen, toimena, toimessa, toimesta, toimet, toimetta, toimi, toimia, toimien, toimiin, toimiksi, toimilla, toimille, toimilta, toimin, toimina, toimineen, toimissa, toimista, toimitta, tointa, tointen* — “chore” (25);

*pieneen, pieneksi, pienelle, pienellä, pieneltä, pienen, pienenä, pienessä, pienestä, pienet, pienettä, pieni, pienien, pieniin, pieniksi, pienille, pienillä, pieniltä, pienin, pienine, pieninä, pienissä, pienistä, pienittä, pieniä, pienten, pientä* — “small” (26);

*kädeksi, kädelle, kädellä, kädeltä, käden, kädessä, kädestä, kädet, kädettä, käsi, käsien, käsiin, käsiksi, käsille, käsillä, käsiltä, käsin, käsineen, käsinä, käsissä, käsistä, käsittä, käsiä, käteen, kätenä, kännen, kättä* — “arm” (27);

*kynneksi, kynnelle, kynnellä, kynneltä, kynnen, kynnessä, kynnestä, kynnet, kynnettä, kynsi, kynsien, kynsiin, kynsiksi, kynsille, kynsillä, kynsiltä, kynsin, kynsineen, kynsinä, kynsissä, kynsistä, kynsittä, kynsiä, kynteen, kyntenä, kyntten, kynttä* — “fingernail” (28);

*lapsen, lapseksi, lapsella, lapselle, lapselta, lapsen, lapsena, lapsessa, lapsesta, lapset, lapsetta, lapsi, lapsia, lapsien, lapsiin, lapsiksi, lapsilla, lapsille, lapsilta, lapsin, lapsina, lapsineen, lapsissa, lapsista, lapsitta* — “child” (29);

*veisten, veistä, veitseen, veitseksi, veitselle, veitsellä, veitseltä, veitsen, veitsenä, veitsessä, veitsestä, veitset, veitsettä, veitsi, veitsien, veitsiin, veitsiksi, veitsille, veitsillä, veitsiltä, veitsin, veitsineen, veitsinä, veitsissä, veitsistä, veitsittä, veitsiä* — “knife” (30);

*kahdeksi, kahdella, kahdelle, kahdelta, kahden, kahdessa, kahdesta, kahdesti, kahdet, kahdetta, kahta, kahtaalla, kahtaalle, kahtaalta, kahteen, kahtena, kahtia, kaksi, kaksia, kaksien, kaksiin, kaksiksi, kaksilla, kaksille, kaksilta, kaksin, kaksina, kaksine, kaksissa, kaksista, kaksitta, kaksittain* — “two” (31);

*sisar, sisareen, sisareksi, sisarella, sisarelle, sisarelta, sisaren, sisarena, sisaressa, sisaresta, sisaret, sisaretta, sisaria, sisarien, sisariin, sisariksi, sisarilla, sisarille, sisarilta, sisarin, sisarina, sisarineen, sisarissa, sisarista, sisaritta, sisarta, sisarten* — “sister” (32);

*kytkimeen, kytkimeksi, kytkimelle, kytkimellä, kytkimeltä, kytkimen, kytkimenä, kytkimessä, kytkimestä, kytkimet, kytkimettä, kytkimien, kytkimiin, kytkimiksi, kytkimille, kytkimillä, kytkimiltä, kytkimin, kytkimineen, kytkiminä, kytkimissä, kytkimistä, kytkimittä, kytkimiä, kytkin, kytkinten, kytkintä* — “switch” (33);

*onneton, onnetonta, onnetonten, onnettomaan, onnettomaksi, onnettomalla, onnettomalle, onnettomalta, onnettoman, onnettomana, onnettomassa, onnettomasta, onnettomat, onnettomatta, onnettomia, onnettomien, onnettomiin, onnettomiksi, onnettomilla, onnettomille, onnettomilta, onnettomin, onnettomina, onnettomine, onnettomis-  
sa, onnettomista, onnettomitta* — “unhappy” (34);

*lämmin, lämmintä, lämpimien, lämpimiin, lämpimiksi, lämpimille, lämpimillä, lämpimiltä, lämpimin, lämpimi-  
ne, lämpiminä, lämpimissä, lämpimistä, lämpimittä, lämpimiä, lämpimäin, lämpimäksi, lämpimälle, lämpimäl-  
lä, lämpimältä, lämpimän, lämpimänä, lämpimässä, lämpimästä, lämpimät, lämpimättä, lämpimään* — “warm” (35);

*sisimmiksi, sisimmille, sisimmillä, sisimmiltä, sisimmin, sisimmissä, sisimmistä, sisimmittä, sisimmäksi, sisimmäl-  
le, sisimmällä, sisimmältä, sisimmän, sisimmässä, sisimmästä, sisimmät, sisimmättä, sisimpien, sisimpiin, sisim-  
pine, sisimpinä, sisimpiä, sisimpäin, sisimpänä, sisimpään, sisin, sisinten, sisintä* — “innermost” (36);

*vasemmaksi, vasemmalla, vasemmalle, vasemmalta, vasemman, vasemmassa, vasemmasta, vasemmat, vasem-  
matta, vasemmiksi, vasemmilla, vasemmille, vasemmilta, vasemmin, vasemmissa, vasemmista, vasemmitta, va-  
sempaa, vasempan, vasempain, vasempana, vasempia, vasempien, vasempiin, vasempina, vasempine, vasen,  
vasenta, vasenten* — “left” (37);

*nainen, naiseen, naiseksi, naisella, naiselle, naiselta, naisen, naisena, naisessa, naisesta, naiset, naisetta, naisia,  
naisien, naisiin, naisiksi, naisilla, naisille, naisilta, naisin, naisina, naisineen, naisissa, naisista, naisitta, naista,  
naisten* — “woman” (38);

*vastaukseen, vastaukseksi, vastauksella, vastaukselle, vastaukselta, vastauksen, vastauksena, vastauksessa, vas-  
tauksesta, vastaukset, vastauksetta, vastauksia, vastauksien, vastauksiin, vastauksiksi, vastauksilla, vastauksille,  
vastauksilta, vastauksin, vastauksina, vastauksineen, vastauksissa, vastauksista, vastauksitta, vastaus, vastausta,  
vastausten* — “answer” (39);

*kalleudeksi, kalleudella, kalleudelle, kalleudelta, kalleuden, kalleudessa, kalleudesta, kalleudet, kalleudetta, kal-  
leuksia, kalleuksien, kalleuksiin, kalleuksiksi, kalleuksilla, kalleuksille, kalleuksilta, kalleuksin, kalleuksina, kal-  
leuksineen, kalleuksissa, kalleuksista, kalleuksitta, kalleus, kalleuteen, kalleutena, kalleutta* — “expensiveness” (40);

*vieraaksi, vieraalla, vieraalle, vieraalta, vieraan, vieraana, vieraaseen, vieraassa, vieraasta, vieraat, vieraat-  
ta, vieraiden, vieraihin, vieraiksi, vierailta, vieraille, vierailta, vierain, vieraina, vieraine, vieraisiin, vieraissa,  
vieraista, vieraita, vieraitta, vieraitten, vieras, vierasta* — “unfamiliar” (41);

*mieheen, mieheksi, miehelle, miehellä, mieheltä, miehen, miehenä, miehessä, miehestä, miehet, miehettä, miehien,  
miehiin, miehiksi, miehille, miehillä, miehiltä, miehin, miehineen, miehinä, miehissä, miehistä, miehittä, miehiä,  
mies, miesten, miestä* — “man” (42);

*ohueen, ohueksi, ohuella, ohuelle, ohuelta, ohuen, ohuena, ohuessa, ohuesta, ohuet, ohuetta, ohuiden, ohuihin,  
ohuiksi, ohuilla, ohuille, ohuilta, ohuin, ohuina, ohuine, ohuisiin, ohuissa, ohuista, ohuita, ohuitta, ohuitten, ohut,  
ohutta* — “thin” (43);

*keväiden, keväihin, keväiksi, keväille, keväillä, keväiltä, keväin, keväineen, keväinä, keväisiin, keväissä, keväistä,  
keväitten, keväittä, keväitä, kevät, kevättä, kevääksi, keväälle, keväällä, keväältä, kevään, keväänä, kevääseen,  
keväässä, keväästä, keväätt, keväättä* — “spring” (44);

*kahdeksanneksi, kahdeksannella, kahdeksannelle, kahdeksannelta, kahdeksannen, kahdeksannessa, kahdeksan-  
nesta, kahdeksannet, kahdeksannetta, kahdeksansia, kahdeksansien, kahdeksansiin, kahdeksansiksi, kahdeksan-  
silla, kahdeksansille, kahdeksansilta, kahdeksansin, kahdeksansina, kahdeksansineen, kahdeksansissa, kahdek-  
sansista, kahdeksansitta, kahdeksanteen, kahdeksantena, kahdeksas, kahdeksatta* — “eighth” (45);

*tuhaneksi, tuhannella, tuhannelle, tuhannelta, tuhannen, tuhannessa, tuhannesta, tuhannet, tuhannetta, tuhansia, tuhansien, tuhansiin, tuhansiksi, tuhansilla, tuhansille, tuhansilta, tuhansin, tuhansina, tuhansine, tuhansissa, tuhansista, tuhansitta, tuhanteen, tuhanten, tuhantena, tuhat, tuhatta* — “thousand” (46);

*kuolleeksi, kuolleella, kuolleelle, kuolleelta, kuolleen, kuolleena, kuolleeseen, kuolleessa, kuolleesta, kuolleet, kuolleetta, kuolleiden, kuolleihin, kuolleiksi, kuolleilla, kuolleille, kuolleilta, kuollein, kuolleina, kuolleine, kuolleisiin, kuolleissa, kuolleista, kuolleita, kuolleitta, kuolleitten, kuollut, kuollutta* — “dead” (47);

*hame, hameeksi, hameella, hameelle, hameelta, hameen, hameena, hameeseen, hameessa, hameesta, hameet, hameetta, hameiden, hameihin, hameiksi, hameilla, hameille, hameilta, hamein, hameina, hameineen, hameisiin, hameissa, hameista, hameita, hameitta, hameitten, hametta* — “skirt” (48);

*askel, askele, askeleeksi, askeleella, askeleelle, askeleelta, askeleen, askeleena, askeleeseen, askeleessa, askeleesta, askeleet, askeleetta, askeleiden, askeleiksi, askeleilla, askeleille, askeleilta, askelein, askeleina, askeleineen, askeleisiin, askeleissa, askeleista, askeleita, askeleitta, askeleitten, askeleksi, askelella, askelelle, askelelta, askelen, askelena, askelessa, askelesta, askelet, askeletta, askelia, askelien, askeliin, askeliksi, askelilla, askelille, askelilta, askelin, askelina, askelineen, askelissa, askelista, askelitta, askelta, askelten* — “step” (49);

*isoäideiksi, isoäideille, isoäideillä, isoäideiltä, isoäidein, isoäideissä, isoäideistä, isoäideittä, isoäidiksi, isoäidille, isoäidillä, isoäidiltä, isoäidin, isoäidissä, isoäidistä, isoäidit, isoäidittä, isoäiteihin, isoäiteineen, isoäiteinä, isoäitejä, isoäiti, isoäitien, isoäitiin, isoäitinä, isoäitiä* — “grandmother” (50);

*nuoreenpariin, nuoreksipariksi, nuorellaparilla, nuorelleparille, nuoreltaparilta, nuorenaparina, nuorenaparin, nuoressaparissa, nuorestaparista, nuoretparit, nuoretapparitta, nuoriapareja, nuorienparien, nuoriinpareihin, nuoriksipareiksi, nuorillapareilla, nuorillepareille, nuoriltapareilta, nuorinapareina, nuorinepareineen, nuorinparein, nuoripari, nuorissapareissa, nuoristapareista, nuorittapareitta, nuortaparia, nuortenparien* — “newly-wed couple” (51).

Throwing all the words above to our algorithm, we receive the following output:

{*valo, valoa, valoihin, valoiksi, valoilla, valoille, valoilta, valoin, valoina, valoineen, valoissa, valoista, valoitta, valoja, valojen, valoksi, valolla, valolle, valolta, valon, valona, valoon, valossa, valosta, valot, valotta*} — (1) 26 words;

{*palvelu, palvelua, palveluiden, palveluihin, palveluiksi, palveluilla, palveluille, palveluilta, palveluin, palveluina, palveluineen, palveluissa, palveluista, palveluita, palveluitta, palveluitten, palveluja, palvelujen, palveluksi, palvelulla, palvelulle, palvelulta, palvelun, palveluna, palvelussa, palvelusta, palvelut, palvelutta, palveluun*} — (2) 29 words;

{*valtio, valtioiden, valtioihin, valtioiksi, valtioilla, valtioille, valtioilta, valtiolin, valtioina, valtioineen, valtioissa, valtioista, valtioita, valtioitta, valtioitten, valtioksi, valtiolla, valtiolle, valtiolta, valtion, valtiona, valtioon, valtiossa, valtiosta, valtiot, valtiota, valtiotta*} — (3) 27 words;

{*laatikko, laatikkoa, laatikkoihin, laatikkoina, laatikkoineen, laatikkoja, laatikkojen, laatikkona, laatikkoon, laatikoiden, laatikoihin, laatikoiksi, laatikoilla, laatikoille, laatikoilta, laatikoin, laatikoissa, laatikoista, laatikoita, laatikoitta, laatikoitten, laatikoksi, laatikolla, laatikolle, laatikolta, laatikon, laatikossa, laatikosta, laatikot, laatikotta*} — (4) 30 words;

{*risteihin, risteiksi, risteille, risteillä, risteiltä, ristein, risteineen, risteinä, risteissä, risteistä, risteittä, ristejä, risti, ristien, ristiin, ristiksi, ristille, ristillä, ristiltä, ristin, ristinä, ristissä, rististä, rstit, ristittä, ristiä*} — (5) 26 words;

{*papereiden, papereihin, papereiksi, papereilla, papereille, papereilta, paperein, papereina, papereineen, papereissa, papereista, papereita, papereitta, papereitten, papereja, paperi, paperia, paperien, paperiin, paperiksi, paperilla, paperille, paperilta, paperin, paperina, paperissa, paperista, paperit, paperitta*} — (6) 29 words;

{*ovea, oveen, oveksi, ovelle, ovelta, oven, ovena, ovesta, ovet, ovetta, ovi, ovia, ovien, oviin, oviksi, ovilla, oville, ovilta, ovin, ovina, ovineen, ovissa, ovista, ovitta*} — (7) 26 words;

{*nalle, nallea, nalleen, nalleihin, nalleiksi, nalleilla, nalleille, nalleilta, nallein, nalleina, nalleineen, nalleissa, nalleista, nalleitta, nalleja, nallejen, nalleksi, nallella, nallelle, nallelta, nallen, nallena, nallessa, nallesta, nallet, nalletta*} — (8) 26 words;

{*kala, kalaa, kalaan, kalain, kalaksi, kalalla, kalalle, kalalta, kalan, kalana, kalassa, kalasta, kalat, kalatta, kaloihin, kaloiksi, kaloilla, kaloille, kaloilta, kaloin, kaloina, kaloineen, kaloissa, kaloista, kaloitta, kaloja, kalojen*} — (9) 27 words;

{*koira, koiraa, koiraan, koirain, koiraksi, koiralla, koiralle, koiralta, koiran, koirana, koirassa, koirasta, koirat, koiratta, koiria, koirien, koiriin, koiriksi, koirilla, koirille, koirilta, koirin, koirina, koirineen, koirissa, koirista, koiritta*} — (10) 27 words;

{*omena, omenaa, omenaan, omenain, omenaksi, omenalla, omenalle, omenalta, omenan, omenana, omenassa, omenasta, omenat, omenatta, omenia, omenien, omeniin, omeniksi, omenilla, omenille, omenilta, omenin, omenina, omenineen, omenissa, omenista, omenitta, omenoiden, omenoihin, omenoiksi, omenoilla, omenoille, omenoilta, omenoin, omenoina, omenoineen, omenoissa, omenoista, omenoita, omenoitta, omenoitten, omenoja, omenojen*} — (11) 43 words;

{*kulkija, kulkijaa, kulkijaan, kulkijain, kulkijaksi, kulkijalla, kulkijalle, kulkijalta, kulkijan, kulkijana, kulkijassa, kulkijasta, kulkijat, kulkijatta, kulkijoiden, kulkijoihin, kulkijoiksi, kulkijoilla, kulkijoille, kulkijoilta, kulkijoin, kulkijoina, kulkijoineen, kulkijoissa, kulkijoista, kulkijoita, kulkijoitta, kulkijoitten*} — (12) 28 words;

{*katiska, katiskaa, katiskaan, katiskain, katiskaksi, katiskalla, katiskalle, katiskalta, katiskan, katiskana, katiskassa, katiskasta, katiskat, katiskatta, katiskoiden, katiskoihin, katiskoiksi, katiskoilla, katiskoille, katiskoilta, katiskoin, katiskoina, katiskoineen, katiskoissa, katiskoista, katiskoita, katiskoitta, katiskoitten, katiskoja, katiskojen*} — (13) 30 words;

{*solakaksi, solakalla, solakalle, solakalta, solakan, solakassa, solakasta, solakat, solakatta, solakka, solakkaa, solakkaan, solakkain, solakkana, solakkoihin, solakkoina, solakkoineen, solakkoja, solakkojen, solakoiden, solakoihin, solakoiksi, solakoilla, solakoille, solakoilta, solakoin, solakoissa, solakoista, solakoita, solakoitta, solakoitten*} — (14) 31 words;

{*korkea, korkeaa, korkeaan, korkeain, korkeaksi, korkealla, korkealle, korkealta, korkean, korkeana, korkeassa, korkeasta, korkeat, korkeata, korkeatta, korkeiden, korkeihin, korkeiksi, korkeilla, korkeille, korkeilta, korkein, korkeina, korkeine, korkeisiin, korkeissa, korkeista, korkeita, korkeitta, korkeitten*} — (15) 30 words;

{*vanhemmaksi, vanhemmalla, vanhemmalle, vanhemmalta, vanhemman, vanhemmassa, vanhemmasta, vanhemmat, vanhemmatta, vanhemmiksi, vanhemmilla, vanhemmille, vanhemmilta, vanhemmin, vanhemmissa, vanhemmista, vanhemmitta, vanhempaa, vanhempaan, vanhempain, vanhempana, vanhempi, vanhempia, vanhempien, vanhempisiin, vanhempina, vanhempine*} — (16) 27 words;

{*vapaa, vapaaksi, vapaalla, vapaalle, vapaalta, vapaan, vapaana, vapaaseen, vapaassa, vapaasta, vapaat, vapaata, vapaatta, vapaiden, vapaihin, vapaiiksi, vapailta, vapaille, vapailta, vapain, vapaina, vapaine, vapaisiin, vapaissa, vapaista, vapaita, vapaitta, vapaitten*} — (17) 28 words;

{*maineen*} — (18) 1 word;

{*maa, maahan, maaksi, maalla, maalle, maalta, maan, maana, maassa, maasta, maat, maata, maatta, maiden, maihin, maiksi, mailla, maille, mailta, main, maina, maissa, maista, maita, maitta, maitten*} — (18) 26 words;

{*soiden, soihin, soiksi, soilla, soille, soilta, soin, soina, soineen, soissa, soista, soita, soitta, soitten, suo, suohon, suoksi, suolla, suolle, suolta, suon, suona, suossa, suosta, suot, suota, suotta*} — (19) 27 words;

{*filee, fileehen, fileeksi, fileelle, fileellä, fileeltä, fileen, fileenä, fileeseen, fileessä, fileestä, fileet, fileettä, fileetä, fileiden, fileihin, fileiksi, fileille, fileillä, fileiltä, filein, fileineen, fileinä, fileisiin, fileissä, fileistä, fileitten, fileittä, fileitä*} — (20) 29 words;

{*rosé, roséhen, roséiden, roséihin, roséiksi, roséilla, roséille, roséilta, roséin, roséina, roséineen, roséissa, roséista, roséita, roséitta, roséitten, roséksi, rosélla, rosélle, rosélta, rosén, roséna, roséssa, rosésta, rosét, roséta, rosétta*} — (21) 27 words;

{*parfait, parfait 'hen, parfait 'iden, parfait 'ihin, parfait 'iksi, parfait 'illa, parfait 'ille, parfait 'ilta, parfait 'in, parfait 'ina, parfait 'ineen, parfait 'issa, parfait 'ista, parfait 'ita, parfait 'itta, parfait 'itten, parfait 'ksi, parfait 'lla, parfait 'lle, parfait 'lta, parfait 'n, parfait 'na, parfait 'ssa, parfait 'sta, parfait 't, parfait 'ta, parfait 'tta*} — (22) 27 words;

{*tiileen, tiileksi, tiilelle, tiilellä, tiileltä, tiilen, tiilenä, tiilessä, tiilestä, tiilet, tiilettä, tiili, tiilien, tiiliin, tiiliksi, tiilille, tiilillä, tiililtä, tiilin, tiilineen, tiilinä, tiilissä, tiilistä, tiilitä, tiiliä, tiiltä*} — (23) 26 words;

{*uneen, uneksi, unella, unelle, unelta, unen, unena, unessa, unesta, unet, unetta, uni, unia, unien, uniin, uniksi, unilla, unille, unilta, unin, unina, unineen, unissa, unista, unitta, unta, unten*} — (24) 27 words;

{*toimea, toimeen, toimeksi, toimella, toimelle, toimelta, toimen, toimena, toimessa, toimesta, toimet, toimetta, toimi, toimia, toimien, toimiin, toimiksi, toimilla, toimille, toimilta, toimin, toimina, toimineen, toimissa, toimista, toimitta, tointa, tointen*} — (25) 28 words;

{*pieneen, pieneksi, pienelle, pienellä, pieneltä, pienen, pienenä, pienessä, pienestä, pienet, pienettä, pieni, pieneen, pieniin, pieniksi, pienille, pienillä, pieniltä, pienin, pieneen, pieninä, pienissä, pienistä, pienittä, pieniä, pieneen, pientä*} — (26) 27 words;

{*kädeksi, kädelle, kädellä, kädeltä, käden, kädessä, kädestä, kädet, kädetä, käsi, käsien, käsiin, käsiksi, käsille, käsillä, käsiltä, käsin, käsineen, käsinä, käsissä, käsistä, käsittä, käsiä, käteen, kätenä, kännen, kättä*} — (27) 27 words;

{*kynneksi<sub>28</sub>, kynnelle<sub>28</sub>, kynnellä<sub>28</sub>, kynneltä<sub>28</sub>, kynnen<sub>28</sub>, kynnessä<sub>28</sub>, kynnestä<sub>28</sub>, kynnet<sub>28</sub>, kynnettä<sub>28</sub>, kynsi<sub>28</sub>, kynsien<sub>28</sub>, kynsiin<sub>28</sub>, kynsiksi<sub>28</sub>, kynsille<sub>28</sub>, kynsillä<sub>28</sub>, kynsiltä<sub>28</sub>, kynsin<sub>28</sub>, kynsineen<sub>28</sub>, kynsinä<sub>28</sub>, kynsissä<sub>28</sub>, kynsistä<sub>28</sub>, kynsittä<sub>28</sub>, kynsiä<sub>28</sub>, kynteen<sub>28</sub>, kyntenä<sub>28</sub>, kyntten<sub>28</sub>, kynttä<sub>28</sub>, kytkin<sub>33</sub>*} — (28) 27 words; (33) 1 word;

{*lapseen, lapseksi, lapsella, lapselle, lapselta, lapsen, lapsena, lapsessa, lapsesta, lapset, lapsetta, lapsi, lapsia, lapsien, lapsiin, lapsiksi, lapsilla, lapsille, lapsilta, lapsin, lapsina, lapsineen, lapsissa, lapsista, lapsitta*} — (29) 25 words;

{*veisten, veistä, veitseen, veitseksi, veitselle, veitsellä, veitseltä, veitsen, veitsenä, veitsessä, veitsestä, veitset, veitsettä, veitsi, veitsien, veitsiin, veitsiksi, veitsille, veitsillä, veitsiltä, veitsin, veitsineen, veitsinä, veitsissä, veitsistä, veitsittä, veitsiä*} — (30) 27 words;

{*kahdeksi, kahdella, kahdelle, kahdelta, kahden, kahdessa, kahdesta, kahdesti, kahdet, kahdetta, kahta, kahtaalla, kahtaalle, kahtaalta, kahteen, kahtena, kahtia, kaksi, kaksia, kaksien, kaksiin, kaksiksi, kaksilla, kaksille, kaksilta, kaksin, kaksina, kaksine, kaksissa, kaksista, kaksitta, kaksittain*} — (31) 32 words;

{*sisar, sisareen, sisareksi, sisarella, sisarelle, sisarelta, sisaren, sisarena, sisaressa, sisaresta, sisaret, sisaretta, sisaria, sisarien, sisariin, sisariksi, sisarilla, sisarille, sisarilta, sisarin, sisarina, sisarineen, sisarissa, sisarista, sisaritta, sisarta, sisarten*} — (32) 27 words;

{*kytkimeen, kytkimeksi, kytkimelle, kytkimellä, kytkimeltä, kytkimen, kytkimenä, kytkimessä, kytkimestä, kytkimet, kytkimettä, kytkimien, kytkimiin, kytkimiksi, kytkimille, kytkimillä, kytkimiltä, kytkimin, kytkimineen, kytkiminä, kytkimissä, kytkimistä, kytkimittä, kytkimiä, kytkinten, kytkintä*} — (33) 26 words;

{*onneton, onnetonta, onnetonten, onnettomaan, onnettomaksi, onnettomalla, onnettomalle, onnettomalta, onnettoman, onnettomana, onnettomassa, onnettomasta, onnettomat, onnettomatta, onnettomia, onnettomiin, onnettomiin, onnettomiksi, onnettomilla, onnettomille, onnettomilta, onnettomin, onnettomina, onnettomine, onnettomissa, onnettomista, onnettomitta*} — (34) 27 words;

{*lämmiin, lämmintä, lämpimien, lämpimiin, lämpimiksi, lämpimille, lämpimillä, lämpimiltä, lämpimin, lämpimine, lämpiminä, lämpimissä, lämpimistä, lämpimittä, lämpimiä, lämpimäin, lämpimäksi, lämpimälle, lämpimällä, lämpimältä, lämpimän, lämpimänä, lämpimässä, lämpimästä, lämpimät, lämpimättä, lämpimään*} — (35) 27 words;

{*sisimmiksi, sisimmille, sisimmillä, sisimmiltä, sisimmin, sisimmissä, sisimmistä, sisimmittä, sisimmäksi, sisimmälle, sisimmällä, sisimmältä, sisimmän, sisimmässä, sisimmästä, sisimmät, sisimmättä, sisimpien, sisimpiin, sisimpine, sisimpinä, sisimpä, sisimpäin, sisimpänä, sisimpään, sisin, sisinten, sisintä*} — (36) 28 words;

{*vasemmaksi, vasemmalla, vasemmalle, vasemmalta, vasemman, vasemmassa, vasemmasta, vasemmat, vasemmatta, vasemmiksi, vasemmilla, vasemmille, vasemmilta, vasemmin, vasemmissa, vasemmista, vasemmitta, vasempaa, vasempaan, vasempain, vasempana, vasempia, vasempien, vasempiin, vasempina, vasempine, vasen, vasenta, vasenten*} — (37) 29 words;

{*naisin*} — (38) 1 word;

{*nainen, naiseen, naiseksi, naisella, naiselle, naiselta, naisen, naisena, naisessa, naisesta, naiset, naisetta, naisia, naisien, naisiin, naisiksi, naisilla, naisille, naisilta, naisina, naisineen, naisissa, naisista, naisitta, naista, naisten*} — (38) 26 words;

{*vastaukseen, vastaukseksi, vastauksella, vastaukselle, vastaukselta, vastauksen, vastauksena, vastauksessa, vastauksesta, vastaukset, vastauksetta, vastauksia, vastauksien, vastauksiin, vastauksiksi, vastauksilla, vastauksille, vastauksilta, vastauksin, vastauksina, vastauksineen, vastauksissa, vastauksista, vastauksitta, vastaus, vastausta, vastausten*} — (39) 27 words;

{*kalleudeksi, kalleudella, kalleudelle, kalleudelta, kalleuden, kalleudessa, kalleudesta, kalleudet, kalleudetta, kalleuksia, kalleuksien, kalleuksiin, kalleuksiksi, kalleuksilla, kalleuksille, kalleuksilta, kalleuksin, kalleuksina, kalleuksineen, kalleuksissa, kalleuksista, kalleuksitta, kalleus, kalleuteen, kalleutena, kalleutta*} — (40) 26 words;

{*vieraaksi, vieraalla, vieraalle, vieraalta, vieraan, vieraana, vieraaseen, vieraassa, vieraasta, vieraat, vieraatta, vieraiden, vieraihin, vieraiksi, vierailta, vieraille, vierailta, vierain, vieraina, vieraine, vieraisiin, vieraiassa, vieraista, vieraita, vieraitta, vieraitten, vieras, vierasta*} — (41) 28 words;

{*mieheen, mieheksi, miehelle, miehellä, mieheltä, miehen, miehenä, miehessä, miehestä, miehet, miehettä, miehien, miehiin, miehiksi, miehille, miehillä, miehiltä, miehin, miehineen, miehinä, miehissä, miehistä, miehittä, miehiä, mies, miesten, miestä*} — (42) 27 words;

{*ohueen, ohueksi, ohuella, ohuelle, ohuelta, ohuen, ohuena, ohuessa, ohuesta, ohuet, ohuetta, ohuiden, ohuihin, ohuiksi, ohuilla, ohuille, ohuilta, ohuin, ohuina, ohuine, ohuisiin, ohuissa, ohuista, ohuita, ohuitta, ohuitten, ohut, ohutta*} — (43) 28 words;

{*keväiden, keväihin, kevääksi, keväille, keväällä, keväältä, kevään, kevääneen, keväänä, kevääsiin, keväässä, keväästä, keväättien, keväättä, keväättä, kevät, kevättä, kevääksi, keväälle, keväällä, keväältä, kevään, keväänä, kevääseen, keväässä, keväästä, keväätt, keväättä*} — (44) 28 words;

{*kahdeksanneksi, kahdeksannella, kahdeksannelle, kahdeksannelta, kahdeksannen, kahdeksannessa, kahdeksannesta, kahdeksannet, kahdeksannetta, kahdeksansia, kahdeksansien, kahdeksansiin, kahdeksansiksi, kahdeksansilla, kahdeksansille, kahdeksansilta, kahdeksansin, kahdeksansina, kahdeksansineen, kahdeksansissa, kahdeksansista, kahdeksansitta, kahdeksanteen, kahdeksantena, kahdeksas, kahdeksatta*} — (45) 26 words;

{*tuhanneksi, tuhannella, tuhannelle, tuhannelta, tuhannen, tuhannessa, tuhannesta, tuhannet, tuhannetta, tuhansia, tuhansien, tuhansiin, tuhansiksi, tuhansilla, tuhansille, tuhansilta, tuhansin, tuhansina, tuhansine, tuhansissa, tuhansista, tuhansitta, tuhanteen, tuhanten, tuhantena, tuhat, tuhatta*} — (46) 27 words;

{*kuolleeksi, kuolleella, kuolleelle, kuolleelta, kuolleen, kuolleena, kuolleeseen, kuolleessa, kuolleesta, kuolleet, kuolleetta, kuolleiden, kuolleihin, kuolleiksi, kuolleilla, kuolleille, kuolleilta, kuollein, kuolleina, kuolleine, kuolleisiin, kuolleissa, kuolleista, kuolleita, kuolleitta, kuolleitten, kuollut, kuollutta*} — (47) 28 words;

{*hame, hameeksi, hameella, hameelle, hameelta, hameen, hameena, hameeseen, hameessa, hameesta, hameet, hameetta, hameiden, hameihin, hameiksi, hameilla, hameille, hameilta, hamein, hameina, hameineen, hameisiin, hameissa, hameista, hameita, hameitta, hameitten, hametta*} — (48) 28 words;

{*askel, askele, askeleeksi, askeleella, askeleelle, askeleelta, askeleen, askeleena, askeleeseen, askeleessa, askeleesta, askeleet, askeleetta, askeleiden, askeleiksi, askeleilla, askeleille, askeleilta, askelein, askeleina, askeleineen, askeleisiin, askeleissa, askeleista, askeleita, askeleitta, askeleitten, askeleksi, askelella, askelelle, askelelta, askelen, askelena, askelessa, askelesta, askelet, askeletta, askelia, askelien, askeliin, askeliksi, askelilla, askelille, askelilta, askelin, askelina, askelineen, askelissa, askelista, askelitta, askelta, askelten*} — (49) 52 words;

{*isoäideiksi, isoäideille, isoäideillä, isoäideiltä, isoäidein, isoäideissä, isoäideistä, isoäideittä, isoäidiksi, isoäidille, isoäidillä, isoäidiltä, isoäidin, isoäidissä, isoäidistä, isoäidit, isoäidittä, isoäiteihin, isoäiteineen, isoäiteinä, isoäitejä, isoäiti, isoäitien, isoäitiin, isoäitinä, isoäitiä*} — (50) 26 words;

{*nuoreenpariin*} — (51) 1 word;

{*nuoreksipariksi*} — (51) 1 word;

{*nuorellaparilla*} — (51) 1 word;  
 {*nuorelleparille*} — (51) 1 word;  
 {*nuoreltaparilta*} — (51) 1 word;  
 {*nuorenaparina*} — (51) 1 word;  
 {*nuorenparin*} — (51) 1 word;  
 {*nuoretparit*} — (51) 1 word;  
 {*nuorettaparitta*} — (51) 1 word;  
 {*nuoriapareja*} — (51) 1 word;  
 {*nuorienparien*} — (51) 1 word;  
 {*nuoriinpareihin*} — (51) 1 word;  
 {*nuoriksipareiksi*} — (51) 1 word;  
 {*nuorinapareina*} — (51) 1 word;  
 {*nuorinepareineen*} — (51) 1 word;  
 {*nuorinparein*} — (51) 1 word;  
 {*nuoripari*} — (51) 1 word;  
 {*nuorittapareitta*} — (51) 1 word;  
 {*nuortaparia*} — (51) 1 word;  
 {*nuortenparien*} — (51) 1 word;  
 {*nuoressaparissa, nuorestaparista*} — (51) 2 words;  
 {*nuorissapareissa, nuoristapareista*} — (51) 2 words;  
 {*nuorillapareilla, nuorillepareille, nuoriltapareilta*} — (51) 3 words;

Here, as we present the results above, each cluster is followed by a brief description about the KOTUS affiliations of the words therein. When a cluster contains words from more than one KOTUS class, the words within the cluster are labeled with class numbers in subscripts.

The word *maineen* is both the comitative plural form of *maa* “earth” and the genitive singular form of *maine* “fame”. Since the comitative case is rarely used, it is understandable that our algorithm separated *maineen* from the other inflected forms of *maa*.

For a similar reason, the word *naisin* was not treated as the instructive plural (a rarely used inflection) form of *nainen* “woman”, but was considered as the first personal singular conditional present of *naida* “marry”.

For more information regarding the compound word in KOTUS-51, see Example 8.14.1.

As we test our algorithm against the following sample verbs:

*sano, sanoa, sanoakseen, sanoen, sanoessa, sanoi, sanoimme, sanoin, sanoisi, sanoisimme, sanoisin, sanoisit, sanoisitte, sanoisivat, sanoit, sanoitte, sanoivat, sanokaa, sanokaamme, sanoko, sanokoon, sanokoot, sanoma, sanomaan, sanomaisillaan, sanomalla, sanoman, sanomassa, sanomasta, sanomaton, sanomatta, sanominen, sanomista, sanomme, sanon, sanone, sanonee, sanoneet, sanonemme, sanonen, sanonet, sanonette, sanonevat, sanonut, sanoo, sanot, sanota, sanotaan, sanottaessa, sanottaisi, sanottaisiin, sanottako, sanottakoon, sanottaman, sanottane, sanottaneen, sanottava, sanotte, sanottiin, sanottu, sanova, sanovat* — “tell” (52);

*muista, muistaa, muistaakseen, muistaen, muistaessa, muistaisi, muistaisimme, muistaisin, muistaisit, muistaisitte, muistaisivat, muistakaa, muistakaamme, muistako, muistakoon, muistakoot, muistama, muistamaan, muistamaisillaan, muistamalla, muistaman, muistamassa, muistamasta, muistamaton, muistamatta, muistaminen, muistamista, muistamme, muistan, muistane, muistaneen, muistaneet, muistanemme, muistanen, muistanet, muistanette, muistanevat, muistanut, muistat, muistatte, muistava, muistavat, muisteta, muistetaan, muistettaessa, muistettaisi, muistettaisiin, muistettako, muistettakoon, muistettaman, muistettane, muistettaneen, muistettava, muistettiin, muistettu, muisti, muistimme, muistin, muistit, muistitte, muistivat* — “remember” (53);



voisivat, voit, voitaessa, voitaisi, voitaisiin, voitako, voitakoon, voitaman, voitane, voitaneen, voitava, voitiin, voitte, voitu, voiva, voivat — “can” (62);

saa, saada, saadaan, saadakseen, saaden, saadessa, saakaa, saakaamme, saako, saakoon, saakoot, saama, saamaan, saamaisillaan, saamalla, saaman, saamassa, saamasta, saamaton, saamatta, saaminen, saamista, saamme, saan, saane, saanee, saaneet, saanemme, saanen, saanet, saanette, saanevat, saanut, saat, saataessa, saataisi, saataisiin, saatako, saatakoon, saataman, saatane, saataneen, saatava, saatiin, saatte, saatu, saava, saavat — “receive” (63);

juo, juoda, juodaan, juodakseen, juoden, juodessa, juokaa, juokaamme, juoko, juokoon, juokoot, juoma, juomaan, juomaisillaan, juomalla, juoman, juomassa, juomasta, juomaton, juomatta, juominen, juomista, juomme, juon, juone, juonee, juoneet, juonemme, juonen, juonet, juonette, juonevat, juonut, juot, juotaessa, juotaisi, juotaisiin, juotako, juotakoon, juotaman, juotane, juotaneen, juotava, juotiin, juotte, juotu, juova, juovat — “drink” (64);

kävi, kävimme, kävin, kävisi, kävisimme, kävisin, kävisit, kävisitte, kävisivät, kävit, kävitte, kävivät, käy, käyden, käydessä, käydä, käydäkseen, käydään, käykää, käykäämme, käykö, käyköön, käykööt, käyminen, käymistä, käymme, käymä, käymäisillään, käymällä, käymän, käymässä, käymästä, käymättä, käymätön, käymään, käyn, käyne, käynee, käyneet, käynemme, käynen, käynet, käynette, käynevät, käynyt, käyt, käytiin, käytte, käyty, käytässä, käytäisi, käytäisiin, käytäkö, käytäköön, käytämän, käytäne, käytäneen, käytävä, käyvä, käyvät — “go” (65);

rohkaise, rohkaisee, rohkaisema, rohkaisemaan, rohkaisemaisillaan, rohkaisemalla, rohkaiseman, rohkaisemassa, rohkaisemasta, rohkaisematon, rohkaisematta, rohkaiseminen, rohkaisemista, rohkaisemme, rohkaisen, rohkaiset, rohkaisette, rohkaiseva, rohkaisevat, rohkaisi, rohkaisimme, rohkaisin, rohkaisisi, rohkaisisimme, rohkaisisin, rohkaisisit, rohkaisisitte, rohkaisisivat, rohkaisit, rohkaisitte, rohkaisivat, rohkaiskaa, rohkaiskaamme, rohkaisko, rohkaiskoon, rohkaiskoot, rohkaisse, rohkaissee, rohkaisseet, rohkaissemme, rohkaisseen, rohkaisset, rohkaissette, rohkaissevat, rohkaisut, rohkaista, rohkaistaan, rohkaistaessa, rohkaistaisi, rohkaistaisiin, rohkaistako, rohkaistakoon, rohkaistakseen, rohkaistaman, rohkaistane, rohkaistaneen, rohkaistava, rohkaisten, rohkais-  
tessa, rohkaistiin, rohkaistu — “encourage” (66);

tule, tulee, tulema, tulemaan, tulemaisillaan, tulemalla, tuleman, tulemassa, tulemasta, tulematon, tulematta, tuleminen, tulemista, tulemme, tulen, tulet, tulette, tuleva, tulevat, tuli, tulimme, tulin, tulisi, tulisimme, tulisin, tulisit, tulisitte, tulisivat, tulit, tulitte, tulivat, tulkaa, tulkaamme, tulko, tulkoon, tulkoot, tulla, tullaan, tullakseen, tulle, tullee, tulleet, tullemme, tullen, tullessa, tullet, tullette, tullevat, tullut, tultaessa, tultaisi, tultaisiin, tultako, tultakoon, tultaman, tultane, tultaneen, tultava, tultiin, tultu — “come” (67);

tupakoi, tupakoida, tupakoidaan, tupakoidakseen, tupakoiden, tupakoidessa, tupakoikaa, tupakoikaamme, tupakoiko, tupakoikoon, tupakoikoot, tupakoima, tupakoimaan, tupakoimaisillaan, tupakoimalla, tupakoiman, tupakoimassa, tupakoimasta, tupakoimaton, tupakoimatta, tupakoiminen, tupakoimista, tupakoimme, tupakoin, tupakoinne, tupakoinee, tupakoineet, tupakoinemme, tupakoinen, tupakoinet, tupakoinette, tupakoinevat, tupakoinut, tupakoisi, tupakoisimme, tupakoisin, tupakoisit, tupakoisitte, tupakoisivat, tupakoit, tupakoitaessa, tupakoitaisi, tupakoitaisiin, tupakoitako, tupakoitakoon, tupakoitaman, tupakoitane, tupakoitaneen, tupakoitava, tupakoitiin, tupakoitse, tupakoitsee, tupakoitsema, tupakoitsemaan, tupakoitsemaisillaan, tupakoitsemalla, tupakoitseman, tupakoitsemassa, tupakoitsemasta, tupakoitsematon, tupakoitsematta, tupakoitseminen, tupakoitsemista, tupakoitsemme, tupakoitsen, tupakoitset, tupakoitsette, tupakoitseva, tupakoitsevat, tupakoitsi, tupakoitsimme, tupakoitsin, tupakoitsisi, tupakoitsisimme, tupakoitsisin, tupakoitsisit, tupakoitsisitte, tupakoitsisivat, tupakoitsit, tupakoitsitte, tupakoitsivat, tupakoitte, tupakoitu, tupakoiva, tupakoivat — “smoke” (68);

valinne, valinnee, valinneet, valinemme, valinnen, valinnet, valinnette, valinnevat, valinnut, valita, valitaan, valitakseen, valiten, valitessa, valitkaa, valitkaamme, valitko, valitkoon, valitkoot, valitse, valitsee, valitsema, valitsemaan, valitsemaisillaan, valitsemalla, valitseman, valitsemassa, valitsemasta, valitsematon, valitsematta, valitseminen, valitsemista, valitsemme, valitsen, valitset, valitsette, valitseva, valitsevat, valitsi, valitsimme, valitsin, valitsisi, valitsisimme, valitsisin, valitsisit, valitsisitte, valitsisivat, valitsit, valitsitte, valitsivat, valittaessa, valittaisi, valittaisiin, valittako, valittakoon, valittaman, valittane, valittaneen, valittava, valittiin, valittu — “choose” (69);

juokse, juoksee, juoksema, juoksemaan, juoksemaisillaan, juoksemalla, juokseman, juoksemassa, juoksemasta, juoksematon, juoksematta, juokseminen, juoksemista, juoksemme, juoksen, juokset, juoksette, juokseva, juoksevat, juoksi, juoksimme, juoksin, juoksisi, juoksisimme, juoksisin, juoksisit, juoksisitte, juoksisivat, juoksit, juoksisitte, juoksisivat, juoskaa, juoskaamme, juosko, juoskoon, juoskoot, juosse, juossee, juosseet, juossemme, juossen, juosset, juossette, juossevat, juosut, juosta, juostaan, juostaessa, juostaisi, juostaisiin, juostako, juostakoon, juostakseen, juostaman, juostane, juostaneen, juostava, juosten, juostessa, juostiin, juostu — “run” (70);

*näe, näemme, näen, näet, näette, nähden, nähdessä, nähdä, nähdäkseen, nähdään, nähkää, nähkäämme, nähkö, nähköön, nähkööt, nähne, nähnee, nähneet, nähnemme, nähnen, nähnet, nähnette, nähnevät, nähnyt, nähtiin, nähty, nähtäessä, nähtäisi, nähtäisiin, nähtäkö, nähtäköön, nähtämän, nähtäne, nähtäneen, nähtävä, näimme, näin, näit, näitte, näkee, näkeminen, näkemistä, näkemä, näkemäisillään, näkemällä, näkemän, näkemässä, näkemästä, näkemättä, näkemätön, näkemään, näkevä, näkevät, näki, näkisi, näkisimme, näkisin, näkisit, näkisitte, näkisivät, näkivät* — “see” (71);

*vanhene, vanhenee, vanhenema, vanhenemaan, vanhenemaisillaan, vanhenemalla, vanheneman, vanhenemassa, vanhenemasta, vanhenematon, vanhenematta, vanheneminen, vanhenemista, vanhenemme, vanhenen, vanhenet, vanhenette, vanheneva, vanhenevat, vanheni, vanhenimme, vanhenin, vanhenisi, vanhenisimme, vanhenisin, vanhenisit, vanhenisitte, vanhenisivat, vanhenit, vanhenitte, vanhenivat, vanhenne, vanhennee, vanhenneet, vanhenemme, vanhennen, vanhennet, vanhennette, vanhennevat, vanhennut, vanheta, vanhetaan, vanhetakseen, vanheten, vanhetessa, vanhetkaa, vanhetkaamme, vanhetko, vanhetkoon, vanhetkoot, vanhettaessa, vanhettaisi, vanhettaisiin, vanhettako, vanhettakoon, vanhettaman, vanhettane, vanhettaneen, vanhettava, vanhettiin, vanhettu* — “age” (72);

*salaa, salaama, salaamaan, salaamaisillaan, salaamalla, salaaman, salaamassa, salaamasta, salaamaton, salaamatta, salaaminen, salaamista, salaamme, salaan, salaat, salaatte, salaava, salaavat, salaisi, salaisimme, salaisiin, salaisit, salaisitte, salaisivat, salanne, salannee, salanneet, salannemme, salannen, salannet, salannette, salannevat, salannut, salasi, salasimme, salasiin, salasit, salasitte, salasivat, salata, salataan, salatakseen, salaten, salatessa, salatkaa, salatkaamme, salatko, salatkoon, salatkoot, salattaessa, salattaisi, salattaisiin, salattako, salattakoon, salattaman, salattane, salattaneen, salattava, salattiin, salattu* — “conceal” (73);

*katkea, katkeaa, katkeaisi, katkeaisimme, katkeaisin, katkeaisit, katkeaisitte, katkeaisivat, katkeama, katkeamaan, katkeamaisillaan, katkeamalla, katkeaman, katkeamassa, katkeamasta, katkeamaton, katkeamatta, katkeaminen, katkeamista, katkeamme, katkean, katkeat, katkeatte, katkeava, katkeavat, katkeisi, katkeisimme, katkeisin, katkeisit, katkeisitte, katkeisivat, katkenne, katkennee, katkenneet, katkenemme, katkennin, katkennet, katkennette, katkennevat, katkennut, katkesi, katkesimme, katkesiin, katkesit, katkesitte, katkesivat, katketa, katketaan, katketakseen, katketen, katketessa, katketkaa, katketkaamme, katketko, katketkoon, katketkoot, katkettaessa, katkettaisi, katkettaisiin, katkettako, katkettakoon, katkettaman, katkettane, katkettaneen, katkettava, katkettiin, katkettu* — “cut” (74);

*selvinne, selvinnee, selvinneet, selvinemme, selvinnen, selvinnet, selvinnette, selvinnevät, selvinnyt, selvisi, selvisimme, selvisiin, selvisit, selvisitte, selvisivät, selviten, selvitessä, selvitkää, selvitkäämme, selvitkö, selvitköön, selvitkööt, selvittiin, selvitty, selvittäessä, selvittäisi, selvittäisiin, selvittäkö, selvittäköön, selvittämän, selvittäne, selvittäneen, selvittävä, selvitä, selvitäkseen, selvittään, selviä, selviäisi, selviäisimme, selviäisin, selviäisit, selviäisitte, selviäisivät, selviäminen, selviämistä, selviämme, selviämä, selviämäisillään, selviämällä, selviämän, selviämässä, selviämästä, selviämättä, selviämätön, selviämään, selviän, selviät, selviätte, selviävä, selviävät, selviää* — “escape” (75);

*taida, taidamme, taidan, taidat, taidatte, taideta, taidetaan, taidettaessa, taidettaisi, taidettaisiin, taidettako, taidettakoon, taidettaman, taidettane, taidettaneen, taidettava, taidettiin, taidettu, tainne, tainnee, tainneet, tainnemme, tainnen, tainnet, tainnette, tainnevat, tainnut, taisi, taisimme, taisiin, taisit, taisitte, taisivat, taitaa, taitakseen, taitaen, taitaessa, taitaisi, taitaisimme, taitaisiin, taitaisit, taitaisitte, taitaisivat, taitakaa, taitakaamme, taitako, taitakoon, taitakoot, taitama, taitamaan, taitamaisillaan, taitamalla, taitaman, taitamassa, taitamasta, taitamaton, taitamatta, taitaminen, taitamista, taitane, taitanee, taitaneet, taitanemme, taitanen, taitanet, taitanette, taitanevat, taitanut, taitava, taitavat* — “master” (76);

*kumajaa, kumajaisi, kumaji* — “boom” (77);

*kaikaa, kaikaavat, kaikaisi, kaikaisivat* — “echo” (78),

we obtain

{*sanomaton*} — (52) 1 word;

{*sano, sanoa, sanoakseen, sanoen, sanoessa, sanoi, sanoimme, sanoin, sanoisi, sanoisimme, sanoisin, sanoisit, sanoisitte, sanoisivat, sanoit, sanoitte, sanoivat, sanokaa, sanokaamme, sanoko, sanokoon, sanokoot, sanoma, sanomaan, sanomaisillaan, sanomalla, sanoman, sanomassa, sanomasta, sanomatta, sanominen, sanomista, sanomme, sanon, sanone, sanonee, sanoneet, sanonemme, sanonen, sanonet, sanonette, sanonevat, sanonut, sanoo, sanot, sanota, sanotaan, sanottaessa, sanottaisi, sanottaisiin, sanottako, sanottakoon, sanottaman, sanottane, sanottaneen, sanottava, sanotte, sanottiin, sanottu, sanova, sanovat*} — (52) 61 words;

{*muistamaton*} — (53) 1 word;

{*muista, muistaa, muistaakseen, muistaen, muistaessa, muistaisi, muistaisimme, muistaisin, muistaisit, muistaisitte, muistaisivat, muistakaa, muistakaamme, muistako, muistakoon, muistakoot, muistama, muistamaan, muistamaisillaan, muistamalla, muistaman, muistamassa, muistamasta, muistamatta, muistaminen, muistamista, muistamme, muistan, muistane, muistanee, muistaneet, muistanemme, muistanen, muistanet, muistanette, muistanevat, muistanut, muistat, muistatte, muistava, muistavat, muisteta, muistetaan, muistettaessa, muistettaisi, muistettaisiin, muistettako, muistettakoon, muistettaman, muistettane, muistettaneen, muistettava, muistettiin, muistettu, muisti, muistimme, muistin, muistit, muistitte, muistivat*} — (53) 60 words;

{*huutamaton*} — (54) 1 word;

{*huuda, huudamme, huudan, huudat, huudatte, huudeta, huudetaan, huudettaessa, huudettaisi, huudettaisiin, huudettako, huudettakoon, huudettaman, huudettane, huudettaneen, huudettava, huudettiin, huudettu, huusi, huusimme, huusin, huusit, huusitte, huusivat, huutaa, huutaakseen, huutaen, huutaessa, huutaisi, huutaisimme, huutaisin, huutaisit, huutaisitte, huutaisivat, huutakaa, huutakaamme, huutako, huutakoon, huutakoot, huutama, huutamahan, huutamaisillaan, huutamalla, huutaman, huutamassa, huutamasta, huutamatta, huutaminen, huutamista, huutane, huutanee, huutaneet, huutanemme, huutanen, huutanet, huutanette, huutanevat, huutanut, huutava, huutavat*} — (54) 60 words;

{*sousitte*} — (55) 1 word;

{*soutamaton*} — (55) 1 word;

{*souda, soudamme, soudan, soudat, soudatte, soudeta, soudetaan, soudettaessa, soudettaisi, soudettaisiin, soudettako, soudettakoon, soudettaman, soudettane, soudettaneen, soudettava, soudettiin, soudettu, soudimme, soudin, soudit, souditte, sousi, sousimme, sousin, sousit, sousivat, soutaa, soutaakseen, soutaen, soutaessa, soutaisi, soutaisimme, soutaisin, soutaisit, soutaisitte, soutaisivat, soutakaa, soutakaamme, soutako, soutakoon, soutakoot, soutama, soutamaan, soutamaisillaan, soutamalla, soutaman, soutamassa, soutamasta, soutamatta, soutaminen, soutamista, soutane, soutanee, soutaneet, soutanemme, soutanen, soutanet, soutanette, soutanevat, soutanut, soutava, soutavat, souti, soutivat*} — (55) 65 words;

{*kaiva, kaivaa, kaivaisi, kaivaisimme, kaivaisin, kaivaisit, kaivaisitte, kaivaisivat, kaivakaa, kaivakaamme, kaivako, kaivakoon, kaivakoot, kaivamme, kaivan, kaivaneet, kaivanut, kaivat, kaivatte, kaivavat, kaiveta, kaivetaan, kaivettaisi, kaivettaisiin, kaivettako, kaivettakoon, kaivettiin, kaivettu, kaivoi, kaivoimme, kaivoin, kaivoit, kaivoitte, kaivoivat*} — (56) 34 words;

{*saartamaton*} — (57) 1 word;

{*saarra, saarramme, saarran, saarrat, saarratte, saarreta, saarretaan, saarrettaessa, saarrettaisi, saarrettaisiin, saarrettako, saarrettakoon, saarrettaman, saarrettane, saarrettaneen, saarrettava, saarrettiin, saarrettu, saarroimme, saarroin, saarroit, saarroitte, saarsi, saarsimme, saarsin, saarsit, saarsitte, saarsivat, saartaa, saartaakseen, saartaen, saartaessa, saartaisi, saartaisimme, saartaisin, saartaisit, saartaisitte, saartaisivat, saartakaa, saartakaamme, saartako, saartakoon, saartakoot, saartama, saartamaan, saartamaisillaan, saartamalla, saartaman, saartamassa, saartamasta, saartamatta, saartaminen, saartamista, saartane, saartanee, saartaneet, saartanemme, saartanen, saartanet, saartanette, saartanevat, saartanut, saartava, saartavat, saartoi, saartoivat*} — (57) 66 words;

{*laskematon*} — (58) 1 word;

{*laske, laskea, laskeakseen, laskee, laskekaa, laskekaamme, laskeko, laskekoon, laskekoot, laskema, laskemaan, laskemaisillaan, laskemalla, laskeman, laskemassa, laskemasta, laskematta, laskeminen, laskemista, laskemme, lasken, laskene, laskenee, laskeneet, laskenemme, laskenen, laskenet, laskenette, laskenevat, laskenut, lasket, lasketa, lasketaan, laskettaessa, laskettaisi, laskettaisiin, laskettako, laskettakoon, laskettaman, laskettane, laskettaneen, laskettava, laskette, laskettiin, laskettu, laskeva, laskevat, laski, laskien, laskiessa, laskimme, laskin, laskisi, laskisimme, laskisin, laskisit, laskisitte, laskisivat, laskit, laskitte, laskivat*} — (58) 61 words;

{*tuntematon*} — (59) 1 word;

{*tunne, tunnemme, tunnen, tunnet, tunneta, tunnetaan, tunnetaessa, tunnetaisi, tunnetaisiin, tunnetaako, tunneta-  
takoon, tunnettaman, tunnettane, tunnettaneen, tunnettava, tunnette, tunnettiin, tunnettu, tunsii, tunsimme, tunsin,  
tunsit, tunsitte, tunsivat, tuntea, tunteakseen, tuntee, tuntekaa, tuntekaamme, tunteko, tuntekoon, tuntekoot, tunte-  
ma, tuntemaan, tuntemaisillaan, tunteamalla, tunteman, tuntemassa, tuntemasta, tuntematta, tunteminen, tuntemis-  
ta, tuntene, tuntenee, tunteneet, tuntenemme, tuntenen, tuntenet, tuntenette, tuntenevat, tuntenut, tunteva, tuntevat,  
tuntien, tuntiessa, tuntisi, tuntisimme, tuntisin, tuntisit, tuntisitte, tuntisivat*} — (59) 61 words;

{*lähtemätön*} — (60) 1 word;

{*lähde, lähdemme, lähden, lähdet, lähdette, lähdettiin, lähdetty, lähdettäessä, lähdettäisi, lähdettäisiin, lähdet-  
täksi, lähdettäköön, lähdettamän, lähdettäne, lähdettäneen, lähdettävä, lähdetä, lähdetään, lähdimme, lähdin,  
lähdit, lähditte, lähtee, lähtekää, lähtekäämme, lähtekö, lähteköön, lähtekööt, lähteminen, lähtemistä, lähtemä,  
lähtemäisillään, lähtemällä, lähtemän, lähtemässä, lähtemästä, lähtemättä, lähtemään, lähtene, lähtenee, lähte-  
neet, lähtenemme, lähtenen, lähtenet, lähtenette, lähtenevät, lähtenyt, lähtevä, lähtevät, lähteä, lähteäkseen, lähti,  
lähtien, lähtiessä, lähtisi, lähtisimme, lähtisin, lähtisit, lähtisitte, lähtisivät, lähtivät*} — (60) 61 words;

{*sallimaton*} — (61) 1 word;

{*salli, sallia, salliakseen, sallien, salliessa, sallii, sallikaa, sallikaamme, salliko, sallikoon, sallikoot, sallima, sal-  
limaan, sallimaisillaan, sallimalla, salliman, sallimassa, sallimasta, sallimatta, salliminen, sallimista, sallimme,  
sallin, salline, sallinee, sallineet, sallinemme, sallinen, sallinet, sallinette, sallinevat, sallinut, sallisi, sallisimme,  
sallisin, sallisit, sallisitte, sallisivat, sallit, sallita, sallitaan, sallittaessa, sallittaisi, sallittaisiin, sallittako, sal-  
littakoon, sallittaman, sallittane, sallittaneen, sallittava, sallitte, sallittiin, sallittu, salliva, sallivat*} — (61) 55  
words;

{*voimaton*} — (62) 1 word;

{*voi, voida, voidaan, voidakseen, voiden, voidessa, voikaa, voikaamme, voiko, voikoon, voikoot, voima, voimaan,  
voimaisillaan, voimalla, voiman, voimassa, voimasta, voimatta, voiminen, voimista, voimme, voin, voine, voinee,  
voineet, voinemme, voinen, voinet, voinette, voinevat, voinut, voisi, voisimme, voisin, voisit, voisitte, voisivat,  
voit, voitaessa, voitaisi, voitaisiin, voitako, voitakoon, voitaman, voitane, voitaneen, voitava, voitiin, voitte, voitu,  
voiva, voivat*} — (62) 53 words;

{*saamaton*} — (63) 1 word;

{*saataisiin, saataman, saatane, saataneen, saatiin, saatu*} — (63) 6 words;

{*saa, saada, saadaan, saadakseen, saaden, saadessa, saakaa, saakaamme, saako, saakoon, saakoot, saama, saa-  
maan, saamaisillaan, saamalla, saaman, saamassa, saamasta, saamatta, saaminen, saamista, saamme, saan,  
saane, saanee, saaneet, saanemme, saanen, saanet, saanette, saanevat, saanut, saat, saataessa, saataisi, saatako,  
saatakoon, saatava, saatte, saava, saavat*} — (63) 41 words;

{*juomaton*} — (64) 1 word;

{*juo, juoda, juodaan, juodakseen, juoden, juodessa, juokaa, juokaamme, juoko, juokoon, juokoot, juoma, juo-  
maan, juomaisillaan, juomalla, juoman, juomassa, juomasta, juomatta, juominen, juomista, juomme, juon, juone,  
juonee, juoneet, juonemme, juonen, juonet, juonette, juonevat, juonut, juot, juotaessa, juotaisi, juotaisiin, juotako,  
juotakoon, juotaman, juotane, juotaneen, juotava, juotiin, juotte, juotu, juova, juovat*} — (64) 47 words;

{*käymätön*} — (65) 1 word;

{*kävi, kävimme, kävin, kävisi, kävisimme, kävisin, kävisit, kävisitte, kävisivät, kävit, kävitte, kävivät, käy, käy-  
den, käydessä, käydä, käydäkseen, käydään, käykää, käykäämme, käykö, käyköön, käykööt, käyminen, käymistä,  
käymme, käymä, käymäisillään, käymällä, käymän, käymässä, käymästä, käymättä, käymään, käyn, käyne, käy-  
nee, käyneet, käynemme, käynen, käynet, käynette, käynevät, käynyt, käyt, käytiin, käytte, käyty, käytäessä, käy-  
täisi, käytäisiin, käytäkö, käytäköön, käytämän, käytäne, käytäneen, käytävä, käyvä, käyvät*} — (65) 59 words;

{*rohkaisematon*} — (66) 1 word;

{*rohkaise, rohkaisee, rohkaisema, rohkaisemaan, rohkaisemaisillaan, rohkaisemalla, rohkaiseman, rohkaisemas-  
sa, rohkaisemasta, rohkaisematta, rohkaiseminen, rohkaisemista, rohkaisemme, rohkaisen, rohkaiset, rohkaisette,  
rohkaiseva, rohkaisevat, rohkaisi, rohkaisimme, rohkaisin, rohkaisisi, rohkaisisimme, rohkaisisin, rohkaisisit, roh-  
kaisisitte, rohkaisivat, rohkaisit, rohkaisitte, rohkaisivat, rohkaiskaa, rohkaiskaamme, rohkaisko, rohkaiskoon,  
rohkaiskoot, rohkaisse, rohkaissee, rohkaisseet, rohkaissemme, rohkaisseen, rohkaisset, rohkaissette, rohkaissevat,  
rohkaisut, rohkaiista, rohkaiistaan, rohkaiistaessa, rohkaiistaisi, rohkaiistaisiin, rohkaiistako, rohkaiistakoon, roh-  
kaiistakseen, rohkaiistaman, rohkaiistane, rohkaiistaneen, rohkaiistava, rohkaiisten, rohkaiistessa, rohkaiistiin, roh-  
kaiistu*} — (66) 60 words;

{*tulematon*} — (67) 1 word;

{*tule, tulee, tulema, tulemaan, tulemaisillaan, tulemalla, tuleman, tulemassa, tulemasta, tulematta, tuleminen,  
tulemista, tulemme, tulen, tulet, tulette, tuleva, tulevat, tuli, tulimme, tulin, tulisi, tulisimme, tulisin, tulisit, tulisitte,  
tulisivat, tulit, tulitte, tulivat, tulkaa, tulkaamme, tulko, tulkoon, tulkoot, tulla, tullaan, tullakseen, tulle, tullee,  
tulleet, tullemme, tullen, tullessa, tullet, tullette, tullevat, tullut, tultaessa, tultaisi, tultaisiin, tultako, tultakoon,  
tultaman, tultane, tultaneen, tultava, tultiin, tultu*} — (67) 59 words;

{*tupakoimaton, tupakoitsematon*} — (68) 2 words;

{*tupakoi, tupakoida, tupakoidaan, tupakoidakseen, tupakoiden, tupakoidessa, tupakoikaa, tupakoikaamme, tupa-  
koiko, tupakoikoon, tupakoikoot, tupakoima, tupakoimaan, tupakoimaisillaan, tupakoimalla, tupakoiman, tupa-  
koimassa, tupakoimasta, tupakoimatta, tupakoiminen, tupakoimista, tupakoimme, tupakoin, tupakoine, tupakoi-  
nee, tupakoineet, tupakoinemme, tupakoinen, tupakoinet, tupakoinette, tupakoinevat, tupakoinut, tupakoisi, tupa-  
koisimme, tupakoisin, tupakoisit, tupakoisitte, tupakoisivat, tupakoit, tupakoitaessa, tupakoitaisi, tupakoitaisiin,  
tupakoitako, tupakoitakoon, tupakoitaman, tupakoitane, tupakoitaneen, tupakoitava, tupakoitiin, tupakoitse, tu-  
pakoitsee, tupakoitsema, tupakoitsemaan, tupakoitsemaisillaan, tupakoitseamalla, tupakoitseman, tupakoitsemas-  
sa, tupakoitsehasta, tupakoitsehatta, tupakoitseminen, tupakoitsemistä, tupakoitsemme, tupakoitsen, tupakoitset,  
tupakoitsette, tupakoitseva, tupakoitsevat, tupakoitsi, tupakoitsimme, tupakoitsin, tupakoitsisi, tupakoitsisimme,  
tupakoitsisin, tupakoitsisit, tupakoitsisitte, tupakoitsisivat, tupakoitsit, tupakoitsitte, tupakoitsivat, tupakoitte, tu-  
pakoitu, tupakoiva, tupakoivat*} — (68) 83 words;

{*valitsematon*} — (69) 1 word;

{*valinne, valinnee, valinneet, valinemme, valininen, valinnet, valinnette, valinnevat, valinnut, valita, valitaan,  
valitakseen, valiten, valitessa, valitkaa, valitkaamme, valitko, valitkoon, valitkoot, valitse, valitsee, valitsema,  
valitsemaan, valitsemaisillaan, valitseamalla, valitseman, valitsemassa, valitsehasta, valitsehatta, valitseminen,  
valitsemistä, valitsemme, valitsen, valitset, valitsette, valitseva, valitsevat, valitsi, valitsimme, valitsin, valitsisi,  
valitsisimme, valitsisin, valitsisit, valitsisitte, valitsisivat, valitsit, valitsitte, valitsivat, valittaessa, valittaisi, valit-  
taisiin, valittako, valittakoon, valittaman, valittane, valittaneen, valittava, valittiin, valittu*} — (69) 60 words;

{*juoksematon*} — (70) 1 word;

{*juokse, juoksee, juoksema, juoksemaan, juoksemaisillaan, juoksemalla, juokseman, juoksemassa, juoksemas-  
ta, juoksematta, juokseminen, juoksemista, juoksemme, juoksen, juokset, juoksette, juokseva, juoksevat, juoksi,  
juoksimme, juoksin, juoksisi, juoksisimme, juoksisin, juoksisit, juoksisitte, juoksisivat, juoksit, juoksitte, juoksivat,  
juoskaa, juoskaamme, juosko, juoskoon, juoskoot, juosse, juossee, juosseet, juossemme, juossen, juosset, juosset-  
te, juossevat, juosset, juosta, juostaan, juostaessa, juostaisi, juostaisiin, juostako, juostakoon, juostakseen, juos-  
taman, juostane, juostaneen, juostava, juosten, juostessa, juostiin, juostu*} — (70) 60 words;

{*näkemätön*} — (71) 1 word;

{*näe, näemme, näen, näet, näette, nähden, nähdessä, nähdä, nähdäkseen, nähdään, nähkää, nähkäämme, nähkö,  
nähkөөn, nähkөөt, nähne, nähnee, nähneet, nähnemme, nähnen, nähnet, nähnette, nähnevät, nähnyt, nähtiin, näh-  
ty, nähtäessä, nähtäisi, nähtäisiin, nähtäkö, nähtäkөөn, nähtämän, nähtäne, nähtäneen, nähtävä, näimme, näin,  
näit, näitte, näkee, näkeminen, näkemistä, näkemä, näkemäisillään, näkemällä, näkemän, näkemässä, näkemäs-  
tä, näkemättä, näkemään, näkevä, näkevät, näki, näkisi, näkisimme, näkisin, näkisit, näkisitte, näkisivät, näkivät*}  
— (71) 60 words;

{*vanhenematon*} — (72) 1 word;

{*vanhene, vanhenee, vanhenema, vanhenemaan, vanhenemaisillaan, vanhenemalla, vanheneman, vanhenemas-  
sa, vanhenemasta, vanhenematta, vanheneminen, vanhenemista, vanhenemme, vanhenen, vanhenet, vanhenet-  
te, vanheneva, vanhenevat, vanheni, vanhenimme, vanhenin, vanhenisi, vanhenisimme, vanhenisin, vanhenisit,  
vanhenisitte, vanhenisivat, vanhenit, vanheniitte, vanhenivat, vanhenne, vanhennee, vanhenneet, vanhennemme,  
vanhennen, vanhennet, vanhennette, vanhennevat, vanhennut, vanheta, vanhetaan, vanhetakseen, vanheten, van-  
hetessa, vanhetkaa, vanhetkaamme, vanhetko, vanhetkoon, vanhetkoot, vanhettaessa, vanhettaisi, vanhettaisiin,  
vanhettako, vanhettakoon, vanhettaman, vanhettane, vanhettaneen, vanhettava, vanhettiin, vanhettu*} — (72) 60  
words;

{*salaamaton*} — (73) 1 word;

{*salaa, salaama, salaamaan, salaamaisillaan, salaamalla, salaaman, salaamassa, salaamasta, salaamatta, sa-  
laaminen, salaamista, salaamme, salaan, salaat, salaatte, salaava, salaavat, salaisi, salaisimme, salaisin, salai-  
sit, salaisitte, salaisivat, salanne, salannee, salanneet, salannemme, salannen, salannet, salannette, salannevat,  
salannut, salasi, salasimme, salasin, salasit, salasitte, salasivat, salata, salataan, salatakseen, salaten, salatessa,  
salatkaa, salatkaamme, salatko, salatkoon, salatkoot, salattaessa, salattaisi, salattaisiin, salattako, salattakoon,  
salattaman, salattane, salattaneen, salattava, salattiin, salattu*} — (73) 59 words;

{*katkeamaton*} — (74) 1 word;

{*katkea, katkeaa, katkeaisi, katkeaisimme, katkeaisin, katkeaisit, katkeaisitte, katkeaisivat, katkeama, katkea-  
maan, katkeamaisillaan, katkeamalla, katkeaman, katkeamassa, katkeamasta, katkeamatta, katkeaminen, katkea-  
mista, katkeamme, katkean, katkeat, katkeatte, katkeava, katkeavat, katkeisi, katkeisimme, katkeisin, katkeisit,  
katkeisitte, katkeisivat, katkenne, katkennee, katkenneet, katkennemme, katkennenen, katkennet, katkennette, kat-  
kennevat, katkennut, katkesi, katkesimme, katkesin, katkesit, katkesitte, katkesivat, katketa, katketaan, katketak-  
seen, katketen, katketessa, katketkaa, katketkaamme, katketko, katketkoon, katketkoot, katkettaessa, katkettaisi,  
katkettaisiin, katkettako, katkettakoon, katkettaman, katkettane, katkettaneen, katkettava, katkettiin, katkettu*} —  
(74) 66 words;

{*selviämätön*} — (75) 1 word;

{*selvinne, selvinnee, selvinneet, selvinemme, selvinnen, selvinnet, selvinnette, selvinnevät, selvinnyt, selvisi, sel-  
visimme, selvisin, selvisit, selvisitte, selvisivät, selviten, selvitessä, selvittä, selvittäämme, selvittäkö, selvittäköön,  
selvittäkööt, selvittiin, selvitty, selvittäessä, selvittäisi, selvittäisiin, selvittäkö, selvittäköön, selvittämän, selvittäne,  
selvittäneen, selvittävä, selvitä, selvitäkseen, selvittään, selviä, selviäisi, selviäisimme, selviäisin, selviäisit, sel-  
viäisitte, selviäisivät, selviäminen, selviämistä, selviämme, selviämä, selviämäisillään, selviämällä, selviämän,  
selviämässä, selviämästä, selviämättä, selviämään, selviän, selviät, selviätte, selviävä, selviävät, selviää*} — (75)  
60 words;

{*taitamaton*} — (76) 1 word;

{*taida, taidamme, taidan, taidat, taidatte, taideta, taidetaan, taidettaessa, taidettaisi, taidettaisiin, taidettako,  
taidettakoon, taidettaman, taidettane, taidettaneen, taidettava, taidettiin, taidettu, tainne, tainnee, tainneet, tain-  
nemme, tainnen, tainnet, tainnette, tainnevat, tainnut, taisi, taisimme, taisin, taisit, taisitte, taisivat, taitaa, tai-  
taakseen, taitaen, taitaessa, taitaisi, taitaisimme, taitaisin, taitaisit, taitaisitte, taitaisivat, taitakaa, taitakaamme,  
taitako, taitakoon, taitakoot, taitama, taitamaan, taitamaisillaan, taitamalla, taitaman, taitamassa, taitamasta,  
taitamatta, taitaminen, taitamista, taitane, taitanee, taitaneet, taitanemme, taitanen, taitanet, taitanette, taitane-  
vat, taitanut, taitava, taitavat*} — (76) 69 words;

{*kumajaa, kumajaisi, kumaji*} — (77) 3 words;

{*kaikaa, kaikaavat, kaikaisi, kaikaisivat*} — (78) 4 words.

Here, words ending in *-maton* and *mätön* are negative participles, which roughly translate into English words with prefixes *il-*, *im-*, *in-*, *ir-*, *non-*, *un-*, or suffix *-less*. To be consistent with our clustering policy for English words, we have separated negative participles from other inflected forms of Finnish verbs.

### 8.1.3 Heuristic detection of compounds

The following algorithm for heuristic detection of Finnish compounds differs from the Danish version (Algorithm 5.12) only in some specific details. To make the context clear, we still state the algorithm in full. (In what follows, the string minus operation  $\hat{\beta} \ominus \hat{\alpha}$  is prescribed by Definition 5.11.)

**Algorithm 8.13** (Heuristic identification of Finnish binary compounds). Let  $\Lambda^{\hat{\rho}} = \{\hat{\rho}_1, \dots, \hat{\rho}_Q\}$  be a list of distinct Finnish essential roots (without vowel blotting) that contain at least one instance of  $\mathbf{V}$  (in either upper or lower case) and DO NOT match the following string patterns:

$$(\mathbf{CV}ij|\mathbf{VC}|ko|mi|te|tu|(ant|ei|ent|nut|nyt|to|vat|v\ddot{a}l|v\ddot{a}t)\mathbf{X}).$$

The output of the function  $\text{CpdDet}(\Lambda^{\hat{\rho}})$  is obtained through the following procedures:

- (1) Construct a list  $\{(\hat{\rho}_1, \lambda_1^{\hat{\rho}}), \dots, (\hat{\rho}_Q, \lambda_Q^{\hat{\rho}})\}$  where  $\lambda_q^{\hat{\rho}} = \{\hat{\rho}_{(q,1)}, \dots, \hat{\rho}_{(q,n_q)}\}$  is a subset of  $\Lambda^{\hat{\rho}}$  whose members all match the string pattern  $\hat{\rho}_{q\sim}$ , for  $q \in \mathbb{Z} \cap [1, Q]$ .
- (2) Expand the aforementioned entry  $(\hat{\rho}_q, \lambda_q^{\hat{\rho}})$  into a list of triplets  $\{(\hat{\rho}_{(q,1)}, \hat{\rho}_q, \hat{\rho}_{(q,1)} \ominus \hat{\rho}_q), \dots, (\hat{\rho}_{(q,n_q)}, \hat{\rho}_q, \hat{\rho}_{(q,n_q)} \ominus \hat{\rho}_q)\}$  for every  $q \in \mathbb{Z} \cap [1, Q]$  such that  $\lambda_q^{\hat{\rho}} \neq \emptyset$ . Collect all these triplets as one runs through the list  $\{(\hat{\rho}_1, \lambda_1^{\hat{\rho}}), \dots, (\hat{\rho}_Q, \lambda_Q^{\hat{\rho}})\}$ . The list of these triplets  $\{(\hat{\rho}_{(1)}, \hat{\eta}_{(1)}, \hat{\rho}_{(1)} \ominus \hat{\eta}_{(1)}), \dots, (\hat{\rho}_{(Q')}, \hat{\eta}_{(Q')}, \hat{\rho}_{(Q')} \ominus \hat{\eta}_{(Q')})\}$  contains potentially valid decompositions of compounds.
- (3) Screen the aforementioned list of triplets as follows: for every  $q' \in \mathbb{Z} \cap [1, Q']$ , if  $(\hat{\rho}_{(q')}, \hat{\eta}_{(q')}, \hat{\tau}_{(q')} = \hat{\rho}_{(q')} \ominus \hat{\eta}_{(q')})$  satisfies

$$\ell(\hat{\rho}_{(q')} \ominus \hat{\eta}_{(q')}) \geq 2 \quad \text{AND} \quad \hat{\rho}_{(q')} \ominus \hat{\eta}_{(q')} = \mathbf{X}_1 \mathbf{V} \mathbf{X}_2,$$

then construct  $\hat{\tau}_{(q')}$  by performing  $(ei)ksi\sim \rightarrow \emptyset$ ,  $(en|En|et|i|ta|ten|t\ddot{a})\sim \rightarrow \emptyset$ ,  $(i|l|ie)n\sim \rightarrow \emptyset$ ,  $e(L|l|n|S|T)(a|e|\ddot{a})\sim \rightarrow \emptyset$ ,  $i(n|S|T)(a|e|\ddot{a})\sim \rightarrow \emptyset$  on  $\hat{\tau}_{(q')}$ , before generating a list  $\lambda_{(q')}^{\hat{\tau}}$  by members of  $\Lambda^{\hat{\rho}}$  that match the pattern  $(\hat{\tau}_{(q')}|\hat{\tau}_{(q')}^*)$ ; otherwise, set  $\lambda_{(q')}^{\hat{\tau}} = \emptyset$ .

- (4) Collect all the triplets  $(\hat{\rho}_{(q')}, \hat{\eta}_{(q')}, \lambda_{(q')}^{\hat{\tau}})$  where  $\lambda_{(q')}^{\hat{\tau}}$  is non-void and  $\hat{\tau}_{(q')}$  DOES NOT match the following string patterns:

$$(\text{Tom|ton|T\ddot{o}m|t\ddot{o}n|\tau\nu\tau)\mathbf{X}.$$

Trim the tags in the triplets by doing  $\sim \mathbf{X}^{\in}(\mathbf{VC})\mathbf{V}_m \rightarrow \mathbf{X}$  on the strings. This resulting list of triplets  $\text{CpdDet}(\Lambda_{\hat{\rho}})$  contains the heuristic decompositions of all the identified binary compounds.

**Algorithm 8.14** (Approximate clustering of Finnish words with heuristic detection of compounds). The approximate clustering of a list of Finnish words  $\{\hat{\alpha}_1, \dots, \hat{\alpha}_N\}$  respecting compounding is completed in four stages:

- (1) Do as in Algorithm 8.12(1).
- (2) Do as in Algorithm 8.12(2). Save both the tagged clusters  $\{\Gamma_1 = \{G_{(1,1)}, \dots, G_{(1,m_1)}\}, \dots, \Gamma_K = \{G_{(K,1)}, \dots, G_{(1,m_K)}\}\}$  and the list of word clusters  $\{\check{I}_1, \dots, \check{I}_K\}$  for further use.
- (3) Construct a tagged list of word clusters  $\{(\check{I}_1, \Lambda_1^{\hat{\rho}}), \dots, (\check{I}_K, \Lambda_K^{\hat{\rho}})\}$  where  $\Lambda_k^{\hat{\rho}}$  is the union of all Finnish essential roots (without vowel blotting) available to  $\Gamma_k$ , for  $k \in \mathbb{Z} \cap [1, K]$ . Set  $\Lambda^{\hat{\rho}} = \Lambda_1^{\hat{\rho}} \cup \dots \cup \Lambda_K^{\hat{\rho}}$ , and evaluate  $\text{CpdDet}(\Lambda^{\hat{\rho}})$ .
- (4) The first component  $\hat{\rho}_{(q')}$  of each triplet  $(\hat{\rho}_{(q')}, \hat{\eta}_{(q')}, \lambda_{(q')}^{\hat{\tau}})$  in  $\text{CpdDet}(\Lambda^{\hat{\rho}})$  is called a “dissolvable compound”, the second component  $\hat{\eta}_{(q')}$  a “heuristic head”, and the first member in the third component  $\lambda_{(q')}^{\hat{\tau}}$  a “heuristic tail”. In the tagged list  $\{(\check{I}_1, \Lambda_1^{\hat{\rho}}), \dots, (\check{I}_K, \Lambda_K^{\hat{\rho}})\}$ , every entry containing a “dissolvable compound” is removed, and regrouped with the entries matching its “heuristic head” and “heuristic tail”. Finally, remove all tags.

*Example 8.14.1.* If we have the inflected compound words from the aforementioned KOTUS-51 sample (containing 27 words), as well as the words *nuori* “young” and *pari* “couple”, then our heuristic compound detection generates the following output:

*{nuoreenpariin, nuoreksipariksi, nuorellaparilla, nuorelleparille, nuoreltaparilta, nuorenaparina, nuorenaparin, nuoressaparissa, nuorestaparista, nuoretparit, nuorettaaparitta, nuorienparien, nuoriinpareihin, nuoriksipareiksi, nuorinapareina, nuorinepareineen, nuorinparein, nuoripari, nuorissapareissa, nuoristapareista, nuorittapareitta, nuortaparia, nuortenparien, pari}* — 24 words;

*{nuoreenpariin, nuoreksipariksi, nuorellaparilla, nuorelleparille, nuoreltaparilta, nuorenaparina, nuorenaparin, nuoressaparissa, nuorestaparista, nuoretparit, nuorettaaparitta, nuori, nuoriapareja, nuorienparien, nuoriinpareihin, nuoriksipareiksi, nuorillapareilla, nuorillepareille, nuoriltapareilta, nuorinapareina, nuorinepareineen, nuorinparein, nuoripari, nuorissapareissa, nuoristapareista, nuorittapareitta, nuortaparia, nuortenparien}* — 28 words.

This is partially satisfactory: a small fraction of the compounds were not decomposed properly (component *pari* undetected), but were simply regarded as derivatives of the word *nuori*. If we have *nuorin* “youngest” instead of *nuori* “young” in our input, then we get something slightly worse:

{*nuoriapareja*} — 1 word;

{*nuoreenpariin, nuoreksipariksi, nuorellaparilla, nuorelleparille, nuoreltaparilta, nuorenaparina, nuorenaparin, nuoressaparissa, nuorestaparista, nuoretparit, nuorettaparitta, nuorienparien, nuoriinpareihin, nuoriksipareiksi, nuorinepareineen, nuorinparein, nuoripari, nuorissapareissa, nuoristapareista, nuorittapareitta, nuortaparia, nuortenparien, pari*} — 23 words;

{*nuoreenpariin, nuoreksipariksi, nuorellaparilla, nuorelleparille, nuoreltaparilta, nuorenaparina, nuorenaparin, nuoressaparissa, nuorestaparista, nuoretparit, nuorettaparitta, nuorienparien, nuoriinpareihin, nuoriksipareiksi, nuorillapareilla, nuorillepareille, nuoriltapareilta, nuorin, nuorinapareina, nuorinepareineen, nuorinparein, nuoripari, nuorissapareissa, nuoristapareista, nuorittapareitta, nuortaparia, nuortenparien*} — 27 words.

*Example 8.14.2.* In Fig. S12, we further test the aforementioned word clustering algorithm (with heuristic detection of compounds) on topic extraction and machine translation (see Table S1 for text sources).

*Peni(n)kulma* is an archaic measure of length used in Finland. Although this is not numerically equivalent to the English *mile*, we consider these length units exact matches in Fig. S12b' and b''.

In Darwin's *Origin of Species*, the word “fresh” is generally used in the context of *fresh water* and the word “reciprocal” is mostly used in the phrase *reciprocal cross*. Therefore, we consider *suolattoman* (genitive singular of *suolaton* “saltless”) an exact match to *fresh* and *vastavuoroinen* “reciprocal” a close match to *graft* in Fig. S12b''. Similarly, we regard *siitoselimistö* “breeding organ” as a near synonym to *reciprocal*.

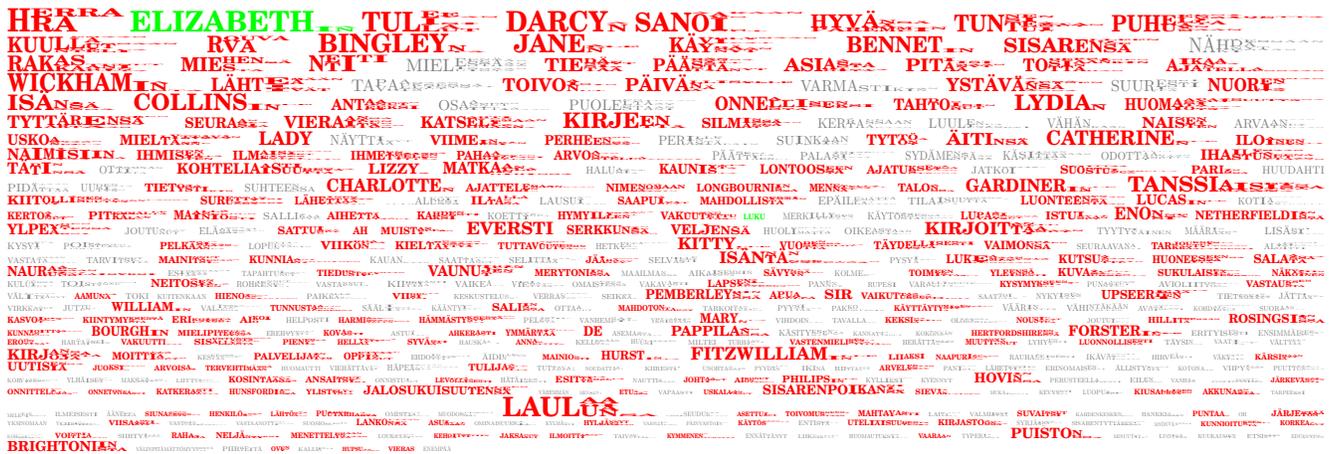

(a)

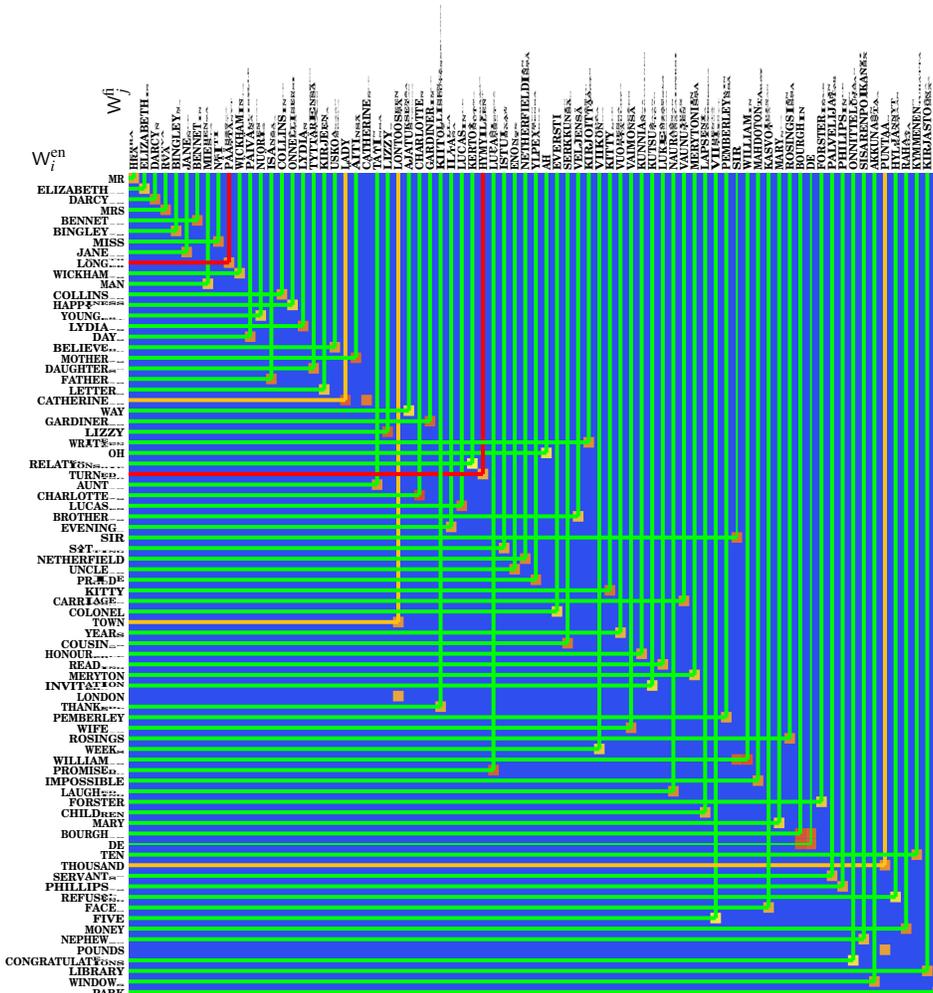

(b)

Fig. S12. Text mining in Finnish. (a) Statistically identified topics ( $n_{ii} \geq 20$ ) in a Finnish version of *Pride and Prejudice*, with the same color encoding scheme as Fig. S3. (b) Semantic similarities  $s(W_i^{en}, W_j^{fi})$  between selected topics in English and Finnish versions of *Pride and Prejudice*. Cross-hairs meet at optimal nodes that solve the bipartite matching problem. The thickness of each horizontal (resp. vertical) cross-hair is inversely proportional to the row-wise (resp. column-wise) ranking of the similarity score for the optimal node. Green (resp. red) cross-hair indicates a correct (resp. incorrect) match. Amber cross-hair marks a link between distinct concepts that share the same hypernyms.





## 8.2 Modified Porter stemming algorithm for Hungarian

In our presentation below, we will disable hyphenation for all the Hungarian words. There are two reasons for doing so: (1) The hyphenation rules for Hungarian are both complex and counterintuitive, which may baffle non-Hungarian readers of this document. (2) The Hungarian language option in the  $\LaTeX$  `babel` package is incompatible with many other  $\LaTeX$  packages, which discourages us from loading it.

**Definition 8.15** (Hungarian stop words). If a word, up to removal of  $\sim e$  (hyphen and the letter  $e$ , attached at the end<sup>100</sup>), belongs to the following list<sup>101</sup>:

*a, abban, ahhoz, ahogy, ahogyan, ahol, ahonnan, ahonnét, ahova, akár, akárhol, akárhonnán, akárhonnét, akárhova, aki, akik, akkor, aközben, alá, alád, alájuk, alám, alánk, alátok, alatt, alatta, alattad, alattam, alattatok, alattuk, alattunk, alig, aligha, alighanem, alighogy, alól, alóla, alólad, alólam, alólatok, alóluk, alólunk, által, általa, általában, általad, általam, általatok, általuk, általunk, alul, amely, amelyek, amelyekben, amelyeket, amelyet, amelynek, ami, amíg, amikor, amint, amit, amolyan, annak, annyi, annyiba, annyiban, annyiból, annyiért, annyihez, annyiig, annyiként, annyin, annyinak, annyinál, annyira, annyiról, annyiszor, annyit, annyitól, annyivá, annyival, arra, arról, át, az, azaz, azért, azok, azon, azonban, azt, aztán, azután, azzal, azzonal, bár, bárcsak, bárhogy, bárhol, bárhonnán, bárhonnét, bárhova, bármikor, be, belé, beléd, beléjük, belém, belénk, belétek, beljebb, belőle, belőled, belőlem, belőletek, belőlük, belőlünk, belül, benn, benne, benned, bennem, bennetek, benneteket, bennük, bennünk, bennünket, bent, bizony, cikk, cikkek, cikkeket, csak, csaknem, csinál, csinálendő, csináld, csinálhat, csinálj, csinálja, csináljad, csináljak, csinálják, csináljal, csináljalak, csináljam, csináljanak, csináljatok, csináljátok, csináljon, csináljuk, csináljunk, csinállak, csinálna, csinálná, csinálnád, csinálnak, csinálnák, csinálnál, csinálnálak, csinálnám, csinálnának, csinálnánk, csinálnátok, csinálnék, csinálni, csinálnia, csinálniuk, csinálnod, csinálnom, csinálnotok, csinálnunk, csináló, csinálod, csinálok, csinálom, csinálsz, csinált, csinálta, csináltad, csináltak, csinálták, csináltál, csináltalak, csináltam, csináltatok, csináltátok, csináltok, csináltuk, csináltunk, csinálunk, csinálva, de, dehát, dehogy, e, ebben, eddig, egész, egy, egybe, egyben, egyből, egye, egyéb, egyébként, egyed, egyem, egyen, egyért, egyes, egyet, egyetek, egyetlen, eggyé, eggyel, egyhez, egyig, egyik, egyikbe, egyikben, egyikből, egyike, egyiked, egyikek, egyikekbe, egyikekben, egyikekből, egyikeken, egyikekért, egyikeket, egyikekhez, egyikekig, egyikekké, egyikekkel, egyikekként, egyikeknek, egyikeknél, egyikekre, egyikekről, egyikektől, egyikem, egyikem, egyikért, egyiket, egyiketek, egyikhez, egyikig, egyikké, egyikkel, egyikként, egyiknek, egyiknél, egyikre, egyikről, egyiktől, egyikük, egyikünk, egyként, egymás, egymásba, egymásban, egymásból, egymásért, egymáshoz, egymásig, egymásként, egymásnak, egymásnál, egymáson, egymásra, egymásról, egymással, egymással, egymástól, egynek, egynél, egyre, egyről, egytől, együk, együnk, együtt, ehhez, ekkor, eközben, el, elé, eléd, elég, eléjük, elem, elénk, elétek, ellen, ellenben, ellene, ellened, ellenem, ellenére, ellenetek, ellenük, ellenünk, elő, elől, előle, előled, előlem, előletek, előlük, előlünk, először, előtt, előtte, előtted, előttem, előtetek, előttük, előttünk, első, emilyen, én, énből, engem, ennek, éppen, erre, érte, érted, értem, értetek, értük, értünk, és, esetében, esetekben, esetemben, esetén, esetetekben, esetleg, esetükben, esetünkben, ez, ezek, ezen, ezért, ezt, ezzel, fel, fele, felé, feléd, feléjük, felém, felénk, felétek, felett, felől, felőle, felőled, felőlem, felőletek, felőlük, felőlünk, felül, fenn, fent, fenti, fentibe, fentiben, fentiből, fentiek, fentiekbe, fentiekben, fentiekből, fentieken, fentiekért, fentieket, fentiekhez, fentiekig, fentiekké, fentiekkel, fentiekként, fentieknek, fentieknél, fentiekre, fentiekről, fentiektől, fentiért, fentihez, fentiig, fentiként, fentin, fentinek, fentinél, fentire, fentiről, fentit, fentitől, fentivé, fentivel, fog, fogja, fogják, fogjátok, fogjuk, fognak, fogod, fogok, fogom, fogsz, fogtok, fogunk, fogva, folyamán, folytán, föl, fölé, föled, föléjük, fölem, fölénk, föletek, följobb, fölött, fölötte, fölötted, fölöttem, fölöttetek, fölöttük, fölöttünk, fölül, fölüle, fölüled, fölülelem, fölületek, fölülük, fölülünk, gyanánt, ha, hadd, hanem, hány, hasonlóan, hát, hátha, helyett, helyette, helyetted, helyettem, helyettetek, helyettük, helyettünk, hiszen, hogy, hogyan, hogyha, hogyne, hol, holott, honnan, honnét, hosszát, hova, hozzá, hozzád, hozzájuk, hozzám, hozzánk, hozzátok, ide, időközben, igen, így, ill, ill., illetve, ily, ilyen, ilyenkor, innen, iránt, iránta, irántad, irántam, irántatok, irántuk, irántunk, is, ismét, ison, itt, jóvoltából, kedvéért, kegyed, kegyedbe, kegyedben, kegyedből, kegyeddé, kegyeddel, kegyeden, kegyedért, kegyedet, kegyedhez, kegyedig, kegyedként, kegyednek, kegyednél, kegyedre, kegyedről, kegyedtől, kell, kellett, képest, keressünk, keresztül, kezdve, ki, kijebb, kinn, kint, kivéve, kívül, köré, köréd, köréjük, körém, körénk, körétek, körül, körülötte, körülöttem, körülöttetek, körülöttük, körülöttünk, következtében, közben, közbeni, közé, közéd, közéjük, közém, közénk, közétek, között, közöttte, közötted, közötttem, közöttetek, közöttük, közöttünk, közt, közte, közted, köztem, köztetek, köztüik, köztünk, közül, közüle, közüled, közülem, közületek, közülük, közülünk, különben, le, leendő, legalább, légy, legyek, legyél, legyen, legyenek, legyetek, legyünk, lehet, lehetett, lejjebb, lenn, lenne, lenned, lennék, lennél, lennem, lennének, lennék, lennetek,*

<sup>100</sup>Word final  $\sim e$  occurs in Hungarian tag questions.

<sup>101</sup>Our list of Hungarian stop words is based on <http://snowball.tartarus.org/algorithms/hungarian/stop.txt> (prepared by Anna Tordai), with extensive additions to roughly match their counterparts in English. Although the words *jó* “good”, *jobb* “better”, *jól* “well”, *nagy* “big”, *nagobb* “bigger”, *új* “new”, *újabb* “newer” showed up in Anna Tordai’s list of Hungarian stop words, they do not appear in our list here, for the sake of consistency with other languages.











**Algorithm 8.22** (Admissible suffix mismatch and vowel alternation). For two strings  $\hat{\alpha}$  and  $\hat{\beta}$ , the Boolean-valued function

$$\text{AdmMut}(\text{RootNW}(\hat{\alpha}, \hat{\beta}), \text{SuffixNW}(\hat{\alpha}, \hat{\beta}), \text{NW}^*(\hat{\alpha}, \hat{\beta}))$$

returns **TRUE** if at least one of the following two conditions holds:

- (i)  $\text{SuffixNW}(\hat{\alpha}, \hat{\beta}) = [\emptyset | \mathbf{V}k, \emptyset | \mathbf{V}k]$  **AND**  $(\text{NW}^*(\hat{\alpha}, \hat{\beta}) = [\emptyset, e] | [\emptyset, o] | [\emptyset, \ddot{o}] | [a, \acute{a}] | [e, \acute{e}] | [o, \acute{o}]$  **OR**  $\text{NW}^*(\hat{\beta}, \hat{\alpha}) = [\emptyset, e] | [\emptyset, o] | [\emptyset, \ddot{o}] | [a, \acute{a}] | [e, \acute{e}] | [o, \acute{o}]$  **OR**  $(\text{NW}^*(\hat{\alpha}, \hat{\beta}) = \emptyset$  **AND** the lowercase form of  $\text{RootNW}(\hat{\alpha}, \hat{\beta})$  contains at least one instance of  $\mathbf{V}$ );
- (ii)  $\text{NW}^*(\hat{\alpha}, \hat{\beta}) = \emptyset$  **AND**  $\text{SuffixNW}'(\hat{\alpha}, \hat{\beta}) = [a, \acute{o}] | [ava, \acute{o}] | [\ddot{o}, \ddot{o}] | [\ddot{o}ve, \ddot{o}]$ , where one obtains  $\text{SuffixNW}'(\hat{\alpha}, \hat{\beta})$  by doing  $\sim(k|st|v) \rightarrow \emptyset$  on both components of  $\text{SuffixNW}(\hat{\alpha}, \hat{\beta})$ .

Similarly, one can evaluate another Boolean-valued function

$$\text{AdmMut}(\text{RootSW}(\hat{\alpha}, \hat{\beta}), \text{SuffixSW}(\hat{\alpha}, \hat{\beta}), \text{SW}^*(\hat{\alpha}, \hat{\beta}))$$

by trading all the occurrences of **NW** in the statements above with **SW**.

**Algorithm 8.23** (Heredity test function). The structure of the Hungarian heredity test function  $\text{HrdTest}(\hat{\alpha}, \hat{\beta})$  is identical to the German version (Algorithm 8.1.2), except that the functions  $\text{SimpHrdTest}$ ,  $\text{RootNW}$ ,  $\text{SuffixNW}$ ,  $\text{NW}^*$ ,  $\text{RootSW}$ ,  $\text{SuffixSW}$ ,  $\text{SW}^*$  must follow the Hungarian rules stated above.

The structure of the following clustering algorithm differs from the Finnish counterpart only in cosmetic details.

**Algorithm 8.24** (Approximate clustering of Hungarian words). The approximate clustering of a list of Hungarian words  $\{\hat{\alpha}_1, \dots, \hat{\alpha}_N\}$  is completed in two stages:

- (1) We sort the list  $\{(\hat{\alpha}_1, \text{EffSpell}(\hat{\alpha}_1), \text{RdFinLV}(\text{EffSpell}(\hat{\alpha}_1))), \dots, (\hat{\alpha}_N, \text{EffSpell}(\hat{\alpha}_N), \text{RdFinLV}(\text{EffSpell}(\hat{\alpha}_N)))\}$  alphabetically according to the third component (with higher priority) and the second component (with lower priority). If two consecutive neighbors in the alphabetized list  $\{(\hat{\alpha}_{(1)}, \text{EffSpell}(\hat{\alpha}_{(1)}), \text{RdFinLV}(\text{EffSpell}(\hat{\alpha}_{(1)}))), \dots, (\hat{\alpha}_{(N)}, \text{EffSpell}(\hat{\alpha}_{(N)}), \text{RdFinLV}(\text{EffSpell}(\hat{\alpha}_{(N)})))\}$  satisfies both  $\text{HrdTest}(\text{EffSpell}(\hat{\alpha}_{(n)}), \text{EffSpell}(\hat{\alpha}_{(n+1)})) = \mathbf{FALSE}$  and  $\text{HrdTest}(\text{EffSpell}(\hat{\alpha}_{(n+1)}), \text{EffSpell}(\hat{\alpha}_{(n)})) = \mathbf{FALSE}$ , where  $n \in \mathbb{Z} \cap [1, N)$ , then add a demarcation line between these two entries. In this way, the alphabetized list is divided into separate groups of words with tags:  $\{g_1 = \{(\hat{\alpha}_{(1,1)}, \text{EffSpell}(\hat{\alpha}_{(1,1)}), \dots), \dots, (\hat{\alpha}_{(1,n_1)}, \text{EffSpell}(\hat{\alpha}_{(1,n_1)}), \dots)\}, \dots, g_M = \{(\hat{\alpha}_{(M,1)}, \text{EffSpell}(\hat{\alpha}_{(M,1)}), \dots), \dots, (\hat{\alpha}_{(M,n_M)}, \text{EffSpell}(\hat{\alpha}_{(M,n_M)}), \dots)\}$ , where each sublist also preserves alphabetic order. In particular, we have  $\hat{\alpha}_{(1,1)} = \hat{\alpha}_{(1)}$  and  $\hat{\alpha}_{(M,n_M)} = \hat{\alpha}_{(N)}$ .
- (2) For each group of words  $g_m = \{(\hat{\alpha}_{(m,1)}, \text{EffSpell}(\hat{\alpha}_{(m,1)}), \dots, (\hat{\alpha}_{(m,n_m)}, \text{EffSpell}(\hat{\alpha}_{(m,n_m)}))\}$  where  $m \in \mathbb{Z} \cap [1, M]$ , we augment it into a tagged entry  $G_m = (g_m, \text{EffSpell}(\hat{\alpha}_{(m,1)}), \text{EssRoot}(\text{EffSpell}(\hat{\alpha}_{(m,1)})), T_m)$ , where

$$T_m = \text{RdFinLV}(\text{EssRoot}(\text{EffSpell}(\hat{\alpha}_{(m,1)}))).$$

The list  $\{G_1, \dots, G_M\}$  is sorted alphabetically, with respect to  $T_m$  (with highest priority),  $\text{EssRoot}(\text{EffSpell}(\hat{\alpha}_{(m,1)}))$  (with medium priority), and  $\text{EffSpell}(\hat{\alpha}_{(m,1)})$  (with lowest priority). If two consecutive neighbors in the alphabetized list  $\{G_{(1)} = (g_{(1)}, \hat{\gamma}'_{(1)}, \hat{\gamma}''_{(1)}, \hat{\gamma}'''_{(1)}), \dots, G_{(M)} = (g_{(M)}, \hat{\gamma}'_{(M)}, \hat{\gamma}''_{(M)}, \hat{\gamma}'''_{(M)})\}$  satisfy

$$\text{HrdTest}(\hat{\gamma}''_{(m)}, \hat{\gamma}''_{(m+1)}) = \mathbf{FALSE}$$

**AND**

$$\text{HrdTest}(\hat{\gamma}'_{(m)}, \hat{\gamma}'_{(m+1)}) = \mathbf{FALSE}$$

where  $m \in \mathbb{Z} \cap [1, M)$ , then add a demarcation line between these two entries. In this manner, the alphabetized list  $\{G_{(1)}, \dots, G_{(M)}\}$  is divided into separate groups of tagged clusters  $\{\Gamma_1 = \{G_{(1,1)}, \dots, G_{(1,m_1)}\}, \dots, \Gamma_K = \{G_{(K,1)}, \dots, G_{(1,m_K)}\}\}$ . Finally, generate a list of word clusters  $\{\check{I}_1 = (\check{G}_{(1,1)}, \dots), \dots, \check{I}_K = (\check{G}_{(K,1)}, \dots)\}$  by discarding all the tags.

*Example 8.24.1.* The following samples of regular nouns (declined in all cases, in singular and plural) are extracted from [48, Appendix 2].

*álmaitok, álmaitokat, álmaitokba, álmaitokban, álmaitokból, álmaitokért, álmaitokhoz, álmaitokig, álmaitokká, álmaitokkal, álmaitoknak, álmaitoknál, álmaitokon, álmaitokra, álmaitokról, álmaitoktól, álmotok, álmotokat, álmotokba, álmotokban, álmotokból, álmotokért, álmotokhoz, álmotokig, álmotokká, álmotokkal, álmotokként, álmotoknak, álmotoknál, álmotokon, álmotokra, álmotokról, álmotoktól, álom* — “your dream”;

*bokor, bokorba, bokorban, bokorból, bokorért, bokorhoz, bokorig, bokorként, bokornak, bokornál, bokorra, bokorra, bokorral, bokorról, bokortól, bokrok, bokrokat, bokrokba, bokrokban, bokrokból, bokrokért, bokrokhoz, bokrokig, bokrokká, bokrokkal, bokrokként, bokroknak, bokroknál, bokrokon, bokrokra, bokrokról, bokroktól, bokron, bokronként, bokrostul, bokrot* — “bush”;

*dinnye, dinnyébe, dinnyében, dinnyéből, dinnyéért, dinnyéhez, dinnyéig, dinnyék, dinnyékbe, dinnyékben, dinnyékből, dinnyéken, dinnyeként, dinnyékért, dinnyéket, dinnyékhez, dinnyékig, dinnyékké, dinnyékkel, dinnyékként, dinnyéknek, dinnyéknél, dinnyékre, dinnyékről, dinnyéktől, dinnyén, dinnyének, dinnyénél, dinnyénként, dinnyére, dinnyéről, dinnyéstül, dinnyét, dinnyétől, dinnyévé, dinnyével* — “melon”;

*ház, házak, házakat, házakba, házakban, házából, házakért, házakhoz, házakig, házakká, házakkal, házakként, házaknak, házaknál, házakon, házakra, házokról, házaktól, házanként, házastul, házat, házba, házban, házból, házért, házhoz, házig, házként, háznak, háznál, házon, házra, házról, háztól, házzá, házzal* — “house”;

*ház, házaim, házaimat, házaimba, házaimban, házaimból, házaimért, házaimhoz, házaimig, házaimmá, házaimmal, házaimnak, házaimnál, házaimon, házaimra, házaimról, házaimtól, házám, házamat, házamba, házamban, házamból, házamért, házámhoz, házámig, házámként, házammá, házammal, házamnak, házamnál, házamon, házamra, házamról, házamtól* — “my house”;

*iker, ikerbe, ikerben, ikerből, ikerért, ikerhez, ikerig, ikerként, ikernek, ikernél, ikerre, ikerré, ikerrel, ikerről, ikertől, ikrek, ikrekbe, ikrekben, ikrekből, ikreken, ikrekért, ikreket, ikrekhez, ikrekig, ikrekke, ikrekkel, ikreként, ikreknek, ikreknél, ikrekre, ikrekről, ikrektől, ikren, ikrenként, ikrestül, ikret* — “twin”;

*jutalmaink, jutalmainkat, jutalmainkba, jutalmainkban, jutalmainkból, jutalmainkért, jutalmainkhoz, jutalmainkig, jutalmainkká, jutalmainkkal, jutalmainknak, jutalmainknál, jutalmainkon, jutalmainkra, jutalmainkról, jutalmaintól, jutalmunk, jutalmunkat, jutalmunkba, jutalmunkban, jutalmunkból, jutalmunkért, jutalmunkhoz, jutalmunkig, jutalmunkká, jutalmunkkal, jutalmunkként, jutalmunknak, jutalmunknál, jutalmunkon, jutalmunkra, jutalmunkról, jutalmunktól, jutalom* — “our reward”;

*kép, képeik, képeikbe, képeikben, képeikből, képeiken, képeikért, képeiket, képeikhez, képeikig, képeikké, képeikkel, képeiknek, képeiknél, képeikre, képeikről, képeiktől, képük, képükbe, képükben, képükből, képükért, képüket, képükhöz, képükig, képükké, képükkel, képüként, képüknek, képüknél, képükön, képükre, képükről, képüktől* — “their picture”;

*kéz, kézbe, kézben, kézből, kezek, kezekbe, kezekben, kezekből, kezeken, kezekért, kezeket, kezekhez, kezekig, kezekké, kezekkel, kezeként, kezeknek, kezeknél, kezekre, kezekről, kezeiktől, kézen, kezenként, kézért, kezestül, kezet, kézhez, kézig, kézként, kéznek, kéznél, kézre, kézről, kéztől, kézzé, kézzel* — “hand”;

*kő, kőbe, kőben, kőből, kőért, kőhöz, kőig, kőként, kőnek, kőnél, kőre, kőről, kőtől, kővé, kővek, kővekbe, kővekben, kővekből, kőveken, kővekért, kőveket, kővekhez, kővekig, kővekké, kővekkel, kővekként, kőveknek, kőveknél, kővekre, kővekről, kővektől, kővel, kővenként, kővestül, követ, kövön* — “stone”;

*könyv, könyvbe, könyvben, könyvből, könyvek, könyvekbe, könyvekben, könyvekből, könyveken, könyvekért, könyveket, könyvekhez, könyvekig, könyvekké, könyvekkel, könyvekként, könyveknek, könyveknél, könyvekre, könyvekről, könyvektől, könyvenként, könyvért, könyvestül, könyvet, könyvhöz, könyvig, könyvként, könyvnek, könyvnél, könyvön, könyvre, könyvről, könyvtől, könyvvé, könyvvel* — “book”;

*lány, lányastul, lányba, lányban, lányból, lányért, lányhoz, lányig, lányként, lánynak, lánynál, lánnyá, lánnyal, lányok, lányokat, lányokba, lányokban, lányokból, lányokért, lányokhoz, lányokig, lányokká, lányokkal, lányokként, lányoknak, lányoknál, lányokon, lányokra, lányokról, lányoktól, lányon, lányonként, lányra, lányról, lányt, lánytól* — “girl”;

*levél, leveled, leveledbe, leveledben, leveledből, leveleddé, leveleddel, leveleden, leveledért, leveledet, leveledhez, leveledig, leveledként, levelednek, levelednél, leveledre, leveledről, leveledtől, leveleid, leveleidbe, leveleidben, leveleidből, leveleiddé, leveleiddel, leveleiden, leveleidért, leveleidet, leveleidhez, leveleidig, leveleidnek, leveleidnél, leveleldre, leveleldről, leveleidtől* — “your letter”;

*lova, lovába, lovában, lovából, lováért, lovához, lovai, lovaiba, lovaiban, lovaiból, lovaiért, lováig, lovaihoz, lovaiig, lovaiként, lovain, lovainak, lovainál, lovaira, lovaíró, lovait, lovaitól, lovaivá, lovaival, lovaként, lován, lovának, lovánál, lovára, lováról, lovát, lovától, lovává, lovával* — “his/her horse”;



*édes, édesebb* — “sweet”;

*érthető, érthetőbb* — “understandable”;

*fekete, feketébb* — “black”;

*hosszabb, hosszú* — “long”;

*hű, hűbb* — “faithful”;

*ifjabb, ifjú* — “young”;

*jó, jobb* — “good”;

*keserű, keserűbb* — “bitter”;

*kevés, kevesebb* — “few”;

*kicsi, kisebb* — “small”;

*könnyebb, könnyű* — “easy”;

*különös, különösebb* — “special”;

*lassabb, lassú* — “slow”;

*nehéz, nehezebb* — “difficult”;

*olcsó, olcsóbb* — “cheap”;

*piros, pirosabb* — “red”;

*régi, régibb* — “old”;

*szébb, szép* — “beautiful”;

*szomorú, szomorúbb* — “sad”;

*szörnyebb, szörnyű* — “awful”.

Our clustering algorithm groups these adjectives correctly.

*Example 8.24.2.* Our sample of regular Hungarian verbs are chosen from a representative subset of [48, §4.1], so as to cover all the possible regular verb typologies.

*cselekedd, cselekeded, cselekedek, cselekedem, cselekedendő, cselekedett, cselekedhet, cselekedni, cselekedik, cselekeditek, cselekedj, cselekedje, cselekedjed, cselekedjek, cselekedjék, cselekedjél, cselekedjelek, cselekedjem, cselekedjen, cselekedjenek, cselekedjete, cselekedjétek, cselekedjük, cselekedjünk, cselekedlek, cselekedne, cselekedné, cselekedned, cselekednéd, cselekednek, cselekednék, cselekednél, cselekednélek, cselekednem, cselekedném, cselekednének, cselekednénk, cselekednetek, cselekednétek, cselekedni, cselekednie, cselekedniük, cselekednünk, cselekedő, cselekedsz, cselekedte, cselekedted, cselekedtek, cselekedték, cselekedtél, cselekedtelek, cselekedtem, cselekedtetek, cselekedtétek, cselekedtük, cselekedtünk, cselekedünk, cselekedve, cselekszed, cselekszel, cselekszem, cselekszenek, cselekszete, cselekszi, cselekszik, cselekszitek, cselekszünk, cselekvő* — “act”;

*emlékezek, emlékezel, emlékezett, emlékezhetsz, emlékezne, emlékezned, emlékeznek, emlékeznék, emlékeznél, emlékezniem, emlékeznének, emlékeznénk, emlékeznetek, emlékeznétek, emlékezni, emlékeznie, emlékezniük, emlékeznünk, emlékező, emlékeztetek, emlékeztél, emlékeztem, emlékeztetek, emlékeztünk, emlékeznünk, emlékezve, emlékezz, emlékezzek, emlékezzél, emlékezzen, emlékezzenek, emlékezzetek, emlékezzünk, emlékszel, emlékszem, emlékszenek, emlékszete, emlékszik, emlékszünk* — “remember”;

*gyarapodhat, gyarapodik, gyarapodj, gyarapodjak, gyarapodjál, gyarapodjanak, gyarapodjatok, gyarapodjon, gyarapodjunk, gyarapodna, gyarapodnak, gyarapodnál, gyarapodnának, gyarapodnánk, gyarapodnátok, gyarapodnék, gyarapodni, gyarapodnia, gyarapodniuk, gyarapodnod, gyarapodnom, gyarapodnotok, gyarapodnunk, gyarapodó, gyarapodok, gyarapodott, gyarapodsz, gyarapodtak, gyarapodtál, gyarapodtam, gyarapodtatok, gyarapodtok, gyarapodtunk, gyarapodunk, gyarapodva* — “increase”;

*igyekezek, igyekezel, igyekezett, igyekezhet, igyekezne, igyekezned, igyekeznek, igyekeznék, igyekeznél, igyekeznem, igyekeznének, igyekeznénk, igyekeznetek, igyekeznétek, igyekezni, igyekeznie, igyekezniük, igyekezniük, igyekező, igyekeztek, igyekeztél, igyekeztem, igyekeztetek, igyekeztiük, igyekezünk, igyekezve, igyekezz, igyekezzek, igyekezzél, igyekezzen, igyekezzenek, igyekezzetek, igyekezzüink, igyekszel, igyekszem, igyekszenek, igyekszetek, igyekszik, igyekszüink, igyekvő — “strive”;*

*mosolygandó, mosolygó, mosolygod, mosolygok, mosolygom, mosolygott, mosolygunk, mosolyog, mosolyogd, mosolyoghat, mosolyogj, mosolyogja, mosolyogjad, mosolyogjak, mosolyogják, mosolyogjál, mosolyogjalak, mosolyogjam, mosolyogjanak, mosolyogjatok, mosolyogjátok, mosolyogjon, mosolyogjuk, mosolyogjunk, mosolyoglak, mosolyogna, mosolyogná, mosolyognád, mosolyognak, mosolyognák, mosolyognál, mosolyognálak, mosolyognám, mosolyognának, mosolyognánk, mosolyognátok, mosolyognék, mosolyogni, mosolyognia, mosolyogniuk, mosolyognod, mosolyognom, mosolyognotok, mosolyognunk, mosolyogsz, mosolyogta, mosolyogtad, mosolyogtak, mosolyogták, mosolyogtál, mosolyogtalak, mosolyogtam, mosolyogtatok, mosolyogtátok, mosolyogtok, mosolyogtuk, mosolyogtunk, mosolyogva — “smile”;*

*sző, sződd, szőj, szője, szőjed, szőjek, szőjék, szőjél, szőjelek, szőjem, szőjenek, szőjetek, szőjétek, szőjön, szőjük, szőjünk, szőlek, szőne, szőné, szőnéd, szőnek, szőnék, szőnél, szőnélek, szőném, szőnének, szőnénk, szőnétek, szőni, szőnie, szőniük, szőnöd, szőnöm, szőnötök, szőnünk, szősz, szőtt, szötte, szötted, szötték, szötték, szöttél, szöttetek, szöttetek, szöttétek, szöttök, szöttük, szöttünk, szöve, szövendő, szövi, szövik, szövitek, szövő, szövöd, szövök, szövöm, szöviük — “weave”;*

*utazhat, utazik, utazna, utaznak, utaznál, utaznának, utaznánk, utaznátok, utaznék, utazni, utaznia, utazniuk, utaznod, utaznom, utaznotok, utaznunk, utazó, utazok, utazol, utazom, utazott, utaztak, utaztál, utaztam, utaztatok, utaztok, utaztunk, utazunk, utazva, utazz, utazzak, utazzál, utazzanak, utazzatok, utazzon, utazzunk — “travel”.*

These verbs are clustered correctly by our algorithm.

Our selection of irregular Hungarian verbs are based on [48, Appendix 1].

*edd, egve, egyed, egyek, egyék, egyél, egyelek, egyem, egyen, egyenek, egyetek, egyétek, együk, együnk, ehét, enne, enné, enned, ennéd, ennék, ennél, ennélek, ennem, enném, ennének, ennének, ennetek, ennétek, enni, ennie, enniük, enniük, eszed, eszek, eszel, eszem, eszi, eszik, eszitek, eszlek, esznek, esszük, esztek, eszünk, ette, etted, ettek, ették, etél, ettelek, ettem, ettetek, ettétek, ettük, ettünk, evett, evő — “eat”;*

*gyere, gyertek, gyeriük, jöhet, jöjj, jöjjenek, jöjjél, jöjjenek, jöjjetek, jöjjön, jöjjünk, jön, jönne, jönnek, jönnék, jönnél, jönnének, jönnénk, jönnétek, jönni, jönnie, jönniük, jönnöd, jönnöm, jönnötök, jönnünk, jössz, jösztek, jött, jöttek, jöttél, jöttem, jöttetek, jöttök, jöttünk, jöve, jövendő, jövő, jövök, jöviük — “come”;*

*hidd, hiendő, higgy, higgye, higgyed, higgyek, higgyék, higgyél, higgyelek, higgyem, higgyen, higgyenek, higgyetek, higgyétek, higgyük, higgyünk, híhet, hinne, hinné, hinned, hinnéd, hinnék, hinnél, hinnélek, hinnem, hinném, hinnének, hinnénk, hinnenek, hinnenétek, hinni, hinnie, hinniük, hinniük, hisz, hiszed, hiszek, hiszel, hiszem, hiszi, hiszik, hiszitek, hiszlek, hisznek, hisszük, hisztek, hiszünk, hitt, hitte, hitted, hittek, hitték, hittél, hittelek, hittem, hittetek, hittétek, hittük, hittünk — “believe”;*

*idd, igya, igyad, igyak, igyák, igyál, igyalak, igyam, igyanak, igyatok, igyátok, igyon, igyuk, igyunk, ihat, inna, inná, innád, innák, innál, innalak, innám, innának, innánk, innátok, innék, inni, innia, inniuk, innod, innom, innotok, innunk, iszik, iszlak, isznak, iszod, iszok, iszol, iszom, issza, isszák, isszátok, isszük, isztek, iszunk, itta, ittad, ittak, itták, ittál, ittalak, ittam, ittatok, ittátok, ittuk, ittunk, ivandó, ivó, ivott — “drink”;*

*megy, megyek, megyünk, mehet, menj, menjek, menjél, menjen, menjenek, menjetek, menjünk, menne, menned, mennek, mennék, mennél, mennem, mennének, mennénk, mennetek, mennétek, menni, mennie, menniük, menniük, mennünk, menő, ment, mentek, mentél, mentem, mentetek, mentünk, menve — “go”;*

*vedd, veendő, végy, vegye, vegyed, vegyek, vegyék, vegyél, vegyelek, vegyem, vegyen, vegyének, vegyetek, vegyétek, vegyük, vegyünk, vehet, venne, venné, vened, vennéd, vennék, vennél, vennélek, vennem, venném, vennének, vennénk, vennenek, vennenétek, venni, vennie, venniük, venniük, vesz, veszed, veszek, veszel, veszem, veszi, veszik, veszitek, veszlek, vesznek, vesszük, vesztek, veszünk, vett, vette, vetted, vettek, vették, vettél, vettelek, vettem, vettetek, vettétek, vettük, vettünk, véve, vevő — “buy”;*

*vidd, viendő, vigye, vigyed, vigyek, vigyék, vigyél, vigyelek, vigyem, vigyen, vigyének, vigyetek, vigyétek, vigyük, vigyünk, vihet, vinne, vinné, vinned, vinnéd, vinnék, vinnél, vinnélek, vinnem, vinném, vinnének, vinnénk, vinnenek, vinnenétek, vinni, vinnie, vinniük, vinniük, visz, viszed, viszek, viszel, viszem, viszi, viszik, viszitek, viszlek, visznek, viszzük, visztek, viszünk, vitt, vitte, vitted, vittek, vitték, vittél, vittelek, vittem, vittetek, vittétek, vittük, vittünk, vive, vivő — “carry”.*

Sending them to our algorithm, we receive the correct clustering results.

### 8.2.3 Heuristic detection of compounds

The following algorithm for heuristic detection of Hungarian compounds differs from the Danish version (Algorithm 5.12) only in some specific details. To make the context clear, we still state the algorithm in full. (In what follows, the string minus operation  $\hat{\beta} \ominus \hat{\alpha}$  is prescribed by Definition 5.11.)

**Algorithm 8.25** (Heuristic identification of Hungarian binary compounds). *Let  $\Lambda^{\hat{\rho}} = \{\hat{\rho}_1, \dots, \hat{\rho}_Q\}$  be a list of distinct Hungarian essential roots (without vowel blotting) that are at two characters long, contain at least one instance of  $\mathbf{V}$  in the first two letters, and DO NOT match either*

(ag|ar|az|ba|bo|cel|č|de|dö|dul|em|ha|he|hi|ig|is|ka|ke|ko|kő|li|mas|mi|mu|ne|od|ős|rá|re|ta|te|tor|tű|va|vá|vas)

or

(βka|(a|e|o|ö)(s|z)|a|lam|d|ileg|er|ér|fe|fog|hi|kor|mag|meg|ol|or|ot|š $\mathbf{V}$ |ter|ve) $\mathbf{X}$ .

The output of the function  $\text{CpdDet}(\Lambda^{\hat{\rho}})$  is obtained through the following procedures:

- (1) Construct a list  $\{(\hat{\rho}_1, \lambda_1^{\hat{\rho}}), \dots, (\hat{\rho}_Q, \lambda_Q^{\hat{\rho}})\}$  where  $\lambda_q^{\hat{\rho}} = \{\hat{\rho}_{(q,1)}, \dots, \hat{\rho}_{(q,n_q)}\}$  is a subset of  $\Lambda^{\hat{\rho}}$  whose members all match the string pattern  $\hat{\rho}_q \sim$ , for  $q \in \mathbb{Z} \cap [1, Q]$ .
- (2) Expand the aforementioned entry  $(\hat{\rho}_q, \lambda_q^{\hat{\rho}})$  into a list of triplets  $\{(\hat{\rho}_{(q,1)}, \hat{\rho}_q, \hat{\rho}_{(q,1)} \ominus \hat{\rho}_q), \dots, (\hat{\rho}_{(q,n_q)}, \hat{\rho}_q, \hat{\rho}_{(q,n_q)} \ominus \hat{\rho}_q)\}$  for every  $q \in \mathbb{Z} \cap [1, Q]$  such that  $\lambda_q^{\hat{\rho}} \neq \emptyset$ . Collect all these triplets as one runs through the list  $\{(\hat{\rho}_1, \lambda_1^{\hat{\rho}}), \dots, (\hat{\rho}_Q, \lambda_Q^{\hat{\rho}})\}$ . The list of these triplets  $\{(\hat{\rho}_{(1)}, \hat{\eta}_{(1)}, \hat{\rho}_{(1)} \ominus \hat{\eta}_{(1)}), \dots, (\hat{\rho}_{(Q)}, \hat{\eta}_{(Q)}, \hat{\rho}_{(Q)} \ominus \hat{\eta}_{(Q)})\}$  contains potentially valid decompositions of compounds.
- (3) Screen the aforementioned list of triplets as follows: for every  $q' \in \mathbb{Z} \cap [1, Q']$ , if  $(\hat{\rho}_{(q')}, \hat{\eta}_{(q')}, \hat{\tau}_{(q')} = \hat{\rho}_{(q')} \ominus \hat{\eta}_{(q')})$  satisfies

$$\ell(\hat{\rho}_{(q')} \ominus \hat{\eta}_{(q')}) \geq 2 \quad \text{AND} \quad \hat{\rho}_{(q')} \ominus \hat{\eta}_{(q')} = \mathbf{X}_1 \mathbf{V} \mathbf{X}_2,$$

then construct  $\hat{\tau}_{(q')}$  by performing  $(\emptyset|a|e)(\emptyset|i|ñ|i|s|t|ú|ű) \sim \rightarrow \emptyset$  and

$$(\lambda(\emptyset|e|\delta)|a|á|a\delta|ala|be|f(\emptyset|e|e|\acute{e}|l)|h(\acute{a}|e|l|o|z)|id|k(ere|i|ör|öz)|le(\emptyset|n)|meg|neki|od|ős|ra|rá|sél|ser|to|túl|u|vég|vin) \sim \rightarrow \emptyset$$

on  $\hat{\tau}_{(q')}$ , before generating a list  $\lambda_{(q')}^{\hat{\tau}}$  by members of  $\Lambda^{\hat{\rho}}$  that match the pattern  $(\hat{\tau}_{(q')}|\hat{\tau}_{(q')}^*)$ ; otherwise, set  $\lambda_{(q')}^{\hat{\tau}} = \emptyset$ .

- (4) Collect all the triplets  $(\hat{\rho}_{(q')}, \hat{\eta}_{(q')}, \lambda_{(q')}^{\hat{\tau}})$  where  $\lambda_{(q')}^{\hat{\tau}}$  is non-void and  $\hat{\tau}_{(q')}$  DOES NOT match  $z\tau\mathbf{X}$ . This list of triplets  $\text{CpdDet}(\Lambda_{\hat{\rho}})$  contains the heuristic decompositions of all the identified binary compounds.

**Algorithm 8.26** (Approximate clustering of Hungarian words with heuristic detection of compounds). *The approximate clustering of a list of Hungarian words  $\{\hat{\alpha}_1, \dots, \hat{\alpha}_N\}$  respecting compounding is completed in four stages:*

- (1) Do as in Algorithm 8.24(1).
- (2) Do as in Algorithm 8.24(2). Save both the tagged clusters  $\{\Gamma_1 = \{G_{(1,1)}, \dots, G_{(1,m_1)}\}, \dots, \Gamma_K = \{G_{(K,1)}, \dots, G_{(1,m_K)}\}\}$  and the list of word clusters  $\{\check{\Gamma}_1, \dots, \check{\Gamma}_K\}$  for further use.
- (3) Construct a tagged list of word clusters  $\{(\check{\Gamma}_1, \Lambda_1^{\hat{\rho}}), \dots, (\check{\Gamma}_K, \Lambda_K^{\hat{\rho}})\}$  where  $\Lambda_k^{\hat{\rho}}$  is the union of all Hungarian essential roots (without vowel blotting) available to  $\Gamma_k$ , for  $k \in \mathbb{Z} \cap [1, K]$ . Set  $\Lambda^{\hat{\rho}} = \Lambda_1^{\hat{\rho}} \cup \dots \cup \Lambda_K^{\hat{\rho}}$ , and evaluate  $\text{CpdDet}(\Lambda^{\hat{\rho}})$ .
- (4) The first component  $\hat{\rho}_{(q')}$  of each triplet  $(\hat{\rho}_{(q')}, \hat{\eta}_{(q')}, \lambda_{(q')}^{\hat{\tau}})$  in  $\text{CpdDet}(\Lambda^{\hat{\rho}})$  is called a “dissolvable compound”, the second component  $\hat{\eta}_{(q')}$  a “heuristic head”, and the first member in the third component  $\lambda_{(q')}^{\hat{\tau}}$  a “heuristic tail”. In the tagged list  $\{(\check{\Gamma}_1, \Lambda_1^{\hat{\rho}}), \dots, (\check{\Gamma}_K, \Lambda_K^{\hat{\rho}})\}$ , every entry containing a “dissolvable compound” is removed, and regrouped with the entries matching its “heuristic head” and “heuristic tail”. Finally, remove all tags.

*Example 8.26.1.* In Fig. S13, we apply the aforementioned word clustering algorithm to topic extraction and machine translation (see Table S1 for text sources).

According to Hungarian orthography, vowel lengths ( $a$  vs.  $\acute{a}$ ,  $\ddot{o}$  vs.  $\acute{o}$  etc.) are ignored during alphabetization. If implemented as is, stacked vowels in word clusters may become illegible at times. As a compromise, we always sort long vowels after short vowels in Fig. S13.

In Hungarian, *de* “but” is a stop word, so it is understandable that our algorithm does not provide a perfect translation of the proper name *de Bourgh* in Fig. S13b.

In Darwin’s *Origin of Species*, the word “reciprocal” is mostly used in the phrase *reciprocal cross*. Therefore, we consider “reciprocal” and “graft” near synonyms in Fig. S13b”. Furthermore, in Fig. S13b”, sometimes an English word may correspond to a Hungarian phrase or vice versa: we consider English *fresh* an exact match to Hungarian *édesvízi* “fresh water” (literally “sweet water”), and similarly for English *rock-pigeon* and Hungarian *szirti* (the latter being part of the phrase *szirti galamb* that translates *rock-pigeon* into Hungarian).







## 9 Approximate word clustering in various agglutinative languages

Basque, Korean and Turkish are three agglutinative SOV languages with different linguistic ancestors,<sup>104</sup> but they do share a few typological and morphological features:

- All these languages are rich in suffixes, but have almost no prefixes. A typical word in these languages assumes the form of

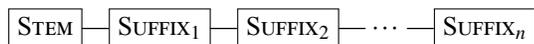

- Typically, the word stem is one or two syllables long.<sup>105</sup> However, due to strong and persisted foreign influences on these languages (French/Spanish on Basque, Chinese/English/Japanese on Korean, Arabic/Persian on Turkish), there are certain exceptions to this estimate. Sometimes, stems of loanwords may be confused with native suffixes, if not handled properly.
- There are hardly any irregular verbs or nouns. Unlike Finnish, the suffixes in these languages (usually) do not cause sound changes upon interactions.
- These languages have more sophisticated systems for kinship terms than typical Indo-European languages. There could be different words for a sibling of a given gender, depending on seniority (Korean) or the gender of the possessor (Basque and Korean); there could be different words for extended family members depending on maternal/paternal sides (Korean and Turkish). Our word clustering algorithms will accommodate to such cultural differences, as much as possible.

### 9.1 Modified Porter stemming algorithm for Basque

Our Basque stemming algorithm is adapted from the method of Mikel Otxandorena (<http://snowball.tartarus.org/algorithms/basque/stemmer.html>). Our modest contributions include the following aspects:

- We add special treatments for the only irregular adjective in Basque: *on* “good” [50, §3.1.3.3].
- We add special routines to cluster finite forms<sup>106</sup> of Basque verbs [50, §3.5.2.1].
- We carefully handle loanwords that begin with *des~*, *err~*, *irr~* and so on.
- We carefully treat the negative suffixes *~gabe* and *~gabea*, which carry similar functions as the English prefix *un~* and suffix *~less*.
- We group Basque kinship terms according to (roughly) their English equivalents.

Basque stop words can carry various agglutinative suffixes. Instead of enumerating all of them in a single list, we will define several string patterns that match the criterion for stop words.

**Definition 9.1** (Basque stop words). Define the pattern **BasqueStopRoot** as any one from the following list:

*aitzin, albo, alde, arte, asko, atze, aurre, azken, azpi, barru, batega, batek, baten, batera, batet, behe, beza, buruzko, dela, denaren, denet, ditu, dizu, eduki, egote, erdi, ere, gain, garen, genieza, genitu, genu, geure, gibel, hain, heure, hieza, hitu, huen, inguru, izan, izate, lizki, neure, nieza, nitu, nuen, ondo, zela, zenieza, zenitu, zenu, zeuen, zeure, zieza, zire, zitu, zizki, zuen.*

Define the pattern **BasqueStopString** as any one from the following list:

*abar, agertutako, agian, ahal, ahaztuak, al, ala, alde, aldera, aplikatuta, arabera, ari, arren, arte, artean, aski, asko, askotan, atzean, atzera, aurka, aurrean, aurrera, aurrerantzean, aurretik, azpian, ba, bada, bagengozkie, bagengozkik, bagengozkin, bagengozkio, bagengozkizu, bagengozkizue, bagenie, bagenik, bagenin, bagenio, bagenizu, bagenizue, bagenkizkie, bagenkizkik, bagenkizkio, bagenkizkizu, bagenkizkizue, bageunde, bagina, bagintez, bagintzaizkie, bagintzaizkik, bagintzaizkin, bagintzaizkio, bagintzaizkizu, bagintzaizkizue, bahendi, bahengo, bahengokie, bahengokigu, bahengokio, bahengokit, bahenkie, bahenkigu, bahenkio, bahenkit, bahie, bahigu, bahintz, bahintzaie, bahintzaigu, bahintzaio, bahintzait, bahio, bahit, bai, baina, baino, baitzen, baizik, bakarrik, bakoitza, baldin, baledi, balego, balegokie, balegokigu, balegokik, balegokin, balegokio, balegokit,*

<sup>104</sup>Some Altaicists believe that both Korean and Turkish descend from the same Proto-Altaic language [49].

<sup>105</sup>Since we do not know, *a priori*, whether the second syllable belongs to the stem or the suffix, a non-trivial stemming algorithm is still necessary.

<sup>106</sup>All but a handful verbs (like “come”, “go”, “say” and “walk”) in Basque can only exist in non-finite forms, which do not involve personal prefixes.

*balegokizu, balegokizue, balegozkie, balegozkigu, balegozkik, balegozkin, balegozkio, balegozkit, balegozkizu, balegozkizue, balekie, balekigu, balekik, balekio, balekit, balekizkie, balekizkigu, balekizkik, balekizkio, balekizkit, balekizkizu, balekizkizue, balekizu, balekizue, baleude, baliabideak, baliatie, balidate, balie, baliatie, baligu, baligute, balik, balin, balinate, balio, balioie, balira, balit, balitez, balitz, balitzaie, balitzaigu, balitzaik, balitzaizain, balitzaio, balitzaiz, balitzaizkie, balitzaizkigu, balitzaizkik, balitzaizkin, balitzaizkio, balitzaizkit, balitzaizkizu, balitzaizkizue, balitzaizu, balitzaizue, balizu, balizue, balizuete, balizute, banendi, banengo, banengokie, banengokik, banengokin, banengokio, banengokizu, banengokizue, banenkie, banenkik, banenkio, banenkizu, banenkizue, banie, banik, banin, banintz, banintzaie, banintzaik, banintzain, banintzaio, banintzaizu, banintzaizue, banio, banizu, banizue, barruan, bat, batean, batera, batez, batzuetan, bazengozkidate, bazengozkie, bazengozkiete, bazengozkigu, bazengozkigute, bazengozkio, bazengozkiote, bazengozkit, bazenidate, bazenie, bazeniete, bazenigu, bazenigute, bazenio, bazenioie, bazenit, bazenkizkidate, bazenkizkie, bazenkizkiete, bazenkizkigu, bazenkizkigute, bazenkizkio, bazenkizkiote, bazenkizkit, bazeunde, bazeundete, bazina, bazinete, bazintez, bazintezte, bazintzaizkidate, bazintzaizkie, bazintzaizkiete, bazintzaizkigu, bazintzaizkigute, bazintzaizkio, bazintzaizkiote, bazintzaizkit, bedi, begira, bego, begozkie, begozkigu, begozkik, begozkin, begozkio, begozkit, begozkizu, begozkizue, behar, beharbada, beharko, beharra, beharrean, behean, behera, behin, bengokie, bengokigu, bengokik, bengokin, bengokio, bengokit, bengokizu, bengokizue, beraz, berea, berean, berez, berri, berriro, berriz, bertan, bestalde, beste, bestela, besterik, betetzera, beti, beude, bezala, biak, bidean, bidez, bihurtu, bihurtuz, bihurtzen, bila, biok, bitartean, bitez, borondatea, burua, buruz, da, dadila, dadin, dago, dagoela, dagoeneko, dagoke, dagokiake, dagokidake, dagokie, dagokieke, dagokigu, dagokiguke, dagokik, dagokin, dagokinake, dagokio, dagokioke, dagokit, dagokizu, dagokizue, dagokizueke, dagokizuke, dagozkiake, dagozkidake, dagozkie, dagozkieke, dagozkigu, dagozkiguke, dagozkik, dagozkin, dagozkinake, dagozkio, dagozkiote, dagozkit, dagozkizu, dagozkizue, dagozkizueke, dagozkizuke, daiteke, daitez, daitezela, daitezke, dakiake, dakian, dakidake, dakidan, dakieke, dakien, dakiguke, dakigun, dakioke, dakion, dakizkiake, dakizkian, dakizkidake, dakizkidan, dakizkieke, dakizkien, dakizkiguke, dakizkigun, dakizkiote, dakizkion, dakizkizueke, dakizkizuen, dakizkizuke, dakizkizun, dakizueke, dakizuen, dakizuke, dakizun, dateke, daude, daudeke, daudela, Dekretu, delako, den, dena, denak, denean, denek, denok, dezagun, dira, dirateke, dire, direla, diren, direnak, dituk, ditun, dizkio, du, dua, duela, dugu, dugun, duk, dun, dut, dute, duela, duzu, duzue, duzuela, duzun, ea, edo, egin, egingo, egiten, egon, egongo, egote, egotea, egoten, elkarrekin, eman, emana, ematen, erdian, eske, esker, eskuratzerakoan, eta, euren, ez, ezean, ezen, ezik, ezin, ezinbestekoa, ezta, gabe, gagozkiake, gagozkian, gagozkie, gagozkieke, gagozkien, gagozkik, gagozkin, gagozkinake, gagozkinan, gagozkio, gagozkioke, gagozkion, gagozkizu, gagozkizue, gagozkizueke, gagozkizuen, gagozkizuke, gagozkizun, gainean, gainera, gaitez, gaitezke, gaituk, gaitun, gakizkiake, gakizkian, gakizkieke, gakizkien, gakizkiote, gakizkion, gakizkizueke, gakizkizuen, gakizkizuke, gakizkizun, gara, garateke, gataizkiake, gataizkie, gataizkieke, gataizkik, gataizkin, gataizkinake, gataizkio, gataizkiote, gataizkizu, gataizkizue, gataizkizueke, gataizkizuke, gaude, gaudeke, gauden, gehiago, gehiegi, gehien, gengoziake, gengozkian, gengozkieke, gengozkieken, gengozkien, gengozkinake, gengozkinan, gengozkioke, gengozkiote, gengozkion, gengozkizueke, gengozkizueken, gengozkizuen, gengozkizuke, gengozkizukeen, gengozkizun, genituzke, genituzkeen, genizue, genizkiake, genizkian, genizkieke, genizkieken, genizkien, genizkiote, genizkioteen, genizkion, genizkizueke, genizkizueken, genizkizuen, genizkizuke, genizkizukeen, genizkizun, genuke, genukeen, gero, gerok, geroztik, geu, geundeke, geundekeen, geunden, geure, gineteke, ginetekeen, ginduan, gindunan, ginen, gintez, gintezke, gintezkeen, gintzaizkiake, gintzaizkian, gintzaizkieke, gintzaizkieken, gintzaizkien, gintzaizkinake, gintzaizkinan, gintzaizkiote, gintzaizkioteen, gintzaizkion, gintzaizkizueke, gintzaizkizueken, gintzaizkizuen, gintzaizkizuke, gintzaizkizukeen, gintzaizkizun, gisa, guhaur, gurea, gurekin, gutxi, gutxiago, gutxienez, guztiak, guztion, guztiontzat, hadin, hago, hagoke, hagokidake, hagogie, hagogieke, hagogikigu, hagogiguke, hagogio, hagogioke, hagogit, hainbeste, haiteke, haiz, haizateke, hakidake, hakidan, hakieke, hakien, hakiguke, hakigun, hakioke, hakion, haraino, harantz, haratago, hargatik, hartara, hatzaidake, hatzaie, hatzaieke, hatzaigu, hatzaiguke, hatzaio, hatzaioke, hatzait, hauekin, hauen, hendin, hengoan, hengoke, hengokeen, hengokidake, hengokidakeen, hengokidan, hengokieke, hengokieken, hengokien, hengokiguke, hengokigukeen, hengokigun, hengokioke, hengokiokeen, hengokion, henkidake, henkidakeen, henkidan, henkieke, henkieken, henkien, henkiguke, henkigukeen, henkigun, henkioke, henkiokeen, henkion, herori, heu, heure, hihaur, hinteke, hintekeen, hintzaidake, hintzaidakeen, hintzaidan, hintzaieke, hintzaieken, hintzaian, hintzaiguke, hintzaigukeen, hintzaigun, hintzaioke, hintzaiokeen, hintzaion, hintzateke, hintzatekeen, hintzen, hituzke, hituzkeen, hola, honaino, honantz, honen, horraino, horrantz, horrek, horren, hortxe, huke, hukeen, hurrengo, ia, inguru, inguruan, inolako, inoren, izan, izanen, izango, izate, izatea, izaten, kanpo, kanpoan, kontra, landa, laster, legoke, legokiake, legokidake, legokieke, legokiguke, legokinake, legokioke, legokizueke, legokizuke, legozkiake, legozkidake, legozkieke, legozkiguke, legozkinake, legozkiote, legozkizueke, legozkizuke, lehenago, lekiake, lekidake, lekieke, lekiguke, lekiote, lekiaki, lekiakidake, lekiakieke, lekiakiguke, lekiakioke, lekiakizueke, lekiakizuke, lekiakizueke, lekiakizuke, leudeke, lirateke, liteke, litezke, lituzke, lituzkeen, litzaiake, litzaidake, litzaiake, litzaiaguke, litzainake, litzaiote, litzaiaki, litzaiakidake, litzaiakieke, litzaiakiguke, litzaiakinake, litzaiakioke, litzaiakizue-*

*ke, litzaizkizuke, litzaizueke, litzaizuke, litzateke, lortu, lortzen, luke, lukeen, maiatza, maiz, mundu, nadin, nago, nagoen, nagoke, nagokiake, nagokian, nagokie, nagokieke, nagokien, nagokik, nagokin, nagokinake, nagokinan, nagokio, nagokioko, nagokion, nagokizu, nagokizue, nagokizueke, nagokizuen, nagokizuke, nagokizun, nahiko, nahikoa, nahiz, naiteke, naiz, naizateke, nake, nakiake, nakian, nakieke, nakien, nakioko, nakion, nakizueke, nakizuen, nakizuke, nakizun, nan, natzaiake, natzaie, natzaieke, natzaik, natzain, natzainake, natzaio, natzaioke, natzaizu, natzaizue, natzaizueke, natzaizuke, nau, nauk, naun, nekatu, nekez, nendin, nengoen, nengoke, nengokeen, nengokiake, nengokian, nengokieke, nengokiekeen, nengokien, nengokinake, nengokinan, nengokioko, nengokiokoeken, nengokion, nengokizueke, nengokizuekeen, nengokizuen, nengokizuke, nengokizukeen, nengokizun, nenkiake, nenkian, nenkieke, nenkiekeen, nenkien, nenkioko, nenkiokoeken, nenkion, nenkizueke, nenkizuekeen, nenkizuen, nenkizuke, nenkizukeen, nenkizun, nerau, neu, neure, nihaur, nik, ninduan, nindunan, ninteke, nintekeen, nintzaiake, nintzaian, nintzaieke, nintzaiekeen, nintzaien, nintzainake, nintzainan, nintzaioke, nintzaiokeen, nintzaion, nintzaizueke, nintzaizuekeen, nintzaizuen, nintzaizuke, nintzaizukeen, nintzaizun, nintzateke, nintzatekeen, nintzen, nituzke, nituzkeen, norakoak, norbaiten, norbera, norberaren, nori, nuke, nukeen, omen, omeone, ondo, ondoan, ondoren, ondorioz, oraindik, orde, oso, osoa, ostera, ote, sartu, segidan, sekula, truk, truke, utzi, utziz, zagozkidake, zagozkidakete, zagozkidate, zagozkie, zagozkieke, zagozkiekete, zagozkiete, zagozkigu, zagozkiguke, zagozkigukete, zagozkigute, zagozkio, zagozkioko, zagozkiokete, zagozkiote, zagozkit, zaiake, zaidake, zaie, zaieke, zaigu, zaiguke, zaik, zain, zainake, zaioko, zait, zaitz, zaitzke, zaitzketete, zaitzete, zaizkiako, zaizkidake, zaizkie, zaizkieke, zaizkigu, zaizkiguke, zaizkik, zaizkin, zaizkinake, zaizkio, zaizkioko, zaizkit, zaizkizu, zaizkizue, zaizkizueke, zaizkizuke, zaizu, zaizue, zaizueke, zaizuke, zakizkidake, zakizkidakete, zakizkidan, zakizkidaten, zakizkieke, zakizkiekete, zakizkien, zakizkieten, zakizkiguke, zakizkigukete, zakizkigun, zakizkiguten, zakizkioko, zakizkiokete, zakizkion, zakizkioten, zara, zarateke, zarete, zaretekete, zatekeen, zatia, zataizkidake, zataizkidakete, zataizkidate, zataizkie, zataizkieke, zataizkiekete, zataizkiete, zataizkigu, zataizkiguke, zataizkigukete, zataizkigute, zataizkio, zataizkioko, zataizkiokete, zataizkiote, zataizkit, zaude, zaudeke, zaudete, zaudete, zazu, ze, zedin, zegoen, zegokeen, zegokian, zegokidakeen, zegokidan, zegokiekeen, zegokien, zegokigukeen, zegokigun, zegokinan, zegokiokoeken, zegokion, zegokizuekeen, zegokizuen, zegokizukeen, zegokizun, zegozkian, zegozkidakeen, zegozkidan, zegozkiekeen, zegozkien, zegozkigukeen, zegozkigun, zegozkinan, zegozkiokoeken, zegozkion, zegozkizuekeen, zegozkizuen, zegozkizukeen, zegozkizun, zehar, zekian, zekidakeen, zekidan, zekiekeen, zekien, zekigukeen, zekigun, zekiokoeken, zekion, zekizkian, zekizkidakeen, zekizkidan, zekizkiekeen, zekizkien, zekizkigukeen, zekizkigun, zekizkiokoeken, zekizkion, zekizkizuekeen, zekizkizuen, zekizkizukeen, zekizkizun, zekizuekeen, zekizuen, zekizukeen, zekizun, zen, zengozkidake, zengozkidakeen, zengozkidakete, zengozkidaketen, zengozkidan, zengozkidaten, zengozkieke, zengozkiekeen, zengozkiekete, zengozkieketen, zengozkien, zengozkieten, zengozkiguke, zengozkigukeen, zengozkigukete, zengozkiguketen, zengozkigun, zengozkiguten, zengozkioko, zengozkiokoeken, zengozkiokete, zengozkioketen, zengozkion, zengozkioten, zenidate, zenigute, zenituzke, zenituzkeen, zenituzkete, zenituzketen, zenkizkidake, zenkizkidakeen, zenkizkidakete, zenkizkidaketen, zenkizkidan, zenkizkidaten, zenkizkieke, zenkizkiekeen, zenkizkiekete, zenkizkieketen, zenkizkien, zenkizkieten, zenkizkiguke, zenkizkigukeen, zenkizkigukete, zenkizkiguketen, zenkizkigun, zenkizkiguten, zenkizkioko, zenkizkiokoeken, zenkizkiokete, zenkizkioketen, zenkizkion, zenkizkioten, zenuke, zenukeen, zenukete, zenuketen, zeren, zergatik, zerok, zerori, zertaz, zeu, zeudekeen, zeuden, zeuek, zeundeke, zeundekeen, zeundeketen, zeunden, zeundet, zeure, zinateke, zinatekeen, zinatekete, zinateketen, zinen, zineten, zintez, zintezke, zintezkeen, zintezketen, zintezten, zintzaizkidake, zintzaizkidakeen, zintzaizkidakete, zintzaizkidaketen, zintzaizkidan, zintzaizkidaten, zintzaizkieke, zintzaizkiekeen, zintzaizkiekete, zintzaizkieketen, zintzaizkien, zintzaizkieten, zintzaizkiguke, zintzaizkigukeen, zintzaizkigukete, zintzaizkiguketen, zintzaizkigun, zintzaizkiguten, zintzaizkioko, zintzaizkiokoeken, zintzaizkiokete, zintzaizkioketen, zintzaizkion, zintzaizkioten, ziratekeen, ziren, zitekeen, zitezen, zitezkeen, zituan, zitunan, zitzaian, zitzaidakeen, zitzaidan, zitzaiekeen, zitzaien, zitzaigukeen, zitzaigun, zitzainan, zitzaiokeen, zitzaion, zitzaizkian, zitzaizkidakeen, zitzaizkidan, zitzaizkiekeen, zitzaizkien, zitzaizkigukeen, zitzaizkigun, zitzaizkinan, zitzaizkiokoeken, zitzaizkion, zitzaizkizuekeen, zitzaizkizuen, zitzaizkizukeen, zitzaizkizun, zitzaizuekeen, zitzaizuen, zitzaizukeen, zitzaizun, zuan, zuhaur, zuihauk, zunan, zurea, zutaz.*

Define the pattern **PronBasque** as any one from the following list:

*bera, beraiek, beraien, berak, beraren, berau, berauek, bere, beren, berori, beroriek, eurak, ezer, genian, genien, geninan, genion, genizuen, genizun, gu, gure, haiek, haien, hala, han, handik, hango, hara, haren, hau, hauek, hemen, hemendik, hemengo, hi, hidan, hien, higun, hion, hire, hona, honela, hor, hori, horiek, horko, horra, horrela, hortik, hura, inoiz, inola, inon, inor, ni, nian, nien, ninan, nion, nire, nizuen, nizun, noiz, noizbait, nola, nolabait, non, nonbait, nondik, nongo, nor, nora, norbait, orain, orduan, zein, zenidan, zenidaten, zenien, zenieten, zenigun, zeniguten, zenion, zenioten, zer, zerbait, zian, ziaten, zidan, zidaten, zien, zieten, zigun, ziguten, zinaten, zion, zioten, zizuen, zizueten, zizun, zizuten, zu, zuek, zuen, zure.*

Define **tenerBasque** as the following pattern:

$(\emptyset|ba|e)(\emptyset|hen|le|nen)(\emptyset|be|da|ga|ge|ha|na|za|ze)(\emptyset|n)uka\mathbf{X}$ .

If a word exactly matches any one of the following:

**(BasqueStopRoot)X**,  
**BasqueStopString**,  
 $(\emptyset|edo)\mathbf{PronBasque}(\emptyset|bait|nahi|txe|xe)\mathbf{X}$ ,  
**tenerBasque**,

then we consider it a Basque stop word. All the Basque stop words that appear in a particular document need to be ignored before we perform word clustering on the rest of the vocabulary list.  $\square$

### 9.1.1 Effective spelling and essential root

**Definition 9.2** (Basque protected range). Set  $\mathbf{V} = (a|e|i|o|u)$ ,  $\mathbf{C} = \overline{\mathbf{V}}$ . Search for the pattern  $\mathbf{V}_m\mathbf{C}_m\mathbf{V}\sim$  or

$(\emptyset|ba|bi|ko)(\emptyset|hen|hin|le|li|nen)(\emptyset|be|da|ga|ge|gi|ha|na|ni|za|ze|zi)\mathbf{C}_m\mathbf{V}_m\mathbf{C}\sim$

in the string  $\hat{\sigma}$ . If such a pattern cannot be found, or  $\hat{\sigma}$  does not contain  $\mathbf{V}$ , then define  $\rho_* = 0$ ; otherwise, define  $\rho_*$  as the last position occupied by the aforementioned pattern. If  $\rho_* > 0$ ,  $\ell(\hat{\sigma}) > \rho_*$ ,  $\hat{\sigma}^{(\rho_*)} = r$  (i.e. the  $\rho_*$ -th character is the letter  $r$ ) and  $\hat{\sigma}^{(\rho_*+1)} = \mathbf{C}$  (i.e. the  $(\rho_* + 1)$ -st character is not a vowel), then  $\text{ProtRg}(\hat{\sigma}) = 1 + \rho_*$ ; otherwise, set  $\text{ProtRg}(\hat{\sigma}) = \rho_*$ .

**Algorithm 9.3** (Basque effective spelling). Set  $\mathbf{V} = (a|e|i|o|u)$ ,  $\mathbf{C} = \overline{\mathbf{V}}$ . For a Basque word  $\hat{\sigma}$ , its effective spelling  $\text{EffSpell}(\hat{\sigma})$  is constructed in the following steps:

- (1) Convert to lowercase and do  $\hat{\chi}_m gabe(\emptyset|a)\sim \rightarrow xx\hat{\chi}_m$ .
- (2) Do  $tx \rightarrow \check{c}$ .
- (3) Do  $(izeb|izeko)\sim \rightarrow a\upsilon\eta\tau$ ,  $\mathbf{C}_y \rightarrow \mathbf{C}_i y$ ,  $anai\sim \rightarrow neb$ ,  $arreb\sim \rightarrow ahizp$ ,  $lehengus(in|u)\mathbf{X}\sim \rightarrow c\omega\sigma i\check{v}$ .
- (4) Replace

|                                                       |                |                                    |                             |                                                         |                    |                  |                 |                                                       |                            |                   |                      |
|-------------------------------------------------------|----------------|------------------------------------|-----------------------------|---------------------------------------------------------|--------------------|------------------|-----------------|-------------------------------------------------------|----------------------------|-------------------|----------------------|
| <i>aban</i> ~                                         | <i>abe</i> ~   | <i>agir</i> ~                      | <i>aldarri</i> ~            | <i>andereñ</i> ~                                        | <i>ater</i> ~      | <i>bakar</i> ~   | <i>bar</i> ~    | <i>begira</i> ~                                       | <i>begiru</i> ~            | <i>begitart</i> ~ |                      |
| <i>βa</i>                                             | <i>ab</i>      | <i>ayir</i>                        | <i>aldrri</i>               | <i>μιοσ</i>                                             | <i>atr</i>         | <i>σiṽγr</i>     | <i>λαφ</i>      | <i>λuka</i>                                           | <i>ρεσπtu</i>              | <i>φαστ</i>       |                      |
| <i>bil</i> <sub><math>\hat{\chi}_\#(a)</math></sub> ~ | <i>bila</i> ~  | <i>burg</i> ~                      | <i>buru</i> ~               | <i>carolin</i> ~                                        | <i>charlotte</i> ~ | <i>dantz</i> ~   | <i>denbor</i> ~ | <i>des</i> <sub><math>\hat{\chi}_\#(i)</math></sub> ~ | <i>desio</i> ~             |                   |                      |
| <i>βιλχ</i>                                           | <i>βιαλ</i>    | <i>buγg</i>                        | <i>bru</i>                  | <i>κpαln</i>                                            | <i>karlotte</i>    | <i>δac</i>       | <i>τμεπ</i>     | <i>δdsχ</i>                                           | <i>dsir</i>                |                   |                      |
| <i>desi</i> ~                                         | <i>desk</i> ~  | <i>egona</i> ~                     | <i>eliza</i> $\mathbf{X}$ ~ | <i>era</i> <sub><math>\hat{\chi}_\#(m t)</math></sub> ~ | <i>err</i> ~       | <i>familia</i> ~ | <i>fitz</i> ~   | <i>gela</i> ~                                         | <i>gorrot</i> ~            | <i>hertf</i> ~    |                      |
| <i>dsi</i>                                            | <i>dsk</i>     | <i>σtaya</i>                       | <i>ελζ</i>                  | <i>exqχ</i>                                             | <i>err</i>         | <i>φμαλι</i>     | <i>φτζ</i>      | <i>gela</i>                                           | <i>ηat</i>                 | <i>ηrτεφ</i>      |                      |
| <i>hobe</i> $\mathbf{X}$ ~                            | <i>hunsf</i> ~ | <i>ibil(ald er)</i> $\mathbf{X}$ ~ | <i>ideia</i> ~              | <i>igaro</i> ~                                          | <i>ikar</i> ~      | <i>indi</i> ~    | <i>irr</i> ~    | <i>izen</i> ~                                         | <i>jane</i> $\mathbf{X}$ ~ | <i>kant</i> ~     |                      |
| <i>βεστ</i>                                           | <i>hnsf</i>    | <i>ibili</i>                       | <i>ιδea</i>                 | <i>σpendo</i>                                           | <i>ckar</i>        | <i>ndi</i>       | <i>ιrr</i>      | <i>ṽαμ</i>                                            | <i>jaṽ</i>                 | <i>cant</i>       |                      |
| <i>karta</i> ~                                        | <i>kol</i> ~   | <i>liburuteg</i> ~                 | <i>liydia</i> ~             | <i>londres</i> ~                                        | <i>lots</i> ~      | <i>maria</i> ~   | <i>mariy</i> ~  | <i>meriy</i> ~                                        | <i>mingarri</i> ~          | <i>musik</i> ~    |                      |
| <i>καρτα</i>                                          | <i>kl</i>      | <i>λβιρ</i>                        | <i>ληδία</i>                | <i>lndres</i>                                           | <i>σχαμ</i>        | <i>μαρια</i>     | <i>μαρη</i>     | <i>μρυ</i>                                            | <i>παιṽi</i>               | <i>μουσκ</i>      |                      |
| <i>negozio</i> ~                                      | <i>negu</i> ~  | <i>rst</i>                         | <i>senarra</i> ~            | <i>senti</i> ~                                          | <i>tentel</i> ~    | <i>ugar</i> ~    | <i>zakar</i> ~  | <i>amak</i>                                           | <i>de</i>                  | <i>long</i>       | <i>on(∅ a ak ik)</i> |
| <i>ngoσ</i>                                           | <i>ṽegω</i>    | <i>ρστ</i>                         | <i>huσβα</i>                | <i>φeeλι</i>                                            | <i>φωol</i>        | <i>ugr</i>       | <i>ρyδr</i>     | <i>ama</i>                                            | <i>δεe</i>                 | <i>lṽoy</i>       | <i>βεστ</i>          |

- (5) Replace

|                                                                                                                                 |                            |              |                                                        |                 |                |                                 |                                           |  |  |  |  |
|---------------------------------------------------------------------------------------------------------------------------------|----------------------------|--------------|--------------------------------------------------------|-----------------|----------------|---------------------------------|-------------------------------------------|--|--|--|--|
| $(\emptyset ba bi zi)(\emptyset li)(d g h j n z)(\emptyset in)(\emptyset d)oa(\emptyset k l n t z)\mathbf{X}\sim$               |                            |              |                                                        |                 |                |                                 |                                           |  |  |  |  |
| <i>βgoβ</i>                                                                                                                     |                            |              |                                                        |                 |                |                                 |                                           |  |  |  |  |
| $(\emptyset ba bi zi)(\emptyset li)(d g h j n z)(\emptyset in)(\emptyset d)(\emptyset a)eki(\emptyset k l n t z)\mathbf{X}\sim$ |                            |              |                                                        |                 |                |                                 |                                           |  |  |  |  |
| <i>βknowβ</i>                                                                                                                   |                            |              |                                                        |                 |                |                                 |                                           |  |  |  |  |
| $(\emptyset ba e)(\emptyset hen le nen)(\emptyset be da ga ge ha na za ze)(\emptyset n)ka(r z)\mathbf{X}\sim$                   |                            |              |                                                        |                 |                |                                 |                                           |  |  |  |  |
| <i>ekarr</i>                                                                                                                    |                            |              |                                                        |                 |                |                                 |                                           |  |  |  |  |
| $(\emptyset ba e)(\emptyset hen le nen)(\emptyset be da ga ge ha na za ze)(\emptyset n)rama\mathbf{X}\sim$                      |                            |              |                                                        |                 |                |                                 |                                           |  |  |  |  |
| <i>βτακβ</i>                                                                                                                    |                            |              |                                                        |                 |                |                                 |                                           |  |  |  |  |
| <i>ahazt</i> ~                                                                                                                  | <i>begi</i> $\mathbf{X}$ ~ | <i>ego</i> ~ | <i>eliz</i> <sub><math>\hat{\chi}_\#(a)</math></sub> ~ | <i>elizab</i> ~ | <i>harro</i> ~ | <i>kont(a u)</i> $\mathbf{X}$ ~ | <i>bru(∅ bid</i> $\mathbf{X}$ <i>)ko)</i> |  |  |  |  |
| <i>φορyτ</i>                                                                                                                    | <i>eye</i>                 | <i>eg</i>    | <i>ελιζχ</i>                                           | <i>ελιζαβ</i>   | <i>πιρδο</i>   | <i>κοṽτ</i>                     | <i>bruak</i>                              |  |  |  |  |

(6) Call the result so far as  $\hat{\sigma}^\dagger$ , and break it down into  $\hat{\sigma}^\dagger = \hat{\sigma}_1^\dagger \hat{\sigma}_2^\dagger$ , where  $\ell(\hat{\sigma}_1^\dagger) = \text{ProtRg}(\hat{\sigma}^\dagger)$ . Work on  $\hat{\sigma}_2^\dagger$  as follows:

(6.1) Do  $\check{c} \rightarrow tx$ .

(6.2) Delete any pattern in the following list:

ago, aldatu, aldi, aldia, an, arazi, ari, atu, atze, bera, bide, bidea, dako, du, dura, ean, era, errez, erreza, eta, etan, etari, ez, eza, ezin, ezina, gai, gaia, gailu, gailua, gaitz, gaitza, gale, galea, go, gune, gunea, gura, ide, idea, ka, kaitz, kaitza, kan, kari, karia, karri, karria, kera, keta, ki, kide, kidea, kin, kina, kizun, kizuna, kor, korra, kuna, kunde, kunea, kune, kunea, kuntza, kura, la, lari, le, men, mena, or, orra, pen, pena, pera, pide, pidea, rean, rekin, taile, tailea, taldi, taldia, tarazi, tari, tatu, tezin, tezina, tio, tu, tun, tuna, tura, tzaiga, tzaile, tzailea, tzaka, tzake, tzat, tze, tzeke, tzez

and the letters (if any) thereafter.

(6.3) Delete any pattern in the following list:

ada, ail, aizun, ak, alde, aldea, aldi, aldia, anda, anga, antza, ar, ara, ari, aria, aro, aroa, arte, artea, asi, asia, asun, asuna, aurre, aurrea, behar, bera, bizia, burua, dar, dara, degi, degia, denda, di, du, dua, dun, duna, duri, duria, duru, durua, egi, egia, ek, eko, eme, emea, ena, enea, eria, ero, eroa, eroz, eroza, estu, estua, eta, etako, etan, etara, etxe, etxea, ez, eza, ezia, ga, gabe, gabea, gai, gaia, garna, garren, garrena, ge, gei, geia, gela, gerren, gerrena, gibel, gibela, gile, gilea, gintza, gintzo, gintzu, giro, go, goi, gune, gunea, handi, handia, i, ka, kabe, kabea, kada, kail, kaila, kalde, kaldea, kan, kana, kari, karia, kera, keria, ket, keta, ki, kia, kide, kin, kina, kintza, kirri, kirria, ko, koa, koi, koia, koitz, koitza, kondo, kondoa, kor, korra, kote, kotea, kume, kunea, kuntza, lari, laria, larri, larria, leku, lekua, liar, liara, mendi, mendia, mendu, mendua, mentu, mentua, min, mina, n, na, nahi, nahia, ne, nea, ngo, ngoa, no, noa, o, oa, ohi, ohia, oi, oia, ola, ondo, ondoa, ontzi, ontzia, orde, ordea, ordu, ordua, oro, oroa, os, osa, oso, osoa, oste, ostea, pe, pea, pera, ra, ro, sa, ska, skila, sko, sta, ta, tako, takoa, talde, taldea, taldi, taldia, tan, tar, tara, tari, taria, tarik, tariko, taro, taroa, tasun, tasuna, te, tea, tegi, tegia, teria, ti, tia, tiar, tiara, tila, to, toa, toki, tokia, tra, tsua, tto, ttoa, tu, tua, tuko, txo, txoa, txu, txua, tz, tzain, tzaina, tzale, tzalea, tzar, tzara, tzarra, tzo, tzoa, tzu, tzua, una, une, unea, urren, urrena, xka, z, za, zain, zaina, zale, zalea, zaro, zaroa, zino, zinoa, zio, zioa, zione, zionea, zka, zko, zkoa, zp, zto, ztoa, zu, zua

and the letters (if any) thereafter.

(6.4) Delete any pattern in the following list:

dade, date, era, ero, gi, go, ik, keria, ki, la, lanik, larik, rik, ro, tade, tate, to, ztik

and the letters (if any) thereafter.

(6.5) Call the result so far as  $\hat{\sigma}_2^\ddagger$ . Concatenate  $\hat{\sigma}_1^\dagger$  and  $\hat{\sigma}_2^\ddagger$ .

(7) Replace

|                                                                                                               |
|---------------------------------------------------------------------------------------------------------------|
| $(\emptyset ba e)(\emptyset hen le nen)(\emptyset be da ga ge ha na za ze)(\emptyset n to r z)\mathbf{X}\sim$ |
| <i>etorr</i>                                                                                                  |
| $(\emptyset ba i)(\emptyset hen le nen)(\emptyset be da ga ge ha na za ze)(\emptyset n bi)\mathbf{X}\sim$     |
| <i><math>\beta</math>walk<math>\beta</math></i>                                                               |
| $(b d gen h n z zen)io(d e g k n s t z)\mathbf{X}\sim$                                                        |
| <i>esa</i>                                                                                                    |
| $one(\emptyset g)$                                                                                            |
| <i><math>\beta</math>es<math>\tau</math></i>                                                                  |

**Algorithm 9.4** (Basque essential root). Let  $\hat{\sigma}$  be the effective spelling of a Basque word, then its corresponding essential root  $\text{EssRoot}(\hat{\sigma})$  is constructed as  $\hat{\sigma}^{[\text{ProtRg}(\hat{\sigma})]}$ .

### 9.1.2 Approximate clustering

There will not be any mutation rules in our algorithm for Basque, so  $\text{SimpHrdTest} = \text{HrdTest}$ .

**Algorithm 9.5** (Simple heredity test). Suppose that  $\hat{\alpha}$  and  $\hat{\beta}$  are both lowercase strings. The Boolean-valued function  $\text{SimpHrdTest}(\hat{\alpha}, \hat{\beta})$  returns **TRUE** if  $\hat{\alpha}$  contains at least one instance of  $\mathbf{V}$ , **AND** at least one of the following two conditions holds:<sup>107</sup>

(i)  $\hat{\alpha} = \hat{\beta}$ ;

(ii)  $\hat{\alpha}' = \hat{\beta}'$ , where the strings with prime result from doing  $\sim^{\mathbf{X} \in (\mathbf{V}\hat{\chi})}(\emptyset|b)(a|e) \rightarrow \mathbf{X}$  on their counterparts without prime.

<sup>107</sup>As a general rule in this document, the truth values of items labeled with Roman numerals are connected to each other with logical **OR**.

**Algorithm 9.6** (Approximate clustering of Basque words). *The approximate clustering of a list of Basque words  $\{\hat{\alpha}_1, \dots, \hat{\alpha}_N\}$  is completed in two stages:*

- (1) *We sort the list  $\{(\hat{\alpha}_1, \text{EffSpell}(\hat{\alpha}_1)), \dots, (\hat{\alpha}_N, \text{EffSpell}(\hat{\alpha}_N))\}$  alphabetically according to the last component. If two consecutive neighbors in the alphabetized list  $\{(\hat{\alpha}_{(1)}, \text{EffSpell}(\hat{\alpha}_{(1)})), \dots, (\hat{\alpha}_{(N)}, \text{EffSpell}(\hat{\alpha}_{(N)}))\}$  satisfy  $\text{HrdTest}(\text{EffSpell}(\hat{\alpha}_{(n)}), \text{EffSpell}(\hat{\alpha}_{(n+1)})) = \mathbf{FALSE}$ , where  $n \in \mathbb{Z} \cap [1, N)$ , then add a demarcation line between these two entries. In this way, the alphabetized list is divided into separate groups of words tagged with their effective spellings:  $\{g_1 = \{(\hat{\alpha}_{(1,1)}, \text{EffSpell}(\hat{\alpha}_{(1,1)})), \dots, (\hat{\alpha}_{(1,n_1)}, *)\}, \dots, g_M = \{(\hat{\alpha}_{(M,1)}, *), \dots, (\hat{\alpha}_{(M,n_M)}, *)\}$ , where each sublist also preserves alphabetic order. In particular, we have  $\hat{\alpha}_{(1,1)} = \hat{\alpha}_{(1)}$  and  $\hat{\alpha}_{(M,n_M)} = \hat{\alpha}_{(N)}$ .*
- (2) *For each group of words  $g_m = \{(\hat{\alpha}_{(m,1)}, *), \dots, (\hat{\alpha}_{(m,n_m)}, *)\}$  where  $m \in \mathbb{Z} \cap [1, M]$ , we augment it into a tagged entry  $G_m = (g_m, \text{EffSpell}(\hat{\alpha}_{(m,1)}), \text{EssRoot}(\text{EffSpell}(\hat{\alpha}_{(m,1)})))$ . The list  $\{G_1, \dots, G_M\}$  is sorted alphabetically, with respect to  $\text{EssRoot}(\text{EffSpell}(\hat{\alpha}_{(m,1)}))$  (with higher priority), and  $\text{EffSpell}(\hat{\alpha}_{(m,1)})$  (with lower priority). If two consecutive neighbors in the alphabetized list  $\{G_{(1)} = (g_{(1)}, \hat{\gamma}'_{(1)}, \hat{\gamma}''_{(1)}), \dots, G_{(M)} = (g_{(M)}, \hat{\gamma}'_{(M)}, \hat{\gamma}''_{(M)})\}$  satisfy*

$$\text{HrdTest}(\hat{\gamma}''_{(m)}, \hat{\gamma}''_{(m+1)}) = \mathbf{FALSE}$$

**AND**

$$\text{HrdTest}(\hat{\gamma}'_{(m)}, \hat{\gamma}'_{(m+1)}) = \mathbf{FALSE}$$

where  $m \in \mathbb{Z} \cap [1, M)$ , then add a demarcation line between these two entries. In this manner, the alphabetized list  $\{G_{(1)}, \dots, G_{(M)}\}$  is divided into separate groups of tagged clusters  $\{\Gamma_1 = \{G_{(1,1)}, \dots, G_{(1,m_1)}\}, \dots, \Gamma_K = \{G_{(K,1)}, \dots, G_{(1,m_K)}\}$ . Finally, the output list of word clusters  $\{\tilde{\Gamma}_1, \dots, \tilde{\Gamma}_K\}$  is constructed by discarding all the tags (effective spellings, essential roots) from each  $\Gamma_k$ , where  $k \in \mathbb{Z} \cap [1, K]$ .

*Example 9.6.1.* Our clustering algorithm correctly groups the following families of Basque words:

*ahizpa, ahizpak, ahizparekin, ahizparen, ahizparengan, ahizparengana, ahizparenganaino, ahizparenganako, ahizparenganantz, ahizparengandik, ahizparengatik, ahizparentzat, ahizpari, ahizparik, ahizpatzat, ahizpaz, ahizpei, ahizpek, ahizpekin, ahizpen, ahizpengan, ahizpenganana, ahizpenganaino, ahizpenganako, ahizpenganantz, ahizpenganandik, ahizpenganatik, ahizpentsat, ahizpez, arreba, arrebak, arrebarekin, arrebaren, arrebarengan, arrebarengana, arrebarenganaino, arrebarenganako, arrebarenganantz, arrebarengandik, arrebarengatik, arrebarentzat, arrebari, arrebantik, arrebantz, arrebaz, arrebbei, arrebek, arrebekin, arreben, arrebengan, arrebenganana, arrebenganaino, arrebenganako, arrebenganantz, arrebengandik, arrebengatik, arrebentzat, arrebbez — “sister”;*

*anaia, anaiak, anaiarekin, anaiaren, anaiarengan, anaiarengana, anaiarenganaino, anaiarenganako, anaiarenganantz, anaiarengandik, anaiarengatik, anaiarentzat, anaiari, anaiarik, anaiatzat, anaiaz, anaiei, anaiek, anaiekin, anaieren, anaierengan, anaierenganana, anaierenganaino, anaierenganako, anaierenganantz, anaierengandik, anaierengatik, anaierentzat, anaierari, anaierarik, anaieratzat, anaierz, anaiez, neba, nebak, nebarekin, nebaren, nebarengan, nebarengana, nebarenganaino, nebarenganako, nebarenganantz, nebarengandik, nebarengatik, nebarentzat, nebari, nebarik, nebatzat, nebaz, nebei, nebek, nebekin, neben, nebingan, nebinganana, nebinganaino, nebinganako, nebinganantz, nebingandik, nebingatik, nebingentzat, nebeiz, izeko, izekoa, izekoak, izekoarekin, izekoaren, izekoarengan, izekoarengana, izekoarenganaino, izekoarenganako, izekoarenganantz, izekoarengandik, izekoarengatik, izekoarentzat, izekoari, izekoaz, izekoei, izekoek, izekoekin, izekoen, izekoengan, izekoengana, izekoenganaino, izekoenganako, izekoenganantz, izekoengandik, izekoengatik, izekoentzat, izekoz, izekok, izekorekin, izekoren, izekorengan, izekorengana, izekorenganaino, izekorenganako, izekorenganantz, izekorengandik, izekorengatik, izekorentzat, izekori, izekorik, izekotzat, izekoz — “aunt”.*

It also correctly cluster each of the following verbs:

*bagenbiltza, bagenbilzkie, bagenbilzkik, bagenbilzkin, bagenbilzkio, bagenbilzkizu, bagenbilzkizue, bahenbilkie, bahenbilkigu, bahenbilkio, bahenbilkit, balebilkie, balebilkigu, balebilkik, balebilkin, balebilkio, balebilkit, balebilkizu, balebilkizue, balebiltza, balebilzkie, balebilzkigu, balebilzkik, balebilzkin, balebilzkio, balebilzkit, balebilzkizu, balebilzkizue, banenbilkie, banenbilkik, banenbilkin, banenbilkio, banenbilkizu, banenbilkizue, bazenbiltza, bazenbiltzate, bazenbilzkidate, bazenbilzkie, bazenbilzkiete, bazenbilzkigu, bazenbilzkigute, bazenbilzkio, bazenbilzkio, bazenbilzkite, bebiltza, bebilzkie, bebilzkigu, bebilzkik, bebilzkin, bebilzkio, bebilzkit, bebilzkizu,*

*bebilzkizue, benbilkie, benbilkigu, benbilkik, benbilkin, benbilkio, benbilkit, benbilkizu, benbilkizue, dabilela, dabilke, dabilkiake, dabilkidake, dabilkie, dabilkieke, dabilkigu, dabilkiguke, dabilkik, dabilkin, dabilkinake, dabilkio, dabilkioke, dabilkit, dabilkizu, dabilkizue, dabilkizueke, dabilkizuke, dabiltza, dabiltzala, dabilzke, dabilzkiake, dabilzkidake, dabilzkie, dabilzkieke, dabilzkigu, dabilzkiguke, dabilzkik, dabilzkin, dabilzkinake, dabilzkio, dabilzkioke, dabilzkit, dabilzkizu, dabilzkizue, dabilzkizueke, dabilzkizuke, gabiltza, gabiltzan, gabilzke, gabilzkiake, gabilzkian, gabilzkie, gabilzkieke, gabilzkien, gabilzkik, gabilzkin, gabilzkinake, gabilzkinan, gabilzkio, gabilzkioke, gabilzkion, gabilzkizu, gabilzkizue, gabilzkizueke, gabilzkizuen, gabilzkizuke, gabilzkizun, genbiltzan, genbilzke, genbilzkeen, genbilzkiake, genbilzkian, genbilzkieke, genbilzkiekeen, genbilzkien, genbilzkinake, genbilzkinan, genbilzkioke, genbilzkiokeen, genbilzkion, genbilzkizueke, genbilzkizuekeen, genbilzkizuen, genbilzkizuke, genbilzkizukeen, genbilzkizun, habilke, habilkidake, habilkie, habilkieke, habilkigu, habilkiguke, habilkio, habilkioke, habilkit, henbilen, henbilke, henbilkeen, henbilkidake, henbilkidakeen, henbilkidan, henbilkieke, henbilkiekeen, henbilkien, henbilkiguke, henbilkigukeen, henbilkigun, henbilkioke, henbilkiokeen, henbilkion, ibili, ibiliko, ibiltze, ibiltzen, lebilke, lebilkiake, lebilkidake, lebilkieke, lebilkiguke, lebilkinake, lebilkioke, lebilkizueke, lebilkizuke, lebilzke, lebilzkiake, lebilzkidake, lebilzkieke, lebilzkiguke, lebilzkinake, lebilzkioke, lebilzkizueke, lebilzkizuke, nabilen, nabilke, nabilkiake, nabilkian, nabilkie, nabilkieke, nabilkien, nabilkik, nabilkin, nabilkinake, nabilkinan, nabilkio, nabilkioke, nabilkion, nabilkizu, nabilkizue, nabilkizueke, nabilkizuen, nabilkizuke, nabilkizun, nenbilen, nenbilke, nenbilkeen, nenbilkiake, nenbilkian, nenbilkieke, nenbilkiekeen, nenbilkien, nenbilkinake, nenbilkinan, nenbilkioke, nenbilkiokeen, nenbilkion, nenbilkizueke, nenbilkizuekeen, nenbilkizuen, nenbilkizuke, nenbilkizukeen, nenbilkizun, zabiltza, zabiltzate, zabilzke, zabilzketete, zabilzkidake, zabilzkidakete, zabilzkidate, zabilzkie, zabilzkieke, zabilzkiekete, zabilzkiete, zabilzkigu, zabilzkiguke, zabilzkigukete, zabilzkigute, zabilzkio, zabilzkioke, zabilzkiokeete, zabilzkiokeete, zabilzkit, zebilen, zebilkeen, zebilkian, zebilkidakeen, zebilkidan, zebilkiekeen, zebilkien, zebilkigukeen, zebilkigun, zebilkinan, zebilkiokeen, zebilkion, zebilkizuekeen, zebilkizuen, zebilkizukeen, zebilkizun, zebiltzan, zebilzkeen, zebilzkian, zebilzkidakeen, zebilzkidan, zebilzkiekeen, zebilzkien, zebilzkigukeen, zebilzkigun, zebilzkinan, zebilzkiokeen, zebilzkion, zebilzkizuekeen, zebilzkizuen, zebilzkizukeen, zebilzkizun, zenbiltzan, zenbiltzaten, zenbilzke, zenbilzkeen, zenbilzketete, zenbilzketen, zenbilzkidake, zenbilzkidakeen, zenbilzkidakete, zenbilzkidaketen, zenbilzkidan, zenbilzkidaten, zenbilzkieke, zenbilzkiekeen, zenbilzkiekete, zenbilzkieketen, zenbilzkien, zenbilzkieten, zenbilzkiguke, zenbilzkigukeen, zenbilzkigukete, zenbilzkiguketen, zenbilzkigun, zenbilzkiguten, zenbilzkioke, zenbilzkiokeen, zenbilzkiokete, zenbilzkioketen, zenbilzkion, zenbilzkioten* — “walk”;

*diodaz, diogu, dioguz, diok, diosagu, diosat, diosate, dioska, dioskna, diosku, dioskuk, dioskute, dioskutez, dioskuz, dioskuzak, dioskuzu, dioskuzue, dioskuzuez, dioskuzuz, diosnagu, diosnat, diosnate, diost, diostak, diostate, diostatez, diostaz, diostazak, diostazu, diostazue, diostazuez, diostazuz, diot, diote, diotez, diotse, diotsedaz, diotsegu, diotseguz, diotsek, diotset, diotsete, diotsetez, diotsez, diotsezak, diotsezu, diotsezue, diotsezuez, diotsezuz, diotso, diotsodaz, diotsogu, diotsoguz, diotsok, diotsot, diotsote, diotsotez, diotsoz, diotsozak, diotsozu, diotsozue, diotsozuez, diotsozuz, diotsu, diotsudaz, diotsue, diotsuedaz, diotsuegu, diotsueguz, diotsuet, diotsuete, diotsuetez, diotsuez, diotsugu, diotsuguz, diotsut, diotsute, diotsutez, diotsuz, dioz, diozaa, diozaagu, diozaat, diozaate, diozak, diozana, diozanagu, diozanat, diozanate, diozu, diozue, diozuez, diozuz, esan, esango, esate, esaten, genioen, genioezen, geniosan, geniosnan, geniotsen, geniotsezen, geniotson, geniotsozen, geniotsuen, geniotsuezen, geniotsun, geniotsuzen, geniozaa, geniozana, hioen, hioezen, hioskun, hioskuzen, hiostan, hiostazen, hiotsen, hiotsezen, hiotson, hiotsozen, nioen, nioezen, niosan, niosnan, niostsuen, niostsuezen, niotsen, niotsezen, niotson, niotsozen, niotsun, niotsuzen, niozaan, niozanan, zenioen, zenioezen, zenioskun, zenioskuten, zenioskutezen, zenioskuzen, zeniostan, zeniostaten, zeniostatezen, zeniostaten, zenioten, zeniotezen, zeniotson, zeniotseten, zeniotsetezen, zeniotsezen, zeniotson, zeniotseten, zeniotsetezen, zeniotsozen, zioen, zioezen, ziosan, ziosaten, zioskun, zioskuten, zioskutezen, zioskuzen, ziosnan, ziosnaten, ziostan, ziostaten, ziostatezen, ziostaten, zioten, ziotezen, ziotsen, ziotseten, ziotsetezen, ziotsezen, ziotson, ziotsoten, ziotsotezen, ziotsozen, ziotsuen, ziotsueten, ziotsuetezen, ziotsuezen, ziotsun, ziotsuten, ziotsutezen, ziotsuzen, ziozaa, ziozaate, ziozana, ziozanate* — “say”;

*bagentoz, bagentozkie, bagentozkik, bagentozkin, bagentozkio, bagentozkizu, bagentozkizue, bahentor, bahentorkie, bahentorkigu, bahentorkio, bahentorkit, baletor, baletorkie, baletorkigu, baletorkik, baletorkin, baletorkio, baletorkit, baletorkizu, baletorkizue, baletoz, baletozkie, baletozkigu, baletozkik, baletozkin, baletozkio, baletozkit, baletozkizu, baletozkizue, banentor, banentorkie, banentorkik, banentorkin, banentorkio, banentorkizu, banentorkizue, bazentoz, bazentozkidate, bazentozkie, bazentozkiete, bazentozkigu, bazentozkigute, bazentozkio, bazentozkiote, bazentozkit, bazentozte, bentorkie, bentorkigu, bentorkik, bentorkin, bentorkio, bentorkit, bentorkizu, bentorkizue, betor, betoz, betozkie, betozkigu, betozkik, betozkin, betozkio, betozkit, betozkizu, betozkizue, dator, datorke, datorkiake, datorkidake, datorkie, datorkieke, datorkigu, datorkiguke, datorkik, datorkin, datorkinake, datorkio, datorkioke, datorkit, datorkizu, datorkizue, datorkizueke, datorkizuke, datorrela, datoz, datozela, datozke, datozkiake, datozkidake, datozkie, datozkieke, datozkigu, datozkiguke, datozkik, datozkin, datozkinake, datozkio, datozkioke, datozkit, datozkizu, datozkizue, datozkizueke, datozkizuke, etor, etorri, etorriko, etortze,*

*etortzen, gatoz, gatozen, gatozke, gatozkiake, gatozkian, gatozkie, gatozkieke, gatozkien, gatozkik, gatozkin, gatozkinake, gatozkinan, gatozkio, gatozkioke, gatozkion, gatozkizu, gatozkizue, gatozkizueke, gatozkizuen, gatozkizuke, gatozkizun, gentozen, gentozke, gentozkeen, gentozkiake, gentozkian, gentozkieke, gentozkiekeen, gentozkien, gentozkinake, gentozkinan, gentozkioke, gentozkiokeen, gentozkion, gentozkizueke, gentozkizuekeen, gentozkizuen, gentozkizuke, gentozkizukeen, gentozkizun, hator, hatorke, hatorkidake, hatorkie, hatorkieke, hatorkigu, hatorkiguke, hatorkio, hatorkioke, hatorkit, hentorke, hentorkeen, hentorkidake, hentorkidakeen, hentorkidan, hentorkieke, hentorkiekeen, hentorkien, hentorkiguke, hentorkigukeen, hentorkigun, hentorkioke, hentorkiokeen, hentorkion, hentorren, letorke, letorkiake, letorkidake, letorkieke, letorkiguke, letorkinake, letorkioke, letorkizueke, letorkizuke, letozke, letozkiake, letozkidake, letozkieke, letozkiguke, letozkinake, letozkioke, letozkizueke, letozkizuke, nator, natorke, natorkiake, natorkian, natorkie, natorkieke, natorkien, natorkik, natorkin, natorkinake, natorkinan, natorkio, natorkioke, natorkion, natorkizu, natorkizue, natorkizueke, natorkizuen, natorkizuke, natorkizun, natorren, nentorke, nentorkeen, nentorkiake, nentorkian, nentorkieke, nentorkiekeen, nentorkien, nentorkinake, nentorkinan, nentorkioke, nentorkiokeen, nentorkion, nentorkizueke, nentorkizuekeen, nentorkizuen, nentorkizuke, nentorkizukeen, nentorkizun, nentorren, zatoz, zatozke, zatozketete, zatozkidake, zatozkidakete, zatozkidate, zatozkie, zatozkieke, zatozkiekete, zatozkiete, zatozkigu, zatozkiguke, zatozkigukete, zatozkigute, zatozkio, zatozkioke, zatozkiokete, zatozkiote, zatozkit, zatozte, zentozen, zentozke, zentozkeen, zentozketen, zentozkidake, zentozkidakeen, zentozkidakete, zentozkidaketen, zentozkidan, zentozkidaten, zentozkieke, zentozkiekeen, zentozkiekete, zentozkieketen, zentozkien, zentozkieten, zentozkiguke, zentozkigukeen, zentozkigukete, zentozkiguketen, zentozkigun, zentozkiguten, zentozkioke, zentozkiokeen, zentozkiokete, zentozkioketen, zentozkion, zentozkioten, zentozten, zetorkeen, zetorkian, zetorkidakeen, zetorkidan, zetorkiekeen, zetorkien, zetorkigukeen, zetorkigun, zetorkinan, zetorkiokeen, zetorkion, zetorkizuekeen, zetorkizuen, zetorkizukeen, zetorkizun, zetorren, zetozen, zetozkeen, zetozkian, zetozkidakeen, zetozkidan, zetozkiekeen, zetozkien, zetozkigukeen, zetozkigun, zetozkinan, zetozkiokeen, zetozkion, zetozkizuekeen, zetozkizuen, zetozkizukeen, zetozkizun — “come”;*

*bagindoaz, bagindoazkie, bagindoazkik, bagindoazkin, bagindoazkio, bagindoazkizu, bagindoazkizue, bahindoa, bahindoakie, bahindoakigu, bahindoakio, bahindoakit, balihoa, balihoakie, balihoakigu, balihoakik, balihoakin, balihoakio, balihoakit, balihoakizu, balihoakizue, balihoaz, balihoazkie, balihoazkigu, balihoazkik, balihoazkin, balihoazkio, balihoazkit, balihoazkizu, balihoazkizue, banindoa, banindoakie, banindoakik, banindoakin, banindoakio, banindoakizu, banindoakizue, bazindoaz, bazindoazkidate, bazindoazkie, bazindoazkiete, bazindoazkigu, bazindoazkigute, bazindoazkio, bazindoazkiote, bazindoazkit, bazindoazte, bihoa, bihoaz, bihoazkie, bihoazkigu, bihoazkik, bihoazkin, bihoazkio, bihoazkit, bihoazkizu, bihoazkizue, bindoakie, bindoakigu, bindoakik, bindoakin, bindoakio, bindoakit, bindoakizu, bindoakizue, doa, doake, doakiake, doakidake, doakie, doakieke, doakigu, doakiguke, doakik, doakin, doakinake, doakio, doakioke, doakit, doakizu, doakizue, doakizueke, doakizuke, doala, doaz, doazela, doazke, doazkiake, doazkidake, doazkie, doazkieke, doazkigu, doazkiguke, doazkik, doazkin, doazkinake, doazkio, doazkioke, doazkit, doazkizu, doazkizue, doazkizueke, doazkizuke, gindoazen, gindoazke, gindoazkeen, gindoazkiake, gindoazkian, gindoazkieke, gindoazkiekeen, gindoazkien, gindoazkinake, gindoazkinan, gindoazkioke, gindoazkiokeen, gindoazkion, gindoazkizueke, gindoazkizuekeen, gindoazkizuen, gindoazkizuke, gindoazkizukeen, gindoazkizun, goaz, goazen, goazke, goazkiake, goazkian, goazkie, goazkieke, goazkien, goazkik, goazkin, goazkinake, goazkinan, goazkio, goazkioke, goazkion, goazkizu, goazkizue, goazkizueke, goazkizuen, goazkizuke, goazkizun, hindoake, hindoakeen, hindoakidake, hindoakidakeen, hindoakidan, hindoakieke, hindoakiekeen, hindoakien, hindoakiguke, hindoakigukeen, hindoakigun, hindoakioke, hindoakiokeen, hindoakion, hindoan, hoa, hoake, hoakidake, hoakie, hoakieke, hoakigu, hoakiguke, hoakio, hoakioke, hoakit, joan, joango, joate, joaten, lihoake, lihoakiake, lihoakidake, lihoakieke, lihoakiguke, lihoakinake, lihoakioke, lihoakizueke, lihoakizuke, lihoazke, lihoazkiake, lihoazkidake, lihoazkieke, lihoazkiguke, lihoazkinake, lihoazkioke, lihoazkizueke, lihoazkizuke, nindoake, nindoakeen, nindoakiake, nindoakian, nindoakieke, nindoakiekeen, nindoakien, nindoakinake, nindoakinan, nindoakioke, nindoakiokeen, nindoakion, nindoakizueke, nindoakizuekeen, nindoakizuen, nindoakizuke, nindoakizukeen, nindoakizun, nindoan, noa, noake, noakiake, noakian, noakie, noakieke, noakien, noakik, noakin, noakinake, noakinan, noakio, noakioke, noakion, noakizu, noakizue, noakizueke, noakizuen, noakizuke, noakizun, noan, zihoakeen, zihoakian, zihoakidakeen, zihoakidan, zihoakiekeen, zihoakien, zihoakigukeen, zihoakigun, zihoakinan, zihoakiokeen, zihoakion, zihoakizuekeen, zihoakizuen, zihoakizukeen, zihoakizun, zihoan, zihoazen, zihoazkeen, zihoazkian, zihoazkidakeen, zihoazkidan, zihoazkiekeen, zihoazkien, zihoazkigukeen, zihoazkigun, zihoazkinan, zihoazkiokeen, zihoazkion, zihoazkizuekeen, zihoazkizuen, zihoazkizukeen, zihoazkizun, zindoazen, zindoazke, zindoazkeen, zindoazketen, zindoazkidake, zindoazkidakeen, zindoazkidakete, zindoazkidaketen, zindoazkidan, zindoazkidaten, zindoazkieke, zindoazkiekeen, zindoazkiekete, zindoazkieketen, zindoazkien, zindoazkieten, zindoazkiguke, zindoazkigukeen, zindoazkigukete, zindoazkiguketen, zindoazkigun, zindoazkiguten, zindoazkioke, zindoazkiokeen, zindoazkiokete, zindoazkioketen, zindoazkion, zindoazkioten, zindoazten, zoaz, zoazke, zoazkete, zoazkidake, zoazkidakete, zoazkidate, zoazkie, zoazkieke, zoazkiekete, zoazkiete, zoazkigute, zoazkiguke, zoazkigukete, zoazkigute, zoazkio, zoazkioke, zoazkiokete, zoazkiote, zoazkit, zoazte —*

“go”.

*Example 9.6.2.* In Fig. S14, we further apply the aforementioned word clustering algorithm to topic extraction and machine translation (see Table S1 for text source).



## 9.2 Modified Porter stemming algorithm for Korean

We will be interested in analyzing Modern Korean literary works, written according to the South Korean standard after 1971. This means that texts are spelt out in the native Korean alphabet (known as *Hangul*), with spaces between words.<sup>108</sup> Each *Hangul* block represents exactly one syllable (see Algorithm 9.8 below for romanization of *Hangul*), hence we can use the “uniform reading speed” approximation described in [1, §2.1, Footnote 1].<sup>109</sup> We are not going to deal with an archaic mixed script style (where Sino-Korean vocabulary is spelt out with *Hanja*, the Chinese characters used in the Korean language), which is mostly restricted to academic and legal settings nowadays.<sup>110</sup>

In a Modern Korean translation (see Table S1 for text source) of *Pride and Prejudice*, the opening line reads

재산이 많은 미혼 남성이라면 반드시 아내를 필요로 한다는 말은 널리 인정되는 진리이다.

Its structure can be analyzed as follows:

|               |               |                 |           |             |                    |           |             |
|---------------|---------------|-----------------|-----------|-------------|--------------------|-----------|-------------|
| Hangul:       | 재산이           | 많은              | 미혼        | 남성이         | 라면                 | 반드시       | 아내를         |
| Mixed:        | 財産이           | 많은              | 未婚        | 男性이         | 라면                 | 반드시       | 아내를         |
| Romanization: | jaesan-i      | manh-eun        | mihon     | namseong-il | lameyeon           | bandeusi  | anae-leul   |
| Gloss:        | fortune.NOM   | much.PRS.DET    | unmarried | male        | be.COND            | certainly | wife.ACC    |
| Hangul:       | 필요로           | 한다는             | 말은        | 널리          | 인정되는               | 진리이다      |             |
| Mixed:        | 必要로           | 한다는             | 말은        | 널리          | 認定되는               | 眞理이다      |             |
| Romanization: | pilyo-lo      | handa-neun      | mal-eun   | neolli      | injeong-do         | neun      | jinli-ida   |
| Gloss:        | necessity.INS | do.IND.NPST.DET | word.TOP  | widely      | affirm.PAS.PRS.DET | truth     | be.IND.NPST |

where word stems are shown in red, and various functions of the suffixes include ACC = accusative, COND = conditional, DET = determiner, INS = instrumental, NOM = nominative, NPST = non-past, PAS = passive, PRS = present, TOP = topic. In principle, we want to automatically remove all kinds of grammatical suffixes from a Korean word, no matter the remaining stem is Sino-Korean (*i.e.* of ultimately Chinese origin) or not. In practice, we must admit to certain limitations in our current technology:

- Native Korean stems are sometimes subject to consonant changes. For example, 널리 neolli “widely”, 넓다 neolbda “to be wide” and 너비 neobi “width” are supposed to share the same stem, but their *Hangul* spellings in the first syllable have subtle differences. We will try our best to accommodate to such irregular Korean inflections, at the cost of misclassifying certain native Korean words.
- While Sino-Korean stems are immutable in inflections, they suffer from another serious problem: polysemy. Many words with distinguished pronunciations in Chinese become (nearly) homophonic<sup>111</sup> when adapted into Korean, so the disuse of Chinese characters in Korean writing causes ambiguities. Such pairs of *Hangul* homographs [and also (near) homophones] include 인정(認定) injeong “acknowledgement” vs. 인정(人情) injeong “humanity”; 화장(化粧) hwajang “cosmetics” vs. 화장(火葬) hwajang “cremation” etc. We can do nothing to solve such polysemy puzzles in our current work.
- Some native Korean words are spelt in the same way as Sino-Korean words, despite having very different meanings.<sup>112</sup> For example, we have 거리 geoli “road, street” vs. 거리(距離) geoli “distance”; 시장 sijang “hunger” vs. 시장(市場) sijang “market” and 시장(市長) sijang “mayor” etc. Again, we can do nothing right now, as we face Korean documents free from Chinese characters.
- Depending on context (which determines delicate shades of meaning), a given English word might be translated into either a native Korean word or a Sino-Korean word, with drastically different spellings. For example, both 마음 maeum and 심(心) sim mean “heart” in Korean, but there is no simple way to build such links algorithmically.<sup>113</sup> Traditionally, Koreans would learn each *Hanja* by juxtaposing its native Korean gloss with its Sino-Korean pronunciation, in a formula like 心 마음 심. For technical reasons, we have chosen not to feed our computer a long list of *Hanja* readings for rote learning.

<sup>108</sup>This distinguishes Korean texts from Chinese and Japanese ones. In the latter two cases, word segmentation is a non-trivial task.

<sup>109</sup>Vowel length is not marked in Korean spelling. Its effects on reading speed are ignored in our analysis.

<sup>110</sup>When Korean is written in the mixed script, rules for word segmentation are also somewhat different from the pure *Hangul* style. The current North Korean standard does not employ Chinese characters, but its spelling/spacing rules for Sino-Korean vocabulary are different from the practice in South Korea.

<sup>111</sup>For near homophones, we allow differences in vowel lengths that are not marked in *Hangul* spelling.

<sup>112</sup>There is a similar problem for words transliterated from English. For example, 다시 dasi could be a *Hangul* version of “Darcy” or a native Korean word meaning “again”; 제인 jein could be a *Hangul* version of “Jane” or a Sino-Korean word 제인(諸人) “all people”. In the present study, we draw on neighboring words [cf. Algorithm 3.25(4)] to decide whether 다시 means “again” (which is to be removed as a stop word), and regard all words in the form of 제인X as derivatives of “Jane”.

<sup>113</sup>There is a similar situation in Japanese, where the Chinese character 心 can be pronounced either ころ kokoro (native Japanese) or しん shin (Sino-Japanese). In Japanese, “heart” is always written out using the *kanji* 心, irrespective of pronunciation. Thus in text processing, it is trivial to identify native Japanese and Sino-Japanese versions of the same concept. However, even when Korean is written in the mixed script style, only the Sino-Korean vocabulary can be spelt out with *Hanja*, which typographically obscures the connection between native Korean and Sino-Korean counterparts.

Since the phonetic writing system of Modern Korean is a compromise between accuracy and efficiency, so will be our approximate clustering algorithm based on [45].

### 9.2.1 Stop words and transliterations

Korean stop words can carry various agglutinative suffixes. Instead of enumerating all of them in a single list, we will define several string patterns that match the criterion for stop words.

**Definition 9.7** (Korean stop words). Define the pattern **beKorean** as any one from the following list:

계세요, 계셔, 계셔서, 계셔야, 계세요, 계셨기, 계셨느냐, 계셨다, 계셨습니까, 계셨습니다, 계셨어, 계셨어요, 계셨음, 계시겠다, 계시겠습니다, 계시겠어, 계시겠어요, 계시고, 계시기, 계시느냐, 계시는, 계시는데, 계시니, 계시니까, 계시다, 계시더니, 계시려고, 계시면, 계시지만, 계신, 계신다, 계실, 계심, 계십니까, 계십니다, 계십시오, 아녀, 아녀서, 아녀야, 아녀요, 아녘기, 아녘냐, 아녘다, 아녘습니까, 아녘습니다, 아녘어, 아녘어요, 아녘음, 아니겠다, 아니겠습니까, 아니겠어, 아니겠어요, 아니고, 아니기, 아니냐, 아니니, 아니니까, 아니다, 아니다, 아니더니, 아니면, 아니세요, 아니셔, 아니셔서, 아니셔야, 아니셔요, 아니셨기, 아니셨냐, 아니셨다, 아니셨습니까, 아니셨습니다, 아니셨어, 아니셨어요, 아니셨음, 아니시겠다, 아니시겠습니까, 아니시겠어, 아니시겠어요, 아니시고, 아니시기, 아니시냐, 아니시니, 아니시니까, 아니시다, 아니시더니, 아니시면, 아니시지만, 아니신, 아니신데, 아니실, 아니심, 아니십니까, 아니십니다, 아니어서, 아니어야, 아니어요, 아니었기, 아니었음, 아니지만, 아닌, 아닌데, 아닐, 아님, 아님니까, 아닙니다, 였기, 였느냐, 였다, 였습니까, 였습니다, 였어, 였어요, 였음, 예요, 이겠다, 이겠습니까, 이겠어, 이겠어요, 이고, 이기, 이냐, 이니, 이니까, 이다, 이다, 이더니, 이면, 이세요, 이셔, 이셔서, 이셔야, 이셔요, 이셨기, 이셨냐, 이셨다, 이셨습니까, 이셨습니다, 이셨어, 이셨어요, 이셨음, 이시겠다, 이시겠습니까, 이시겠어, 이시겠어요, 이시고, 이시기, 이시냐, 이시니, 이시니까, 이시다, 이시더니, 이시면, 이시지만, 이신, 이신데, 이실, 이심, 이십니까, 이십니다, 이어서, 이어야, 이었기, 이었느냐, 이었다, 이었습니까, 이었습니다, 이었어, 이었어요, 이었음, 이에, 이에요, 이지만, 인데, 입니까, 입니다, 있겠다, 있겠습니까, 있겠어, 있겠어요, 있고, 있기, 있느냐, 있는, 있는데, 있다, 있다, 있더니, 있습니까, 있습니다, 있어, 있어서, 있어야, 있어요, 있었기, 있었느냐, 있었다, 있었습니까, 있었습니다, 있었어, 있었어요, 있었음, 있으니, 있으니까, 으면, 으세요, 으셔, 으셔서, 으셔야, 으셔요, 으셨기, 으셨냐, 으셨다, 으셨습니까, 으셨습니다, 으셨어, 으셨어요, 으셨음, 으시겠다, 으시겠습니까, 으시겠어, 으시겠어요, 으시고, 으시기, 으시냐, 으시니, 으시니까, 으시다, 으시더니, 으시면, 으시지만, 으신, 으신데, 으실, 으심, 으십니까, 으십니다, 있을, 있음, 있지만.

Define the pattern **notbeKorean** as any one from the following list:

없겠다, 없겠습니까, 없겠어, 없겠어요, 없고, 없기, 없느냐, 없는, 없는데, 없다, 없다, 없더니, 없습니까, 없습니다, 없어, 없어서, 없어야, 없어요, 없었기, 없었느냐, 없었다, 없었습니까, 없었습니다, 없었어, 없었어요, 없었음, 없으니, 없으니까, 없으면, 없으세요, 없으셔, 없으셔서, 없으셔야, 없으셔요, 없으셨기, 없으셨냐, 없으셨다, 없으셨습니까, 없으셨습니다, 없으셨어, 없으셨어요, 없으셨음, 없으시겠다, 없으시겠습니까, 없으시겠어, 없으시겠어요, 없으시고, 없으시기, 없으시냐, 없으시니, 없으시니까, 없으시다, 없으시더니, 없으시면, 없으시지만, 없으신, 없으신데, 없으실, 없으심, 없으십니까, 없으십니다, 없을, 없음, 없지만.

Define the pattern **becomeKorean** as any one from the following list:

돼, 돼라, 돼서, 돼야, 돼요, 됐기, 됐느냐, 됐다, 됐습니까, 됐습니다, 됐어, 됐어요, 됐음, 되, 되겠다, 되겠습니까, 되겠어, 되겠어요, 되고, 되기, 되느냐, 되는, 되는데, 되니, 되니, 되니까, 되다, 되더니, 되려고, 되면, 되세요, 되셔, 되셔서, 되셔야, 되셔요, 되셨기, 되셨느냐, 되셨다, 되셨습니까, 되셨습니다, 되셨어, 되셨어요, 되셨음, 되시겠다, 되시겠습니까, 되시겠어, 되시겠어요, 되시고, 되시기, 되시느냐, 되시는, 되시는데, 되시니, 되시니까, 되시더니, 되시라, 되시려고, 되시면, 되시지만, 되신, 되신다, 되실, 되심, 되십니까, 되십니다, 되십시오, 되어, 되어라, 있어서, 되어야, 되어요, 되었기, 되었음, 되자, 되지만, 된, 된다, 될, 됨, 됩니까, 됩니다, 됩시다, 됩시오.

Define the pattern **haveKorean** as any one from the following list:

가져라, 가져서, 가져야, 가져요, 가졌기, 가졌느냐, 가졌다, 가졌습니까, 가졌습니다, 가졌어, 가졌어요, 가졌음, 가지겠다, 가지겠습니까, 가지겠어, 가지겠어요, 가지고, 가지기, 가지느냐,

가지는, 가지는데, 가지니, 가지니까, 가지다, 가지더니, 가지려고, 가지면, 가지세요, 가지셔, 가지셔서, 가지셔야, 가지셔요, 가지셨기, 가지셨느냐, 가지셨다, 가지셨습니까, 가지셨습니다, 가지셨어, 가지셨어요, 가지셨음, 가지시겠다, 가지시겠습니까, 가지시겠어, 가지시겠어요, 가지시고, 가지시기, 가지시느냐, 가지시는, 가지시는데, 가지시니, 가지시니까, 가지시더니, 가지시라, 가지시려고, 가지시면, 가지시지만, 가지신, 가지신다, 가지실, 가지심, 가지십니까, 가지십니다, 가지십시오, 가지어라, 가지어서, 가지어야, 가지어요, 가지었기, 가지었음, 가지자, 가지지만, 가진, 가진다, 가질, 가짐, 가집니다, 가집시다, 가집시오, 갖겠다, 갖겠습니까, 갖겠어, 갖겠어요, 갖고, 갖기, 갖느냐, 갖는, 갖는다, 갖는데, 갖더니, 갖습니까, 갖습니다, 갖아, 갖아라, 갖아서, 갖아야, 갖아요, 갖았기, 갖았느냐, 갖았다, 갖았습니까, 갖았습니까, 갖았어, 갖았어요, 갖았음, 갖으니, 갖으니까, 갖으려고, 갖으면, 갖으세요, 갖으셔, 갖으셔서, 갖으셔야, 갖으셔요, 갖으셨기, 갖으셨느냐, 갖으셨다, 갖으셨습니까, 갖으셨습니다, 갖으셨어, 갖으셨어요, 갖으셨음, 갖으시겠다, 갖으시겠습니까, 갖으시겠어, 갖으시겠어요, 갖으시고, 갖으시기, 갖으시느냐, 갖으시는, 갖으시는데, 갖으시니, 갖으시니까, 갖으시더니, 갖으시라, 갖으시려고, 갖으시면, 갖으시지만, 갖으신, 갖으신다, 갖으실, 갖으심, 갖으십니까, 갖으십니다, 갖으십시오, 갖은, 갖을, 갖음, 갖읍시다, 갖읍시오, 갖자, 갖지만.

Define the pattern **KoreanStopRoot** as any one from the following list:

가운데, 가져, 개, 거기, 거니, 거라, 거야, 거였, 거예, 거의, 건너편, 겁니, 꽃, 귀하, 그러나, 썩나겠, 썩나느, 썩나는, 썩나니, 썩나더, 썩나려, 썩나세, 썩나셔, 썩나셨, 썩나시, 썩나신, 썩나십, 썩나자, 썩나지, 썩납니, 썩납시, 썩났, 썩보, 썩본, 썩볼, 썩봄, 썩뵈, 썩뵈, 썩뵈, 썩뵈, 썩뵈, 썩뵈, 나네, 나도, 나라면, 나로, 나를, 나만, 나보다, 나중, 나쳐, 나한테, 난다, 남게, 남는, 남들, 남에, 남은, 남을, 남의, 남한테, 내게, 내겐, 너도, 너를, 너만, 너만큼, 너무, 너에, 너와, 너한, 너희, 누구, 누군가, 다음, 당신, 대개, 대신, 대하여, 덕분에, 도중, 되겠, 되나, 되던, 되려, 되리, 되었, 되지, 뒤에, 들끼리, 때까, 때는, 때도, 때때로, 때로, 때마다, 때만, 때만큼, 때면, 때문, 때보다, 때부터, 때에, 때조차, 라고, 마찬가지로, 만큼, 많, 몇, 모두, 모든, 못하, 못했, 무렵, 무엇, 무척, 뭐, 뭘, 뭣, 바에, 별로, 본인, 불과, 뿐이, 뿐입, 속으로, 수시로, 스스로, 심지어, 십상이, 아니, 아니요, 아무, 아직, 안에, 안으로, 안은, 안을, 앓, 애들, 애야, 어느, 어디, 어딘, 어딜, 어때, 어땀, 어떠, 어떤, 어떻게, 어떻, 어찌, 어쩔, 어썸, 언제, 얼마, 없게, 없겠, 없었, 없으, 없이, 없지, 여러, 여부, 여전, 옳, 예가, 오로지, 왜냐, 외치곤, 우리, 위까, 위로, 위를, 위부터, 위에, 위의, 이라고, 이래, 이랬, 이러, 이런, 이럴, 이럼, 이렇, 이로, 이리, 이만, 이분, 이와, 이외, 이전, 이제, 이쯤, 이후, 일도, 일쭙, 일은, 일을, 일이, 일인, 일하, 있, 자기, 자네, 자신, 자체, 저기, 저까, 저로, 저만큼, 저처럼, 저한테, 저희, 전과, 전까, 전보다, 전부터, 전에, 전으로, 전쯤, 전혀, 절대, 정도, 제가, 제게, 중에, 중이, 지금, 지난, 지마느, 지마세, 지마셨, 지마시, 지마십, 지말겠, 지말더, 지말려, 지말았, 지말지, 지맙니, 지맙시, 차라리, 최소, 텐데, 하거, 하겠, 하고, 하곤, 하기, 하긴, 하나, 하네, 하는, 하니, 하다, 하더, 하던, 하든, 하려, 하며, 하면, 하면서, 하세, 하셨, 하시, 하여, 하지, 한다, 한데, 할지, 함께, 해서, 해야, 해왔, 해주, 해준, 해줄, 했, 현재, 흑시, 흑은, 혼자, 후에, 훨씬.

Define the pattern **KoreanStopString** as any one from the following list:

가끔, 가장, 간에, 갖게, 갖은, 같이, 개, 거, 거고, 거나, 거는, 거닌, 거다, 거면, 거야, 거에요, 거예요, 거요, 건, 결, 결로, 겁니다, 것이다, 것입니다, 게, 게다가, 결코, 겸, 고로, 곧, 곧잘, 그, 그대, 그래서, 그러나, 그러면, 그리, 그리고, 그리도, 그만, 그만큼, 금방, 기껏해야, 썩나, 썩나고, 썩나기, 썩나는, 썩나니, 썩나라, 썩나면, 썩나서, 썩나셔, 썩나신, 썩나실, 썩나십, 썩나야, 썩나요, 썩나자, 썩난, 썩난다, 썩날, 썩납, 나, 나는, 나에, 나와, 나의, 난, 남, 내, 내가, 내게, 내내, 내로, 너, 너는, 너무, 너의, 널, 네, 네가, 누가, 늘, 다, 다들, 다소, 대로, 대체로, 맥, 맥은, 더, 더구나, 더욱, 덜, 데, 데가, 데서, 도로, 동안, 되어, 된, 등, 듯, 듯도, 따라, 따라서, 따름, 판, 때, 때껏, 또, 라도, 리, 리가, 마, 마나, 마니, 만, 매우, 맨, 먼저, 모든, 못, 무릇, 무슨, 미리, 바람에, 밖에, 번째, 벌써, 뿐, 사이, 사이에, 서로, 서로서로, 수, 수가, 수는, 아니면, 아마, 아마도, 아주, 안, 앞으로, 애, 어느, 어따, 어떤, 어떻게, 어차피, 언제나, 얼마나, 없, 여기, 옆에, 예, 오히려, 온, 온갖, 왜, 웬, 이, 이는, 이들, 이래, 이로, 이를, 이리, 이미, 이번, 이상, 이상는, 이상에, 이상으로, 이상은, 이상을, 이상의, 이상이, 일, 자, 자넨, 자넨, 자주, 잘, 채, 저, 저기, 저나, 저는, 저도, 저를, 저의, 적, 적이, 전, 전에, 전의, 제, 조금, 줌, 좀처럼, 좀체, 줄, 즉, 지, 지가, 지는, 지마는, 지마니, 지마셔, 지마신, 지마실, 지마십, 지만, 지말, 지말고, 지말기, 지말면, 지말아, 지말자, 지맙, 짝이, 쪽, 채, 채로, 펍, 하고, 하여금, 하지만, 한, 한번, 한번도, 해, 해도, 해라, 해요, 했어, 후, 후로, 흔히.



### 9.2.2 Effective spelling and essential root

Like Japanese, the Korean language has two separate numeral systems, one native and one Chinese, which appear in different contexts. The following algorithm handles this special feature of Korean.

**Algorithm 9.9** (Clustering of Korean numerals). Define **CntKorean** as the following pattern:

(가지개대마리명|번|분|사|람|잔|장|채)(0|가|과|와|의|이).

For a string  $\hat{\sigma}$ , we define  $\text{KorNum}(\hat{\sigma})$  by the following procedures:

- (1) Check whether  $\hat{\sigma}$  matches exactly the pattern  $(\emptyset|제)(\mathbf{D}|구|넷|다|섯|두|둘|삼|세|셋|십|아|홉|어|섯|여|덟|열|육|이|일|일곱|칠|팔|하|나|한)_m(\emptyset|\text{CntKorean}|시|째)$ , where  $\mathbf{D} = (0|1|2|3|4|5|6|7|8|9)$ . If no, define  $\text{KorNum}(\hat{\sigma}) = \hat{\sigma}$  and quit; if yes, go to the next step.
- (2) Work on  $\hat{\sigma}$  as follows:
  - (2.1) Do  $\sim(\text{시}|째|\text{CntKorean}) \rightarrow \emptyset$ ,  $제 \sim \rightarrow \emptyset$ .
  - (2.2) Do  $\sim(\text{구}|아|홉) \rightarrow '9$ ,  $\sim\text{넷} \rightarrow '4$ ,  $\sim\text{다}\text{섯} \rightarrow '5$ ,  $\sim(\text{두}|둘|\text{이}) \rightarrow '2$ ,  $\sim(\text{삼}|세|\text{셋}) \rightarrow '3$ ,  $\sim(\text{십}|열) \rightarrow '0$ ,  $\sim(\text{어}\text{섯}|\text{육}) \rightarrow '6$ ,  $\sim(\text{여}|덟|\text{팔}) \rightarrow '8$ ,  $\sim(\text{하}|나|\text{한}) \rightarrow '1$ ,  $\sim(\text{일}|곱|\text{칠}) \rightarrow '7$ .
  - (2.3) Repeat the last step.
  - (2.4) Do  $' \rightarrow \emptyset$ .
  - (2.5) Call the result so far as  $\hat{\sigma}'$ , and define  $\text{KorNum}(\hat{\sigma}) = \text{숫}\hat{\sigma}'$ .

**Algorithm 9.10** (Regularization of Korean verbs). For a Korean word  $\hat{\sigma}$ , its “regularized verb form”  $\text{RegVb}(\hat{\sigma})$  is defined through the following procedures:

- (1) If  $\hat{\sigma}$  contains  $\text{없}$  and does not start with  $\text{없}$ , then replace it by  $\text{없}\hat{\sigma}$ ; otherwise, leave it intact.
- (2) Replace

|                                     |                              |                                  |                        |
|-------------------------------------|------------------------------|----------------------------------|------------------------|
| (0 새 시)(과 퍼)(라 란 랑 래 랬 러 런 렁 레 렸)X~ |                              | (거 까 꺼 겨)(마 만 망 매 맺 머 먼 명 메 맺)X~ |                        |
| 과랑                                  |                              | 까망                               |                        |
| (검 검 정 감 장)~                        | (노 누)(라 란 랑 래 랬 러 런 렁 레 렸)X~ | (발 벌 빨 빨)                        | (가 간 강 개 갸 겨 긴 경 계 게)~ |
| 까망                                  | 노랑                           | 발강                               |                        |
| (보 뵤)(야 연 양 애 엿)X~                  | (부 뵤)(여 연 영 예 엿)X~           | (하 허)(야 연 양 양 애 엿 여 연 영 영 예 엿)X~ |                        |
| 뵤양                                  | 뵤양                           | 하양                               |                        |
| X $\in$ (곱 뵤 수 좁 썩 입 잡 접 좁)~        | X $\in$ (냥 녕 닿 짙)~           | X $\in$ (단 둔 쏟 언)~               | X $\in$ (빗 빼 앗 숫 셋)~   |
| X뵤                                  | X히려                          | X뜰                               | X숫                     |
| 그(쳐 쳐 치 친 칠 침 침)~                   | 그만~                          | 노래(doKorean 개 는 로 를 에 와 의)X~     |                        |
| 그칩                                  | 그맏                           | 노래                               |                        |
| 돌아(보 본 볼 붐 붐 뵤 뵤)X~                 | 만(나 난 날 남 남 났)X~             |                                  | 붐~                     |
| 랬 뵤다                                | 뵤                            |                                  | 발강                     |
| 여(느 느 네 니 세 셔 섯 시 실 심 심)~           | 열(쟁 고 기 더 니 면 어 였 지만)~       |                                  |                        |
| 엽                                   | 엽                            |                                  |                        |
| 일(은 을)~                             | 허영심~                         | (연 다 열)                          | 건(0 다)                 |
| 일하다                                 | 허용썩                          | 엽                                | 걸다                     |
|                                     |                              |                                  | 이름(0 은 을)              |
|                                     |                              |                                  | 성함                     |

- (3) Do  $\text{마}(\text{셔}|섯|\text{시}|\text{신}|\text{실}|\text{심}|\text{심})\sim \rightarrow \text{마썩}$ ,  $\hat{\chi}\text{어}(\text{보}|\text{본}|\text{볼}|\text{붐}|\text{붐}|\text{뵤}|\text{뵤})\text{X}\sim \rightarrow \hat{\chi}'\text{다}$ , where  $\hat{\chi}'$  derives from  $\hat{\chi}$ , after replacing the latter's final  $\text{ㄷ}$  (if present) with  $\text{ㄷ}$ .<sup>115</sup>

**Algorithm 9.11** (Korean normalization). For a Korean word  $\hat{\sigma}$ , its normalized form  $\text{KN}(\hat{\sigma})$  is constructed in the following steps:

- (1) Do  $\text{X}\in(\text{가}|게|\text{가}|구|\text{거}|실|\text{구}|실|\text{소}|리|\text{시}|시|\text{지}|집|\text{일}|시|\text{포}|도|\text{포}|함)\sim \rightarrow \text{X}\text{함}$  on  $\text{RegVb}(\hat{\sigma})$ .<sup>116</sup>

<sup>115</sup>In practice, such a replacement needs both  $\text{HgRom}$  and  $\text{RomHg}$  to take effect.

<sup>116</sup>The second syllable in many Sino-Korean stems may resemble a Korean suffix. To avoid misidentification of suffixes, we need to protect such stems by a blocker syllable  $\text{함}$ .

## (2) Replace

|                                                               |                     |                               |                           |                       |                      |                    |
|---------------------------------------------------------------|---------------------|-------------------------------|---------------------------|-----------------------|----------------------|--------------------|
| (∅만)(아드님 아들)~<br>엿썰                                           |                     | (가르 가른 가름 가름 가름 갈라 갈랐)~<br>꺾틀 |                           |                       |                      |                    |
| (대 아 어)(보(이) 본 볼 봄 봄 꽤 봤(자))X~<br>뿔뿔                          |                     |                               | (매일 하루)~<br>날             |                       | (문 물 엿 물으)~<br>몬뜰    |                    |
| (벼 서 벼 야 벼 요 벗 기 벗 내 벗 다 벗 습 벗 어 벗 음 빈 데 립 니)X~<br>옻뿔         |                     |                               |                           | (배 뵈 뵈 빈 뵈 뵈 뵈)~<br>보 |                      |                    |
| (이 르 이 른 이 름 이 름 이 름 일 러 일 렀)X~<br>룻웁                         |                     |                               | 가(려 고)렀 리 린 릴 림 립)~<br>꺾웁 |                       | 갈~<br>가다             |                    |
| 결혼식~<br>결혼썰                                                   | 경(doKorean)X~<br>경쟁 | 그리워~<br>∅                     | 늘어(농 서 선 설 섬 섬)~<br>늪늪    | 다(르 리 릴 림 립)X~<br>뿔뿔  |                      |                    |
| 떨어(저 졌 지 진 질 짐 집)X~<br>뿔뿔                                     |                     | 떨어뜨X~<br>뿔                    | 메리턴~<br>메릴턴               | 목사관~<br>목사관           | 물려받~<br>입웁           | 배우자~<br>배웁         |
| 비(졌 고 기 냐 니 다 더 면 세 서 셨 시 신 실 심 십 어 었 우 운 울 움 웁 위 웠 지)~<br>옻뿔 |                     |                               |                           | 쓸데~<br>쓸뿔             | 쓸쓸(doKorean)X~<br>뿔뿔 |                    |
| 어(렵)(려(우 운 울 움 위 웠))~<br>어렵                                   |                     | 어리석~<br>어리썰                   | 일으(켜 켰 키 킨 킬 킴 킵)X~<br>꺾  |                       | 일이X~<br>일하다          | 조지아나~<br>조썰        |
| 친(doKorean)X~<br>친구                                           |                     | 침~<br>침                       | 하녀장~<br>하녀쟁               | 햄~<br>햄               | (벼 비 빈 뵈 뵈)<br>옻뿔    | 달(라 고 라 셔 래)<br>주다 |

## (3) If the string so far begins with any one of the following list:

가문, 가치, 강요, 거리, 거만, 게임, 겨우, 겨울, 견해, 결과, 결심, 결함, 경고, 경련, 경쟁, 고개, 고기, 고려, 고문, 고민, 고의, 고집, 곰곰, 과거, 과시, 관대, 관련, 관리, 관심, 구름, 구입, 군대, 권리, 기대, 기만, 기분, 기여, 기운, 기울, 기질, 기혼, 끝내, 나름, 나무, 나이, 날아, 노골, 노출, 단언, 달리, 당당, 대가, 대기, 대기, 대단, 대답, 대면, 대지, 도구, 도도, 도리, 도서, 동기, 동네, 동요, 동의, 두려, 둘러, 드리, 떠올, 런던, 리지, 마디, 마련, 마을, 마음, 마치, 맞이, 머리, 메리, 모습, 목숨, 몹시, 무례, 무시, 무심, 물건, 물려, 물려, 물론, 물리, 미래, 바람, 바보, 반대, 방도, 방심, 방어, 방입, 방자, 방치, 방해, 배려, 배신, 변심, 부대, 부러, 부분, 부여, 부자, 분개, 분들, 불리, 비중, 비참, 사건, 사고, 사과, 사라, 사랑, 사실, 사이, 사치, 상대, 서재, 섬세, 성함, 세대, 세련, 세심, 소개, 소리, 소심, 소중, 속도, 손님, 수고, 수입, 수처, 시골, 시기, 시도, 시선, 식구, 신랑, 신분, 신중, 아래, 아침, 안심, 암시, 압니, 압시, 양도, 양심, 얼굴, 여름, 여보, 여성, 여인, 여자, 역할, 연구, 연기, 연대, 연습, 연인, 연주, 연출, 열심, 열중, 염려, 예의, 오래, 오만, 오해, 외출, 요구, 요리, 용서, 우려, 우아, 우울, 원래, 원인, 위대, 유감, 유리, 유일, 유지, 의도, 의무, 의문, 의미, 의심, 의아, 의자, 의지, 이유, 이의, 이자, 이치, 이해, 일반, 일어, 일치, 임대, 입구, 자랑, 자리, 자립, 자만, 자세, 자연, 자질, 잠시, 장교, 장군, 장담, 장면, 재산, 적당, 전이, 절대, 점심, 점잖, 정당, 정리, 정보, 정신, 정오, 정중, 제인, 조건, 조심, 조지, 조치, 존재, 존중, 주로, 주요, 주의, 주인, 중대, 중심, 중요, 중재, 지나, 지시, 지인, 지참, 지체, 지출, 직접, 진실, 진심, 진지, 질녀, 집중, 차이, 차지, 책임, 처리, 처신, 처치, 천재, 초과, 초대, 초래, 추구, 축하, 충고, 친구, 태도, 편안, 편지, 피로, 하녀, 하인, 한가, 한심, 합의, 합치, 호감, 호기, 화랑, 화려, 화해, 확고, 확보, 확신, 확실, 확인,

then insert **했** as the third syllable.

## (4) Replace

|                                                  |               |               |                                                  |                                         |               |
|--------------------------------------------------|---------------|---------------|--------------------------------------------------|-----------------------------------------|---------------|
| (∅고)남성~<br>남쟁                                    | (∅고)남아~<br>뿔값 | (∅고)남자~<br>뿔값 | (∅고)남편~<br>남편                                    | (∅만)(따 님 딸)~<br>뿔뜰                      | (가 나)싫~<br>쟁값 |
| (계 수 동 서 새 엔 니 시 누 이 올 케 제 수 처 제 처 형 형 수)~<br>꺾꺾 |               |               |                                                  | (고 모 숙 모 이 모 작 은 어 머 니 큰 어 머 니)X~<br>꺾꺾 |               |
| (금 일 오늘)~<br>금웁                                  |               |               | (길 쟁 길 고 길 기 길 대 길 더 길 면 길 어 길 었 길 지 집 니)~<br>룻룻 |                                         |               |

|                                          |                                                    |                                       |                                   |                         |                     |               |
|------------------------------------------|----------------------------------------------------|---------------------------------------|-----------------------------------|-------------------------|---------------------|---------------|
| (남동생 브라더 아우 오라버님 오빠 형 님 형제)X~<br>별똥      | (내 명)일~<br>뽕끗                                      | (년 단 란 잔)말(씀 이)~<br>엿밧                |                                   |                         |                     |               |
| (누나 누이 시스터 언니 여동생 자매)X~<br>졌튀            |                                                    | (도움 돕)X~<br>헛헛                        |                                   |                         |                     |               |
| (동서 매부 시동생 시매부 시숙 시아주버니 제부 처남 형부)~<br>땡땡 |                                                    | (드 올)(려 렸 리 린 릴 림 립)~<br>주            |                                   |                         |                     |               |
| (마누라 와이프 집사람)~<br>아내                     | (먼 지 우 선 처 음 척)~<br>뽕썰                             | (모르 모른 모를 모름 모릅 몰라 몰랐)~<br>얏늑         | (미 답 민)~<br>밧뽕                    |                         |                     |               |
| (바로 바르 바른 바를 바름 바릅 발라 발랐)X~<br>썰넛        | (봄 봐 봤)~<br>보                                      | (부르 부른 부를 부름 부릅 불리 불렸)~<br>뽕끗         |                                   |                         |                     |               |
| (부친 아버지 아빠 어비)~<br>뽕썰                    | (숙부 아저씨 외삼촌 친삼촌)X~<br>꾸썰                           | (씨 쪄 쓴 쓸 썰)X~<br>쓰다                   | (아이 애 들 자식)~<br>썰뽕                |                         |                     |               |
| (안 대 알)~<br>얏늑                           | (애 이야)기~<br>툭큭                                     | (어 머니 어 미 엄 마)~<br>모친                 | (이 어 이 였 이 은 이 을 이 음 잇)~<br>잇뤼    |                         |                     |               |
|                                          | (자르 자른 자를 자름 자릅 잘라 잘랐)~<br>쪄깅                      |                                       | (조 카 딸 질 녀)X~<br>쪄뽕               |                         |                     |               |
|                                          | (추우 추운 추울 추움 추워 추웠 춥 쪄 춥 기 춥 더 춥 디 춥 습 춥 지)~<br>꺄꺄 |                                       |                                   |                         |                     |               |
| X <sup>ε</sup> ( <del>어</del> 대)답~<br>X뽕 | 가르(쳐 쳤 치 친 칠 침 칩)X~<br>뽕툭                          | 갈(졌 고 더 려 면 아 왔 지만)~<br>꺄             | 값~<br>꺄                           | 감X~<br>꺄X               |                     |               |
|                                          | 강(doKorean)X~<br>강창                                | 걸렸X~<br>걸리다                           | 검~<br>검킵                          | 검(니 시)X~<br>행거걸다        | 경우X~<br>꺄유          |               |
|                                          | 고말(doKorean)X~<br>말하다                              |                                       | 구(doKorean)X~<br>꺄꺄               | 굳~<br>꺄                 | 그~<br>꺄             | 금~<br>꺄꺄      |
| 기(냐 니 세 셔 쪄 시 신 실 심 심 심)~<br>뽕툭          | 길이~<br>뽕툭                                          | 깊~<br>뽕툭                              | 까(보 본 볼 봄 봐 봤)~<br>썰깅             | 나(개 간 갈 감 꺄 꺄)X~<br>나가니 |                     |               |
| 나(아 왔 의 은 을 음 읍)X~<br>넛                  | 나(은 을 음 읍 와 왔)X~<br>꺄넛                             | 너비X~<br>넛다                            | 놀(래 란 랄 람 랴 랴)X~<br>썰랴            | 늘~<br>꺄랴                |                     |               |
|                                          | 느(껴 졌 끼 킨 꺄 꺄 꺄)~<br>느끼                            | 다가X~<br>얏랴                            | 다시X~<br>탈꺄                        | 달(doKorean)X~<br>뤼뤼     |                     |               |
| 달(도 만 에 은 이 제 쪄)~<br>윳                   | 달(라 랴 리)X~<br>뽕꺄                                   | 달라(요)X~<br>얏츄                         | 답~<br>뽕                           | 답~<br>뽕                 | 대(doKorean)X~<br>꺄꺄 | 데(려 리)~<br>데뤼 |
| 돌아(개 간 갈 꺄 꺄 꺄)X~<br>랴꺄다                 | 돌아(오 은 을 음 읍 와 왔)X~<br>랴와라                         |                                       | 드(느 니 니 세 셔 쪄 시 신 실 심 심)X~<br>뽕뽕다 |                         |                     |               |
| 드(세 셔 쪄 시 신 실 심 심)X~<br>먹다               | 드러(내 난 날 남 남 났)X~<br>얏꺄                            |                                       | 들(려 렸 르 른 를 름 름)X~<br>뽕꺄          |                         |                     |               |
| 들(렸 리 린 릴 림 립)X~<br>든다                   | 들려(오 은 을 음 읍 와 왔)X~<br>든다                          |                                       | 들어(개 간 갈 꺄 꺄 꺄)X~<br>얏꺄다          |                         |                     |               |
|                                          | 들어(도 주 준 줄 쪄 쪄 쪄)X~<br>든다                          |                                       | 들어(라 서 야 요)~<br>든다                |                         |                     |               |
|                                          | 들어(서 외 선 설 심 섭)X~<br>얏서다                           |                                       | 들어(오 은 을 음 읍 와 왔)X~<br>얏와라        |                         | 들었X~<br>든다          |               |
|                                          | 듬(니 시)X~<br>뽕뽕다                                    | 떠(내 난 날 났)~<br>뤼툭                     | 뽕~<br>뽕닝                          | 리디아~<br>리떡얏             | 마리아~<br>꺄꺄          |               |
|                                          | 만(doKorean)X~<br>꺄츄                                |                                       | 말(려 렸 리 린 릴 림 립)~<br>마르           |                         | 맘~<br>마훗            | 멤~<br>멧       |
|                                          |                                                    | 모(아 왔 여 였 의 은 을 음 읍 이 인 일 임 입)~<br>꺄넛 |                                   |                         |                     | 몸~<br>뽕뽕      |

|                                     |                       |              |                          |                        |                |                        |                         |                   |             |        |        |
|-------------------------------------|-----------------------|--------------|--------------------------|------------------------|----------------|------------------------|-------------------------|-------------------|-------------|--------|--------|
| 못~<br>뿔                             | 무도회~<br>무도회           | 미움X~<br>미움   | 바(라)란(랄)랍(랏)~<br>뿔       |                        | 반~<br>뽕        | 반아들~<br>뽕해들            | 밤~<br>뽕                 | 뽕~<br>뽕           | 뽕~<br>뽕     |        |        |
| 보잘~<br>뽕                            | 비(doKorean)X~<br>뽕뽕뽕  |              | 상(doKorean)X~<br>뽕       |                        | 샘~<br>뽕        | 생각X~<br>생각             | 세(우 운 울 움 읍 위 웠)X~<br>뽕 |                   |             |        |        |
| 손(실)해~<br>뽕                         |                       | 숨~<br>뽕      | 싫~<br>싫                  | 심(doKorean)X~<br>뽕     |                |                        | 쓸(테모)X~<br>뽕            |                   |             |        |        |
| 아(느 는 니 세 셨 시 신 실 심 십)X~<br>뽕       |                       |              | 얇~<br>뽕                  | 어(려 렸 리 린 릴 림 립)~<br>어 |                | 어(쨌 쨌 찌 쩐 쩨 쩨 쩨)~<br>어 |                         | 업~<br>업           |             |        |        |
| 옛~<br>뽕                             | 오(가 간 갈 감 갑 갓)X~<br>뽕 |              | 웁~<br>뽕                  | 웁~<br>뽕                | 웁~<br>뽕        | 웁~<br>뽕                | 의(의)거(doKorean)X~<br>뽕  |                   |             |        |        |
| 이(루 룬 룰 룸 뤼)~<br>뽕                  |                       |              | 일(doKorean)X~<br>일       |                        | 일라이자~<br>엘리자베스 |                        | 일~<br>뽕                 | 입(에 은 을 이)X~<br>뽕 |             |        |        |
| 자(라)란(랄)랍(랏)~<br>뽕                  |                       | 잡수X~<br>먹다   | 적(혀 혔 히 힌 힐 힘 힝)X~<br>쓰다 |                        |                | 전(doKorean)X~<br>뽕     |                         | 뽕~<br>뽕           |             |        |        |
| 정(doKorean)X~<br>뽕                  |                       | 좋아(오)X~<br>뽕 | 주기X~<br>주                | 주시(doKorean)X~<br>뽕    |                | 준다X~<br>주              | 줘~<br>주                 | 즐거X~<br>즐         | 집~<br>집     |        |        |
| 차(려 렸 리 린 릴 림 립)~<br>뽕              |                       |              | 참~<br>뽕                  | 칭(doKorean)X~<br>뽕     |                | 춤~<br>뽕                | 크리스마스~<br>뽕             | 탓~<br>뽕           |             |        |        |
| 피(doKorean)X~<br>뽕                  |                       | 합~<br>뽕      | 해리엇~<br>해                | 화가X~<br>화              | 힐~<br>뽕        | 간~<br>가                | (긴)긴(데)길<br>뽕           |                   |             |        |        |
| (의)매(주 의)까지 나만 컴 부터 쯤((에)였 일)X<br>뽕 |                       |              | (거)걸(겔)<br>행             |                        | (돈)돈<br>뽕      | (든)대(들)뽕<br>뽕          | (본)본(대)뽕<br>뽕           |                   |             |        |        |
| (안)앞<br>뽕                           | 달<br>월                | 드<br>뽕       | 들려(의)야(요)<br>듣다          |                        | 들어<br>듣다       | 쓰<br>쓰다                | 아<br>항                  | 야<br>쌍            | 오(게)지<br>오면 | 입<br>뽕 | 준<br>주 |

and do (두쨌두고두기두느두는두니두데두려두면두세두셔두셨두시두신두실두심두십두어두였두자두지둔대뽕니뽕시)~→뽕, 나오(의)쨌다쨌습다쨌어쨌어요고기너래느내는테니니까더니려고면세요셔셔셔야셔요쨌기쨌는내쨌다쨌습니까쨌습다쨌어쨌어요쨌음시쨌다시쨌습다시쨌어시쨌어요시고시기시느내시는테시니시니까시더니시라시려고시면시지만신신대실심십니까십니대십시자지지만)X~→뽕, 매<sup>X1</sup>(년|달|번|월|일)(의)까지|나만|컴|부터|을|이|쯤((에)일)X) → X<sub>1</sub>, where X<sub>1</sub> results from doing 년→연, 달→월 on X<sub>1</sub>.

- (5) Do X<sup>ε</sup>(들어부당부인부추상당상세상실상심상의상인)~ → X<sup>합</sup>.
- (6) Do (가)거(라)가(려)고(가)면(가)서(가)세(와)가(셔)가(셔)서(가)셔(야)가(셔)요(가)시(느)내(가)시(려)고(가)시(면)가(신)가(신)대(가)실(가)심(간)다)X~ → 가다, (거)내(거)느(거)는(거)니(거)세(거)셔(거)셨(거)시(거)신(거)심(거)십(거)테(거)겔(거)겔(거)고(거)걸(거)걸(거)기(거)걸(거)대(거)덜(거)덜(거)려(거)겔(거)면(거)겔(거)자(거)겔(거)지(거)겔(거)니(거)겔(거)시)X~ → 행(거)걸(다), (낫)총(최)선)~ → 뽕, (키)쨌(크)린(클)룸(킵)~ → 뽕, 고(말)(의)야)~ → 고(말), 뽕(추)춘(출)춤(취)쨌)~ → 뽕, 남)~ → 뽕, 달(려)렸(리)린(릴)림(립)~ → 뽕, 들(쨌)려(고)면(어)X~ → 뽕, 들(어)은(을)음)X~ → 듣다, 말)~ → 말(뽕), 오(쨌)고(기)너(래)느(내)는(니)더(니)도(록)라(려)고(면)세(요)셔(셔)셨(시)신(신)대(실)심(십)니(까)십(니)대(십)시(자)지(지)만)X~ → 와(라), 이(어)였)~ → 잇, 입)~ → 읊, 점)~ → 껌(뽕), 주(게)까)X~ → 주, (나)가(나)간)~ → 뽕, (온)온(대)울(움)웁(니)까(웁)니(대)웁(시)대(웁)시(오)와(와)서)~ → 와(라).

**Algorithm 9.12** (Korean effective spelling). Set V = {a|e|i|o|u|y}. For a Korean word  $\hat{\sigma}$ , its effective spelling EffSpell( $\hat{\sigma}$ ) is constructed in the following steps:

- (1) Do  $\hat{\chi}$ 한테X →  $\hat{\chi}$  before applying Korean normalization.
- (2) Do 리<sup>합</sup> → 뽕<sup>합</sup>, 하<sup>합</sup> → 항<sup>합</sup>, 한<sup>합</sup> → 함<sup>합</sup>, 할<sup>합</sup> → 함<sup>합</sup>, 할<sup>합</sup> → 함<sup>합</sup>, 함<sup>합</sup> → 함<sup>합</sup>, 해<sup>합</sup> → 함<sup>합</sup>.
- (3) Do  $\hat{\chi}$ (beKorean|becomeKorean)(의)당)doKorean)X →  $\hat{\chi}$ .
- (4) Define KoreanNounSuff as the pattern (의)건(걸)것(게)쪽)(의)들(뿐)뽕만)(의)가(과)랑(로)로부터(로)서(로)써(를)보(대)어(에)에(게)에(서)에(다)에(다)가(서)와(으)로(으)로부터(으)로(서)로(써)을(의)이(이)랑(하)고)(의)같이(까)지(까)지(나)는(대)로(도)따(라)마(대)마(저)만(만)컴(보)다(보)다(도)부(터)씩(야)야(마)로(은)이(내)조(차)조(차)도(쨌)쨌(럼). Do  $\hat{\chi}\hat{\chi}$ 적X →  $\hat{\chi}\hat{\chi}$  and  $\sim\hat{\chi}\hat{\chi}$ (의)가(감)객(경)계(과)관(권)금(기)력(료)방(법)별(복)부(비)사(상)생(서)석(성)세(소)수(식)실(아)어(용)원(인)자(장)지(직)초(당)관(편)품(화)형(화)회)KoreanNounSuff(의)커(녕) →  $\hat{\chi}\hat{\chi}$ .

(5)  $Do \sim \hat{x}(\emptyset|갑|개|계|껏|꾸러기|꾼|님|둥이|맹이|보어|치오|우음|이|쟁이|질|짜리|째|투성이|히) \mathbf{KoreanNounSuff}(\emptyset|다|는데|듯이|라는|데|라|셔|려|무|나|런|마는|렵|망|정|수|록|야|말|고|자|마|지|언|정|커|녕|테|니|테|니|까|텐|데) \rightarrow \hat{x}$ .

(6) Apply KorNum.

(7) Do the following in a sequel, searching for the longest match in each step:

(7.1) Remove one of these word-final patterns if it follows a character:

길래, 끼리, 네요, 다며, 다시피, 담, 되며, 라도, 라며, 라면서, 만, 만은, 며, 면서, 어요, 에서, 예선, 요, 이란, 이며, 이요, 인, 하며.

(7.2) Remove one of these word-final patterns if it follows a character:

내, 는, 대, 라면, 래, 를, 은, 을, 이군, 이라뇨, 이라니, 재

(7.3) Remove one of these word-final patterns if it follows a character:

가, 까, 끄, 늘, 니와, 더러, 도, 든, 라, 뿐, 아, 아라, 야, 어라, 예, 오, 자

and  $do \sim \hat{x}(\emptyset|년|단|란|잔)다 \rightarrow \hat{x}$ ,  $\sim \hat{x}(\emptyset|났|됐|팠|졌)(\emptyset|어) \rightarrow \hat{x}$  in the same sweep.

(7.4) Define **KoreanVerbSuff** as any one of the following patterns:

$\emptyset$ , 가, 같이, 거, 겠, 고, 고말고, 구나, 구만, 구면, 군요, 기, 기만, 기엔, 까지, 께, 는, 다, 다니, 더니, 데, 도록, 든지, 들, 따라, 려고, 로, 로부터, 로서, 로써, 를, 마다, 마저, 만큼, 면, 보다, 부터, 서, 서부터, 셔, 씩, 야, 어, 에, 에게, 에게서, 에겐, 에다, 에다가, 에서, 에서부터, 으로, 으로부터, 으로서, 으으로써, 은, 은데, 을, 음, 의, 이, 자마자, 저서, 조차, 중, 지만, 쯤, 처럼, 처럼, 하곤, 해선, ( $\emptyset$ 는|은)커녕, ( $\emptyset$ 이)나, (과|랑|와|이|랑|하|고)( $\emptyset$ 는|만|은), (내|냅|다|답|래|랍|자|잡)(고|니).

Do  $\hat{x}(\mathbf{KoreanVerbSuff})_m \rightarrow \hat{x}$ .

(7.5) Remove one of these word-final patterns if it follows a character:

게, 네, 는, 니, 더냐, 더라, 던, 데, 디, 세, 시, 어라, 자.

(7.6)  $Do \sim \hat{x}(\emptyset|으)(\emptyset|졌|시|신|실|심|십)(\emptyset|졌|왔|왔|졌|왔|였|였)(\emptyset|습|음) \rightarrow \hat{x}$ .

(7.7) Remove one of these word-final patterns if it follows a character:

겨, 겠, 구, 군, 굴, 굶, 굶, 귀, 꿔, 기, 긴, 길, 김, 깎, 려, 련, 렸, 리, 털, 림, 립, 받, 여, 였, 우, 운, 울, 움, 읊, 워, 윗, 이, 인, 일, 임, 입, 저, 졌, 지, 진, 질, 짐, 집, 추, 춘, 출, 춤, चु, चु, 혀, 혀, 히, 힌, 힐, 힘, 힙.

(7.8)  $Do \sim \hat{x}(\emptyset|대로|(\text{접|답|롭|맞|스|레|스|럽})(\emptyset|겨|우|겨|운|겨|울|겨|움|겨|움|겨|워|겨|웠|다|우|다|운|다|올|다|움|다|움|다|워|다|웠|로|우|로|운|로|울|로|움|로|움|로|워|로|웠|우|운|울|움|움|워|웠)) \rightarrow \hat{x}$ .

(8)  $Do \sim \hat{x}(\text{러|러서|서서}) \rightarrow \hat{x}$ ,  $\hat{x}(\text{빼|뺏|뺏|뺏|뺏|뺏|뺏}) \mathbf{X} \rightarrow \hat{x} \text{뺏}$ ,  $\hat{x}(\text{러|러|린|림}) \mathbf{X} \rightarrow \hat{x} \text{리}$ .

(9) Apply HgRom.

(10)  $Do nolQLX \sim \rightarrow nolQ$ ,  $Q(\emptyset|g|l|s) \mathbf{V}_m \mathbf{S} \mathbf{X} \rightarrow \emptyset$ ,  $QsiQk \mathbf{X} \rightarrow \emptyset$ ,  $\sim(\emptyset|b)Q(\emptyset|eub|seub)(\emptyset|Q)(\emptyset|de|deo|di|ge|go|ja|n|ne|neu|ni|sel|si)(\emptyset|l|m|n) \rightarrow \emptyset$ .

(11) Apply RomHg and do  $\sim \hat{x}(\emptyset|냐|시|으|시) \rightarrow \hat{x}$ .<sup>117</sup>

(12)  $Do \hat{x}(\text{ㄴ|으}) \mathbf{X} \rightarrow \hat{x}$ .

**Algorithm 9.13** (Korean essential root). Let  $\hat{\sigma}$  be the effective spelling of a Korean word, then its corresponding essential root  $\text{EssRoot}(\hat{\sigma})$  is constructed in the following steps:

(1)  $Do \sim \hat{x}(\text{리|아|아|서|어|어|서|음|이}) \rightarrow \hat{x}$ .

(2) Apply HgRom and do  $\sim(b|h|m|s|S) \rightarrow \emptyset$ ,  $\sim(d|Q|eu(\emptyset|b|h|m|n|Q|eo|s|S)) \rightarrow l$ .

(3) Apply RomHg and do  $\sim \text{와} \rightarrow \emptyset$ .

<sup>117</sup>To save execution time, one could have manipulated only the romanized strings, without converting back and forth between *Hangul* and its transliteration. However, we choose to state our algorithm using multiple applications of HgRom and RomHg, to enhance the readability of our substitution rules.

### 9.2.3 Approximate clustering

There will not be any mutation rules in our algorithm for Korean, so  $\text{SimpHrdTest} = \text{HrdTest}$ .

**Algorithm 9.14** (Simple heredity test). *Suppose that  $\hat{\alpha}$  and  $\hat{\beta}$  are both Hangul strings. The Boolean-valued function  $\text{SimpHrdTest}(\hat{\alpha}, \hat{\beta})$  returns **TRUE** if at least one of the following five conditions holds:<sup>118</sup>*

- (i)  $\hat{\alpha} = \hat{\beta}$ ;
- (ii)  $\hat{\beta} = \hat{\alpha}\text{네}$ ;
- (iii)  $\text{HgRom}(\hat{\alpha})l = \text{HgRom}(\hat{\beta})$ ;
- (iv)  $\min\{\ell(\hat{\alpha}), \ell(\hat{\beta})\} \geq 2$ , **AND**  $\text{HgRom}(\hat{\alpha}') = \text{HgRom}(\hat{\beta}')$ , where the prime denotes an operation  $\sim \mathbf{V}_m(\emptyset|n) \rightarrow \emptyset$ ;
- (v)  $\min\{\ell(\hat{\alpha}), \ell(\hat{\beta})\} \geq 2$ , **AND**  $\text{HgRom}(\hat{\alpha})^* = \text{HgRom}(\hat{\beta})^*$ , where the asterisk denotes an operation  $Q(\text{jeog|man|Pun|seong})\mathbf{X} \rightarrow \emptyset$ .

**Algorithm 9.15** (Approximate clustering of Korean words). *The approximate clustering of a list of Korean words  $\{\hat{\alpha}_1, \dots, \hat{\alpha}_N\}$  is completed in two stages:*

- (1) *We sort the list  $\{(\hat{\alpha}_1, \text{HgRom}(\text{EffSpell}(\hat{\alpha}_1))), \dots, (\hat{\alpha}_N, \text{HgRom}(\text{EffSpell}(\hat{\alpha}_N)))\}$  alphabetically according to the last component. If two consecutive neighbors in the alphabetized list  $\{(\hat{\alpha}_{(1)}, \text{HgRom}(\text{EffSpell}(\hat{\alpha}_{(1)}))), \dots, (\hat{\alpha}_{(N)}, \text{HgRom}(\text{EffSpell}(\hat{\alpha}_{(N)})))\}$  satisfy  $\text{HrdTest}(\text{EffSpell}(\hat{\alpha}_{(n)}), \text{EffSpell}(\hat{\alpha}_{(n+1)})) = \text{FALSE}$ , where  $n \in \mathbb{Z} \cap [1, N)$ , then add a demarcation line between these two entries. In this way, the alphabetized list is divided into separate groups of words tagged with their effective spellings:  $\{g_1 = \{(\hat{\alpha}_{(1,1)}, \text{EffSpell}(\hat{\alpha}_{(1,1)})), \dots, (\hat{\alpha}_{(1,n_1)}, *)\}, \dots, g_M = \{(\hat{\alpha}_{(M,1)}, *), \dots, (\hat{\alpha}_{(M,n_M)}, *)\}$ , where each sublist also preserves alphabetic order. In particular, we have  $\hat{\alpha}_{(1,1)} = \hat{\alpha}_{(1)}$  and  $\hat{\alpha}_{(M,n_M)} = \hat{\alpha}_{(N)}$ .*
- (2) *For each group of words  $g_m = \{(\hat{\alpha}_{(m,1)}, *), \dots, (\hat{\alpha}_{(m,n_m)}, *)\}$  where  $m \in \mathbb{Z} \cap [1, M]$ , we augment it into a tagged entry  $G_m = (g_m, \text{HgRom}(\text{EffSpell}(\hat{\alpha}_{(m,1)})), \text{HgRom}(\text{EssRoot}(\text{EffSpell}(\hat{\alpha}_{(m,1)}))))$ . The list  $\{G_1, \dots, G_M\}$  is sorted alphabetically, with respect to  $\text{HgRom}(\text{EssRoot}(\text{EffSpell}(\hat{\alpha}_{(m,1)})))$  (with higher priority), and  $\text{HgRom}(\text{EffSpell}(\hat{\alpha}_{(m,1)}))$  (with lower priority). If two consecutive neighbors in the alphabetized list  $\{G_{(1)} = (g_{(1)}, \hat{\gamma}'_{(1)}, \hat{\gamma}''_{(1)}), \dots, G_{(M)} = (g_{(M)}, \hat{\gamma}'_{(M)}, \hat{\gamma}''_{(M)})\}$  satisfy*

$$\text{HrdTest}(\hat{\gamma}''_{(m)}, \hat{\gamma}''_{(m+1)}) = \text{FALSE}$$

**AND**

$$\text{HrdTest}(\hat{\gamma}'_{(m)}, \hat{\gamma}'_{(m+1)}) = \text{FALSE}$$

where  $m \in \mathbb{Z} \cap [1, M)$ , then add a demarcation line between these two entries. In this manner, the alphabetized list  $\{G_{(1)}, \dots, G_{(M)}\}$  is divided into separate groups of tagged clusters  $\{\Gamma_1 = \{G_{(1,1)}, \dots, G_{(1,m_1)}\}, \dots, \Gamma_K = \{G_{(K,1)}, \dots, G_{(1,m_K)}\}\}$ . Finally, the output list of word clusters  $\{\tilde{\Gamma}_1, \dots, \tilde{\Gamma}_K\}$  is constructed by discarding all the tags (effective spellings, essential roots) from each  $\Gamma_k$ , where  $k \in \mathbb{Z} \cap [1, K]$ .

*Example 9.15.1.* Our clustering algorithm correctly groups the following families of Korean words:

걸겠다, 걸겠습니다, 걸겠어, 걸겠어요, 걸고, 걸기, 걸느냐, 걸는, 걸는다, 걸는데, 걸더니, 걸습니까, 걸습니다, 걸자, 걸지만, 걸어, 걸어라, 걸어서, 걸어야, 걸어요, 걸었기, 걸었느냐, 걸었다, 걸었습니다, 걸었어, 걸었어요, 걸었음, 걸으니, 걸으니까, 걸으려고, 걸으면, 걸으세요, 걸으셔, 걸으셔서, 걸으셔야, 걸으셔요, 걸으셨기, 걸으셨느냐, 걸으셨다, 걸으셨습니까, 걸으셨습니다, 걸으셨어, 걸으셨어요, 걸으셨음, 걸으시겠다, 걸으시겠습니다, 걸으시겠어, 걸으시겠어요, 걸으시고, 걸으시기, 걸으시느냐, 걸으시는, 걸으시는데, 걸으시니, 걸으시니까, 걸으시더니, 걸으시라, 걸으시려고, 걸으시면, 걸으시지만, 걸으신, 걸으신다, 걸으실, 걸으심, 걸으십니까, 걸으십니다, 걸으십시오, 걸은, 걸을, 걸음, 걸읍시다, 걸읍시오 — “walk”;

넓겠다, 넓겠습니다, 넓겠어, 넓겠어요, 넓고, 넓기, 넓다, 넓더니, 넓습니까, 넓습니다, 넓어, 넓어서, 넓어야, 넓어요, 넓었기, 넓었느냐, 넓었다, 넓었습니다, 넓었어, 넓었어요, 넓었음, 넓으냐, 넓으니, 넓으니까, 넓으면, 넓으세요, 넓으셔, 넓으셔서, 넓으셔야, 넓으셔요, 넓으셨기, 넓으셨느냐, 넓으셨다, 넓으셨습니까, 넓으셨습니다, 넓으셨어, 넓으셨어요, 넓으셨음, 넓으시겠다, 넓으시겠습니다, 넓으시겠어, 넓으시겠어요, 넓으시고, 넓으시기, 넓으시느냐, 넓으시니, 넓으시니까, 넓으시다, 넓으시더니, 넓으시면, 넓으시지만, 넓으신, 넓으신데, 넓으실, 넓으심, 넓으십니까, 넓으십니다, 넓은, 넓은데, 넓을, 넓음, 넓지만 — “wide”;

<sup>118</sup>As a general rule in this document, the truth values of items labeled with Roman numerals are connected to each other with logical **OR**.

오겠다, 오겠습니다, 오겠어, 오겠어요, 오고, 오기, 오너라, 오느냐, 오는, 오는데, 오니, 오니까, 오더니, 오려고, 오면, 오세요, 오셔, 오셔서, 오셔야, 오셔요, 오셨기, 오셨느냐, 오셨다, 오셨습니까, 오셨습니다, 오셨어, 오셨어요, 오셨음, 오시겠다, 오시겠습니다, 오시겠어, 오시겠어요, 오시고, 오시기, 오시느냐, 오시는, 오시는데, 오시니, 오시니까, 오시더니, 오시라, 오시려고, 오시면, 오시지만, 오신, 오신다, 오실, 오십, 오십니까, 오십니다, 오십시오, 오자, 오지만, 온, 온다, 울, 읊, 읊니까, 읊니다, 읊시다, 읊시오, 와, 와라, 와서, 와야, 와요, 왔기, 왔느냐, 왔다, 왔습니까, 왔습니다, 왔어, 왔어요, 왔음 — “come”;

높겠다, 높겠습니다, 높겠어, 높겠어요, 높고, 높기, 높다, 높더니, 높습니까, 높습니다, 높아, 높아서, 높아야, 높아요, 높았기, 높았냐, 높았다, 높았습니까, 높았습니까, 높았어, 높았어요, 높았음, 높으냐, 높으니, 높으니까, 높으면, 높으세요, 높으셔, 높으셔서, 높으셔야, 높으셔요, 높으셨기, 높으셨냐, 높으셨다, 높으셨습니까, 높으셨습니까, 높으셨어, 높으셨어요, 높으셨음, 높으시겠다, 높으시겠습니다, 높으시겠어, 높으시겠어요, 높으시고, 높으시기, 높으시냐, 높으시니, 높으시니까, 높으시다, 높으시더니, 높으시면, 높으시지만, 높으신, 높으신데, 높으실, 높으십, 높으십니까, 높으십니다, 높은, 높은데, 높을, 높음, 높지만 — “tall”;

가거라, 가겠다, 가겠습니다, 가겠어, 가겠어요, 가고, 가기, 가느냐, 가는, 가는데, 가니, 가니까, 가더니, 가라, 가려고, 가면, 가서, 가세요, 가셔, 가셔서, 가셔야, 가셔요, 가셨기, 가셨느냐, 가셨다, 가셨습니까, 가셨습니까, 가셨어, 가셨어요, 가셨음, 가시겠다, 가시겠습니다, 가시겠어, 가시겠어요, 가시고, 가시기, 가시느냐, 가시는, 가시는데, 가시니, 가시니까, 가시더니, 가시라, 가시려고, 가시면, 가시지만, 가신, 가신다, 가실, 가십, 가십니까, 가십니다, 가십시오, 가야, 가요, 가자, 가지만, 간다, 갑니까, 갑니다, 갑시다, 갑시오, 갔기, 갔느냐, 갔다, 갔습니까, 갔습니까, 갔어, 갔어요, 갔음 — “go”;

빗겠다, 빗겠습니다, 빗겠어, 빗겠어요, 빗고, 빗기, 빗느냐, 빗는, 빗는다, 빗는데, 빗더니, 빗습니까, 빗습니까, 빗어, 빗어라, 빗어서, 빗어야, 빗어요, 빗었기, 빗었느냐, 빗었다, 빗었습니까, 빗었습니까, 빗었어, 빗었어요, 빗었음, 빗으니, 빗으니까, 빗으려고, 빗으면, 빗으세요, 빗으셔, 빗으셔서, 빗으셔야, 빗으셔요, 빗으셨기, 빗으셨느냐, 빗으셨다, 빗으셨습니까, 빗으셨습니까, 빗으셨어, 빗으셨어요, 빗으셨음, 빗으시겠다, 빗으시겠습니다, 빗으시겠어, 빗으시겠어요, 빗으시고, 빗으시기, 빗으시느냐, 빗으시는, 빗으시는데, 빗으시니, 빗으시니까, 빗으시더니, 빗으시라, 빗으시려고, 빗으시면, 빗으시지만, 빗으신, 빗으신다, 빗으실, 빗으십, 빗으십니까, 빗으십니다, 빗으십시오, 빗은, 빗을, 빗음, 빗읍시다, 빗읍시오, 빗자, 빗지만 — “comb”;

나아, 나아라, 나아서, 나아야, 나아요, 나왔기, 나왔느냐, 나왔다, 나왔습니까, 나왔습니까, 나왔어, 나왔어요, 나왔음, 나오니, 나오니까, 나오려고, 나오면, 나오세요, 나오셔, 나오셔서, 나오셔야, 나오셔요, 나오셨기, 나오셨느냐, 나오셨다, 나오셨습니까, 나오셨습니까, 나오셨어, 나오셨어요, 나오셨음, 나오시겠다, 나오시겠습니다, 나오시겠어, 나오시겠어요, 나오시고, 나오시기, 나오시느냐, 나오시는, 나오시는데, 나오시니, 나오시니까, 나오시더니, 나오시라, 나오시려고, 나오시면, 나오시지만, 나오신, 나오신다, 나오실, 나오십, 나오십니까, 나오십니다, 나오십시오, 나은, 나올, 나움, 나읍시다, 나읍시오, 낫겠다, 낫겠습니다, 낫겠어, 낫겠어요, 낫고, 낫기, 낫느냐, 낫는, 낫는다, 낫는데, 낫더니, 낫습니까, 낫습니까, 낫자, 낫지만 — “recover”;

흐르겠다, 흐르겠습니다, 흐르겠어, 흐르겠어요, 흐르고, 흐르기, 흐르느냐, 흐르는, 흐르는데, 흐르니, 흐르니까, 흐르더니, 흐르려고, 흐르면, 흐르세요, 흐르셔, 흐르셔서, 흐르셔야, 흐르셔요, 흐르셨기, 흐르셨느냐, 흐르셨다, 흐르셨습니까, 흐르셨습니까, 흐르셨어, 흐르셨어요, 흐르셨음, 흐르시겠다, 흐르시겠습니다, 흐르시겠어, 흐르시겠어요, 흐르시고, 흐르시기, 흐르시느냐, 흐르시는, 흐르시는데, 흐르시니, 흐르시니까, 흐르시더니, 흐르시라, 흐르시려고, 흐르시면, 흐르시지만, 흐르신, 흐르신다, 흐르실, 흐르십, 흐르십니까, 흐르십니다, 흐르십시오, 흐르자, 흐르지만, 흐른, 흐른다, 흐를, 흐름, 흐릅니까, 흐릅니다, 흐릅시다, 흐릅시오, 흘러, 흘러라, 흘러서, 흘러야, 흘러요, 흘렀기, 흘렀느냐, 흘렀다, 흘렀습니까, 흘렀습니까, 흘렀어, 흘렀어요, 흘렀음 — “flow”.

Moreover, the words 널리 “widely” and 너비 “width” also cluster correctly with the inflected forms of “wide”.

*Example 9.15.2.* In Fig. S15, we further apply the aforementioned word clustering algorithm to topic extraction and machine translation (see Table S1 for text source).

Following the standard practice in Korean dictionaries, we have inserted etymological information for loanwords from Chinese<sup>119</sup> and English, in the parentheses. This was done by using a manually built look-up table. The etyma in Chinese

<sup>119</sup>Due to partial confluences of native Korean and Sino-Korean vocabulary (as discussed earlier), a *Hanja* form may not apply to all the words in a certain cluster. Furthermore, since we have merged 숙모(叔母) “paternal aunt” and 이모(姨母) “maternal aunt” into the same cluster, but have not built a stacking mechanism for Chinese characters (for legibility reasons), the *Hanja* forms of such word stems are not displayed.

or English were not directly inferrable from the Korean text under investigation, nor were they an integral part of our word clustering algorithm: we track the etymologies of the word stems so that we can assess the reliability of our experimental methods.

The Korean case shown here offers a telling example that meanings of words are determined by their numerical fingerprints, rather than their etymological sources. Korean words of native, Chinese and English origins all behave in a consistent way in the displayed results.

We caution our readers, however, that the performance of our numerical algorithm is indeed affected by mixed etymological sources of a given concept in Korean. From the control experiments in Fig. S15c, we see that certain correct matching pairs have similarity scores below the 0.7 threshold applicable to Fig. S15b. Part of this can be explained by the coexistence of native Korean and Sino-Korean stems, the latter usually reserved for abstract, formal and polite settings. See the (partial) list below:

| English gloss | native Korean stem | Sino-Korean stem                             |
|---------------|--------------------|----------------------------------------------|
| “amiable”     | 상냥 sangnyang       | 친절(親切) chinjeol                              |
| “feel”        | 느끼 neukki          | 감정(感情) gamjeong, 기분(氣分) gibun                |
| “forget”      | 잊 ij               | 망각(忘却) manggag                               |
| “love”        | 사랑 salang          | 애정(愛情) aejeong                               |
| “pride”       | 자랑 jalang          | 오만(傲慢) oman, 자부심(自負心) jabusim, 거만(倨慢) geoman |
| “read”        | 읽 ilg              | 독서(讀書) dogseo                                |
| “walk”        | 걸 geod             | 산책(散策) sanchaeg                              |
| “wish”        | 싶 sip              | 원(願) won                                     |

Had we forcibly merged these native Korean stems with their Sino-Korean counterparts, before performing the numerical experiments in Fig. S15b, we would have achieved a slightly better yield for correct matchings with similarity scores above 0.7.



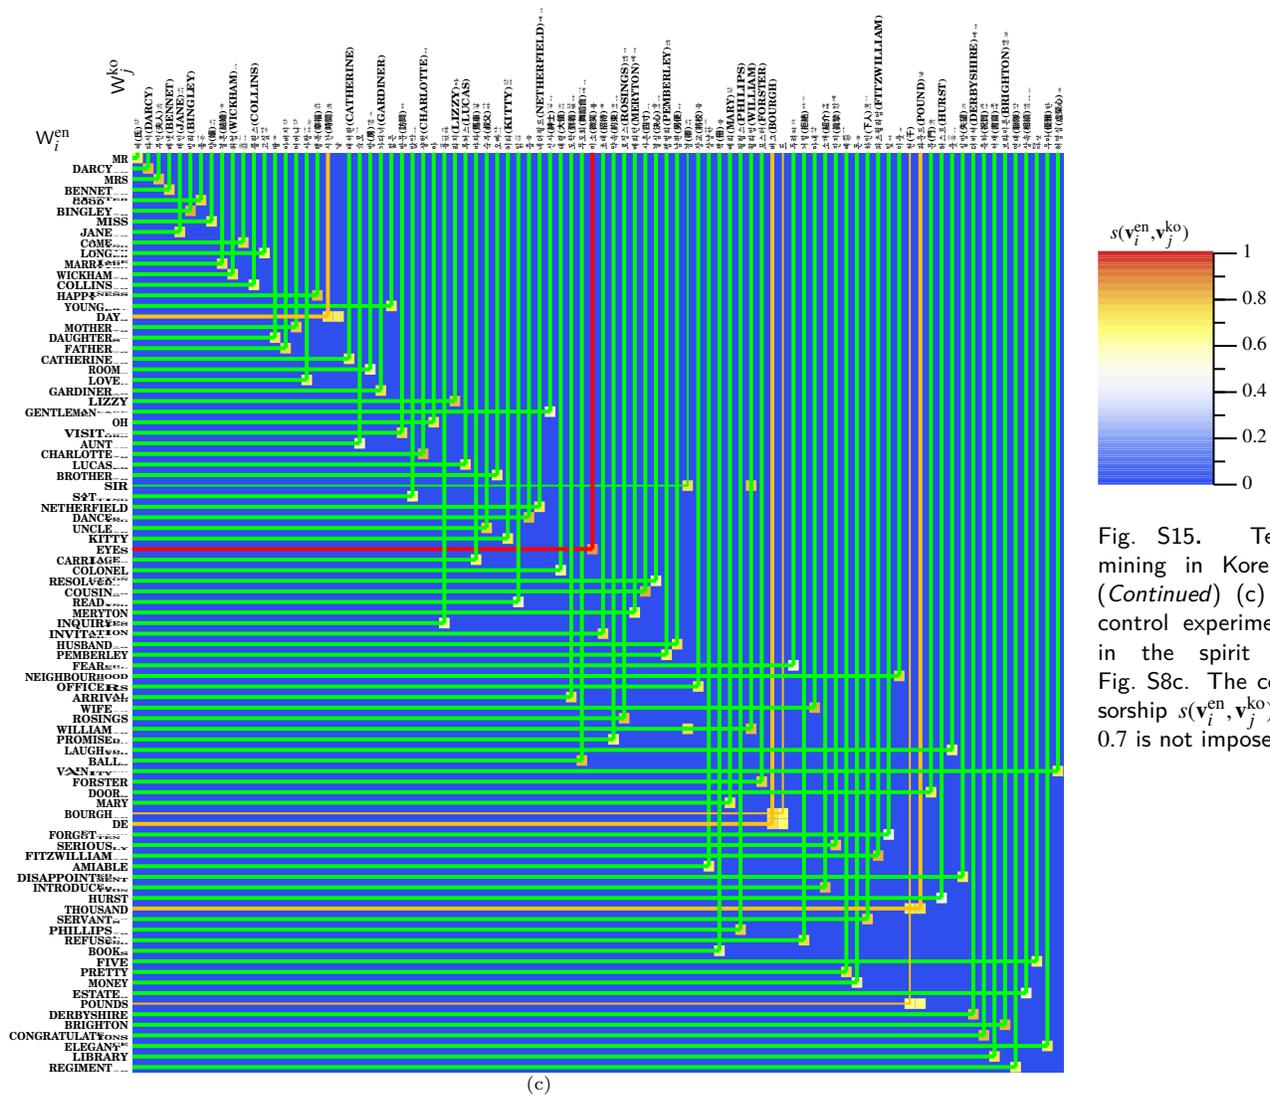

(c)

Fig. S15. Text mining in Korean. (Continued) (c) A control experiment in the spirit of Fig. S8c. The censorship  $s(v_i^{\text{en}}, v_j^{\text{ko}}) \geq 0.7$  is not imposed.

### 9.3 Modified Porter stemming algorithm for Turkish

Our Turkish stemming algorithm is adapted from the method of Gülşen Eryiğit and Eşref Adalı [51], which was previously implemented by Evren (Kapusuz) Çilden (<http://snowball.tartarus.org/algorithms/turkish/stemmer.html>).

Our algorithm works on Modern Turkish (after the Atatürk Reform of 1928), which uses (a modified version of) the Latin alphabet, and phases out most grammatical forms of Arabic and Persian origins. Since Atatürk’s Language Reform, a significant amount of Arabic and Persian loanwords have become obsolete, even if they are apparently more concise (using fewer syllables) than their counterparts in Modern Turkish, such as

| English gloss | via Proto-Turkic | via Arabic  | via Persian |
|---------------|------------------|-------------|-------------|
| “friend”      | <i>arkadaş</i>   | _____       | <i>dost</i> |
| “war”         | <i>savaş</i>     | <i>harp</i> | <i>cenk</i> |

While the native Turkish forms *arkadaş* and *savaş* contain more syllables than their Arabic/Persian equivalents, they are free from awkward consonant clusters.<sup>120</sup> Some Arabic/Persian loanwords still survive in Modern Turkish, as they are phonologically compatible with native Turkish words, such as *saat* “hour” (from Arabic) and *zaman* “time, epoch” (from either Arabic or Persian). It is also possible that a native Turkish word coexists with an Arabic/Persian loan for the same concept, with slightly different connotations, such as *ak* “white” (native Turkish) vs. *beyaz* “white” (via Arabic); *kara* “black” (native Turkish) vs. *siyah* “black” (via Persian). The last situation is similar to the coexistence of native Korean and Sino-Korean vocabularies in Modern Korean (see §9.2).

While we design our stemming algorithm for Modern Turkish, we take into account its phonological restrictions on syllable structure. Like what we did for Korean, we are not going to merge native and non-native etyma into the same word cluster.

Turkish stop words can carry various agglutinative suffixes. Instead of enumerating all of them in a single list, we will define several string patterns that match the criterion for stop words.

**Definition 9.16** (Turkish stop words). Define the pattern **TurkishStopRoot** as any one from the following list:

*aksi, altında, ama, anca, ancak, andan, aralarında, arasında, artık, aşağı, aşağıda, aynı, ayrı, ayrıca, ayriyeten, ayriyeten, az, bana, başına, başka, bazen, bazı, bazıları, bazılarıda, bazılarına, bazılarından, bazılarımla, bazıların, belgeyle, belki, ben, bende, benden, beni, benim, beri, bile, bir, biraz, biri, birileri, birisi, birkaç, birlikte, biz, bizde, bizden, bize, bizi, bizim, bizler, böylece, böyle, böylece, bu, buna, bunda, bundan, bunlar, bunlara, bunlarda, bunlardan, bunları, bunların, bunu, bunun, bununla, bura, burada, buradaki, buradan, buralar, buralara, buralarda, buralardan, buraları, buraların, buranın, buraya, burayı, bütün, civarda, çoğu, çoğunlukla, çok, çünkü, da, daha, dahası, dair, de, dek, dendenle, dışarı, dışında, diğer, diğerleri, diye, dolayı, dolayısıyla, durumda, e, eden, eder, ederim, ederiz, ederler, edersin, edersiniz, edildi, ediyor, ediyordu, ediyorduk, ediyordum, ediyordun, ediyordunuz, ediyorlar, ediyorlardı, ediyorsun, ediyorsunuz, ediyorum, ediyoruz, eğer, en, etmedi, etmedik, etmediler, etmedim, etmedin, etmediniz, etmem, etmeyiz, etmez, etmezler, etmezsin, etmezsiniz, etmiyor, etmiyordu, etmiyorduk, etmiyordum, etmiyordun, etmiyordunuz, etmiyorlar, etmiyorlardı, etmiyorsun, etmiyordsunuz, etmiyorum, etmiyoruz, etrafında, esen, etti, ettik, ettiler, ettim, ettin, ettiniz, ettirdi, ettirdik, ettirdiler, ettirdim, ettirdin, ettirdiniz, ettireceğim, ettireceğiz, ettirecek, ettirecekler, ettireceksin, ettireceksiniz, ettirir, ettiririm, ettiririz, ettirirler, ettirirsin, ettirirsiniz, ettiriyor, ettiriyordu, ettiriyorduk, ettiriyordum, ettiriyordun, ettiriyordunuz, ettiriyorlar, ettiriyorlardı, ettiriyorsun, ettiriyorsunuz, ettiriyorum, ettiriyoruz, ettirmedik, ettirmediler, ettirmedim, ettirmedin, ettirmediniz, ettirmem, ettirmeyeceğim, ettirmeyeceğiz, ettirmeyecek, ettirmeyecekler, ettirmeyeceksin, ettirmeyeceksiniz, ettirmeyiz, ettirmez, ettirmezler, ettirmezsin, ettirmezsiniz, ettirmiyor, ettirmiyordu, ettirmiyorduk, ettirmiyordum, ettirmiyordun, ettirmiyordunuz, ettirmiyorlar, ettirmiyorsun, ettirmiyorsunuz, ettirmiyorum, ettirmiyoruz, evet, evvel, fakat, gayet, gelen, gelişme, gereçler, gerek, gerektiği, geride, gibi, göre, günü, hadi, hakkında, hala, hâlâ, halbuki, halde, haline, hangi, hangileri, hangilerine, hangilerini, hangilerinin, hangisi, hangisinde, hangisinden, hangisine, hangisini, hangisinin, hangisilerinde, hangisilerinden, hani, hariç, hatta, hayır, hem, hemen, henüz, hepsi, hepsinde, hepsinden, hepsine, hepsini, hepsinin, her, herhangi, herkes, herkesin, hiç, hiçbir, icar, içeride, için, içinde, içinden, içine, ile, ilgili, irade, ise, ister, işte, iyi, izin, kadar, kâh, kapalı, karşı, karşımla, karşısında, kazanılmış, kenara, keşke, kez, ki, kim, kimde, kimden, kime, kimi, kimin, kimisi, kimler, kimlerde, kimlerden, kimlere, kimleri, kimlerin, kimse, kişinin, kişiye, konum, lâkin, madem, mademki, meğer, meğerki, meğerse, meselâ, mi, mısın, mısınız, mıydı, mıyım, mıyız, mi, misin, misiniz, miyim, miyiz, mu, musun, musunuz, mıydu, mıyduk, mıydum, mıydun, mıydunuz, muyum, muyuz, mü, nasıl, ne, nede, neden, nedenle, neler, nelerde, nelerden, nelere, neleri, nelerin, nere, nereden, nereden, neredeyse, nereler, nerelerde, nerelerden, nerelere, nereleri, nerelerin, nereye, nereyi, nereyin, neye, neyi, neyin, neyse, niçin, o, ol, olacağım, olacağız, olacak, olacaklar, olacaksın, olacaksınız, olan, olanları, olarak, oldu, olduğu, olduk, oldukça, oldular, oldum, oldun, oldunuz, olma, olmadan, olmadı, olmadık, olmadıkça, olmadılar,*

<sup>120</sup>A typical syllable in a native Turkish word takes the form (C<sub>1</sub>)V(C<sub>2</sub>), containing a single vowel flanked by (optionally present) single consonants at both ends.



(5) *Do* (*amca|dayı*)**X**~ → ω̄νκλε, (*bibi|eme|hala|teyze*)**X**~ → αῡντ.<sup>123</sup>

(6) *Replace*

|                                                 |                             |                                                                          |                             |                                                                          |                          |                                                                                                         |                          |                |                |              |              |
|-------------------------------------------------|-----------------------------|--------------------------------------------------------------------------|-----------------------------|--------------------------------------------------------------------------|--------------------------|---------------------------------------------------------------------------------------------------------|--------------------------|----------------|----------------|--------------|--------------|
| <i>anla</i> <b>X</b> ~                          | <i>der</i> (∅  <i>iz</i> )~ | <i>di</i> (∅  <i>me</i> ) <i>y</i> ( <i>ece</i>   <i>or</i> ) <b>X</b> ~ | <i>düşün</i> <b>X</b> ~     | <i>eleştir</i> <b>X</b> ~                                                | <i>getir</i> <b>X</b> ~  | <i>gid</i> ( <i>e</i>   <i>i</i> )~                                                                     | <i>götür</i> <b>X</b> ~  | <i>gül</i> ~   |                |              |              |
| κομπρ                                           | de                          | de                                                                       | θi̇νκ                       | κpi̇τρ                                                                   | βpi̇γ                    | gitmek                                                                                                  | καρρ                     | γi̇λ           |                |              |              |
| <i>hanım</i> ~                                  | <i>hatır</i> <b>X</b> ~     | <i>his</i> ~                                                             | <i>ileri</i> <b>X</b> ~     | <i>itiraf</i> <b>X</b> ~                                                 | <i>itiraz</i> <b>X</b> ~ | <i>iz</i> <b>X</b> ~                                                                                    | <i>kismet</i> <b>X</b> ~ | <i>kızır</i> ~ | <i>naşam</i> ~ | <i>oda</i> ~ | <i>söz</i> ~ |
| λαδ                                             | mi̇vδ                       | hisset                                                                   | φpov̇τ                      | kov̇φσ                                                                   | ωβjekt                   | φολω                                                                                                    | φατε                     | kizar          | adaμ           | ρi̇μα        | söz          |
| <i>su</i> ( <i>lar</i>   <i>yu</i> ) <b>X</b> ~ | <i>ulaş</i> <b>X</b> ~      | <i>yemin</i> <b>X</b> ~                                                  | <i>yer</i> (∅  <i>iz</i> )~ | <i>yi</i> (∅  <i>me</i> ) <i>y</i> ( <i>ece</i>   <i>or</i> ) <b>X</b> ~ | <i>anda</i>              | <i>su</i> (∅  <i>da</i>   <i>dan</i>   <i>dur</i>   <i>sun</i>   <i>sunuz</i>   <i>uz</i>   <i>ya</i> ) |                          |                |                |              |              |
| hho                                             | peach                       | vow                                                                      | ye                          | ye                                                                       | now                      | hho                                                                                                     |                          |                |                |              |              |

(7) *Call the result so far as*  $\hat{\sigma}^\dagger$ , *and break it down into*  $\hat{\sigma}^\dagger = \hat{\sigma}_1^\dagger \hat{\sigma}_2^\dagger$ , *where*  $\ell(\hat{\sigma}_1^\dagger) = \text{ProtRg}(\hat{\sigma}^\dagger)$ . *Work on*  $\hat{\sigma}_2^\dagger$  *as follows:*

(7.1) *Replace*

|                                                           |                            |                                |                                   |                     |
|-----------------------------------------------------------|----------------------------|--------------------------------|-----------------------------------|---------------------|
| <b>#X</b>                                                 | <b>(abi ebil mak mek)X</b> | <b>(aca ece)(ğ k)X</b>         | <b>c(a e)s(i i)n(a e)X</b>        | <b>l(a e)(r ş)X</b> |
| ∅                                                         | ∅                          | ∅                              | ∅                                 | ∅                   |
| <b>m(i i u ü)şX</b>                                       | <b>r</b> ~                 | <b>yorX</b>                    | <b>~(∅ n)(d t)(a e)(∅ n)</b>      |                     |
| ∅                                                         | ρ                          | ∅                              | Ta                                |                     |
| <b>~(d t)(i i u ü)(∅ k l(a e)r m n(∅ l(i i u ü)z) r)X</b> |                            | <b>~ki(∅ n)(de den e i in)</b> | <b>~s(i i u ü)n(∅ (i i u ü)z)</b> |                     |
| Tu                                                        |                            | ∅                              | ∅                                 |                     |

(7.2) *Do*  $(d|t)(i|i|u|ü)(ğ|k)X \rightarrow \emptyset$ ,  $\mathbf{V}ym(i|i|u|ü)şX \rightarrow \mathbf{V}$ ,  $m(a|e|i|i|u|ü)X \rightarrow \emptyset$ ,  $~(i|i|u|ü)(m|n)(∅|(i|i|u|ü)z) \rightarrow \emptyset$ ,  $~\mathbf{V}y(∅|l)(a|e) \rightarrow \mathbf{V}$ ,  $~\mathbf{V}y(∅|Tu) \rightarrow \mathbf{V}$ ,  $~\mathbf{V}y(i|i|u|ü)(∅|m|z) \rightarrow \mathbf{V}$ ,  $~\mathbf{V}yken \rightarrow \mathbf{V}$ ,  $~\mathbf{V}ys(a|e) \rightarrow \mathbf{V}$ .

(7.3) *Do*  $~(∅|i|i|u|ü)(m|n) \rightarrow \emptyset$ .

(7.4) *Call the result so far as*  $\hat{\sigma}_2^\ddagger$ . *Concatenate*  $\hat{\sigma}_1^\dagger$  *and*  $\hat{\sigma}_2^\ddagger$ .

(8) *Do*  $TX \rightarrow \emptyset$ ,  $~r(∅|(i|i|u|ü)z) \rightarrow \emptyset$ .

**Algorithm 9.19** (Turkish essential root). *Let*  $\hat{\sigma}$  *be the effective spelling of a Turkish word, then its corresponding essential root*  $\text{EssRoot}(\hat{\sigma})$  *is constructed in the following steps:*

(1) *Search for the pattern*  $\mathbf{C}_{m_0} \mathbf{V} \mathbf{C}_{m_0} \mathbf{V}_{m_0} (\emptyset | \overline{(n|s)})$ . *If this search is successful, define*  $\hat{\sigma}^b$  *as the result from doing*  $~(i|i|u|ü) \rightarrow \emptyset$  *on such a pattern; otherwise, define*  $\hat{\sigma}^b$  *as*  $\hat{\sigma}$ .

(2) *On*  $\hat{\sigma}^b$ , *do*  $~b \rightarrow p$ ,  $~c \rightarrow \zeta$ ,  $~d \rightarrow t$ ,  $~ğ \rightarrow k$ .

### 9.3.2 Approximate clustering

There will not be any mutation rules in our algorithm for Turkish, so  $\text{SimpHrdTest} = \text{HrdTest}$ .

**Algorithm 9.20** (Simple heredity test). *Suppose that*  $\hat{\alpha}$  *and*  $\hat{\beta}$  *are both lowercase strings. The Boolean-valued function*  $\text{SimpHrdTest}(\hat{\alpha}, \hat{\beta})$  *returns* **TRUE** *if*  $\hat{\alpha}$  *contains at least one instance of*  $\mathbf{V}$ , **AND** *at least one of the following two conditions holds:*<sup>124</sup>

(i)  $\hat{\alpha} = \hat{\beta}$ ;

(ii)  $\hat{\alpha}' = \hat{\beta}'$ , *where the strings with prime result from doing*  $~\mathbf{X}^\epsilon (\mathbf{V} \hat{\chi}) (\emptyset | l) \mathbf{V} \rightarrow \mathbf{X}$  *on their counterparts without prime.*

**Algorithm 9.21** (Approximate clustering of Turkish words). *The approximate clustering of a list of Turkish words*  $\{\hat{\alpha}_1, \dots, \hat{\alpha}_N\}$  *is completed in two stages:*

(1) *We sort the list*  $\{(\hat{\alpha}_1, \text{EffSpell}(\hat{\alpha}_1)), \dots, (\hat{\alpha}_N, \text{EffSpell}(\hat{\alpha}_N))\}$  *alphabetically according to the last component. If two consecutive neighbors in the alphabetized list*  $\{(\hat{\alpha}_{(1)}, \text{EffSpell}(\hat{\alpha}_{(1)})), \dots, (\hat{\alpha}_{(N)}, \text{EffSpell}(\hat{\alpha}_{(N)}))\}$  *satisfy*  $\text{HrdTest}(\text{EffSpell}(\hat{\alpha}_{(n)}), \text{EffSpell}(\hat{\alpha}_{(n+1)})) = \mathbf{FALSE}$ , *where*  $n \in \mathbb{Z} \cap [1, N)$ , *then add a demarcation line between these two entries. In this way, the alphabetized list is divided into separate groups of words tagged with their effective spellings:*  $\{g_1 = \{(\hat{\alpha}_{(1,1)}, \text{EffSpell}(\hat{\alpha}_{(1,1)})), \dots, (\hat{\alpha}_{(1,n_1)}, *)\}, \dots, g_M = \{(\hat{\alpha}_{(M,1)}, *), \dots, (\hat{\alpha}_{(M,n_M)}, *)\}$ , *where each sublist also preserves alphabetic order. In particular, we have*  $\hat{\alpha}_{(1,1)} = \hat{\alpha}_{(1)}$  *and*  $\hat{\alpha}_{(M,n_M)} = \hat{\alpha}_{(N)}$ .

<sup>123</sup>In this step, we group certain kinship terms in Turkish so as to match their English counterparts. However, since the Turkish word *kardeş* means both “brother” and “sister”, we cannot do anything to compensate for this.

<sup>124</sup>As a general rule in this document, the truth values of items labeled with Roman numerals are connected to each other with logical **OR**.

- (2) For each group of words  $g_m = \{(\hat{\alpha}_{(m,1)}, *), \dots, (\hat{\alpha}_{(m,n_m)}, *)\}$  where  $m \in \mathbb{Z} \cap [1, M]$ , we augment it into a tagged entry  $G_m = (g_m, \text{EffSpell}(\hat{\alpha}_{(m,1)}), \text{EssRoot}(\text{EffSpell}(\hat{\alpha}_{(m,1)})))$ . The list  $\{G_1, \dots, G_M\}$  is sorted alphabetically, with respect to  $\text{EssRoot}(\text{EffSpell}(\hat{\alpha}_{(m,1)}))$  (with higher priority), and  $\text{EffSpell}(\hat{\alpha}_{(m,1)})$  (with lower priority). If two consecutive neighbors in the alphabetized list  $\{G_{(1)} = (g_{(1)}, \hat{\gamma}'_{(1)}, \hat{\gamma}''_{(1)}), \dots, G_{(M)} = (g_{(M)}, \hat{\gamma}'_{(M)}, \hat{\gamma}''_{(M)})\}$  satisfy

$$\text{HrdTest}(\hat{\gamma}'_{(m)}, \hat{\gamma}'_{(m+1)}) = \text{FALSE}$$

AND

$$\text{HrdTest}(\hat{\gamma}'_{(m)}, \hat{\gamma}'_{(m+1)}) = \text{FALSE}$$

where  $m \in \mathbb{Z} \cap [1, M)$ , then add a demarcation line between these two entries. In this manner, the alphabetized list  $\{G_{(1)}, \dots, G_{(M)}\}$  is divided into separate groups of tagged clusters  $\{\Gamma_1 = \{G_{(1,1)}, \dots, G_{(1,m_1)}\}, \dots, \Gamma_K = \{G_{(K,1)}, \dots, G_{(1,m_K)}\}\}$ . Finally, the output list of word clusters  $\{\tilde{\Gamma}_1, \dots, \tilde{\Gamma}_K\}$  is constructed by discarding all the tags (effective spellings, essential roots) from each  $\Gamma_k$ , where  $k \in \mathbb{Z} \cap [1, K]$ .

Example 9.21.1. Our clustering algorithm correctly groups the following families of Turkish words:

*ev, evde, evden, eve, evi, evin, evler, evlerde, evlerden, evlere, evleri, evlerin* — “house”;  
*dedi, dedik, dediler, dedim, dedin, dediniz, demedi, demedik, demediler, demedim, demedin, demediniz, demem, demeyeceğim, demeyeceğiniz, demeyecek, demeyecekler, demeyeceksin, demeyeceksiniz, demeyiz, demez, demezler, demezsin, demezsiniz, demiyor, demiyordu, demiyorduk, demiyordular, demiyordum, demiyordun, demiyordunuz, demiyorlar, demiyorsun, demiyorsunuz, demiyorum, demiyoruz, der, derim, deriz, derler, dersin, dersiniz, dimeyecek, dimeyecekler, diyeceğim, diyeceğiniz, diyecek, diyecekler, diyeceksin, diyeceksiniz, diyor, diyordu, diyorduk, diyordum, diyordun, diyordunuz, diyorlar, diyorlardı, diyorsun, diyorsunuz, diyorum, diyoruz* — “say”;  
*al, alacağım, alacağız, alacak, alacaklar, alacaksın, alacaksınız, aldı, aldık, aldılar, aldım, aldın, aldınız, alır, alırım, alırsınız, alırlar, alırsın, alırsınız, alıyor, alıyordu, alıyorduk, alıyordum, alıyordun, alıyordunuz, alıyorlar, alıyorlardı, alıyorsun, alıyorsunuz, alıyorum, alıyoruz, almadı, almadık, almadılar, almadım, almadın, almadınız, almam, almayacağım, almayacağız, almayacak, almayacaklar, almayacaksın, almayacaksınız, almayız, almaz, almazlar, almazsın, almazsınız, almıyor, almıyordu, almıyorduk, almıyordular, almıyordum, almıyordun, almıyordunuz, almıyorlar, almıyorsun, almıyorsunuz, almıyorum, almıyoruz* — “buy”;  
*okudu, okuduk, okudular, okudum, okudun, okudunuz, okumadı, okumadık, okumadılar, okumadım, okumadın, okumadınız, okumam, okumayacağım, okumayacağız, okumayacak, okumayacaklar, okumayacaksın, okumayacaksınız, okumayız, okumaz, okumazlar, okumazsın, okumazsınız, okumuyor, okumuyordu, okumuyorduk, okumuyordular, okumuyordum, okumuyordun, okumuyordunuz, okumuyorlar, okumuyorsun, okumuyorsunuz, okumuyorum, okumuyoruz, okur, okurlar, okursun, okursunuz, okurum, okuruz, okuyacağım, okuyacağız, okuyacak, okuyacaklar, okuyacaksın, okuyacaksınız, okuyor, okuyordu, okuyorduk, okuyordum, okuyordun, okuyordunuz, okuyorlar, okuyorlardı, okuyorsun, okuyorsunuz, okuyorum, okuyoruz* — “read”;  
*kitaba, kitabı, kitabın, kitap, kitaplar, kitaplara, kitaplarda, kitaplardan, kitapları, kitapların, kitaptan, kitaptan* — “book”.

Example 9.21.2. In Fig. S16, we further apply the aforementioned word clustering algorithm to topic extraction and machine translation (see Table S1 for text source).

Note that the Turkish translation for *disappointment* consists of two words *hayal kırıklığı* (literally “dream brokenness”), where *hayal* means “dream”. This explains why there are two hot spots in the row for *disappointment* in Fig. S16b.

In Turkish, *de* “also, too” is a stop word.



- [1] W. E and Y. Zhou, “A mathematical model for universal semantics,” 2020, arXiv:1907.12293v7 [cs.CL].
- [2] W. A. Gale, K. W. Church, and D. Yarowsky, “A method for disambiguating word senses in a large corpus,” *Comput. Humanities*, vol. 26, no. 5-6, pp. 415–439, 1992.
- [3] D. M. Blei, A. Y. Ng, and M. I. Jordan, “Latent Dirichlet allocation,” *J. Mach. Learn. Res.*, vol. 3, no. Jan, pp. 993–1022, 2003.
- [4] P. D. Turney and P. Pantel, “From frequency to meaning: Vector space models of semantics,” *J. Artificial Intelligence Res.*, vol. 37, pp. 141–188, Feb. 2010.
- [5] T. Mikolov, I. Sutskever, K. Chen, G. S. Corrado, and J. Dean, “Distributed representations of words and phrases and their compositionality,” in *Advances in Neural Information Processing Systems 26*. La Jolla, CA: NIPS, 2013, pp. 3111–3119.
- [6] S. Arora, Y. Li, Y. Liang, T. Ma, and A. Risteski, “A latent variable model approach to PMI-based word embeddings,” *Transactions of the Association for Computational Linguistics*, vol. 4, pp. 385–399, 2016.
- [7] Y. Zhou and X. Zhuang, “Robust reconstruction of the rate constant distribution using the phase function method,” *Biophys. J.*, vol. 91, no. 11, pp. 4045–4053, 2006.
- [8] N. Haydn, Y. Lacroix, and S. Vaienti, “Hitting and return times in ergodic dynamical systems,” *Ann. Probab.*, vol. 33, pp. 2043–2050, 2005.
- [9] T. M. Cover and J. A. Thomas, *Elements of Information Theory*, 2nd ed. Hoboken, NJ: Wiley Interscience, 2006.
- [10] M. Pollicott and M. Yuri, *Dynamical Systems and Ergodic Theory*, ser. London Mathematical Society Student Texts. Cambridge, UK: Cambridge University Press, 1998, vol. 40.
- [11] M. Ružička, “Anwendung mathematisch-statistischer Methoden in der Geobotanik (Synthetische Bearbeitung von Aufnahmen),” *Biológia (Bratislava)*, vol. 13, pp. 647–661, 1958.
- [12] E. Deza and M.-M. Deza, *Dictionary of distances*. Amsterdam, The Netherlands: Elsevier, 2006.
- [13] G. Gilbert, “Distance between sets,” *Nature*, vol. 239, no. 5368, pp. 174–174, 1972.
- [14] F. McSherry and M. Najork, “Computing information retrieval performance measures efficiently in the presence of tied scores,” in *Advances in Information Retrieval. ECIR 2008*, C. Macdonald, I. Ounis, V. Plachouras, I. Ruthven, and R. W. White, Eds. Berlin, Germany: Springer, 2008, pp. 414–421.
- [15] S. Brin and L. Page, “The anatomy of a large-scale hypertextual web search engine,” *Comput. Networks ISDN*, vol. 30, no. 1-7, pp. 107–117, 1998.
- [16] M. Bressan and E. Peserico, “Choose the damping, choose the ranking?” *Journal of Discrete Algorithms*, vol. 8, no. 2, pp. 199–213, 2010.
- [17] D. Lardiere, “Words and their parts,” in *An Introduction to Language and Linguistics*, R. Fasold and J. Connor-Linton, Eds. Cambridge, UK: Cambridge University Press, 2006, ch. 2, pp. 55–96.
- [18] A. D. Friederici, “The neurobiology of language comprehension,” in *Language Comprehension: A Biological Perspective*, A. D. Friederici, Ed. Berlin, Germany: Springer, 1999, ch. 9, pp. 265–304.
- [19] R. Jakobson, “The identification of phonemic entities,” in *Recherches structurales 1949. Interventions dans le débat glossématique*, ser. Travaux du Cercle Linguistique de Copenhague. Copenhagen, Denmark: Nordisk Sprog- og Kulturforlag, 1949, vol. V, pp. 205–213.
- [20] C. Everett, D. E. Blasi, and S. G. Roberts, “Climate, vocal folds, and tonal languages: Connecting the physiological and geographic dots,” *Proc. Natl. Acad. Sci. USA*, vol. 112, pp. 1322–1327, 2015.
- [21] C. R. Ember, “Commentary: Considering language as expressive culture,” *Journal of Language Evolution*, vol. 1, no. 1, pp. 60–61, 2016.
- [22] C. Everett, “Languages in drier climates use fewer vowels,” *Frontiers in Psychology*, vol. 8, p. Article 1285, 2017.

- [23] J. G. Frazer, *The Golden Bough: a study of magic and religion*, abridged ed. New York, NY: MacMillan, 1922.
- [24] W. Labov, *Principles of Linguistic Change: Social Factors*. Malden, MA: Blackwell Publishers, 2001.
- [25] ———, *Principles of Linguistic Change: Cognitive and Cultural Factors*. Malden, MA: Wiley-Blackwell, 2010.
- [26] K. Allan and K. Burridge, *Forbidden Words: Taboo and the Censoring of Language*. Cambridge, UK: Cambridge University Press, 2006.
- [27] A. D. Friederici, J. Bahlmann, S. Heim, R. I. Schubotz, and A. Anwander, “The brain differentiates human and non-human grammars: Functional localization and structural connectivity,” *Proc. Natl. Acad. Sci. USA*, vol. 103, no. 7, pp. 2458–2463, 2006.
- [28] S. M. Wilson, S. Galantucci, M. C. Tartaglia, K. Rising, D. K. Patterson, M. L. Henry, J. M. Ogar, J. DeLeon, B. L. Miller, and M. L. Gorno-Tempini, “Syntactic processing depends on dorsal language tracts,” *Neuron*, vol. 72, no. 2, pp. 397–403, 2011.
- [29] P. F. Brown, P. V. deSouza, R. L. Mercer, V. J. Della Pietra, and J. C. Lai, “Class-based  $n$ -gram models of natural language,” *Computat. Linguist.*, vol. 18, no. 4, pp. 467–479, 1992.
- [30] S. Pinker, *The Stuff of Thought: Language as a Window into Human Nature*. New York: Viking, 2007.
- [31] ———, *Learnability and Cognition: the Acquisition of Argument Structure*. Cambridge, MA: The MIT Press, 2013.
- [32] N. Chomsky, *The Minimalist Program*. Cambridge, MA: MIT Press, 2015.
- [33] M. I. Jordan, Z. Ghahramani, T. S. Jaakkola, and L. K. Saul, “An introduction to variational methods for graphical models,” in *Learning in graphical models*, M. I. Jordan, Ed. Cambridge, MA: MIT Press, 1999, pp. 105–161.
- [34] D. Heckerman, “A tutorial on learning with Bayesian networks,” in *Learning in graphical models*, M. I. Jordan, Ed. Cambridge, MA: MIT Press, 1999, pp. 301–354.
- [35] G. Carlsson, “Topology and data,” *Bull. Amer. Math. Soc. (N.S.)*, vol. 46, no. 2, pp. 255–308, 2009.
- [36] W. E. J. Lu, and Y. Yao, “The landscape of complex networks—critical nodes and a hierarchical decomposition,” *Methods Appl. Anal.*, vol. 20, no. 4, pp. 383–404, 2013.
- [37] S. B. Needleman and C. D. Wunsch, “A general method applicable to the search for similarities in the amino acid sequence of two proteins,” *Journal of Molecular Biology*, vol. 48, no. 3, pp. 443–453, 1970.
- [38] T. F. Smith and M. S. Waterman, “Identification of common molecular subsequences,” *Journal of Molecular Biology*, vol. 147, no. 1, pp. 195–197, 1981.
- [39] M. F. Porter, “An algorithm for suffix stripping,” *Program*, vol. 14, no. 3, pp. 130–137, 1980.
- [40] ———, “Snowball — a small string processing language designed for creating stemming algorithms for use in Information Retrieval,” <http://snowball.tartarus.org/>, 2014.
- [41] S. Pinker, “Words and rules in the human brain,” *Nature*, vol. 387, no. 6633, pp. 547–548, 1997.
- [42] W. D. Marslen-Wilson and L. K. Tyler, “Dissociating types of mental computation,” *Nature*, vol. 387, no. 6633, pp. 592–594, 1997.
- [43] E. Lieberman, J.-B. Michel, J. Jackson, T. Tang, and M. A. Nowak, “Quantifying the evolutionary dynamics of language,” *Nature*, vol. 449, no. 7163, pp. 713–716, 2007.
- [44] Y. Yang, W.-t. Yih, and C. Meek, “WikiQA: A challenge dataset for open-domain question answering,” in *Proceedings of the 2015 Conference on Empirical Methods in Natural Language Processing (EMNLP)*. Lisbon, Portugal: Association for Computational Linguistics, 2015.
- [45] J. Yeon and L. Brown, *Korean: a comprehensive grammar*. London, UK: Routledge, 2011.
- [46] T. Lundskaer-Nielsen and P. Holmes, *Danish: An Essential Grammar*, 2nd ed. London, UK: Routledge, 2000.
- [47] B. C. Donaldson, *Dutch: A Comprehensive Grammar*, 2nd ed. London, UK: Routledge, 2008.
- [48] C. Rounds, *Hungarian: An Essential Grammar*. London, UK: Routledge, 2001.

- [49] S. Starostin, A. Dybo, and O. Mudrak, *Etymological dictionary of the Altaic languages*. Leiden, The Netherlands: Brill, 2003.
- [50] J. I. Hualde and J. Ortiz de Urbina, Eds., *A grammar of Basque*. Berlin, Germany: Mouton de Gruyter, 2003.
- [51] G. Eryiđit and E. Adalı, “An affix stripping morphological analyzer for Turkish,” in *Proceedings of the IASTED International Conference ARTIFICIAL INTELLIGENCE AND APPLICATIONS*, Innsbruck, Austria, 2004.
